# Supplementary material for: Uncertainty quantification of transition operators in the empirical shell model
Source: arXiv:2206.14956 source file (2023-10-09)

$\beta^- : {}^{20}\text{F}(2_1) \rightarrow {}^{20}\text{Ne}(2_1)$

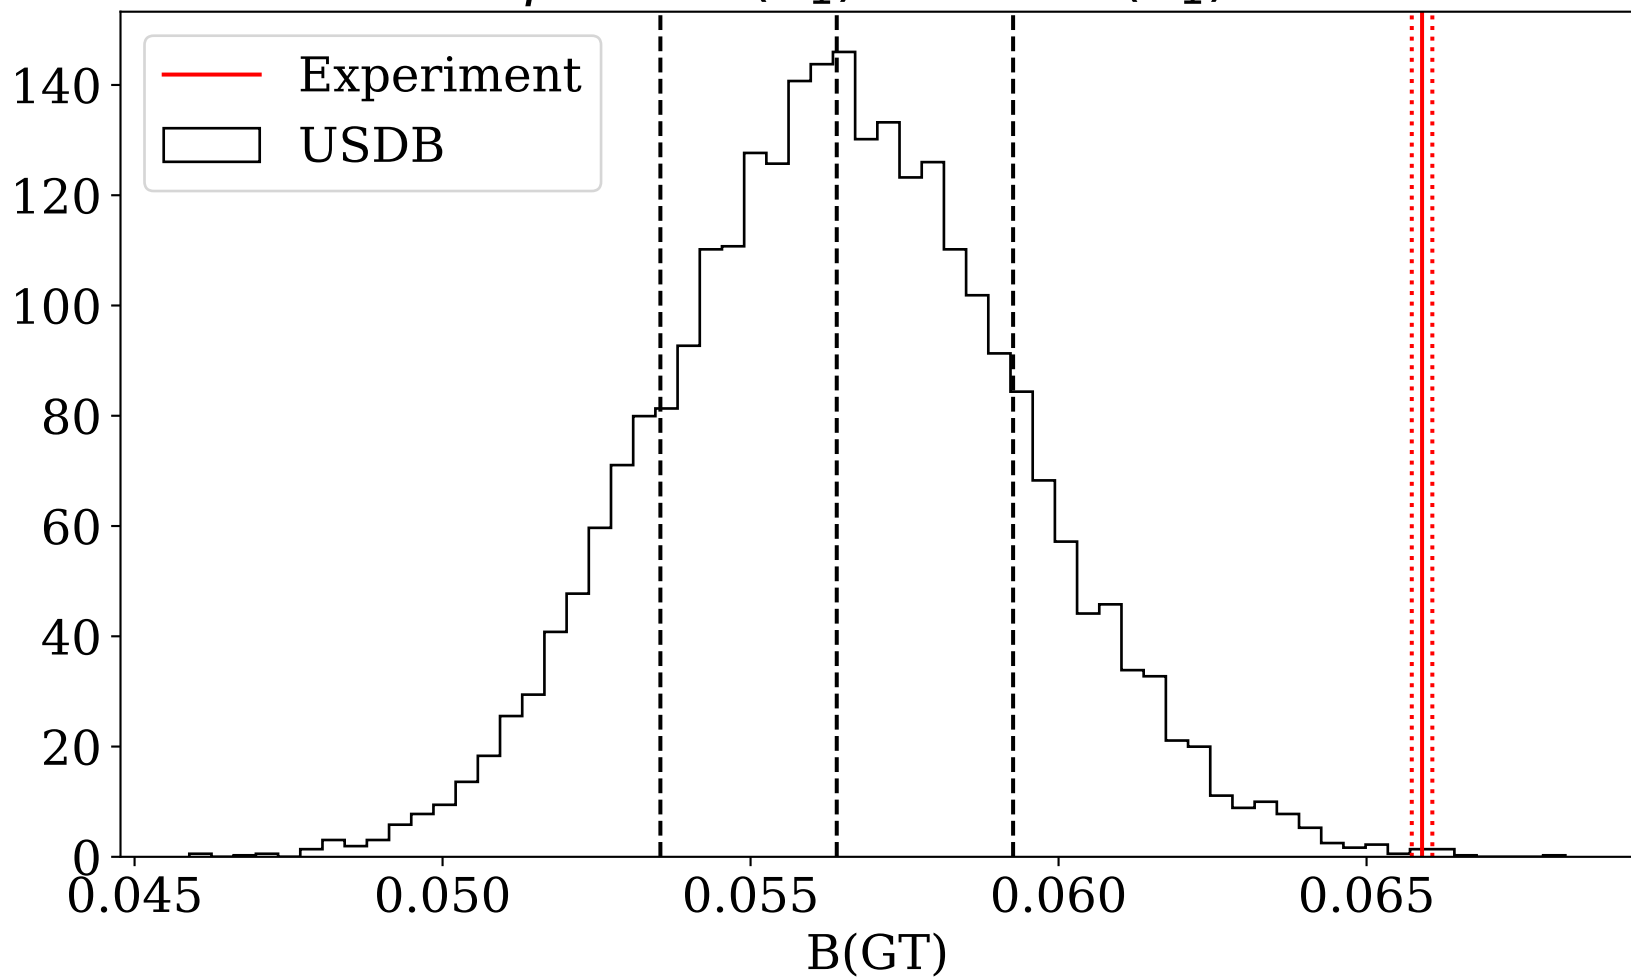

$\beta^- : {}^{21}\text{F}(5/2_1) \rightarrow {}^{21}\text{Ne}(5/2_1)$

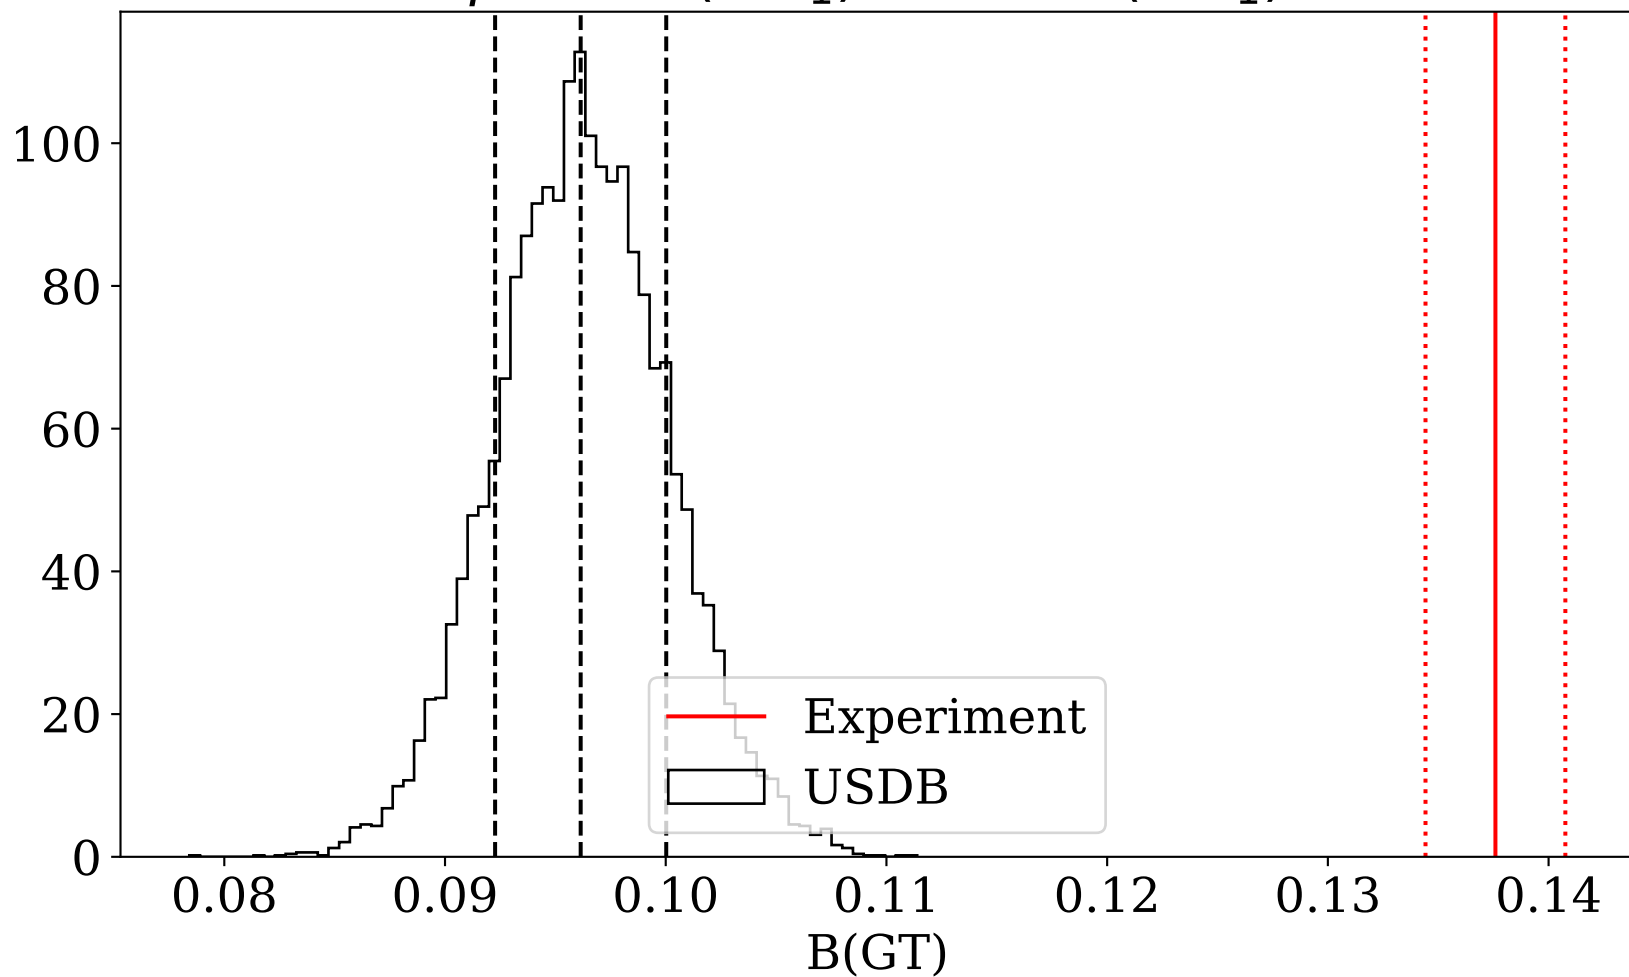

$\beta^- : {}^{21}\text{F}(5/2_1) \rightarrow {}^{21}\text{Ne}(3/2_1)$

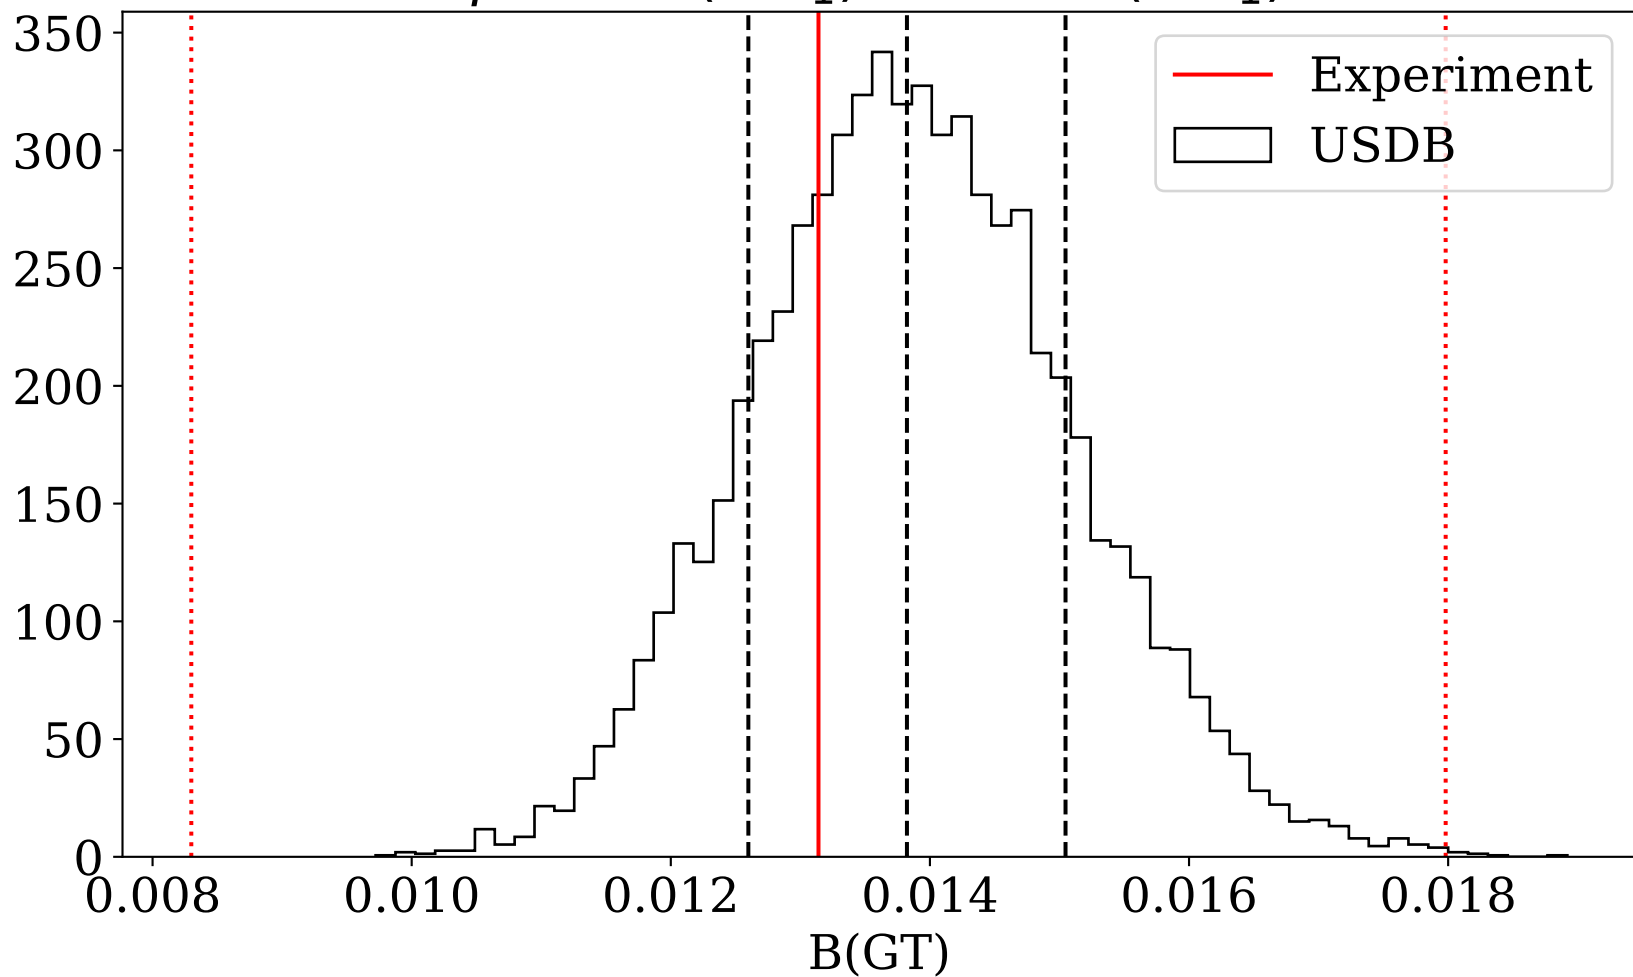

$\beta^- : {}^{21}\text{F}(5/2_1) \rightarrow {}^{21}\text{Ne}(7/2_1)$

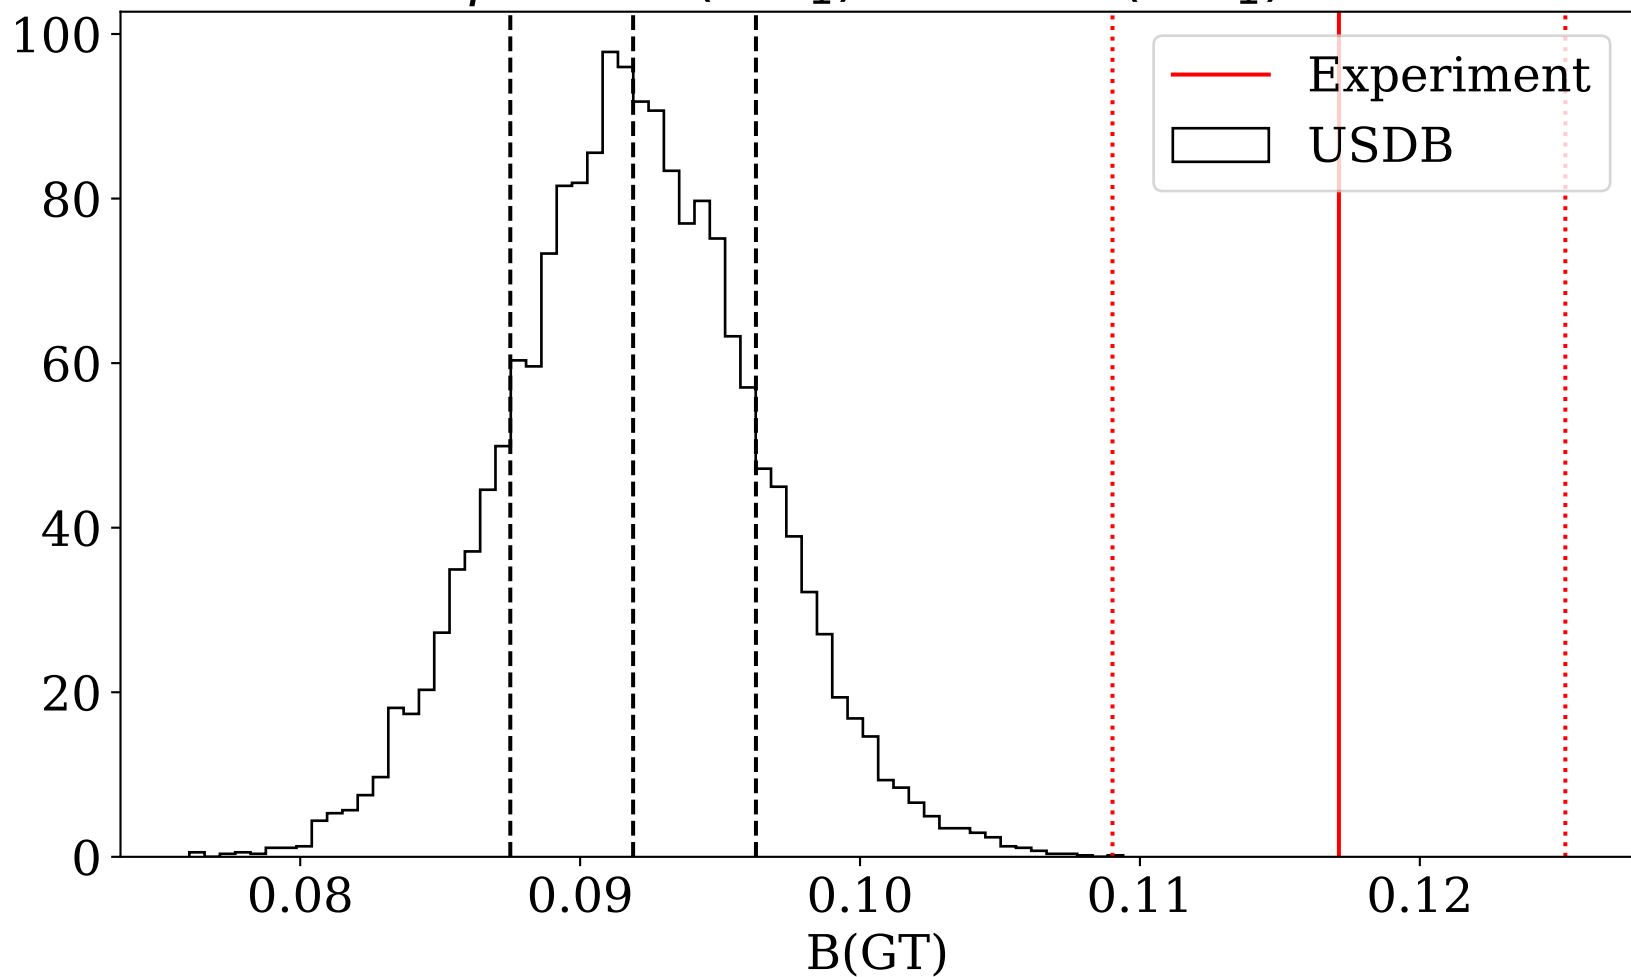

$\beta^- : {}^{21}\text{F}(5/2_1) \rightarrow {}^{21}\text{Ne}(5/2_2)$

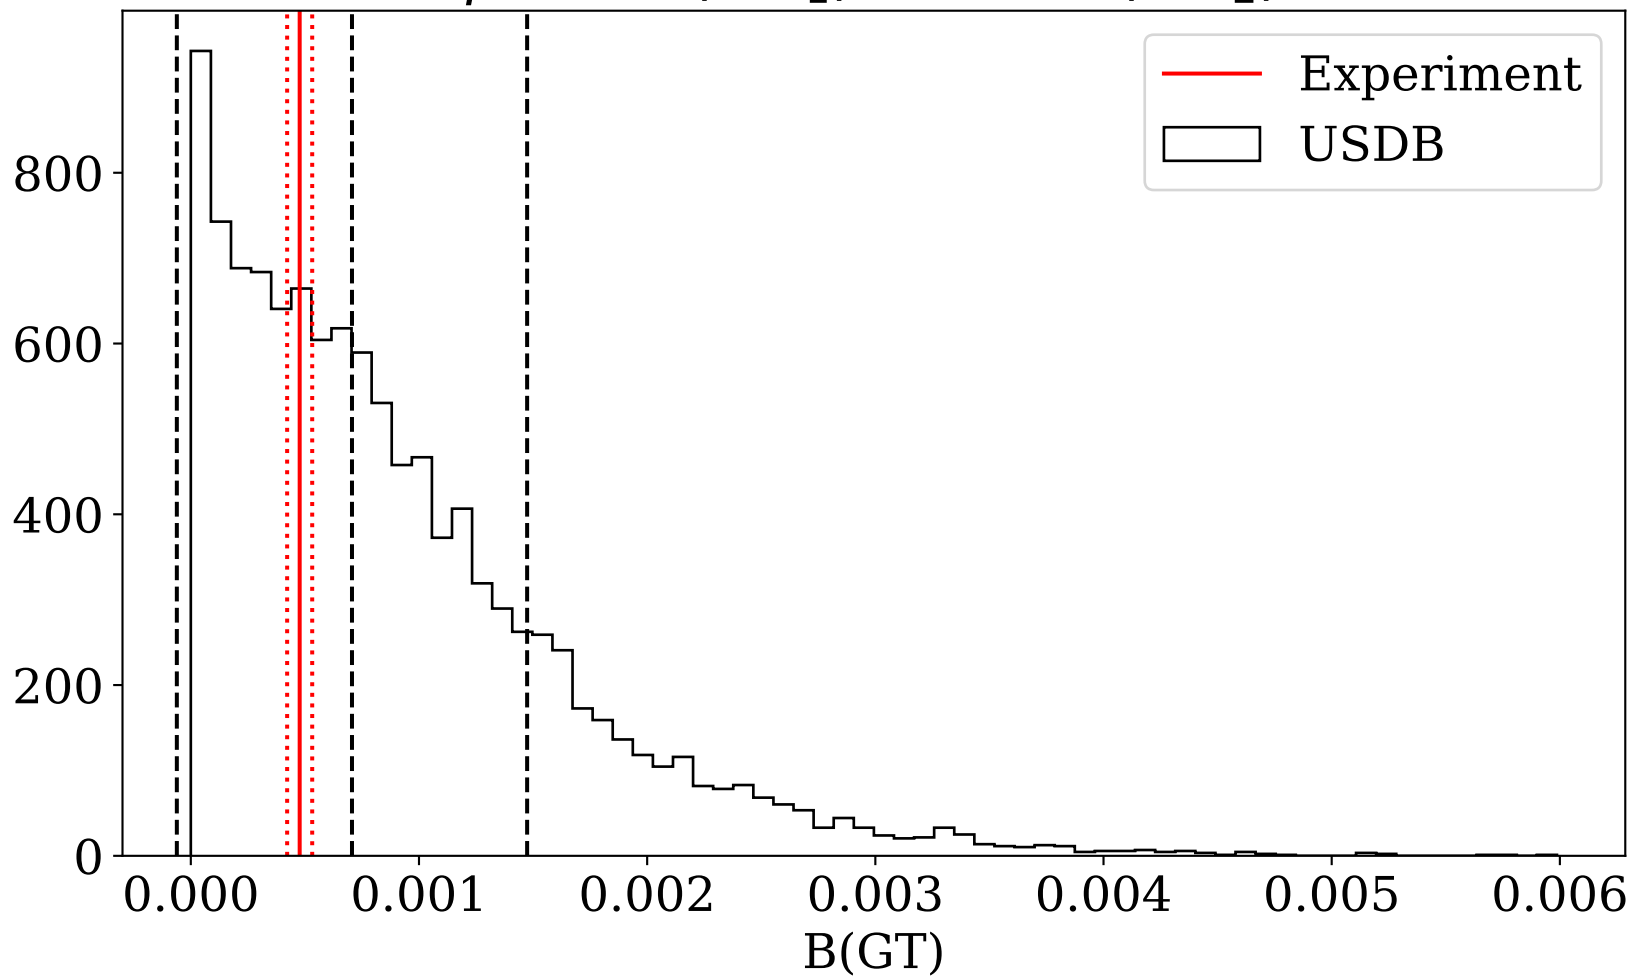

$\beta^- : {}^{21}\text{F}(5/2_1) \rightarrow {}^{21}\text{Ne}(5/2_3)$

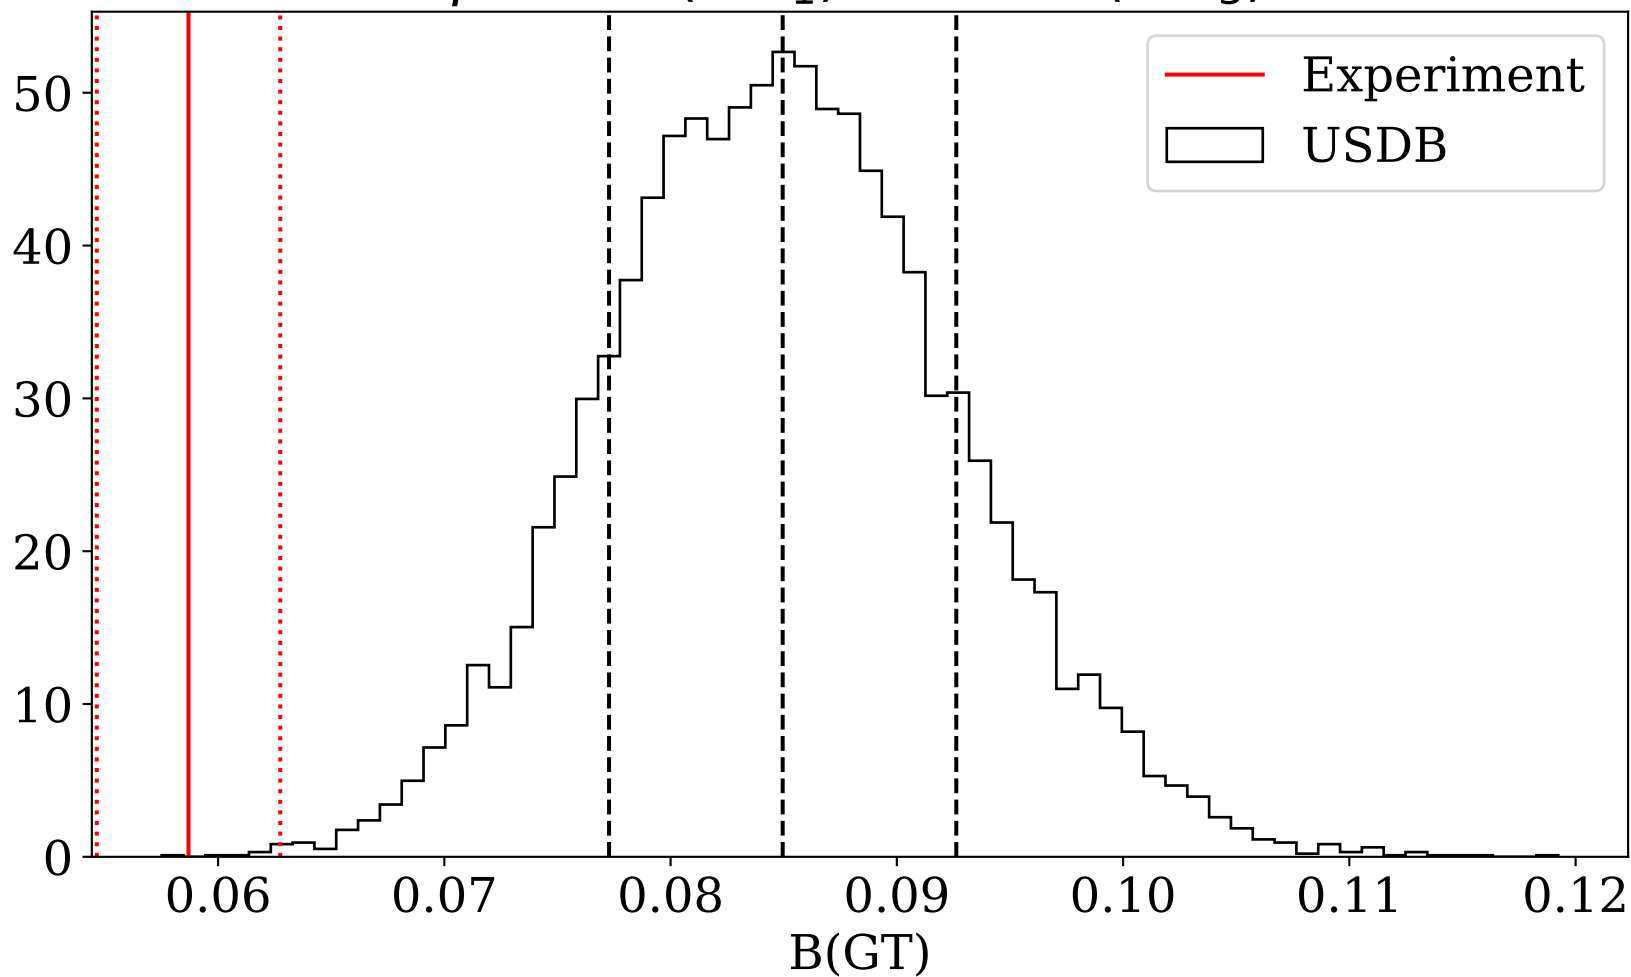

$\beta^- : {}^{21}\text{F}(5/2_1) \rightarrow {}^{21}\text{Ne}(3/2_2)$

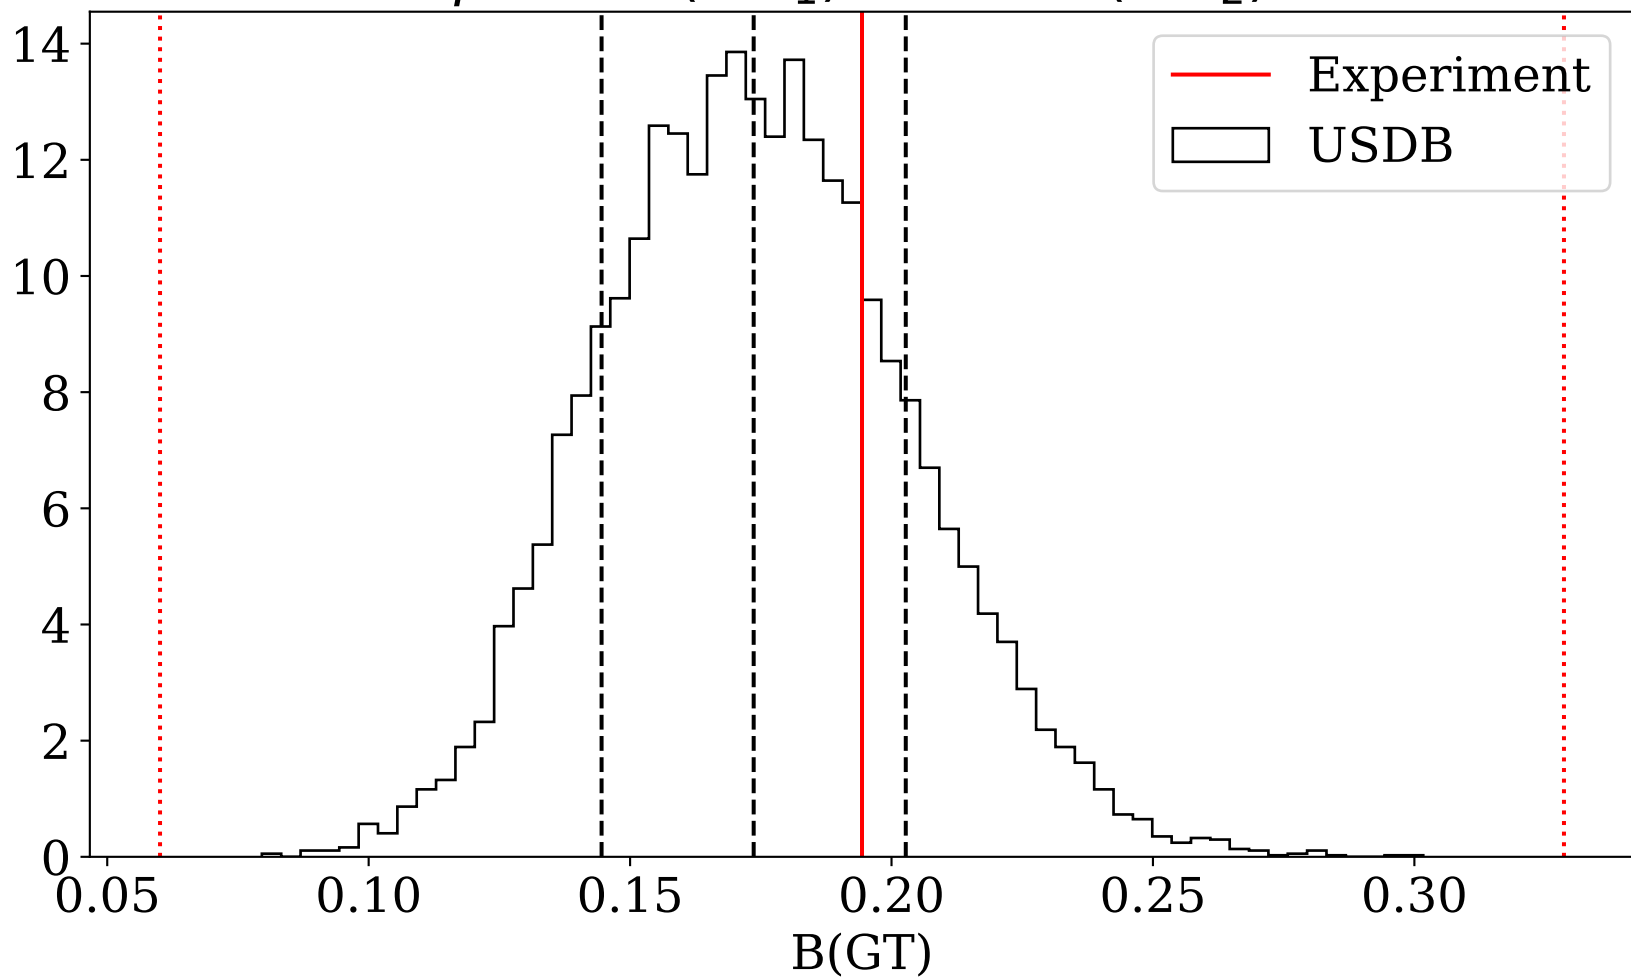

$\beta^- : {}^{22}\text{F}(4_1) \rightarrow {}^{22}\text{Ne}(4_1)$

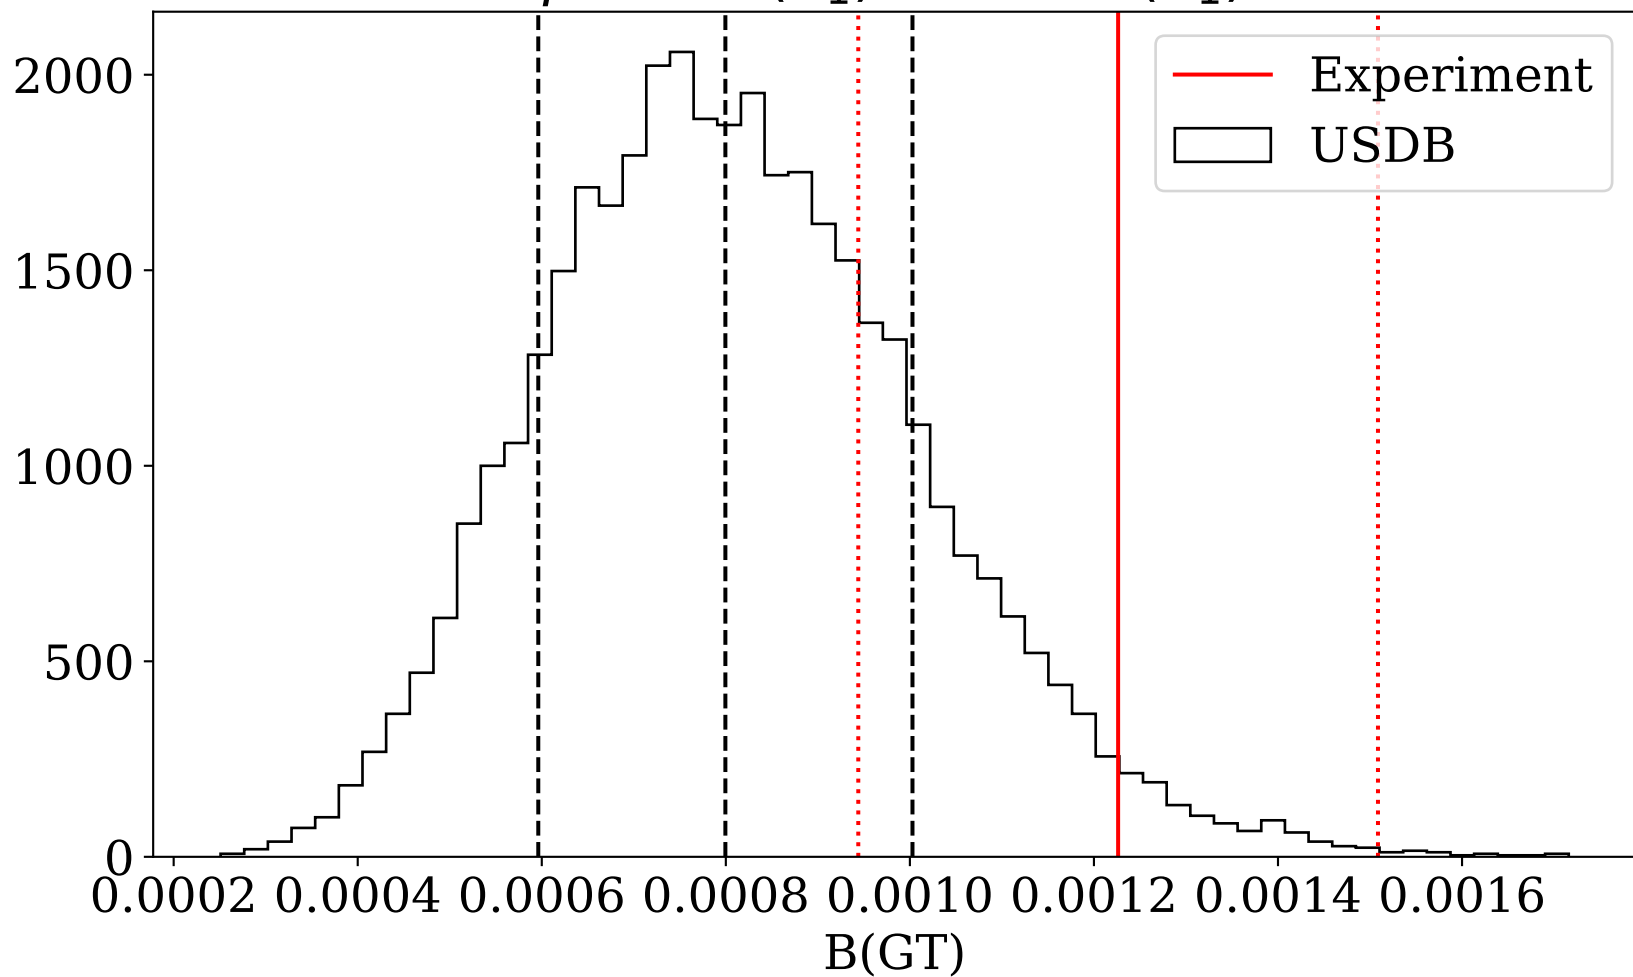



$\beta^- : {}^{22}\text{F}(4_1) \rightarrow {}^{22}\text{Ne}(4_2)$

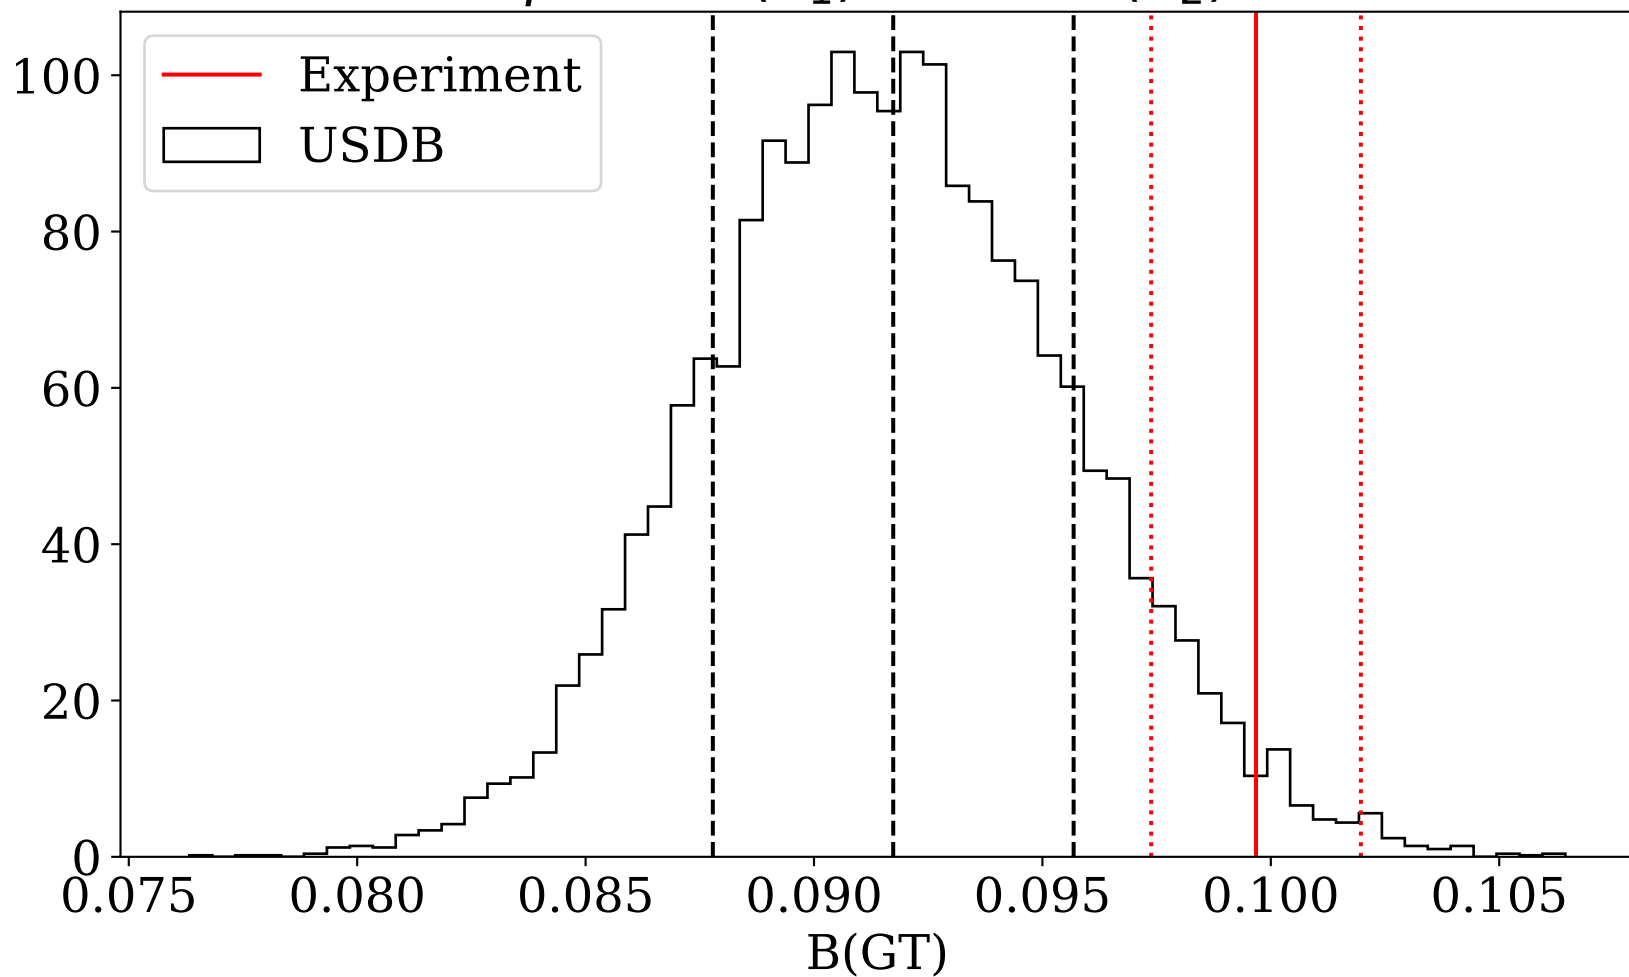

$\beta^- : {}^{22}\text{F}(4_1) \rightarrow {}^{22}\text{Ne}(3_1)$

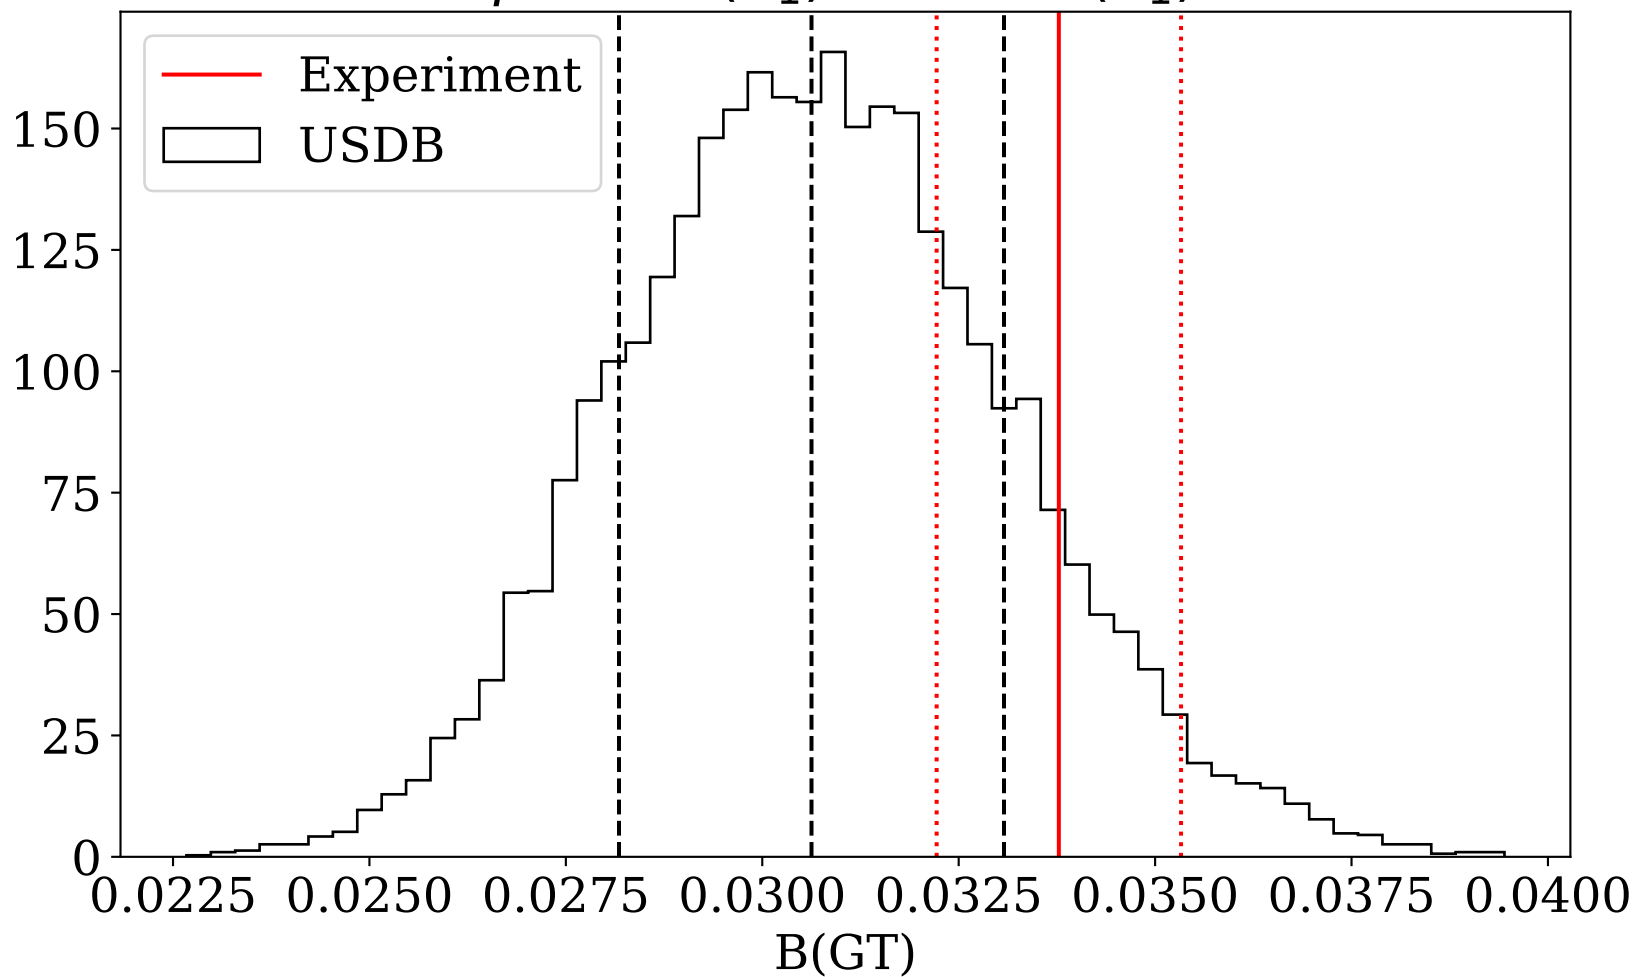

$\beta^- : {}^{22}\text{F}(4_1) \rightarrow {}^{22}\text{Ne}(4_3)$

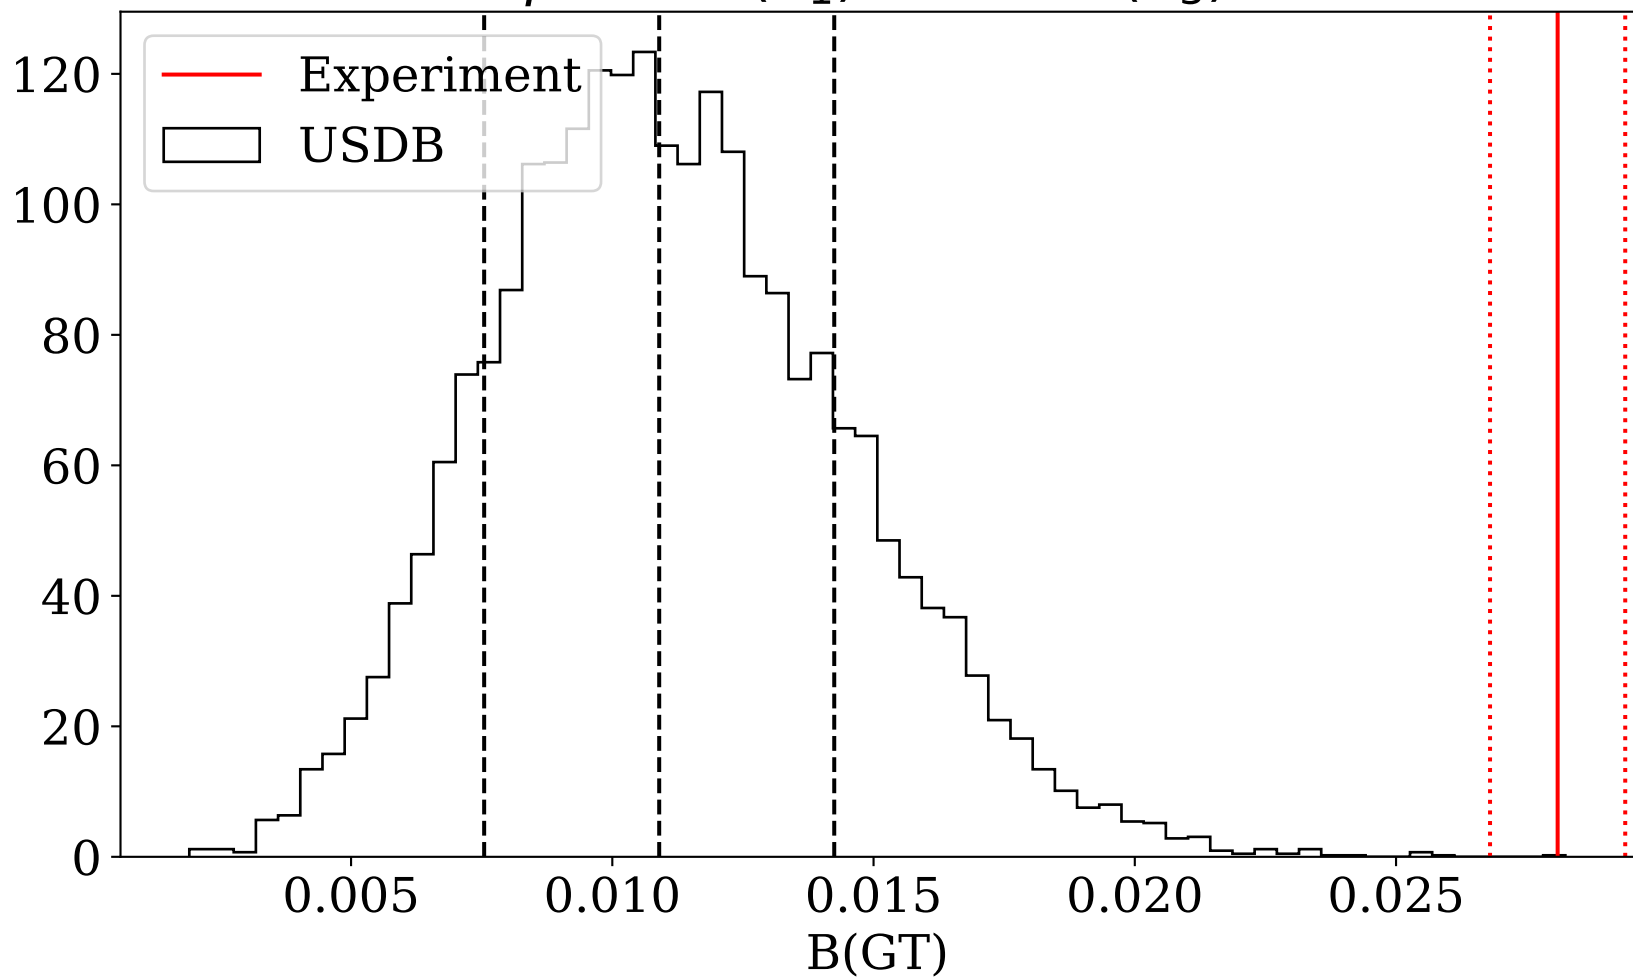

$\beta^- : {}^{22}\text{F}(4_1) \rightarrow {}^{22}\text{Ne}(4_4)$

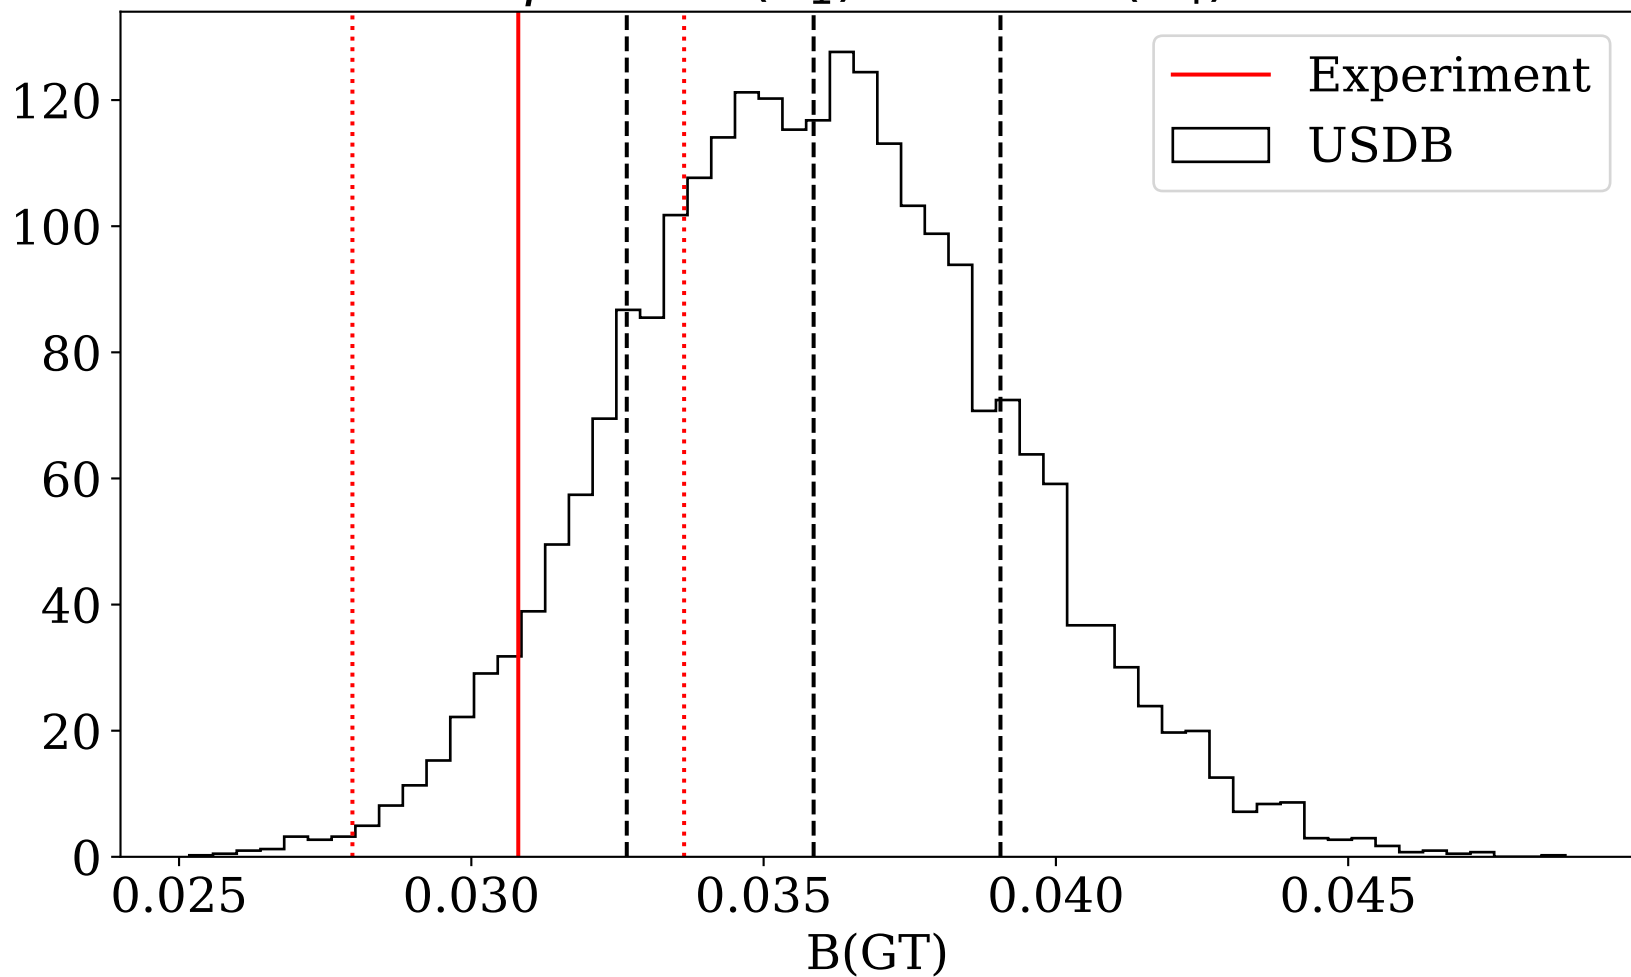

$\beta^- : {}^{23}\text{F}(5/2_1) \rightarrow {}^{23}\text{Ne}(5/2_1)$

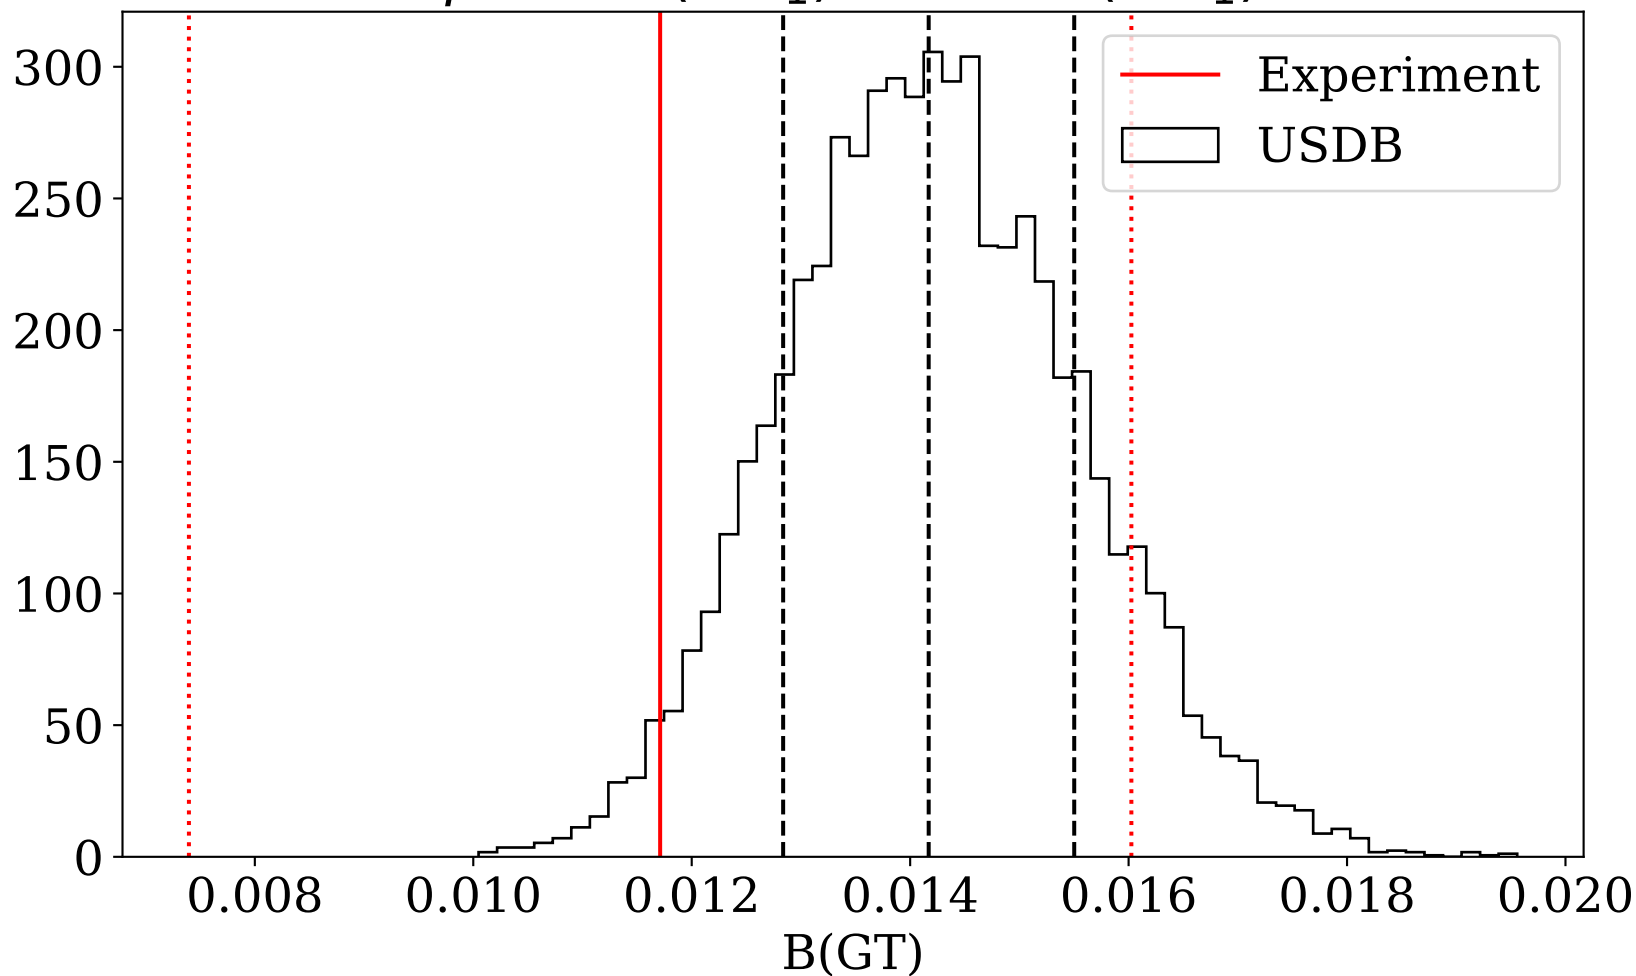

$\beta^- : {}^{23}\text{F}(5/2_1) \rightarrow {}^{23}\text{Ne}(3/2_1)$

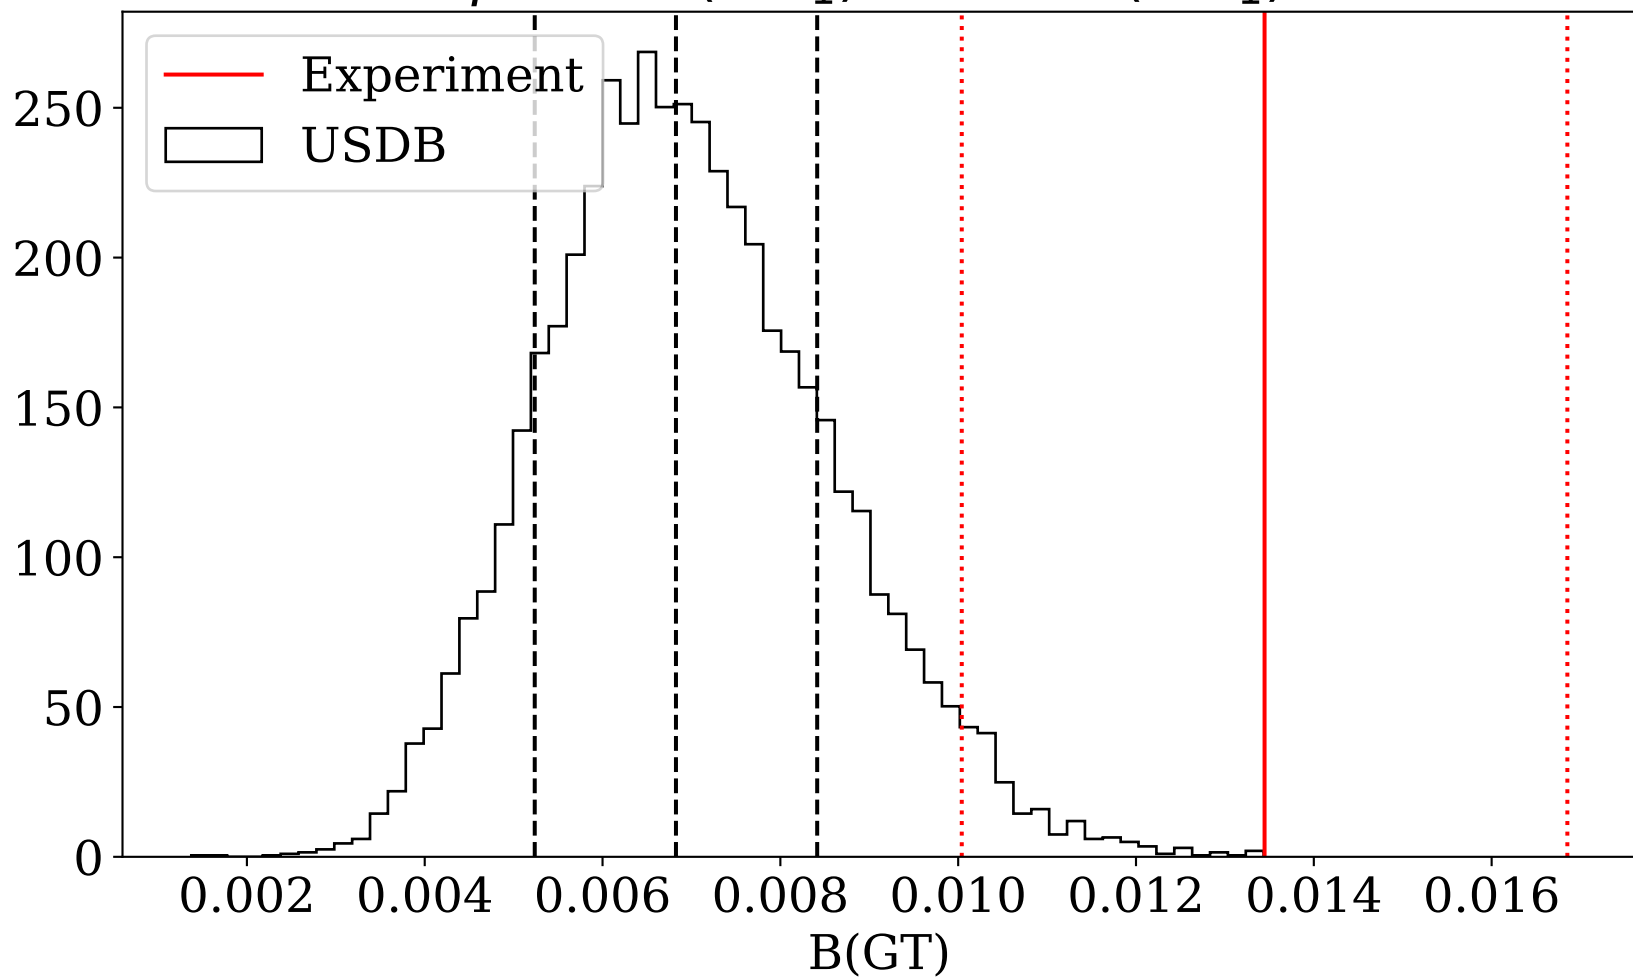

$\beta^- : {}^{23}\text{F}(5/2_1) \rightarrow {}^{23}\text{Ne}(5/2_1)$

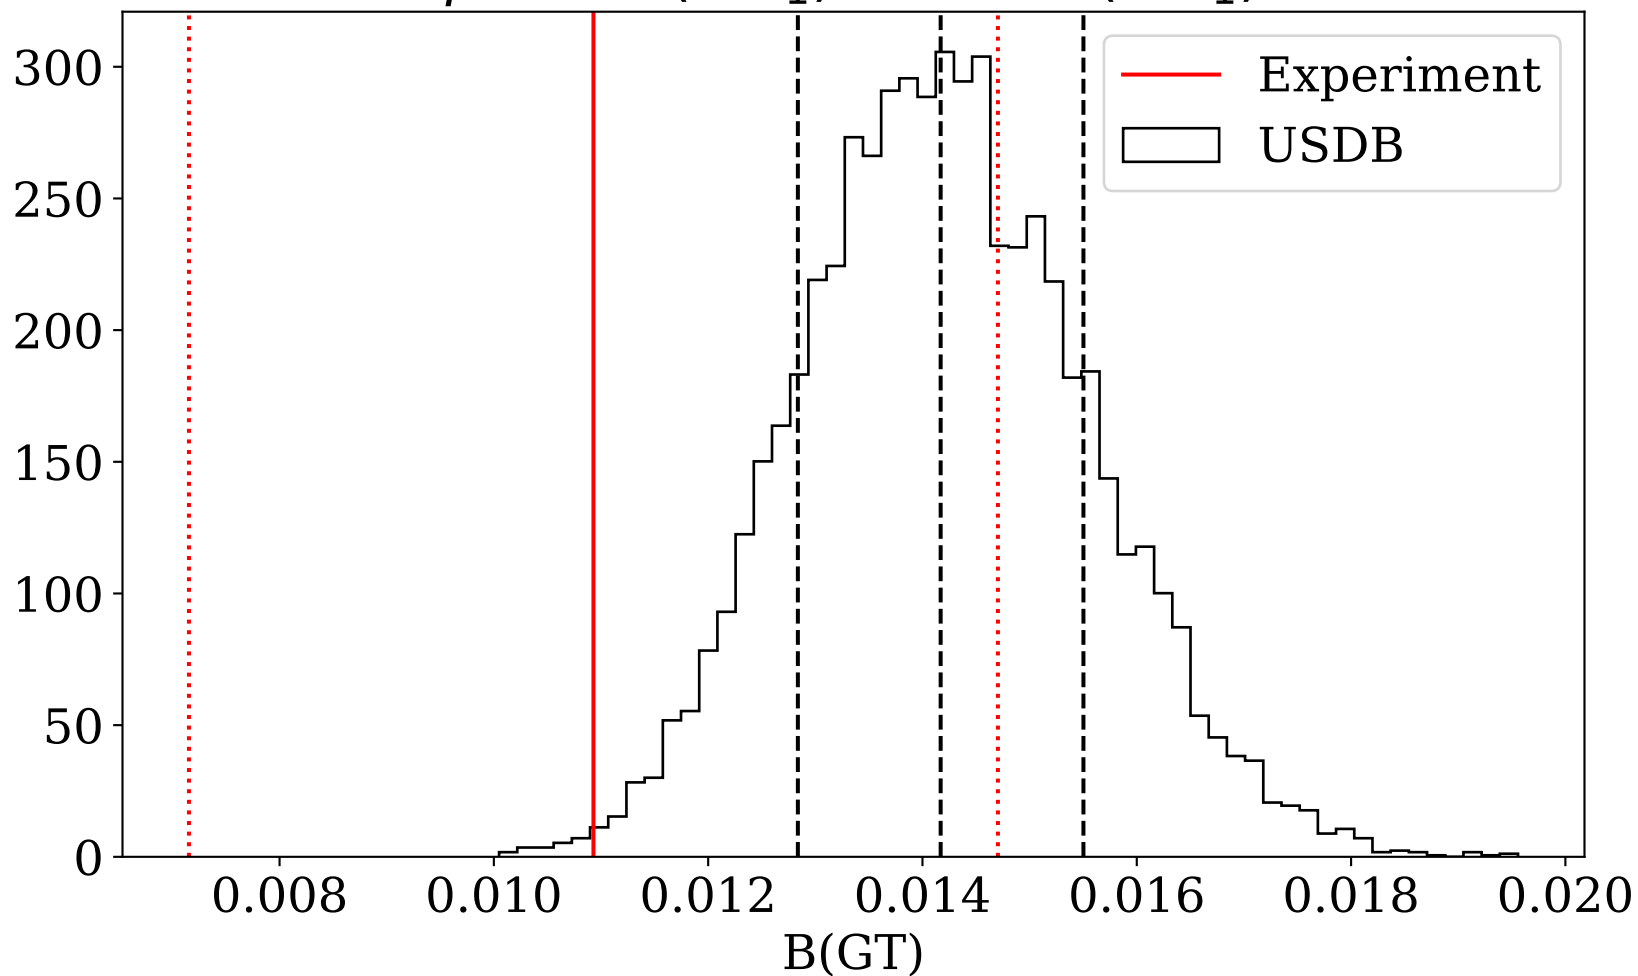

$\beta^- : {}^{23}\text{F}(5/2_1) \rightarrow {}^{23}\text{Ne}(3/2_2)$

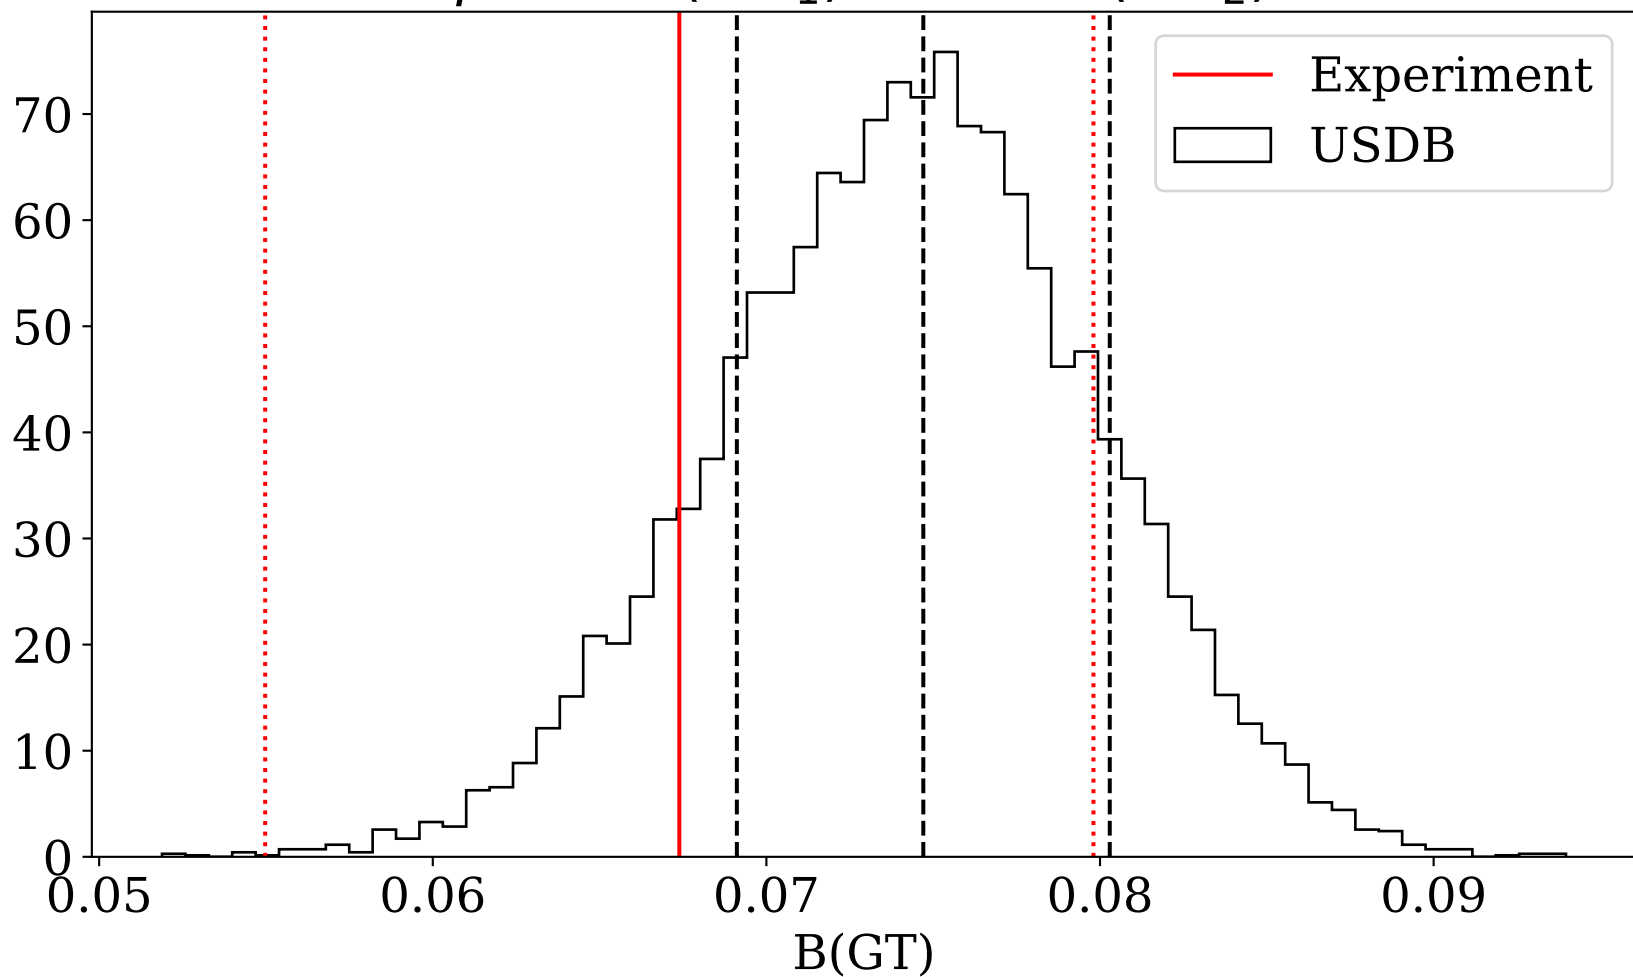



$\beta^- : {}^{23}\text{F}(5/2_1) \rightarrow {}^{23}\text{Ne}(3/2_3)$

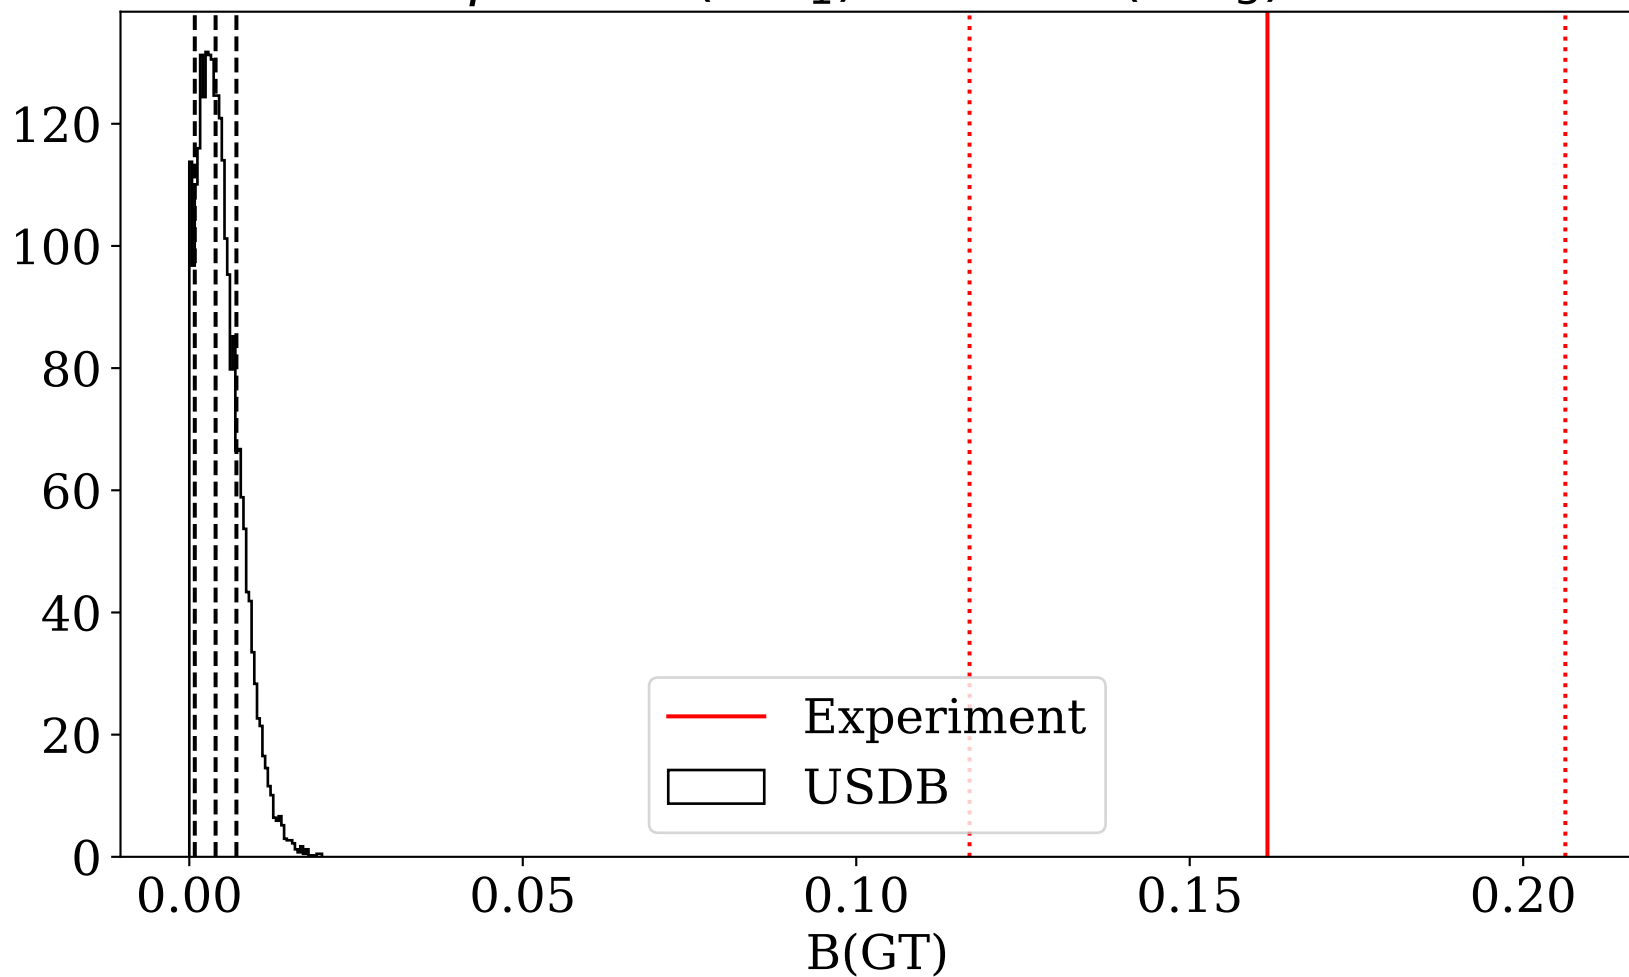

$\beta^- : {}^{23}\text{Ne}(5/2_1) \rightarrow {}^{23}\text{Na}(3/2_1)$

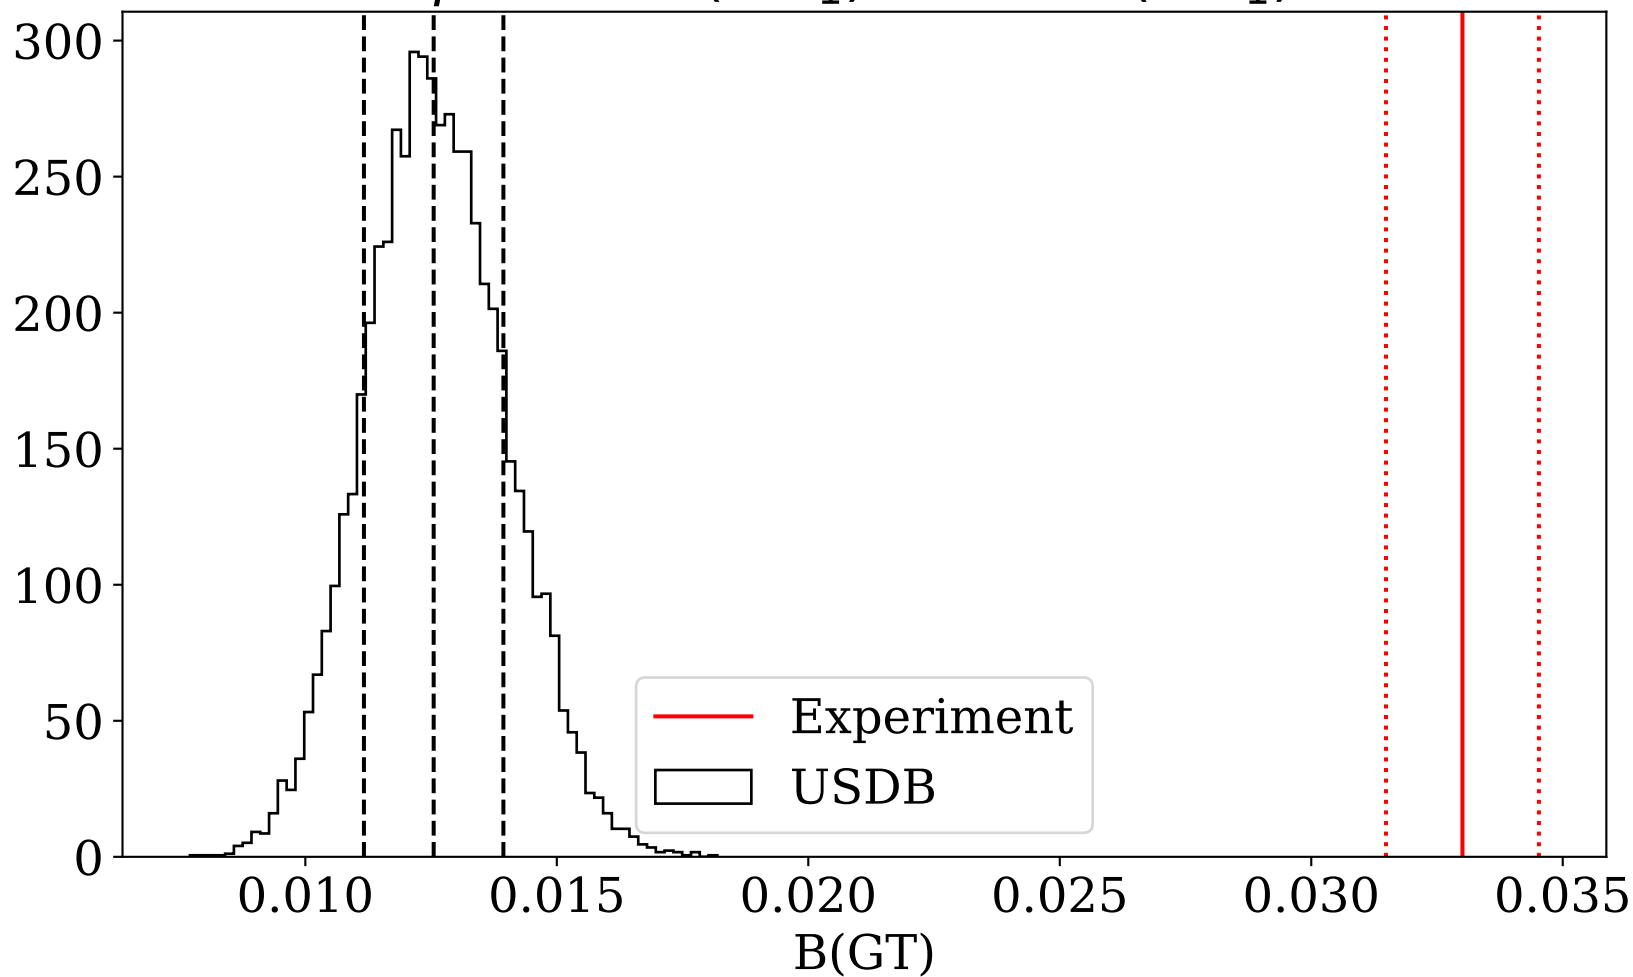

$\beta^- : {}^{23}\text{Ne}(5/2_1) \rightarrow {}^{23}\text{Na}(5/2_1)$

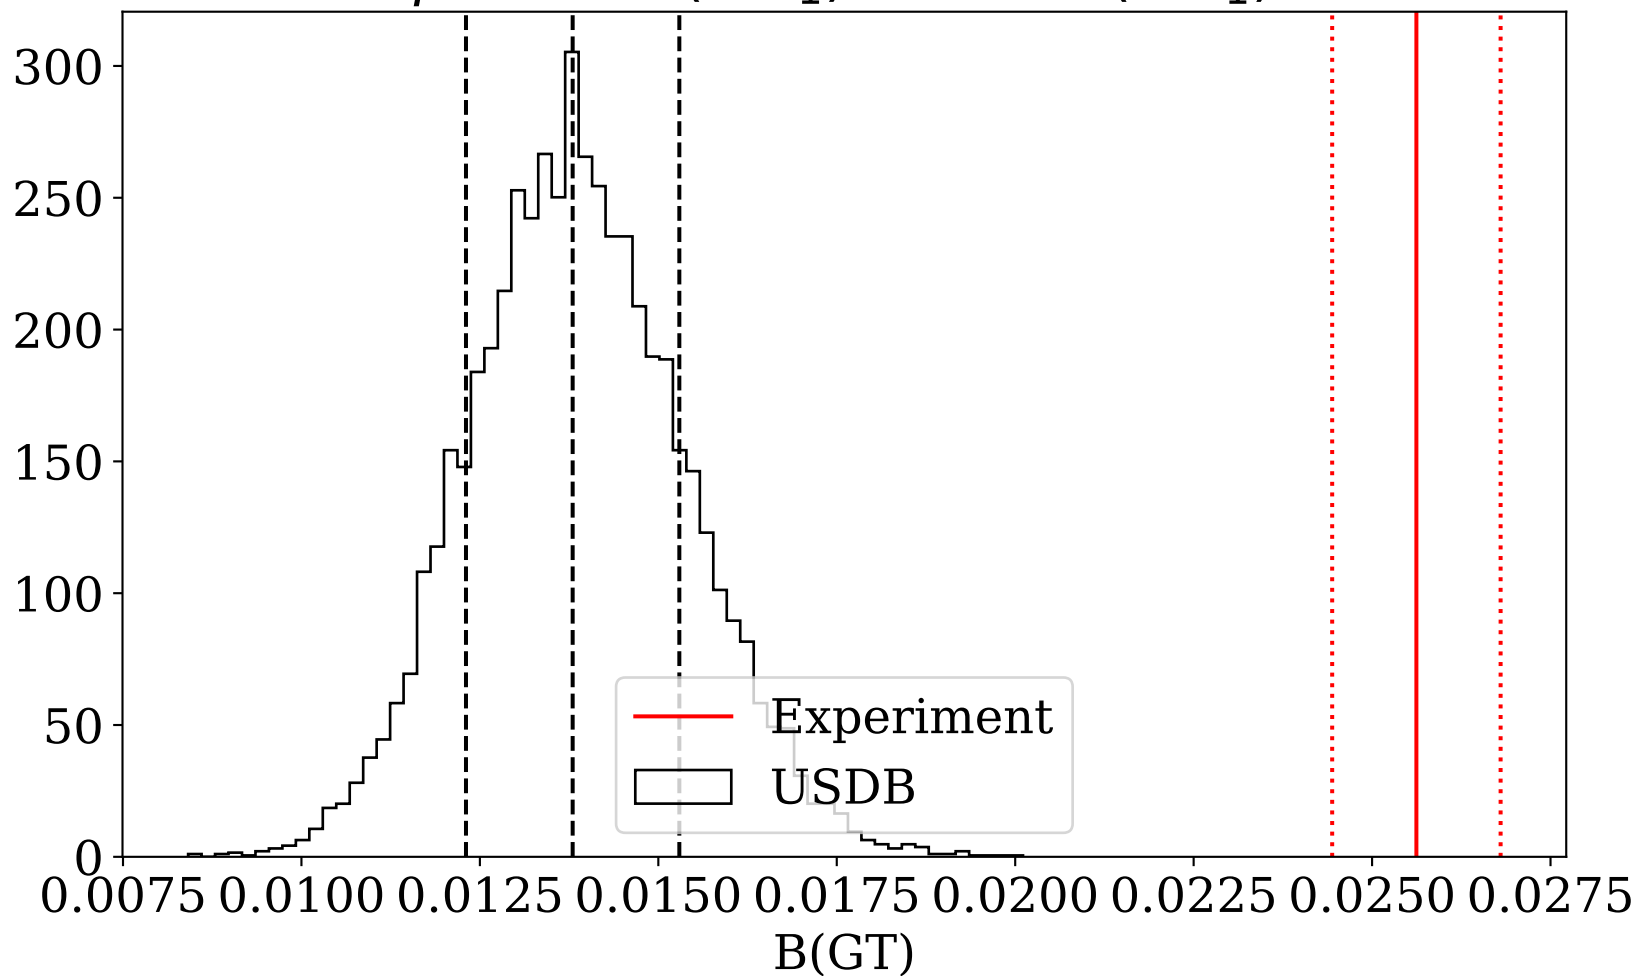

$\beta^- : {}^{23}\text{Ne}(5/2_1) \rightarrow {}^{23}\text{Na}(7/2_1)$

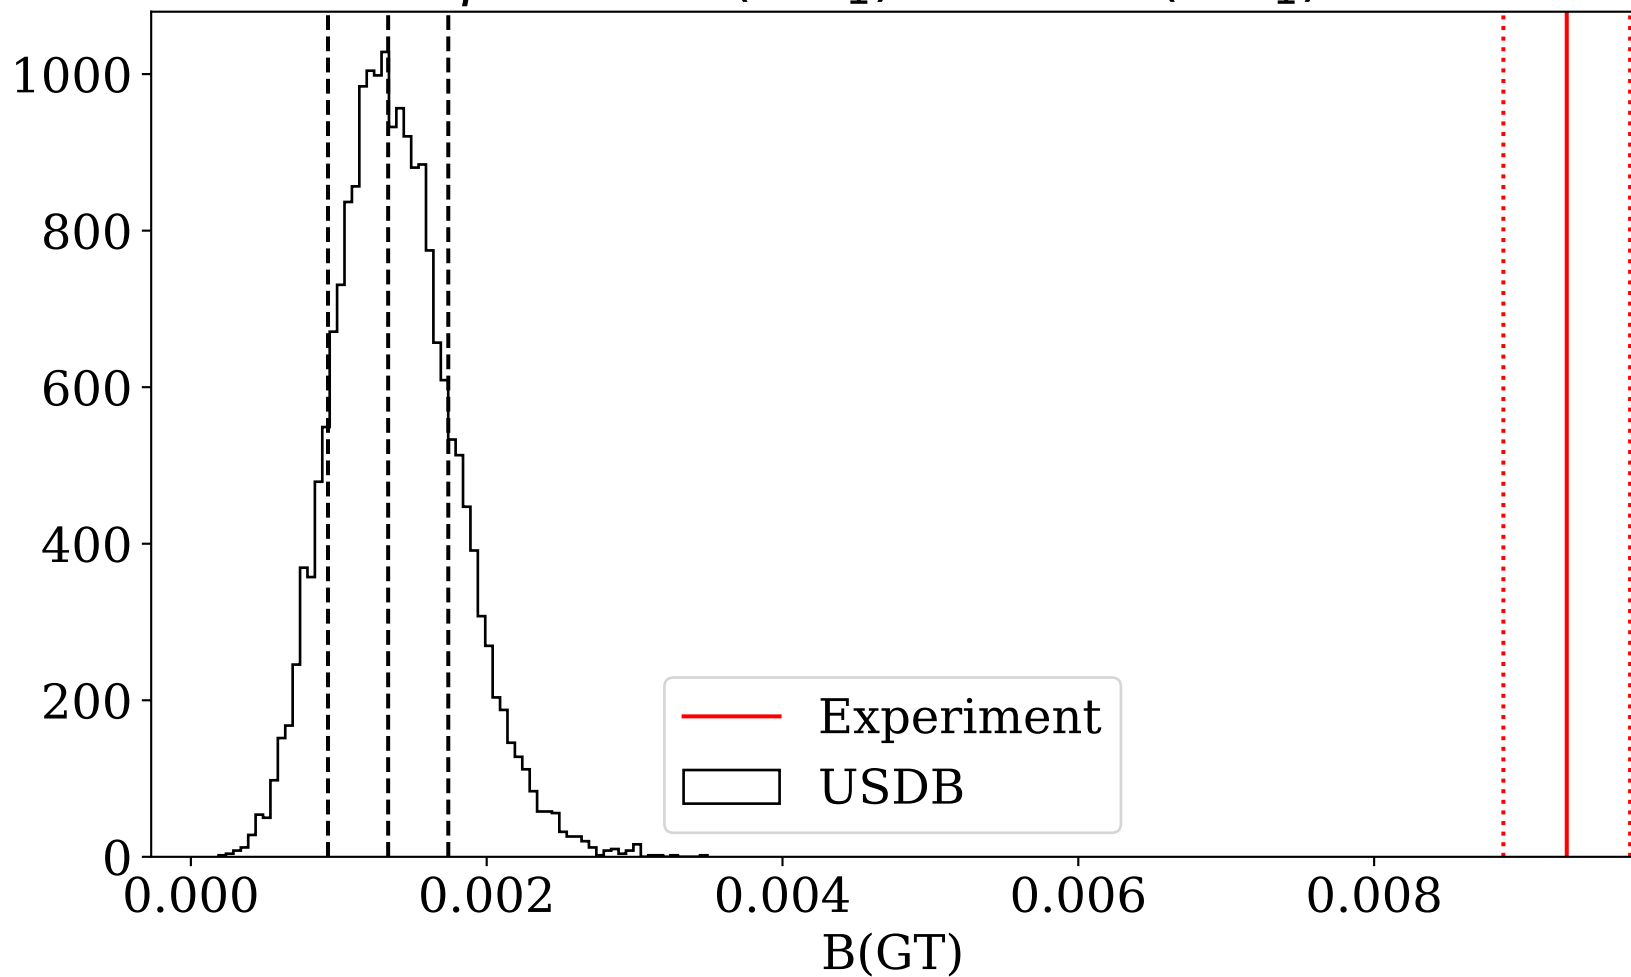

$\beta^- : {}^{23}\text{Ne}(5/2_1) \rightarrow {}^{23}\text{Na}(3/2_2)$

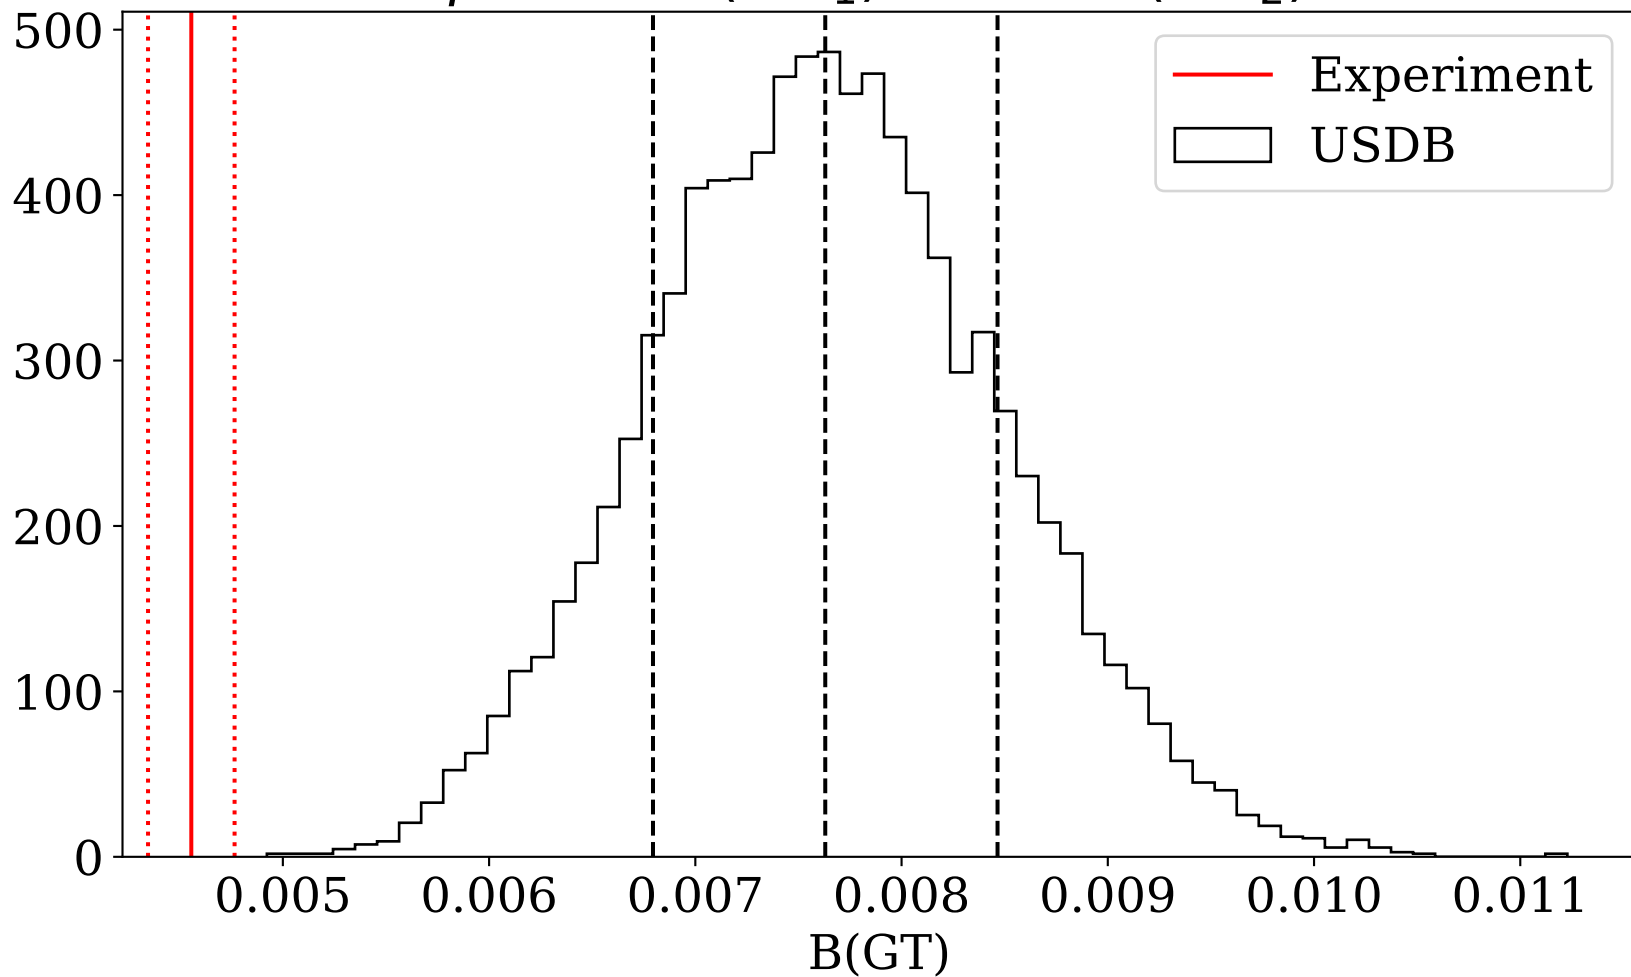

$\beta^- : {}^{24}\text{Ne}(0_1) \rightarrow {}^{24}\text{Na}(1_1)$

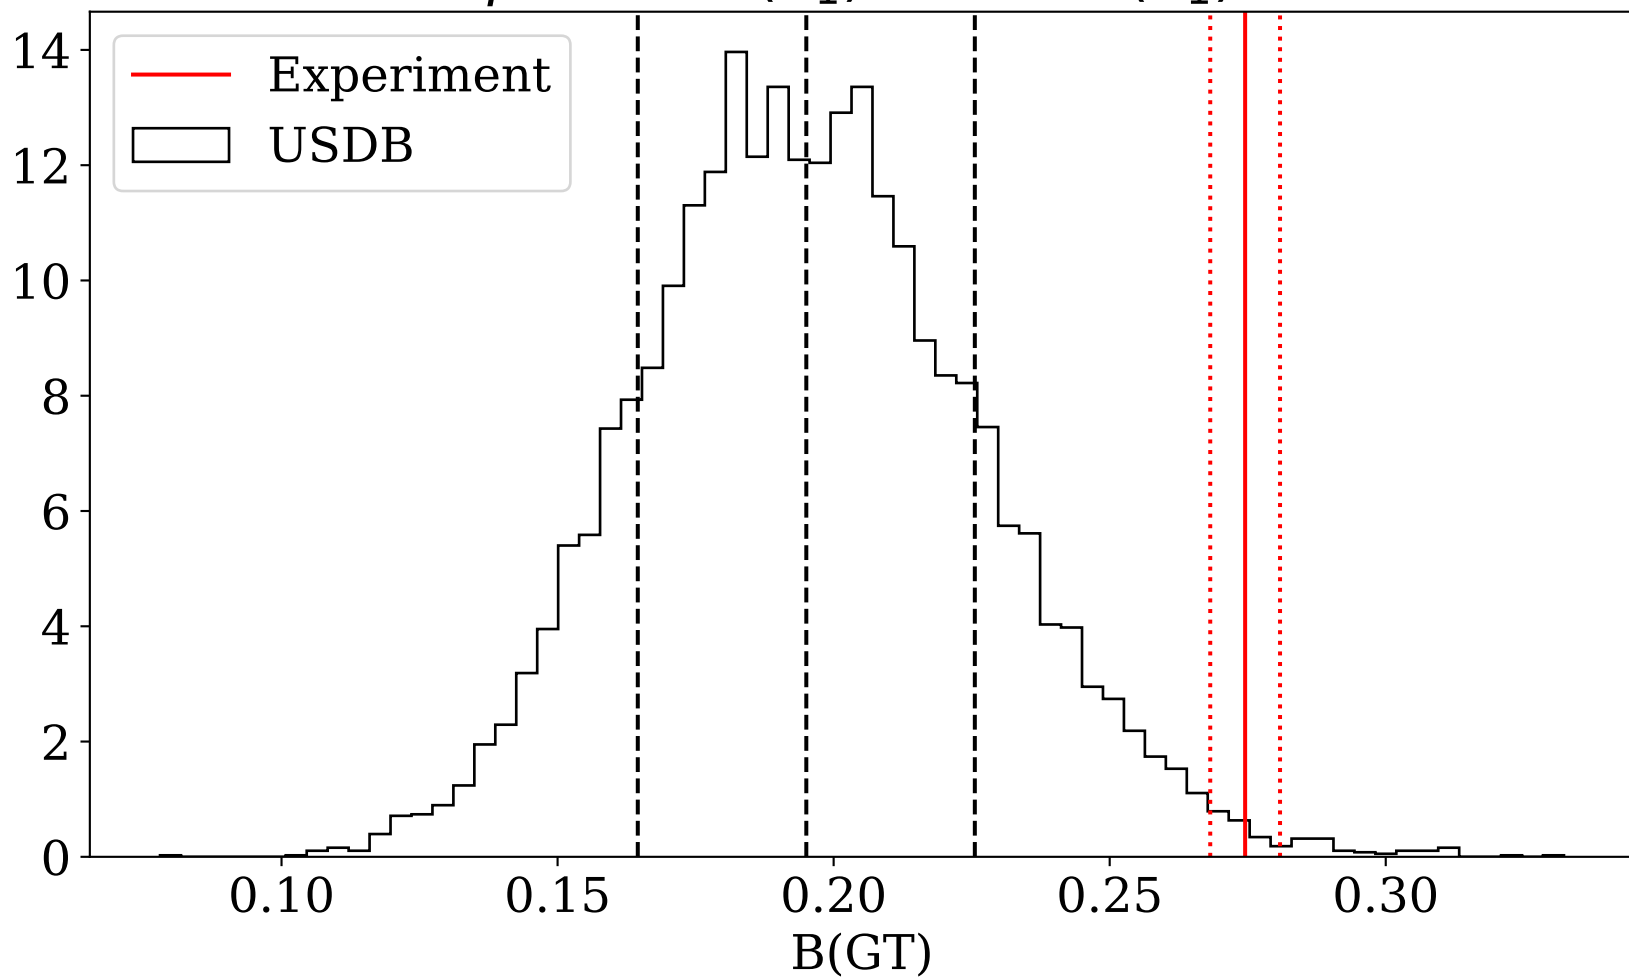

$\beta^- : {}^{24}\text{Ne}(0_1) \rightarrow {}^{24}\text{Na}(1_2)$

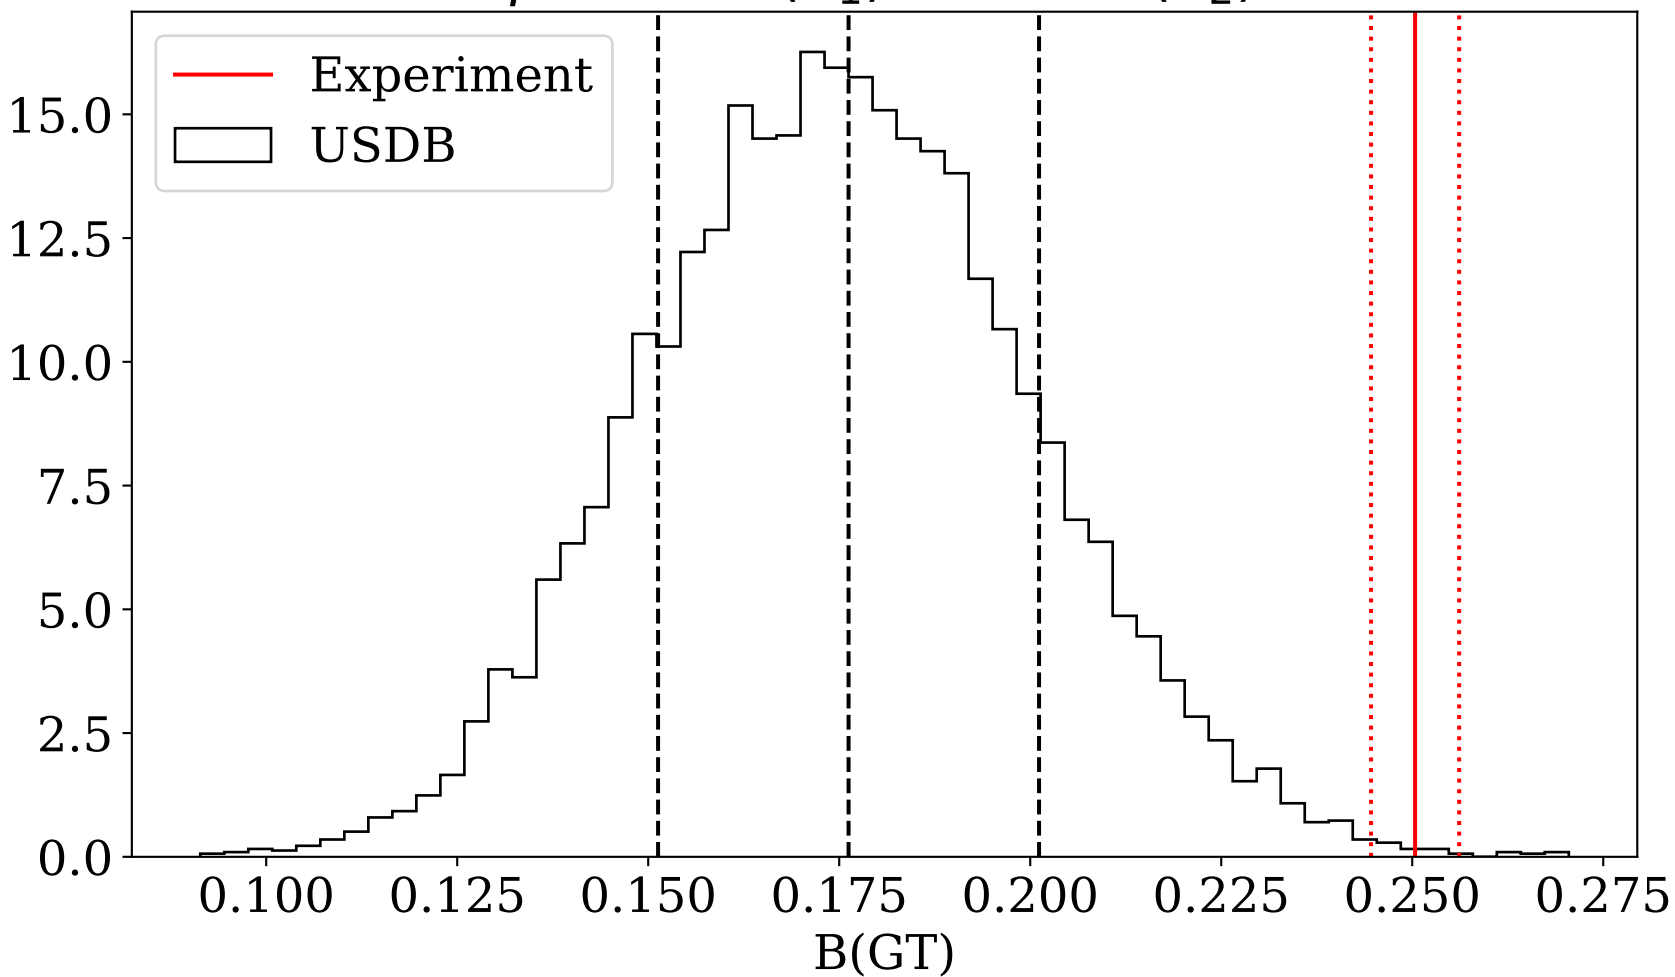

$\beta^- : {}^{25}\text{Ne}(1/2_1) \rightarrow {}^{25}\text{Na}(3/2_1)$

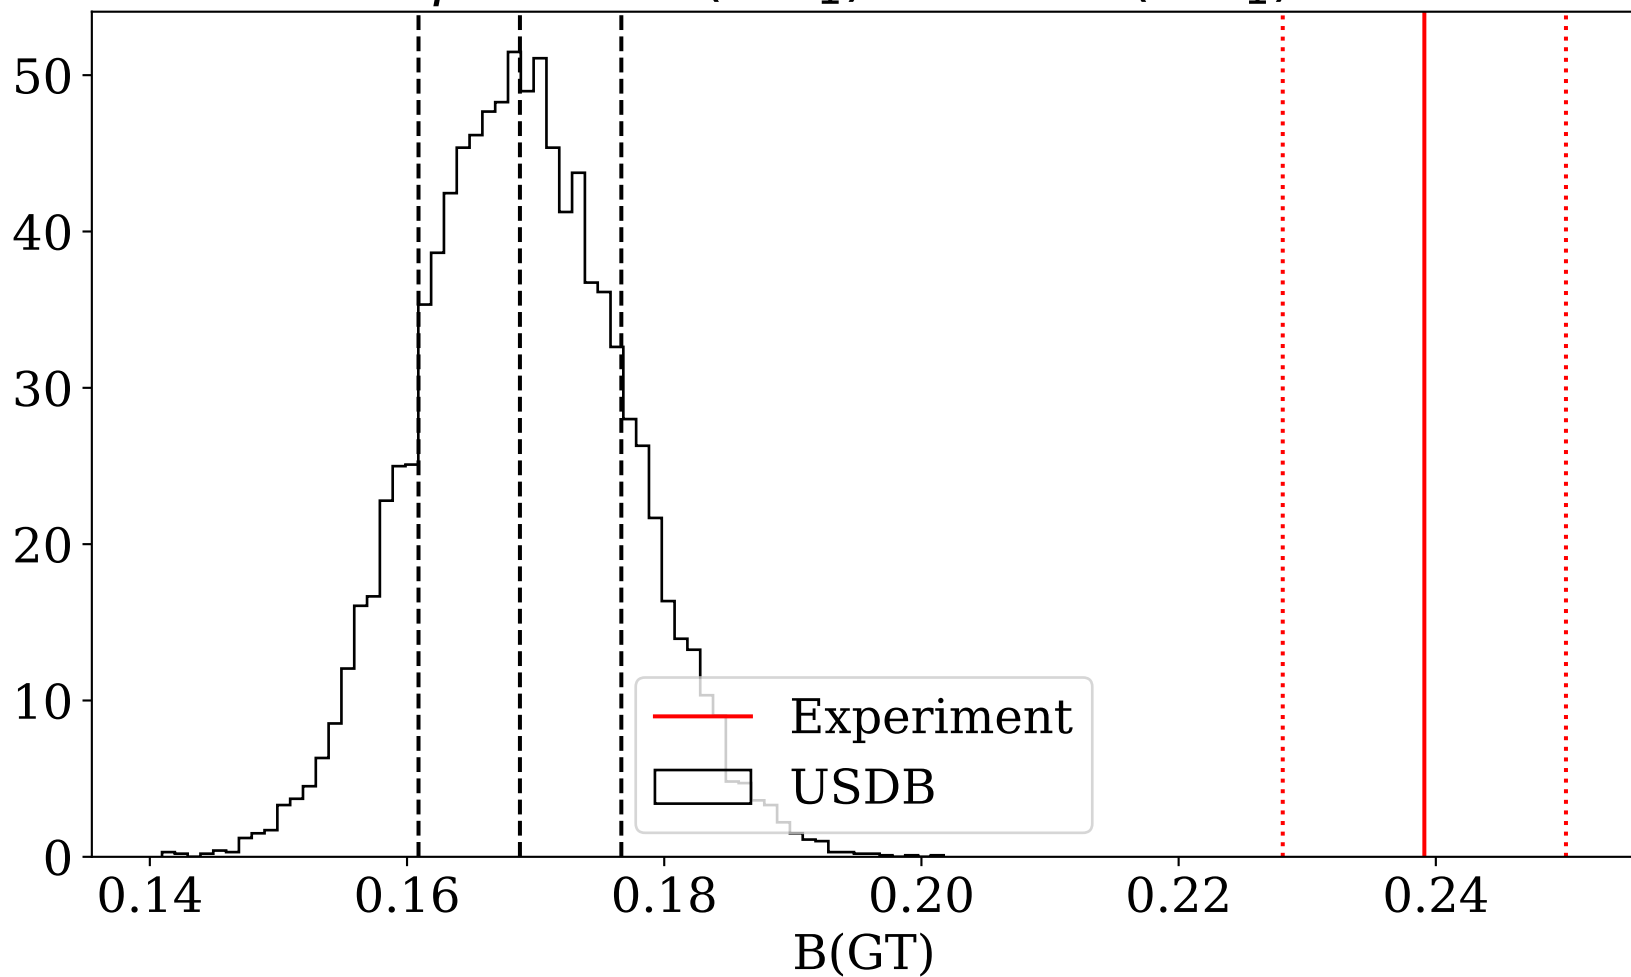



$\beta^- : {}^{25}\text{Ne}(1/2_1) \rightarrow {}^{25}\text{Na}(1/2_1)$

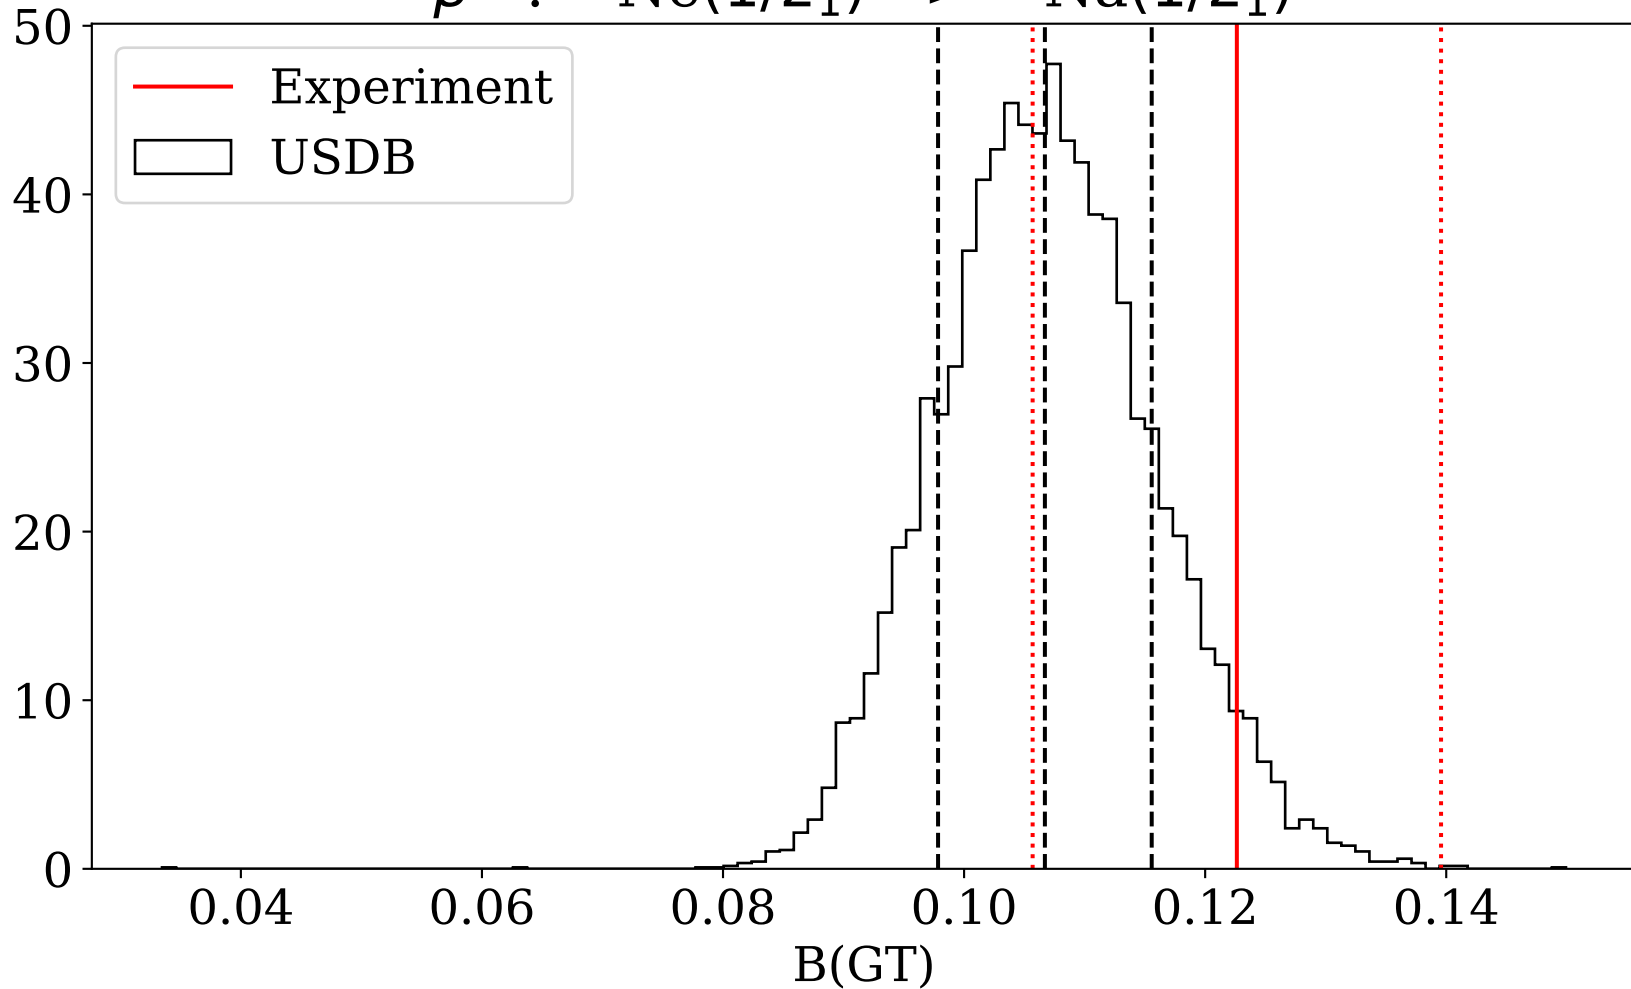

$\beta^- : {}^{25}\text{Ne}(1/2_1) \rightarrow {}^{25}\text{Na}(3/2_2)$

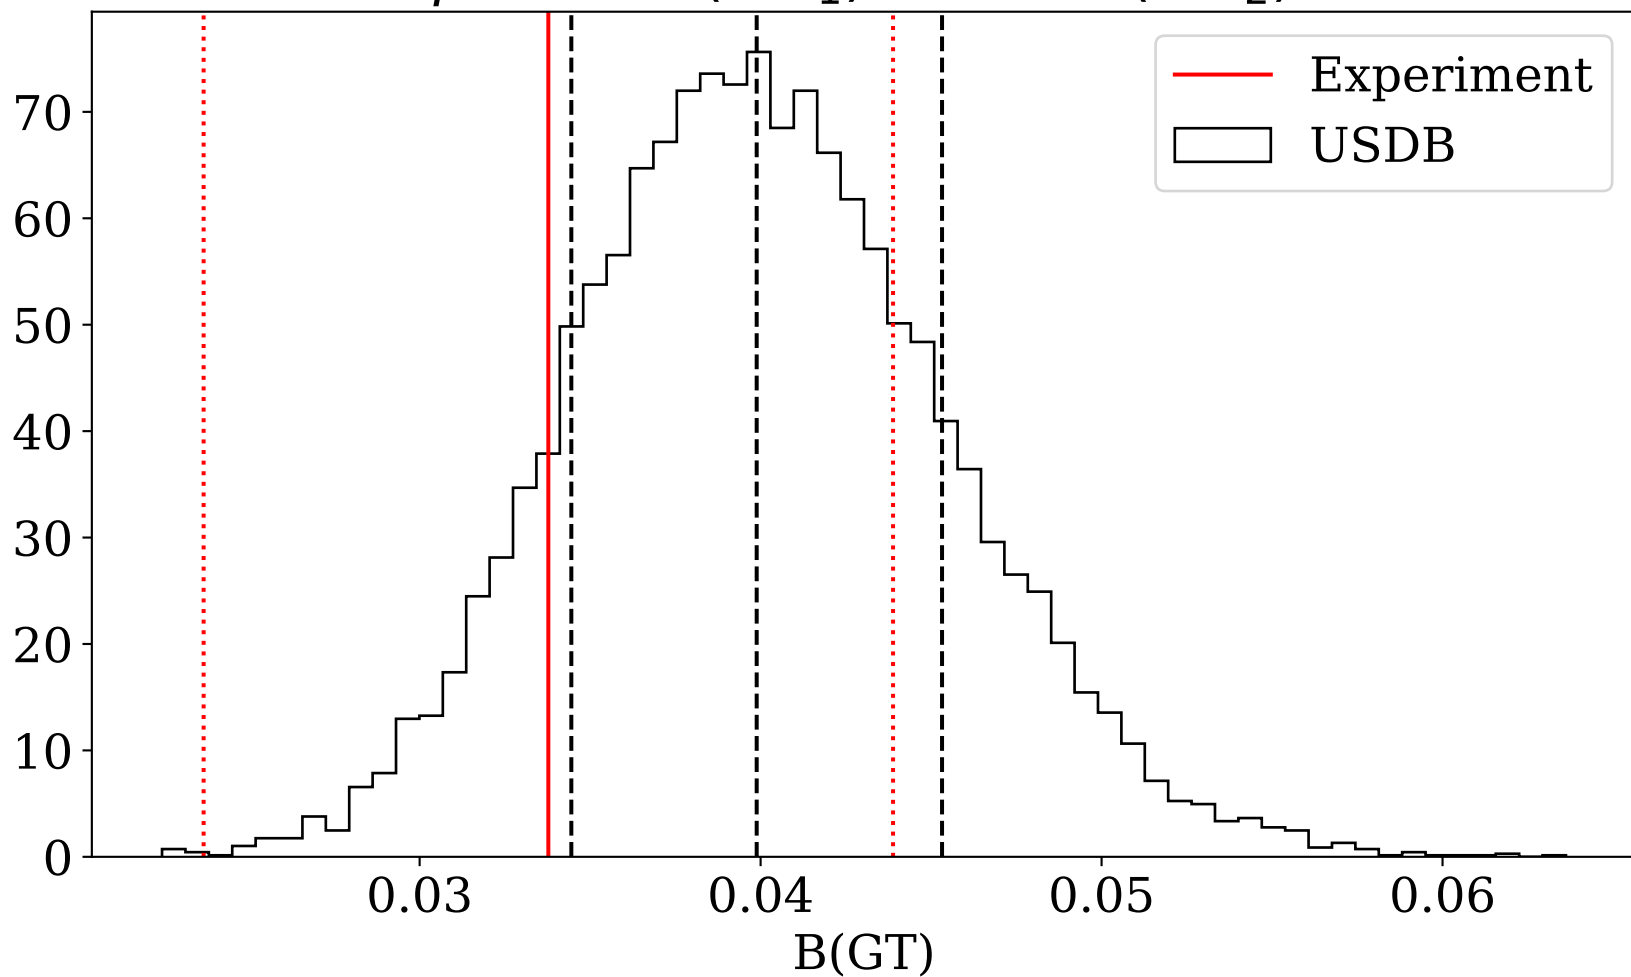

$\beta^- : {}^{25}\text{Ne}(1/2_1) \rightarrow {}^{25}\text{Na}(1/2_2)$

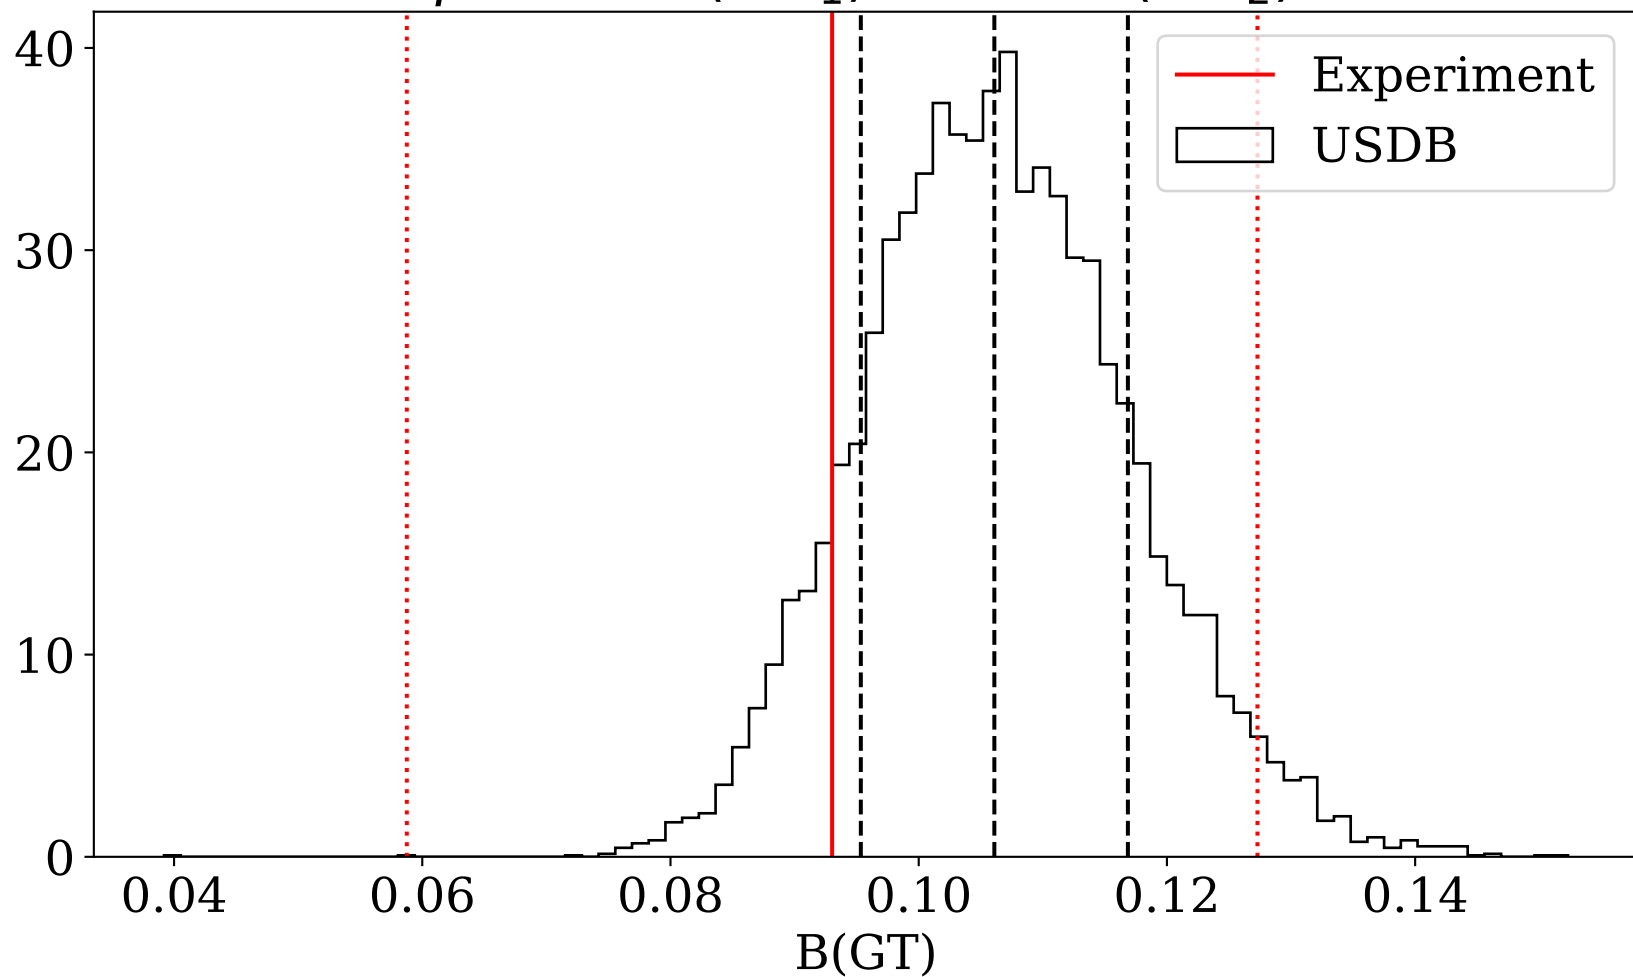

$\beta^- : {}^{26}\text{Ne}(0_1) \rightarrow {}^{26}\text{Na}(1_1)$

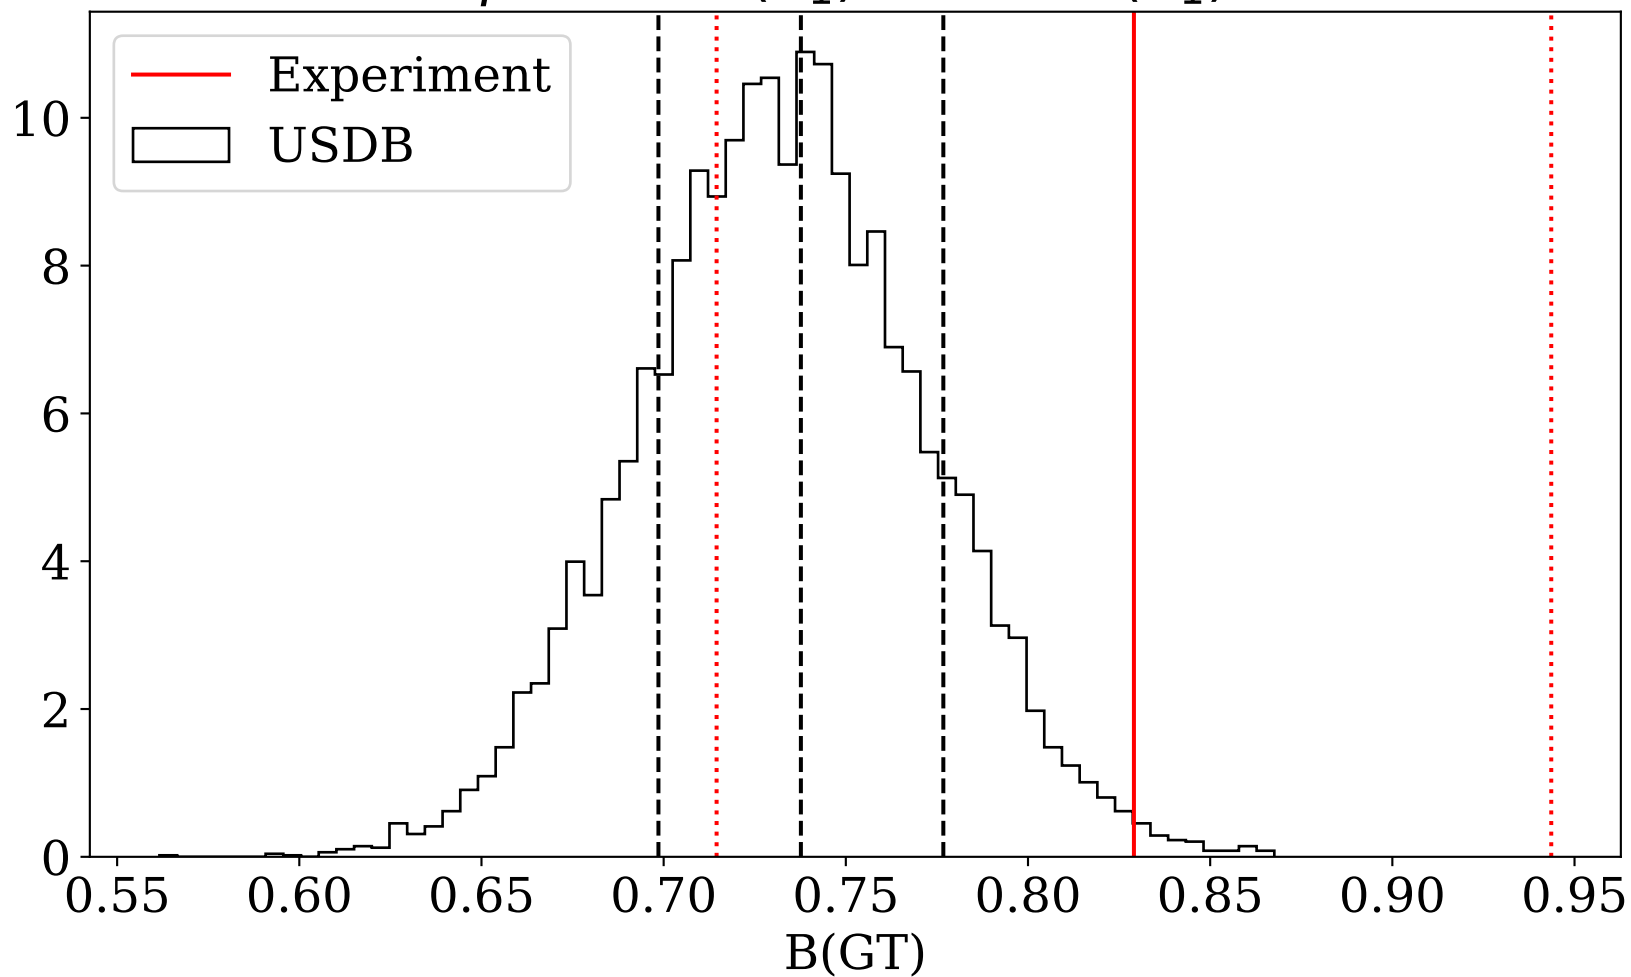

$\beta^- : {}^{27}\text{Ne}(3/2_1) \rightarrow {}^{27}\text{Na}(5/2_1)$

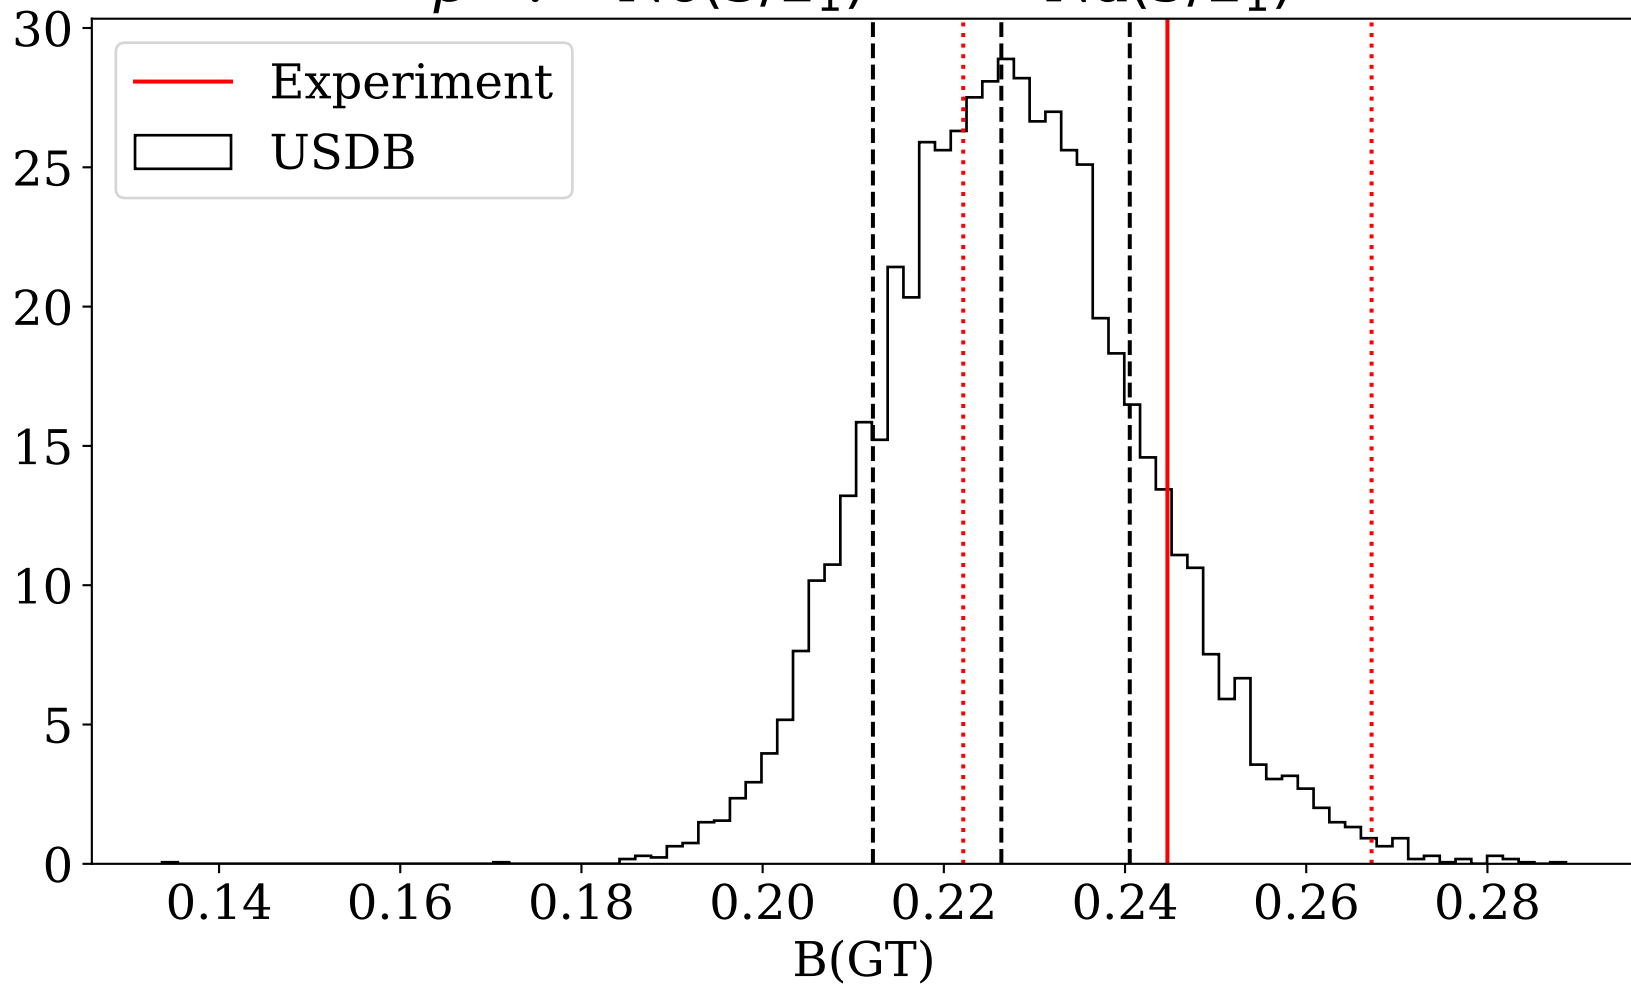

$\beta^- : {}^{27}\text{Ne}(3/2_1) \rightarrow {}^{27}\text{Na}(3/2_1)$

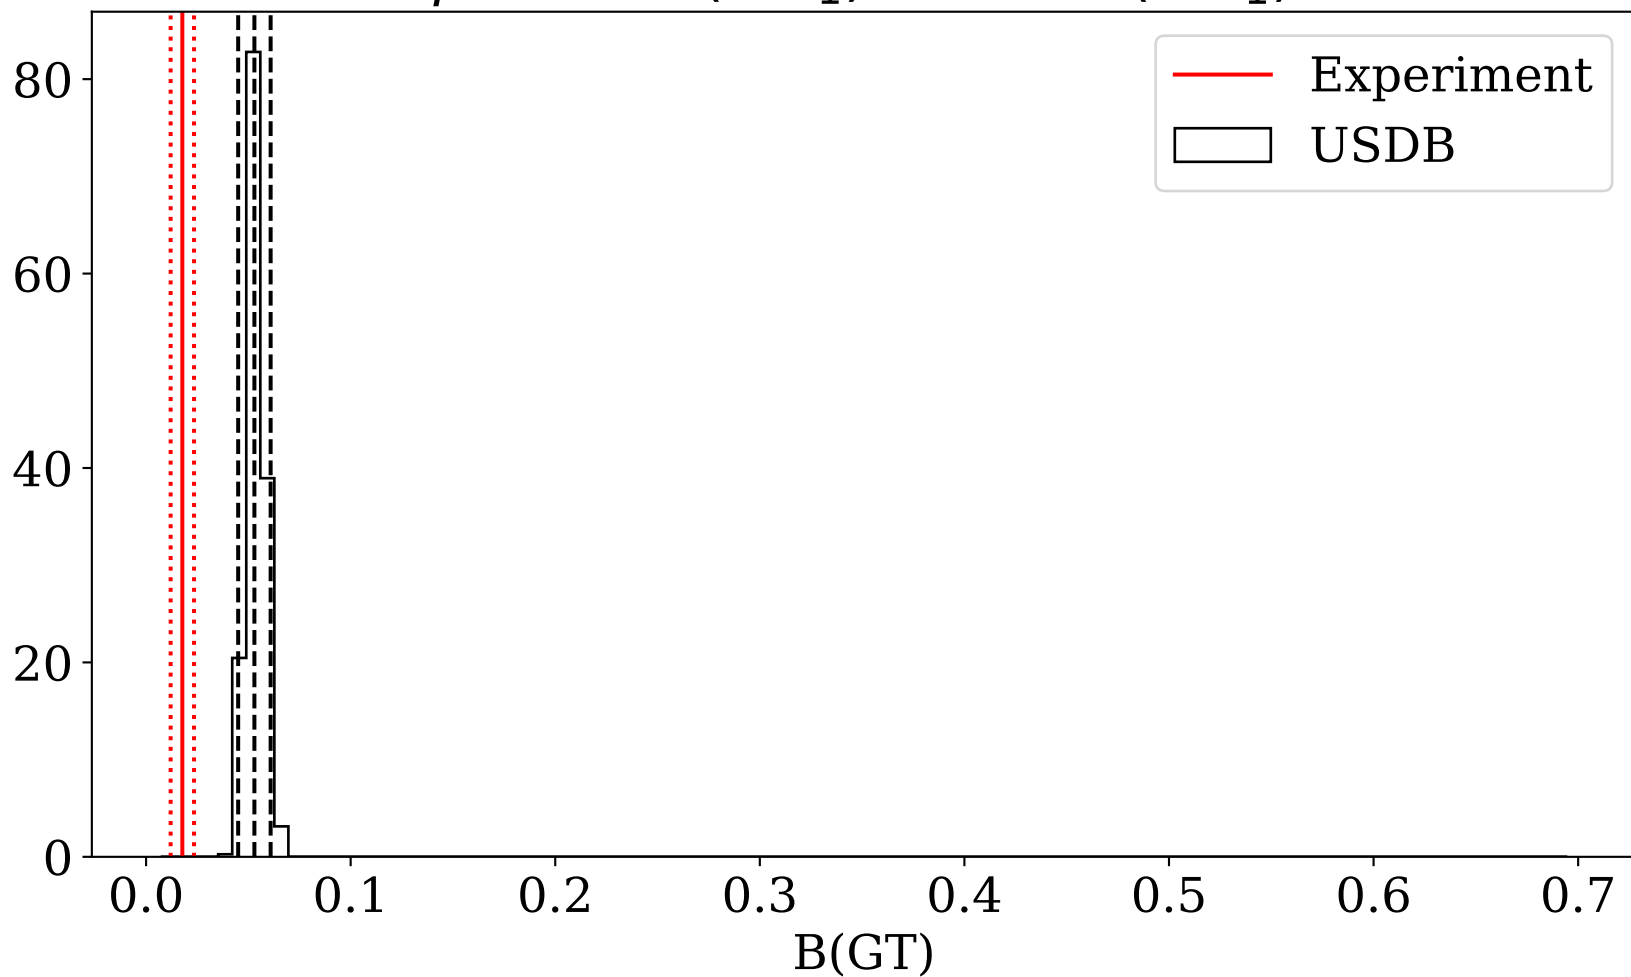

$\beta^- : {}^{27}\text{Ne}(3/2_1) \rightarrow {}^{27}\text{Na}(1/2_1)$

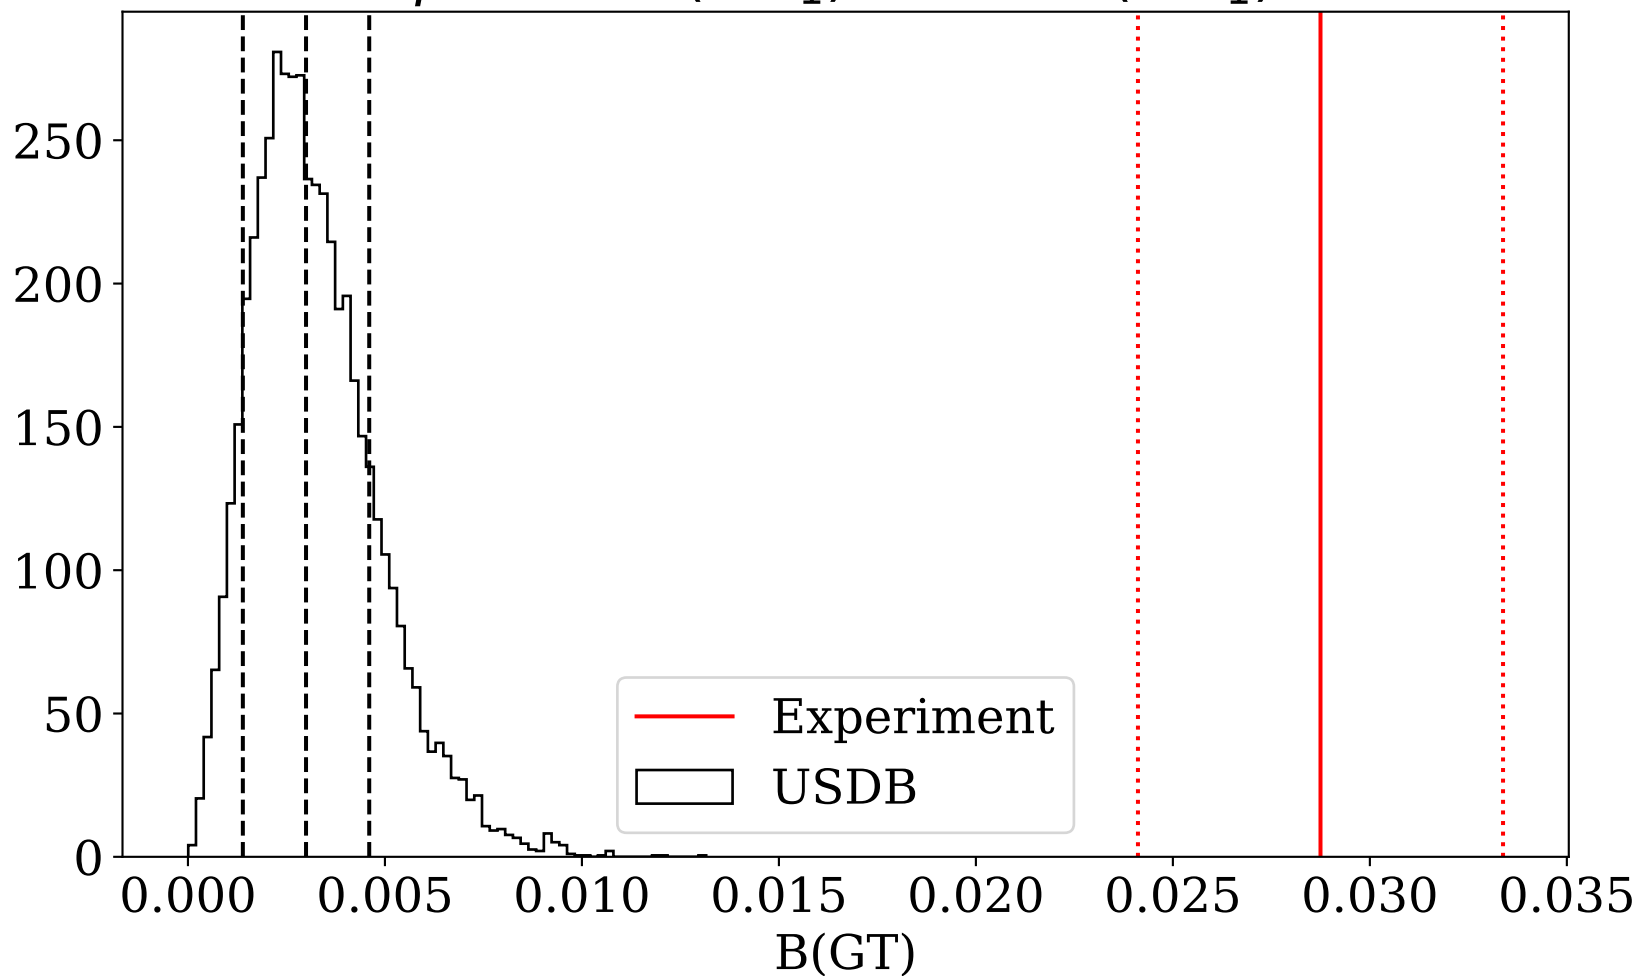

$\beta^- : {}^{28}\text{Ne}(0_1) \rightarrow {}^{28}\text{Na}(1_1)$

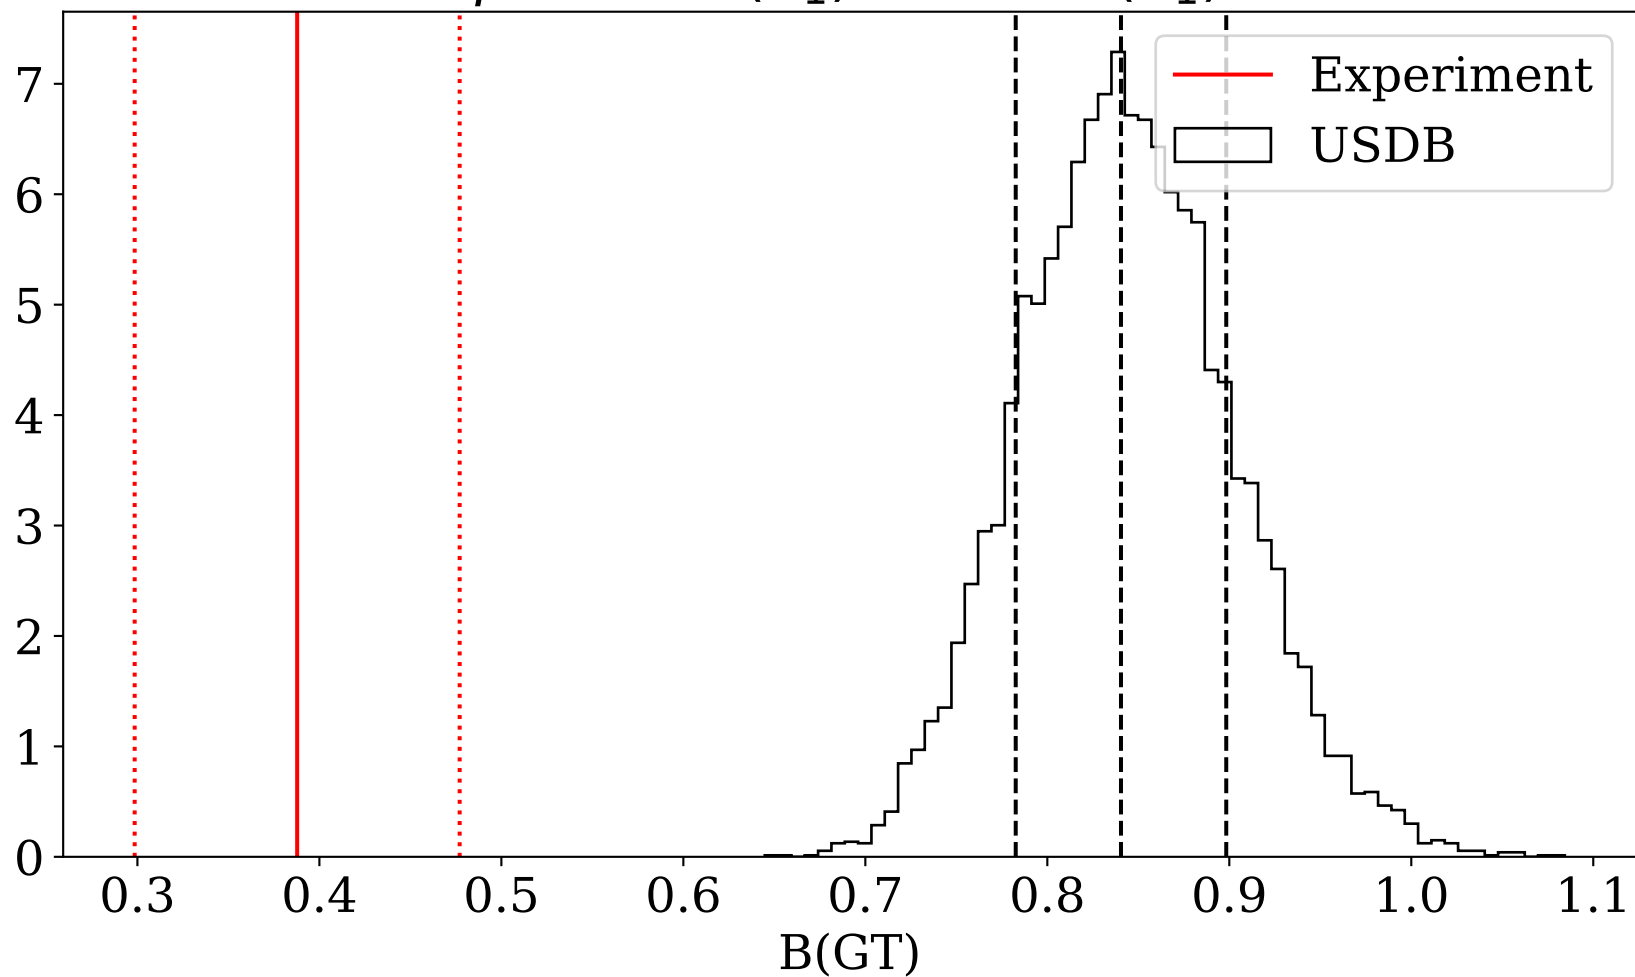



$\beta^- : {}^{28}\text{Ne}(0_1) \rightarrow {}^{28}\text{Na}(1_2)$

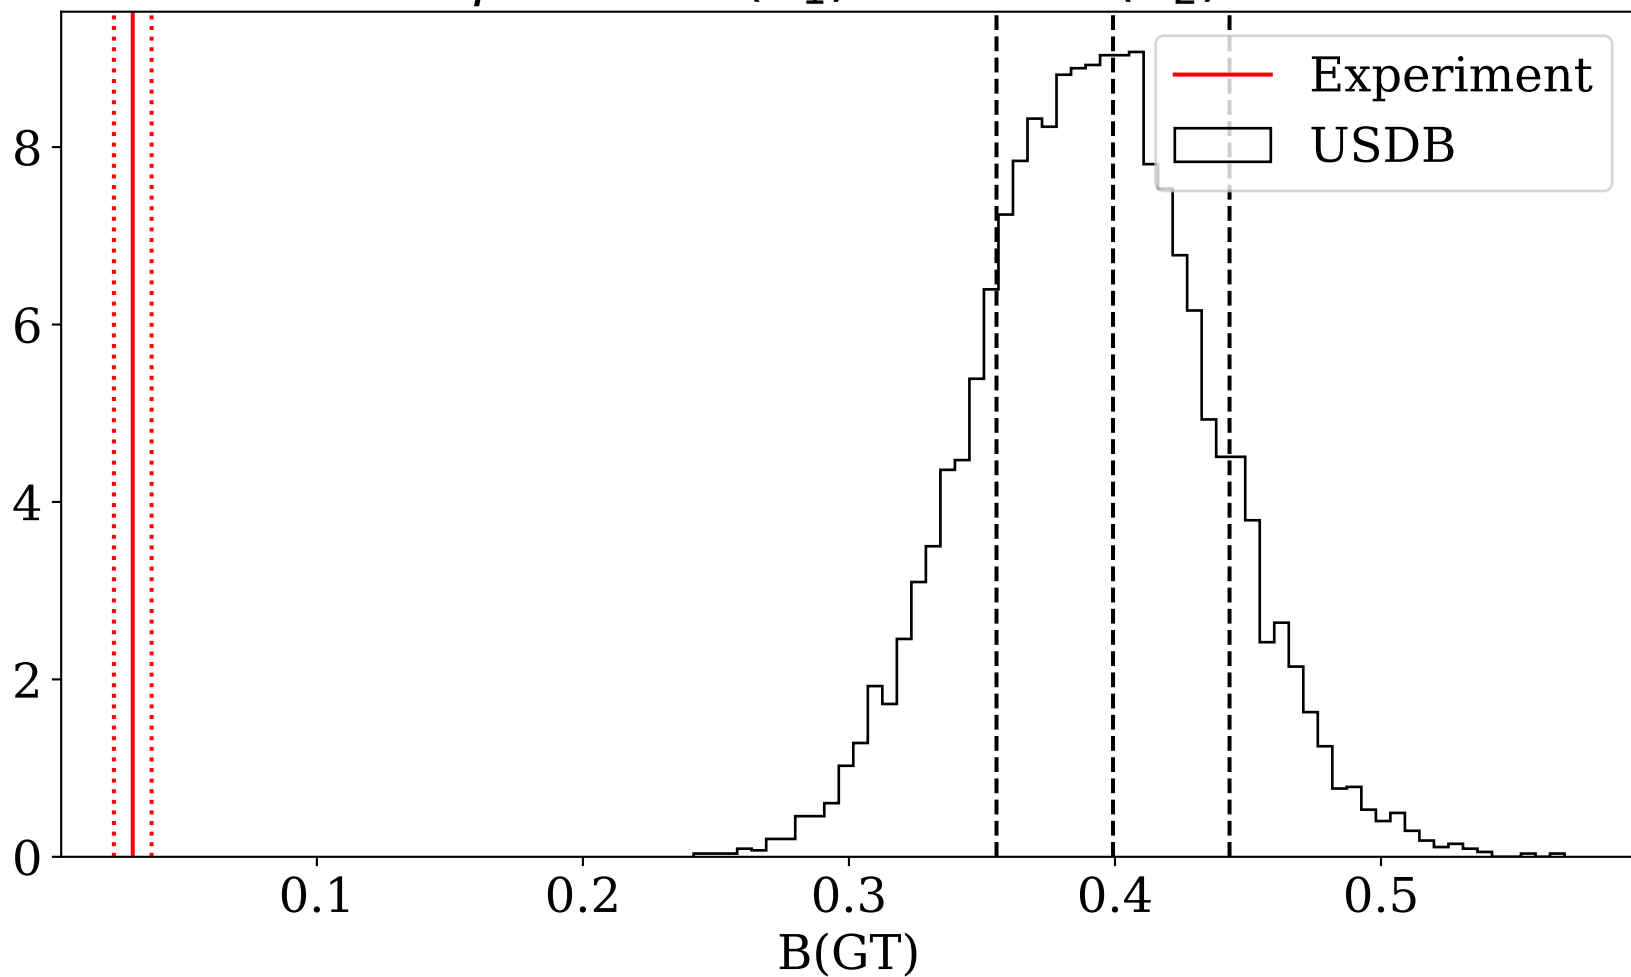

$\beta^- : {}^{28}\text{Ne}(0_1) \rightarrow {}^{28}\text{Na}(1_3)$

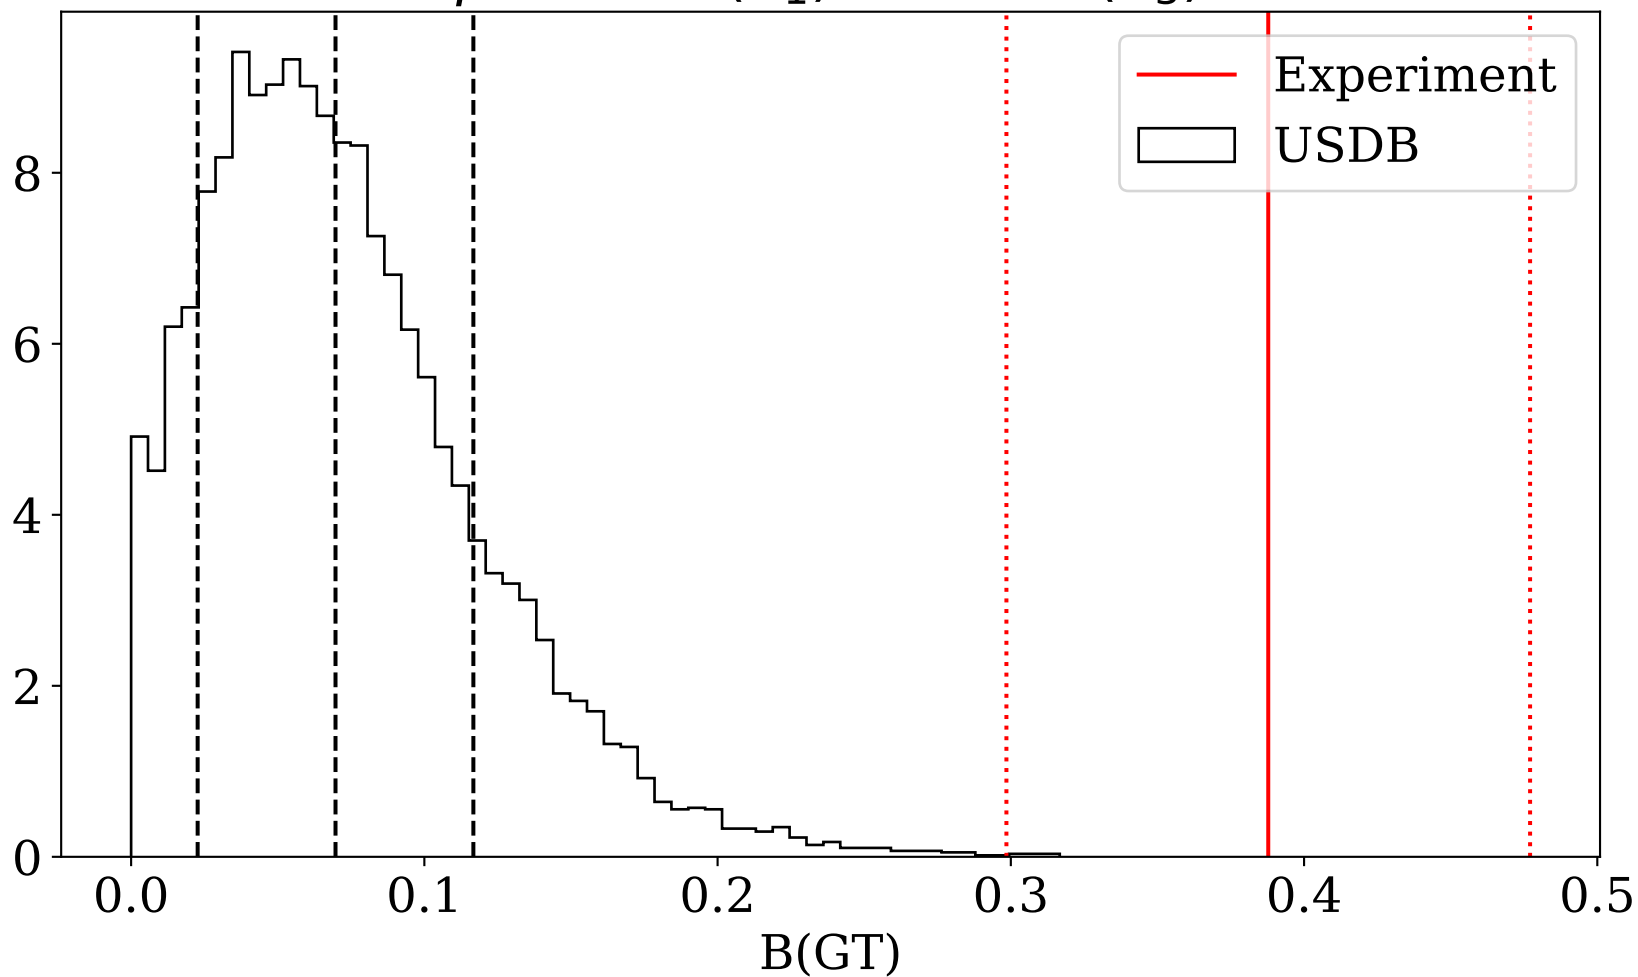

$\beta^- : {}^{28}\text{Ne}(0_1) \rightarrow {}^{28}\text{Na}(1_4)$

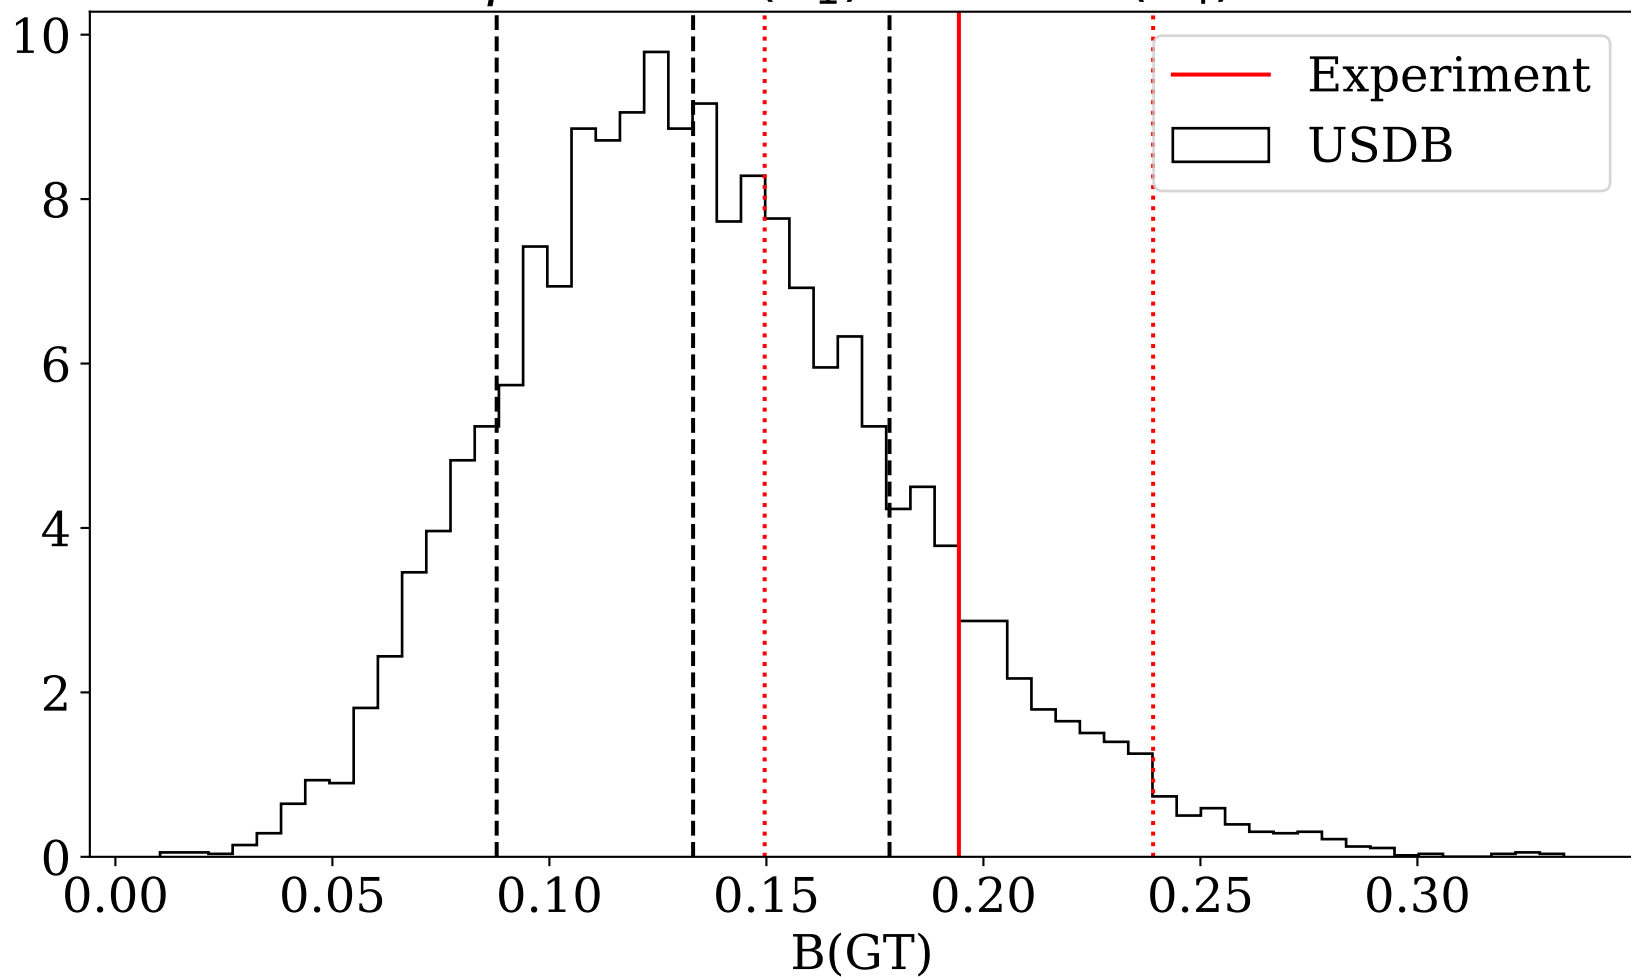

$\beta^- : {}^{28}\text{Ne}(0_1) \rightarrow {}^{28}\text{Na}(1_5)$

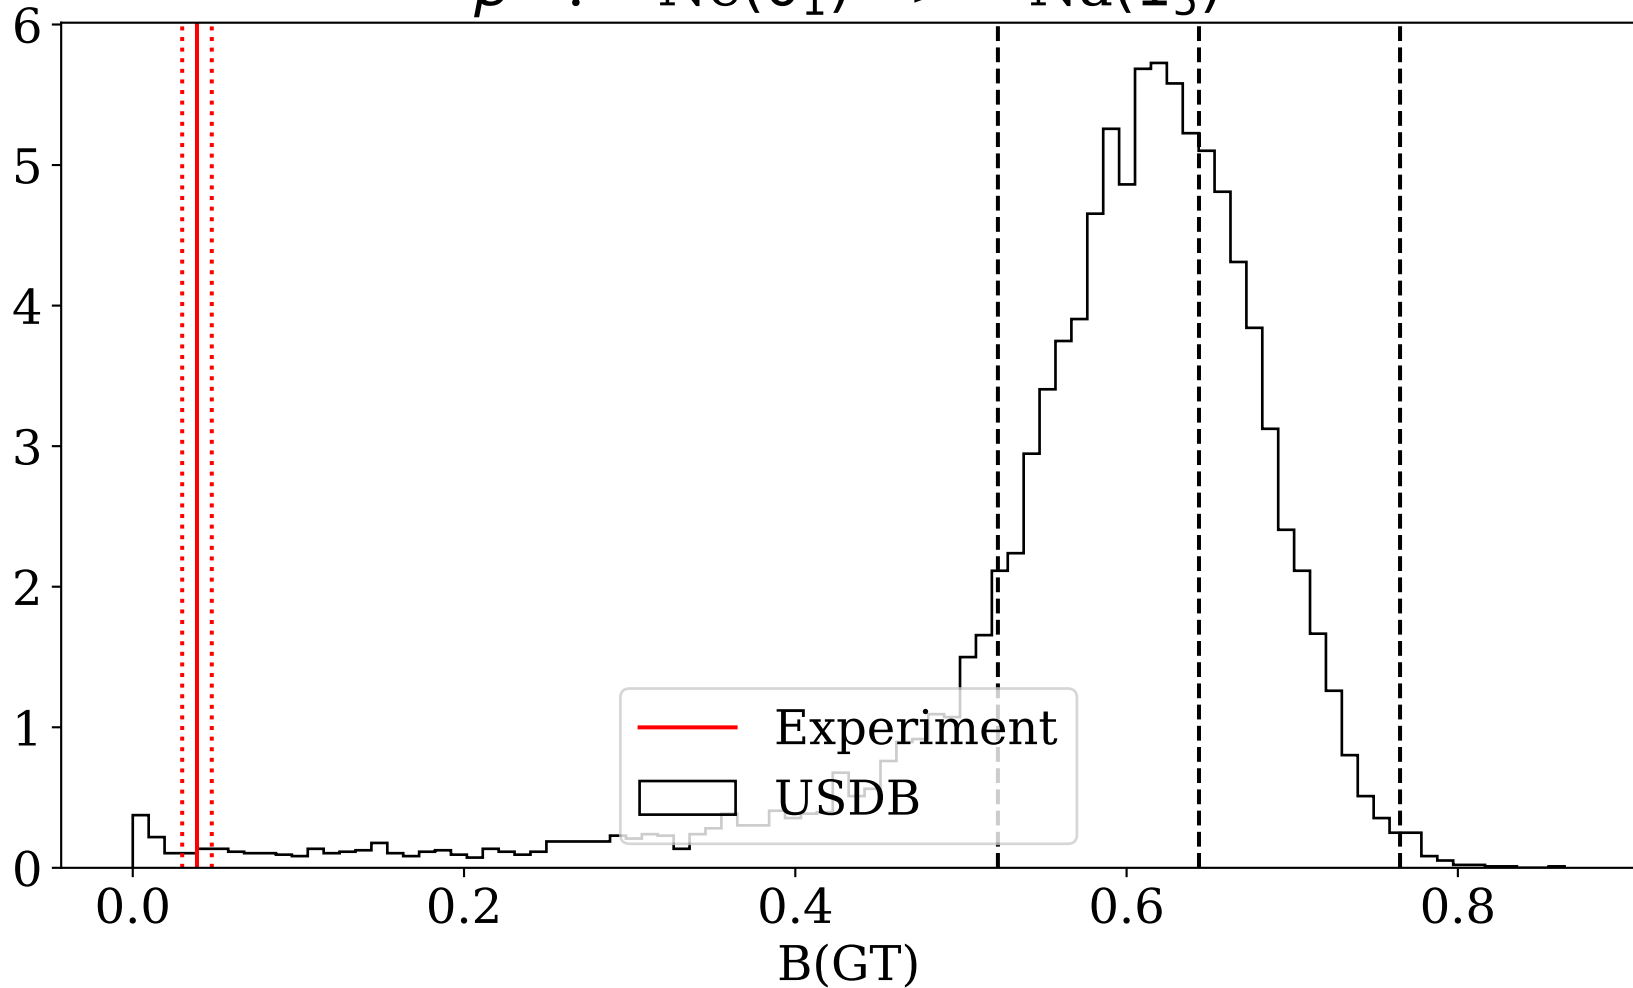

$\beta^- : {}^{28}\text{Ne}(0_1) \rightarrow {}^{28}\text{Na}(1_6)$

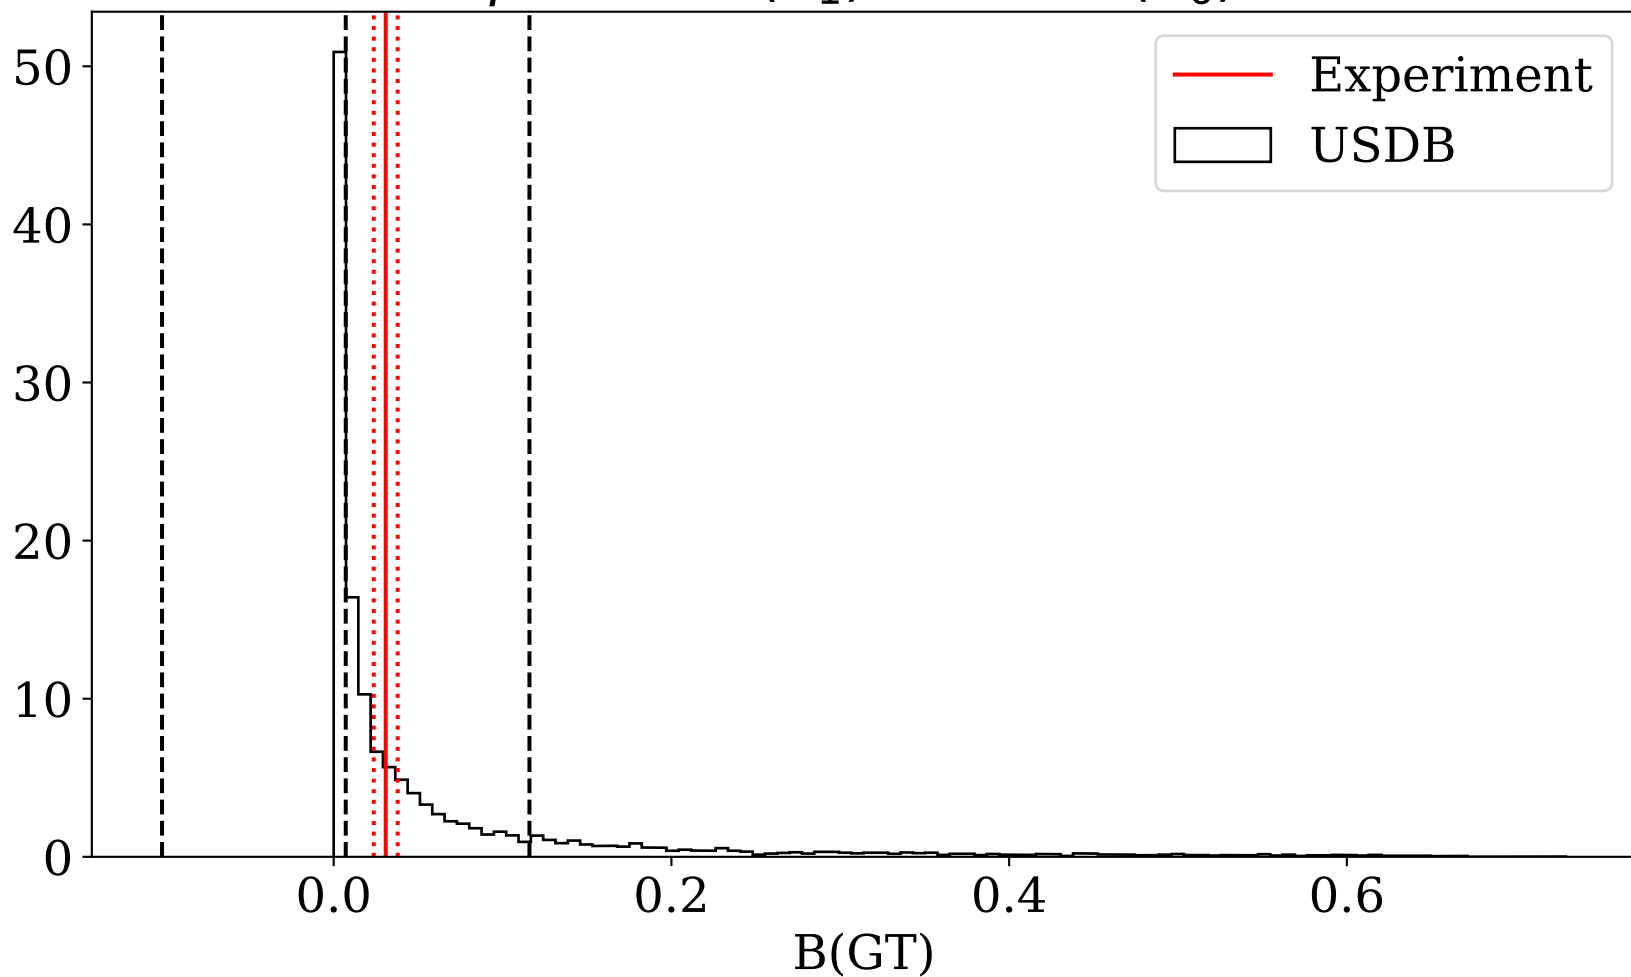

$\beta^- : {}^{24}\text{Na}(1_1) \rightarrow {}^{24}\text{Mg}(0_1)$

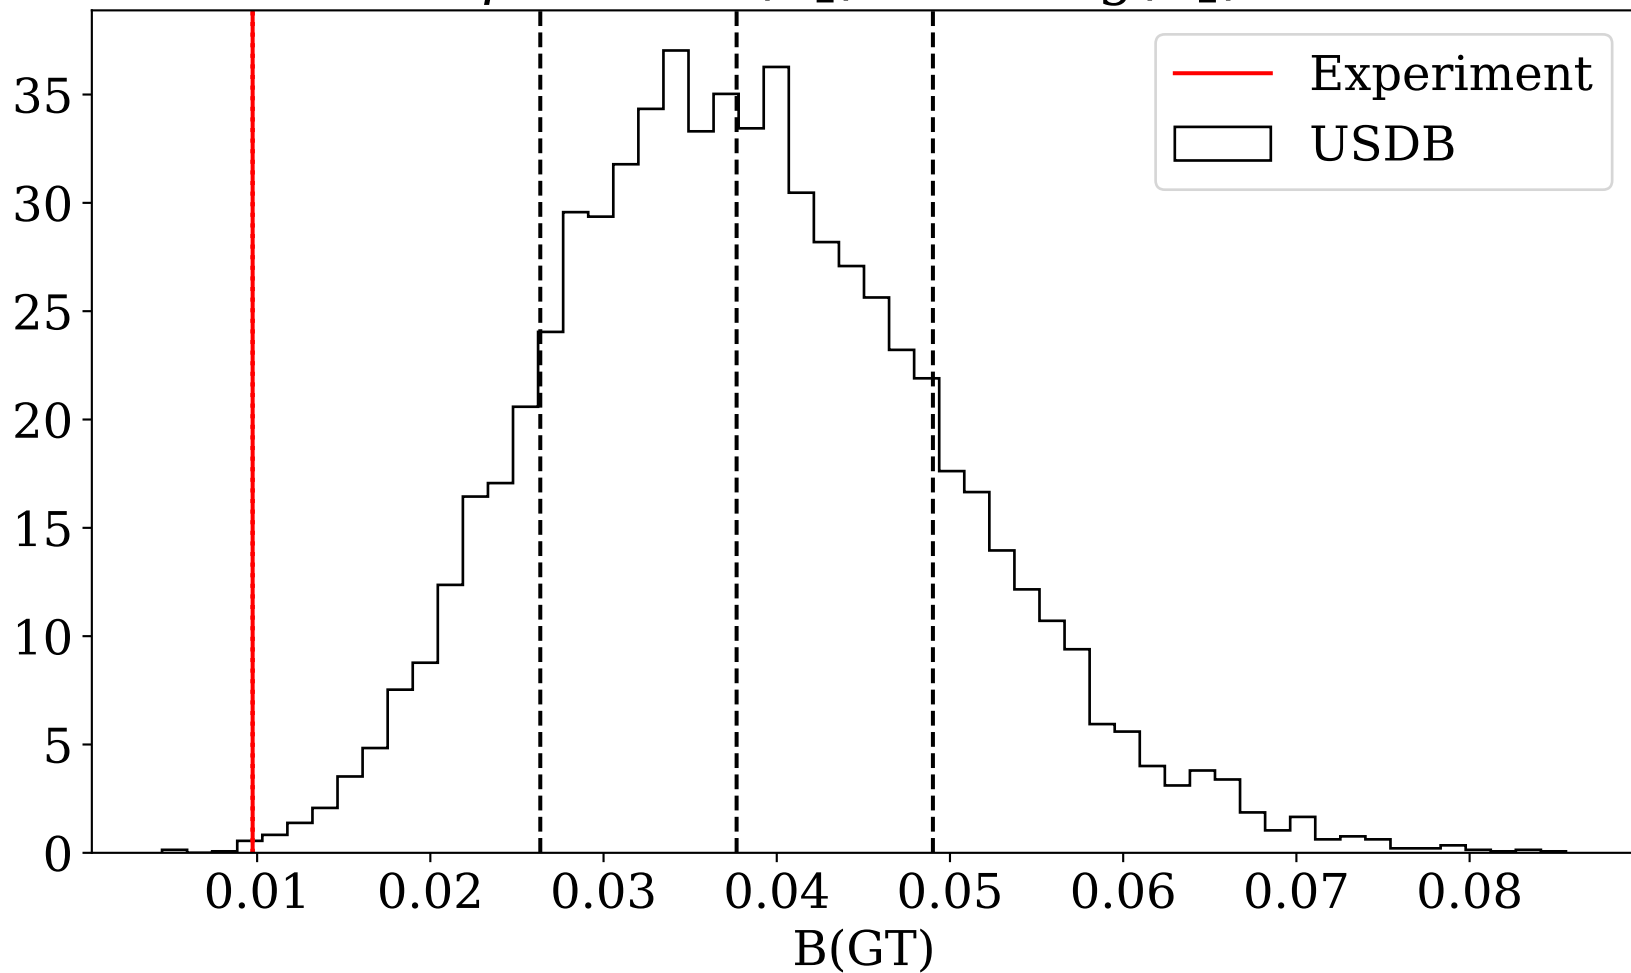

$\beta^- : {}^{25}\text{Na}(5/2_1) \rightarrow {}^{25}\text{Mg}(5/2_1)$

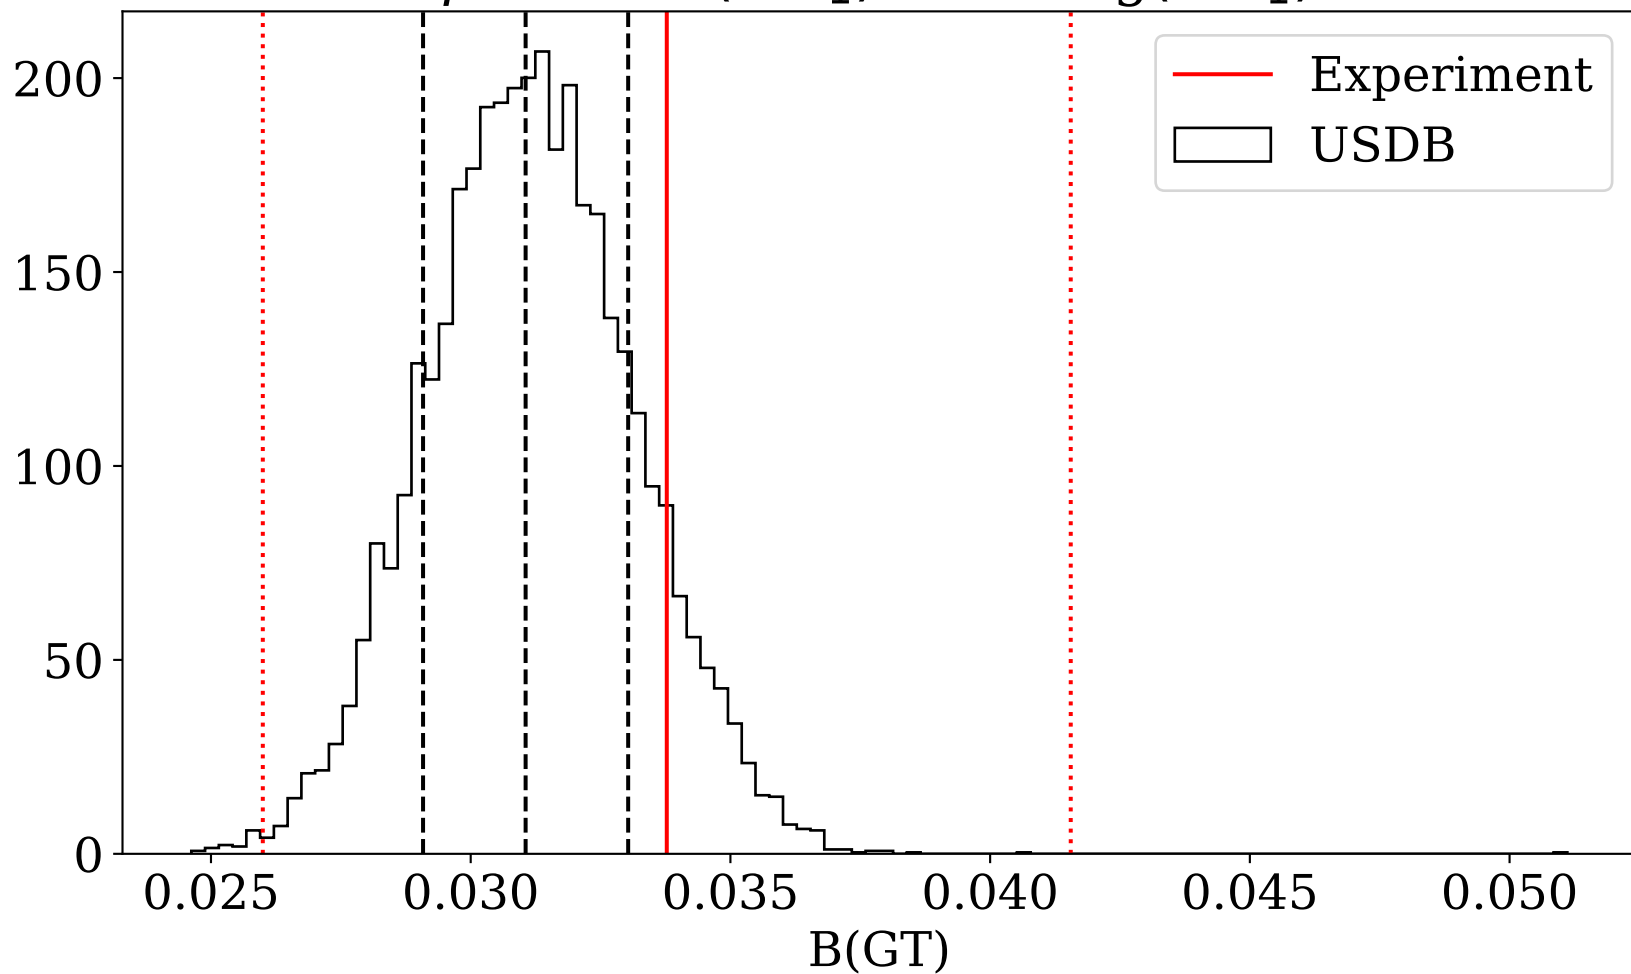

$\beta^- : {}^{25}\text{Na}(5/2_1) \rightarrow {}^{25}\text{Mg}(3/2_1)$

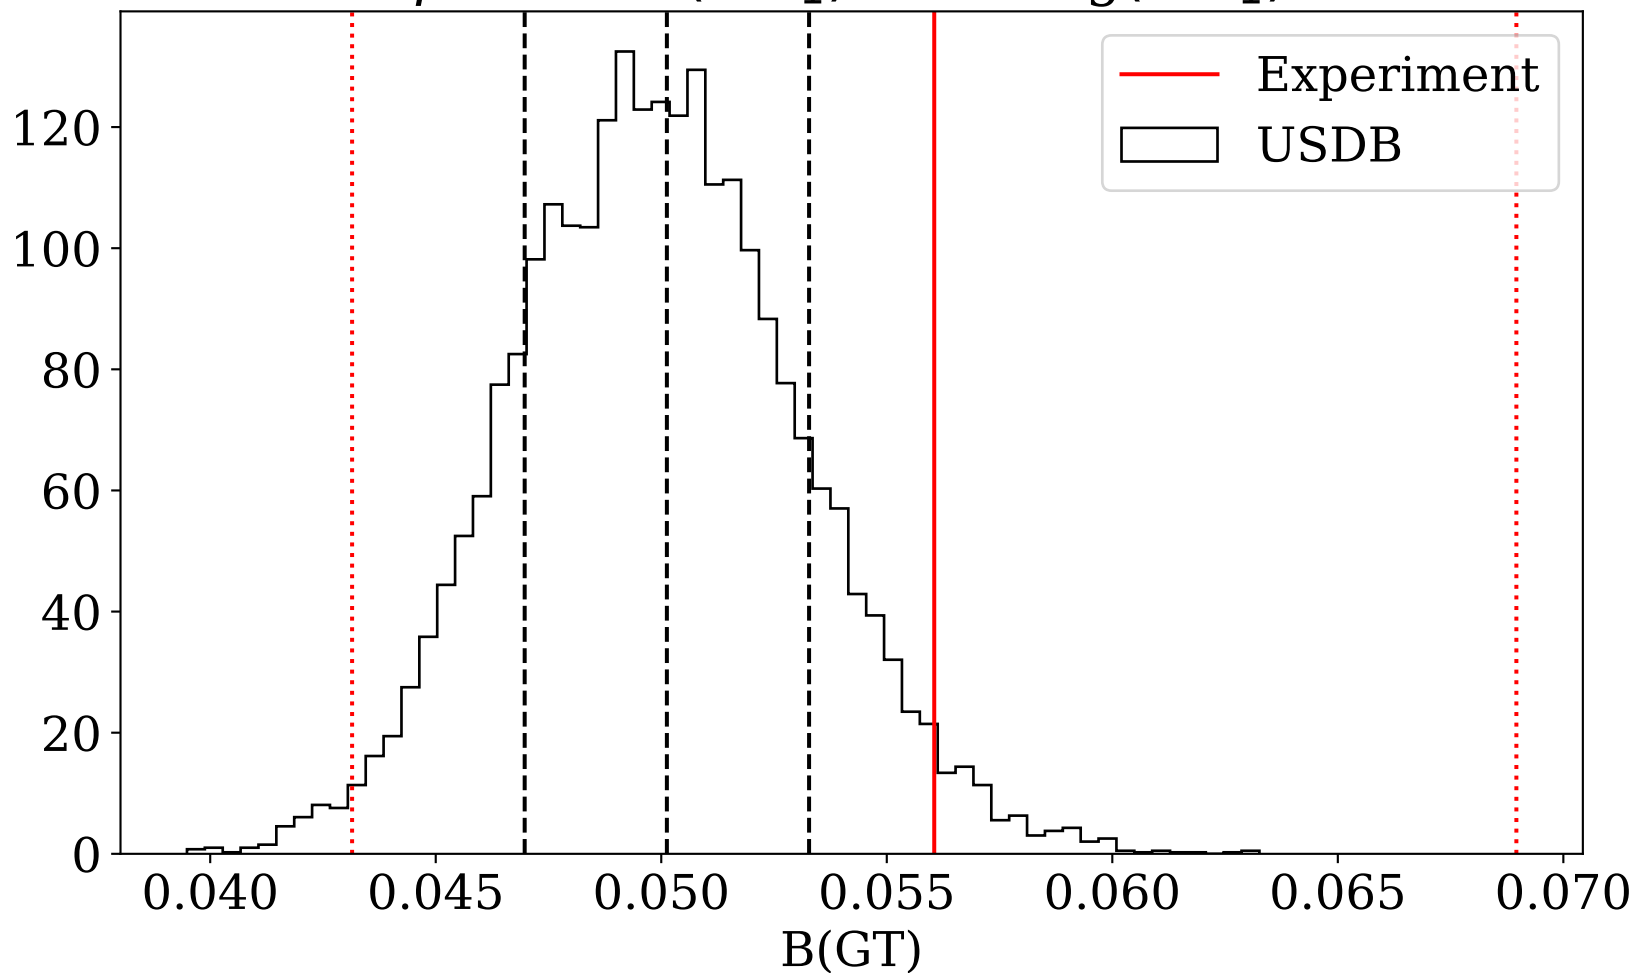



$\beta^- : {}^{25}\text{Na}(5/2_1) \rightarrow {}^{25}\text{Mg}(7/2_1)$

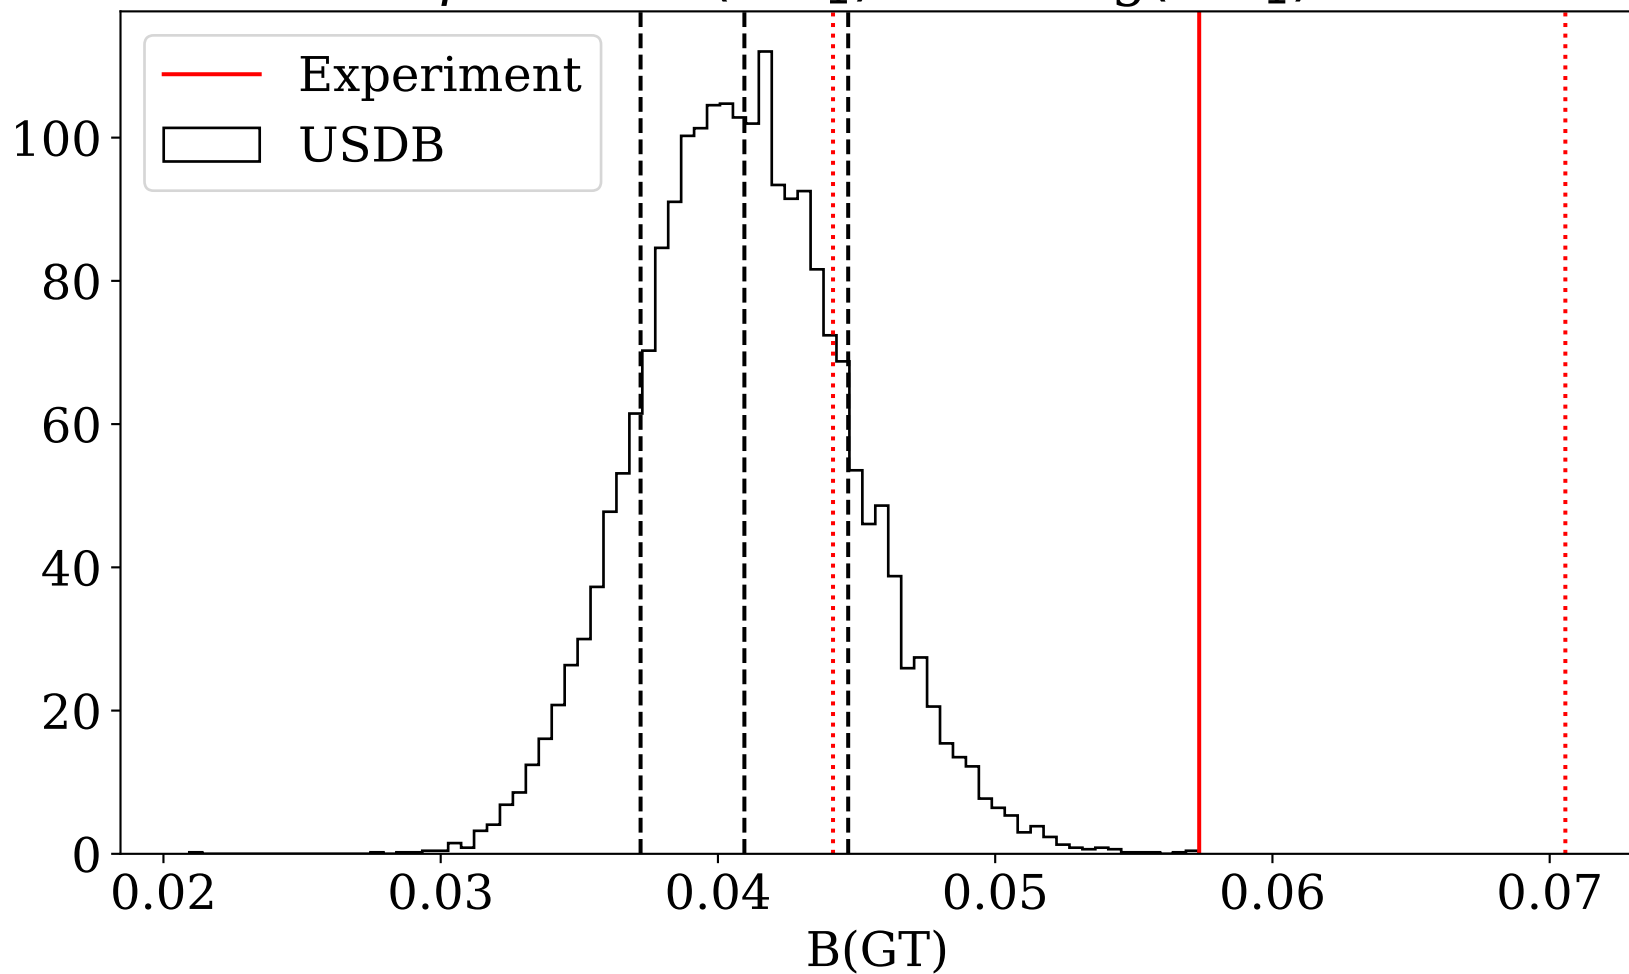

$\beta^- : {}^{25}\text{Na}(5/2_1) \rightarrow {}^{25}\text{Mg}(5/2_2)$

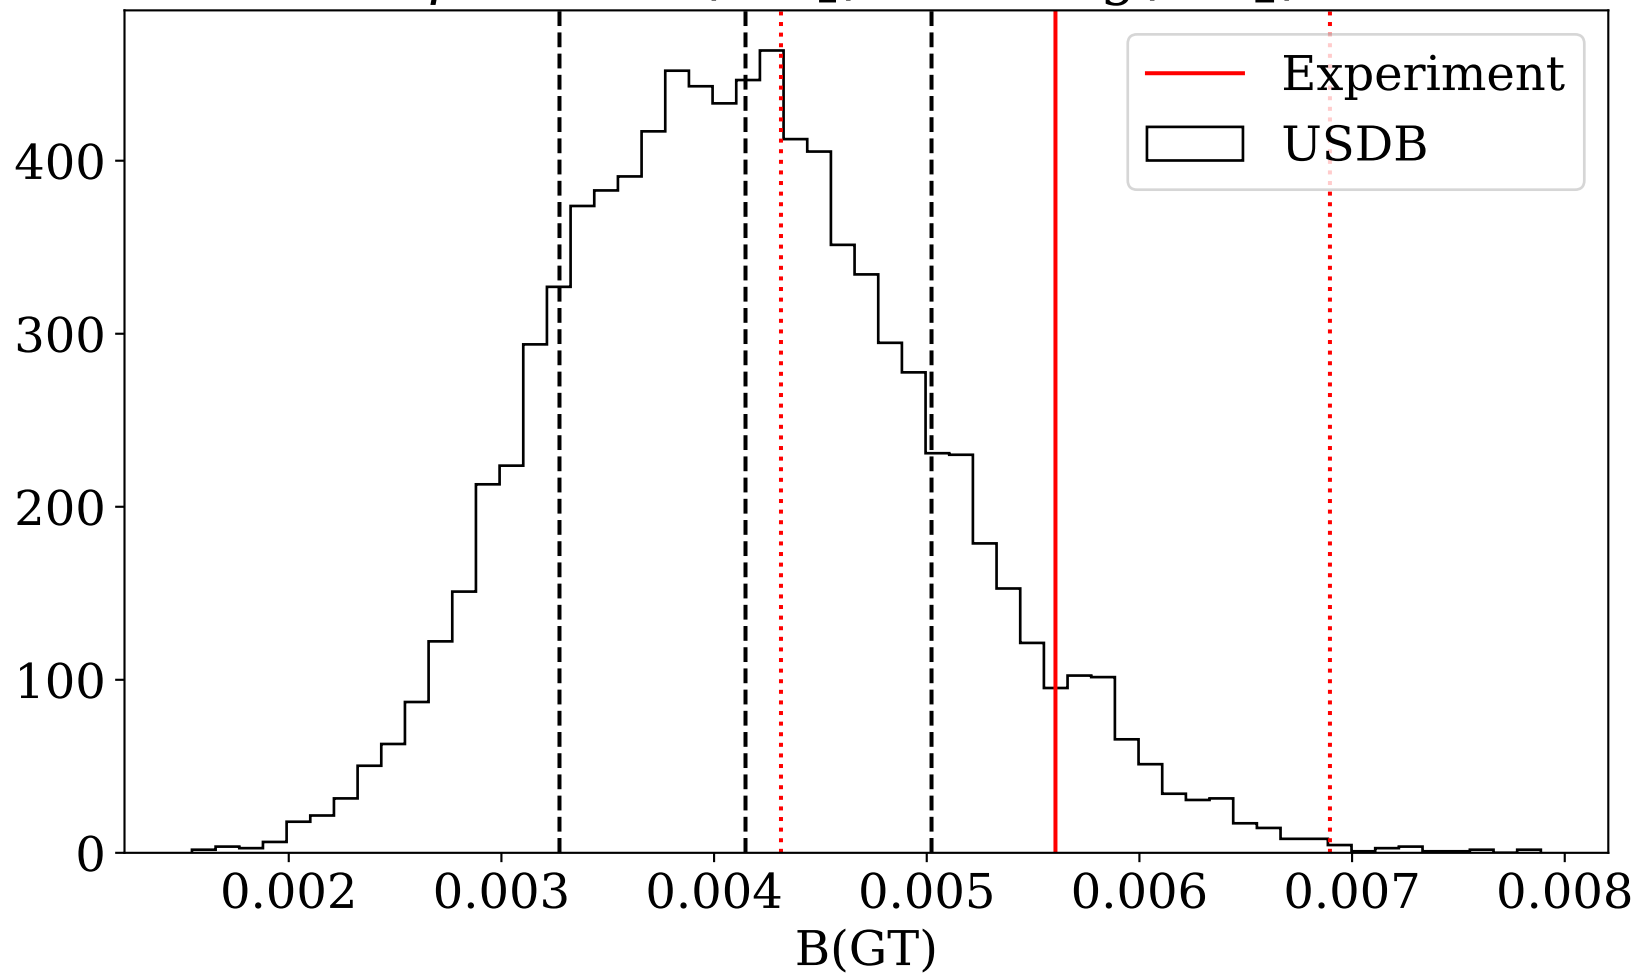

$\beta^- : {}^{25}\text{Na}(5/2_1) \rightarrow {}^{25}\text{Mg}(3/2_2)$

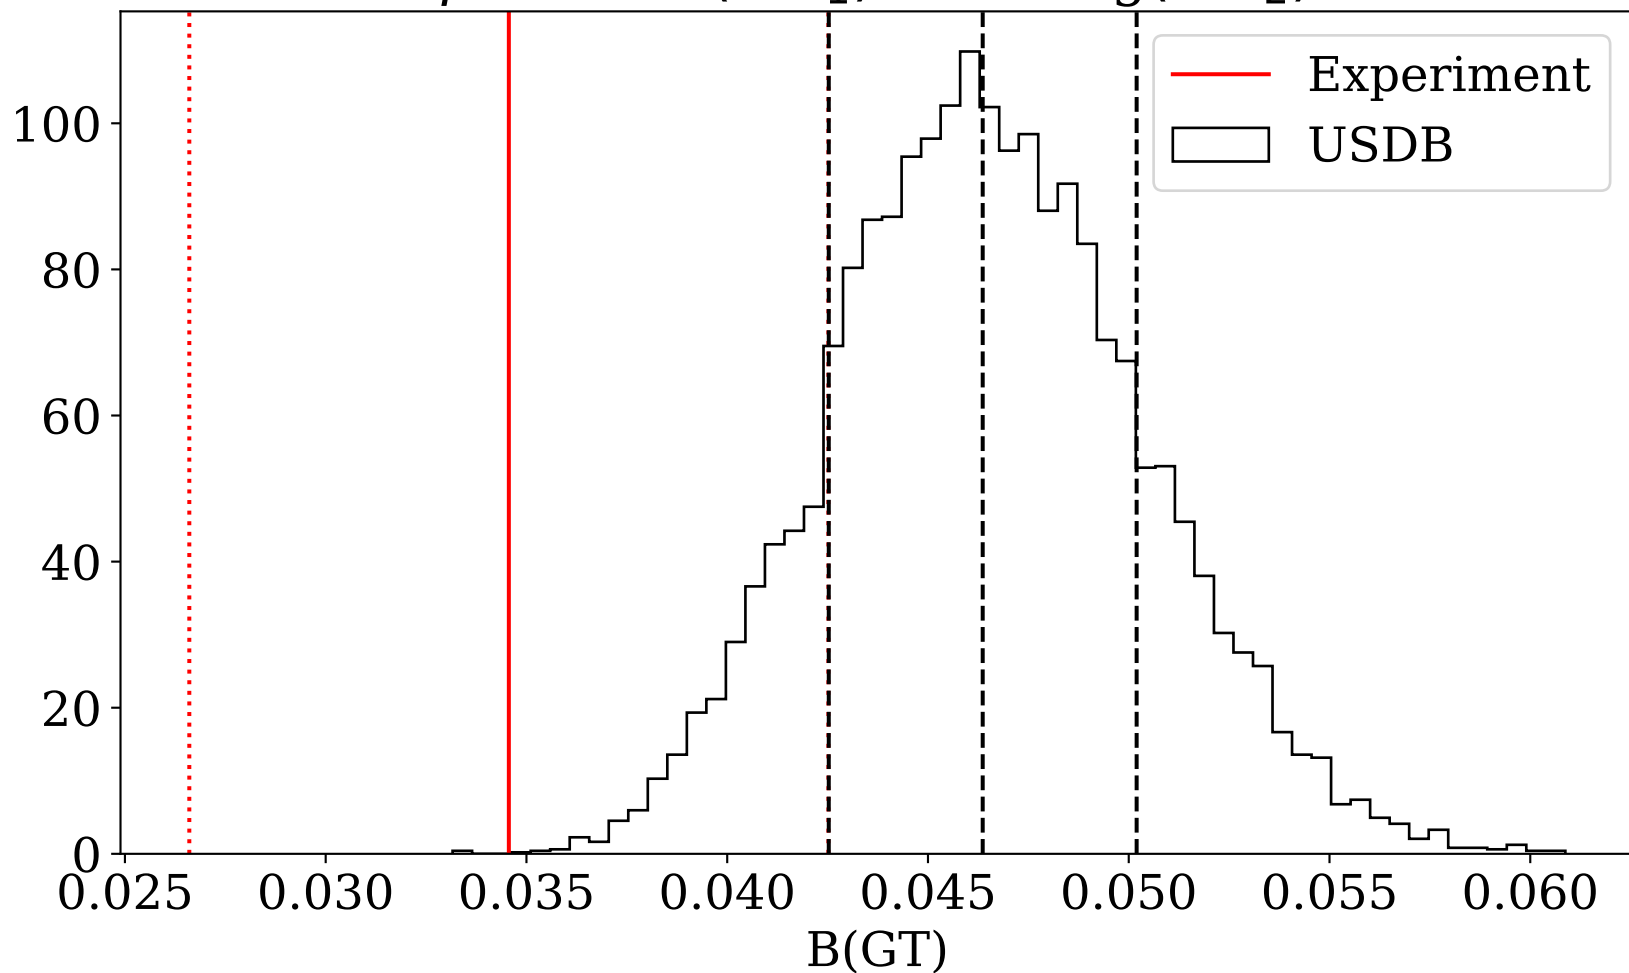

$\beta^- : {}^{26}\text{Na}(3_1) \rightarrow {}^{26}\text{Mg}(2_1)$

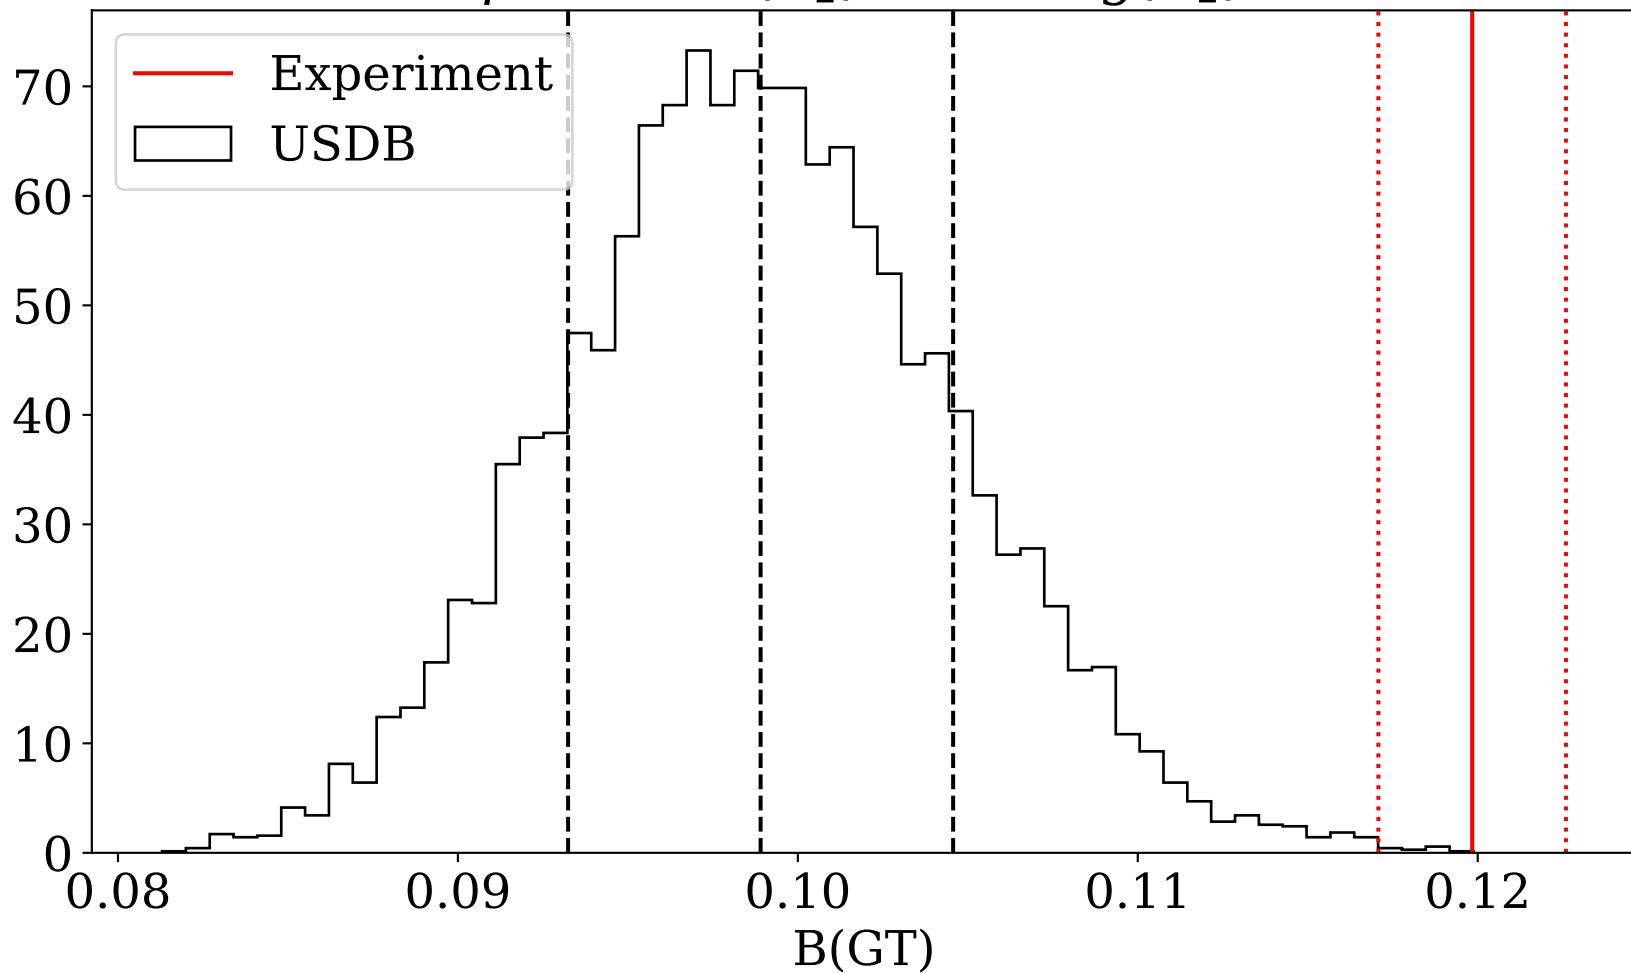

$\beta^- : {}^{26}\text{Na}(3_1) \rightarrow {}^{26}\text{Mg}(2_2)$

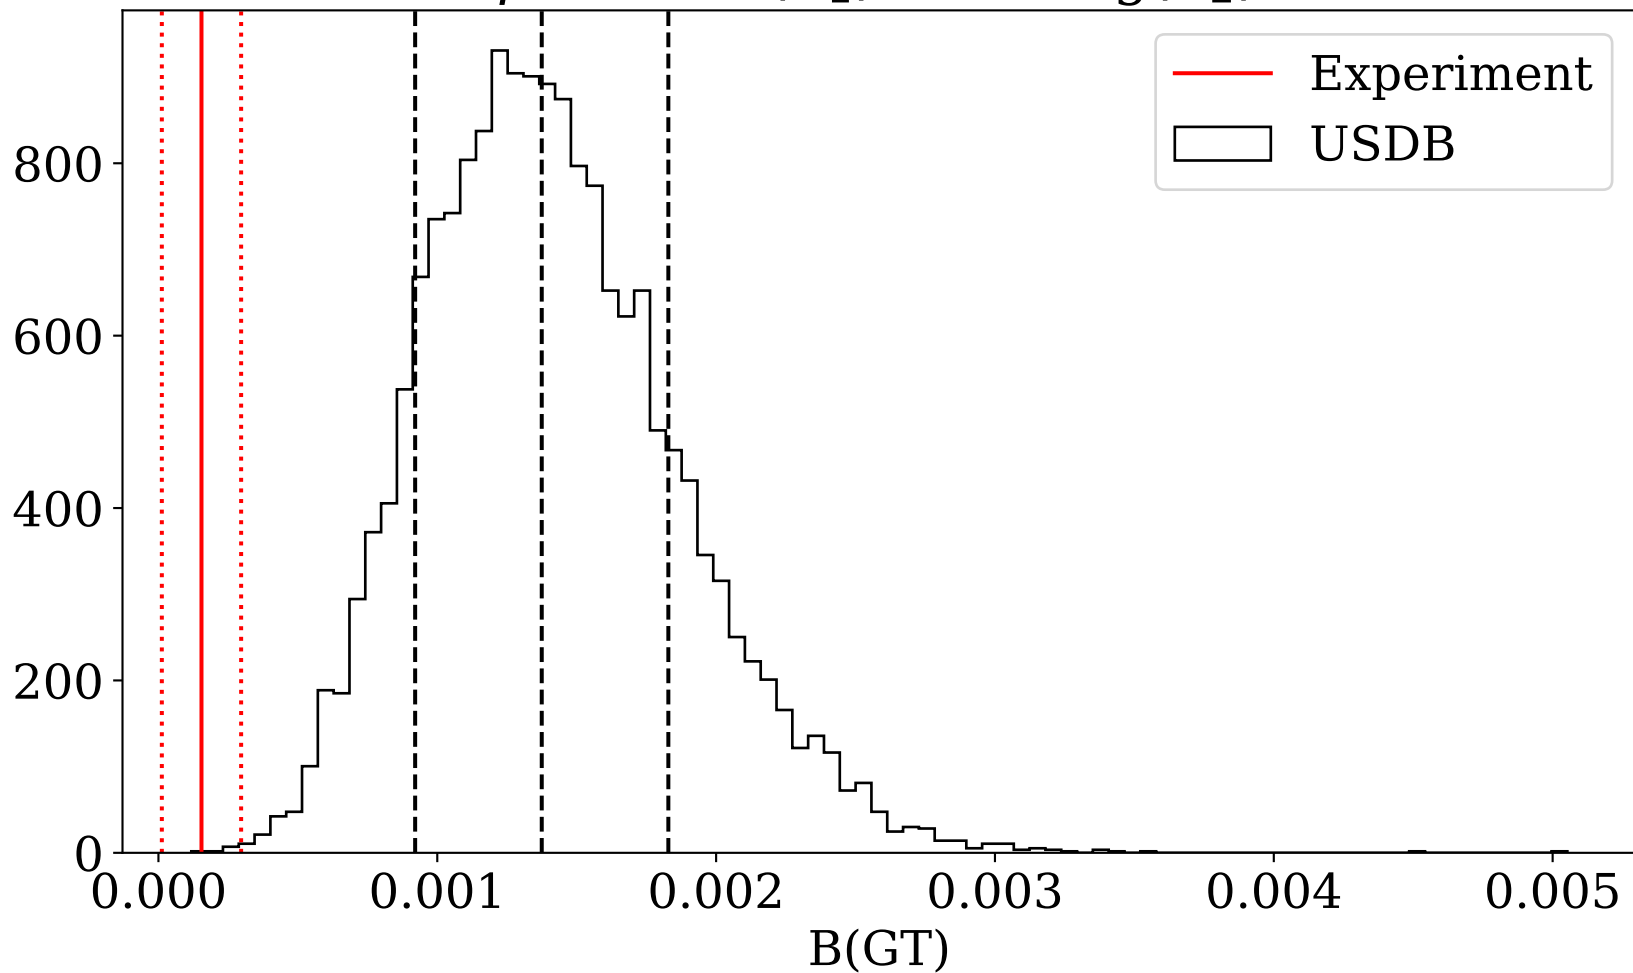

$\beta^- : {}^{26}\text{Na}(3_1) \rightarrow {}^{26}\text{Mg}(3_1)$

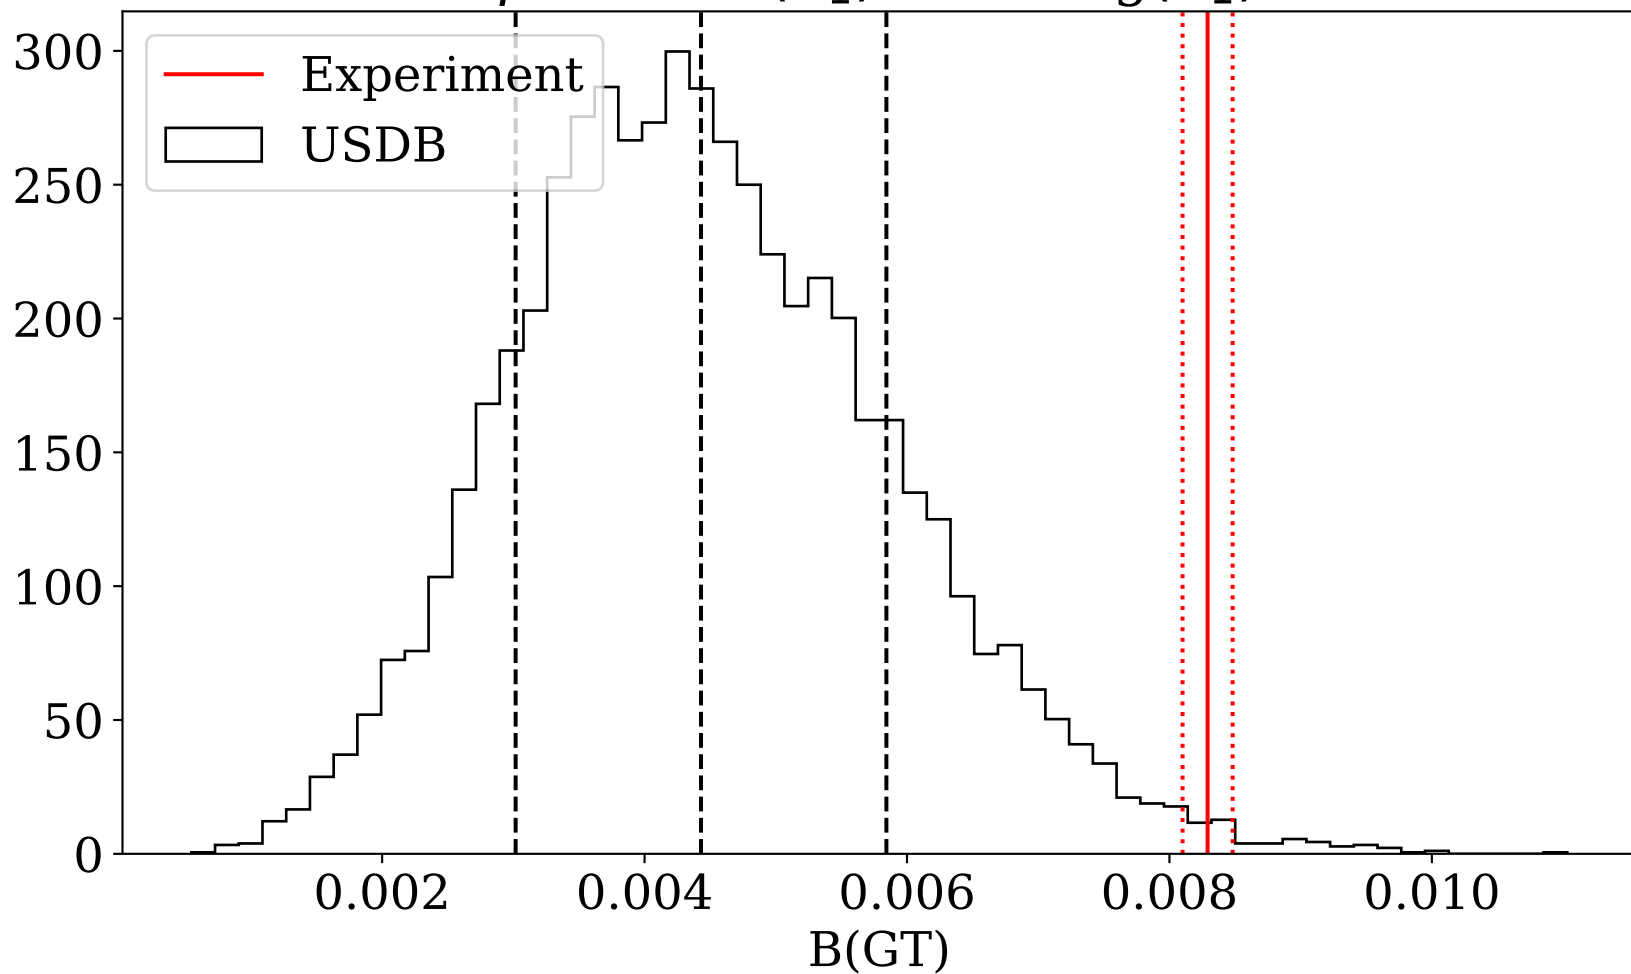

$\beta^- : {}^{26}\text{Na}(3_1) \rightarrow {}^{26}\text{Mg}(4_1)$

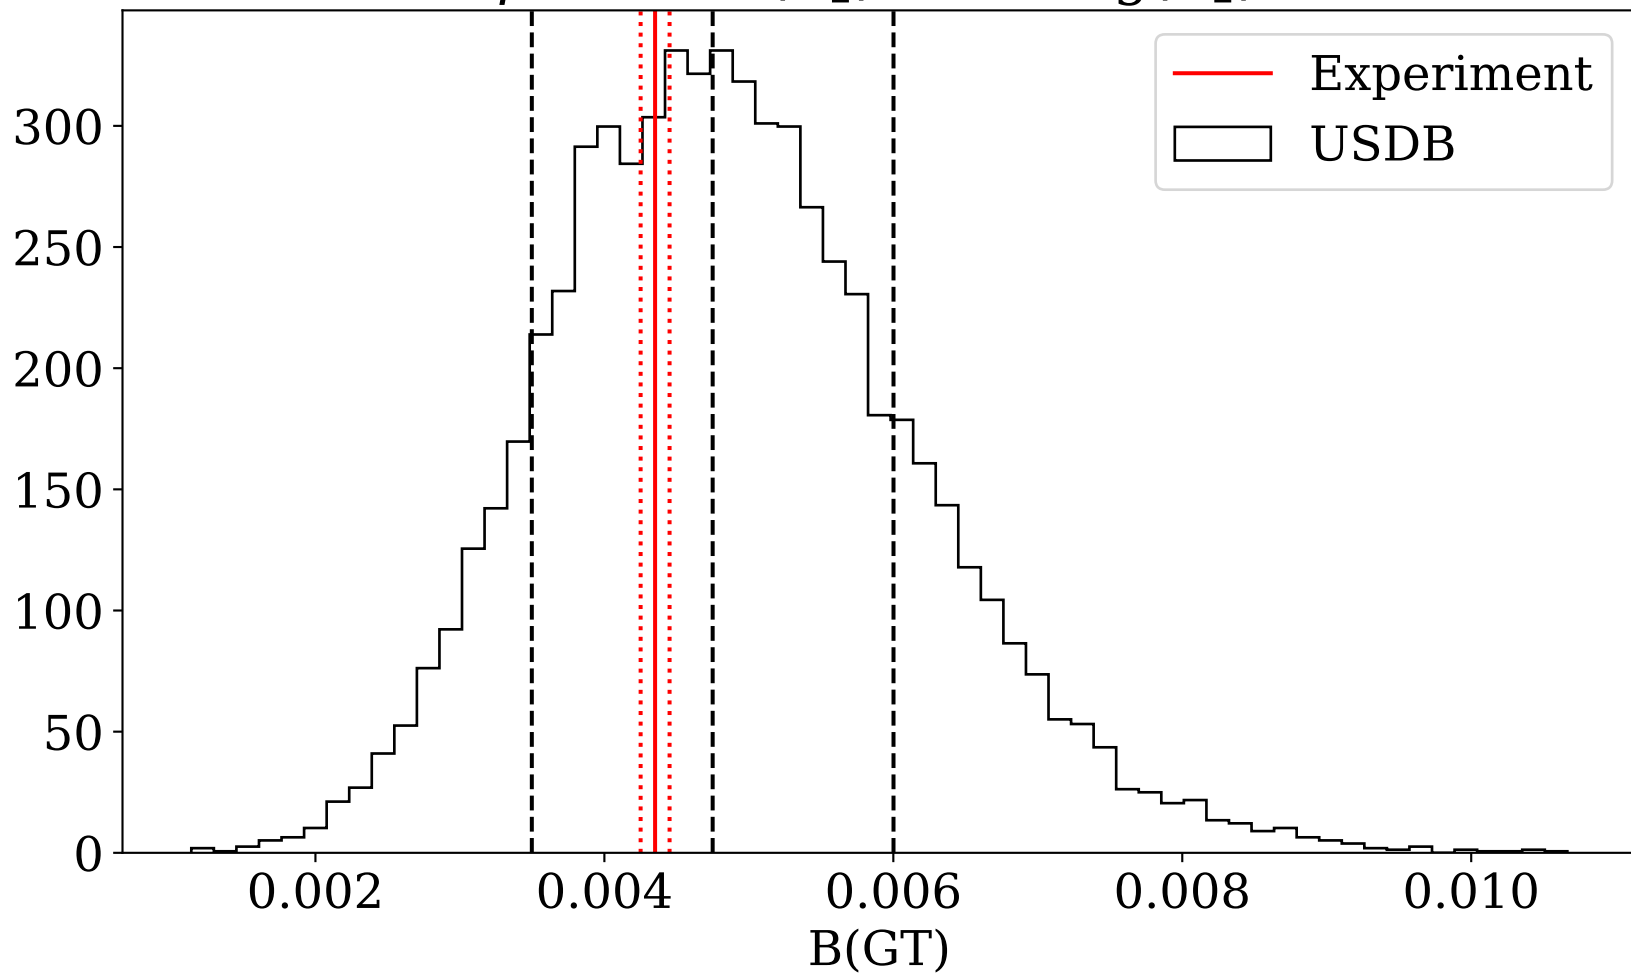

$\beta^- : {}^{26}\text{Na}(3_1) \rightarrow {}^{26}\text{Mg}(2_3)$

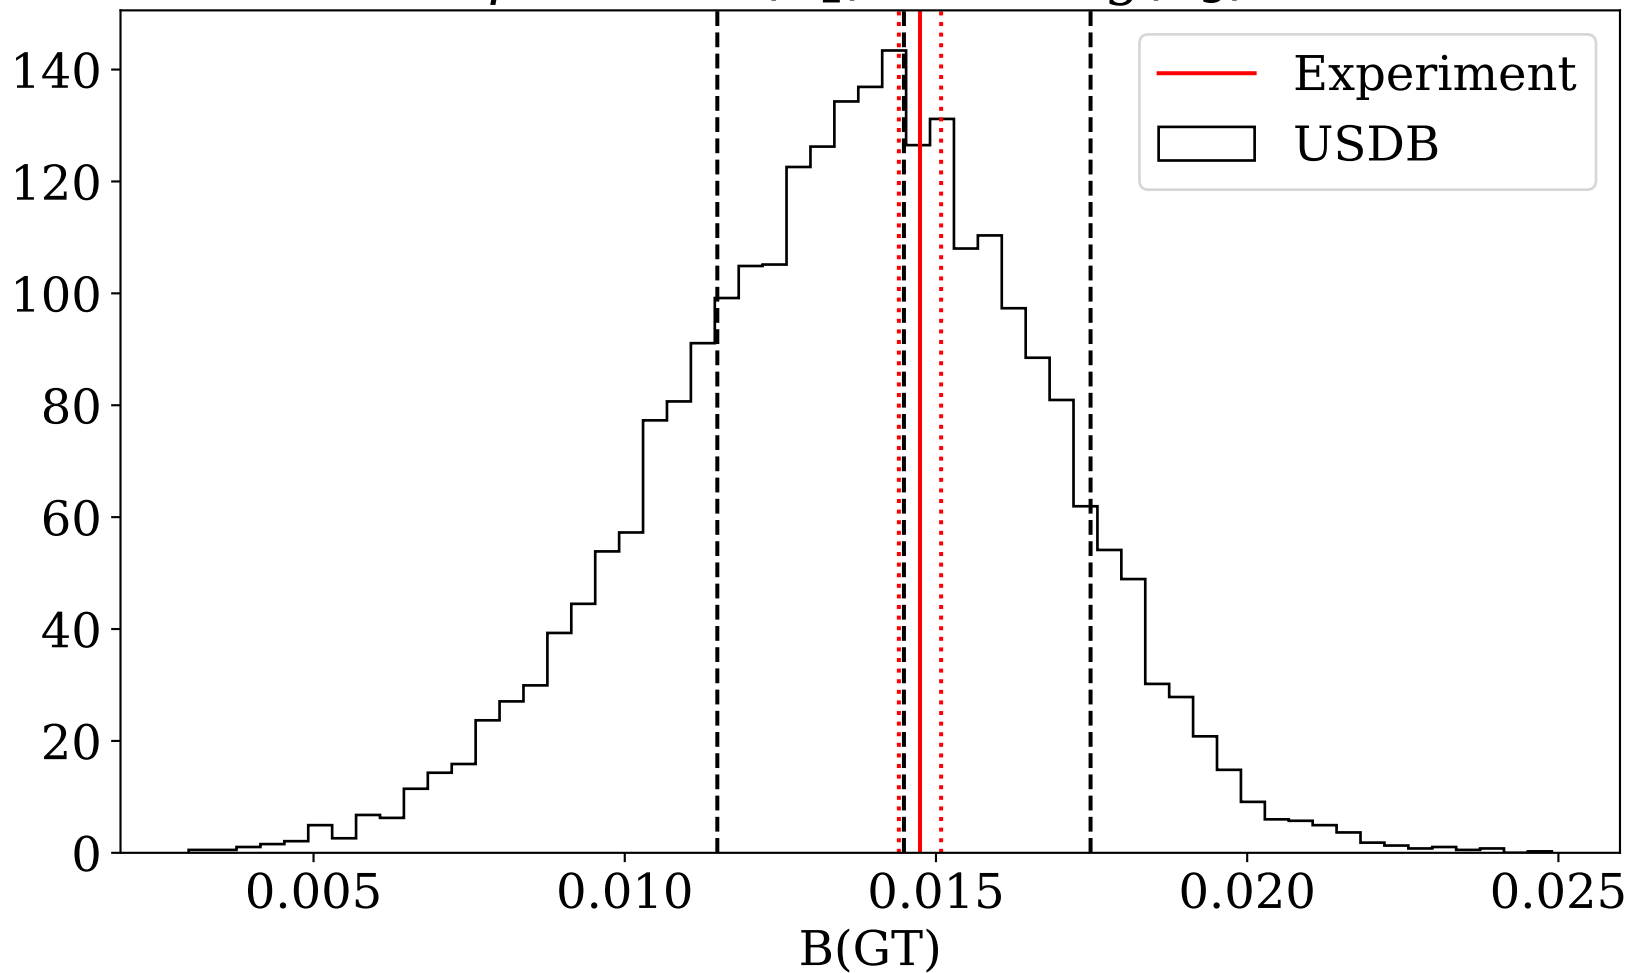



$\beta^- : {}^{26}\text{Na}(3_1) \rightarrow {}^{26}\text{Mg}(3_2)$

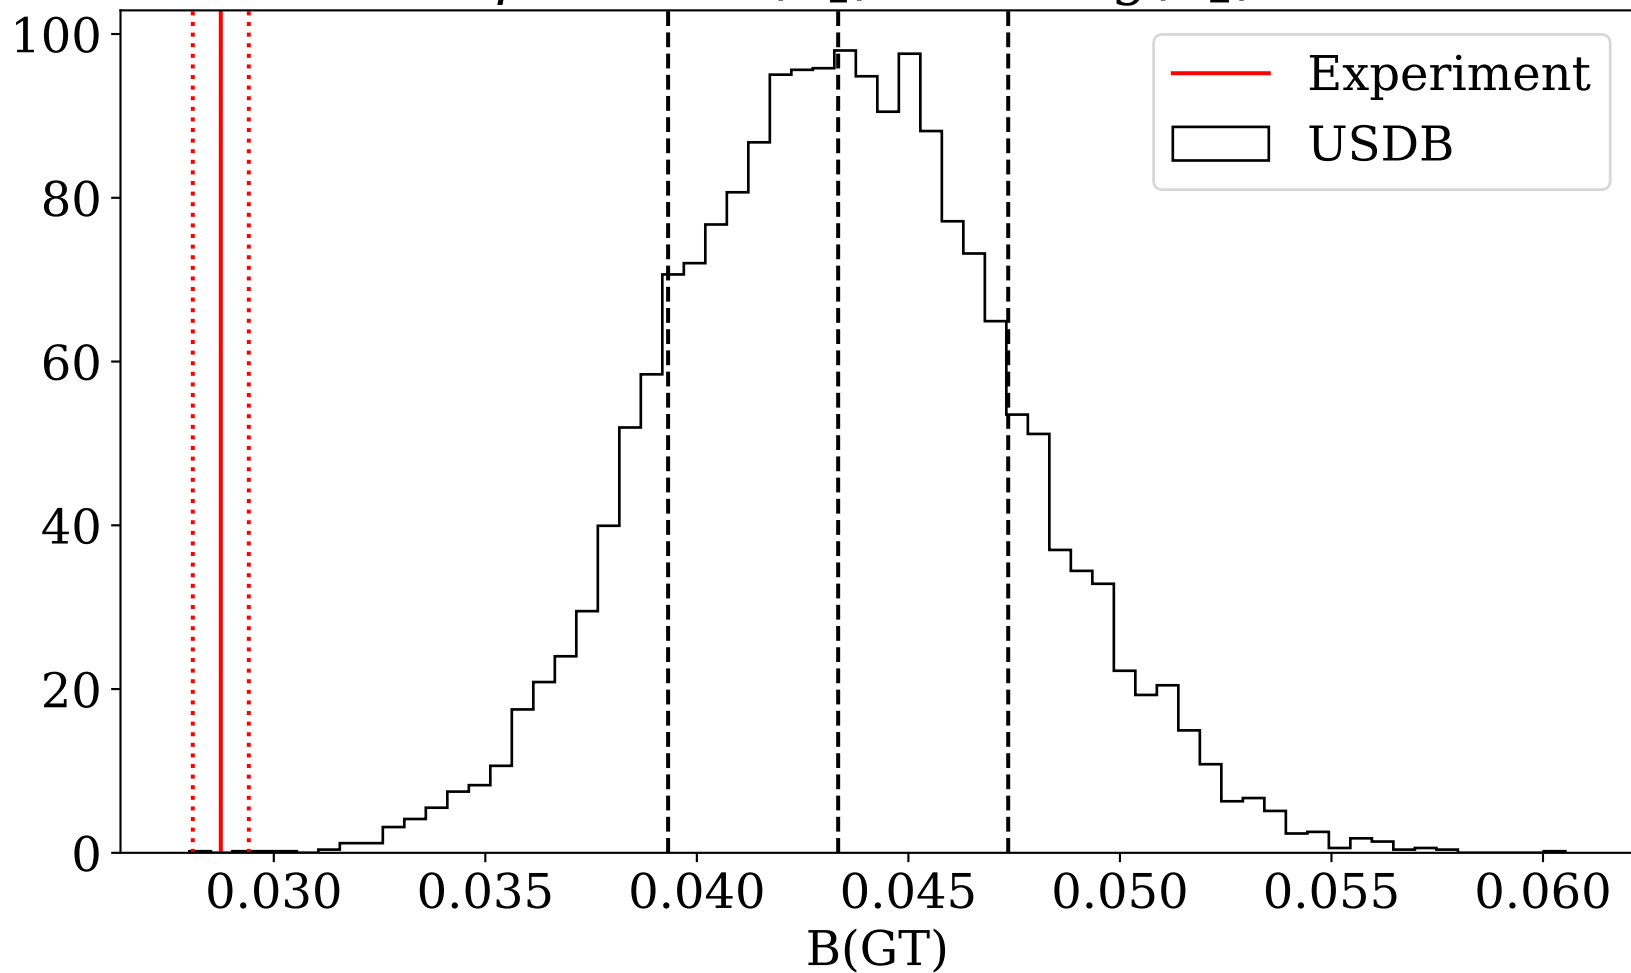

$\beta^- : {}^{26}\text{Na}(3_1) \rightarrow {}^{26}\text{Mg}(2_4)$

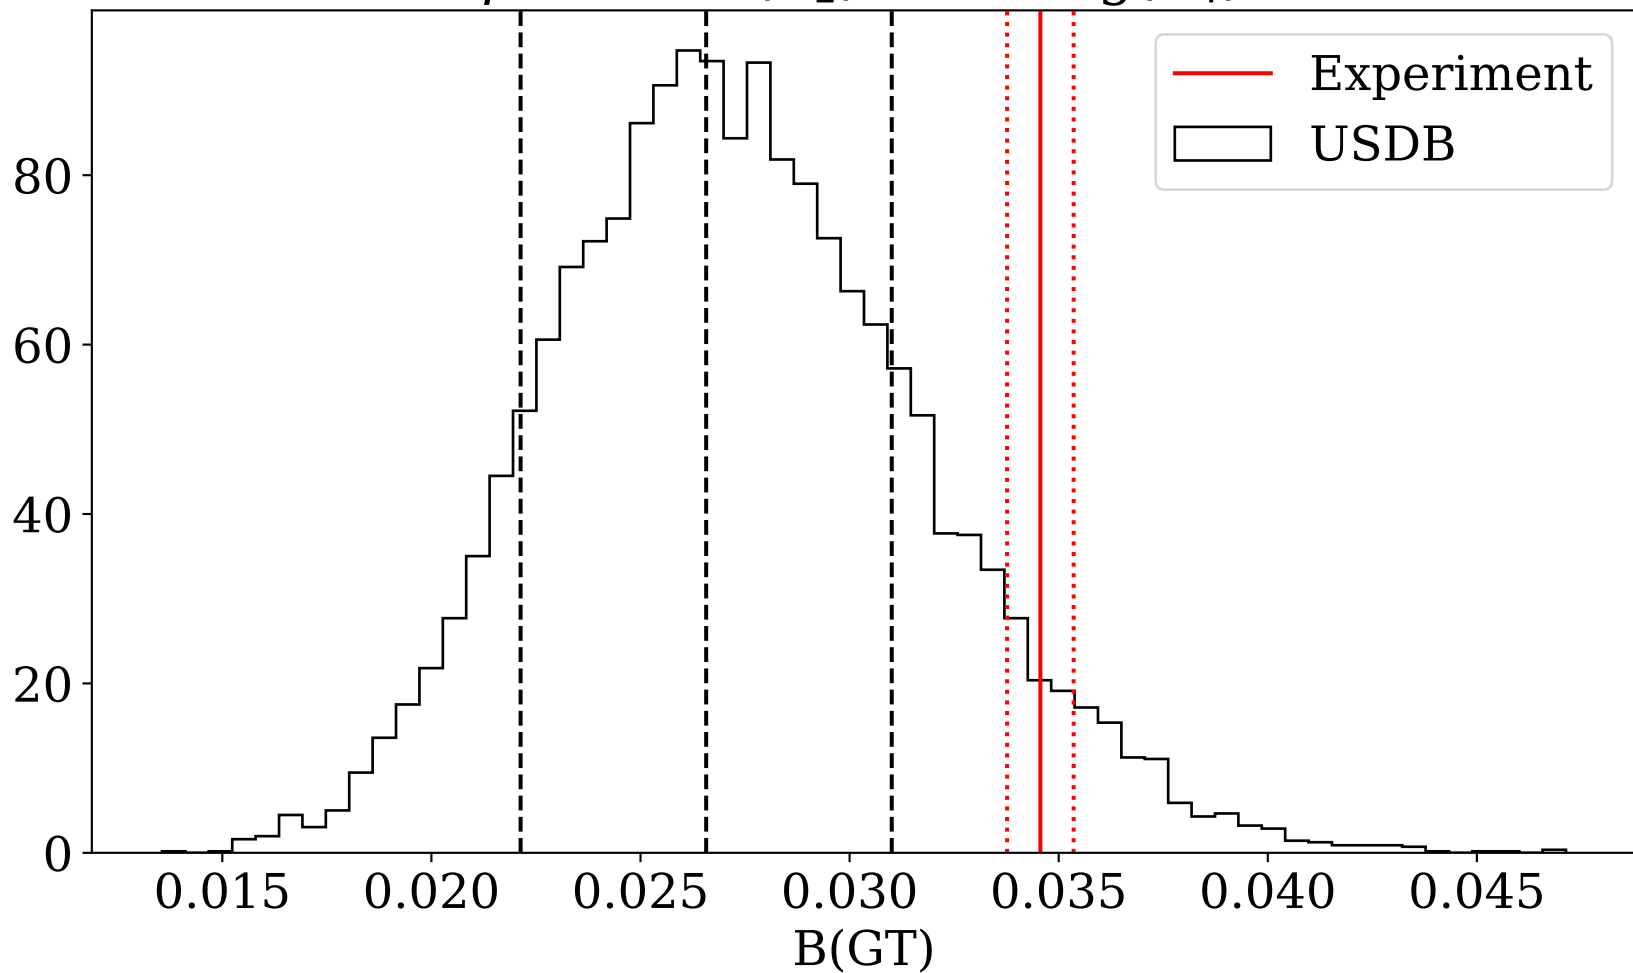

$\beta^- : {}^{26}\text{Na}(3_1) \rightarrow {}^{26}\text{Mg}(4_2)$

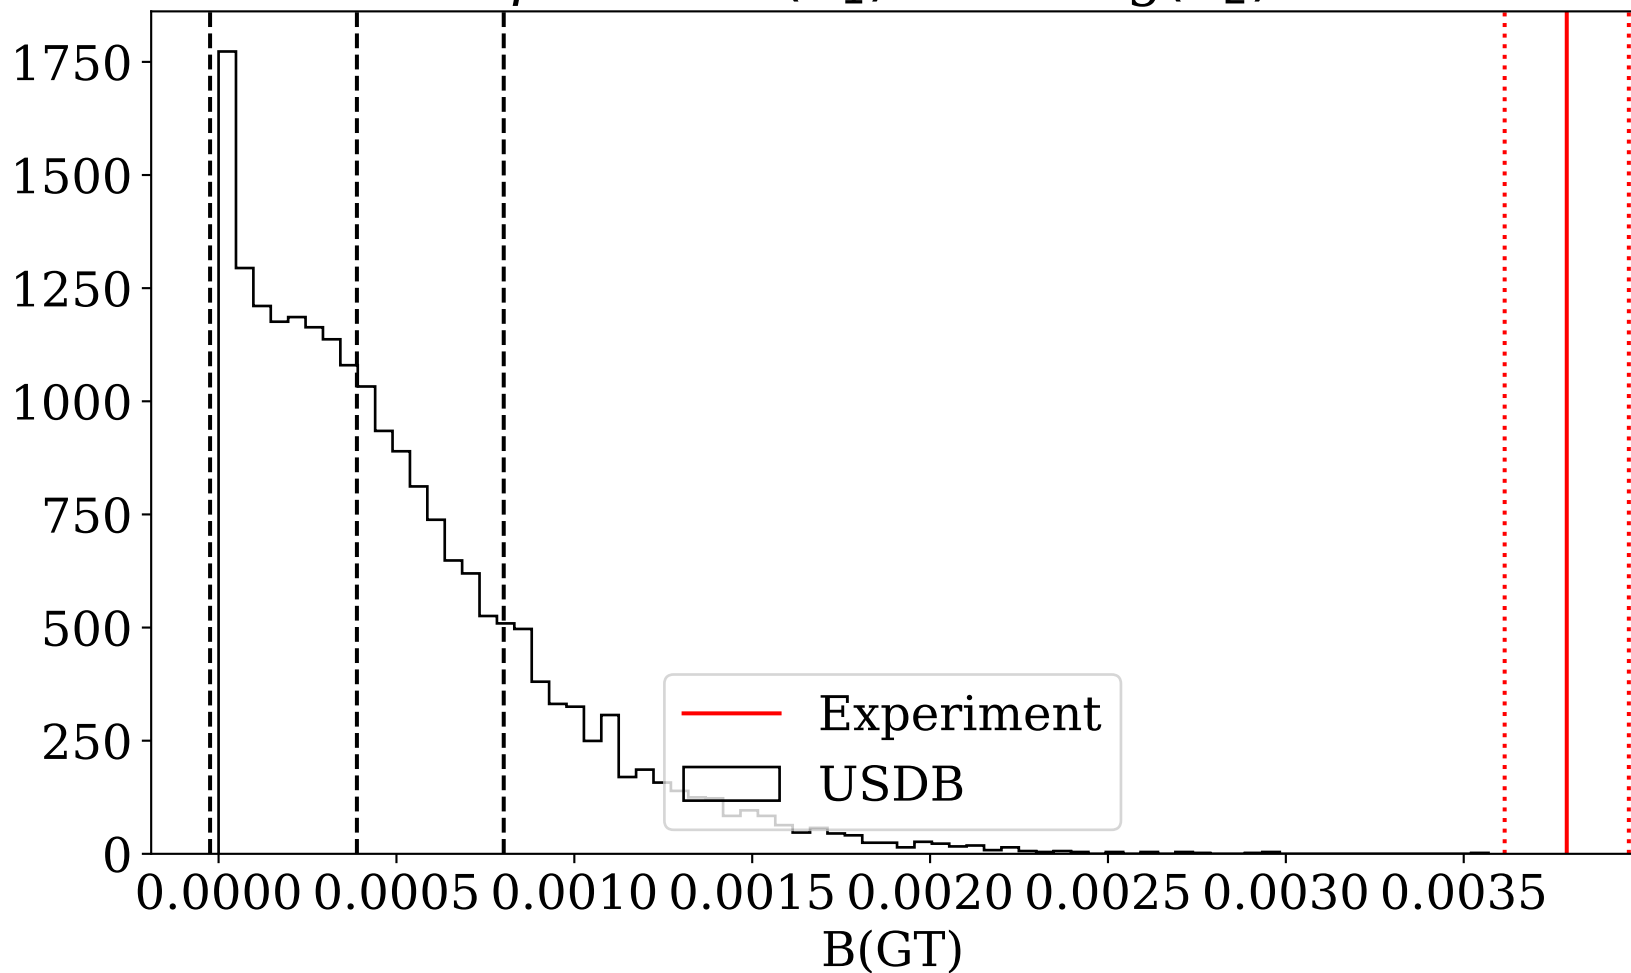

$\beta^- : {}^{26}\text{Na}(3_1) \rightarrow {}^{26}\text{Mg}(2_5)$

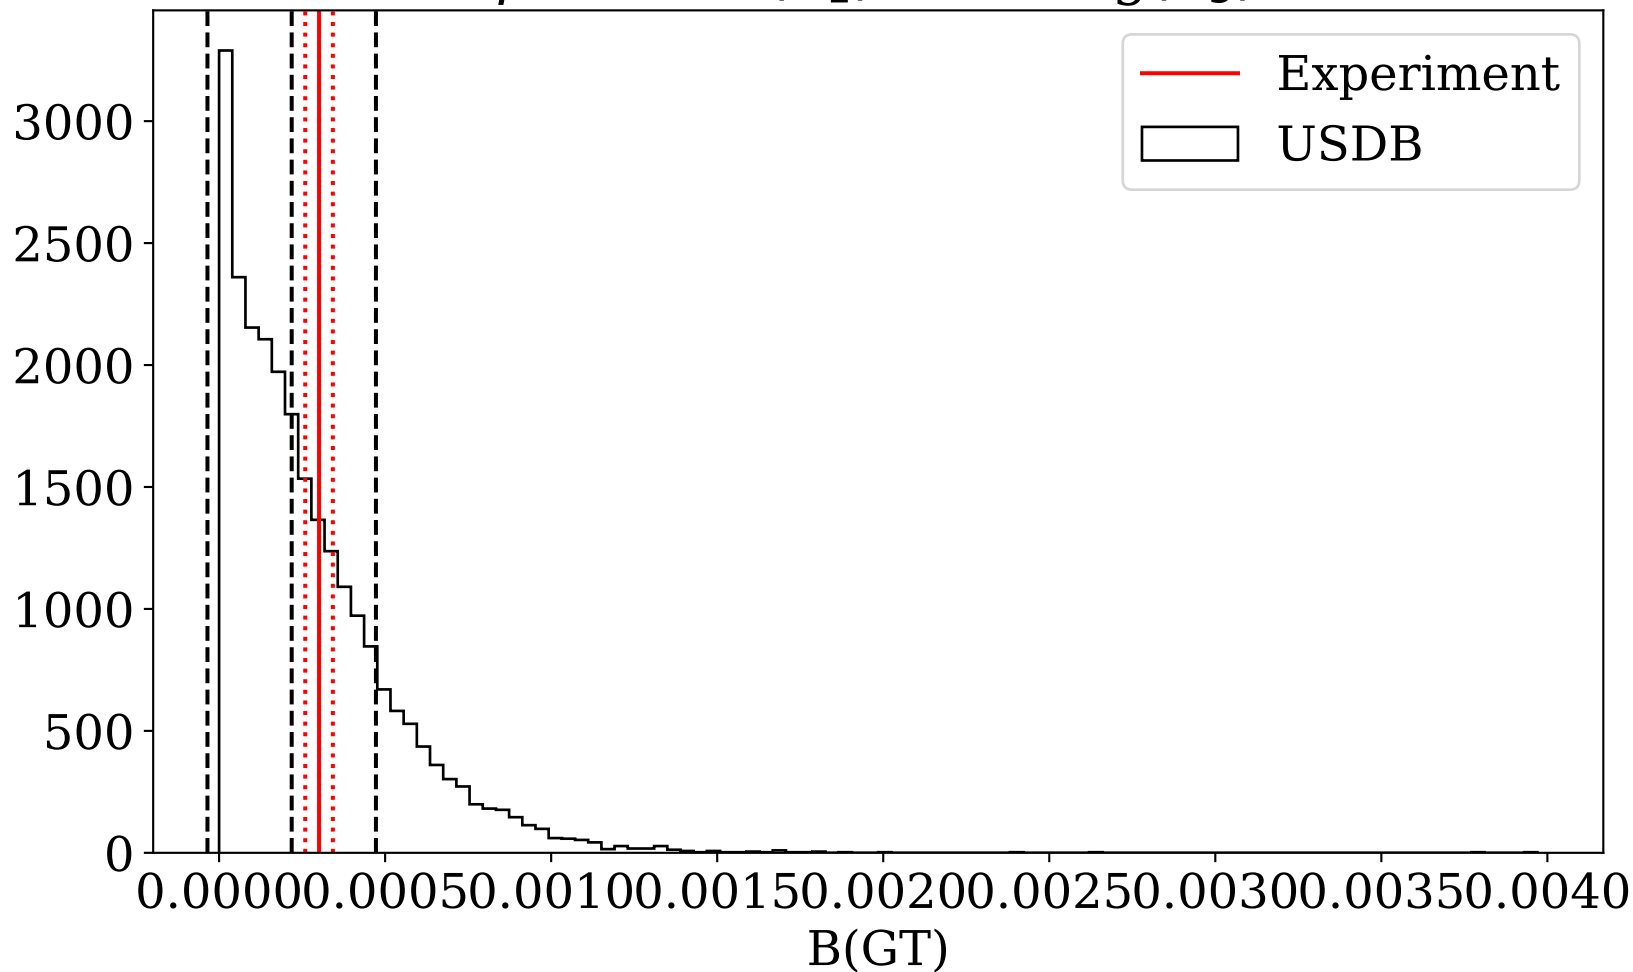

$\beta^- : {}^{27}\text{Na}(5/2_1) \rightarrow {}^{27}\text{Mg}(3/2_1)$

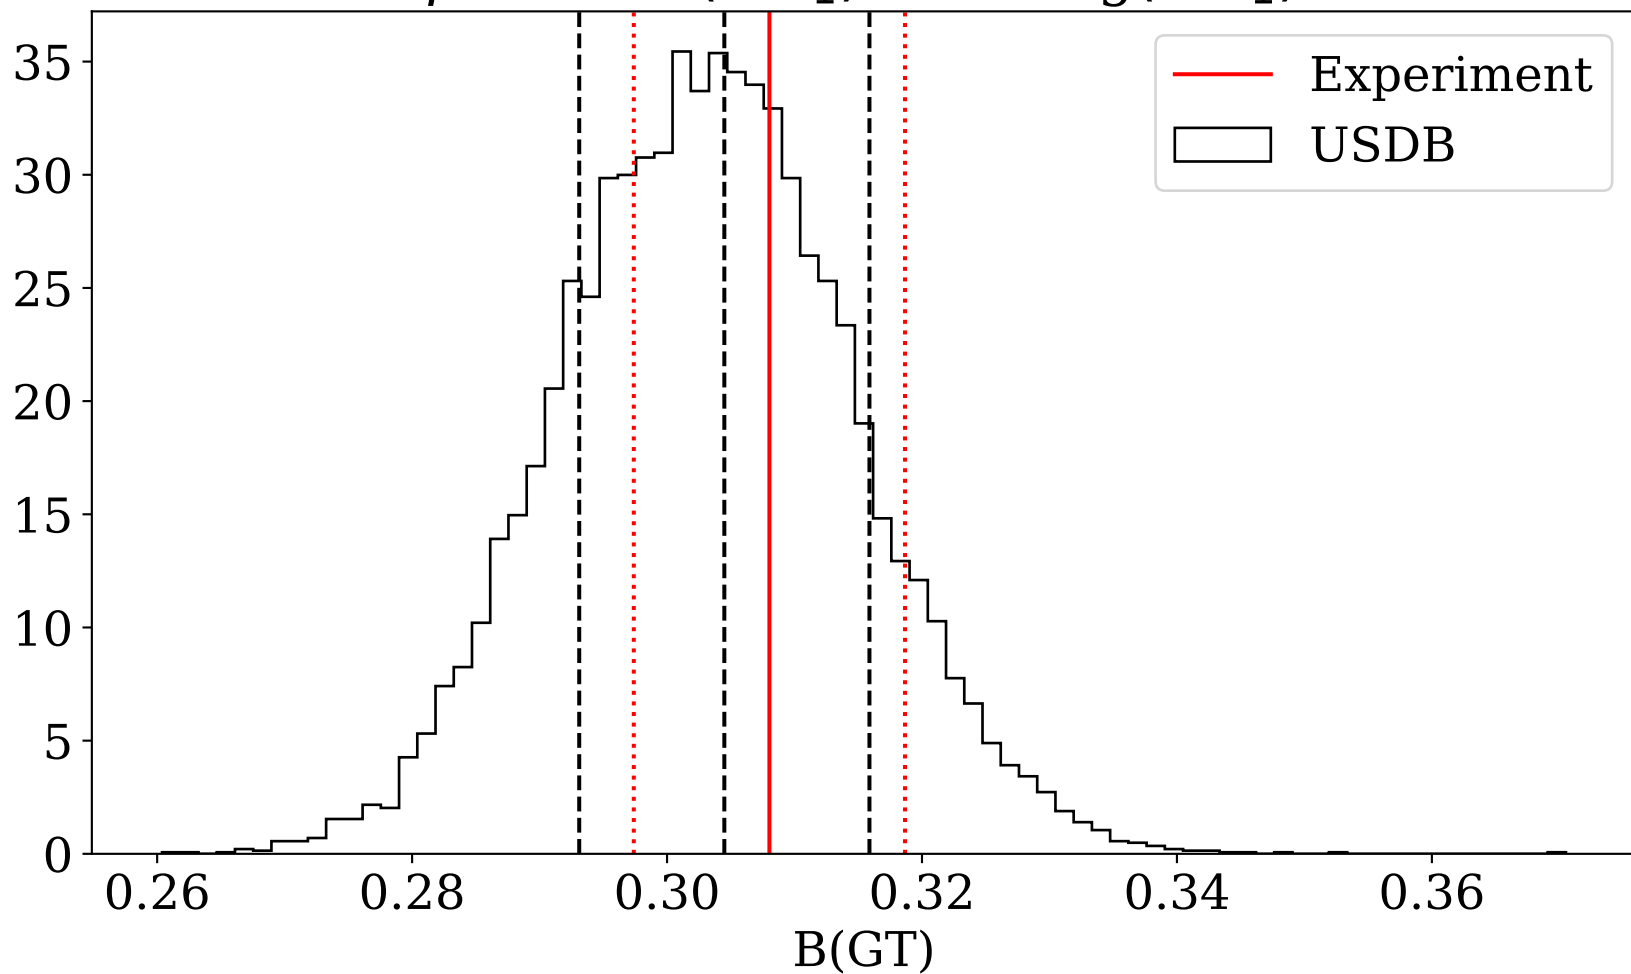

$\beta^- : {}^{27}\text{Na}(5/2_1) \rightarrow {}^{27}\text{Mg}(5/2_1)$

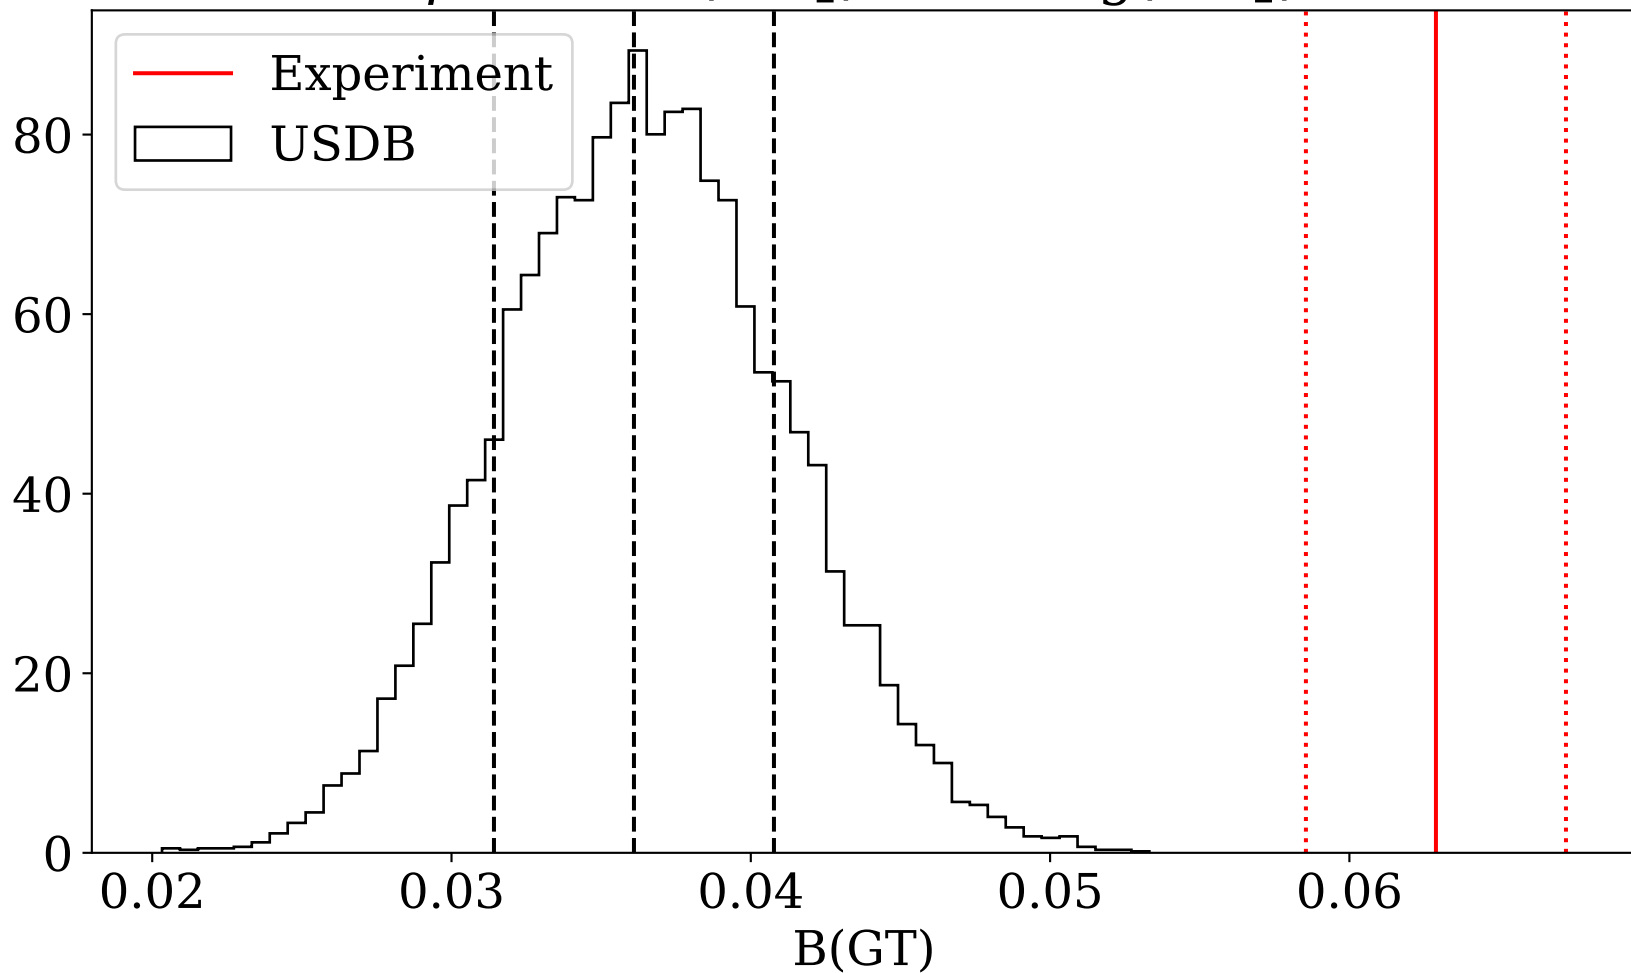

$\beta^- : {}^{27}\text{Na}(5/2_1) \rightarrow {}^{27}\text{Mg}(5/2_2)$

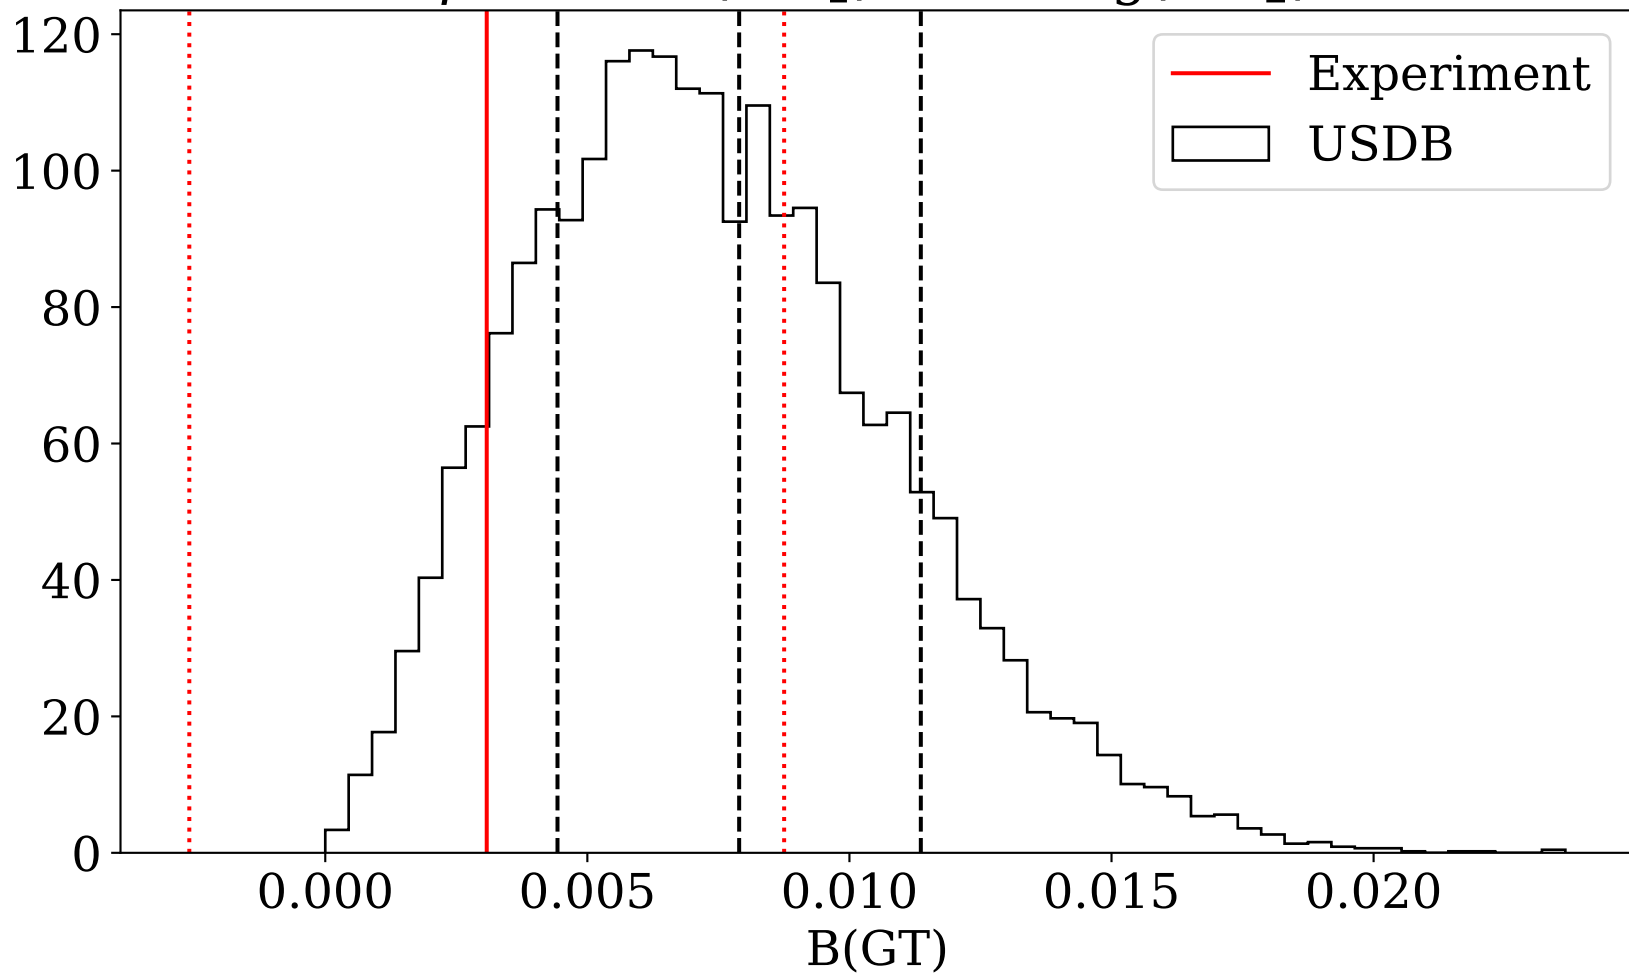

$\beta^- : {}^{28}\text{Na}(1_1) \rightarrow {}^{28}\text{Mg}(0_1)$

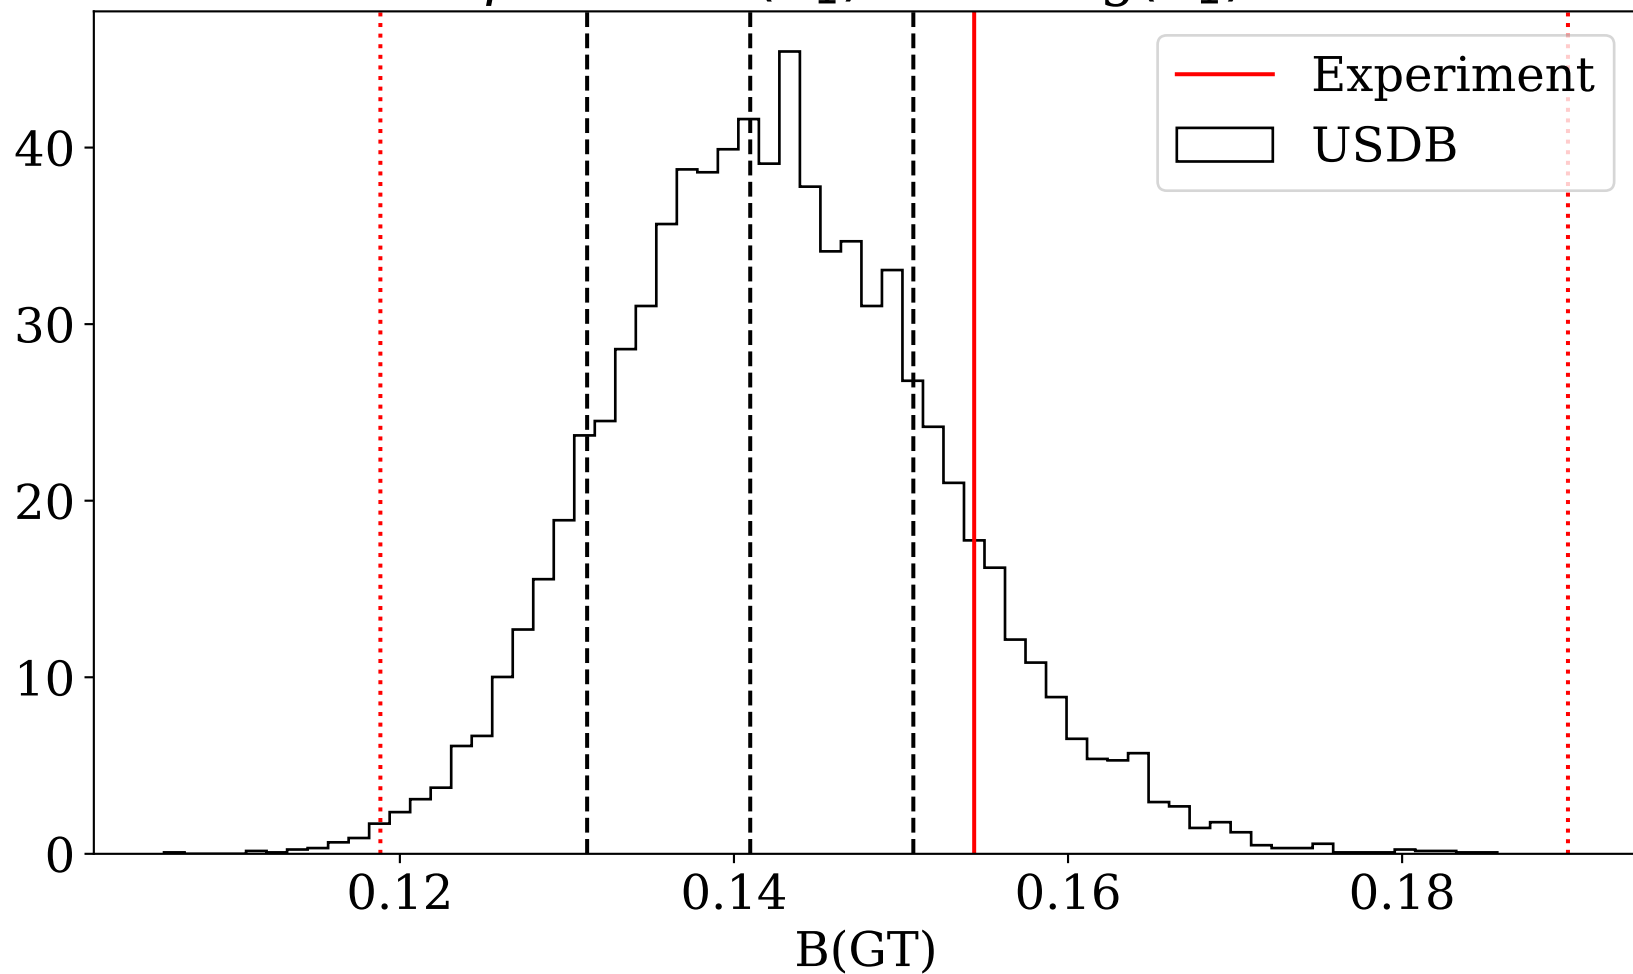



$\beta^- : {}^{28}\text{Na}(1_1) \rightarrow {}^{28}\text{Mg}(2_1)$

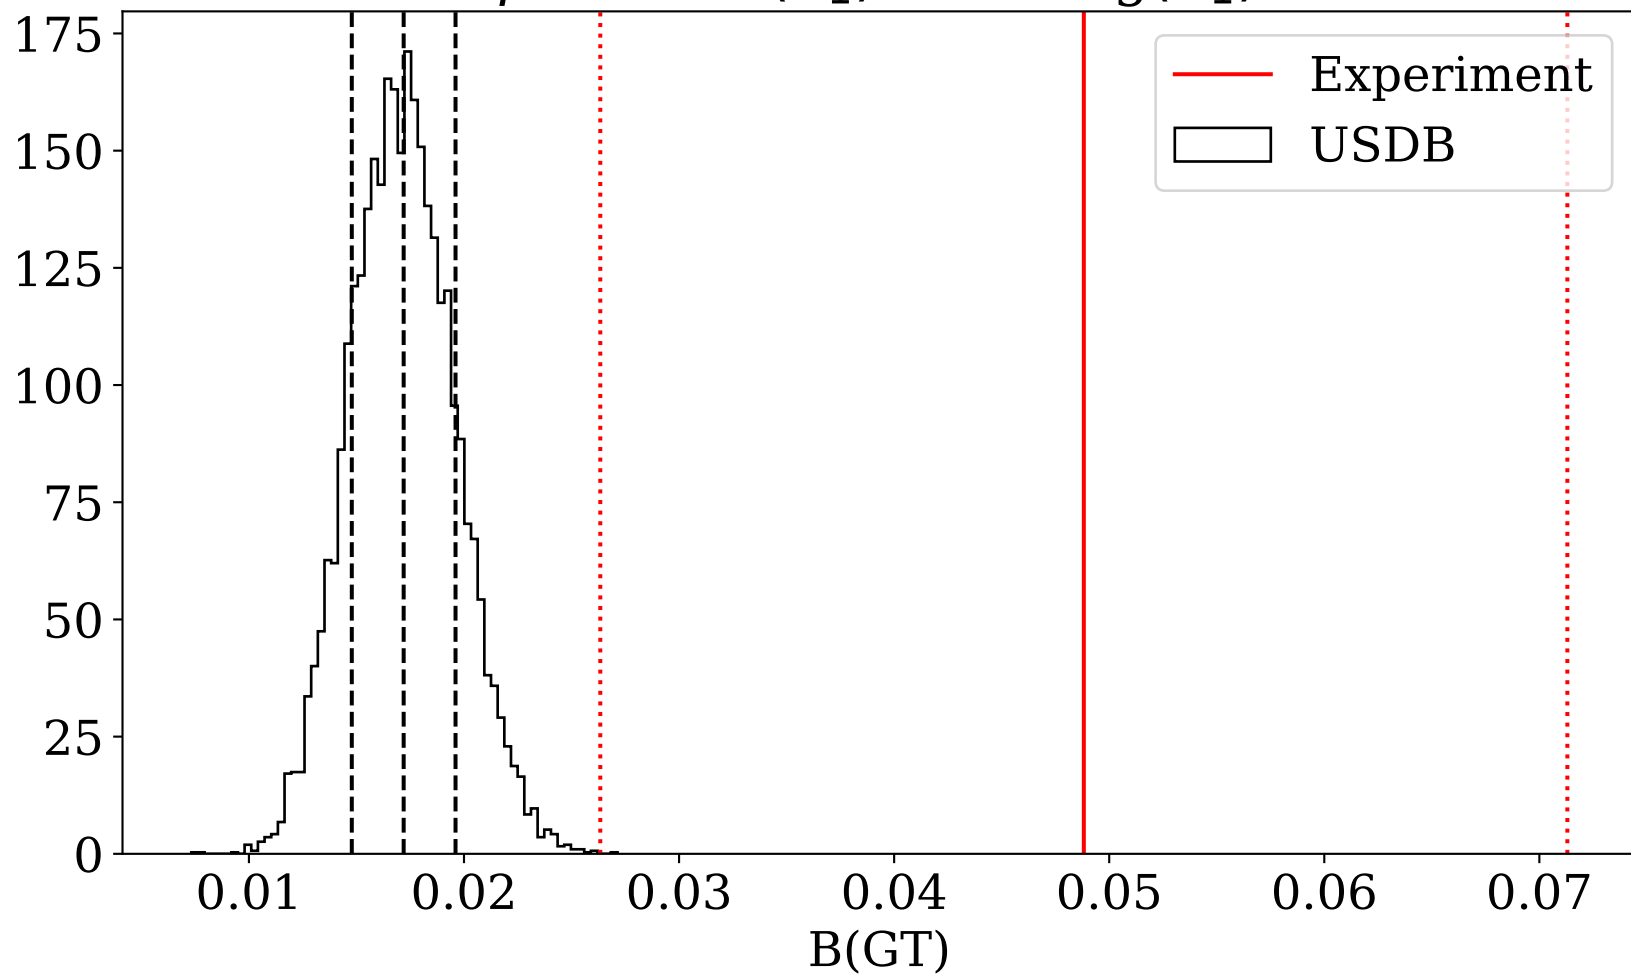

$\beta^- : {}^{28}\text{Na}(1_1) \rightarrow {}^{28}\text{Mg}(0_2)$

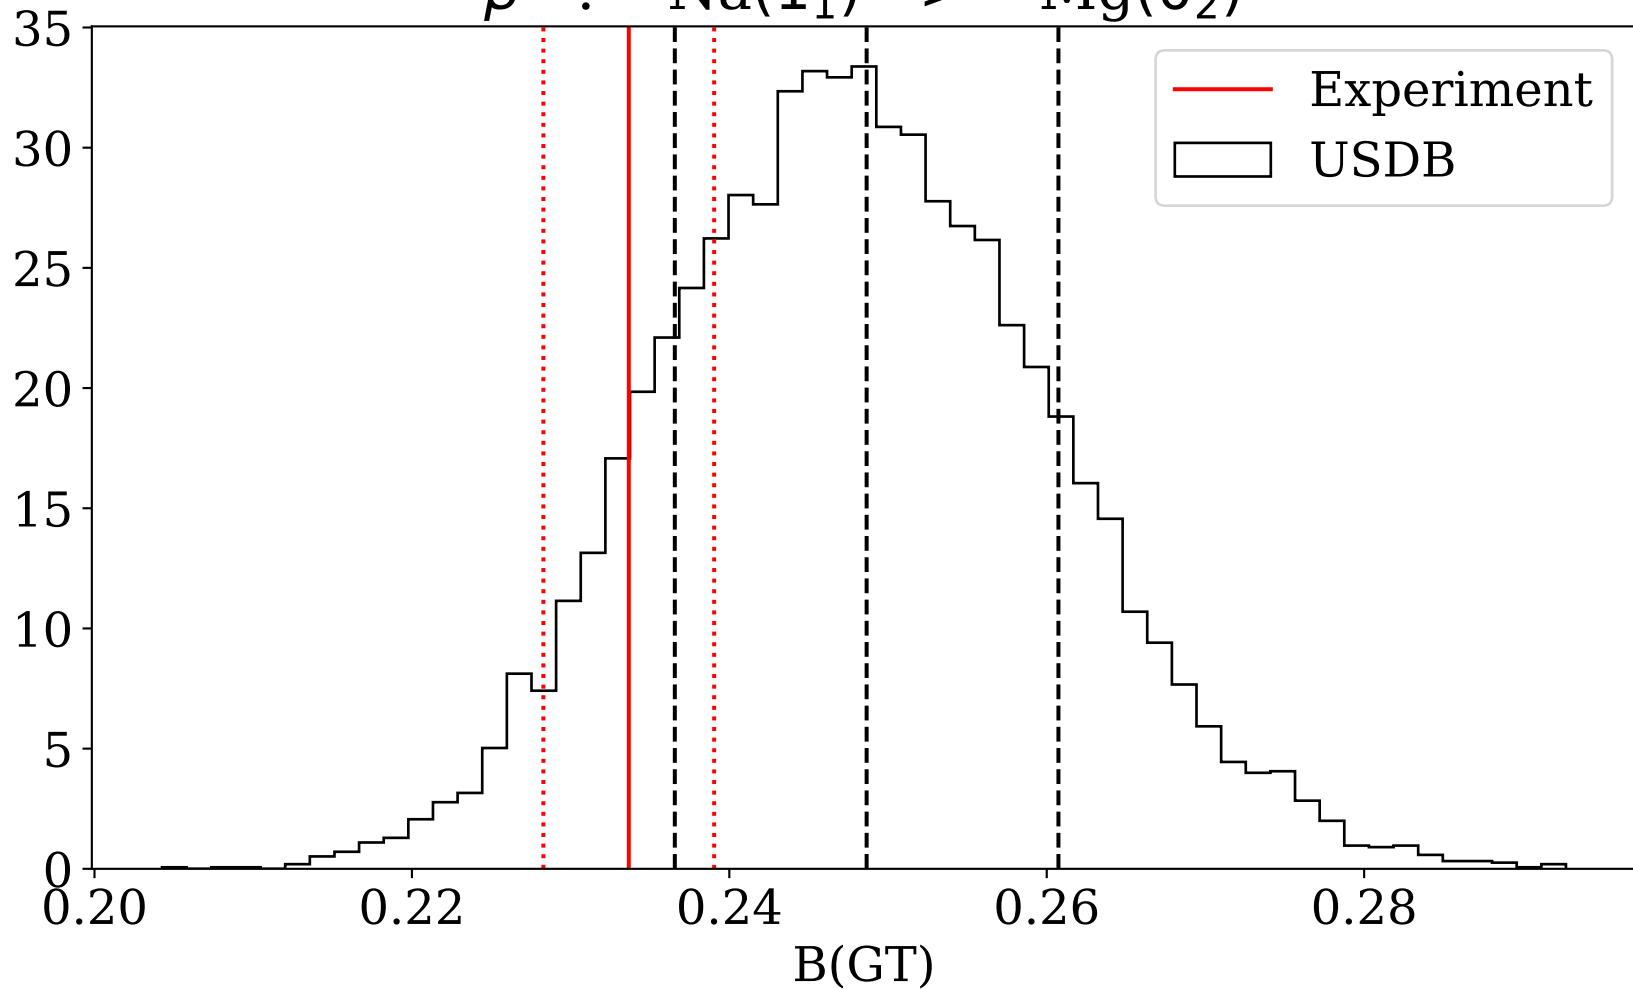

$\beta^- : {}^{28}\text{Na}(1_1) \dashrightarrow {}^{28}\text{Mg}(2_2)$

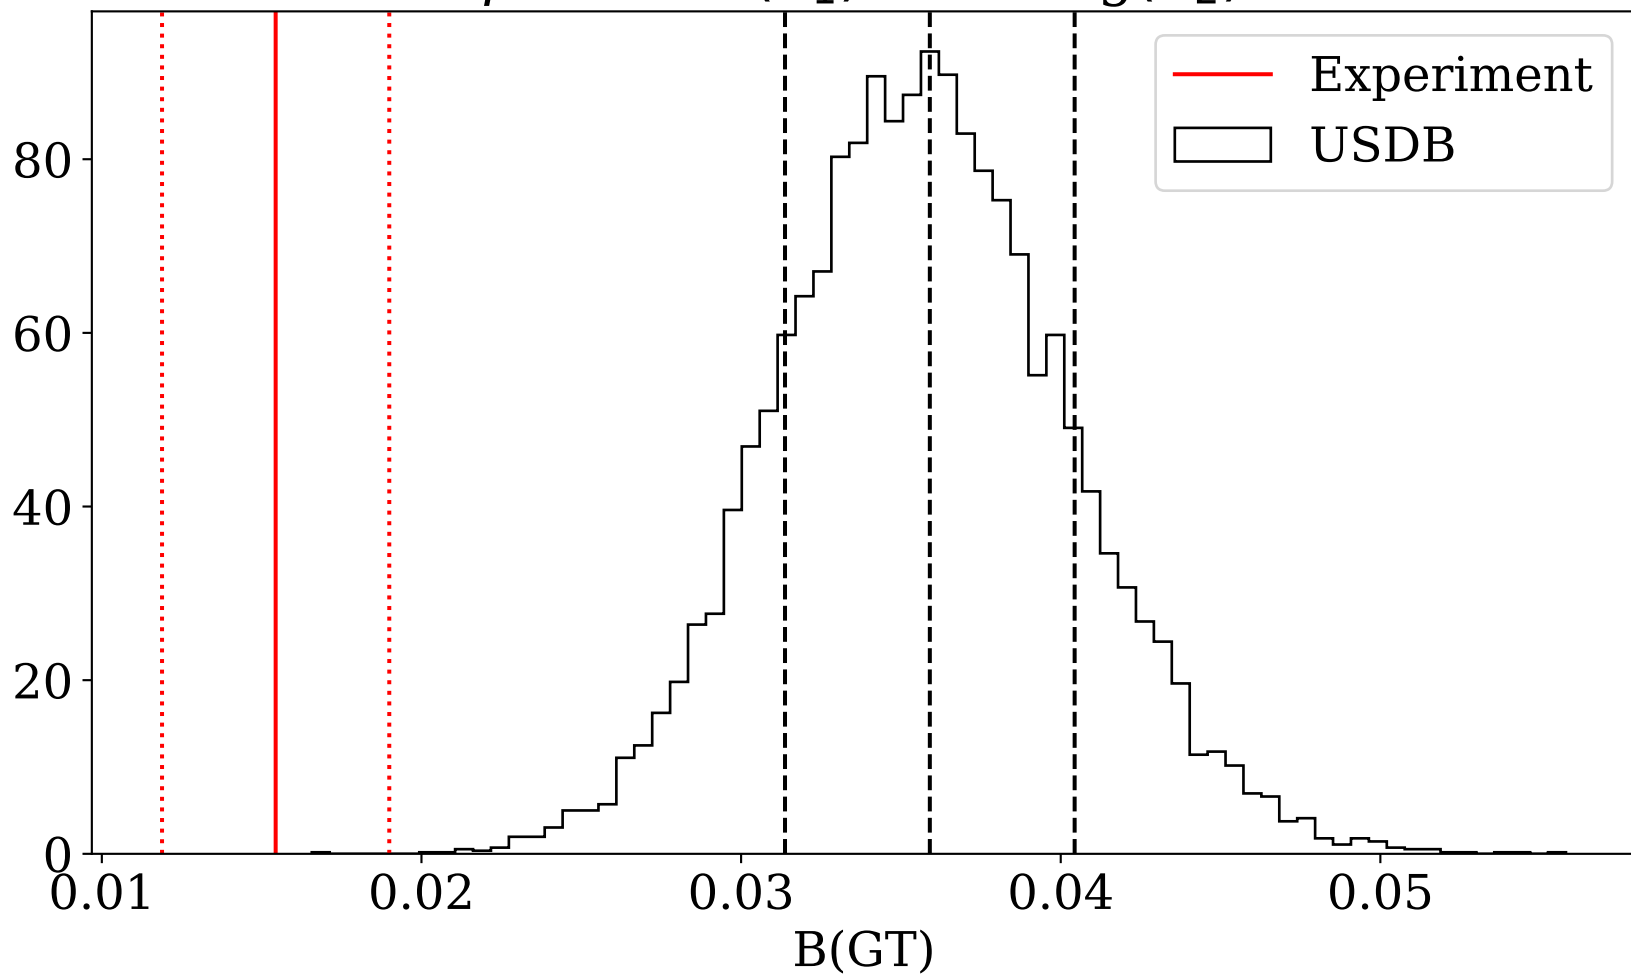

$\beta^- : {}^{29}\text{Na}(3/2_1) \rightarrow {}^{29}\text{Mg}(3/2_1)$

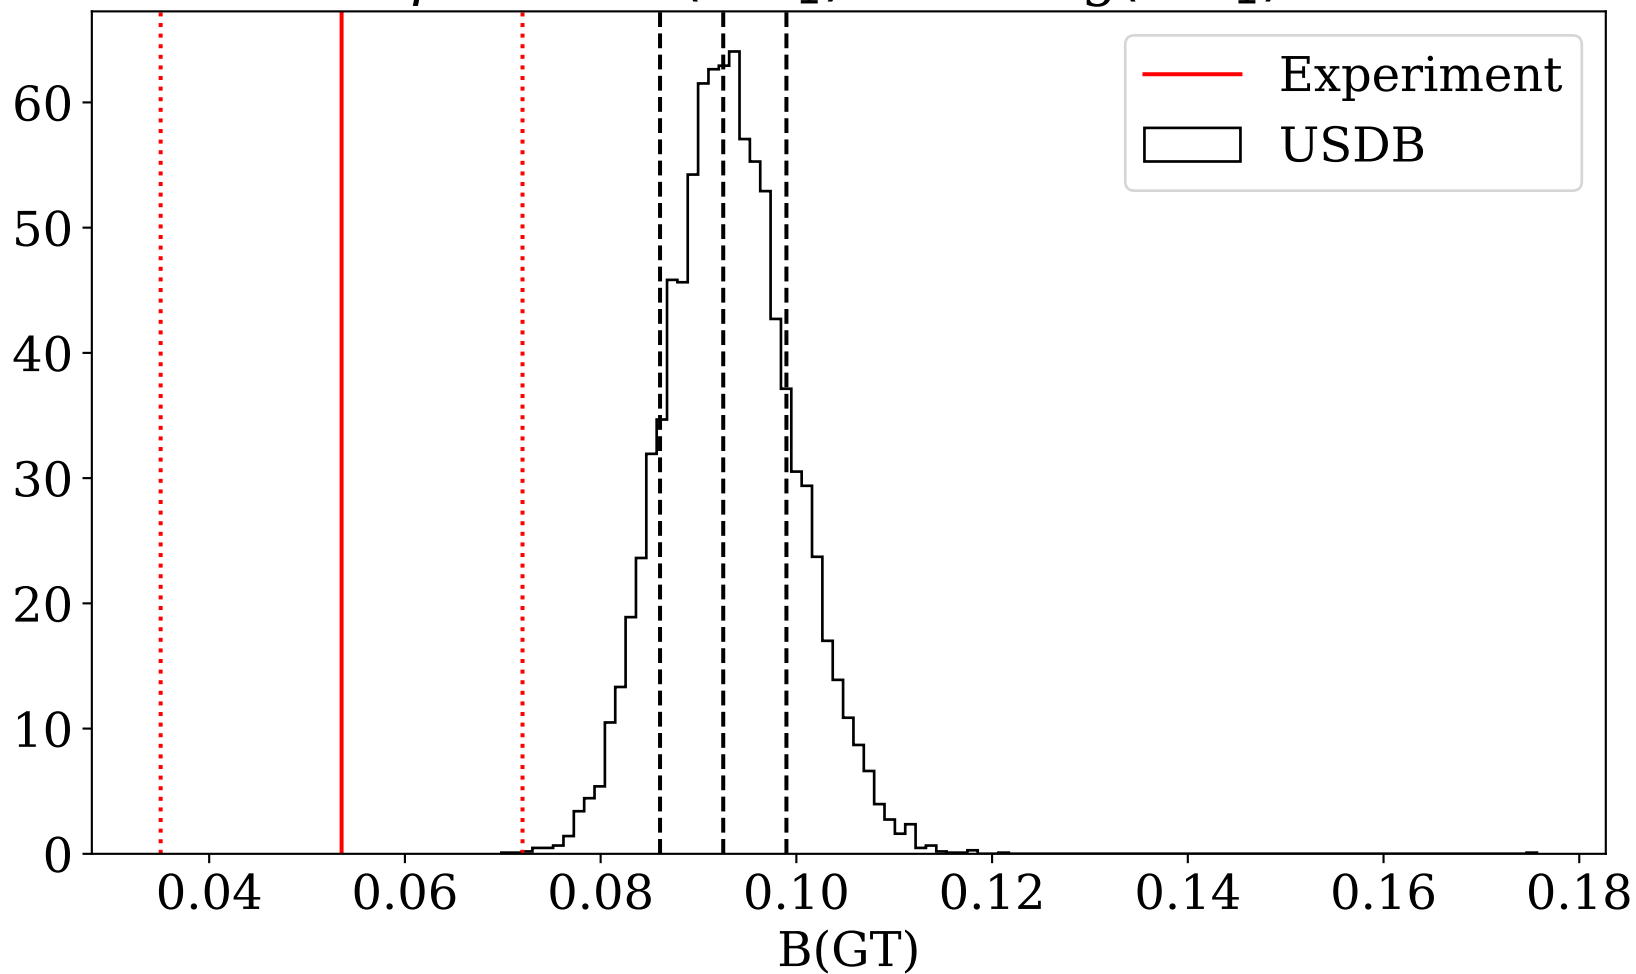

$\beta^- : {}^{27}\text{Mg}(1/2_1) \rightarrow {}^{27}\text{Al}(1/2_1)$

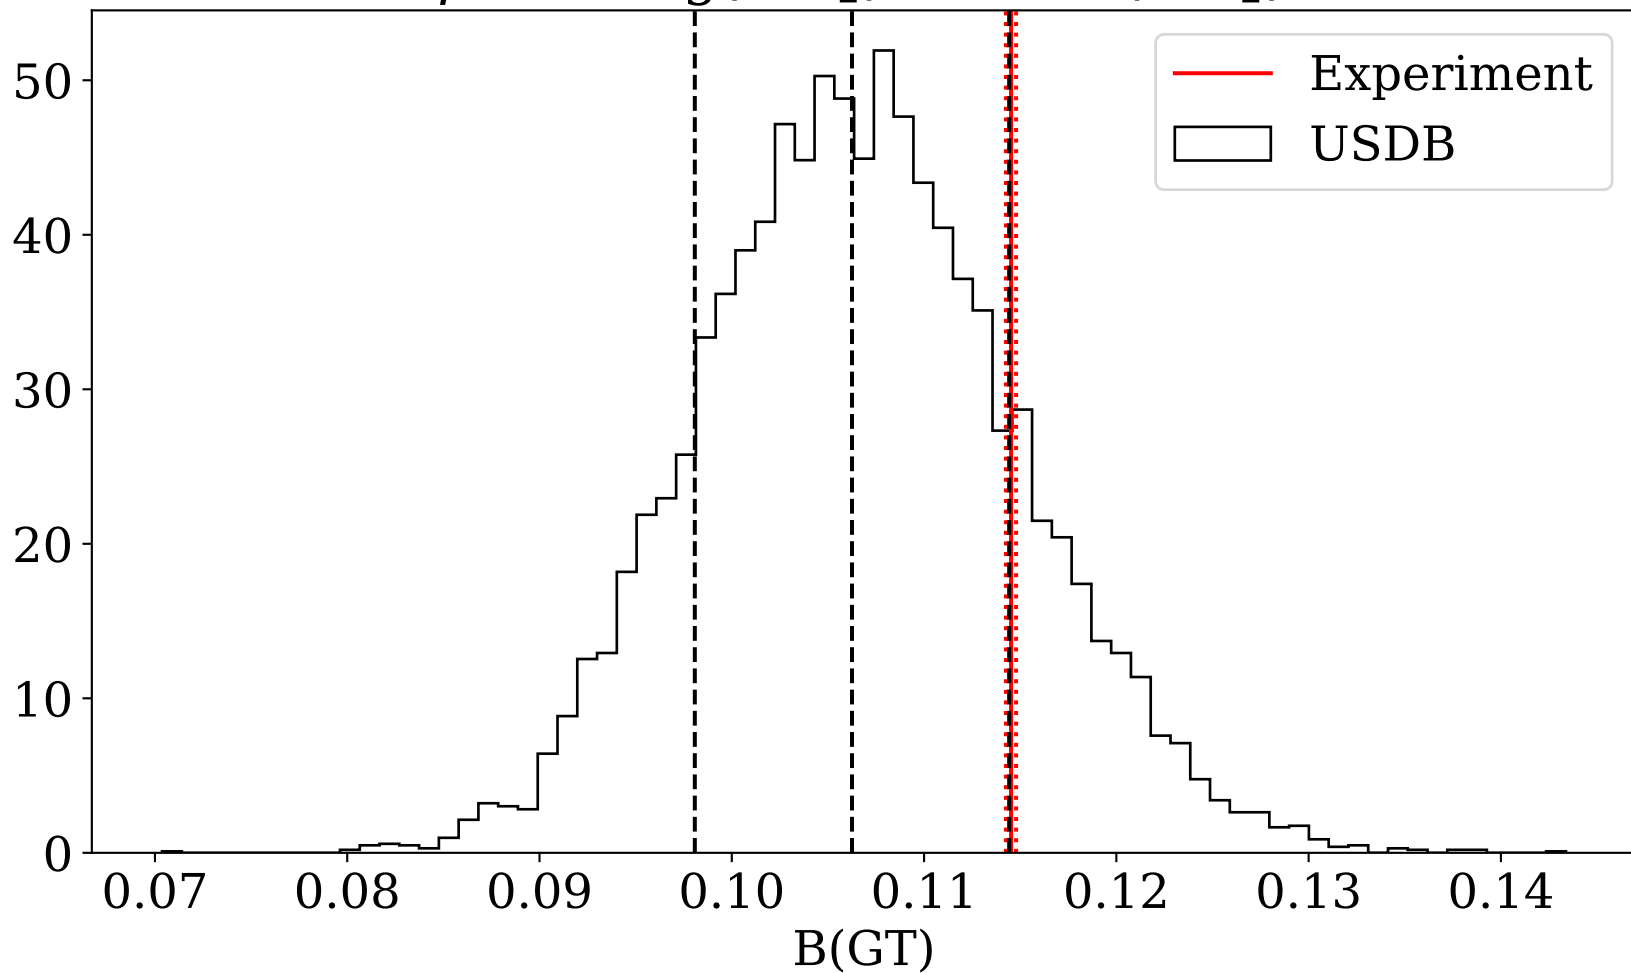

$\beta^- : {}^{27}\text{Mg}(1/2_1) \rightarrow {}^{27}\text{Al}(3/2_1)$

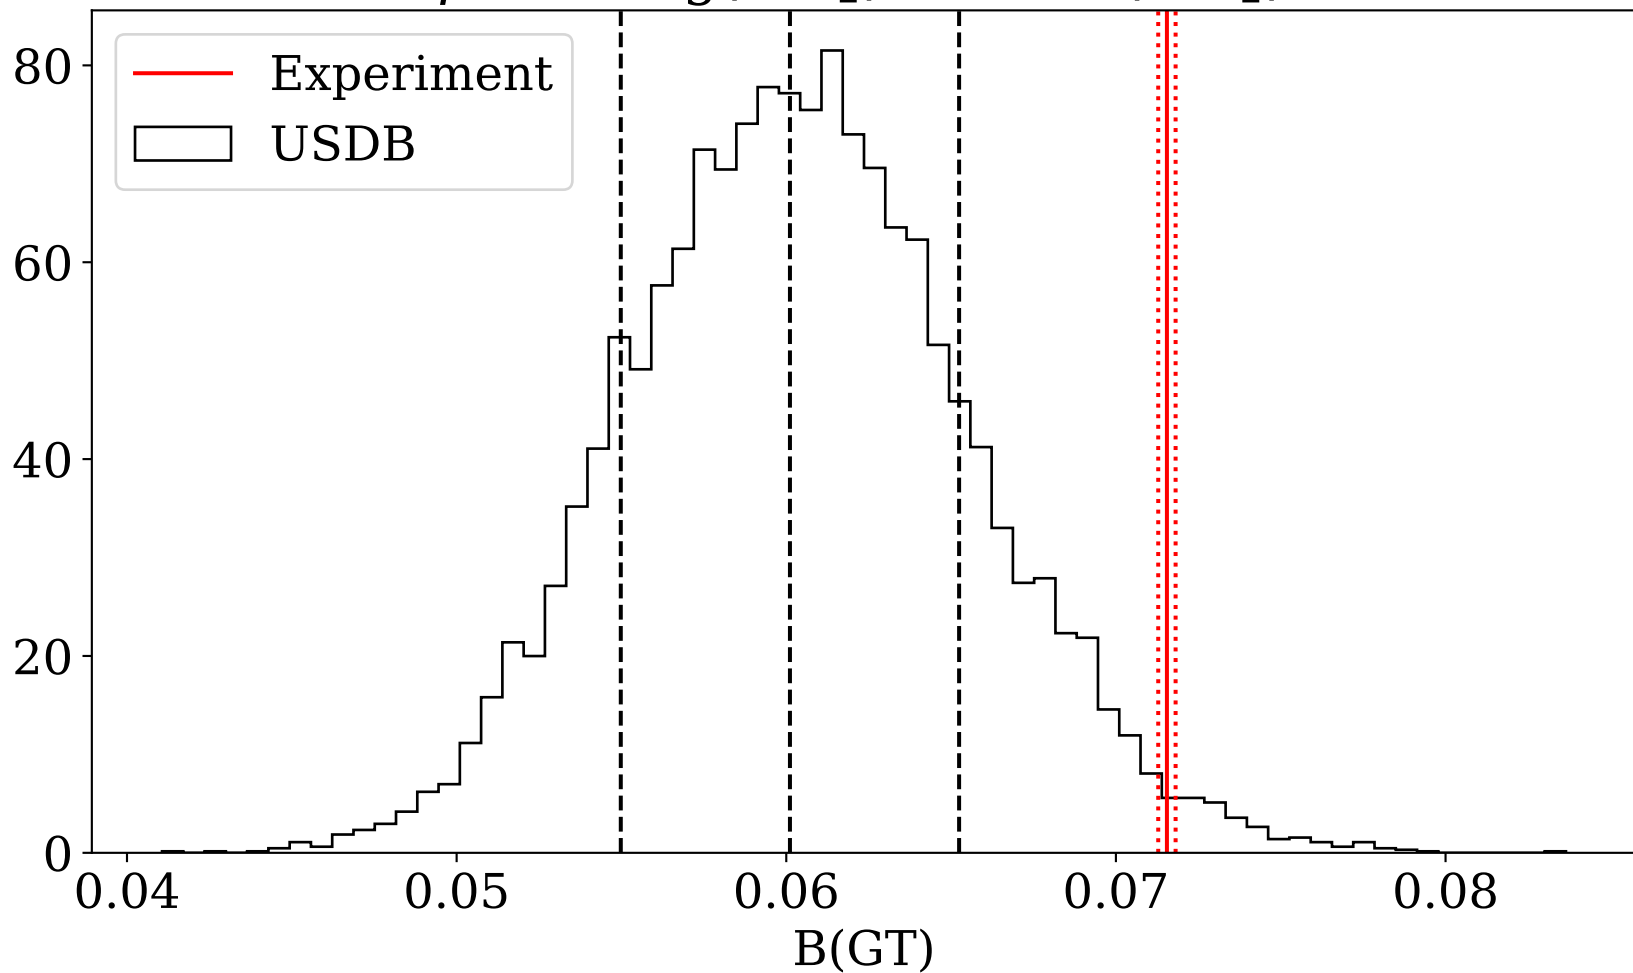

$\beta^- : {}^{28}\text{Mg}(0_1) \rightarrow {}^{28}\text{Al}(1_1)$

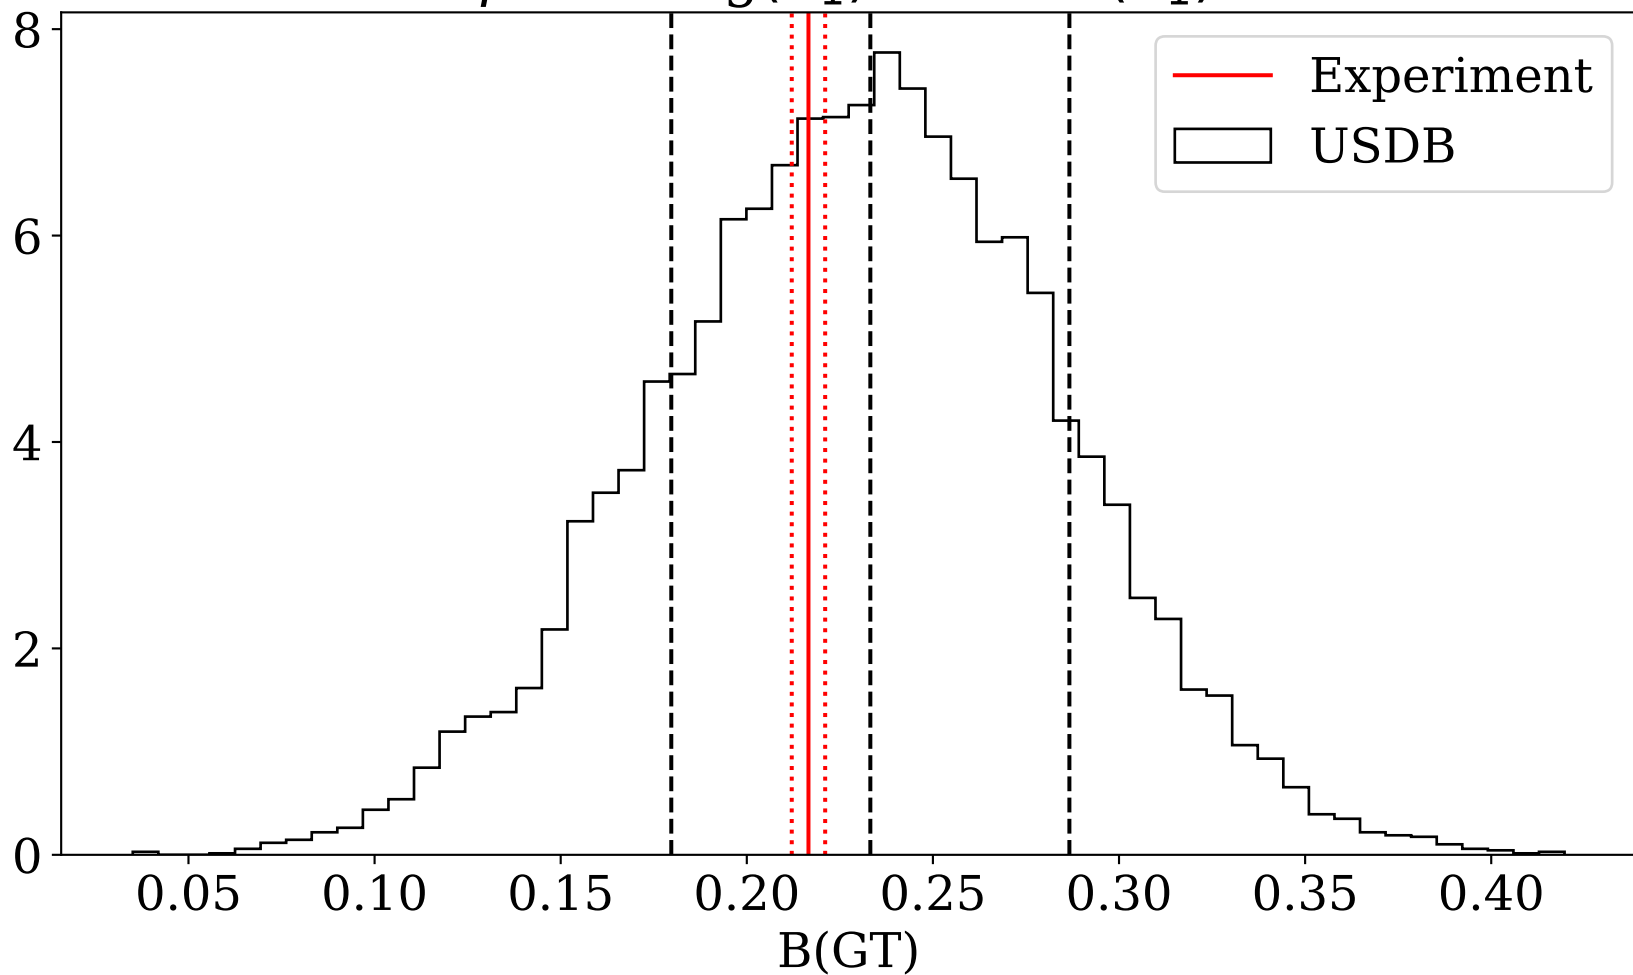

$\beta^- : {}^{28}\text{Mg}(0_1) \rightarrow {}^{28}\text{Al}(1_2)$

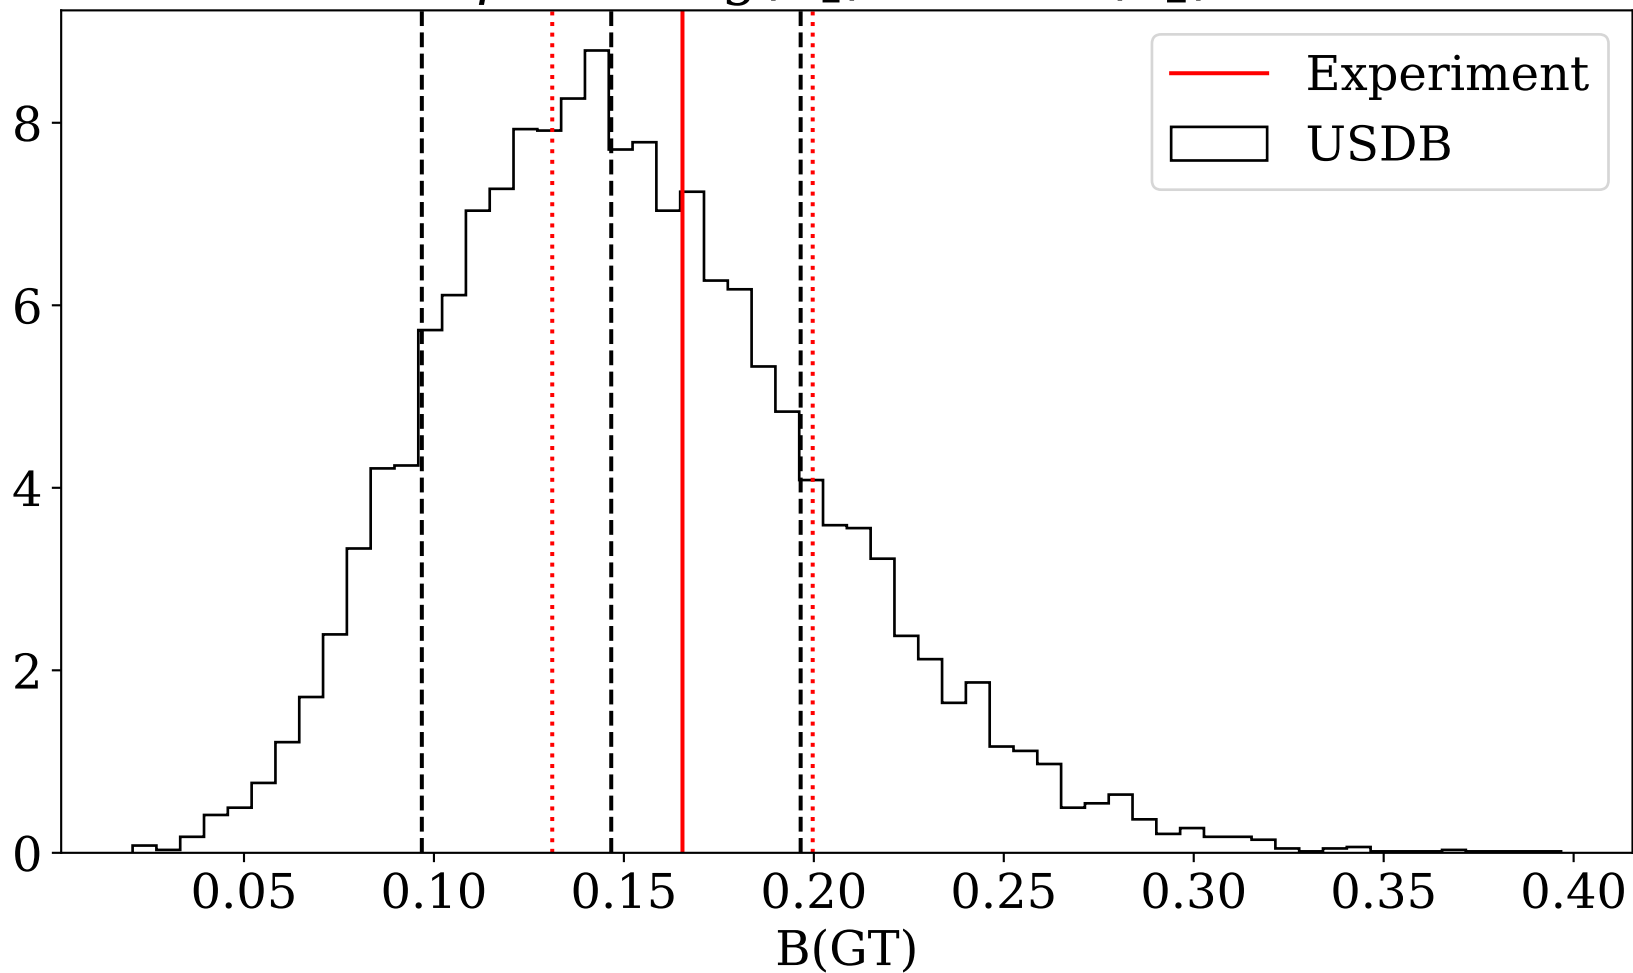



$\beta^- : {}^{29}\text{Mg}(3/2_1) \rightarrow {}^{29}\text{Al}(5/2_1)$

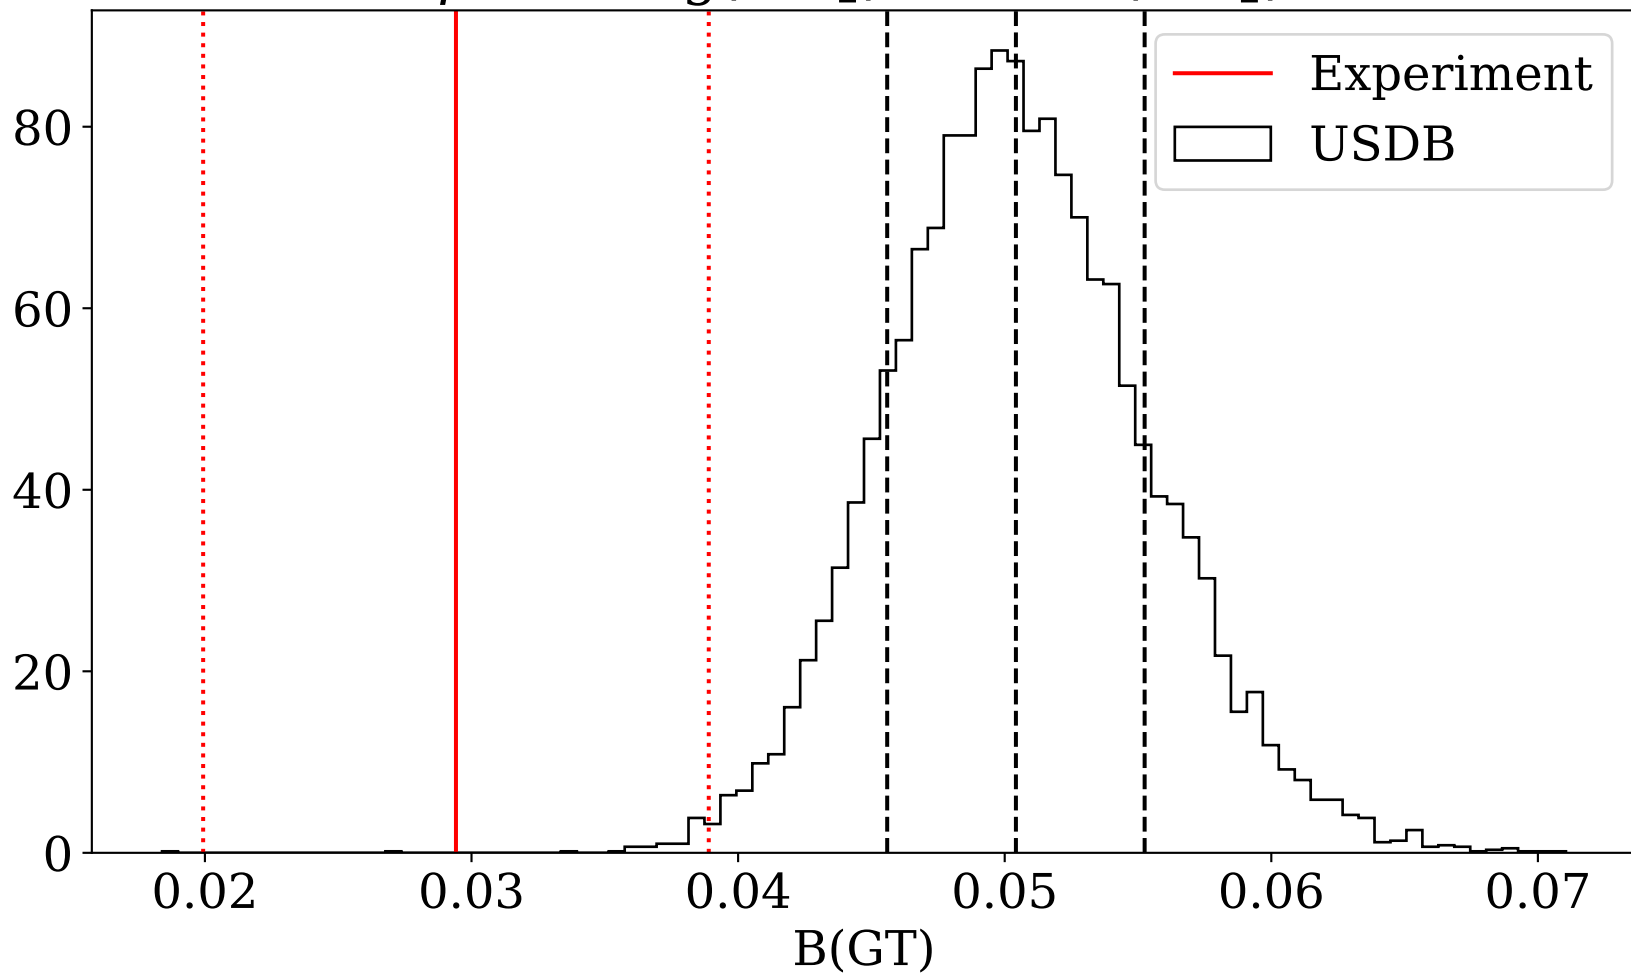

$\beta^- : {}^{29}\text{Mg}(3/2_1) \rightarrow {}^{29}\text{Al}(5/2_3)$

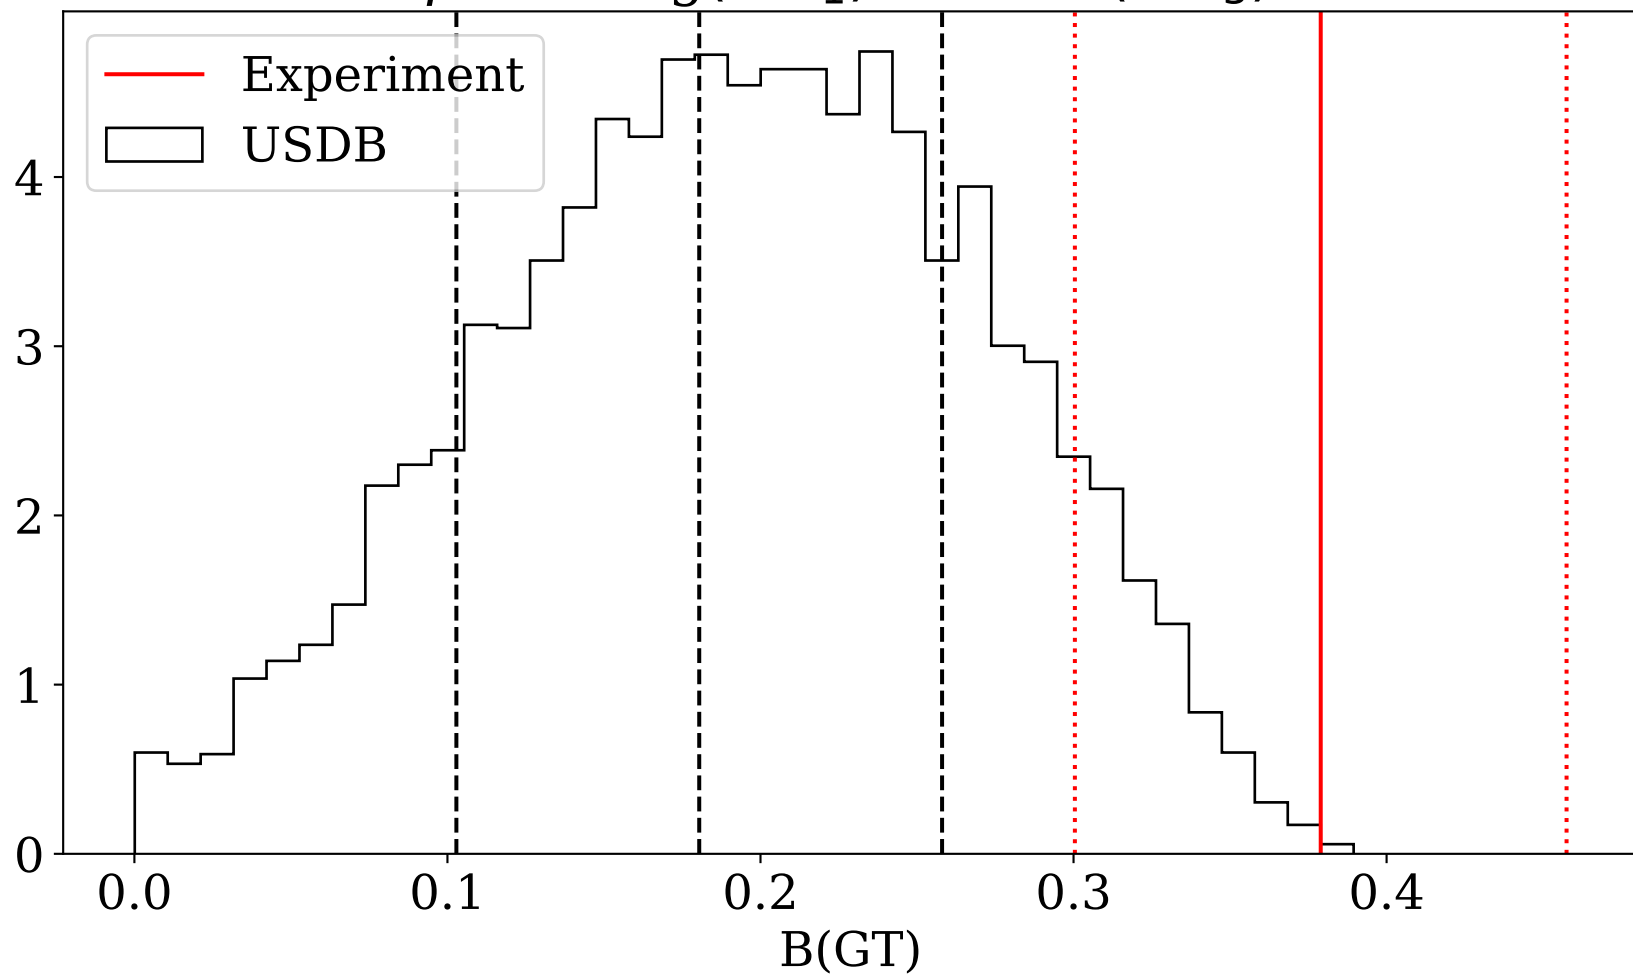

$\beta^- : {}^{29}\text{Mg}(3/2_1) \rightarrow {}^{29}\text{Al}(3/2_1)$

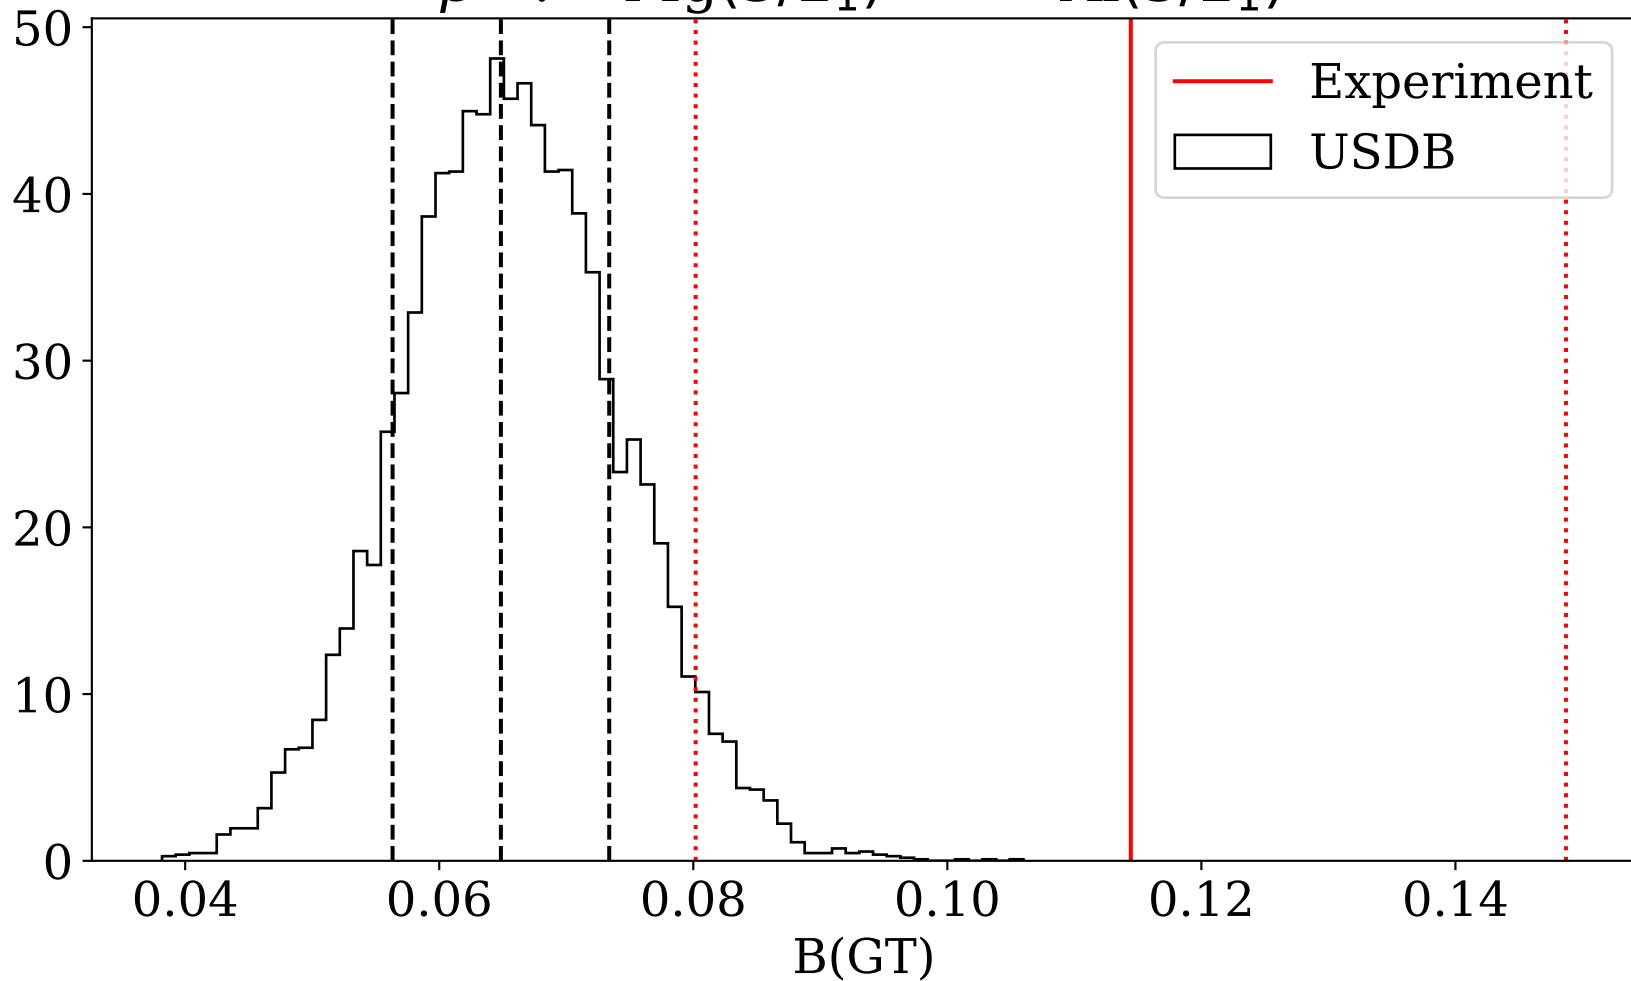

$\beta^- : {}^{29}\text{Mg}(3/2_1) \rightarrow {}^{29}\text{Al}(1/2_1)$

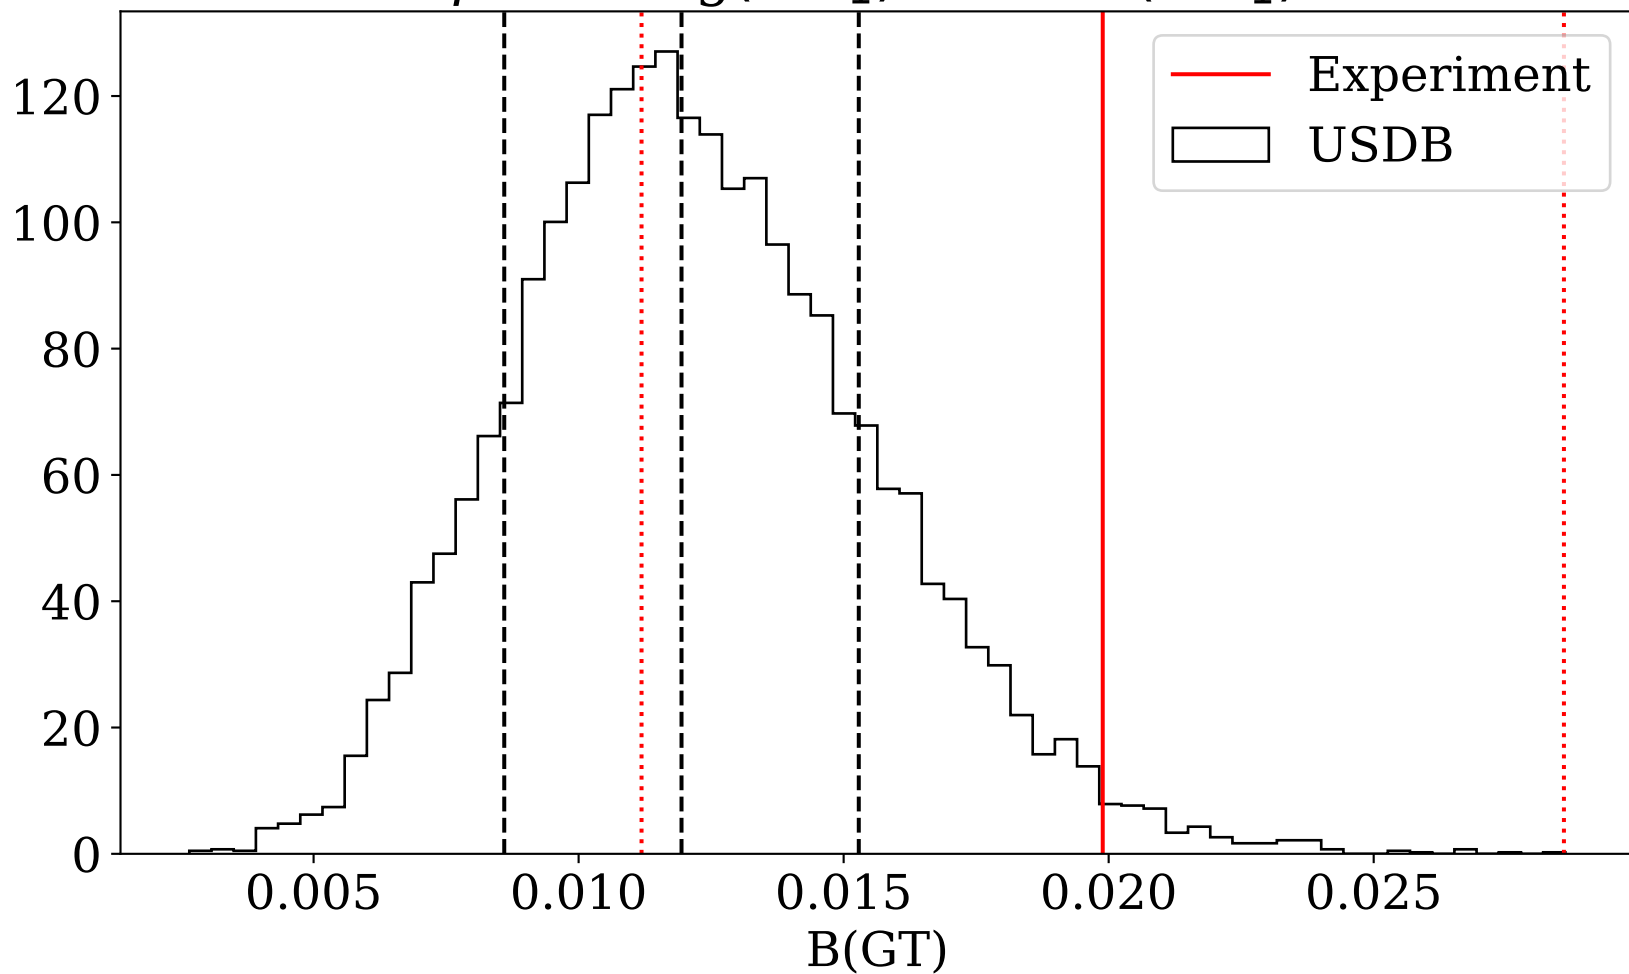

$\beta^- : {}^{29}\text{Mg}(3/2_1) \rightarrow {}^{29}\text{Al}(3/2_2)$

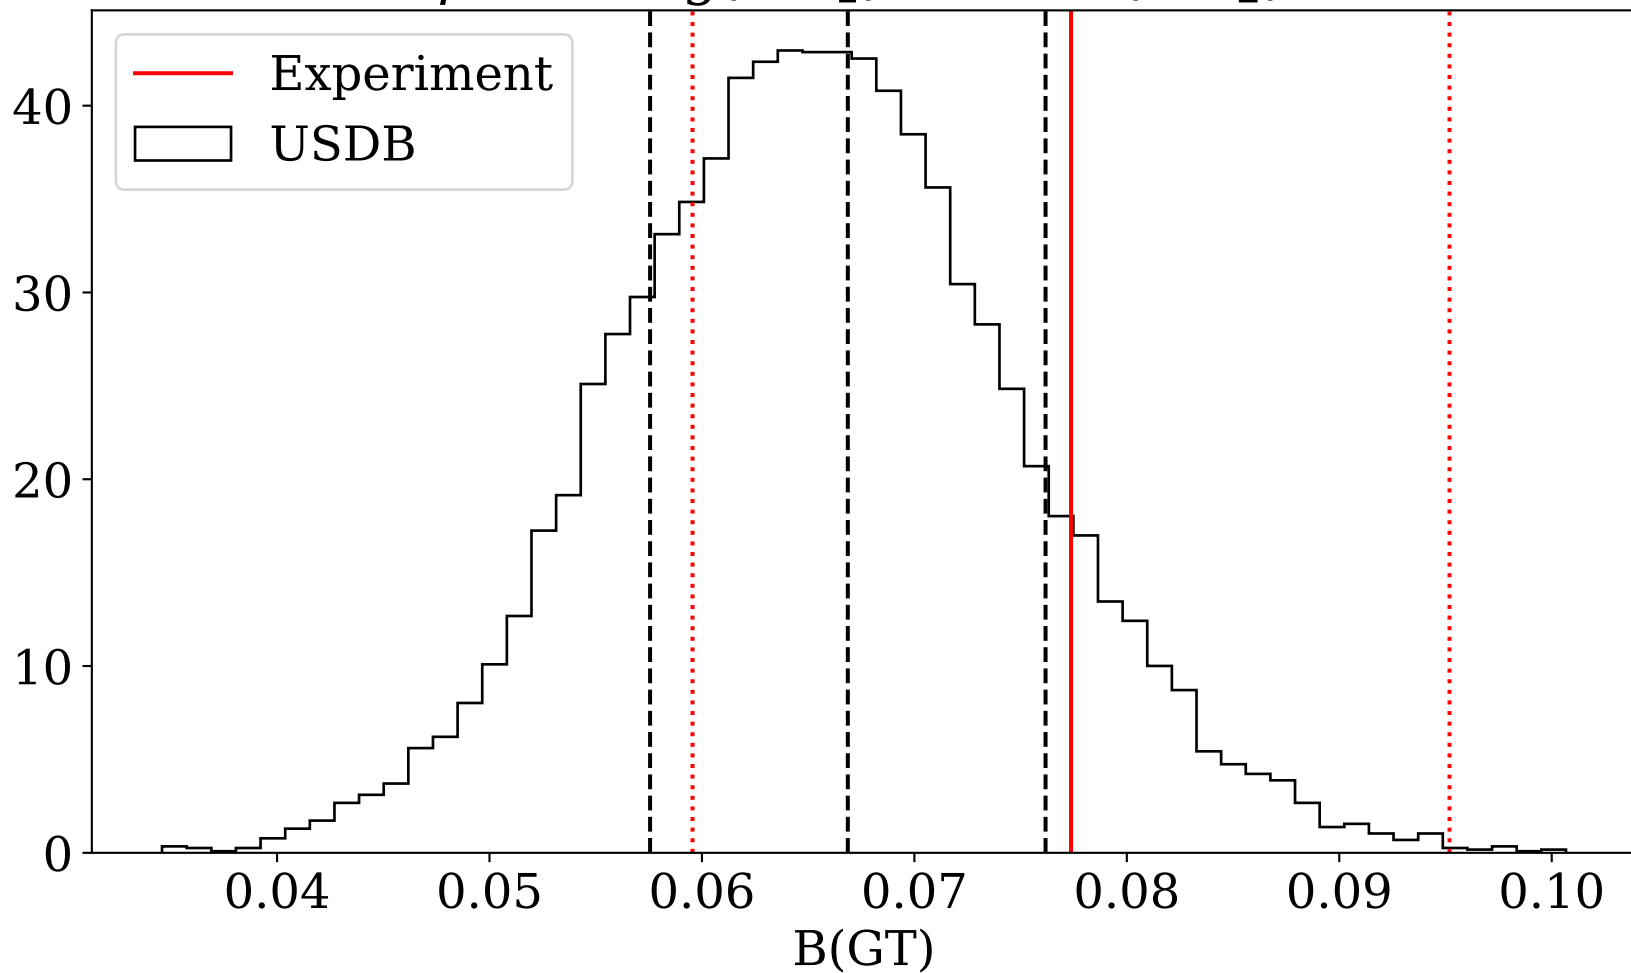

$\beta^- : {}^{29}\text{Mg}(3/2_1) \rightarrow {}^{29}\text{Al}(5/2_2)$

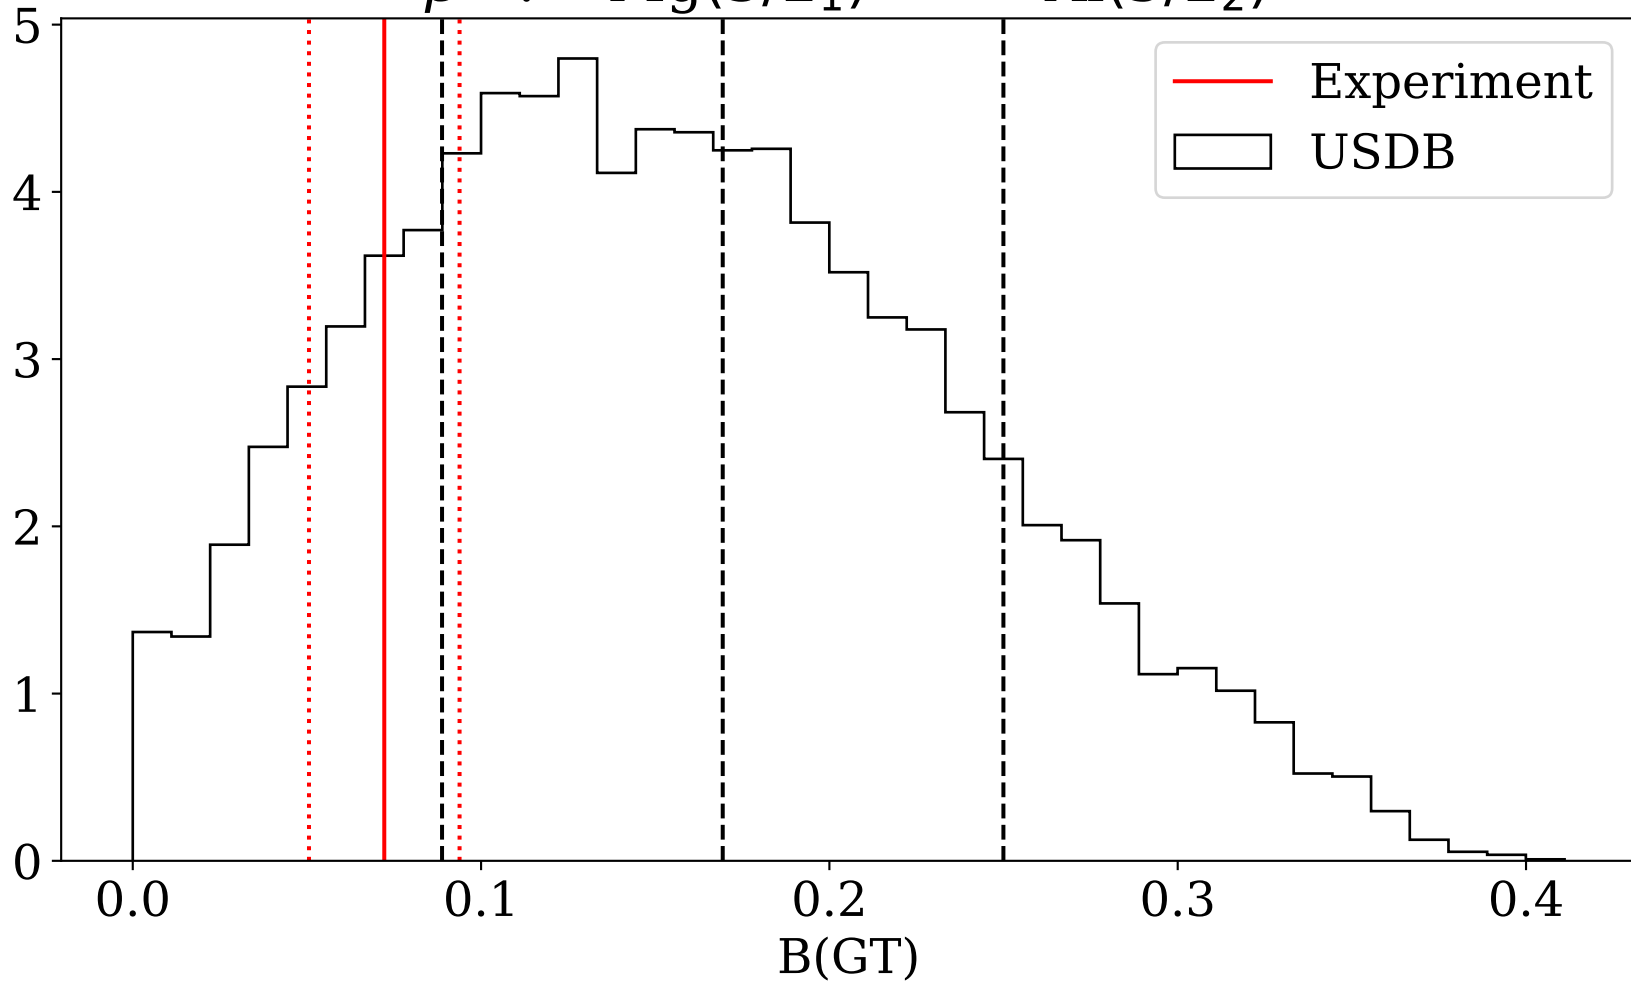

$\beta^- : {}^{29}\text{Mg}(3/2_1) \rightarrow {}^{29}\text{Al}(5/2_3)$

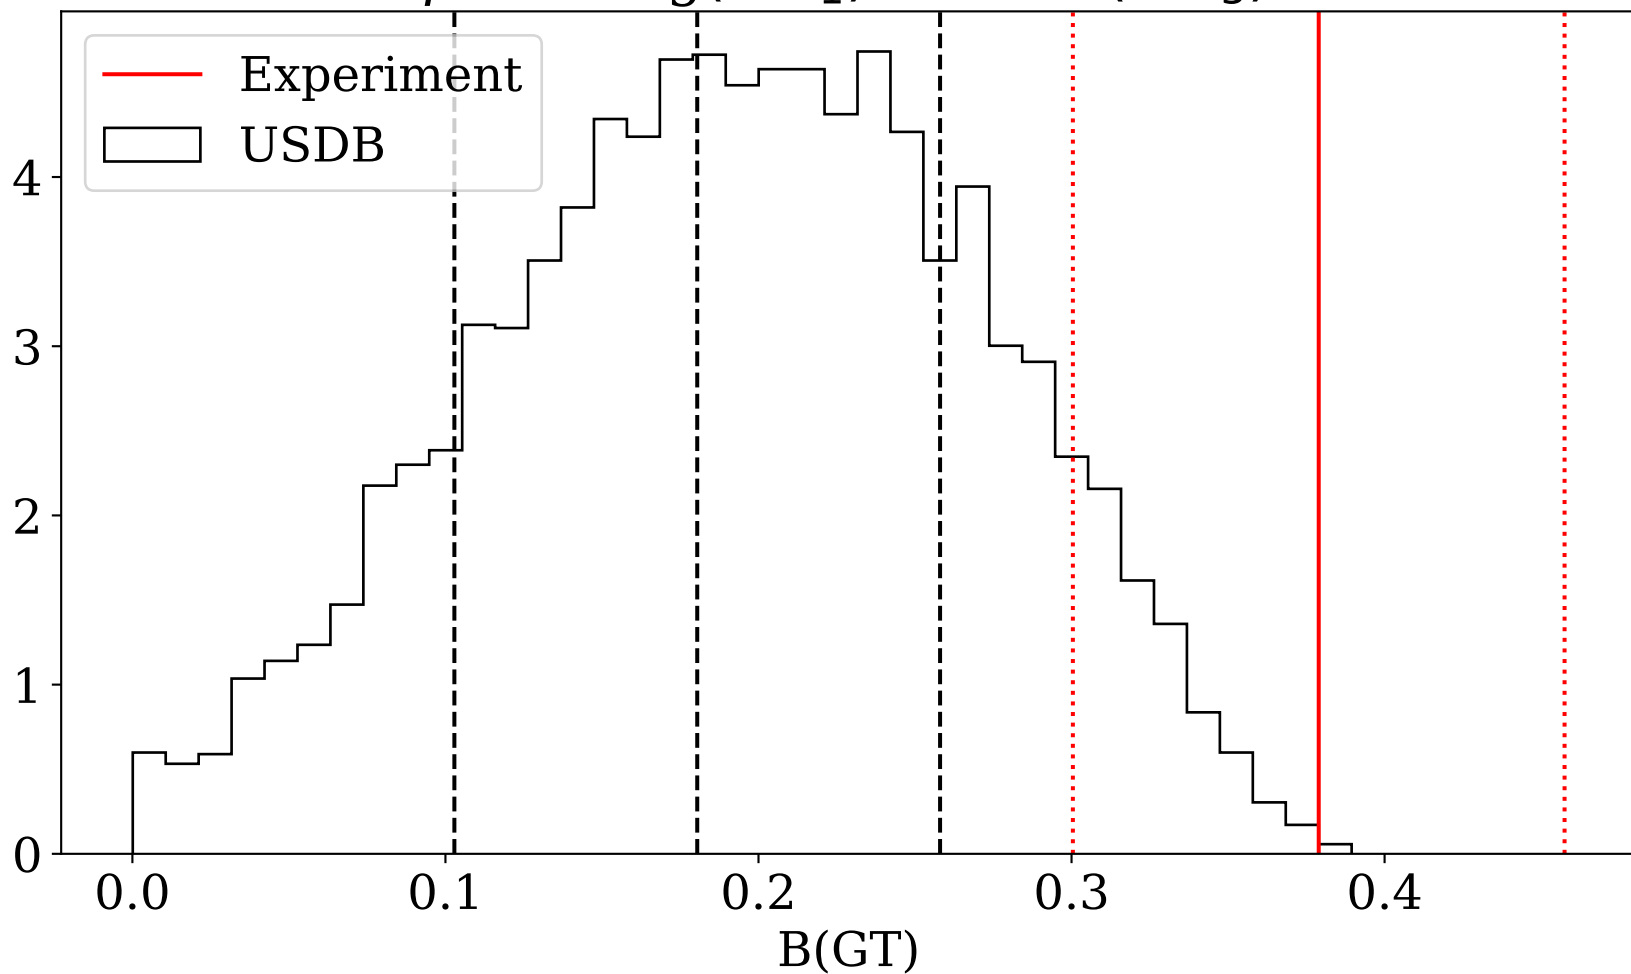

$\beta^- : {}^{29}\text{Mg}(3/2_1) \rightarrow {}^{29}\text{Al}(1/2_2)$

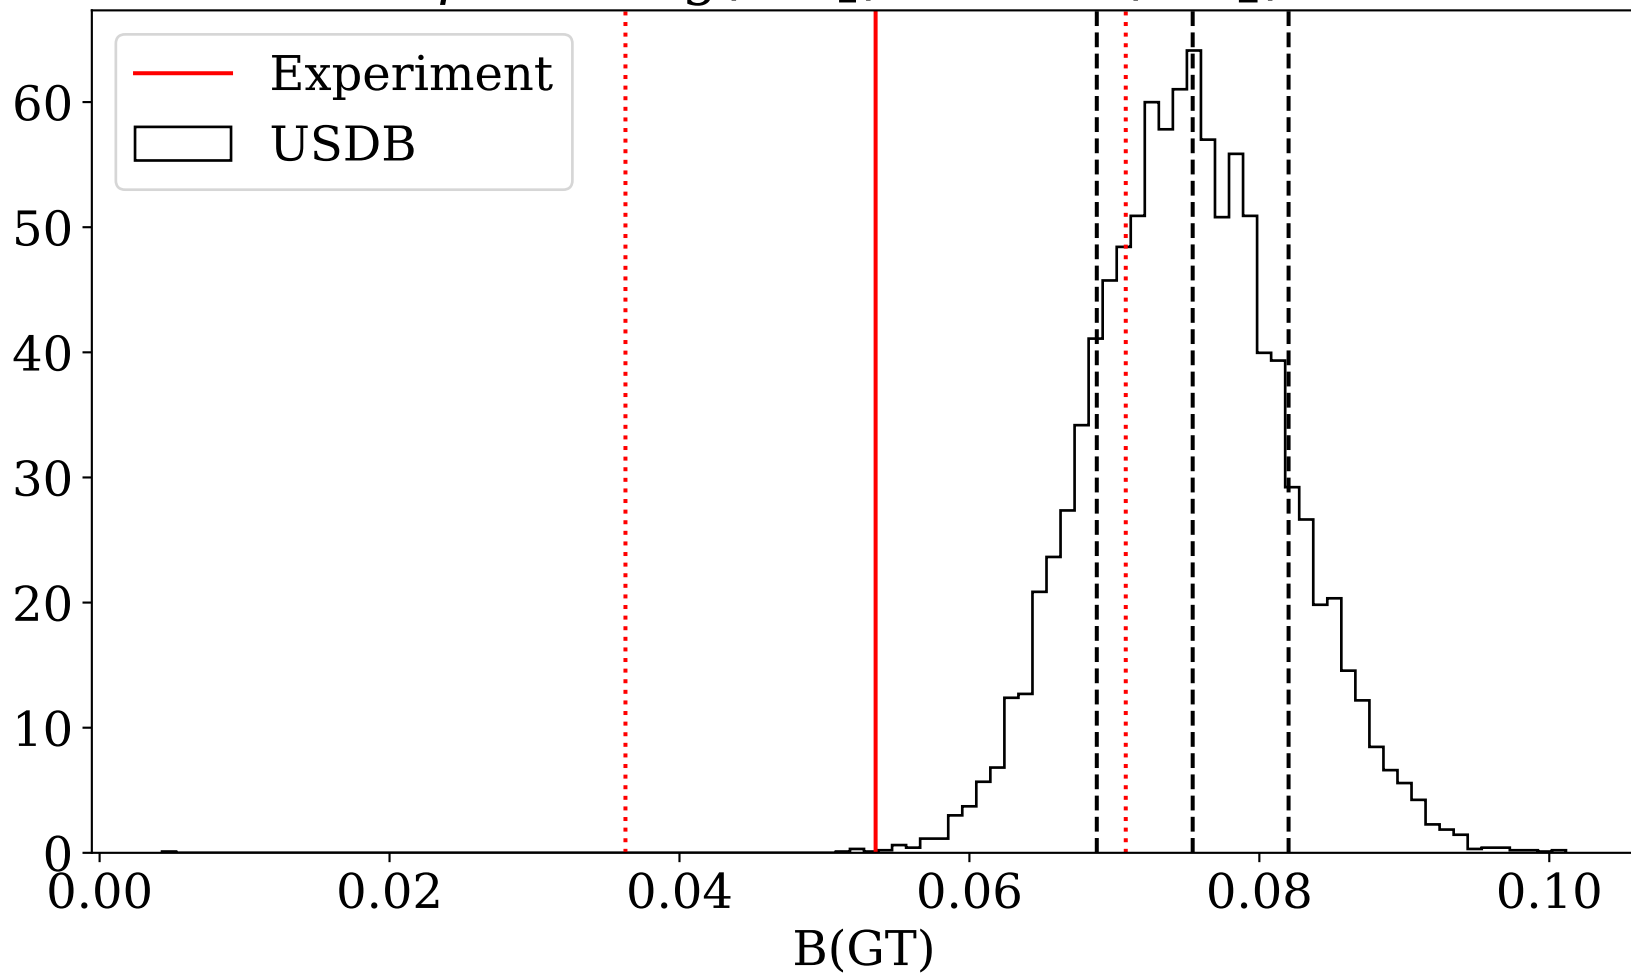



$\beta^- : {}^{30}\text{Mg}(0_1) \rightarrow {}^{30}\text{Al}(1_1)$

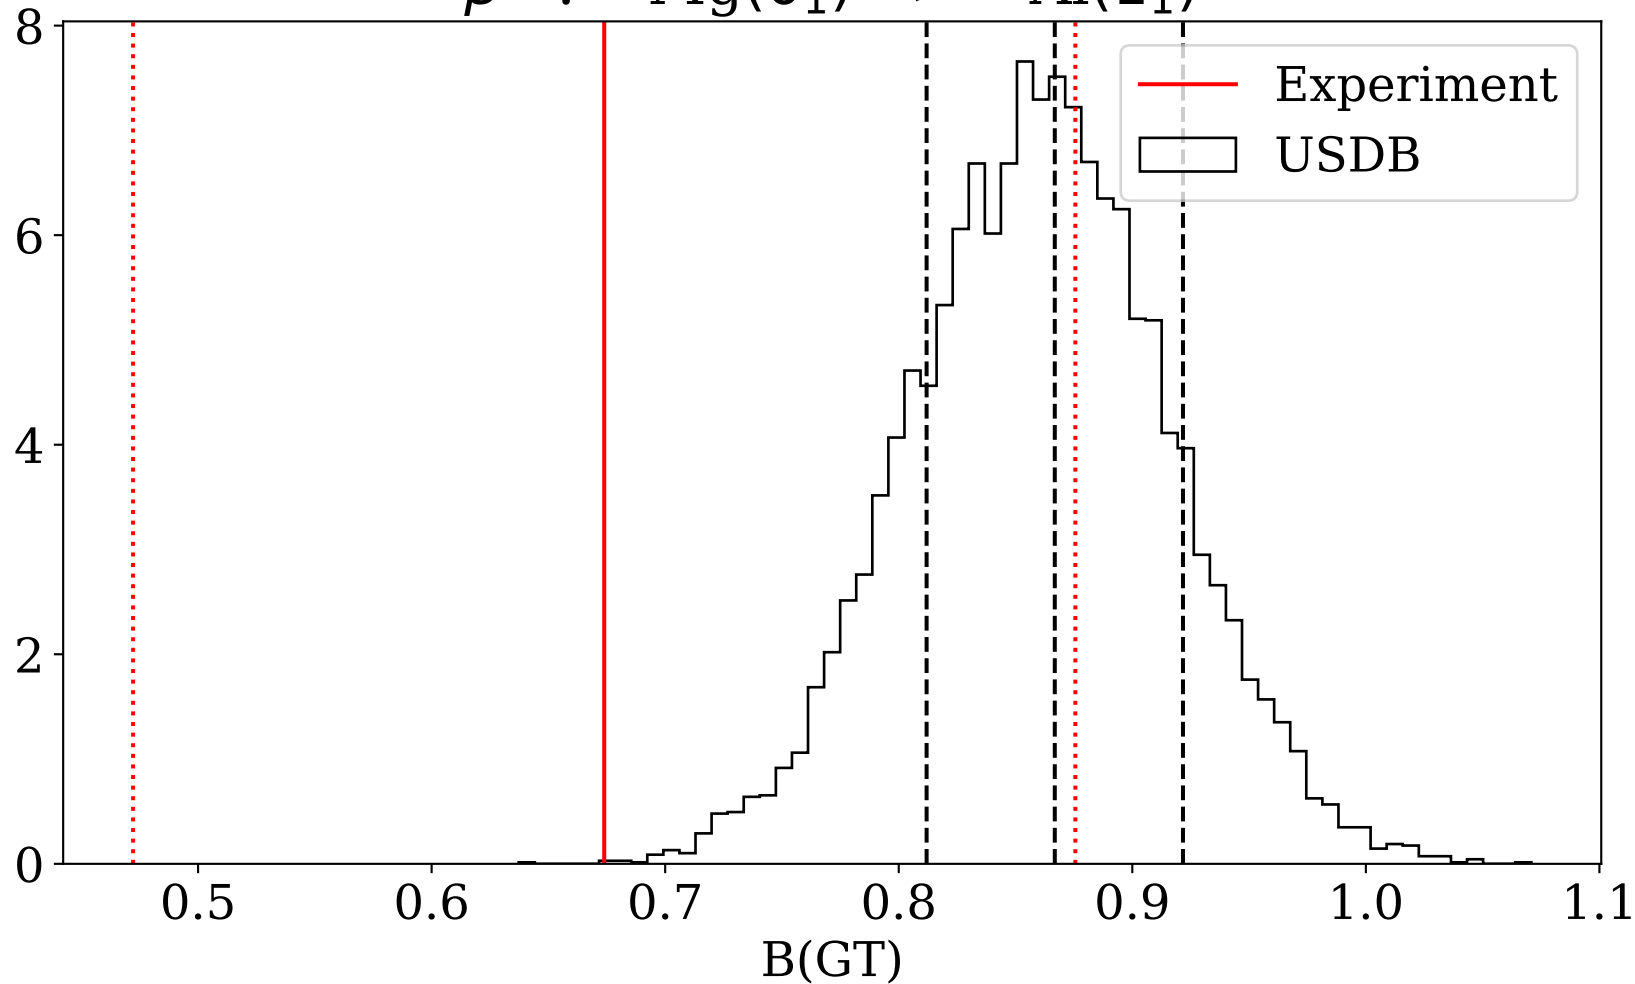

$\beta^- : {}^{30}\text{Mg}(0_1) \rightarrow {}^{30}\text{Al}(1_2)$

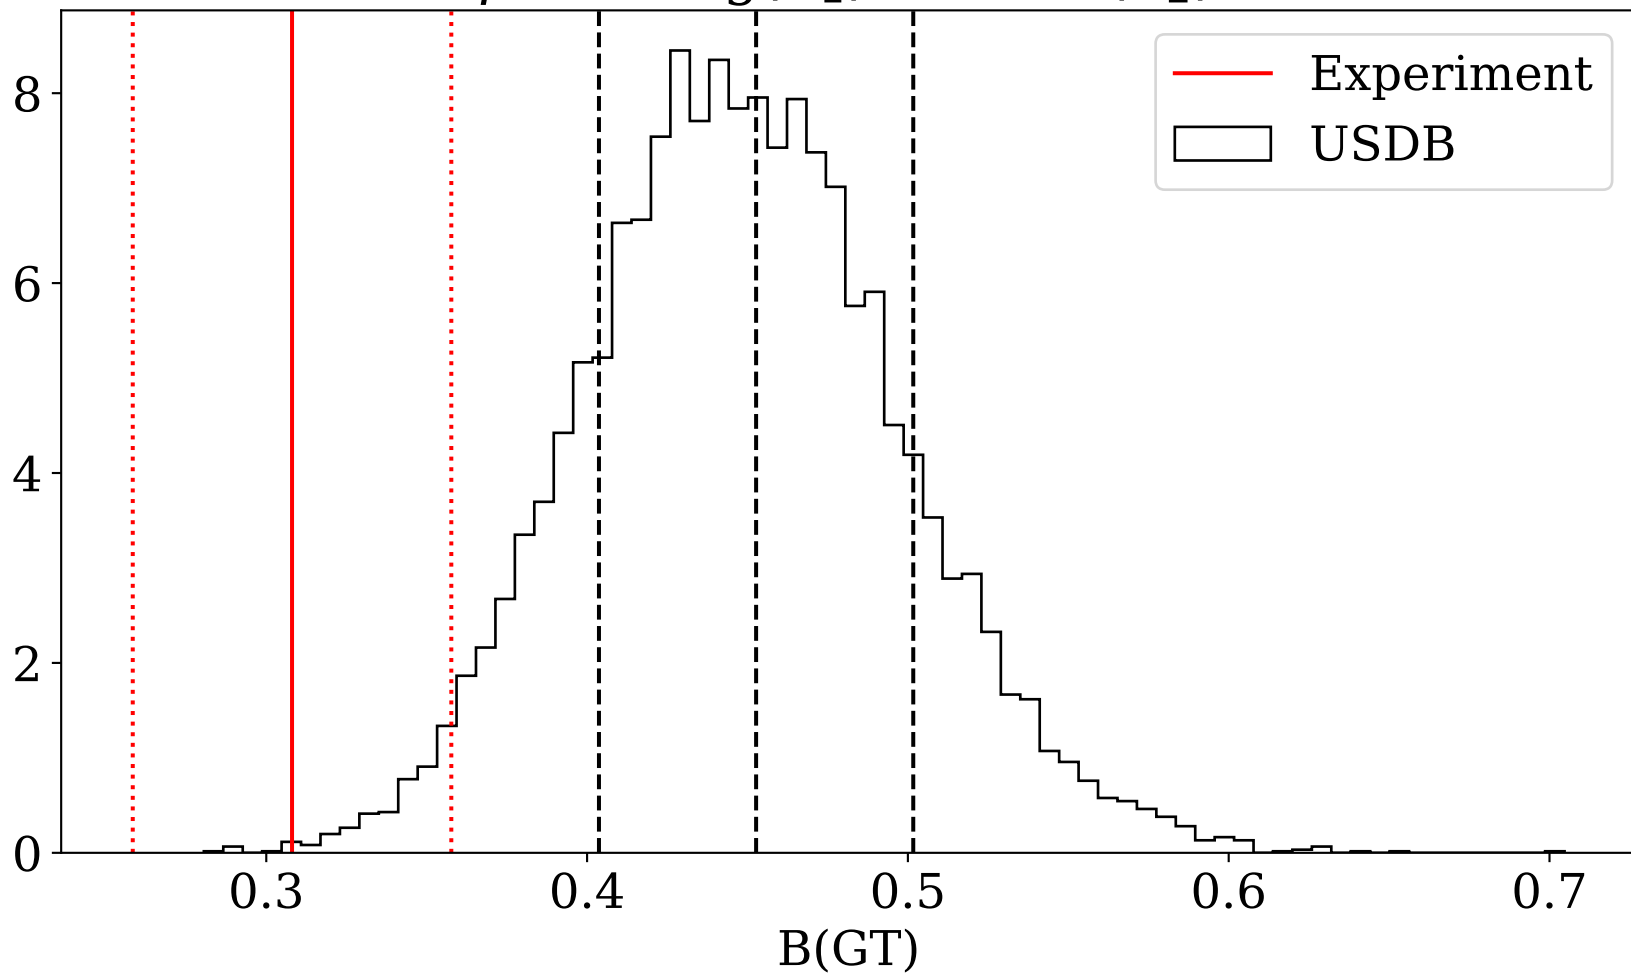

$\beta^- : {}^{28}\text{Al}(3_1) \rightarrow {}^{28}\text{Si}(2_1)$

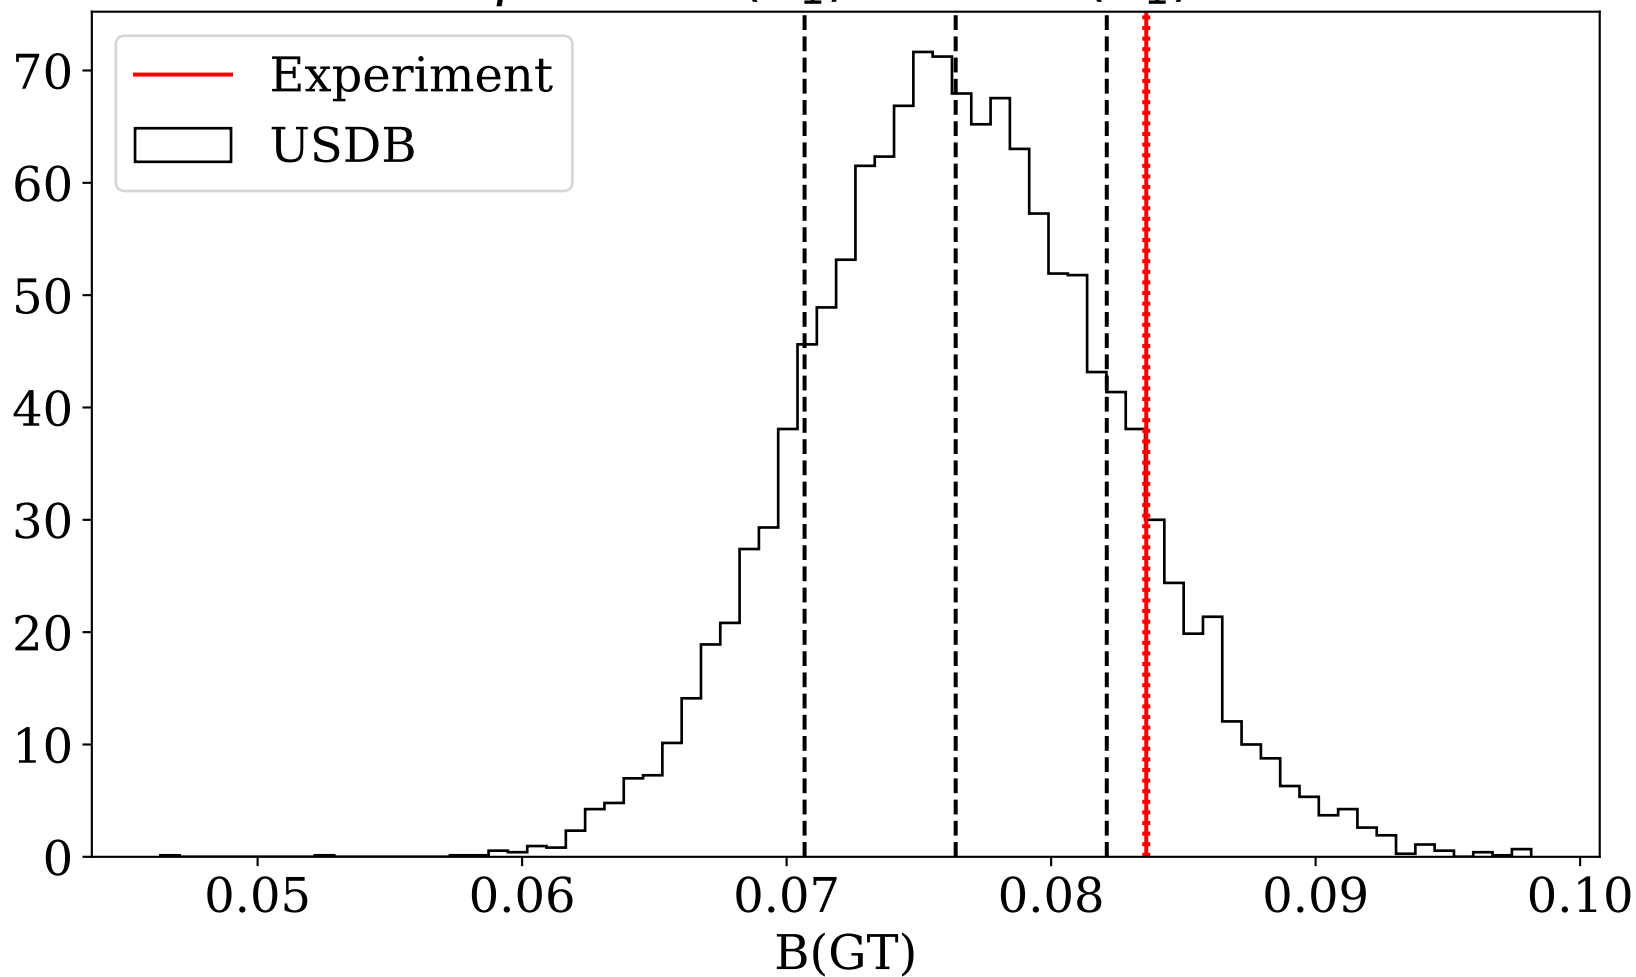

$\beta^- : {}^{29}\text{Al}(5/2_1) \rightarrow {}^{29}\text{Si}(3/2_1)$

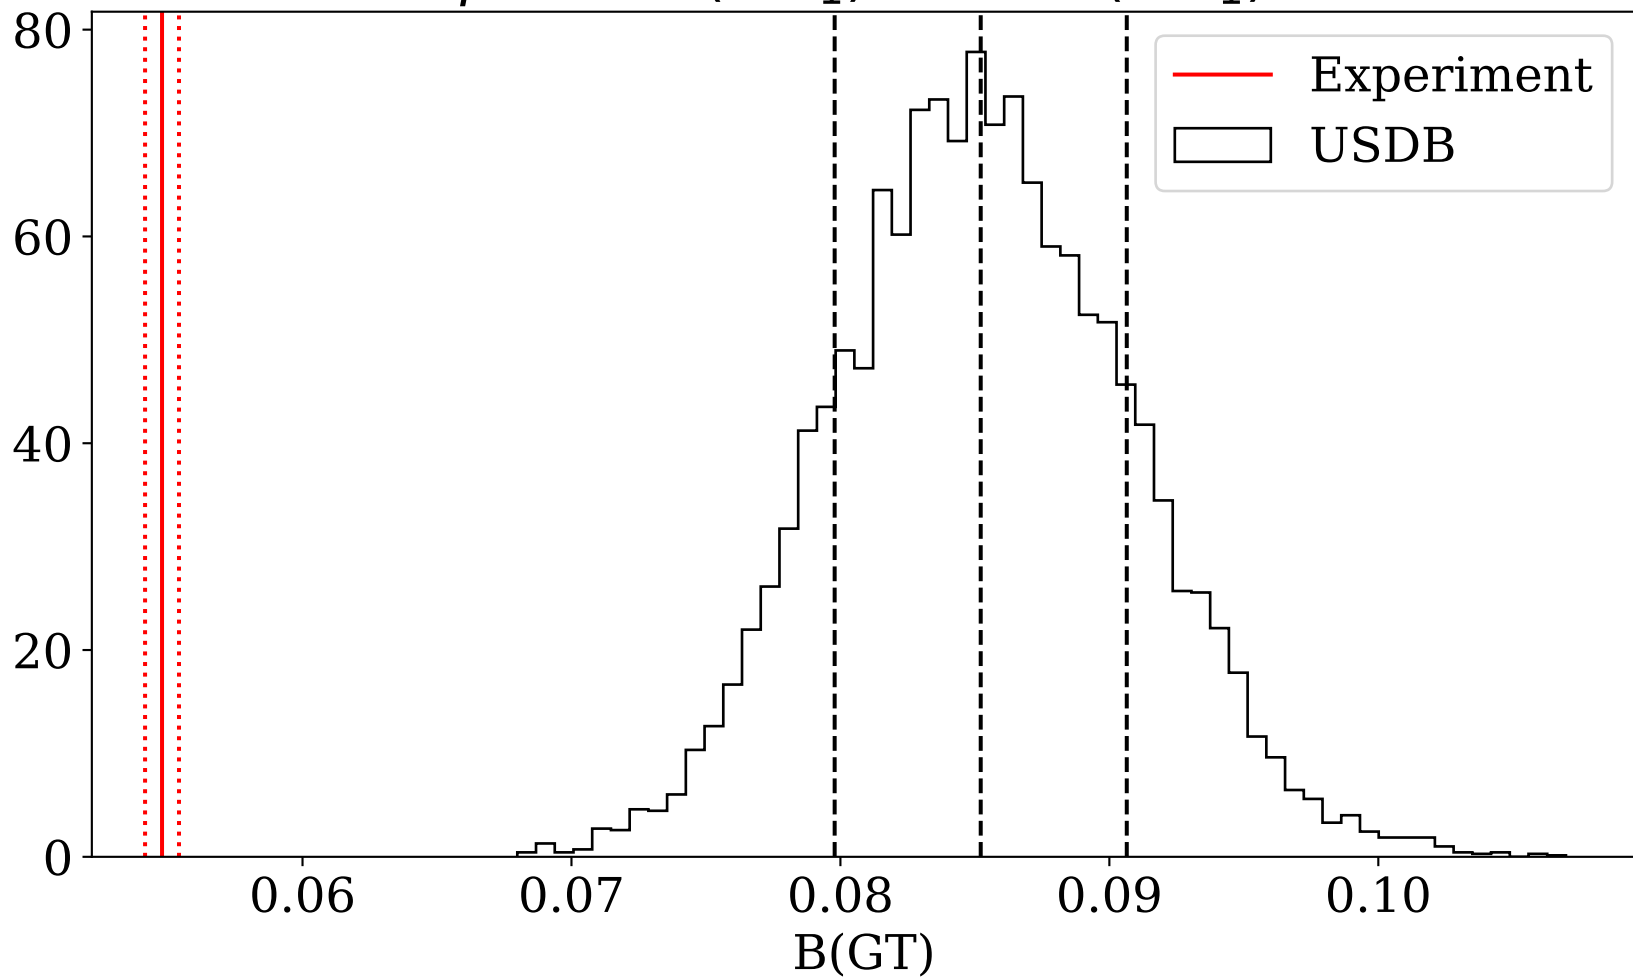

$\beta^- : {}^{29}\text{Al}(5/2_1) \rightarrow {}^{29}\text{Si}(5/2_1)$

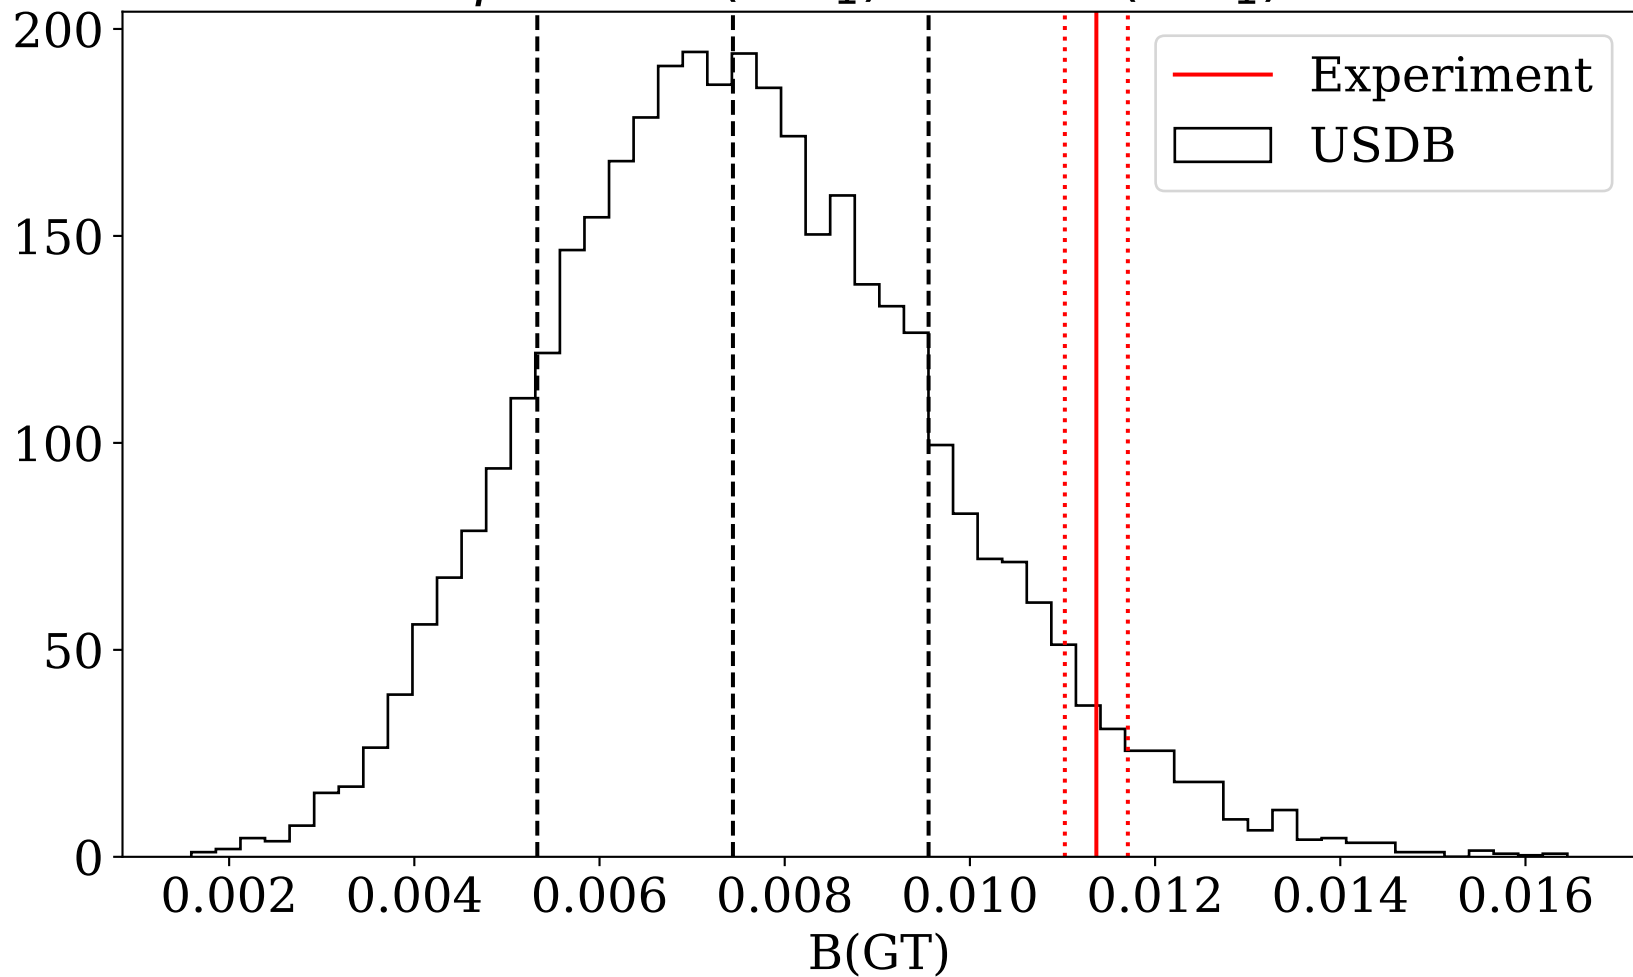

$\beta^- : {}^{29}\text{Al}(5/2_1) \rightarrow {}^{29}\text{Si}(3/2_2)$

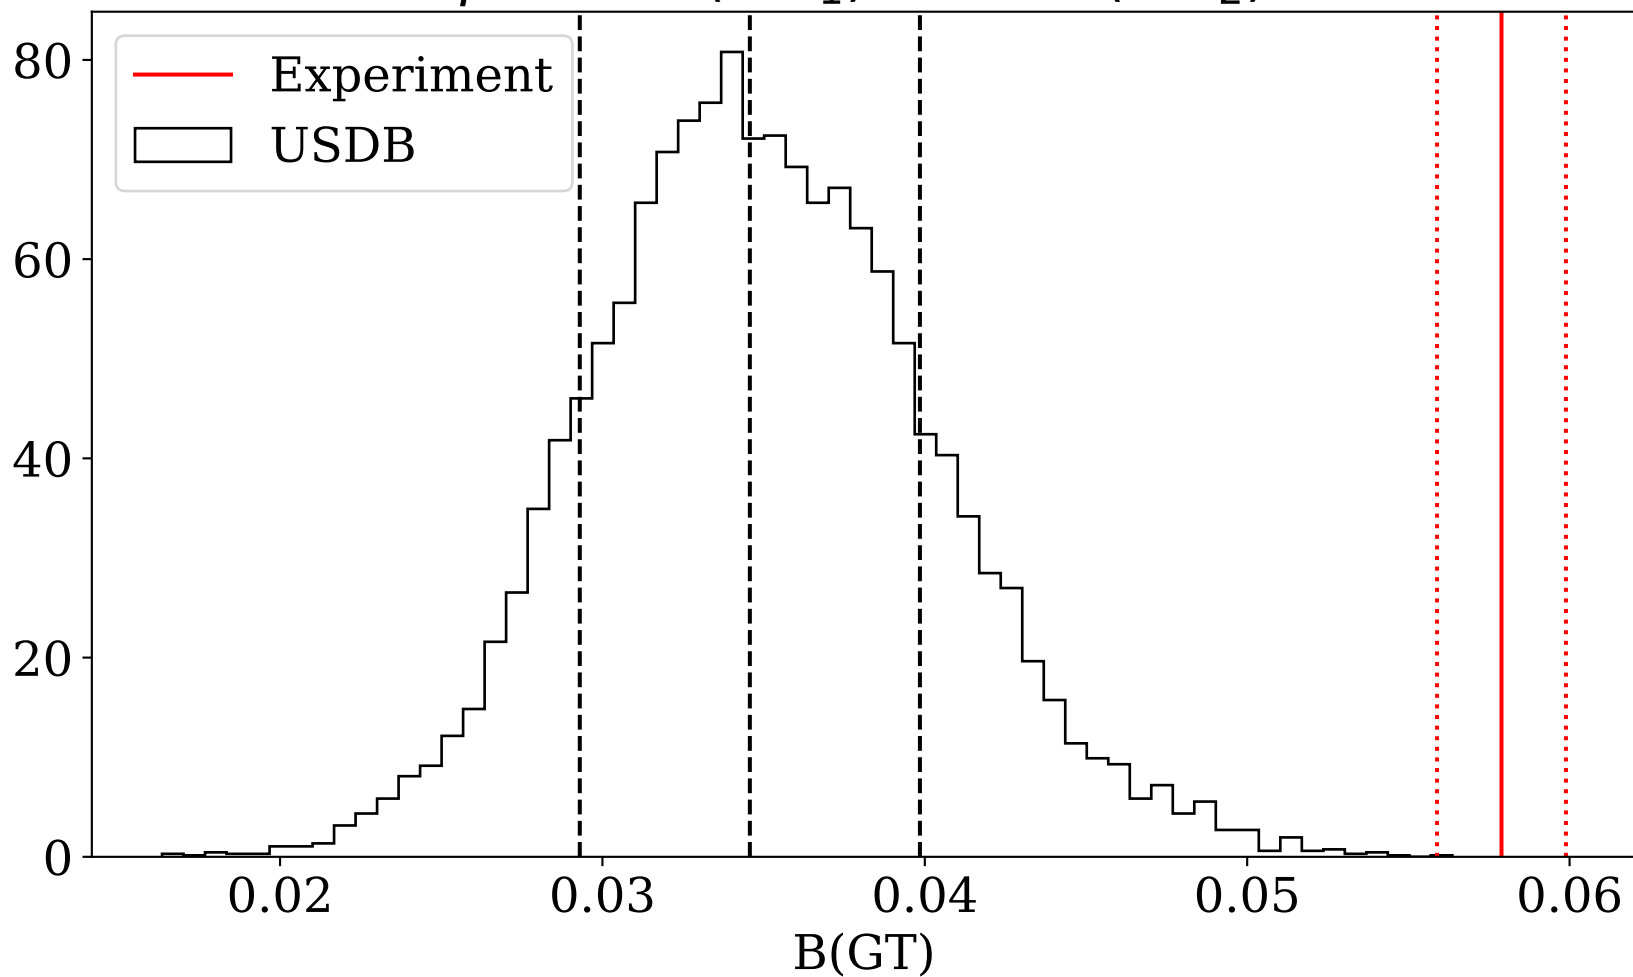

$\beta^- : {}^{30}\text{Al}(3_1) \rightarrow {}^{30}\text{Si}(2_1)$

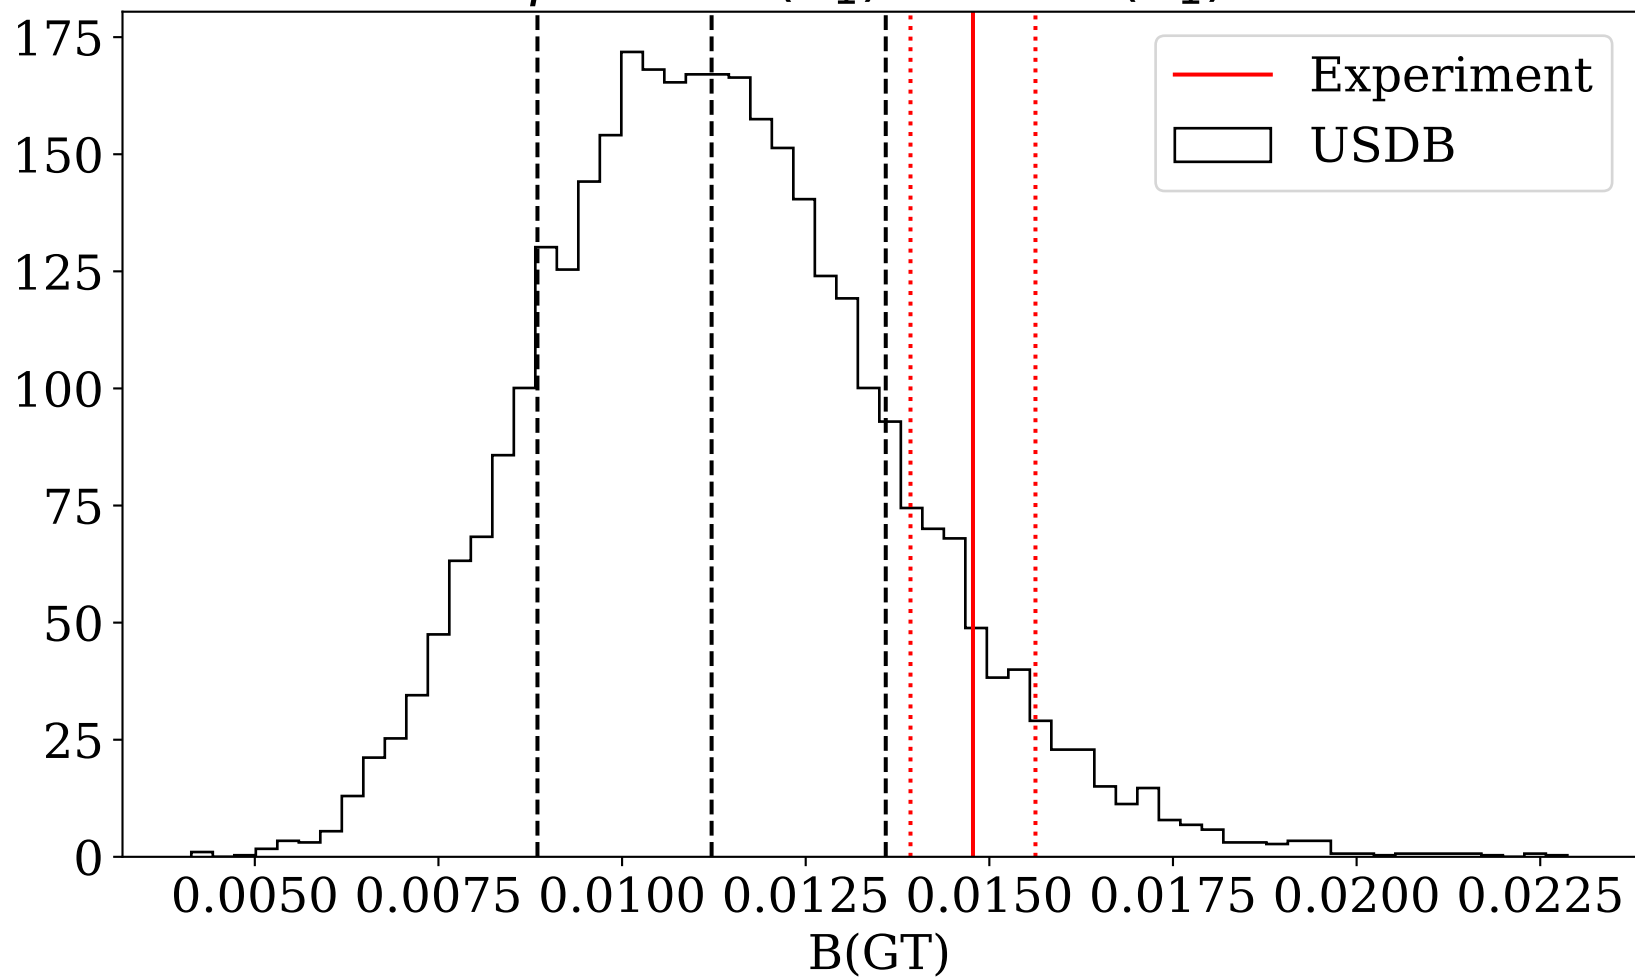

$\beta^- : {}^{30}\text{Al}(3_1) \rightarrow {}^{30}\text{Si}(2_2)$

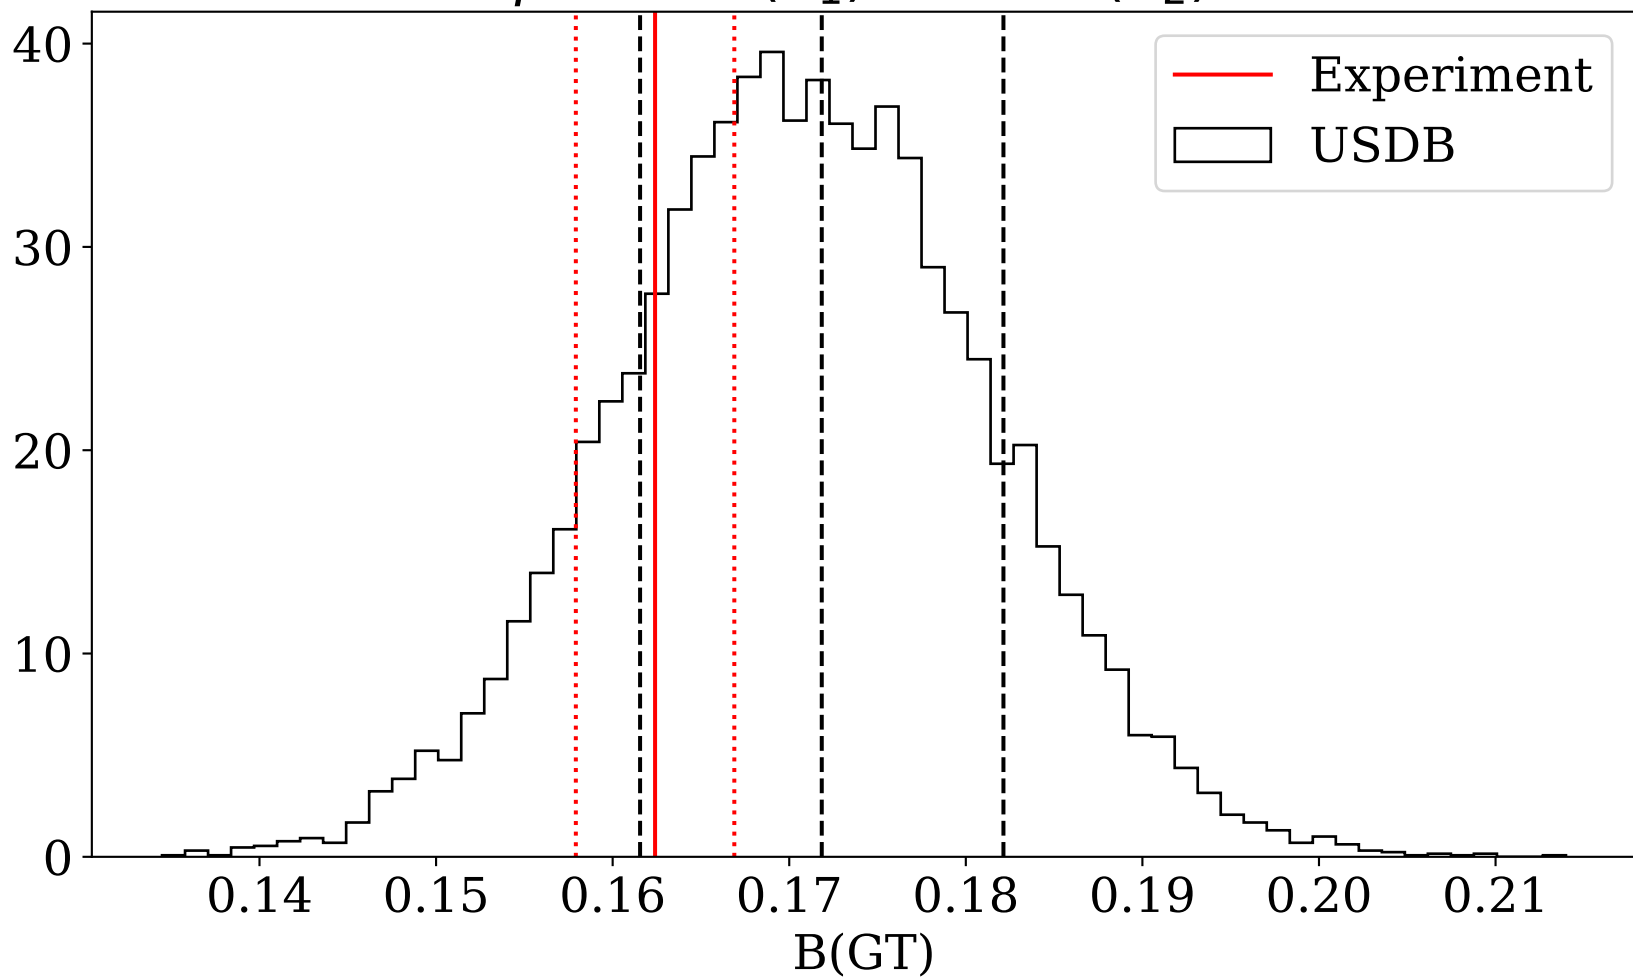



$\beta^- : {}^{30}\text{Al}(3_1) \rightarrow {}^{30}\text{Si}(2_3)$

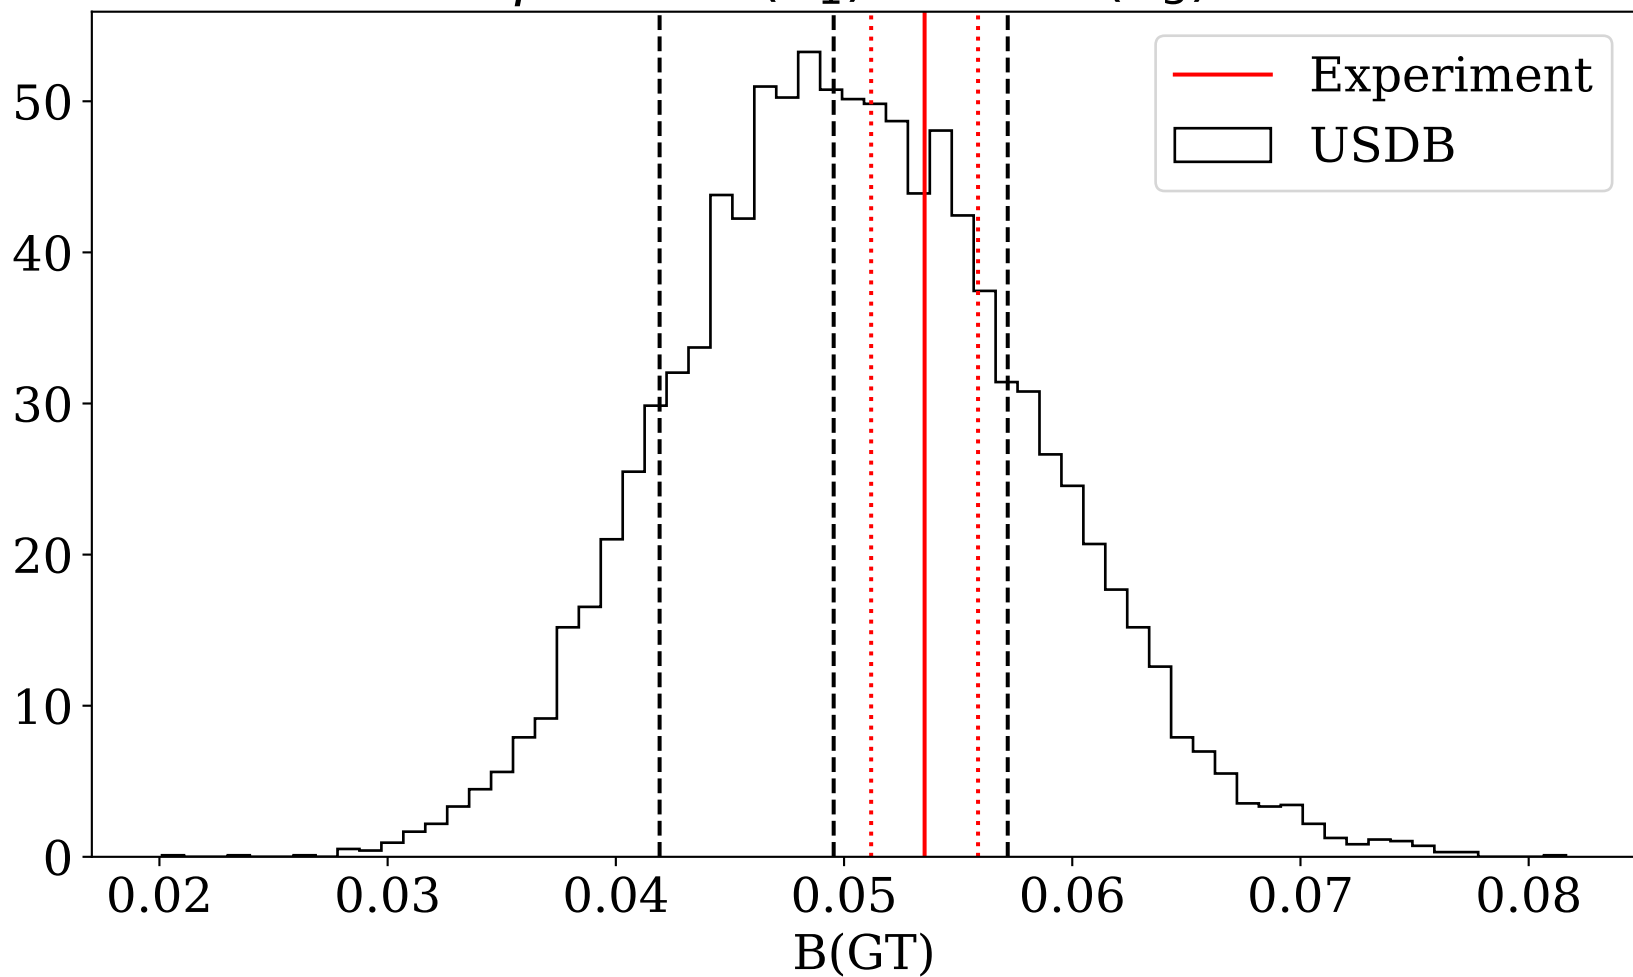

$\beta^- : {}^{30}\text{Al}(3_1) \rightarrow {}^{30}\text{Si}(3_1)$

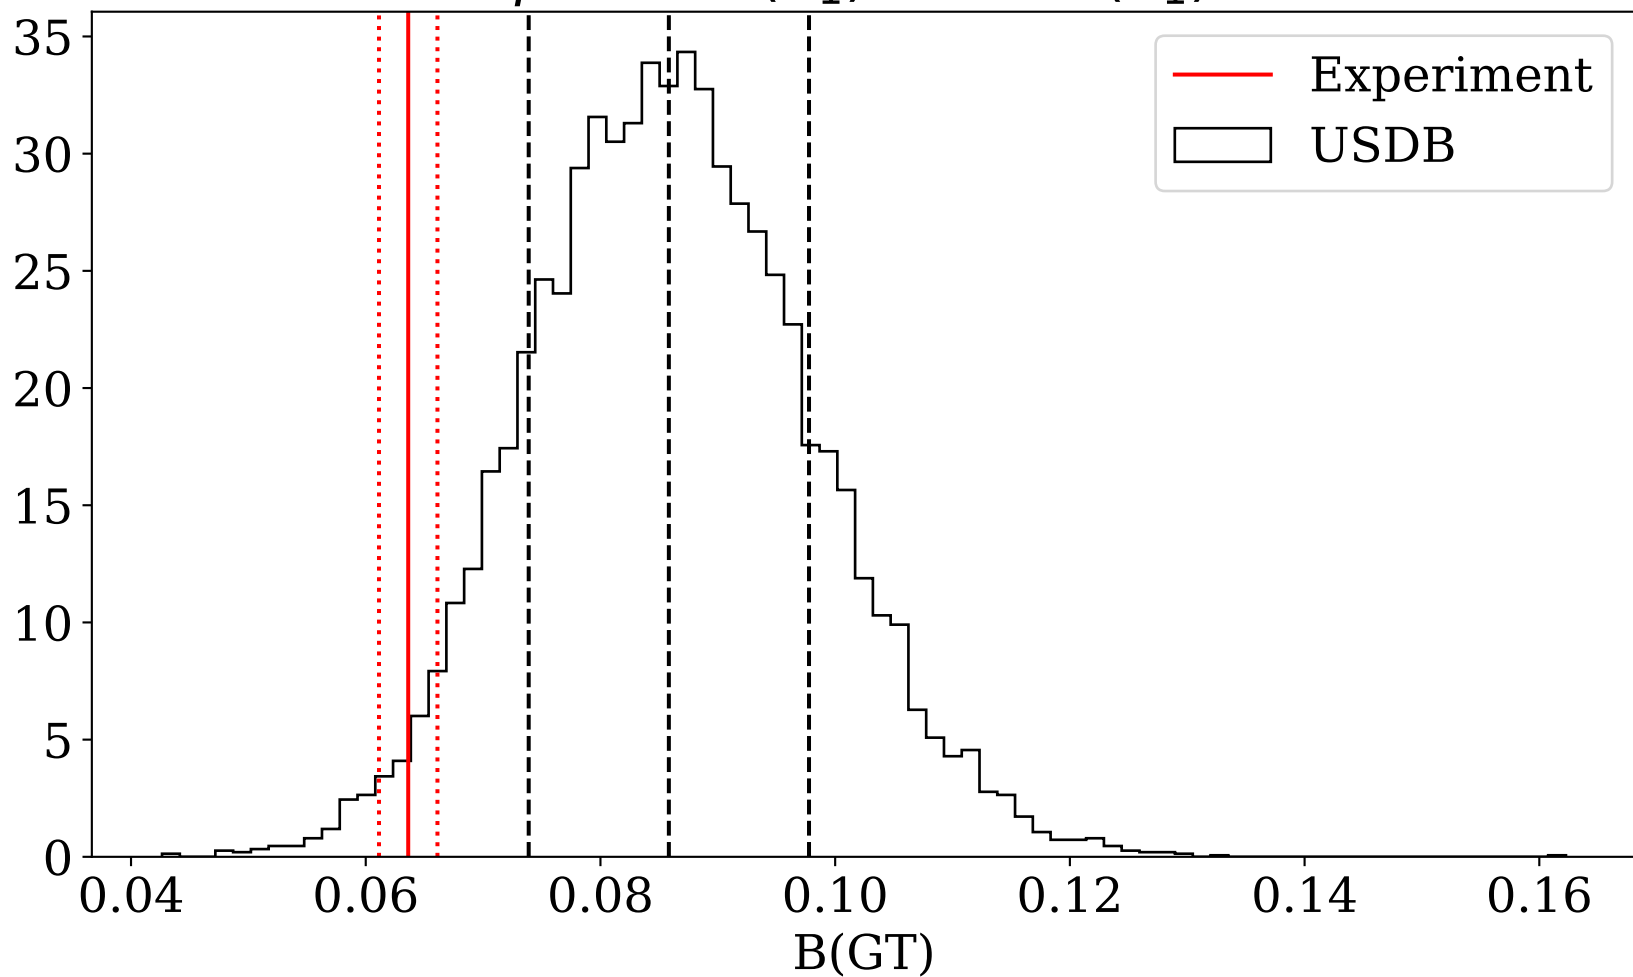

$\beta^- : {}^{30}\text{Al}(3_1) \rightarrow {}^{30}\text{Si}(3_2)$

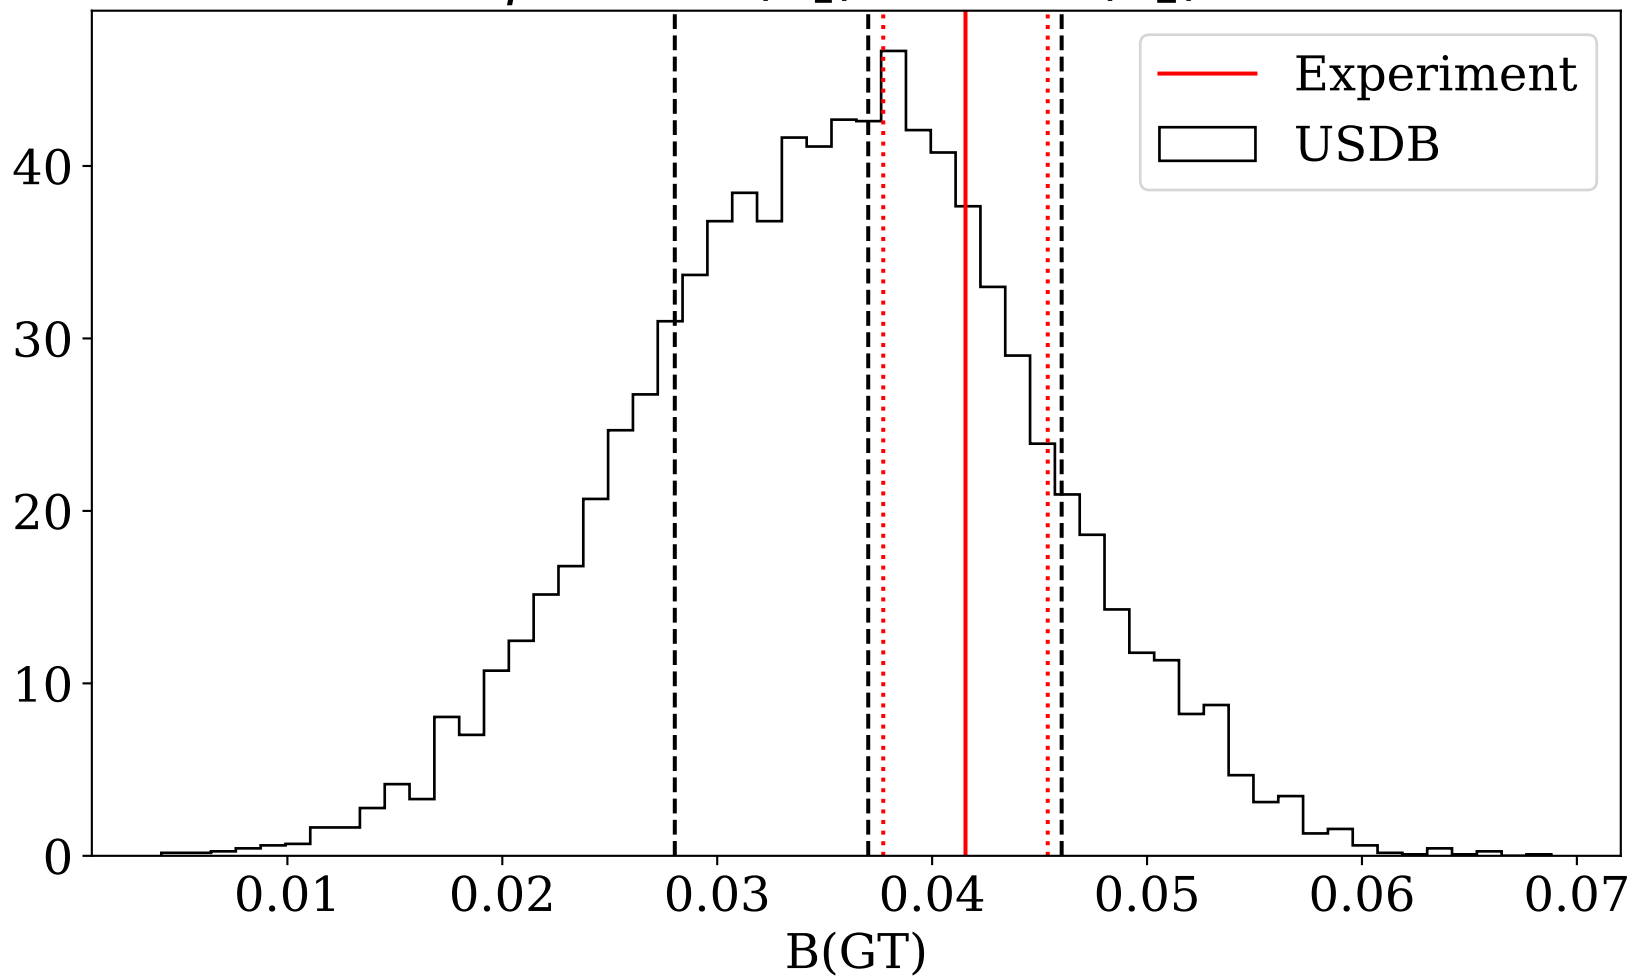

$\beta^- : {}^{31}\text{Si}(3/2_1) \rightarrow {}^{31}\text{P}(1/2_1)$

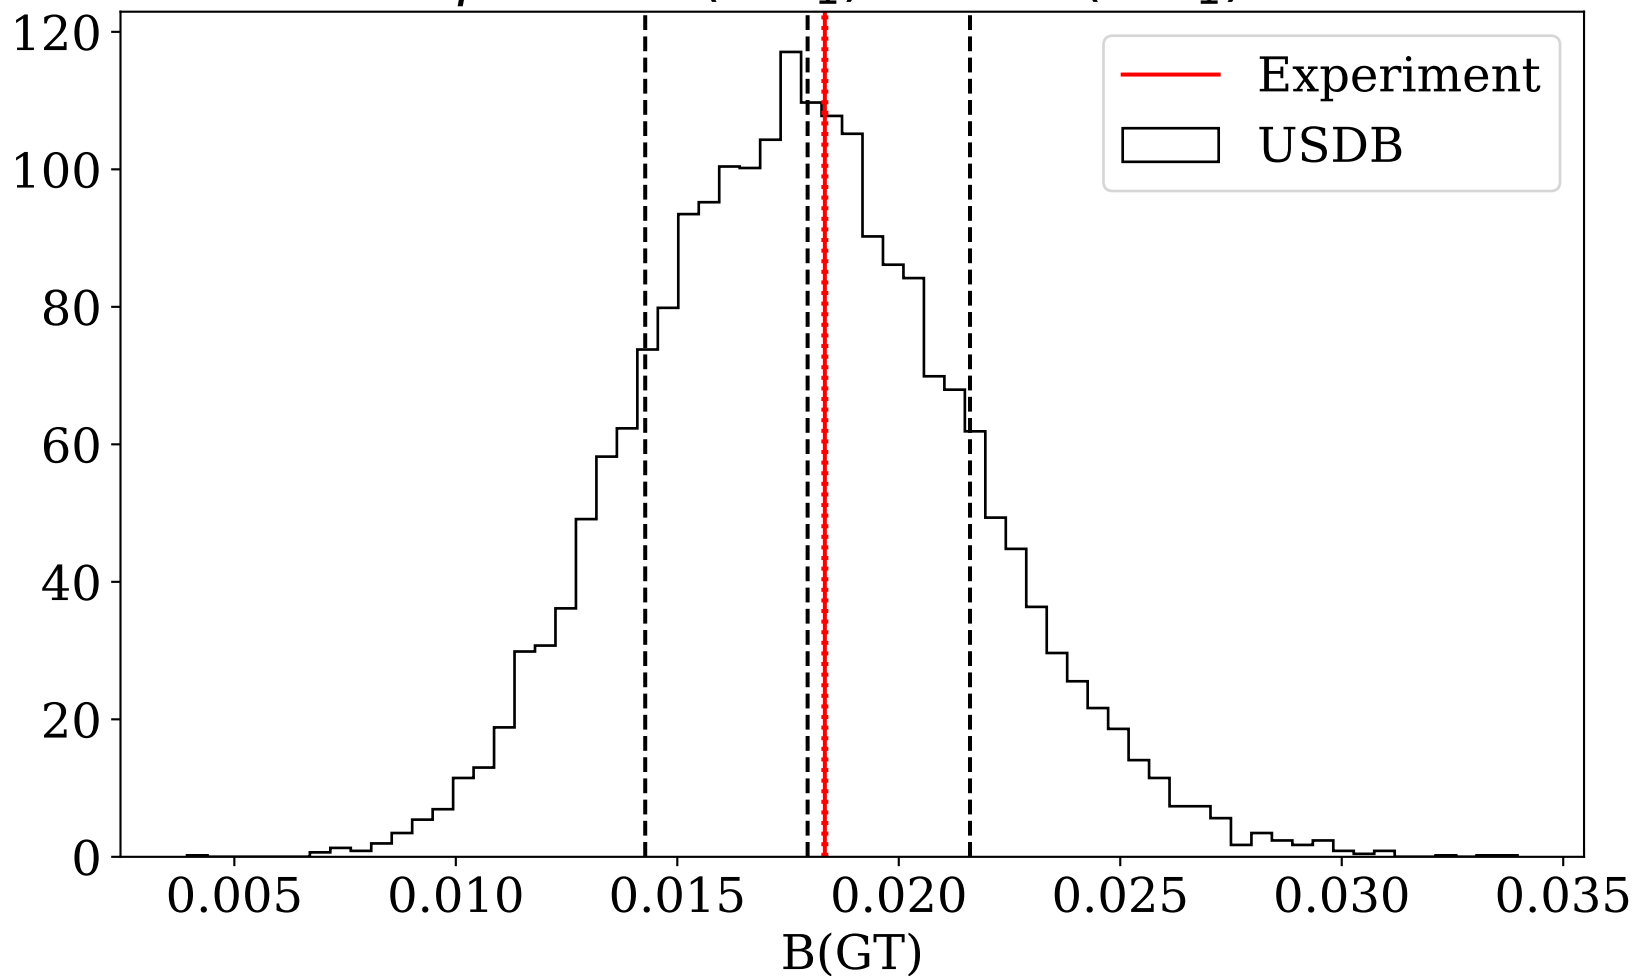

$\beta^- : {}^{31}\text{Si}(3/2_1) \rightarrow {}^{31}\text{P}(3/2_1)$

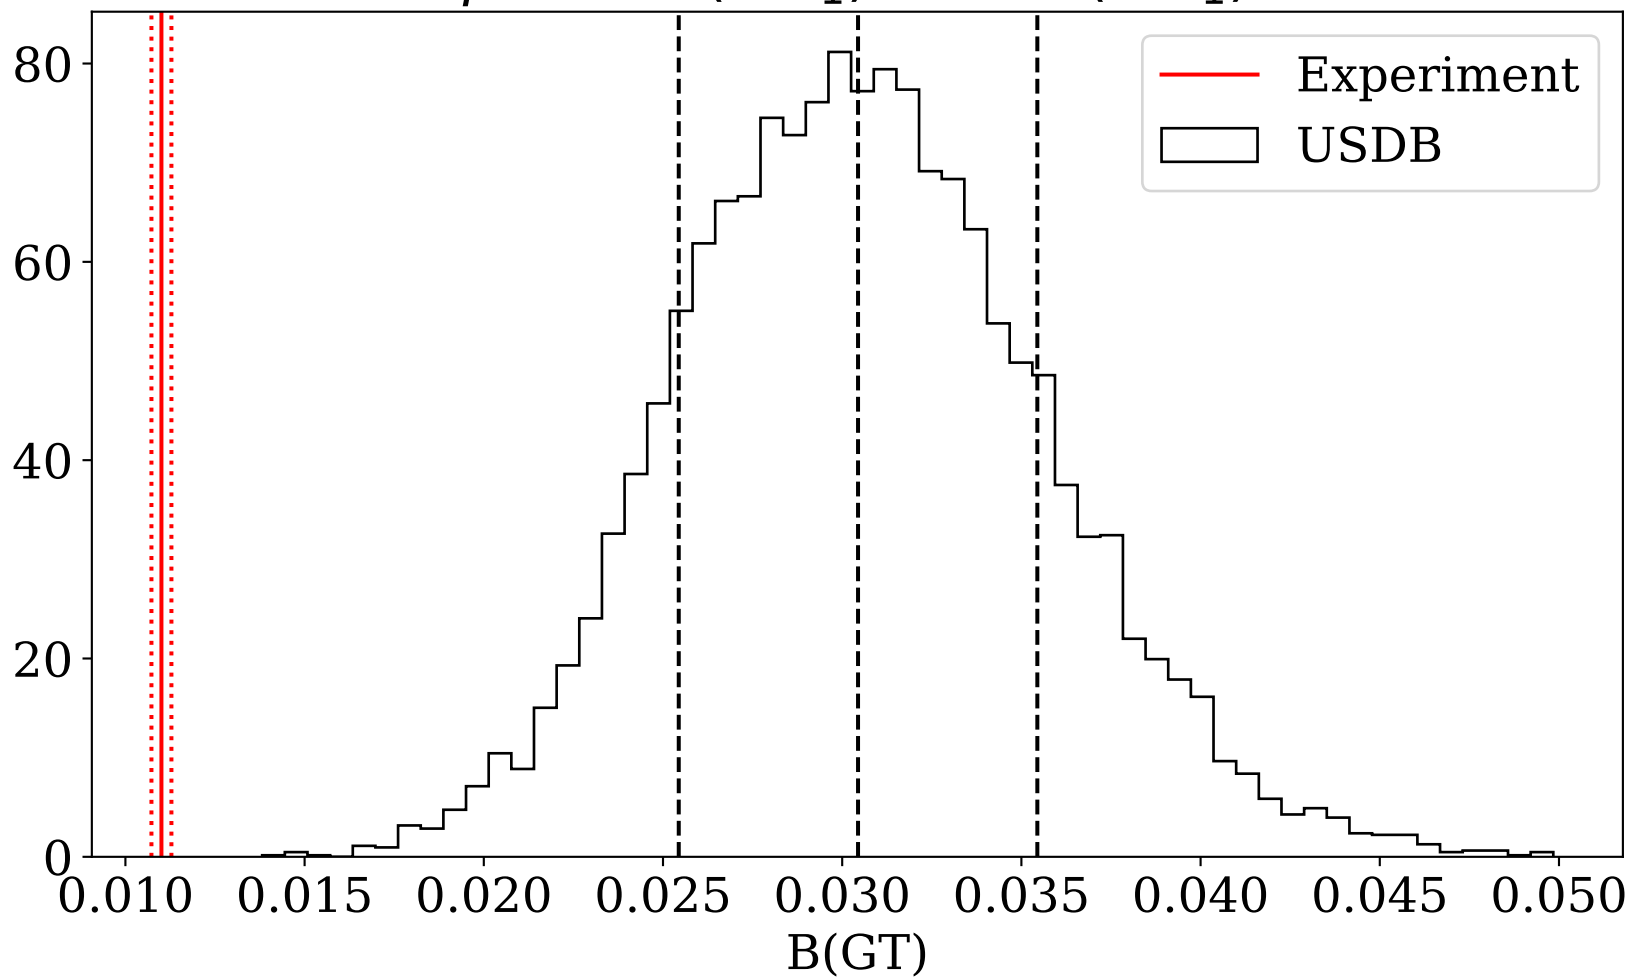

$\beta^- : {}^{33}\text{P}(1/2_1) \rightarrow {}^{33}\text{S}(3/2_1)$

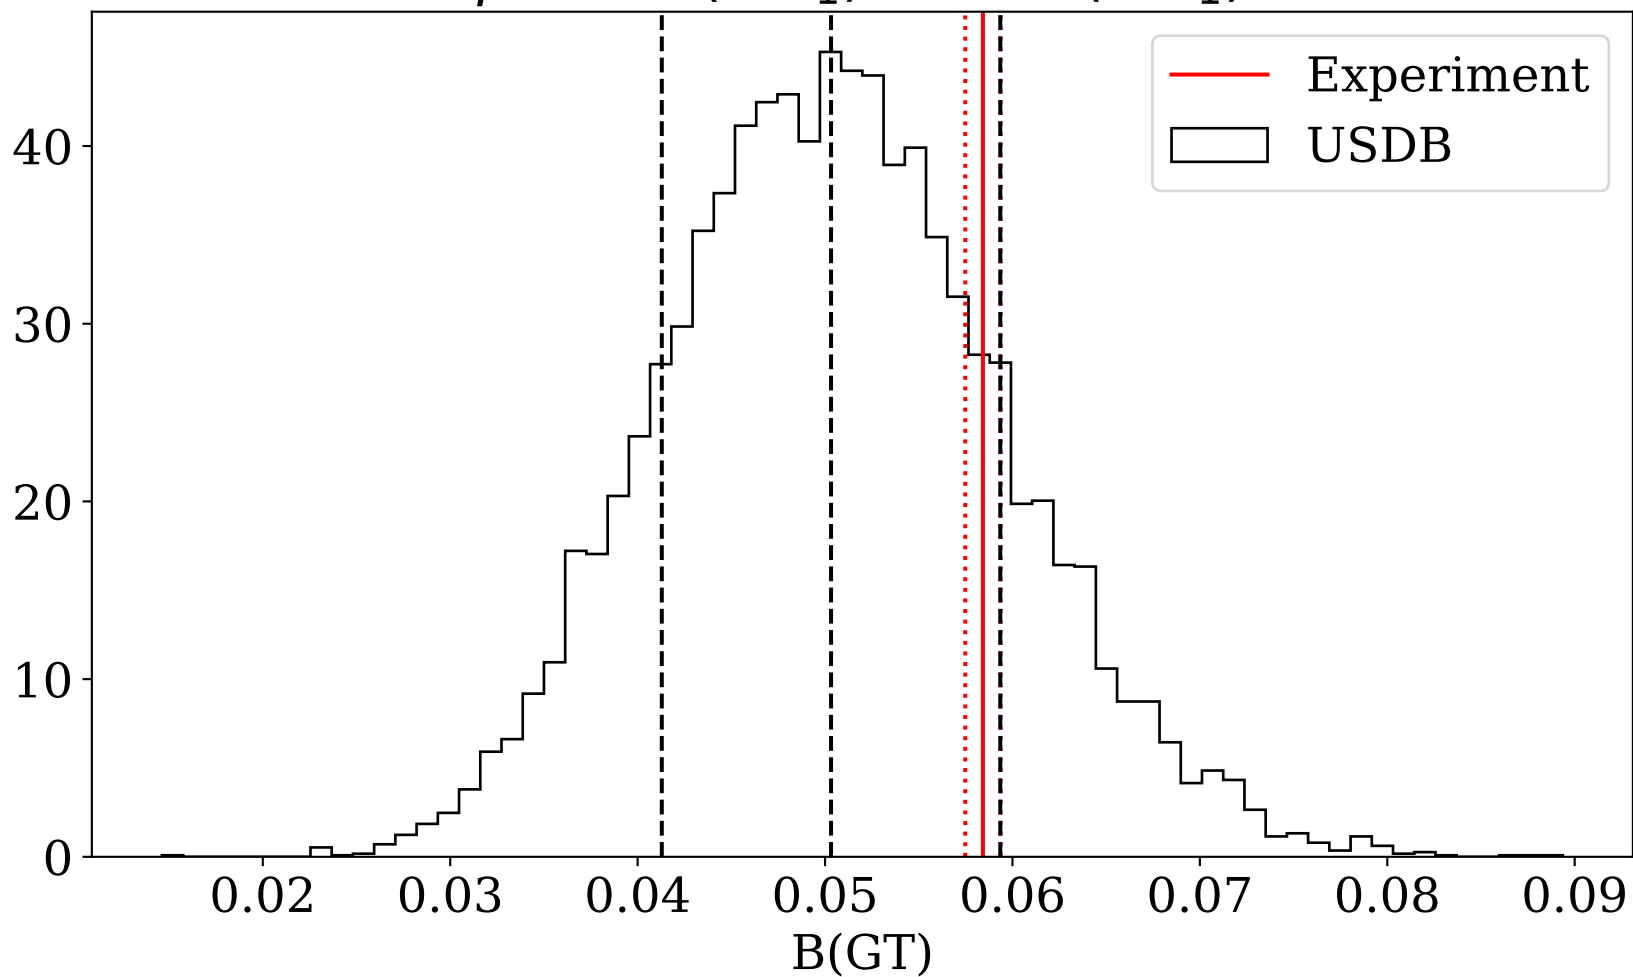

$\beta^- : {}^{34}\text{P}(1_1) \rightarrow {}^{34}\text{S}(0_1)$

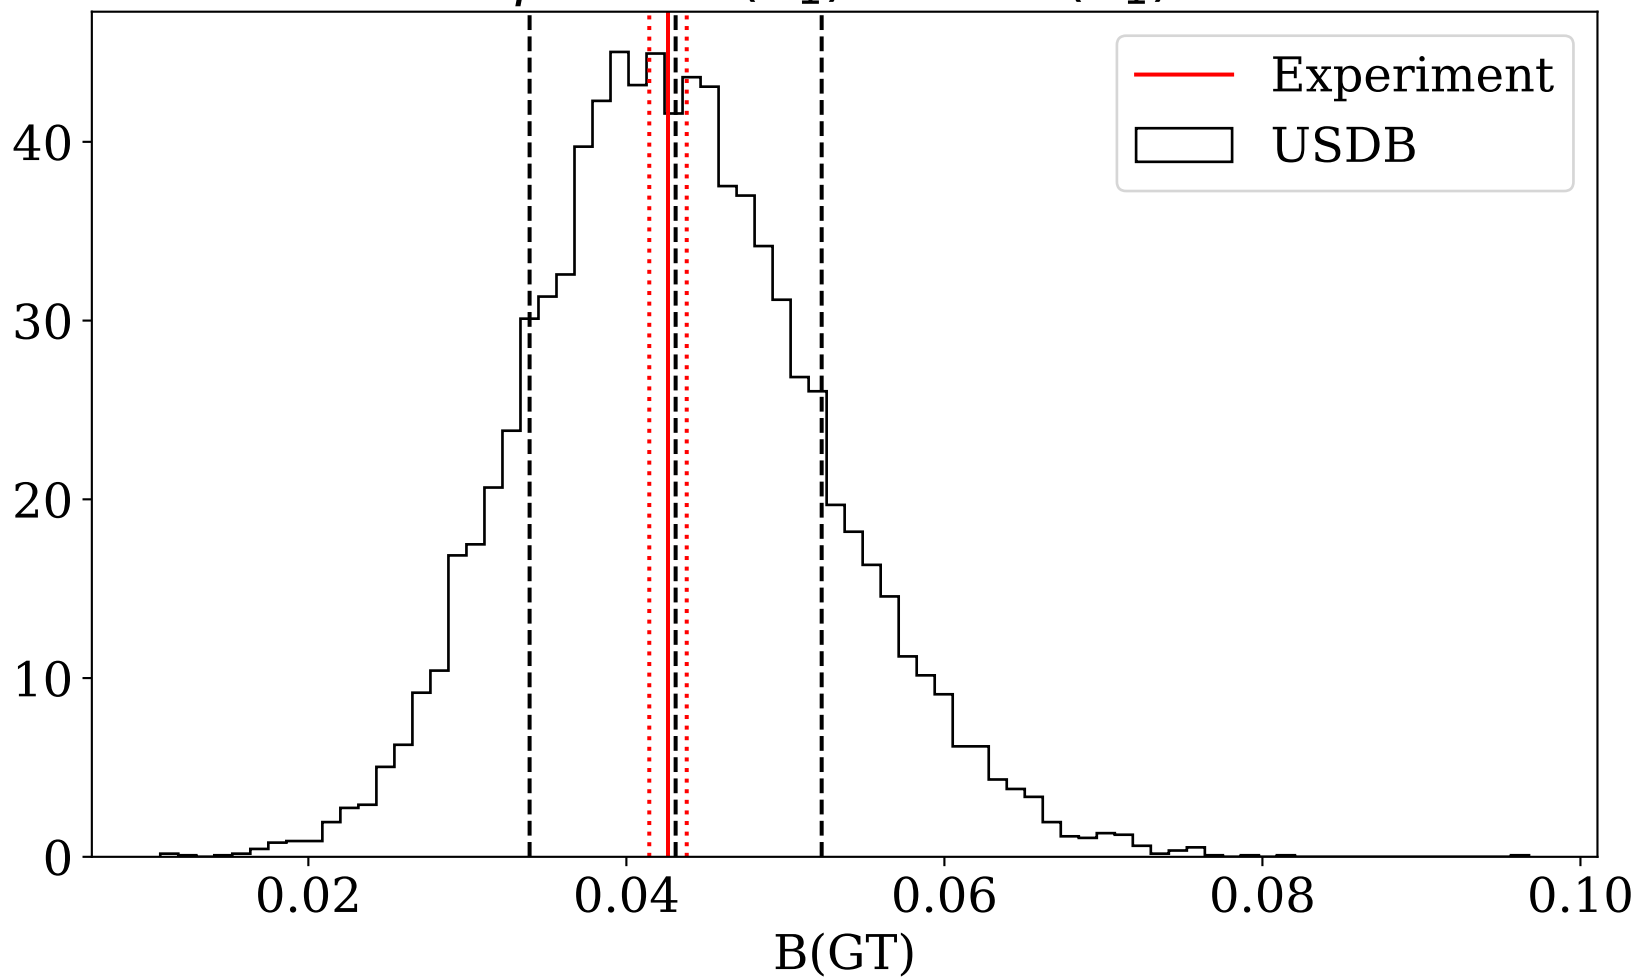

$$\beta^- : {}^{34}\text{P}(1_1) \rightarrow {}^{34}\text{S}(2_1)$$

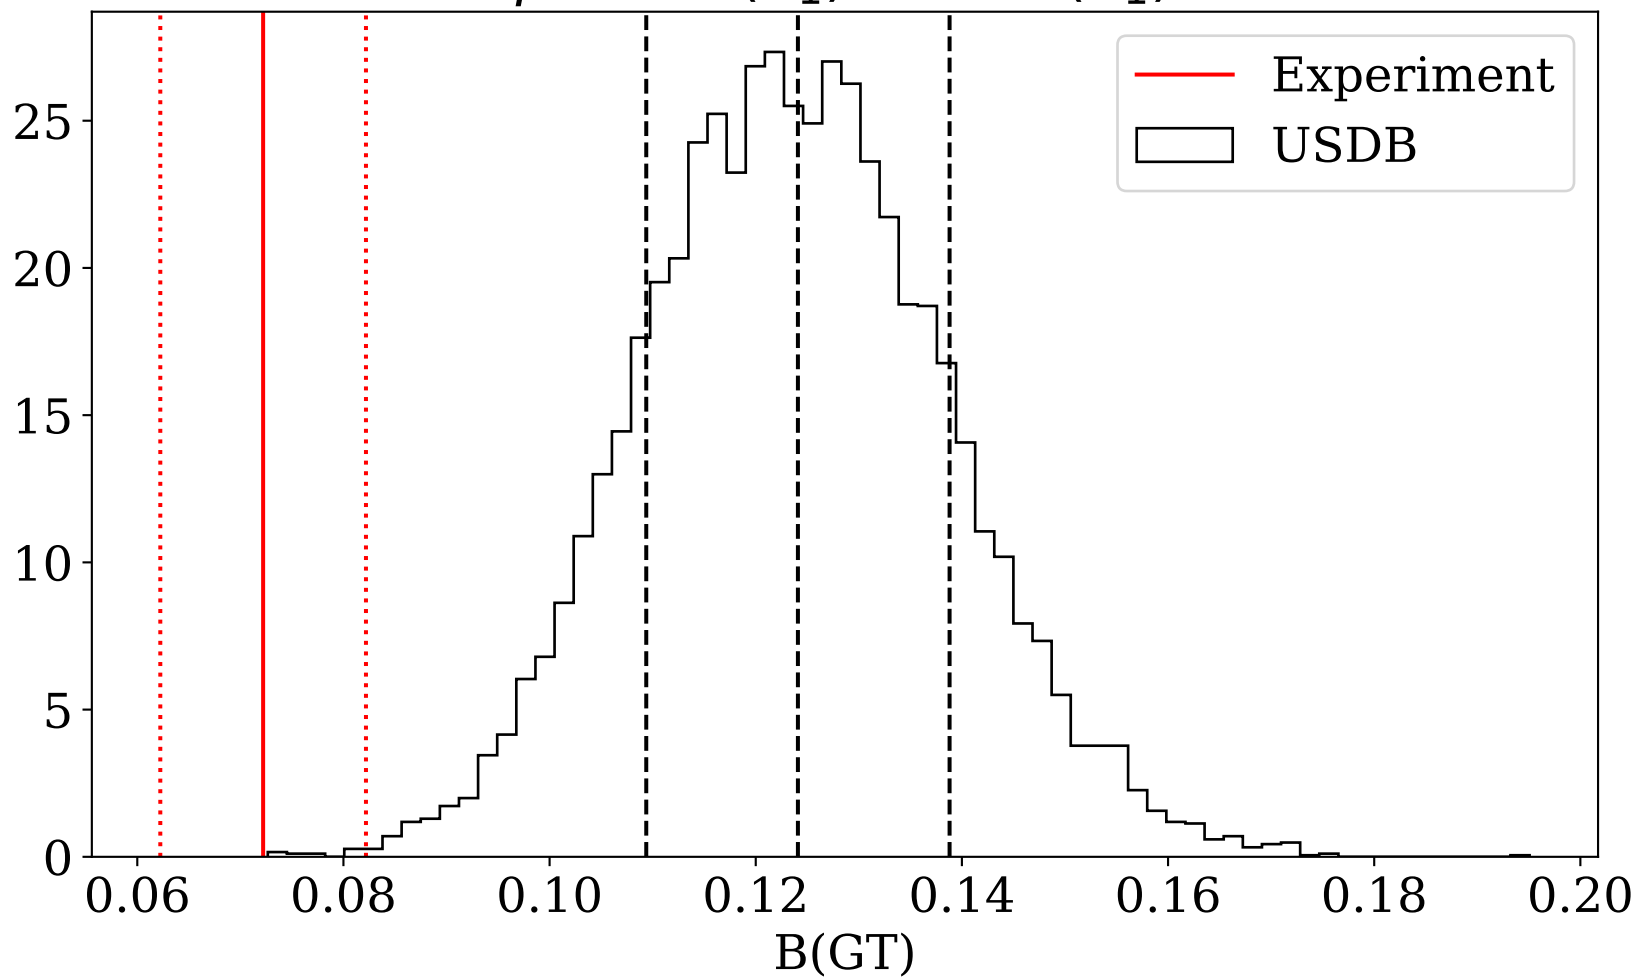



$\beta^- : {}^{34}\text{P}(1_1) \rightarrow {}^{34}\text{S}(0_2)$

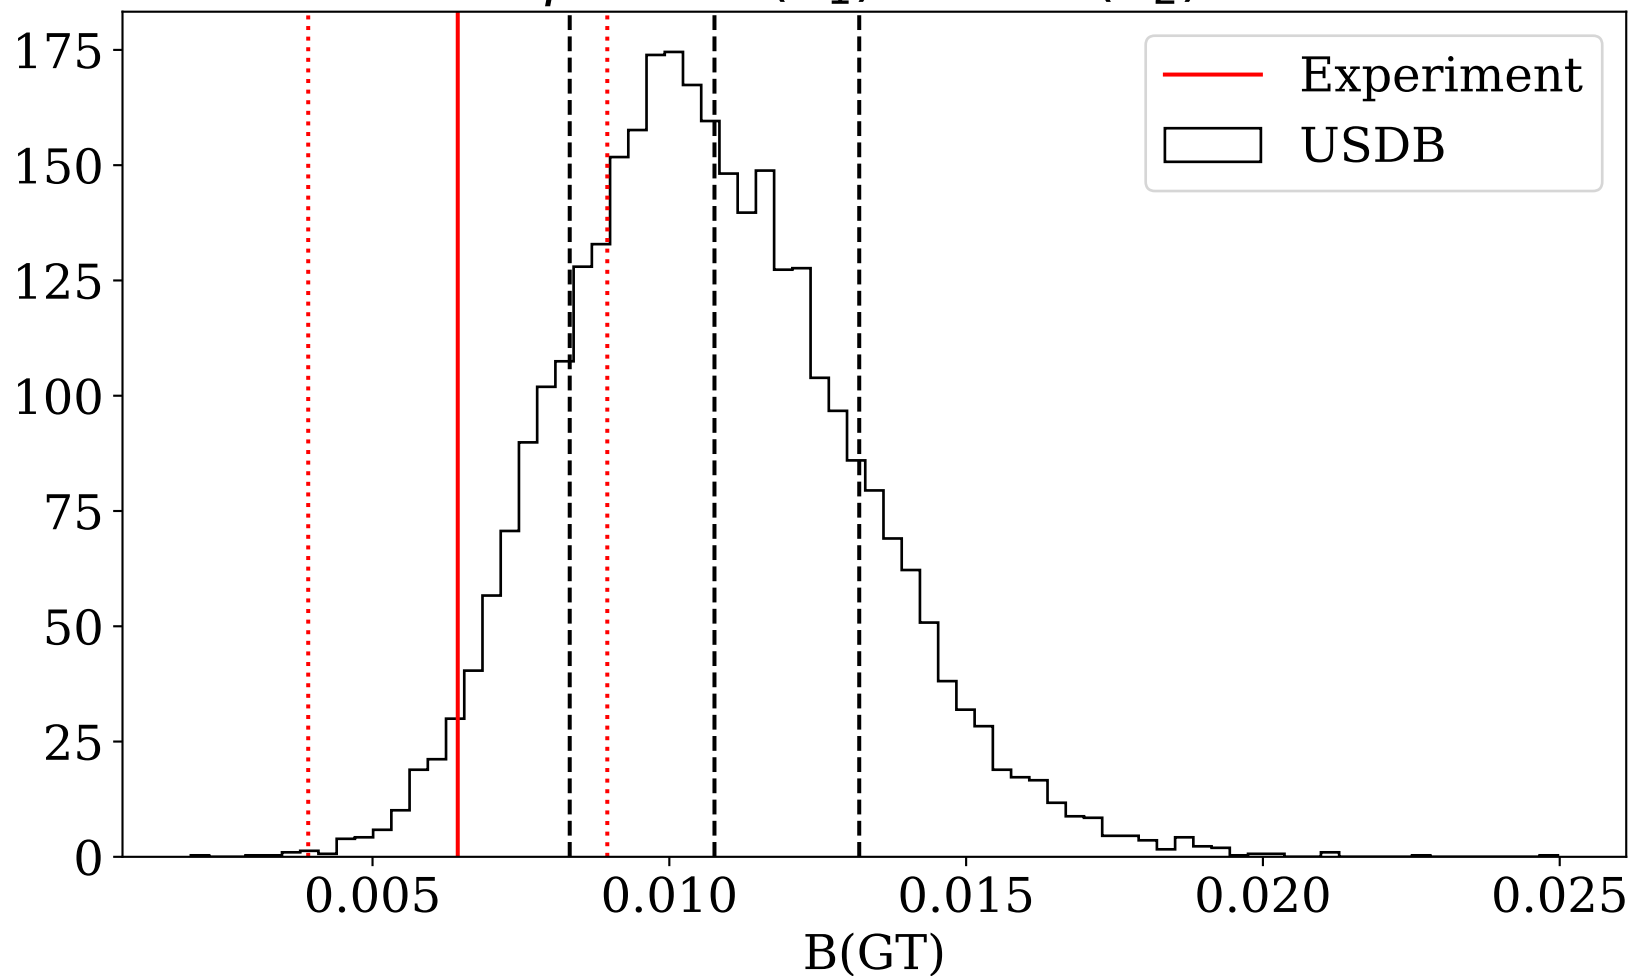

$\beta^- : {}^{34}\text{P}(1_1) \rightarrow {}^{34}\text{S}(1_1)$

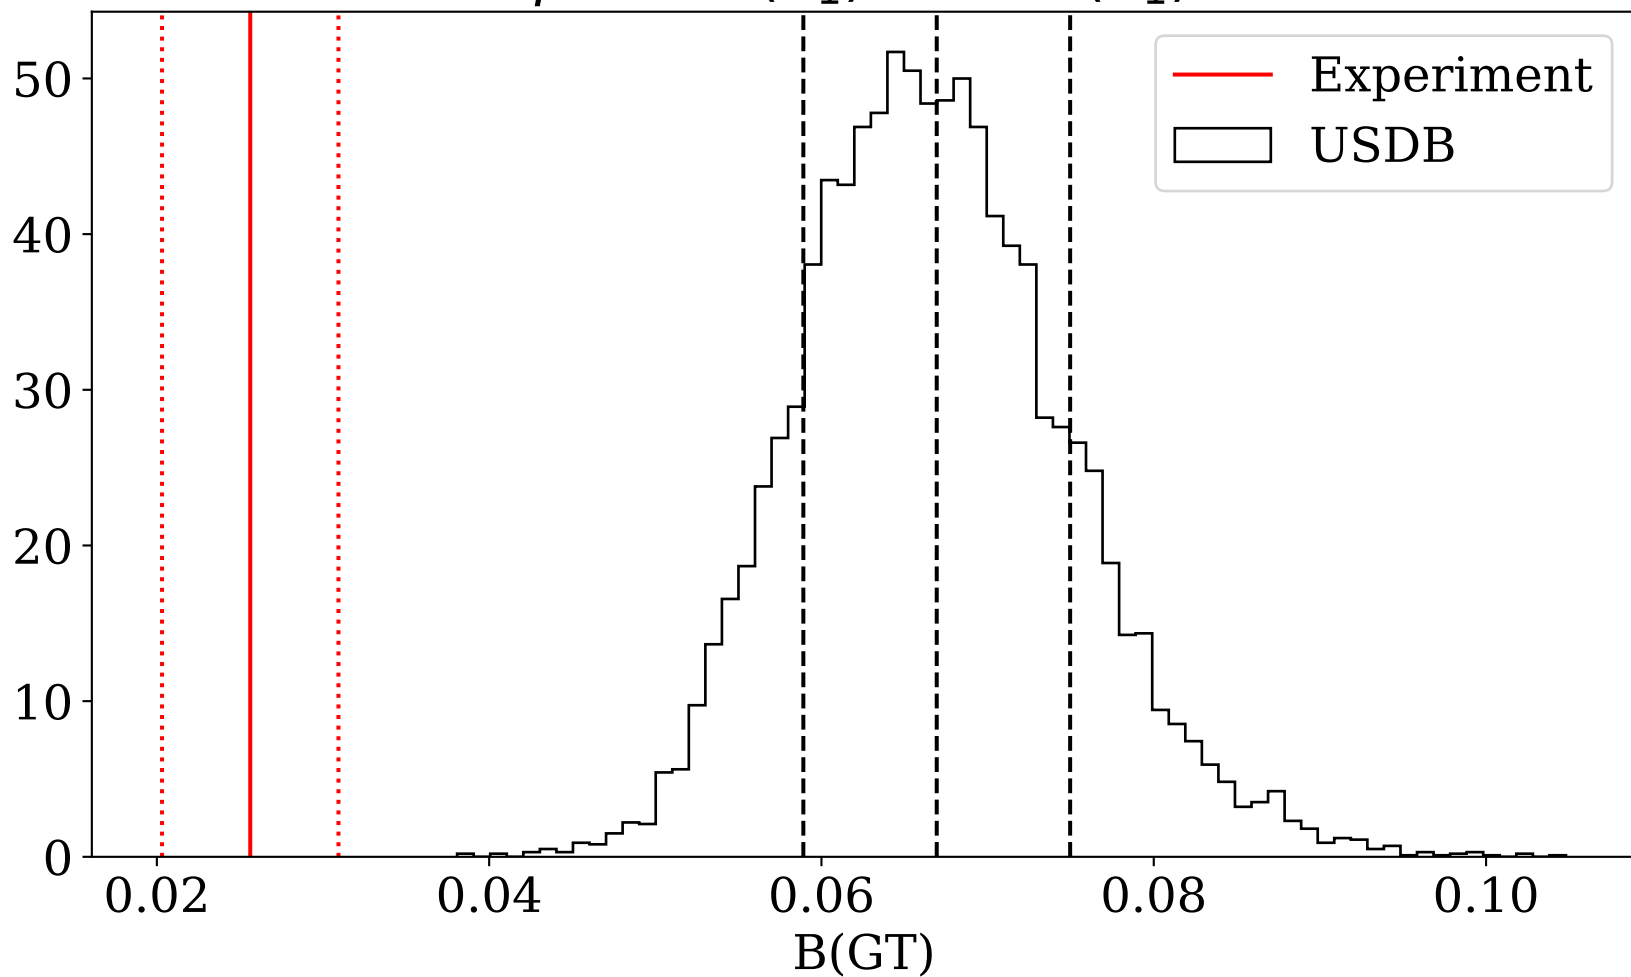

$\beta^- : {}^{34}\text{P}(1_1) \rightarrow {}^{34}\text{S}(2_2)$

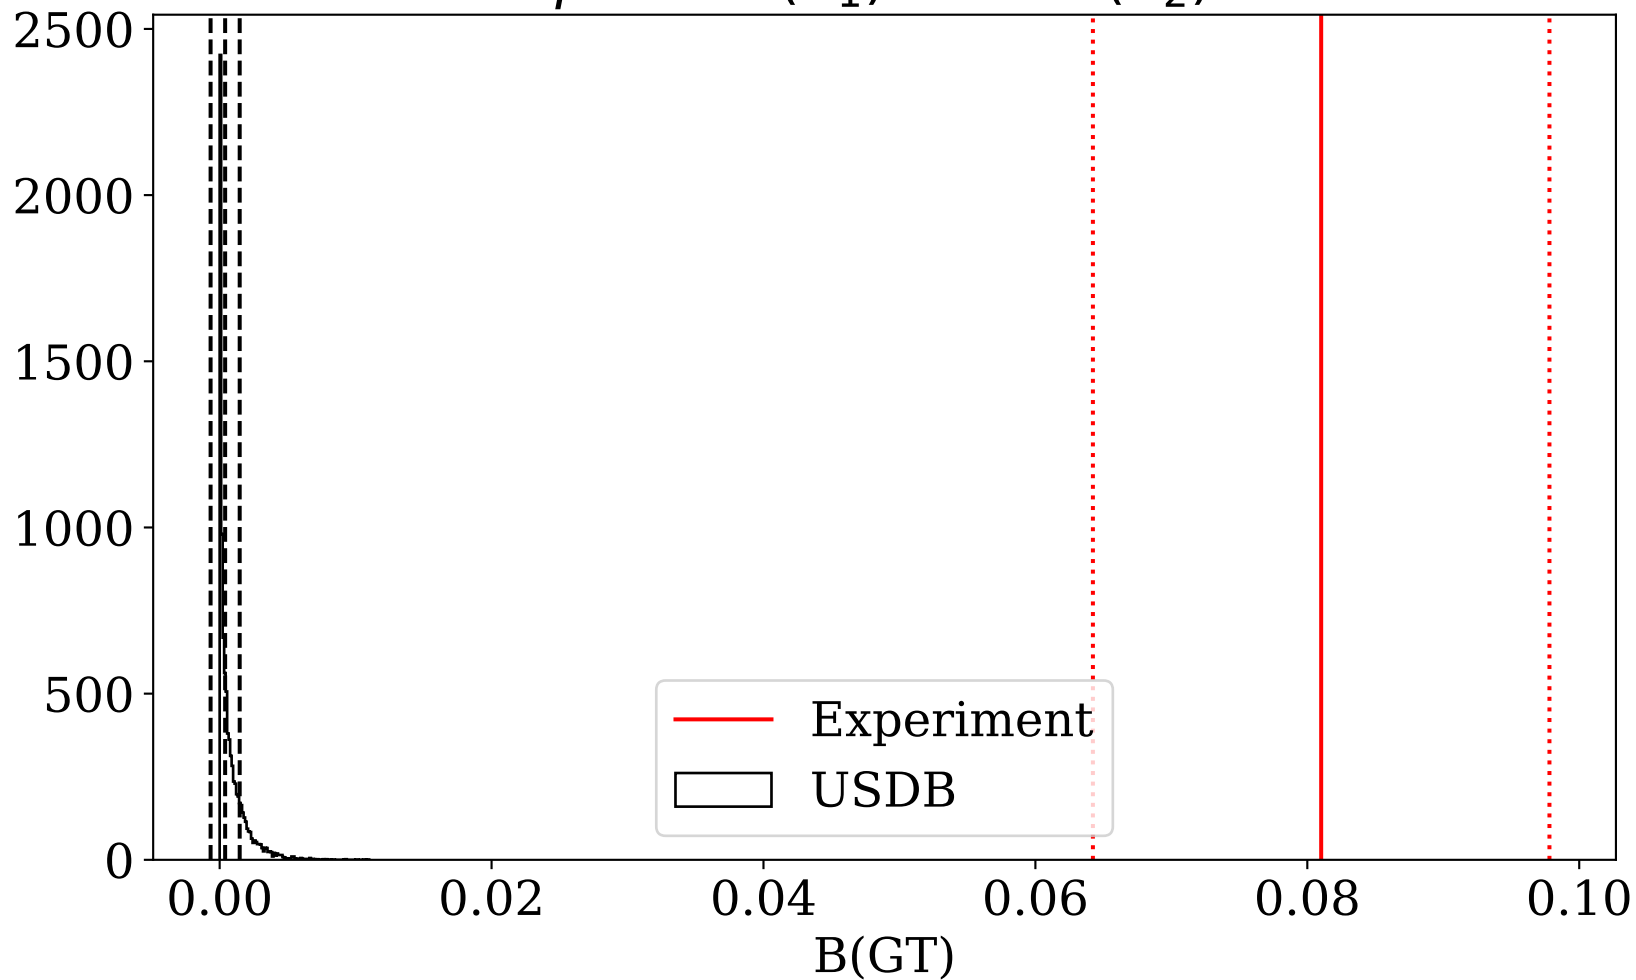

$\beta^- : {}^{35}\text{S}(3/2_1) \rightarrow {}^{35}\text{Cl}(3/2_1)$

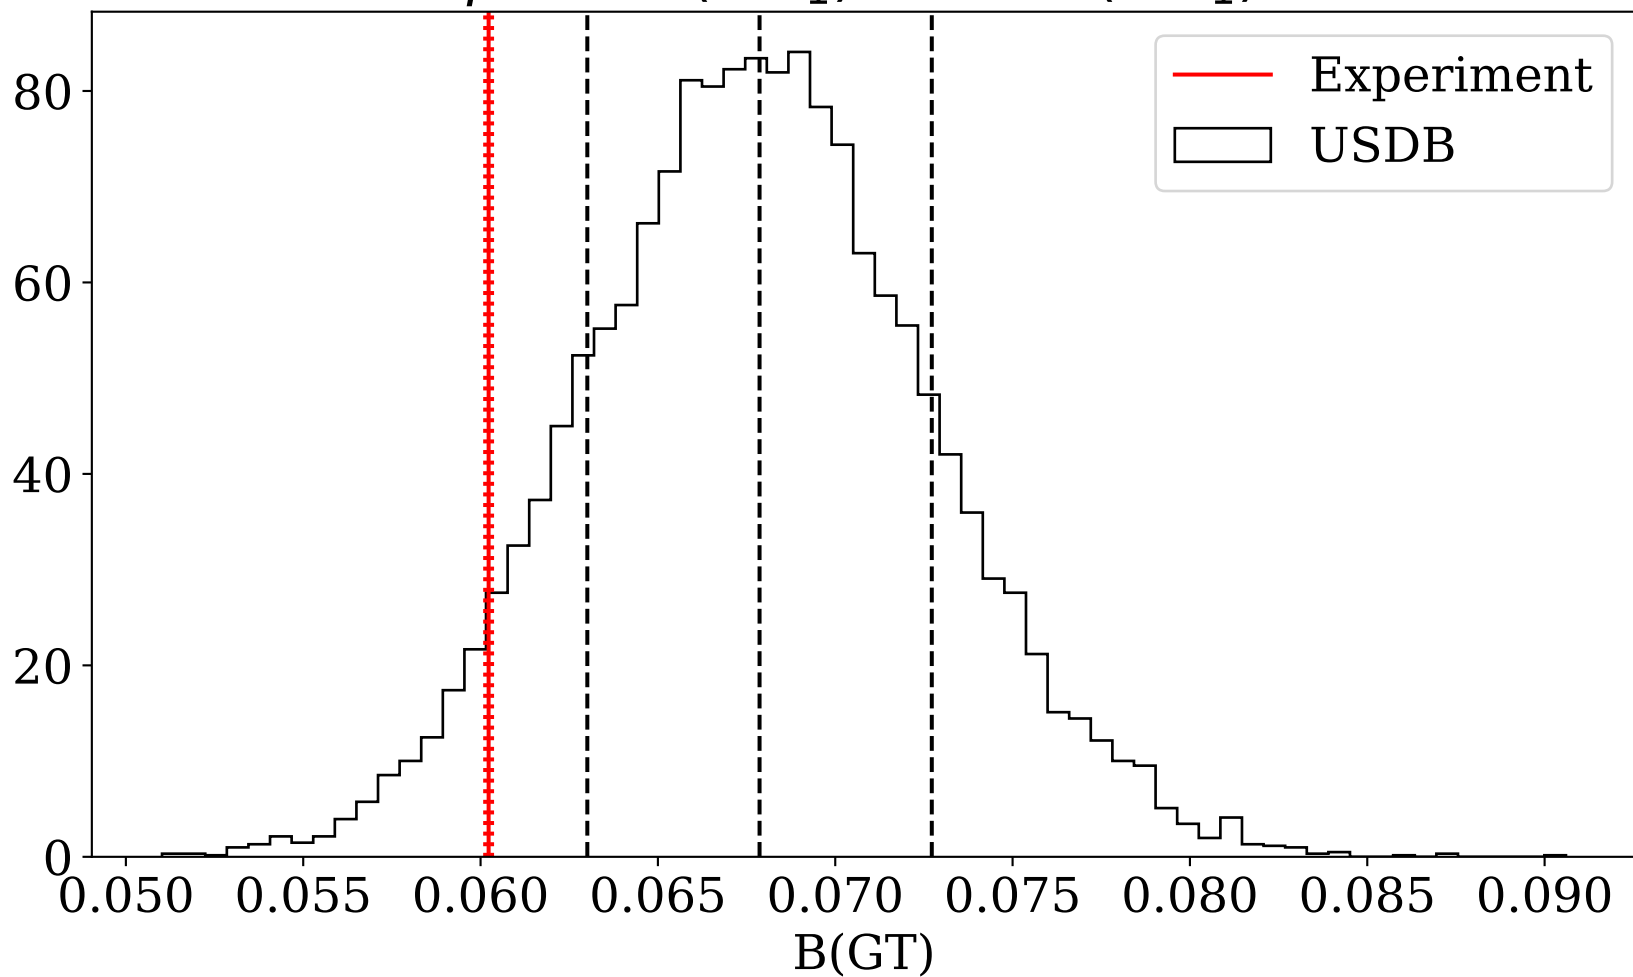

e. c. :  $^{19}\text{Ne}(1/2_1) \rightarrow ^{19}\text{F}(1/2_1)$

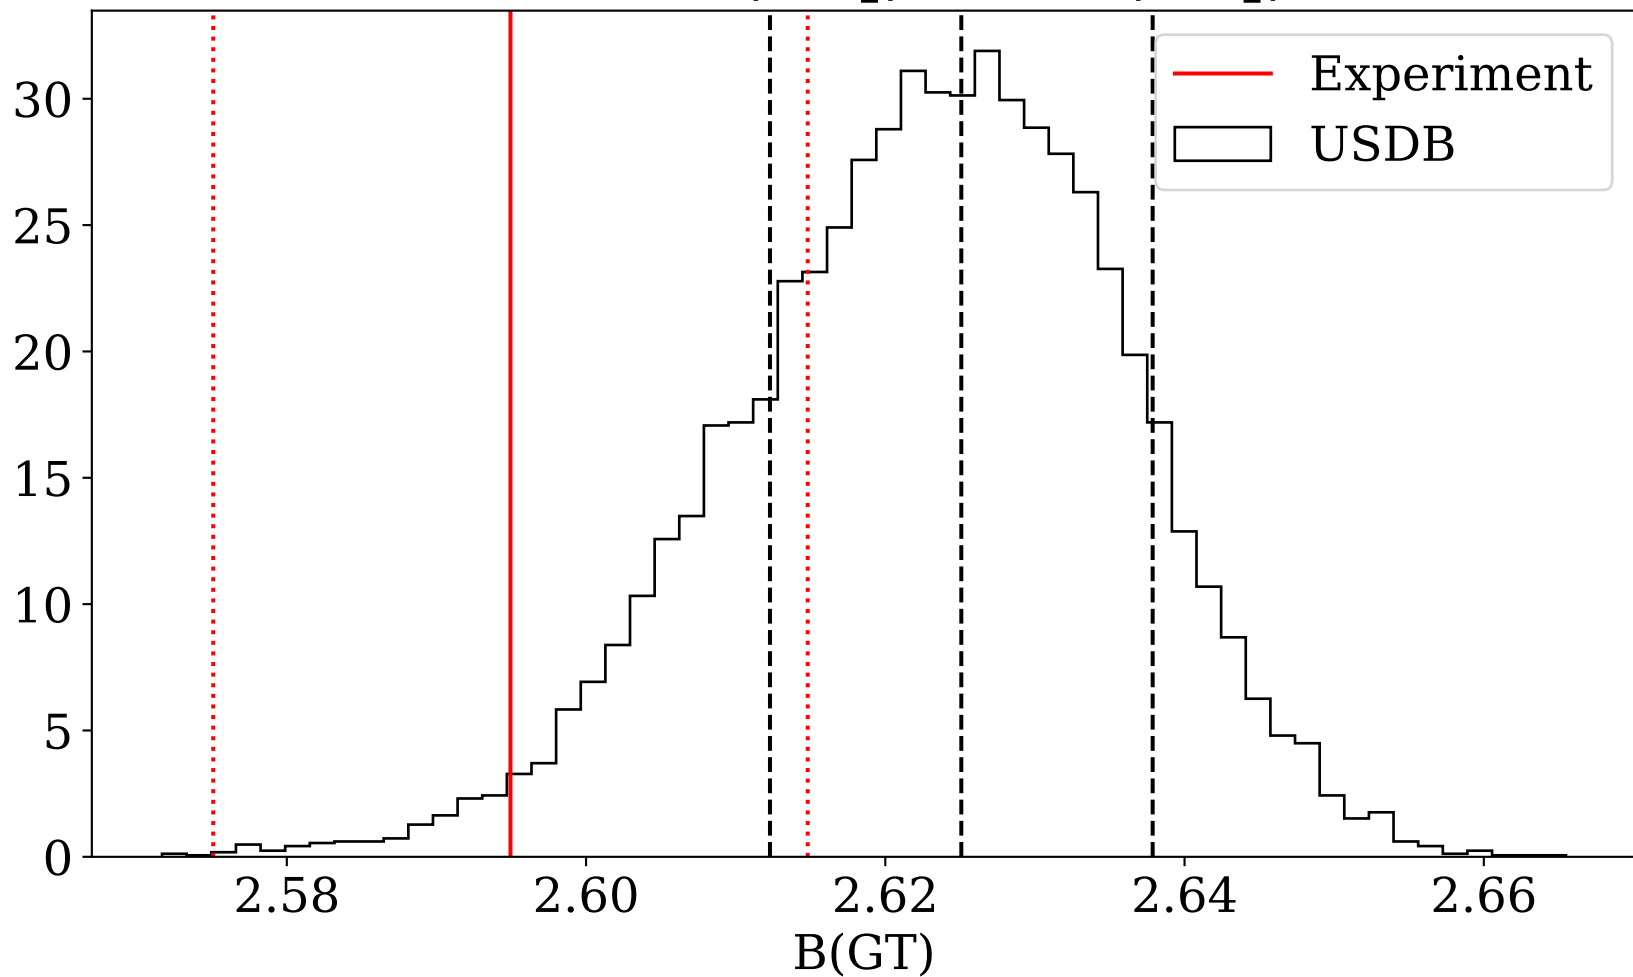

*e. c.* :  $^{19}\text{Ne}(1/2_1) \rightarrow ^{19}\text{F}(3/2_1)$

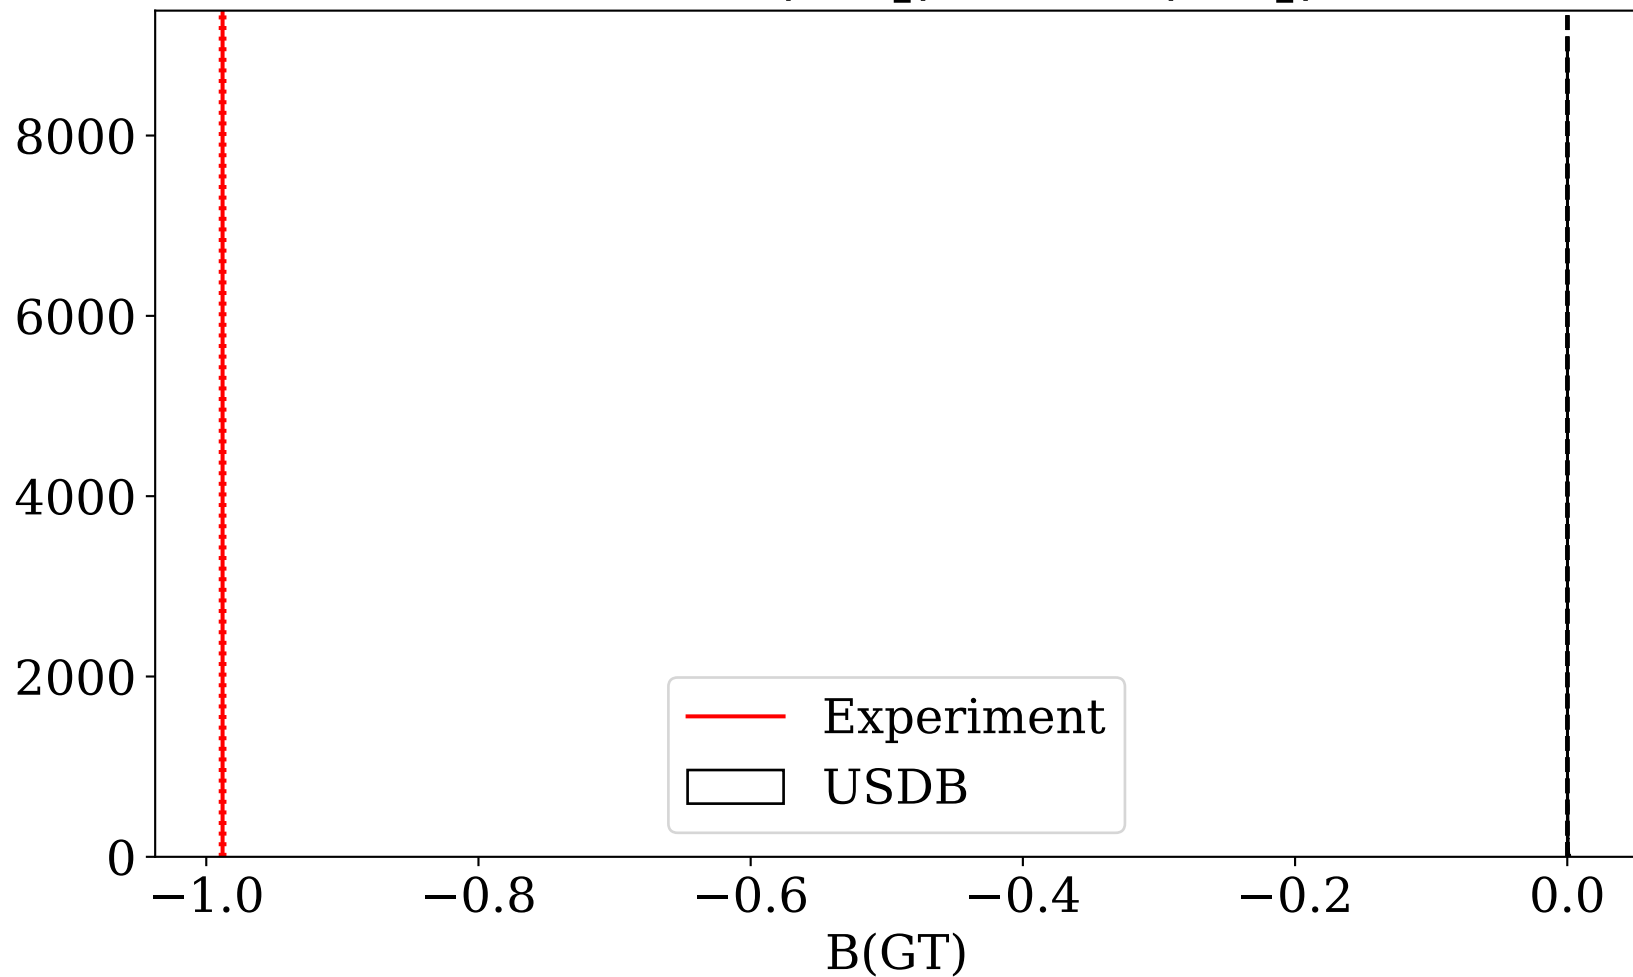

e. c. :  $^{20}\text{Na}(2_1) \rightarrow ^{20}\text{Ne}(2_1)$

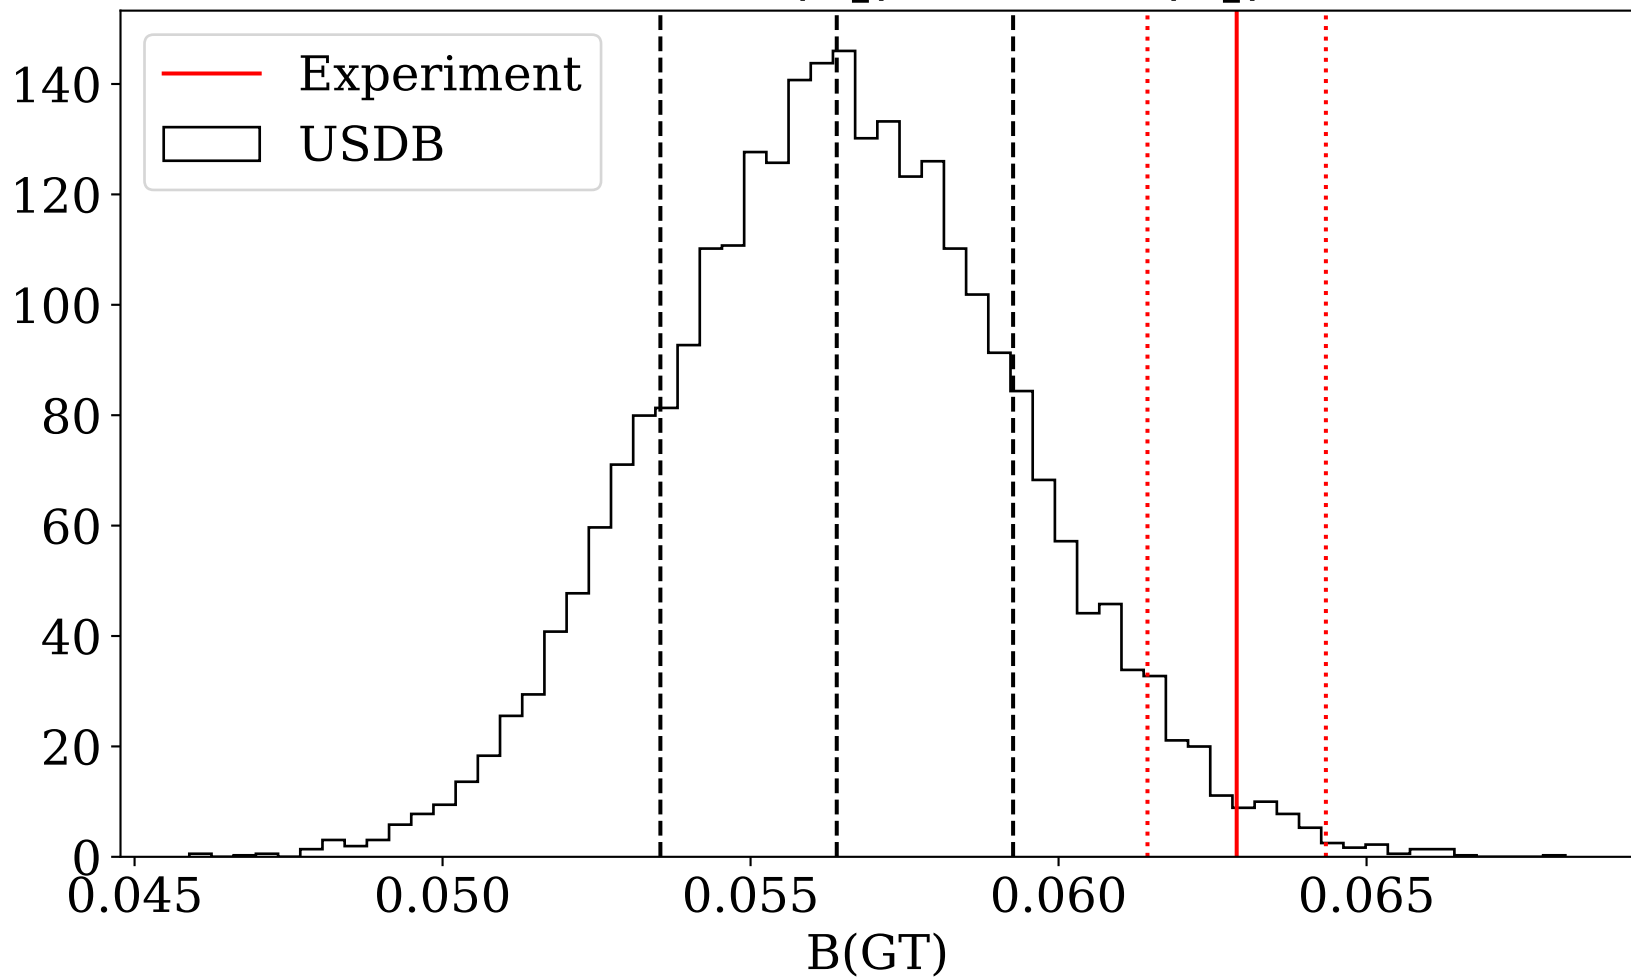

e. c. :  $^{20}\text{Na}(2_1) \rightarrow ^{20}\text{Ne}(2_2)$

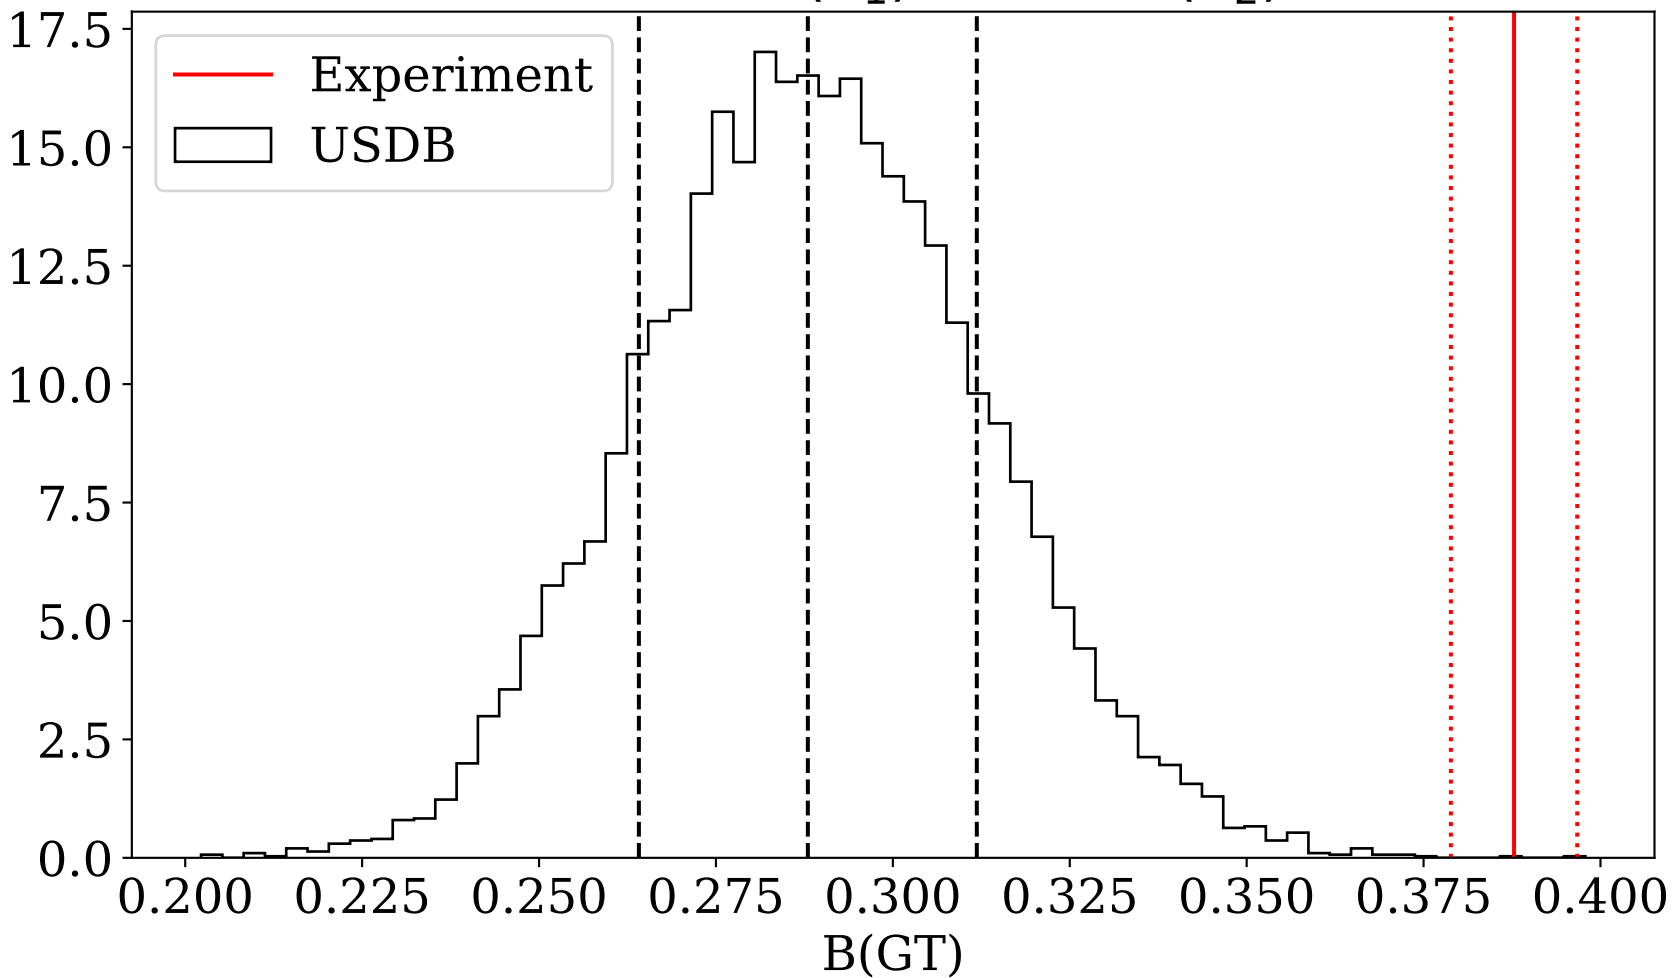



e. c. :  $^{20}\text{Na}(2_1) \rightarrow ^{20}\text{Ne}(2_3)$

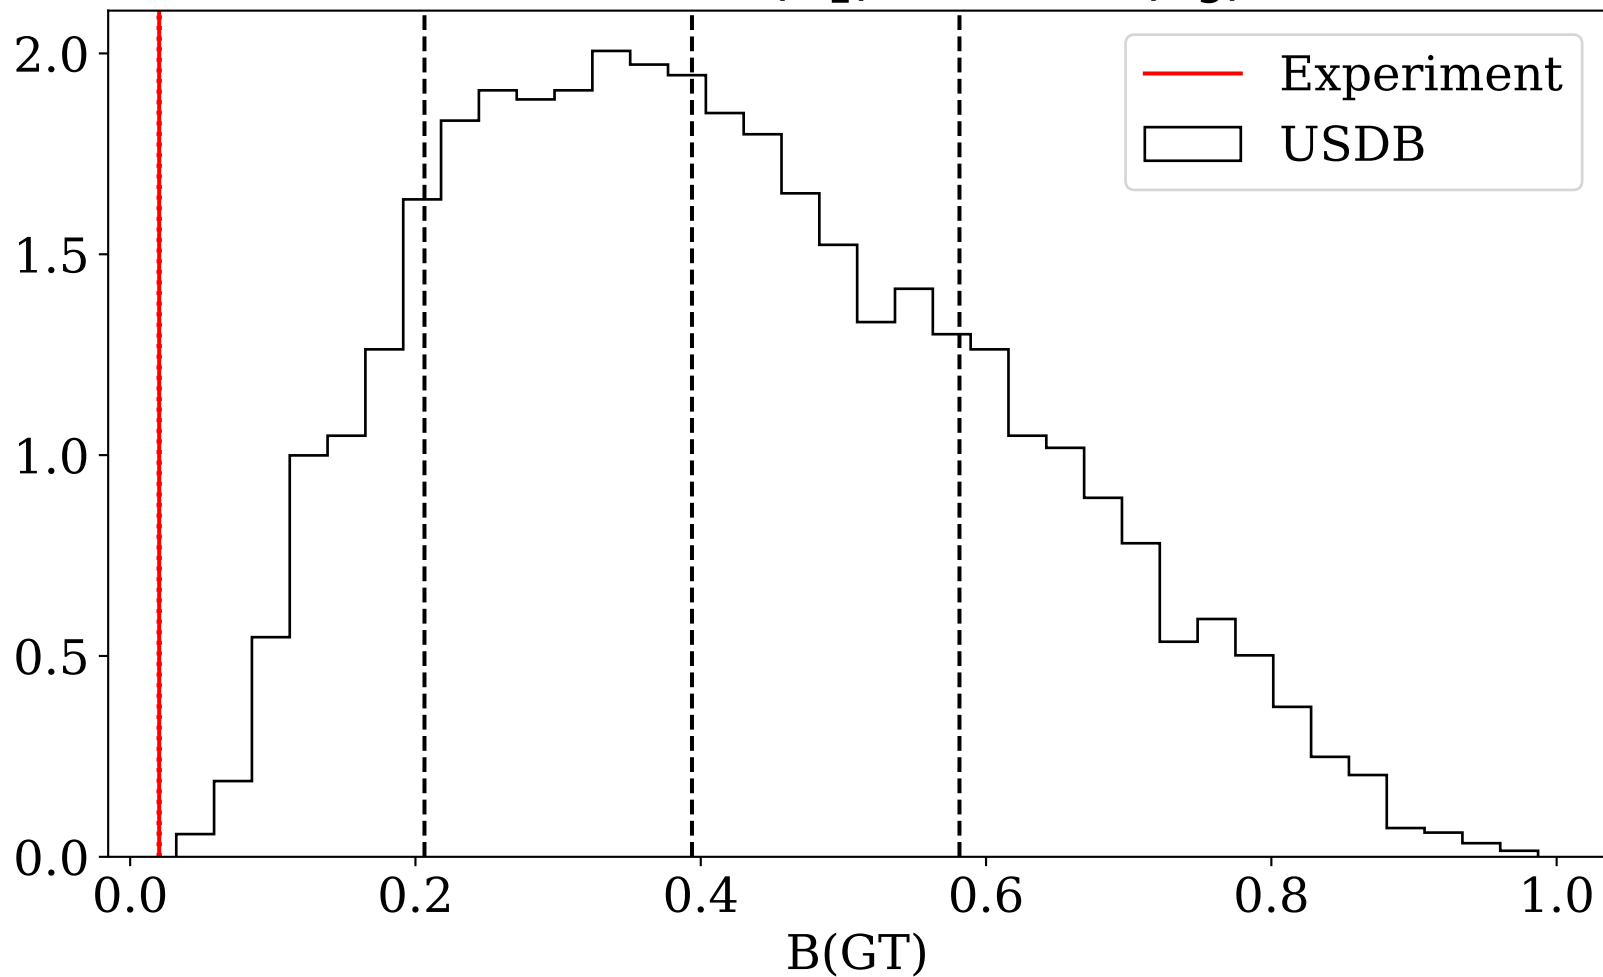

e. c. :  $^{21}\text{Na}(3/2_1) \rightarrow ^{21}\text{Ne}(3/2_1)$

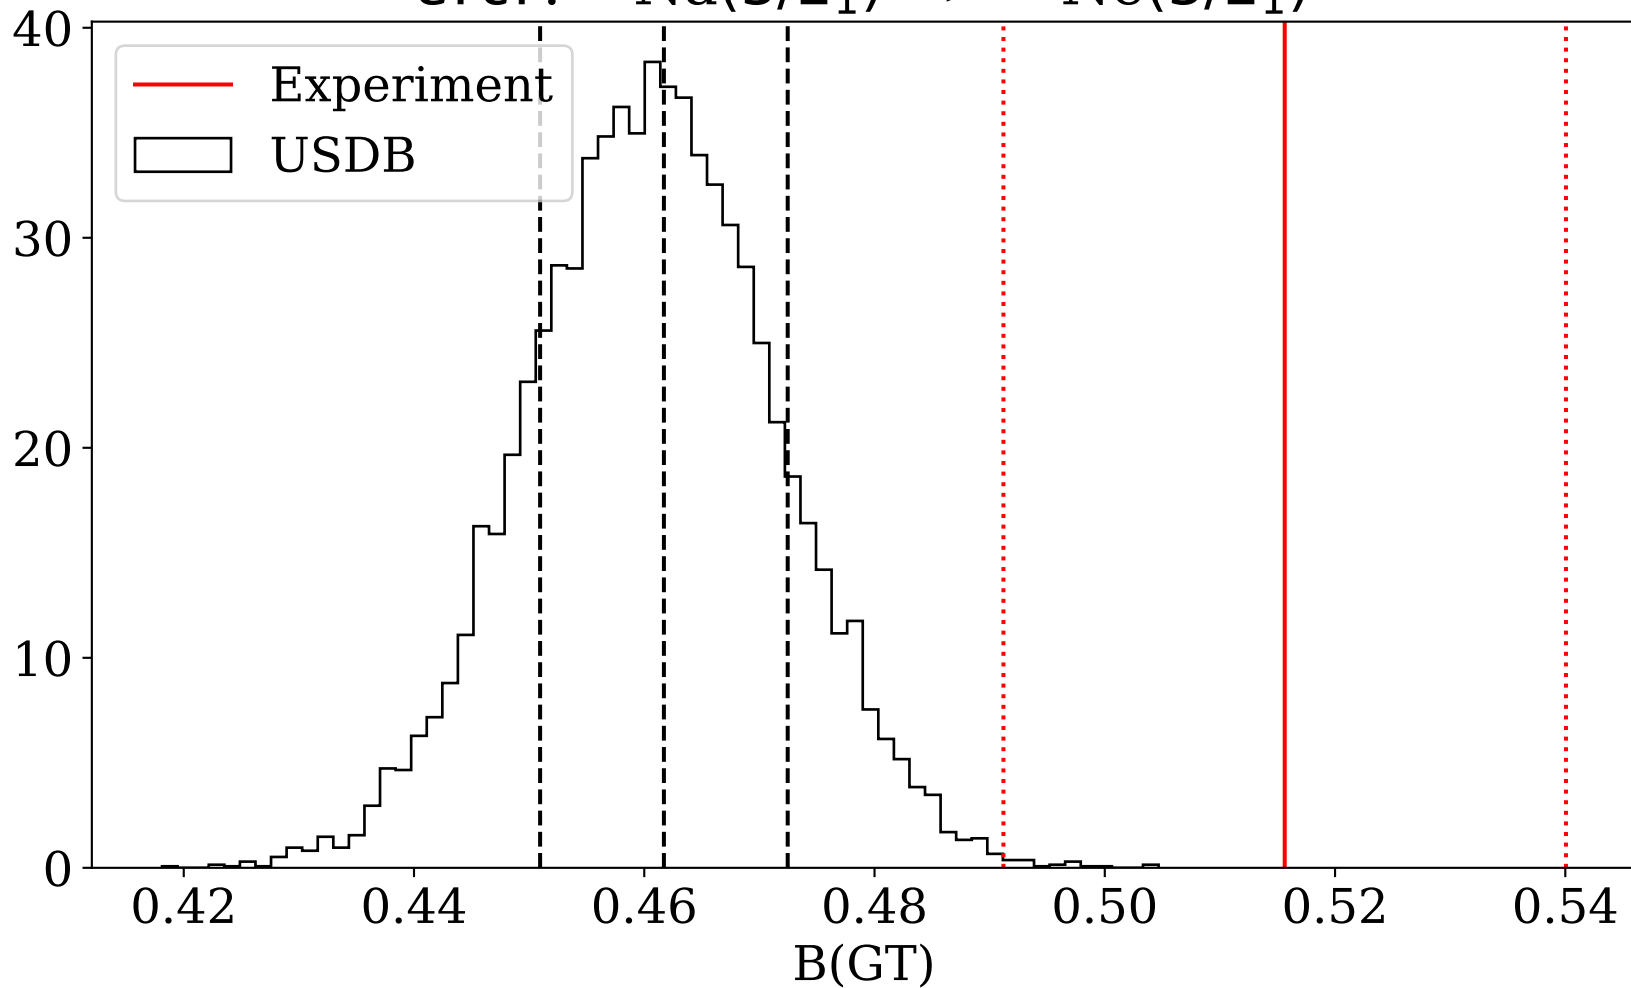

e. c. :  $^{21}\text{Na}(3/2_1) \rightarrow ^{21}\text{Ne}(5/2_1)$

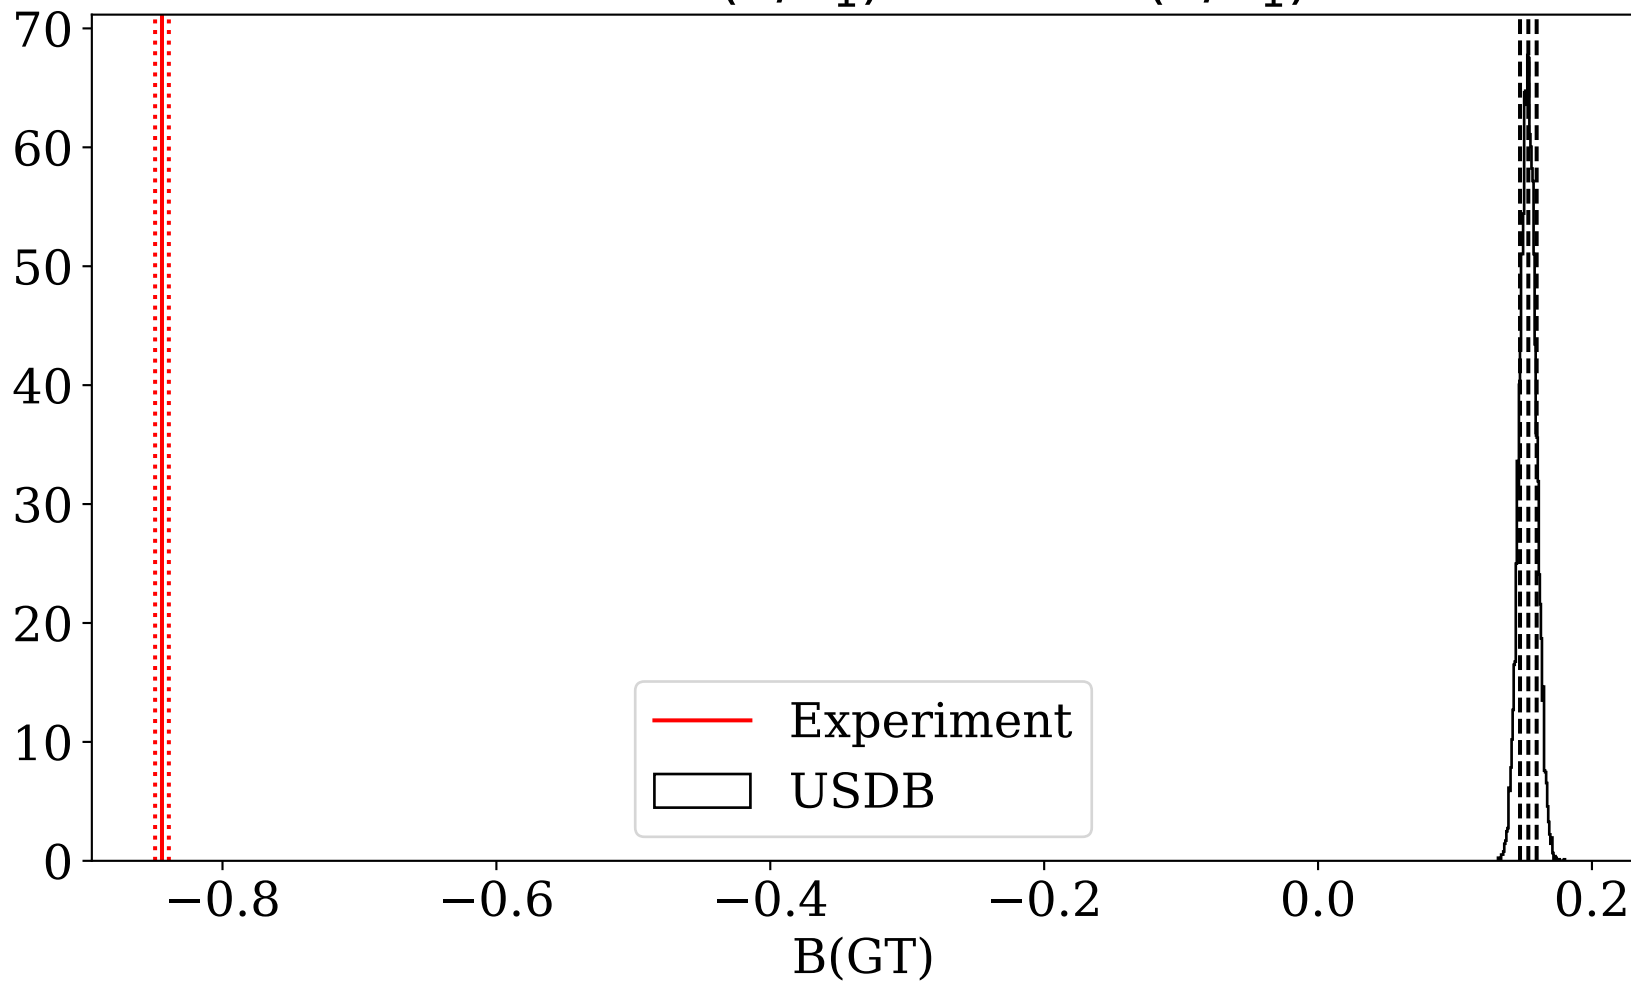

*e. c. :*  $^{22}\text{Mg}(0_1) \rightarrow ^{22}\text{Na}(1_1)$

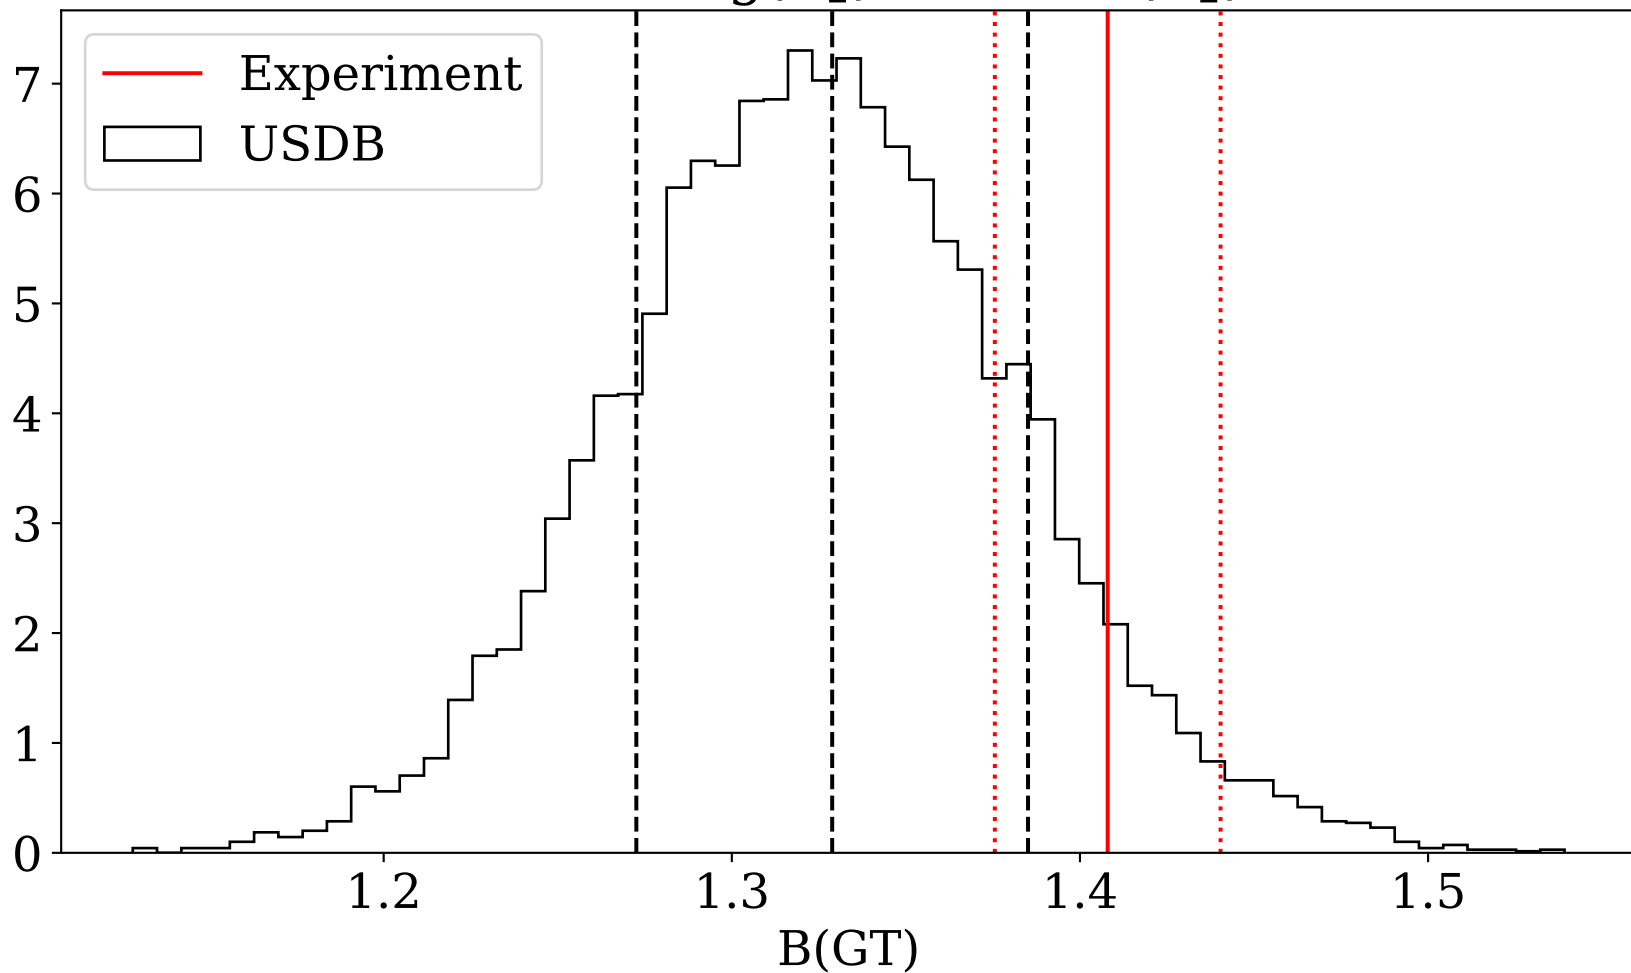

*e. c. :*  $^{22}\text{Mg}(0_1) \rightarrow ^{22}\text{Na}(1_2)$

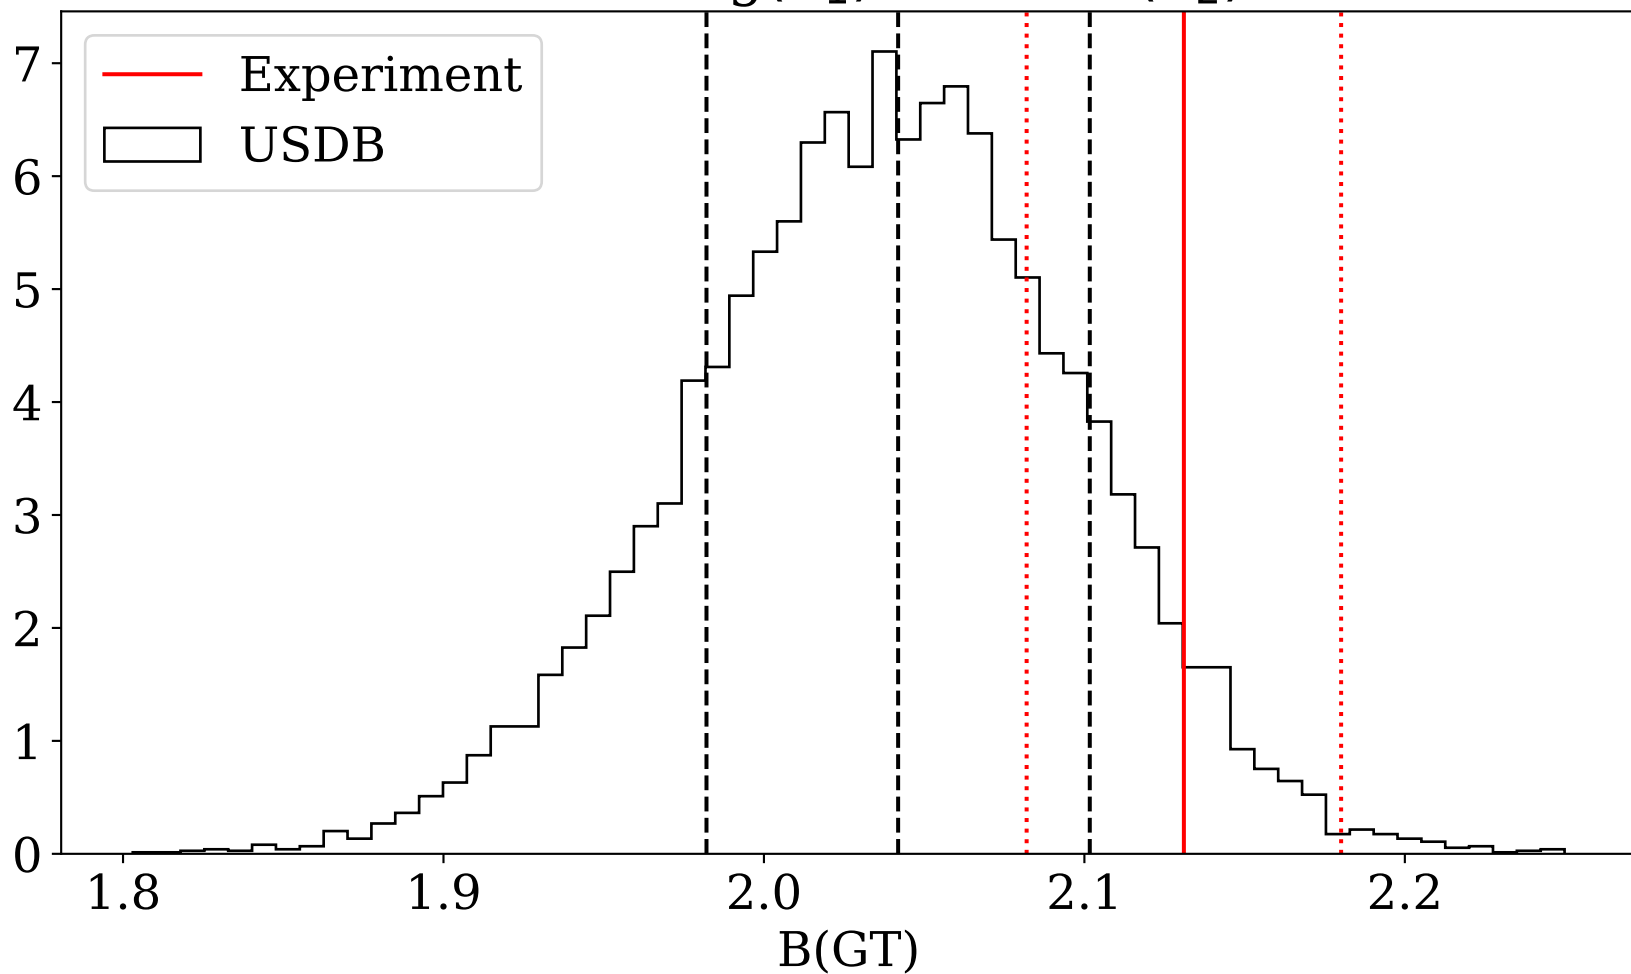

*e. c.* :  $^{23}\text{Mg}(3/2_1) \rightarrow ^{23}\text{Na}(3/2_1)$

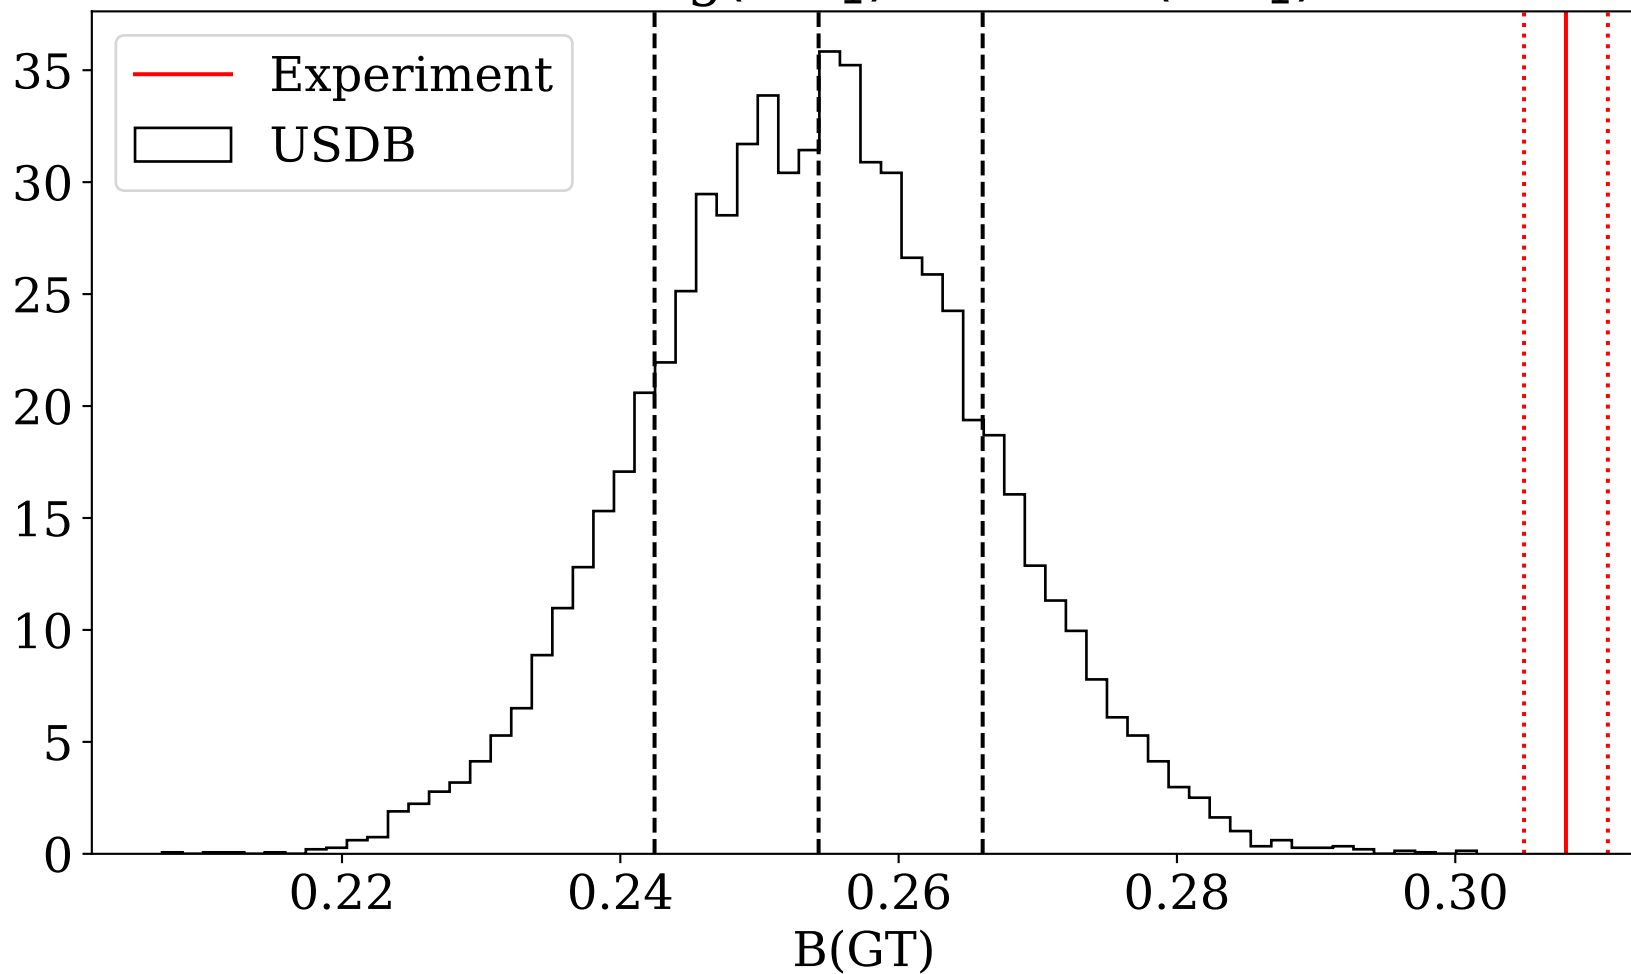

*e. c.* :  $^{23}\text{Mg}(3/2_1) \rightarrow ^{23}\text{Na}(5/2_1)$

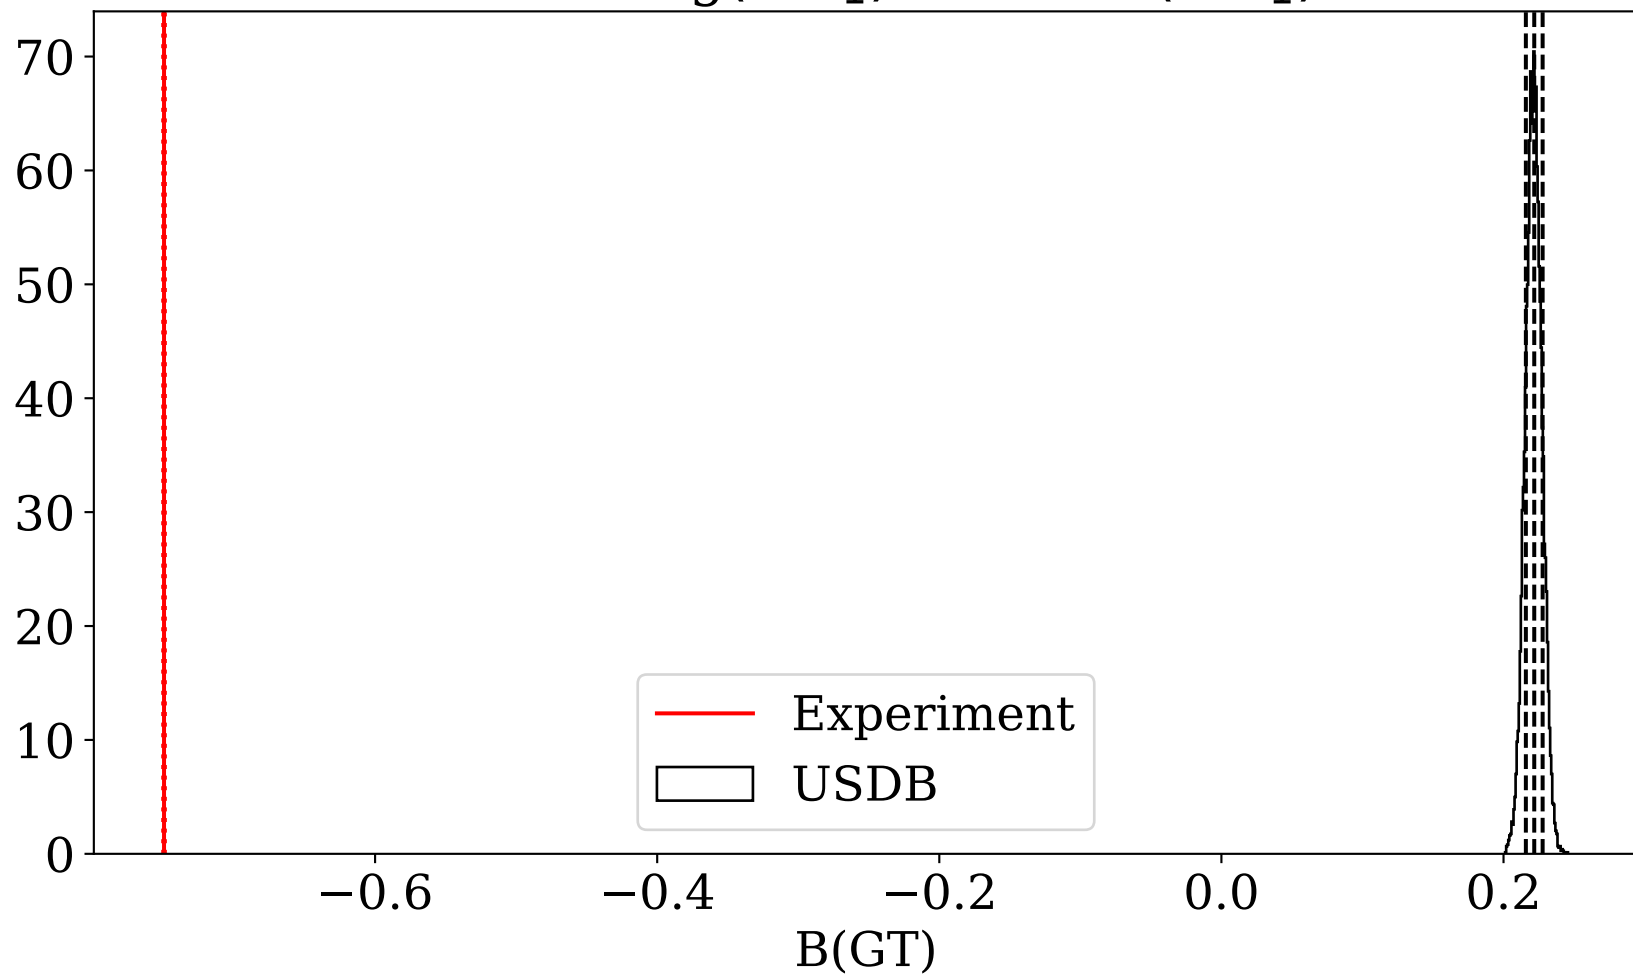

*e. c. :*  $^{23}\text{Mg}(3/2_1) \rightarrow ^{23}\text{Na}(1/2_1)$

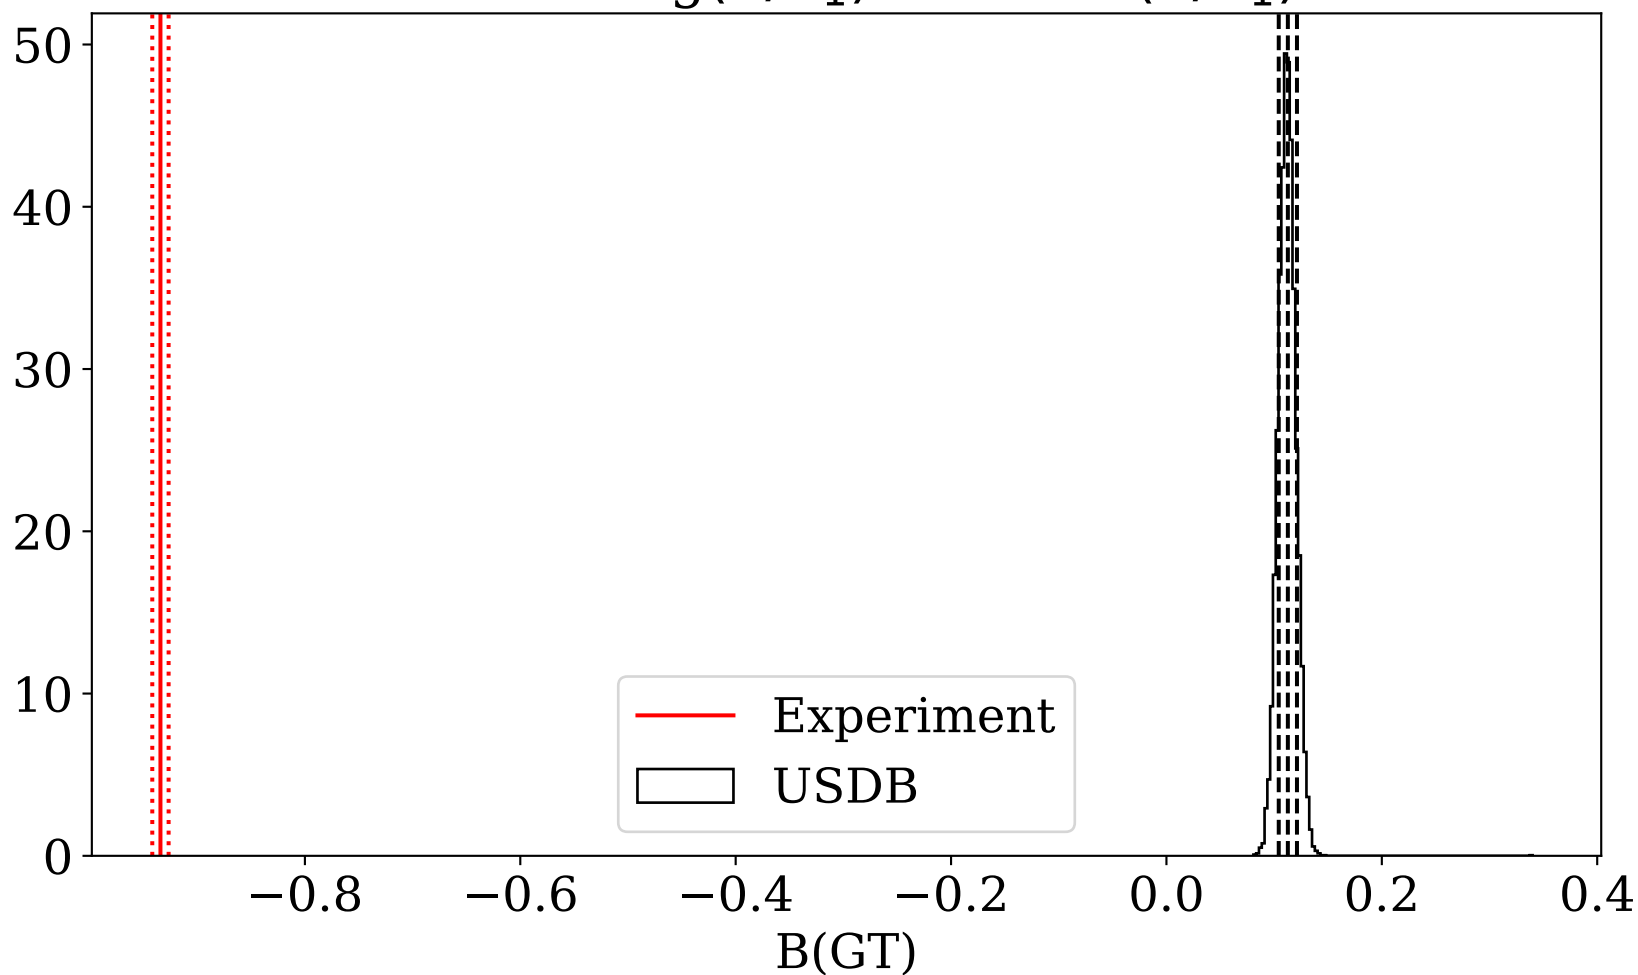



e. c. :  $^{22}\text{Al}(4_1) \rightarrow ^{22}\text{Mg}(4_2)$

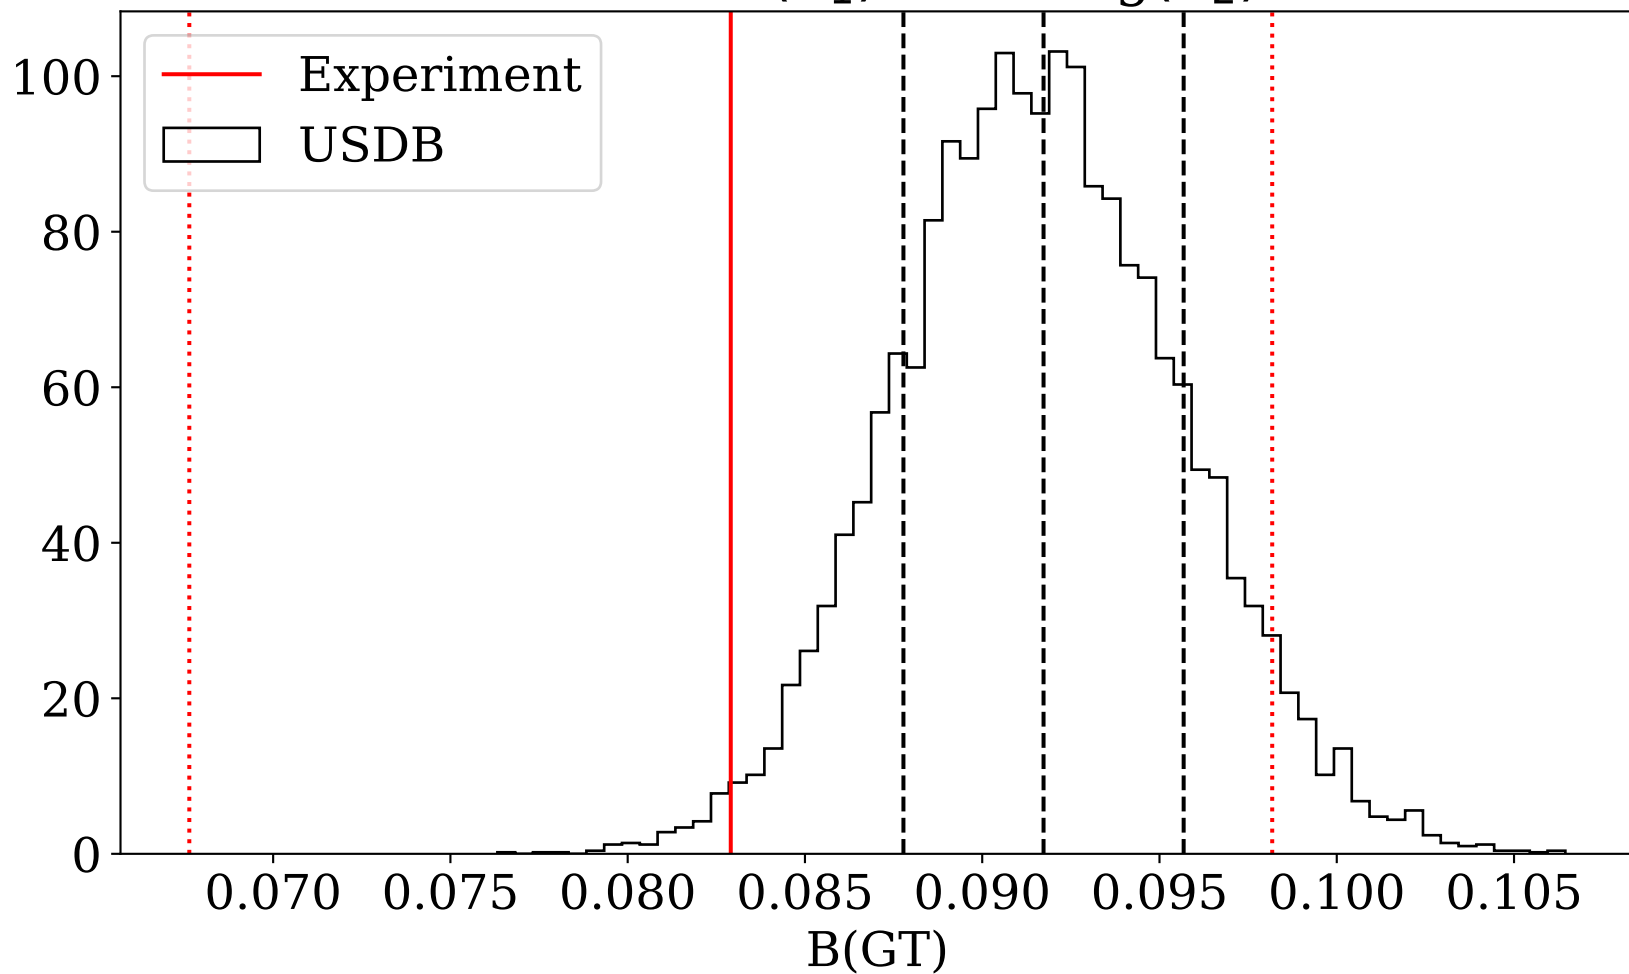

*e. c.* :  $^{22}\text{Al}(4_1) \rightarrow ^{22}\text{Mg}(3_1)$

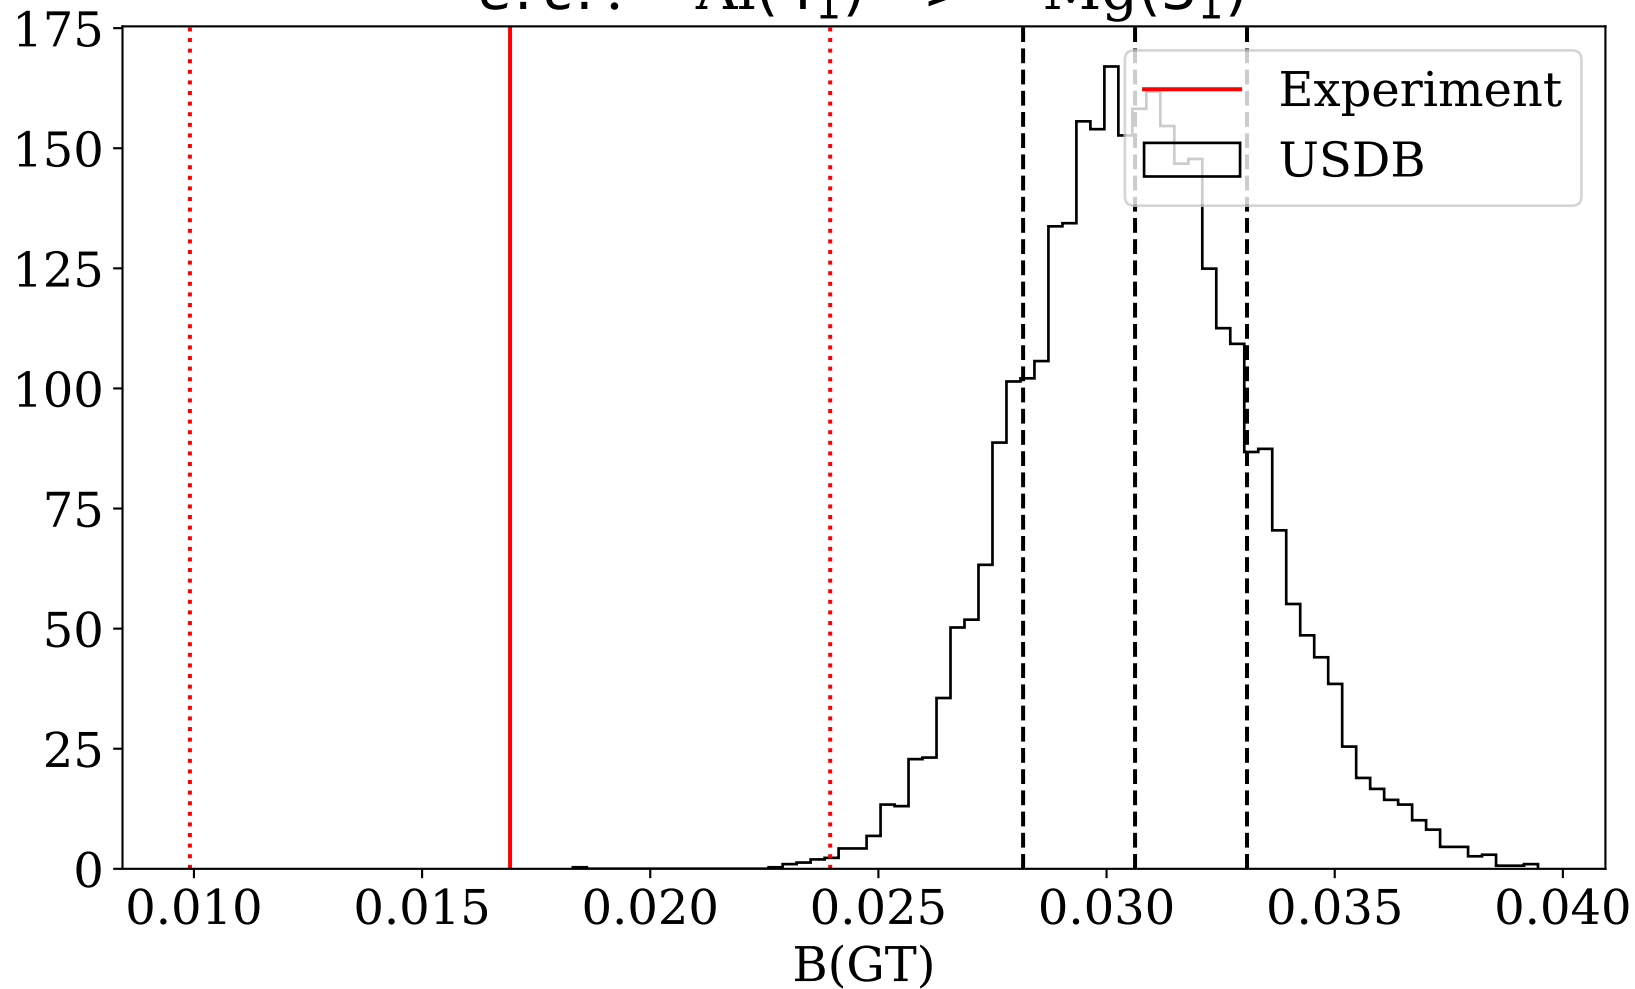

*e. c. :*  $^{22}\text{Al}(4_1) \rightarrow ^{22}\text{Mg}(4_3)$

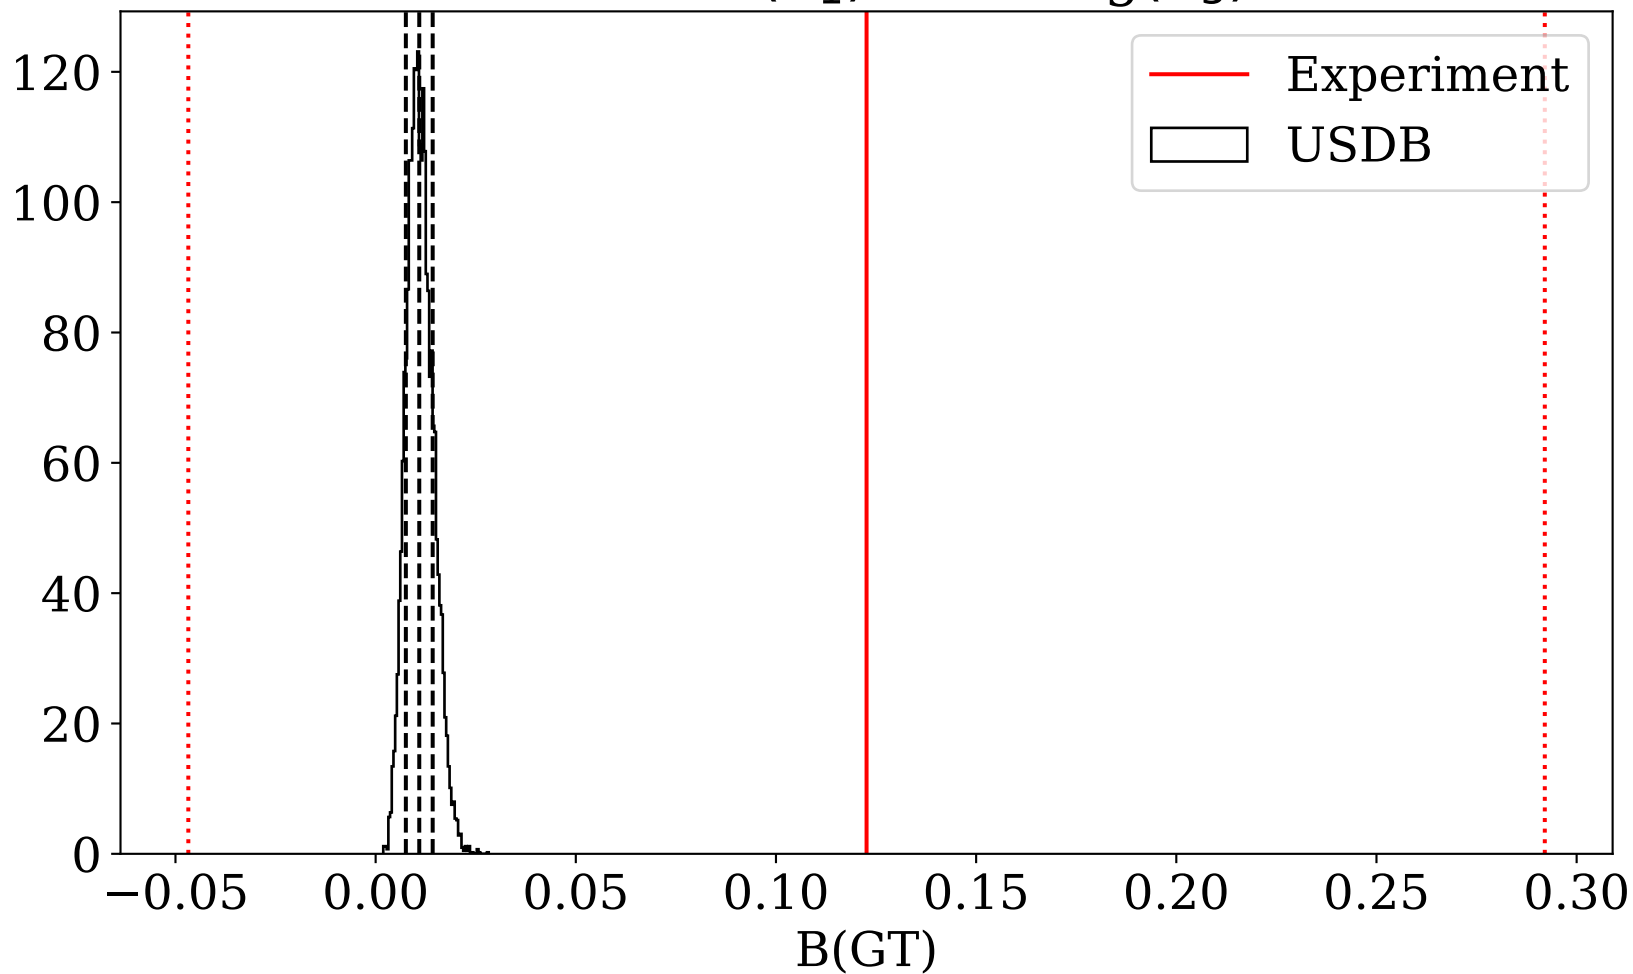

*e. c. :*  $^{23}\text{Al}(5/2_1) \rightarrow ^{23}\text{Mg}(3/2_1)$

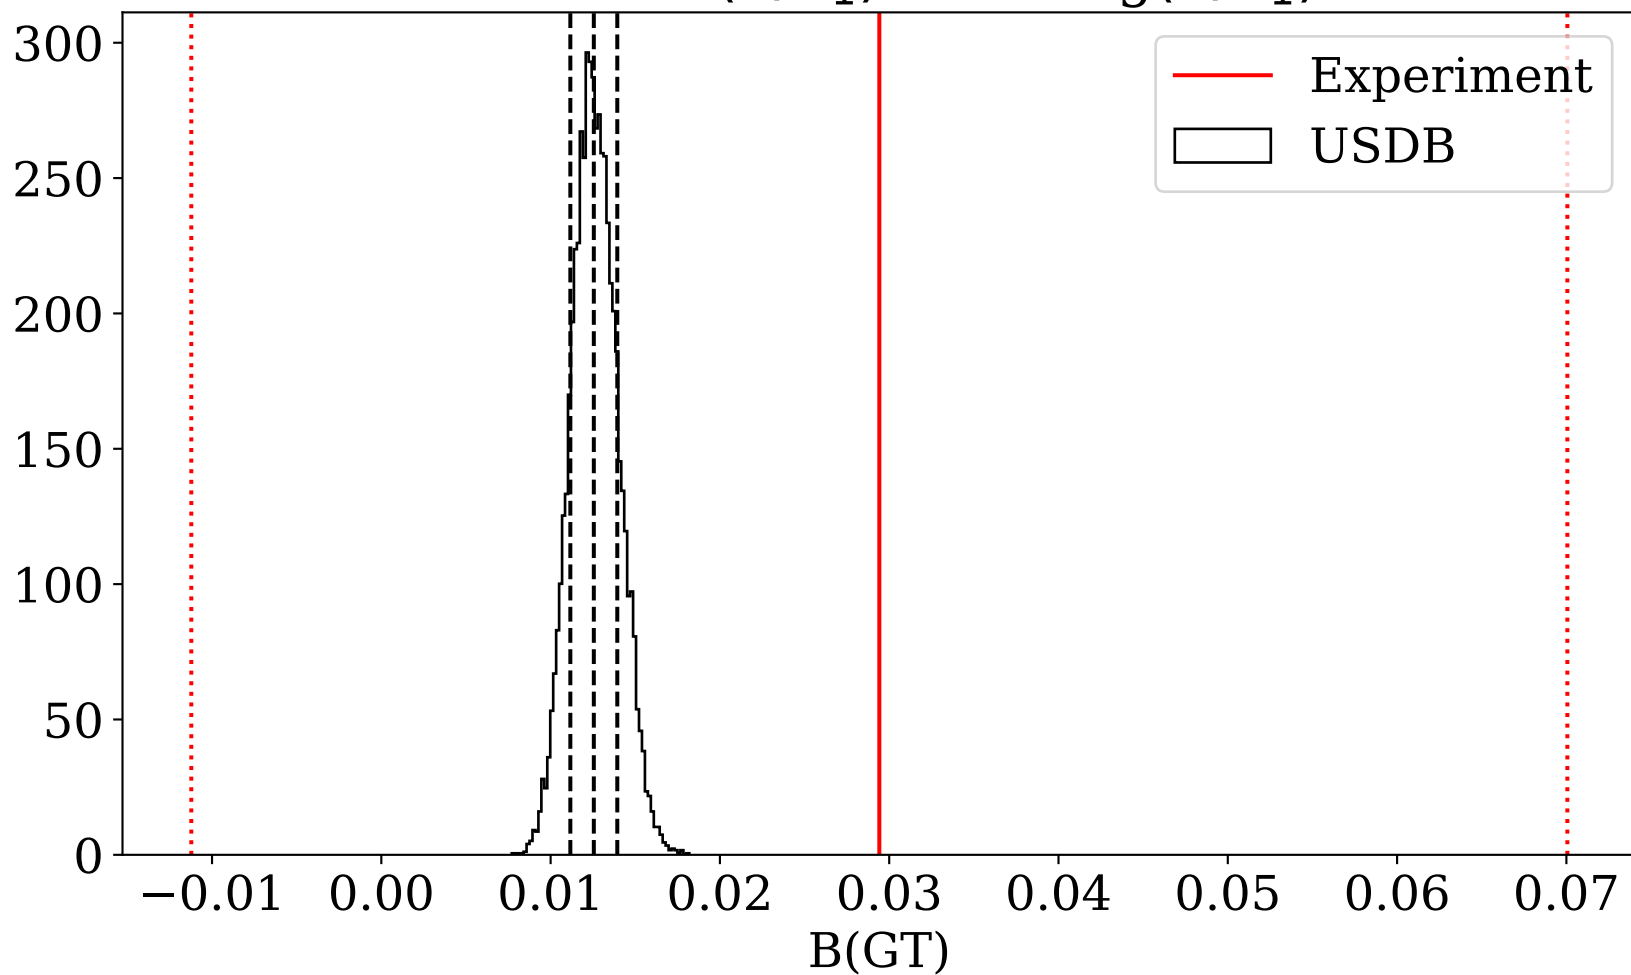

*e. c.* :  $^{23}\text{Al}(5/2_1) \rightarrow ^{23}\text{Mg}(5/2_1)$

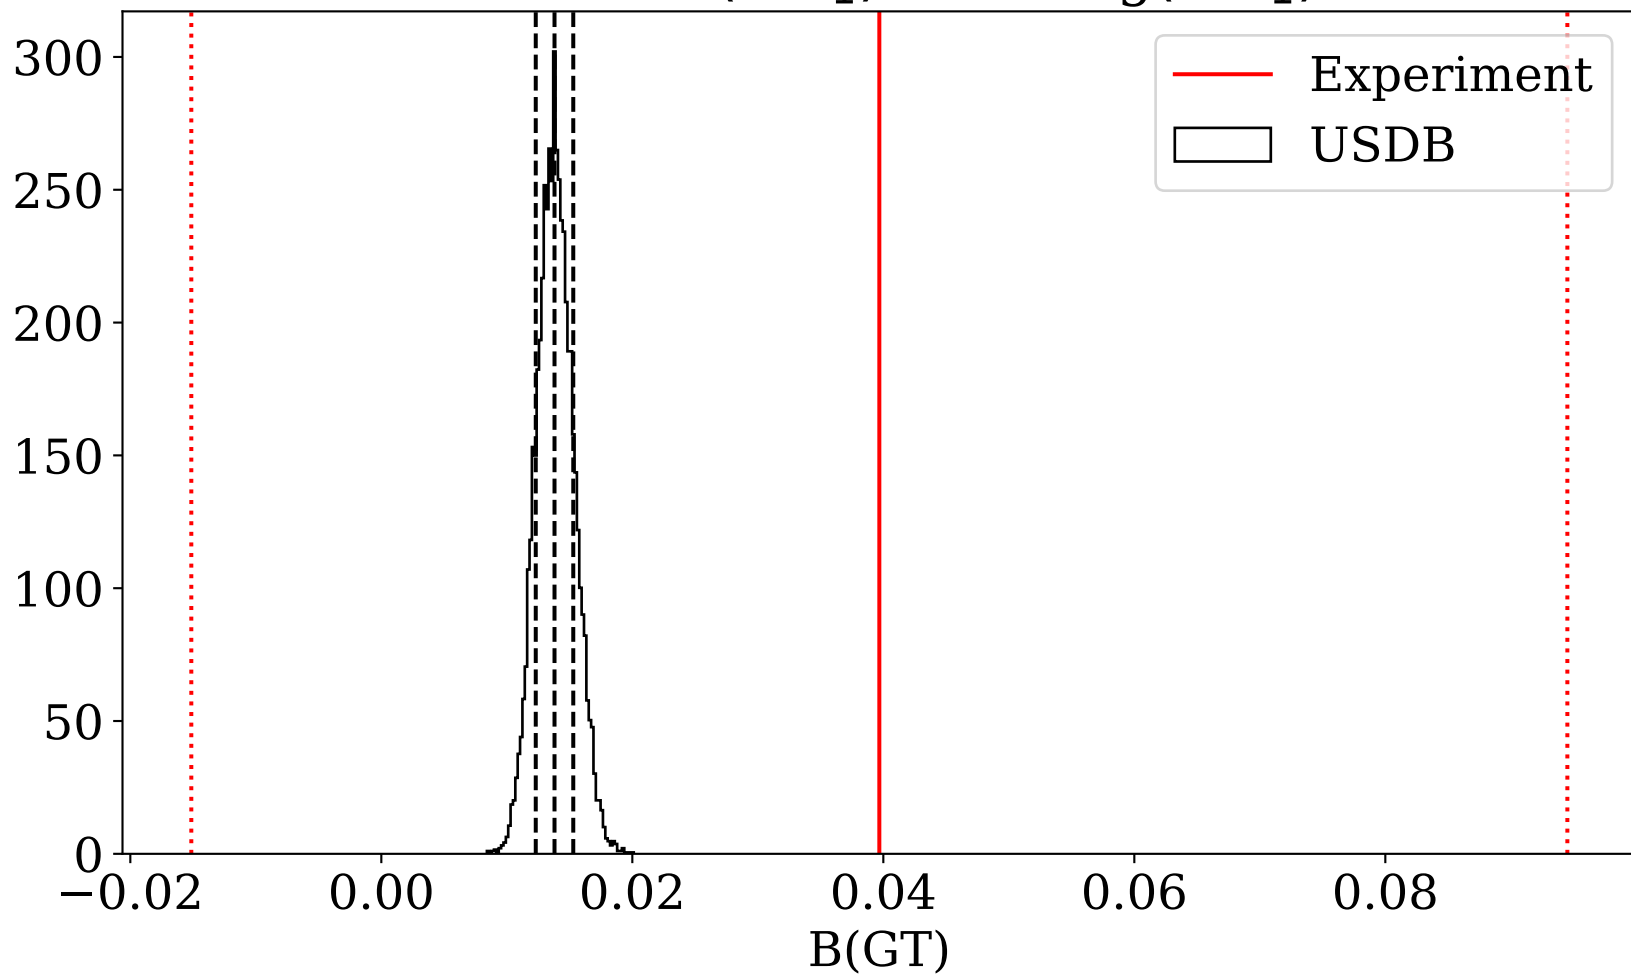

*e. c. :*  $^{23}\text{Al}(5/2_1) \rightarrow ^{23}\text{Mg}(7/2_1)$

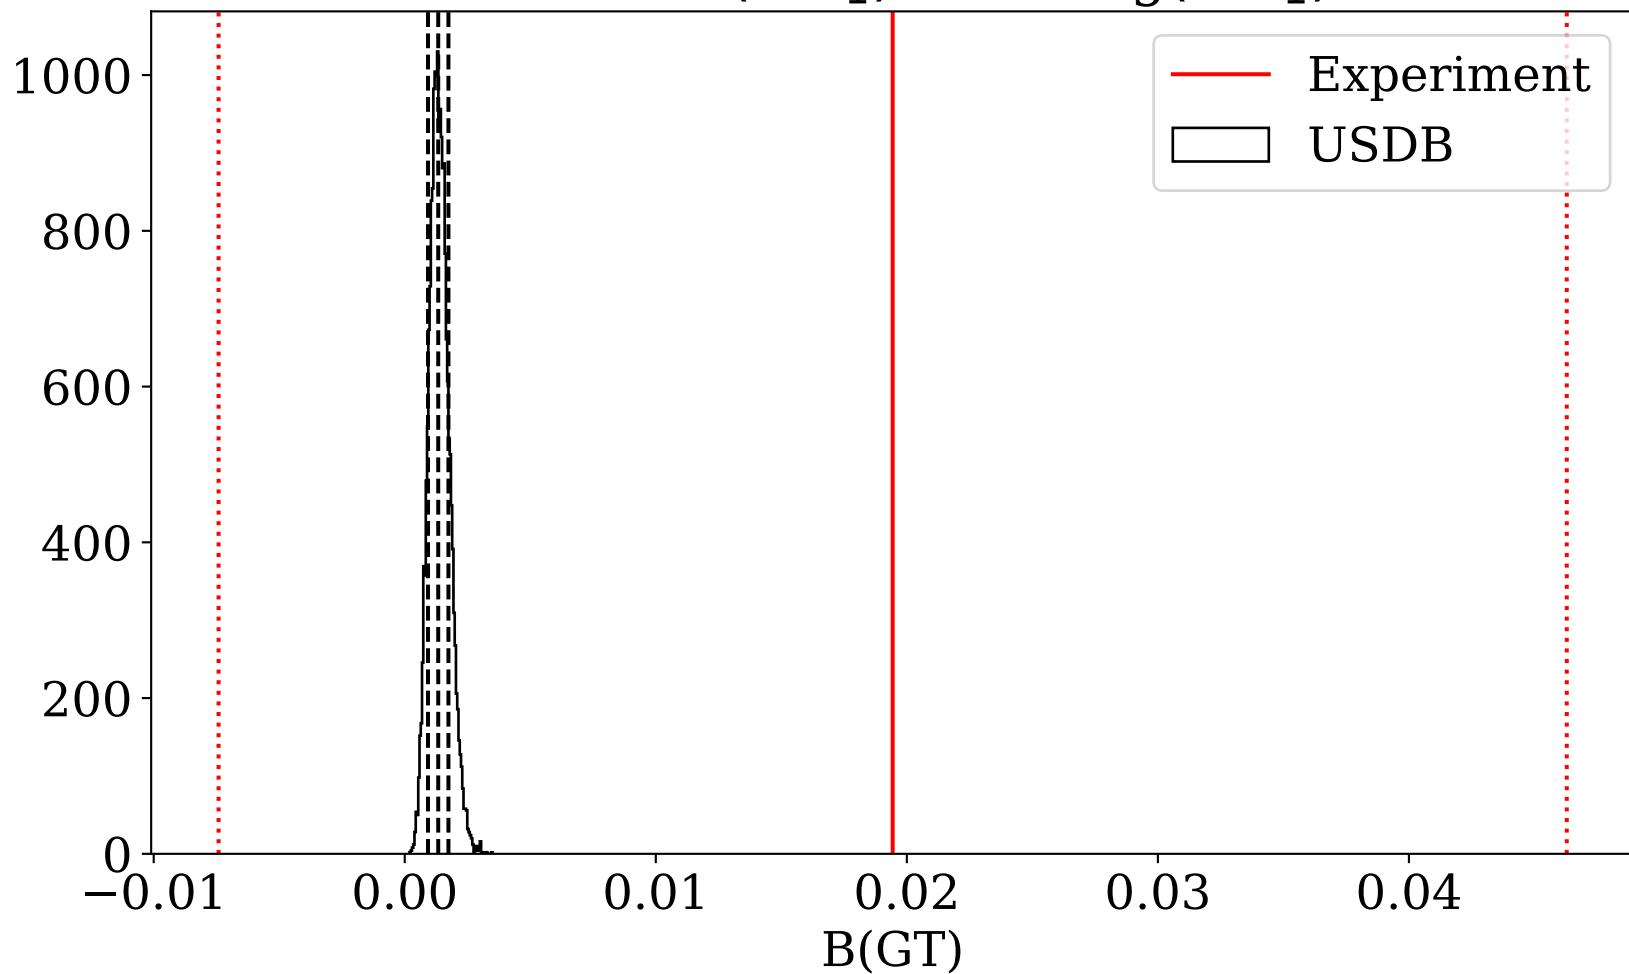

e. c. :  $^{24}\text{Al}(4_1) \rightarrow ^{24}\text{Mg}(4_3)$

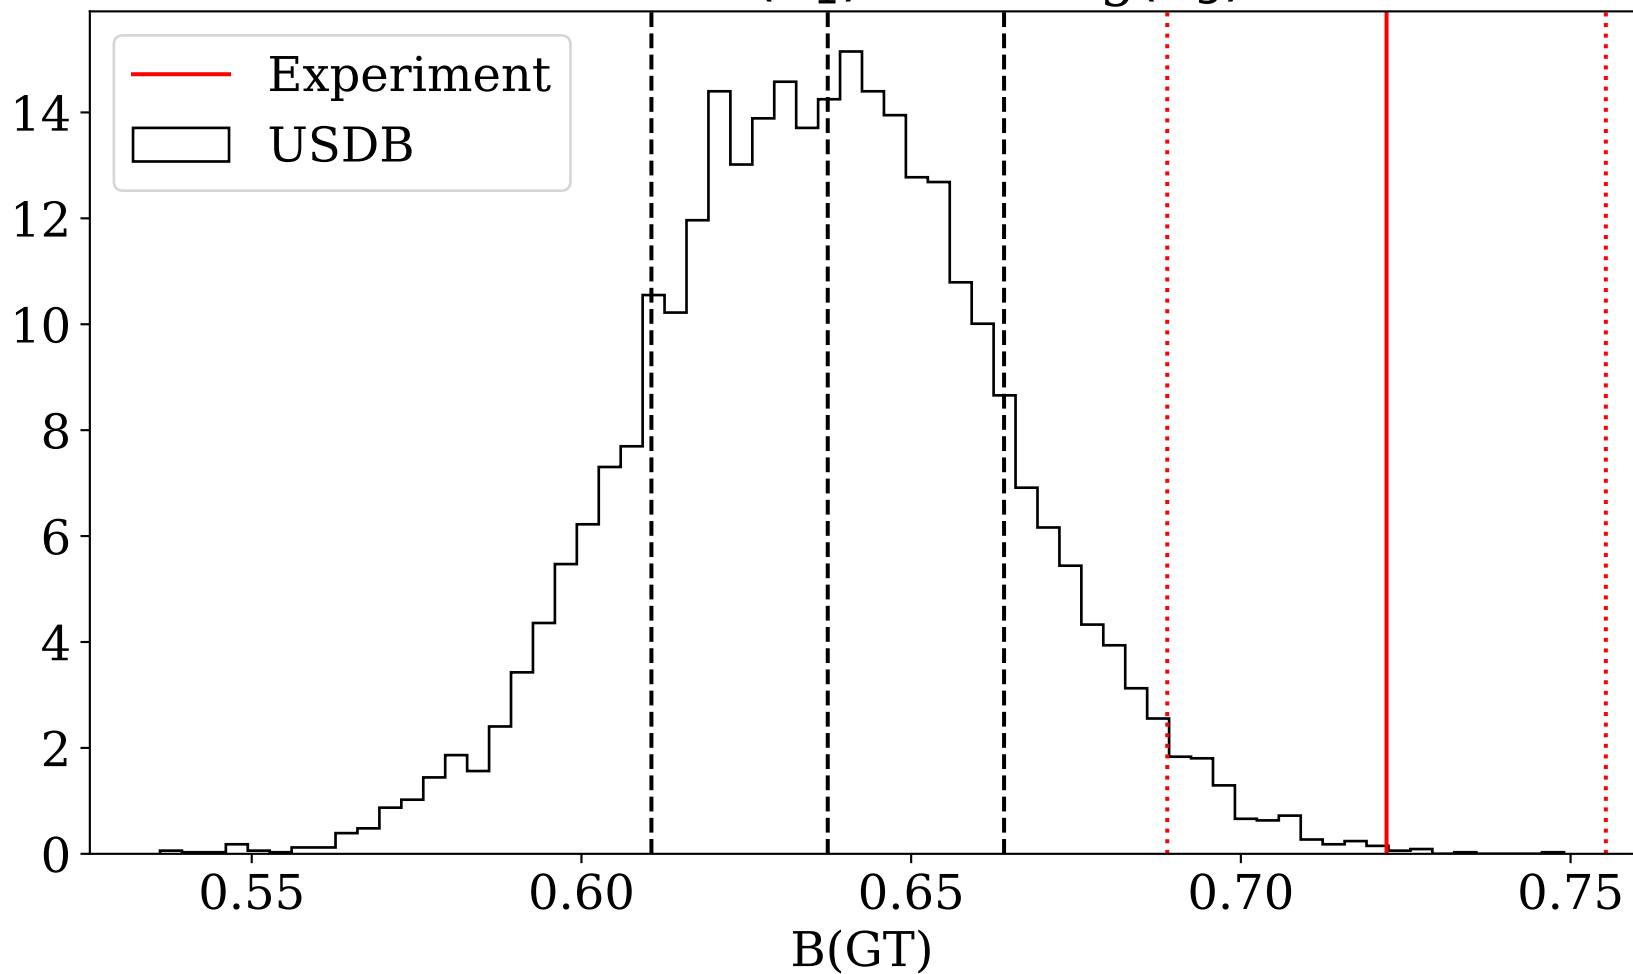

*e. c. :*  $^{24}\text{Al}(4_1) \rightarrow ^{24}\text{Mg}(4_1)$

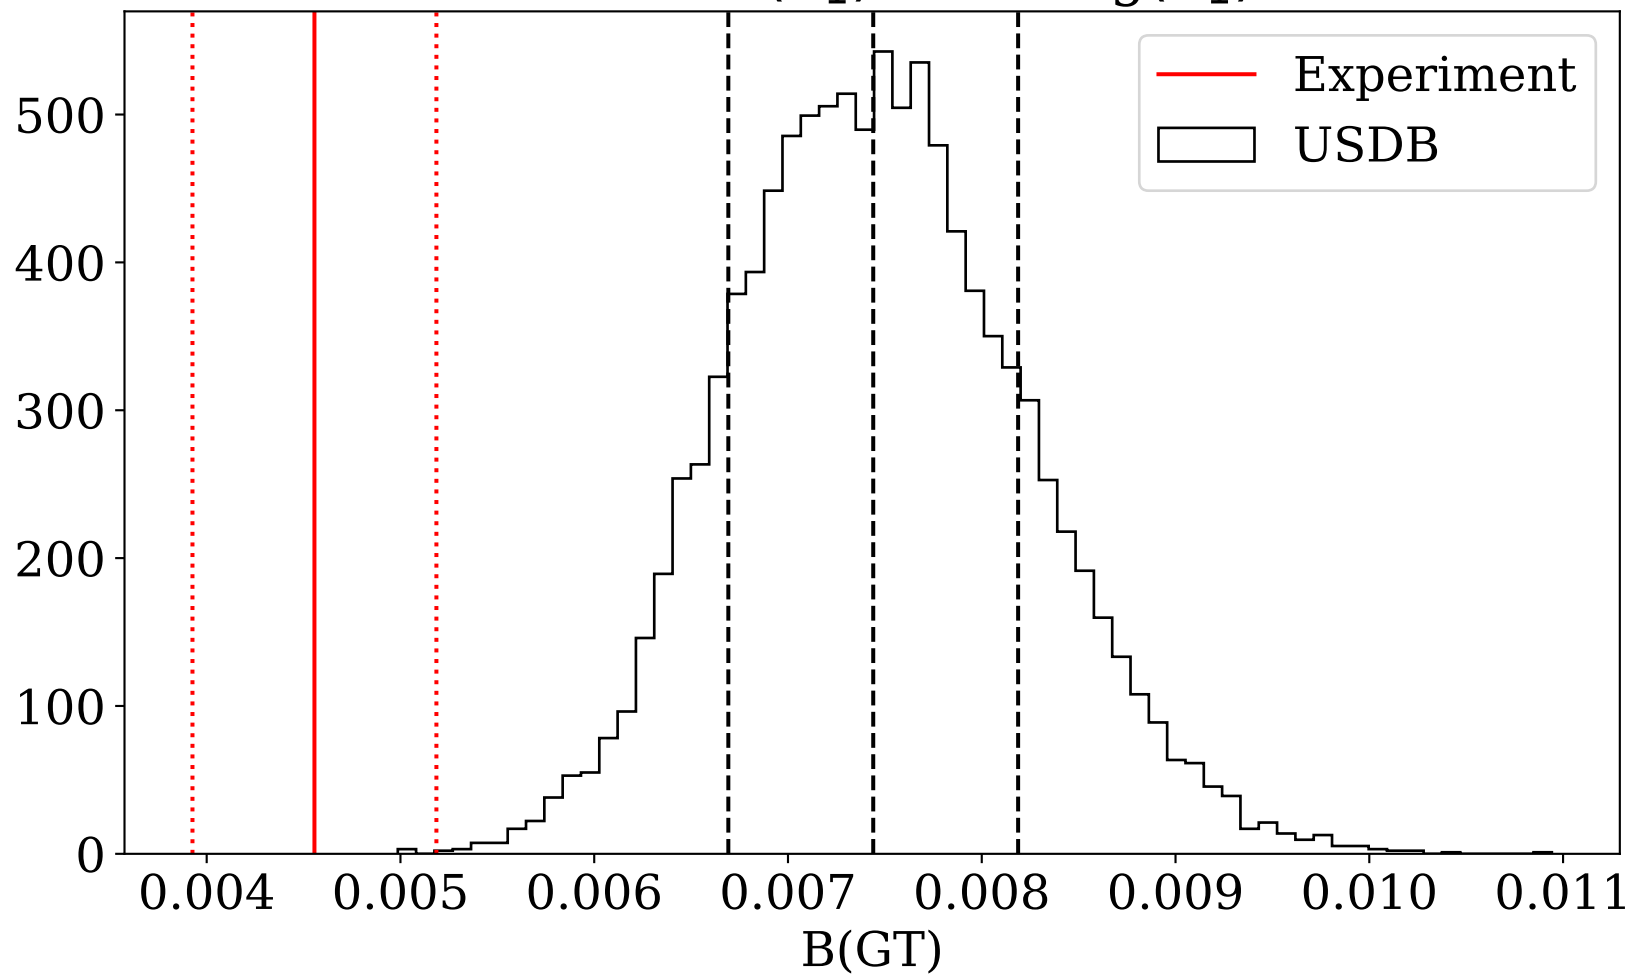



*e. c. :*  $^{24}\text{Al}(4_1) \rightarrow ^{24}\text{Mg}(3_1)$

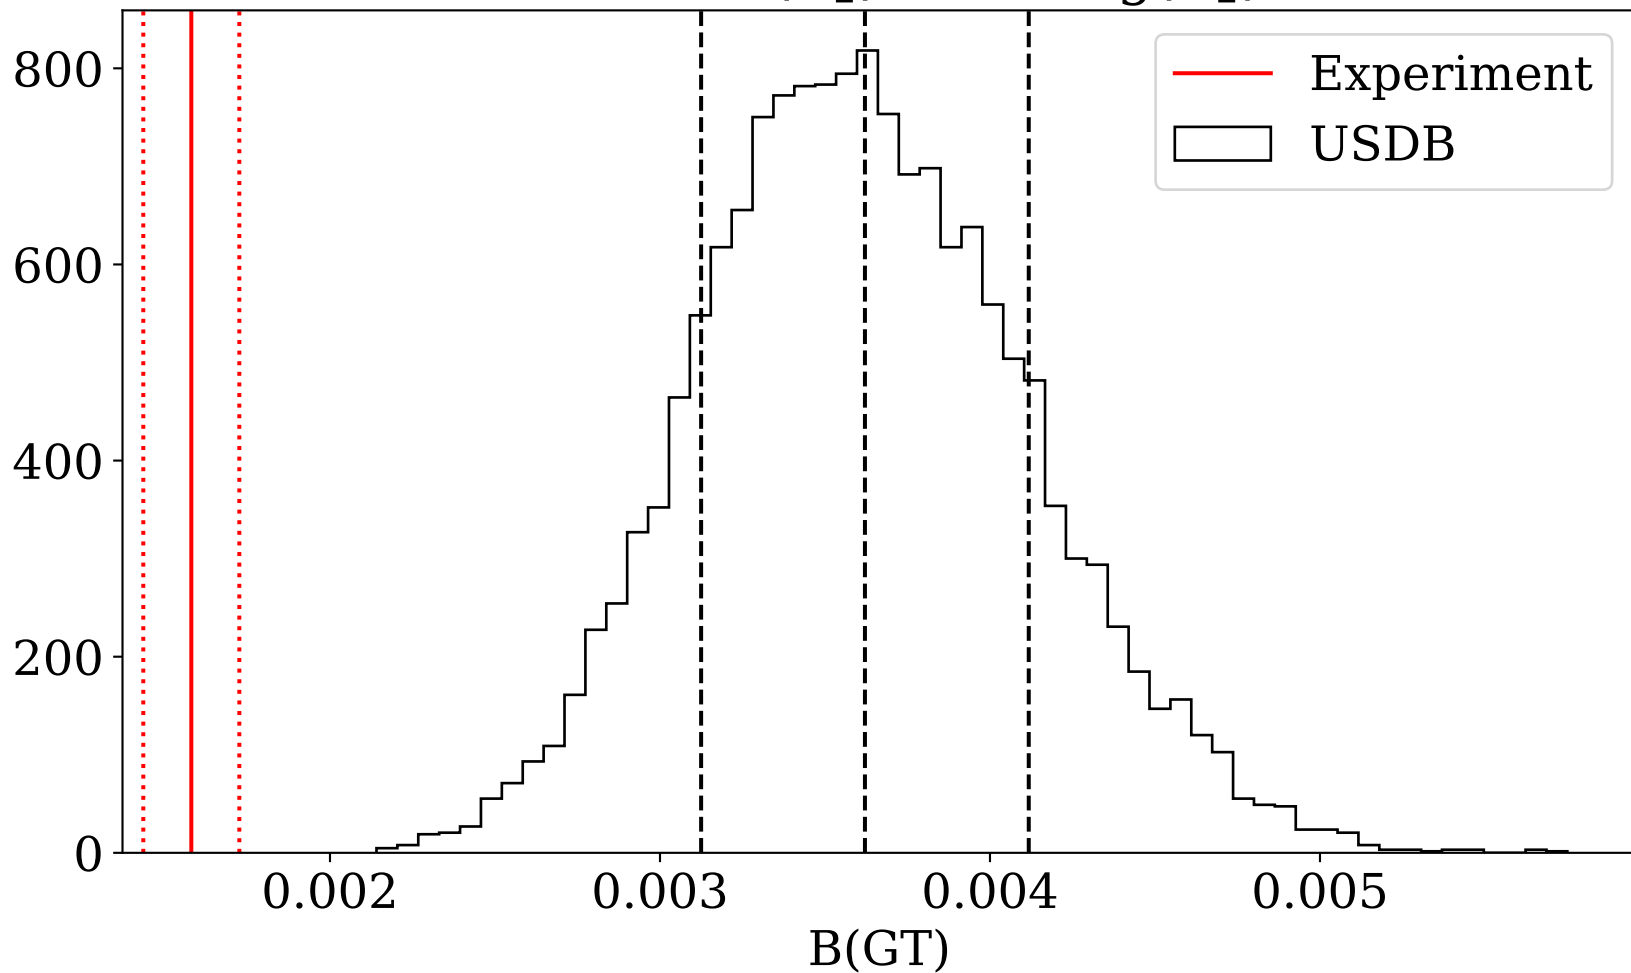

e. c. :  $^{24}\text{Al}(4_1) \rightarrow ^{24}\text{Mg}(4_2)$

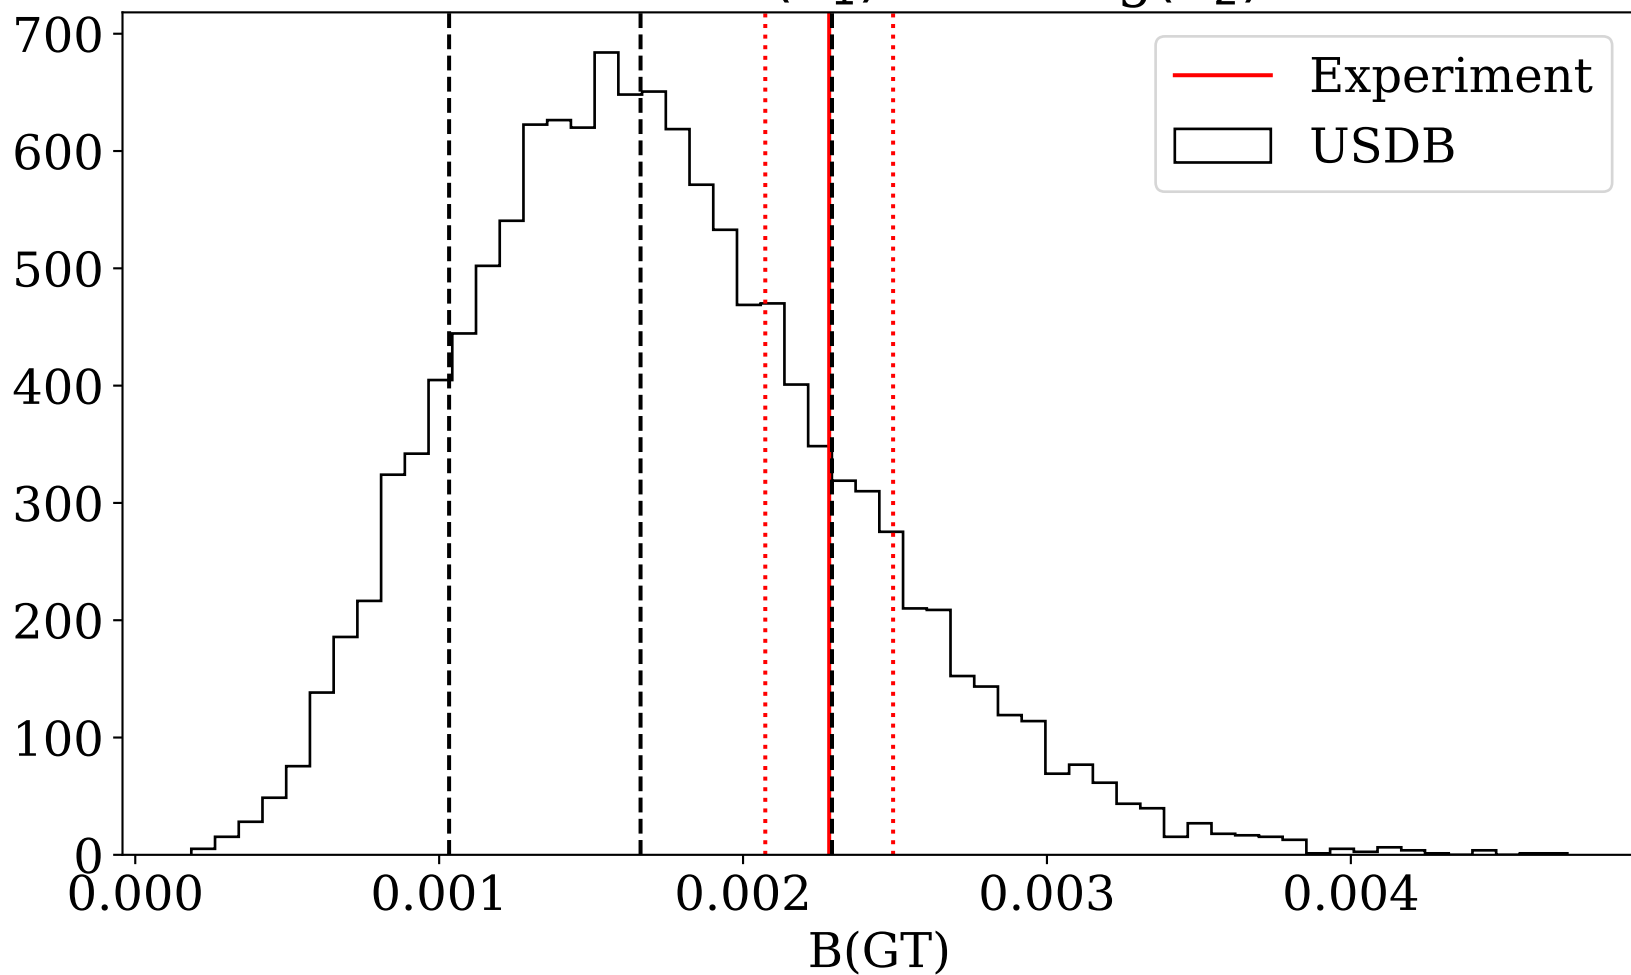

*e. c. :*  $^{24}\text{Al}(4_1) \rightarrow ^{24}\text{Mg}(5_1)$

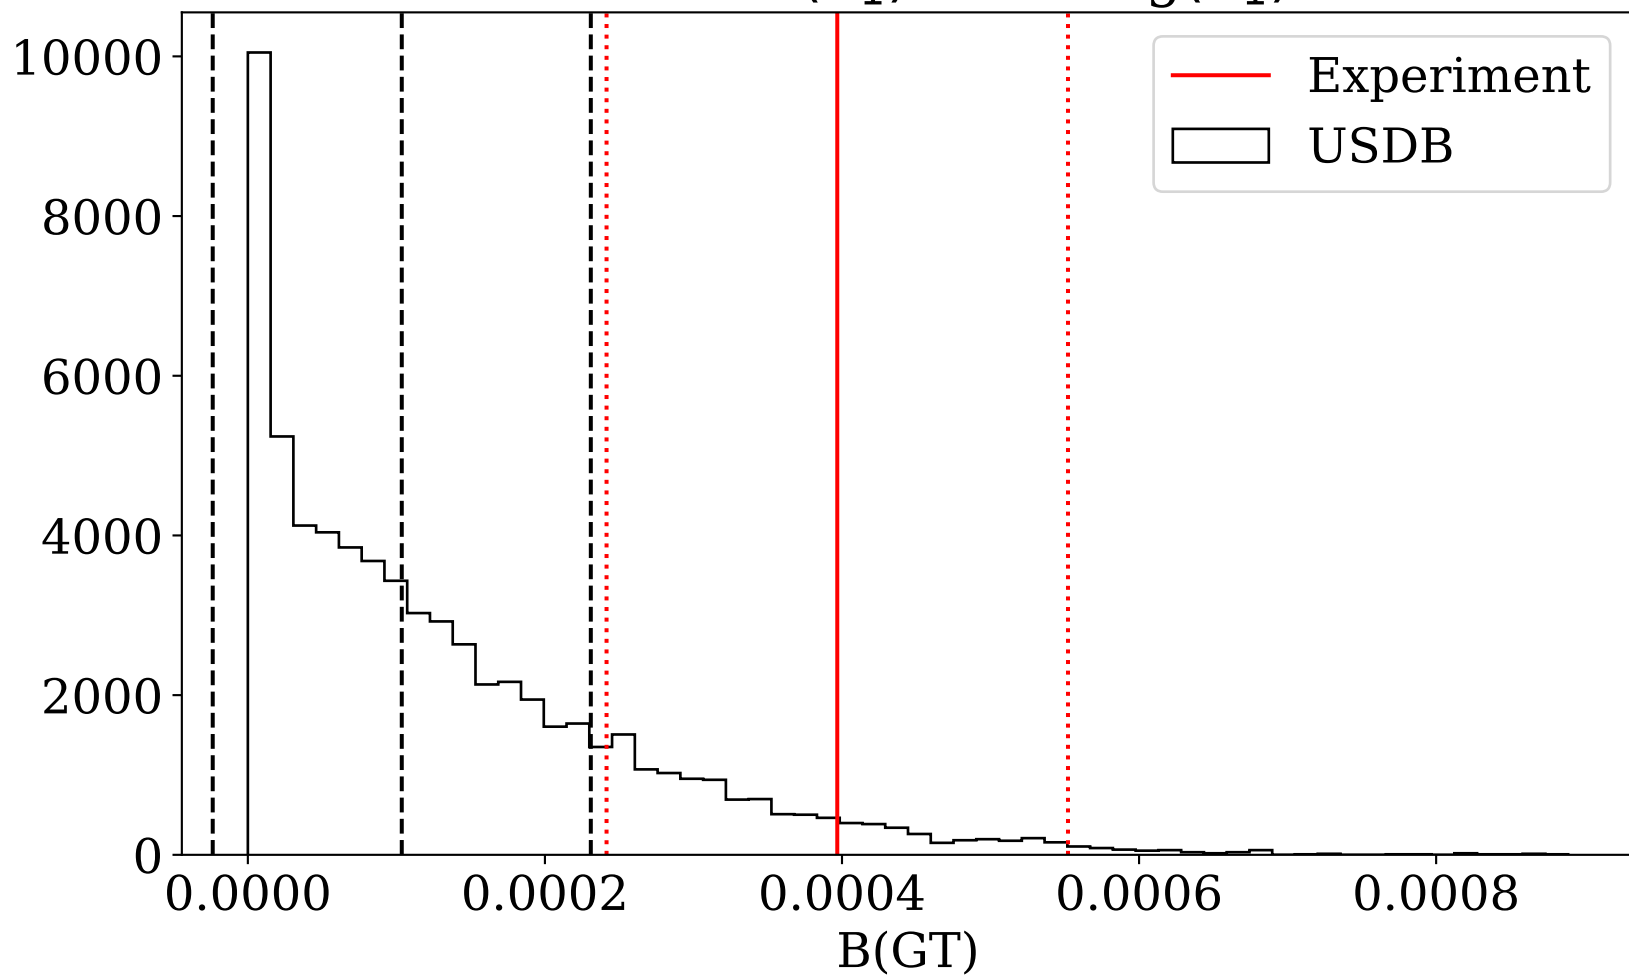

*e. c. :*  $^{25}\text{Al}(5/2_1) \rightarrow ^{25}\text{Mg}(5/2_1)$

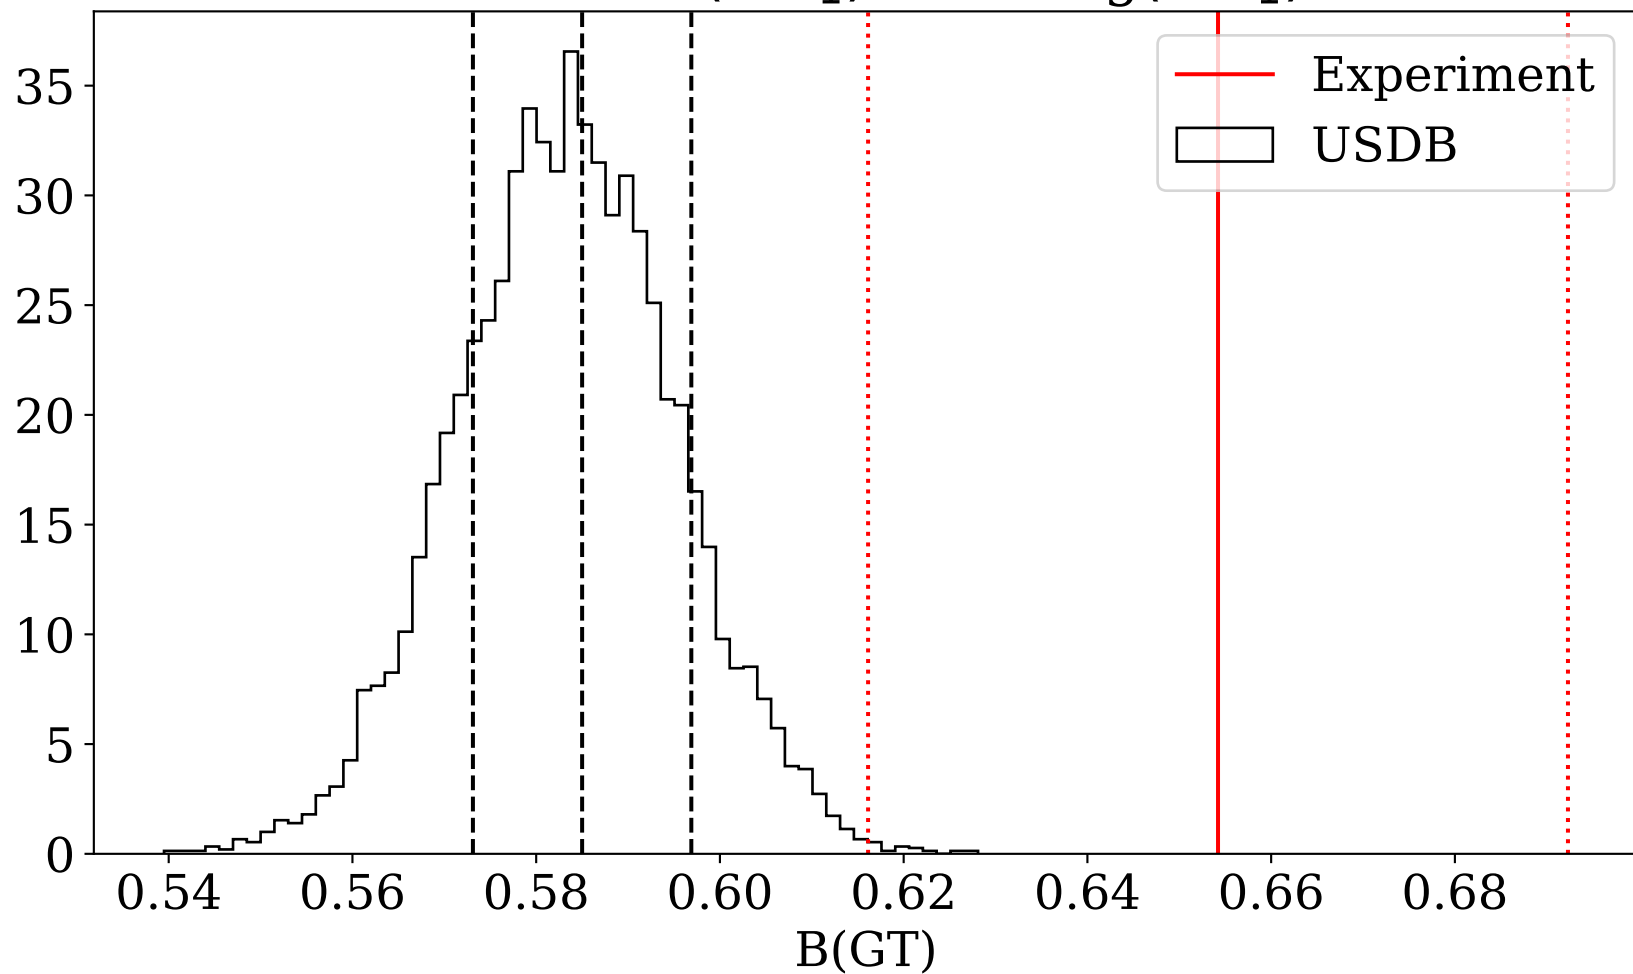

*e. c.* :  $^{25}\text{Al}(5/2_1) \rightarrow ^{25}\text{Mg}(3/2_1)$

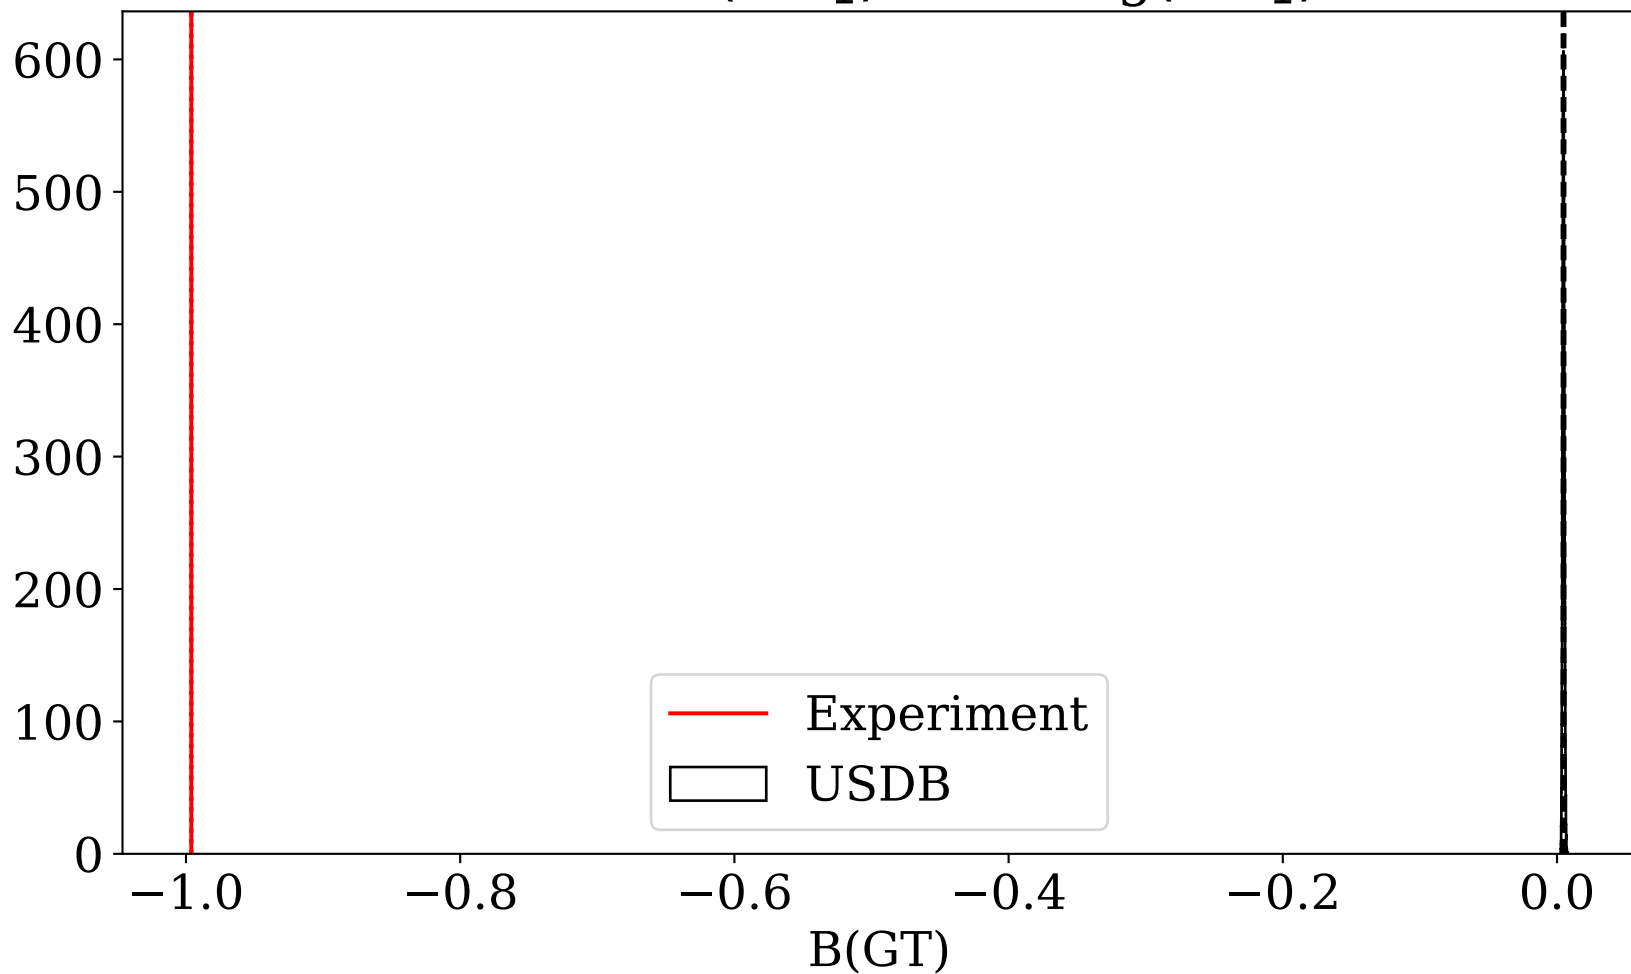

*e. c. :*  $^{25}\text{Al}(5/2_1) \rightarrow ^{25}\text{Mg}(7/2_1)$

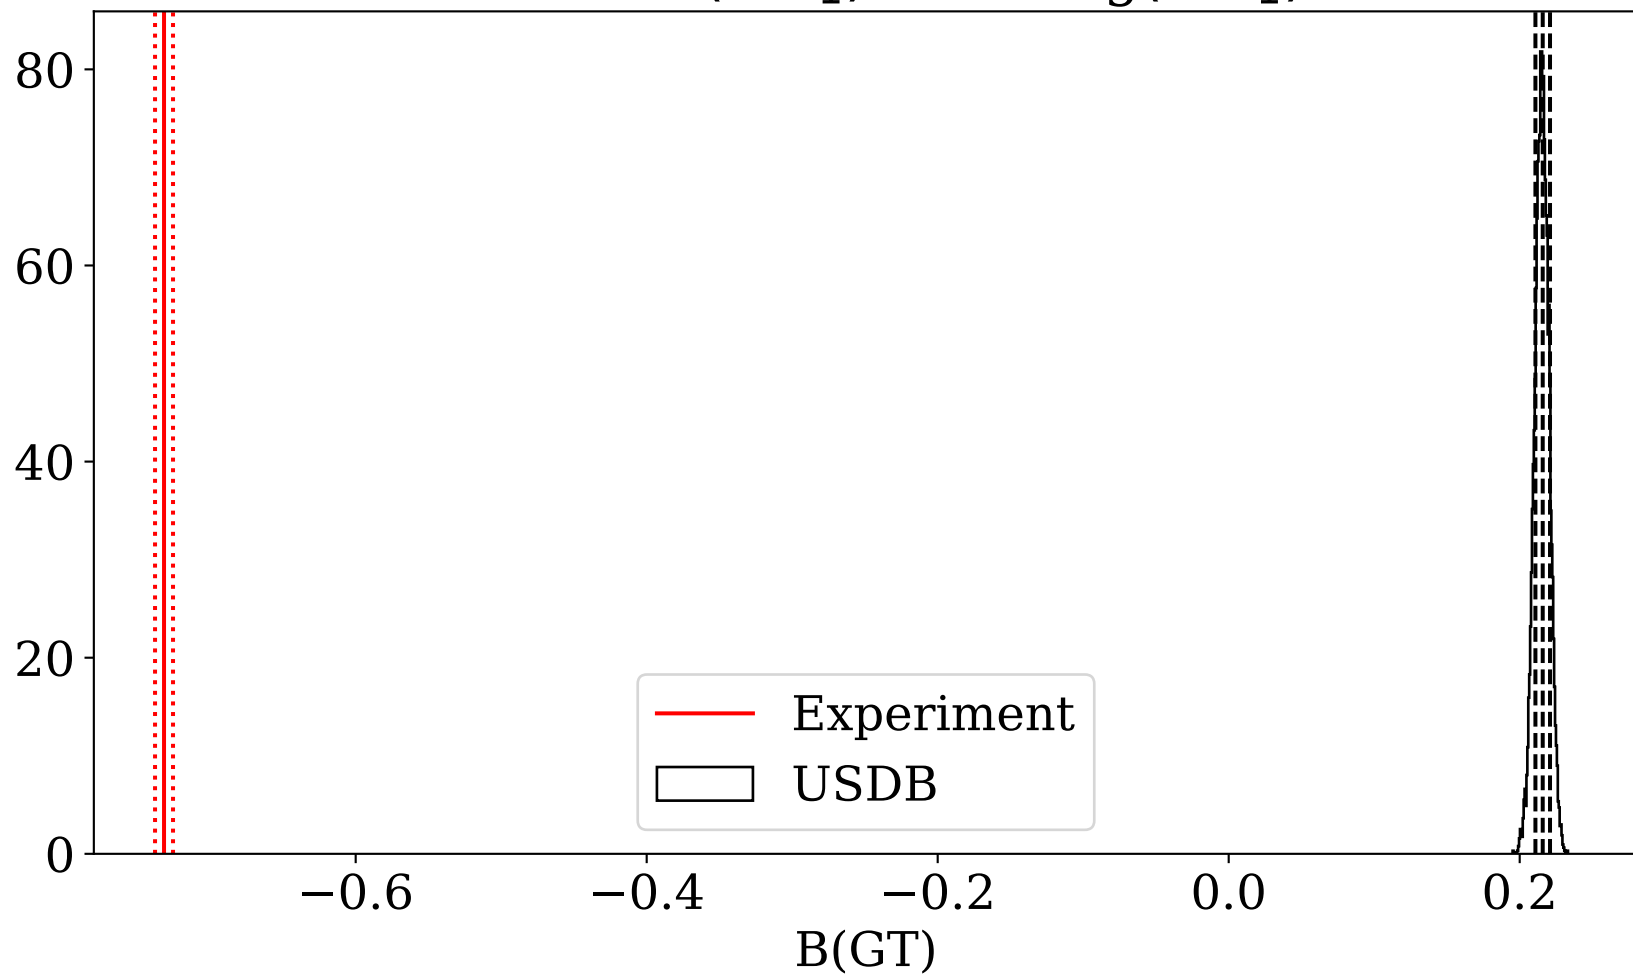

e. c. :  $^{26}\text{Si}(0_1) \rightarrow ^{26}\text{Al}(1_1)$

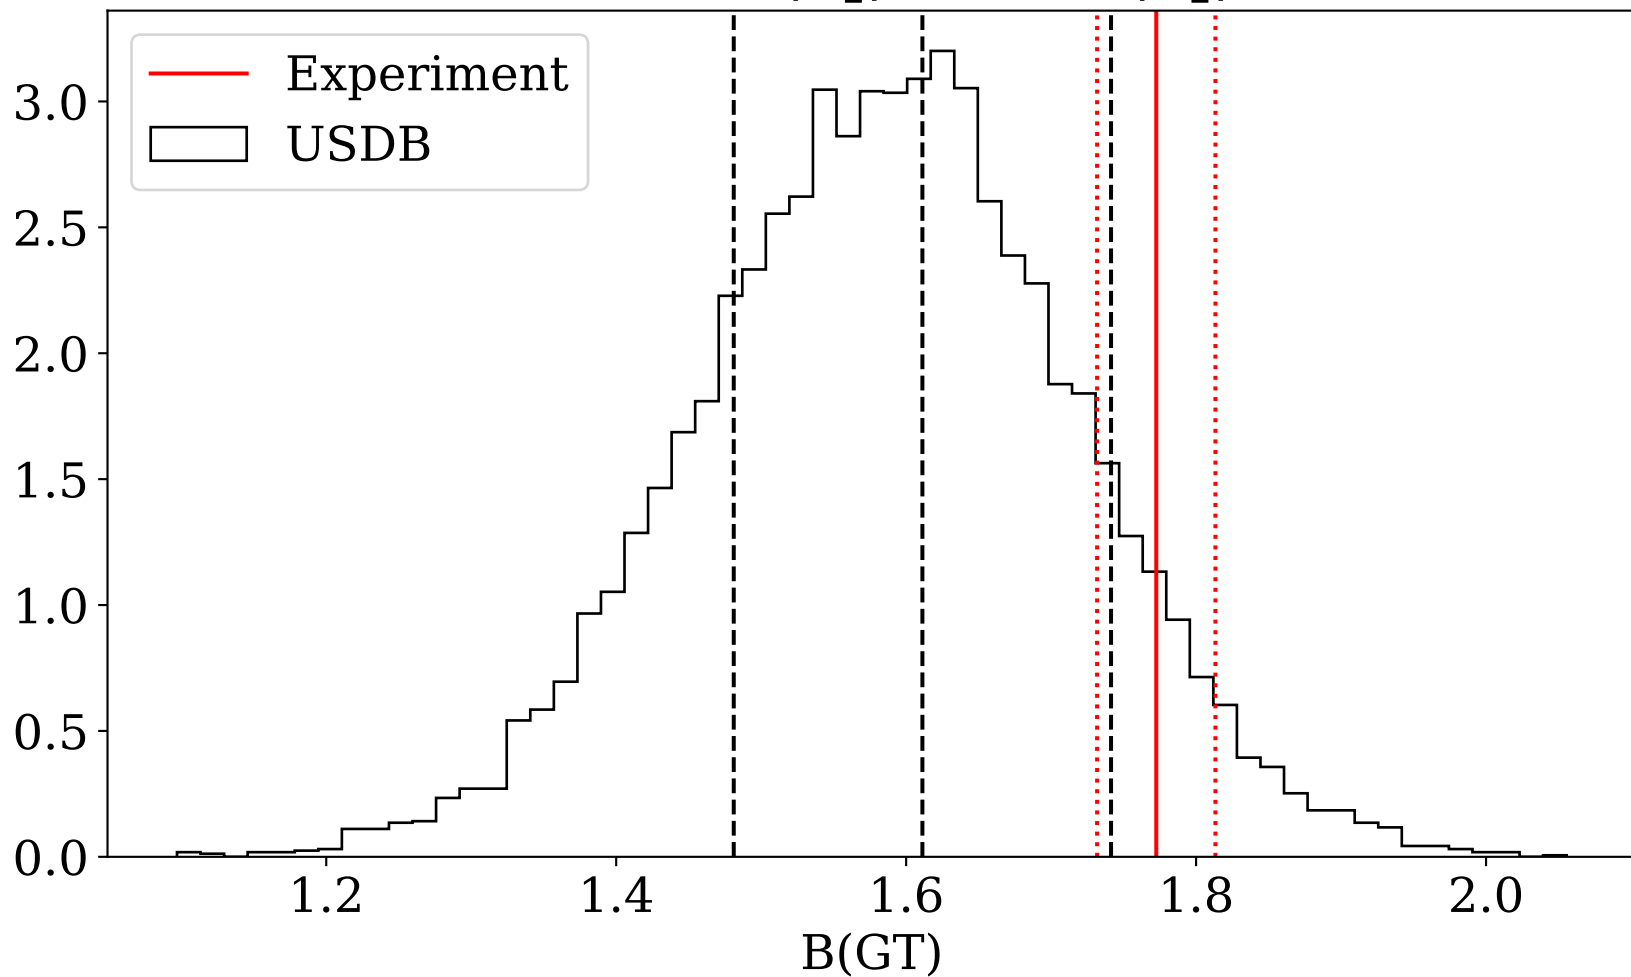

*e. c.*:  $^{26}\text{Si}(0_1) \rightarrow ^{26}\text{Al}(1_2)$

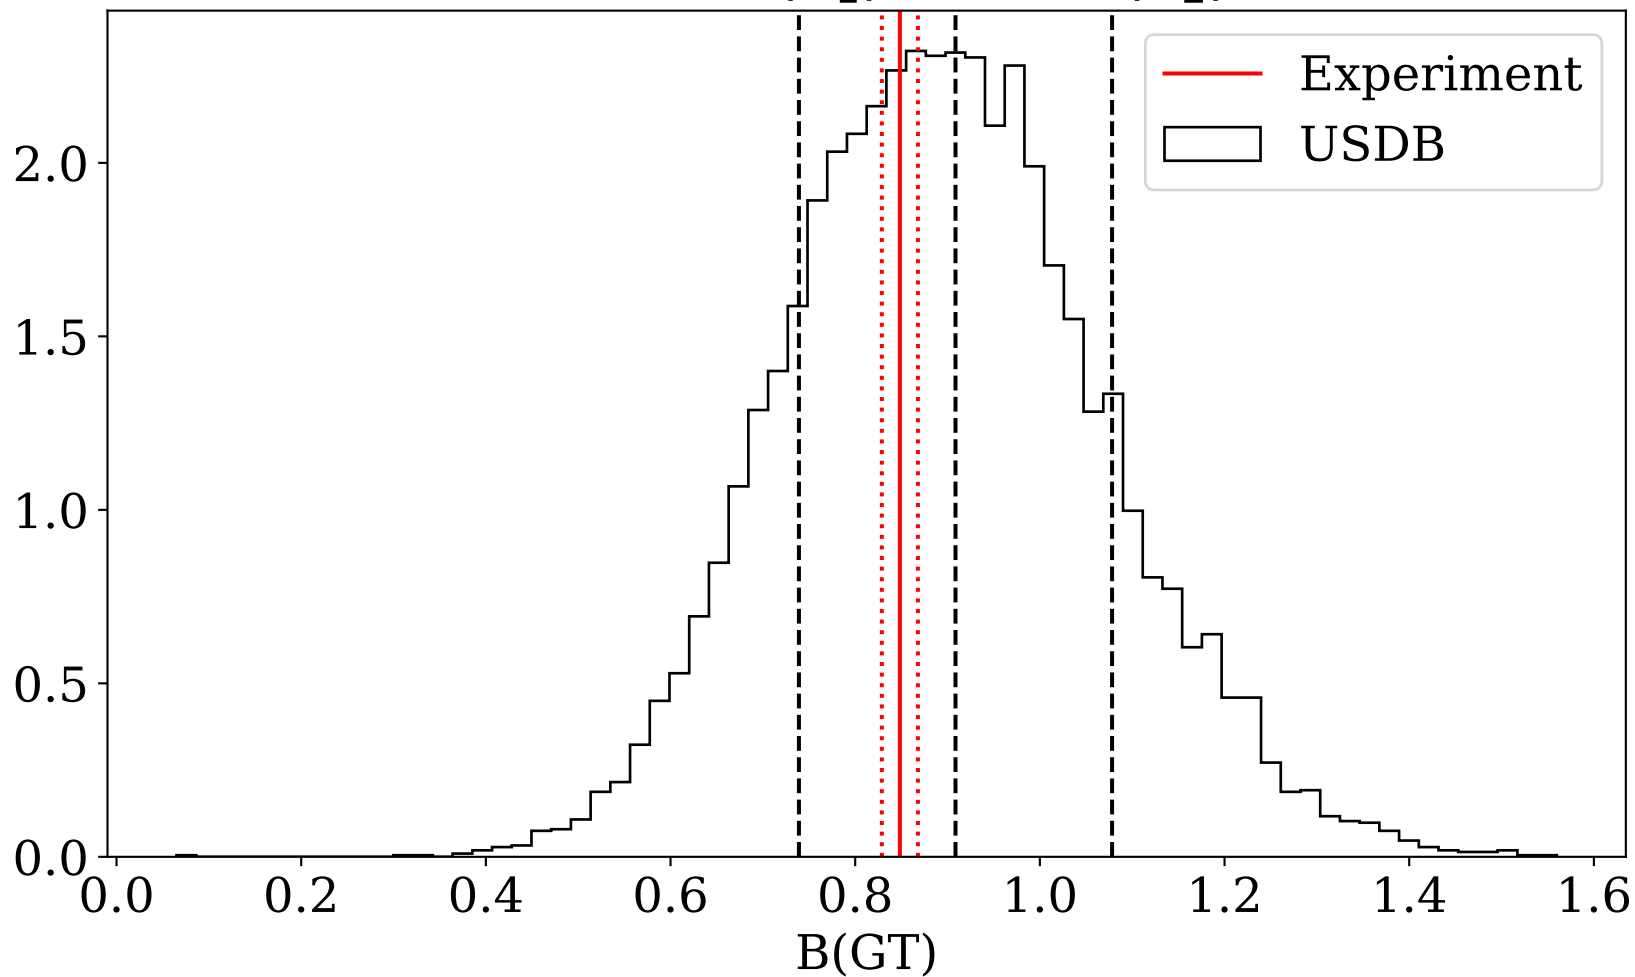



*e. c.*:  $^{26}\text{Si}(0_1) \rightarrow ^{26}\text{Al}(1_3)$

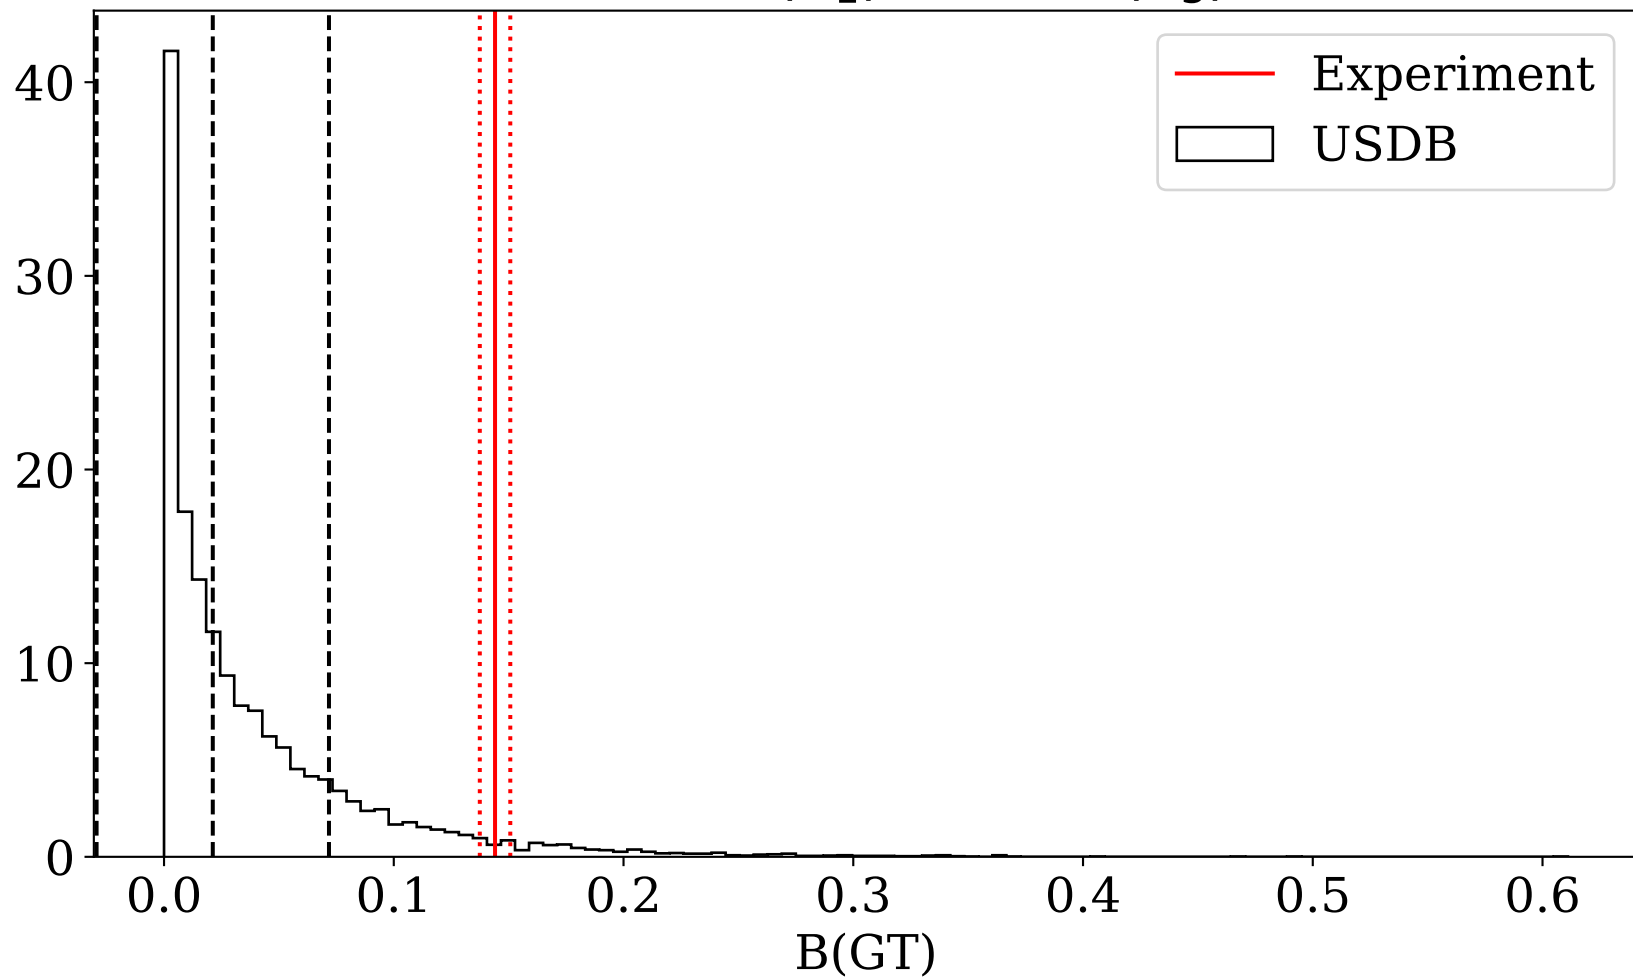

*e. c.* :  $^{26}\text{Si}(0_1) \rightarrow ^{26}\text{Al}(1_4)$

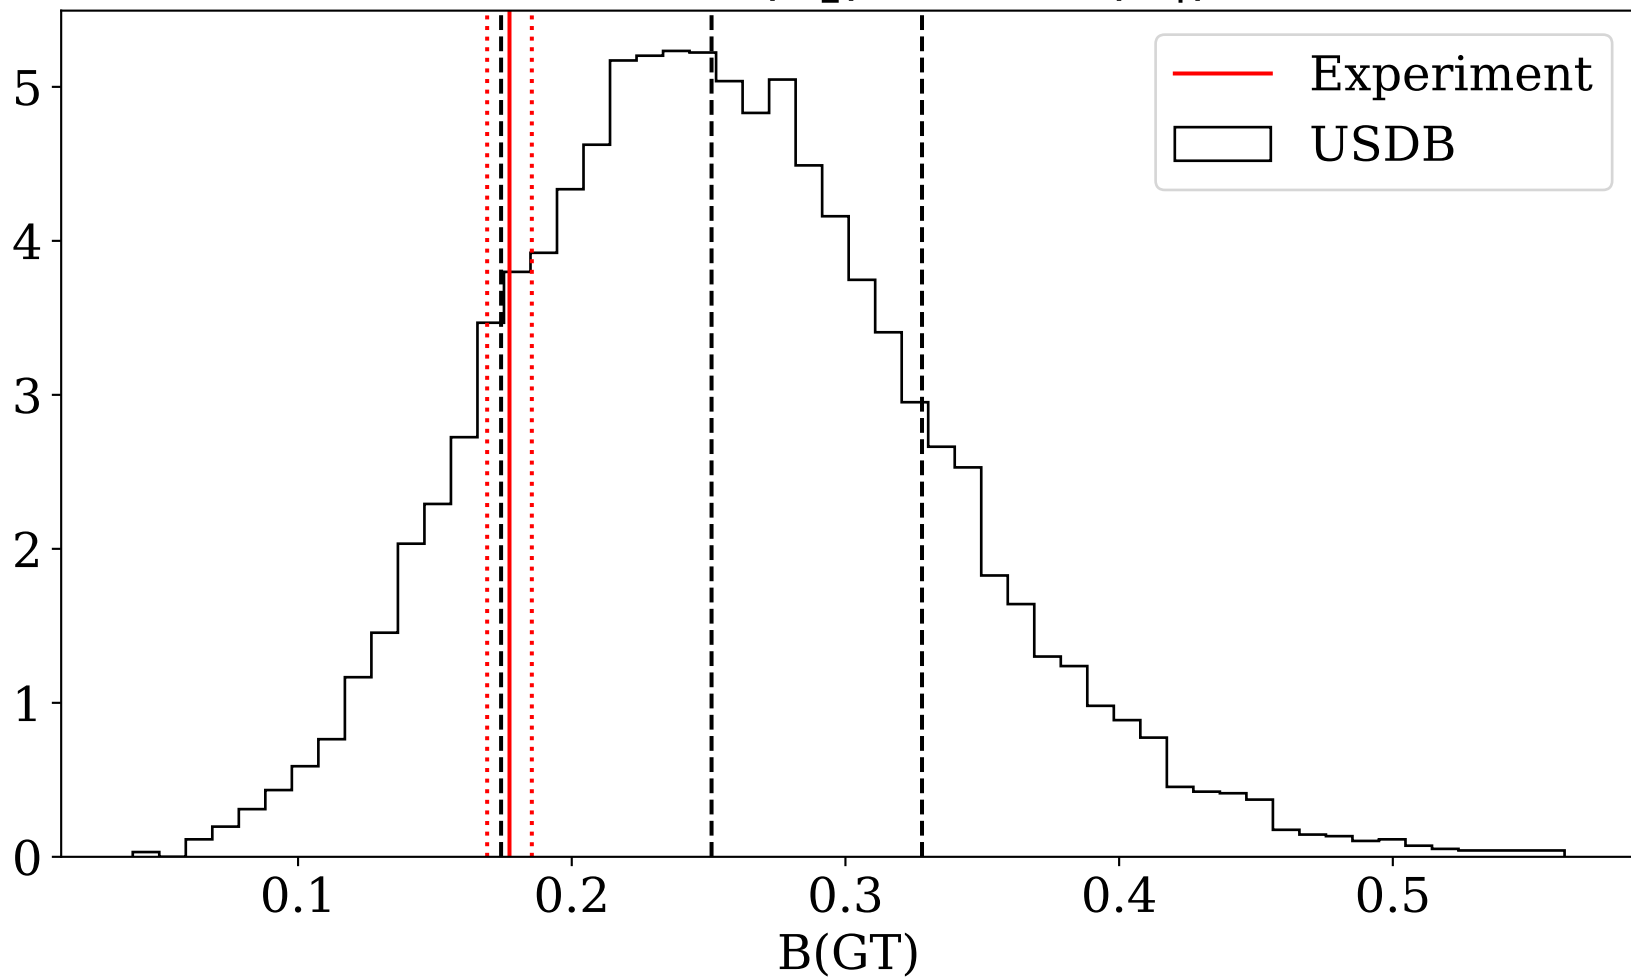

e. c. :  $^{27}\text{Si}(5/2_1) \rightarrow ^{27}\text{Al}(3/2_1)$

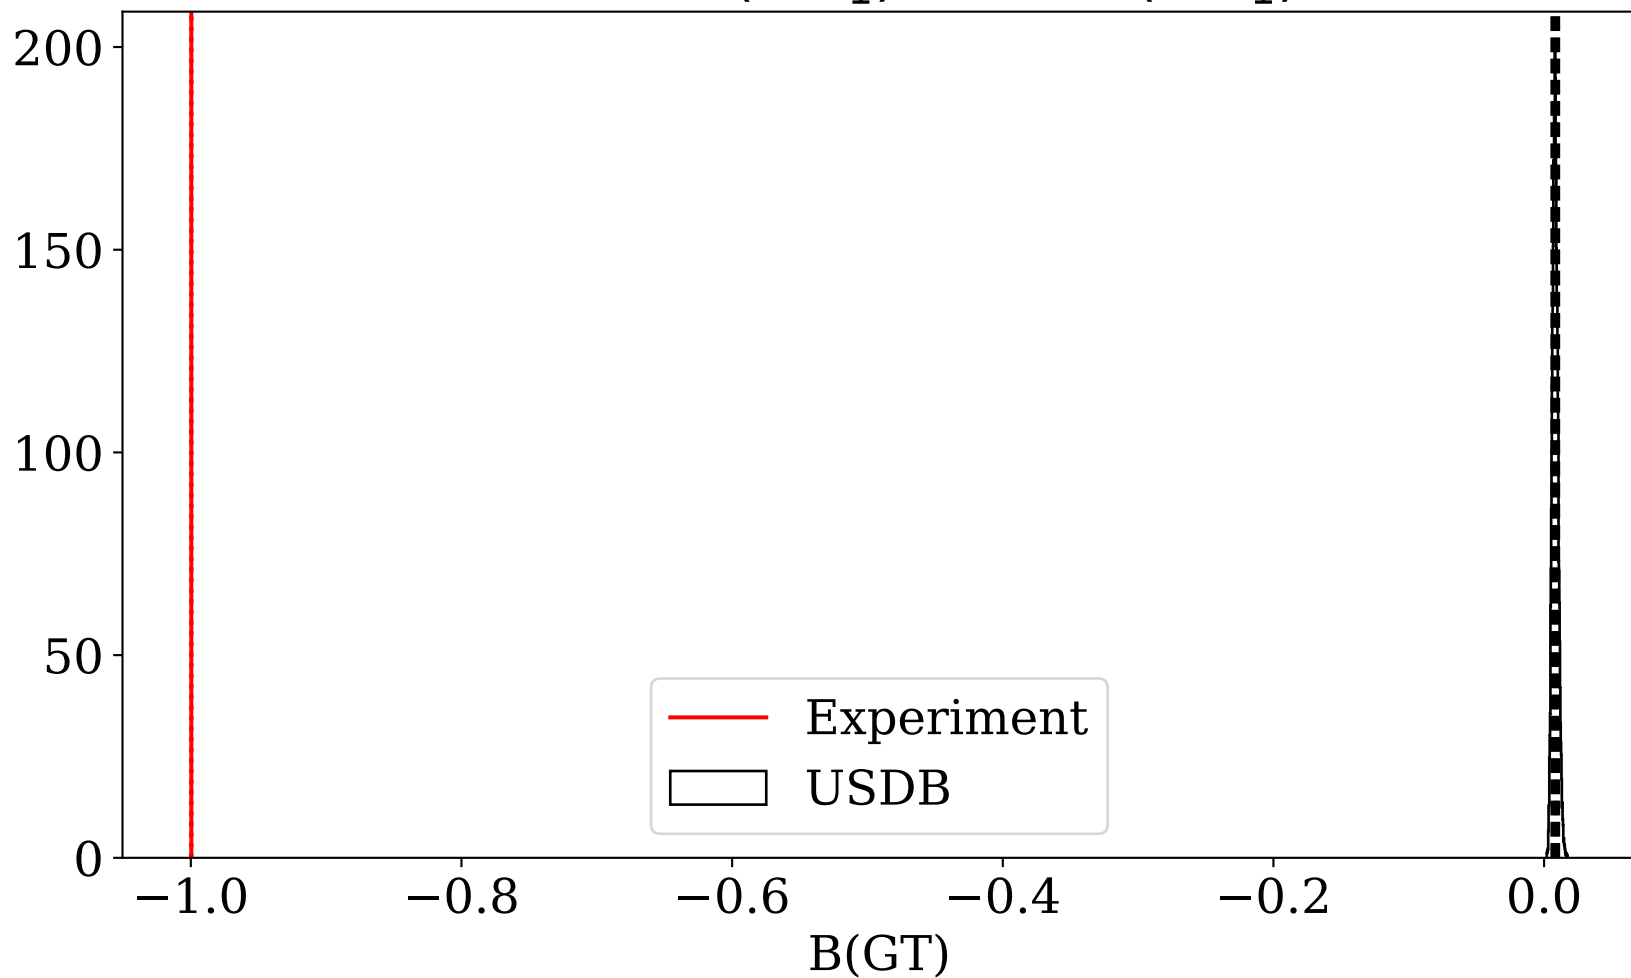

e. c. :  $^{27}\text{Si}(5/2_1) \rightarrow ^{27}\text{Al}(7/2_1)$

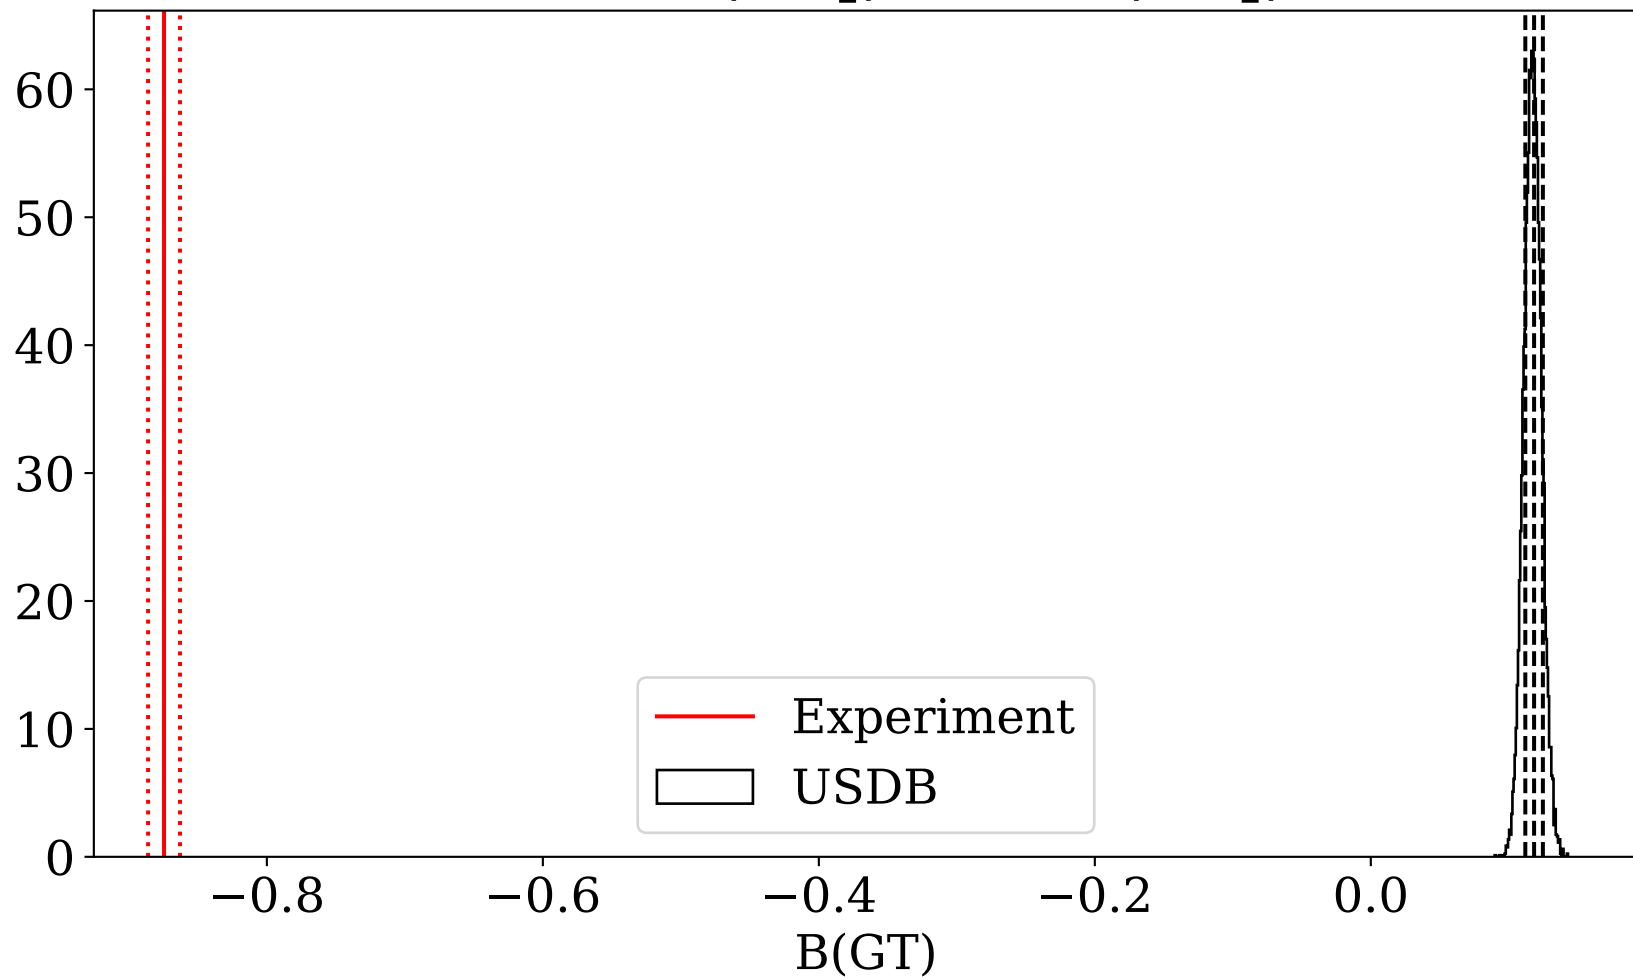

e. c. :  $^{27}\text{Si}(5/2_1) \rightarrow ^{27}\text{Al}(5/2_2)$

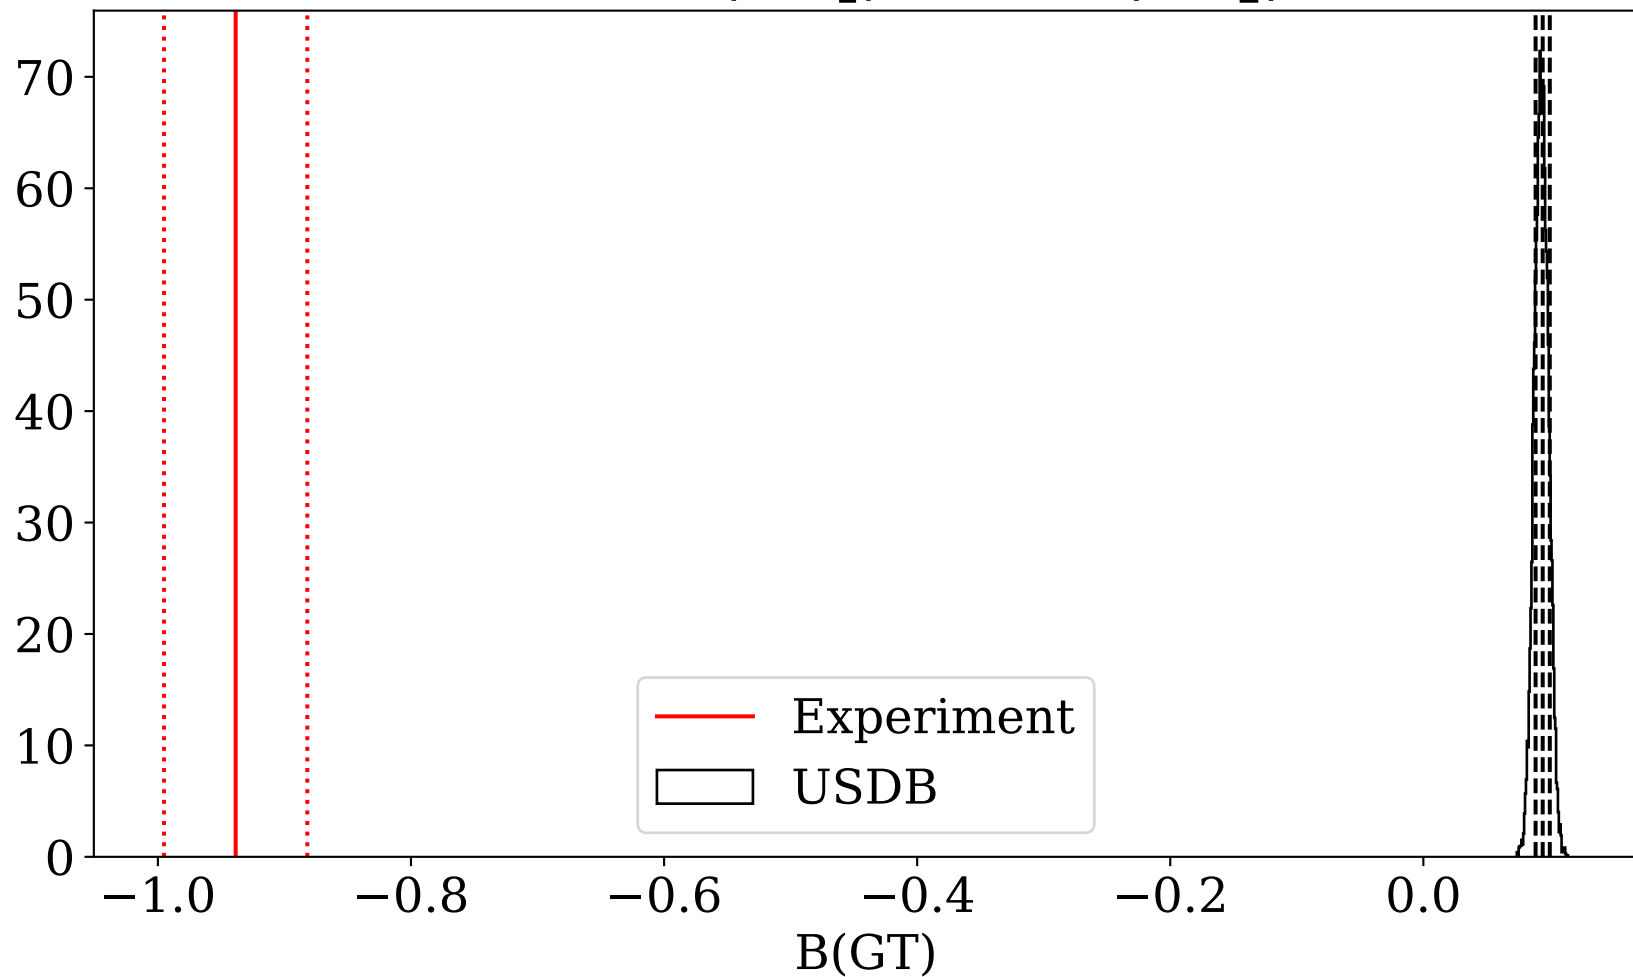

e. c. :  $^{27}\text{Si}(5/2_1) \rightarrow ^{27}\text{Al}(3/2_2)$

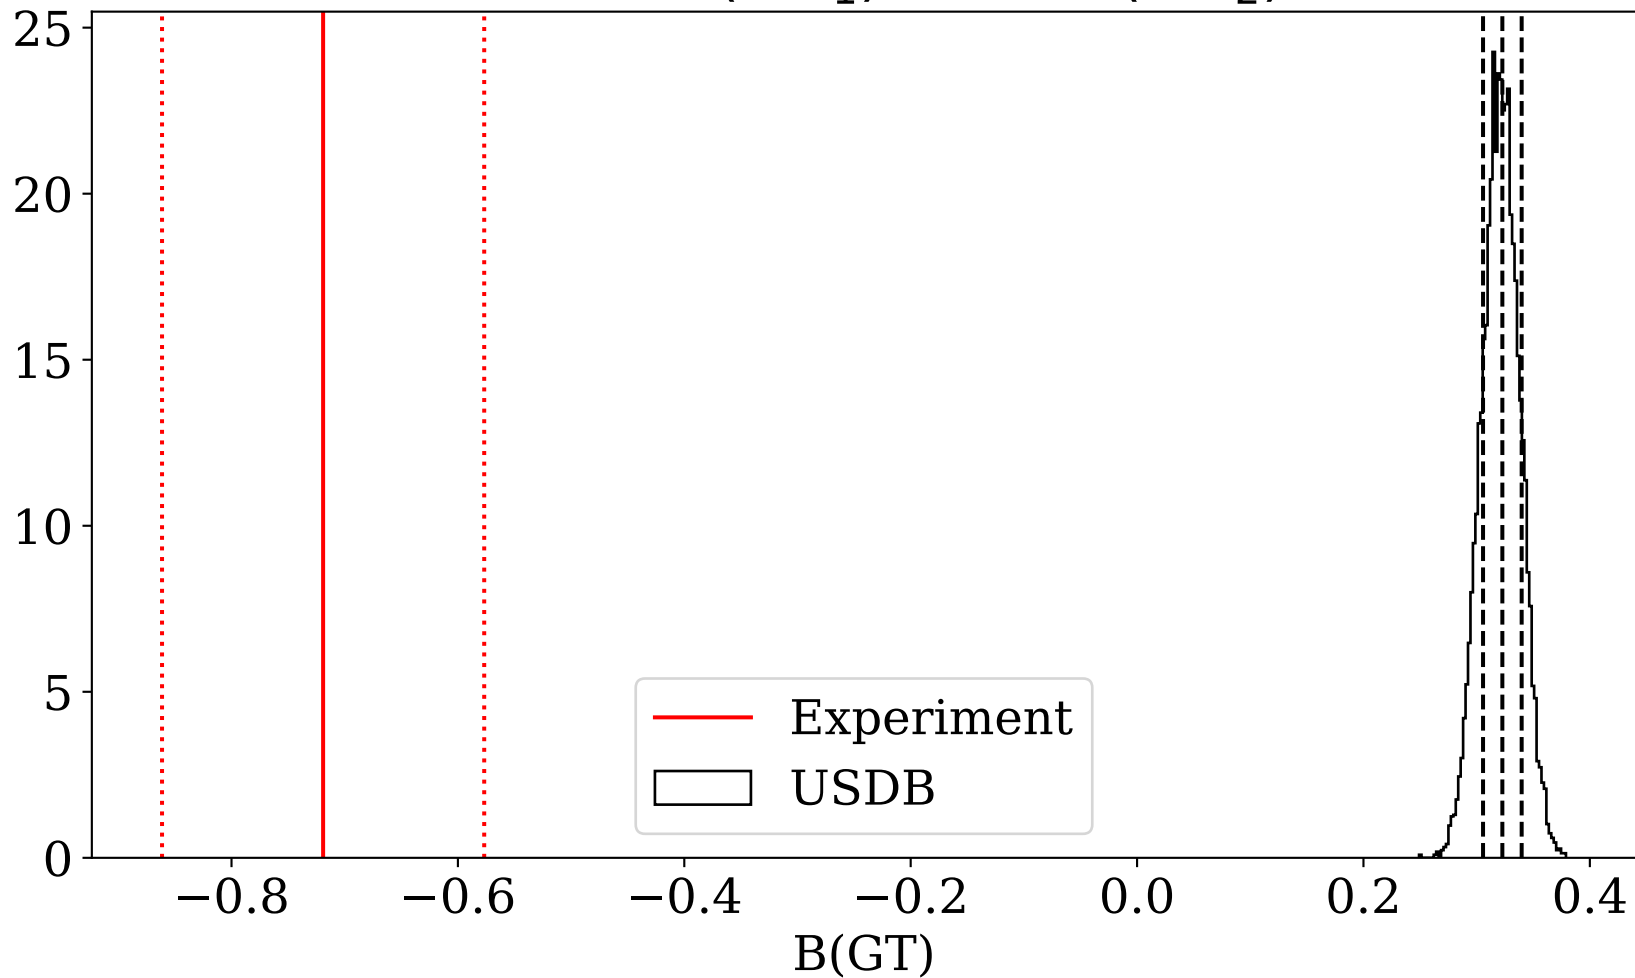

e. c. :  $^{26}\text{P}(3_1) \rightarrow ^{26}\text{Si}(2_1)$

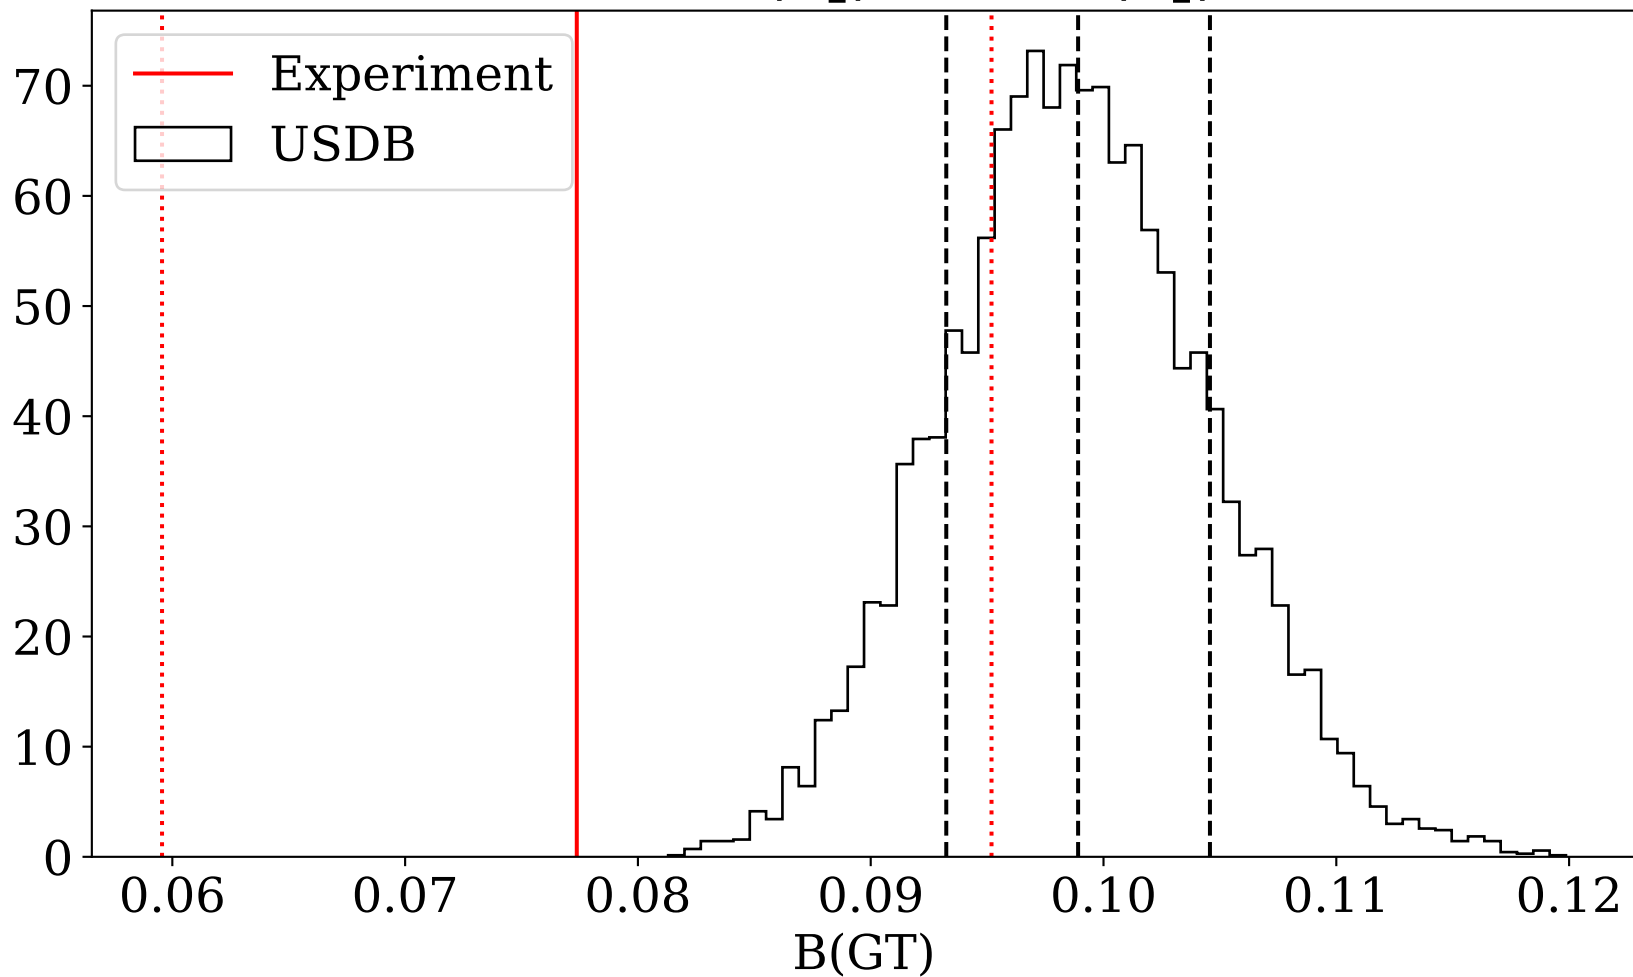

e. c. :  $^{26}\text{P}(3_1) \rightarrow ^{26}\text{Si}(2_2)$

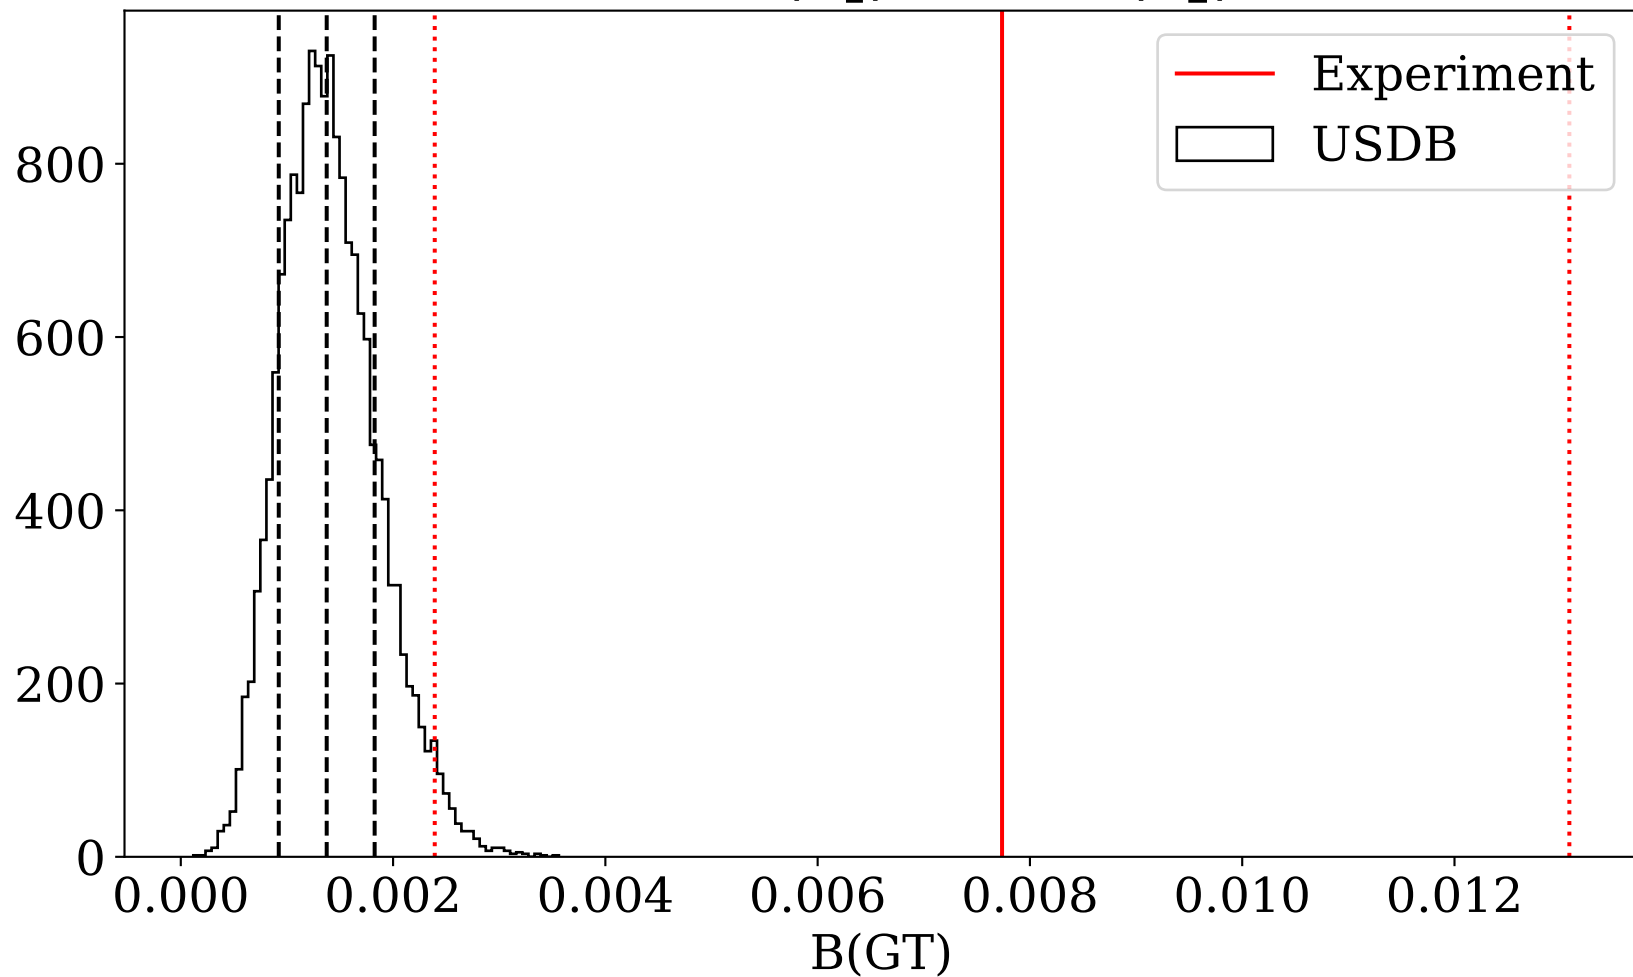



*e. c. :*  $^{26}\text{P}(3_1) \rightarrow ^{26}\text{Si}(3_1)$

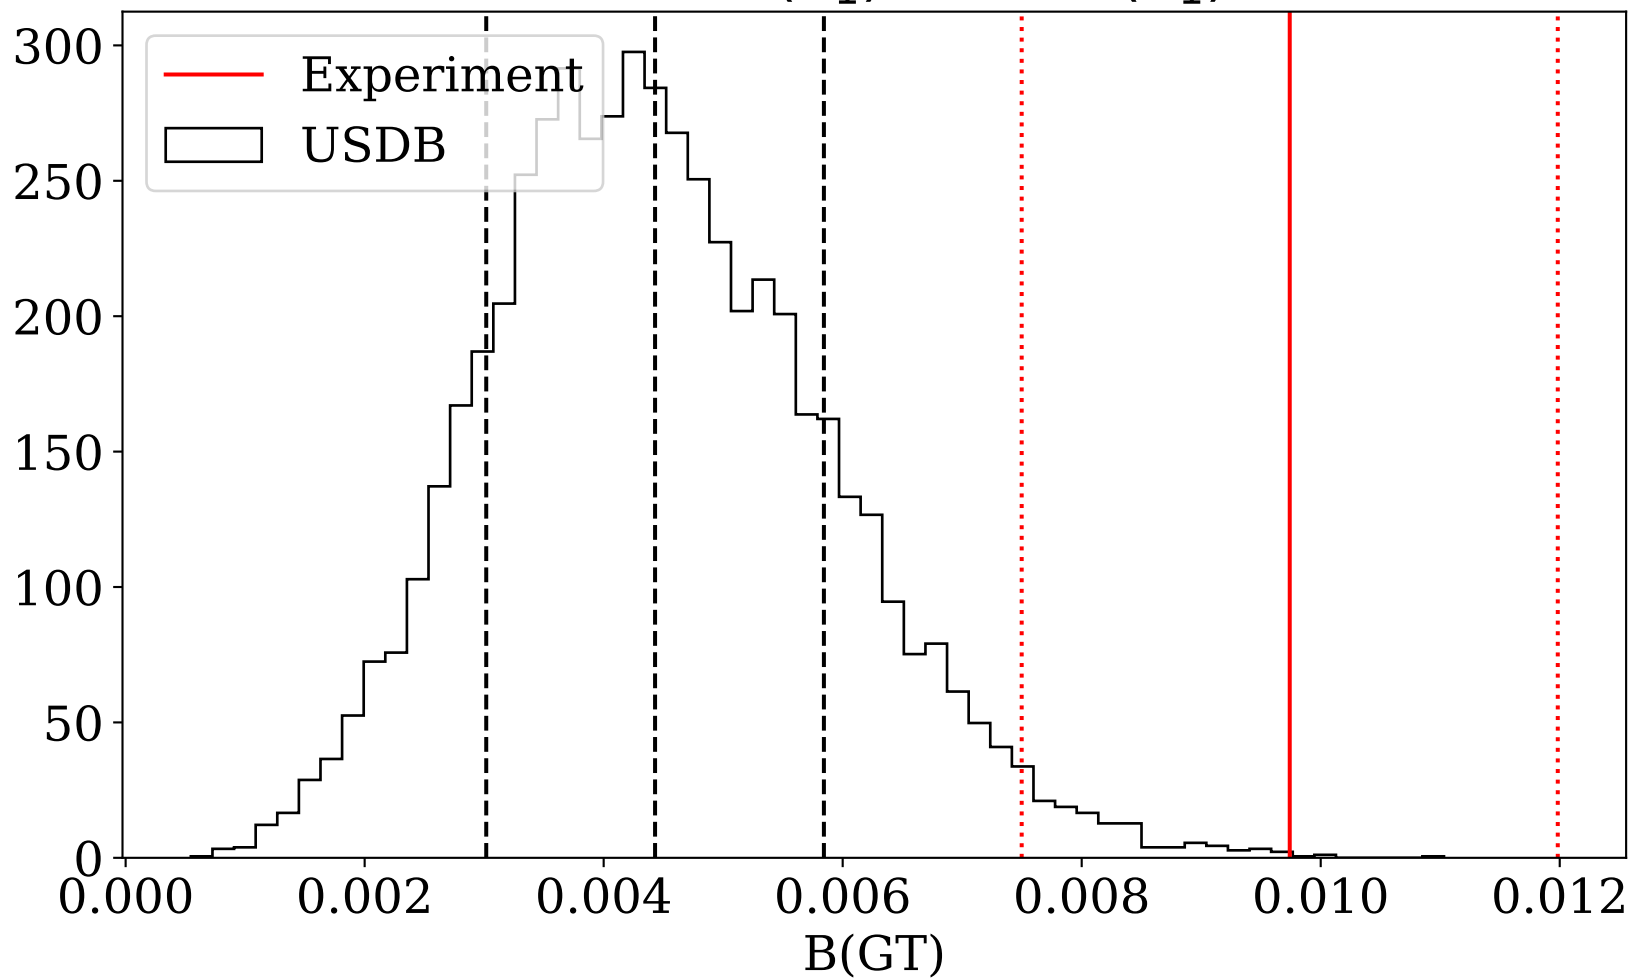

*e. c.* :  $^{26}\text{P}(3_1) \rightarrow ^{26}\text{Si}(4_1)$

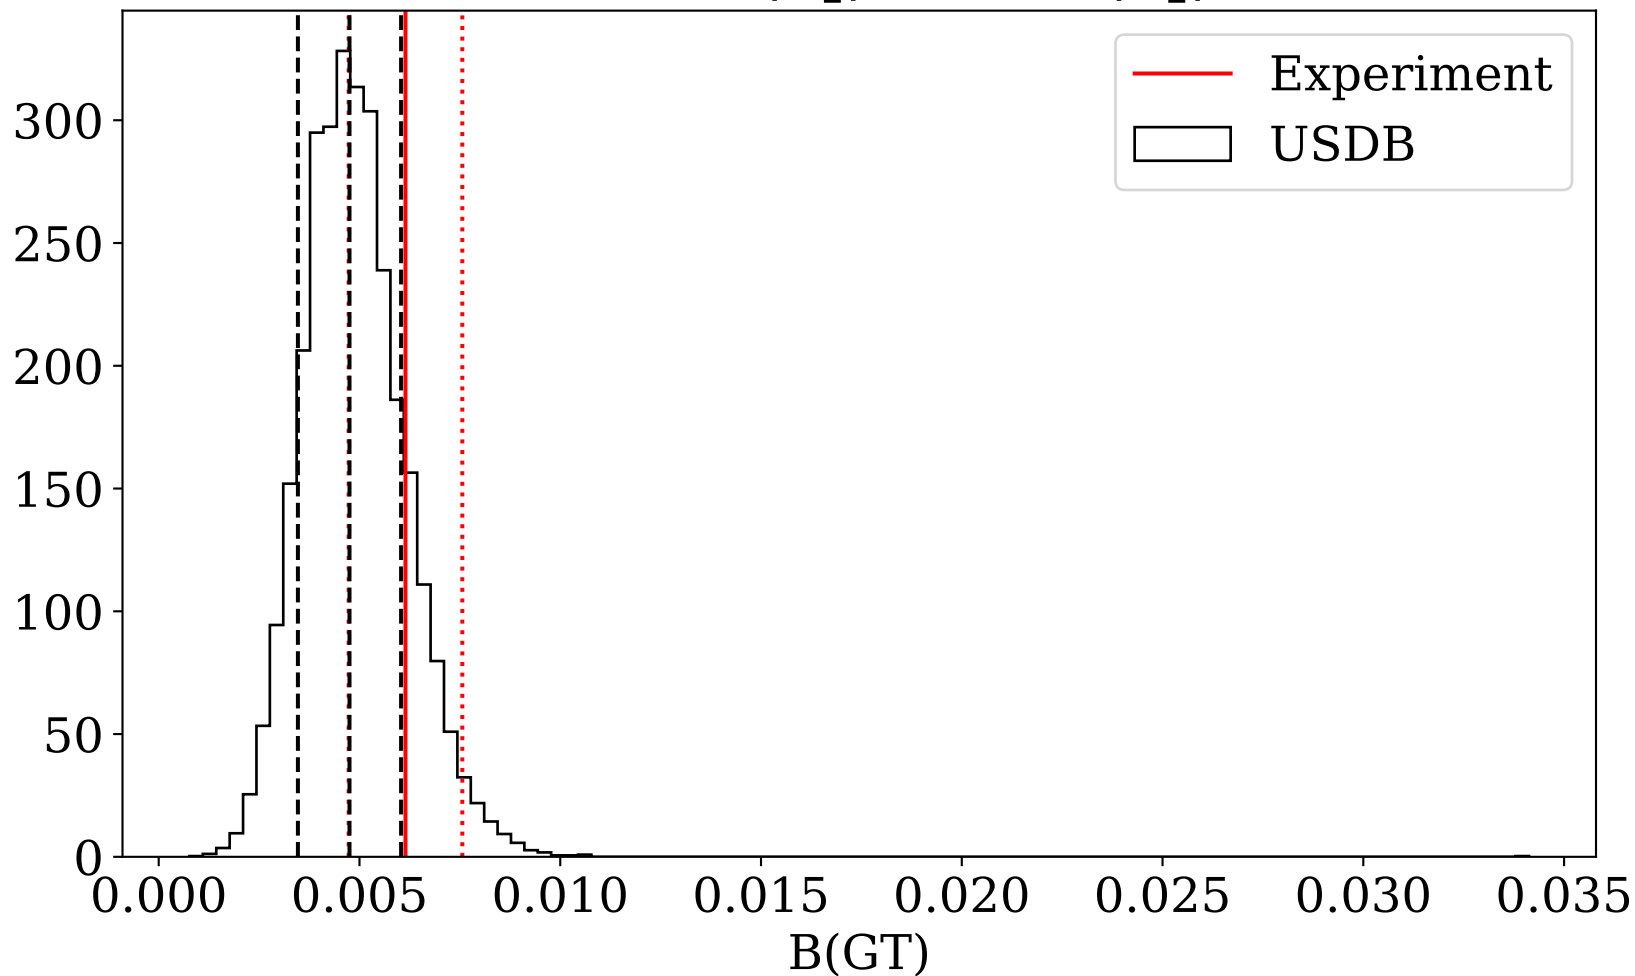

*e. c. :*  $^{26}\text{P}(3_1) \rightarrow ^{26}\text{Si}(2_3)$

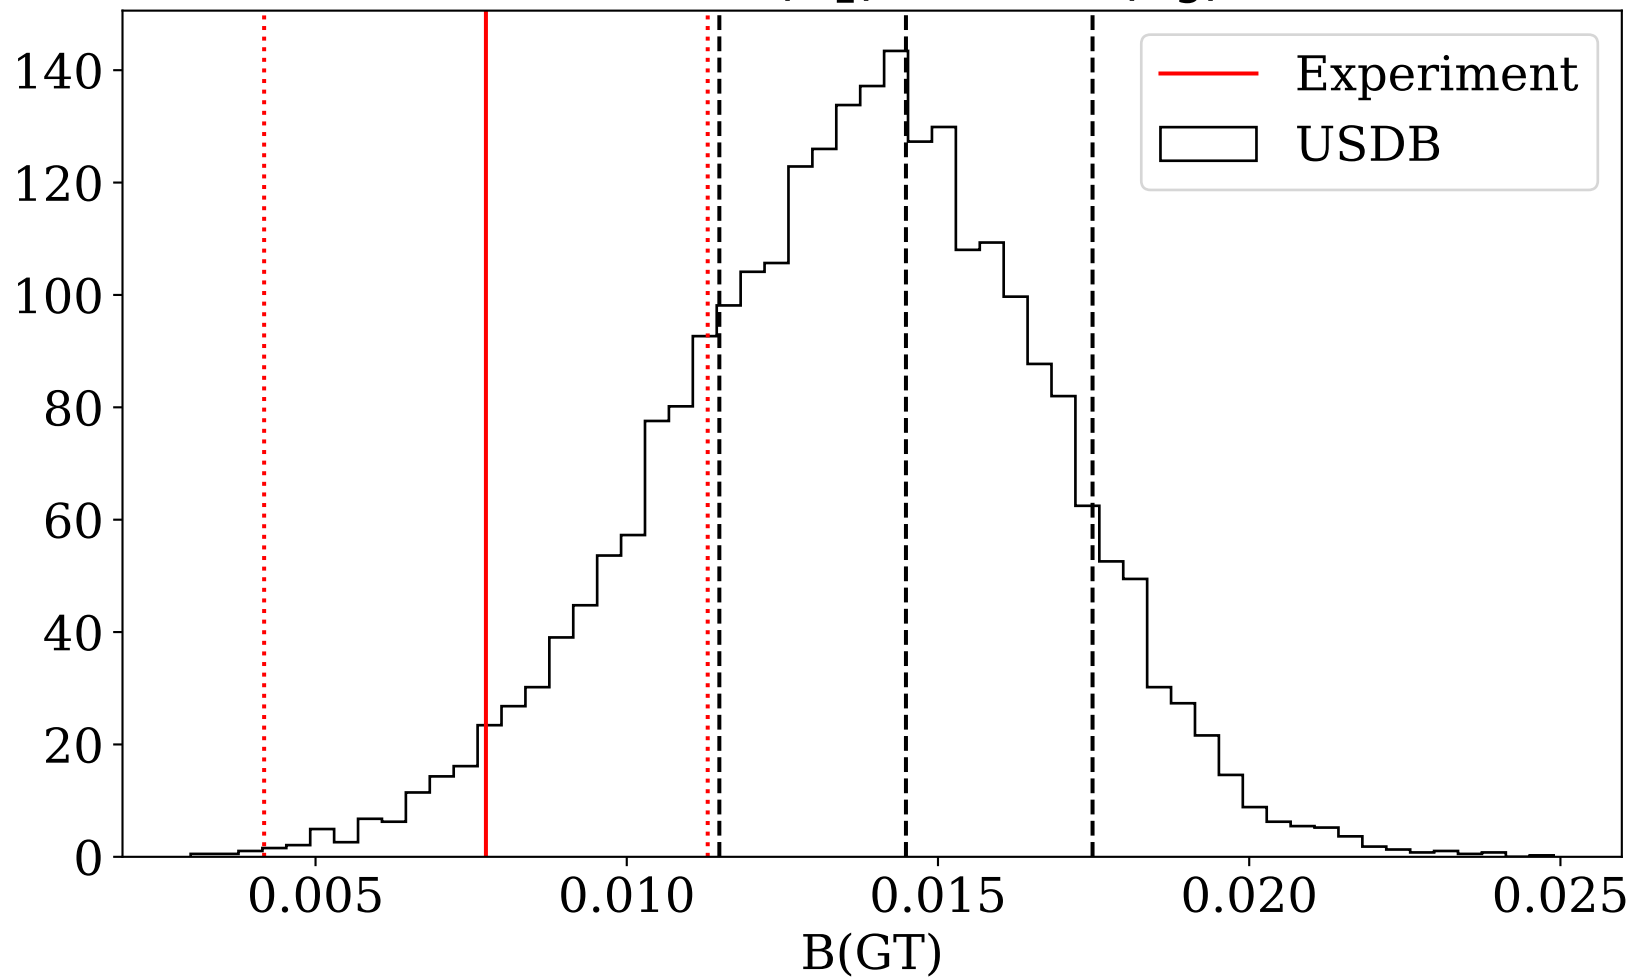

e. c. :  $^{28}\text{P}(3_1) \rightarrow ^{28}\text{Si}(2_1)$

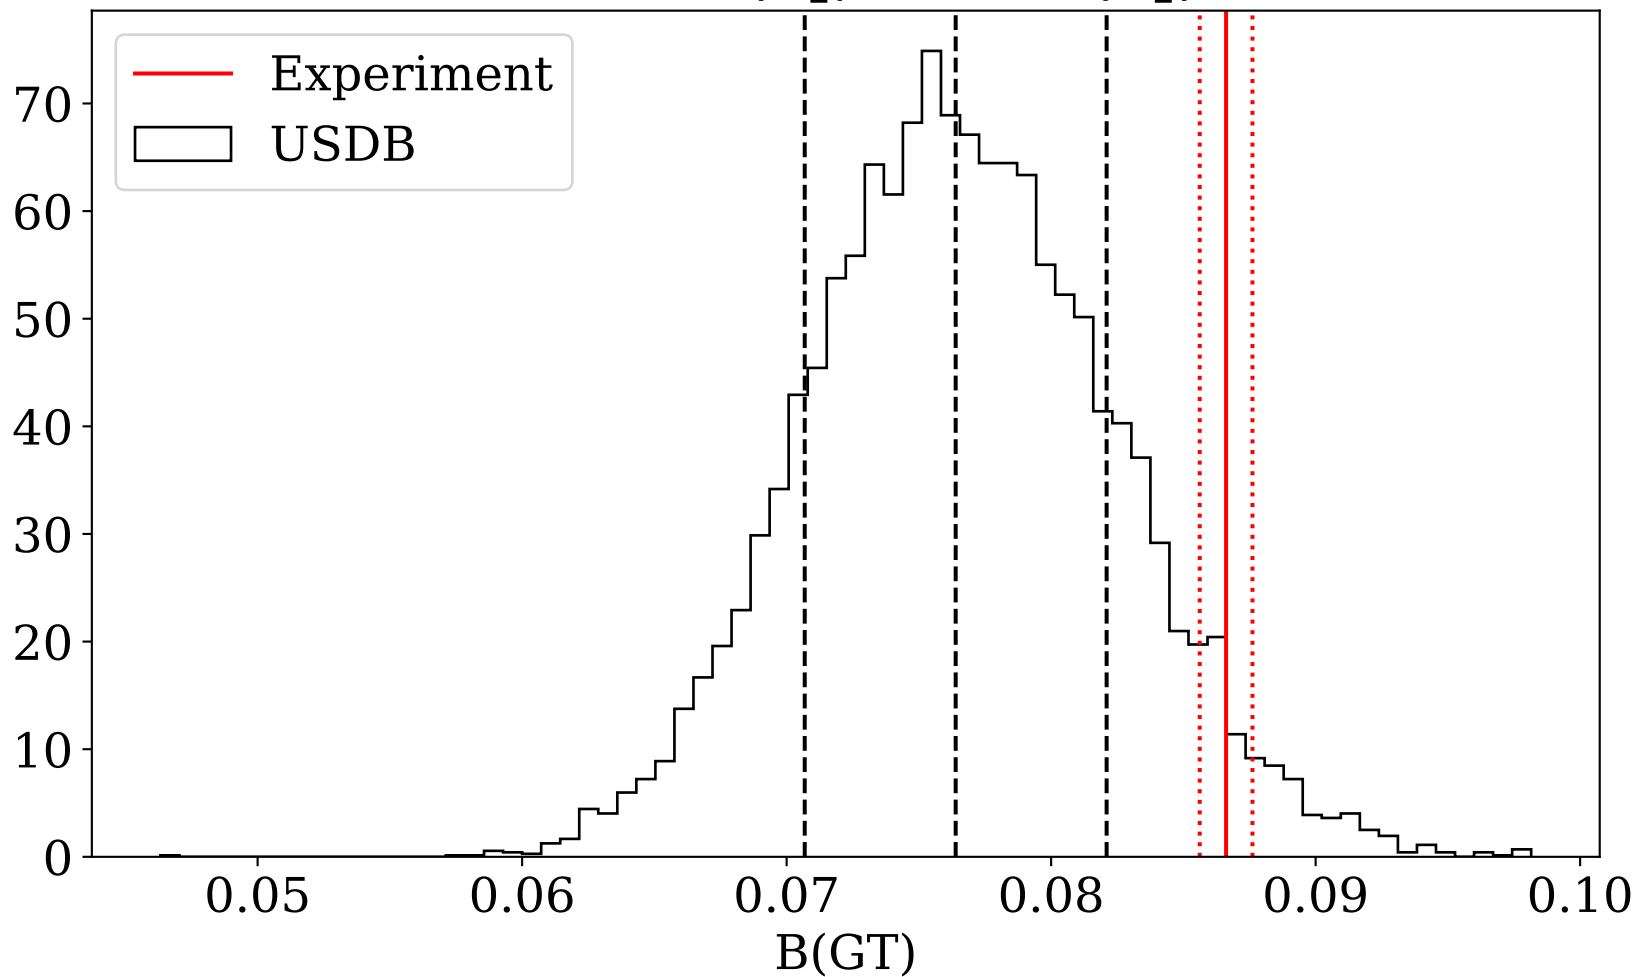

e. c. :  $^{28}\text{P}(3_1) \rightarrow ^{28}\text{Si}(4_1)$

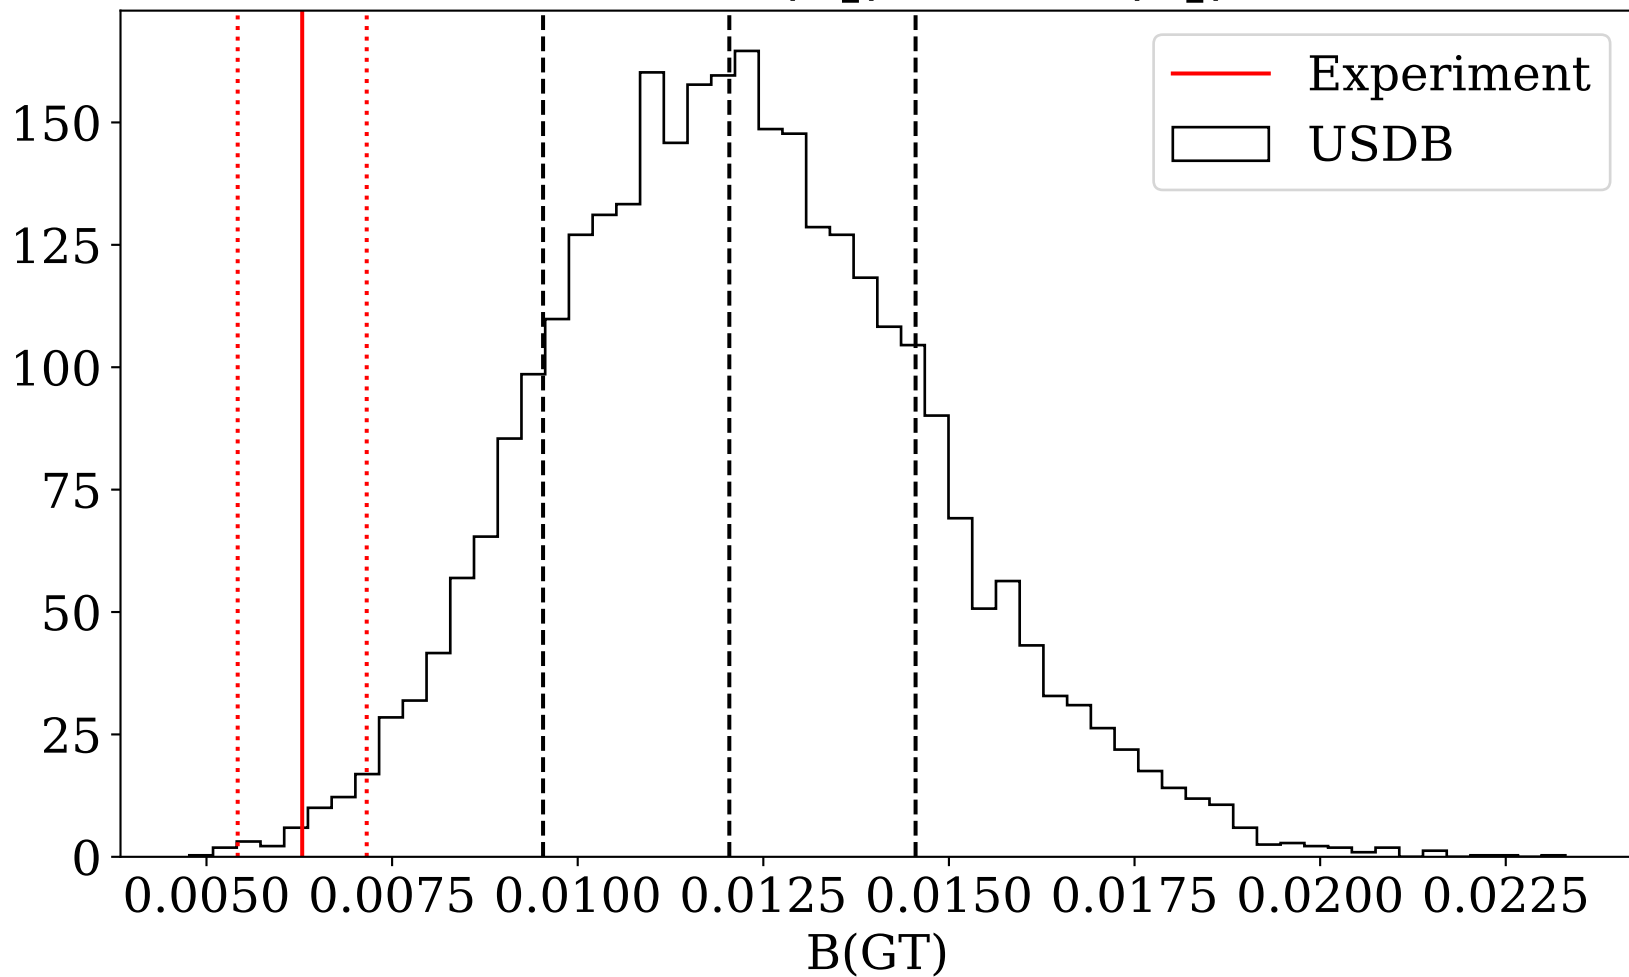

e. c. :  $^{28}\text{P}(3_1) \rightarrow ^{28}\text{Si}(3_1)$

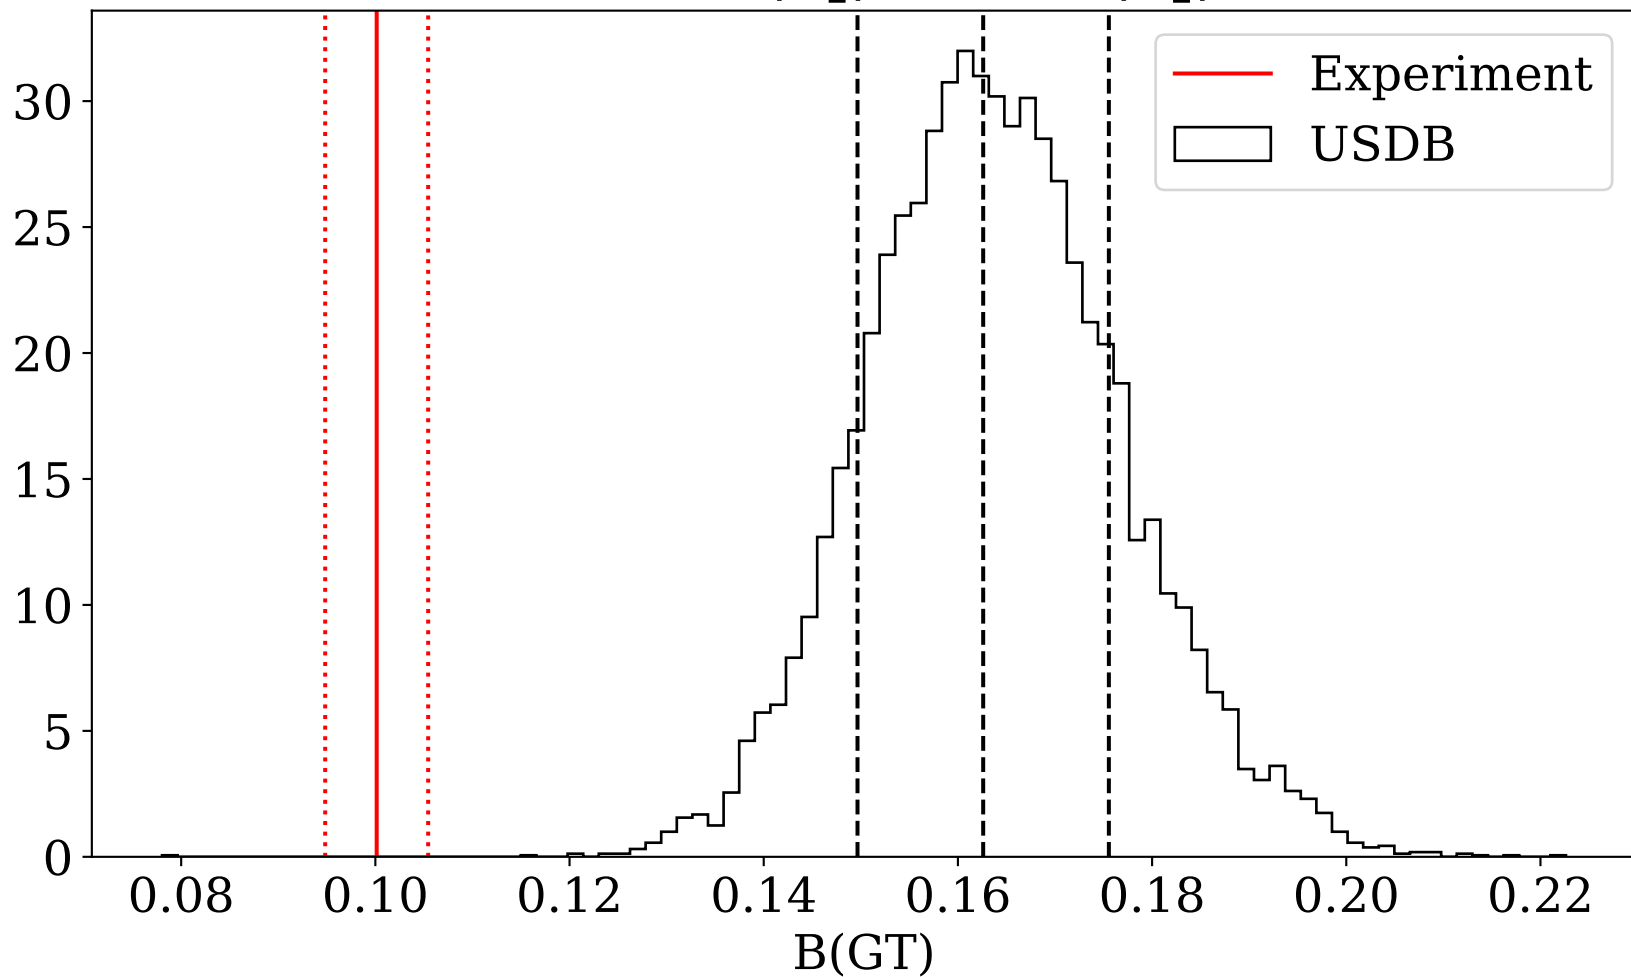

e. c. :  $^{29}\text{P}(1/2_1) \rightarrow ^{29}\text{Si}(1/2_1)$

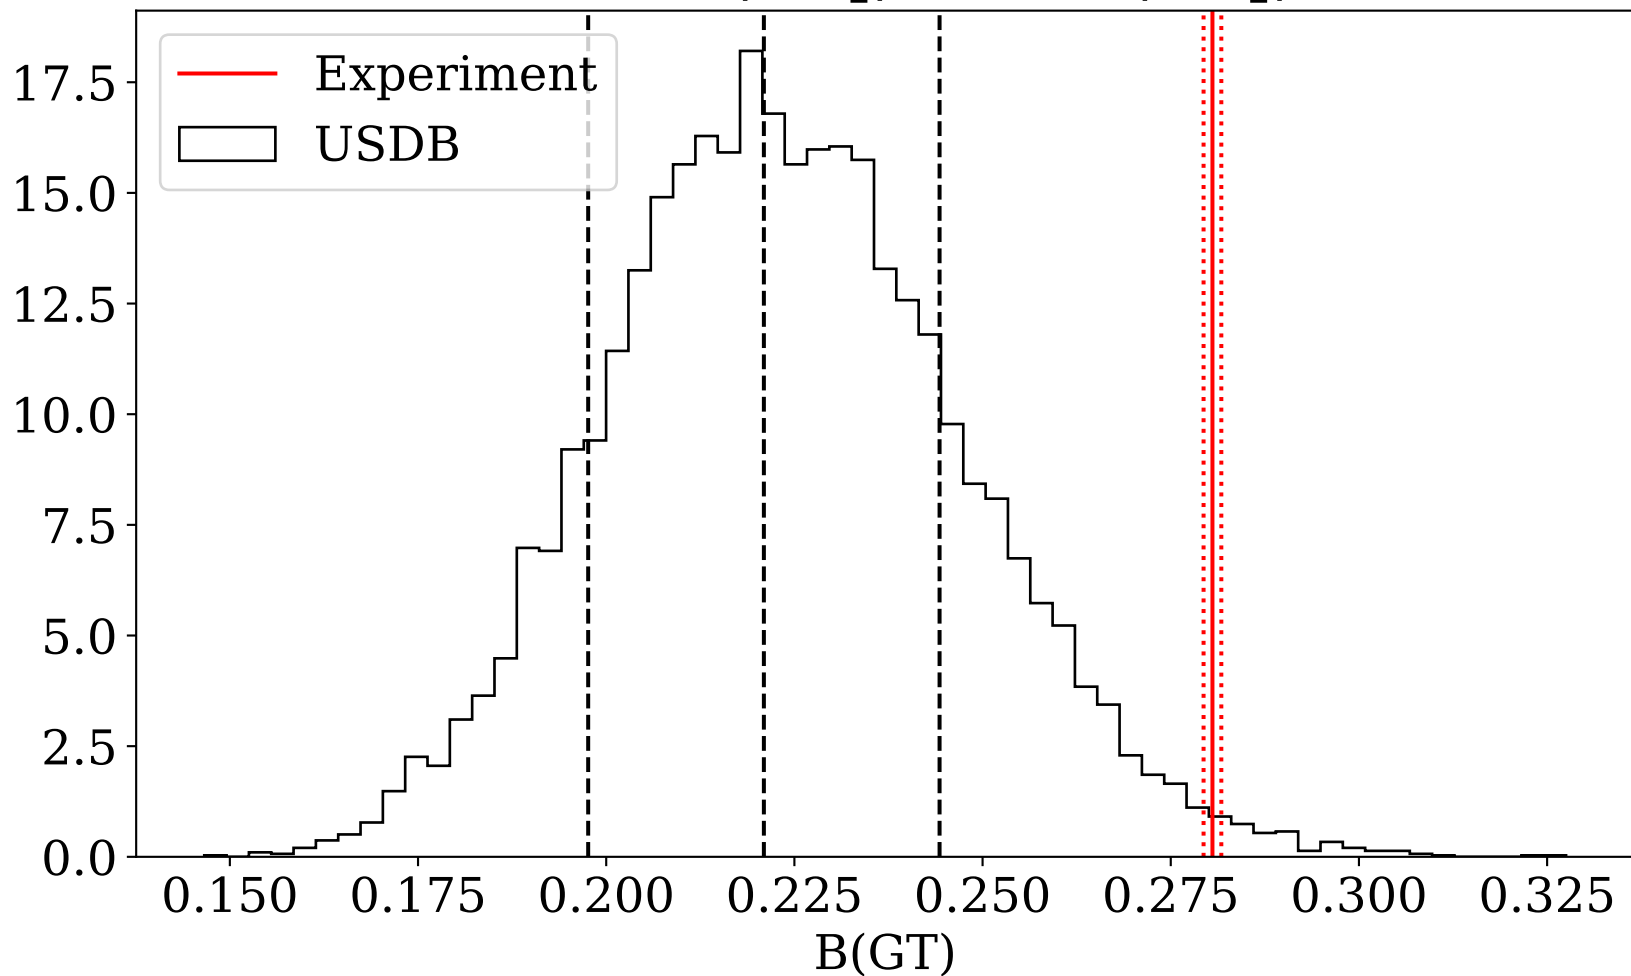

e. c. :  $^{29}\text{P}(1/2_1) \rightarrow ^{29}\text{Si}(3/2_1)$

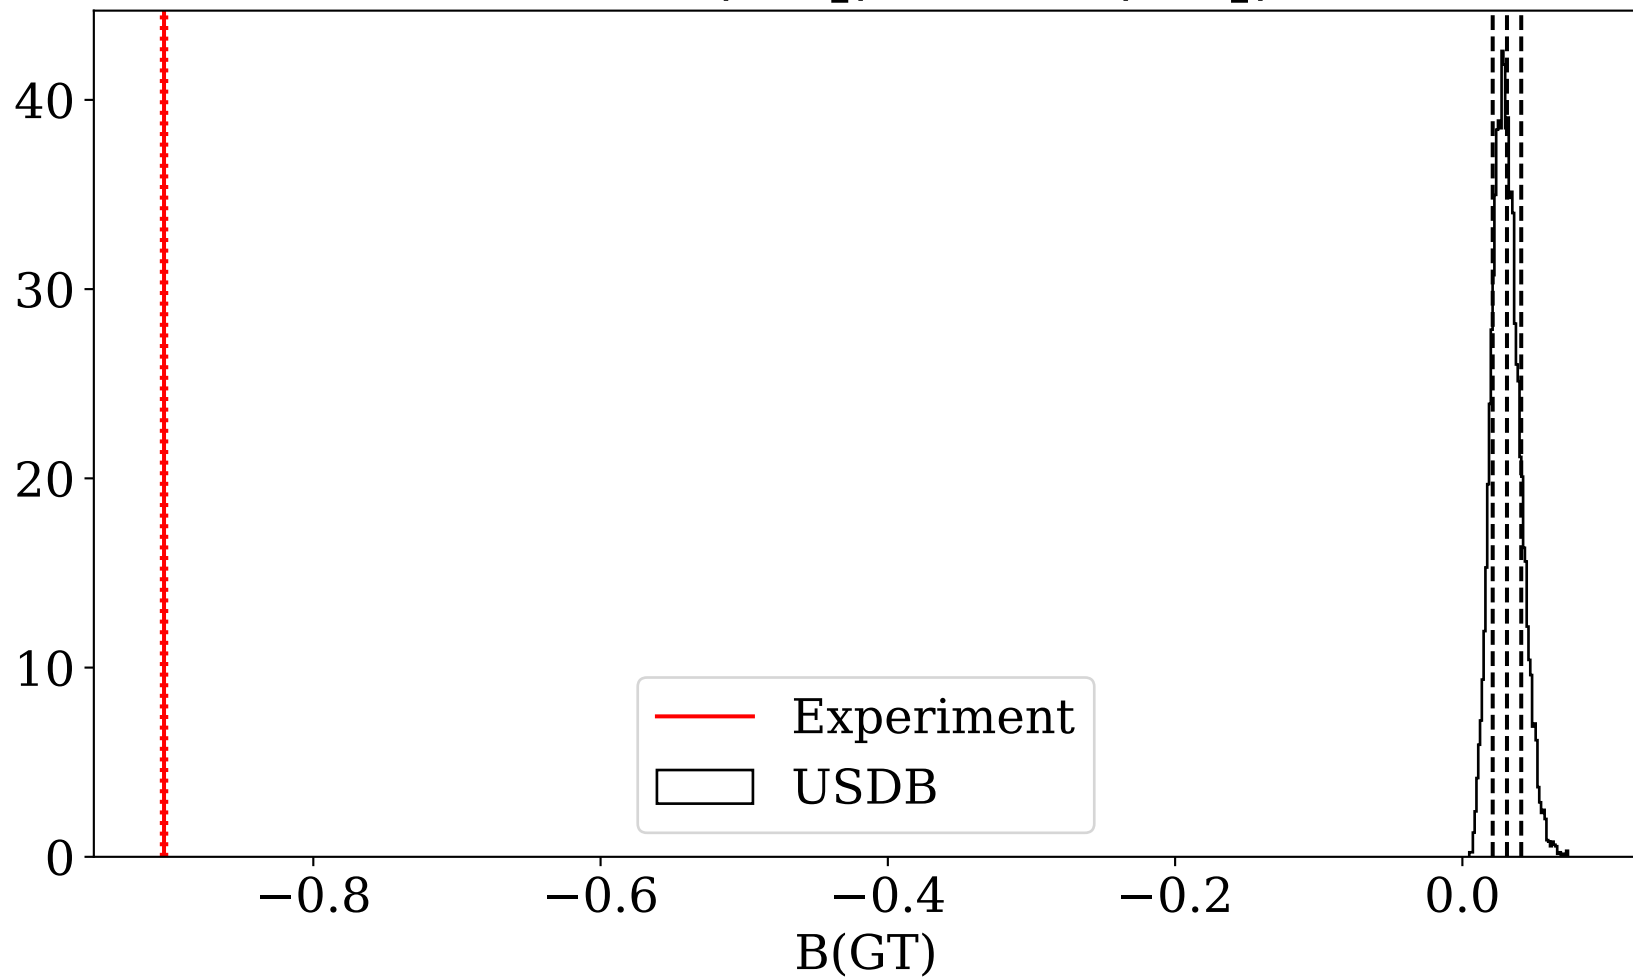



e. c. :  $^{29}\text{P}(1/2_1) \rightarrow ^{29}\text{Si}(3/2_2)$

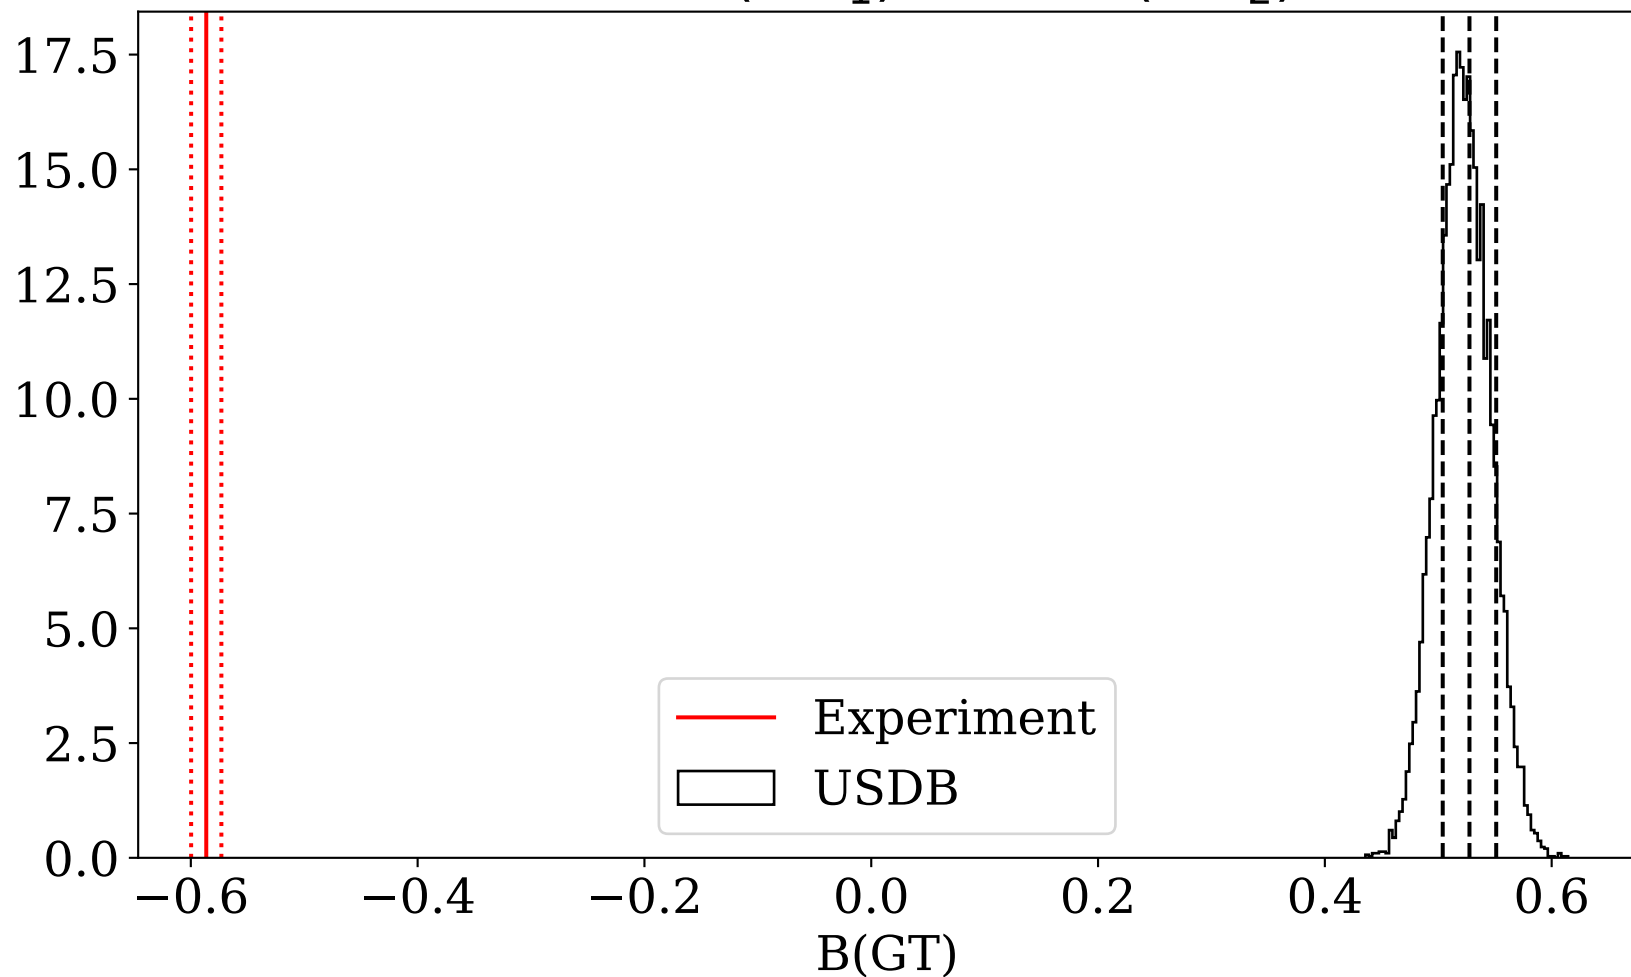

*e. c.*:  $^{30}\text{P}(1_1) \rightarrow ^{30}\text{Si}(0_1)$

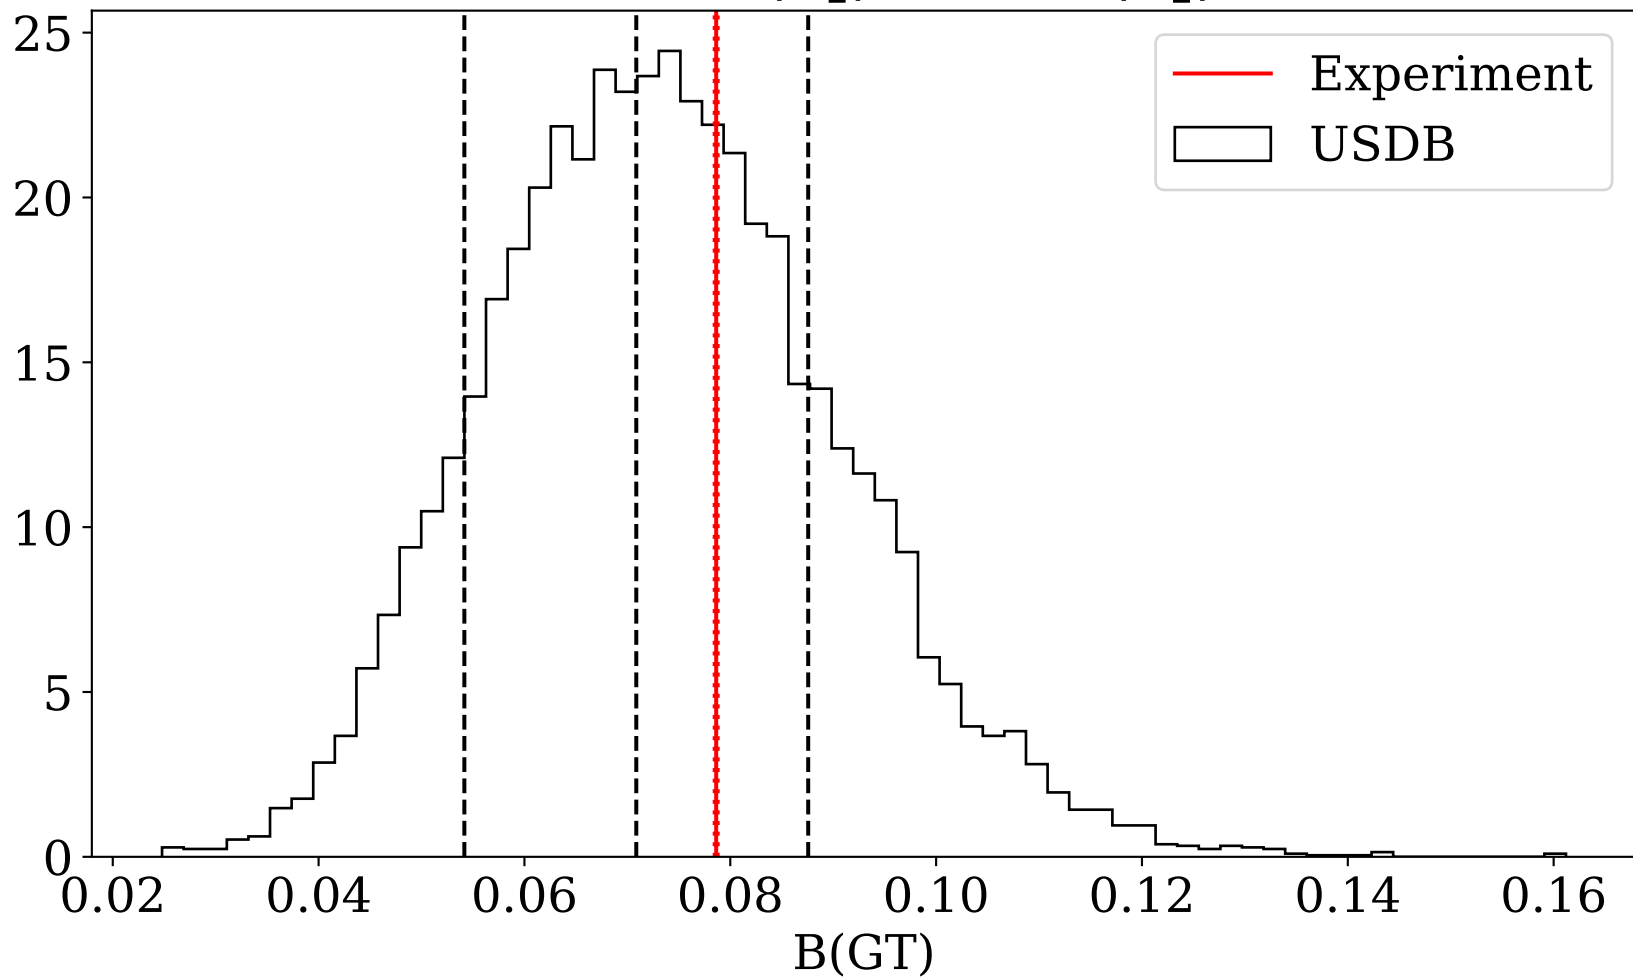

e. c. :  $^{30}\text{P}(1_1) \rightarrow ^{30}\text{Si}(2_1)$

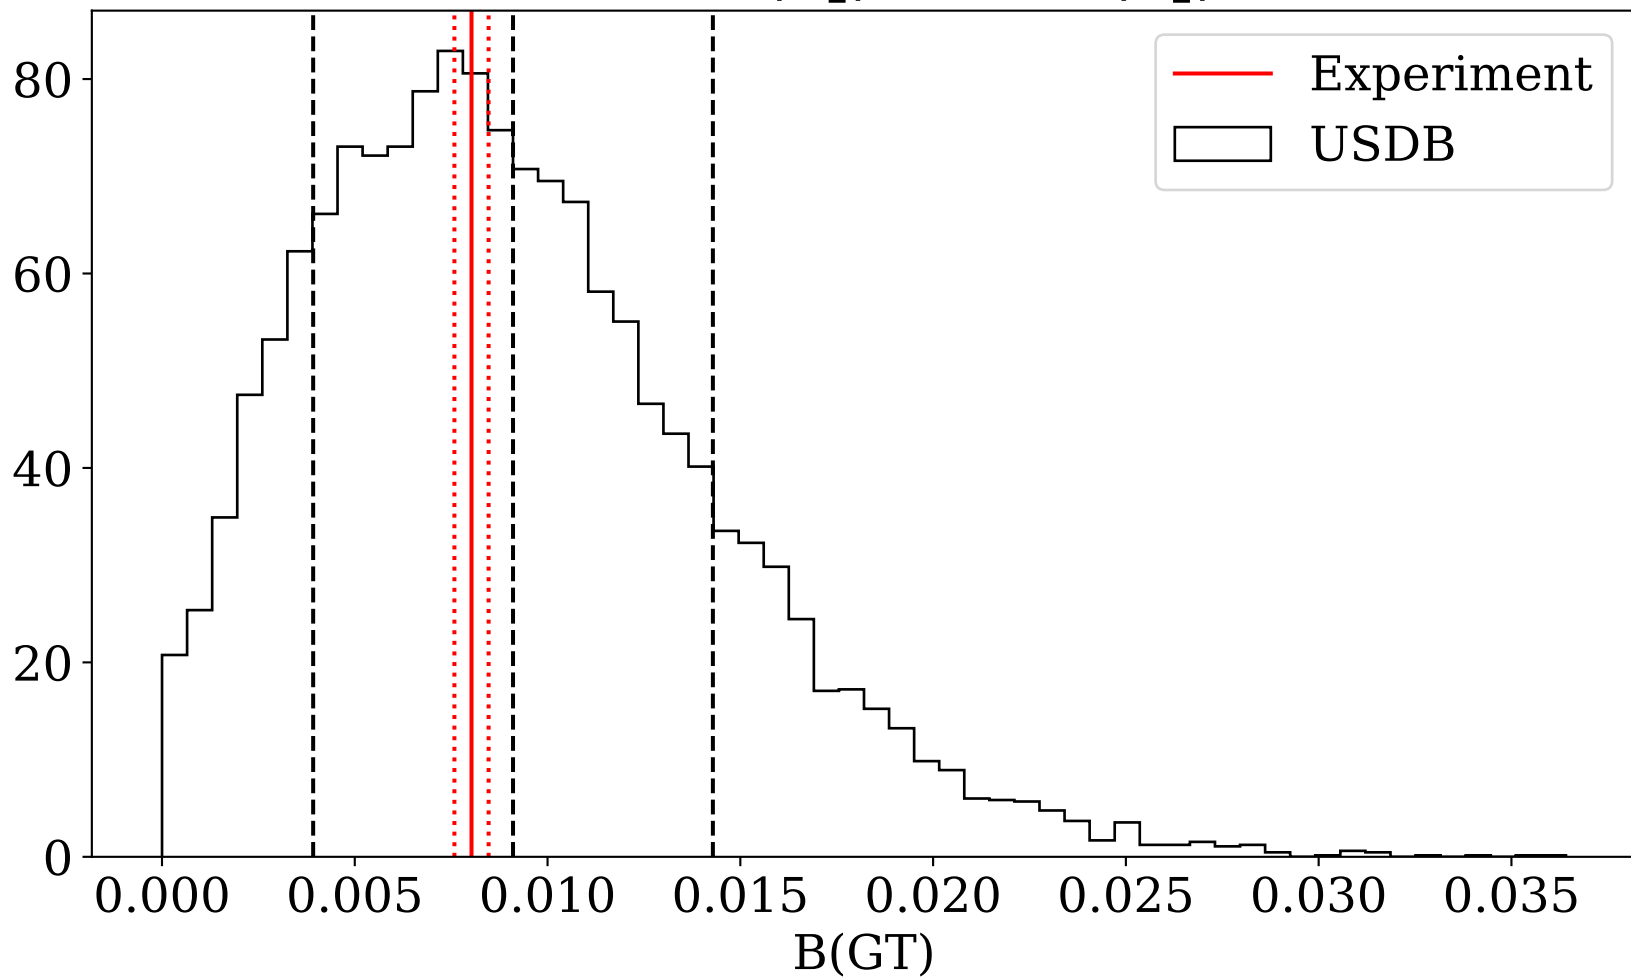

*e. c.* :  $^{30}\text{P}(1_1) \rightarrow ^{30}\text{Si}(2_2)$

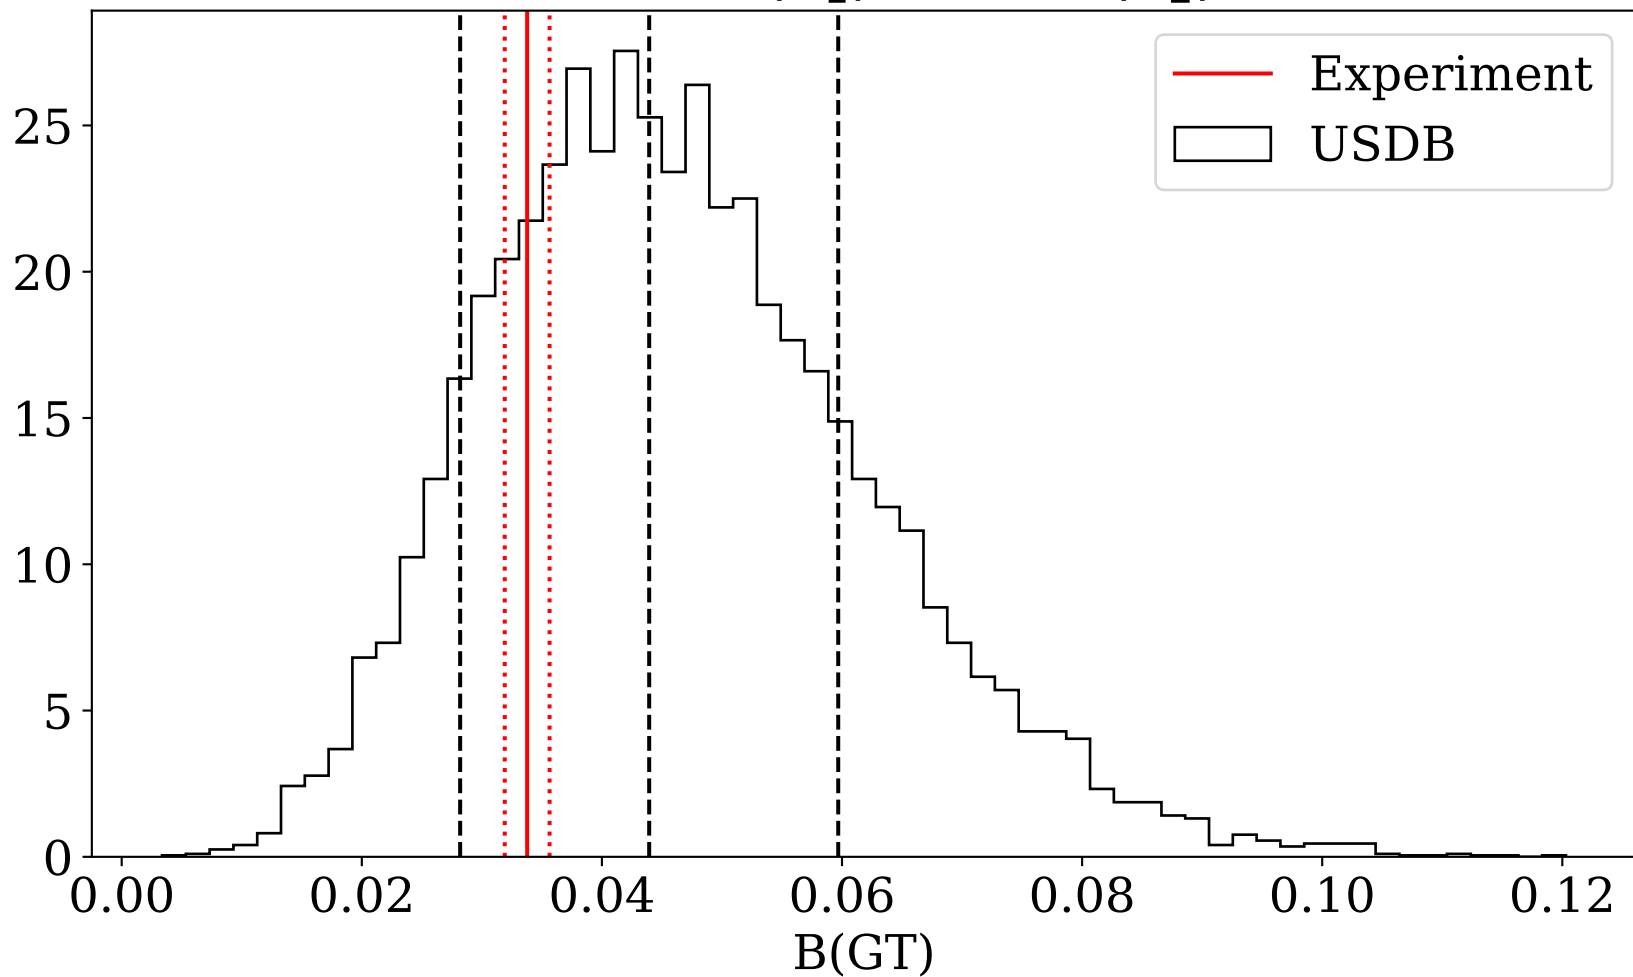

*e. c. :*  $^{30}\text{P}(1_1) \rightarrow ^{30}\text{Si}(0_2)$

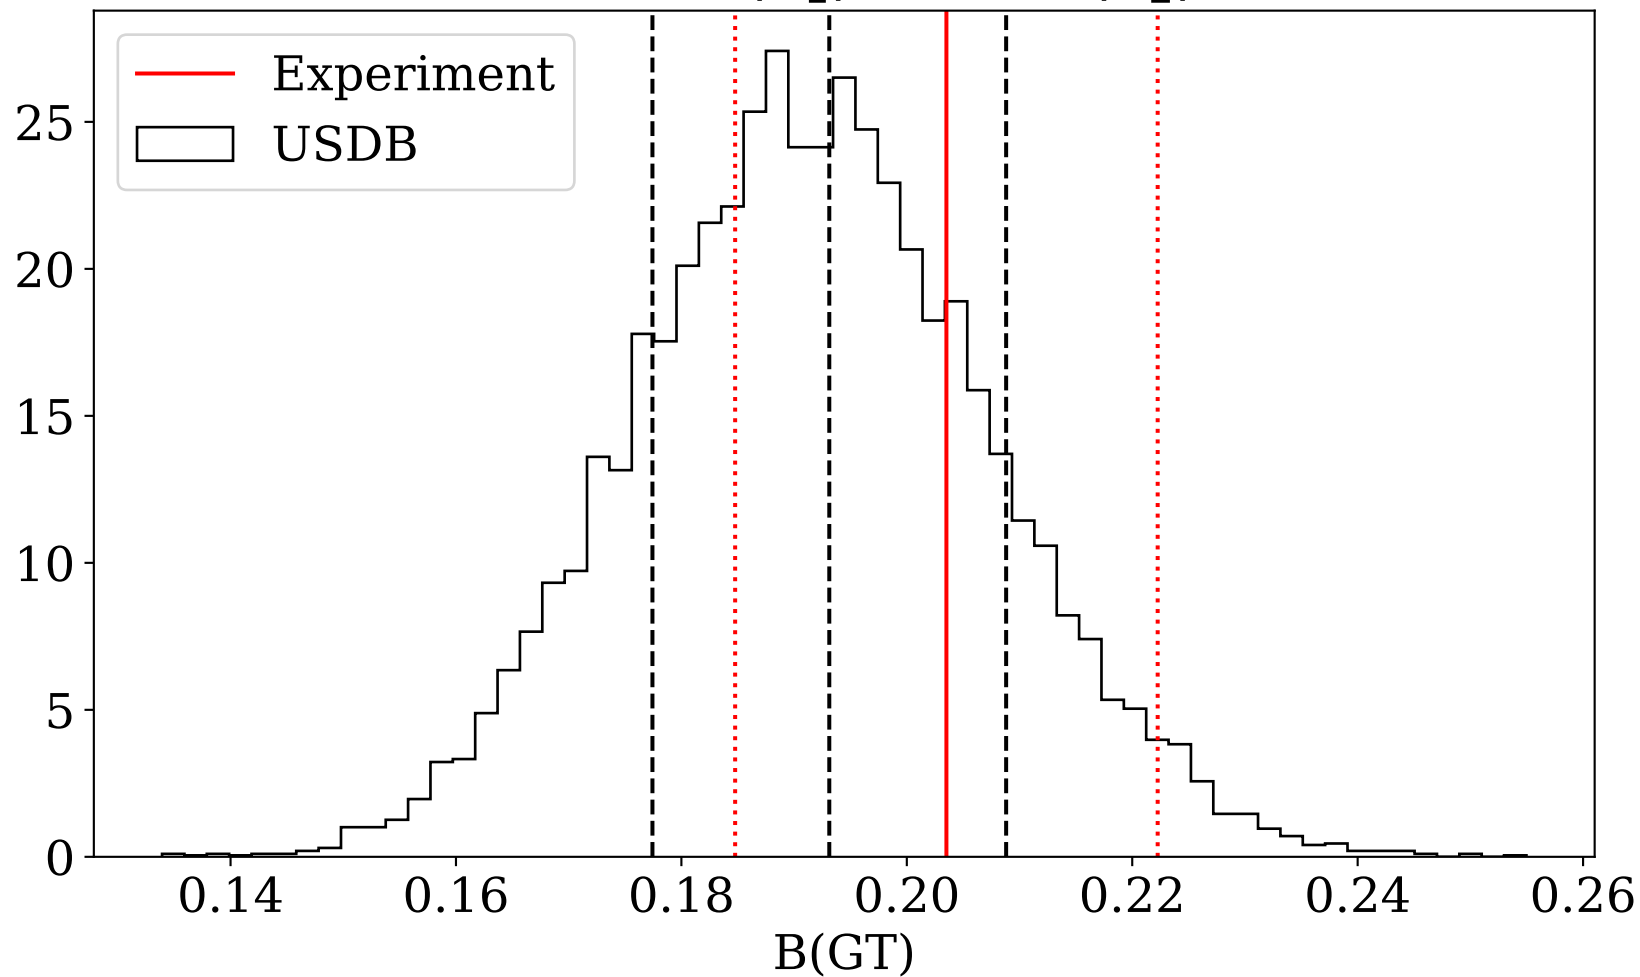

e. c. :  $^{30}\text{S}(0_1) \rightarrow ^{30}\text{P}(1_1)$

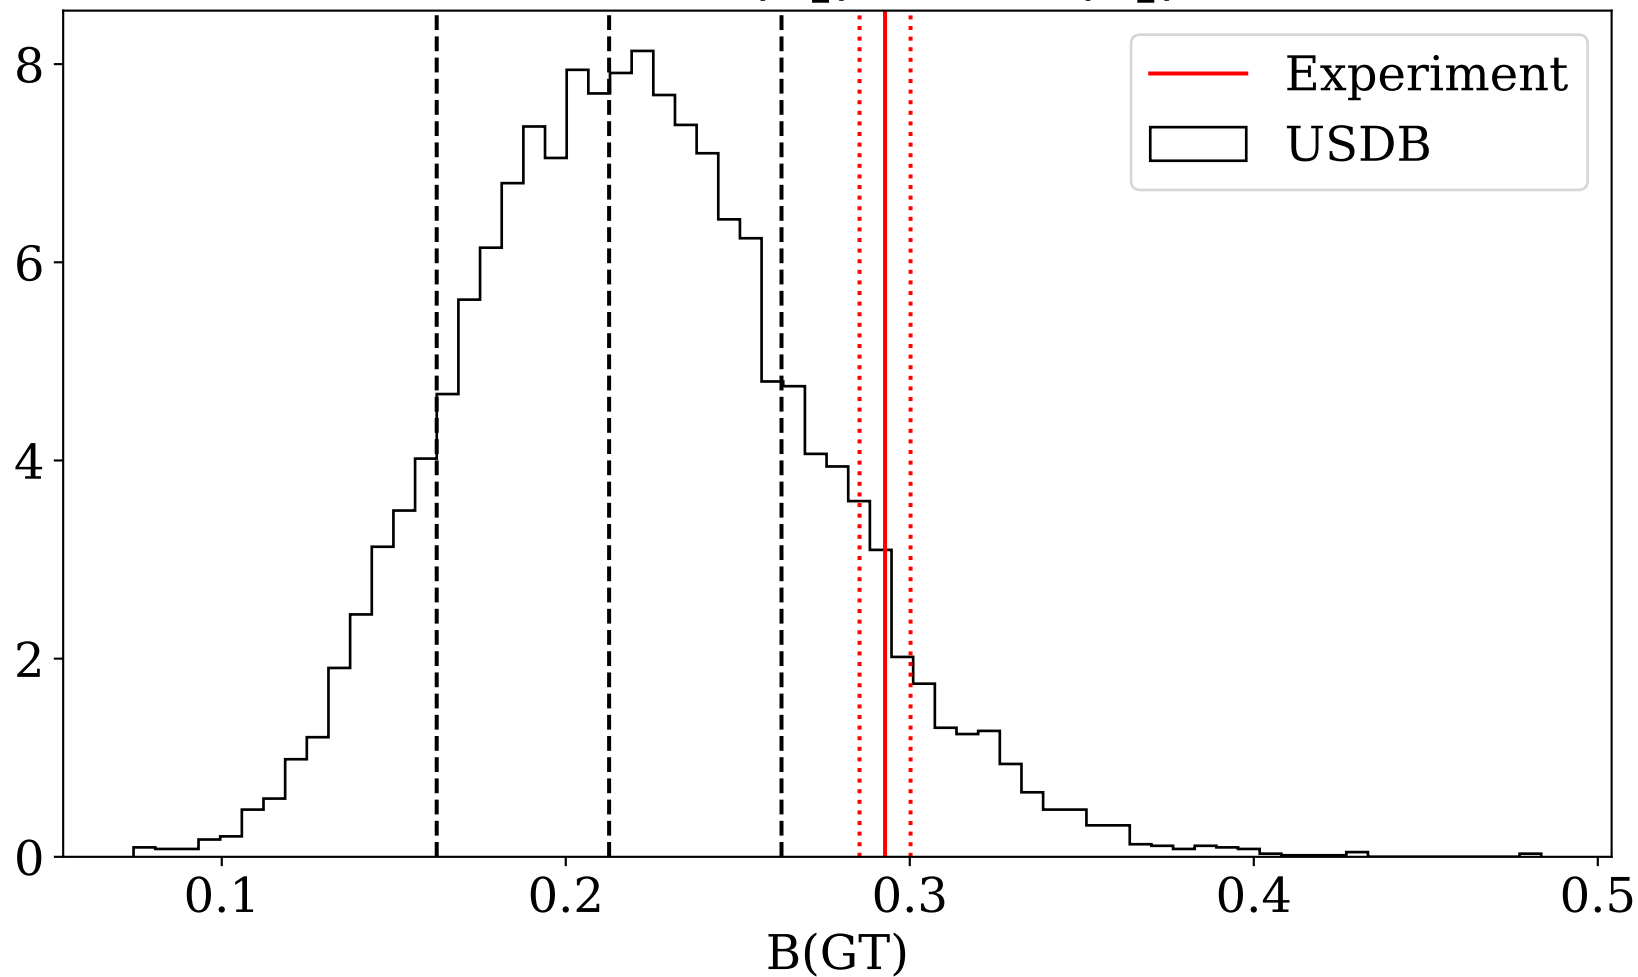

*e. c. :*  $^{30}\text{S}(0_1) \rightarrow ^{30}\text{P}(1_2)$

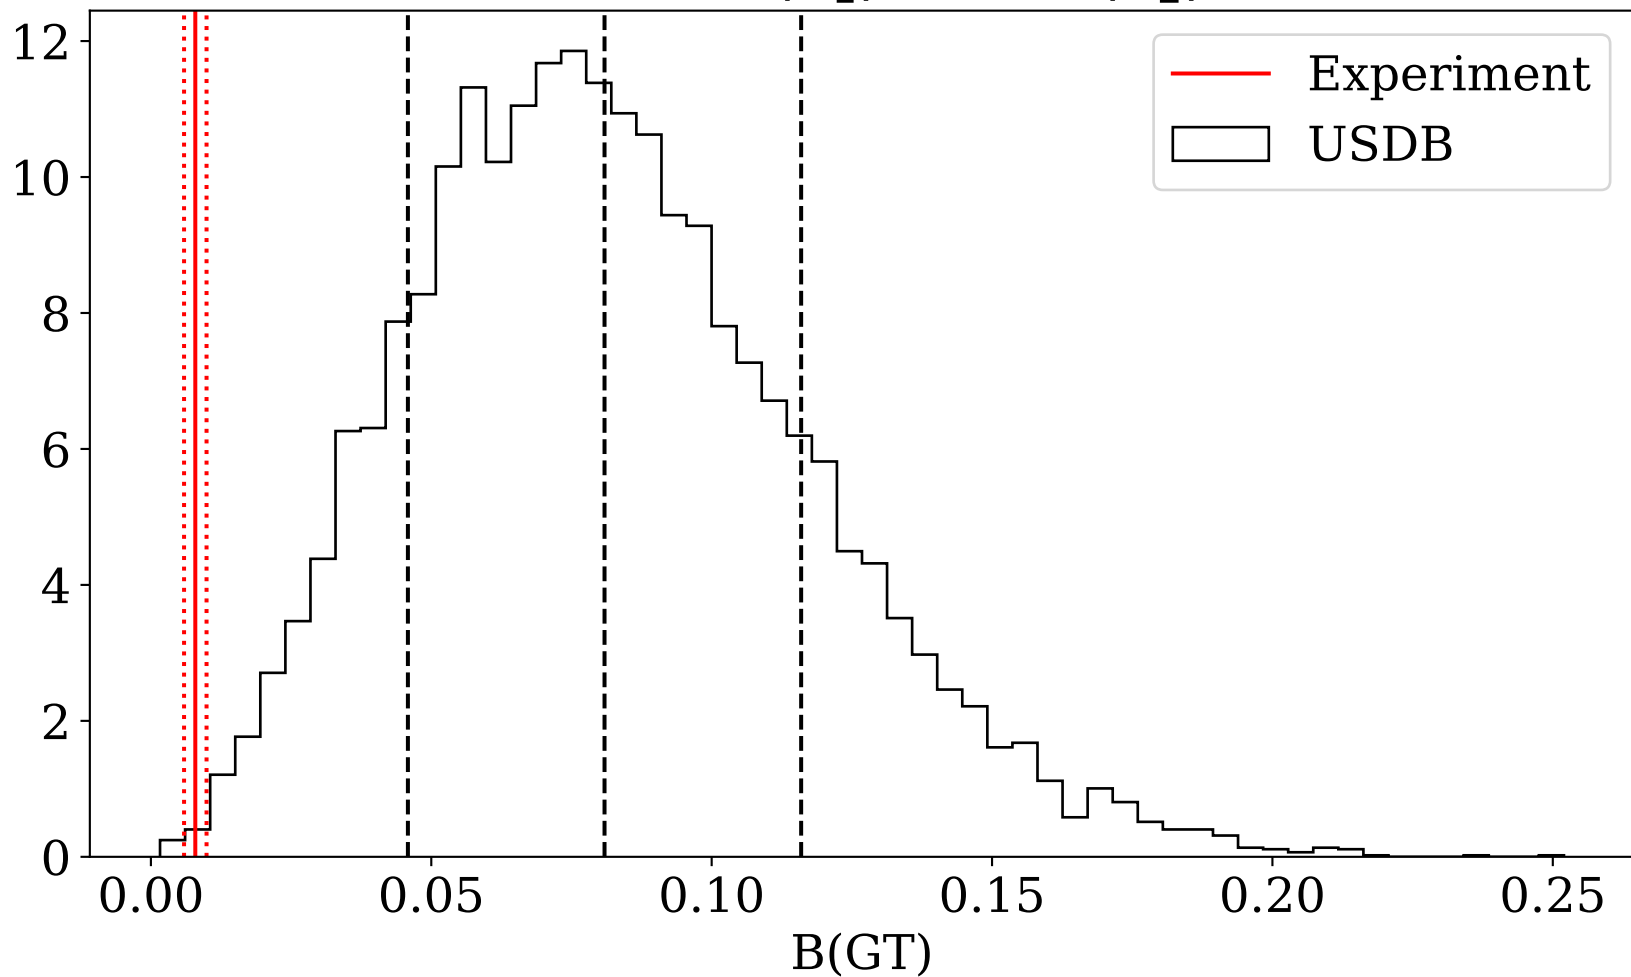

e. c. :  $^{30}\text{S}(0_1) \rightarrow ^{30}\text{P}(1_3)$

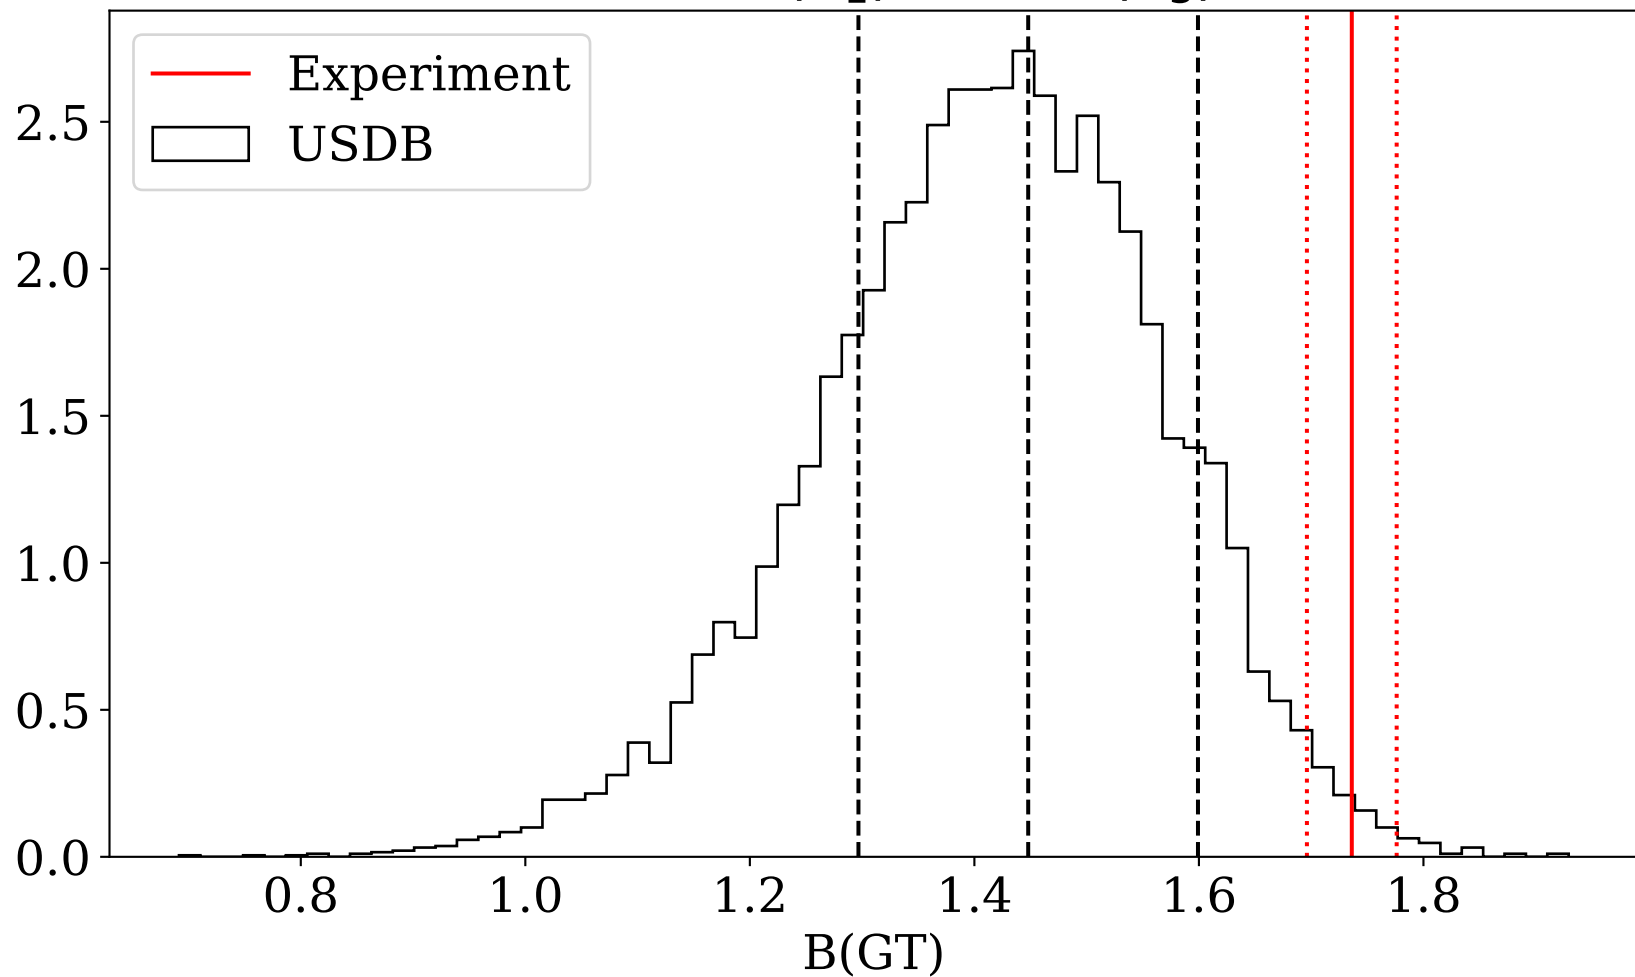



e. c. :  $^{31}\text{S}(1/2_1) \rightarrow ^{31}\text{P}(1/2_1)$

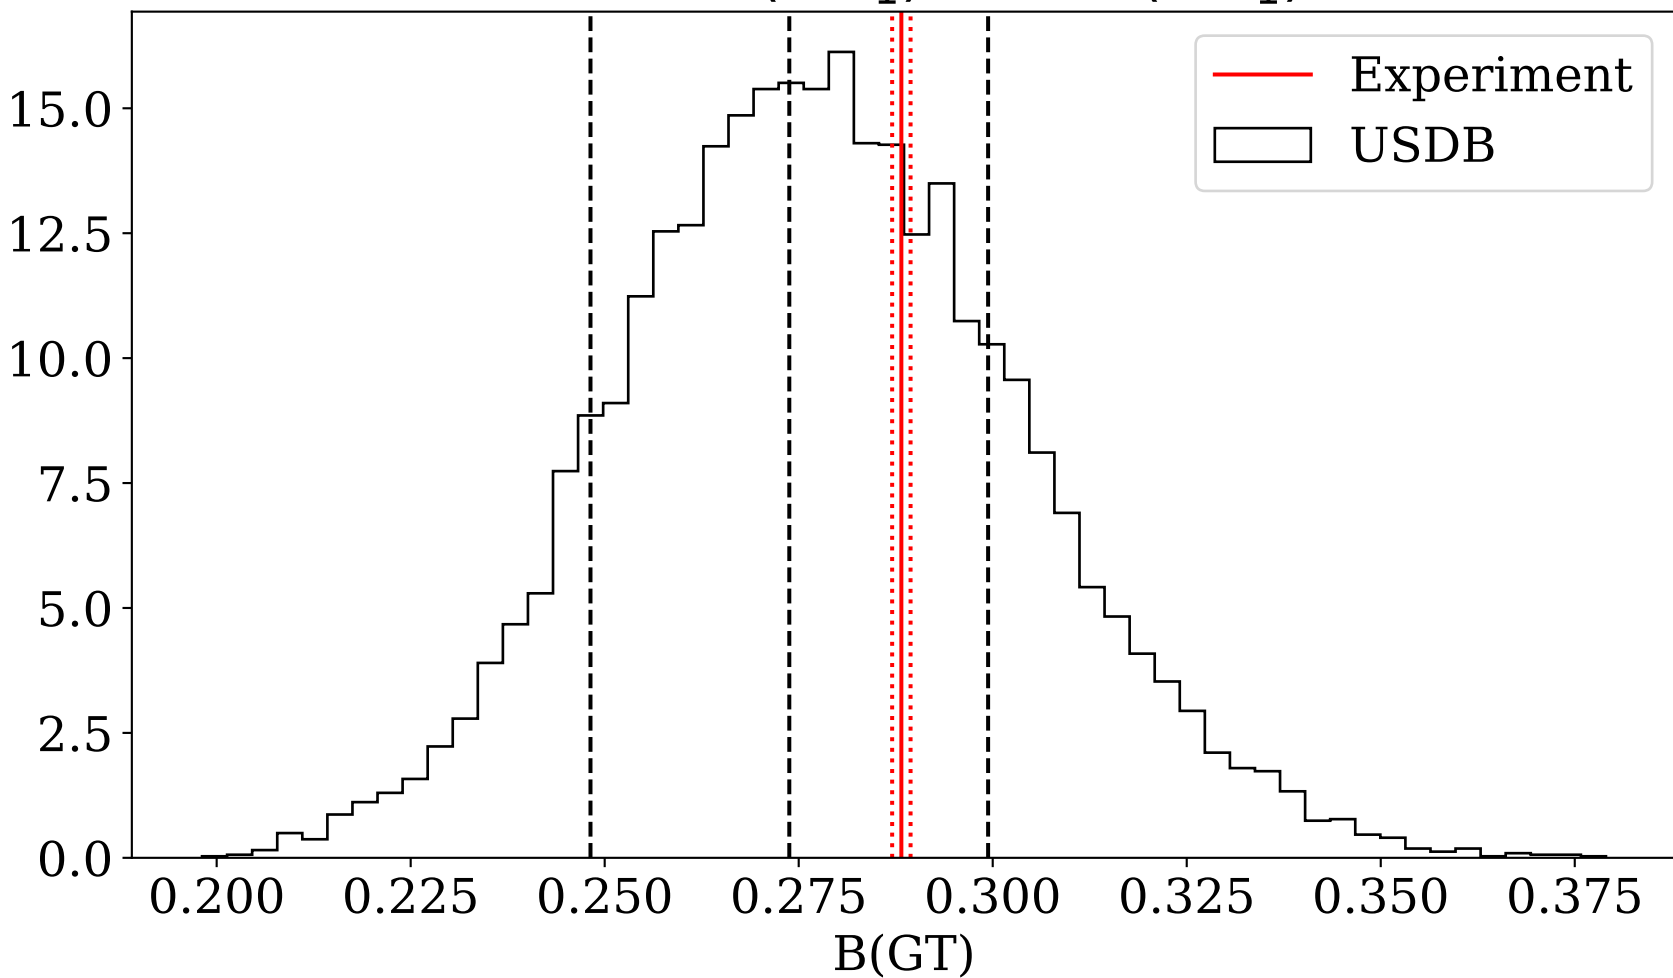

e. c. :  $^{31}\text{S}(1/2_1) \rightarrow ^{31}\text{P}(3/2_1)$

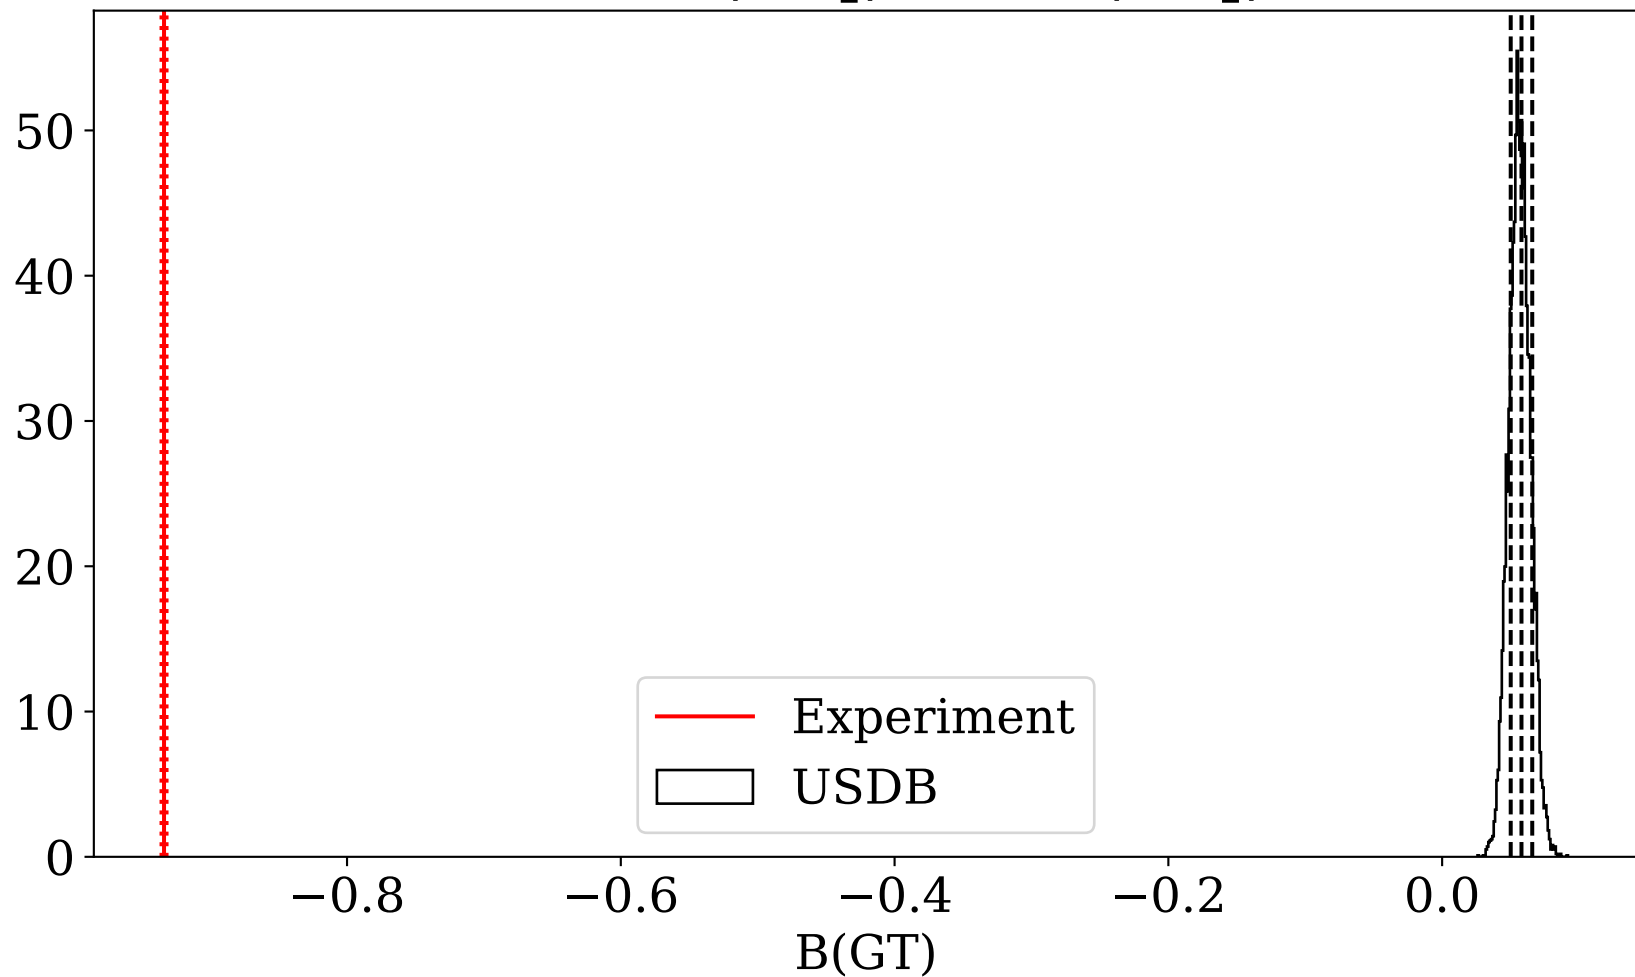

e. c. :  $^{31}\text{S}(1/2_1) \rightarrow ^{31}\text{P}(1/2_2)$

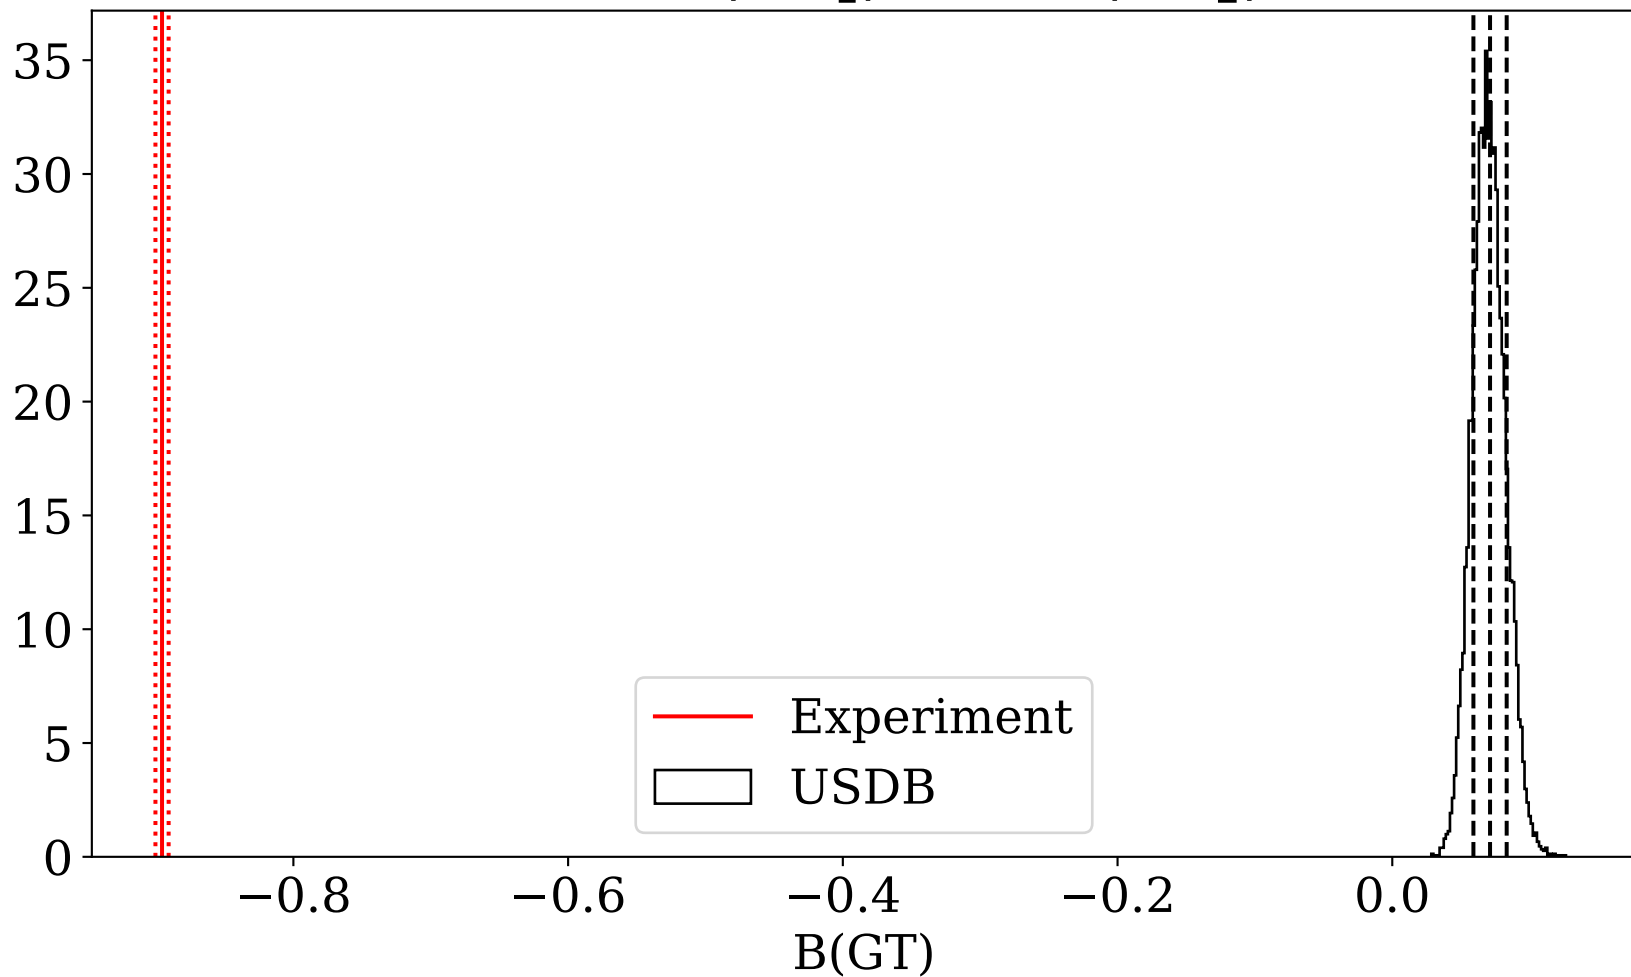

e. c. :  $^{31}\text{S}(1/2_1) \rightarrow ^{31}\text{P}(3/2_2)$

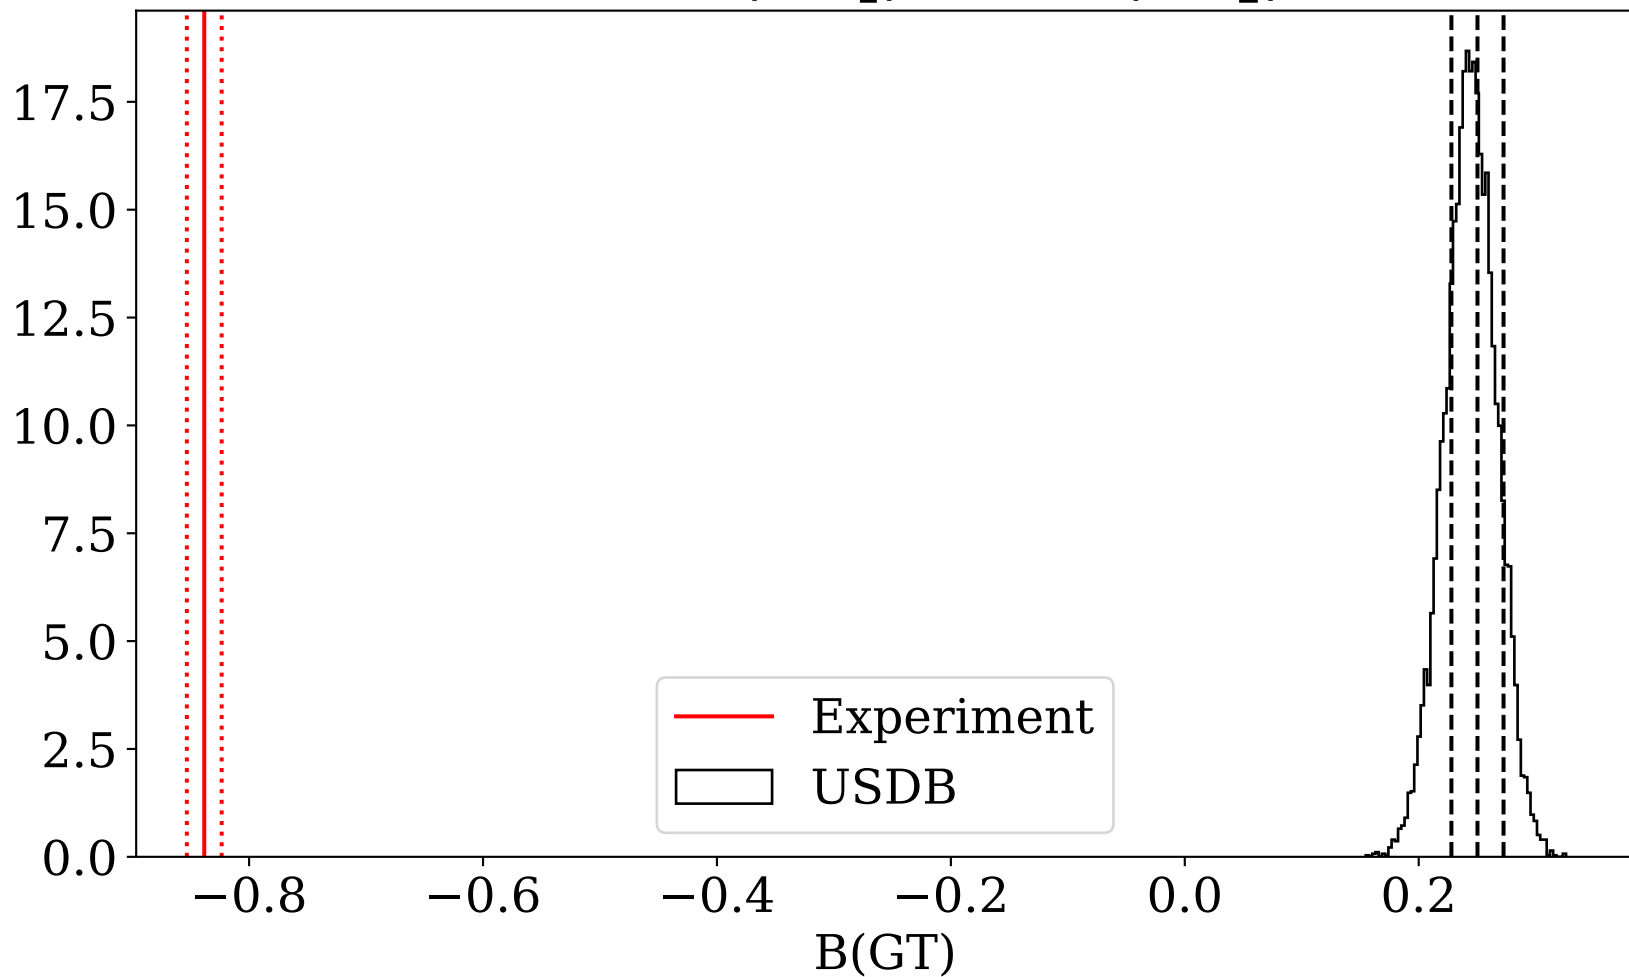

*e. c. :*  $^{31}\text{Cl}(3/2_1) \rightarrow ^{31}\text{S}(5/2_1)$

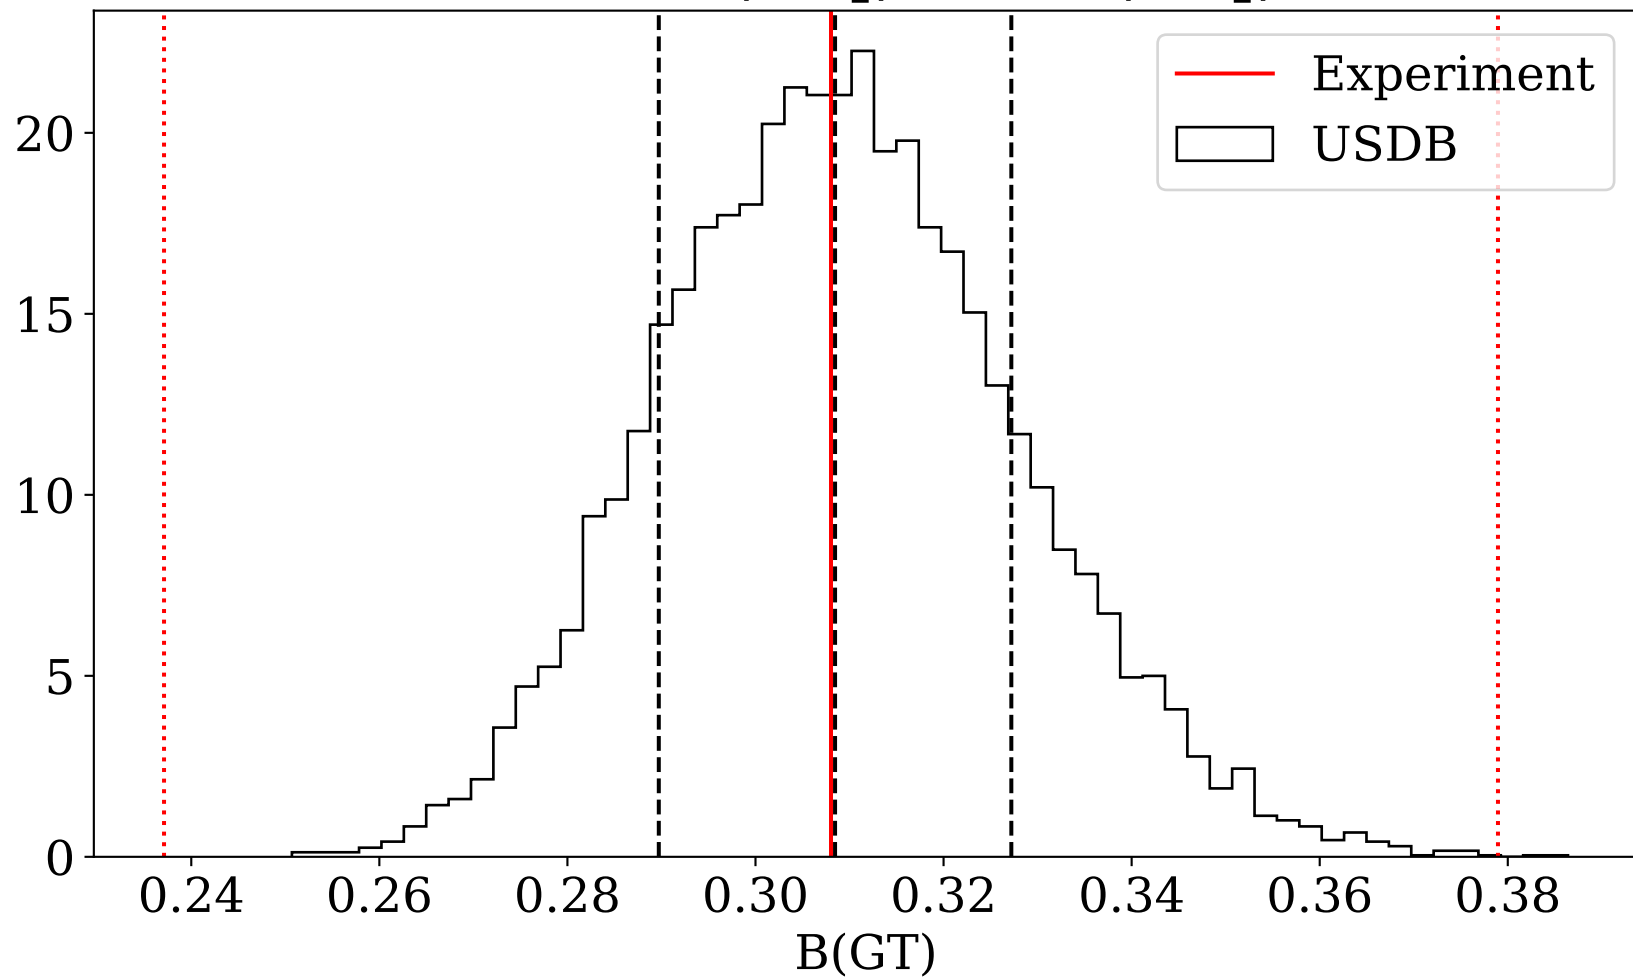

e. c. :  $^{31}\text{Cl}(3/2_1) \rightarrow ^{31}\text{S}(3/2_1)$

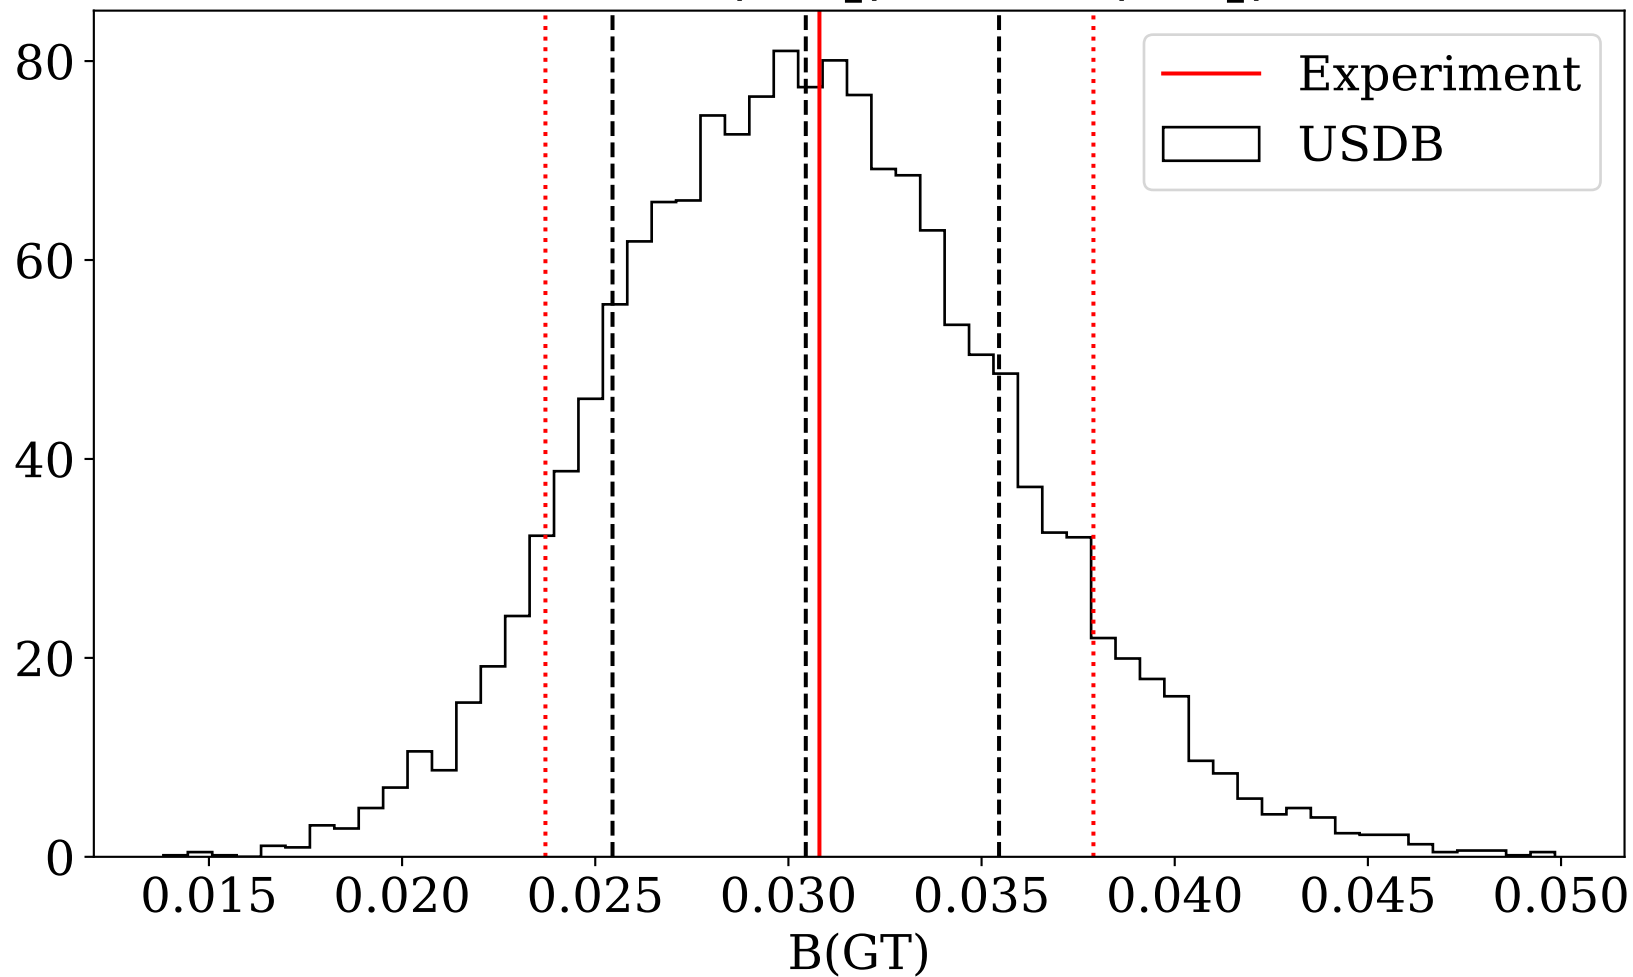

*e. c. :*  $^{31}\text{Cl}(3/2_1) \rightarrow ^{31}\text{S}(1/2_2)$

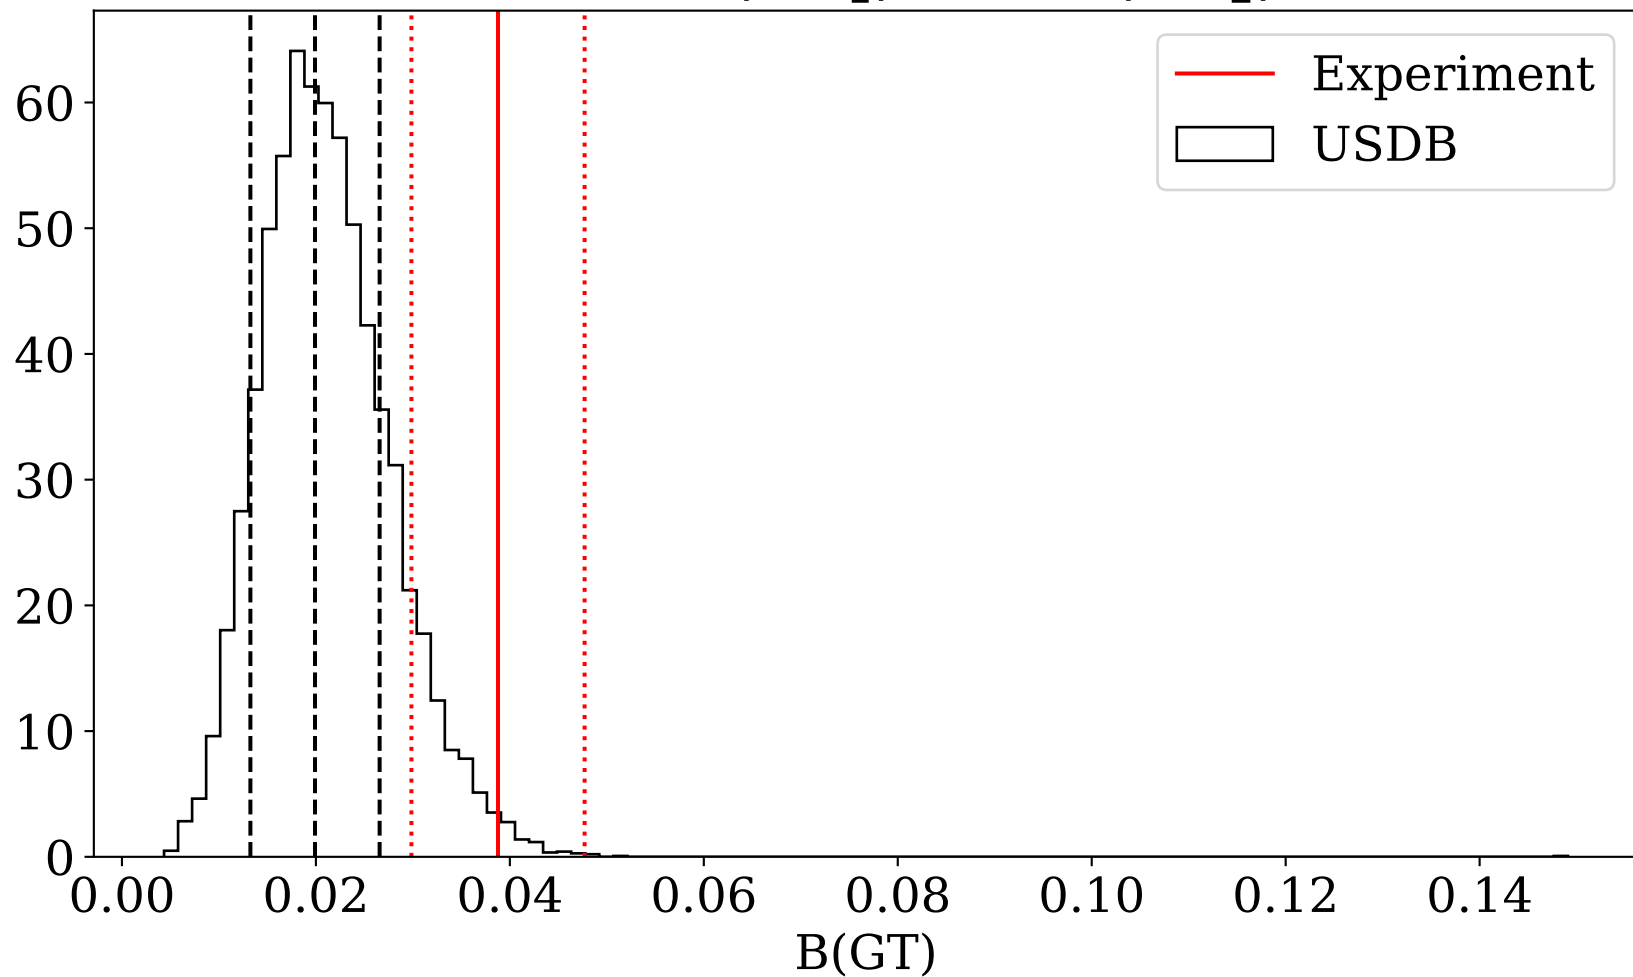

e. c. :  $^{31}\text{Cl}(3/2_1) \rightarrow ^{31}\text{S}(5/2_1)$

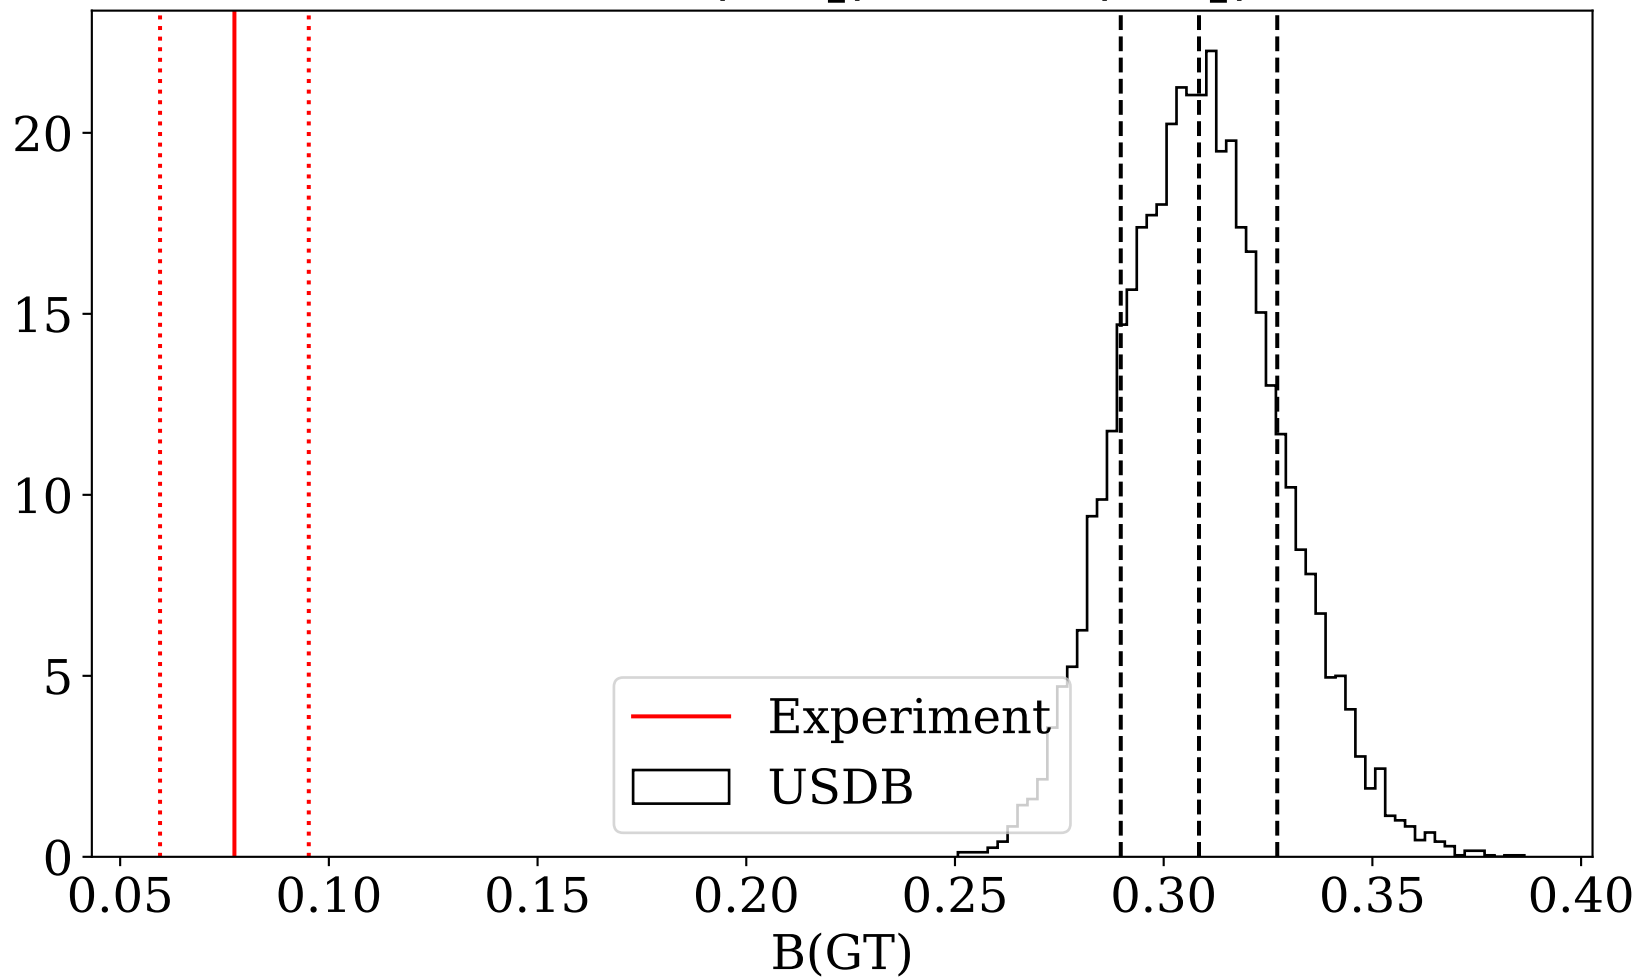



e. c. :  $^{31}\text{Cl}(3/2_1) \rightarrow ^{31}\text{S}(3/2_2)$

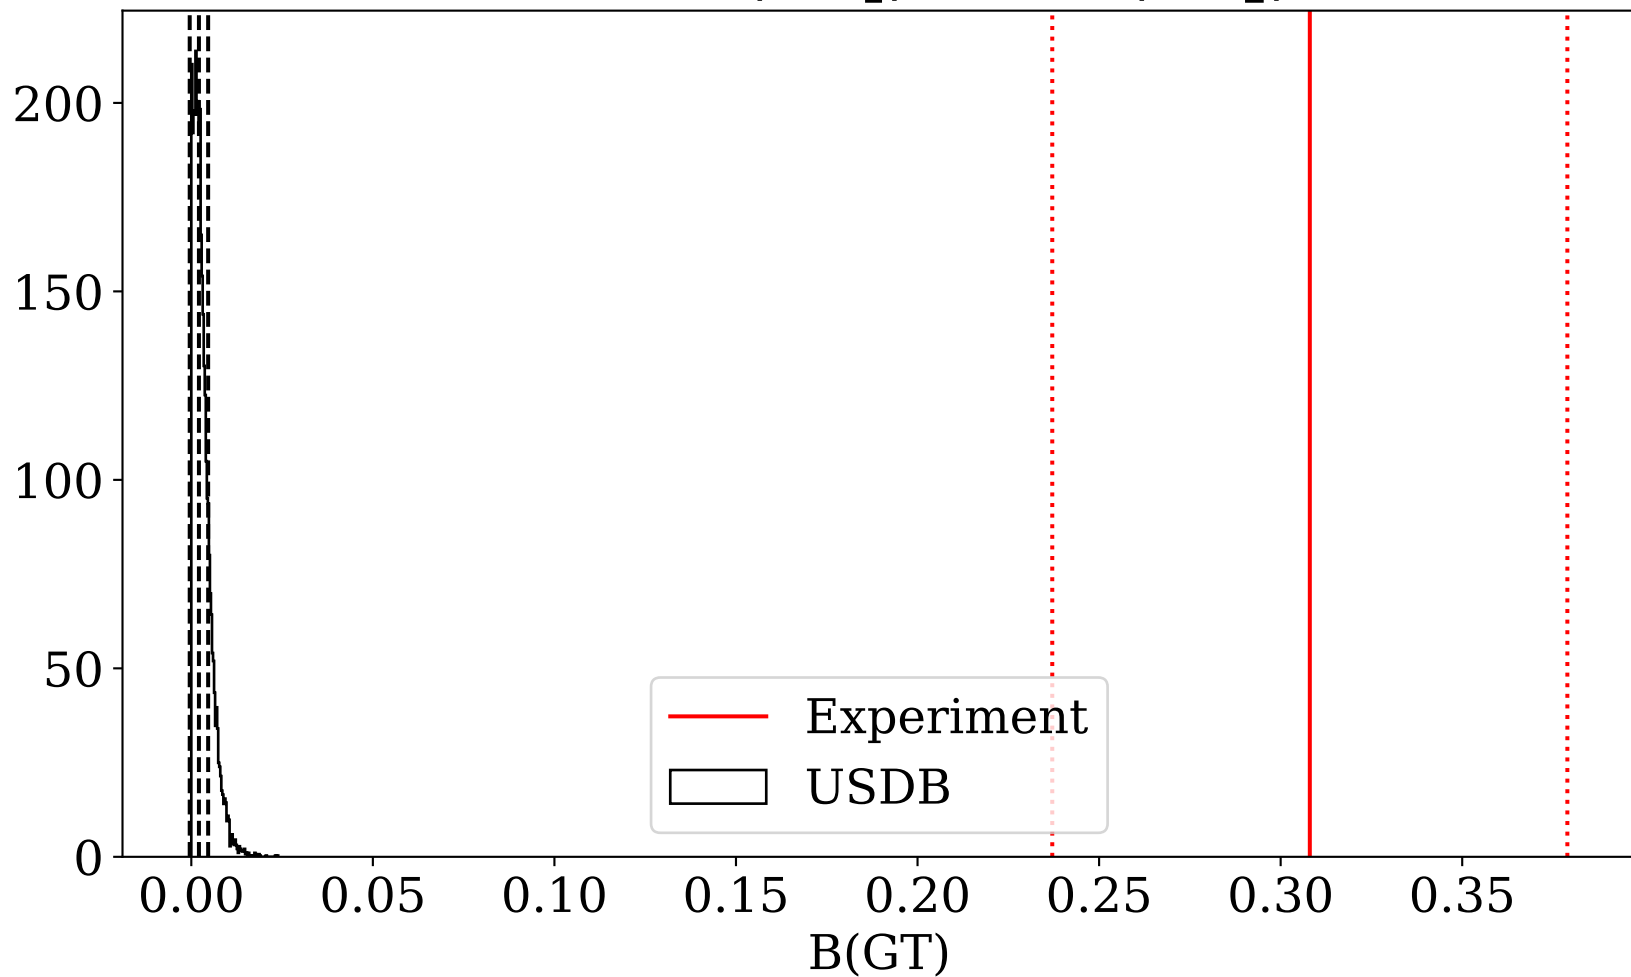

*e. c.*:  $^{31}\text{Cl}(3/2_1) \rightarrow ^{31}\text{S}(3/2_3)$

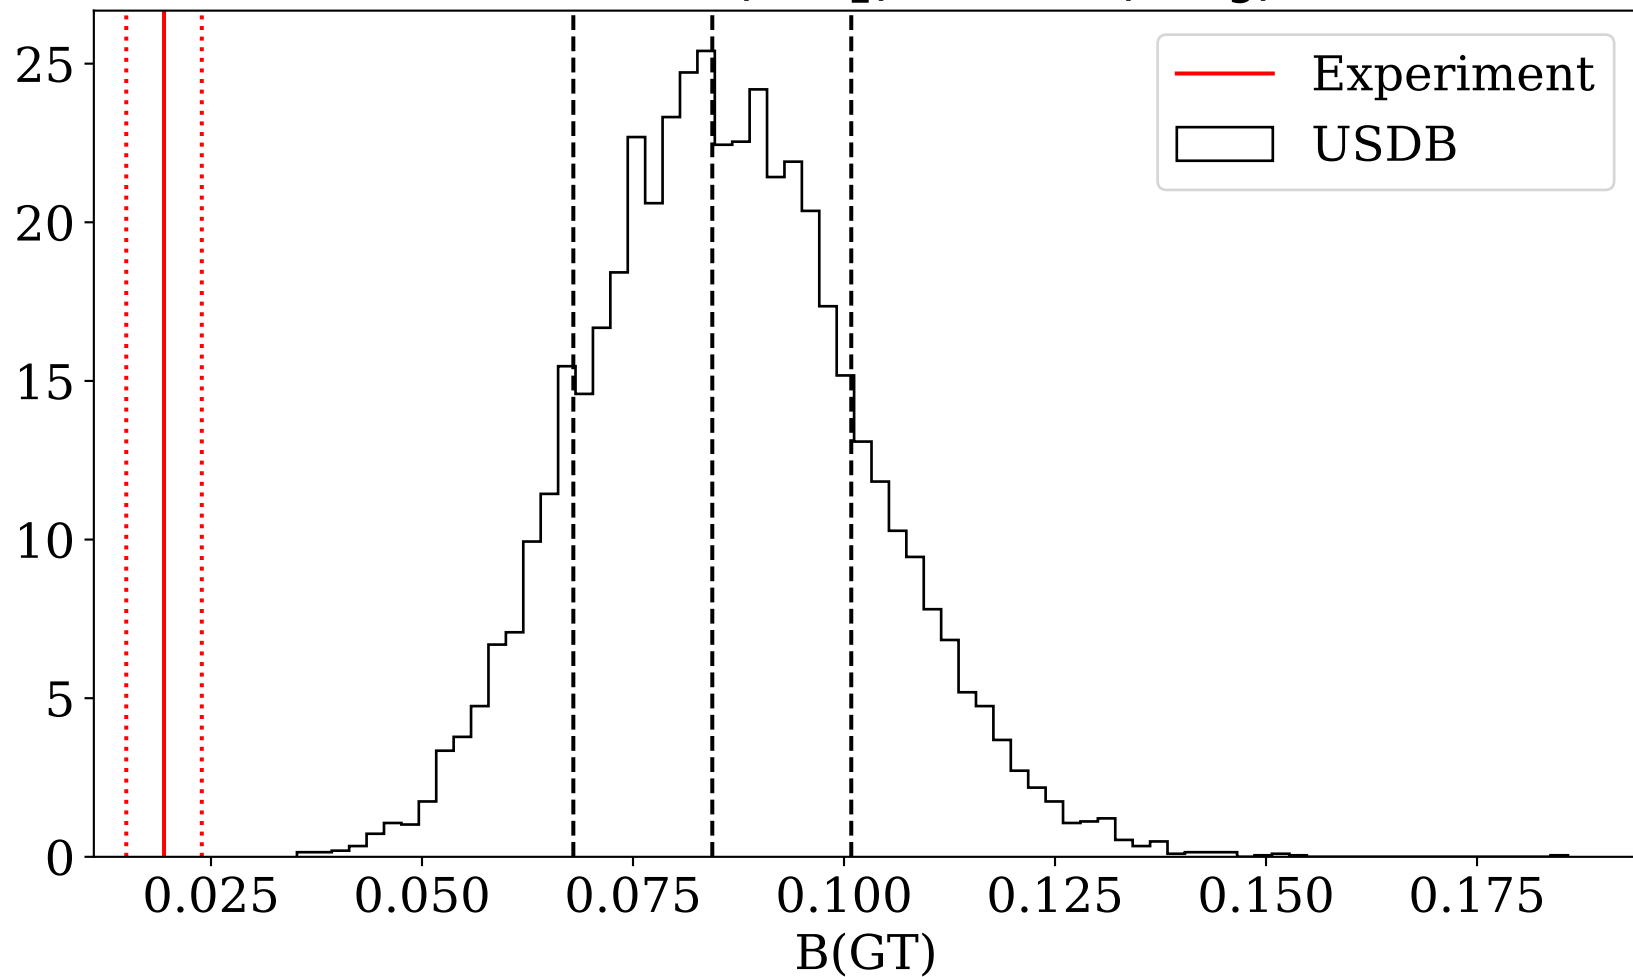

e. c. :  $^{31}\text{Cl}(3/2_1) \rightarrow ^{31}\text{S}(1/2_3)$

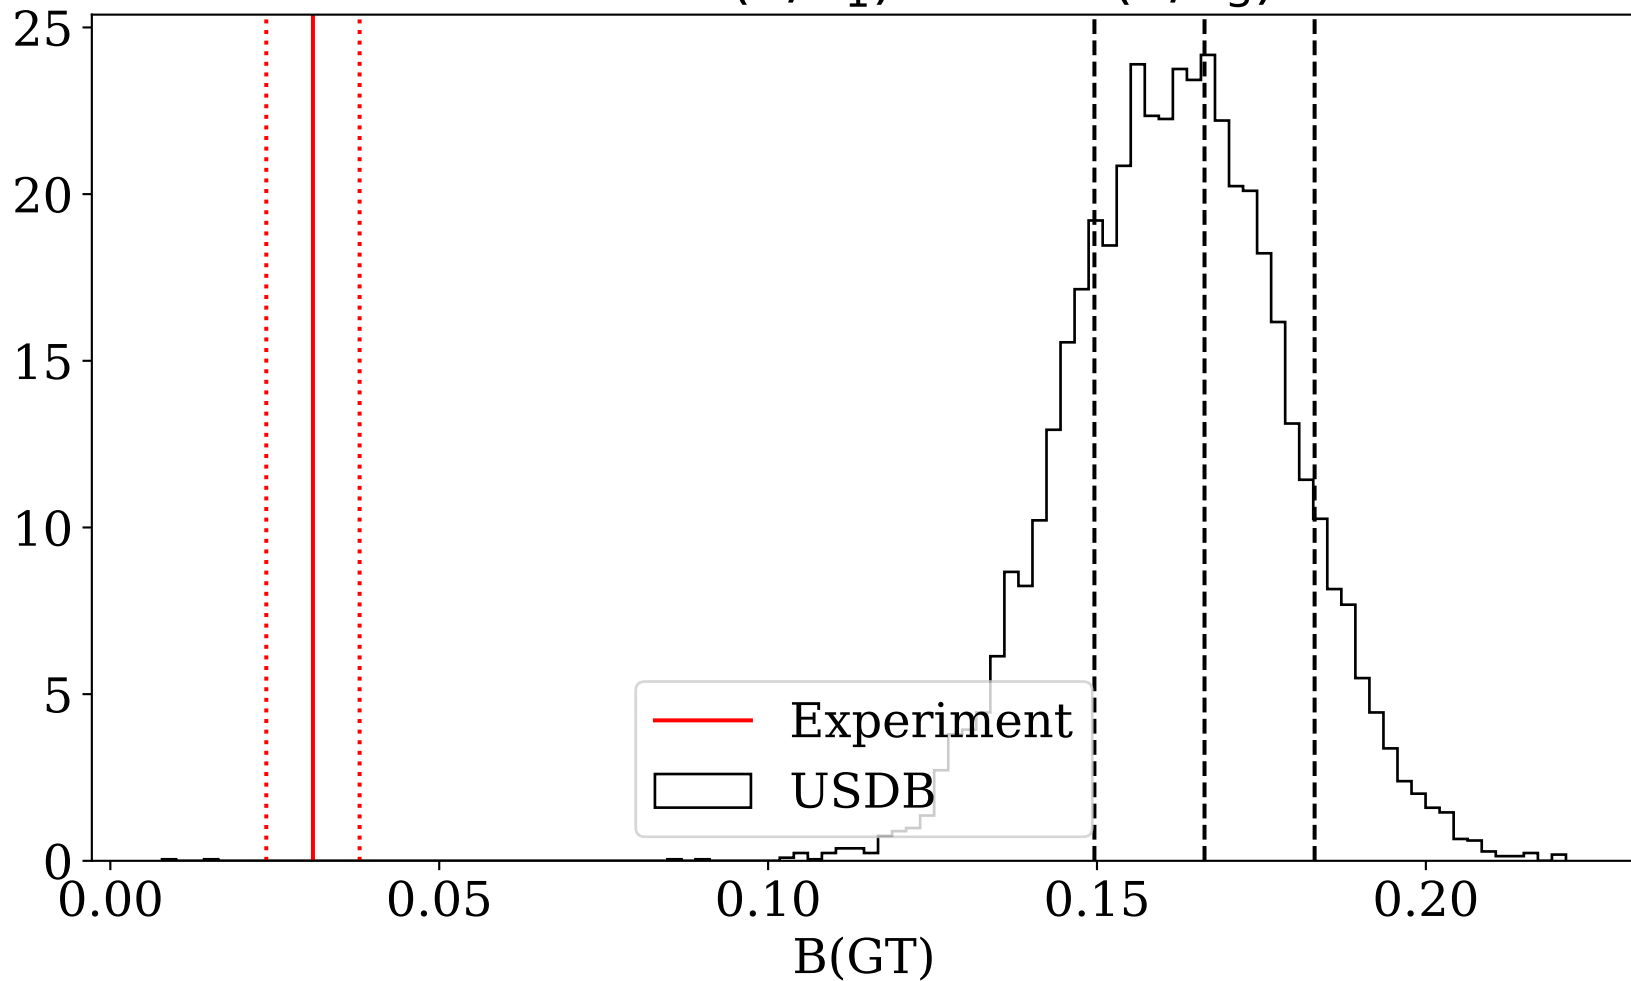

*e. c. :*  $^{31}\text{Cl}(3/2_1) \rightarrow ^{31}\text{S}(1/2_4)$

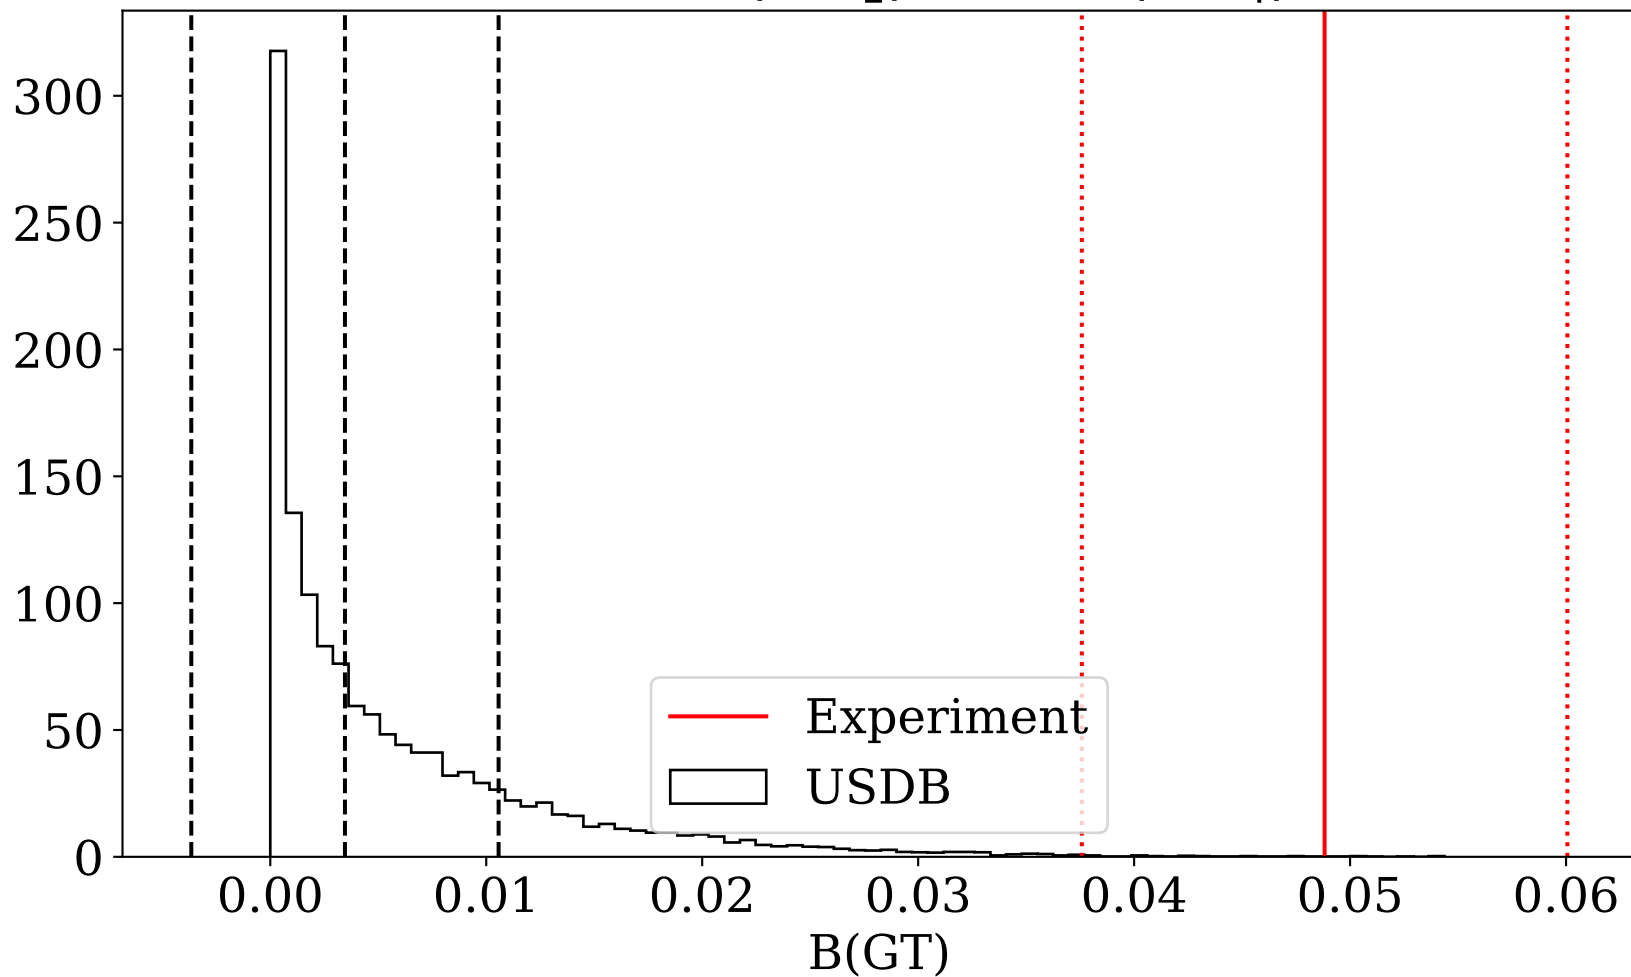

e. c. :  $^{31}\text{Cl}(3/2_1) \rightarrow ^{31}\text{S}(3/2_4)$

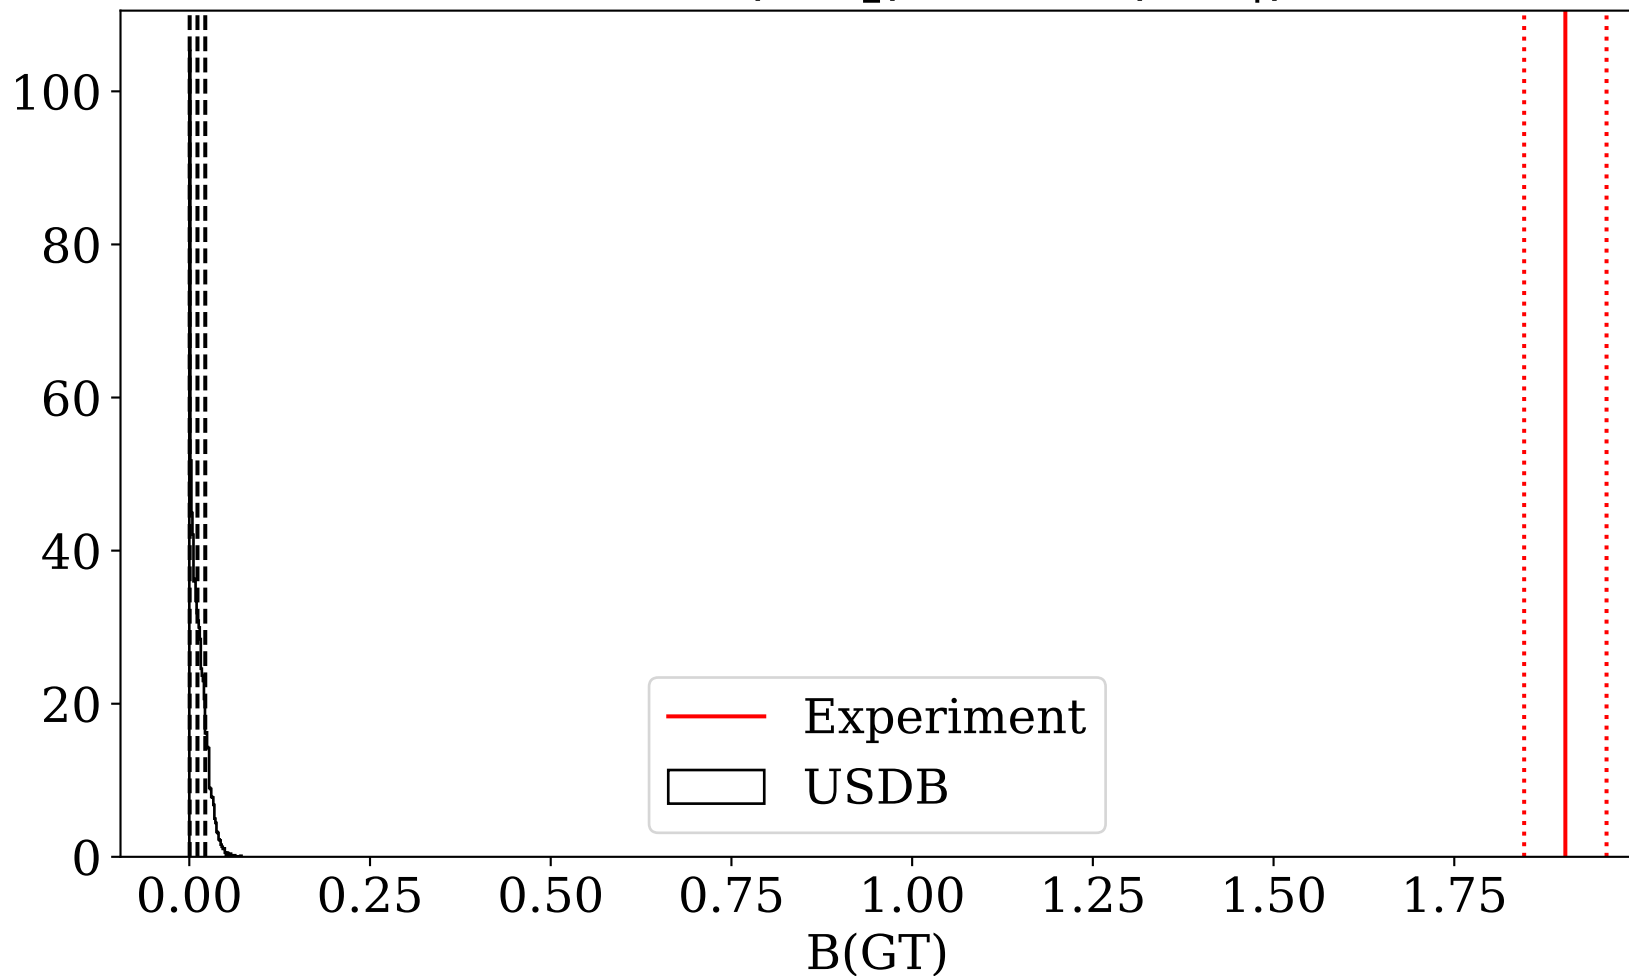

e. c. :  $^{32}\text{Cl}(1_1) \rightarrow ^{32}\text{S}(0_1)$

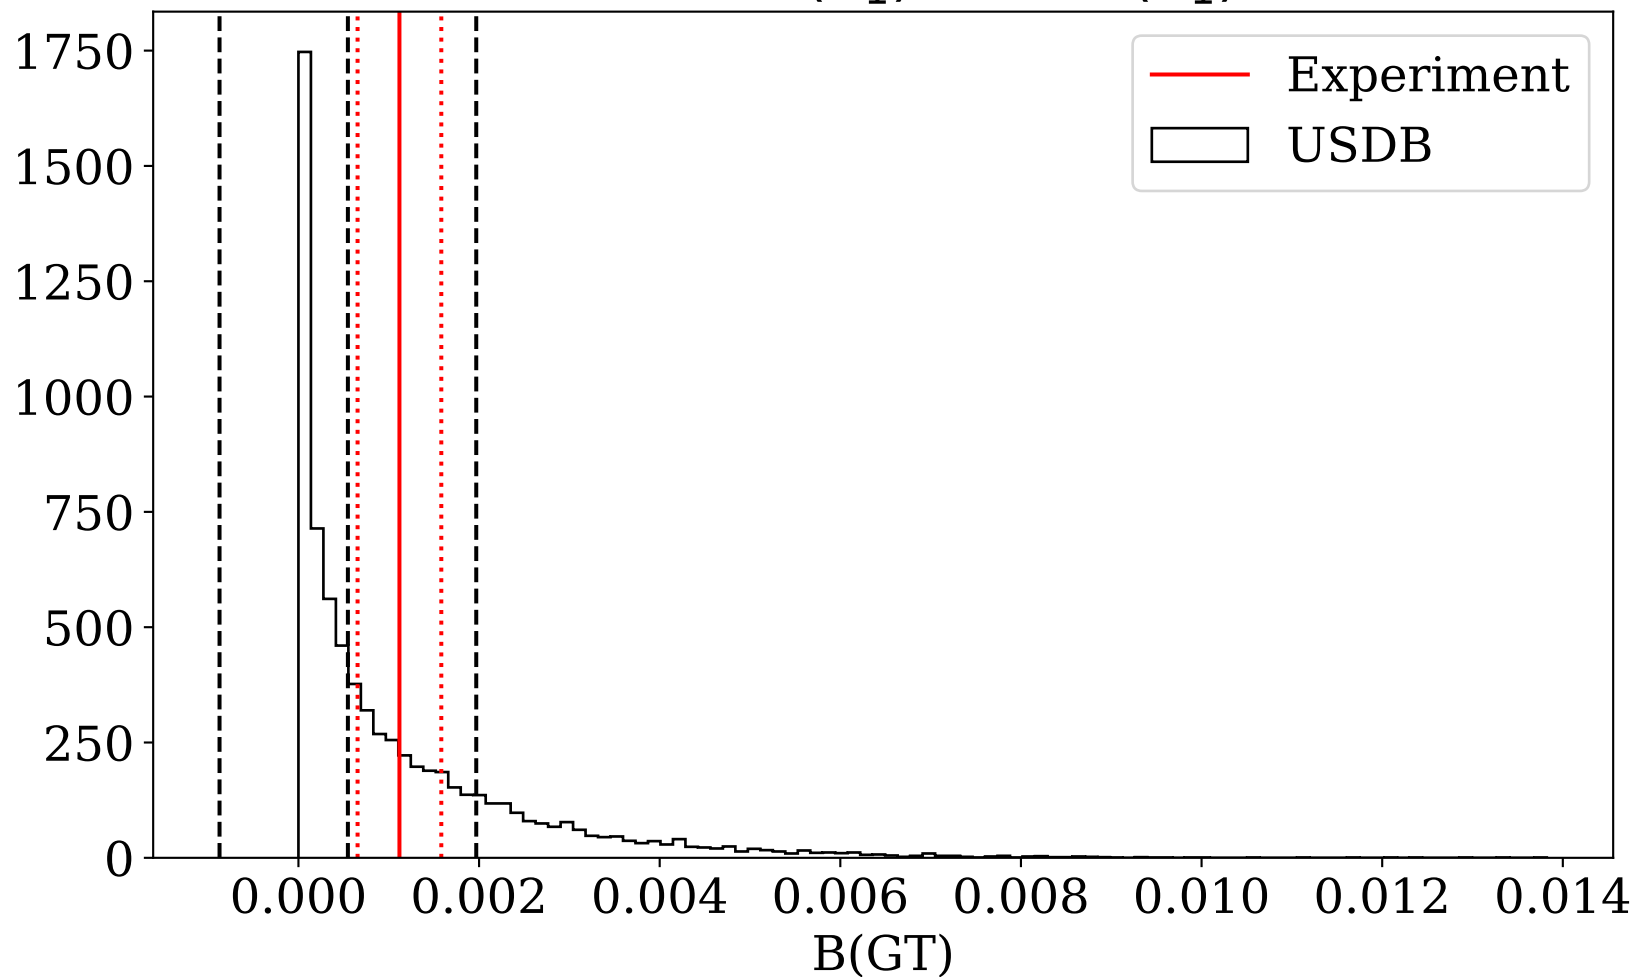

e. c. :  $^{32}\text{Cl}(1_1) \rightarrow ^{32}\text{S}(2_1)$

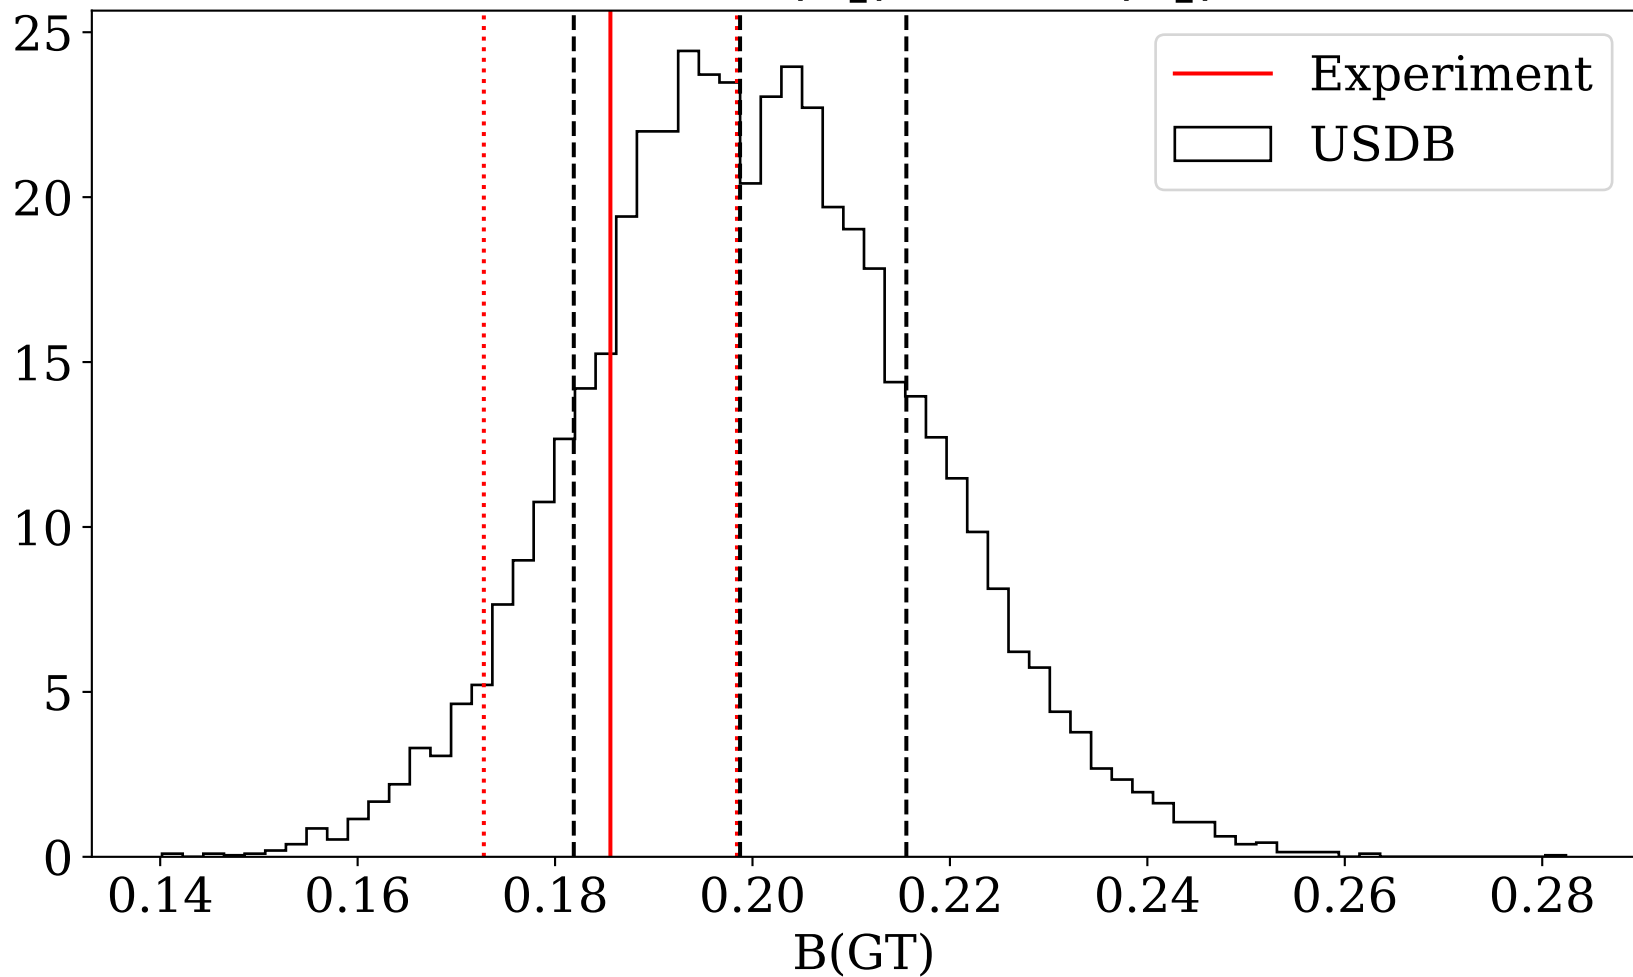

e. c. :  $^{32}\text{Cl}(1_1) \rightarrow ^{32}\text{S}(0_2)$

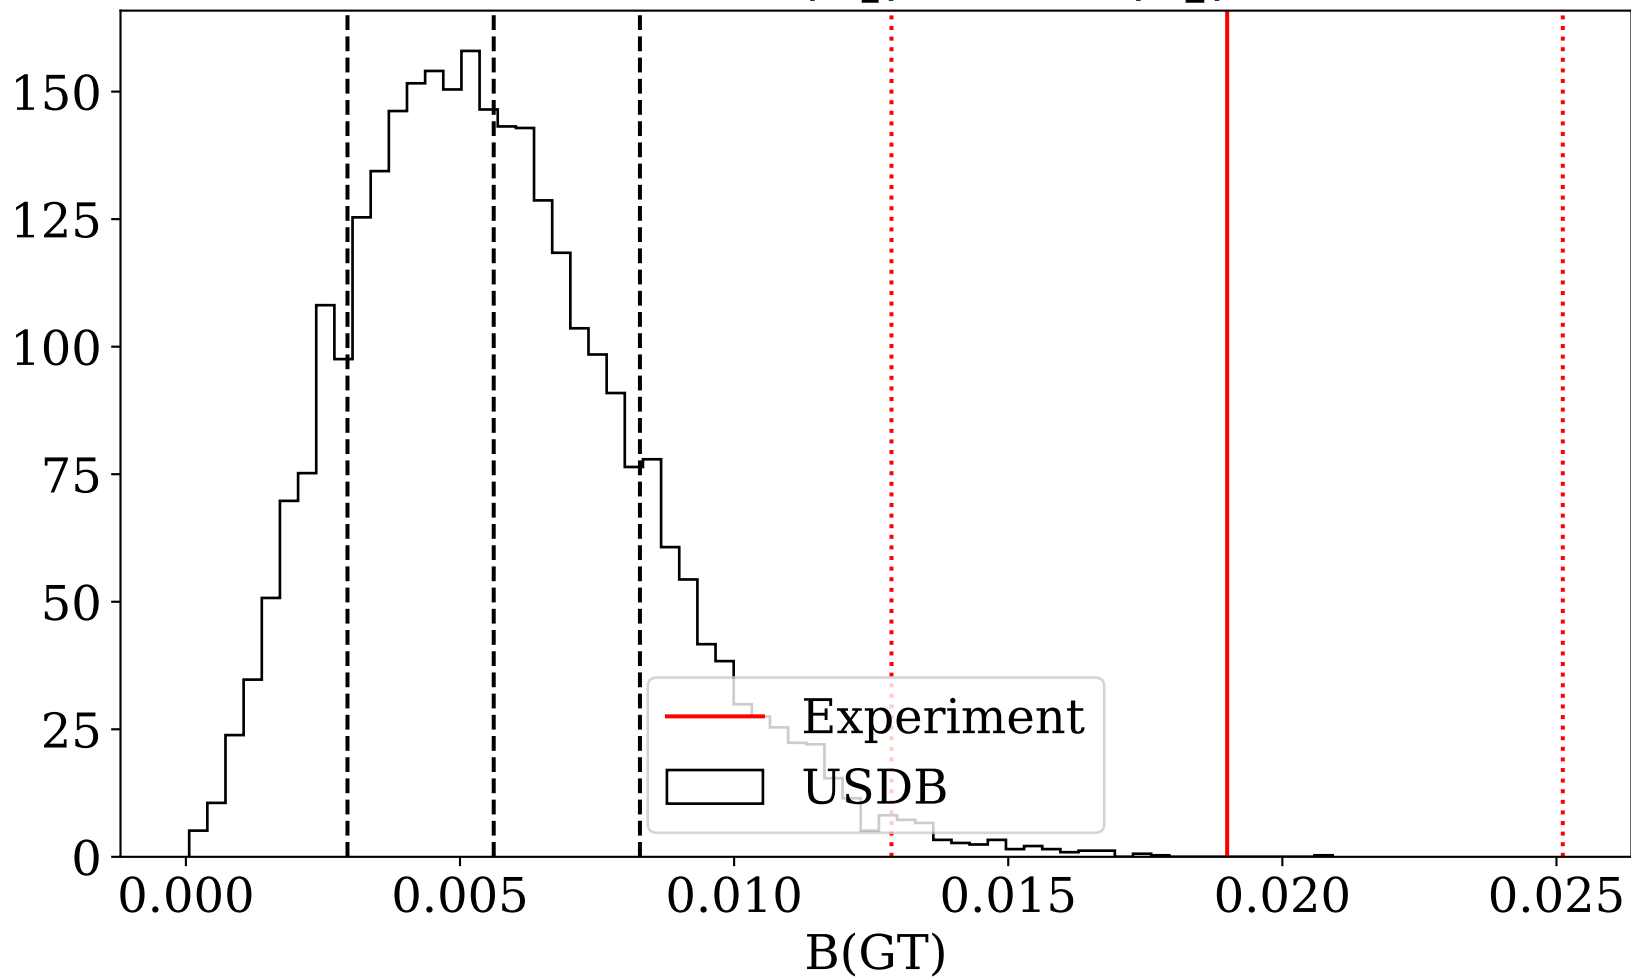



e. c. :  $^{32}\text{Cl}(1_1) \rightarrow ^{32}\text{S}(2_2)$

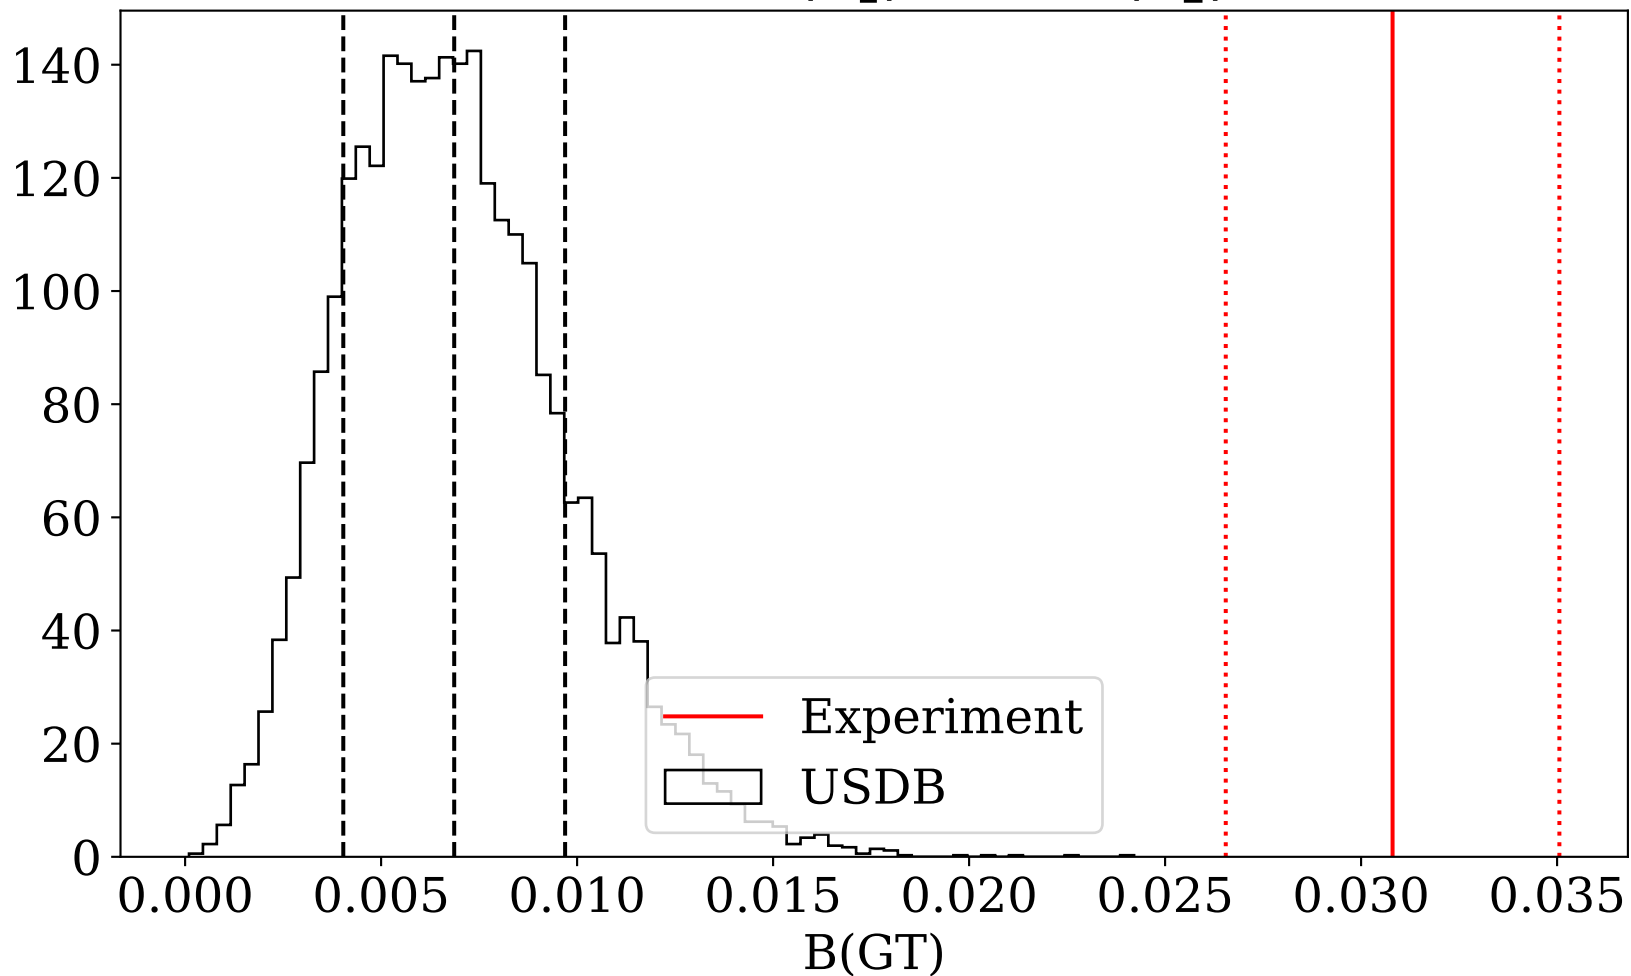

*e. c. :*  $^{32}\text{Cl}(1_1) \rightarrow ^{32}\text{S}(1_1)$

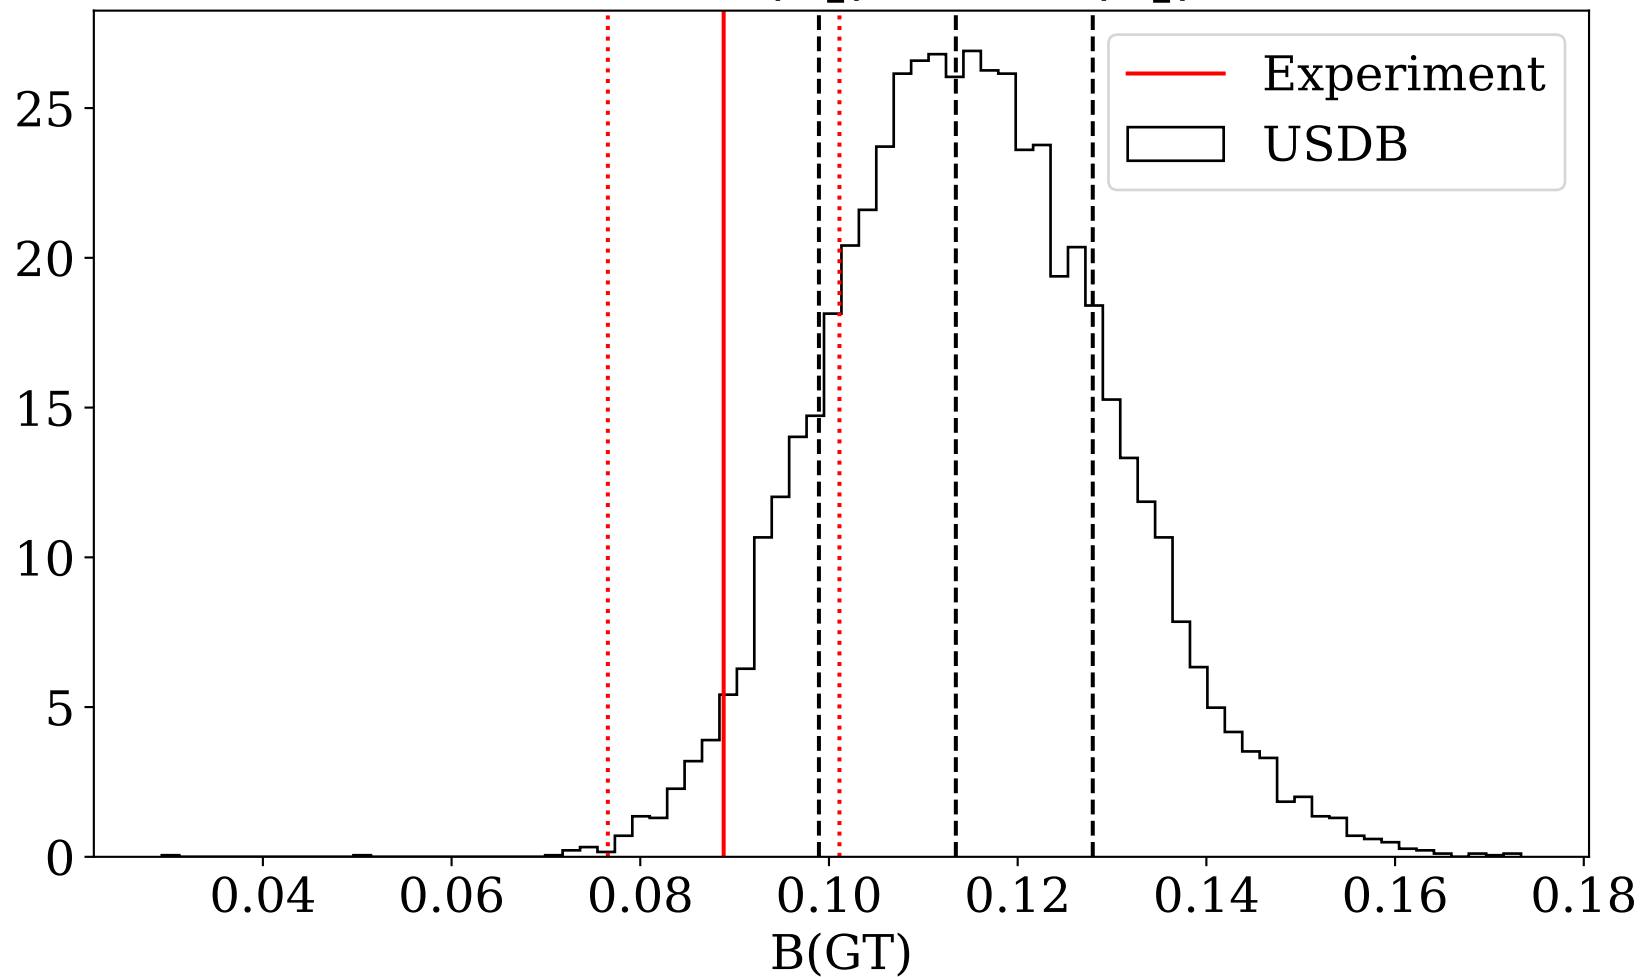

e. c. :  $^{32}\text{Cl}(1_1) \rightarrow ^{32}\text{S}(2_3)$

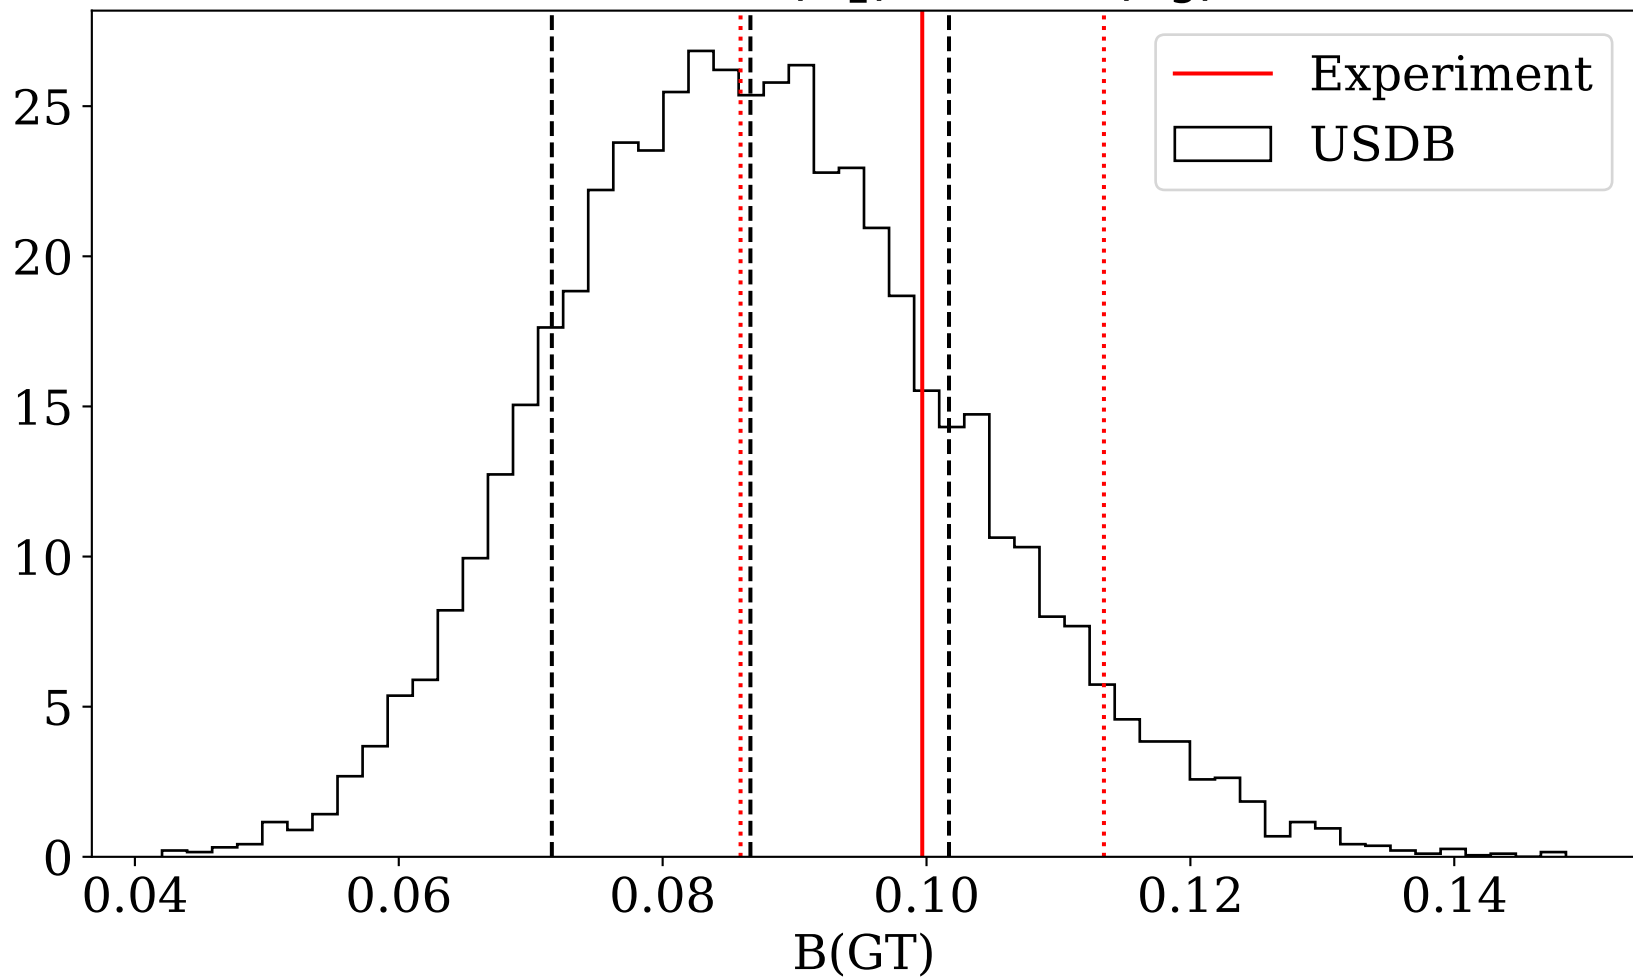

*e. c.* :  $^{33}\text{Cl}(3/2_1) \rightarrow ^{33}\text{S}(3/2_1)$

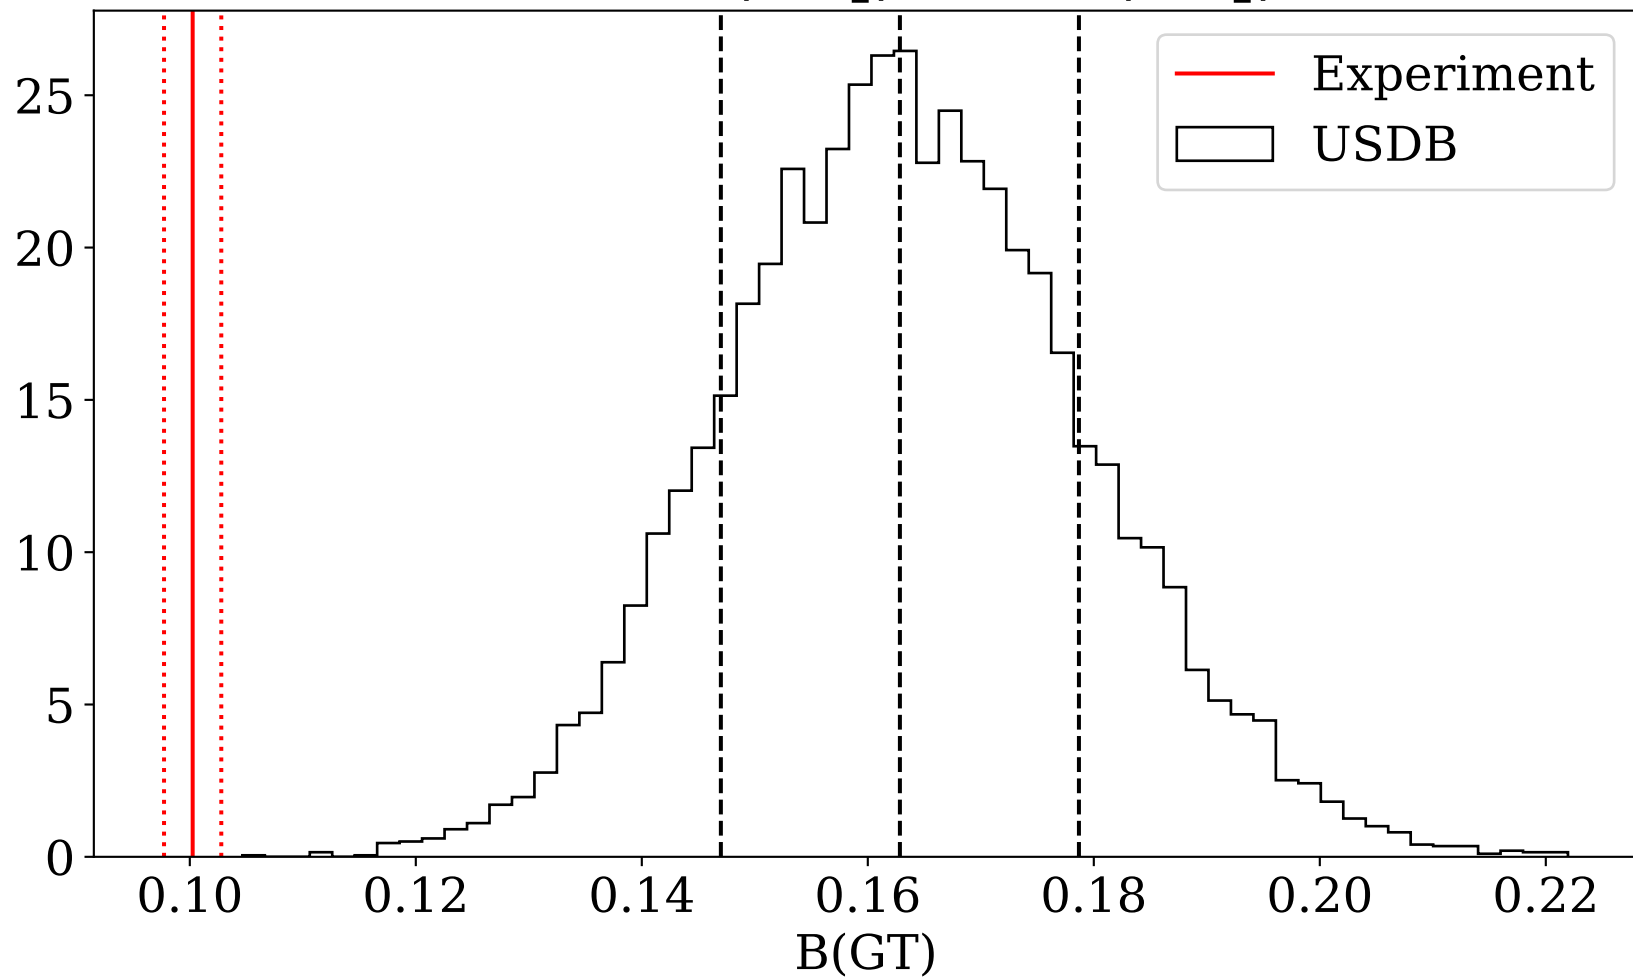

*e. c. :*  $^{33}\text{Cl}(3/2_1) \rightarrow ^{33}\text{S}(1/2_1)$

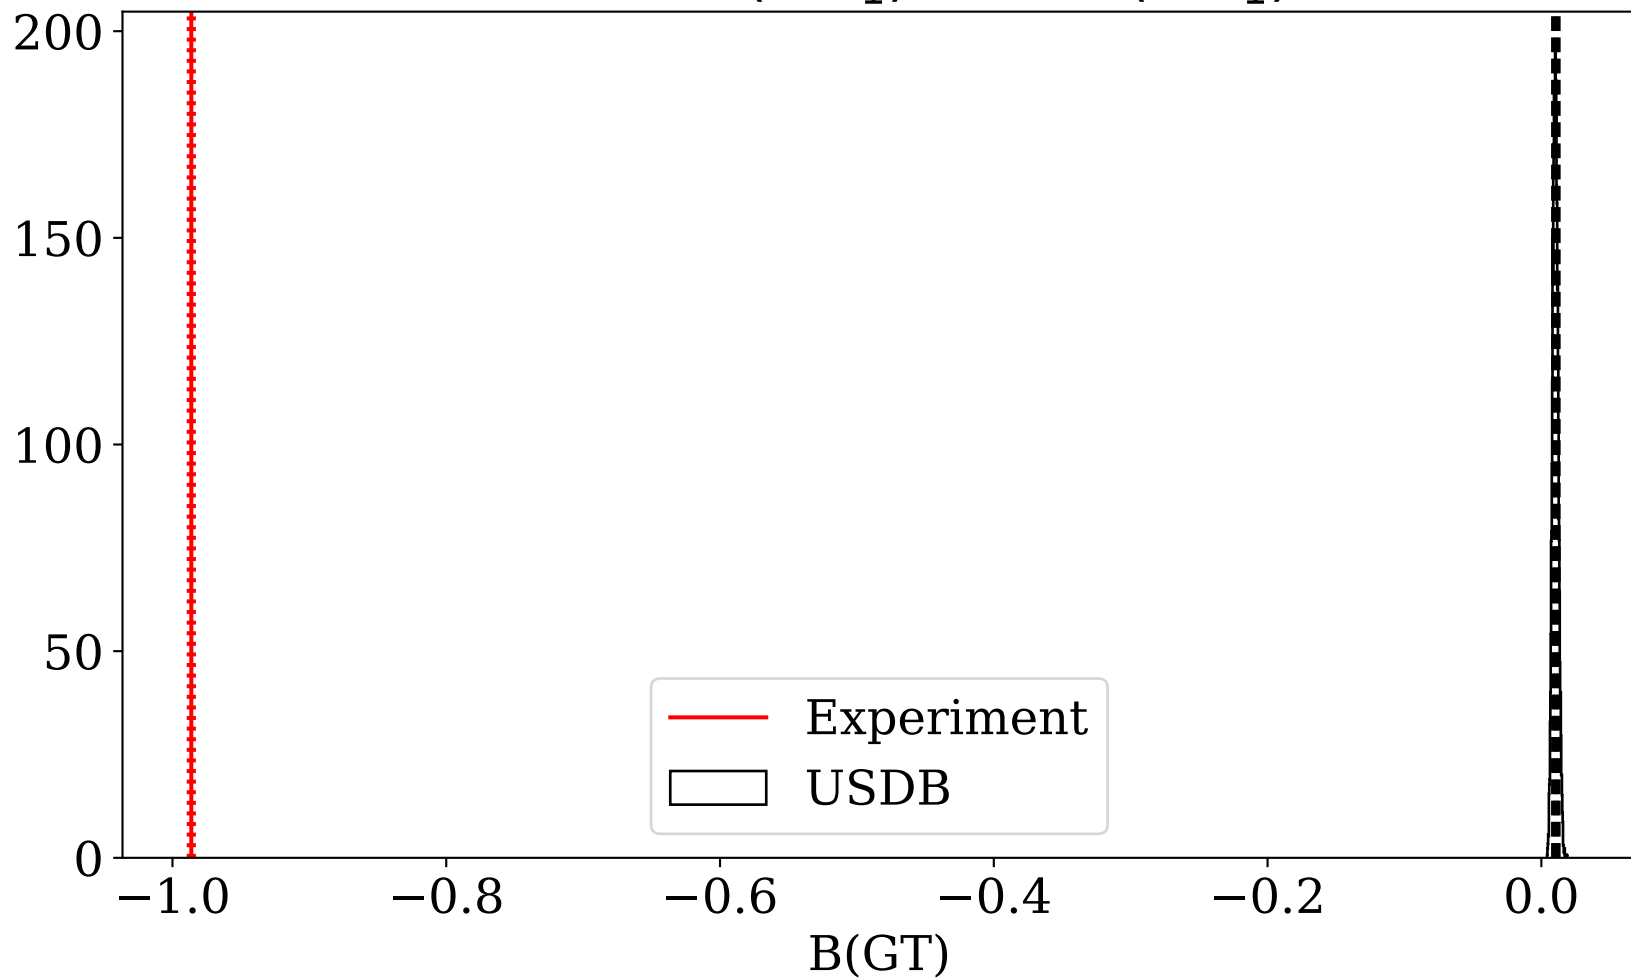

*e. c.* :  $^{33}\text{Cl}(3/2_1) \rightarrow ^{33}\text{S}(5/2_1)$

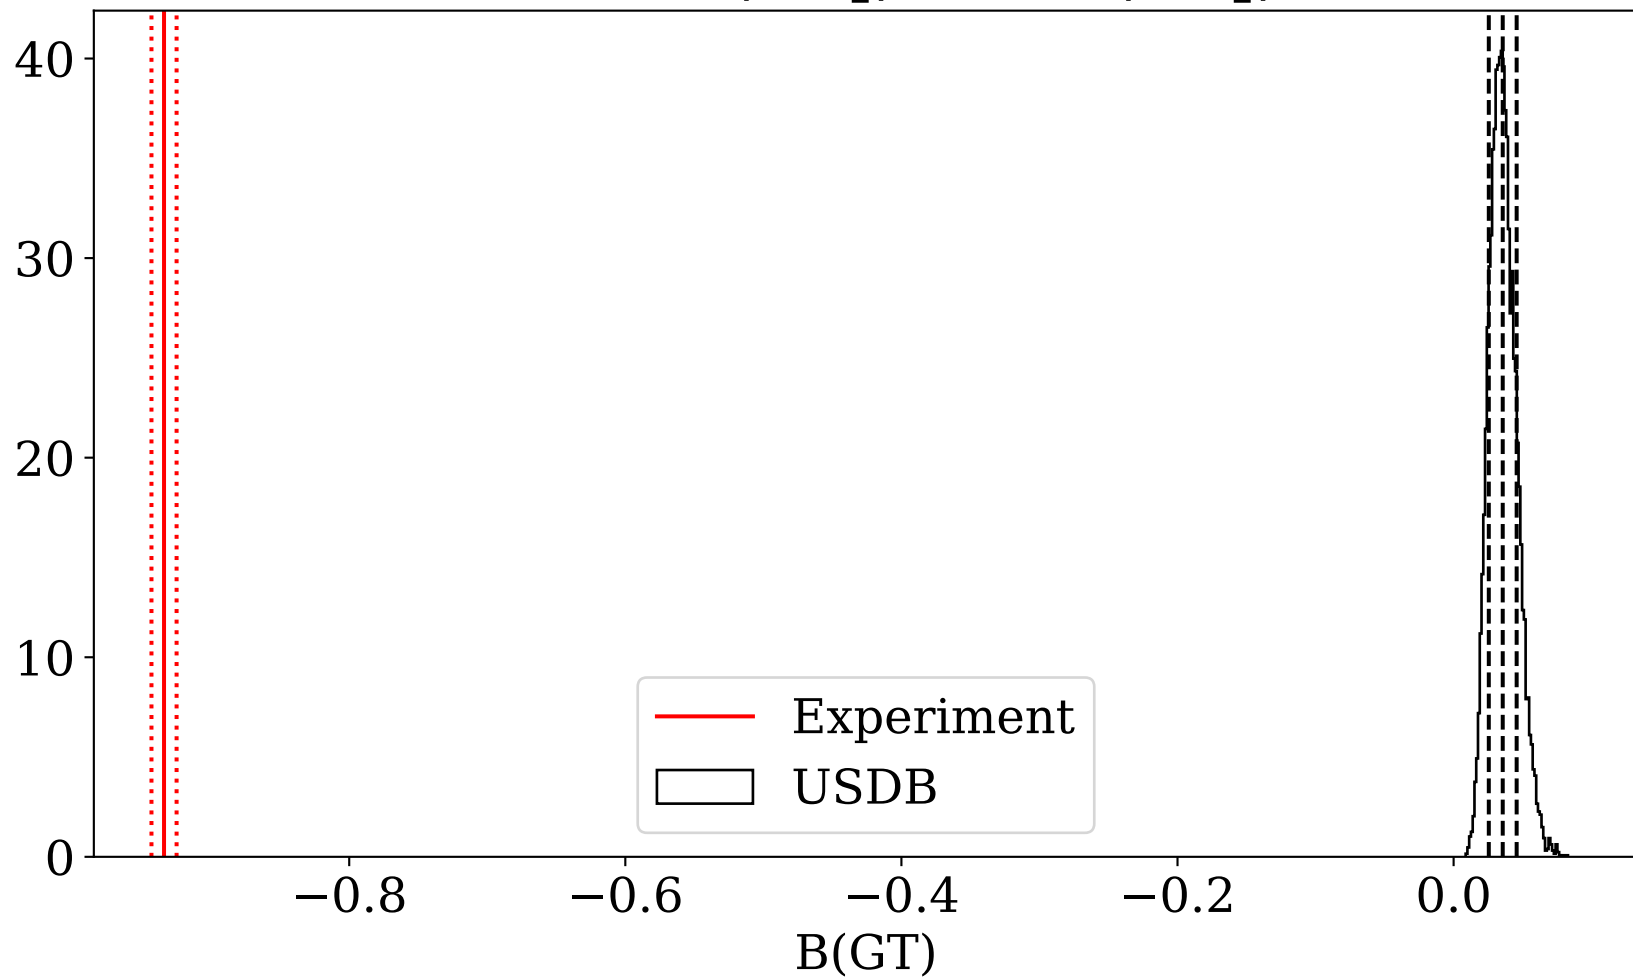

e. c. :  $^{33}\text{Cl}(3/2_1) \rightarrow ^{33}\text{S}(3/2_2)$

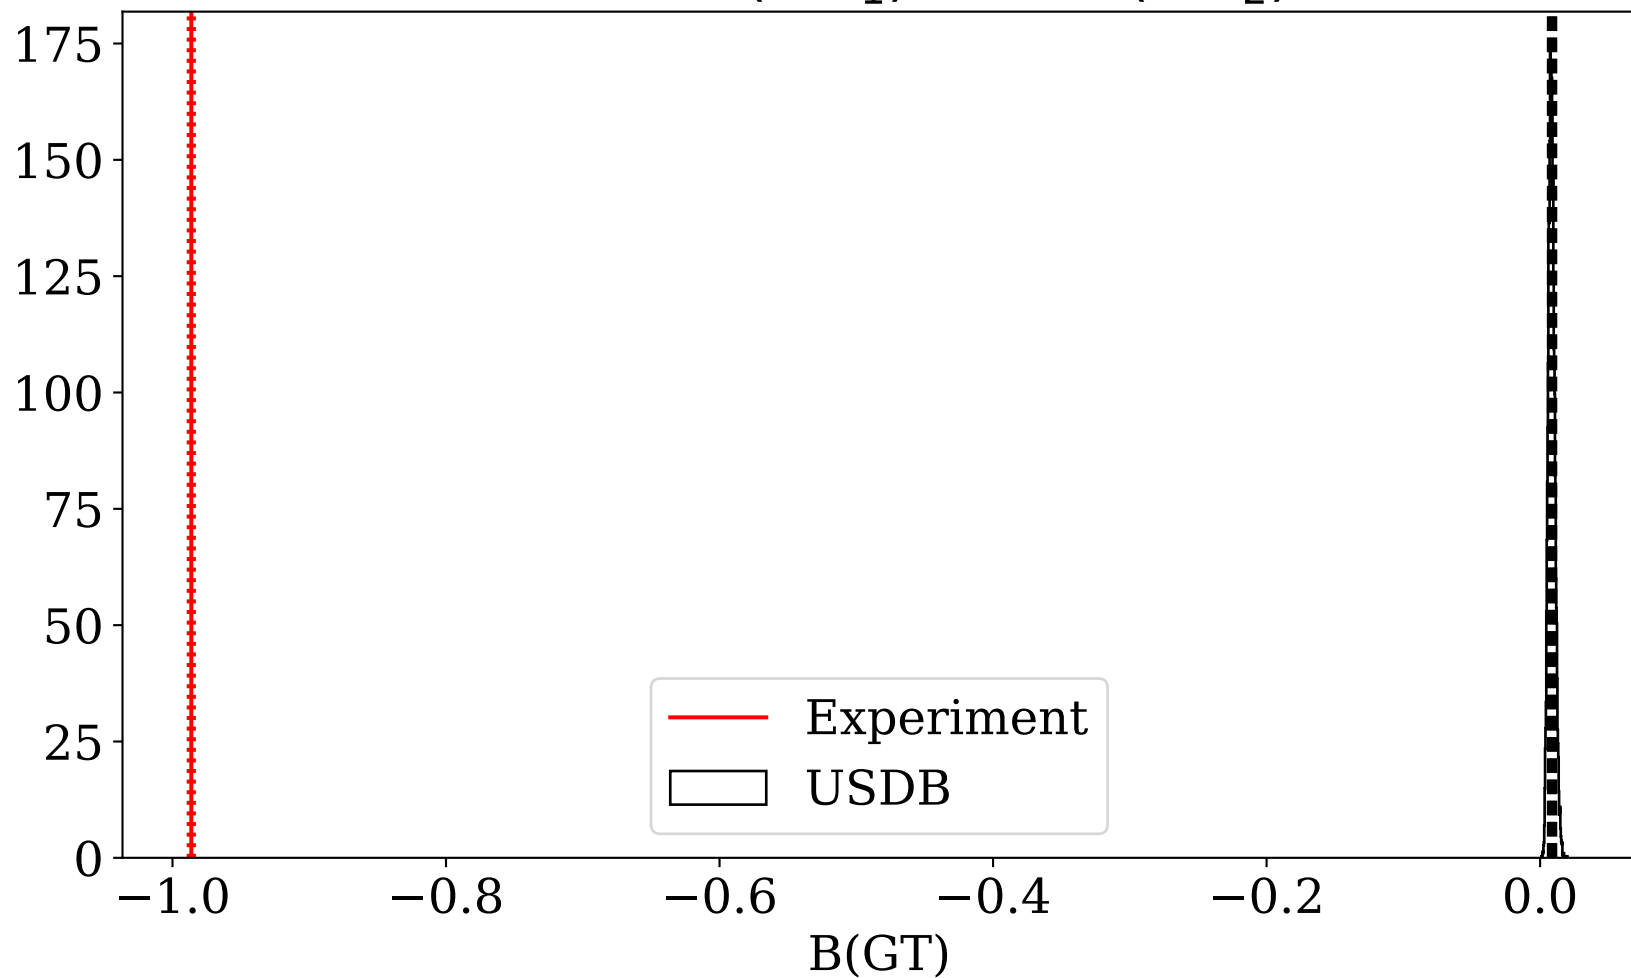

e. c. :  $^{33}\text{Cl}(3/2_1) \rightarrow ^{33}\text{S}(5/2_2)$

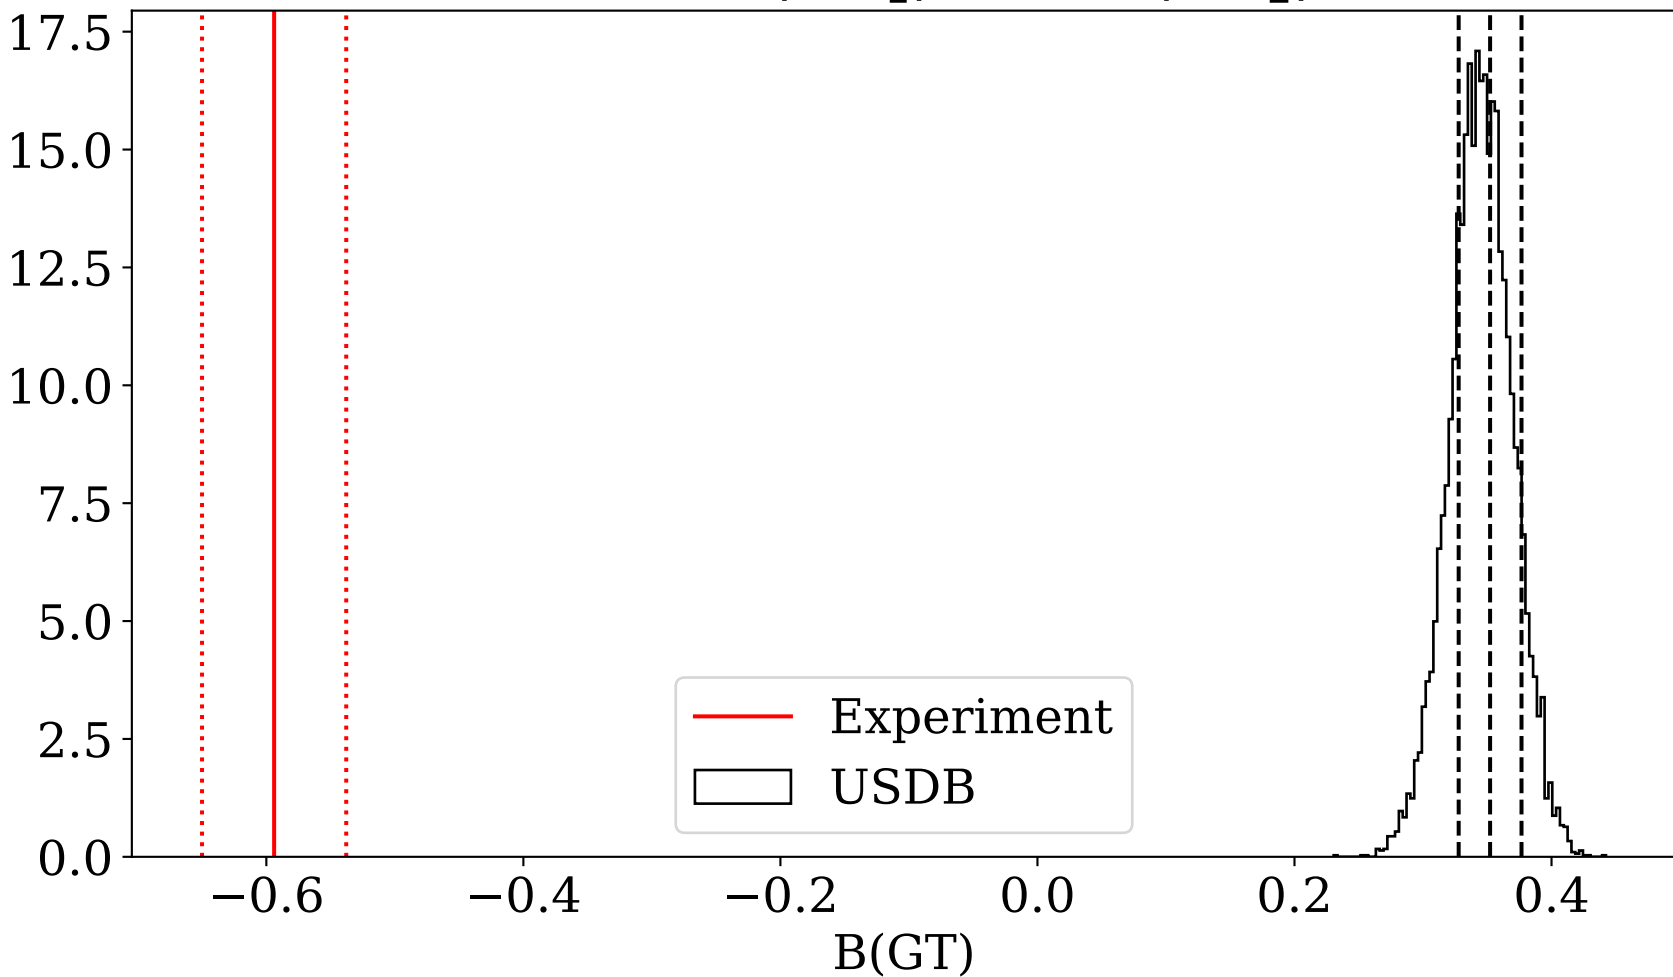



e. c. :  $^{34}\text{Cl}(3_1) \rightarrow ^{34}\text{S}(2_2)$

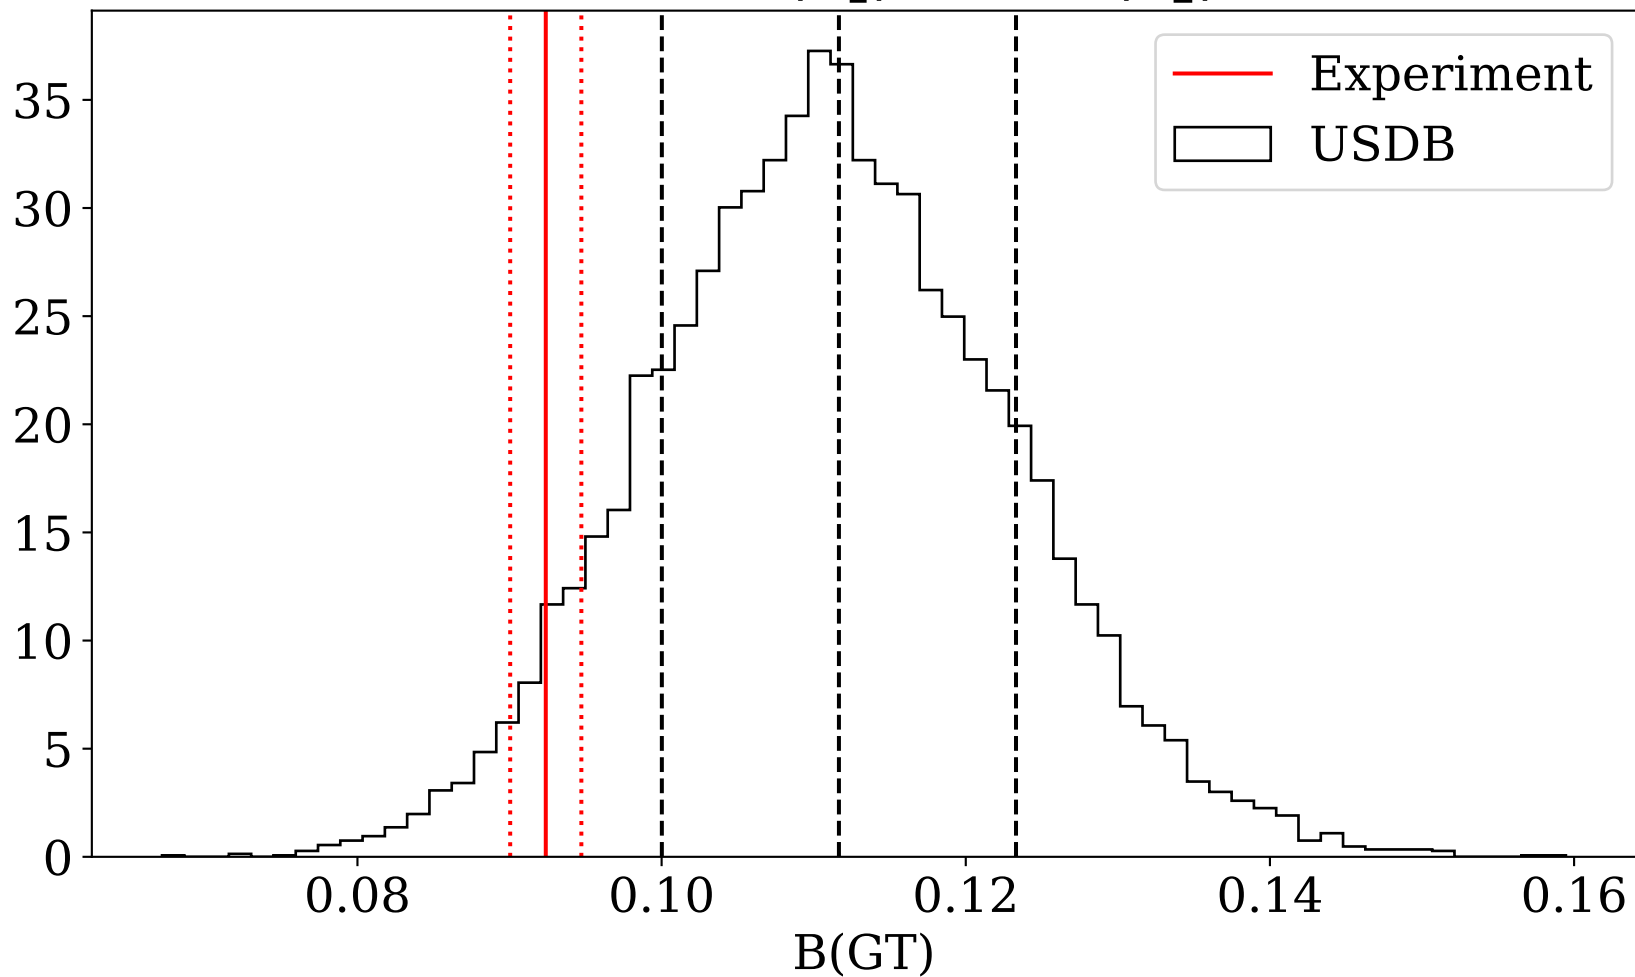

e. c. :  $^{34}\text{Cl}(3_1) \rightarrow ^{34}\text{S}(2_3)$

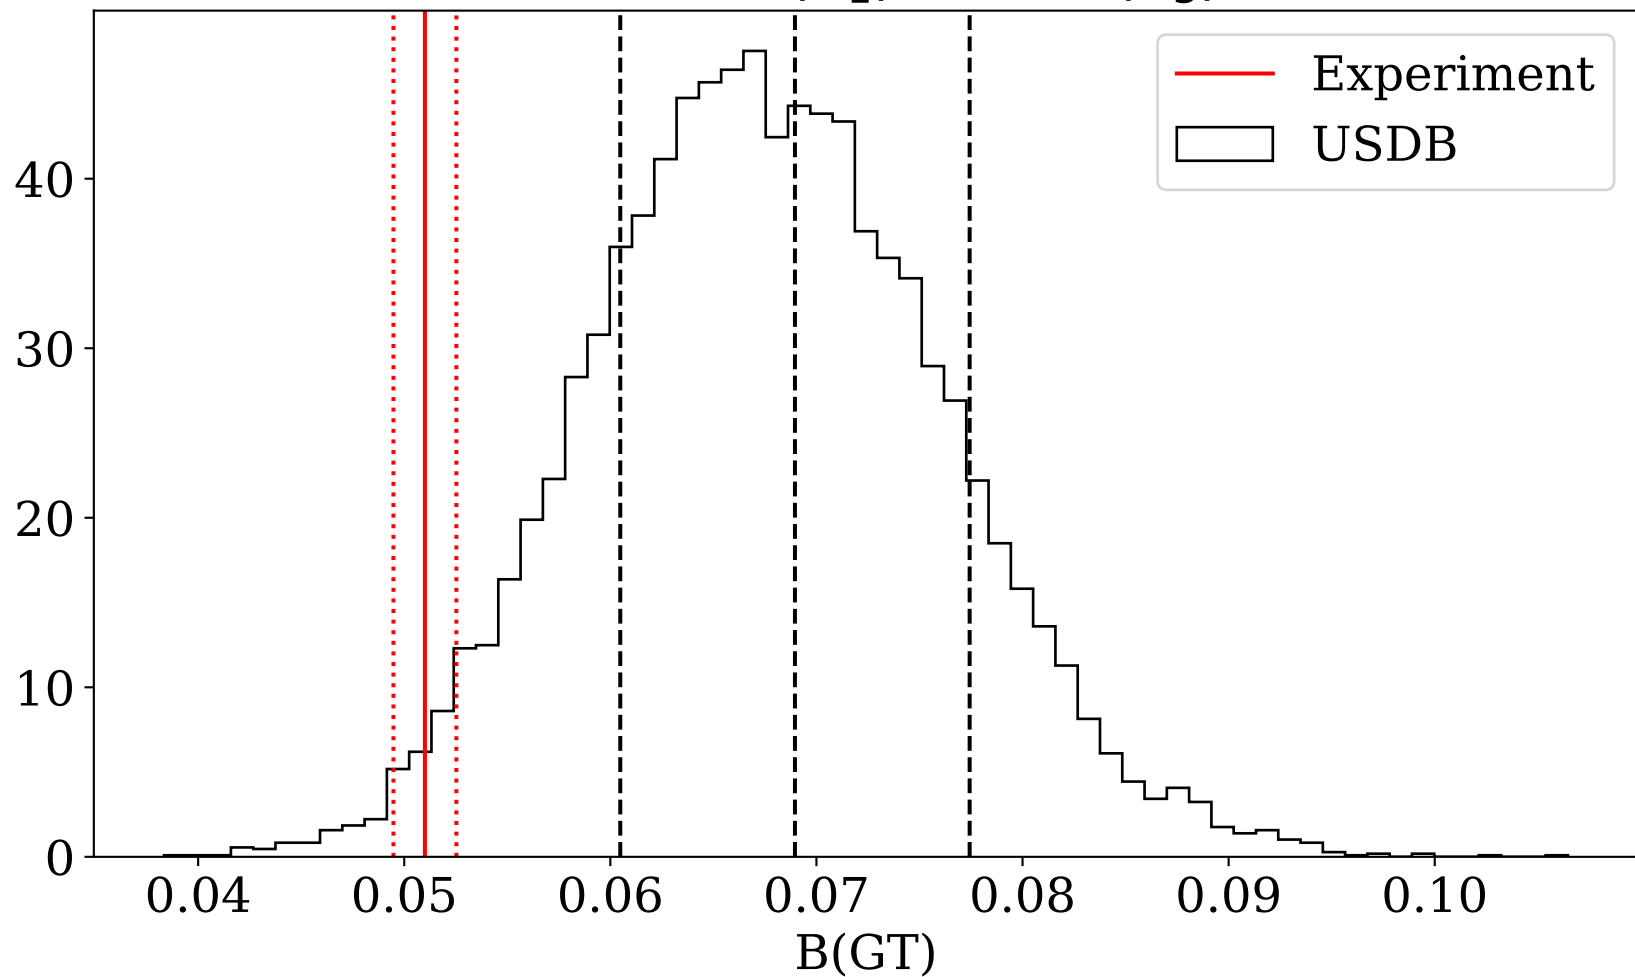

e. c. :  $^{35}\text{Ar}(3/2_1) \rightarrow ^{35}\text{Cl}(3/2_1)$

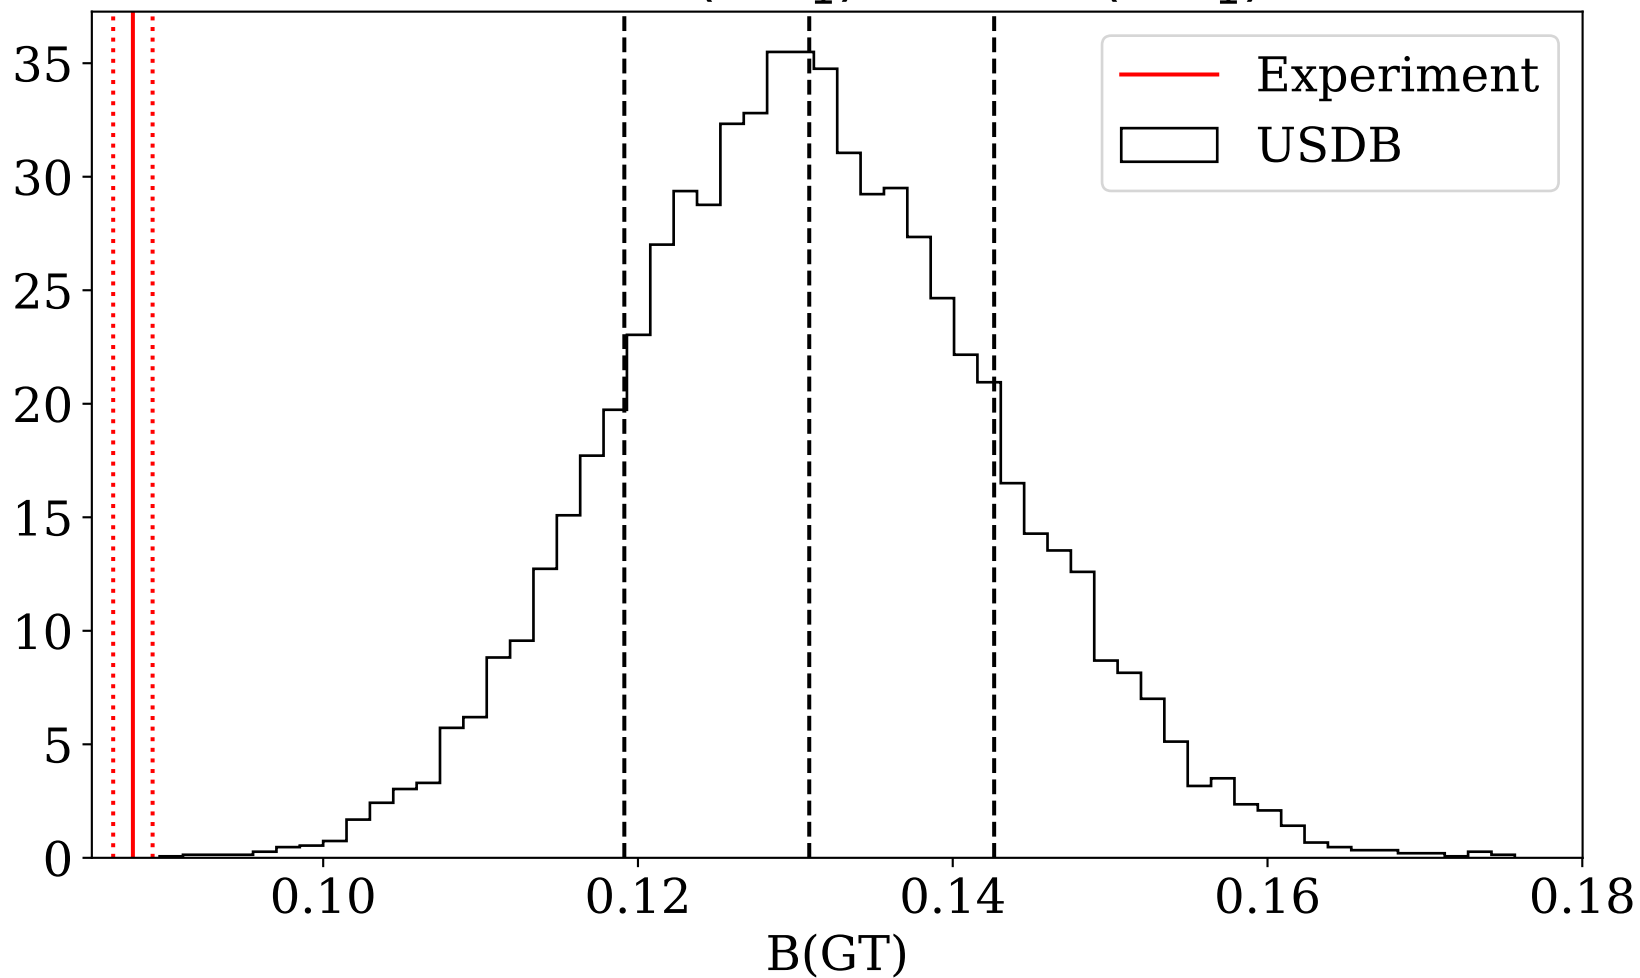

*e. c. :*  $^{35}\text{Ar}(3/2_1) \rightarrow ^{35}\text{Cl}(1/2_1)$

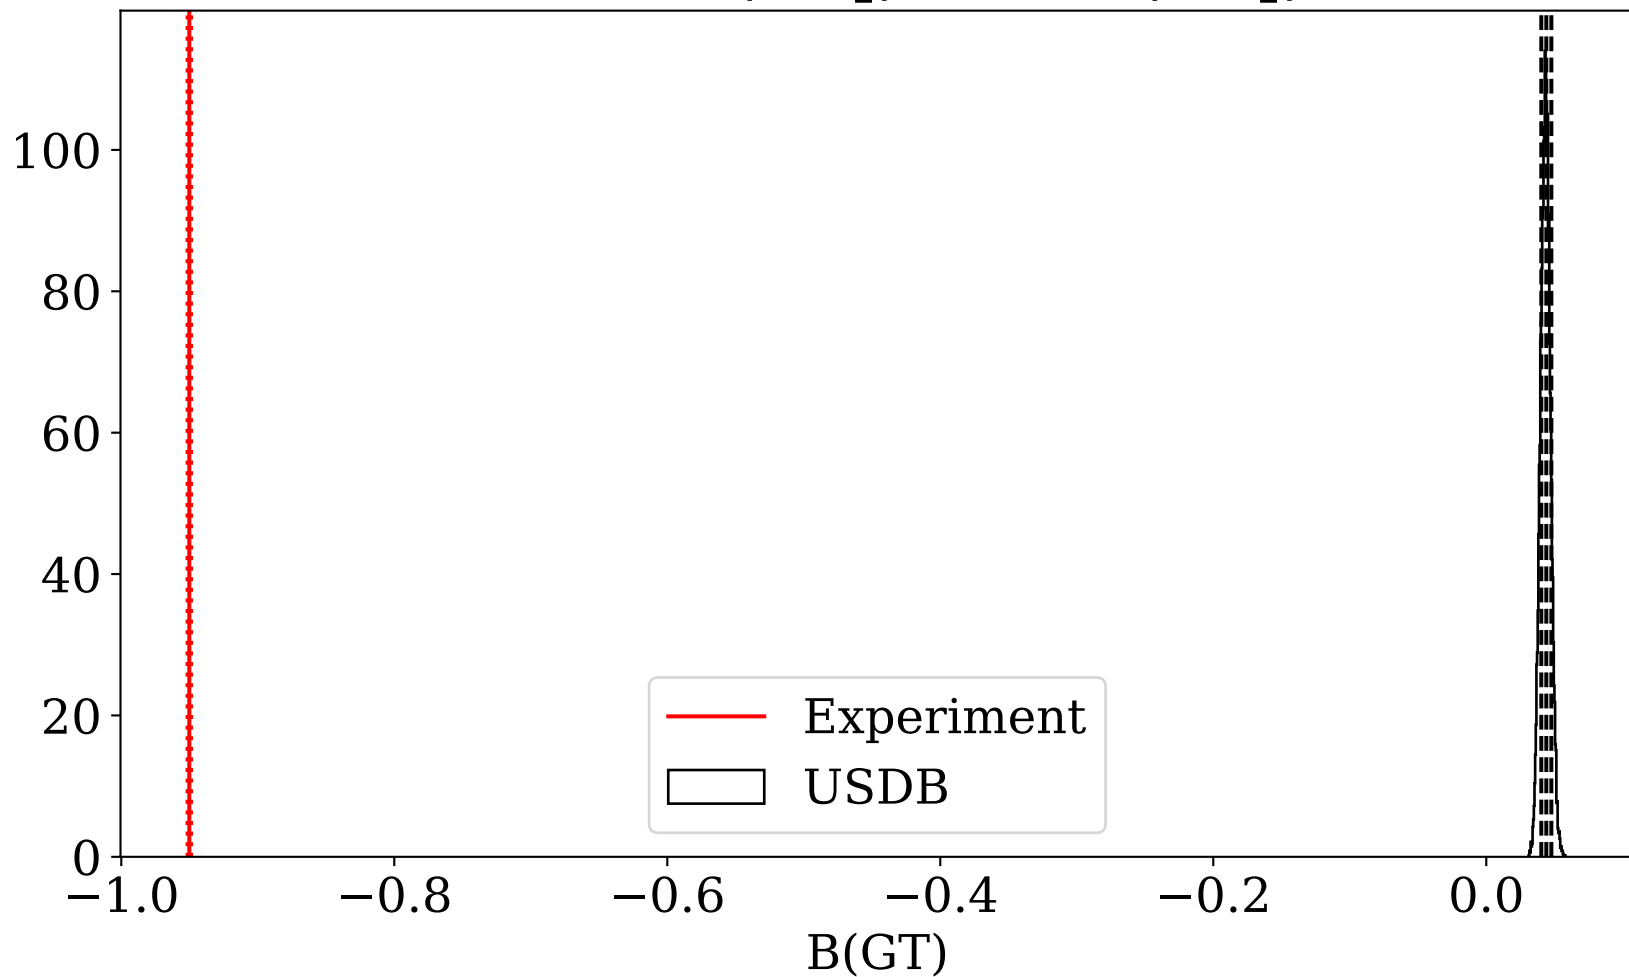

*e. c. :*  $^{35}\text{Ar}(3/2_1) \rightarrow ^{35}\text{Cl}(5/2_1)$

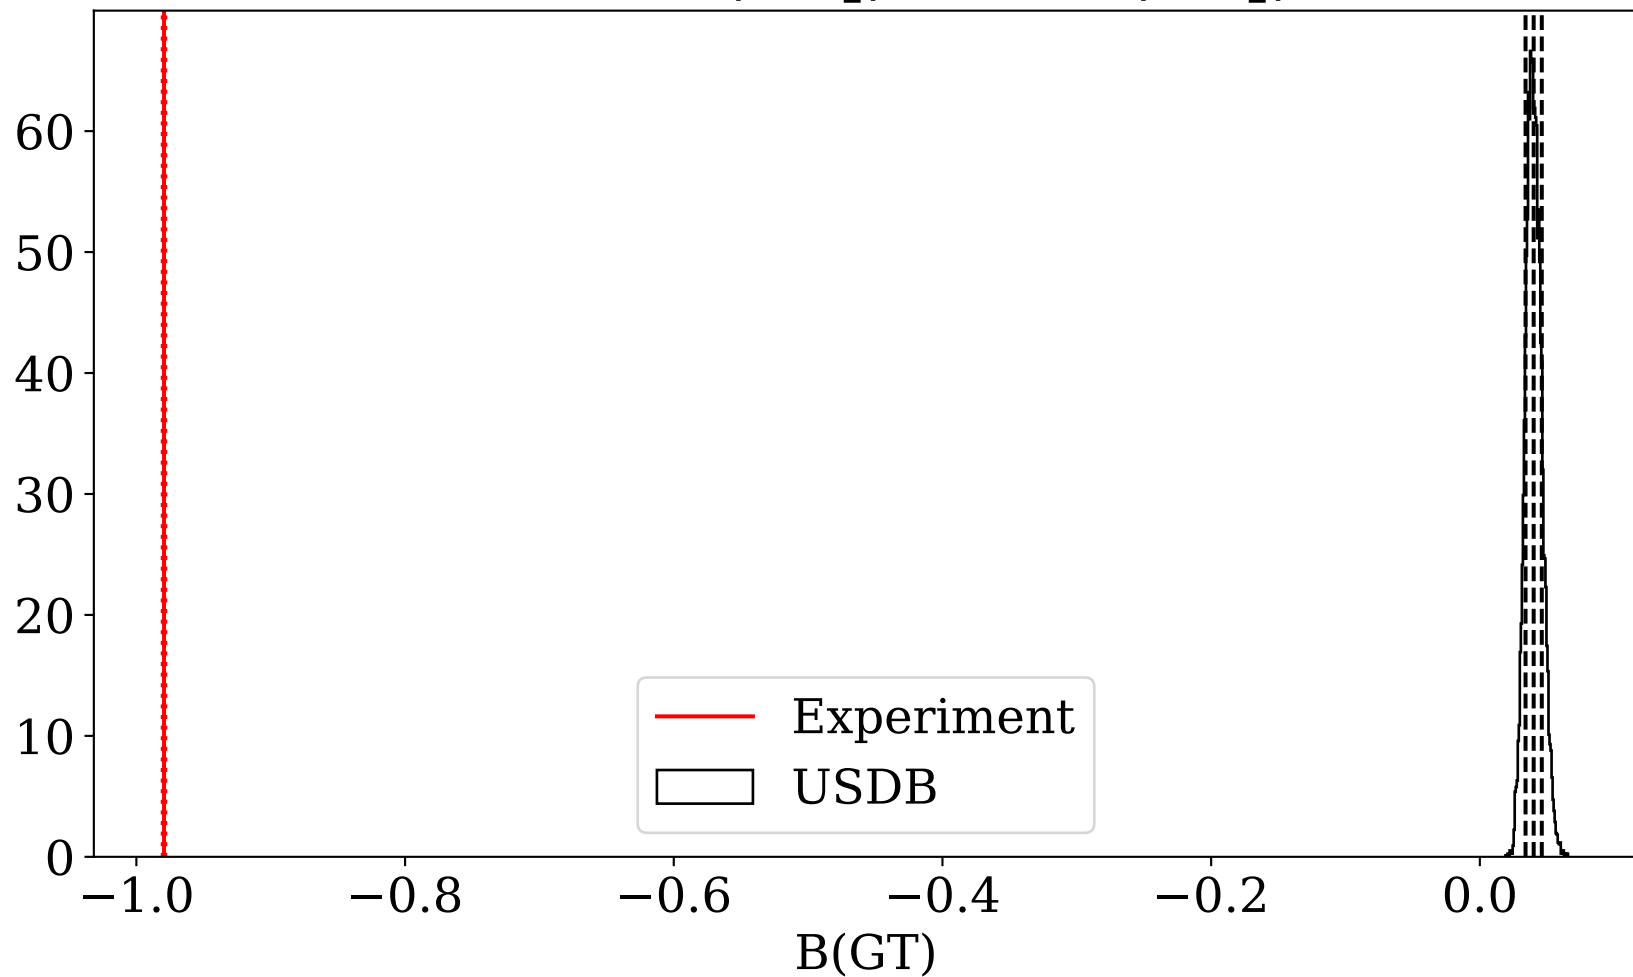

*e. c.* :  $^{35}\text{Ar}(3/2_1) \rightarrow ^{35}\text{Cl}(3/2_3)$

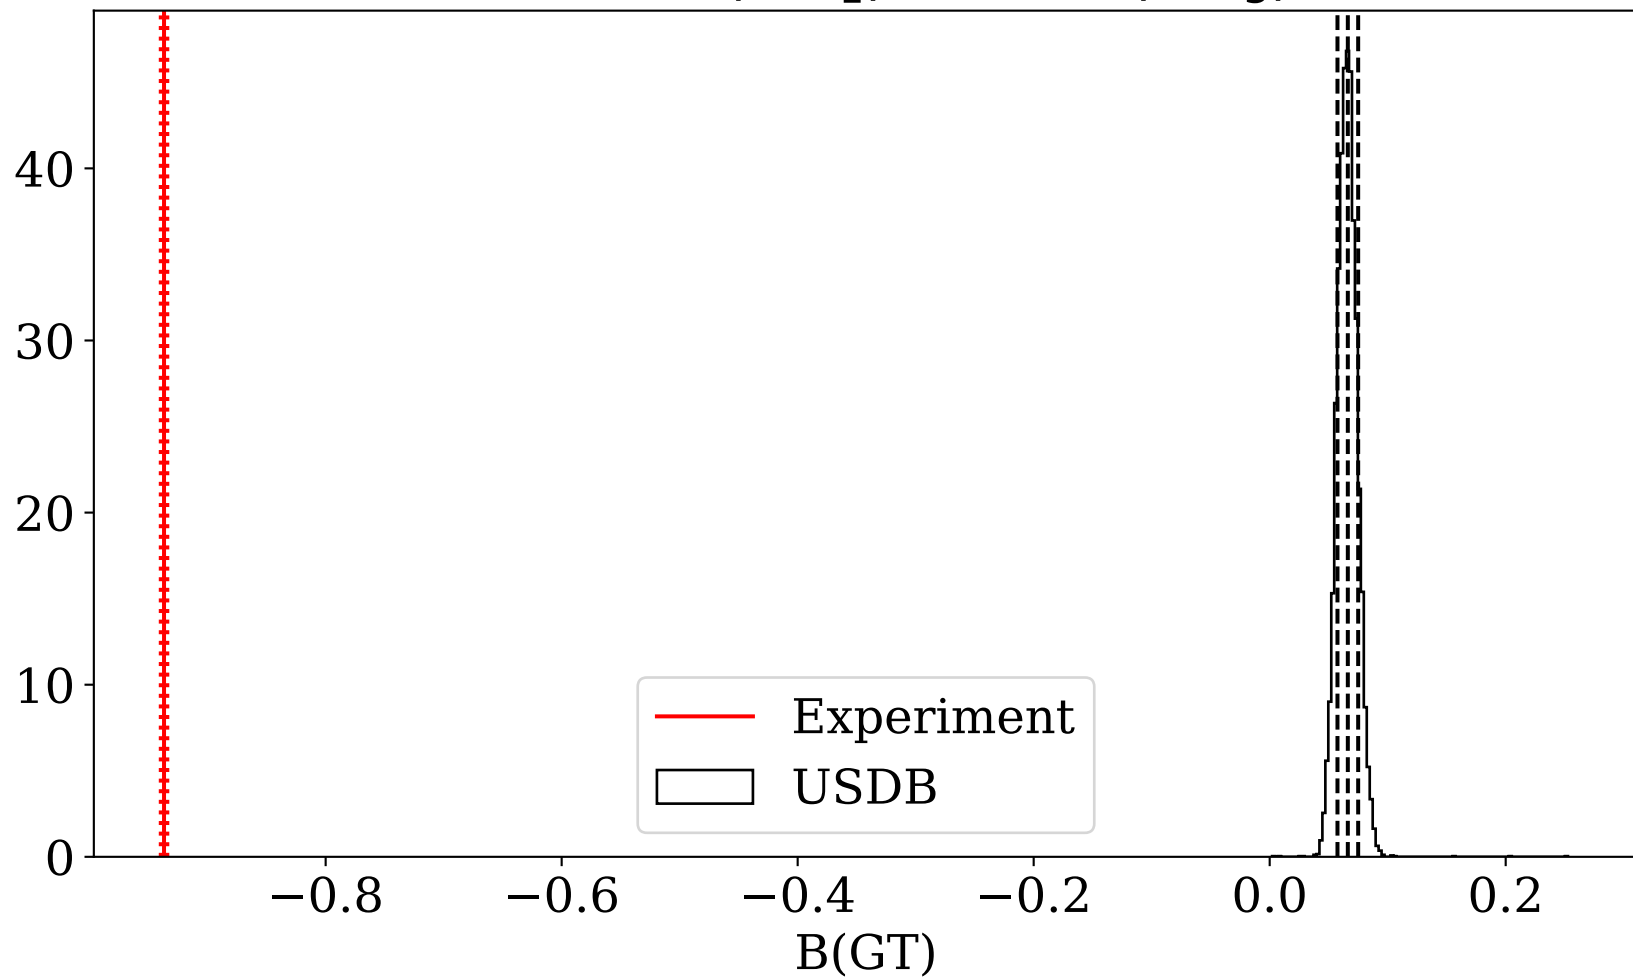

*e. c. :*  $^{35}\text{Ar}(3/2_1) \rightarrow ^{35}\text{Cl}(5/2_2)$

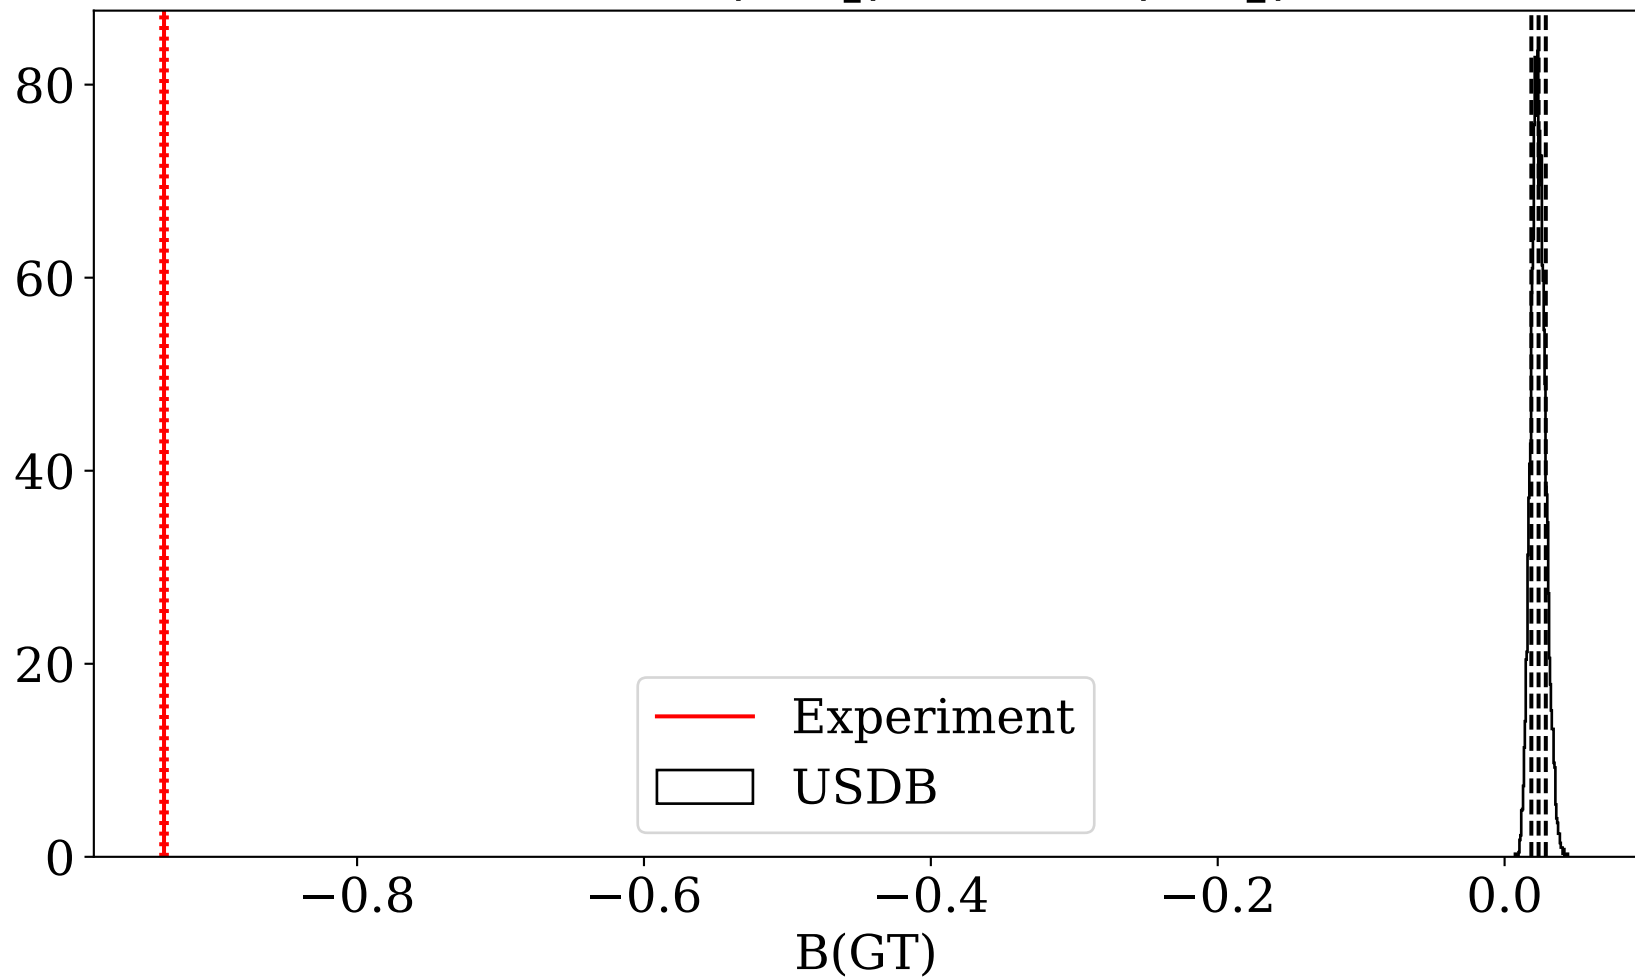

e. c. :  $^{35}\text{K}(3/2_1) \rightarrow ^{35}\text{Ar}(3/2_1)$

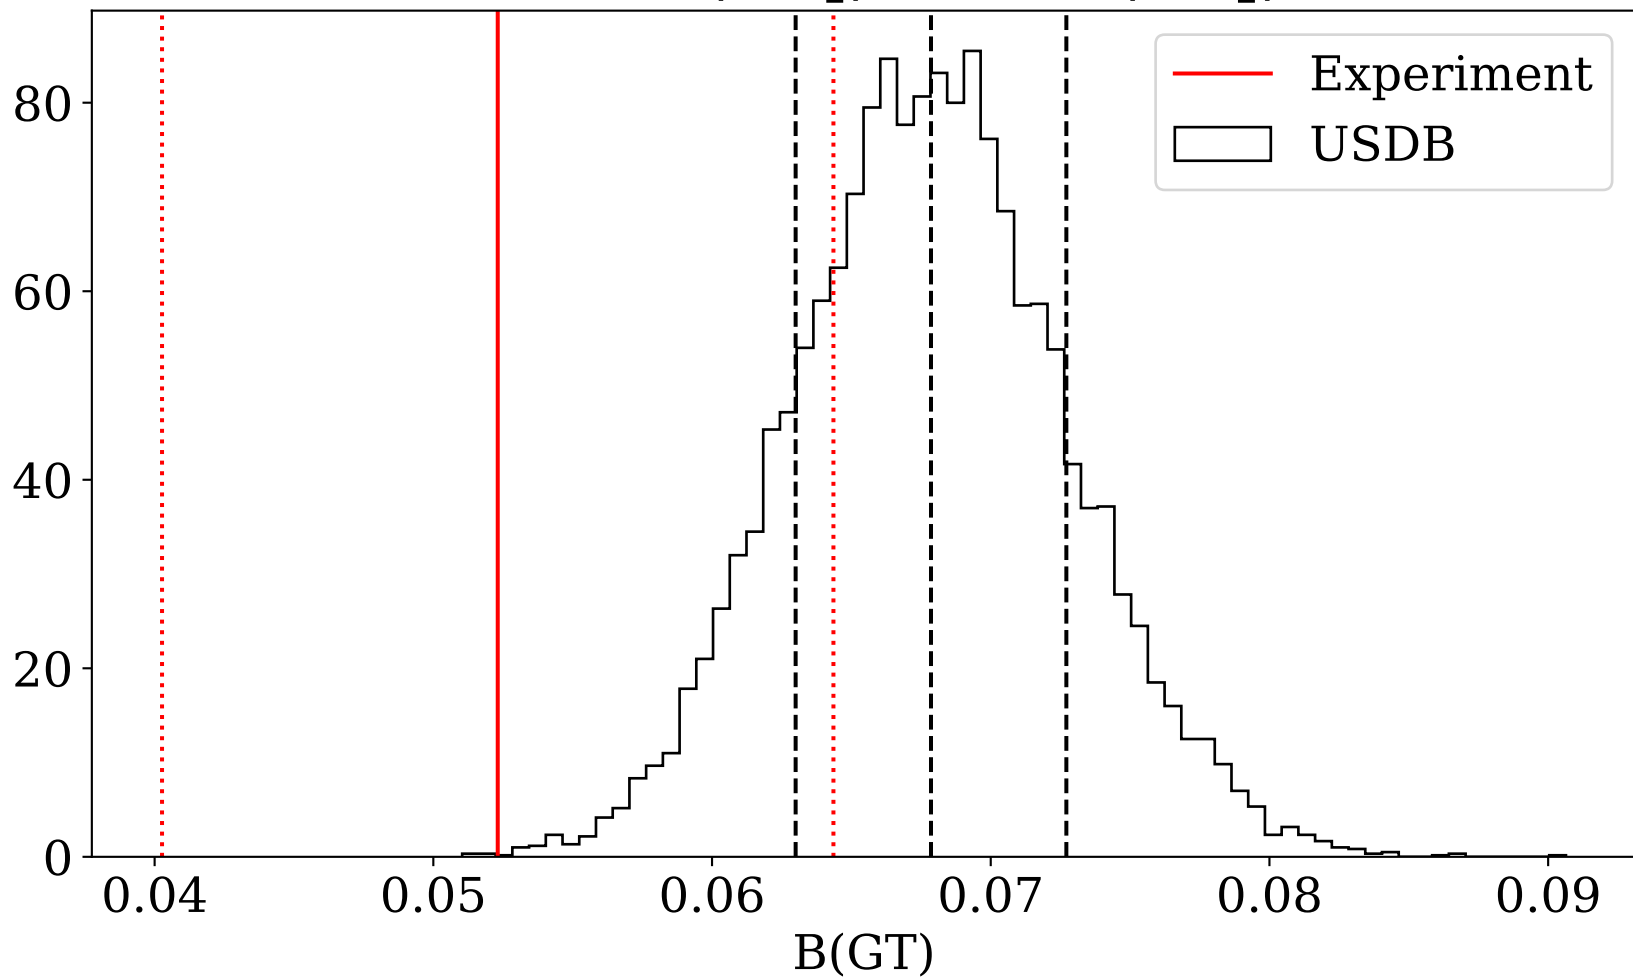



e. c. :  $^{35}\text{K}(3/2_1) \rightarrow ^{35}\text{Ar}(1/2_1)$

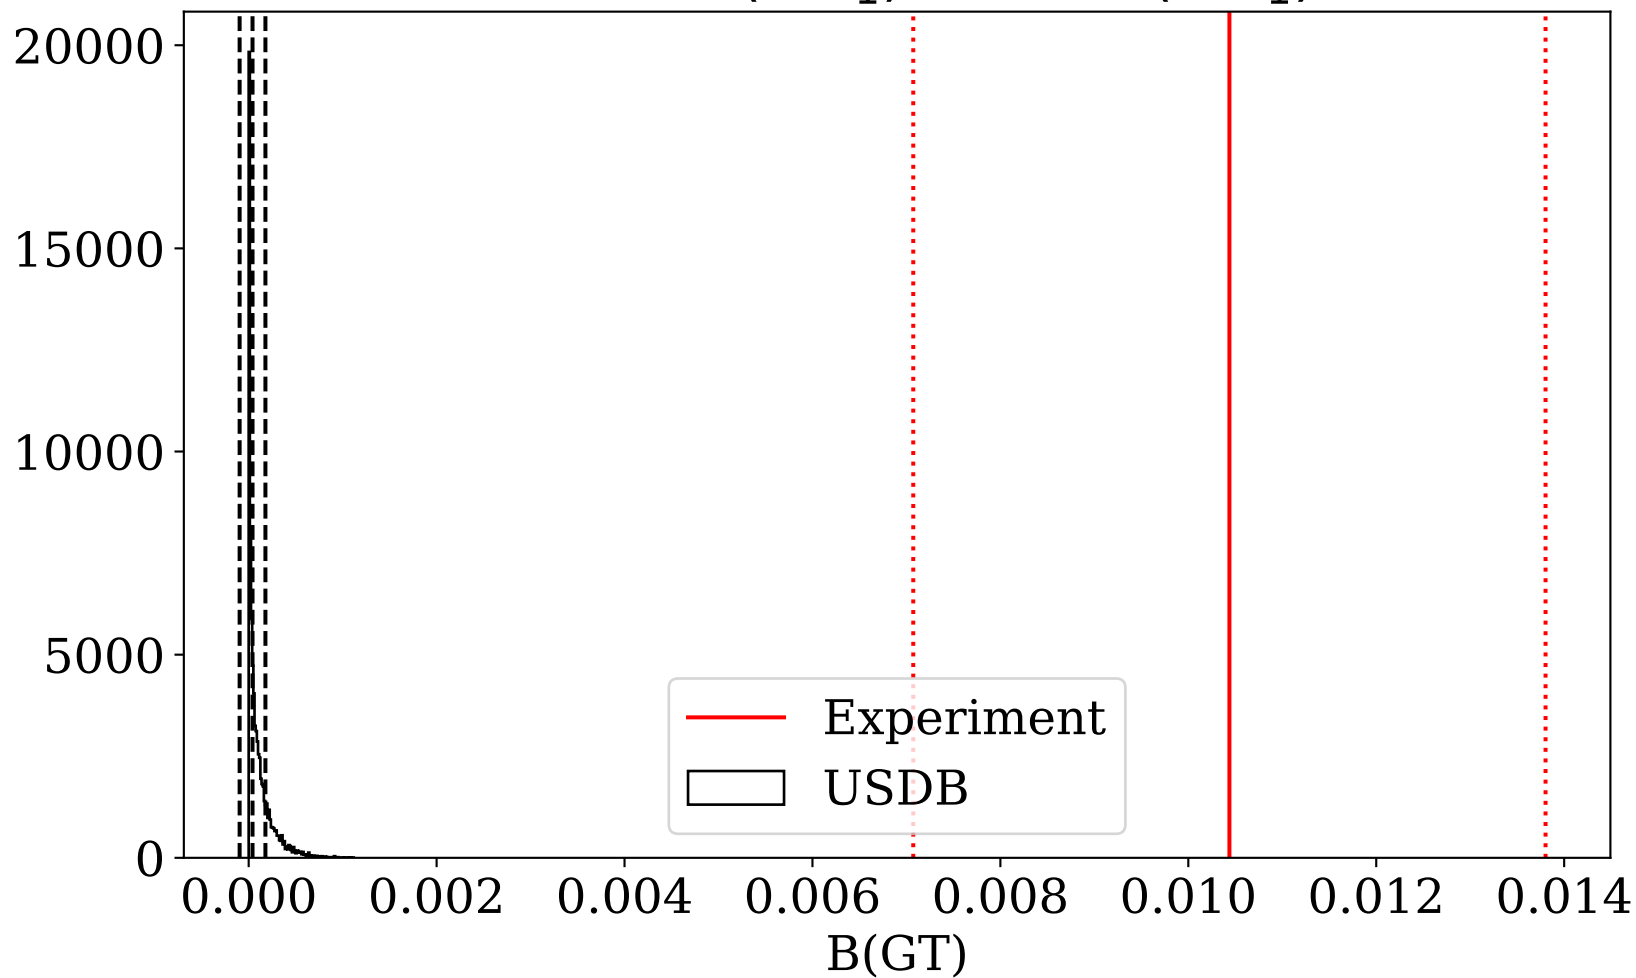

e. c. :  $^{35}\text{K}(3/2_1) \rightarrow ^{35}\text{Ar}(5/2_1)$

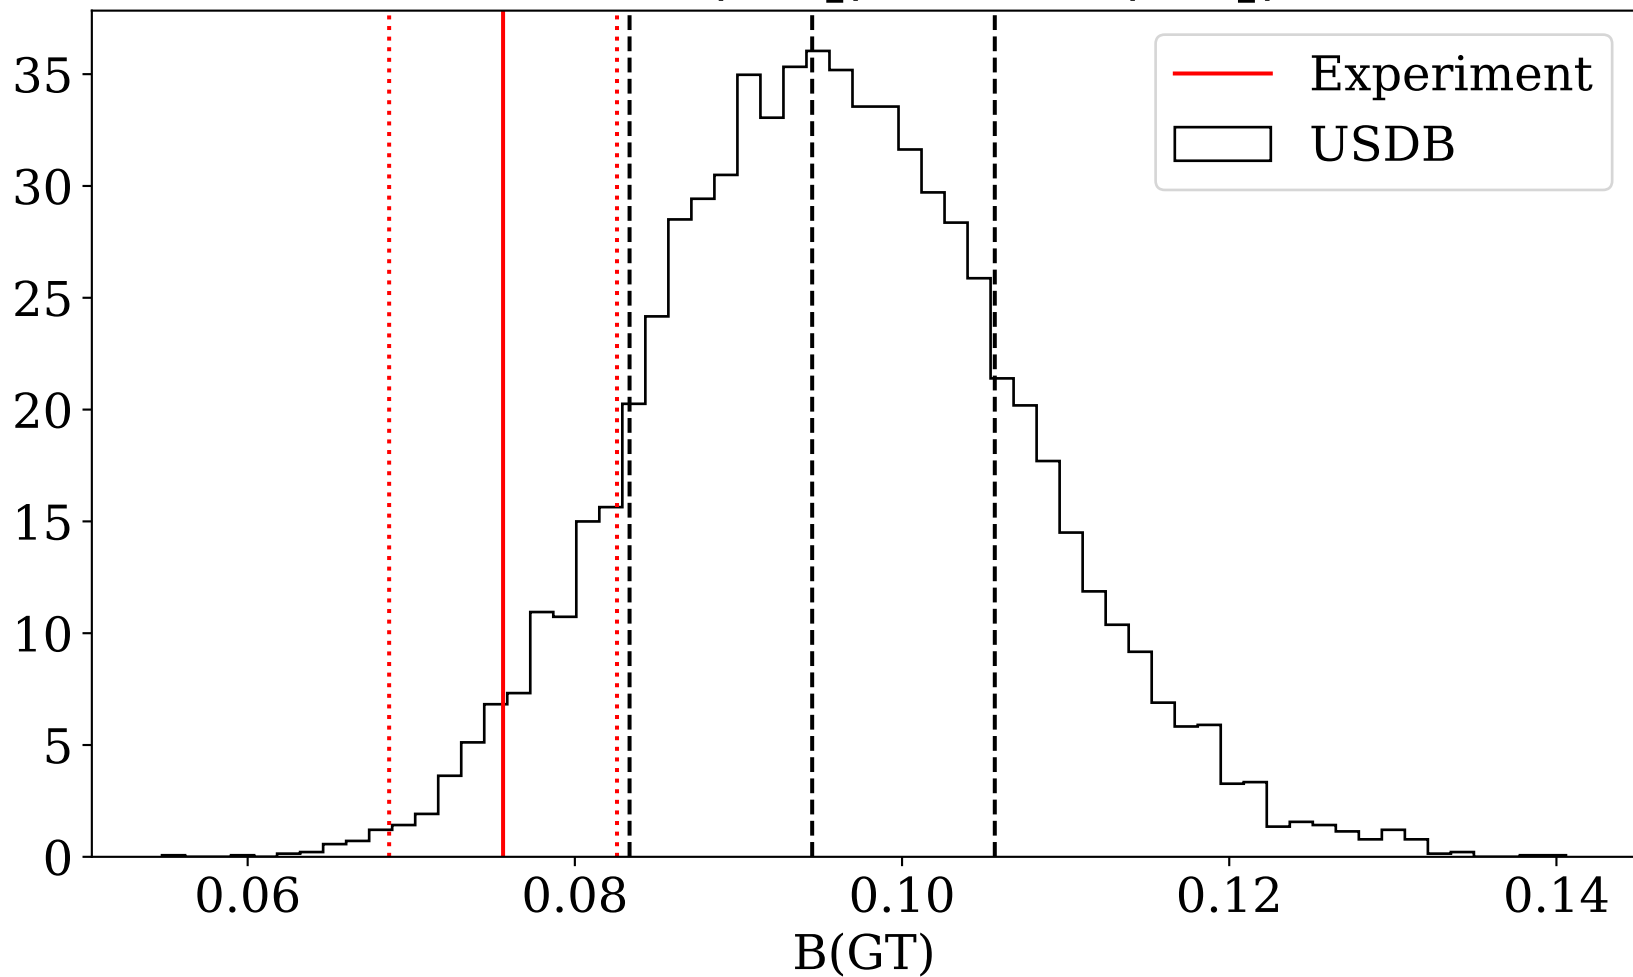

e. c. :  $^{35}\text{K}(3/2_1) \rightarrow ^{35}\text{Ar}(1/2_2)$

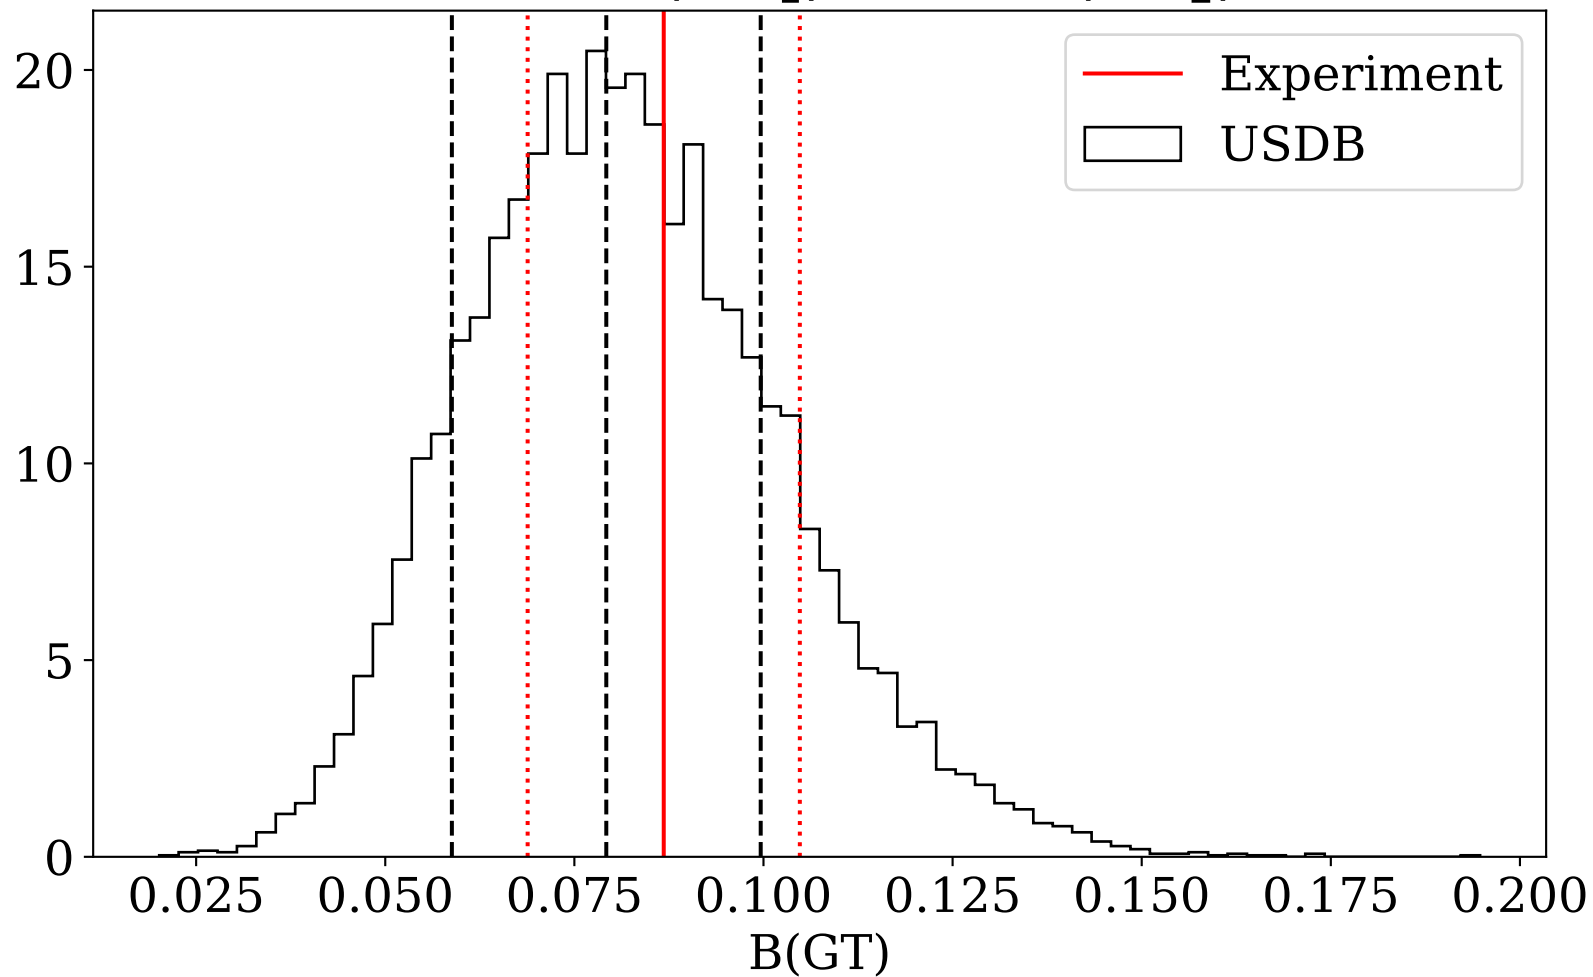

e. c. :  $^{35}\text{K}(3/2_1) \rightarrow ^{35}\text{Ar}(1/2_3)$

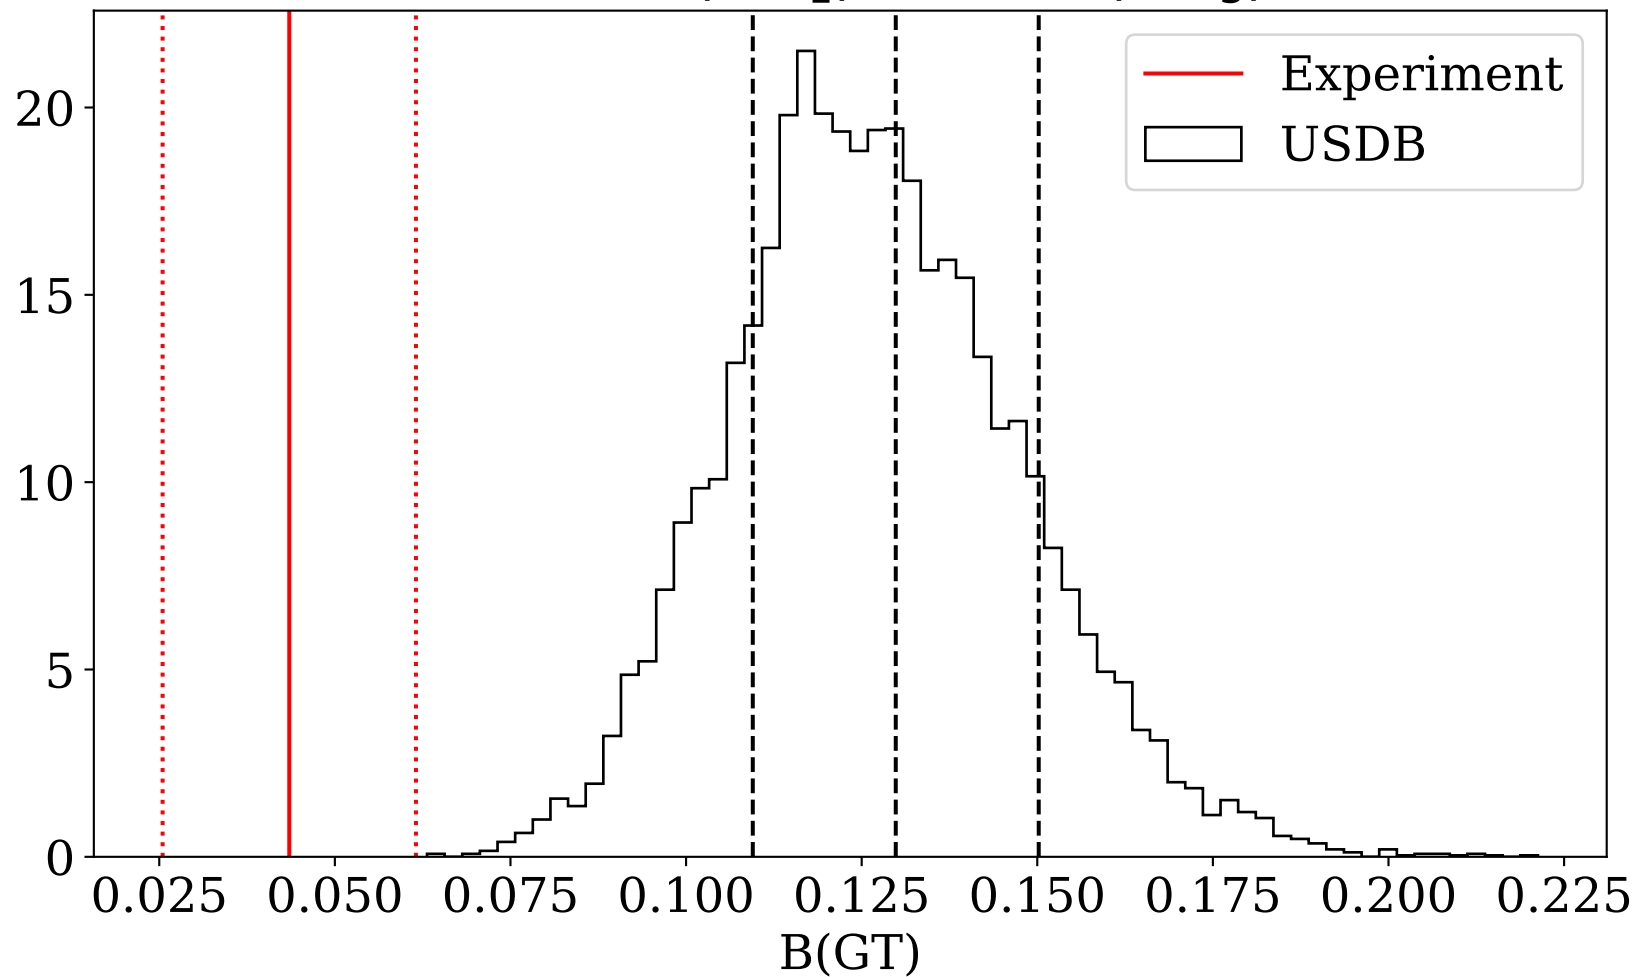

e. c. :  $^{35}\text{K}(3/2_1) \rightarrow ^{35}\text{Ar}(3/2_3)$

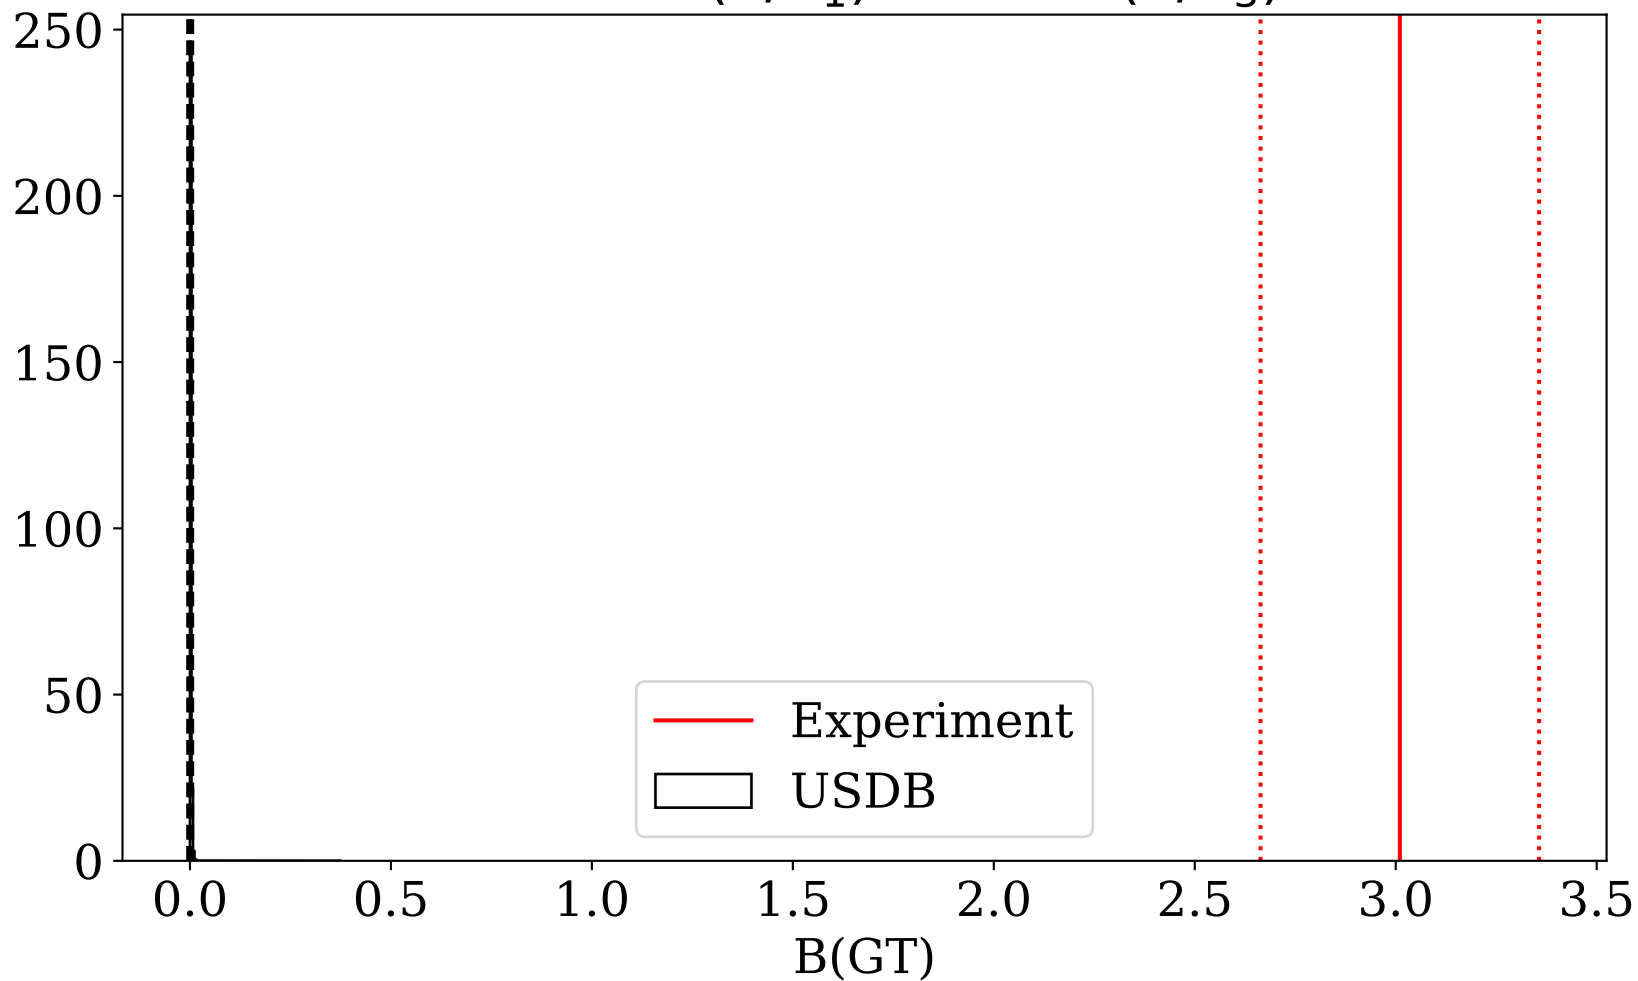

*e. c. :*  $^{36}\text{K}(2_1) \rightarrow ^{36}\text{Ar}(2_1)$

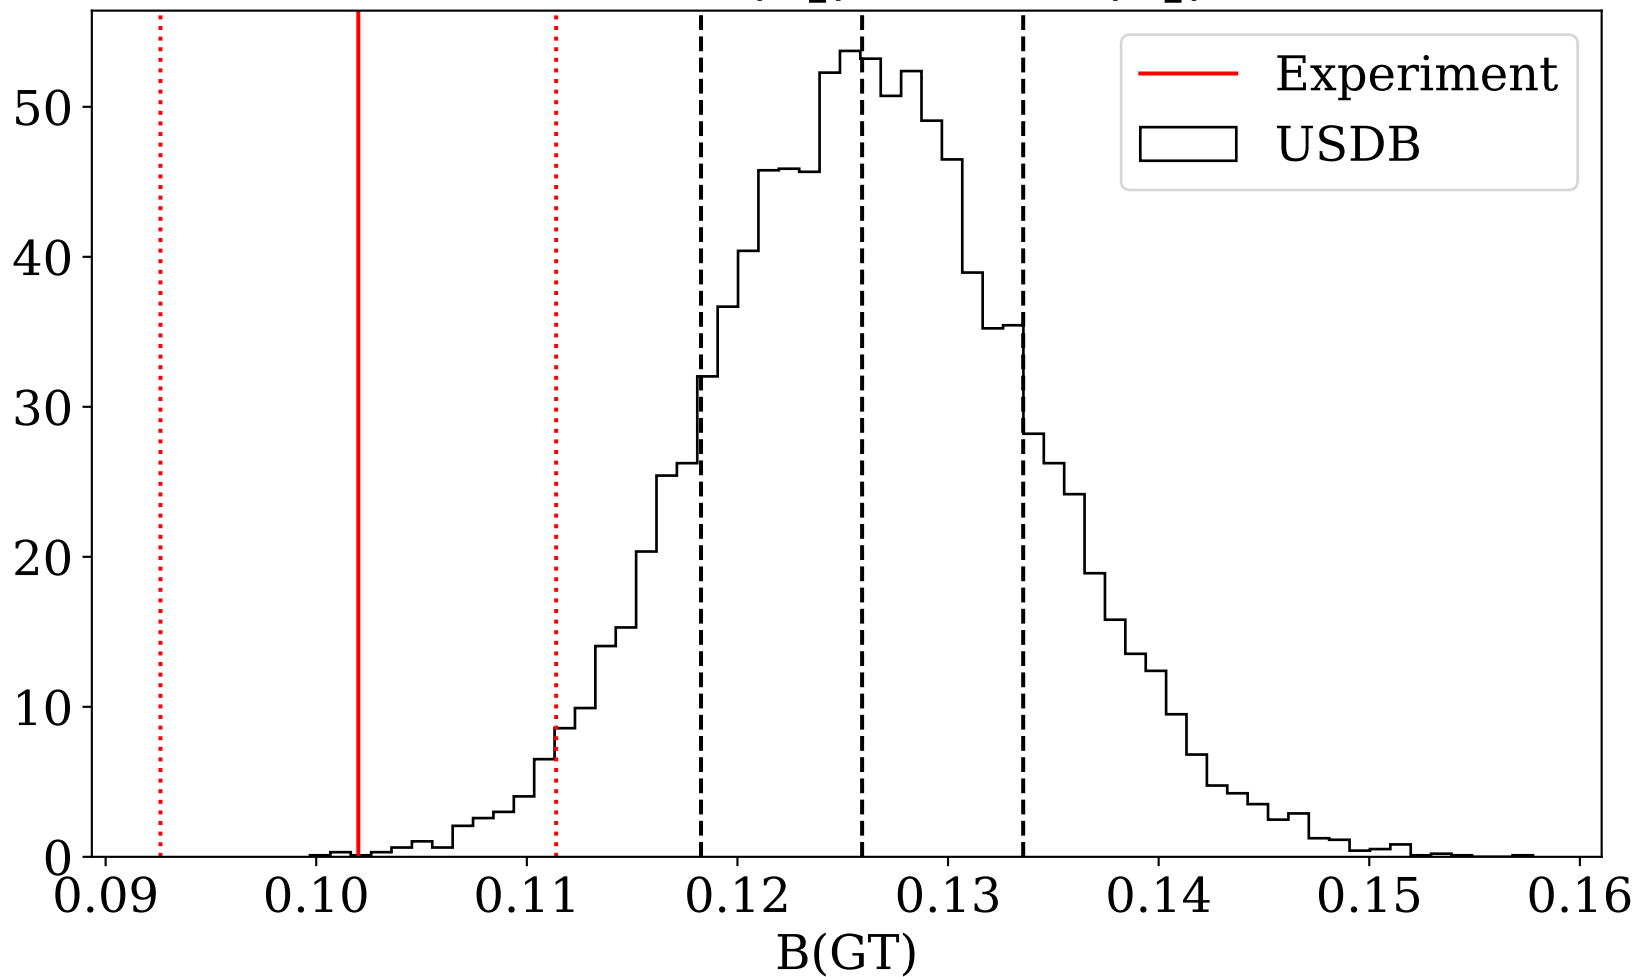

e. c. :  $^{36}\text{K}(2_1) \rightarrow ^{36}\text{Ar}(2_2)$

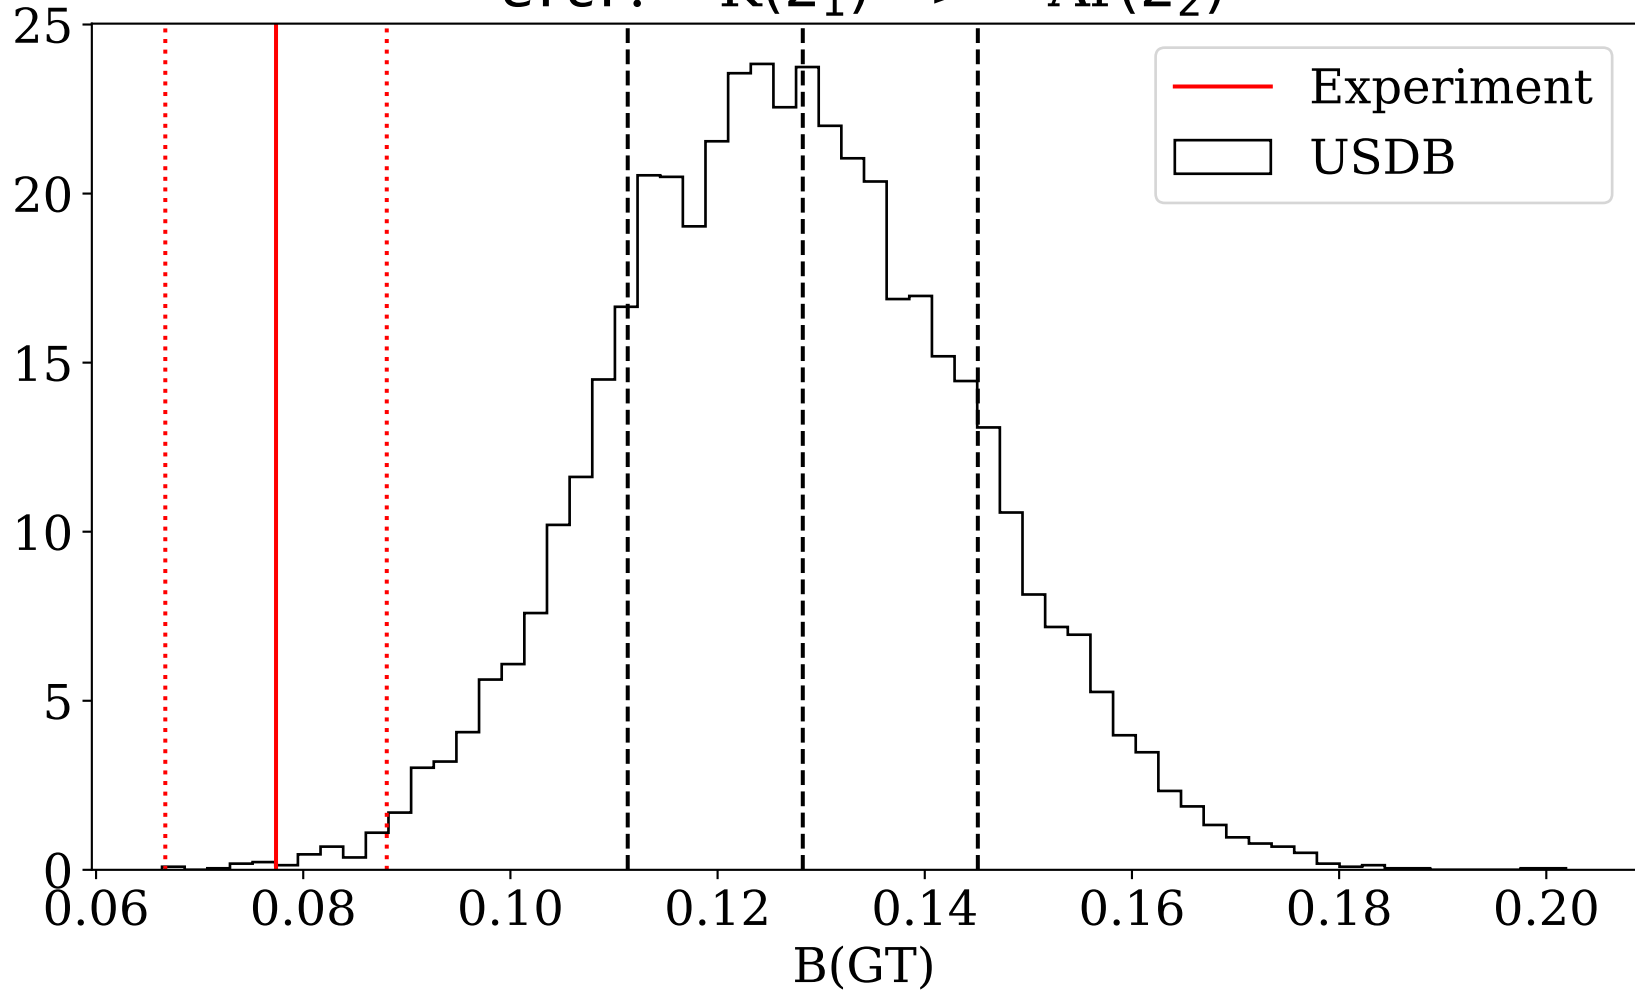

*e. c.* :  $^{36}\text{K}(2_1) \rightarrow ^{36}\text{Ar}(2_3)$

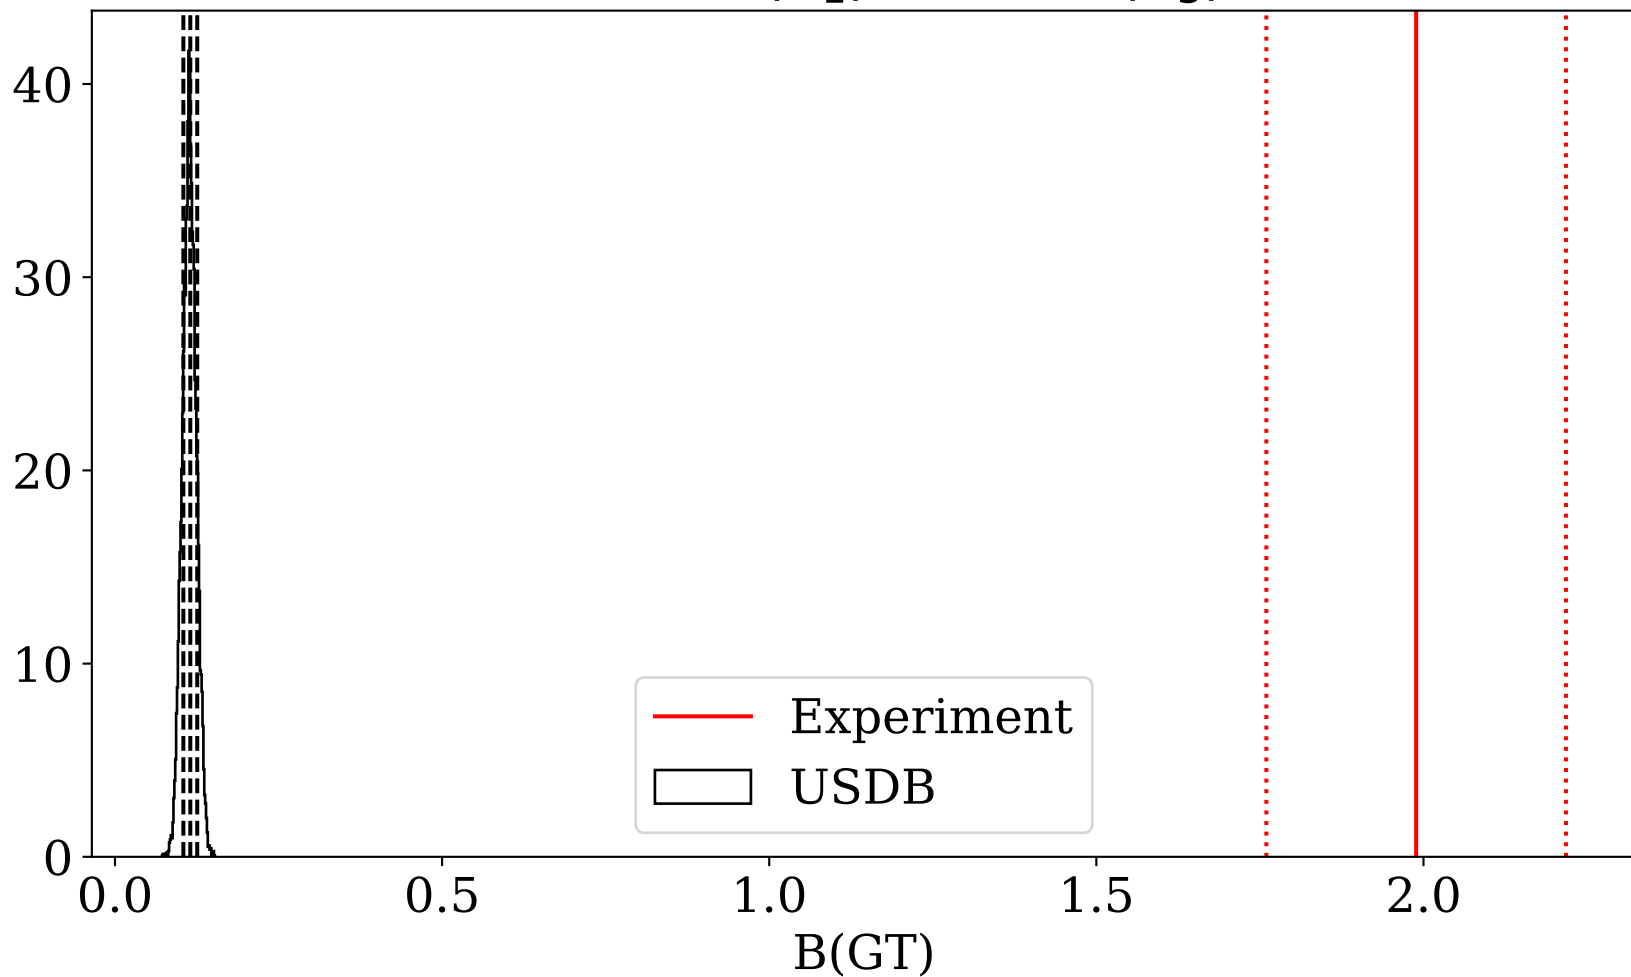



e. c. :  $^{37}\text{K}(3/2_1) \rightarrow ^{37}\text{Ar}(3/2_1)$

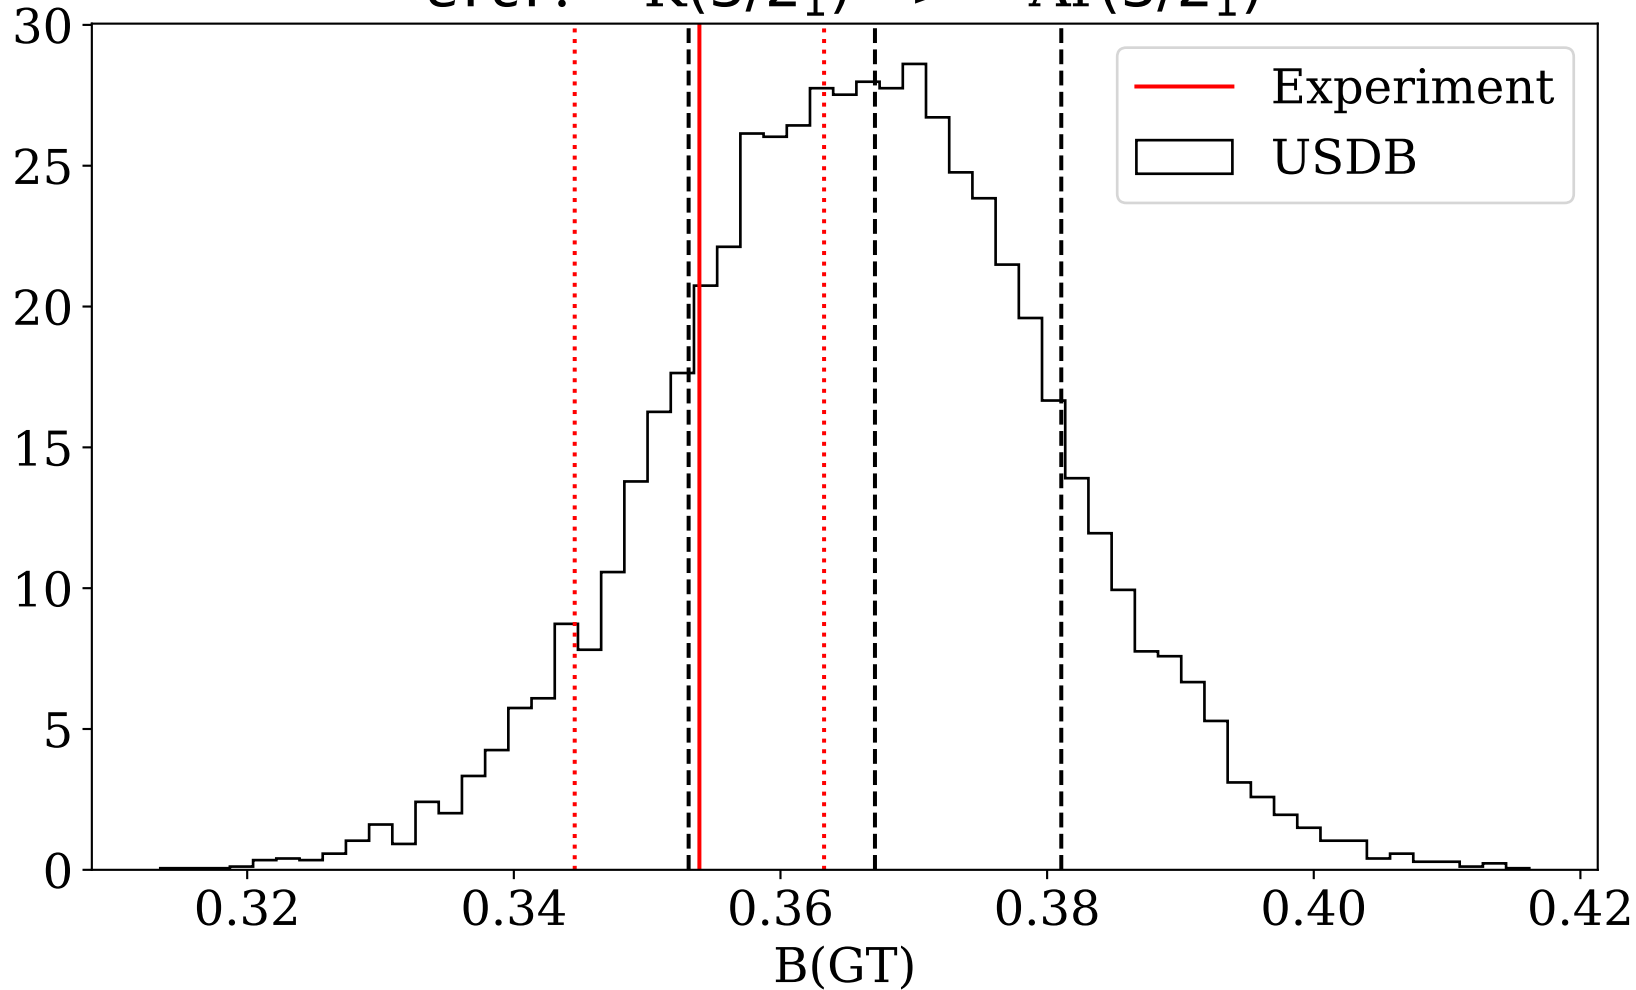

Supplement: Supplementary file 4 [file GT_histograms.pdf]
