# Supplementary material for: Uncertainty quantification of transition operators in the empirical shell model
Source: arXiv:2206.14956 source file (2023-10-09)

$^{18}\text{O} (2_2) \rightarrow (2_1)$   
Included in UQ

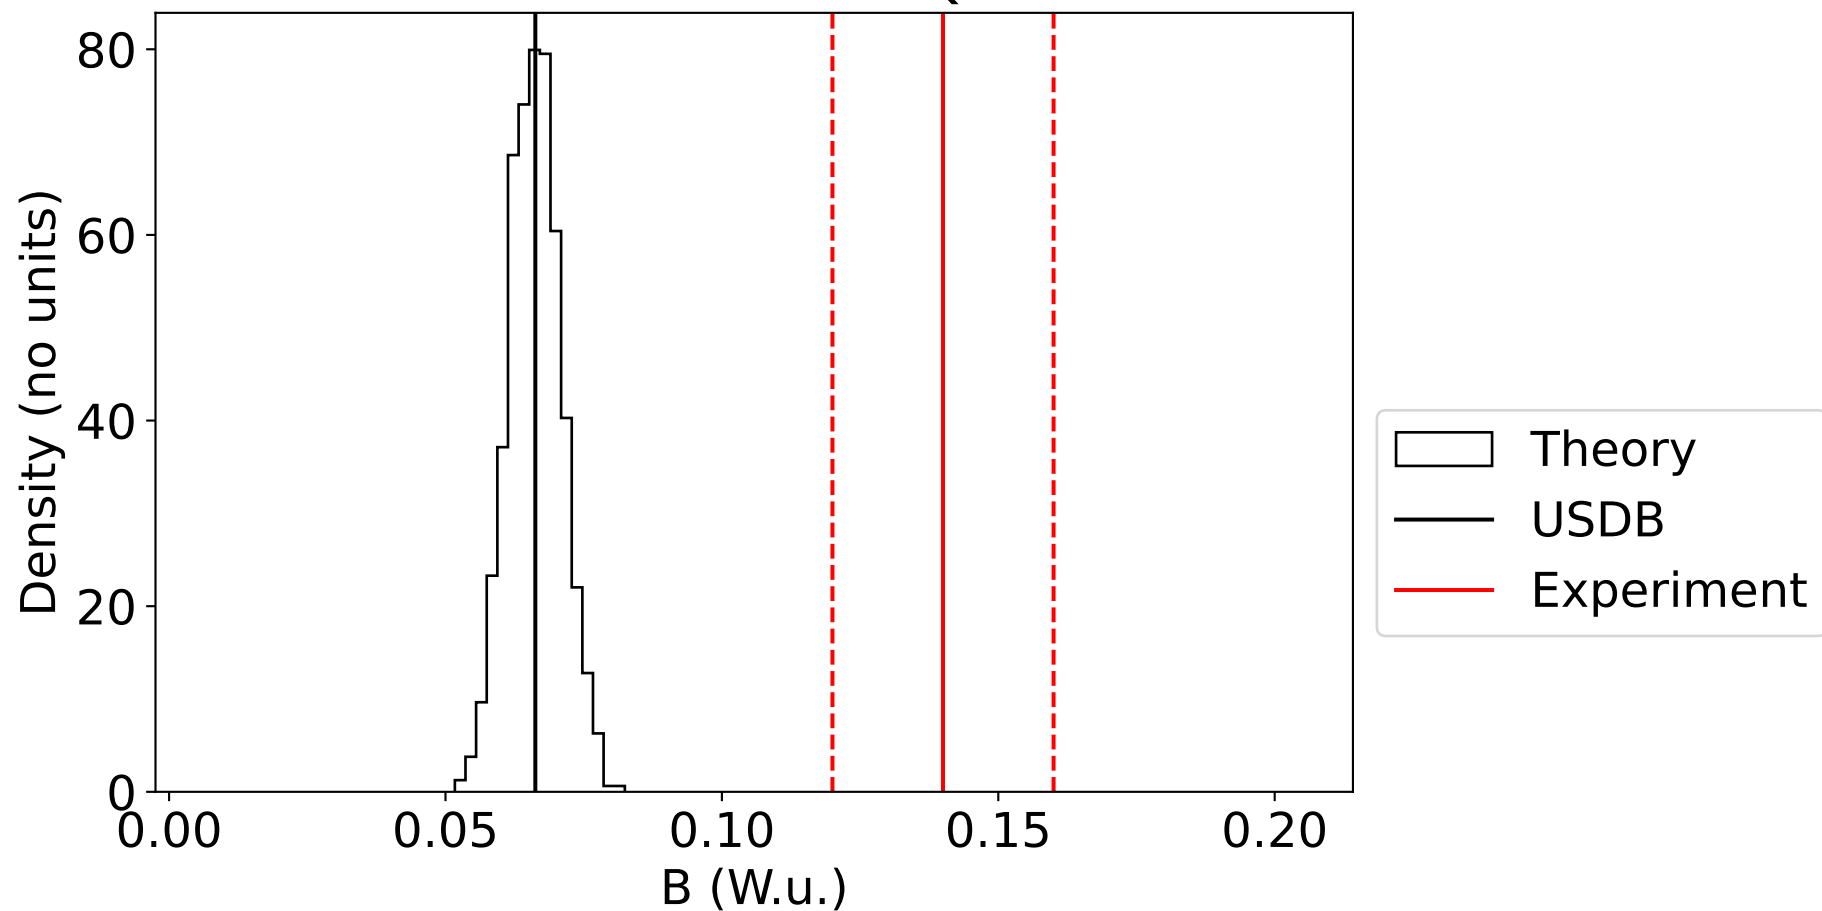

$^{18}\text{O} (2_3) \rightarrow (2_2)$   
Included in UQ

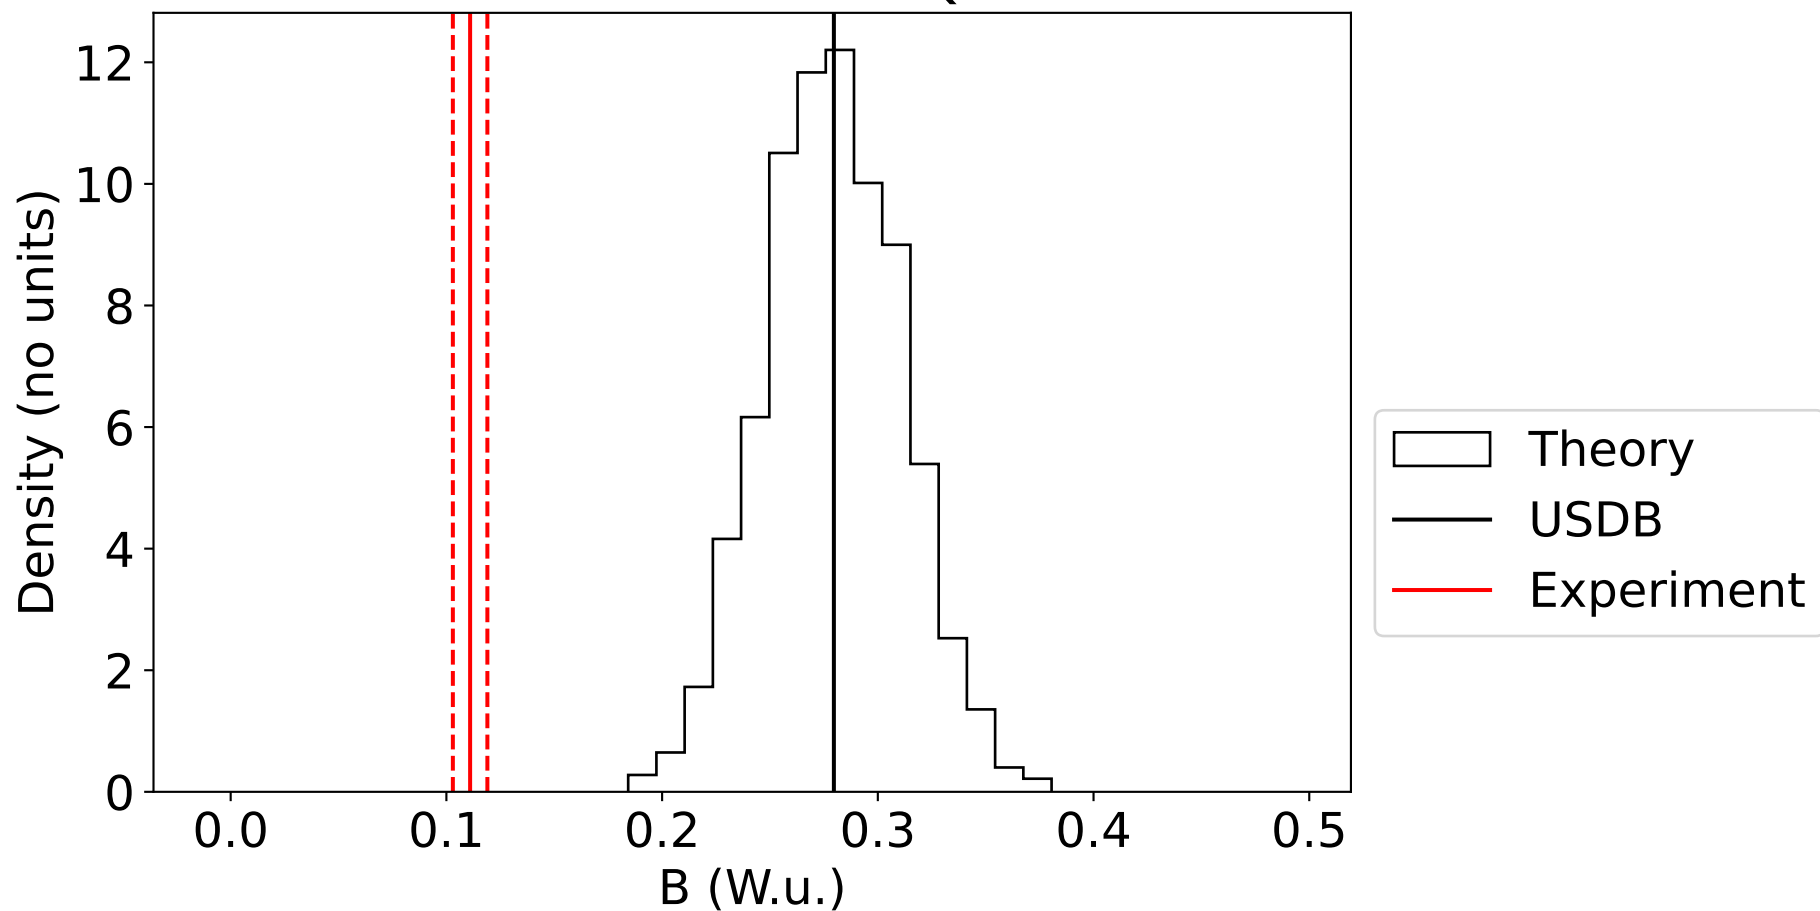

$^{18}\text{O} (4_2) \rightarrow (4_1)$   
Included in UQ

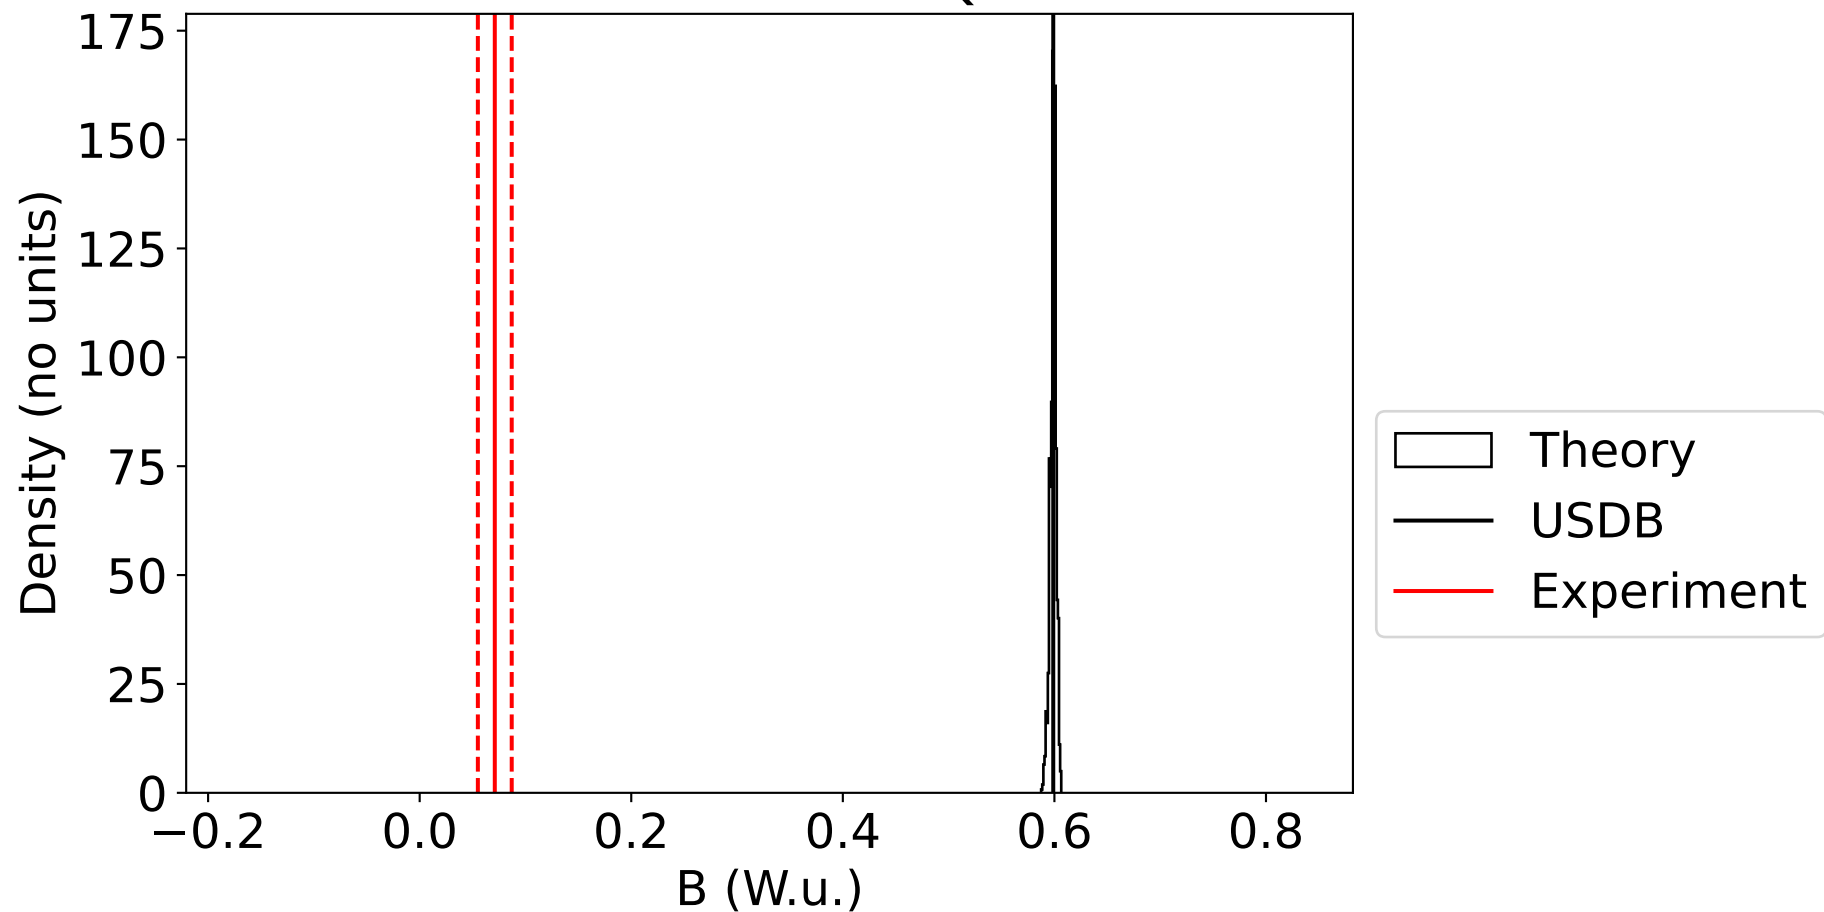

$^{19}\text{O} (3/2_1) \rightarrow (5/2_1)$   
Included in UQ

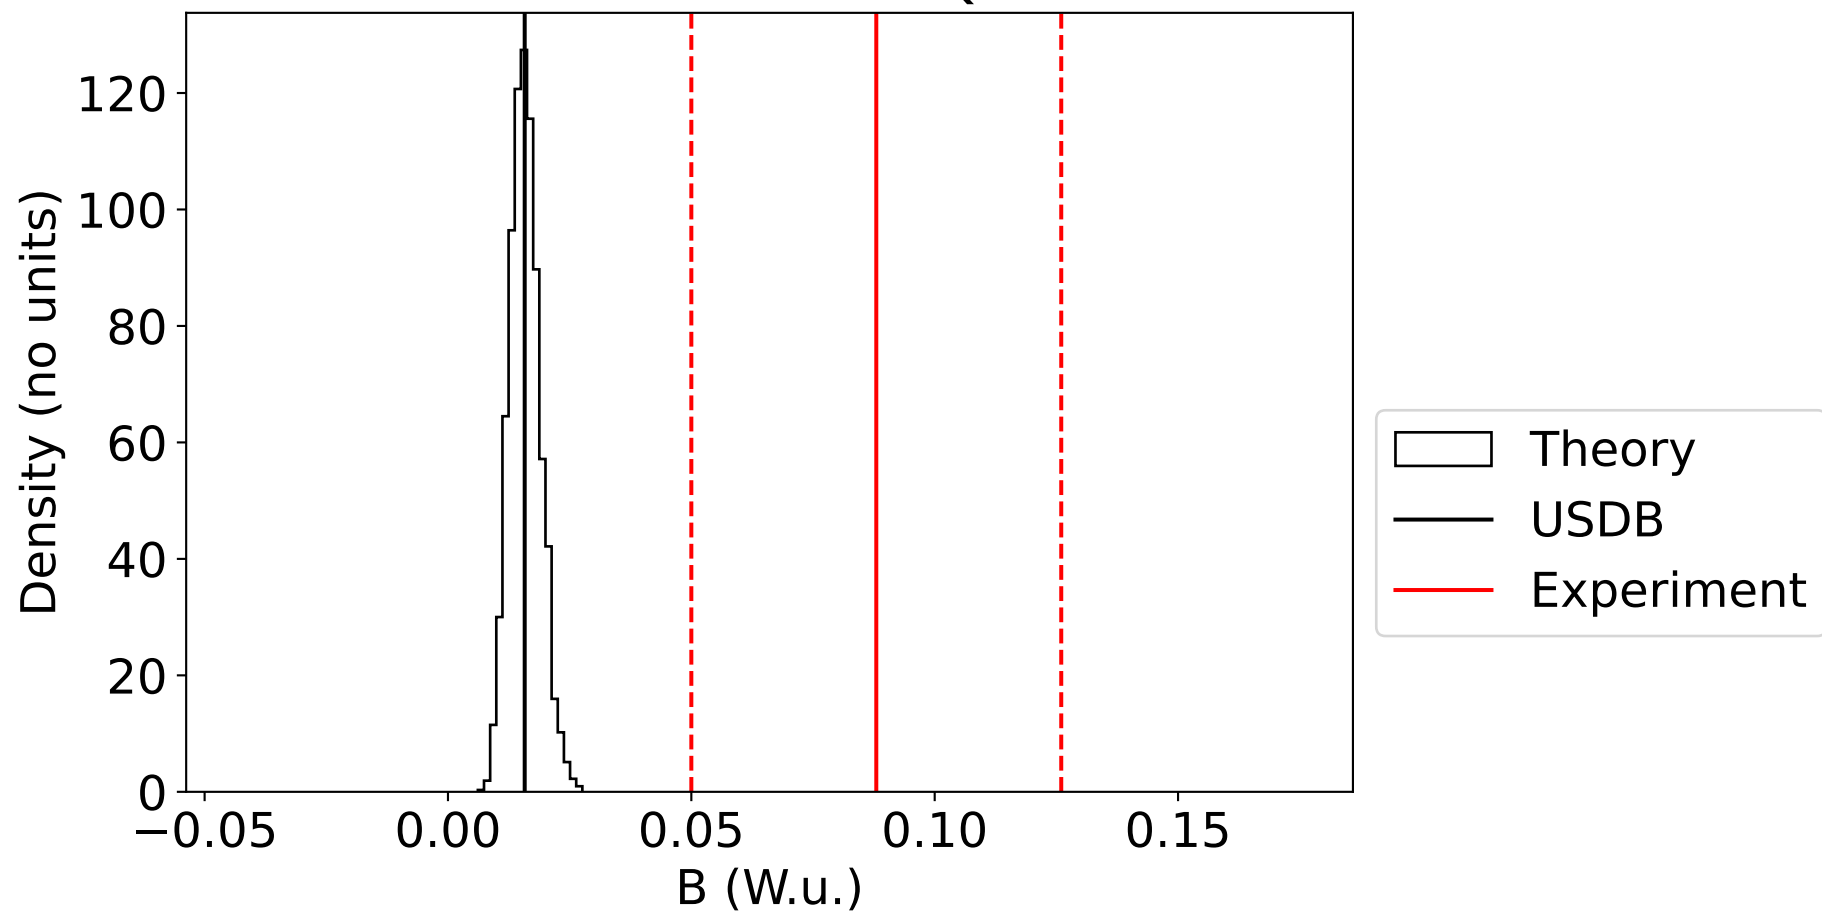

$^{18}\text{F} (0_1) \rightarrow (1_1)$   
Included in UQ

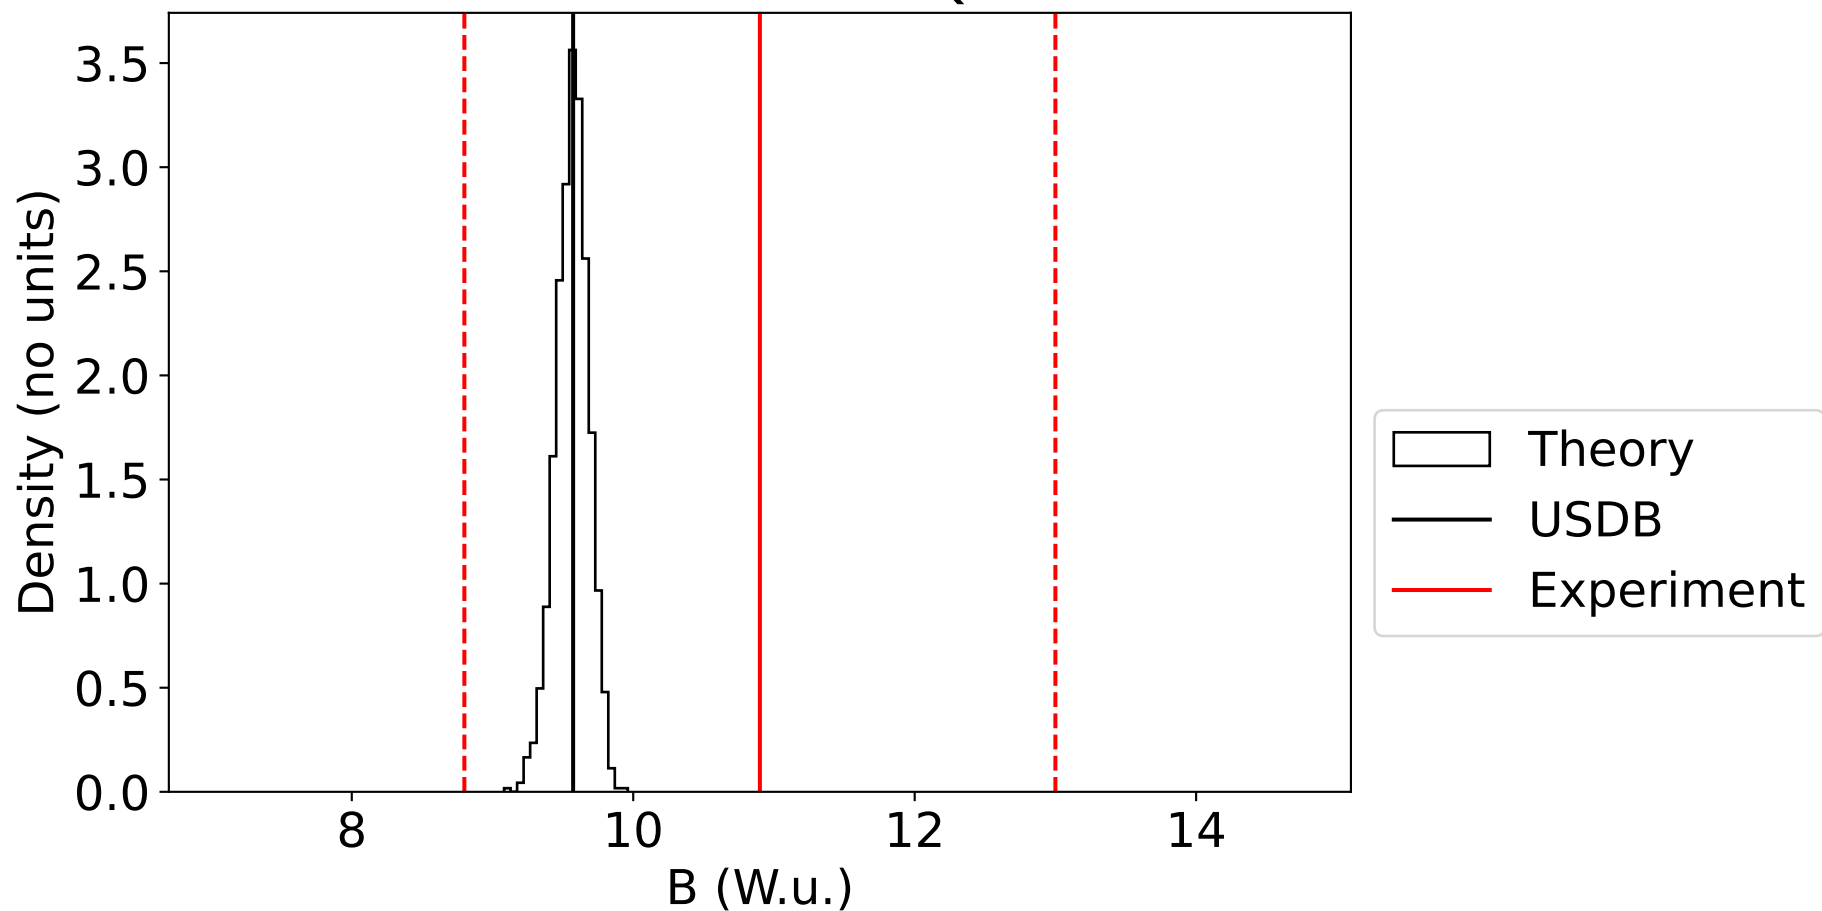

$^{18}\text{F} (1_2) \rightarrow (0_1)$   
Included in UQ

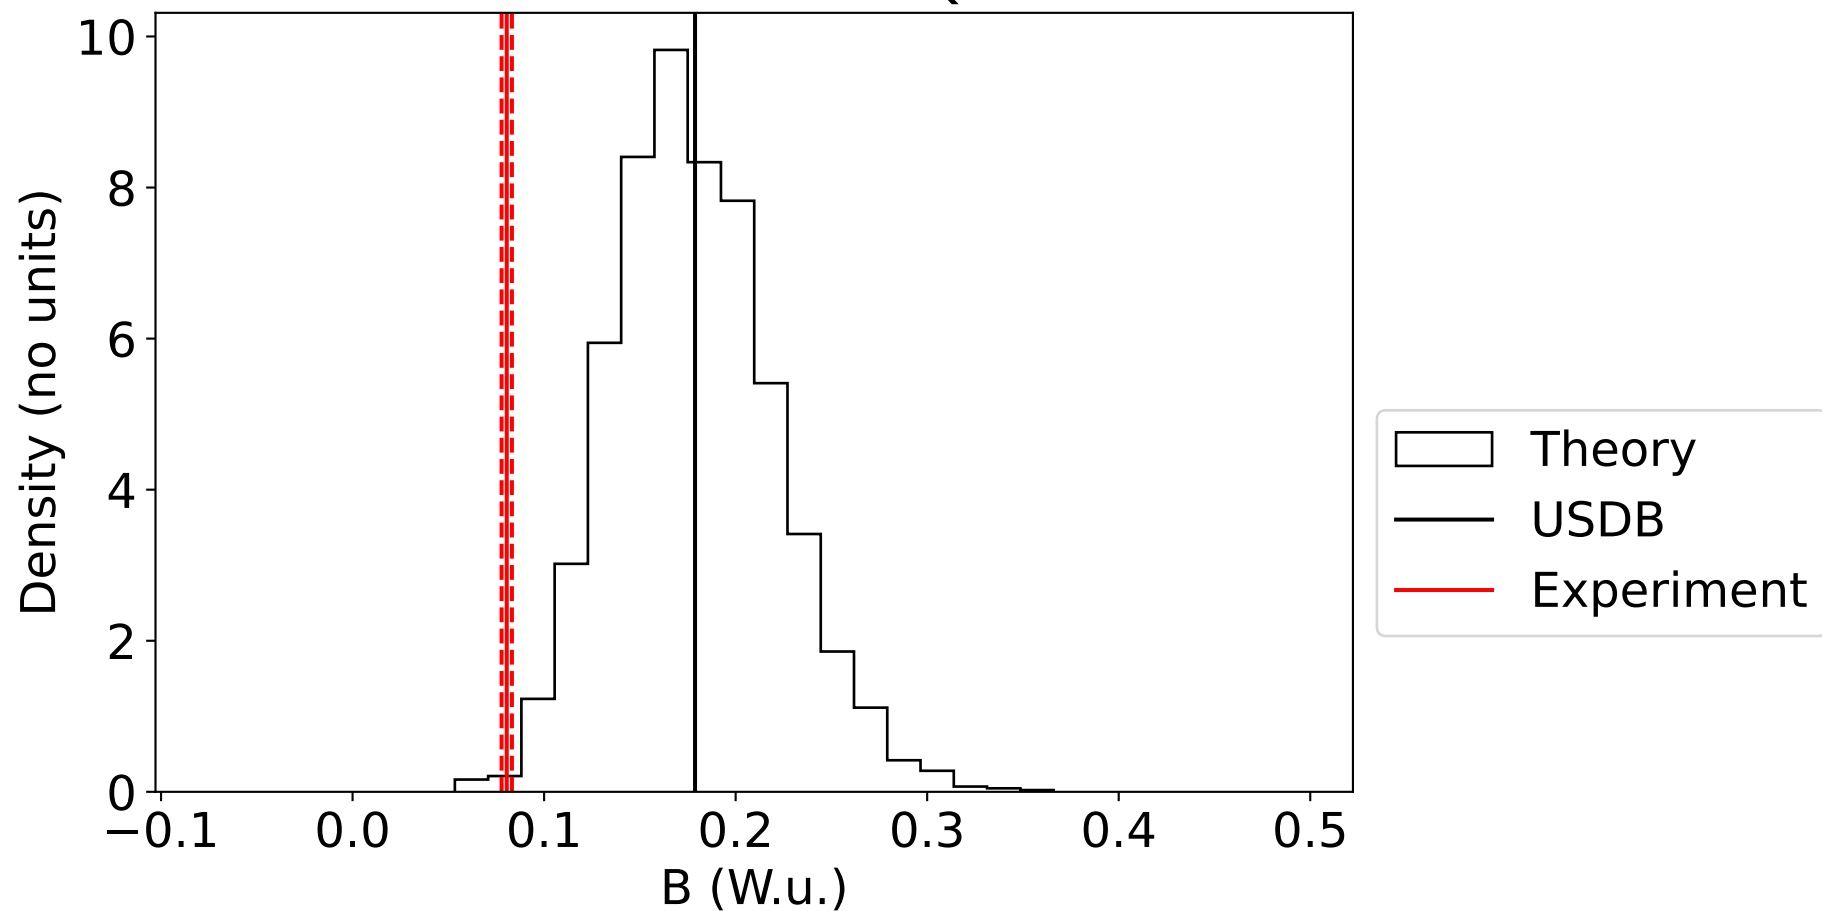

$^{18}\text{F} (2_3) \rightarrow (2_2)$   
Included in UQ

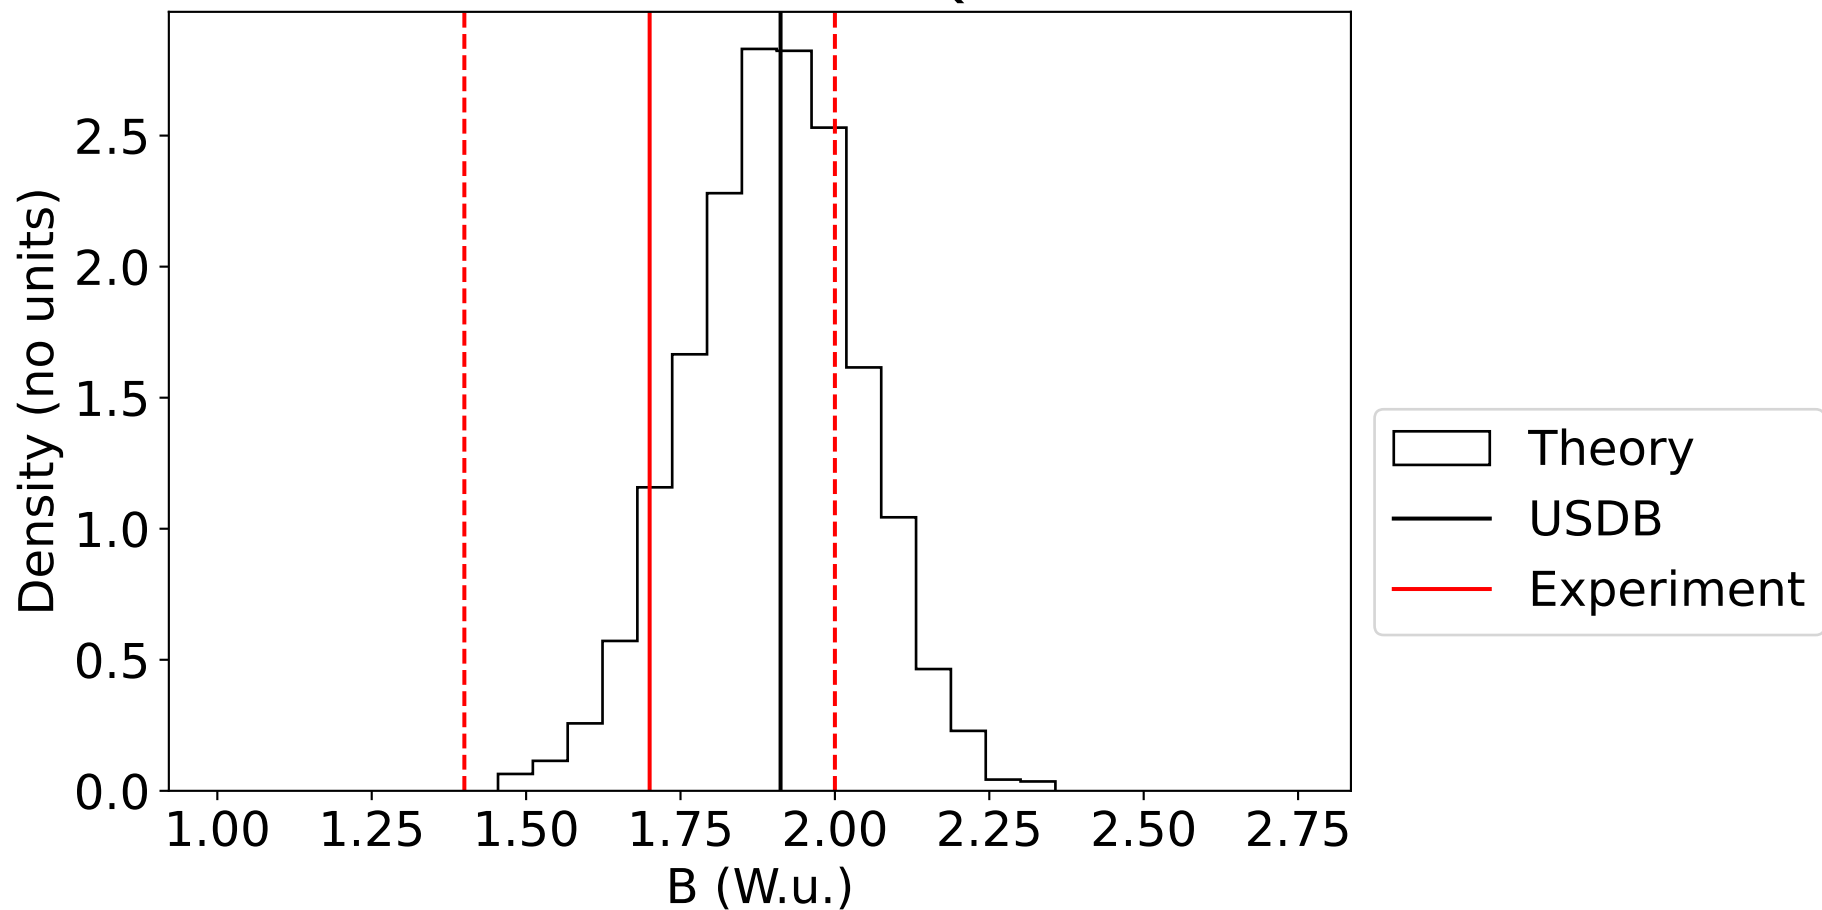

$^{18}\text{F} (3_3) \rightarrow (2_2)$   
Included in UQ

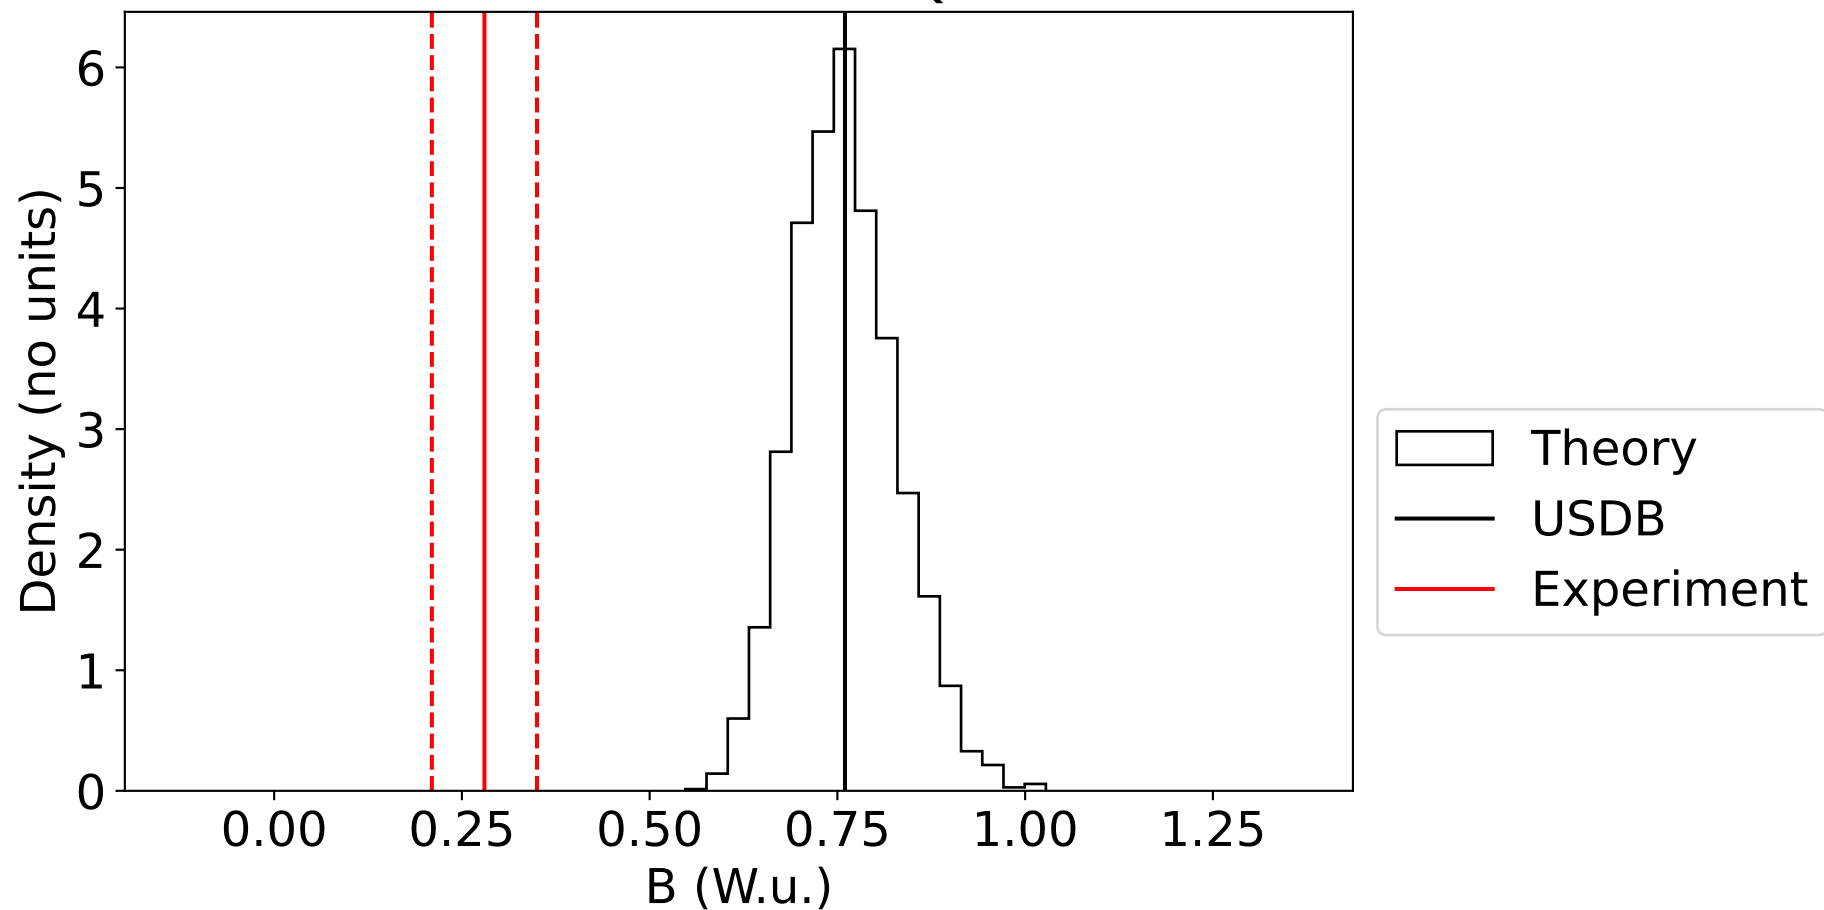



$^{18}\text{F} (1_4) \rightarrow (2_2)$   
Included in UQ

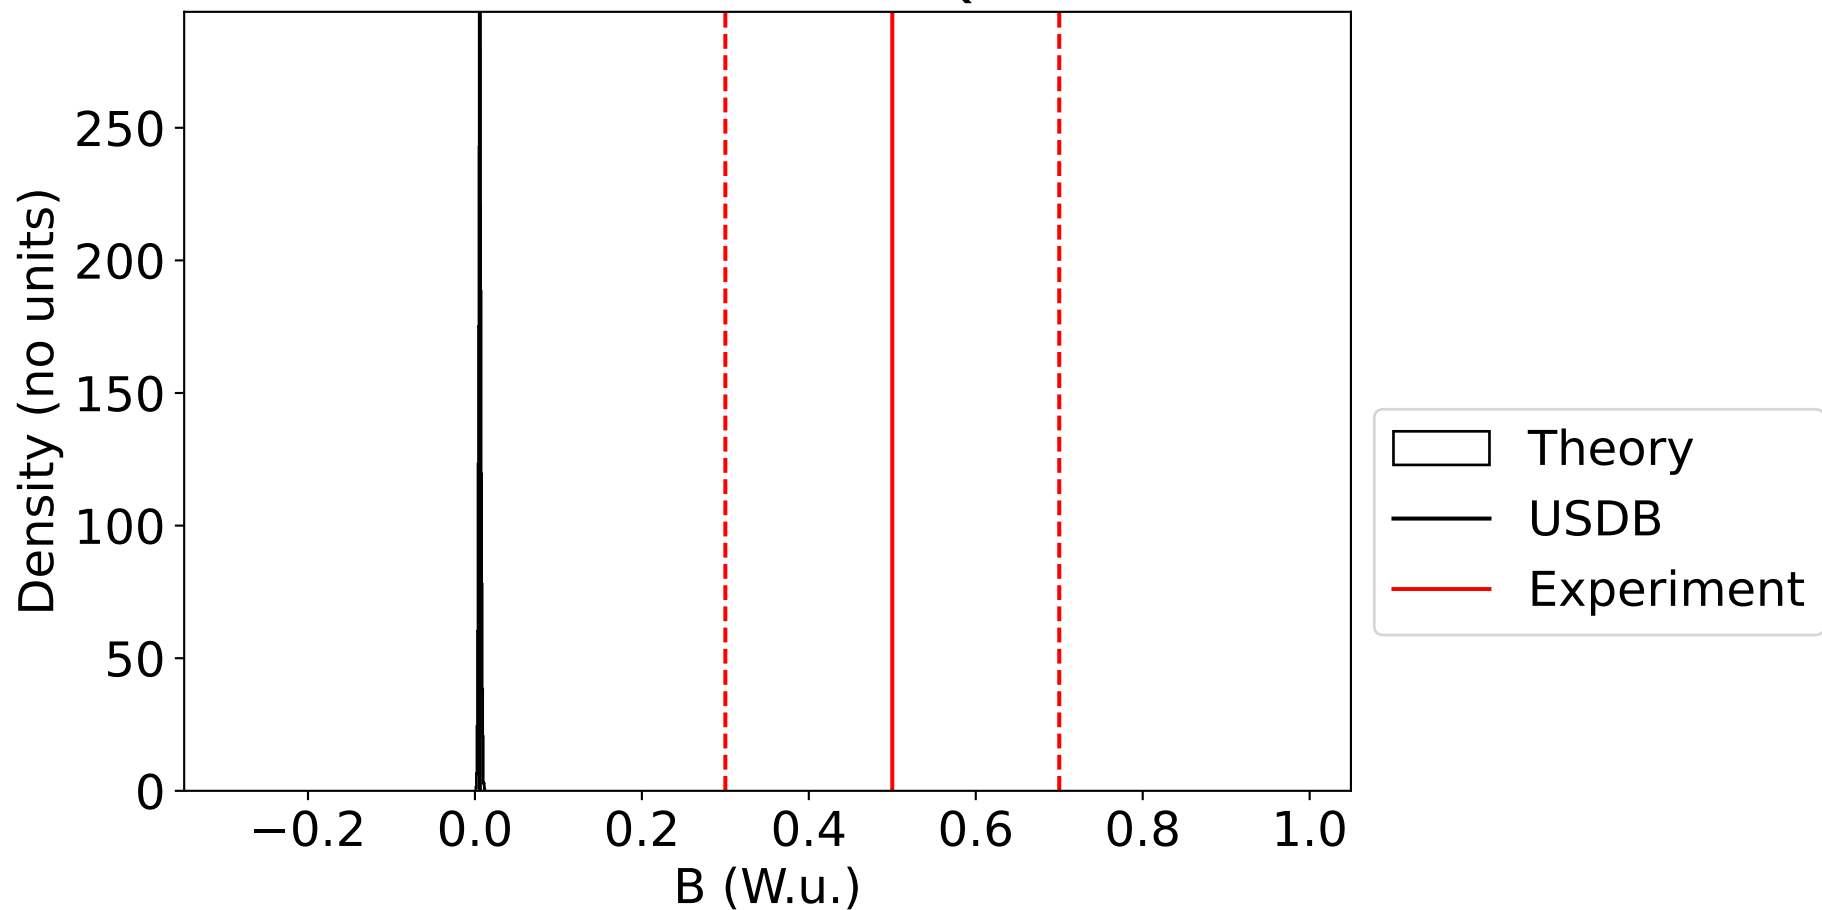

$^{18}\text{F} (4_2) \rightarrow (4_1)$   
Included in UQ

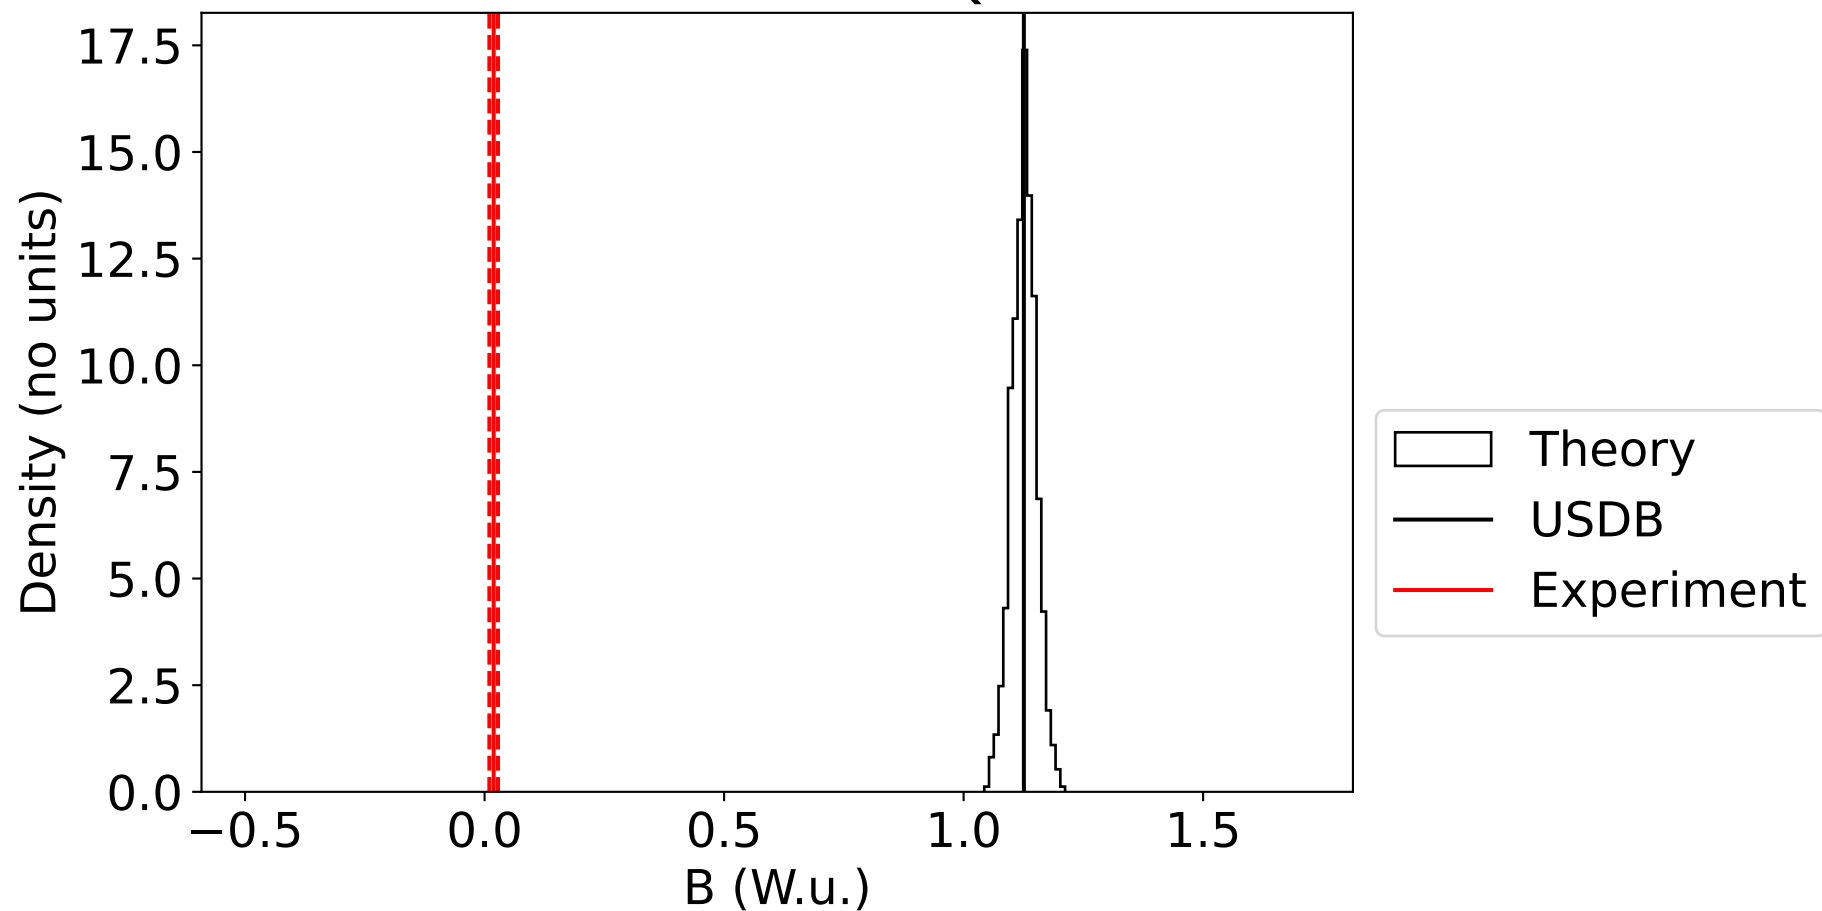

$^{18}\text{F} (1_5) \rightarrow (2_2)$   
Included in UQ

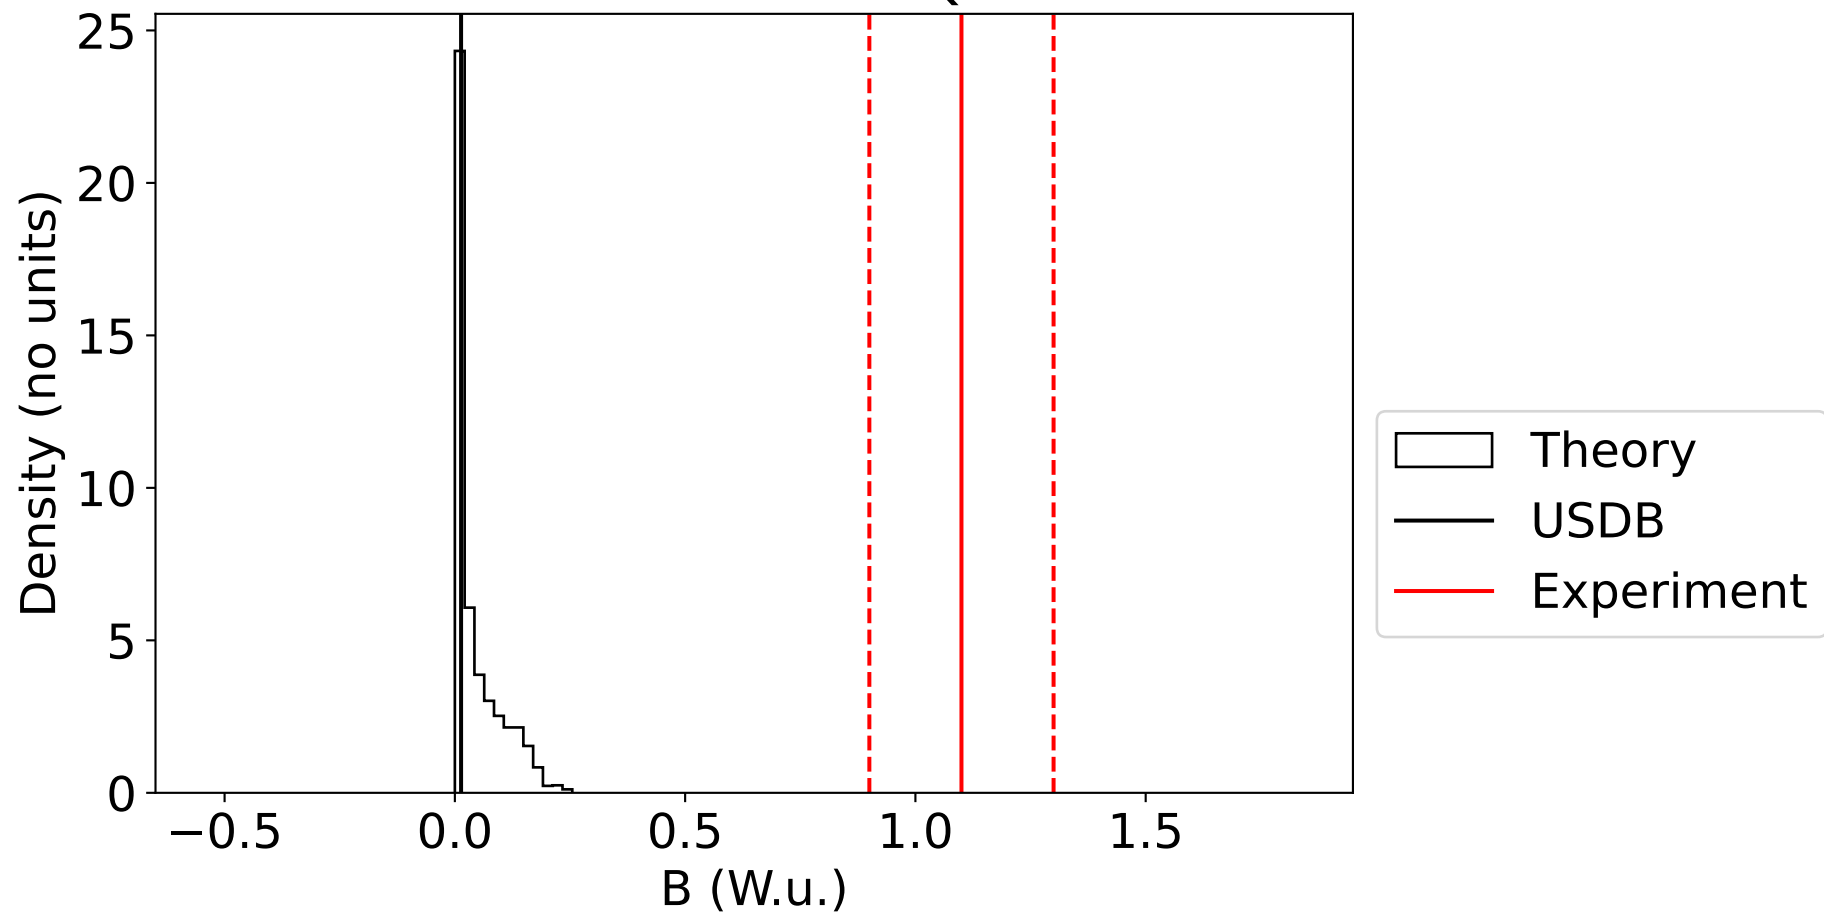

$^{18}\text{F} (3_4) \rightarrow (2_1)$   
Included in UQ

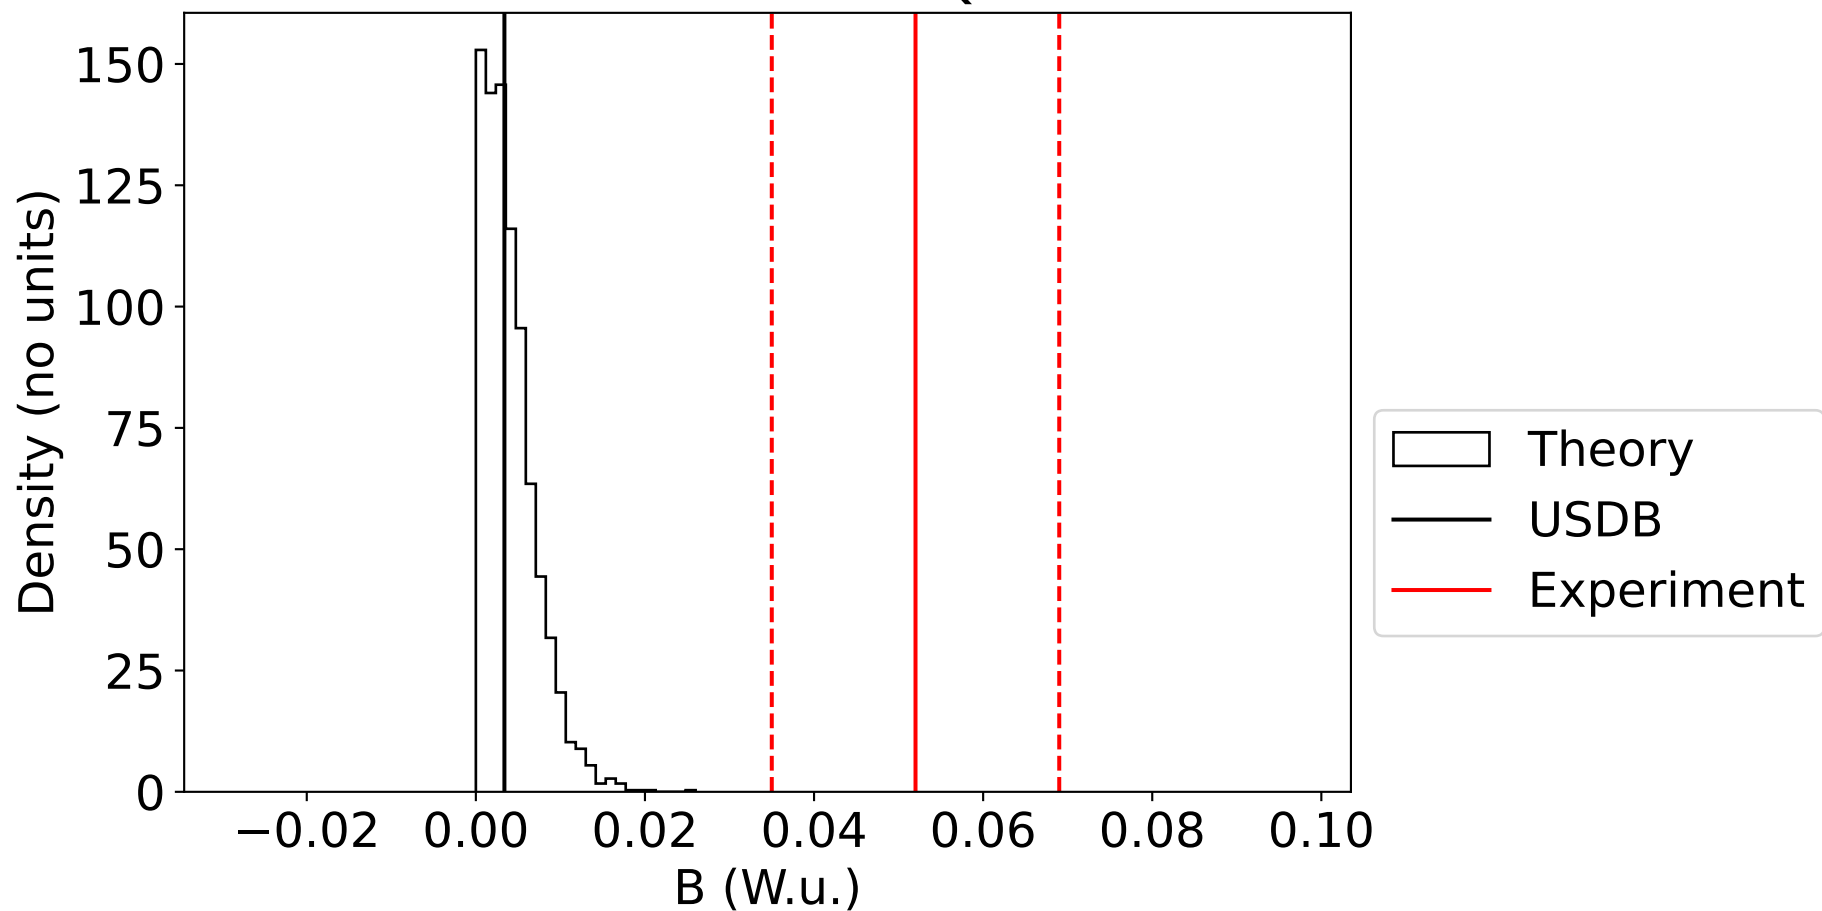

$^{18}\text{F} (3_4) \rightarrow (2_2)$   
Included in UQ

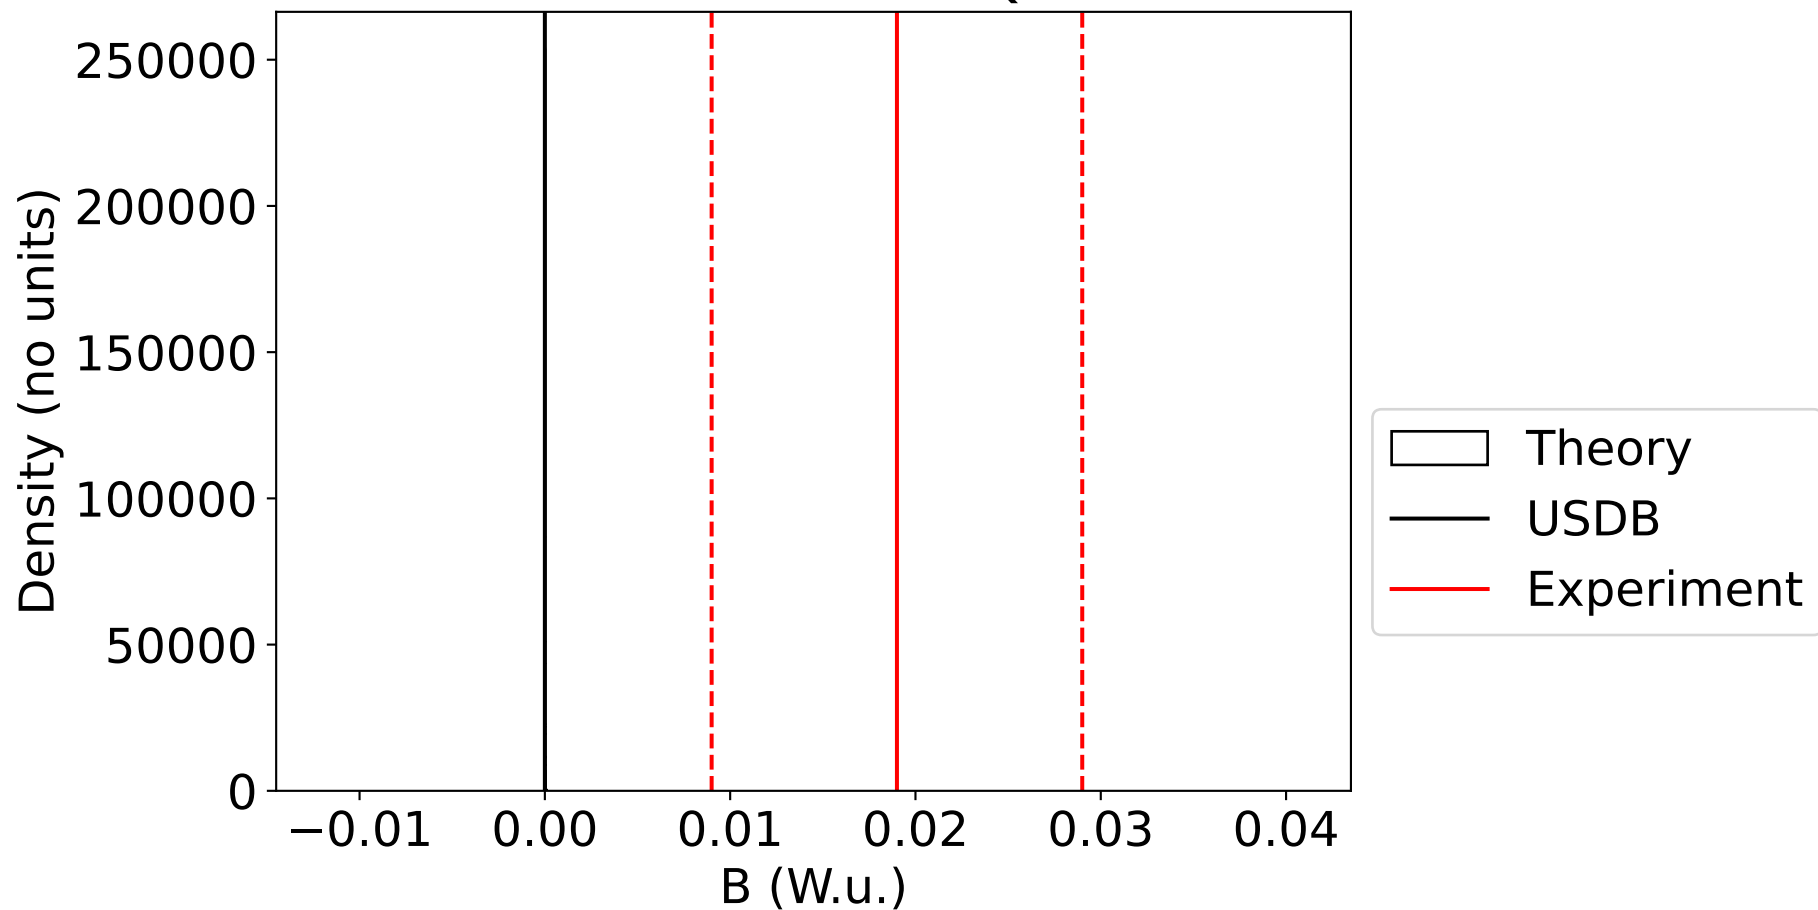

$^{18}\text{F} (3_4) \rightarrow (2_3)$   
Included in UQ

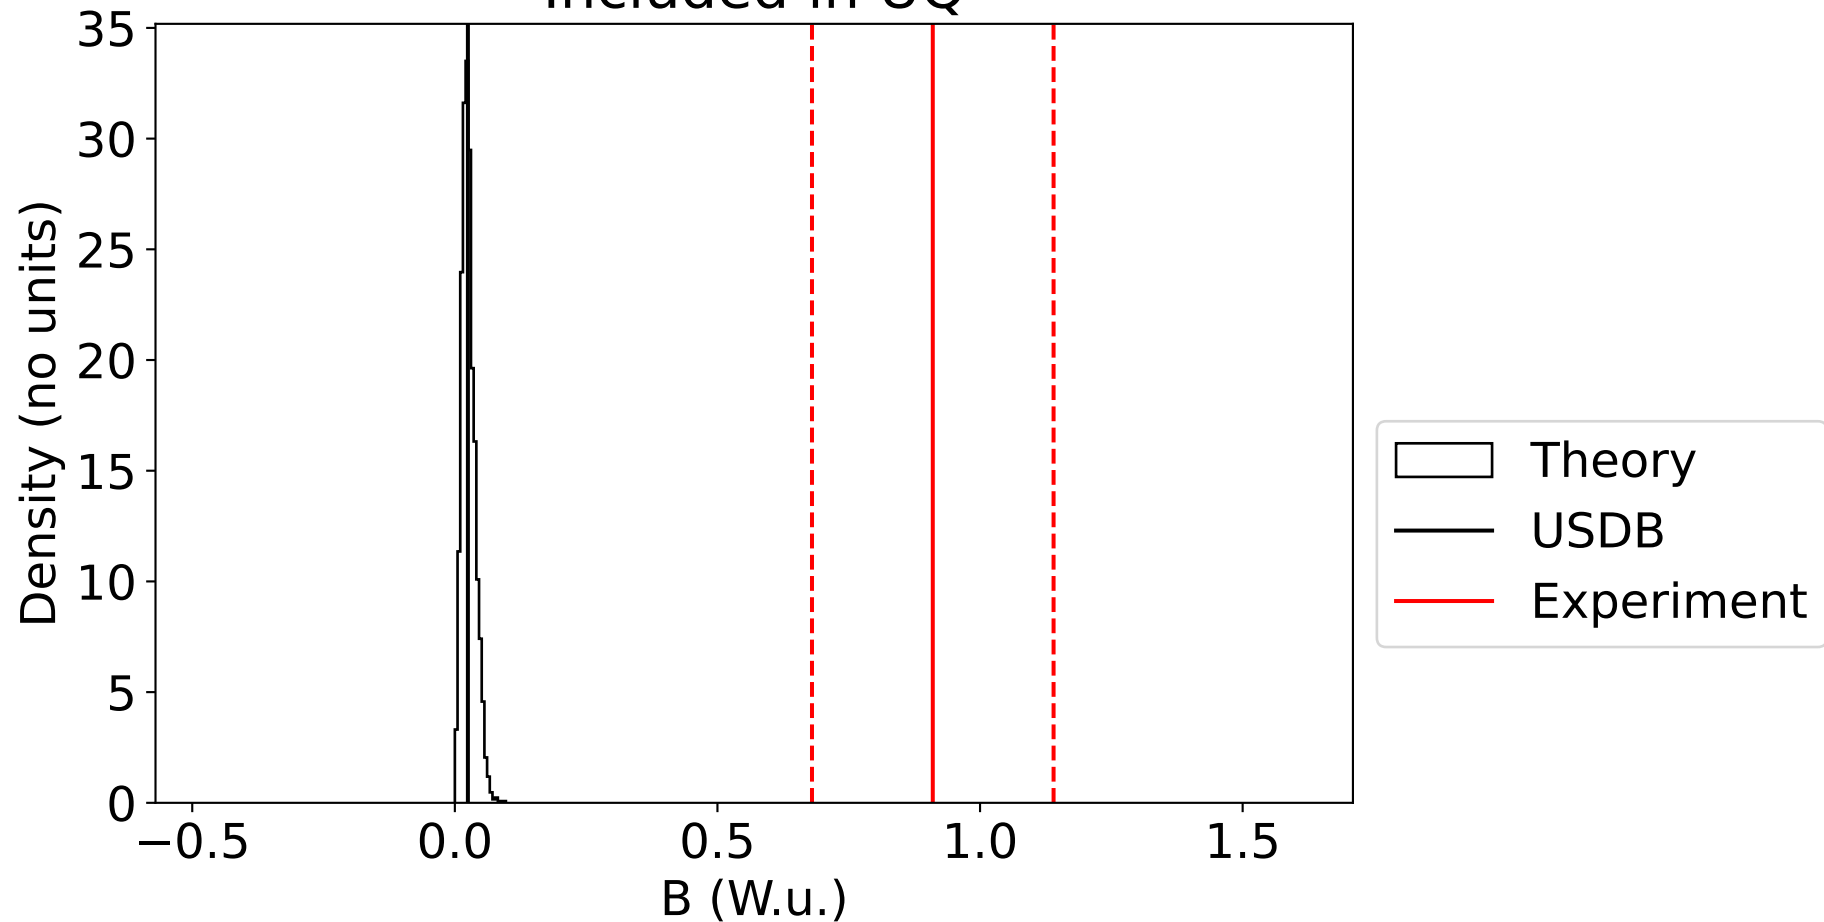

$^{18}\text{F} (3_4) \rightarrow (3_3)$   
Included in UQ

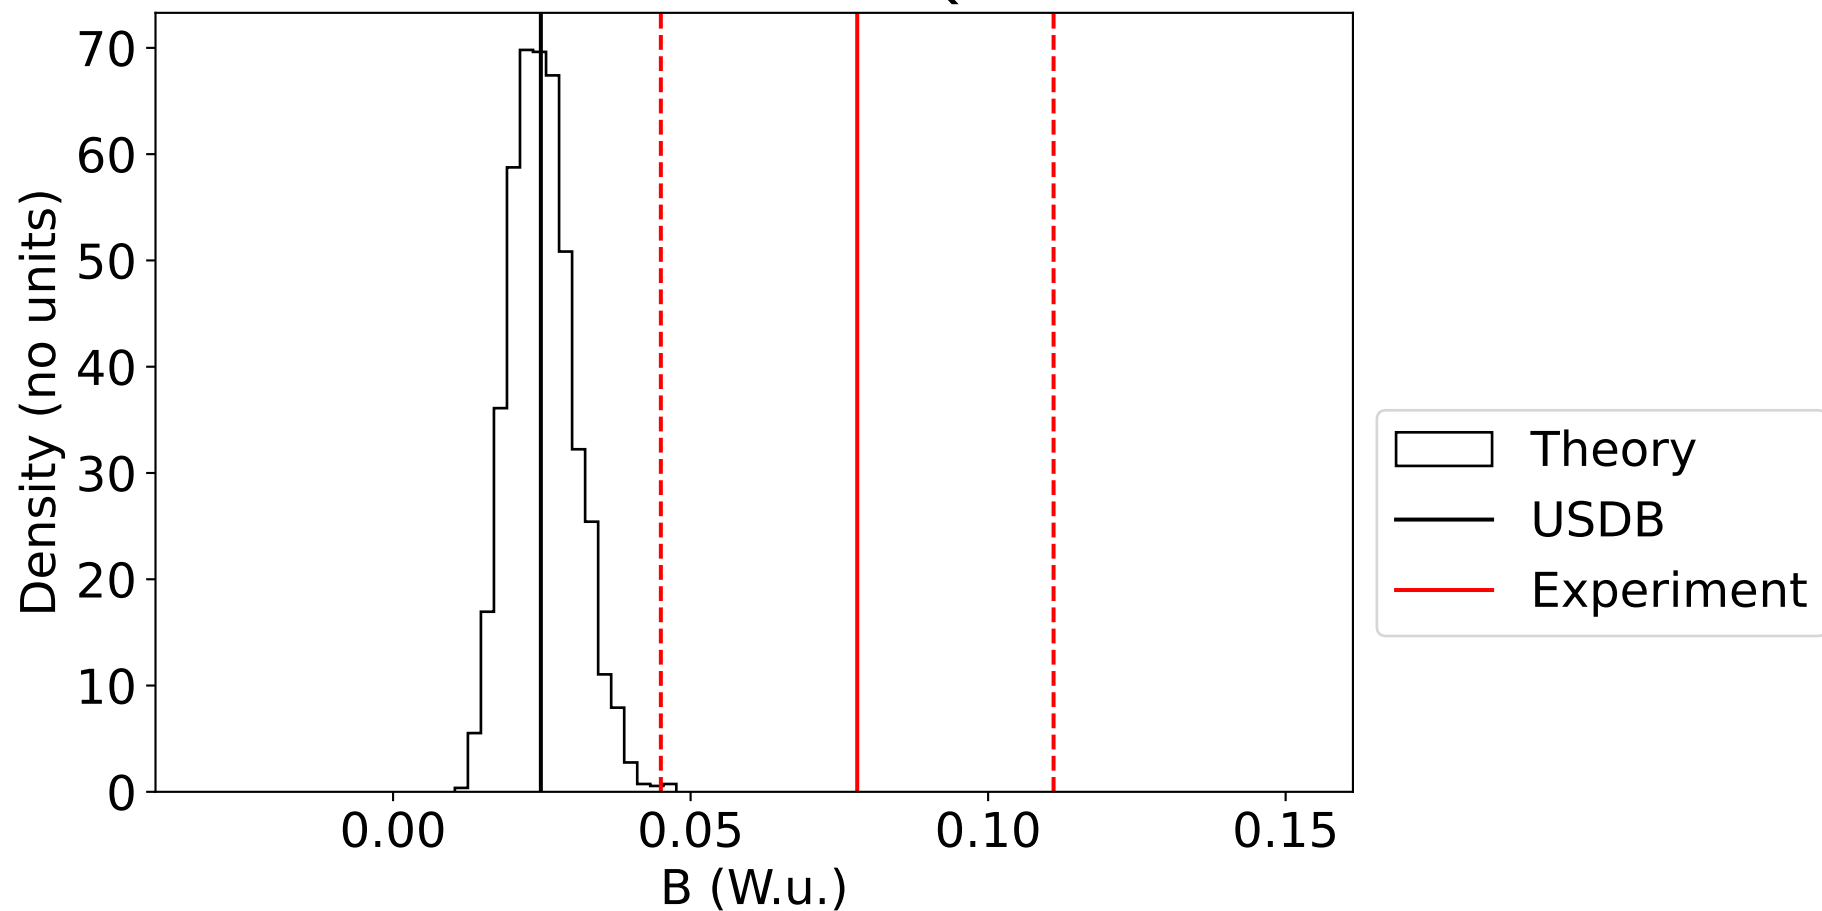

$^{18}\text{F} (2_5) \rightarrow (3_2)$   
Included in UQ

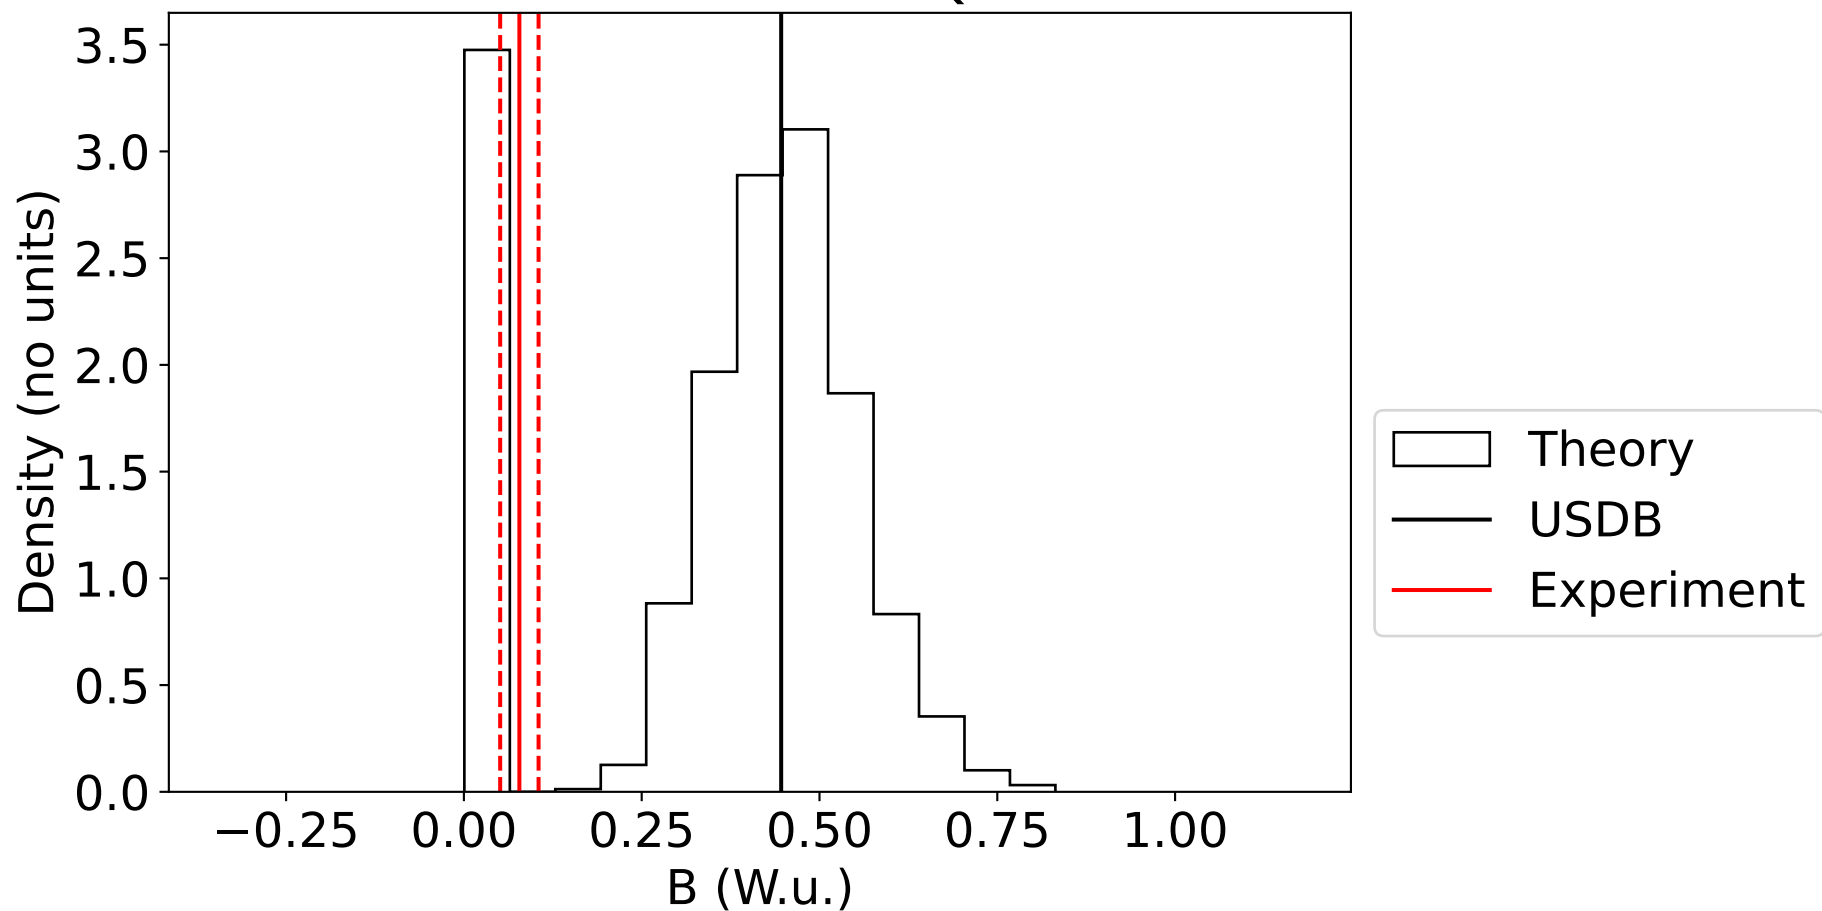



$^{18}\text{F} (2_5) \rightarrow (1_3)$   
Included in UQ

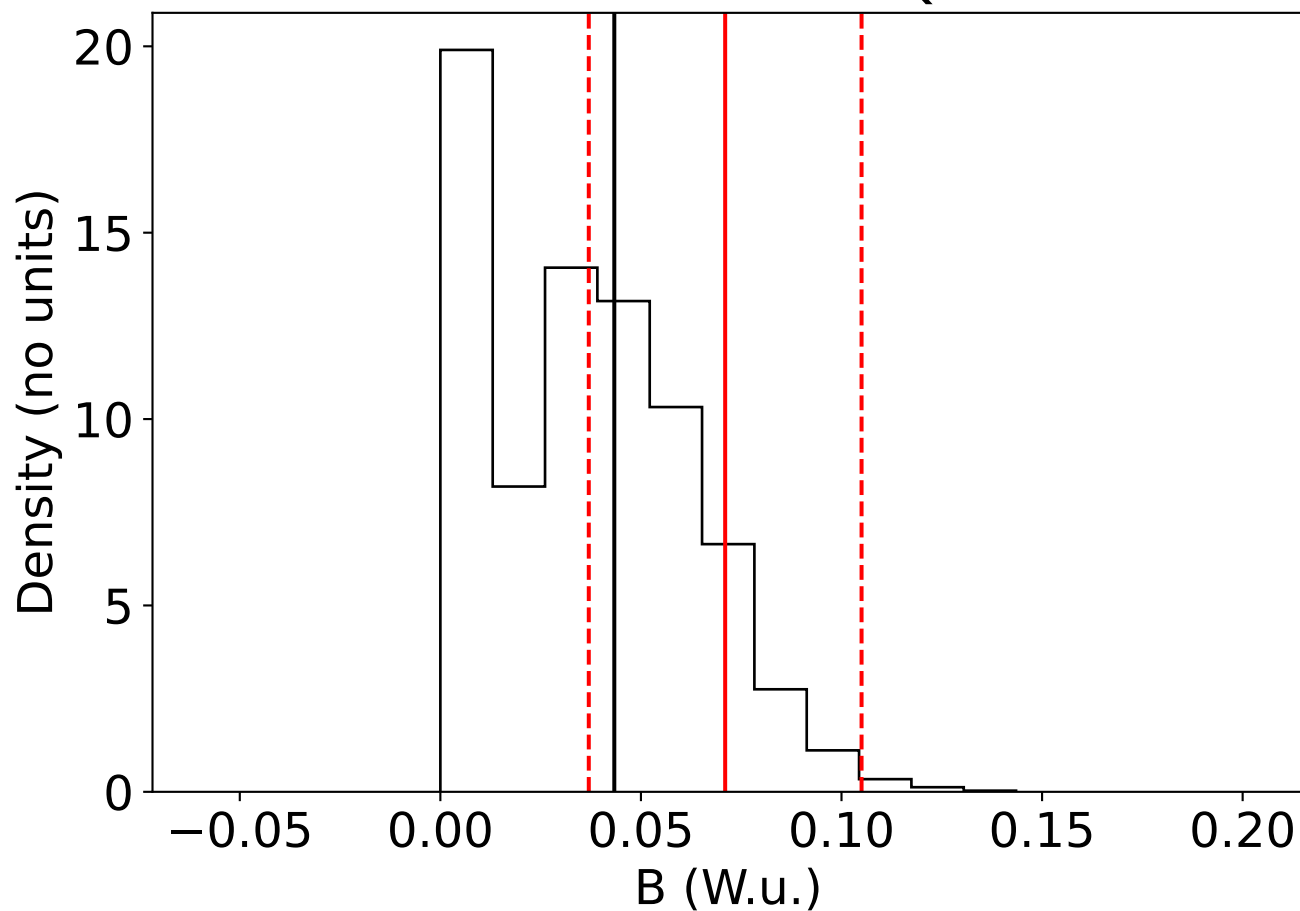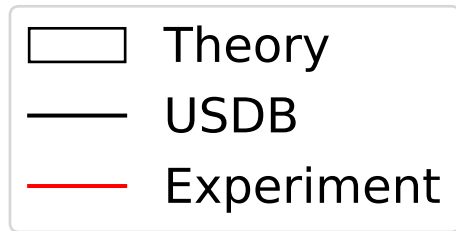

$^{18}\text{F} (2_5) \rightarrow (2_3)$   
Included in UQ

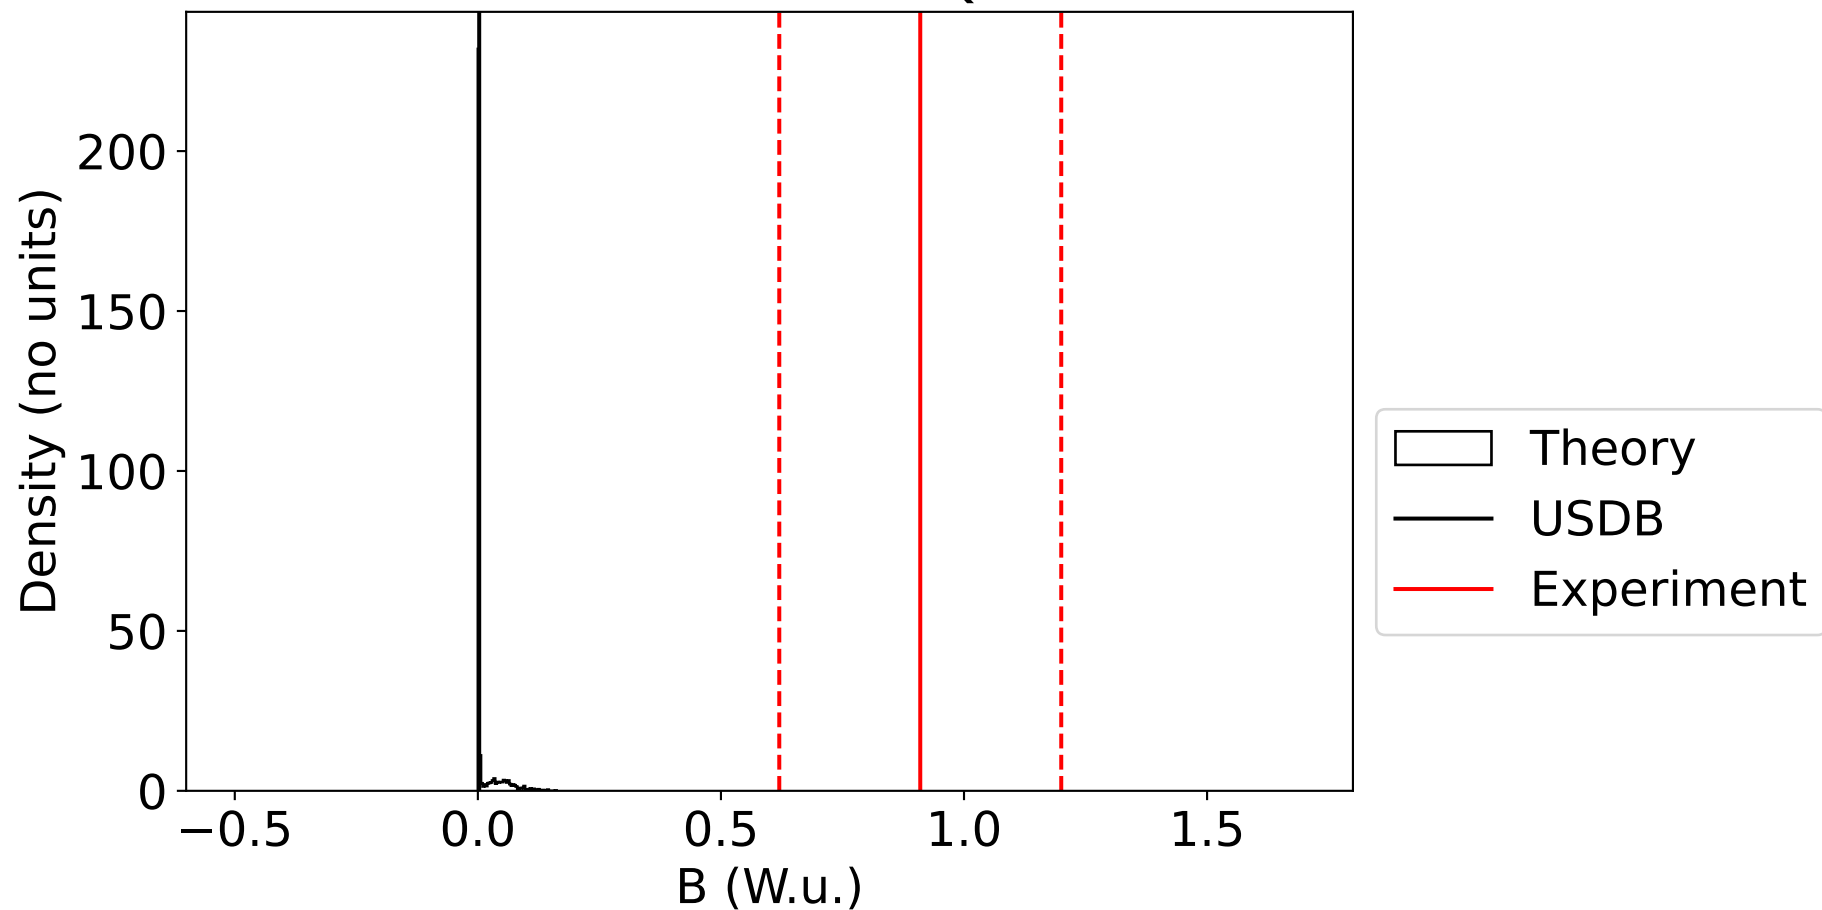

$^{18}\text{F} (2_5) \rightarrow (1_2)$   
Included in UQ

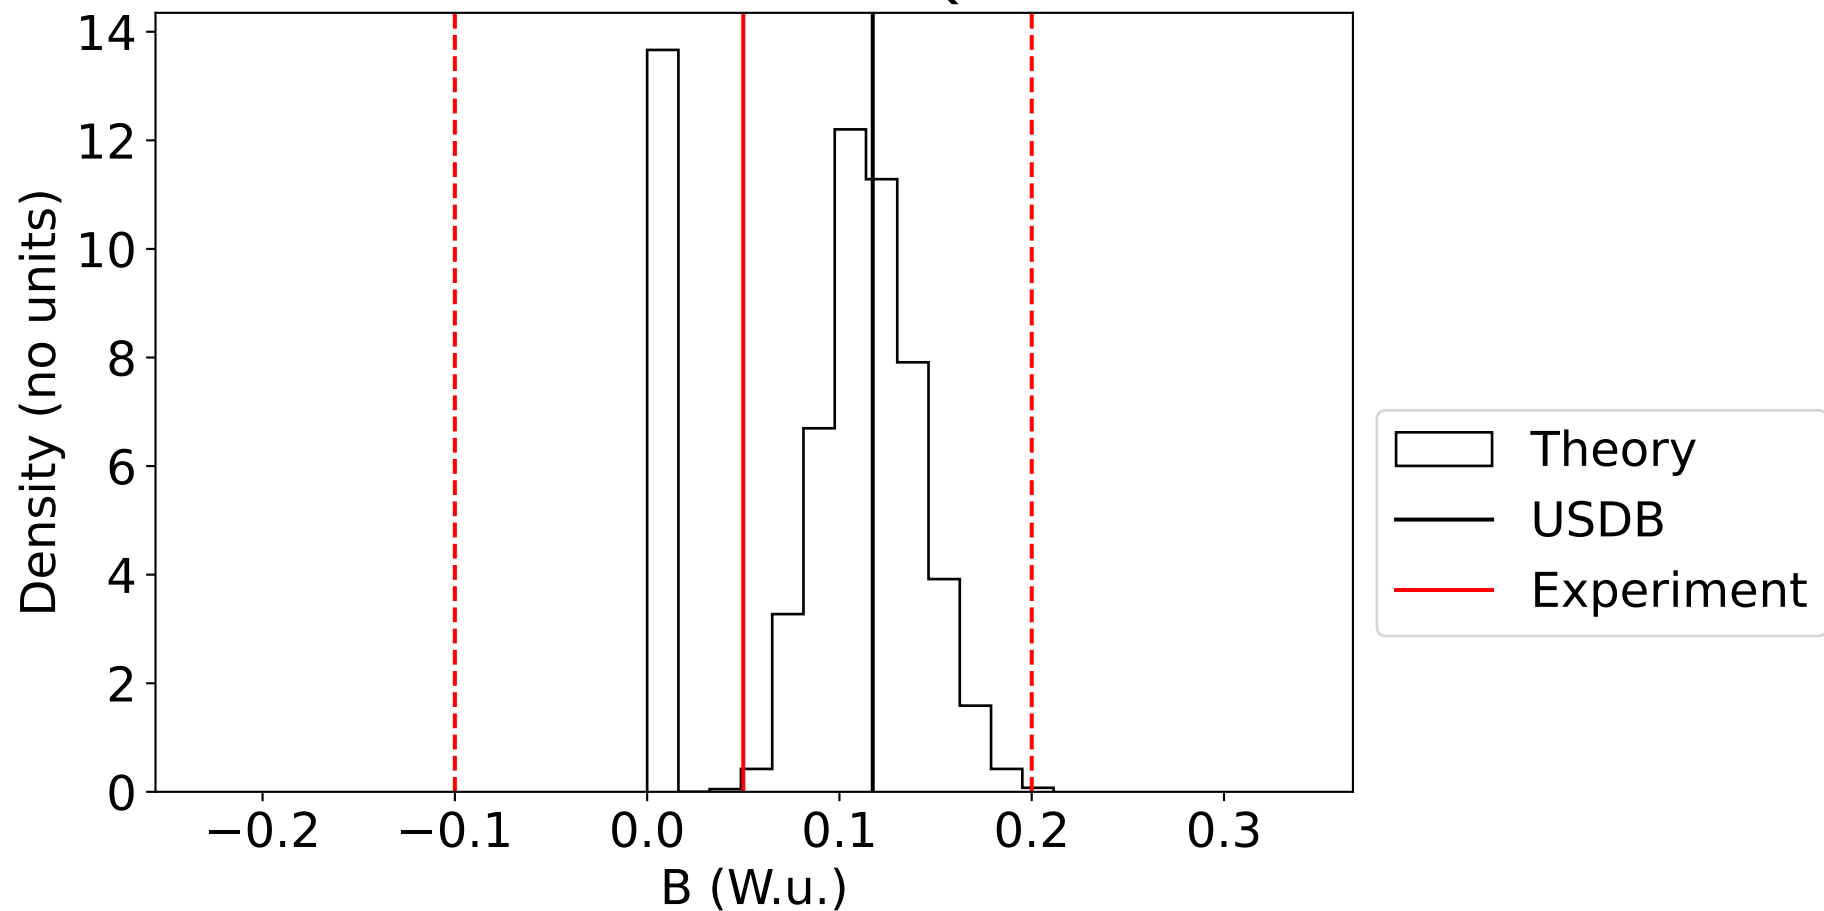

$^{18}\text{F} (2_5) \rightarrow (3_3)$   
Included in UQ

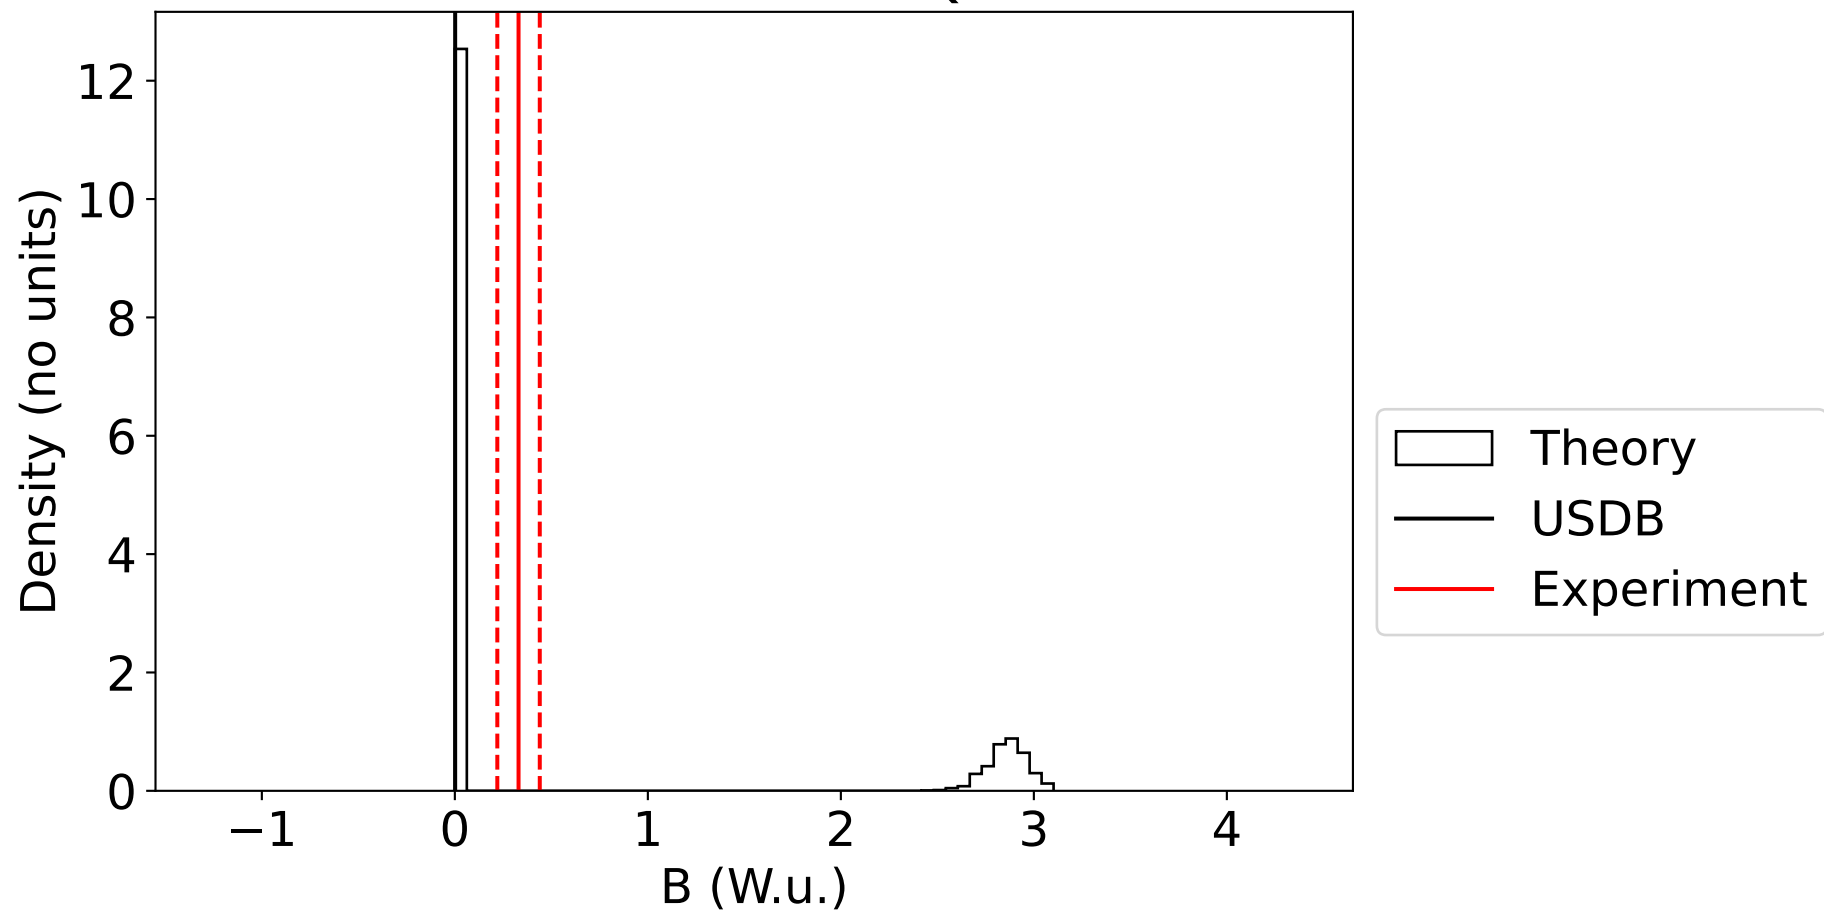

$^{18}\text{F} (2_5) \rightarrow (1_4)$   
Included in UQ

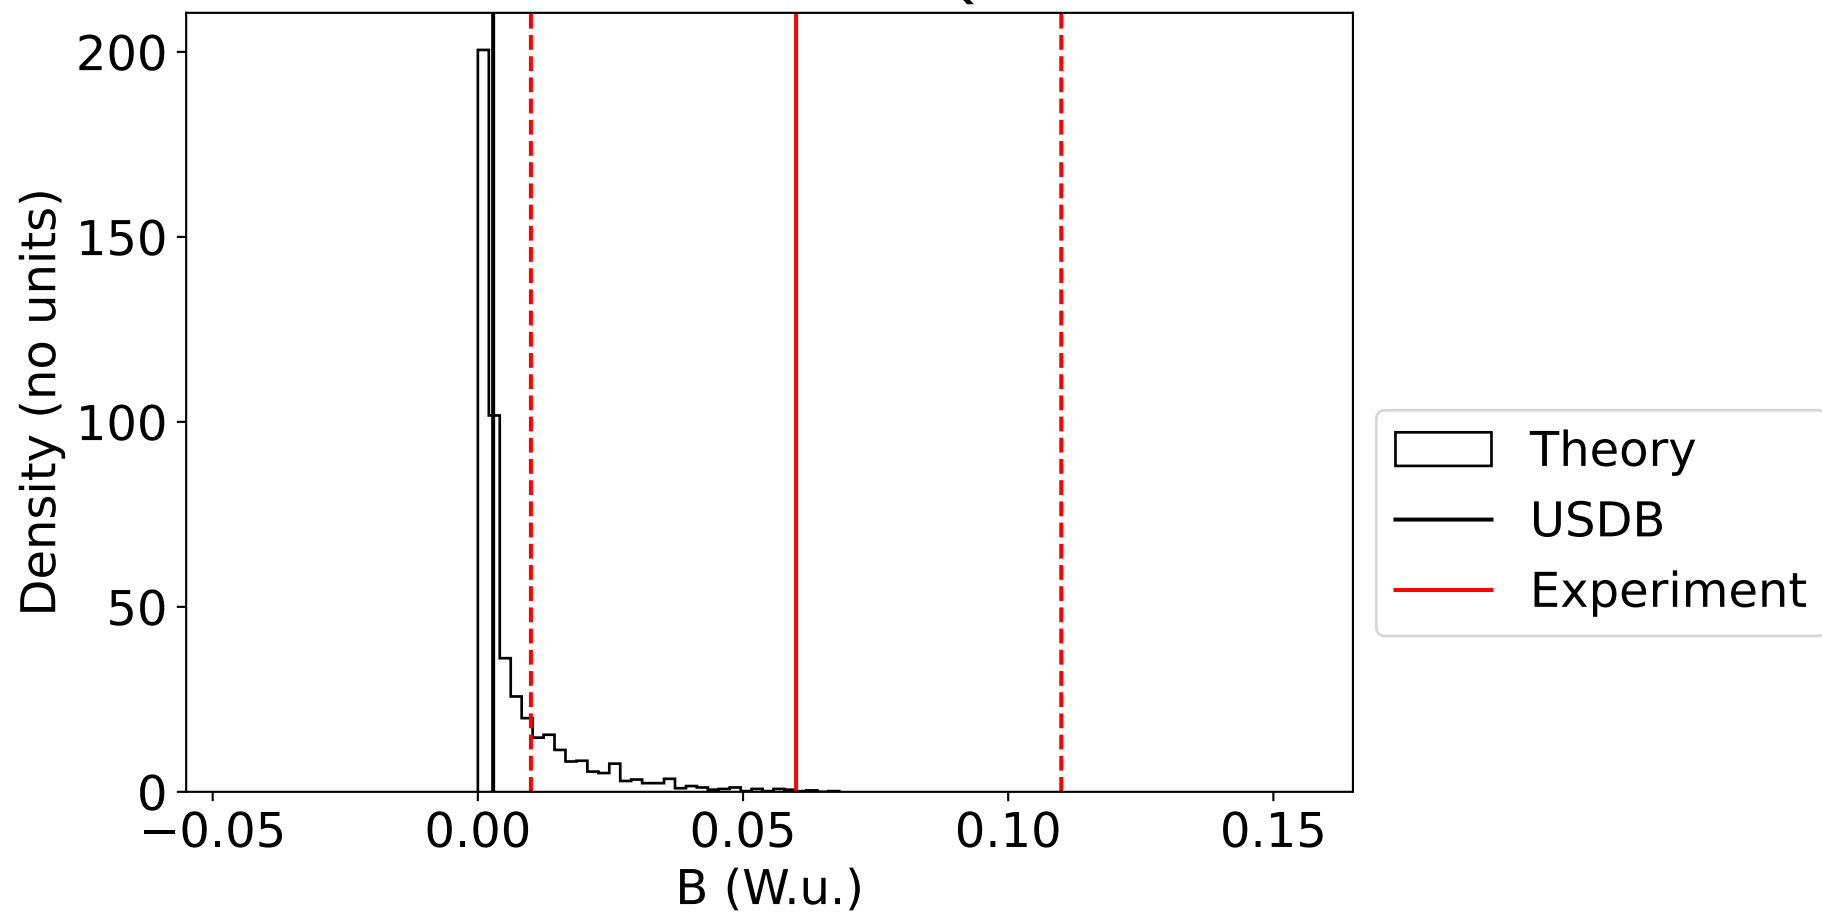

$^{18}\text{F} (3_5) \rightarrow (3_3)$   
Included in UQ

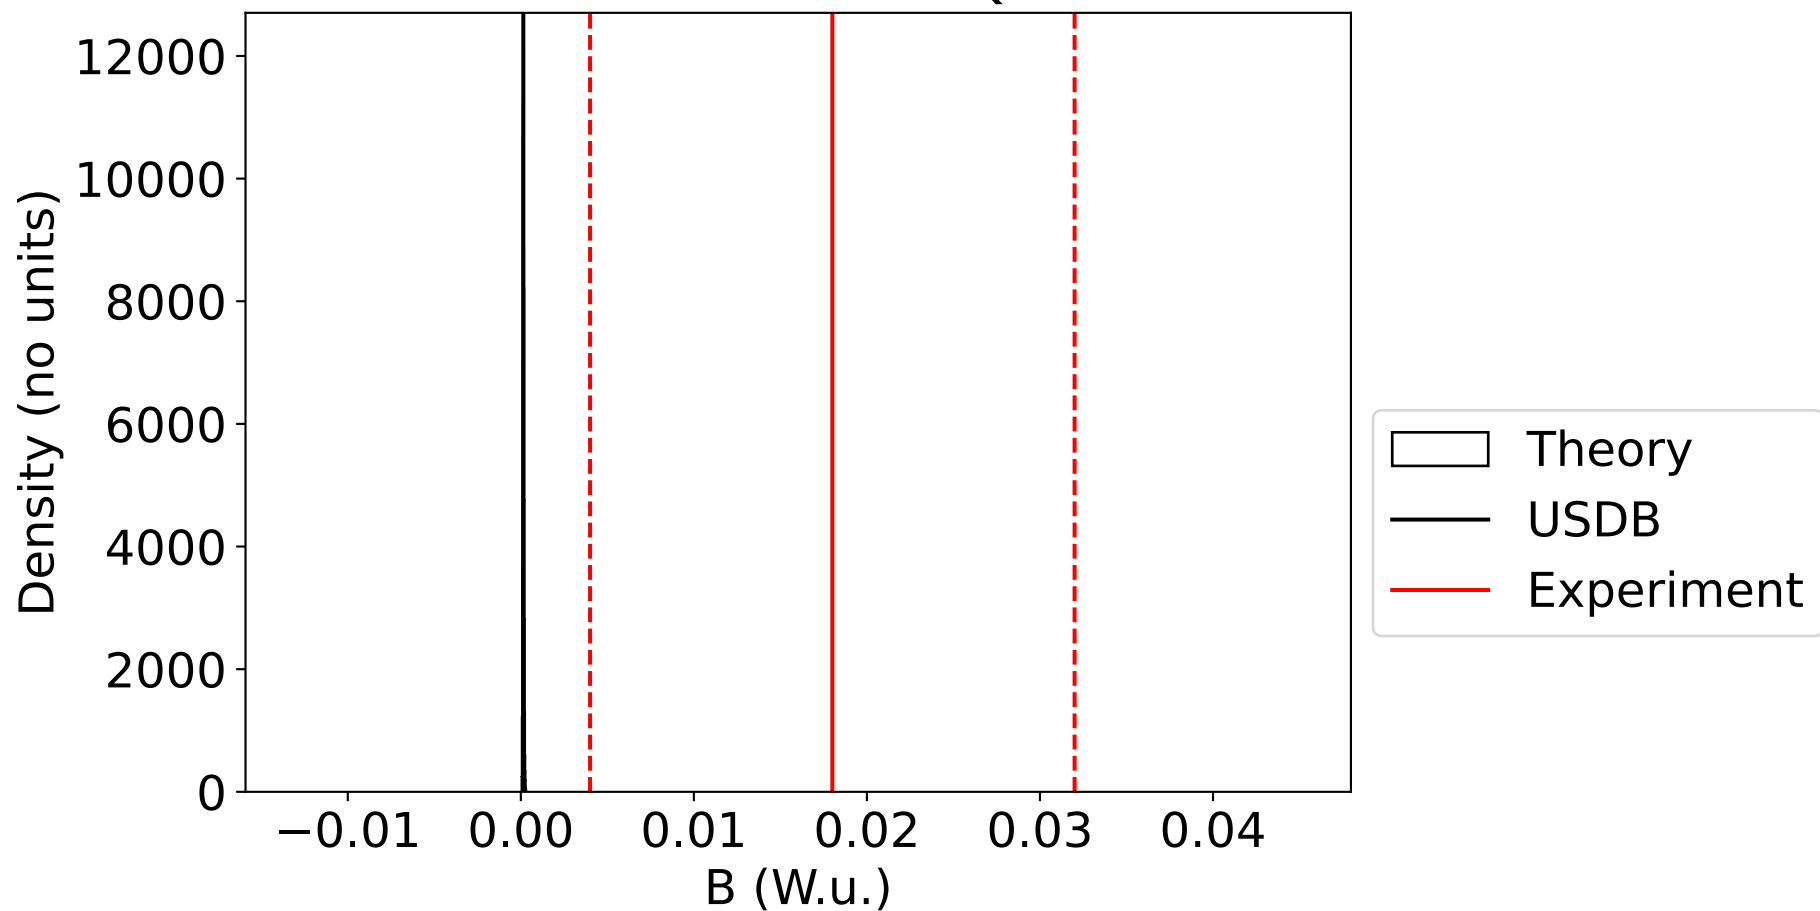

$^{18}\text{F} (3_5) \rightarrow (2_4)$   
Included in UQ

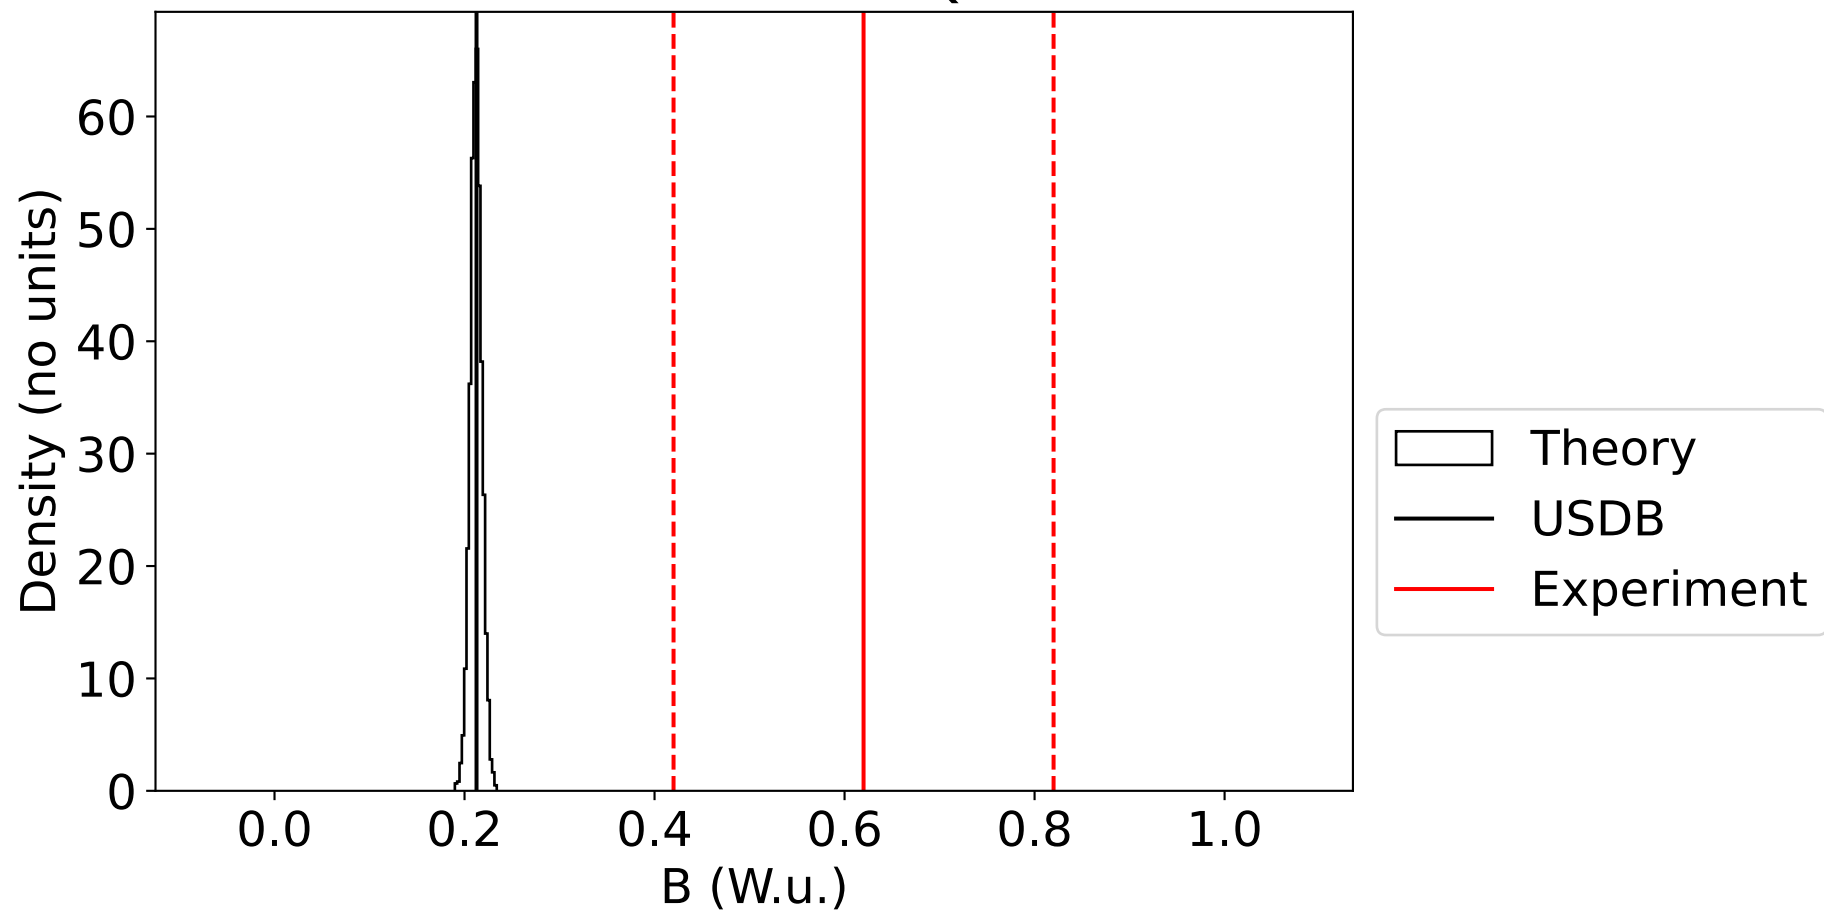

$^{18}\text{F} (3_5) \rightarrow (2_2)$   
Included in UQ

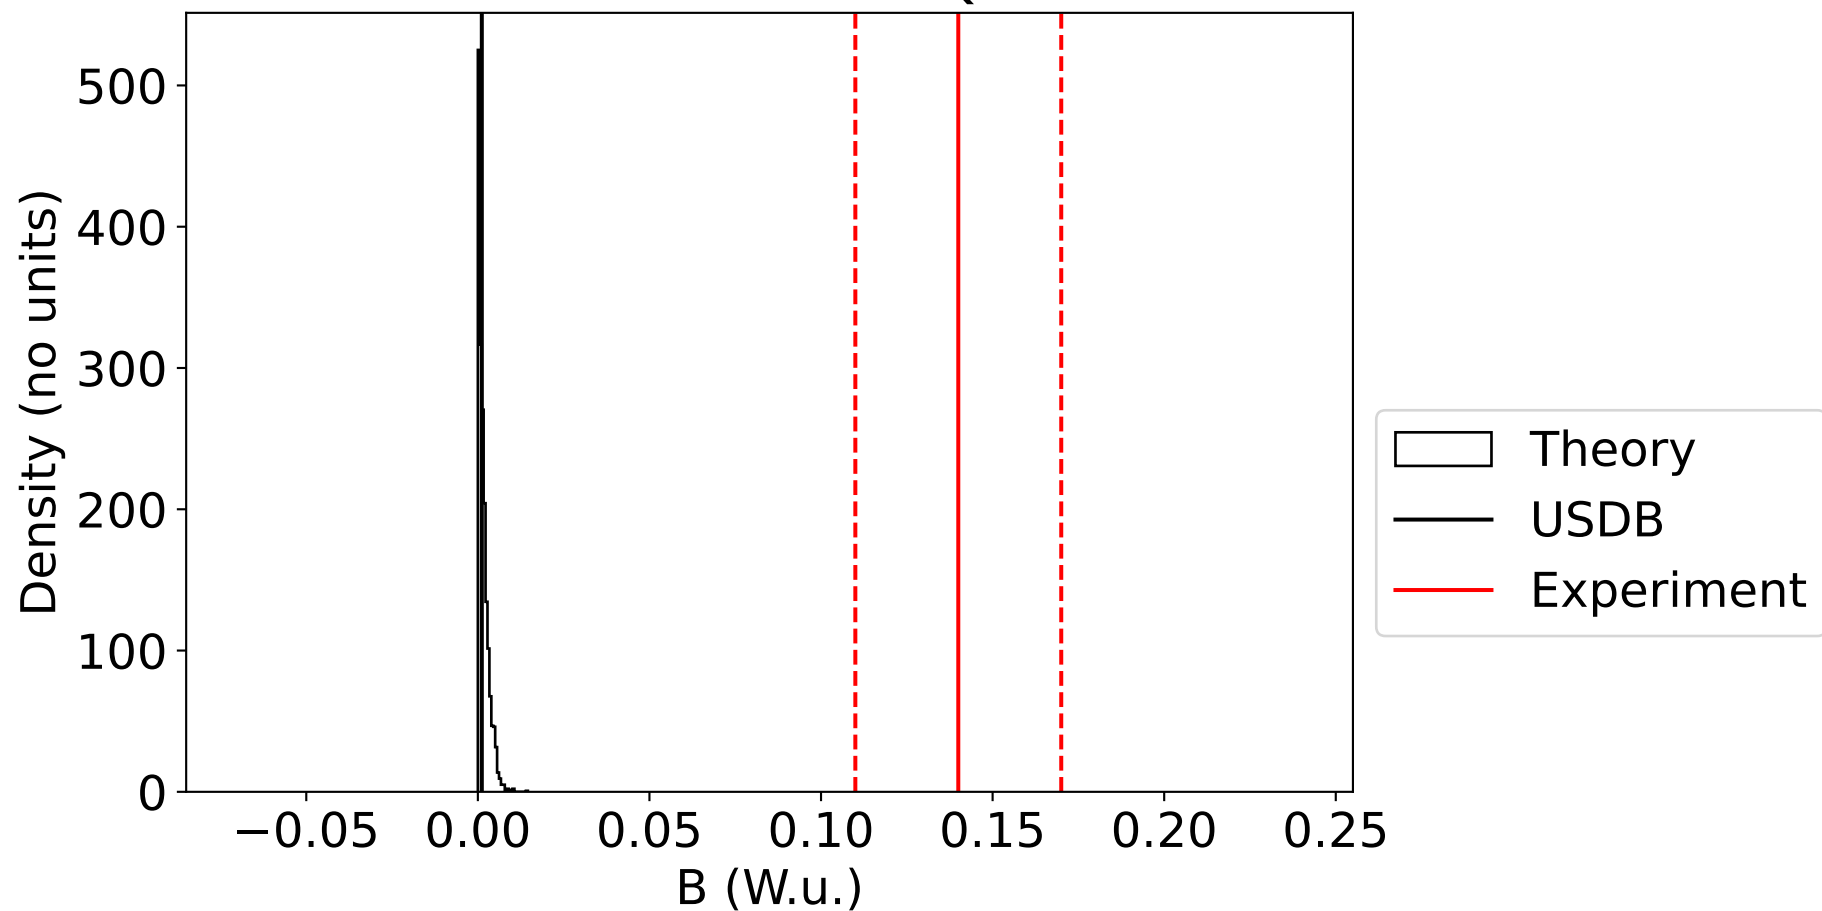



$^{18}\text{F} (3_5) \rightarrow (2_3)$   
Included in UQ

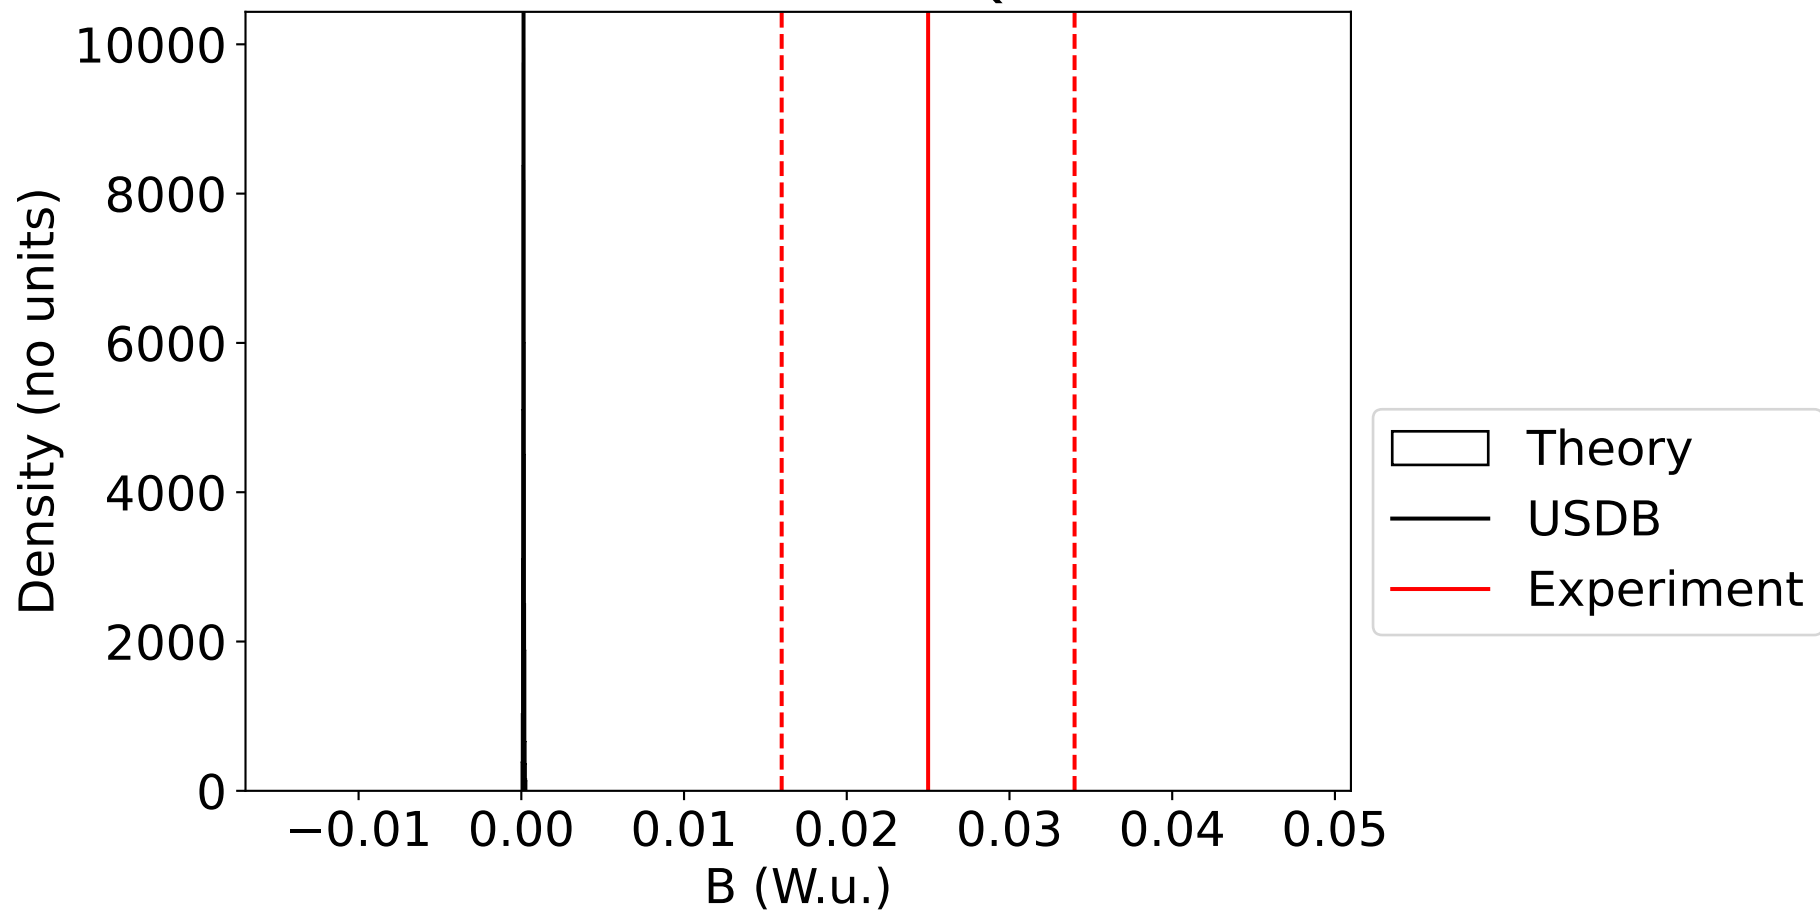

$^{18}\text{F} (2_6) \rightarrow (2_3)$   
Included in UQ

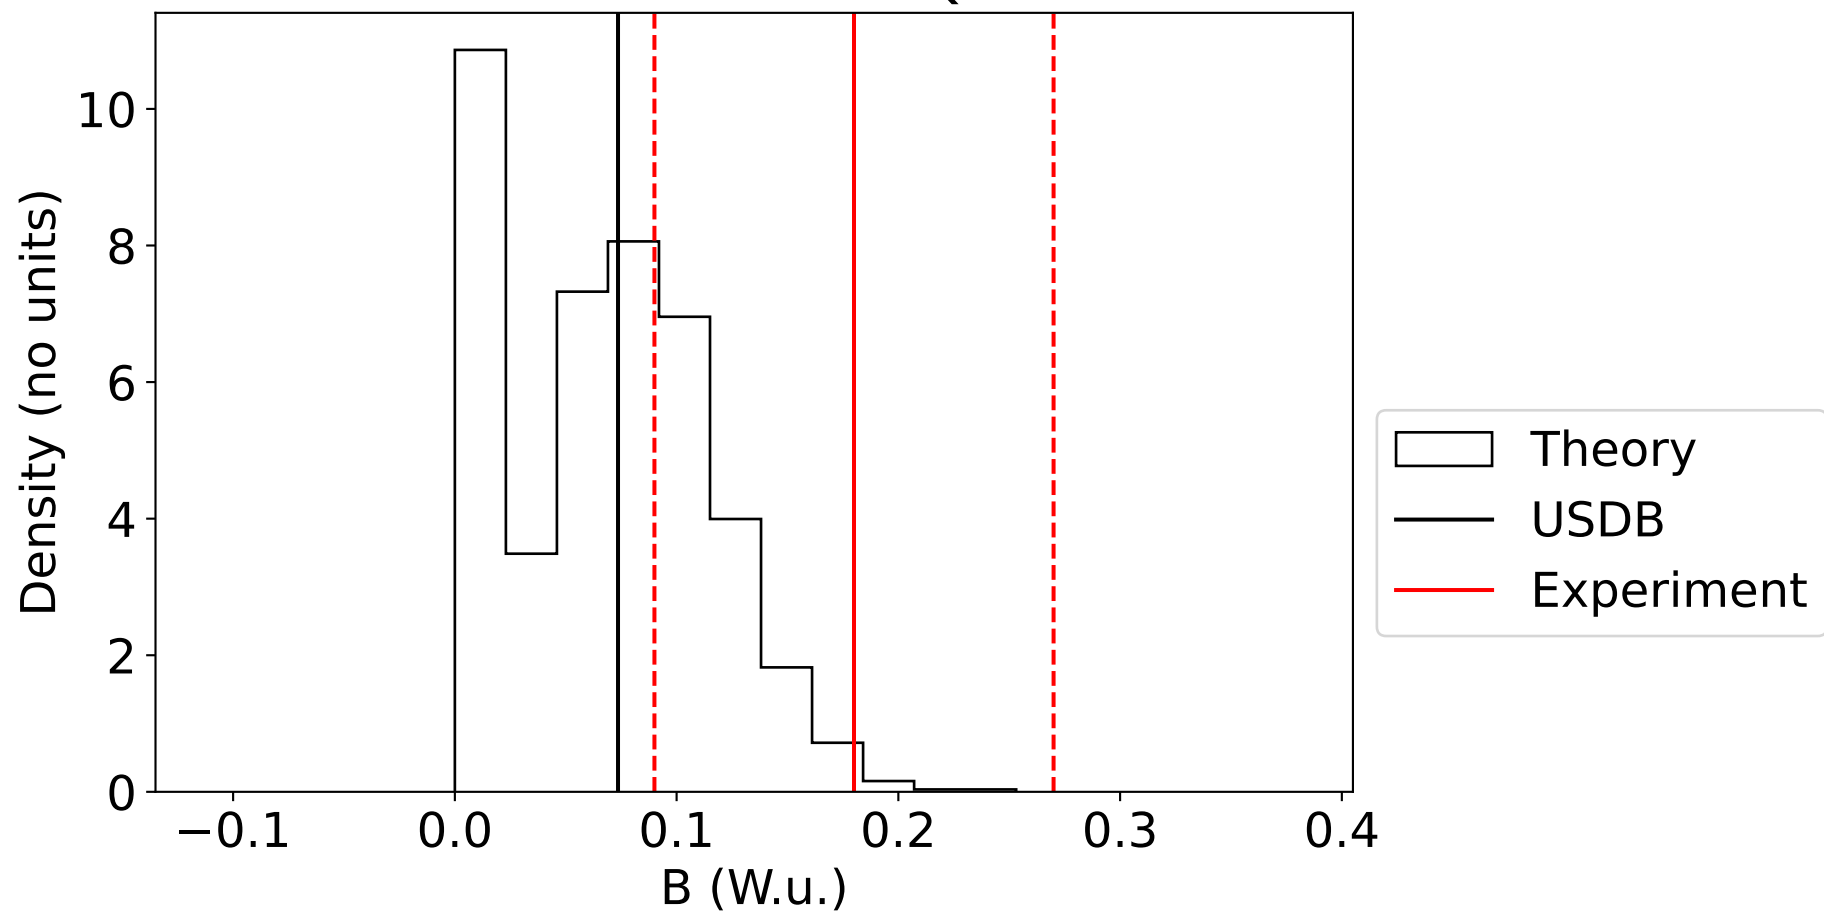

$^{18}\text{F} (2_6) \rightarrow (3_3)$   
Included in UQ

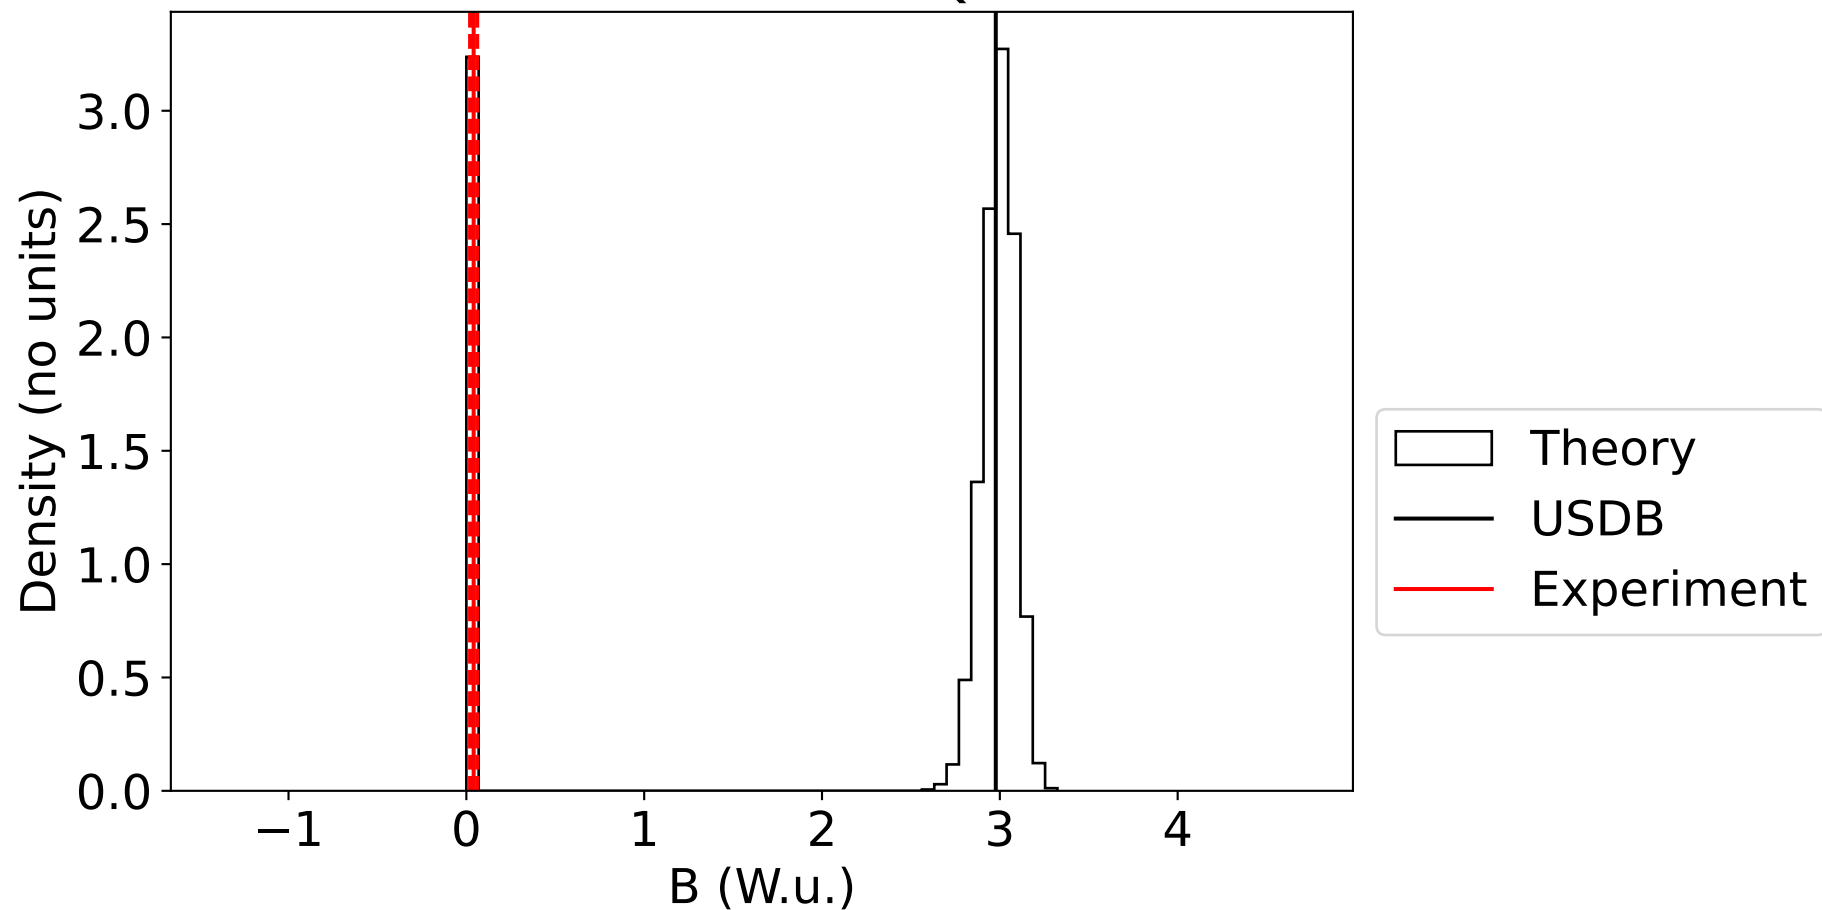

$^{18}\text{F} (2_6) \rightarrow (1_2)$   
Included in UQ

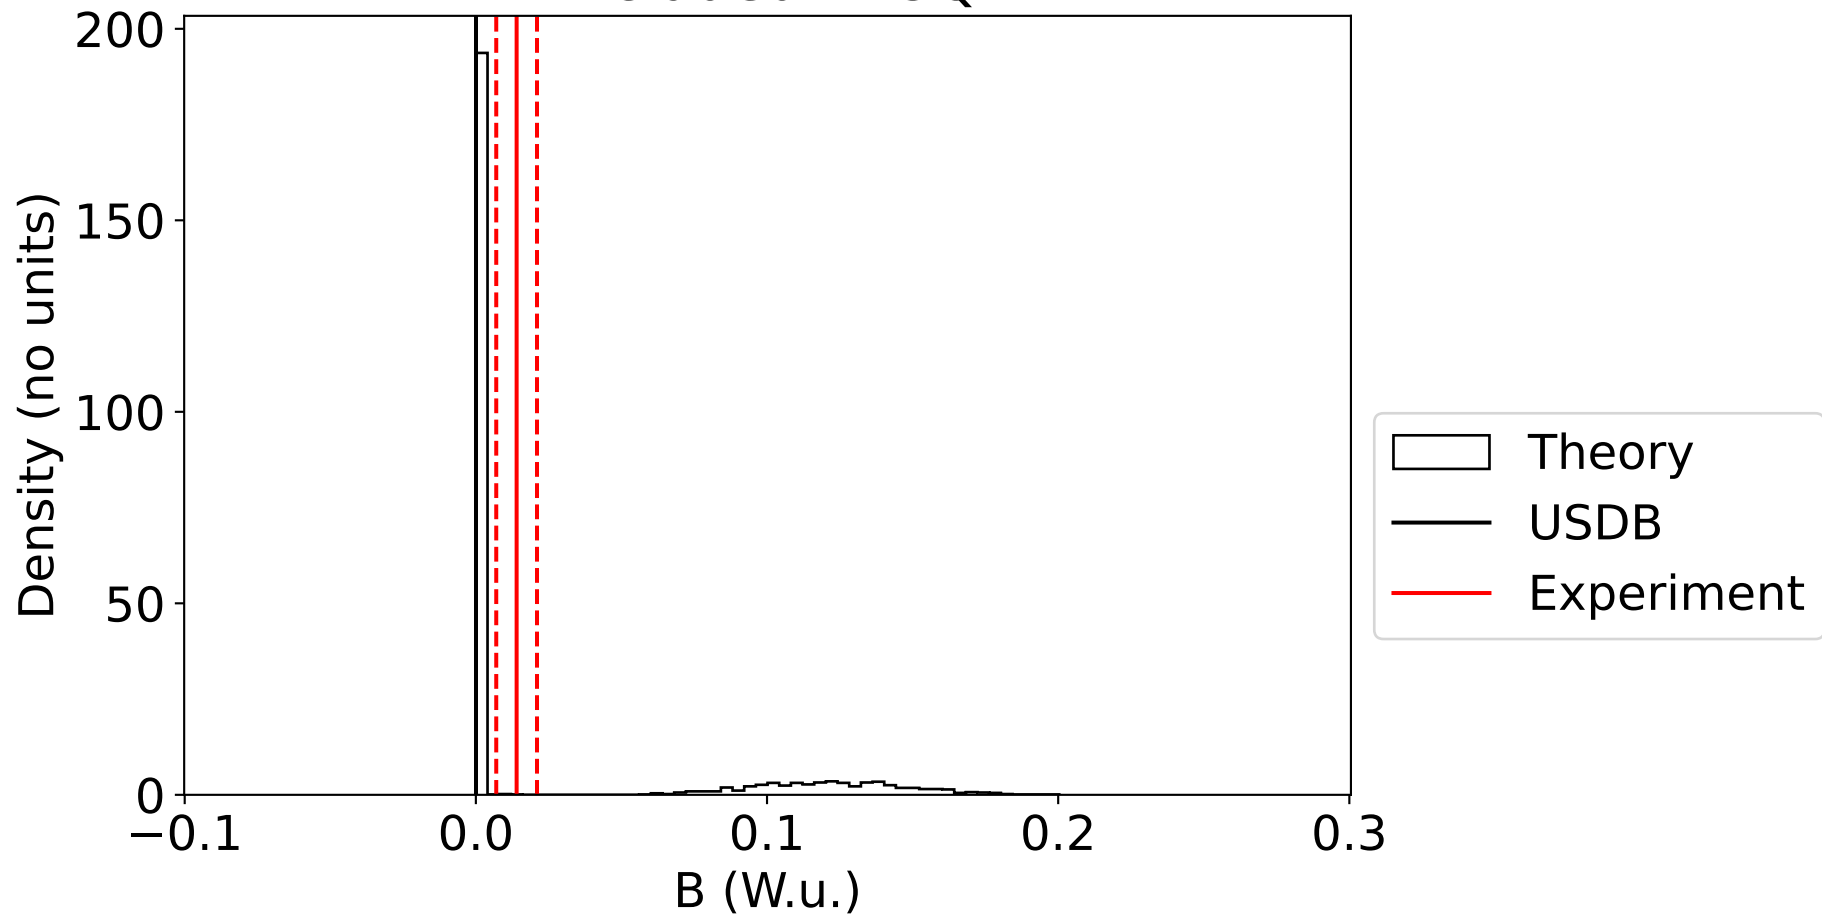

$^{18}\text{F} (3_6) \rightarrow (2_2)$   
Included in UQ

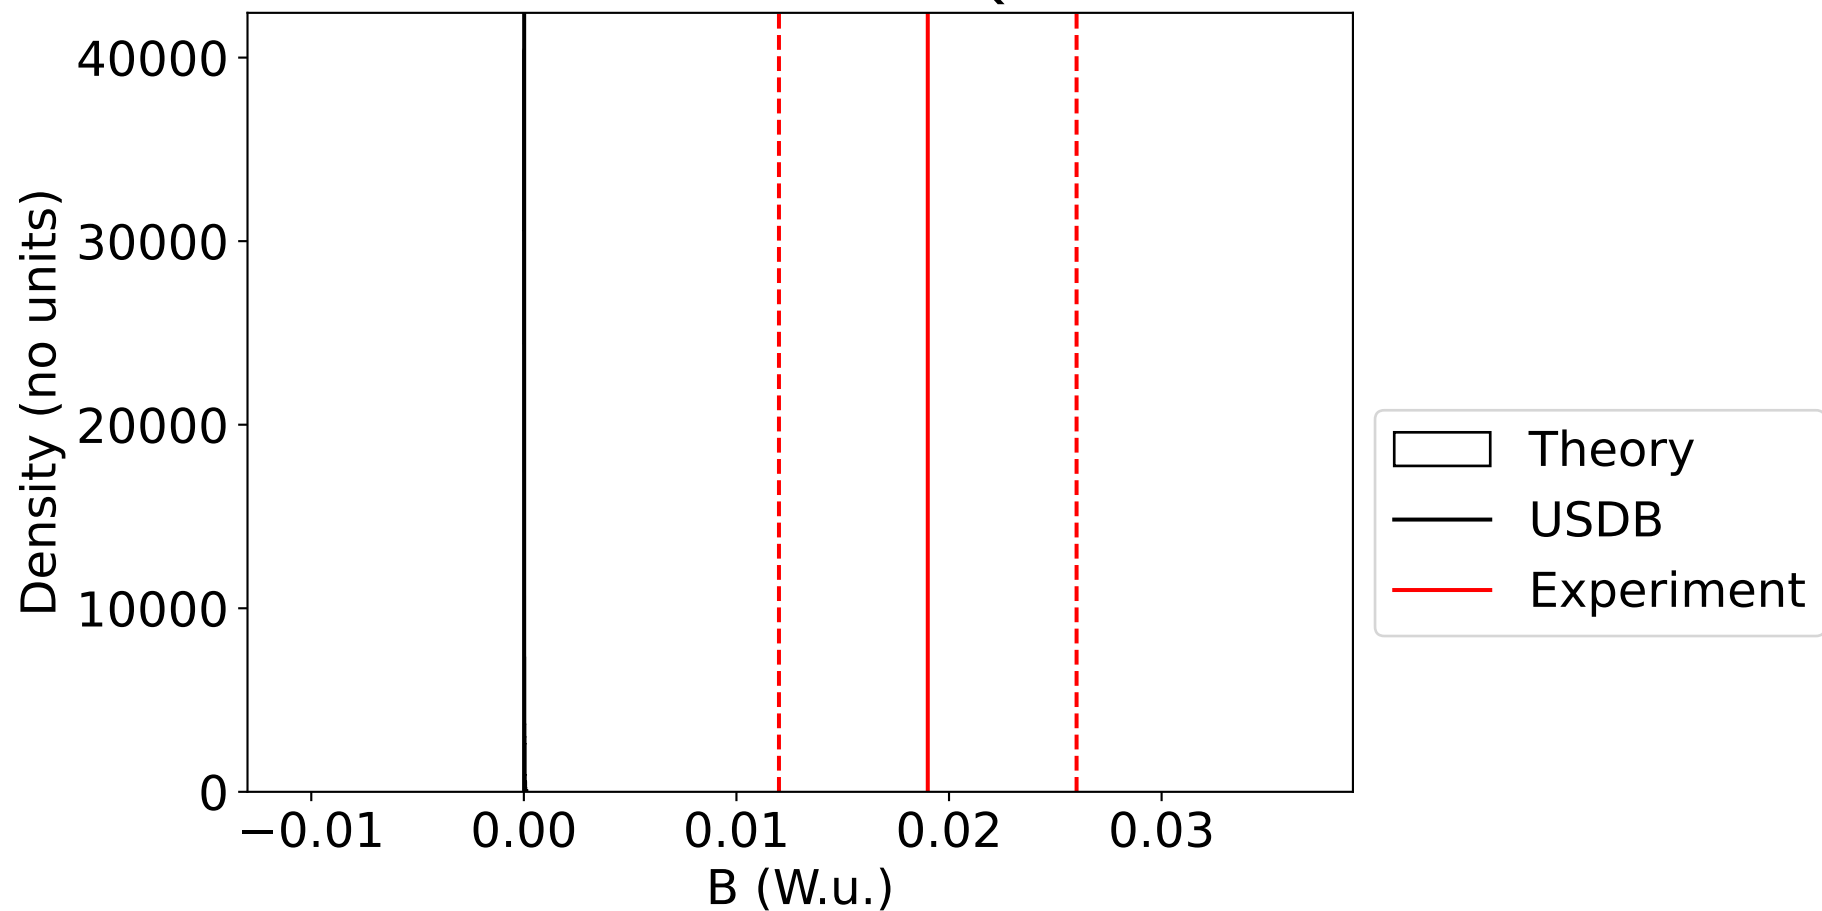

$^{18}\text{F} (3_6) \rightarrow (2_3)$   
Included in UQ

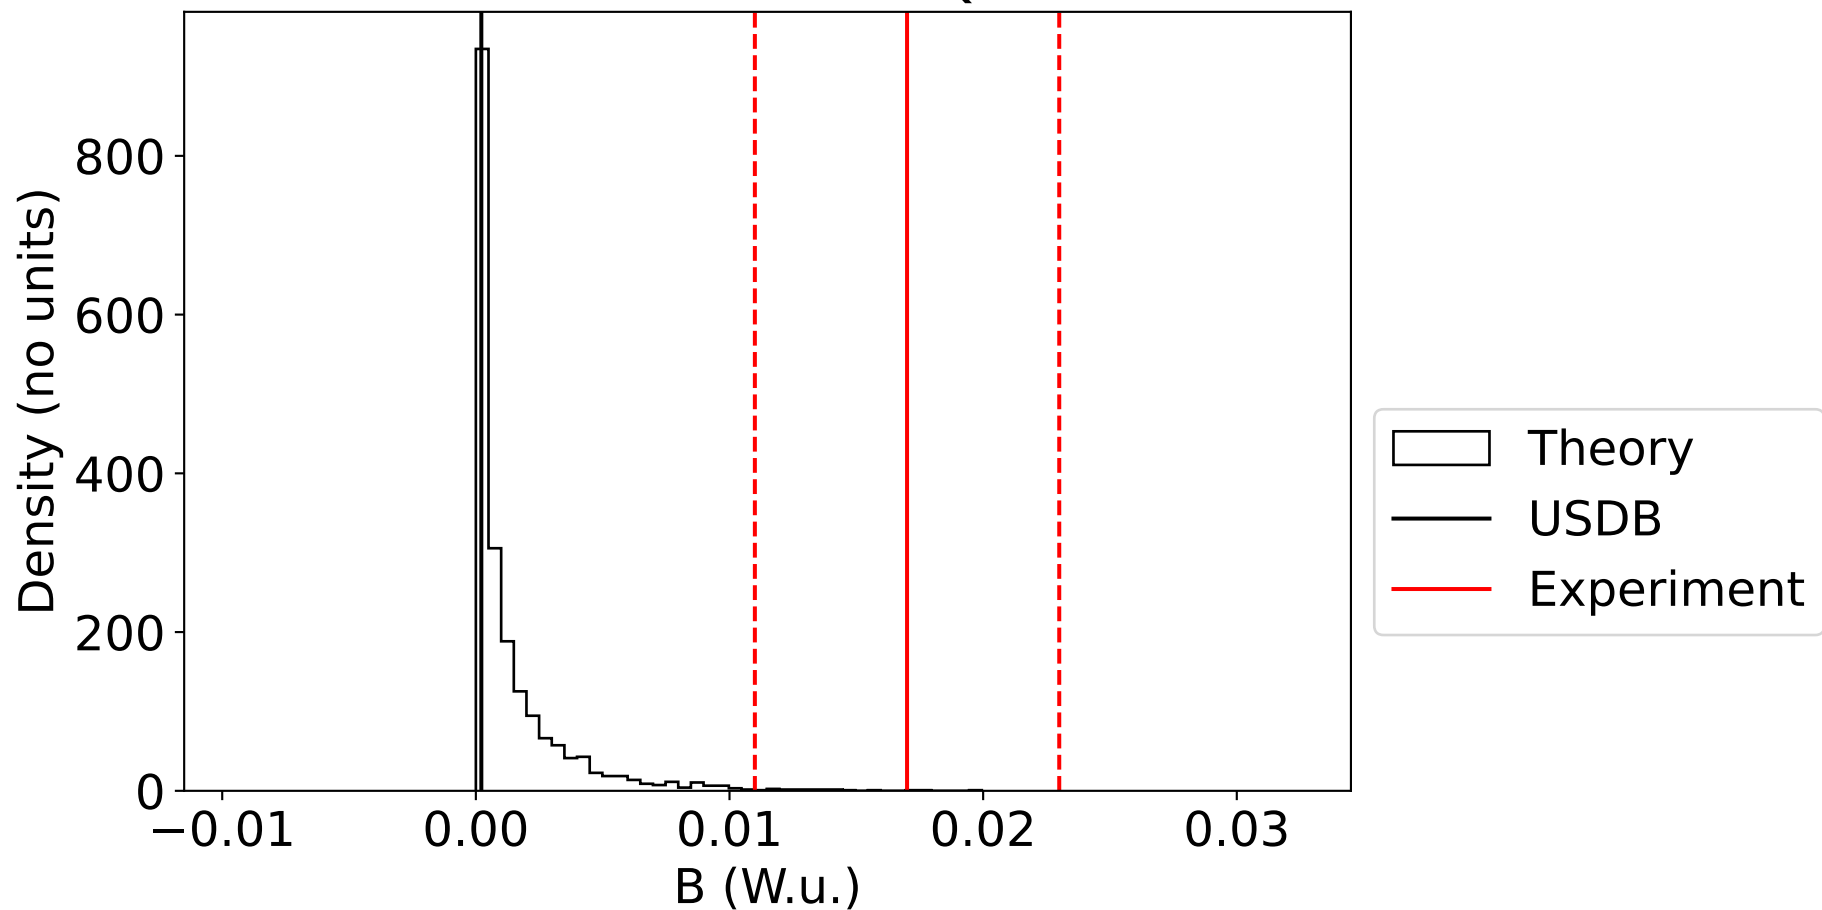

$^{18}\text{F} (3_6) \rightarrow (2_4)$   
Included in UQ

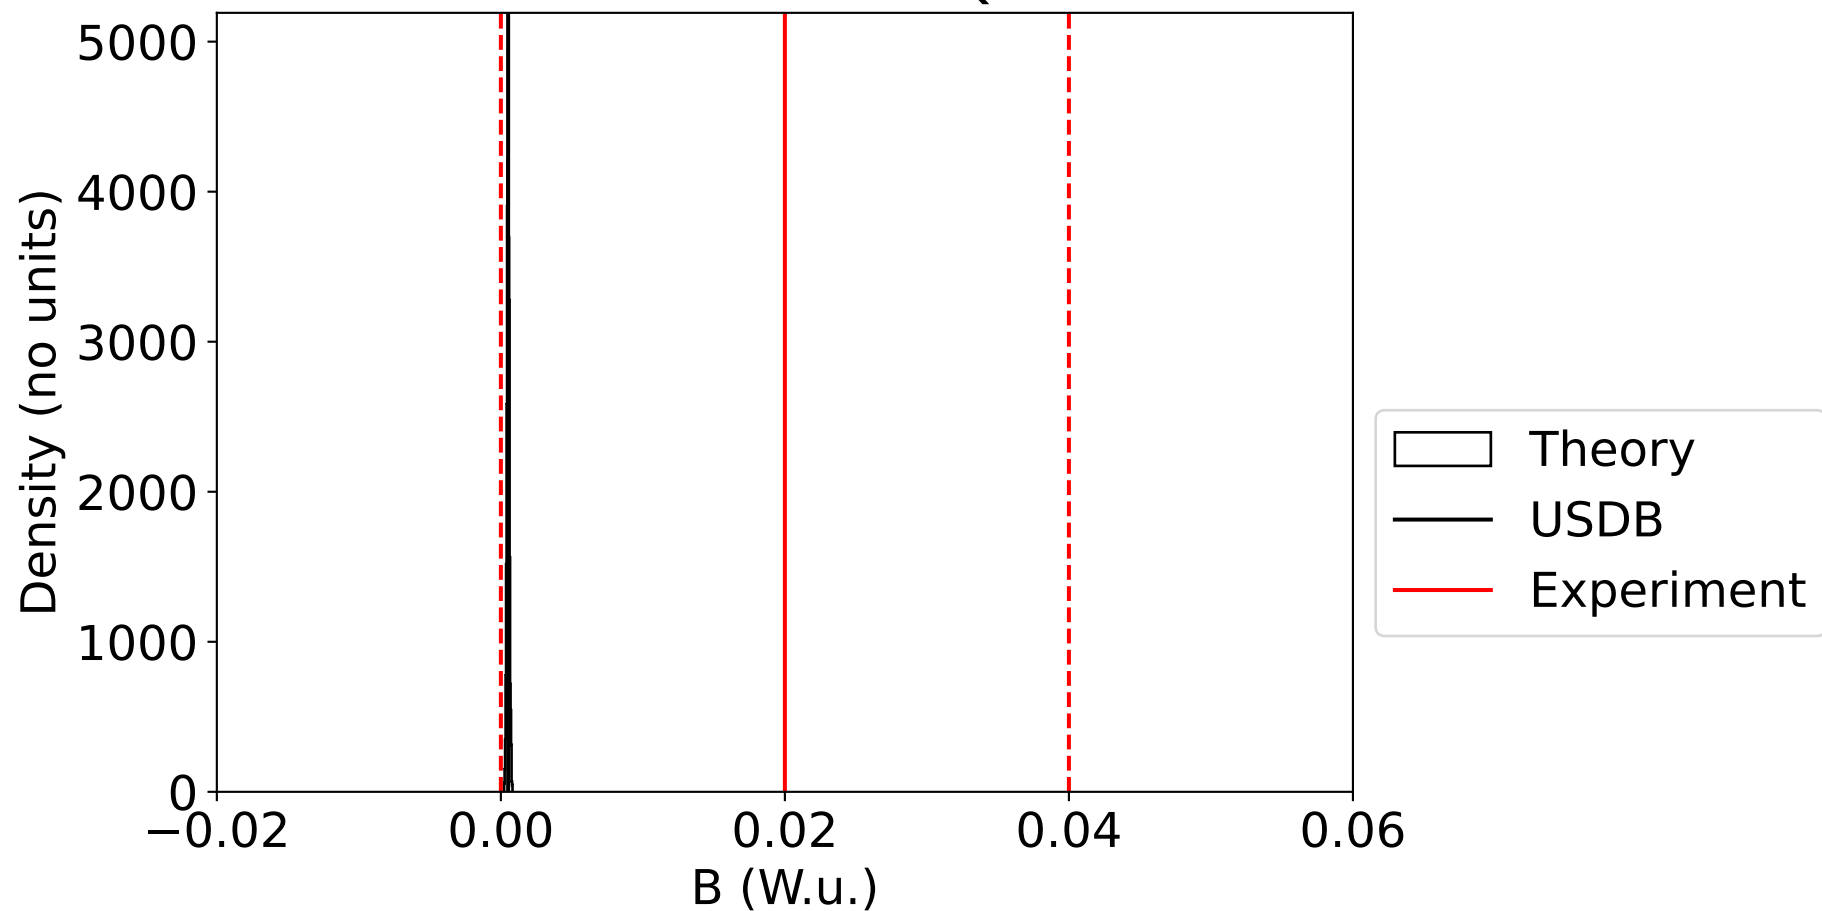

$^{19}\text{F} (3/2_1) \rightarrow (1/2_1)$   
Included in UQ

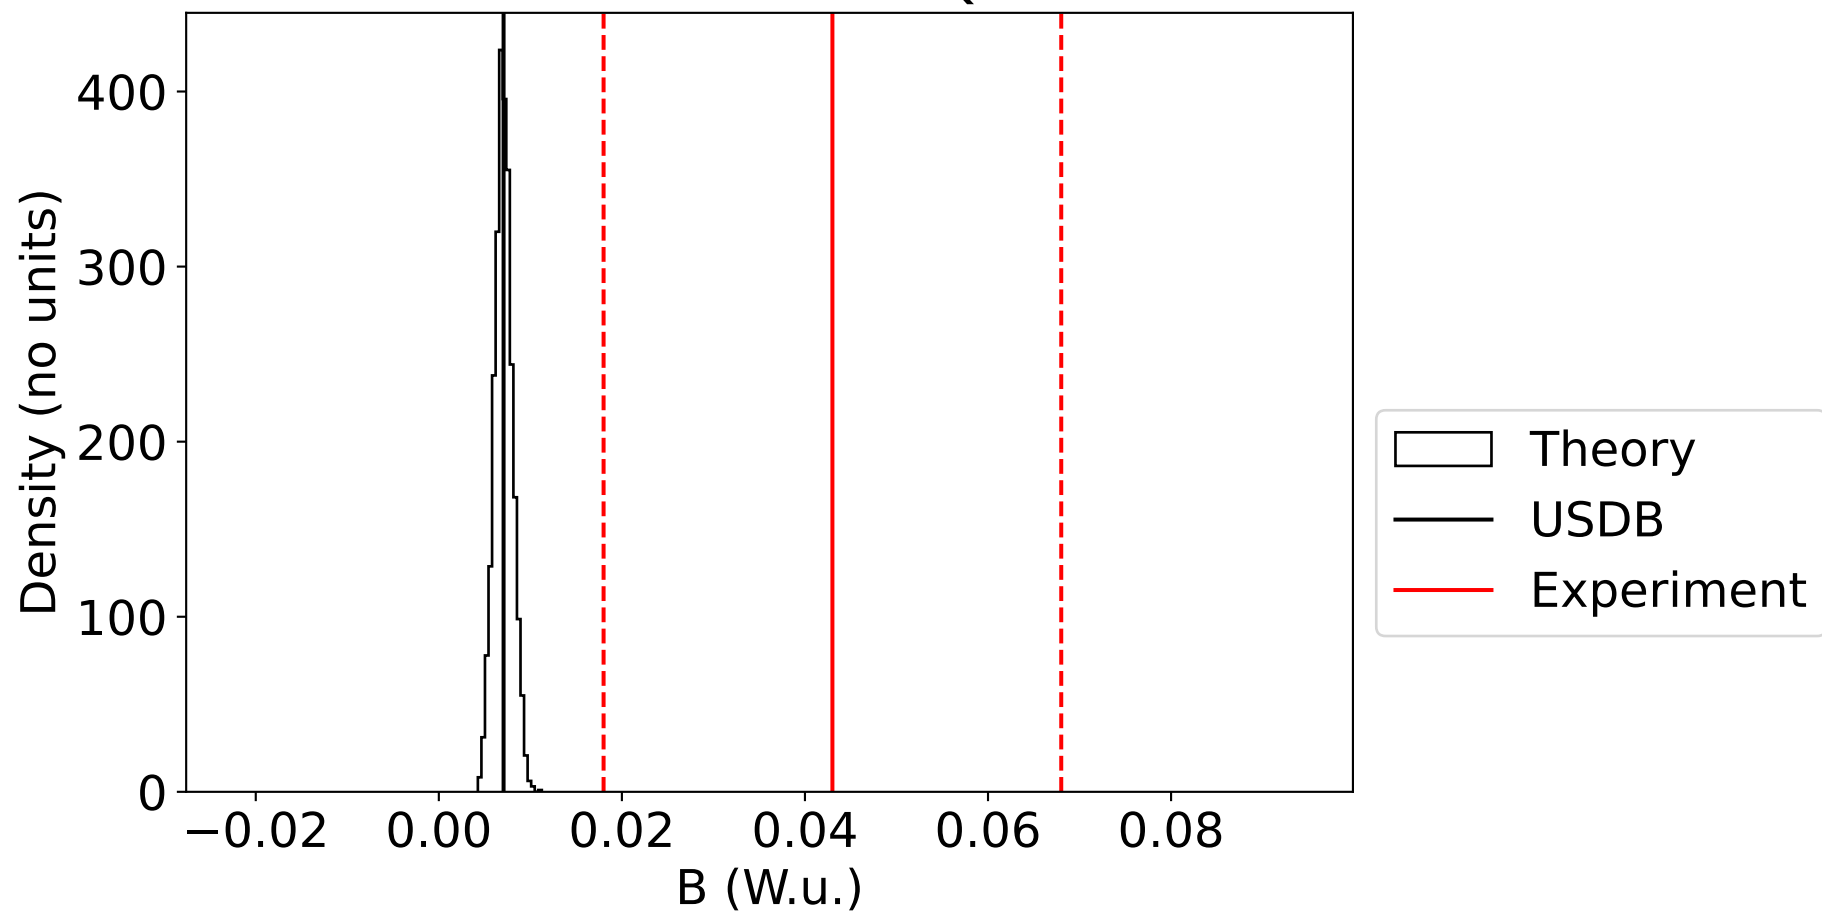



$^{19}\text{F}$  ( $3/2_1$ )  $\rightarrow$  ( $5/2_1$ )  
Included in UQ

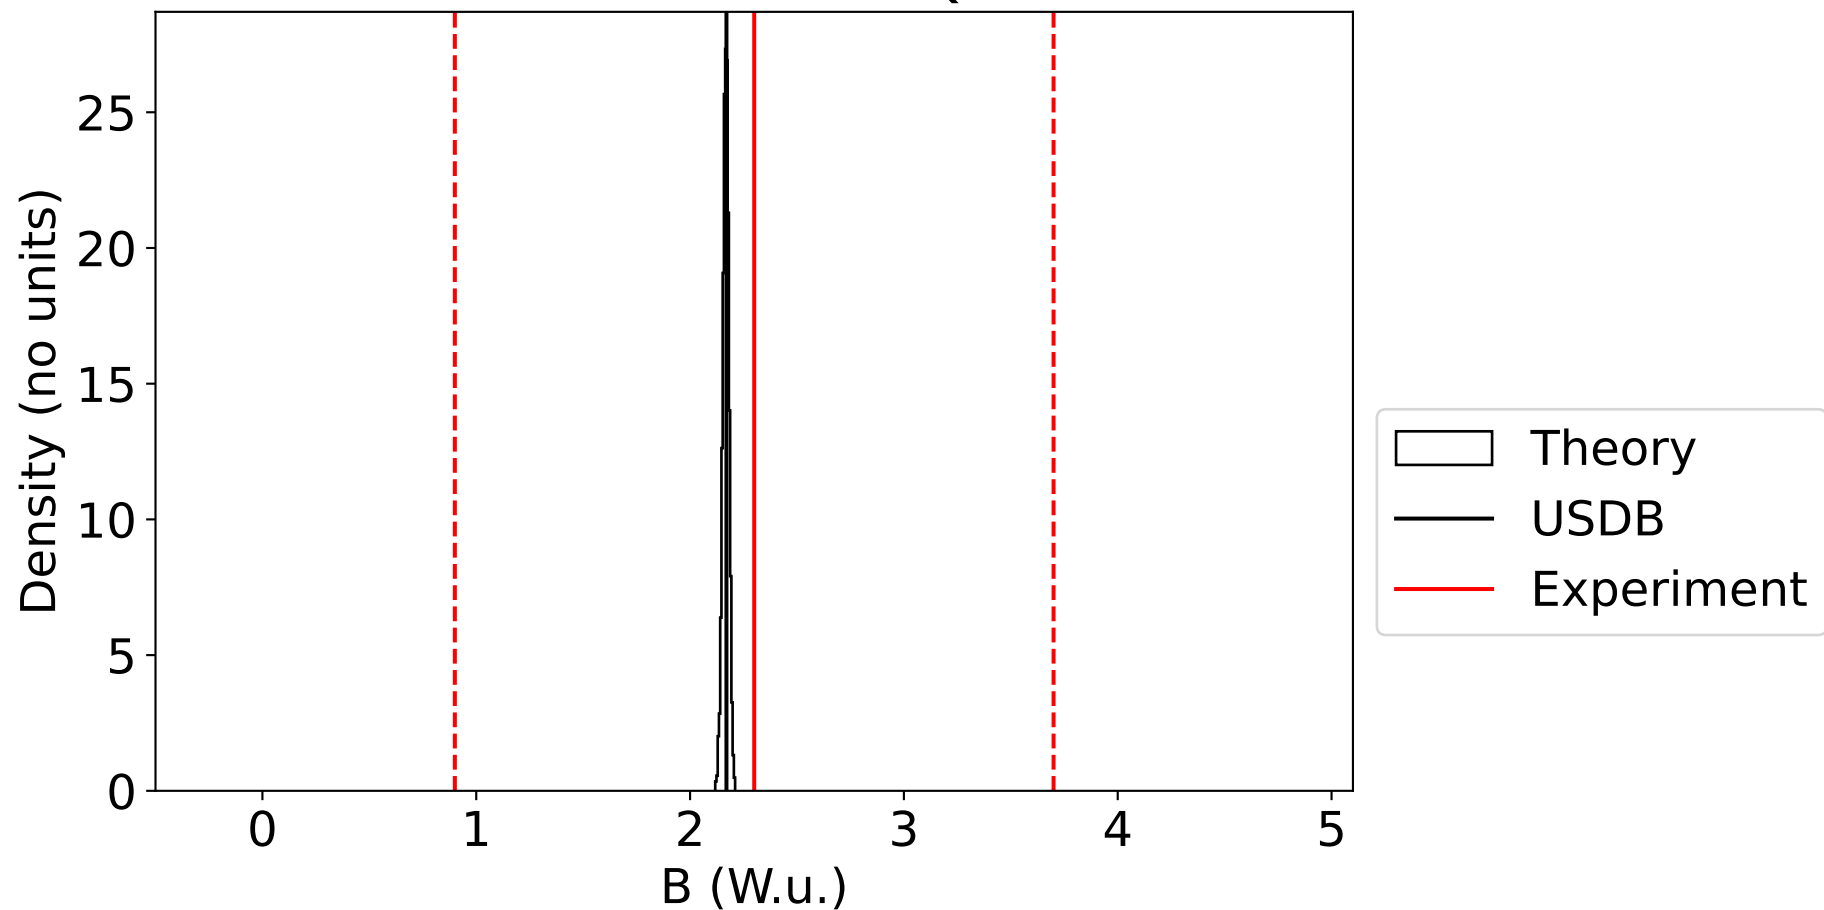

$^{19}\text{F} (3/2_2) \rightarrow (3/2_1)$   
Included in UQ

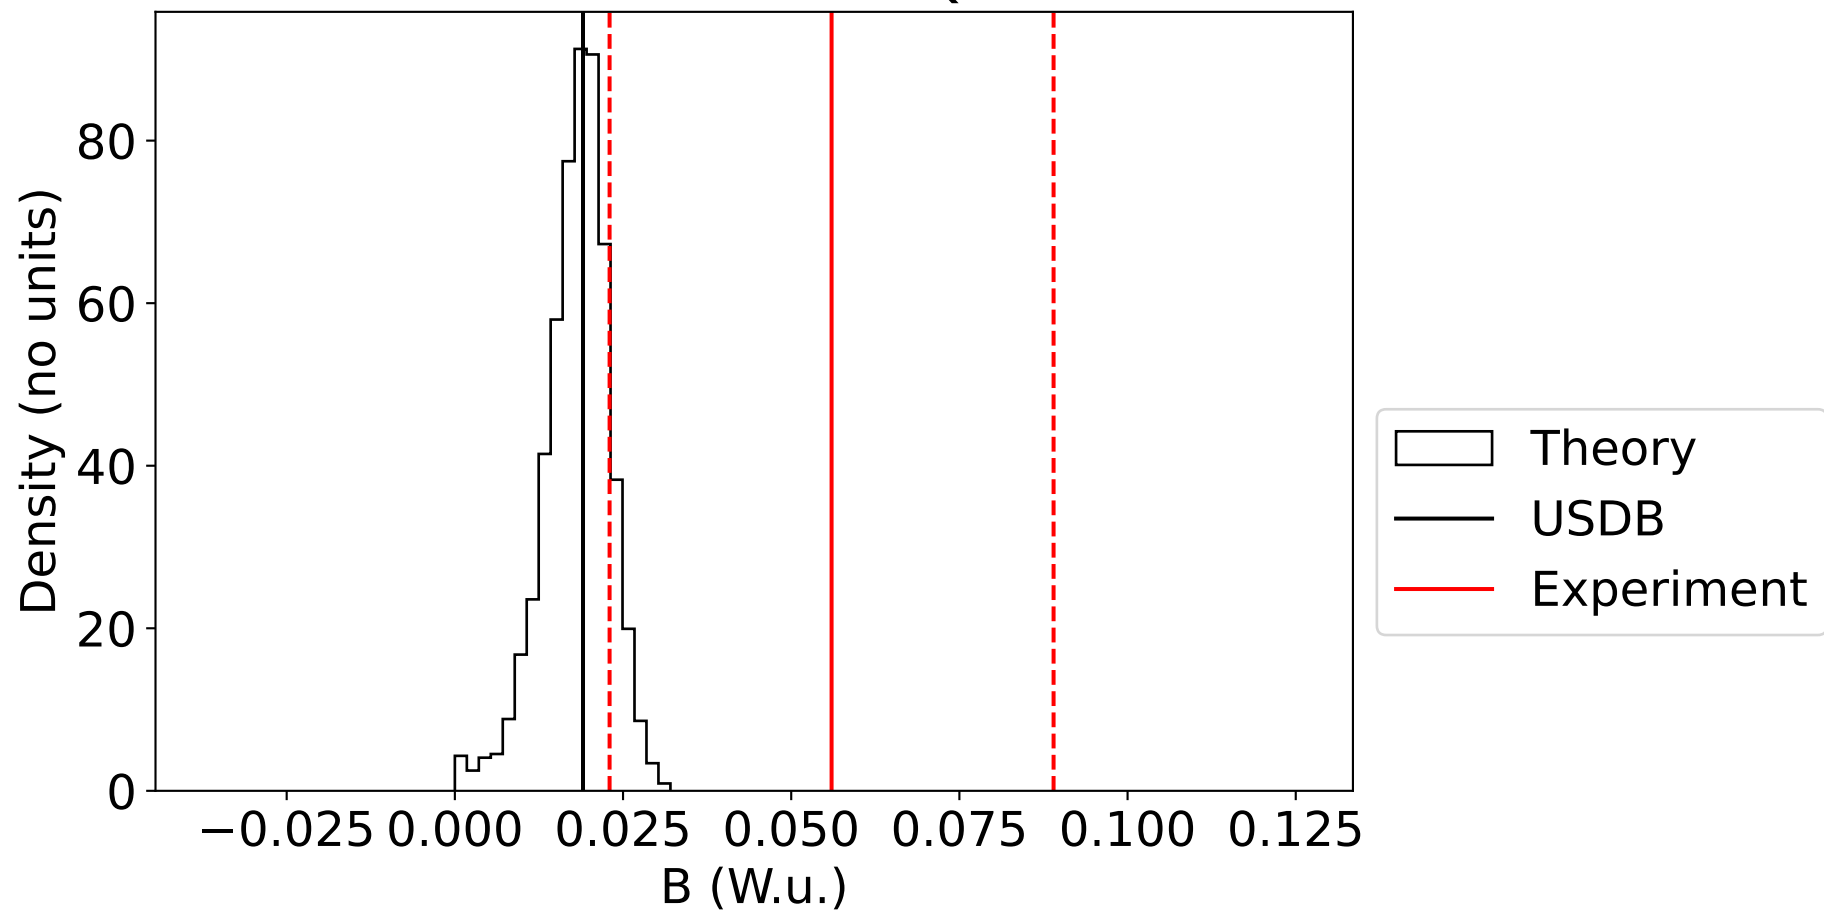

$^{19}\text{F} (3/2_2) \rightarrow (1/2_1)$   
Included in UQ

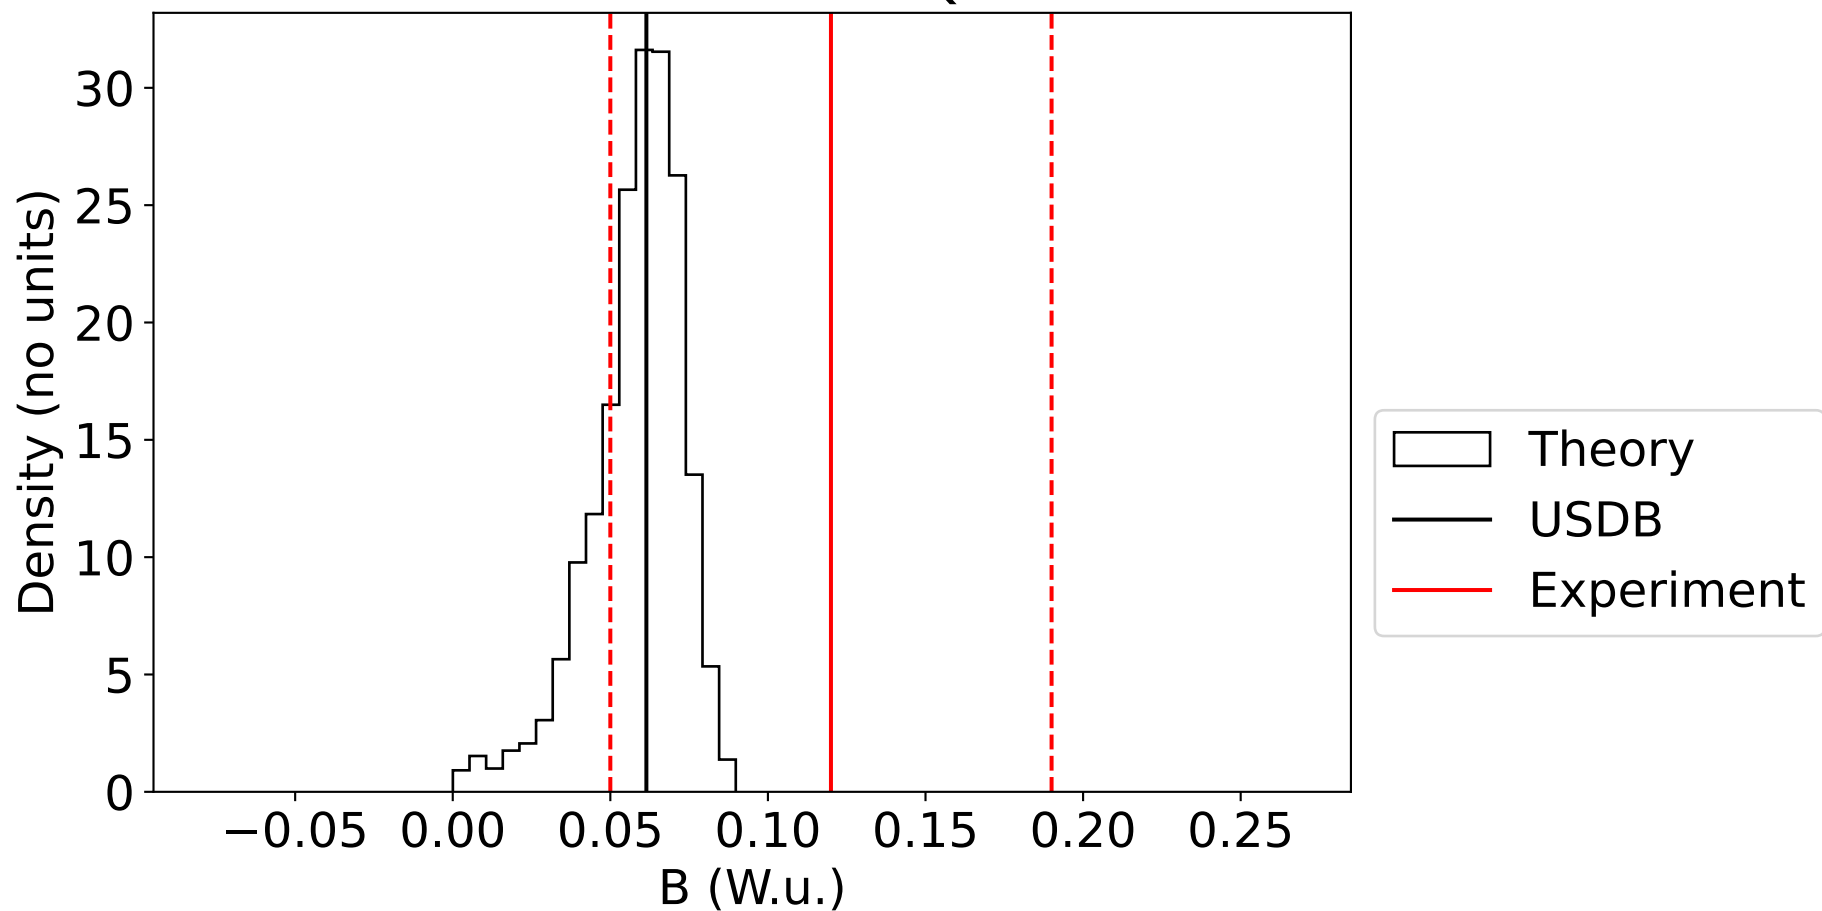

$^{19}\text{F} (7/2_3) \rightarrow (9/2_1)$   
Included in UQ

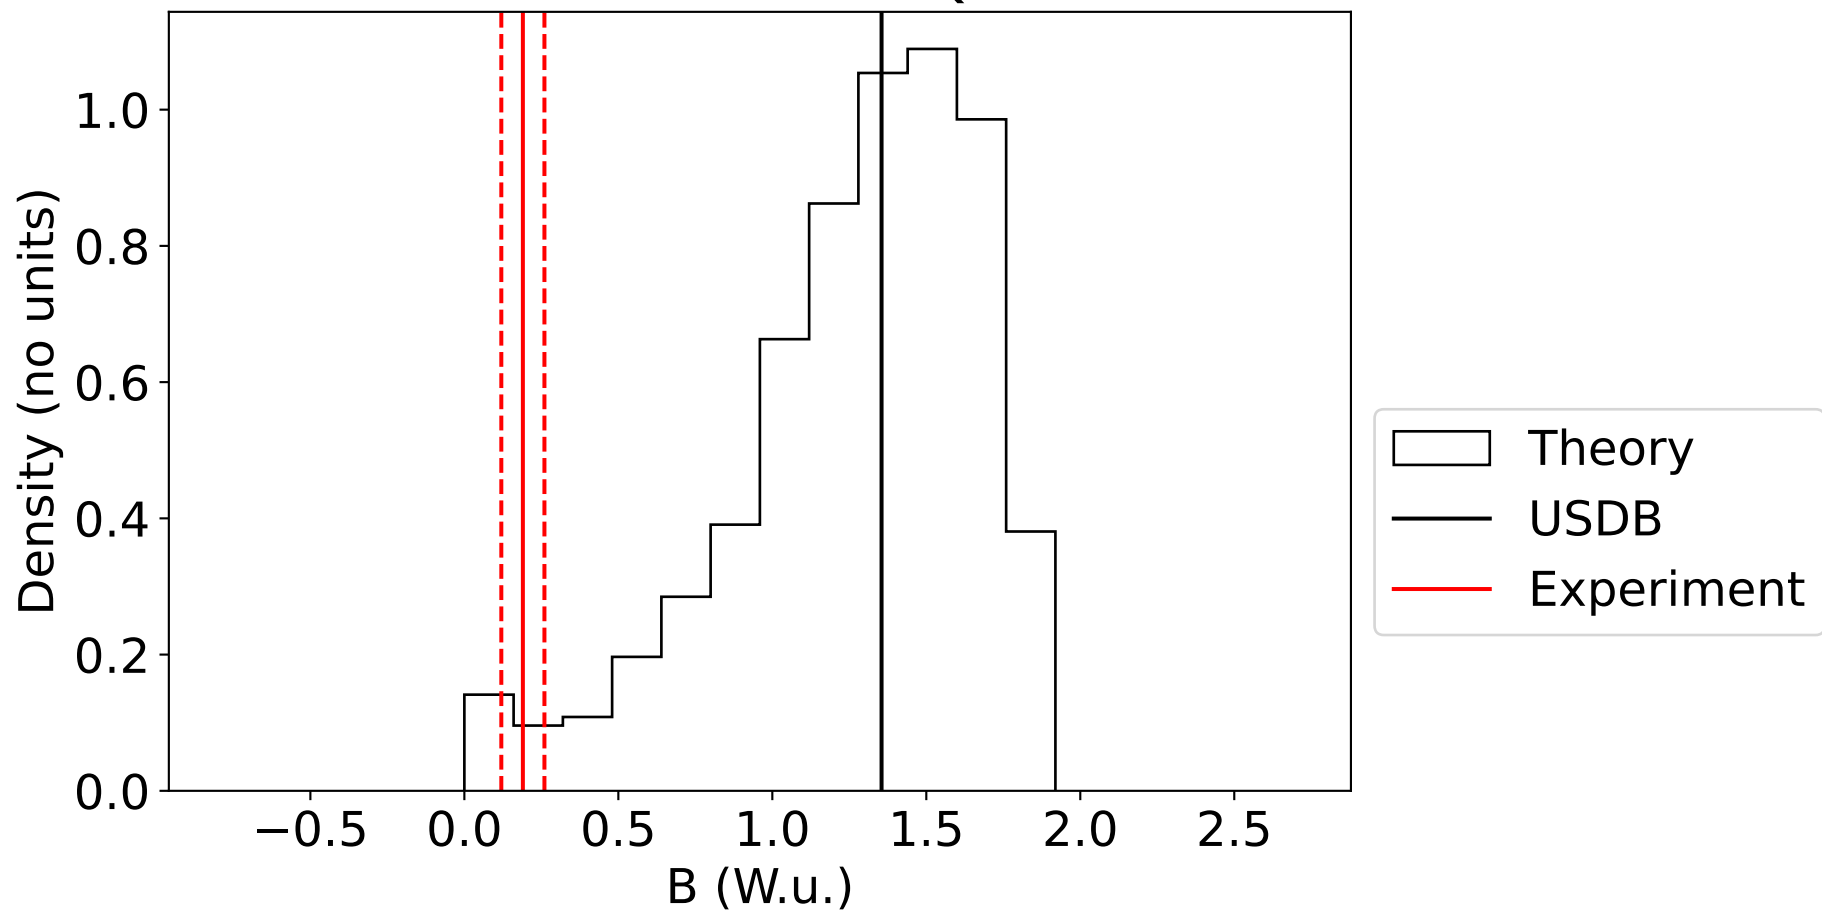

$^{19}\text{F} (7/2_3) \rightarrow (7/2_1)$   
Included in UQ

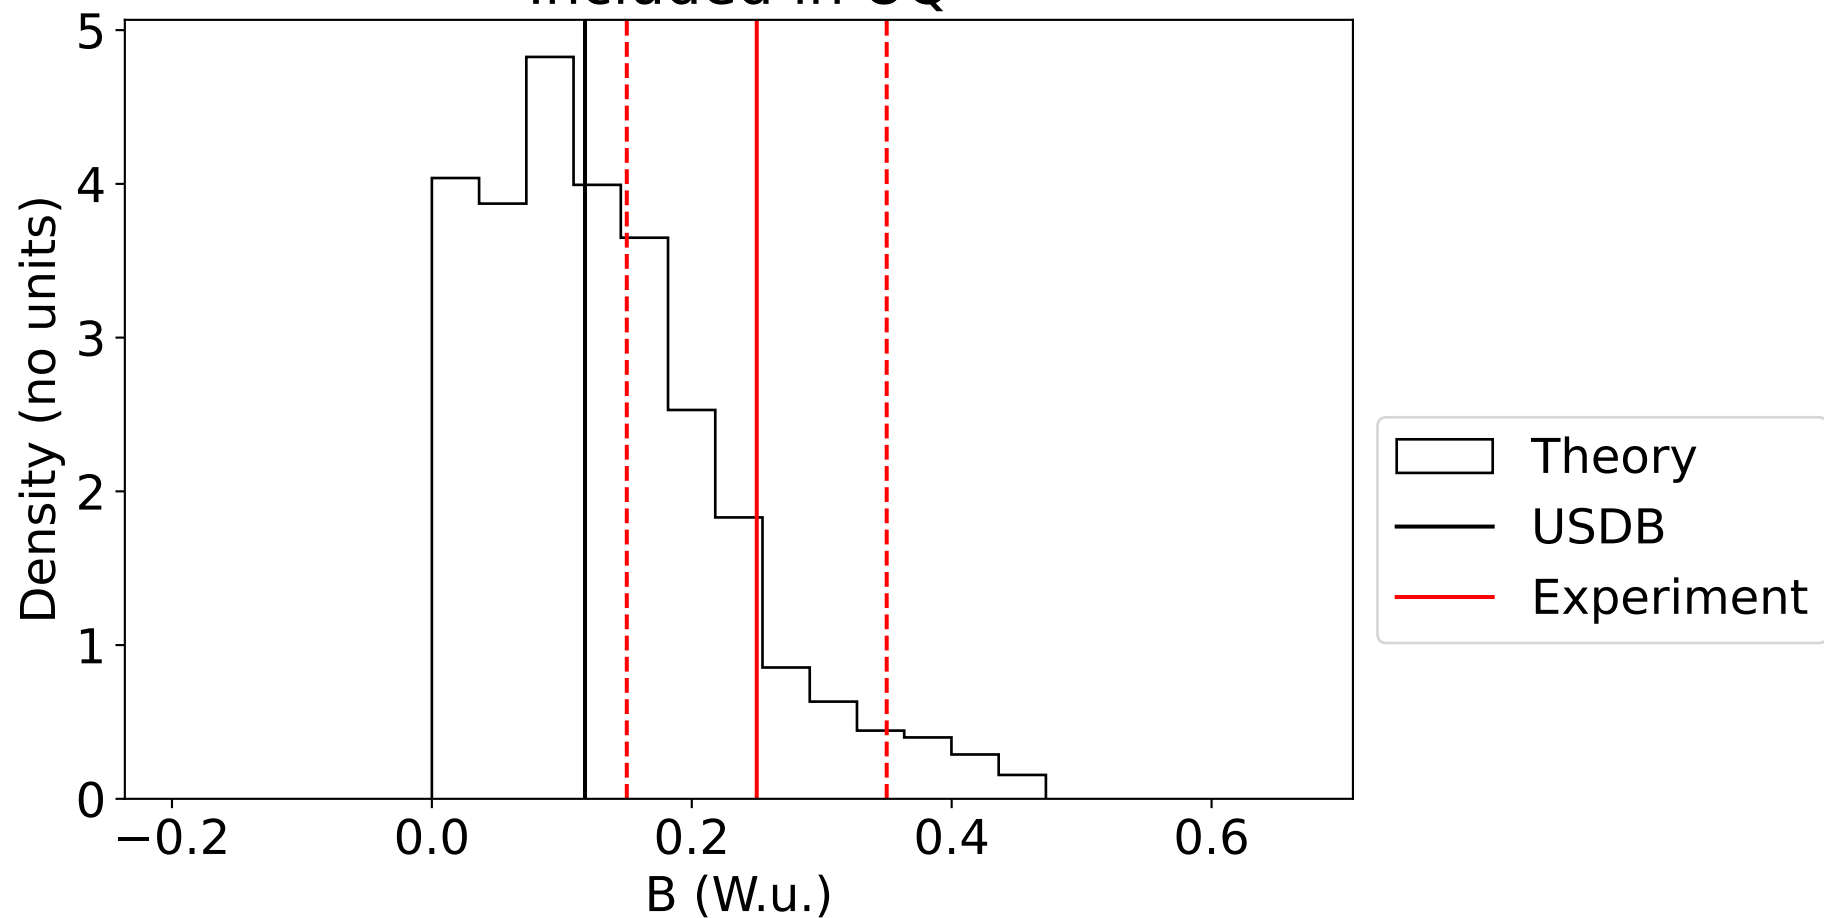

$^{19}\text{F} (5/2_5) \rightarrow (3/2_1)$   
Included in UQ

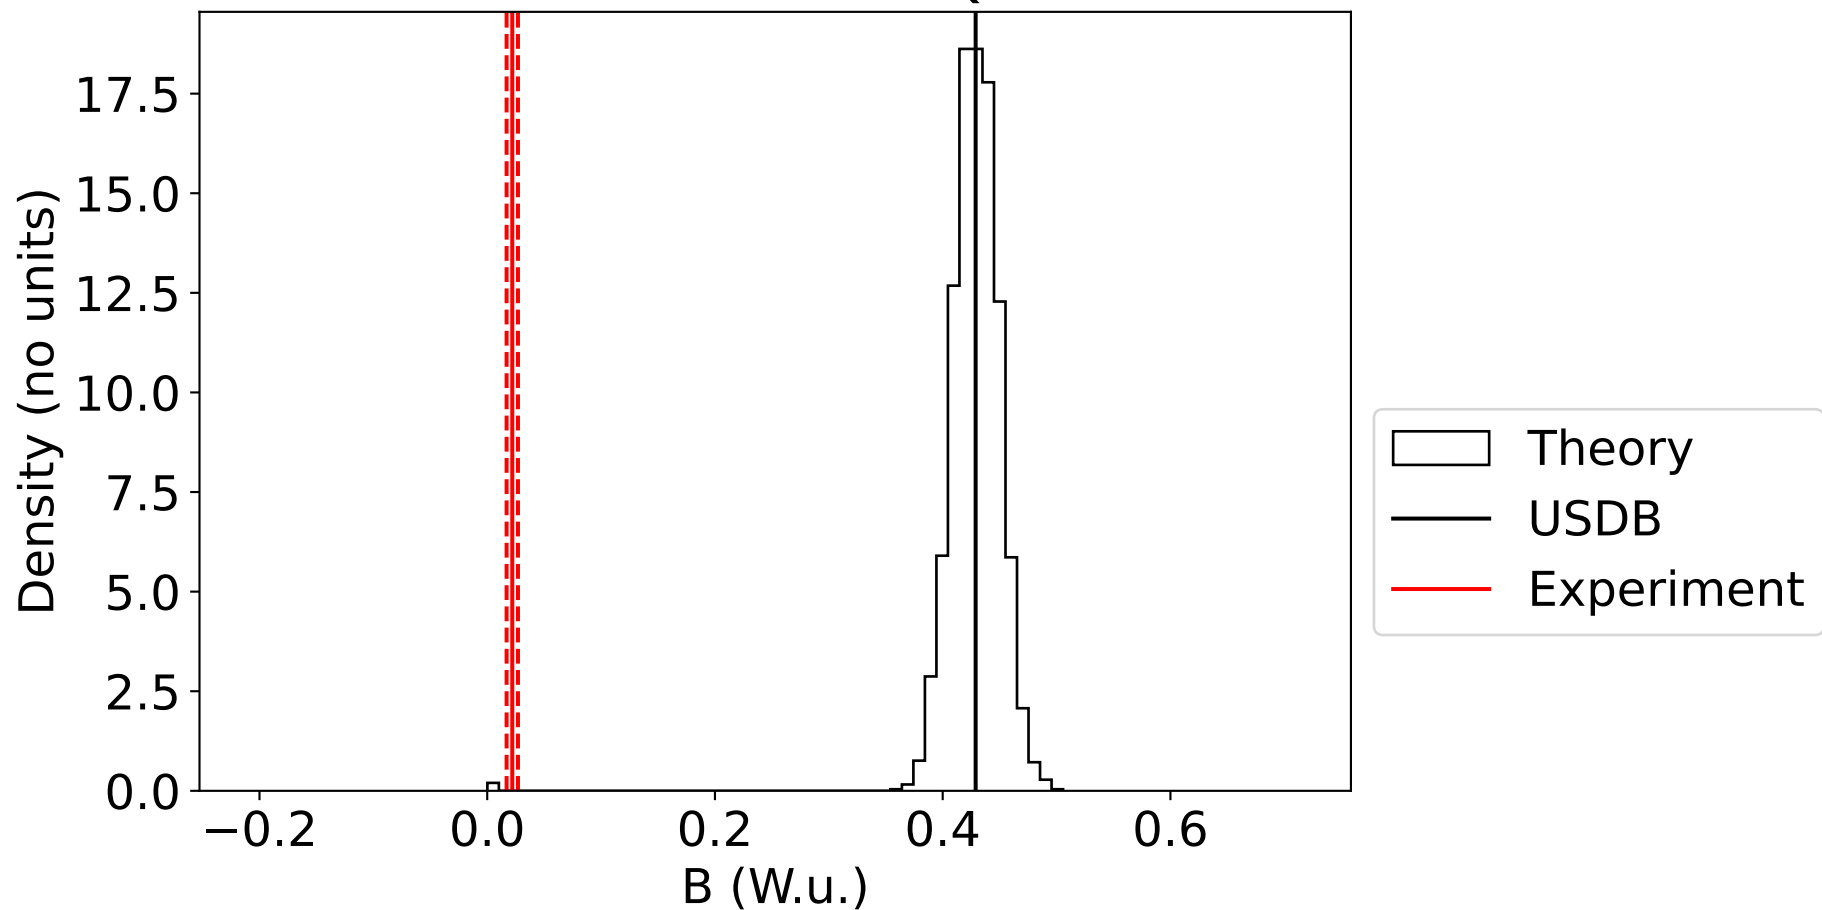

$^{19}\text{F} (7/2_4) \rightarrow (7/2_1)$   
Included in UQ

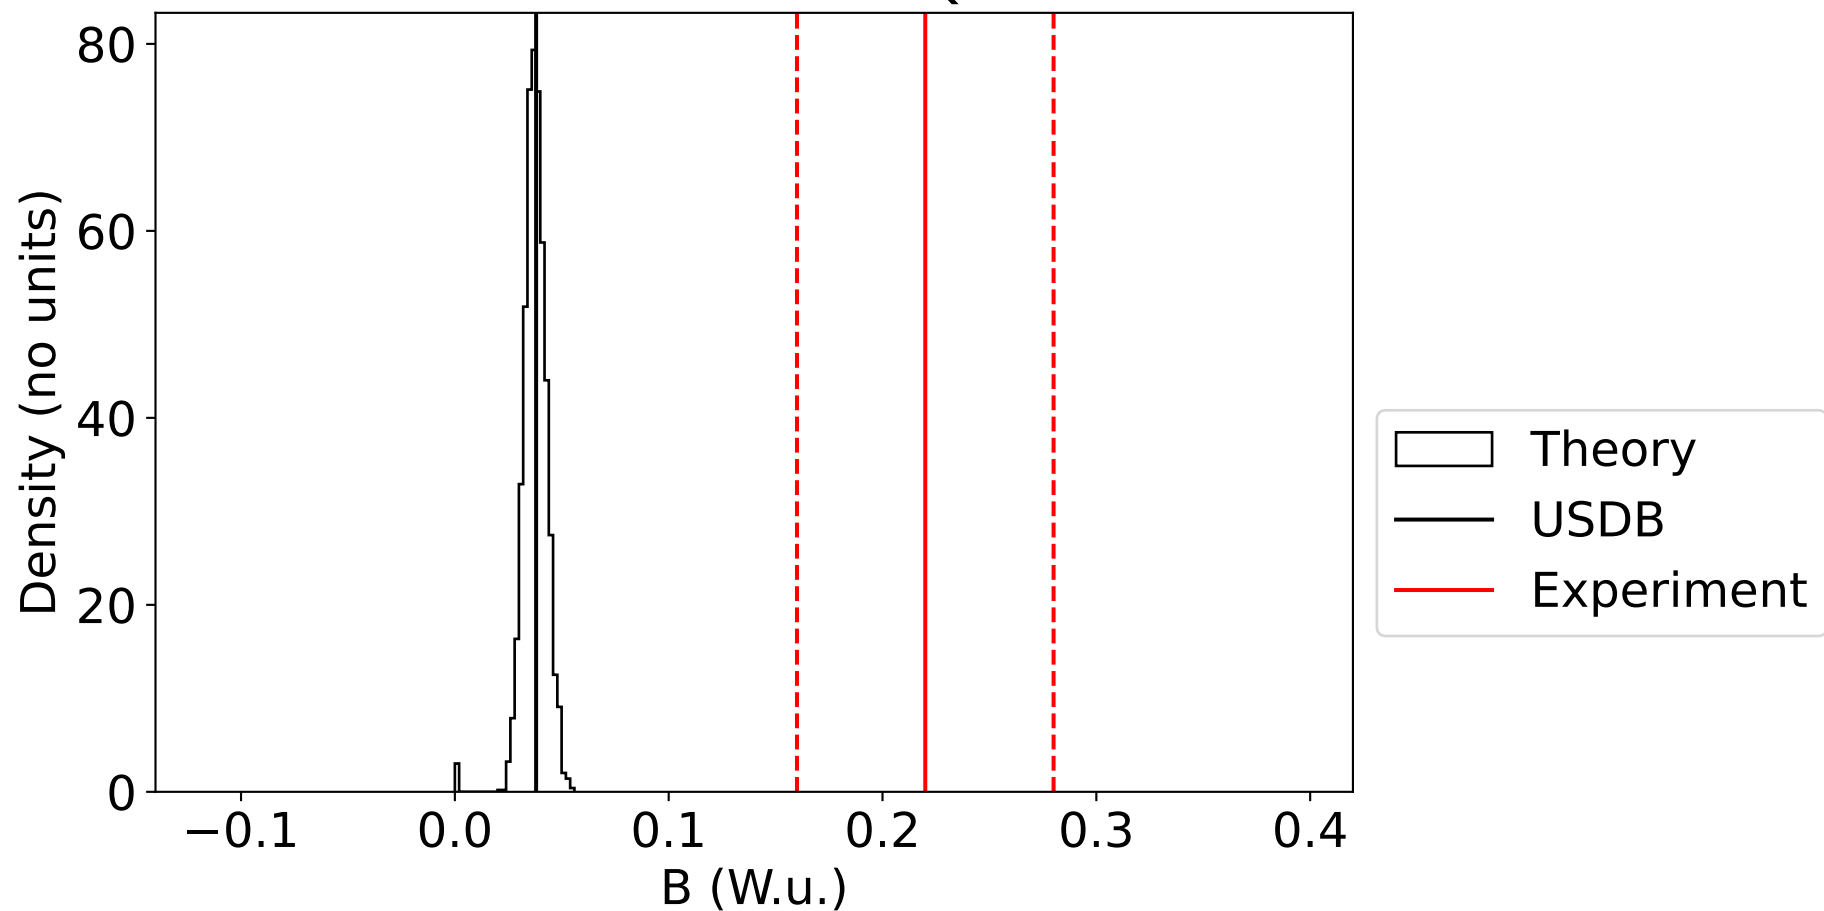

$^{19}\text{F} (9/2_2) \rightarrow (9/2_1)$   
Included in UQ

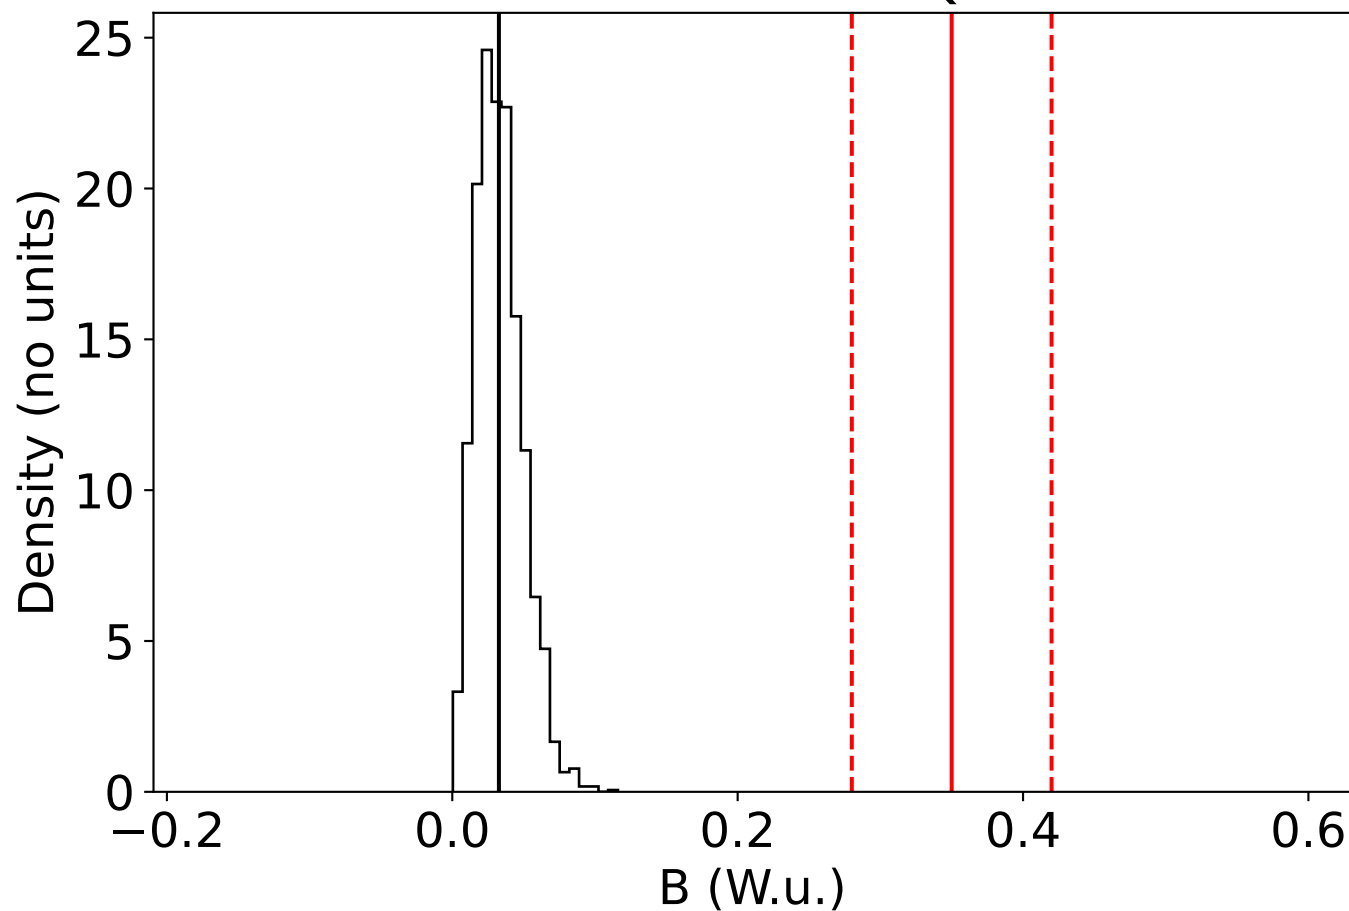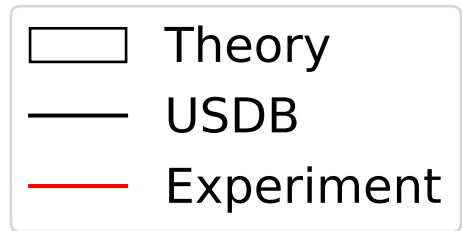



$^{19}\text{F} (9/2_2) \rightarrow (7/2_1)$   
Included in UQ

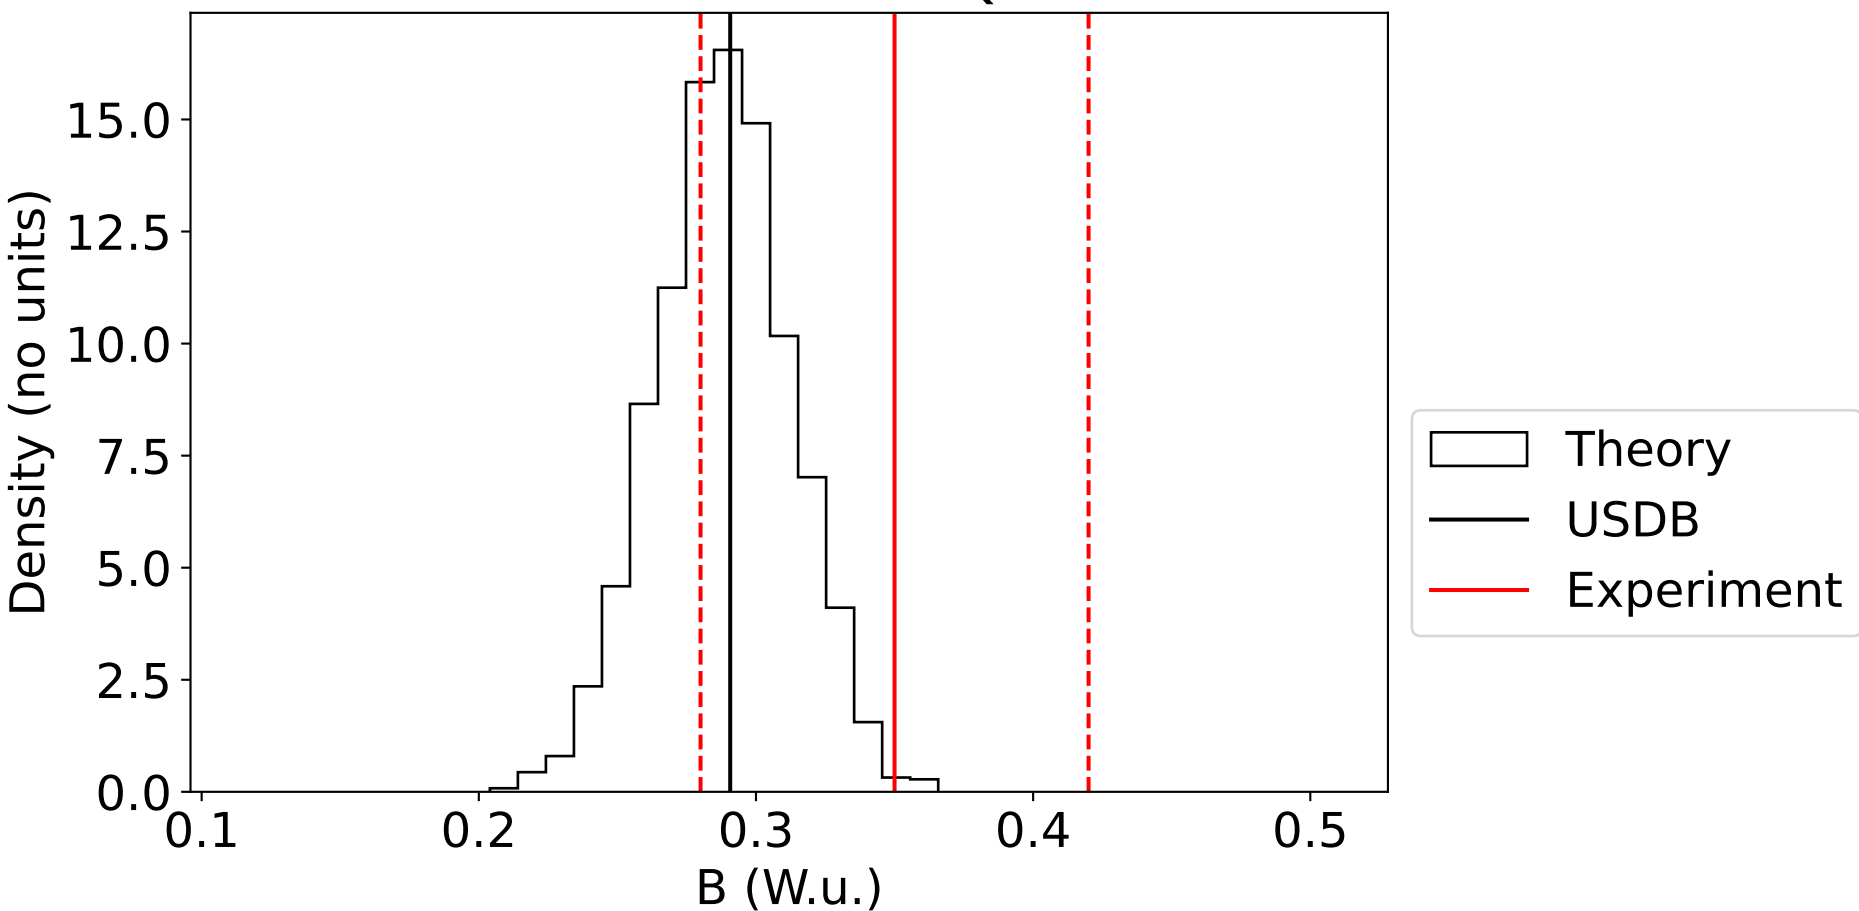

$^{20}\text{F} (3_1) \rightarrow (2_1)$   
Included in UQ

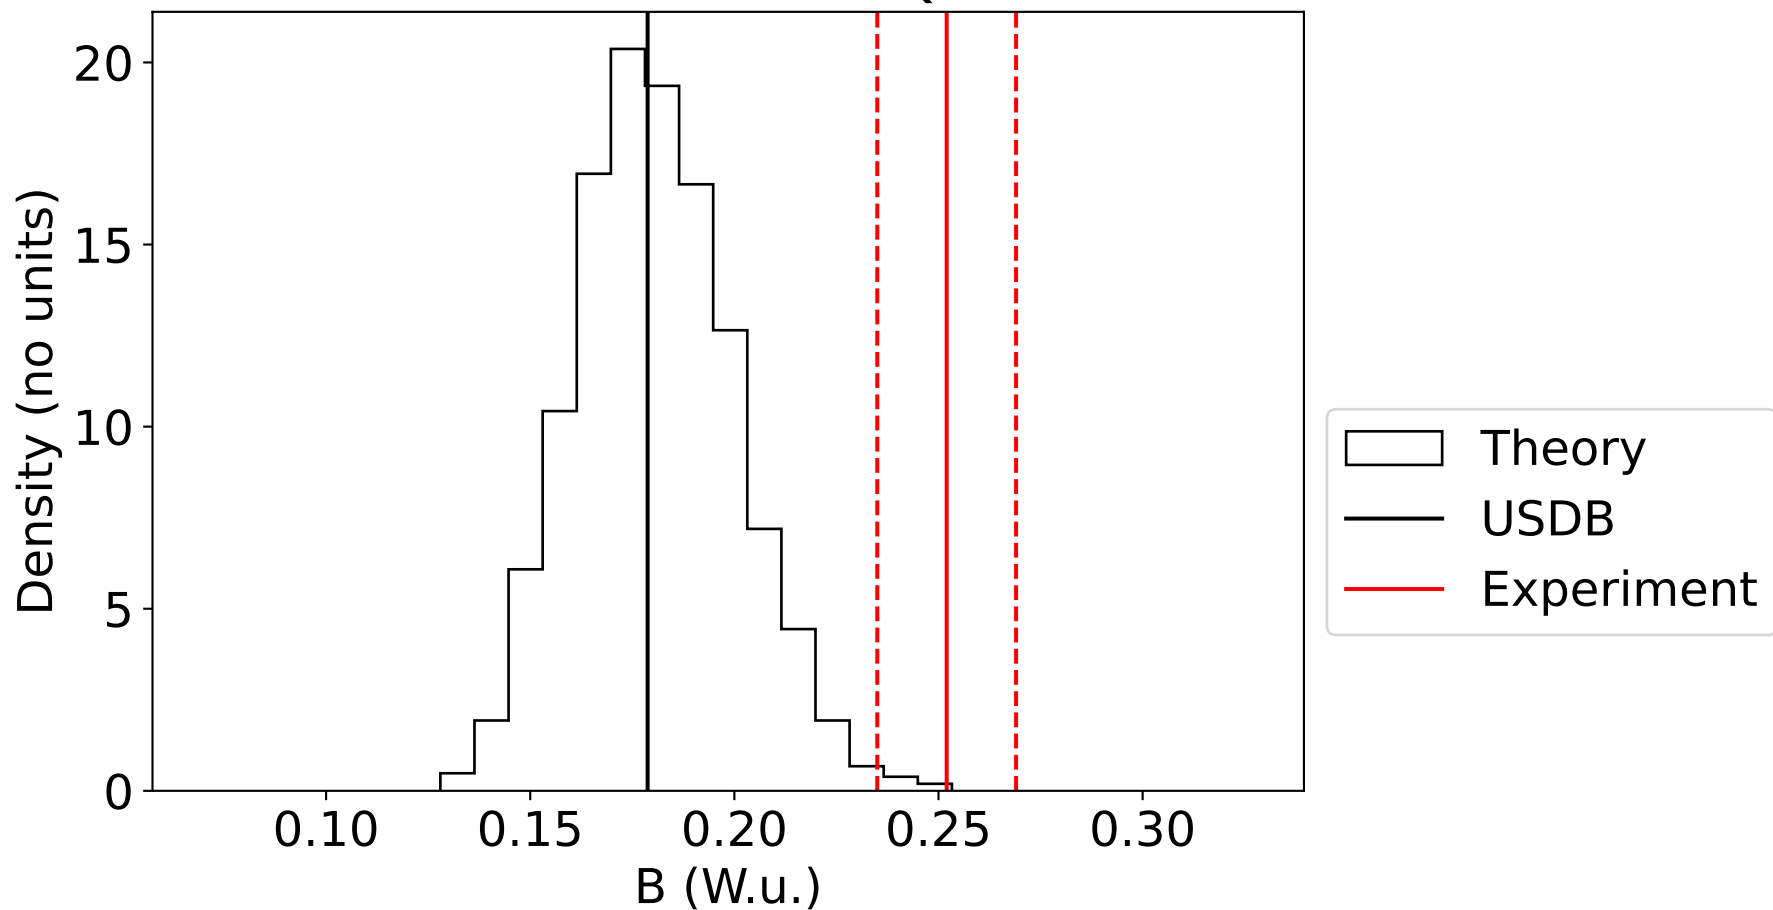

$^{20}\text{F} (4_1) \rightarrow (3_1)$   
Included in UQ

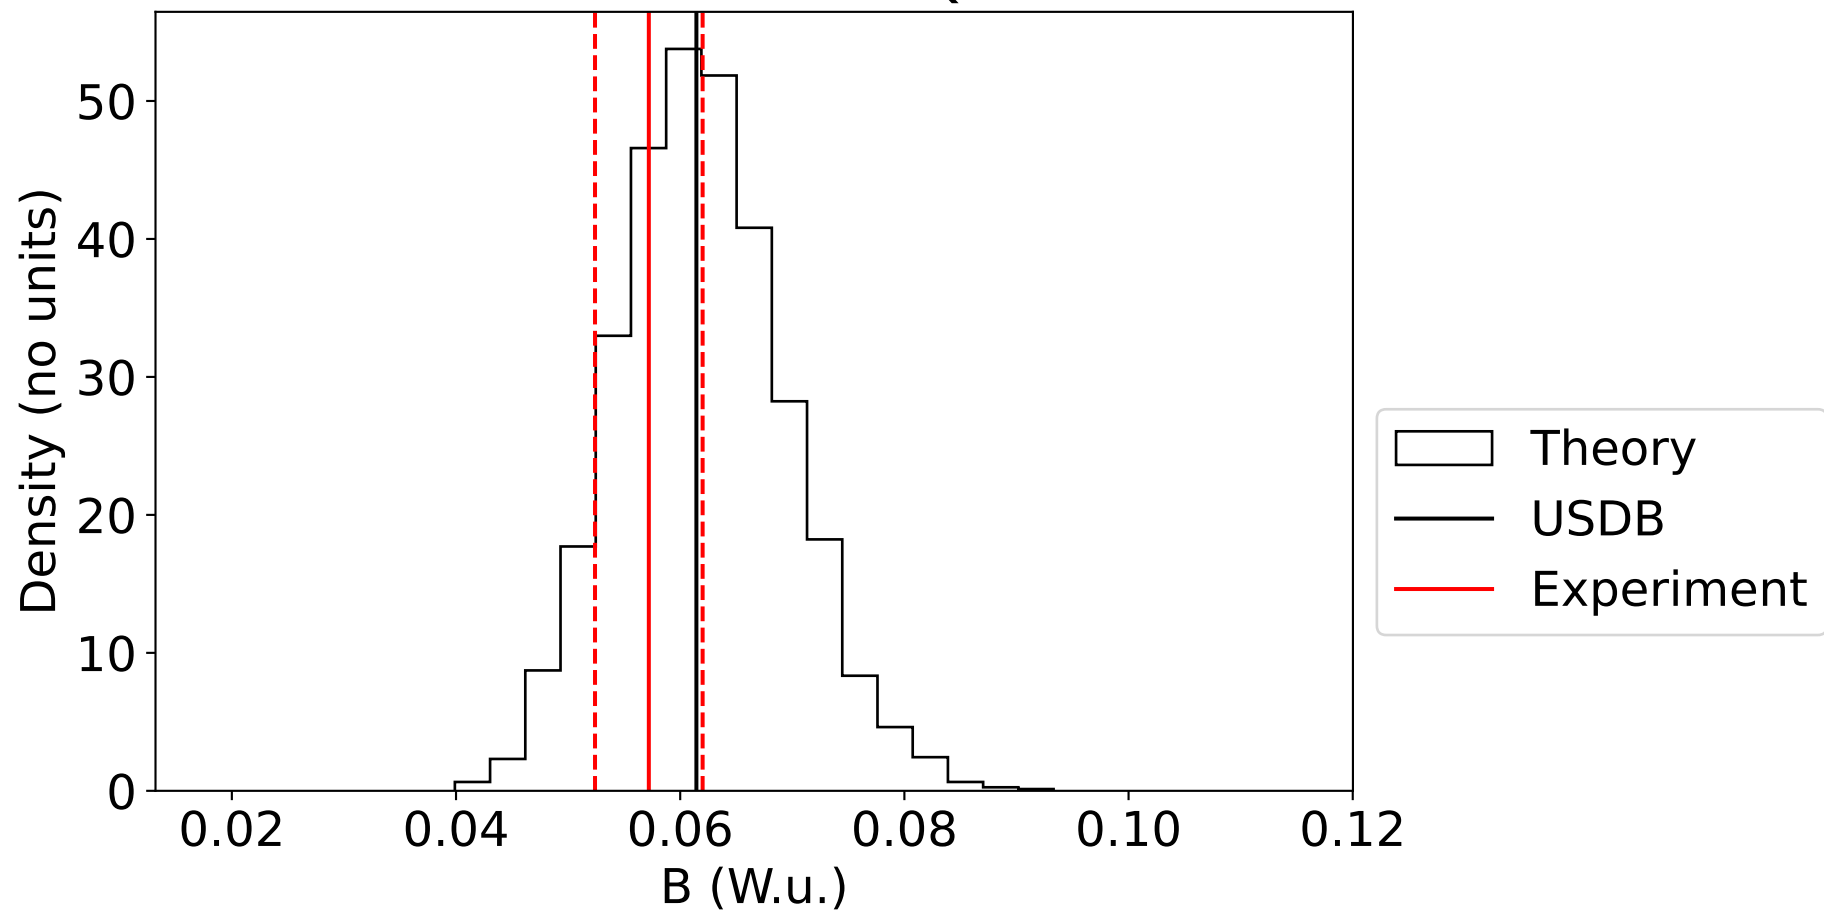

$^{20}\text{F} (1_1) \rightarrow (2_1)$   
Included in UQ

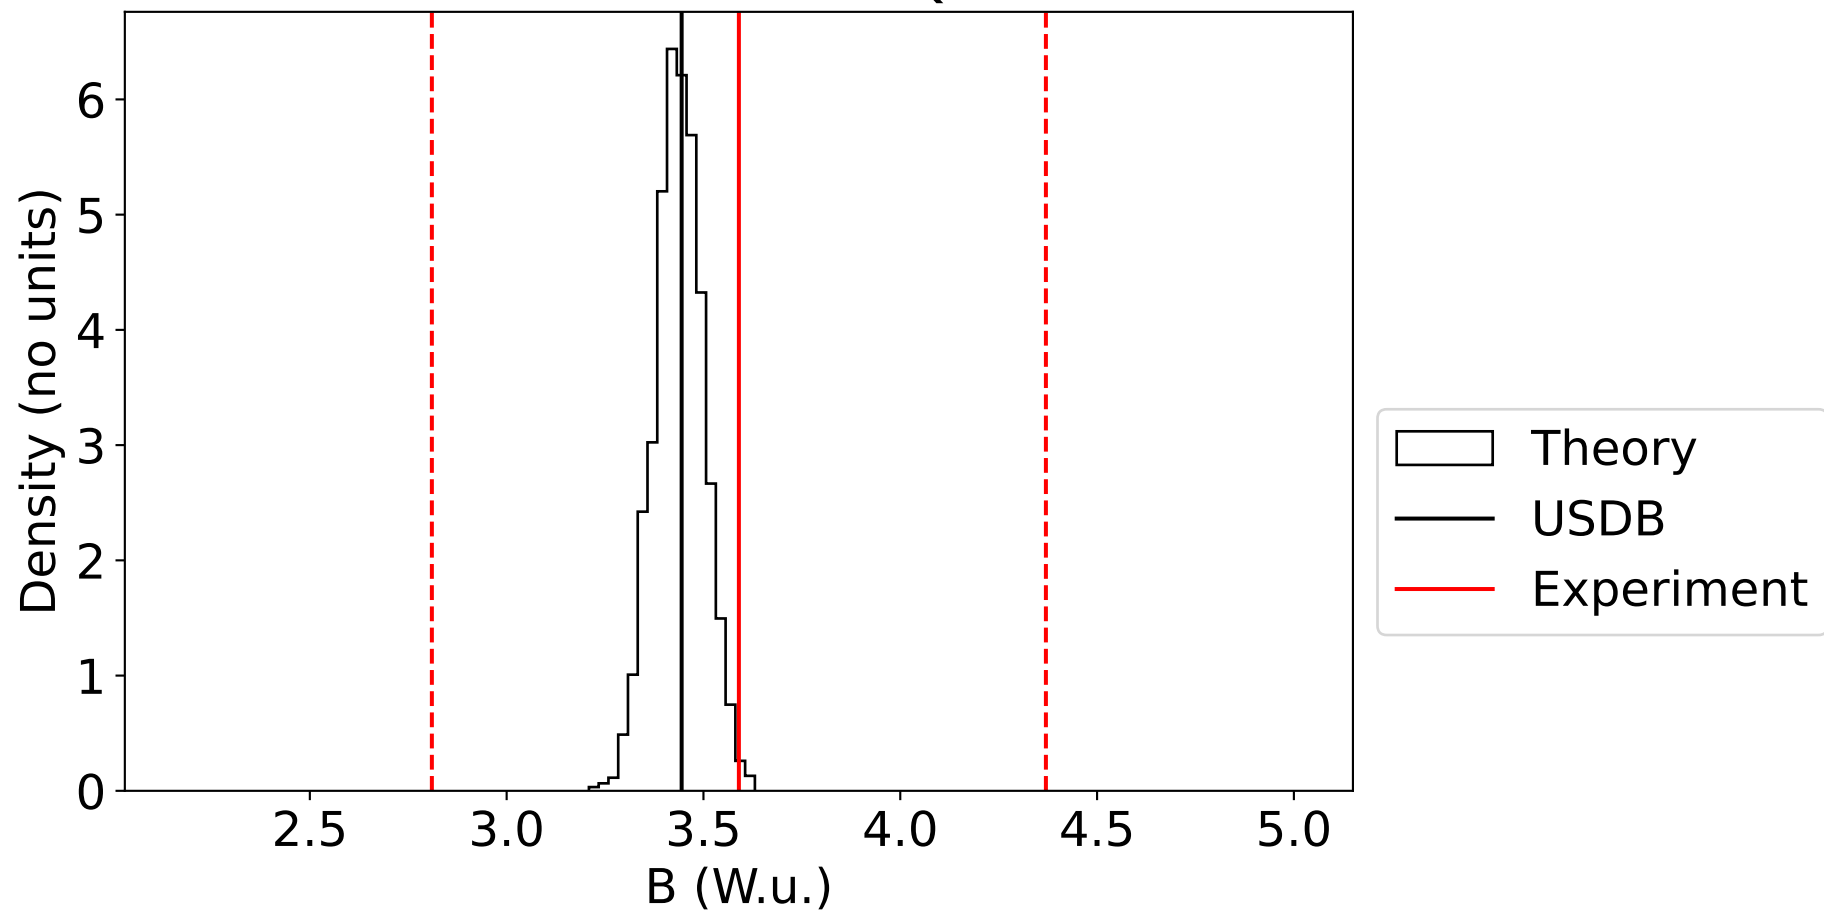

$^{20}\text{F} (2_2) \rightarrow (2_1)$   
Included in UQ

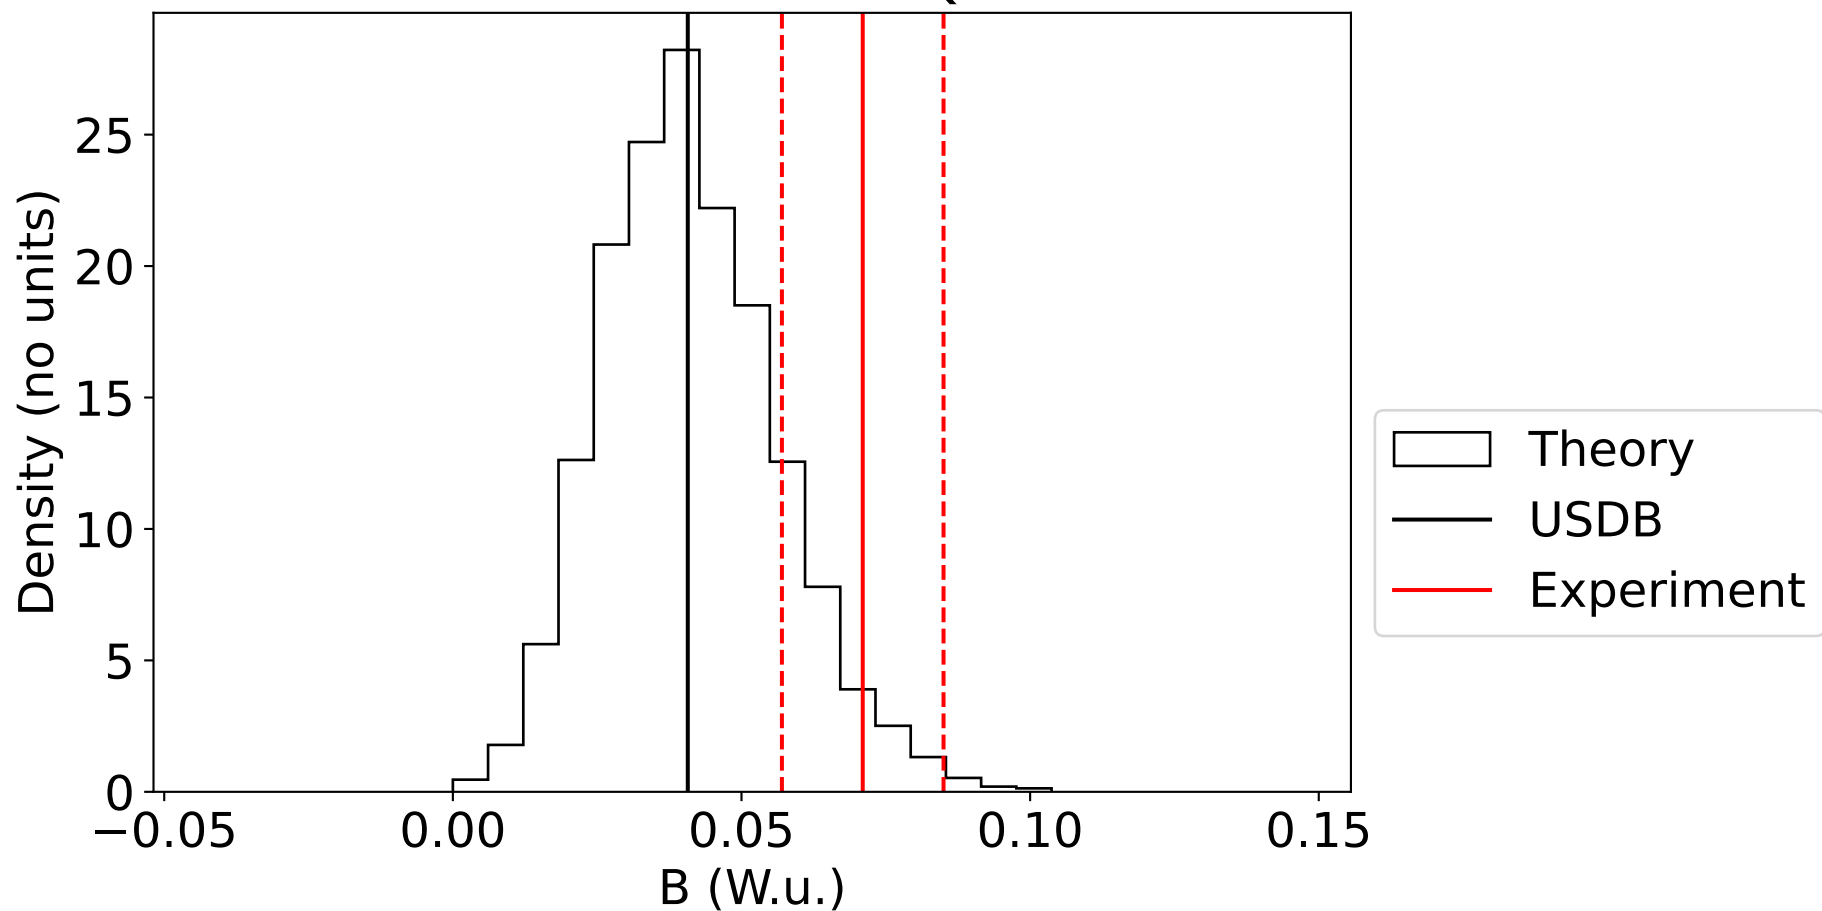

$^{20}\text{F} (2_2) \rightarrow (3_1)$   
Included in UQ

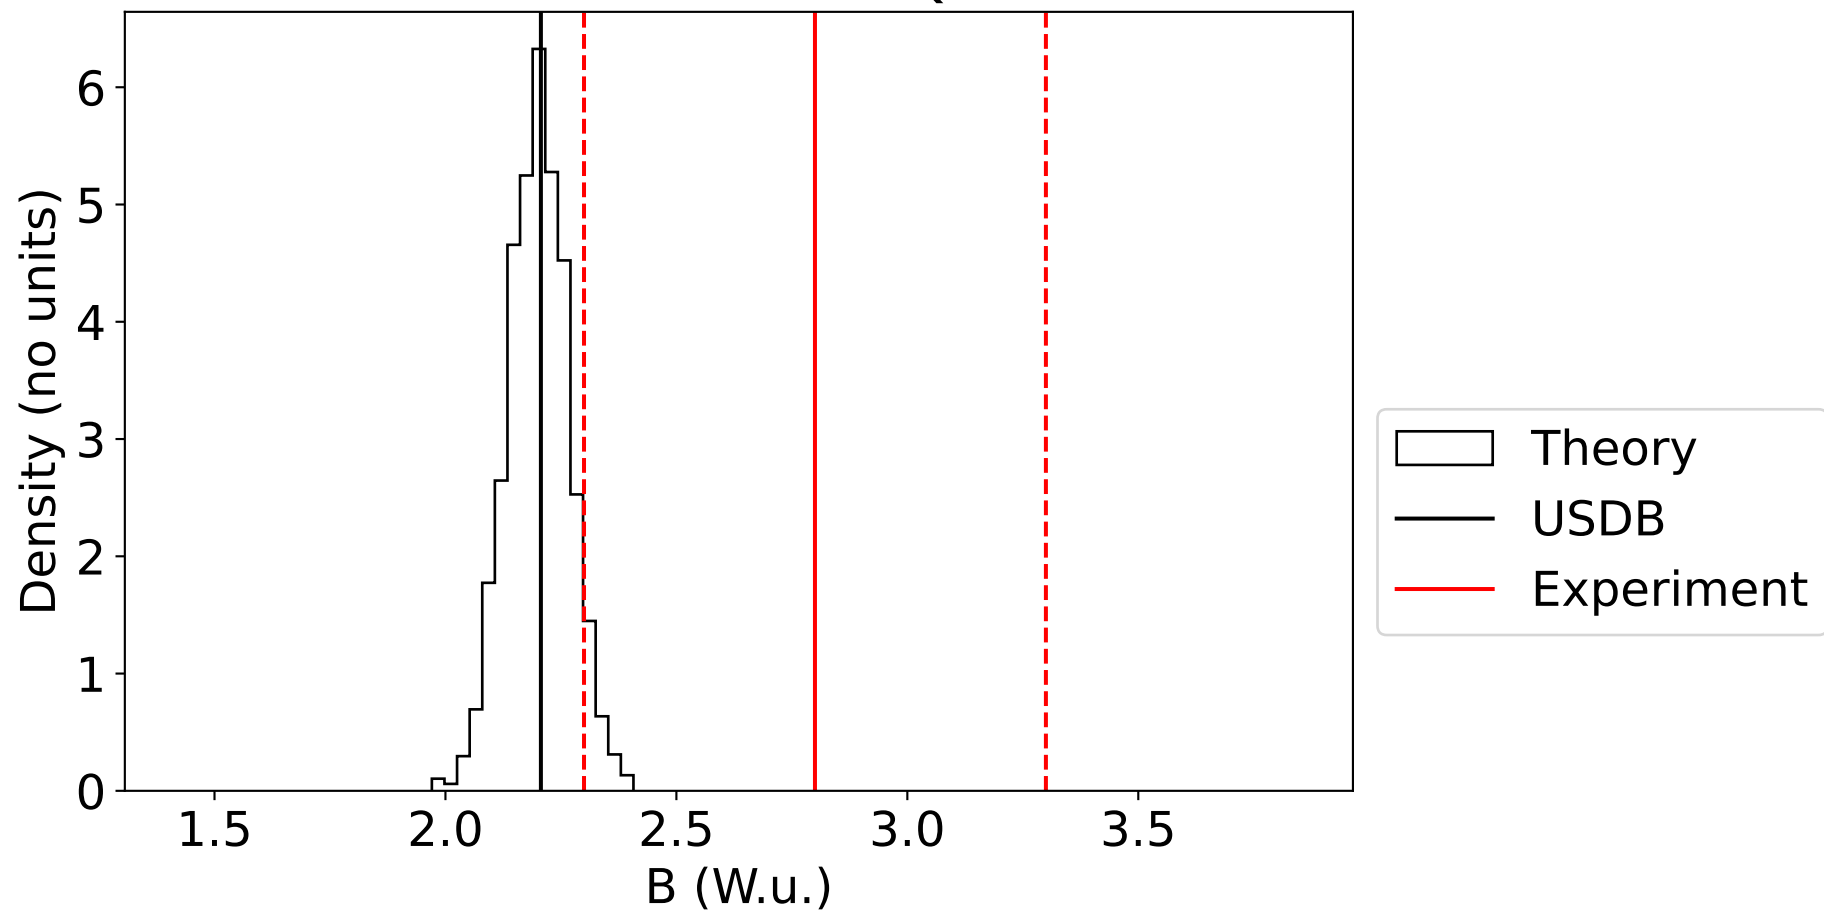

$^{20}\text{F} (3_2) \rightarrow (4_1)$   
Included in UQ

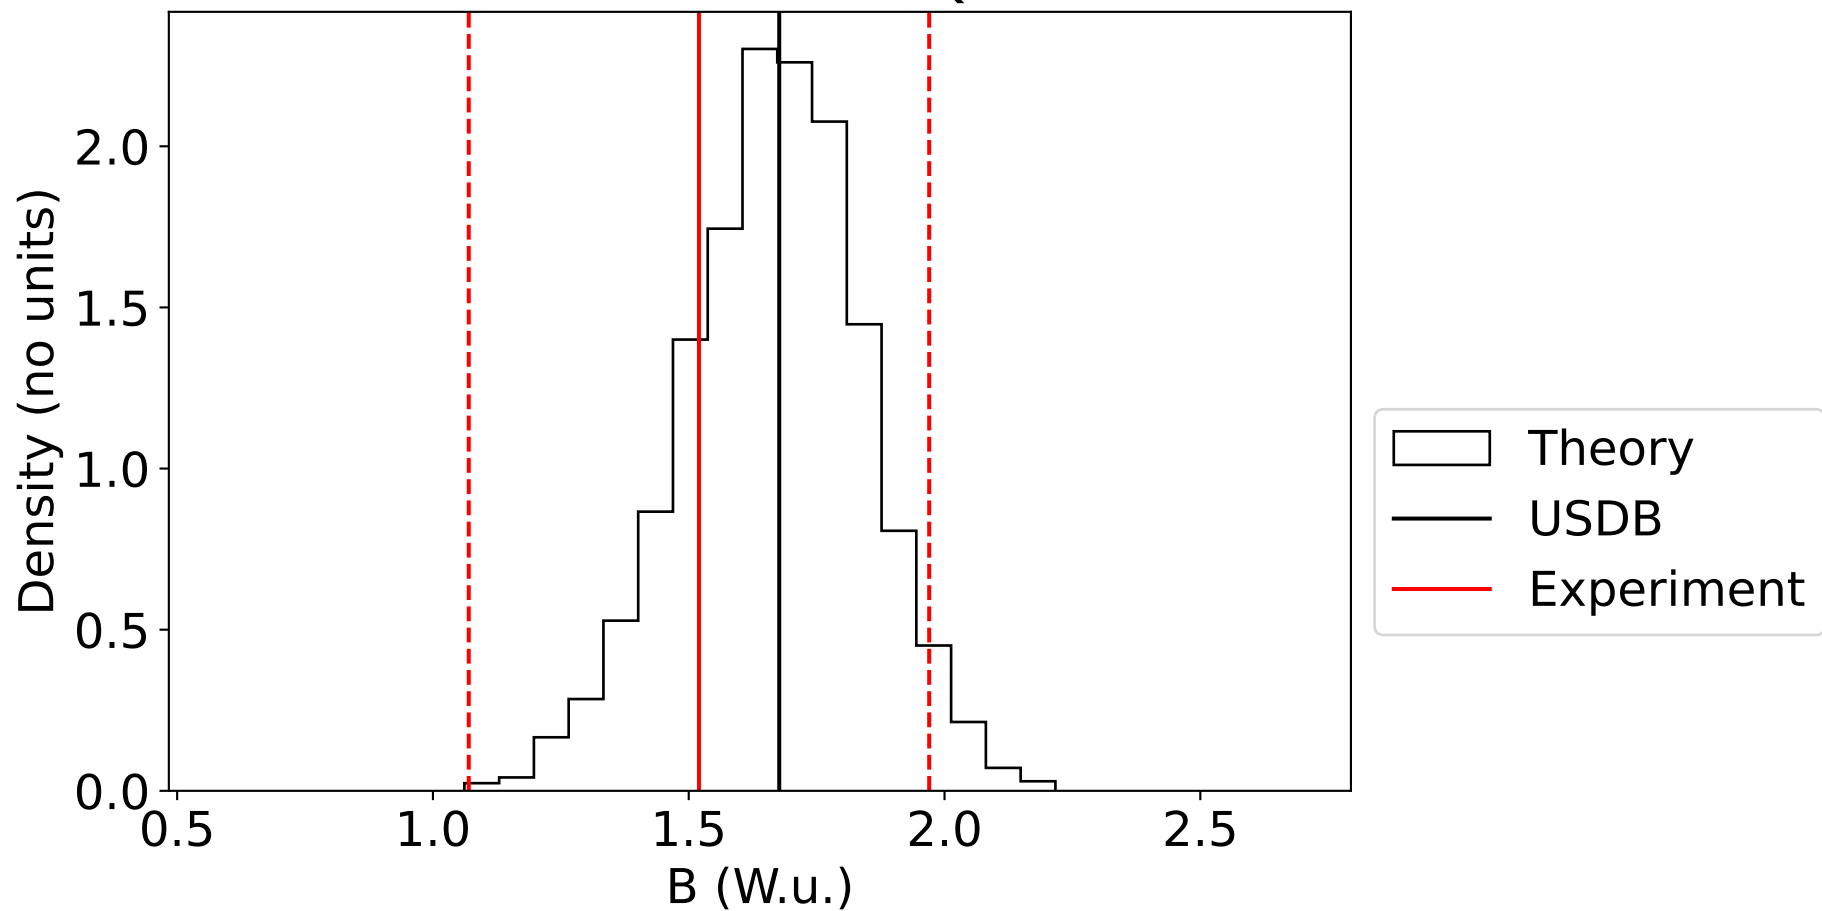

$^{20}\text{F} (3_2) \rightarrow (2_1)$   
Included in UQ

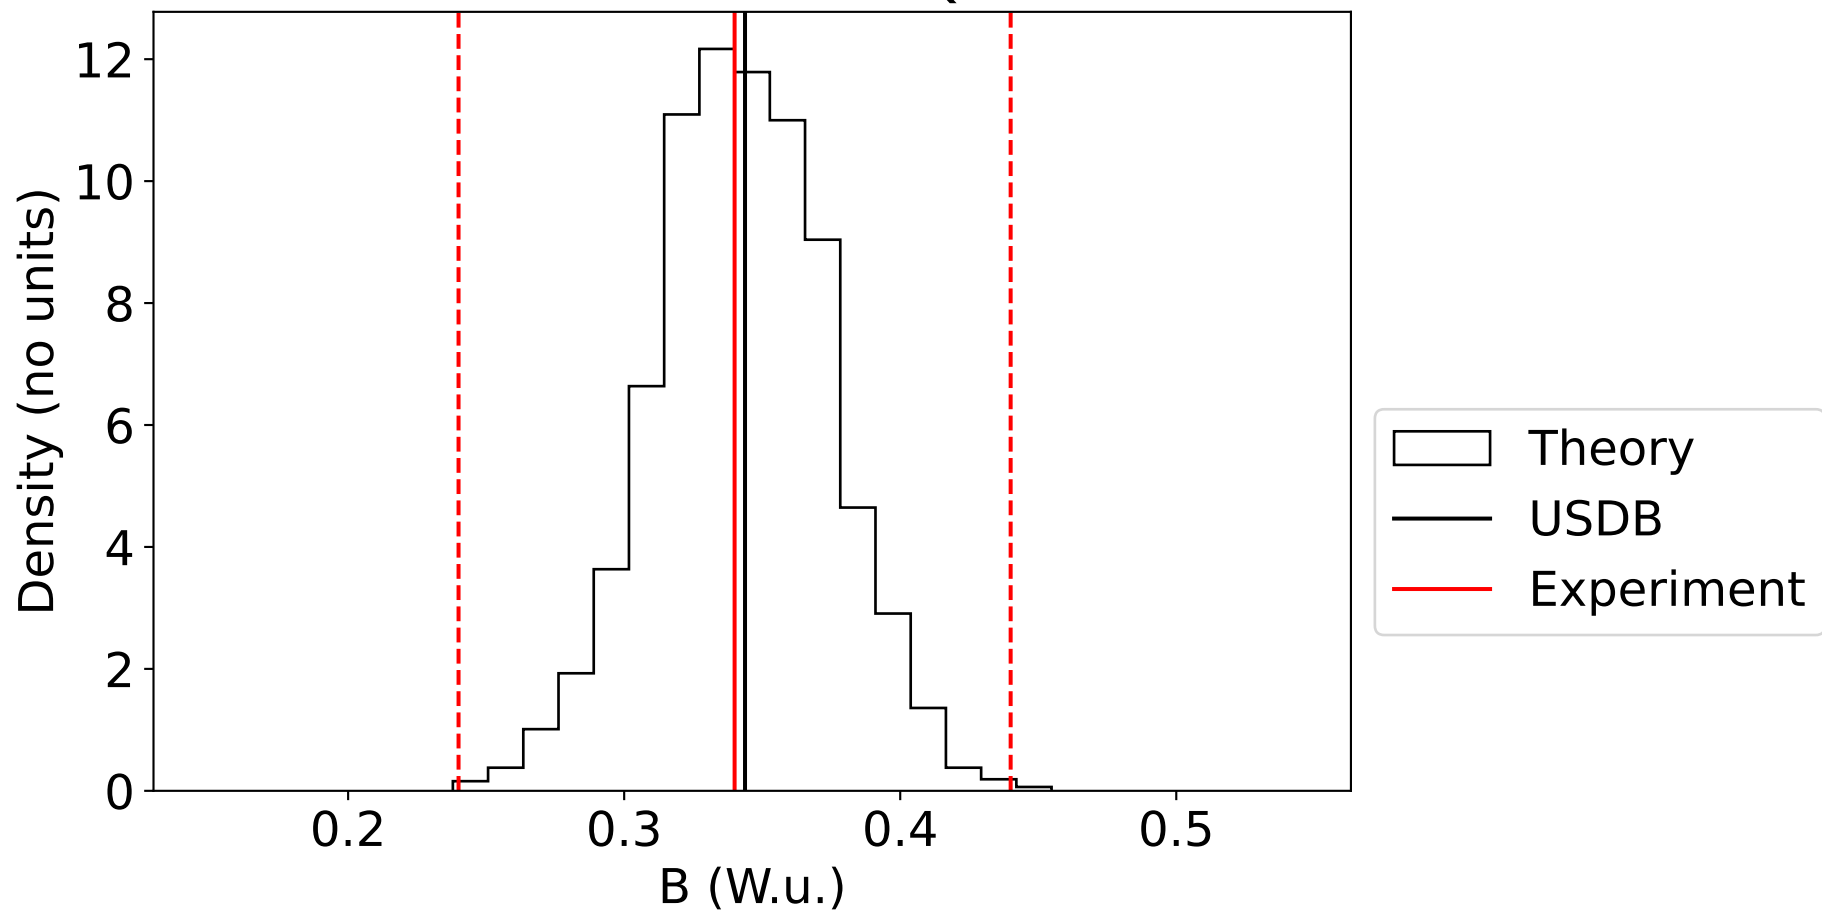



$^{20}\text{F} (3_3) \rightarrow (3_1)$   
Included in UQ

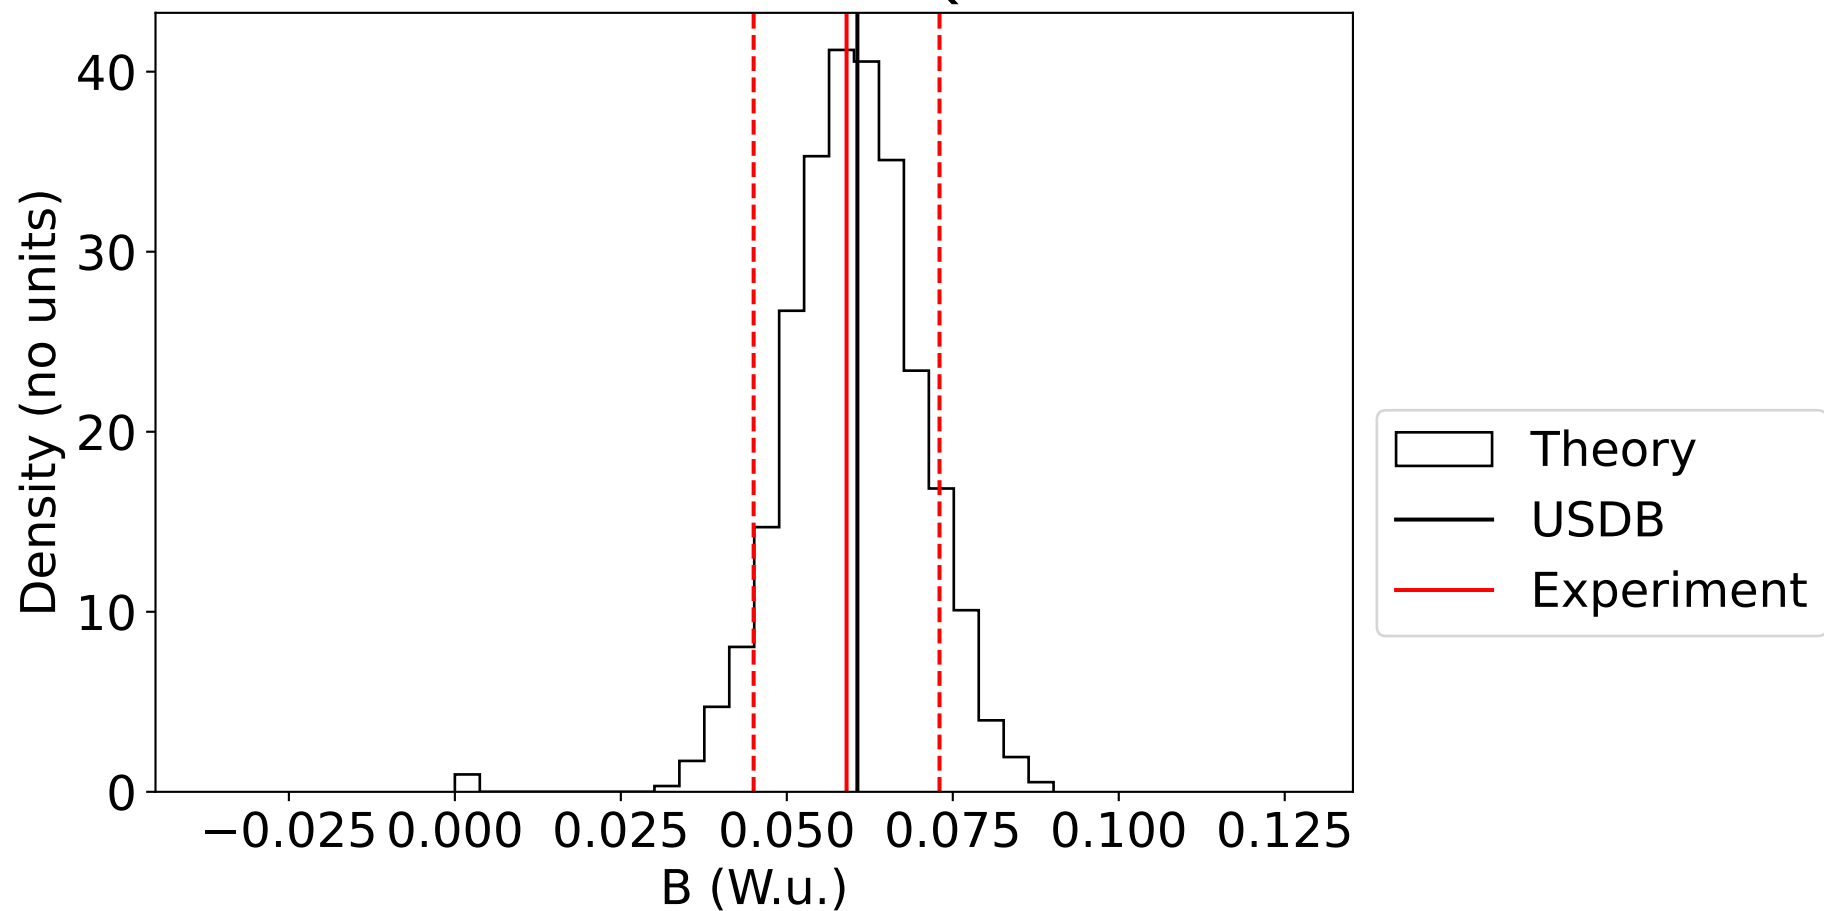

$^{20}\text{F} (3_3) \rightarrow (4_1)$   
Included in UQ

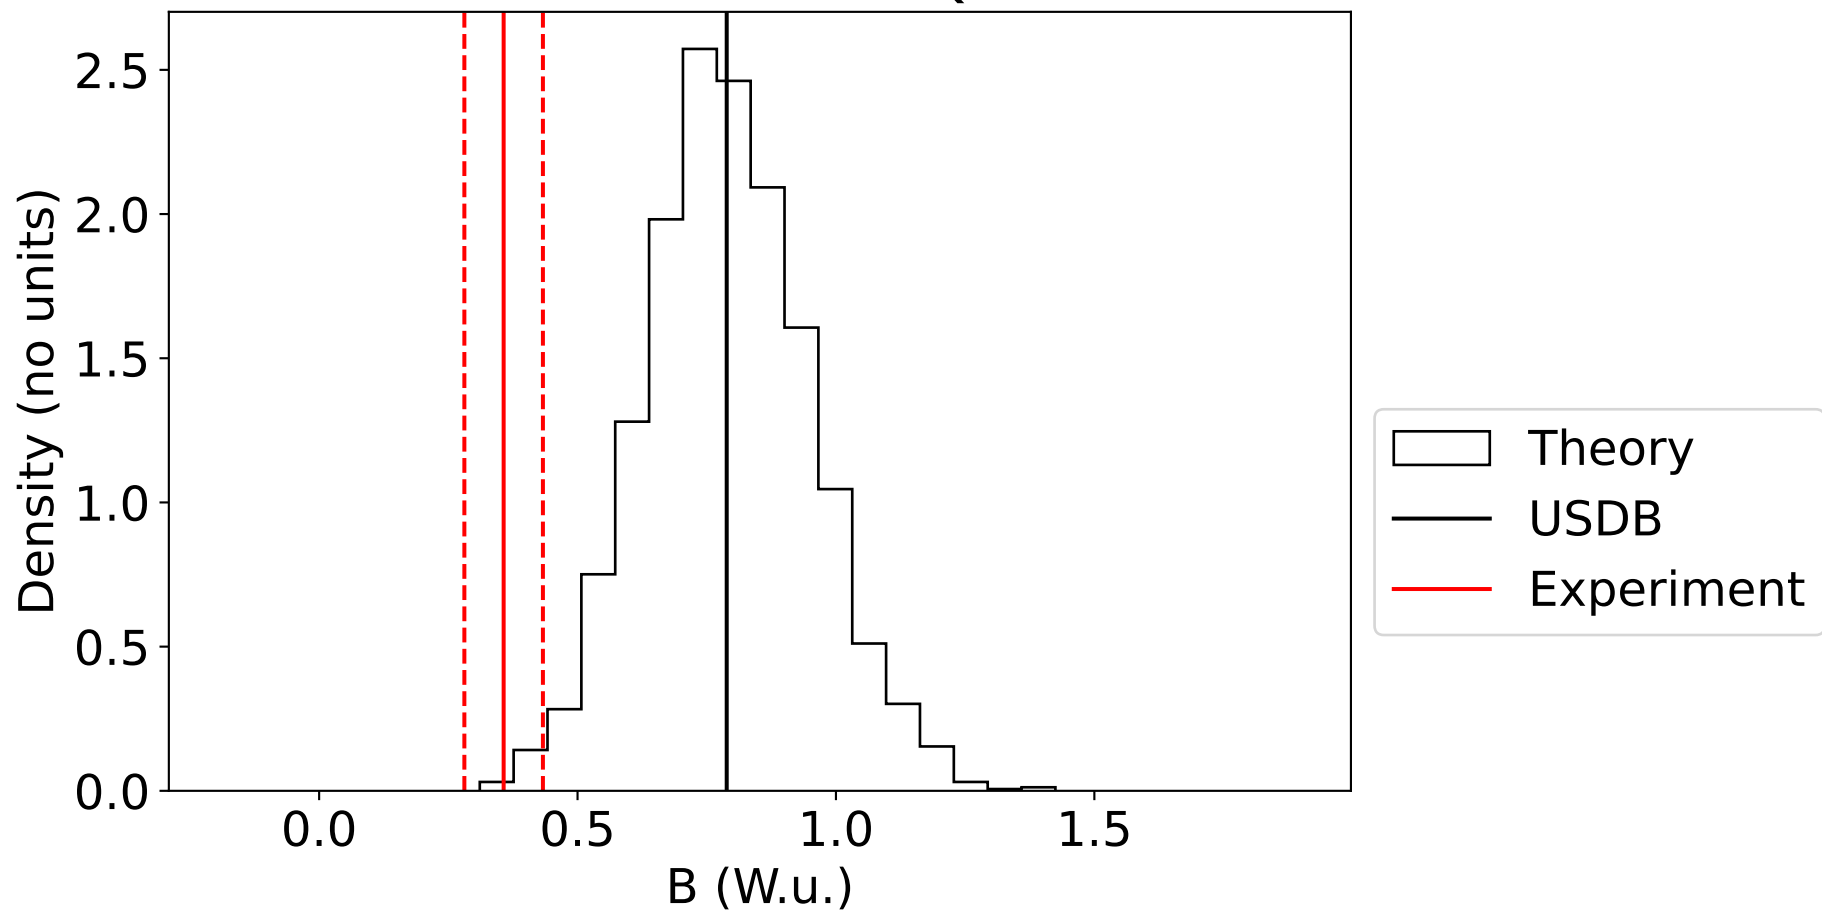

$^{20}\text{F} (3_3) \rightarrow (3_2)$   
Included in UQ

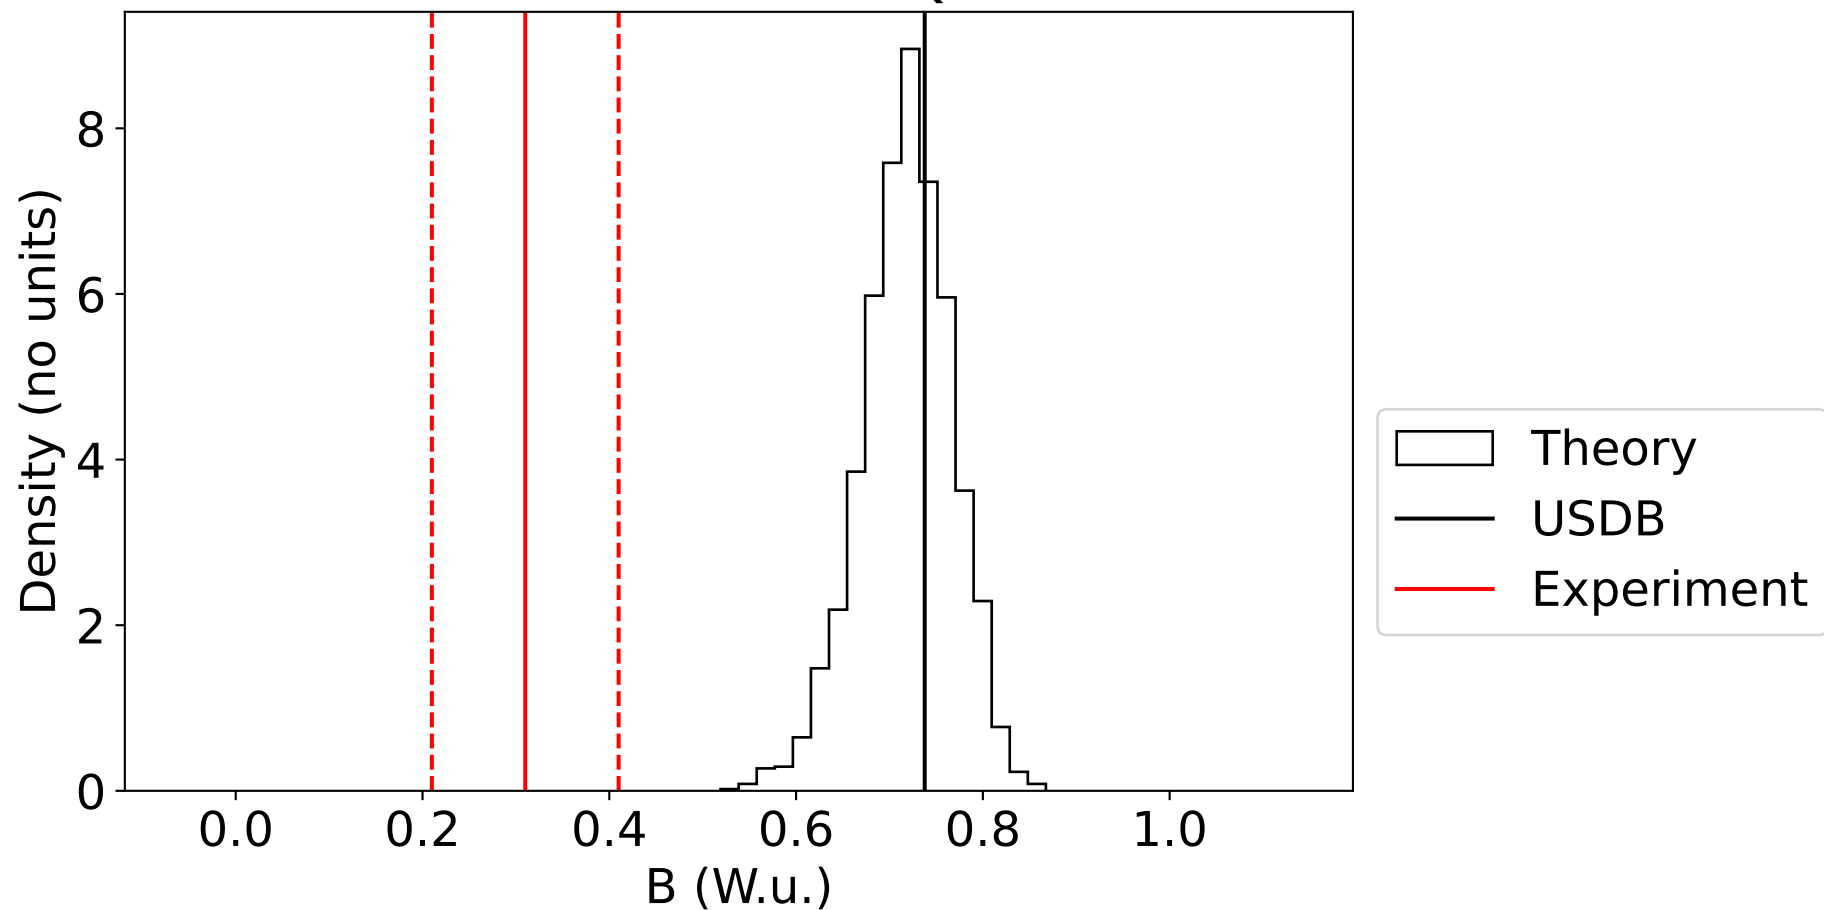

$^{20}\text{F} (3_3) \rightarrow (2_1)$   
Included in UQ

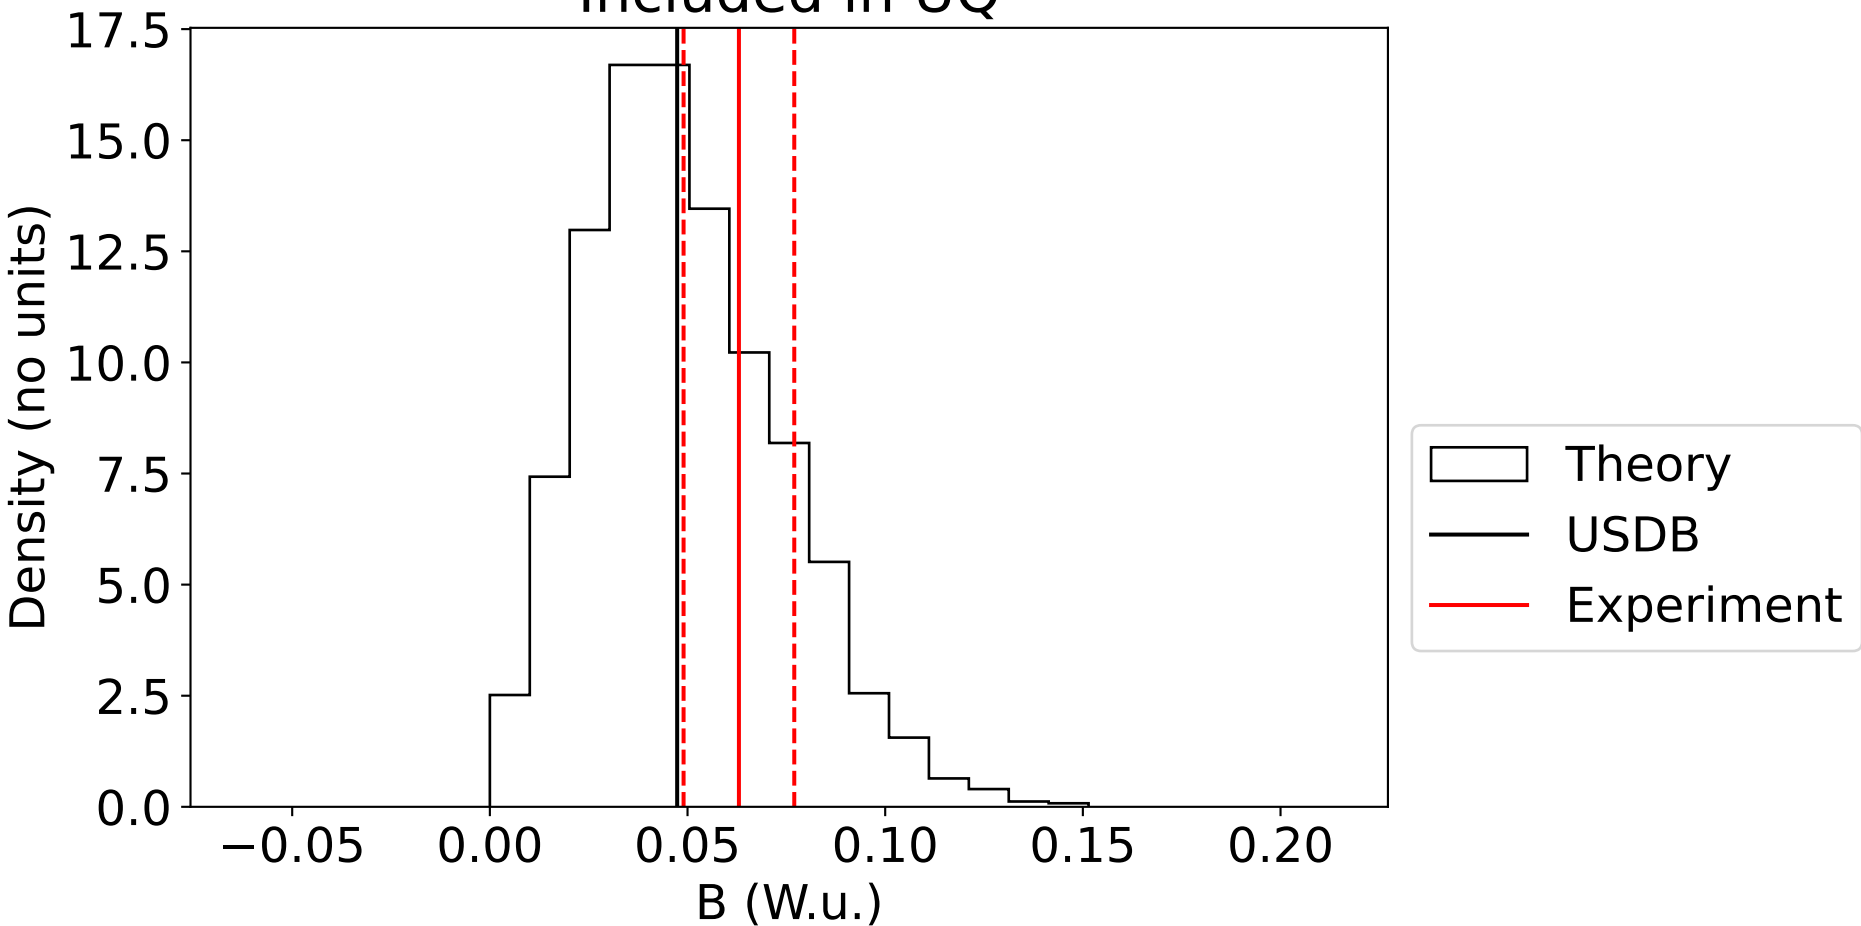

$^{20}\text{F} (1_3) \rightarrow (2_1)$   
Included in UQ

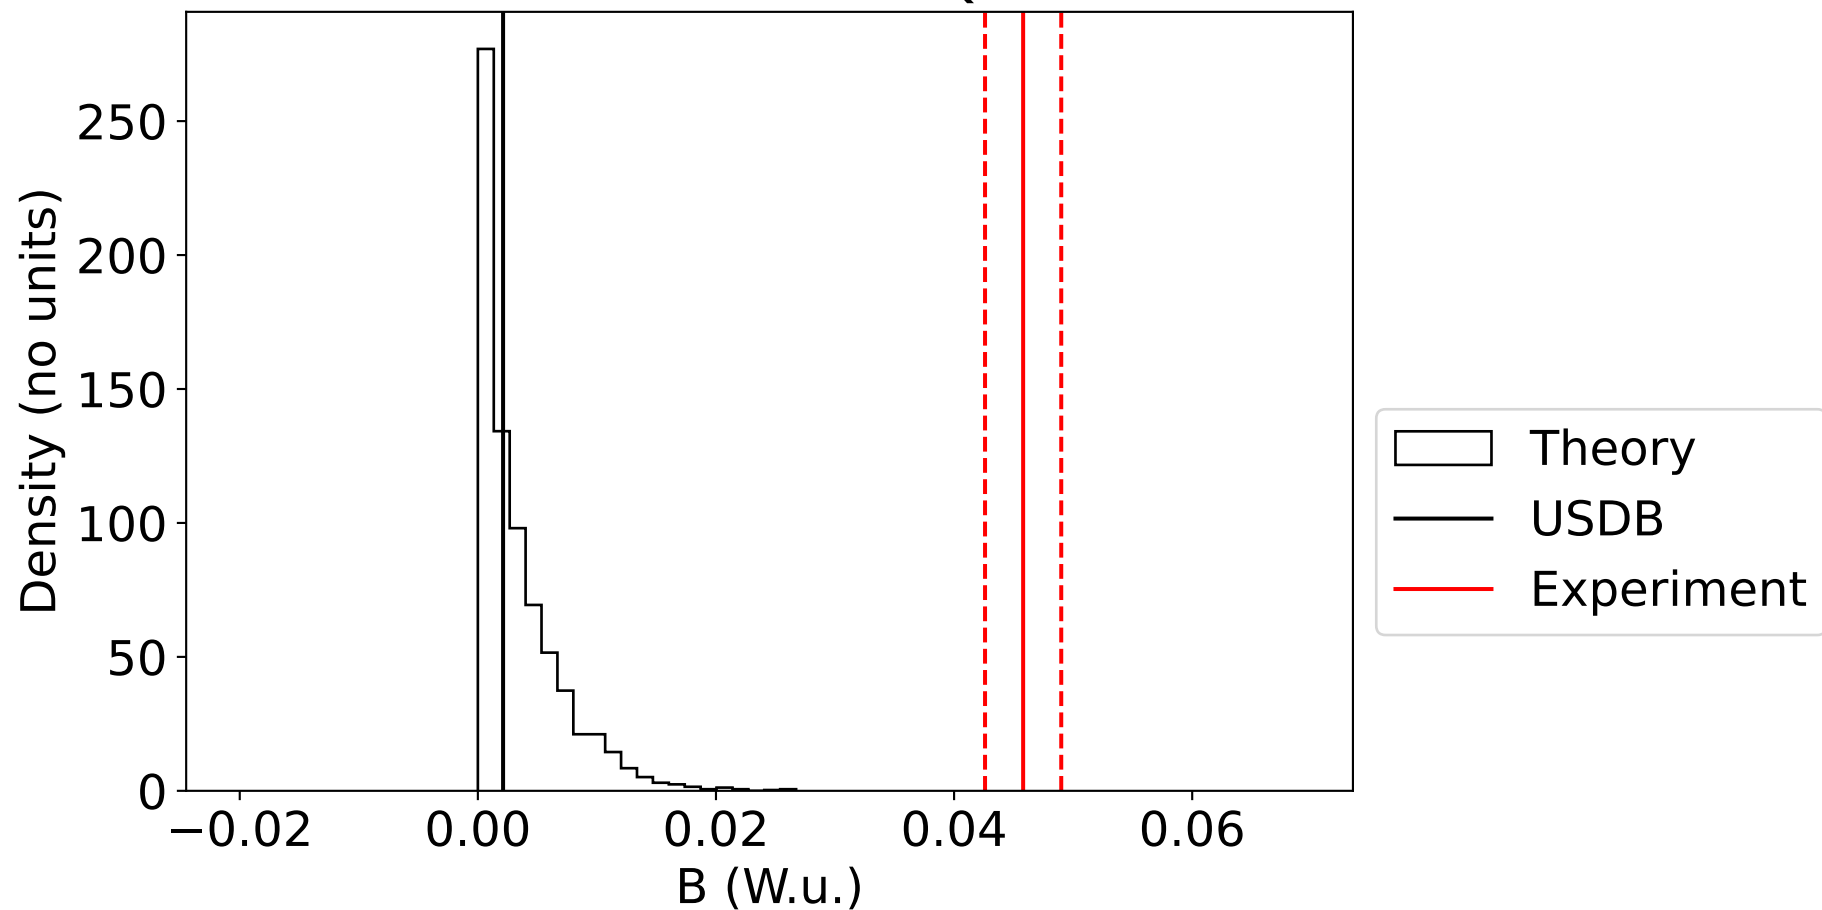

$^{20}\text{F} (1_3) \rightarrow (1_1)$   
Included in UQ

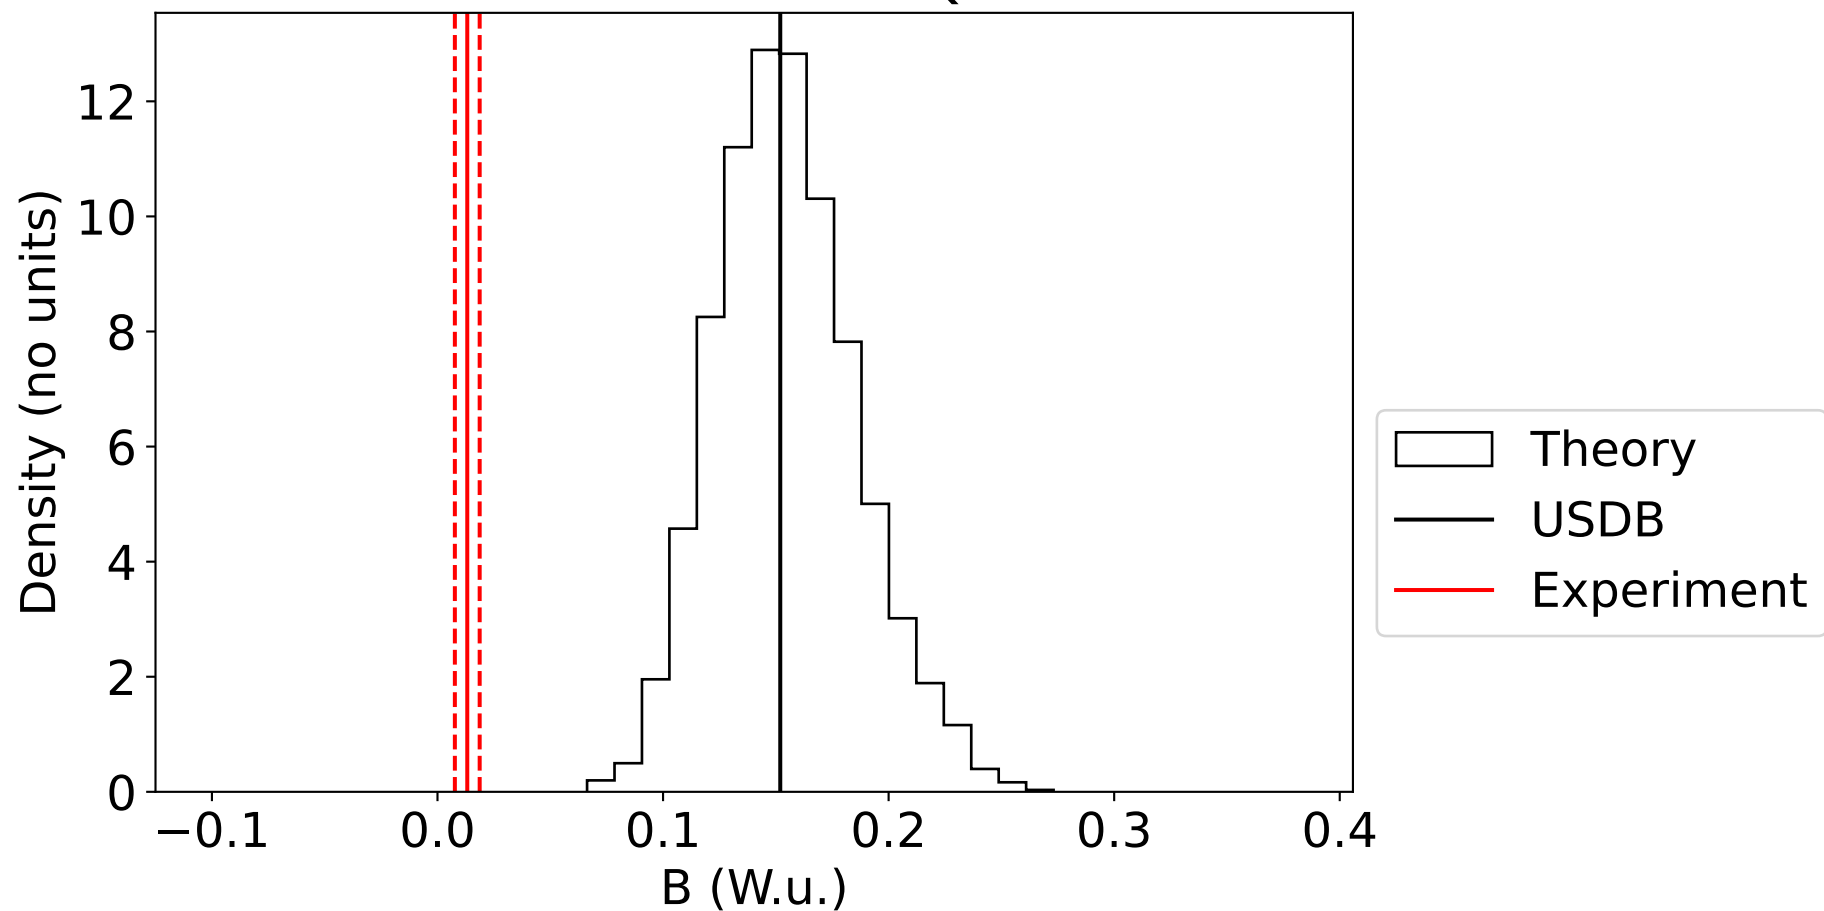

$^{20}\text{F} (0_1) \rightarrow (1_1)$   
Included in UQ

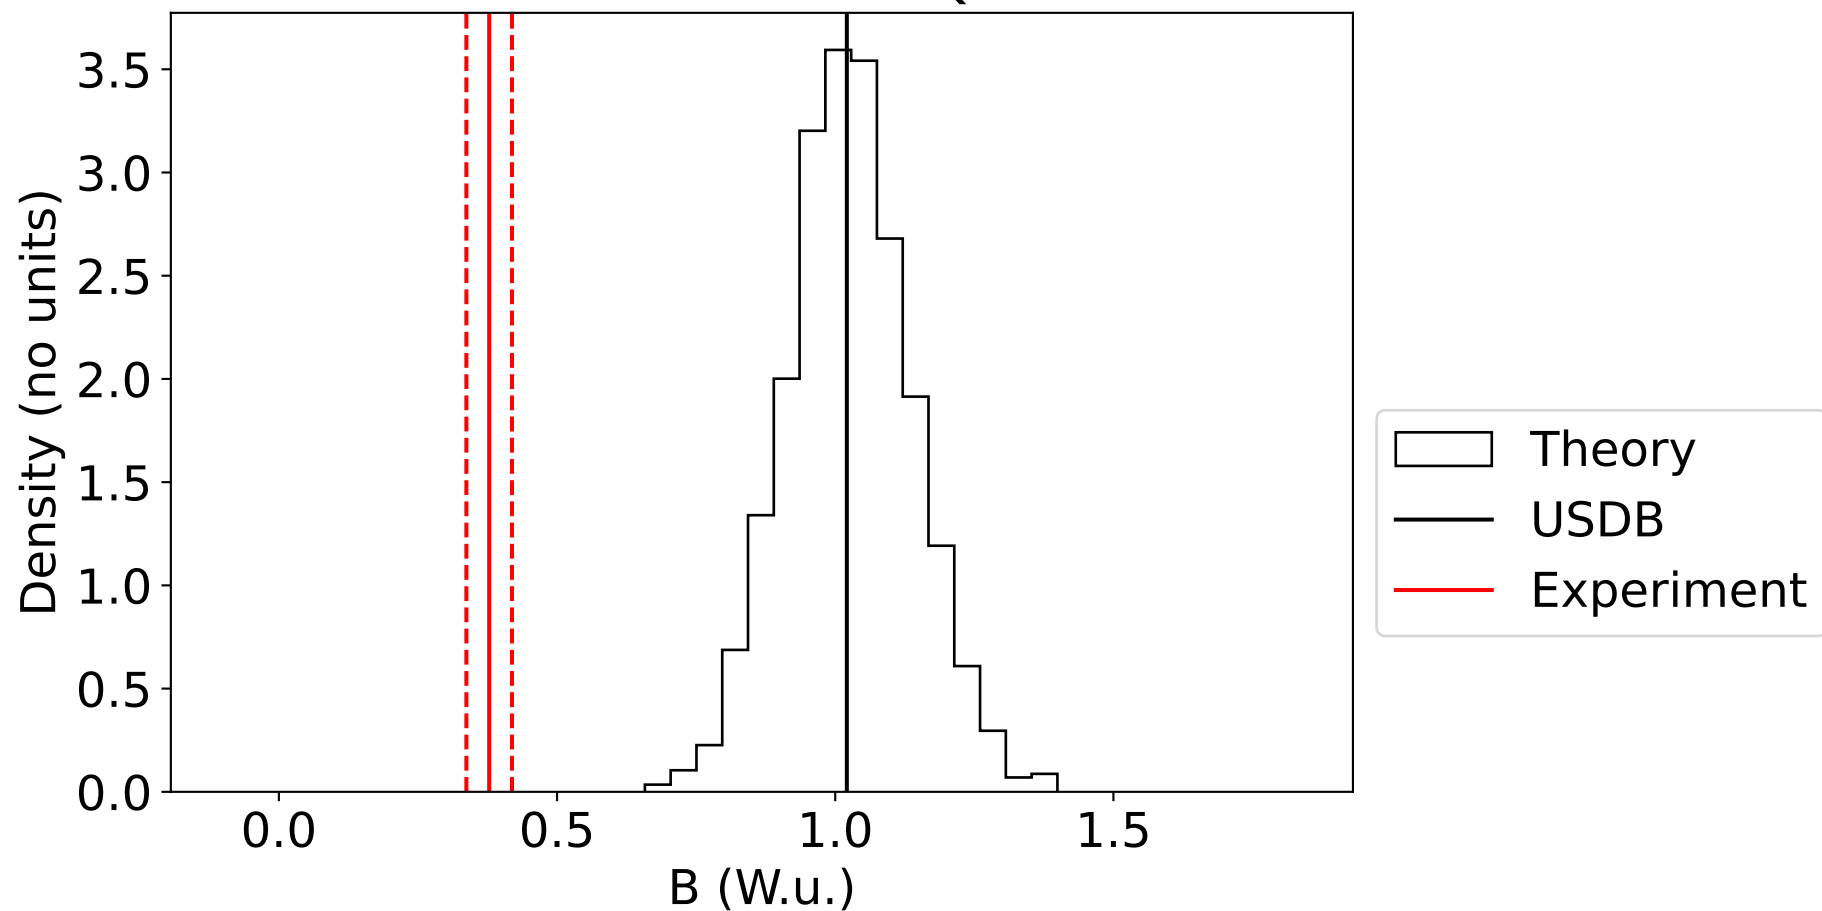

$^{21}\text{F} (3/2_1) \rightarrow (1/2_1)$   
Included in UQ

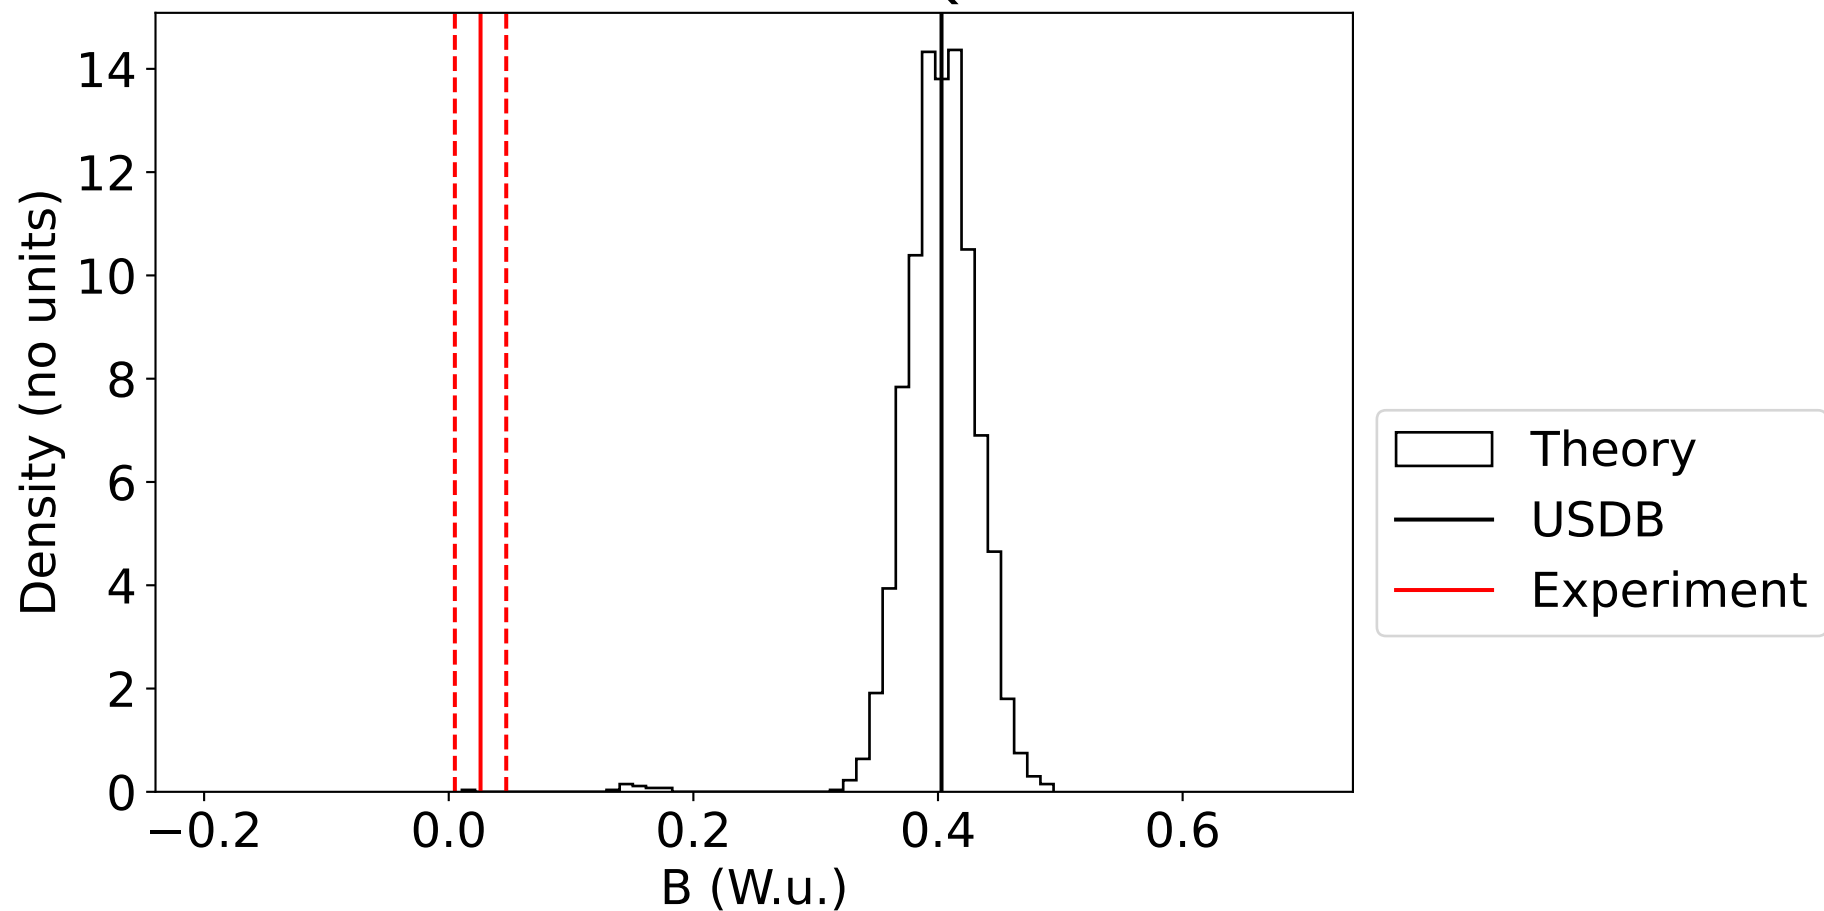



$^{21}\text{F} (3/2_1) \rightarrow (5/2_1)$   
Included in UQ

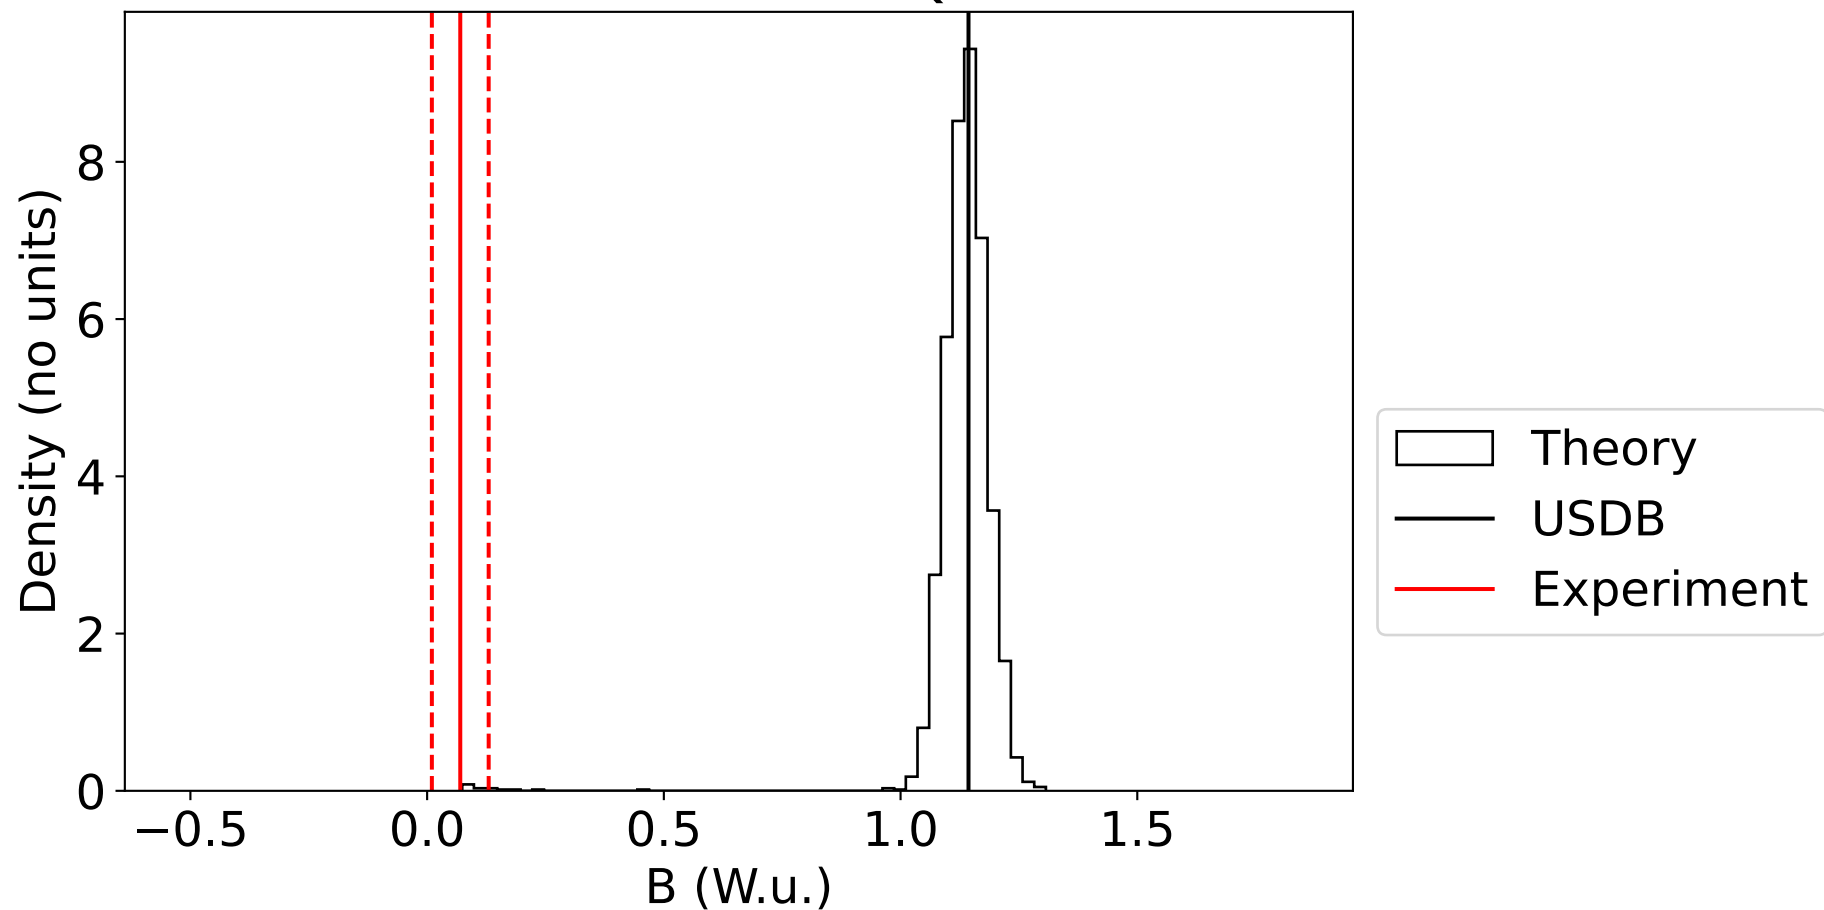

$^{22}\text{F} (2_2) \rightarrow (3_1)$   
Included in UQ

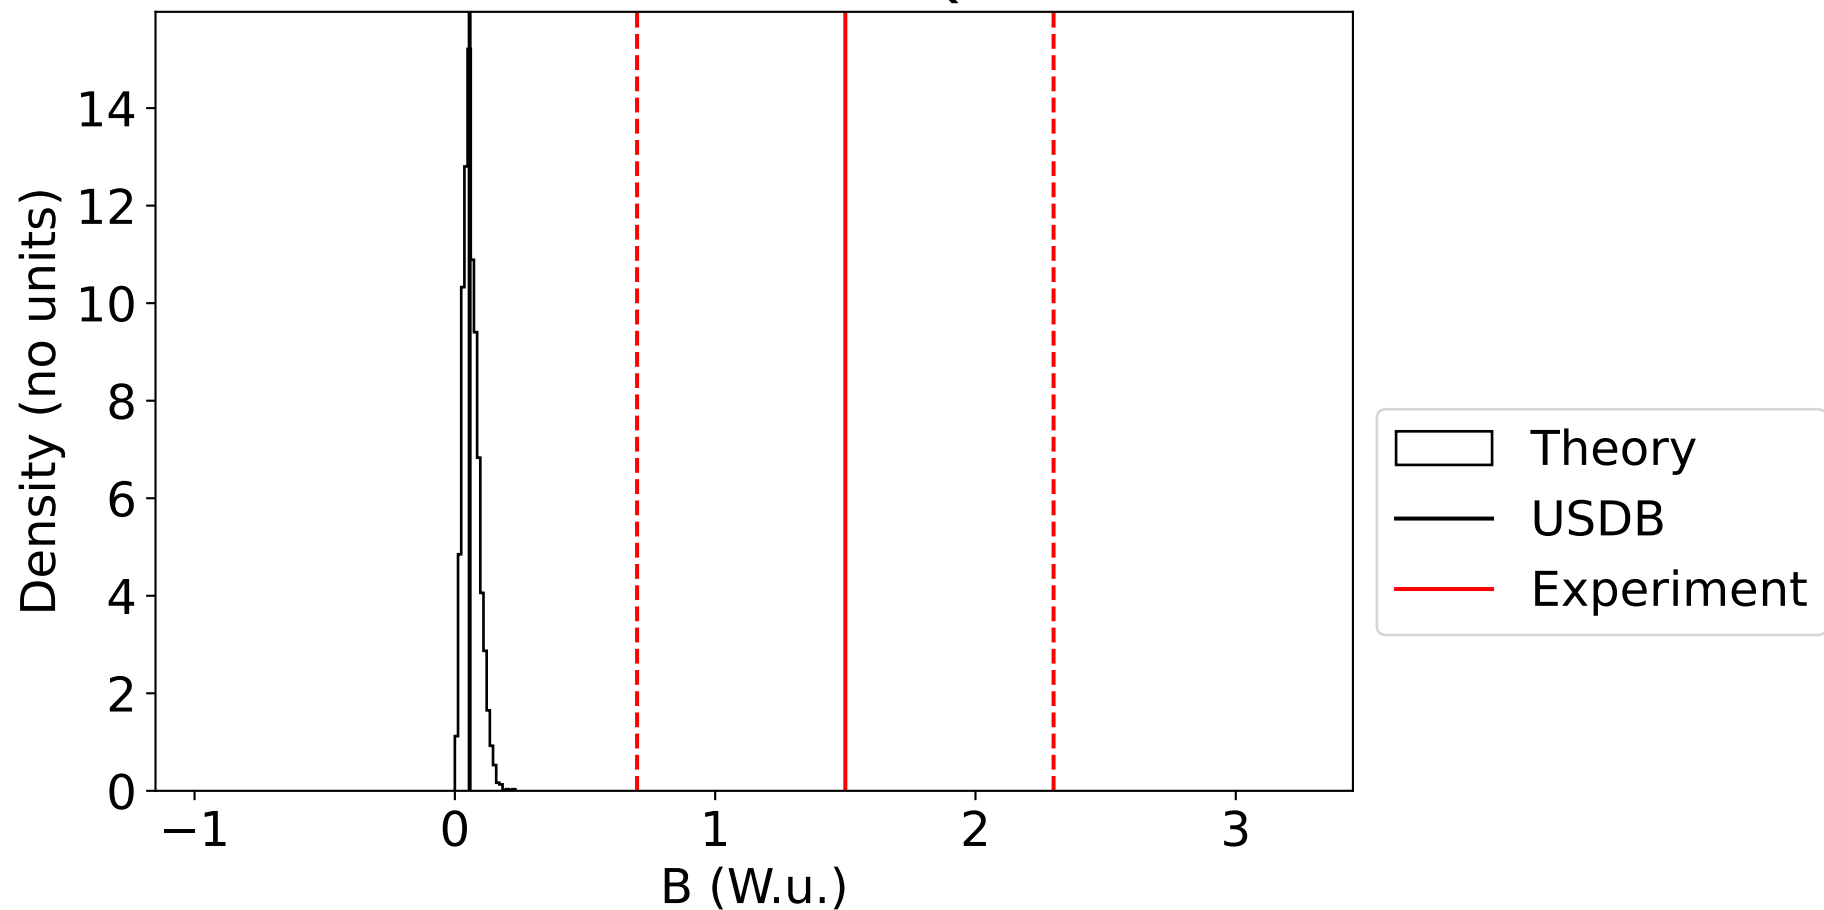

$^{18}\text{Ne} (2_2) \rightarrow (2_1)$   
Included in UQ

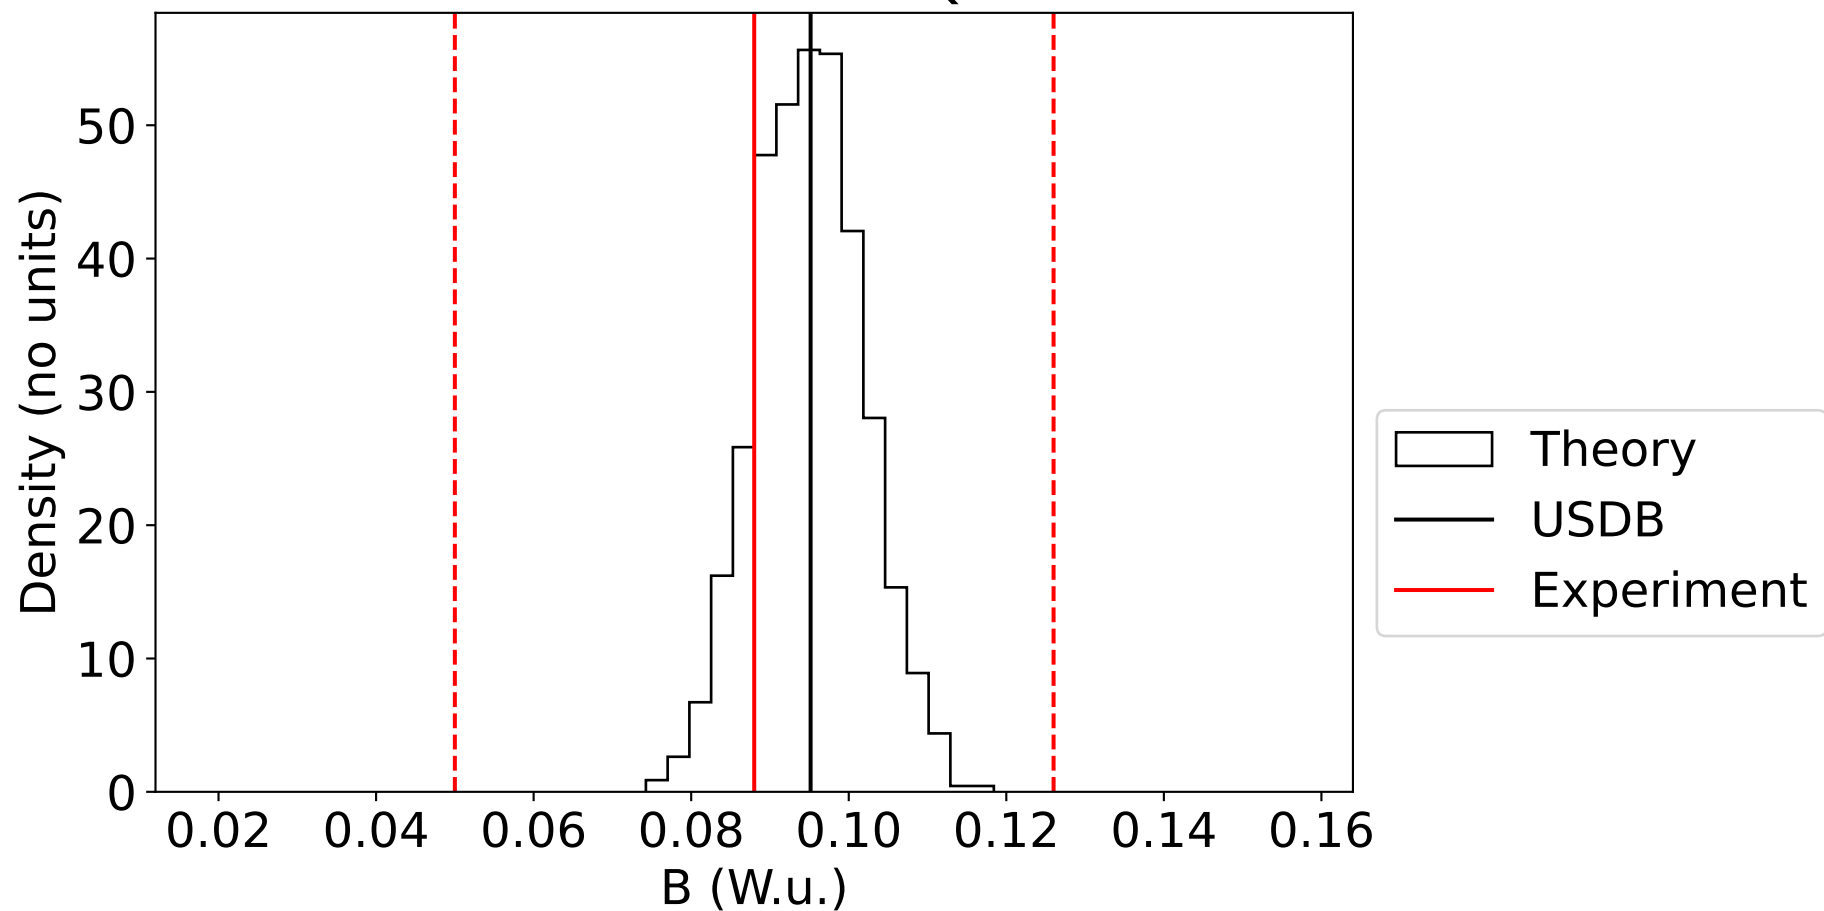

$^{19}\text{Ne} (3/2_1) \rightarrow (5/2_1)$   
Included in UQ

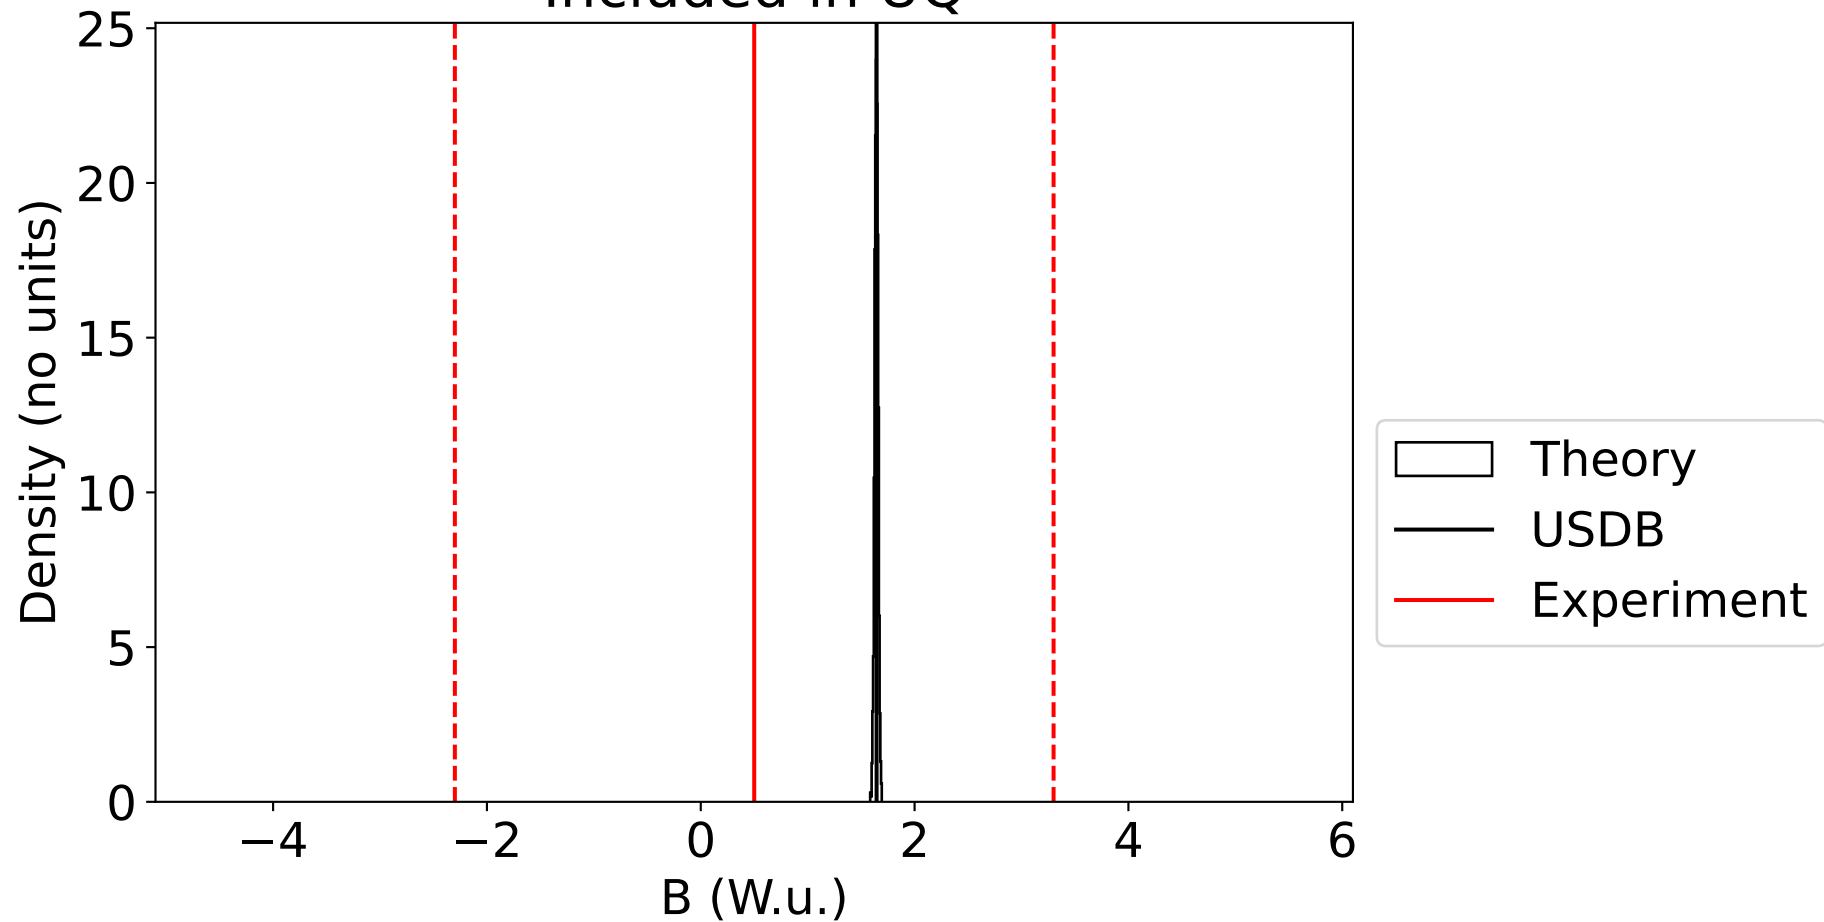

$^{21}\text{Ne} (5/2_1) \rightarrow (3/2_1)$   
Included in UQ

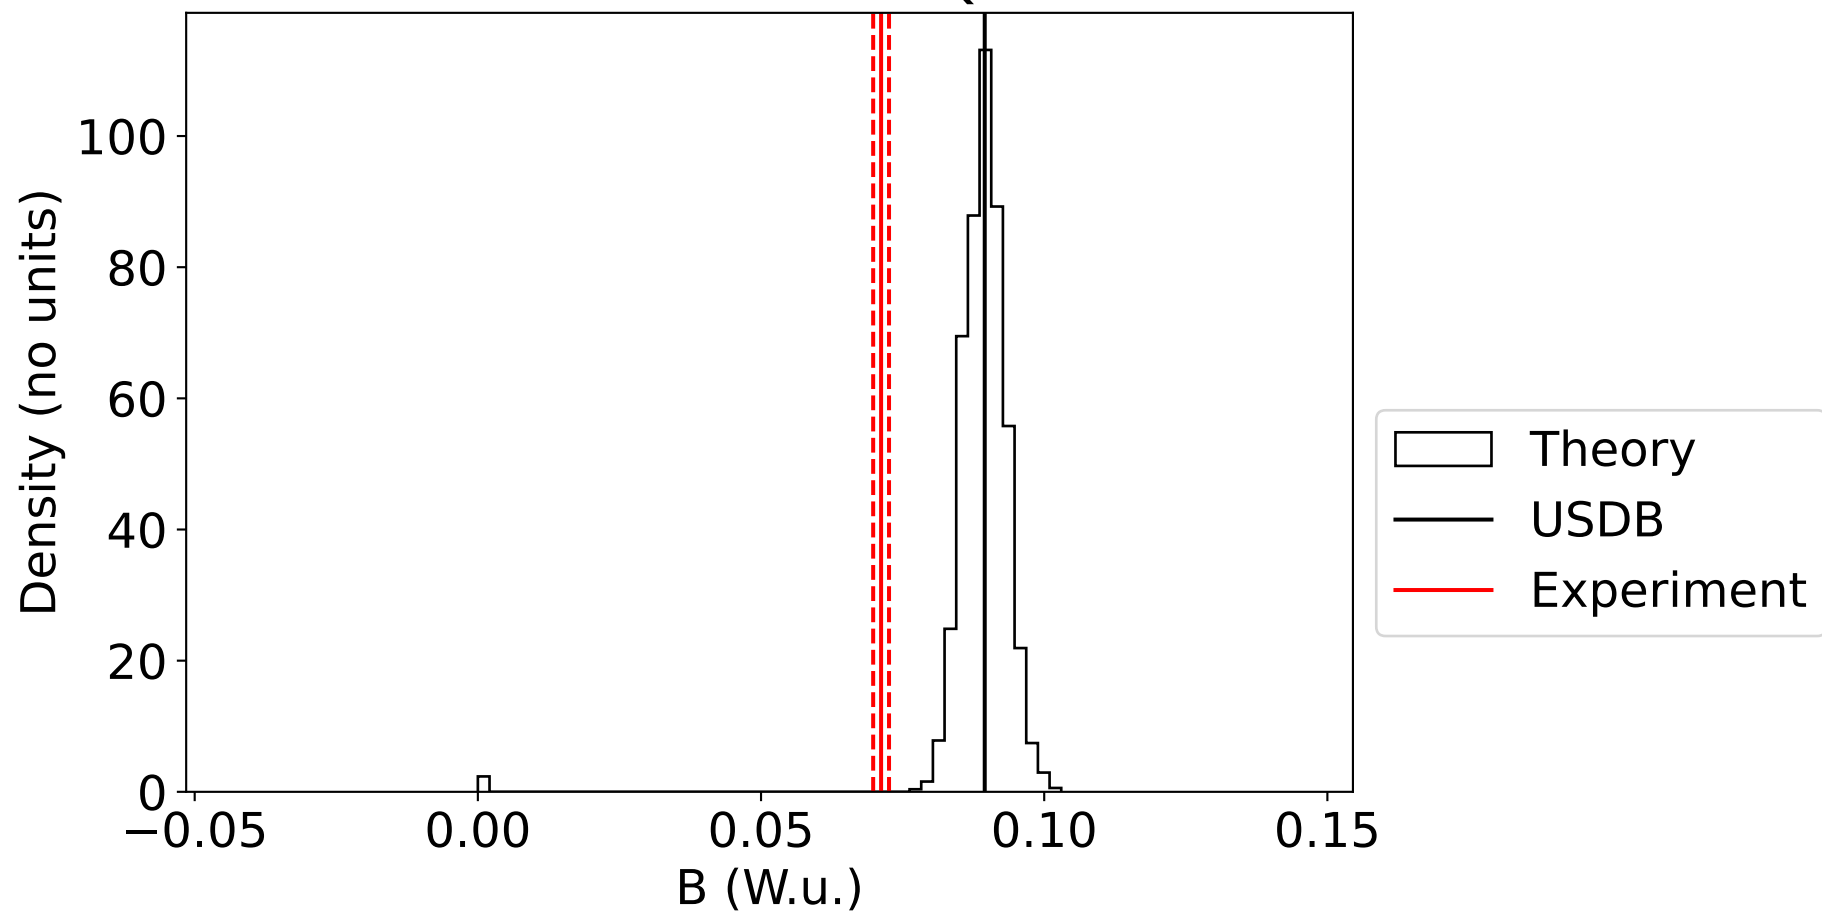

$^{21}\text{Ne} (7/2_1) \rightarrow (5/2_1)$   
Included in UQ

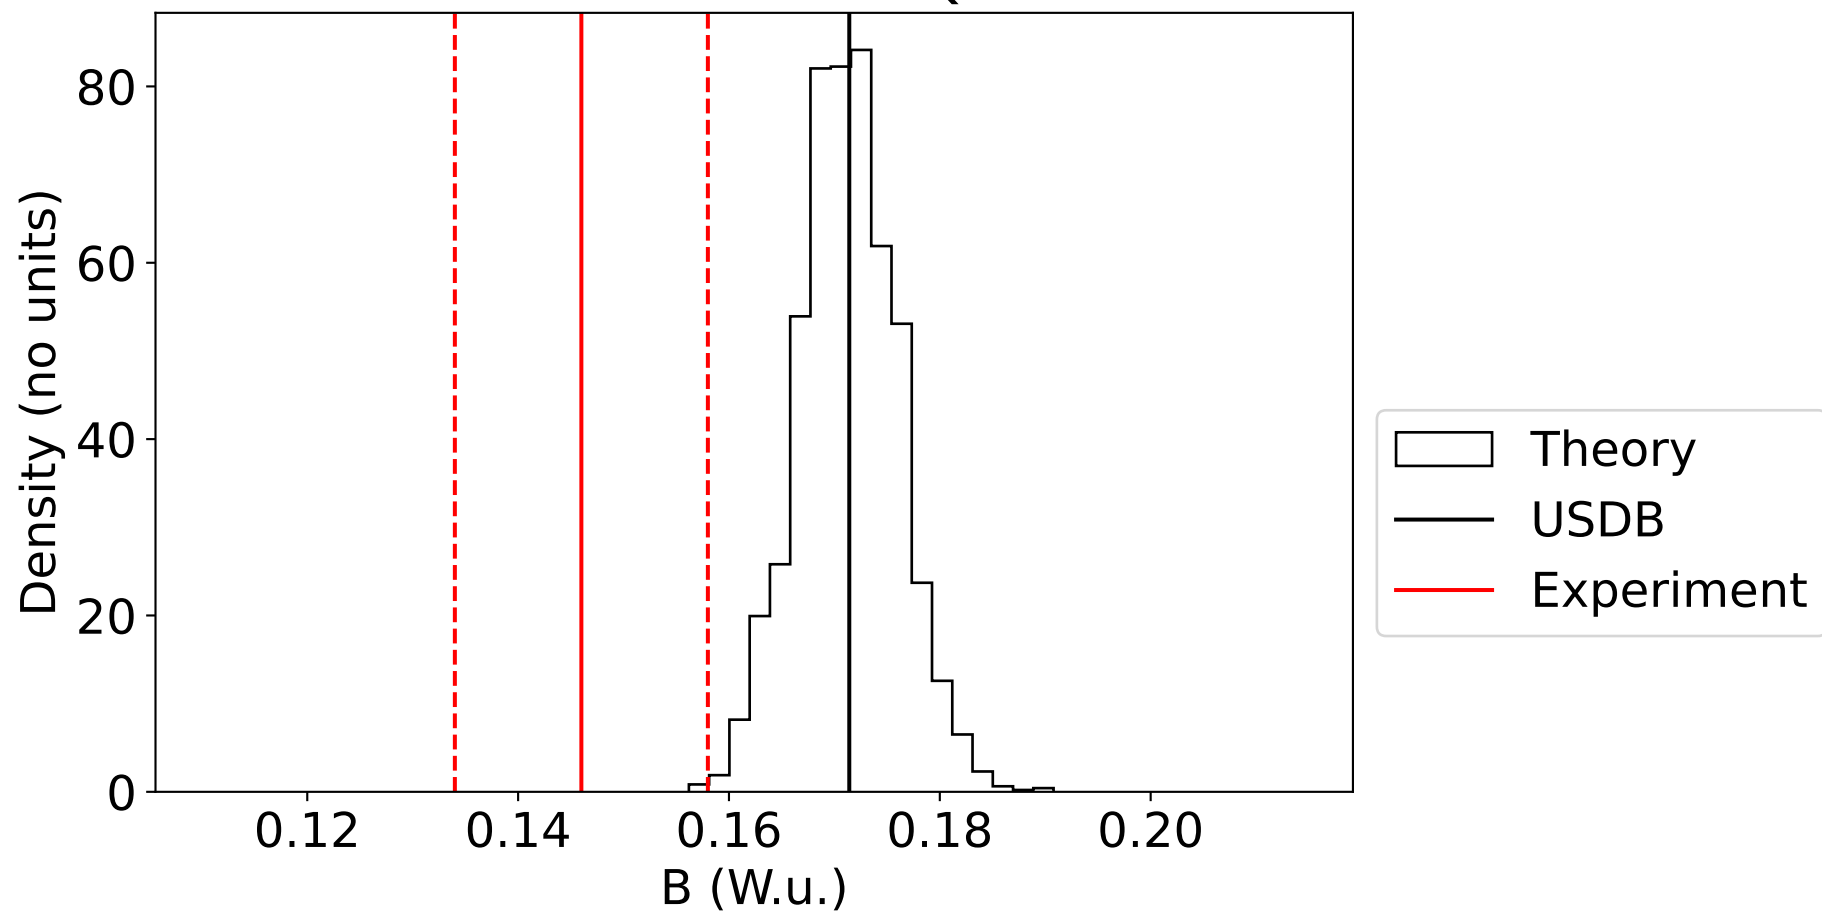

$^{21}\text{Ne} (1/2_1) \rightarrow (3/2_1)$   
Included in UQ

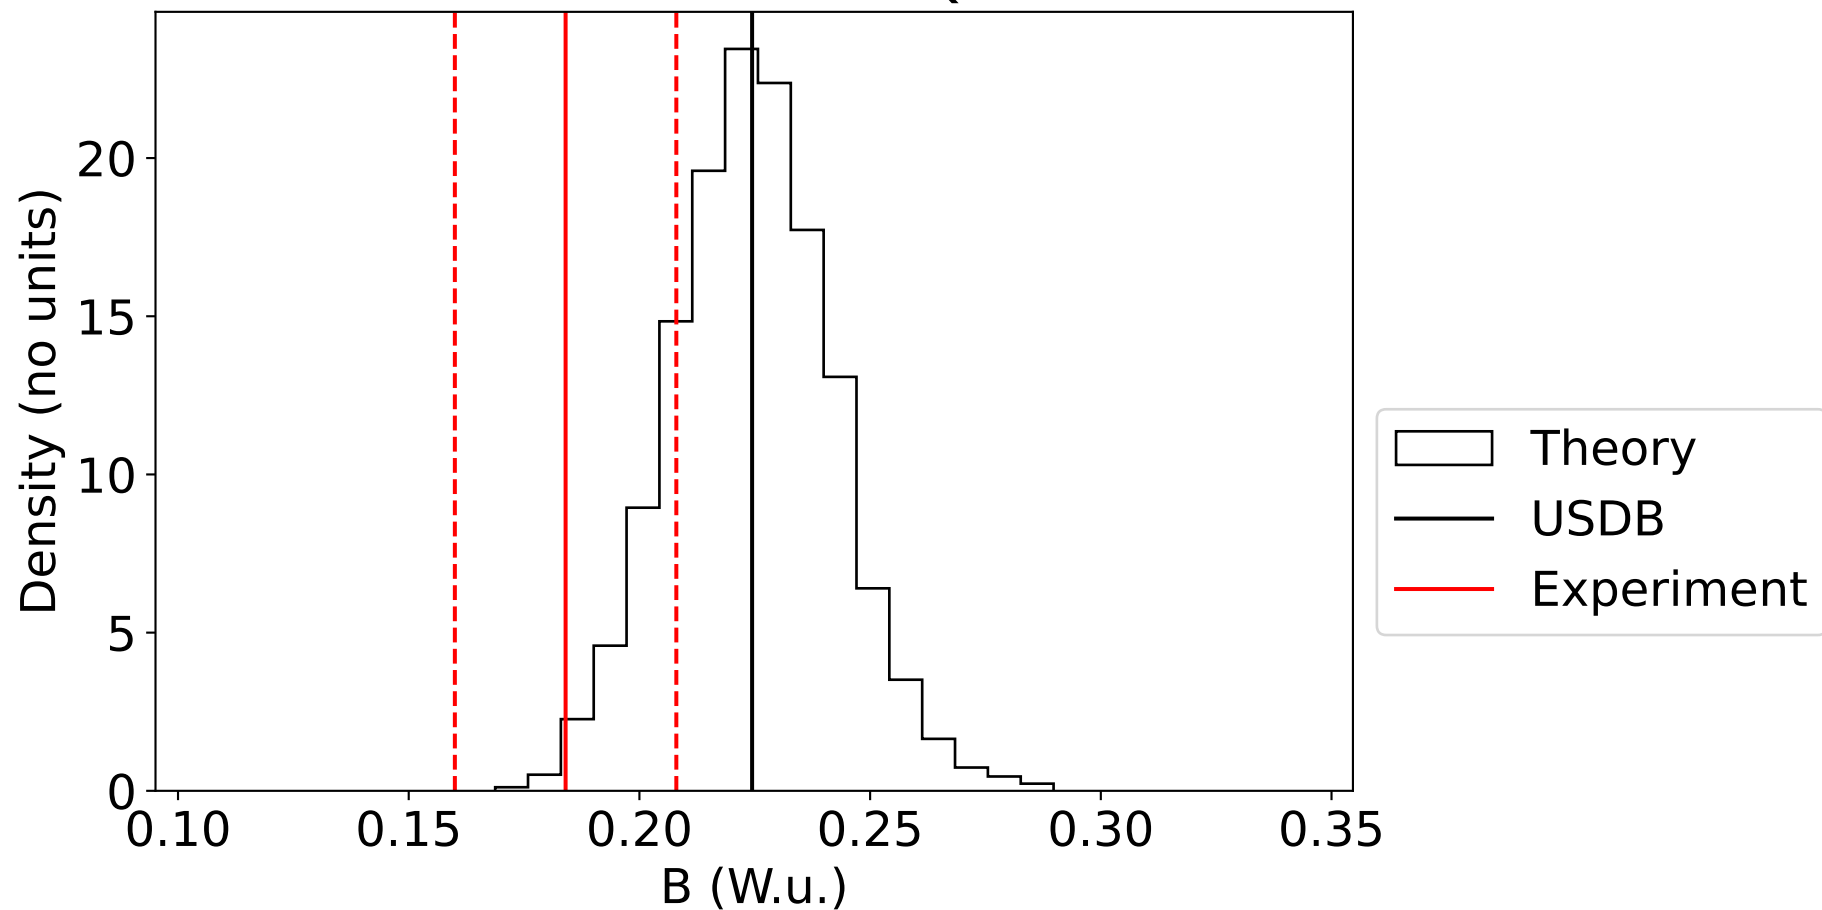

$^{21}\text{Ne } (9/2_1) \rightarrow (7/2_1)$   
Included in UQ

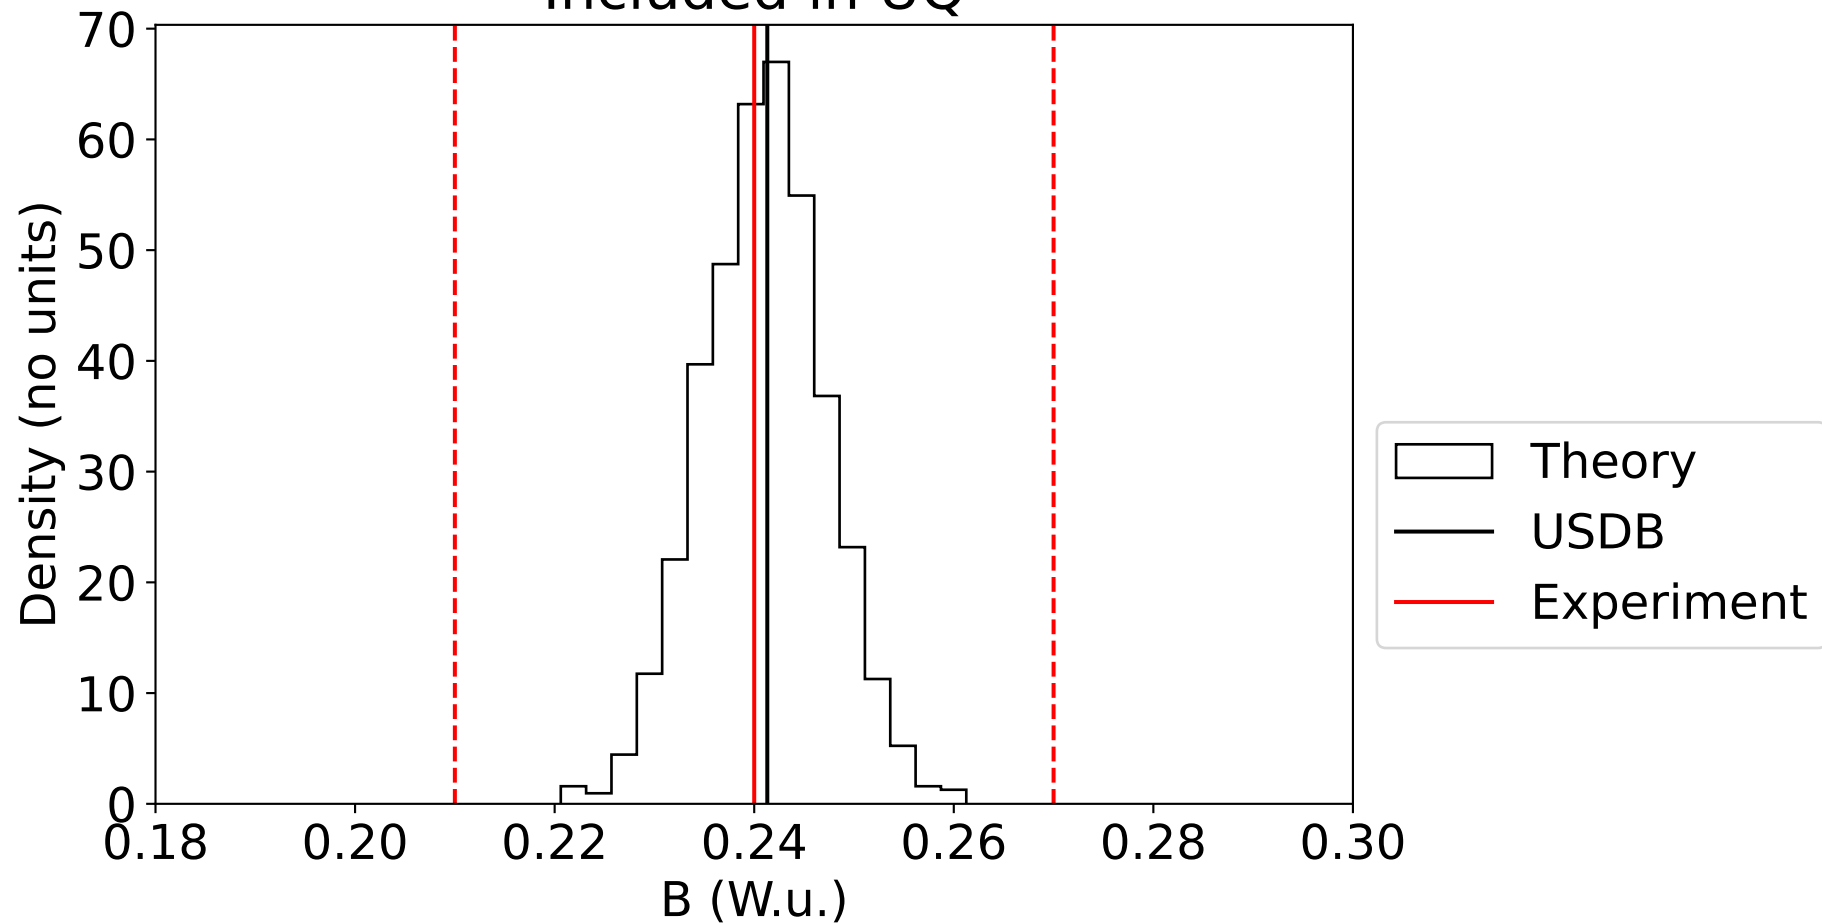



$^{21}\text{Ne} (11/2_1) \rightarrow (9/2_1)$   
Included in UQ

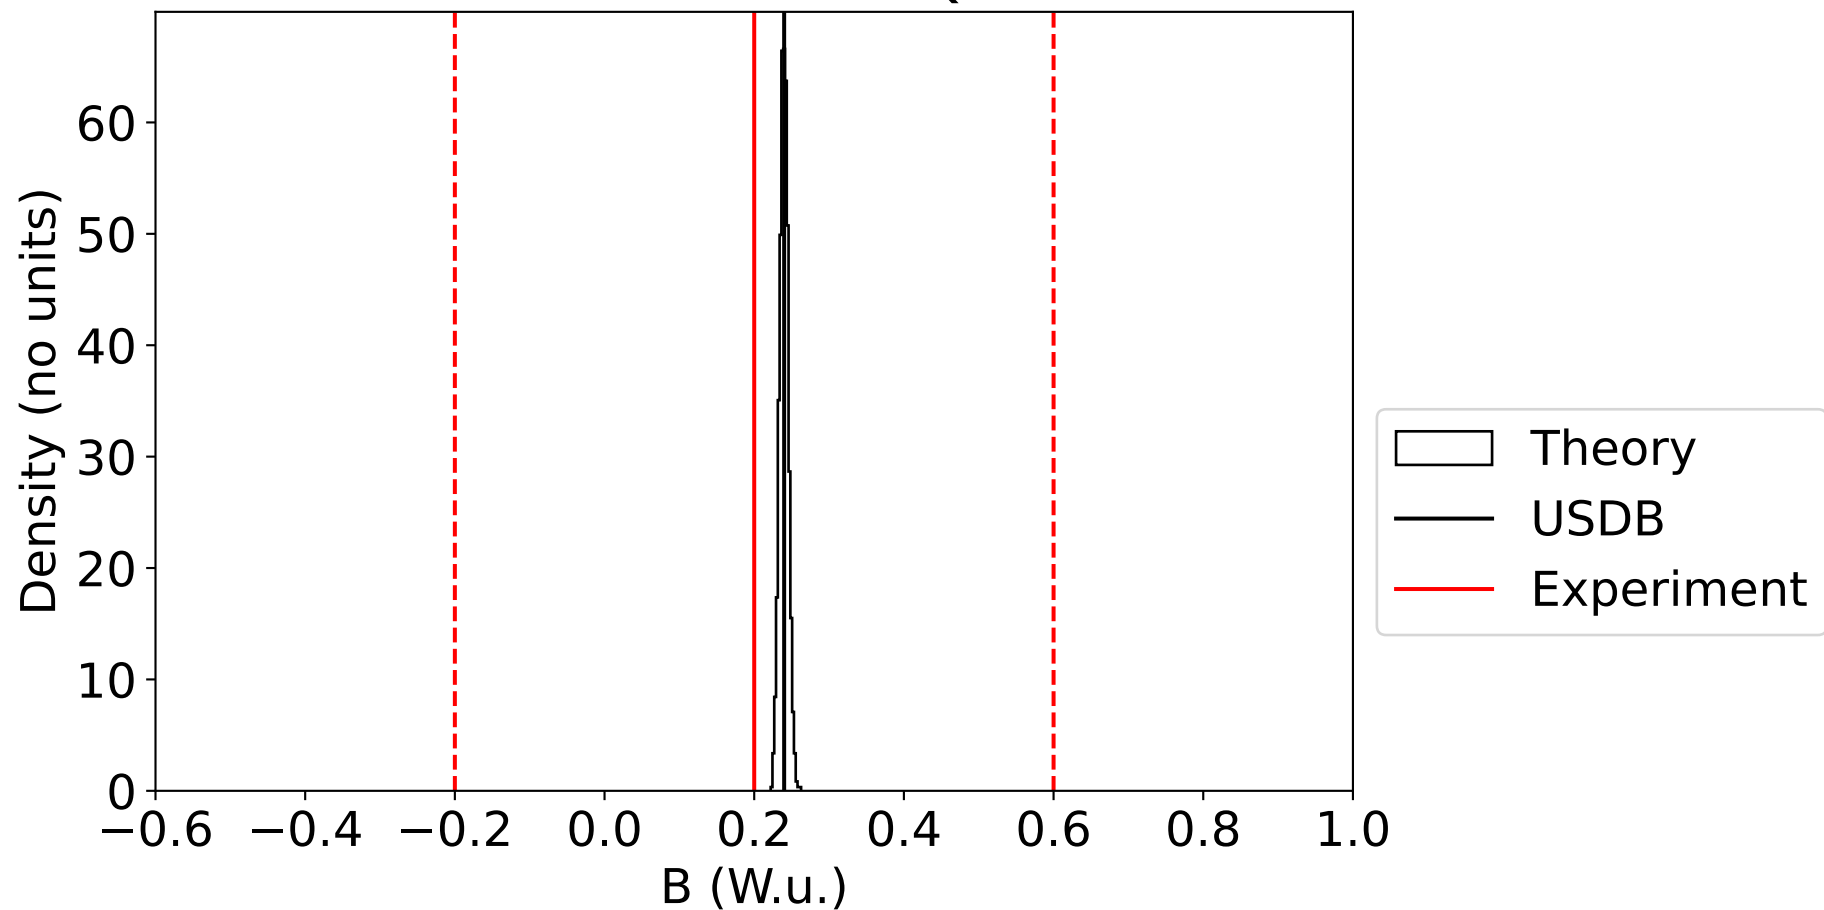

$^{21}\text{Ne} (3/2_2) \rightarrow (5/2_1)$   
Included in UQ

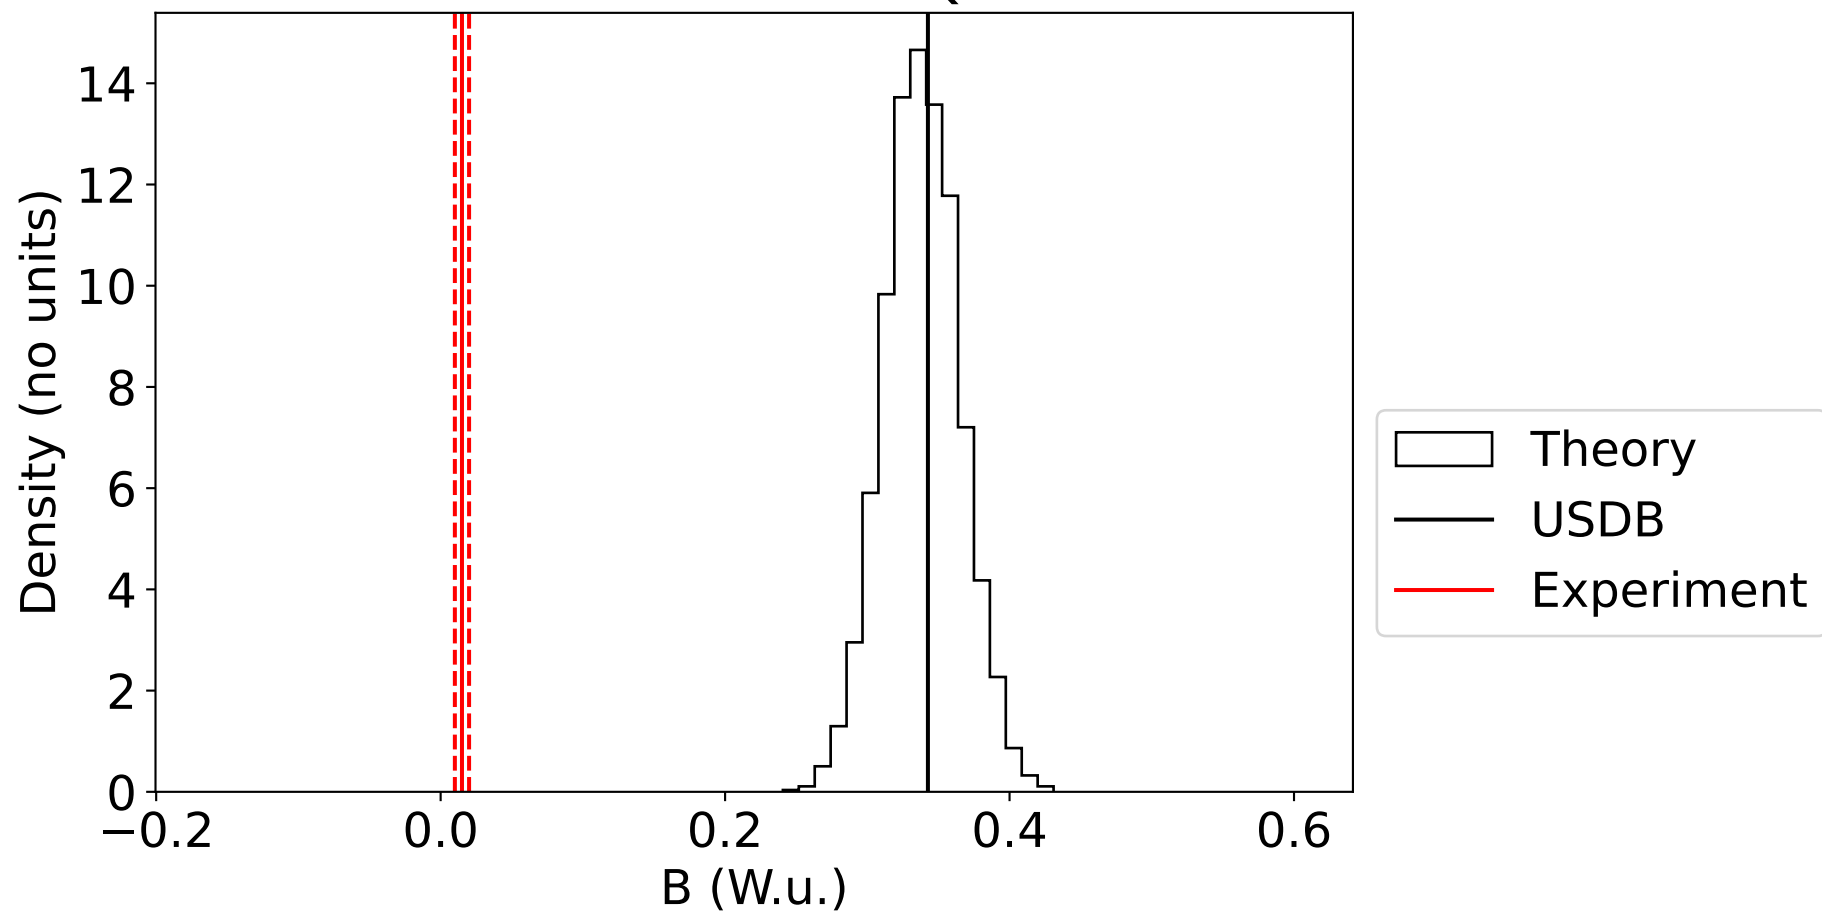

$^{21}\text{Ne } (5/2_4) \rightarrow (7/2_1)$   
Included in UQ

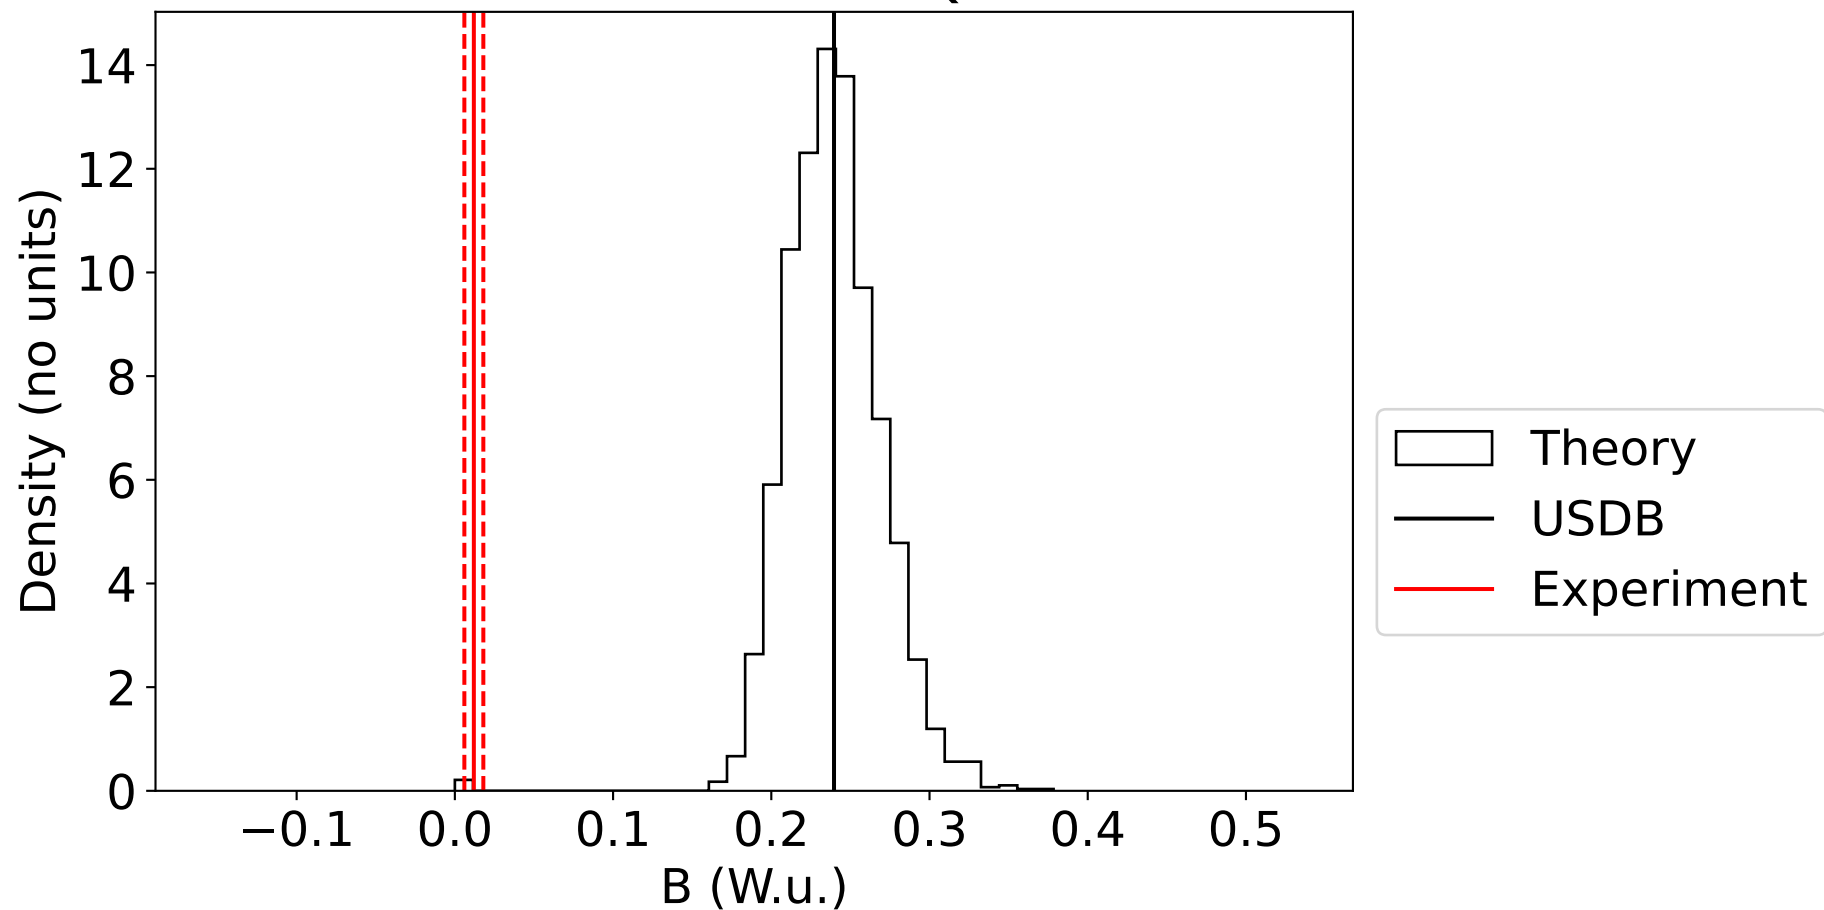

$^{22}\text{Ne} (2_2) \rightarrow (2_1)$   
Included in UQ

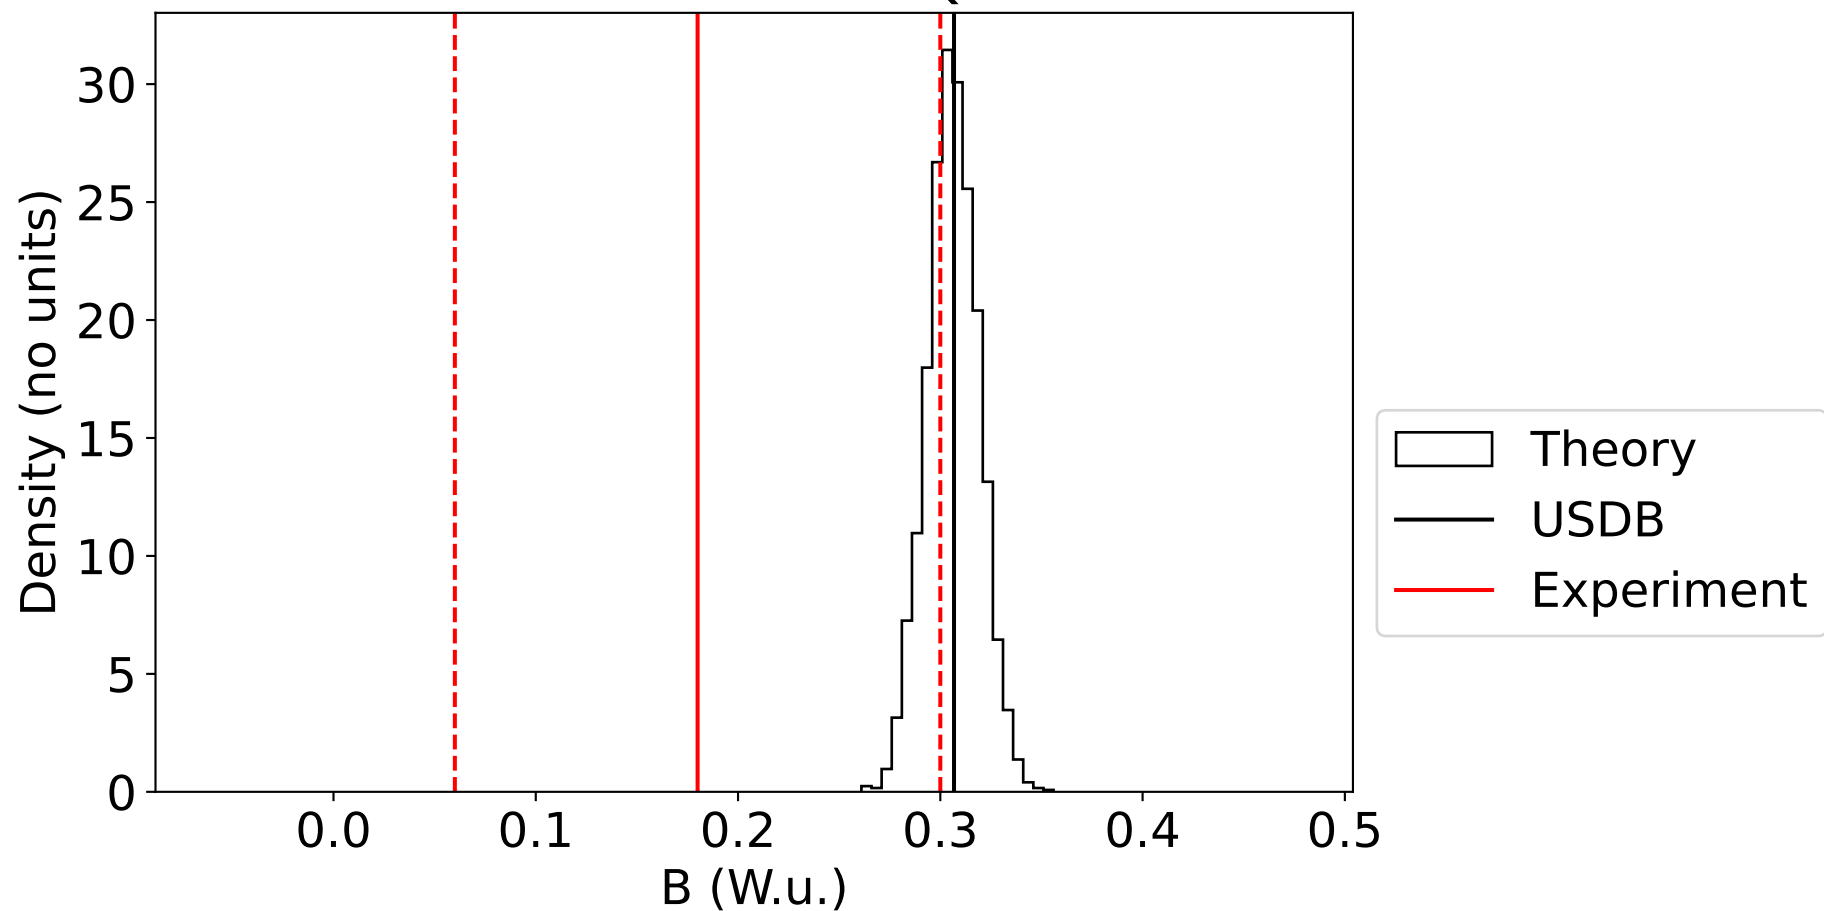

$^{22}\text{Ne} (1_1) \rightarrow (2_1)$   
Included in UQ

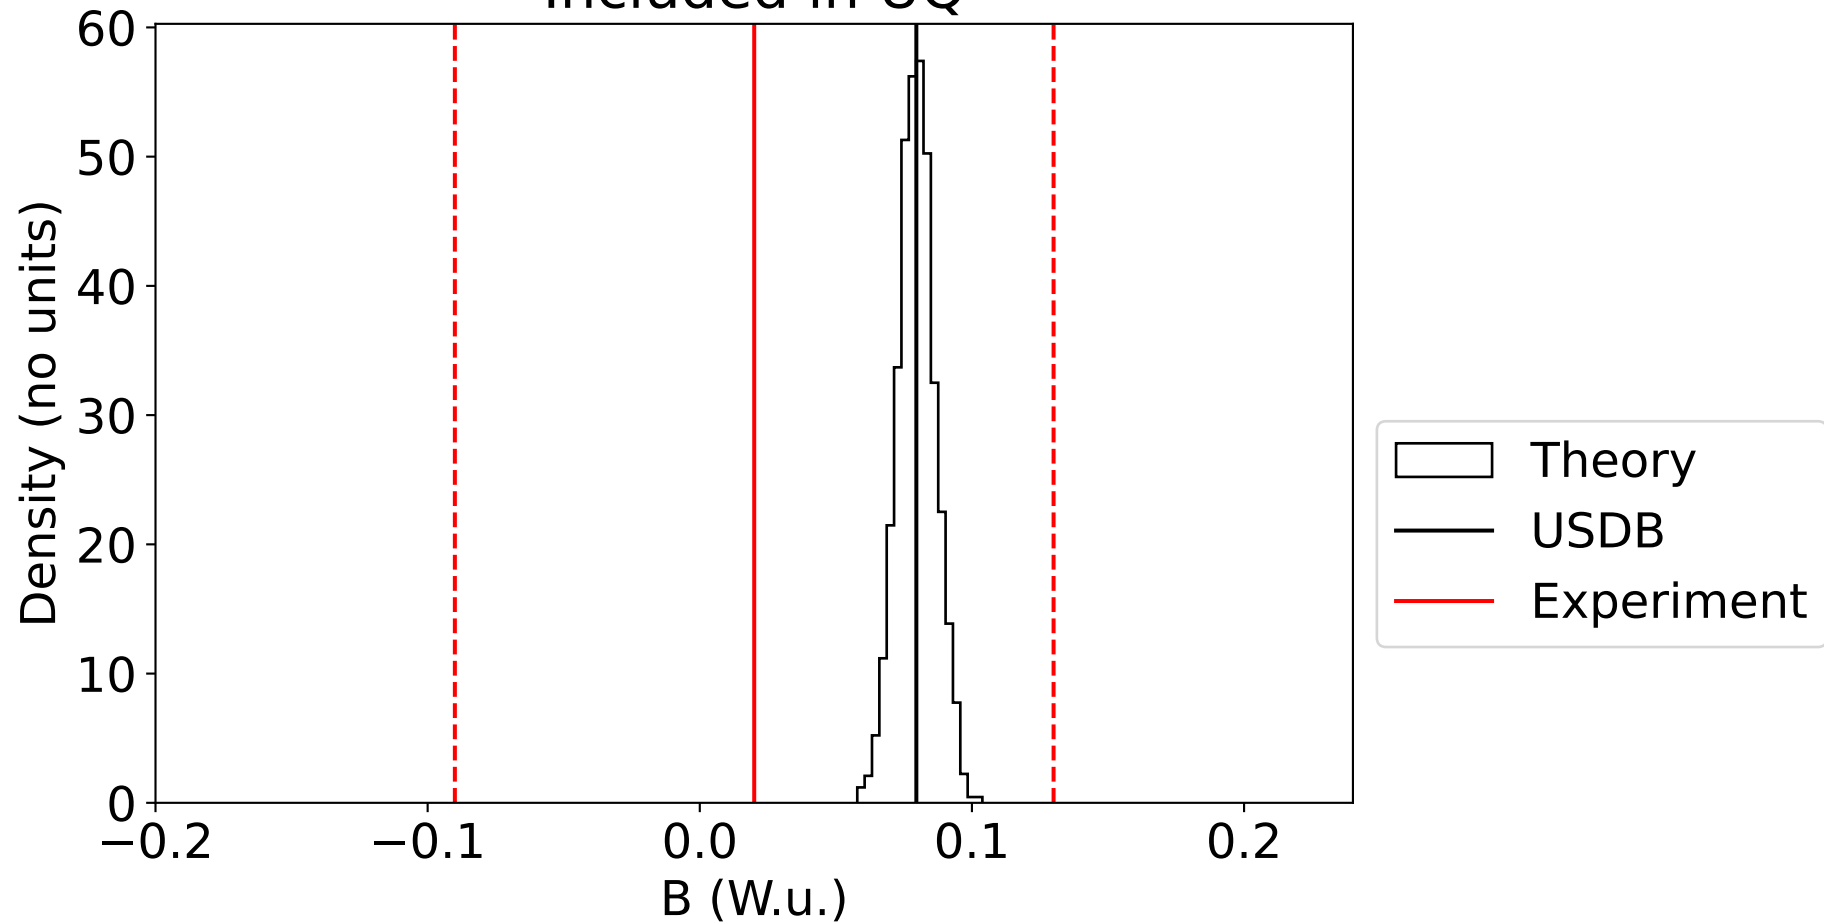

$^{22}\text{Ne} (4_2) \rightarrow (4_1)$   
Included in UQ

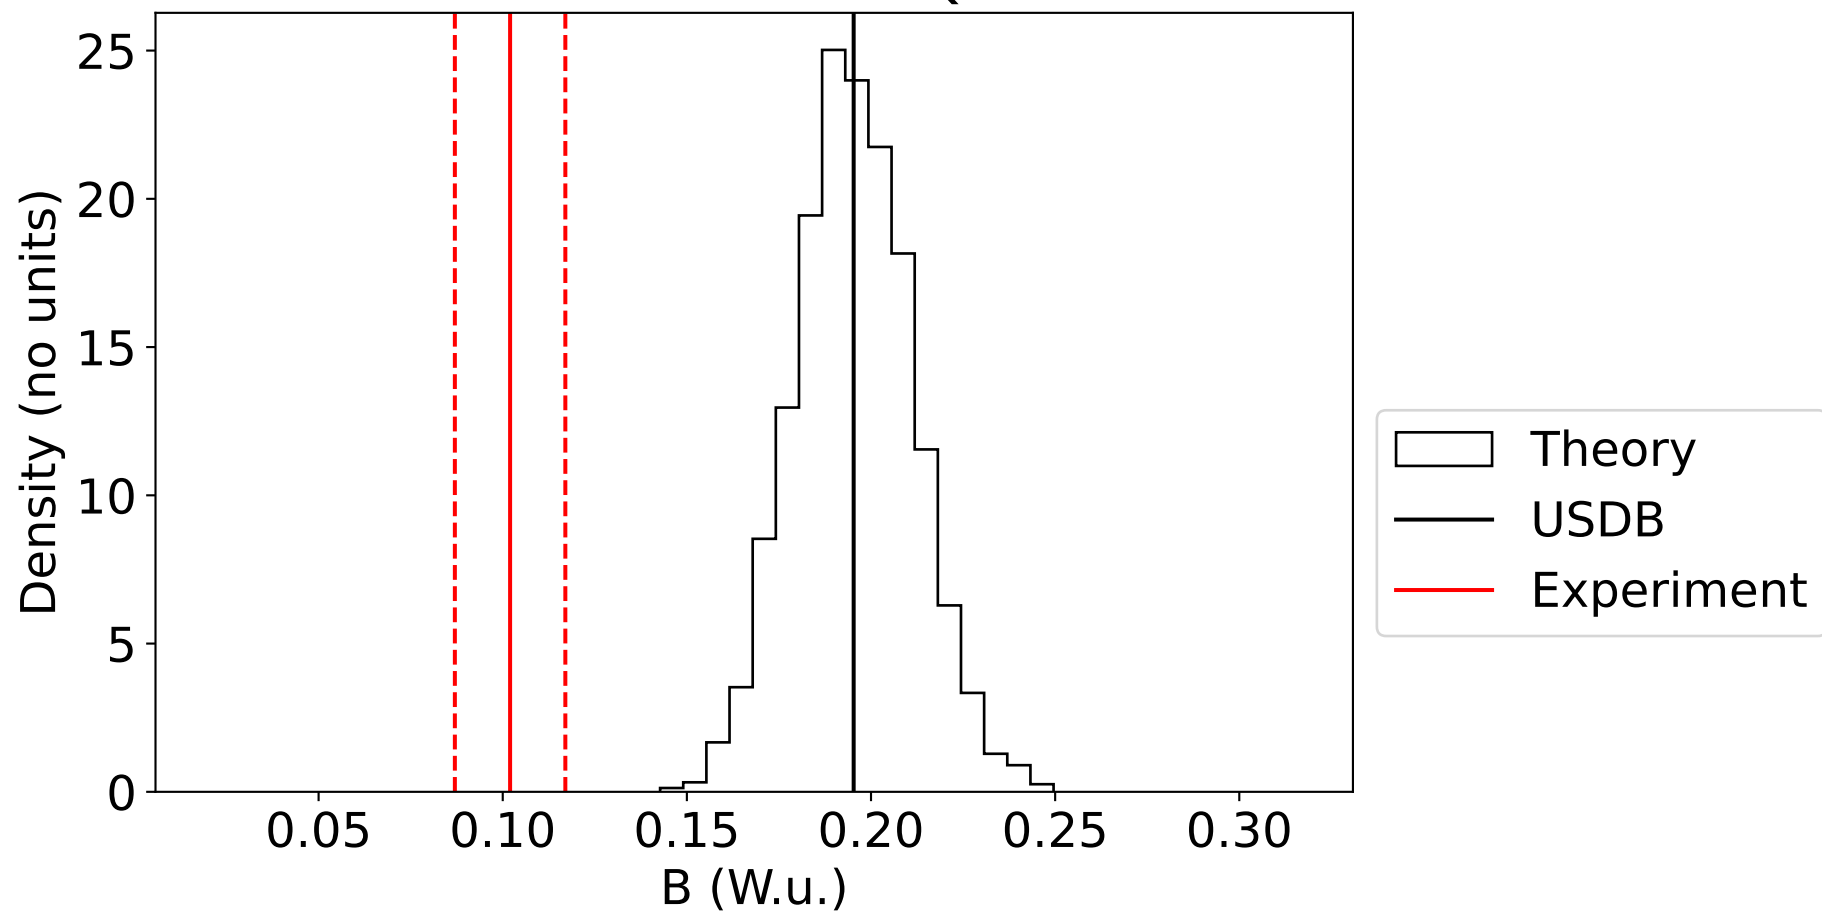

$^{22}\text{Ne} (2_4) \rightarrow (2_2)$   
Included in UQ

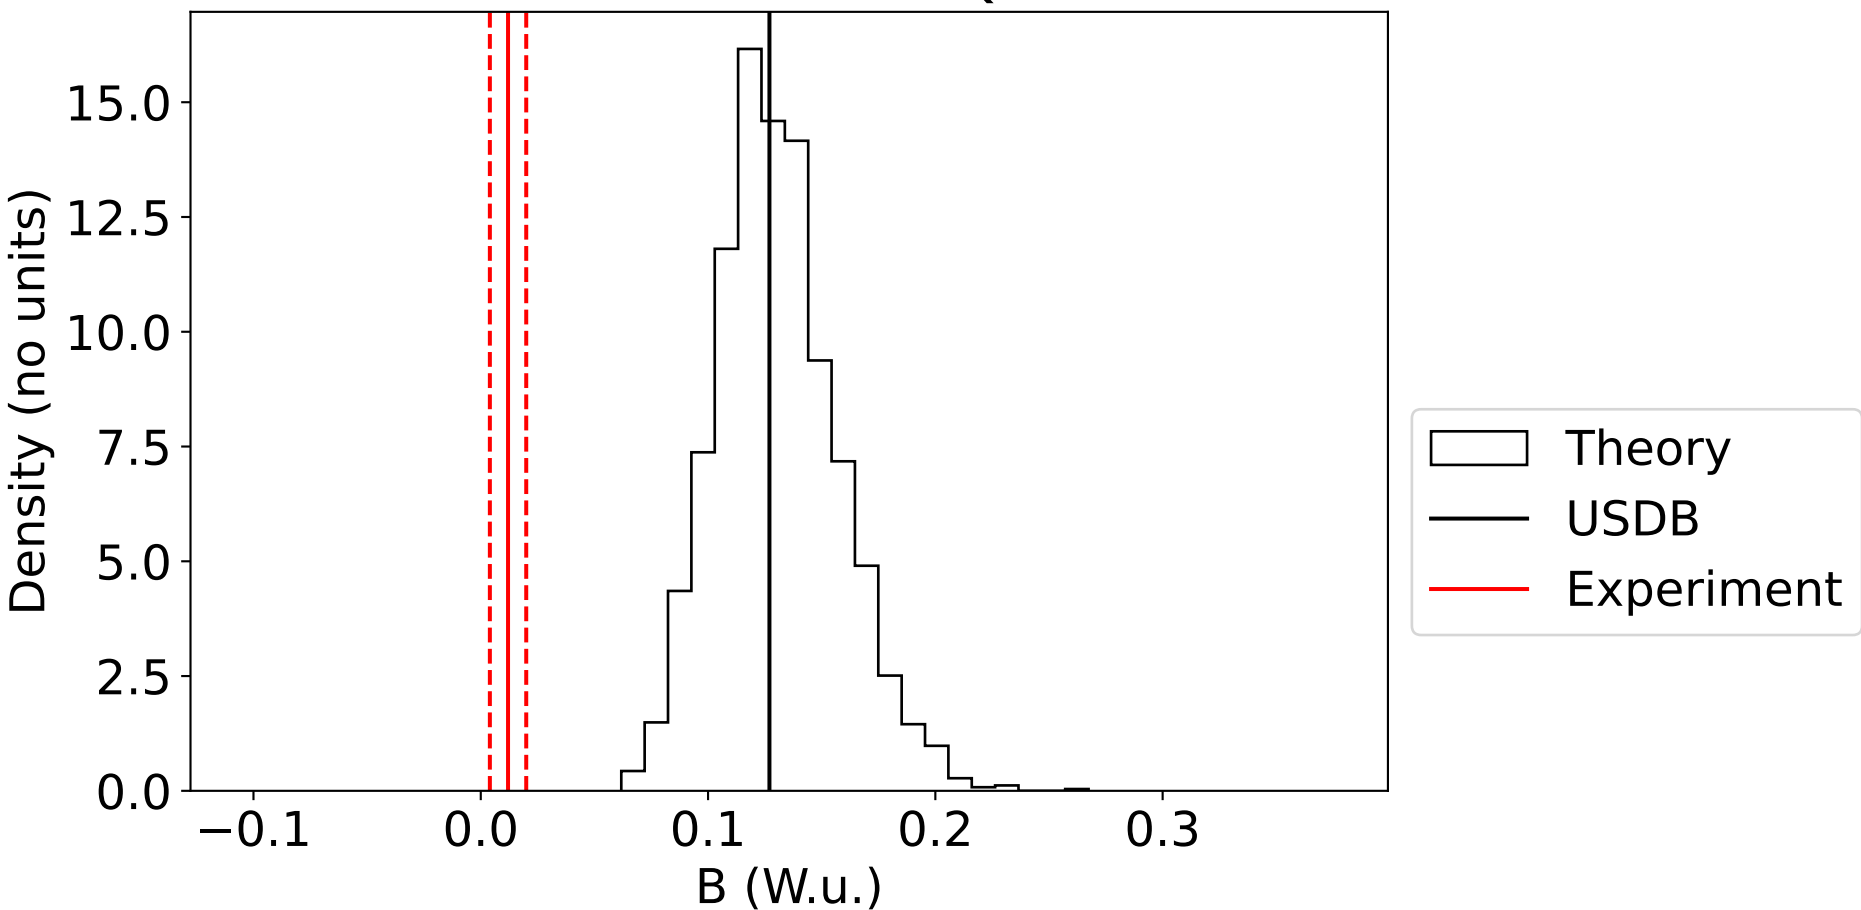

$^{22}\text{Ne} (4_3) \rightarrow (4_1)$   
Included in UQ

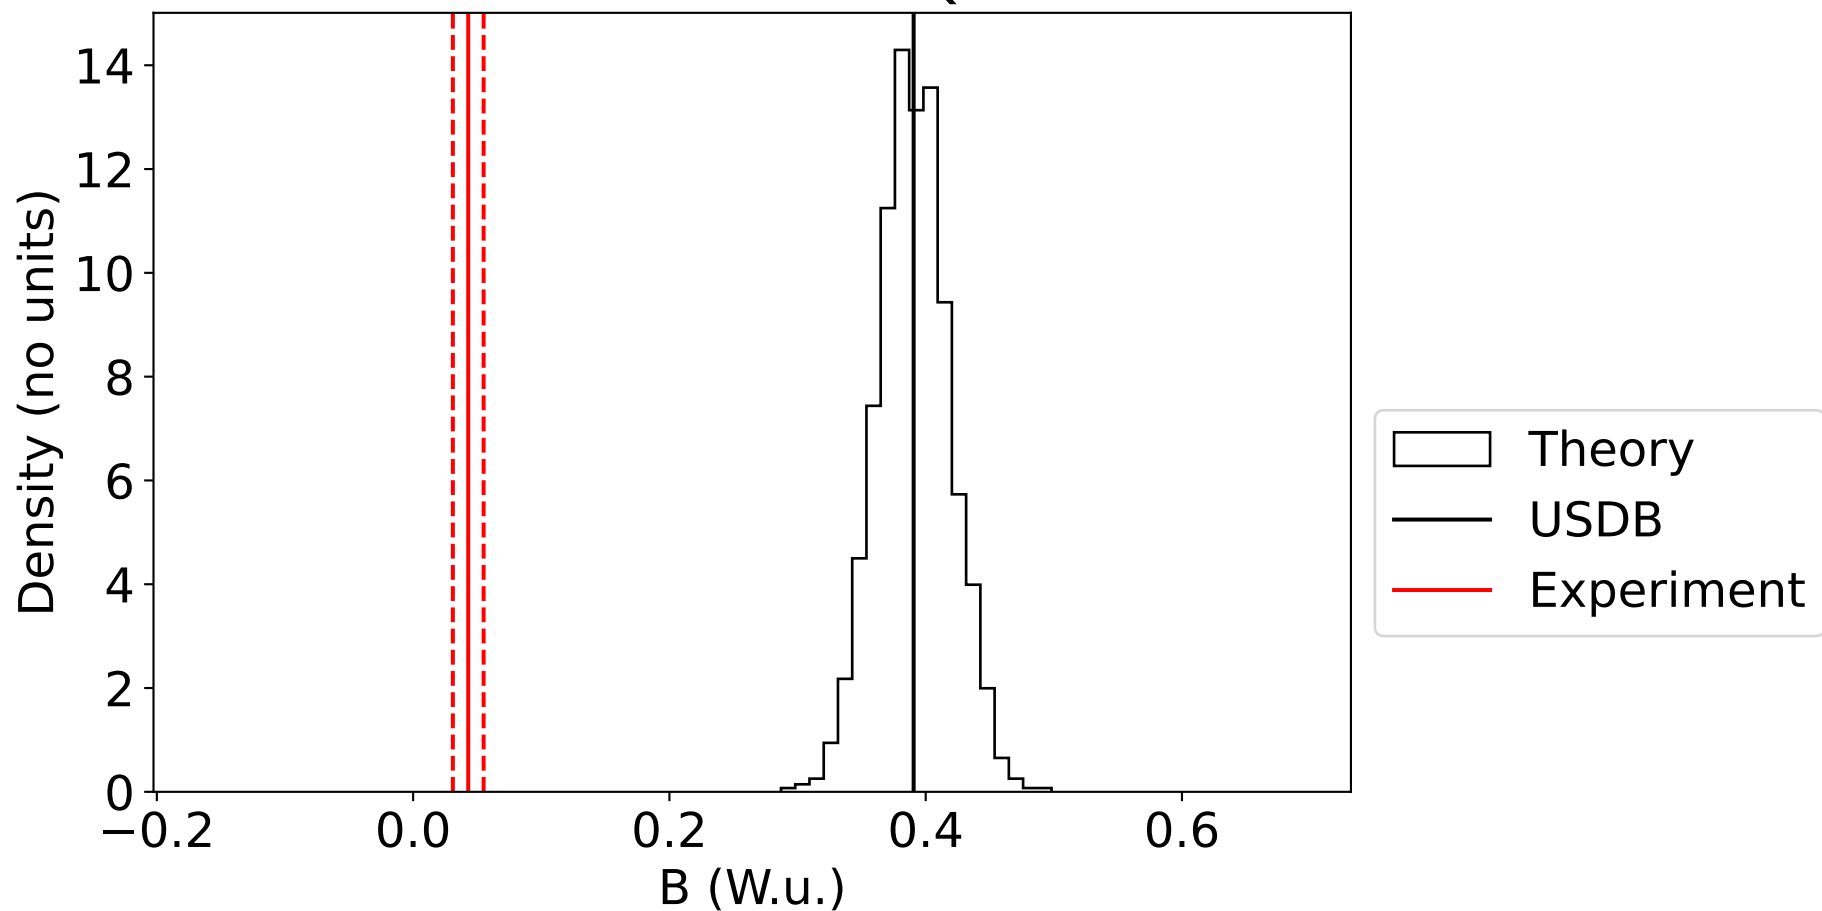



$^{21}\text{Na } (5/2_1) \rightarrow (3/2_1)$   
Included in UQ

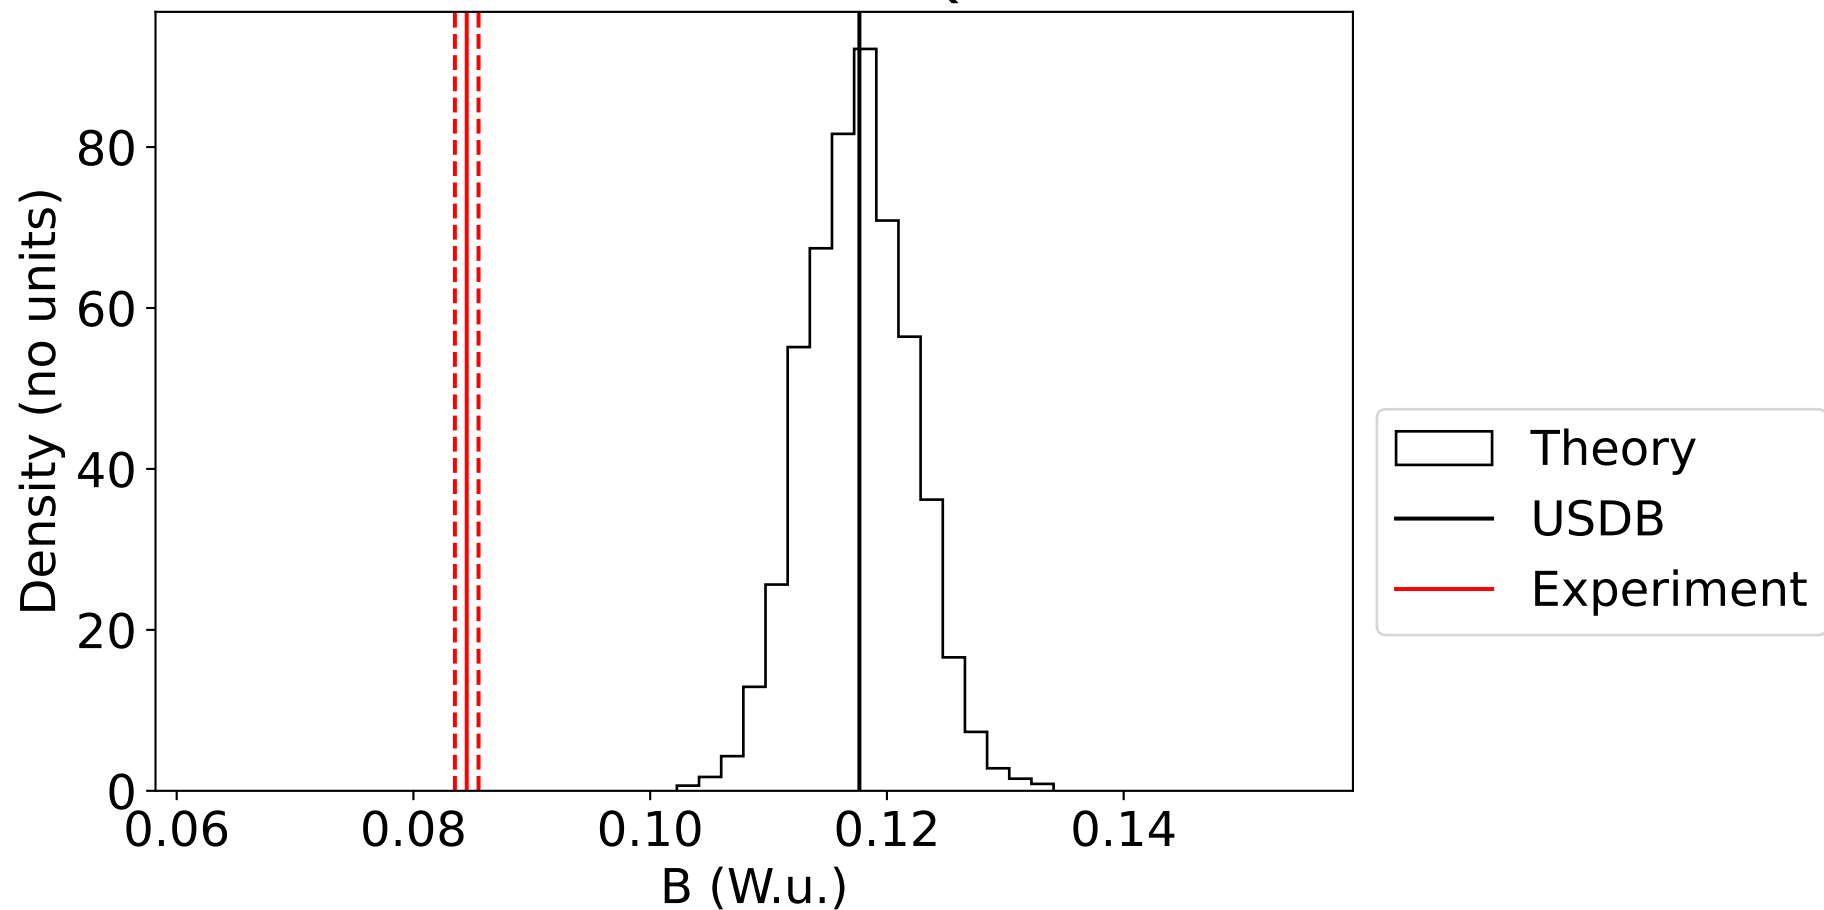

$^{21}\text{Na} (7/2_1) \rightarrow (5/2_1)$   
Included in UQ

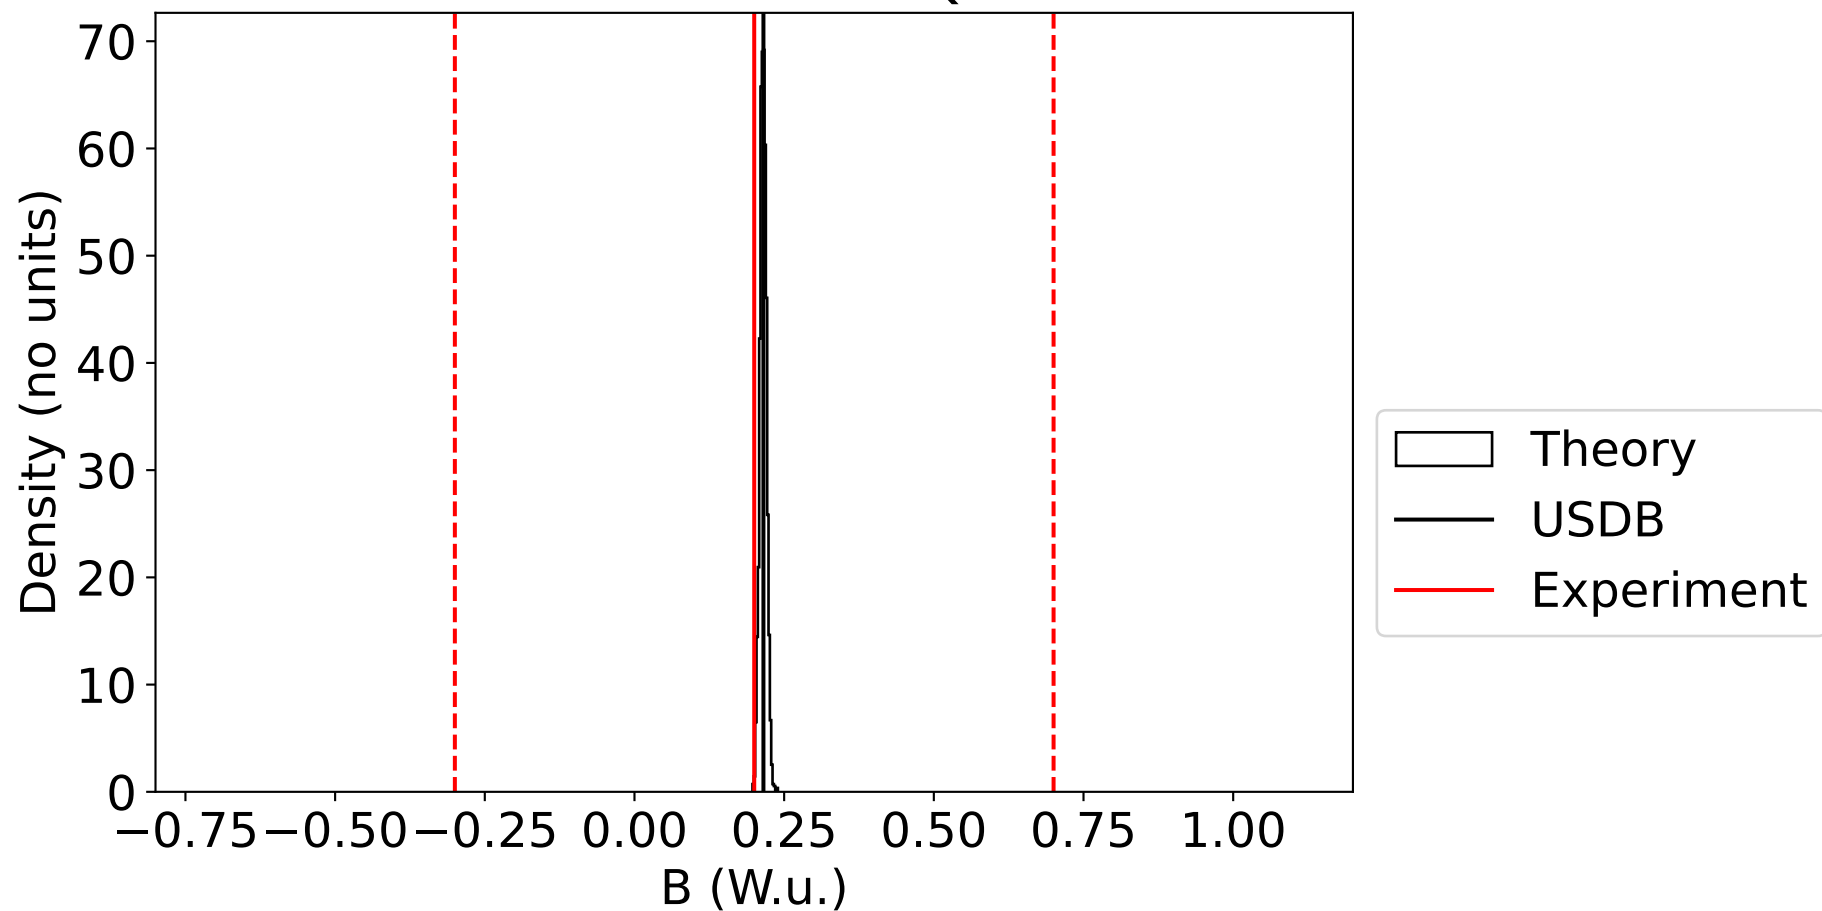

$^{21}\text{Na}$  ( $1/2_1$ )  $\rightarrow$  ( $3/2_1$ )  
Included in UQ

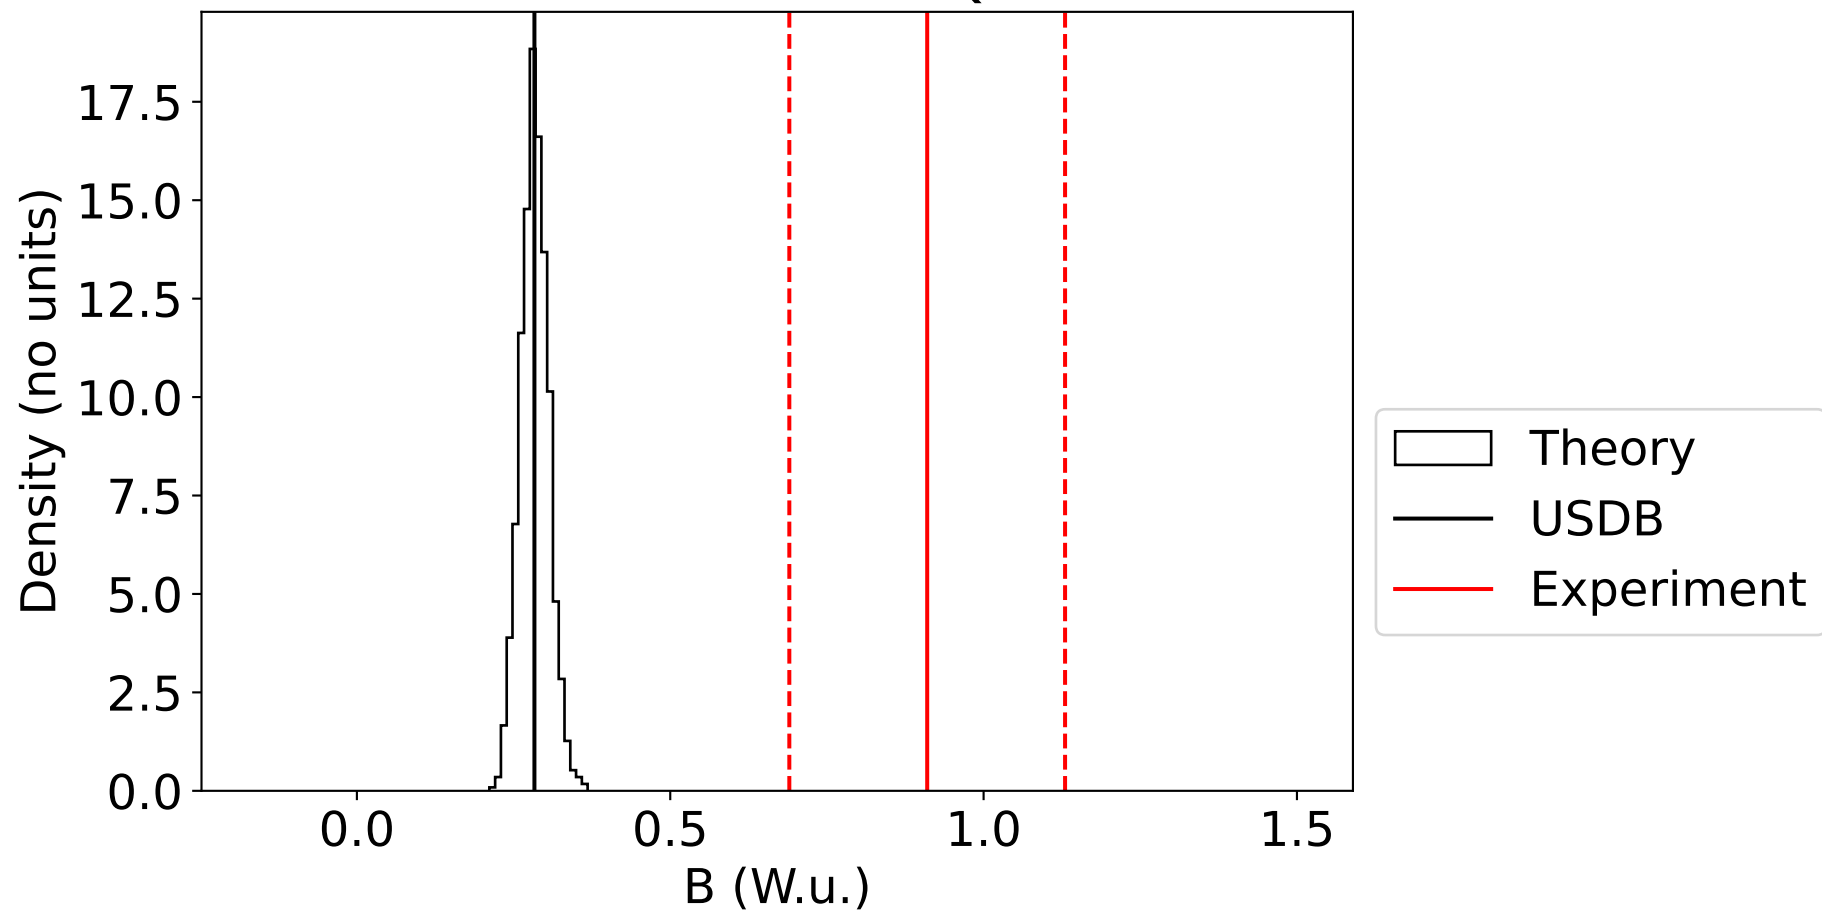

$^{21}\text{Na}$  ( $5/2_2$ )  $\rightarrow$  ( $3/2_1$ )  
Included in UQ

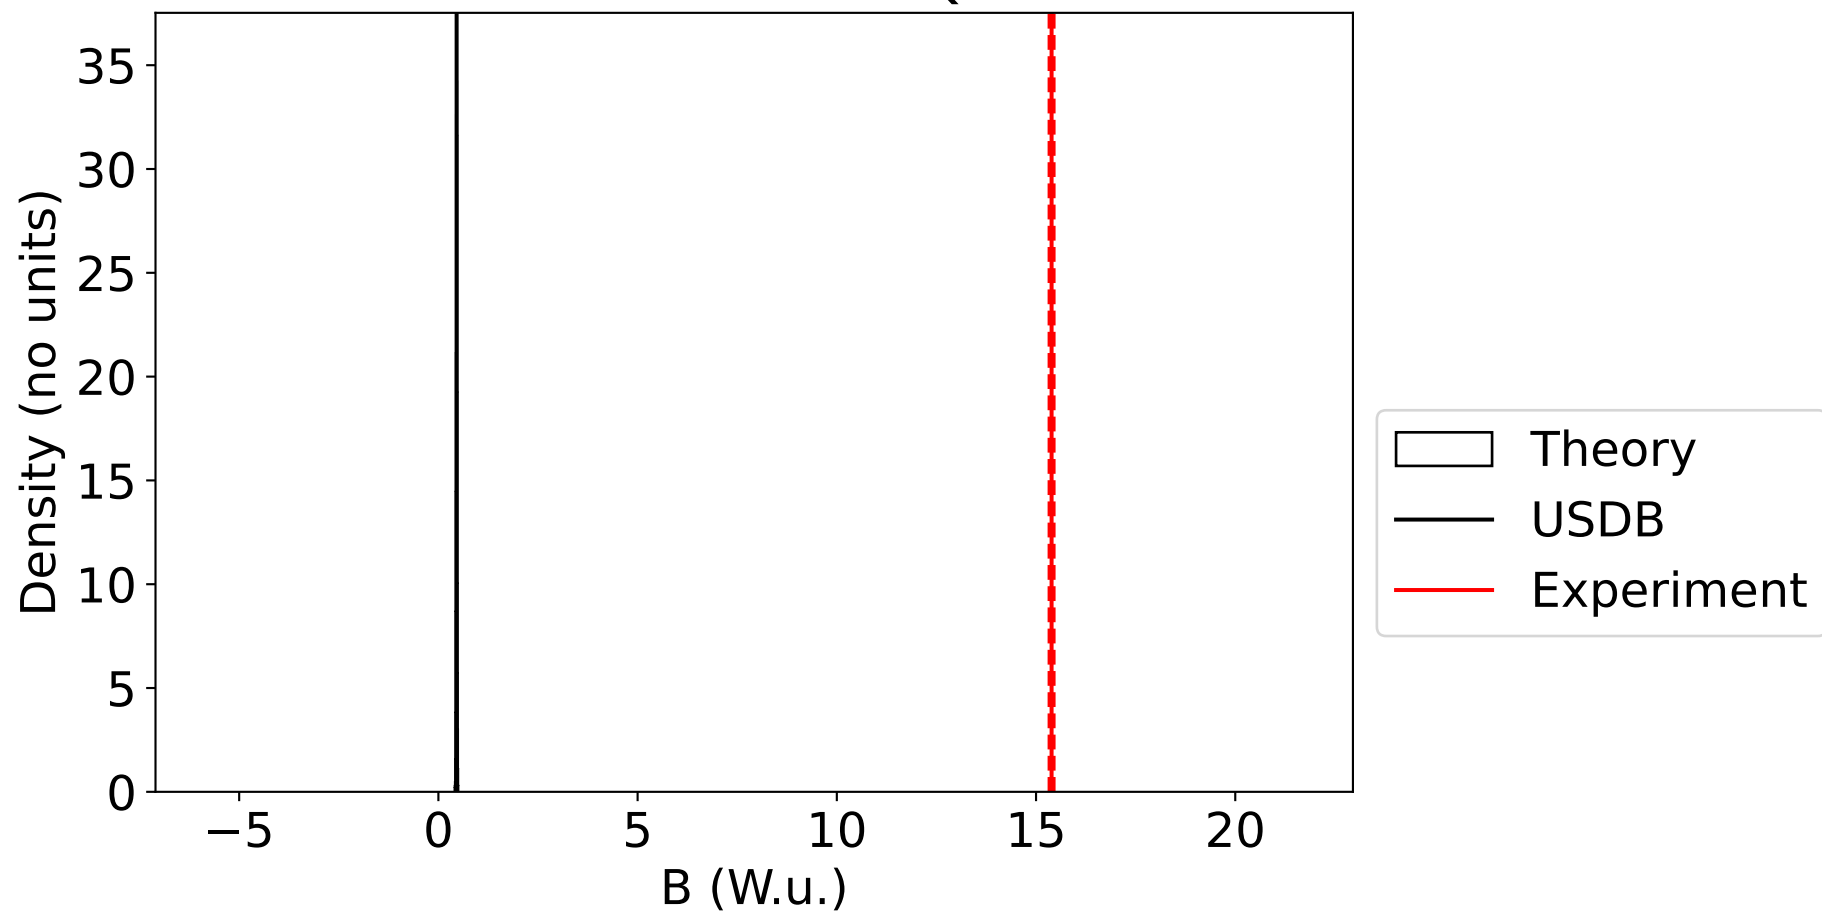

$^{22}\text{Na}$  ( $0_1$ )  $\rightarrow$  ( $1_1$ )  
Included in UQ

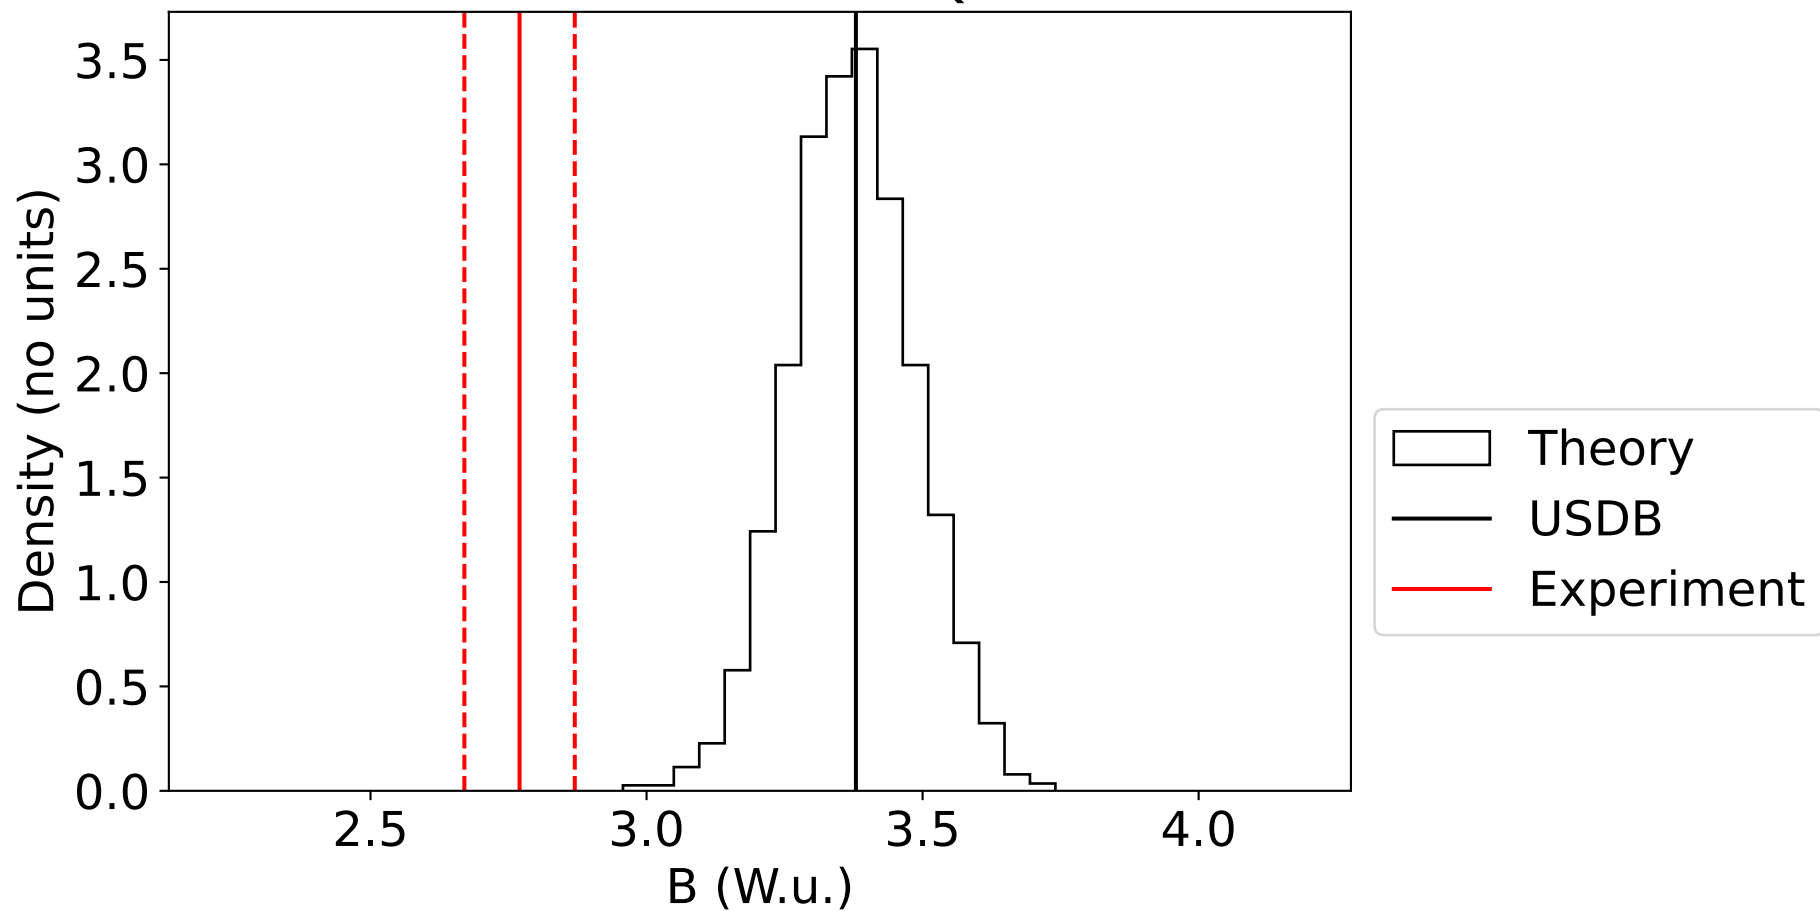

$^{22}\text{Na}$  ( $1_2$ )  $\rightarrow$  ( $0_1$ )  
Included in UQ

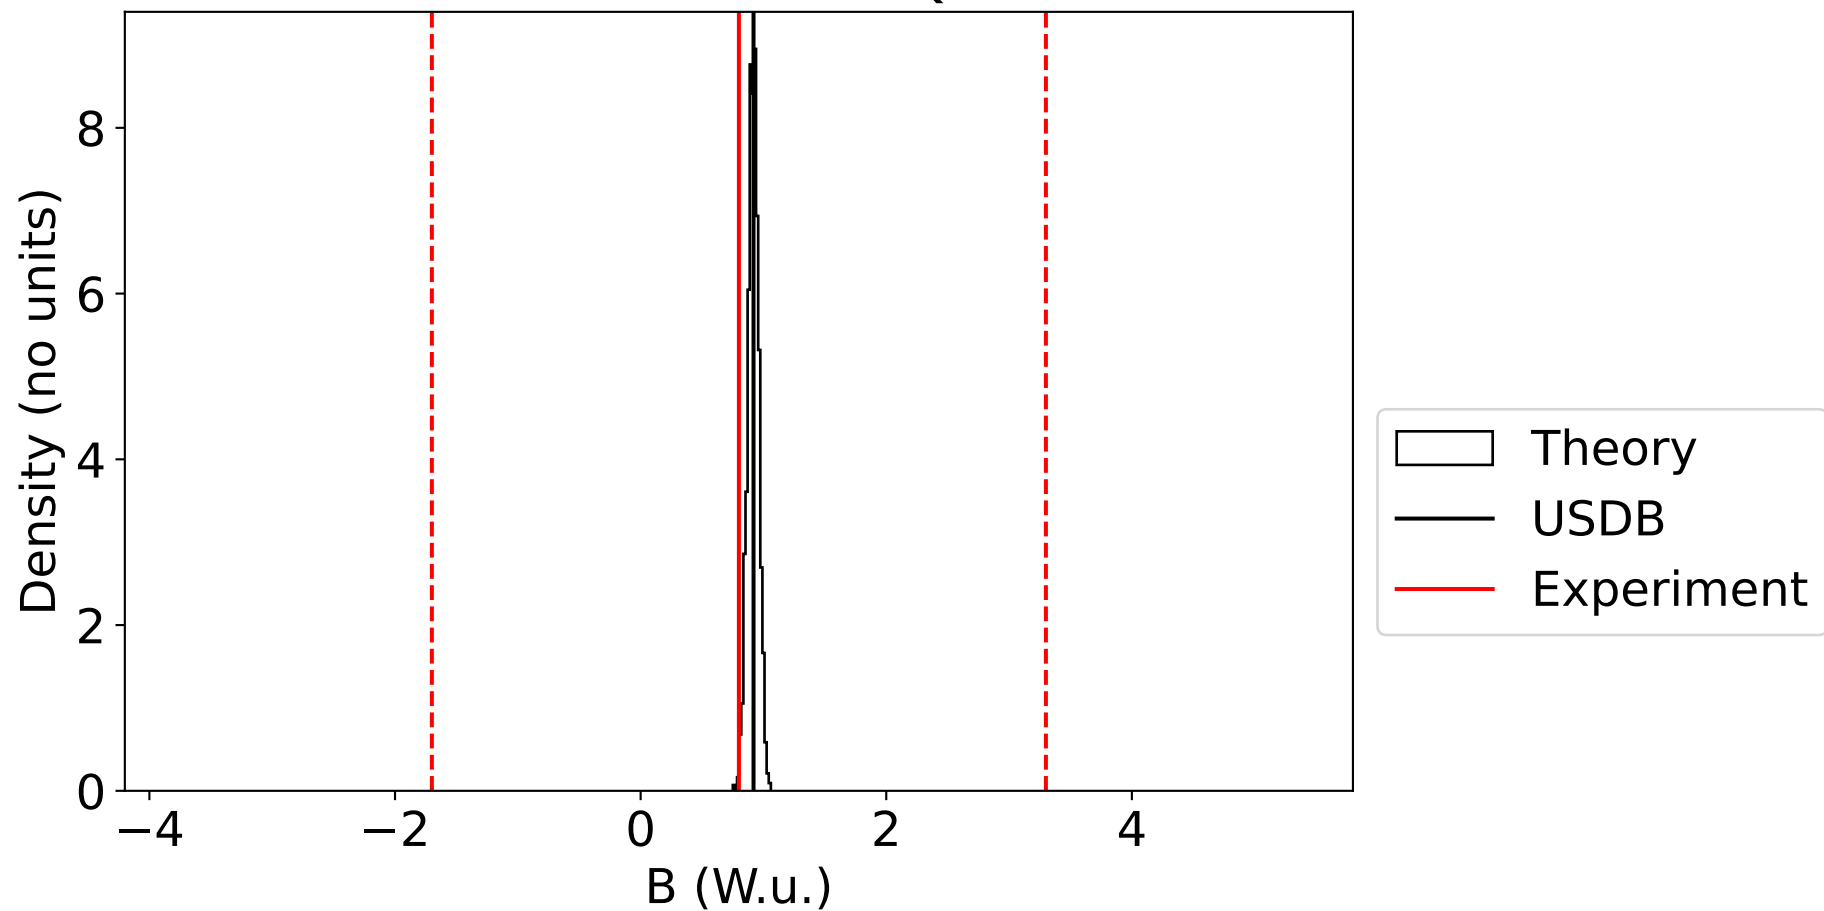

$^{22}\text{Na} (1_4) \rightarrow (0_1)$   
Included in UQ

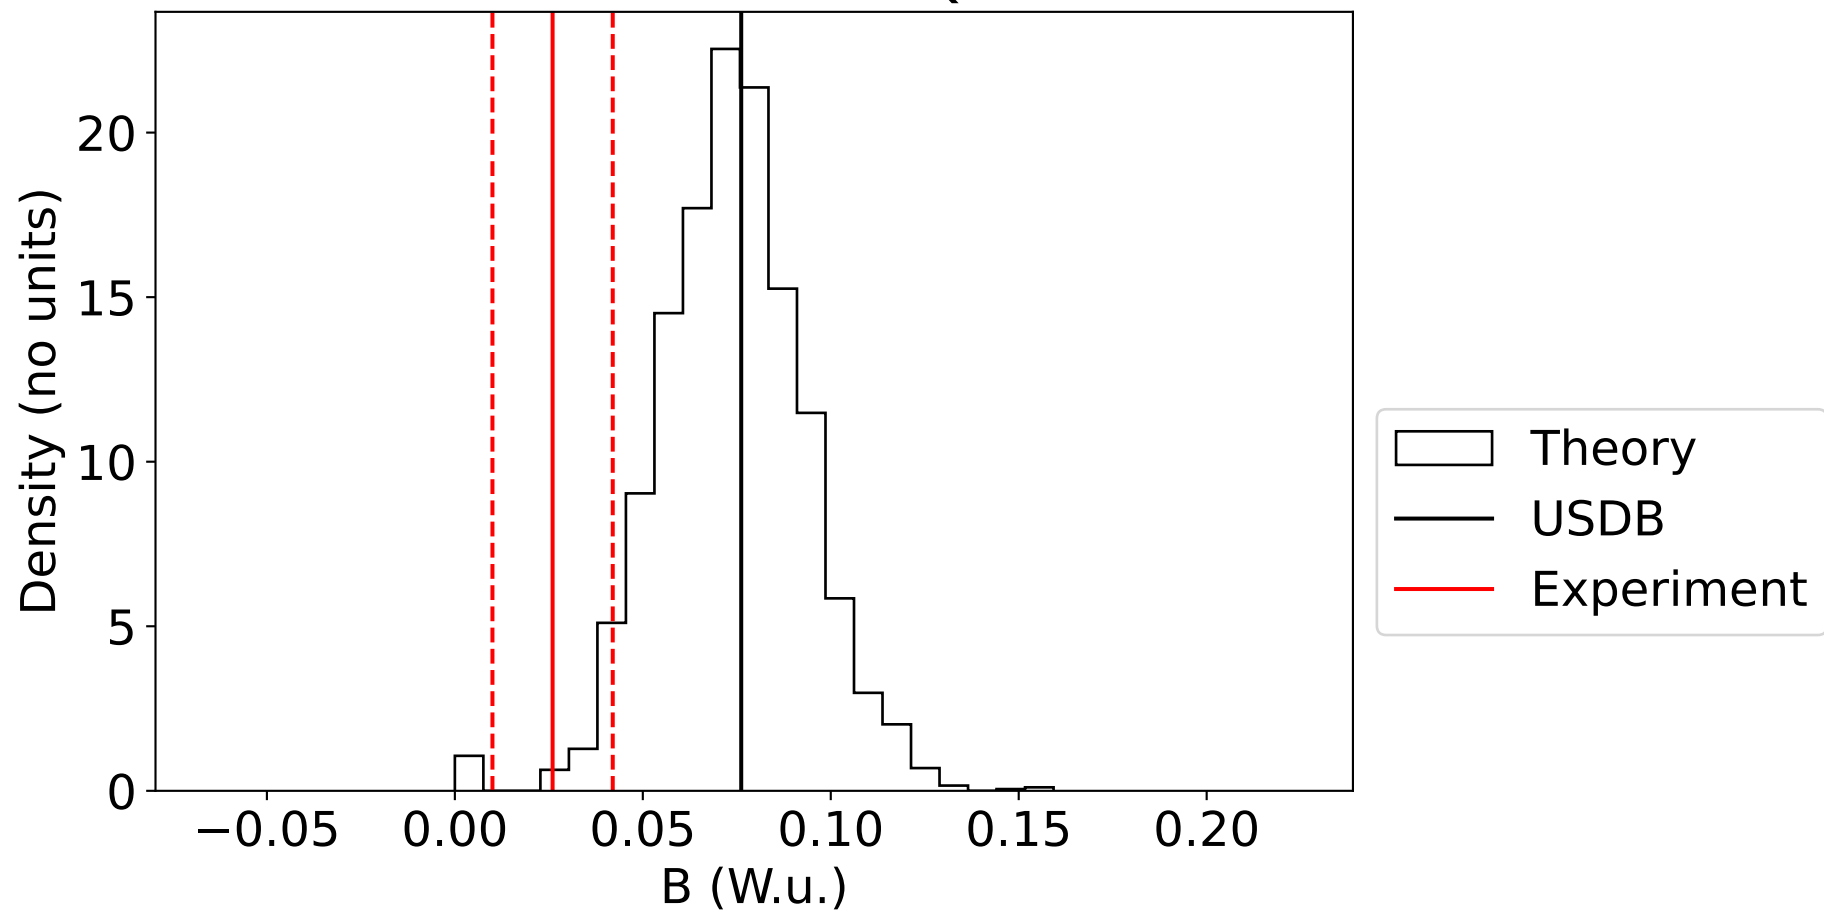

$^{22}\text{Na}$  ( $5_3$ )  $\rightarrow$  ( $4_2$ )  
Included in UQ

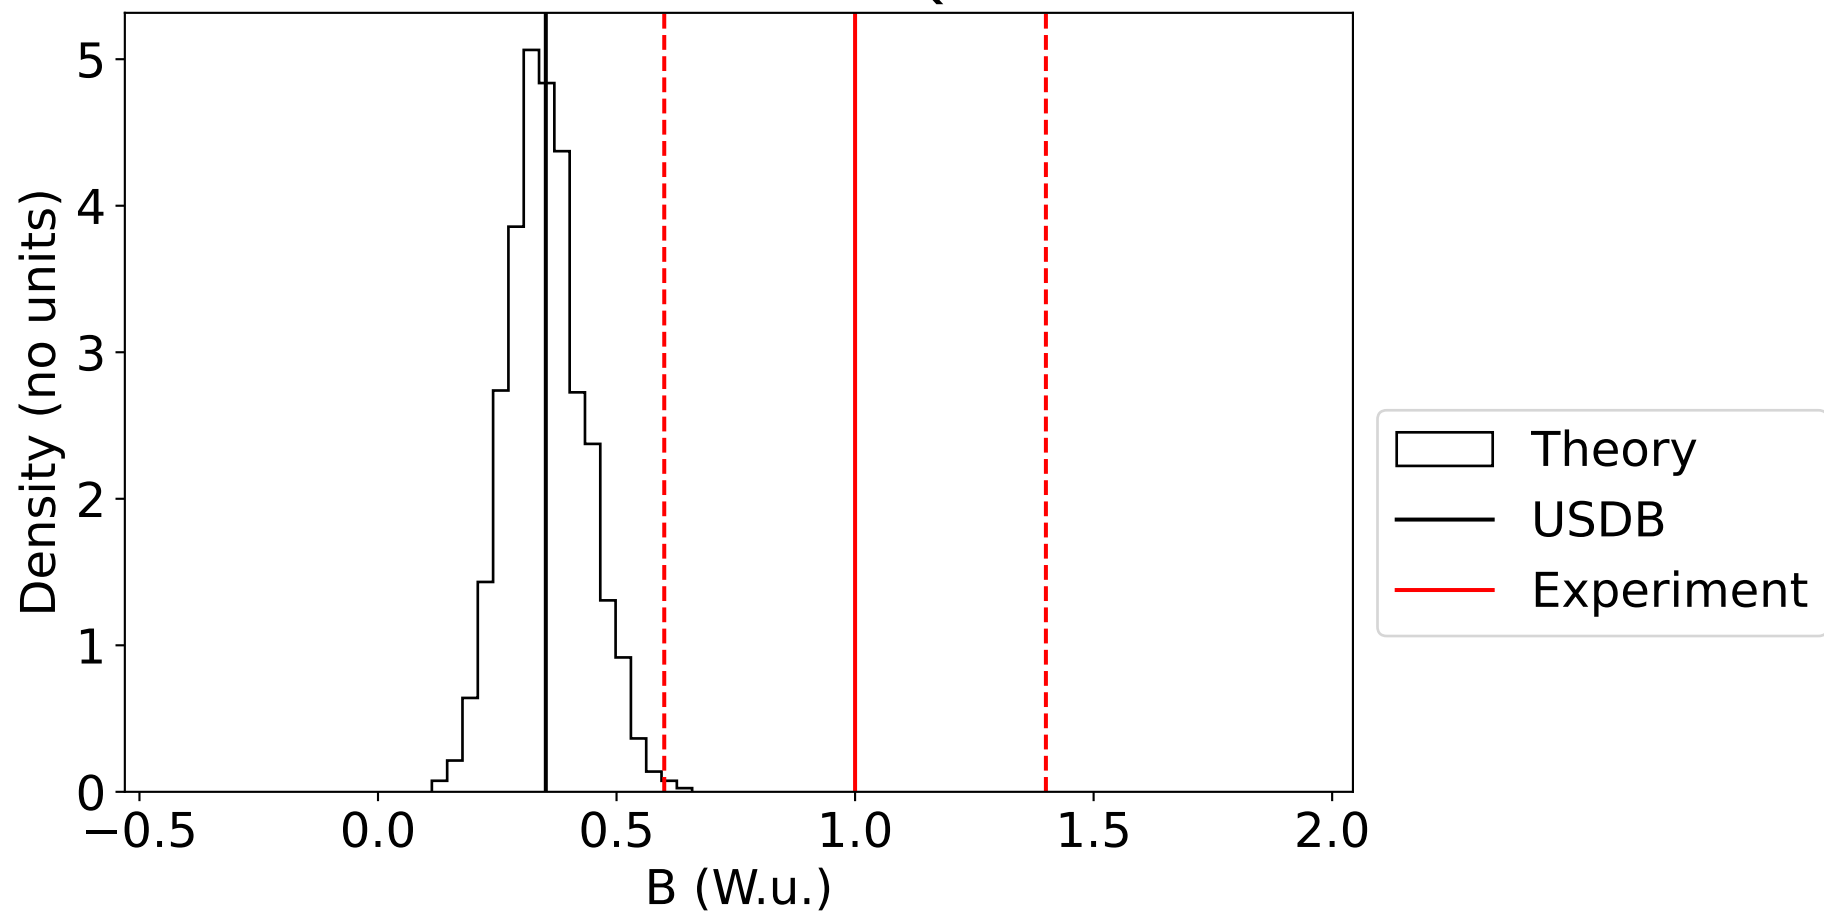



$^{22}\text{Na} (4_3) \rightarrow (4_2)$   
Included in UQ

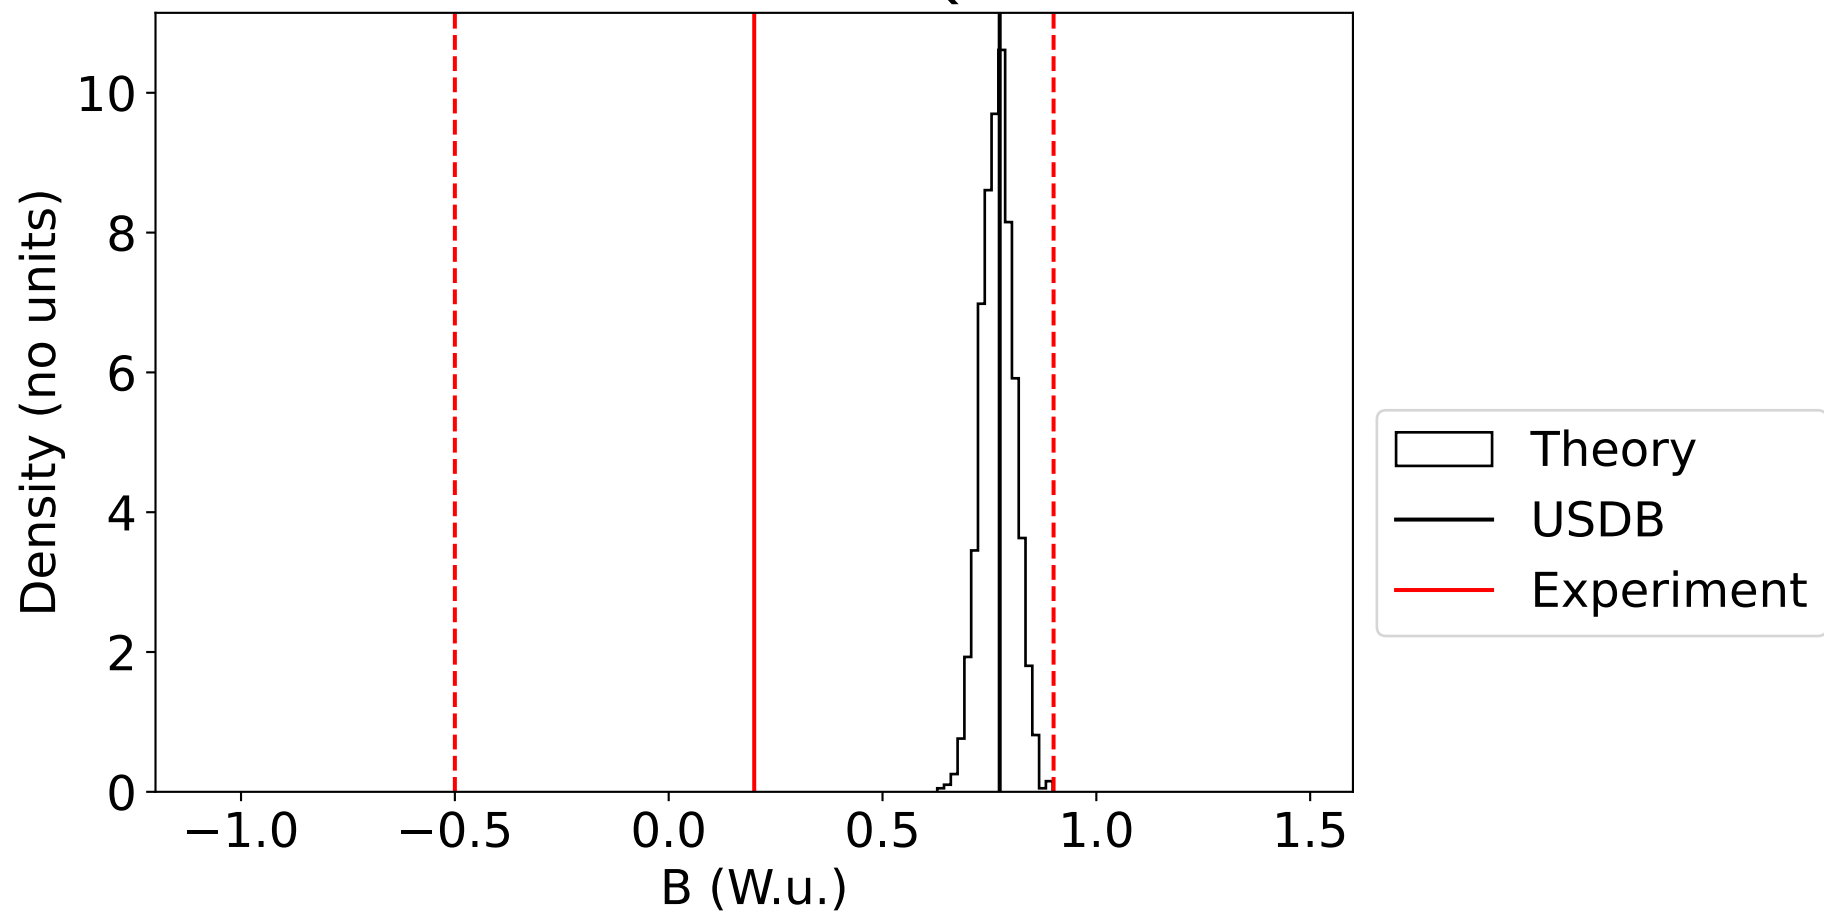

$^{23}\text{Na}$  ( $5/2_1$ )  $\rightarrow$  ( $3/2_1$ )  
Included in UQ

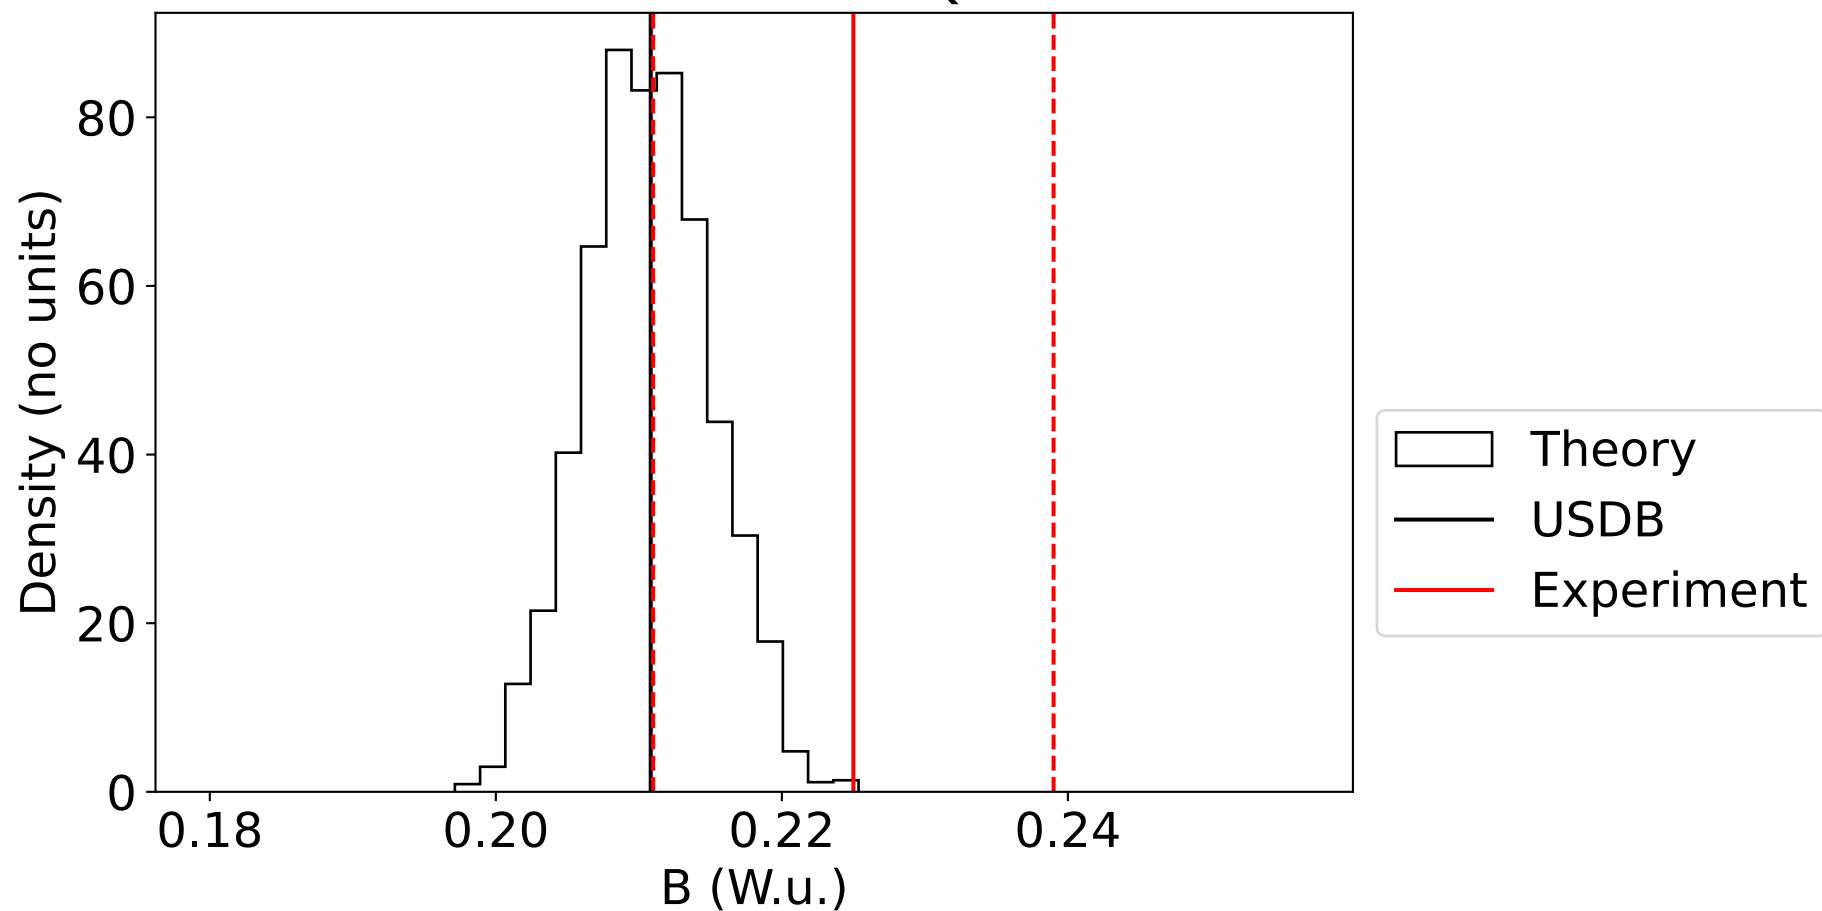

$^{23}\text{Na}$  ( $7/2_1$ )  $\rightarrow$  ( $5/2_1$ )  
Included in UQ

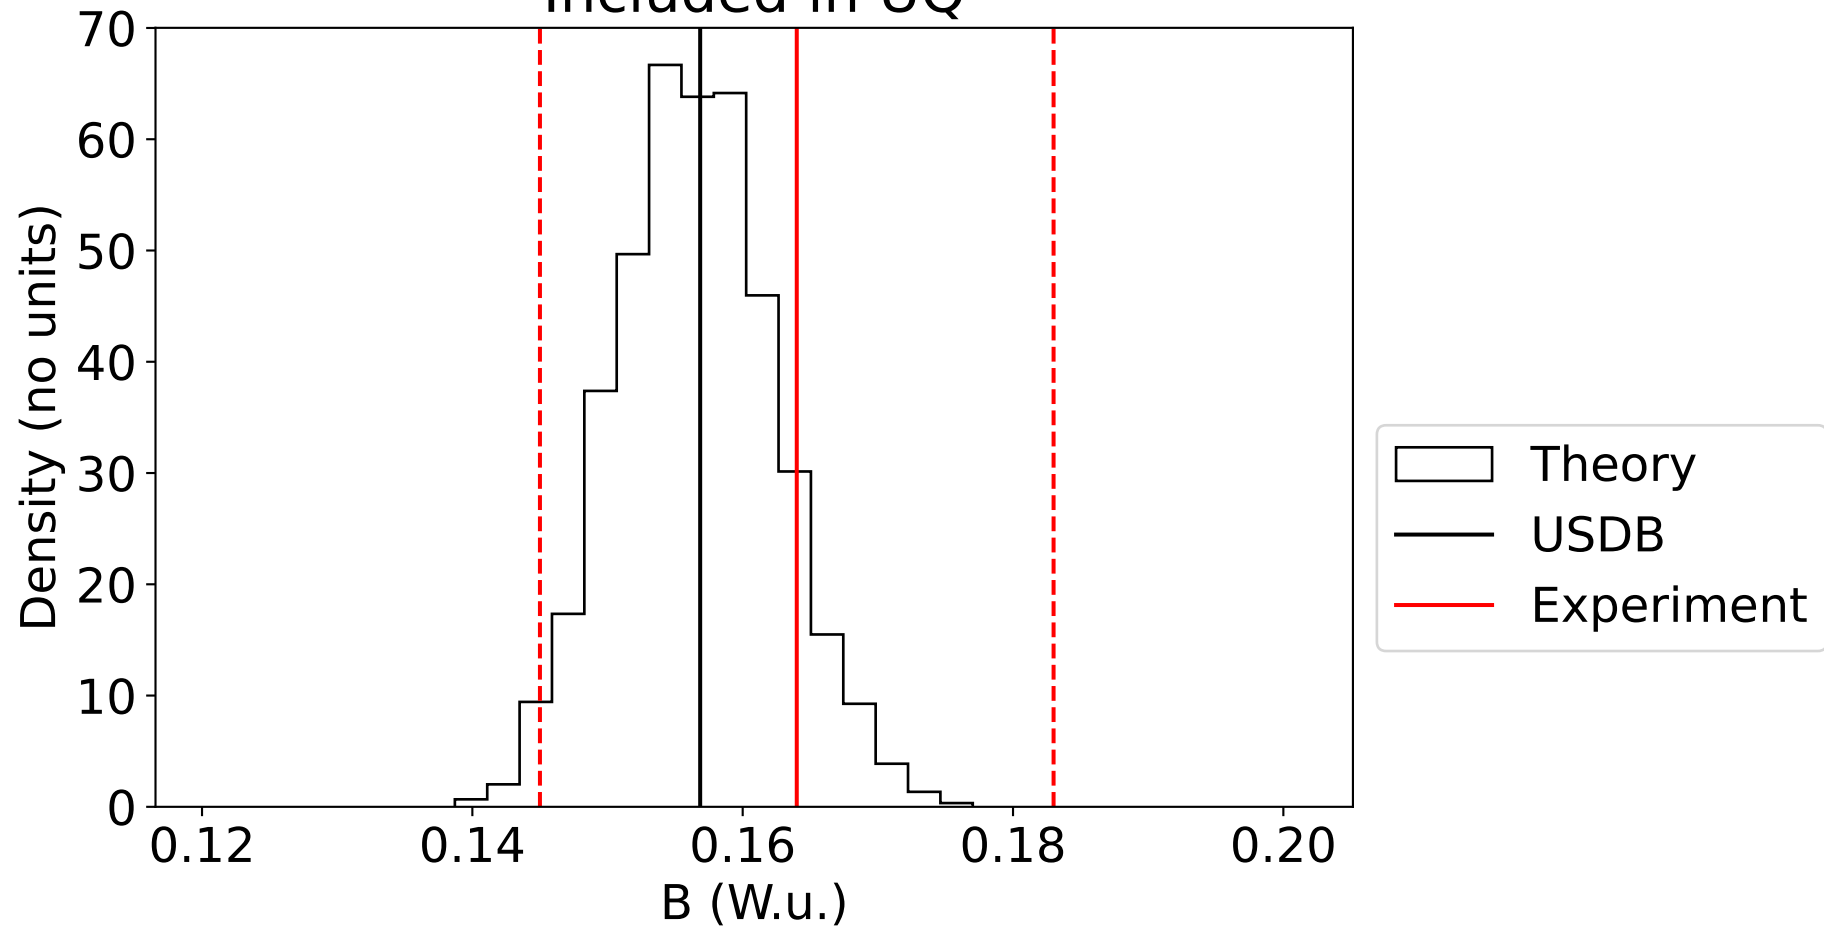

$^{23}\text{Na } (9/2_1) \rightarrow (7/2_1)$   
Included in UQ

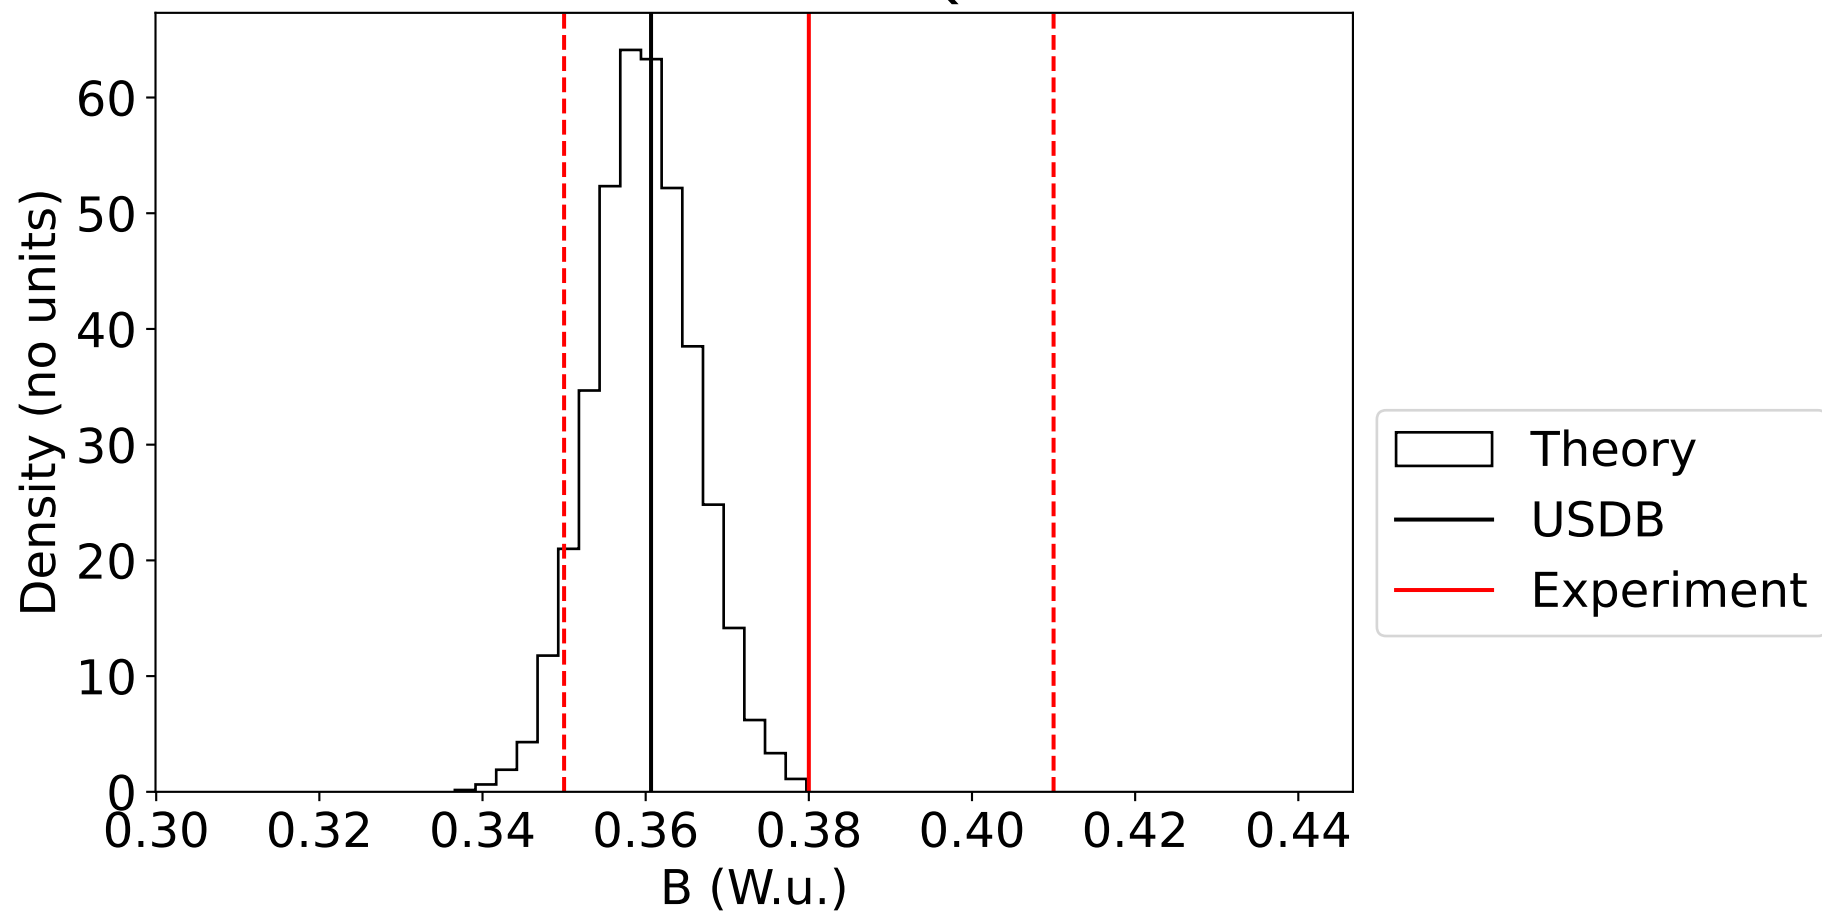

$^{23}\text{Na}$  ( $3/2_2$ )  $\rightarrow$  ( $1/2_1$ )  
Included in UQ

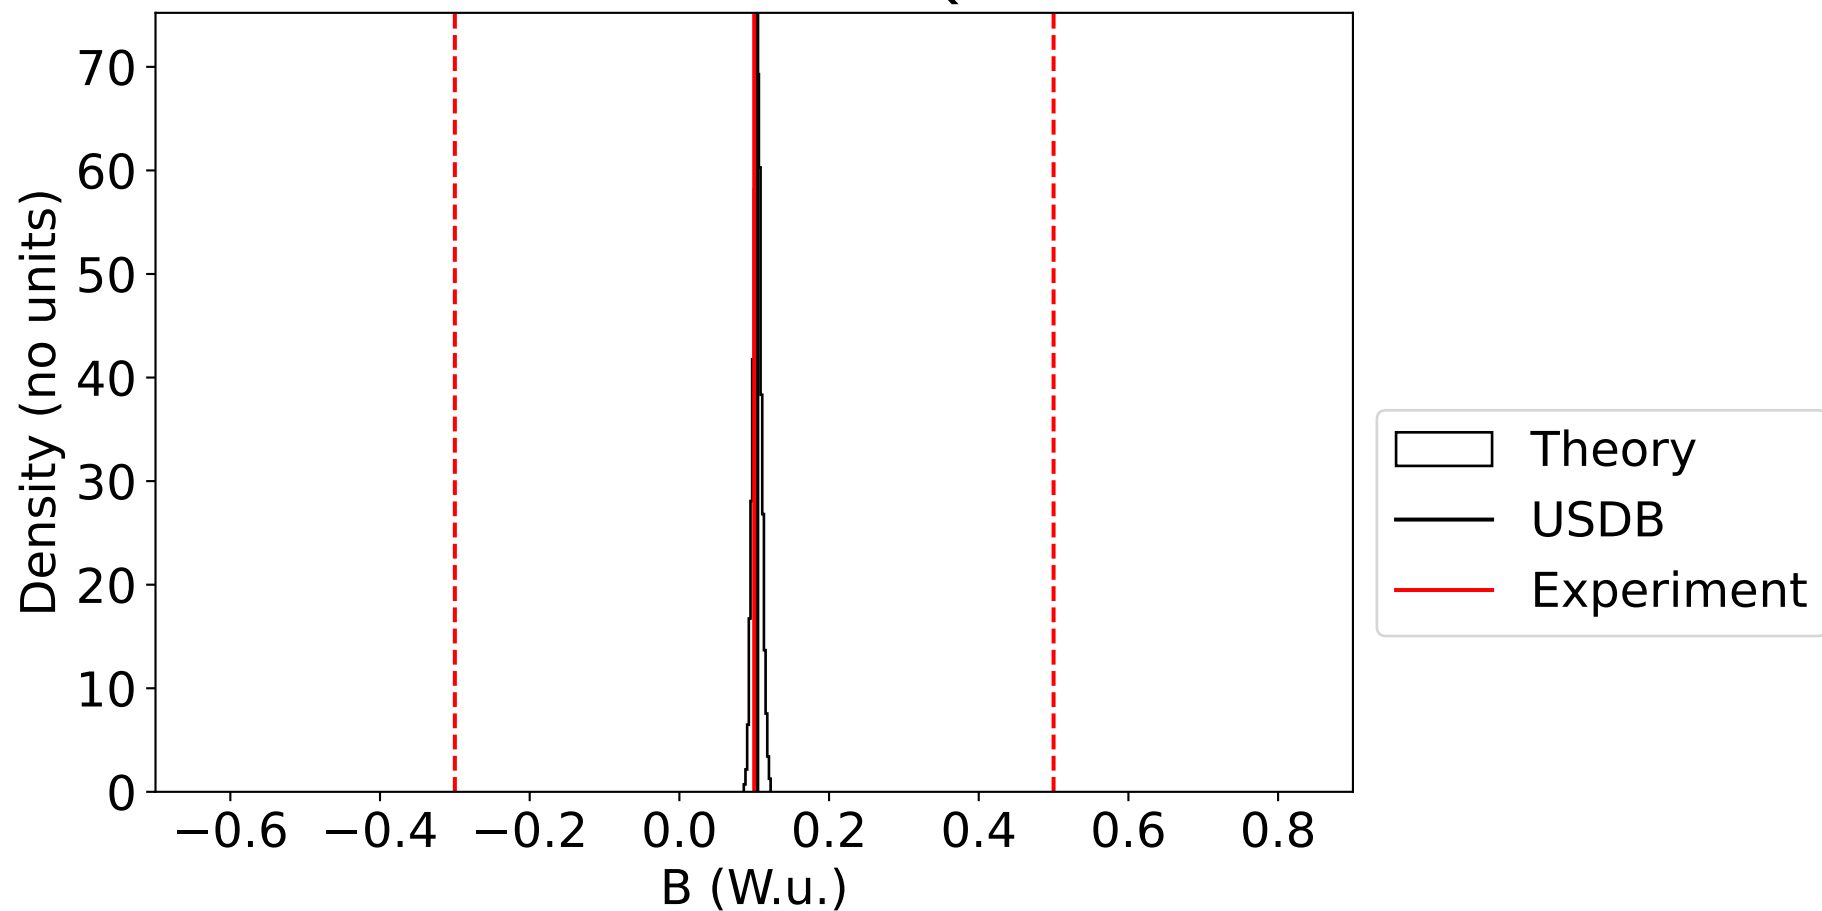

$^{23}\text{Na}$  ( $3/2_2$ )  $\rightarrow$  ( $3/2_1$ )  
Included in UQ

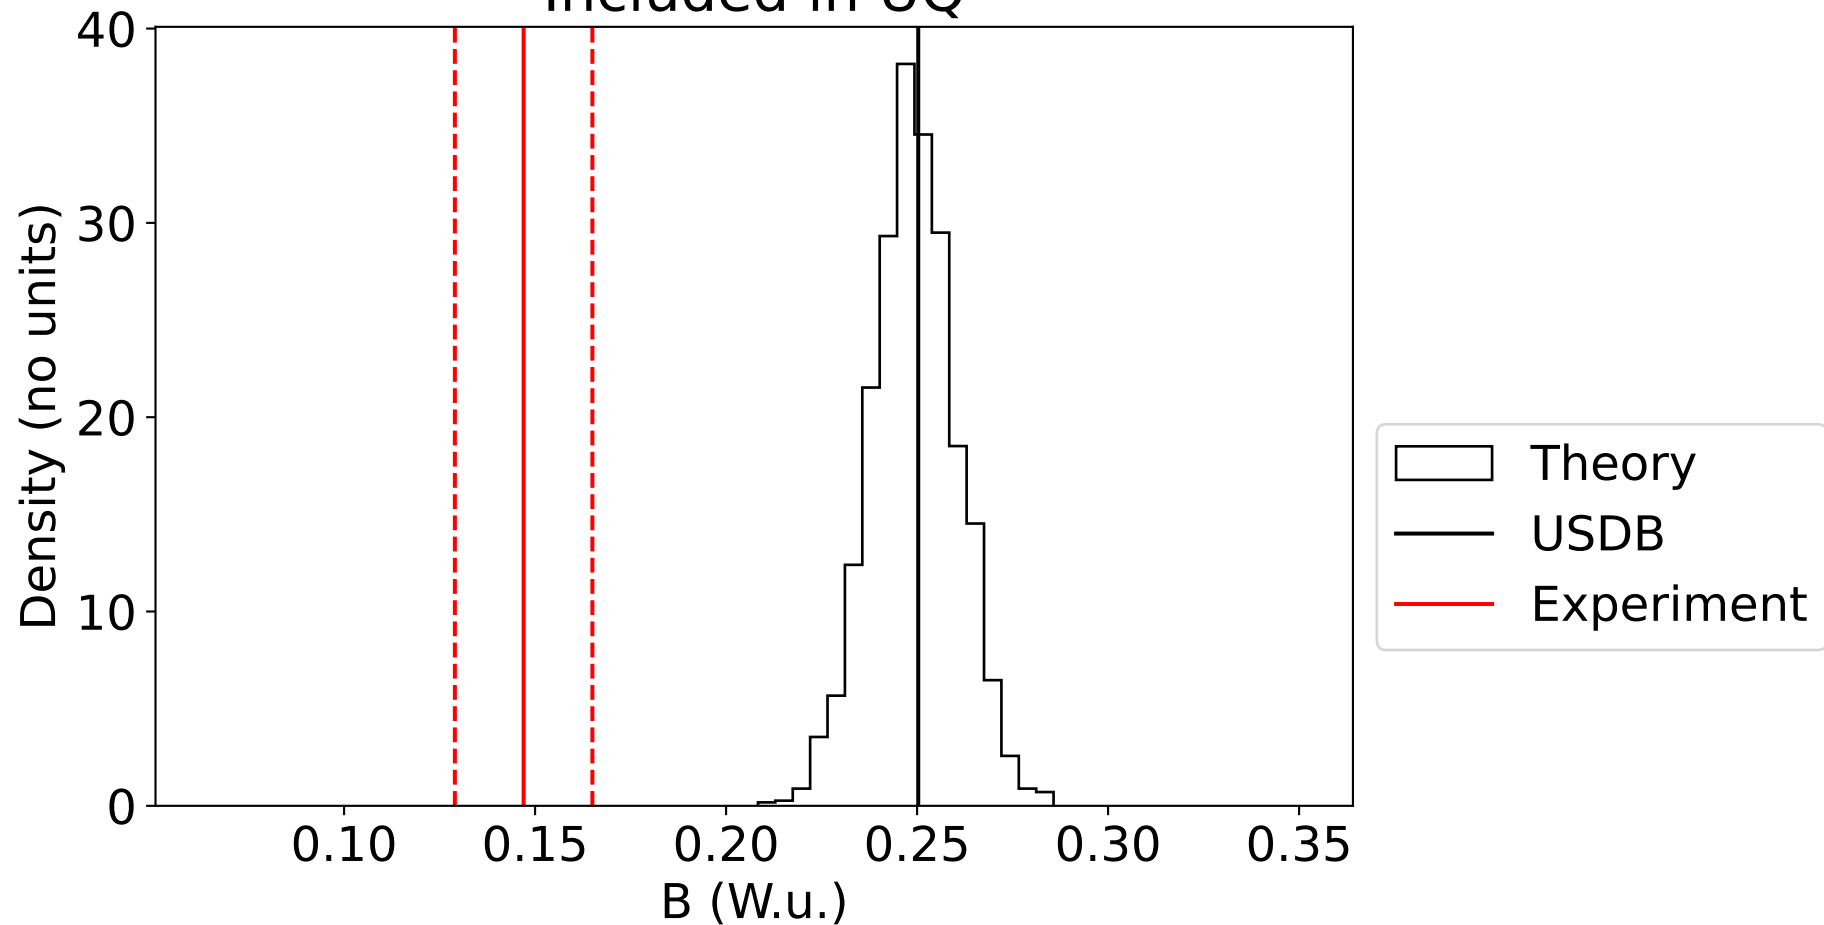

$^{23}\text{Na}$  ( $3/2_2$ )  $\rightarrow$  ( $5/2_1$ )  
Included in UQ

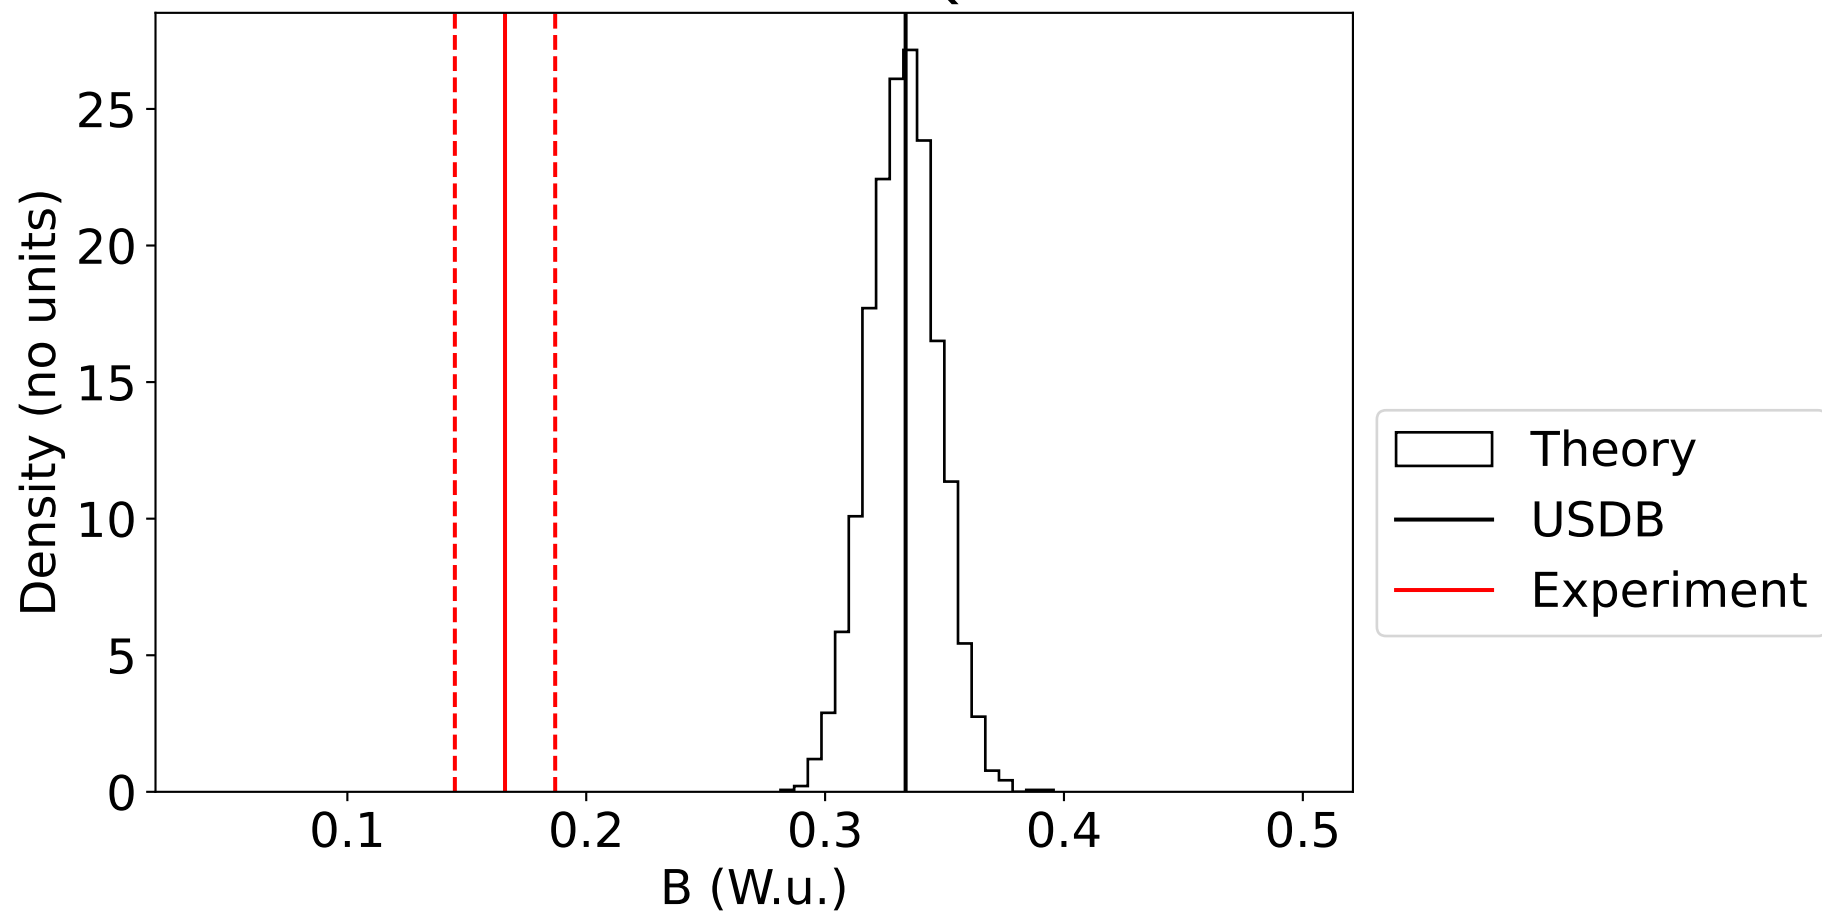

$^{23}\text{Na}$  ( $5/2_2$ )  $\rightarrow$  ( $3/2_1$ )  
Included in UQ

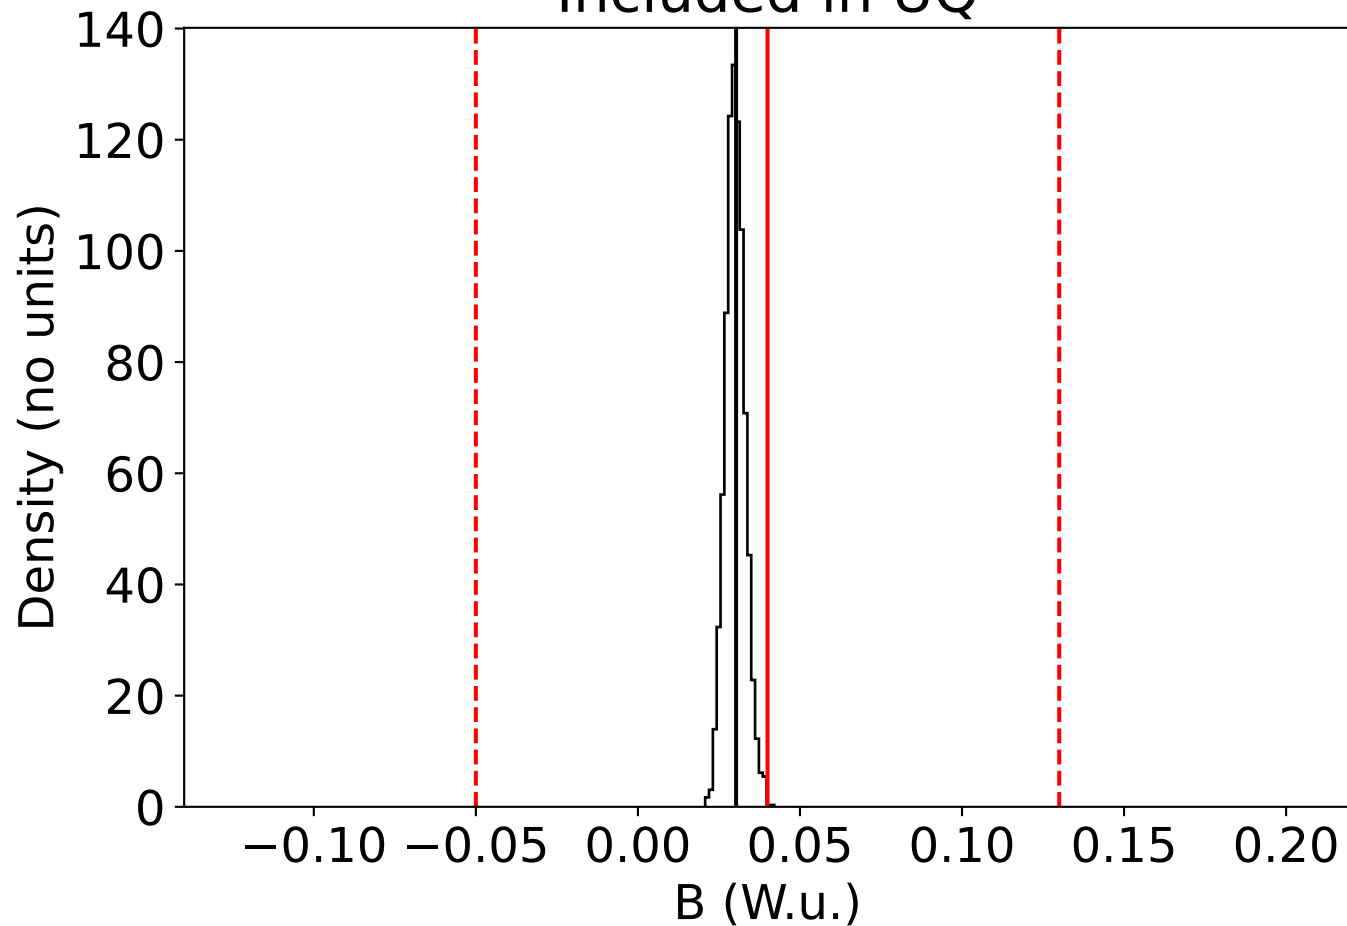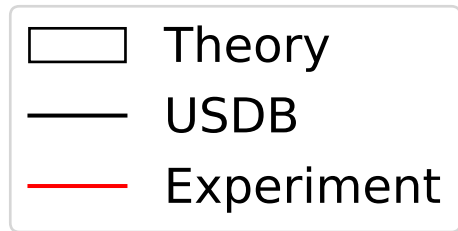



$^{23}\text{Na}$  ( $5/2_2$ )  $\rightarrow$  ( $7/2_1$ )  
Included in UQ

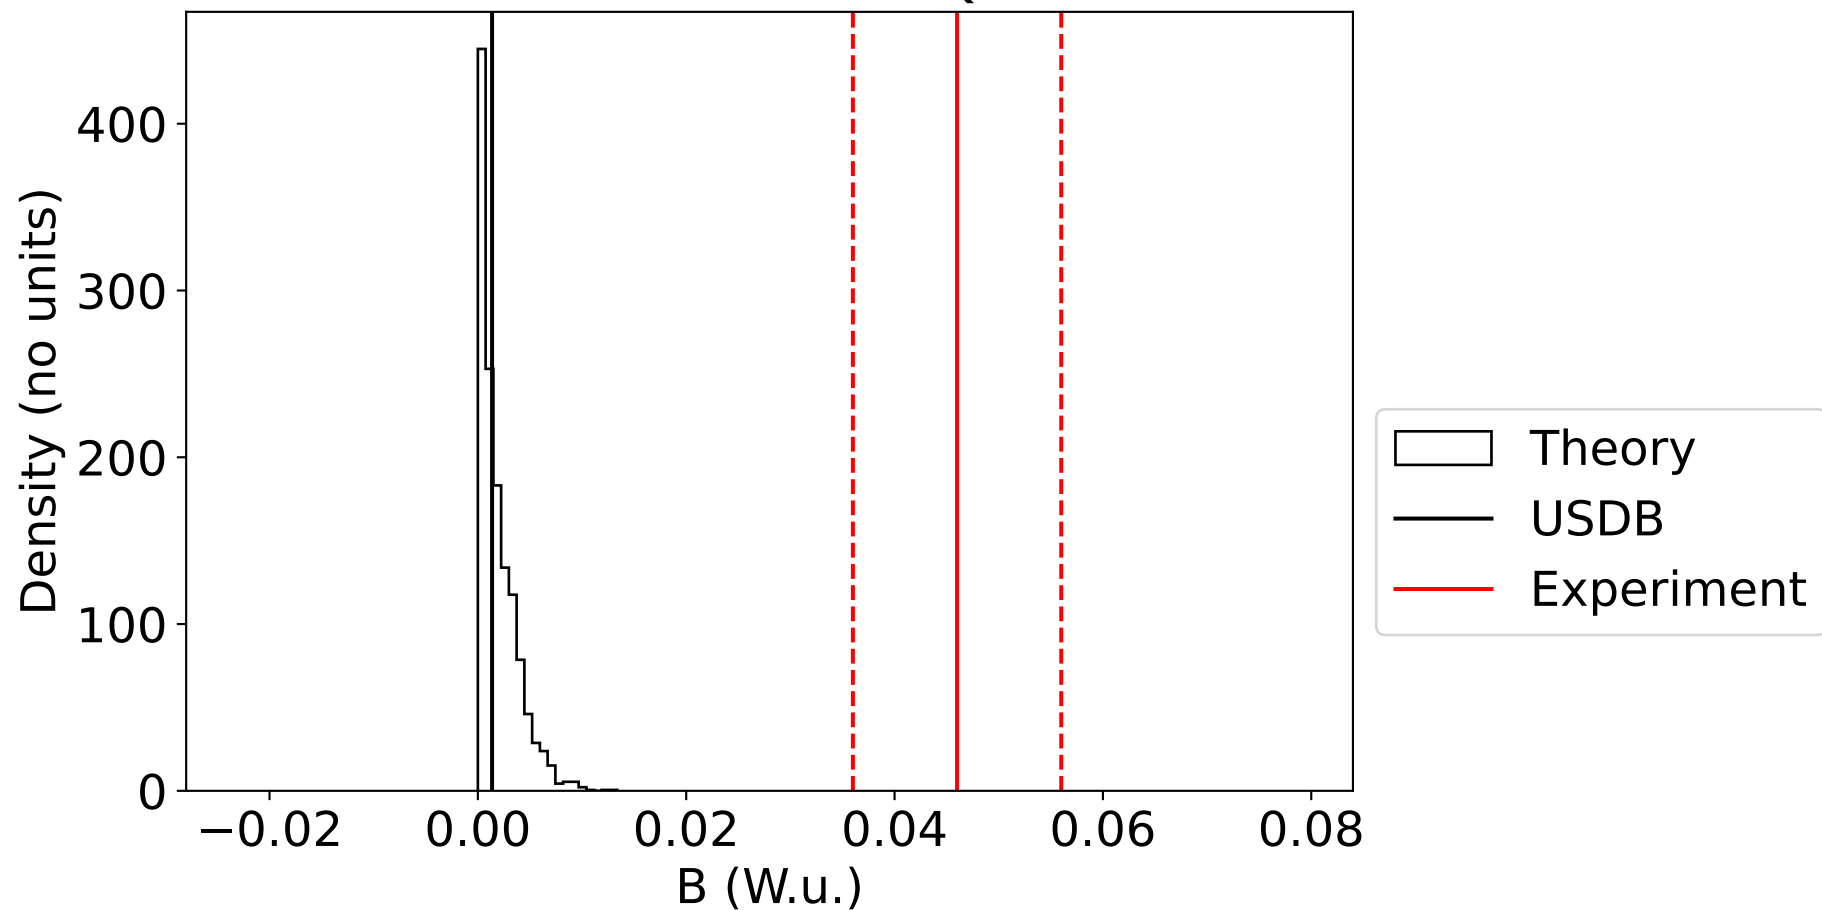

$^{23}\text{Na } (5/2_2) \rightarrow (3/2_2)$   
Included in UQ

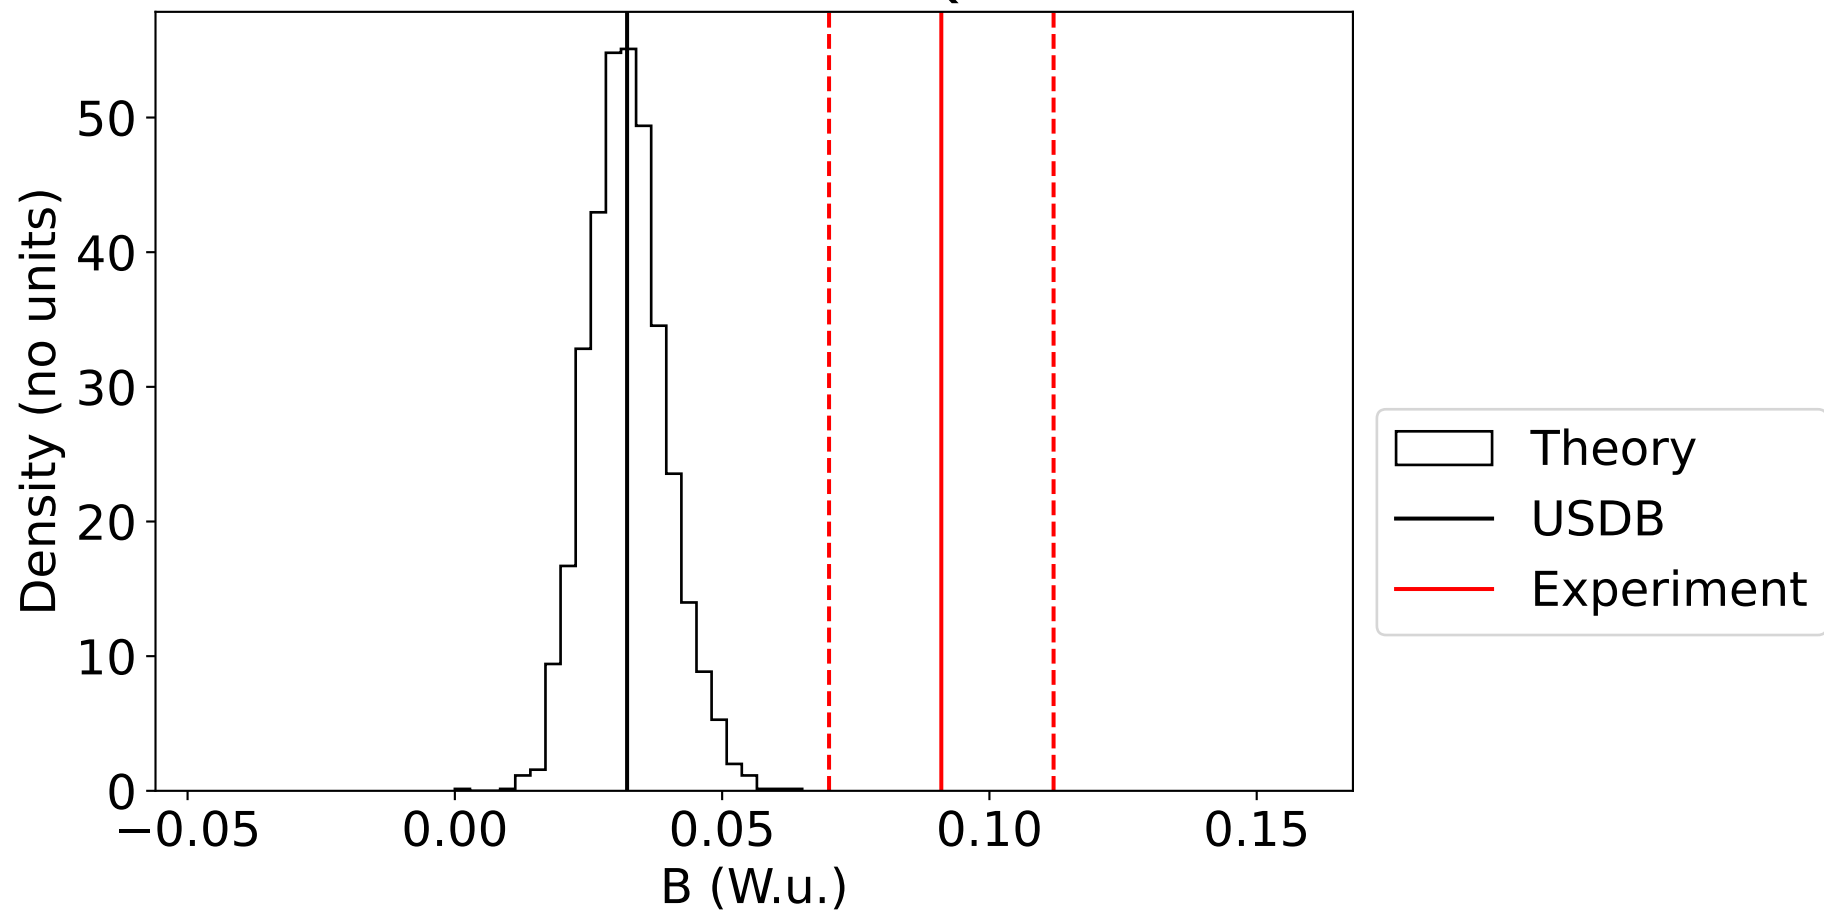

$^{23}\text{Na } (1/2_2) \rightarrow (3/2_1)$   
Included in UQ

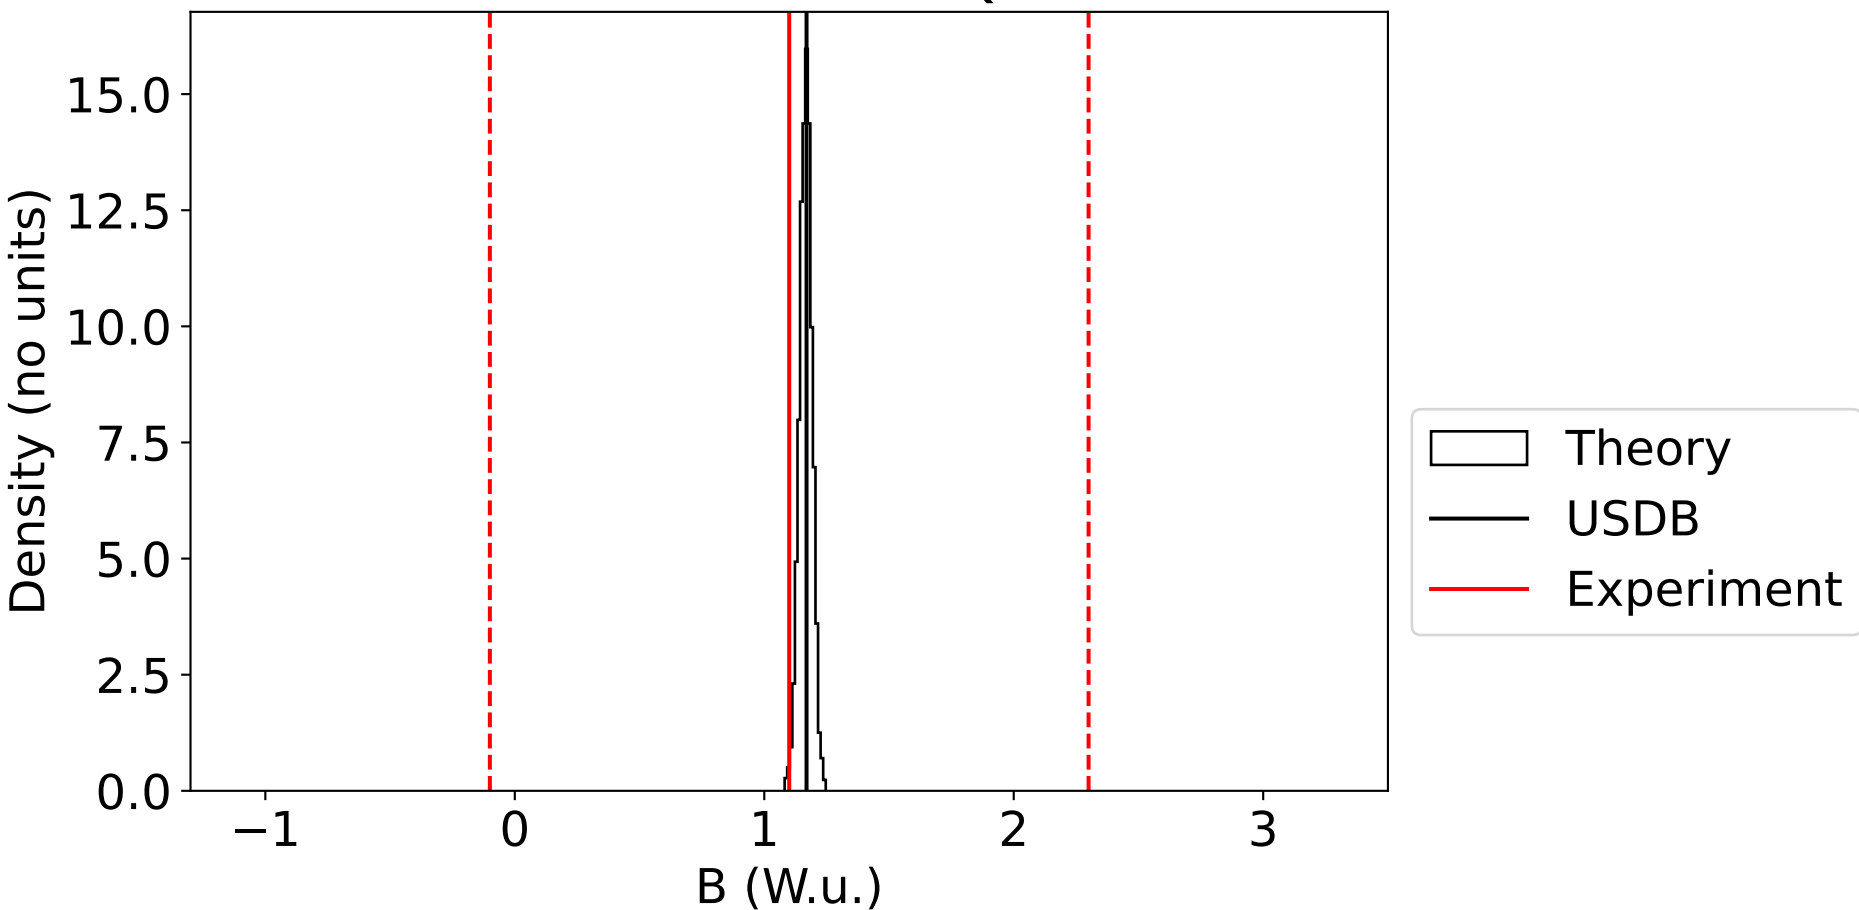

$^{23}\text{Na}$  ( $1/2_2 \rightarrow 1/2_1$ )  
Included in UQ

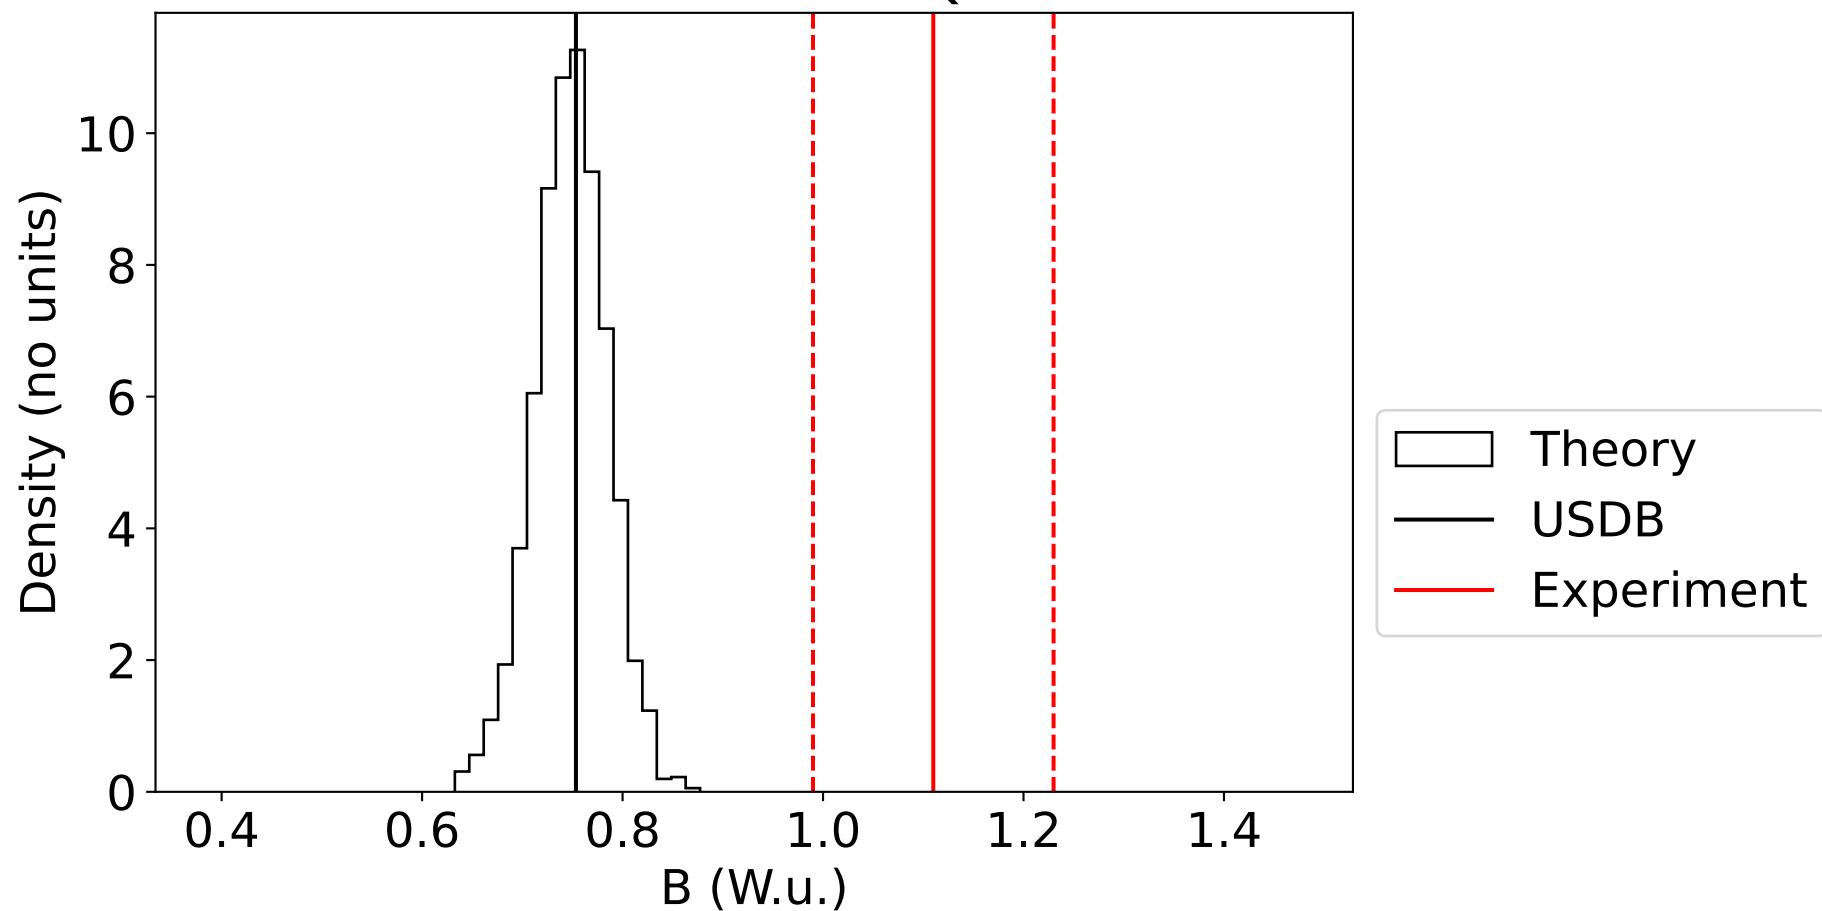

$^{23}\text{Na}$  ( $5/2_3$ )  $\rightarrow$  ( $7/2_1$ )  
Included in UQ

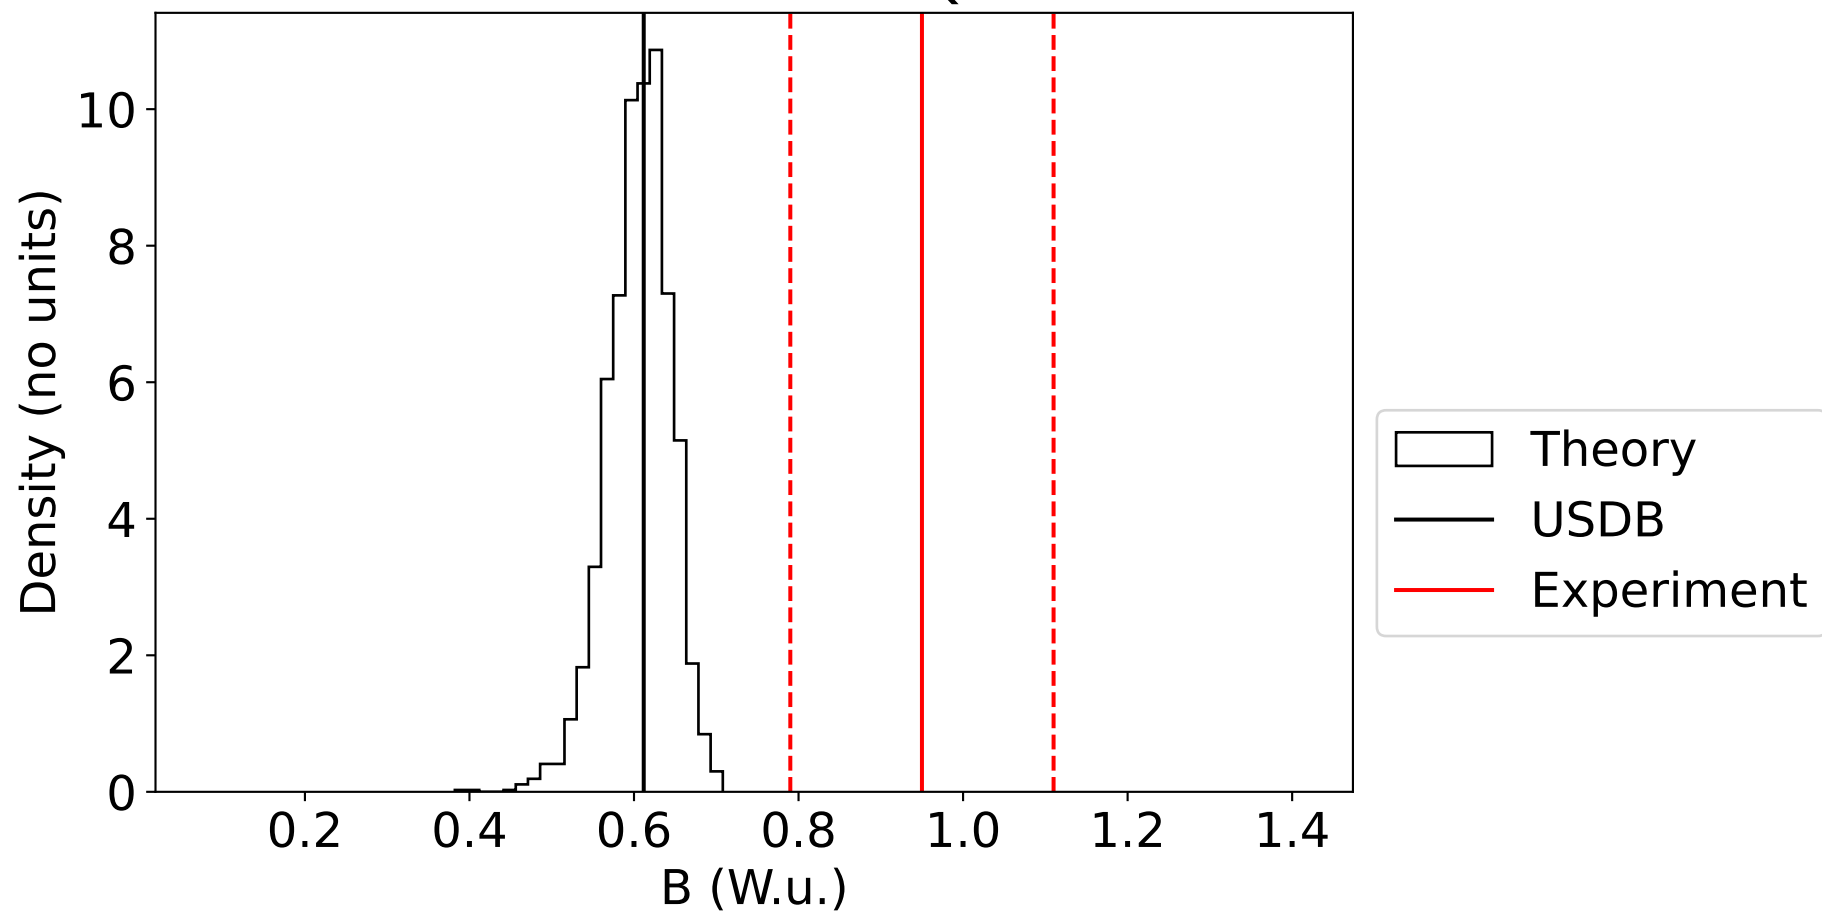

$^{23}\text{Na}$  ( $5/2_3$ )  $\rightarrow$  ( $5/2_1$ )  
Included in UQ

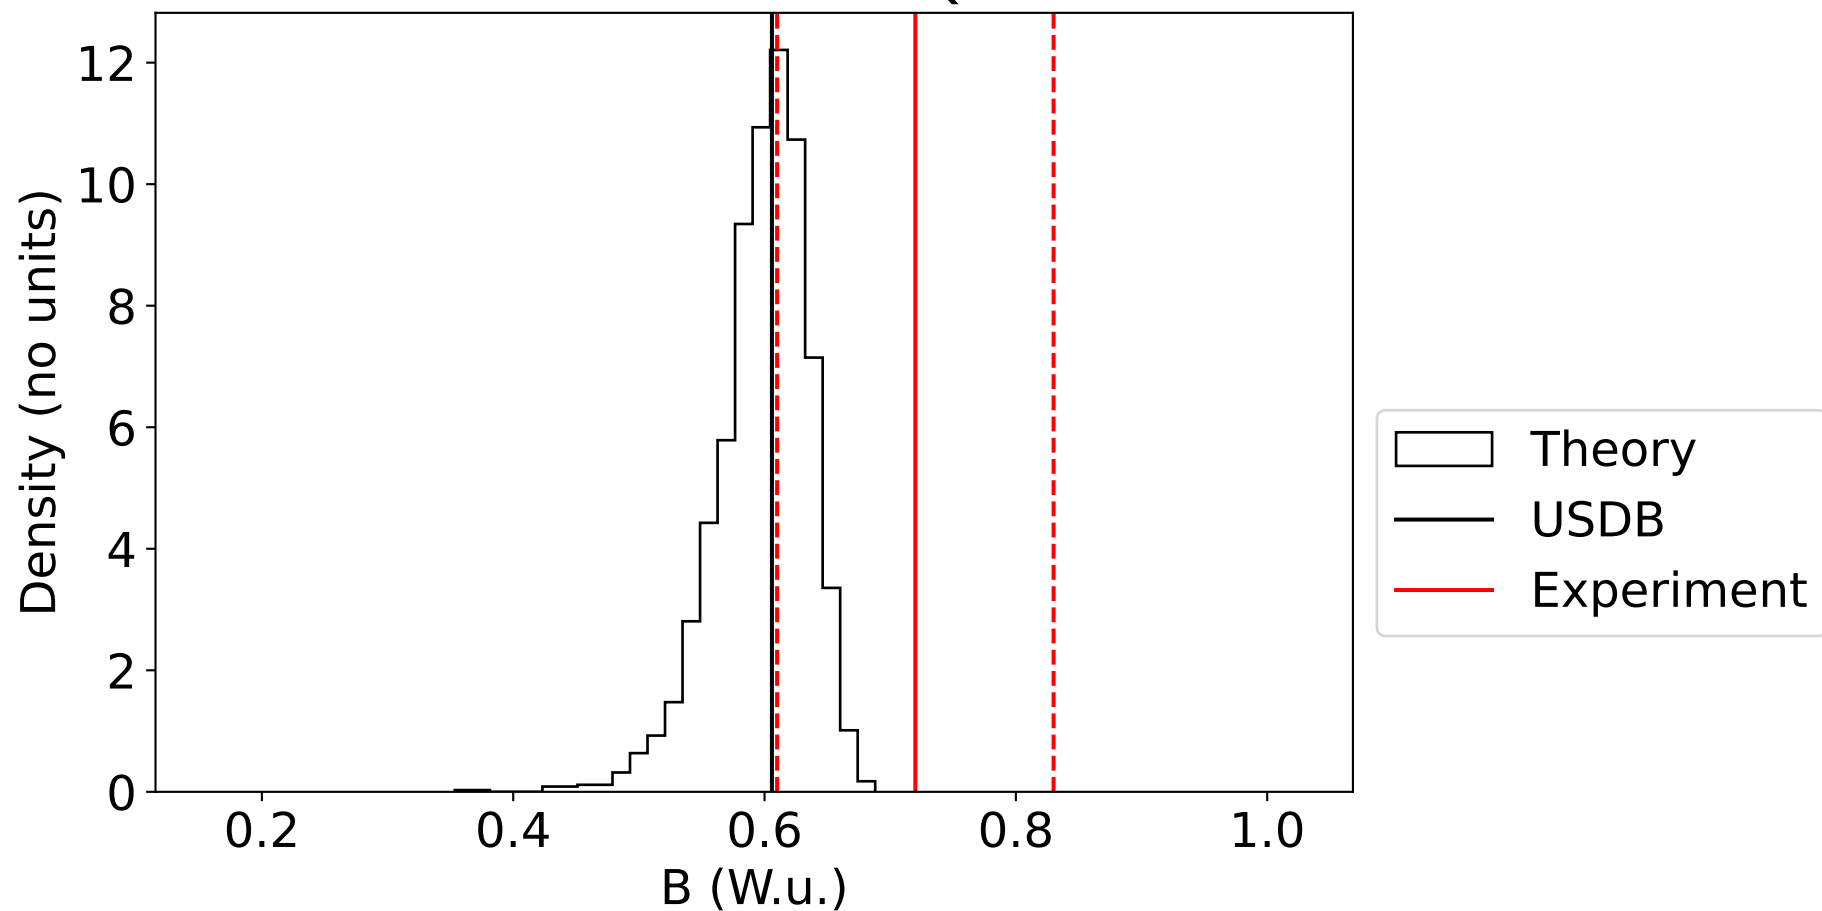

$^{23}\text{Na}$  ( $11/2_1$ )  $\rightarrow$  ( $9/2_1$ )  
Included in UQ

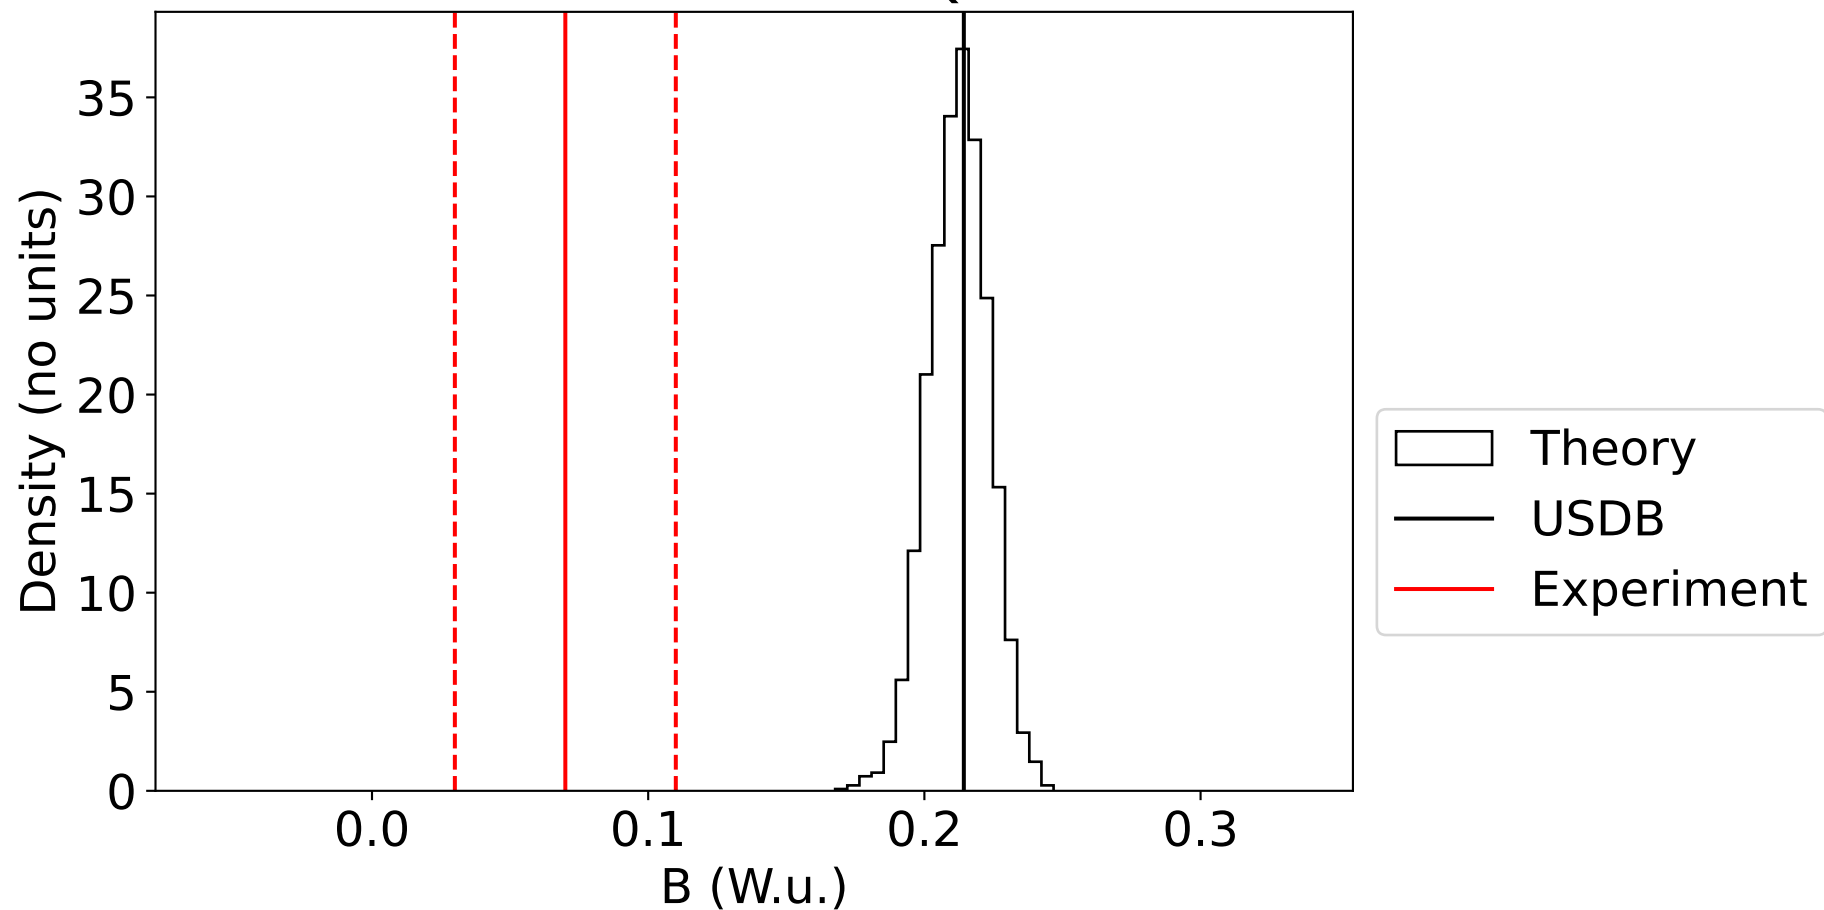

$^{23}\text{Na}$  ( $7/2_3 \rightarrow 5/2_2$ )  
Included in UQ

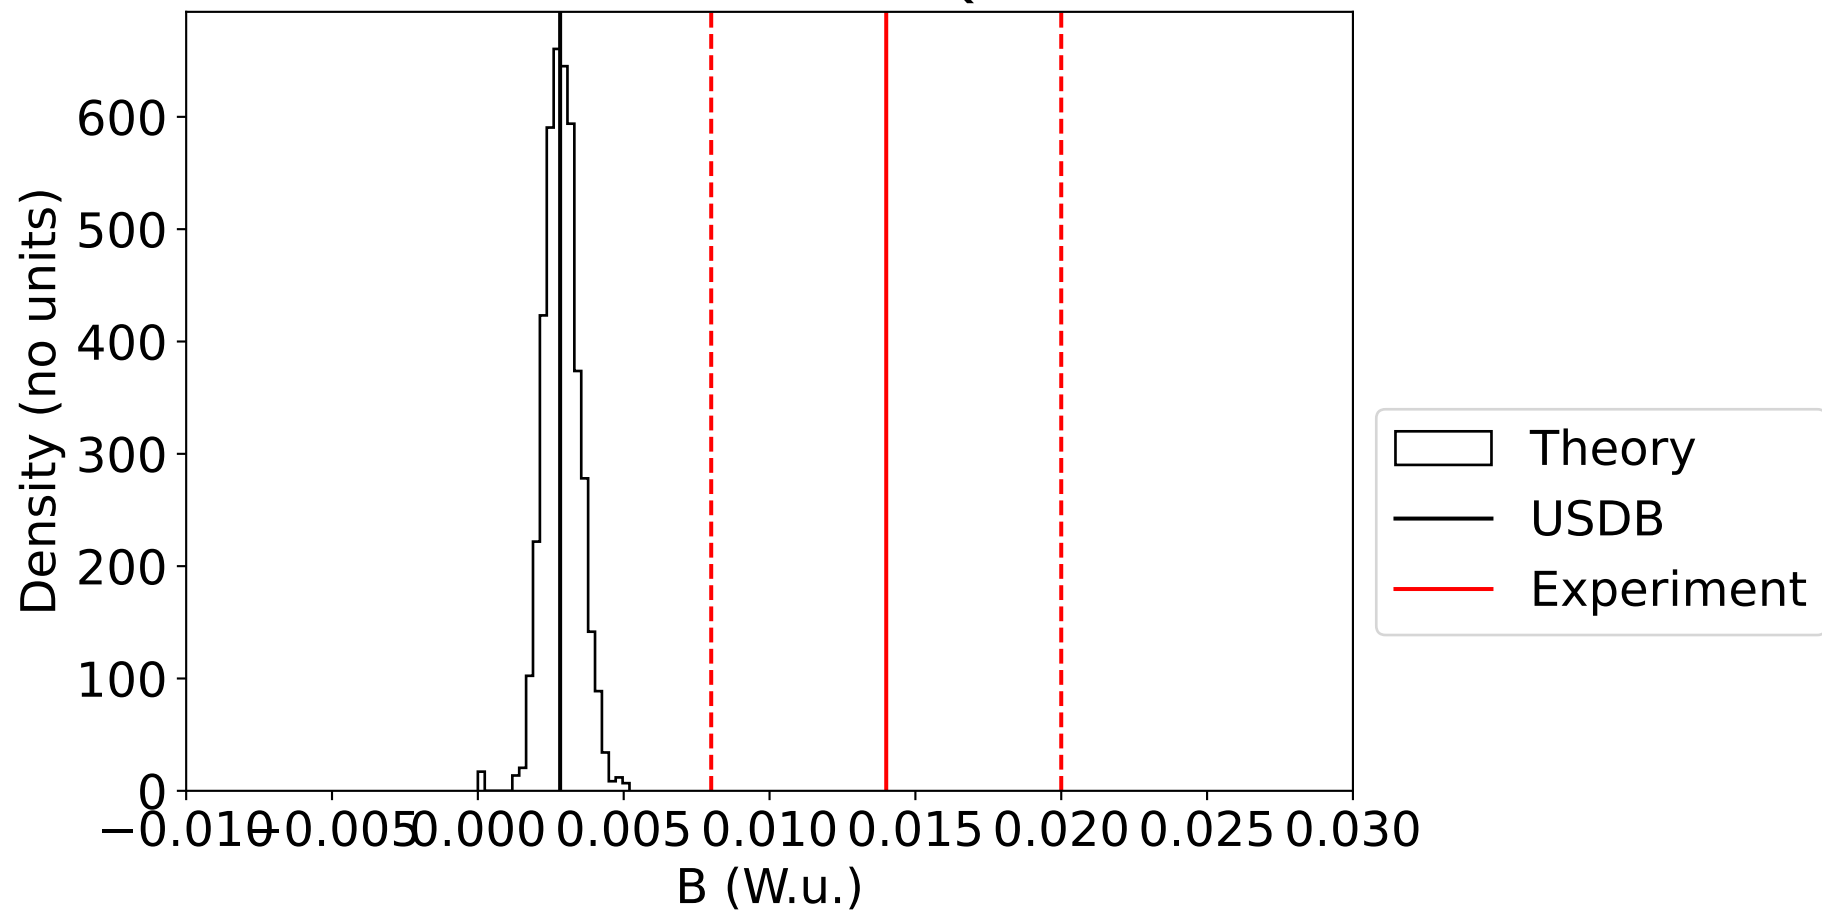



$^{23}\text{Na} (11/2_2) \rightarrow (9/2_1)$   
Included in UQ

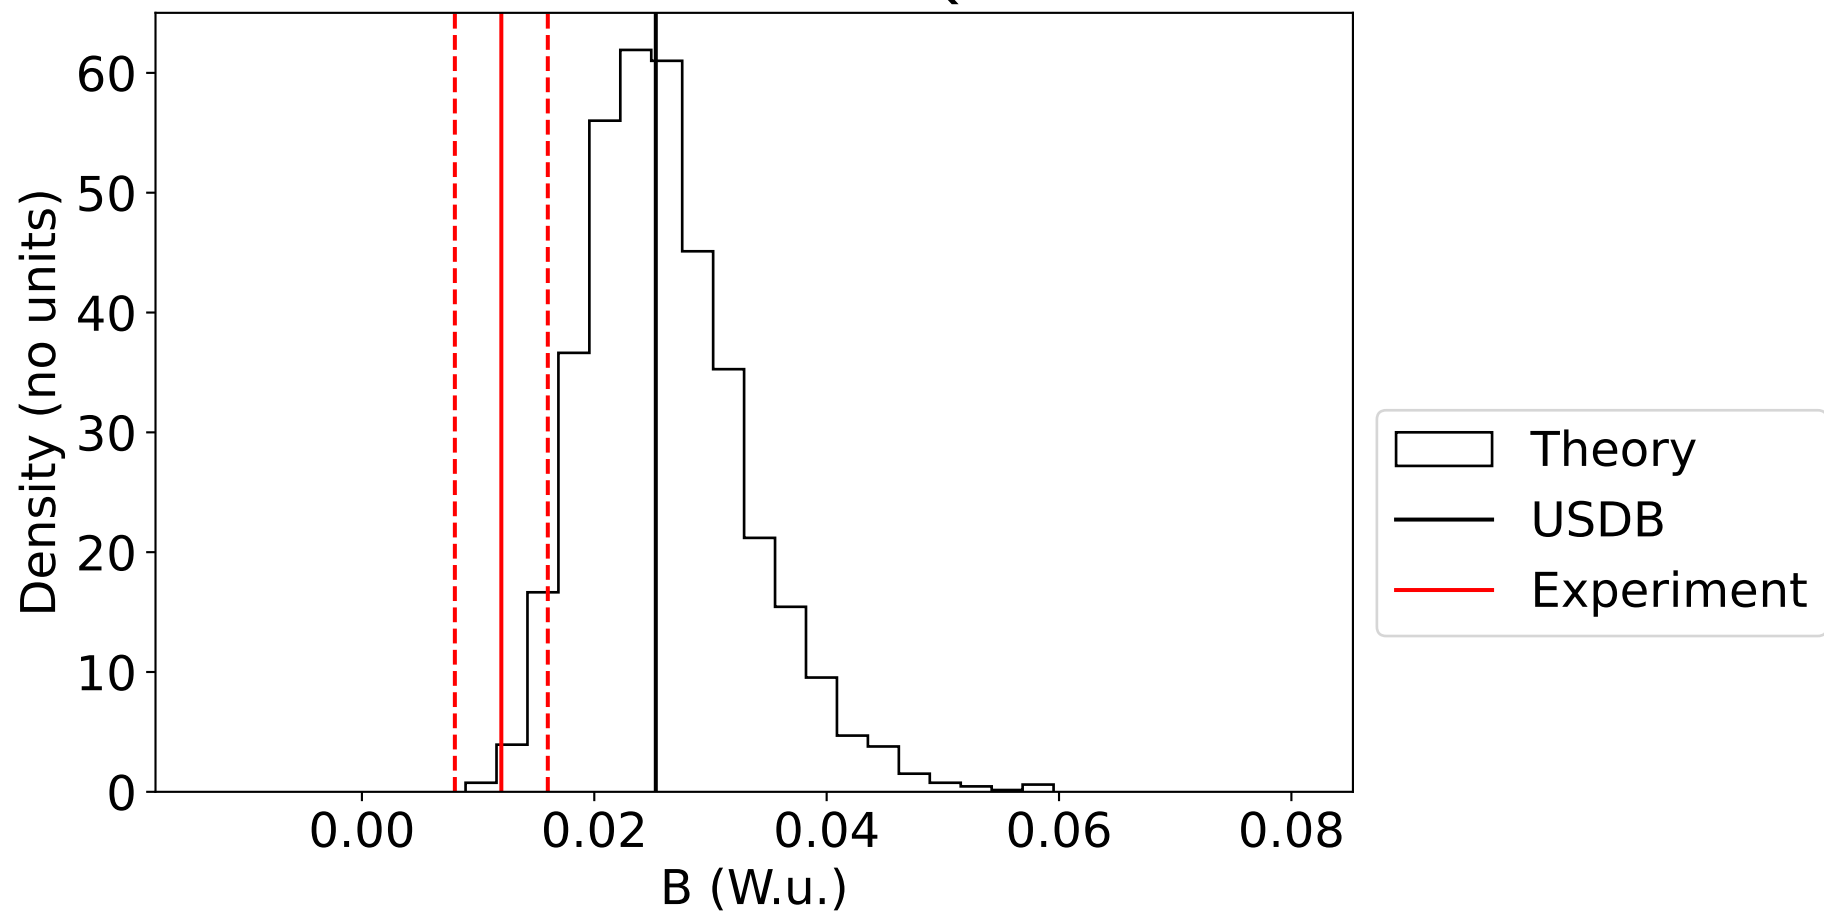

$^{23}\text{Na}$  ( $13/2_1$ )  $\rightarrow$  ( $11/2_1$ )  
Included in UQ

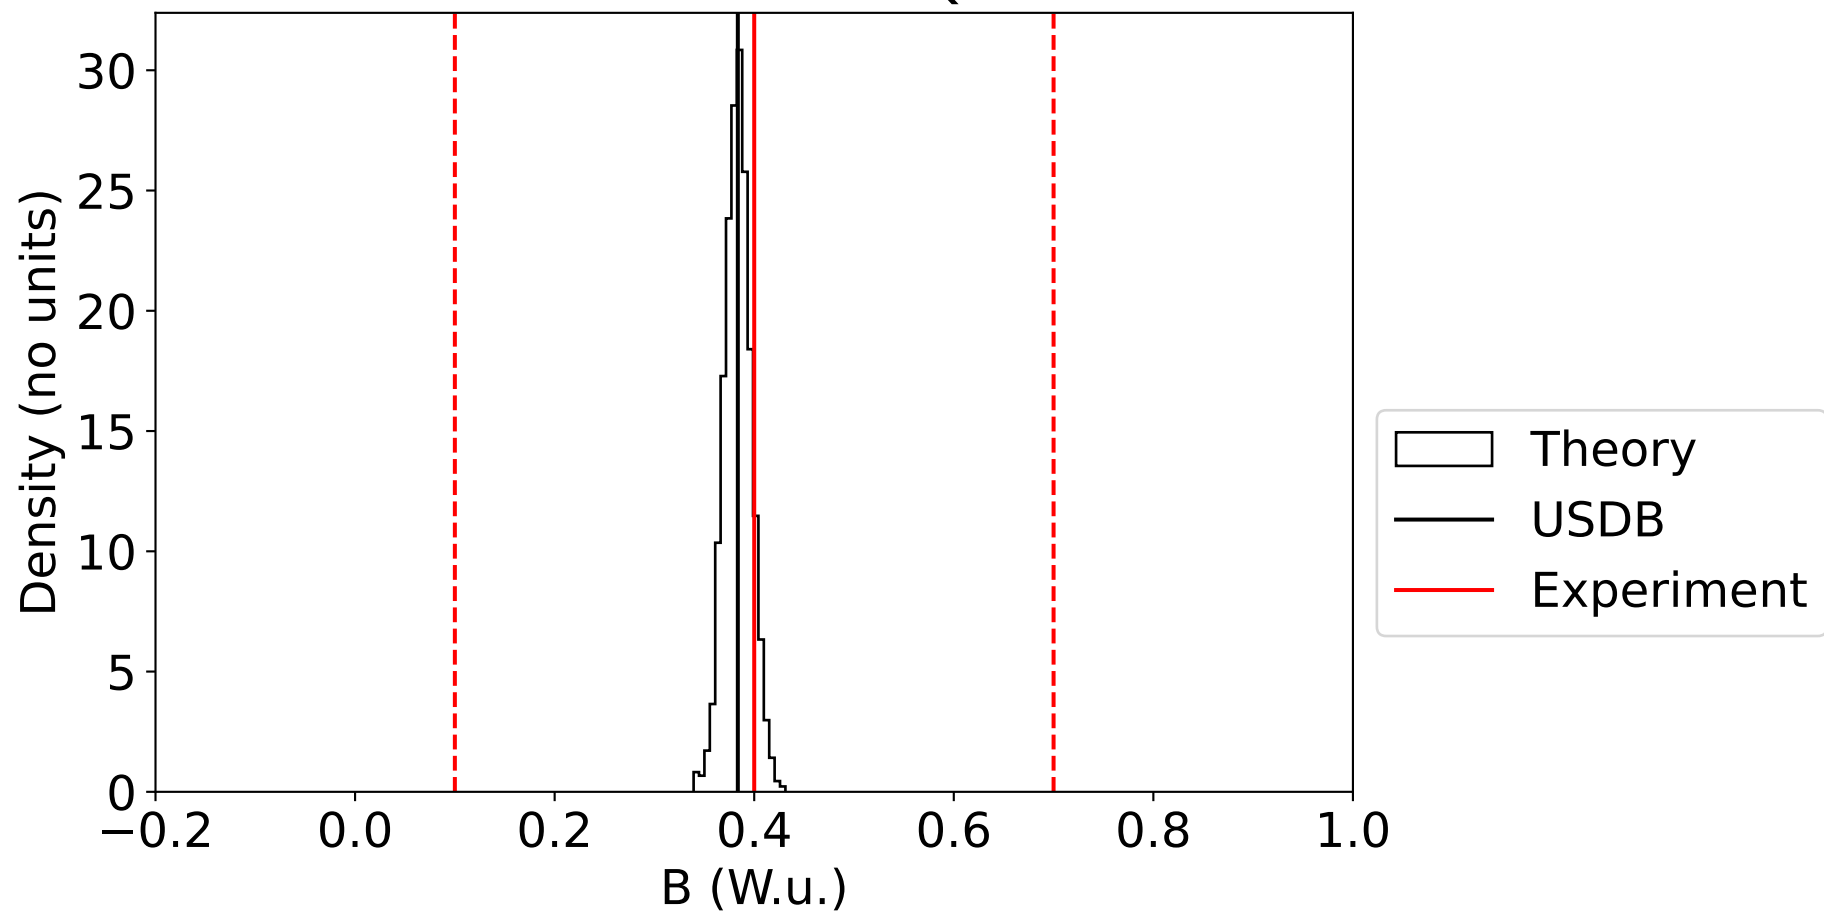

$^{24}\text{Na} (2_3) \rightarrow (1_1)$   
Included in UQ

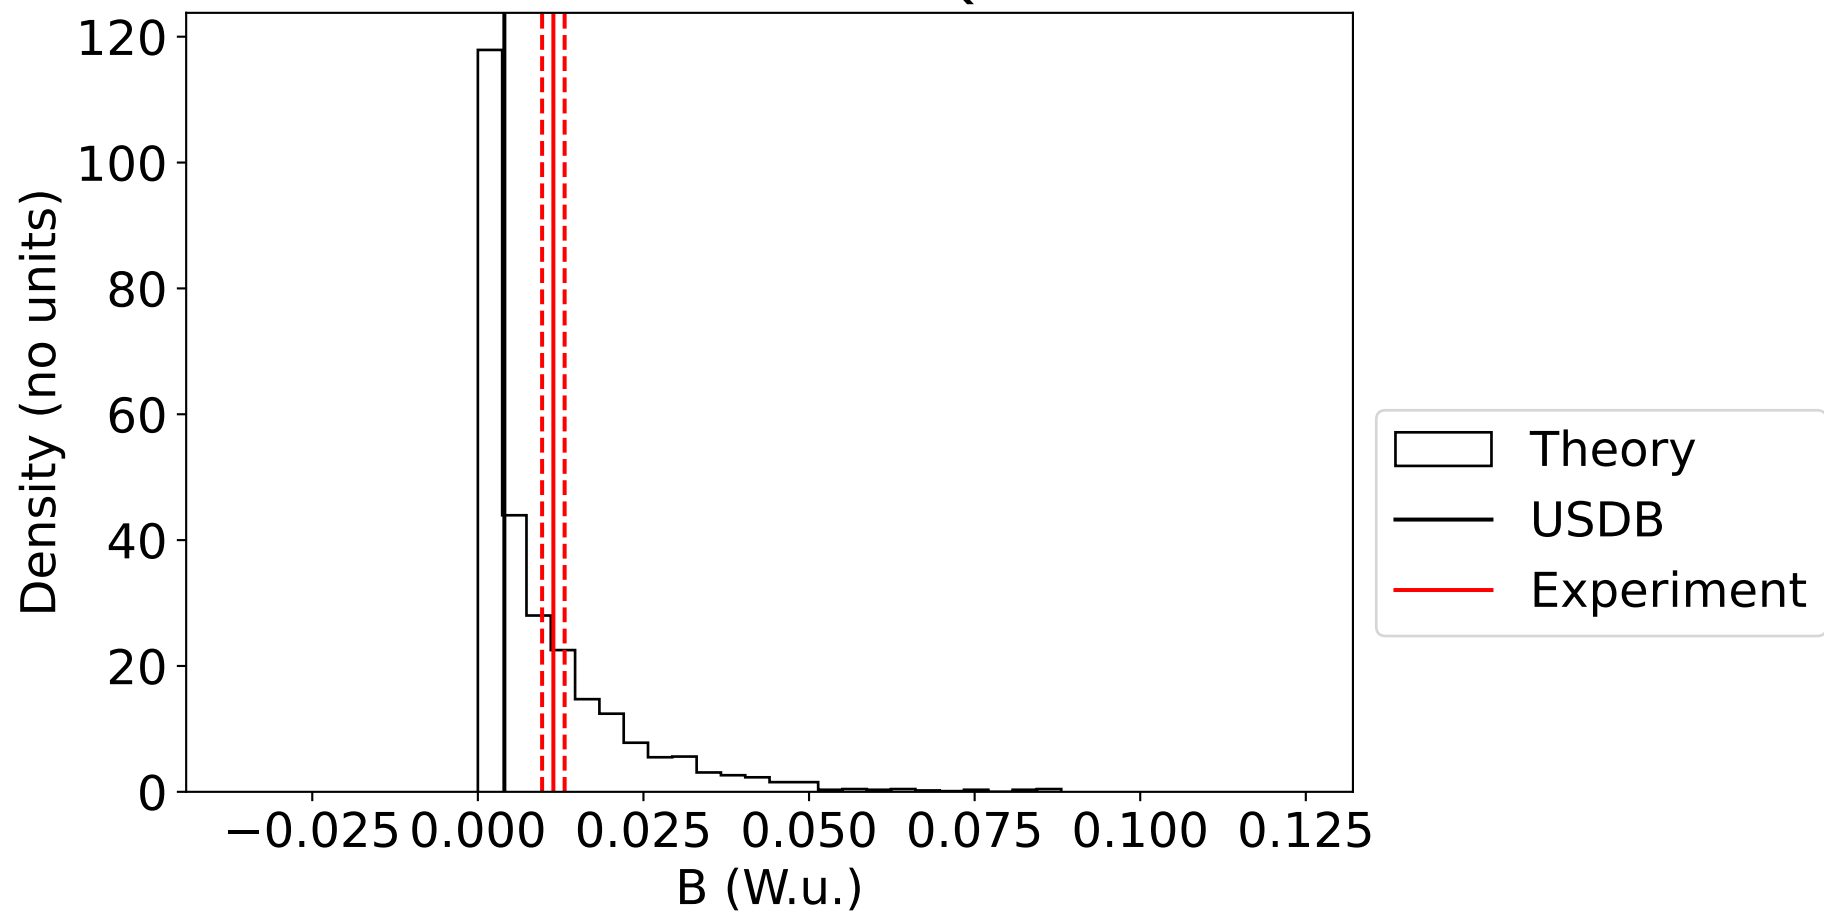

$^{24}\text{Na} (3_2) \rightarrow (4_1)$   
Included in UQ

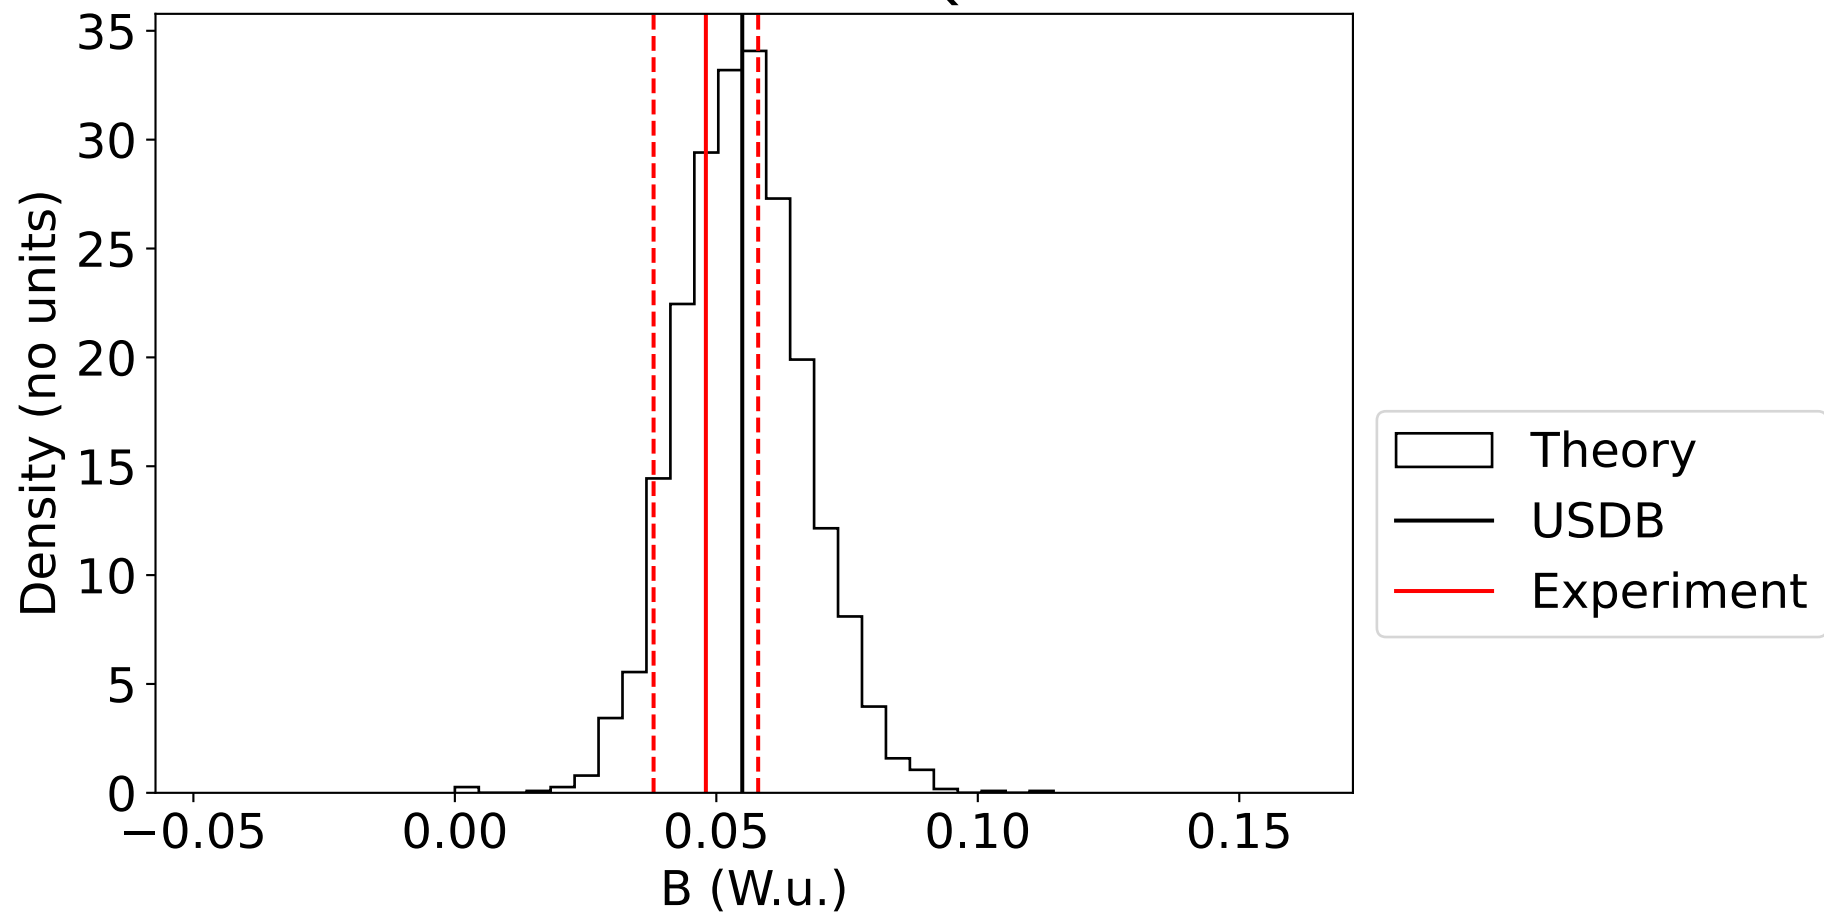

$^{25}\text{Na } (3/2_2) \rightarrow (1/2_1)$   
Included in UQ

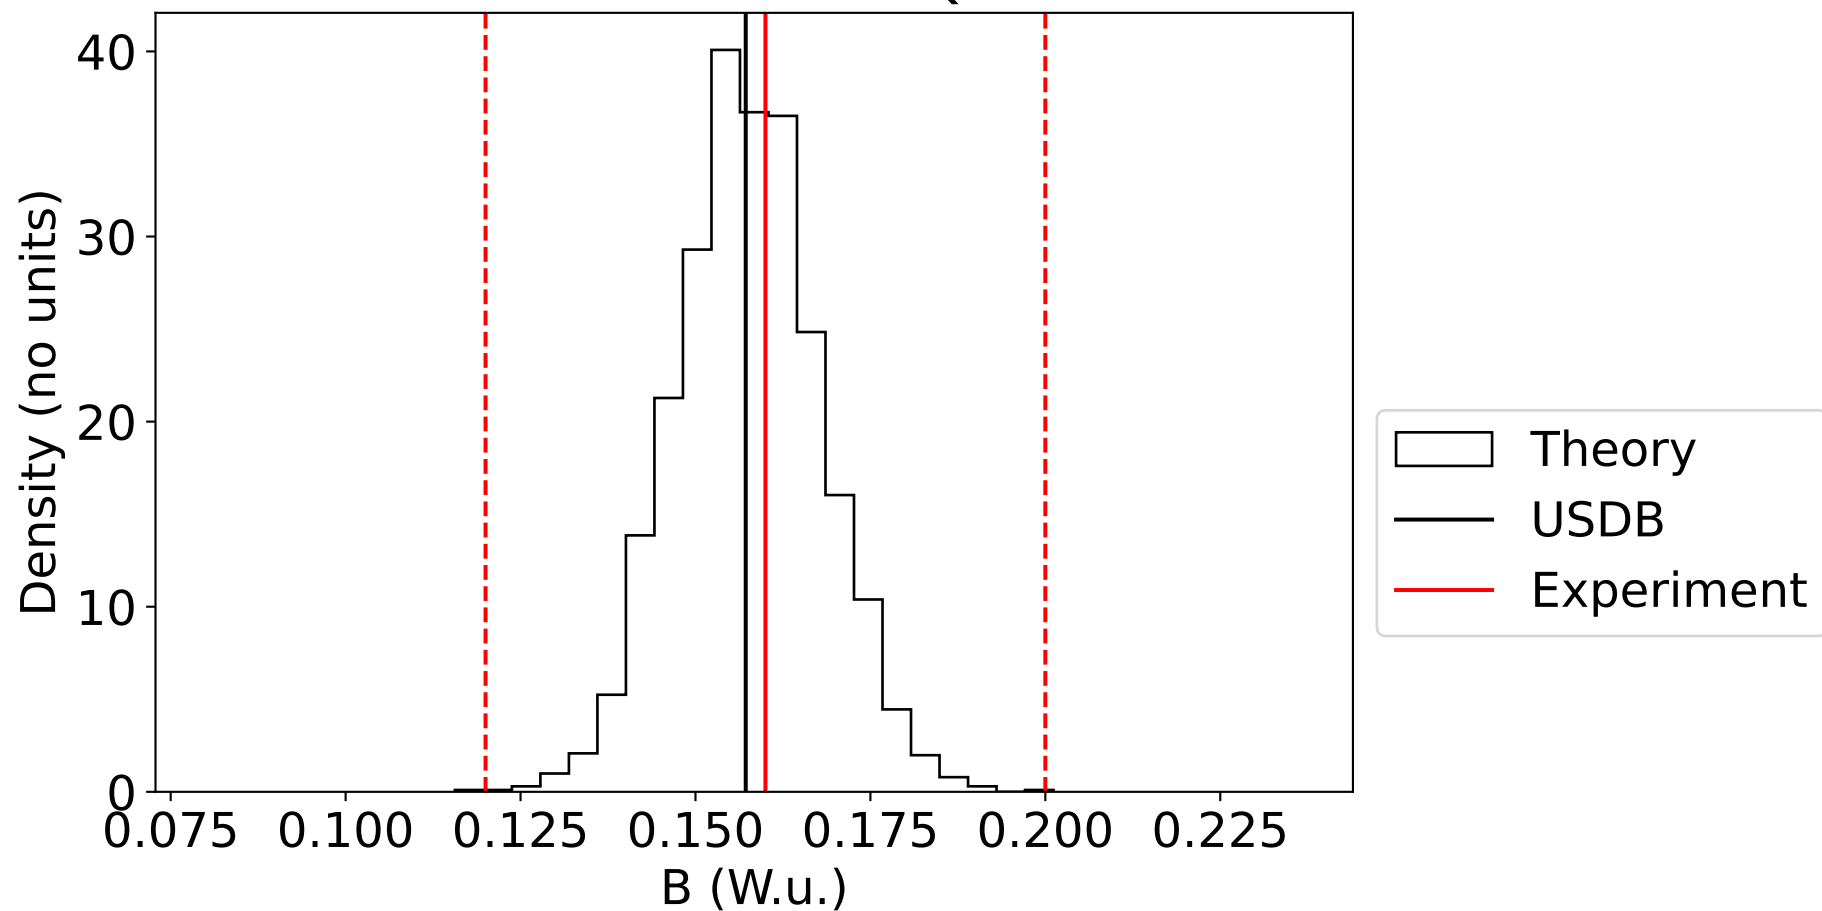

$^{23}\text{Mg}$  ( $5/2_1 \rightarrow 3/2_1$ )  
Included in UQ

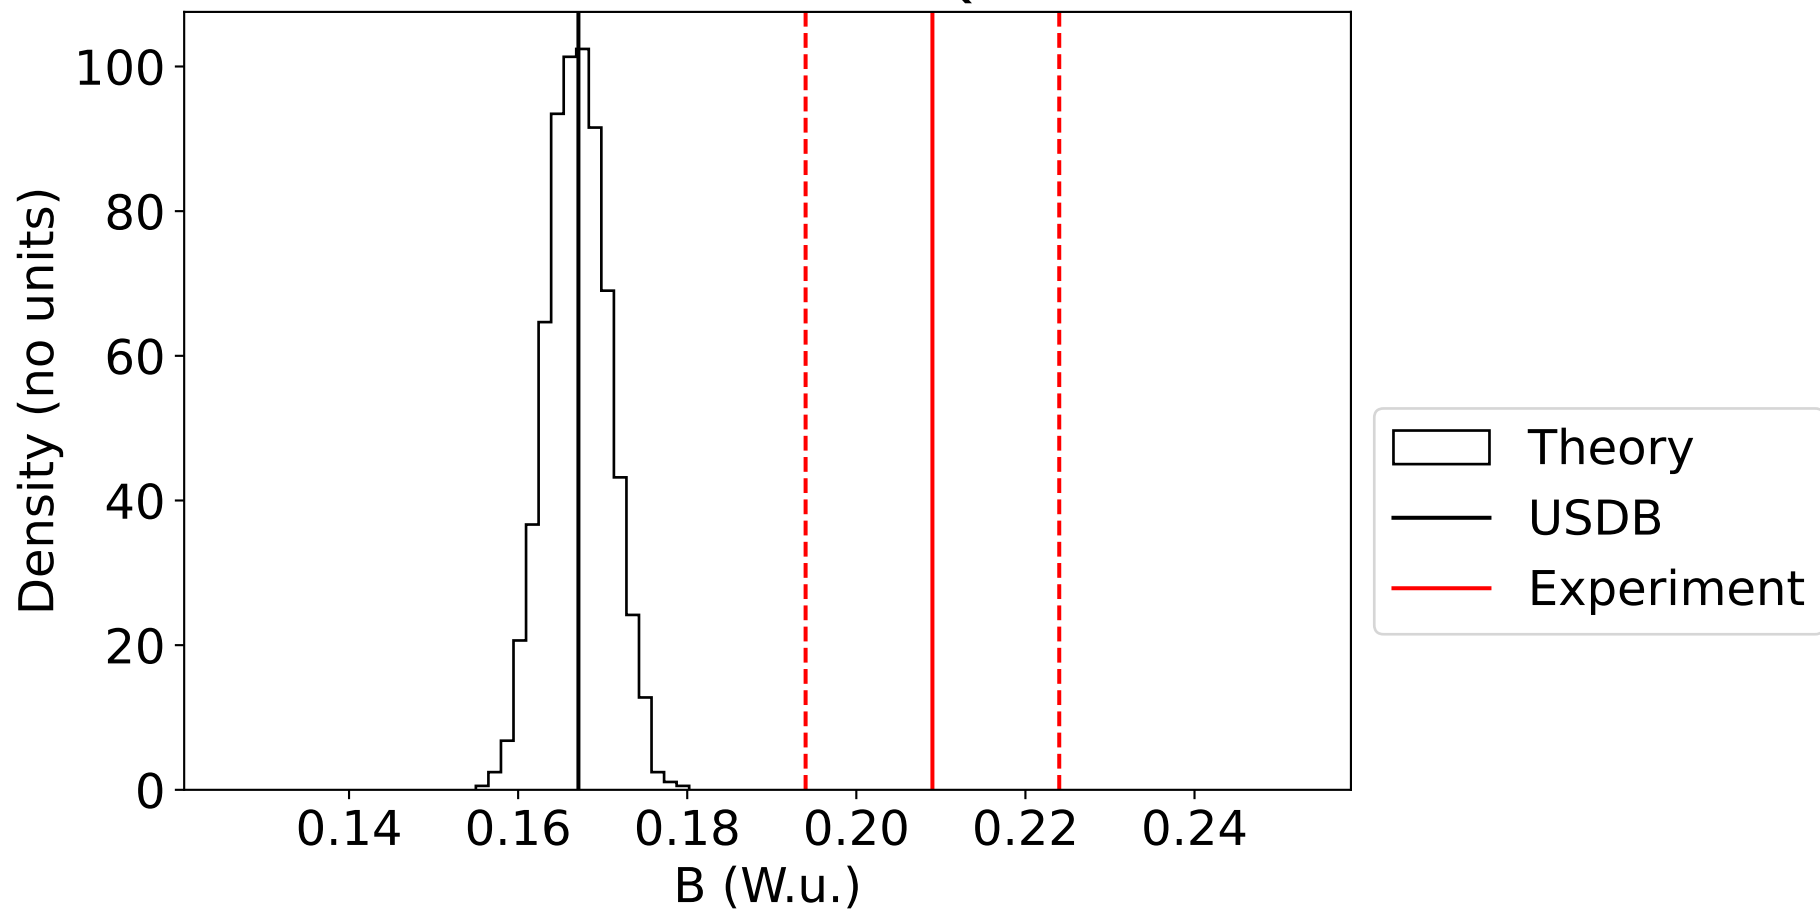

$^{23}\text{Mg} (7/2_1) \rightarrow (5/2_1)$   
Included in UQ

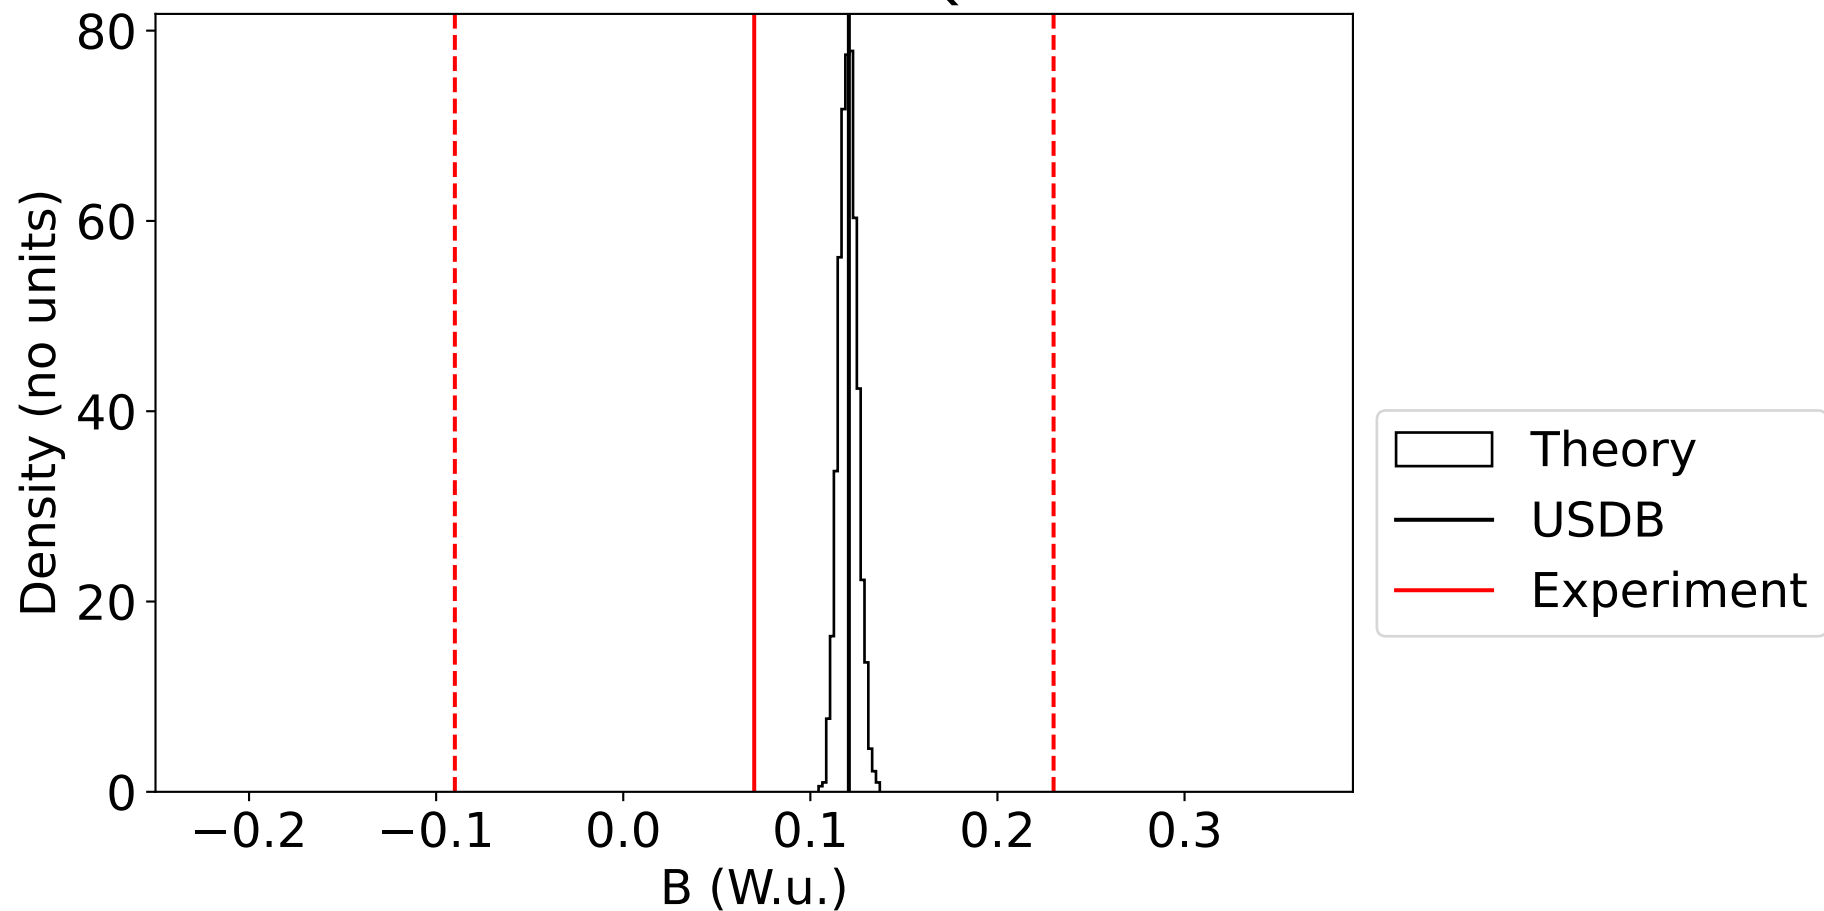

$^{25}\text{Mg} (3/2_1) \rightarrow (1/2_1)$   
Included in UQ

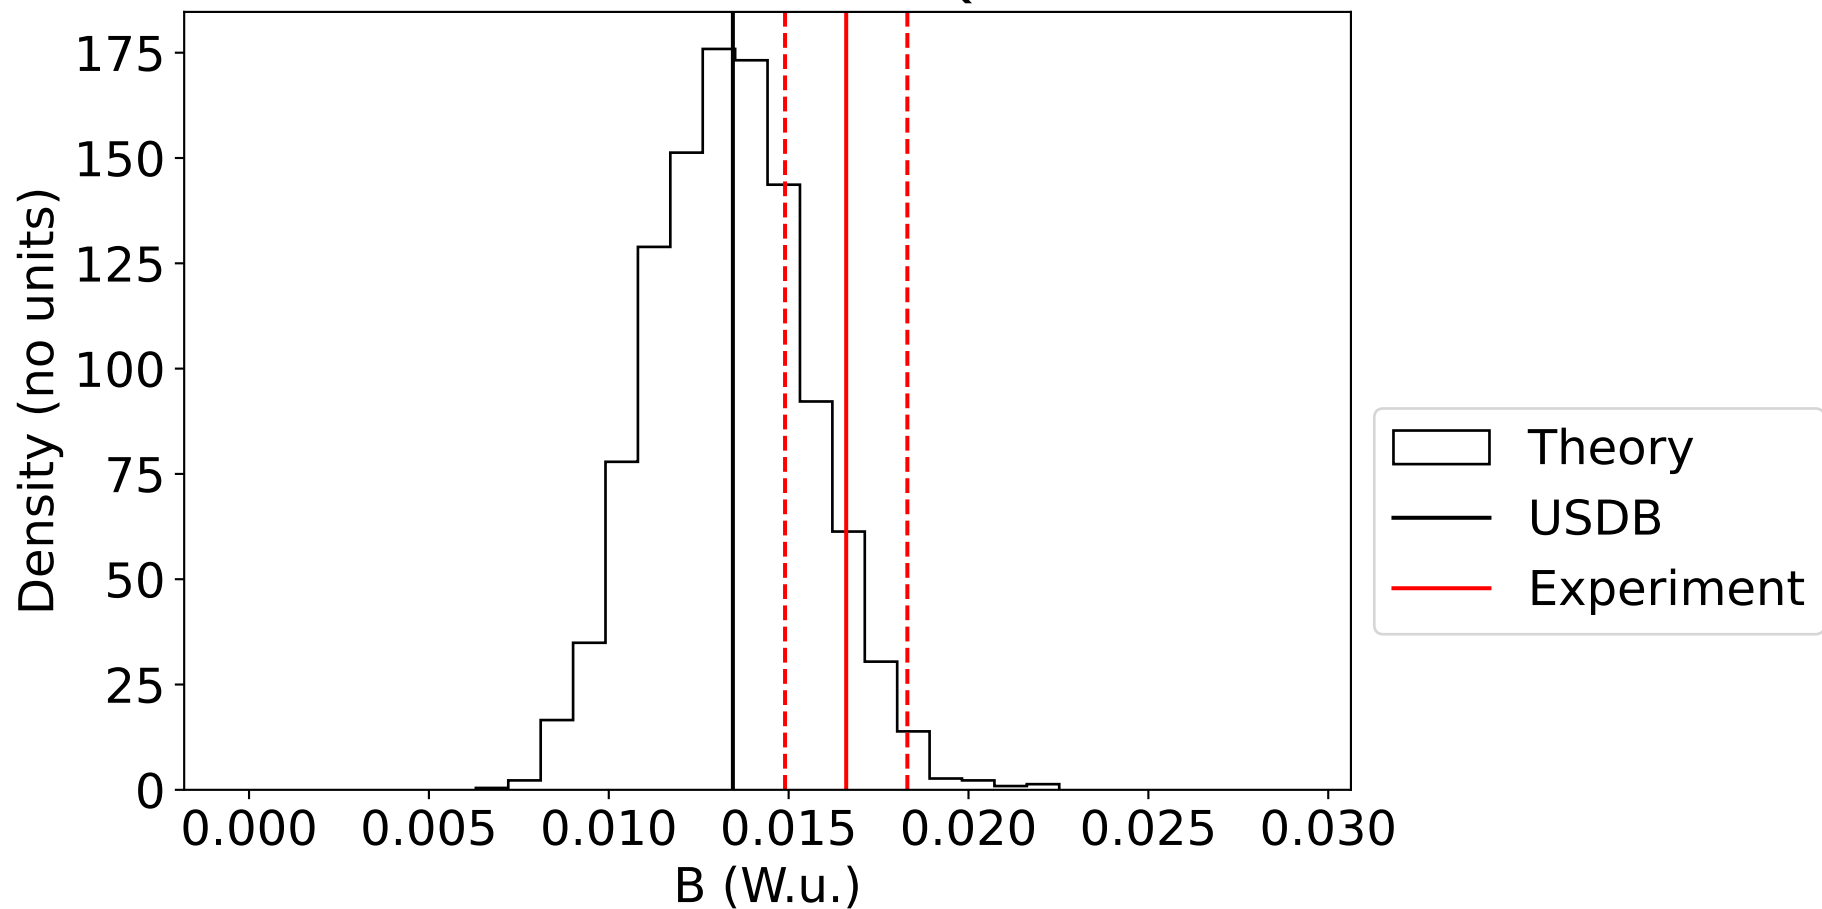



$^{25}\text{Mg } (7/2_1) \rightarrow (5/2_1)$   
Included in UQ

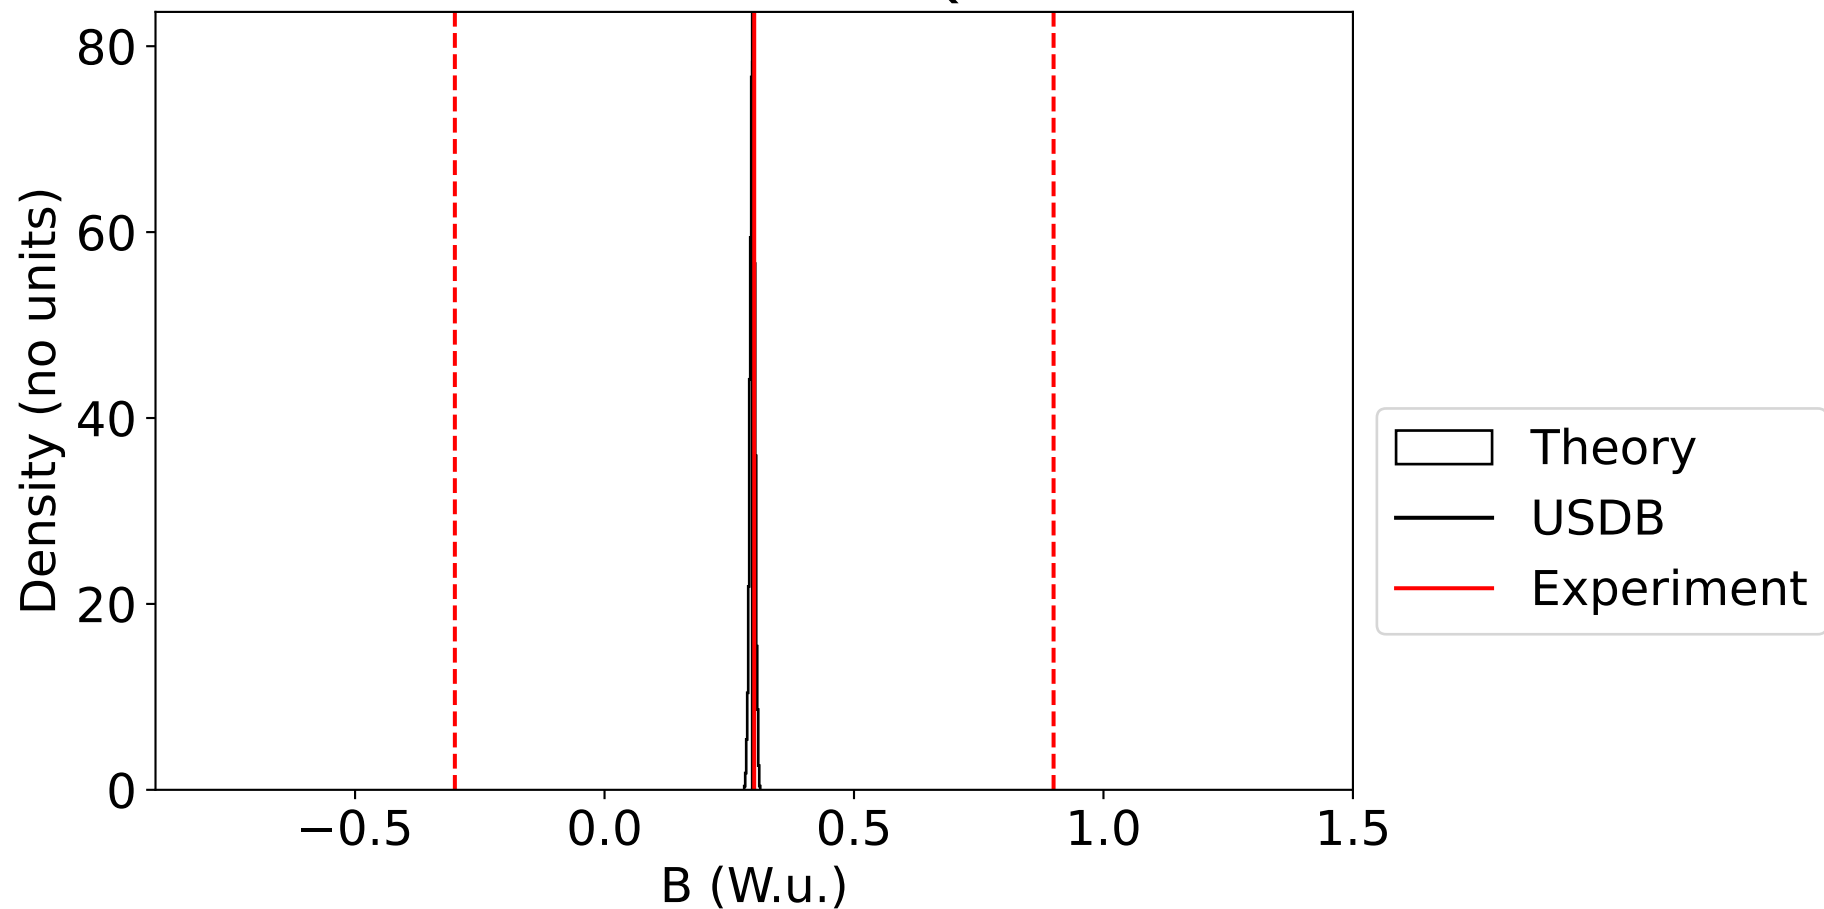

$^{25}\text{Mg } (3/2_2) \rightarrow (1/2_1)$   
Included in UQ

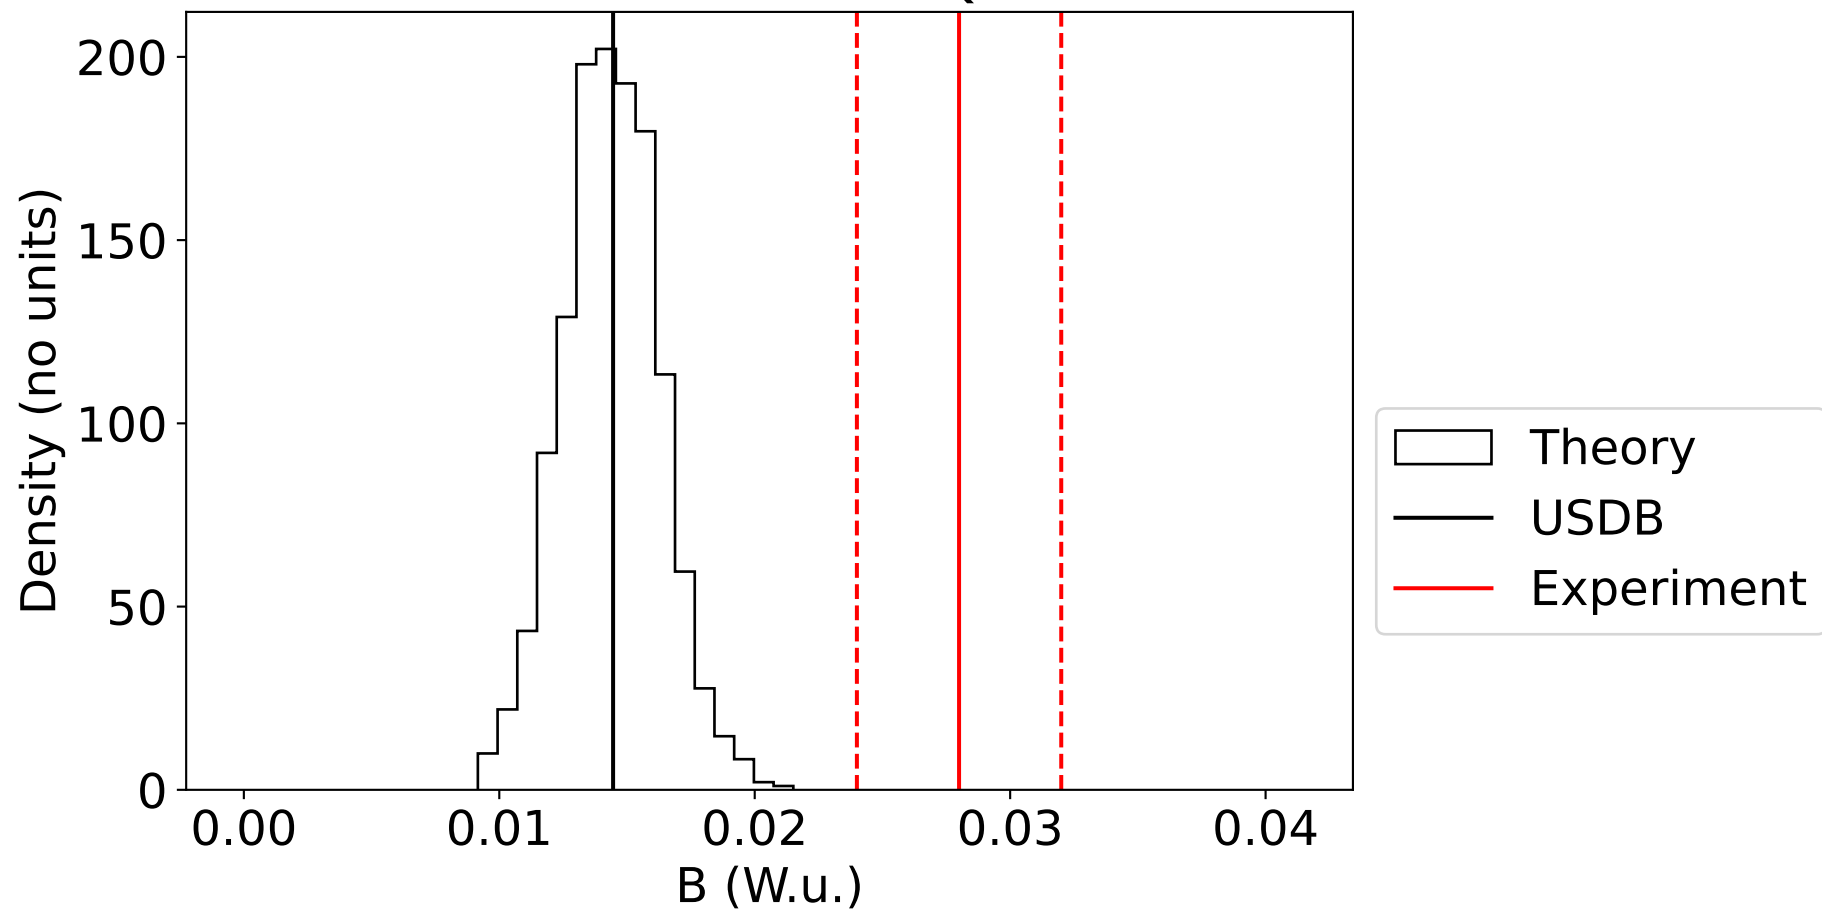

$^{25}\text{Mg } (9/2_1) \rightarrow (7/2_1)$   
Included in UQ

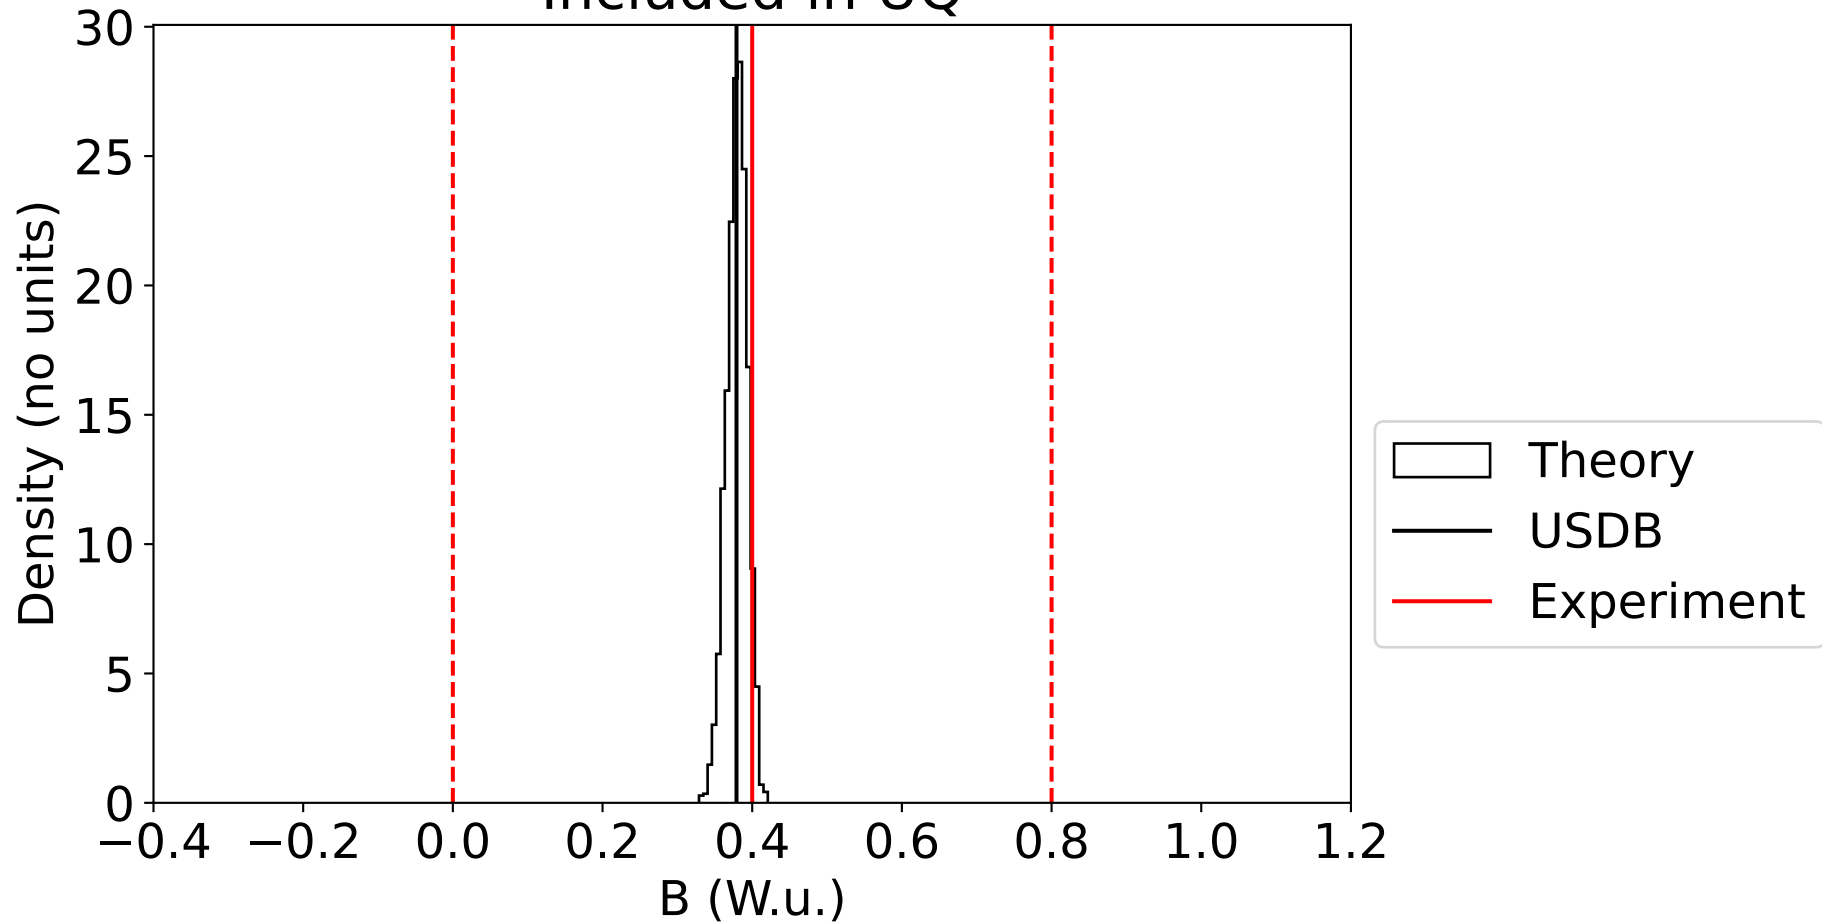

$^{25}\text{Mg } (5/2_3) \rightarrow (7/2_2)$   
Included in UQ

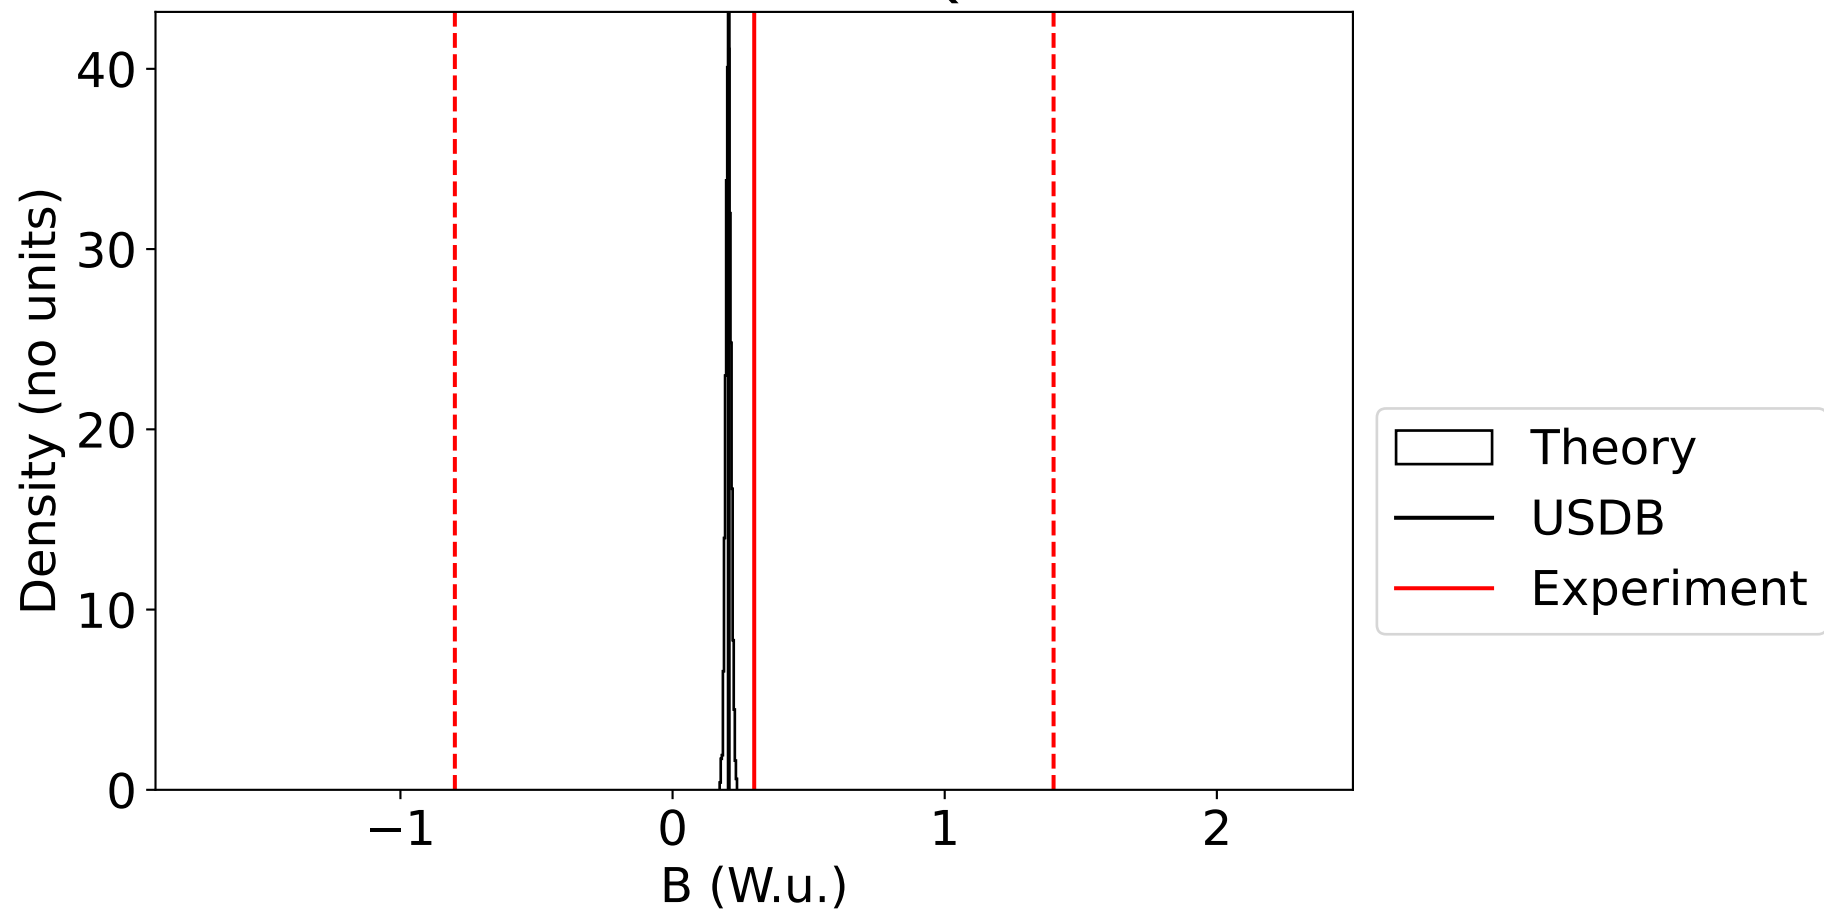

$^{25}\text{Mg } (9/2_2) \rightarrow (7/2_1)$   
Included in UQ

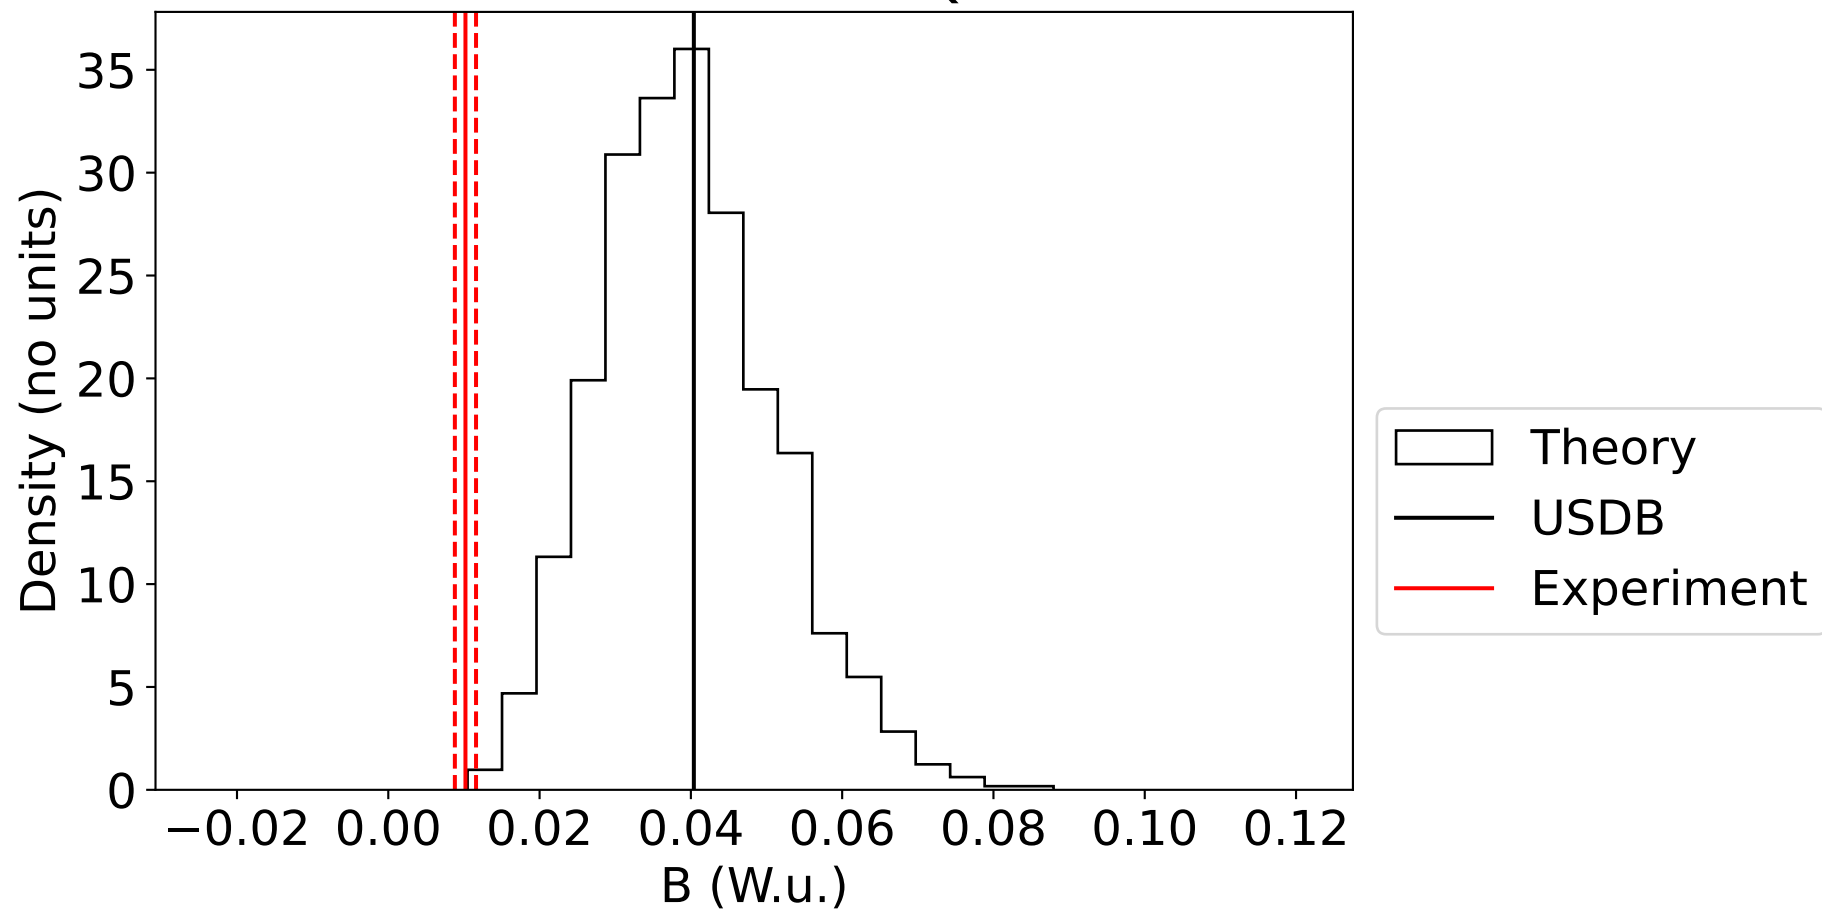

$^{25}\text{Mg} (11/2_1) \rightarrow (9/2_2)$   
Included in UQ

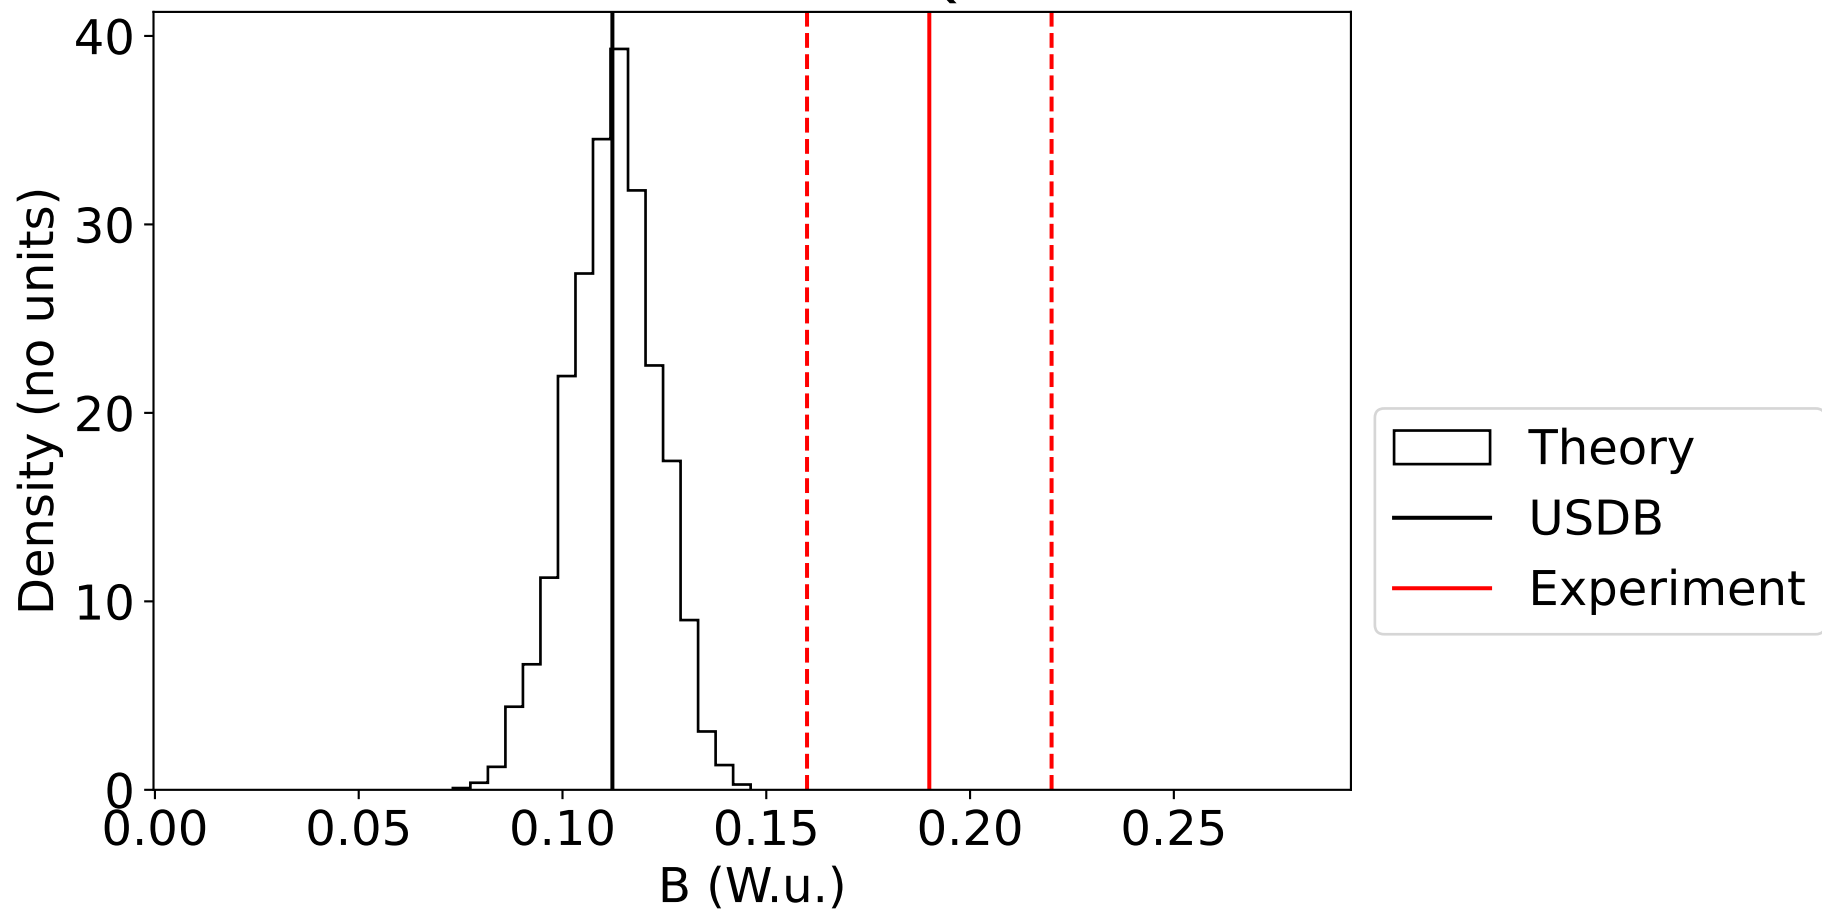

$^{25}\text{Mg} (11/2_1) \rightarrow (9/2_1)$   
Included in UQ

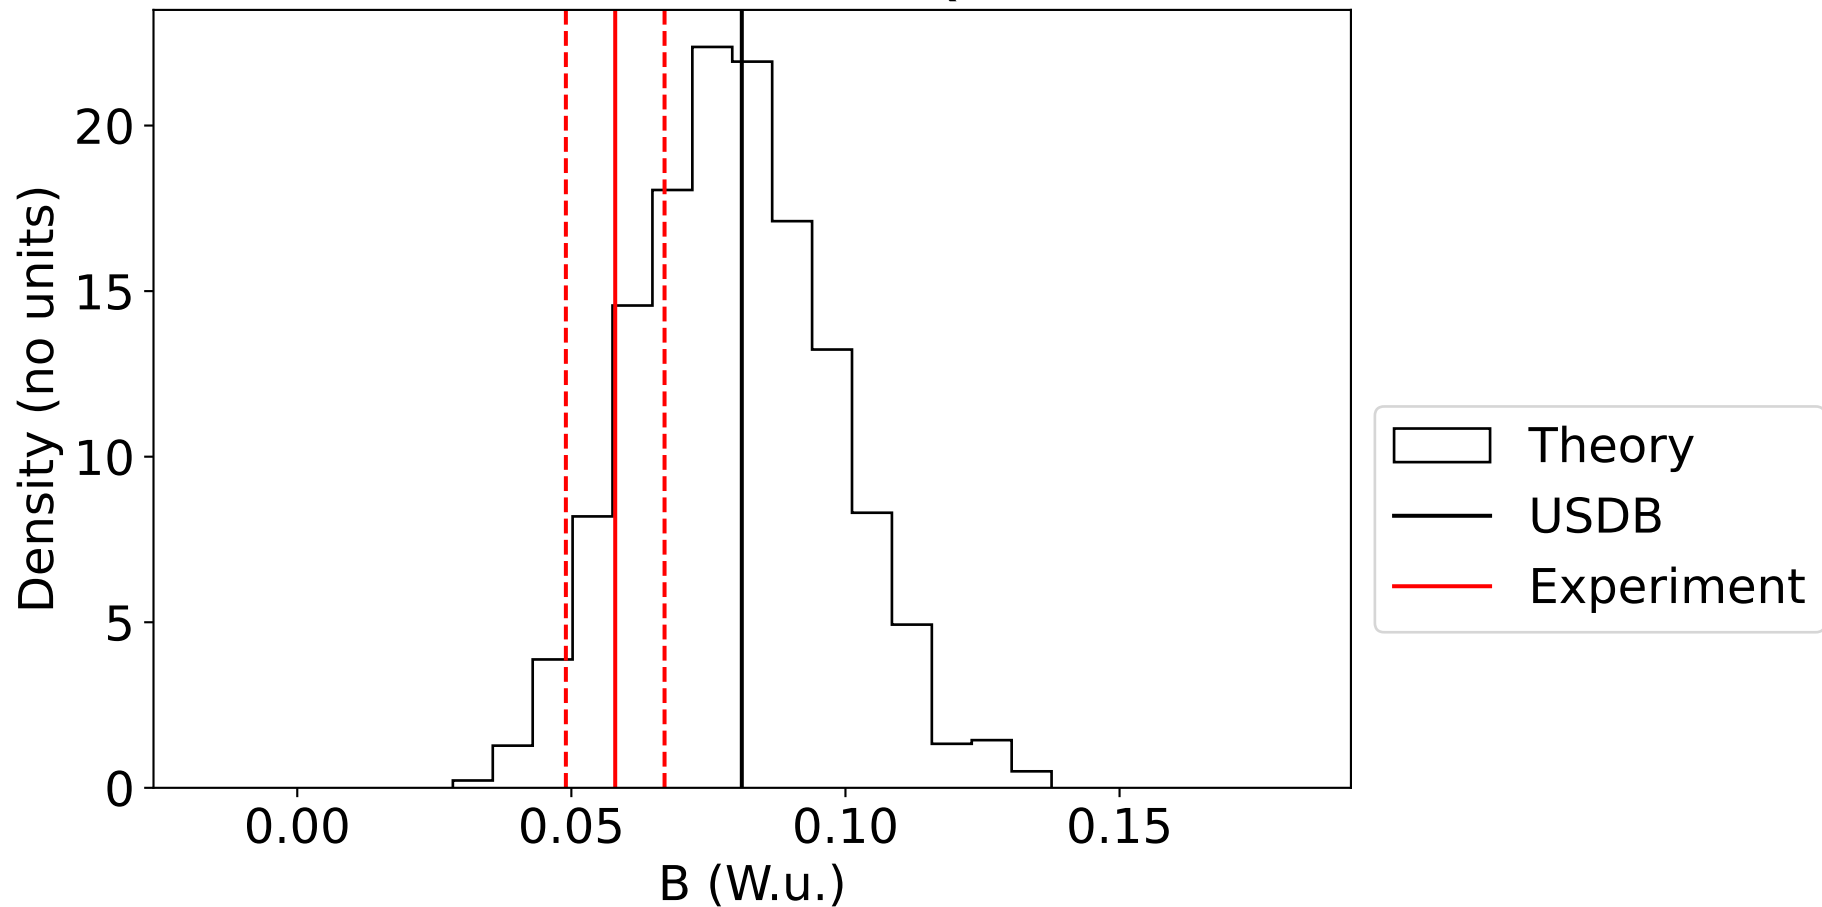

$^{26}\text{Mg} (2_2) \rightarrow (2_1)$   
Included in UQ

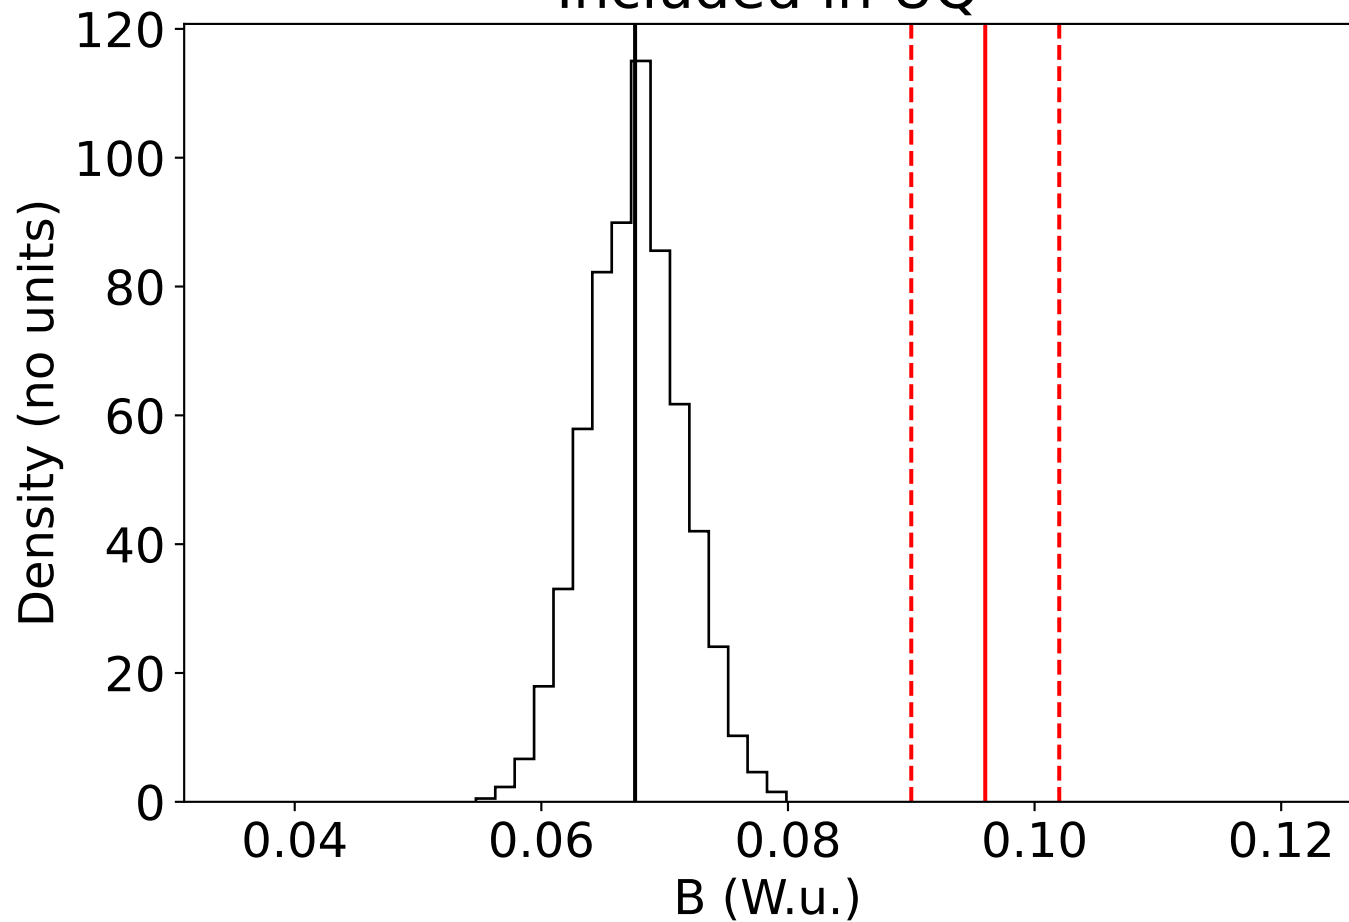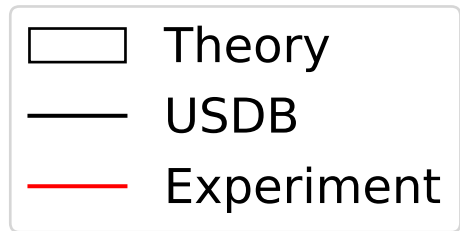



$^{26}\text{Mg} (3_1) \rightarrow (2_2)$   
Included in UQ

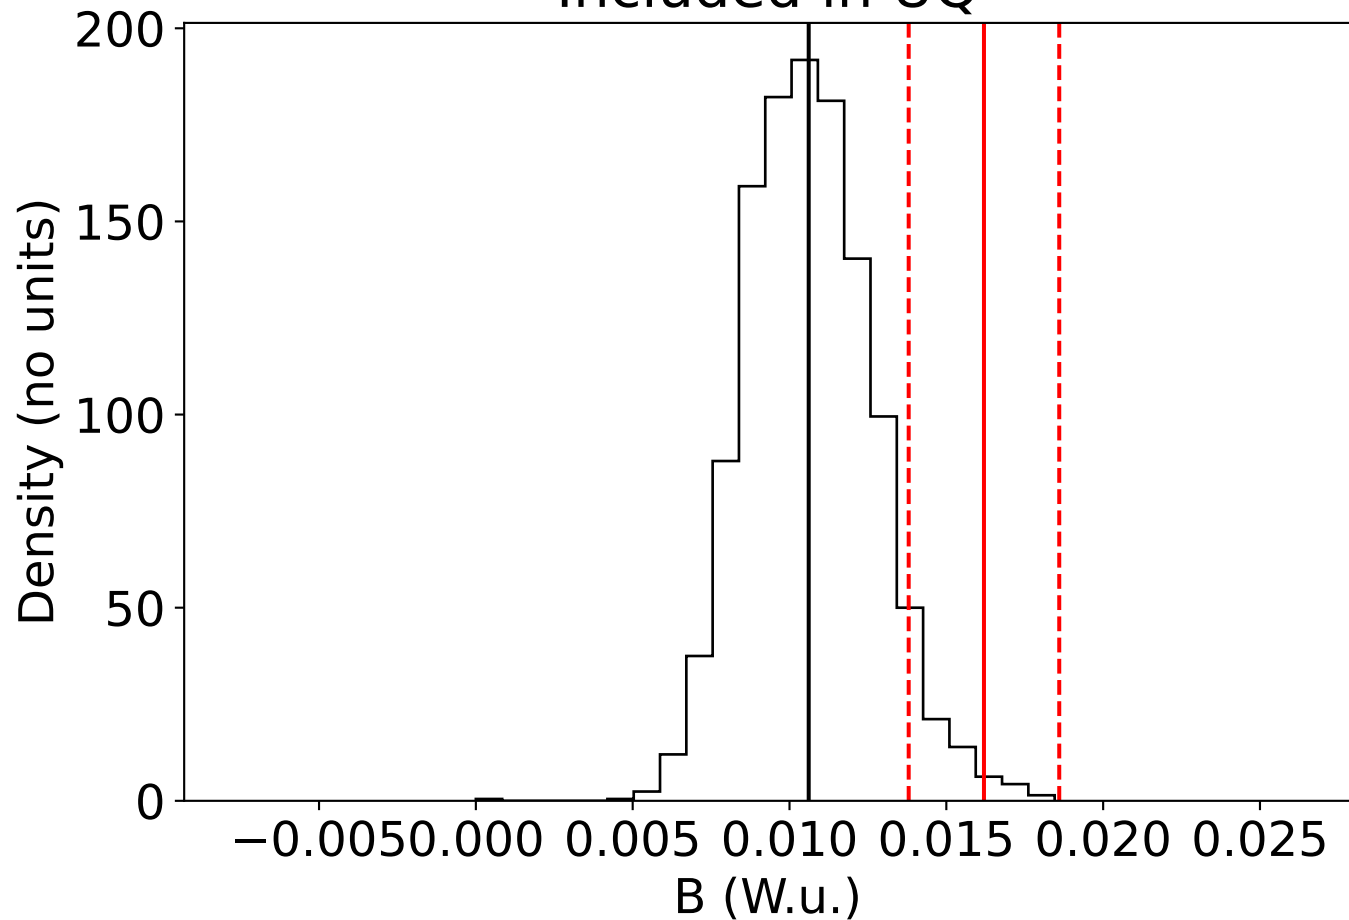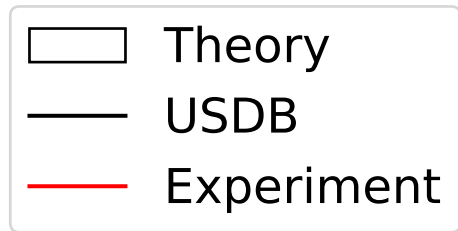

$^{26}\text{Mg} (3_2) \rightarrow (2_2)$   
Included in UQ

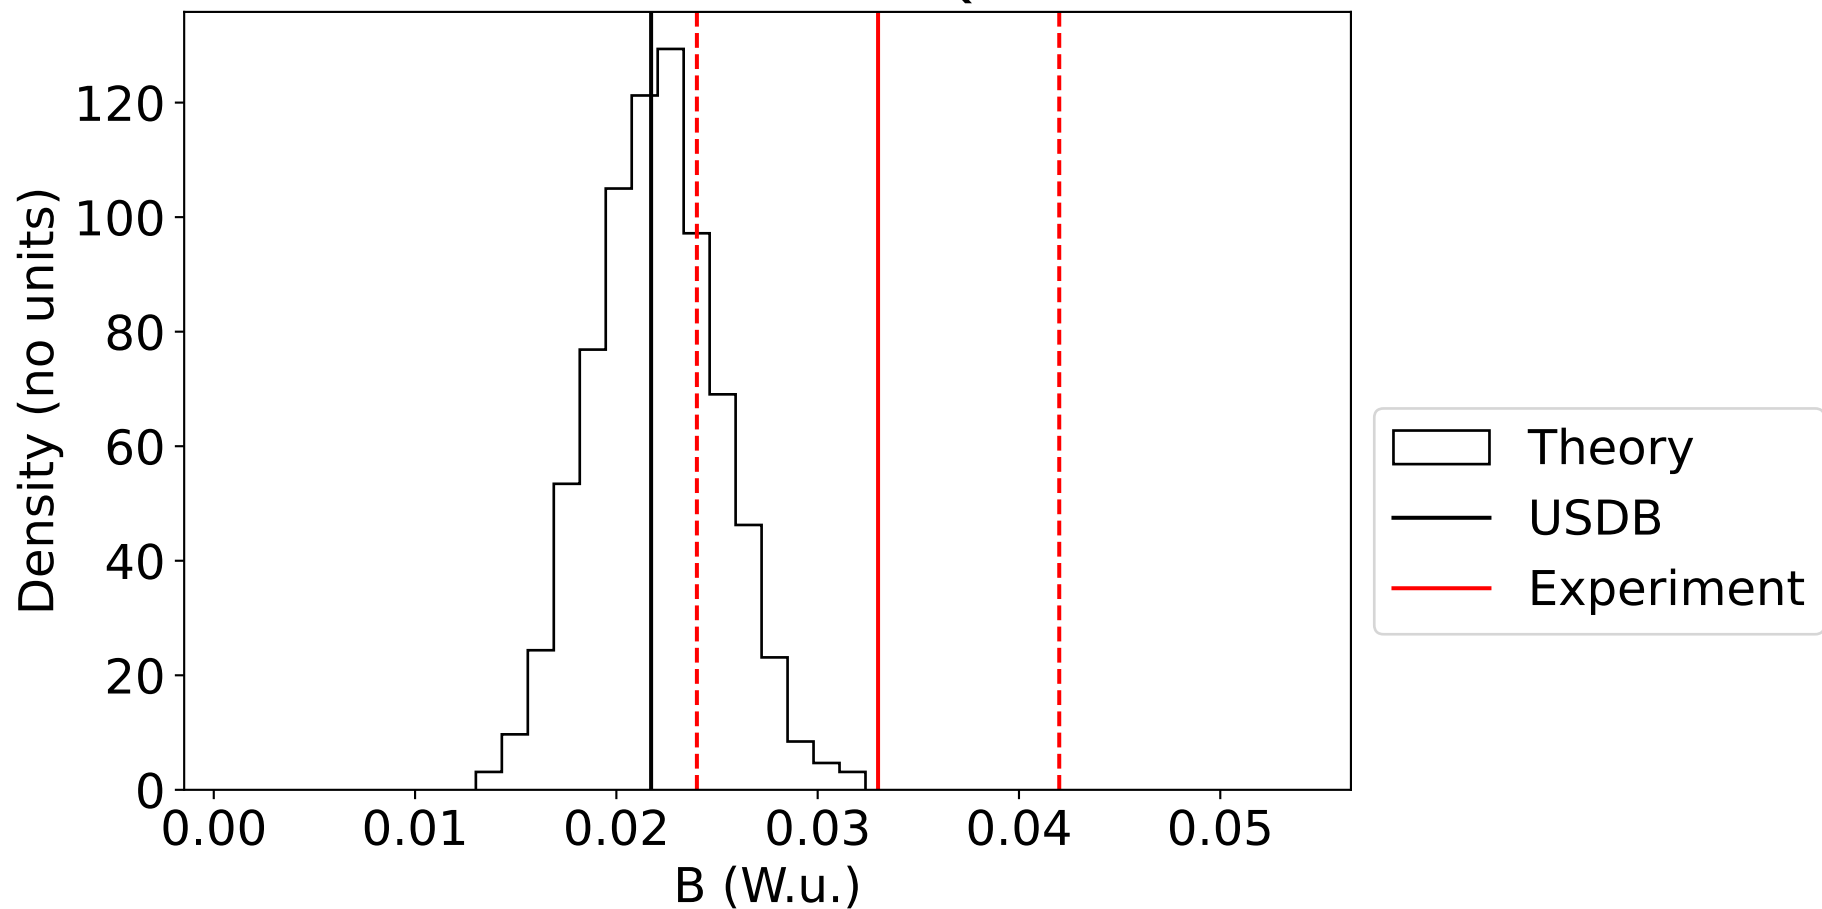

$^{26}\text{Mg} (2_4) \rightarrow (2_2)$   
Included in UQ

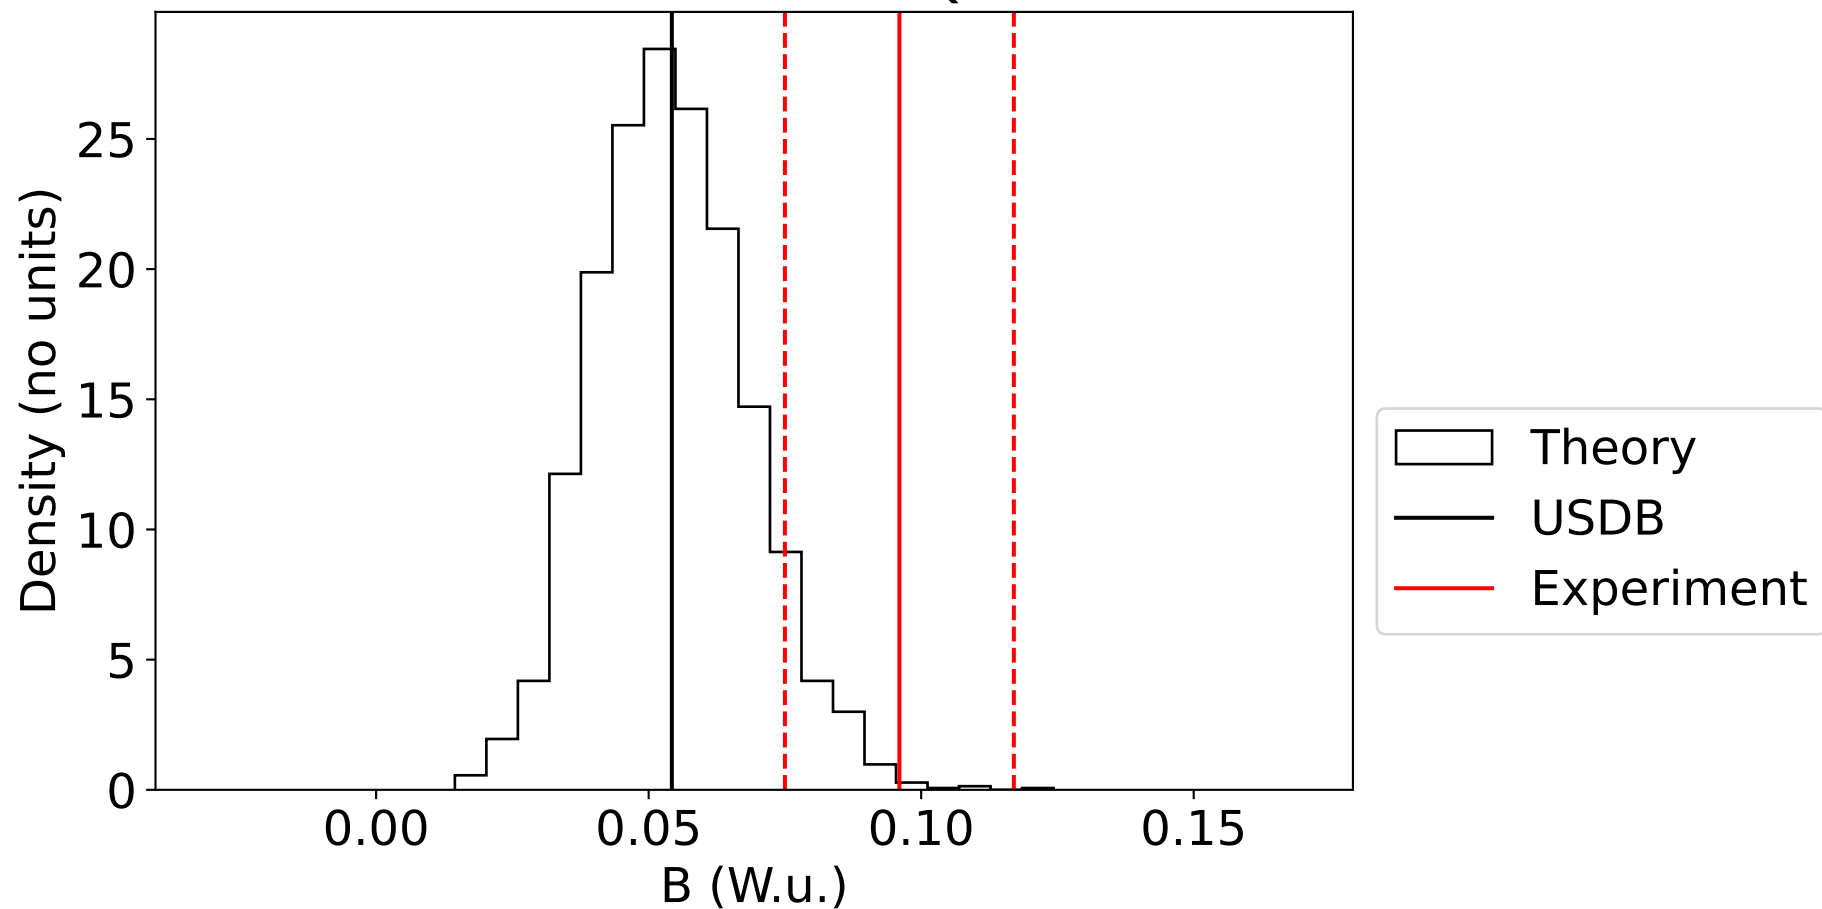

$^{26}\text{Mg} (4_3) \rightarrow (3_1)$   
Included in UQ

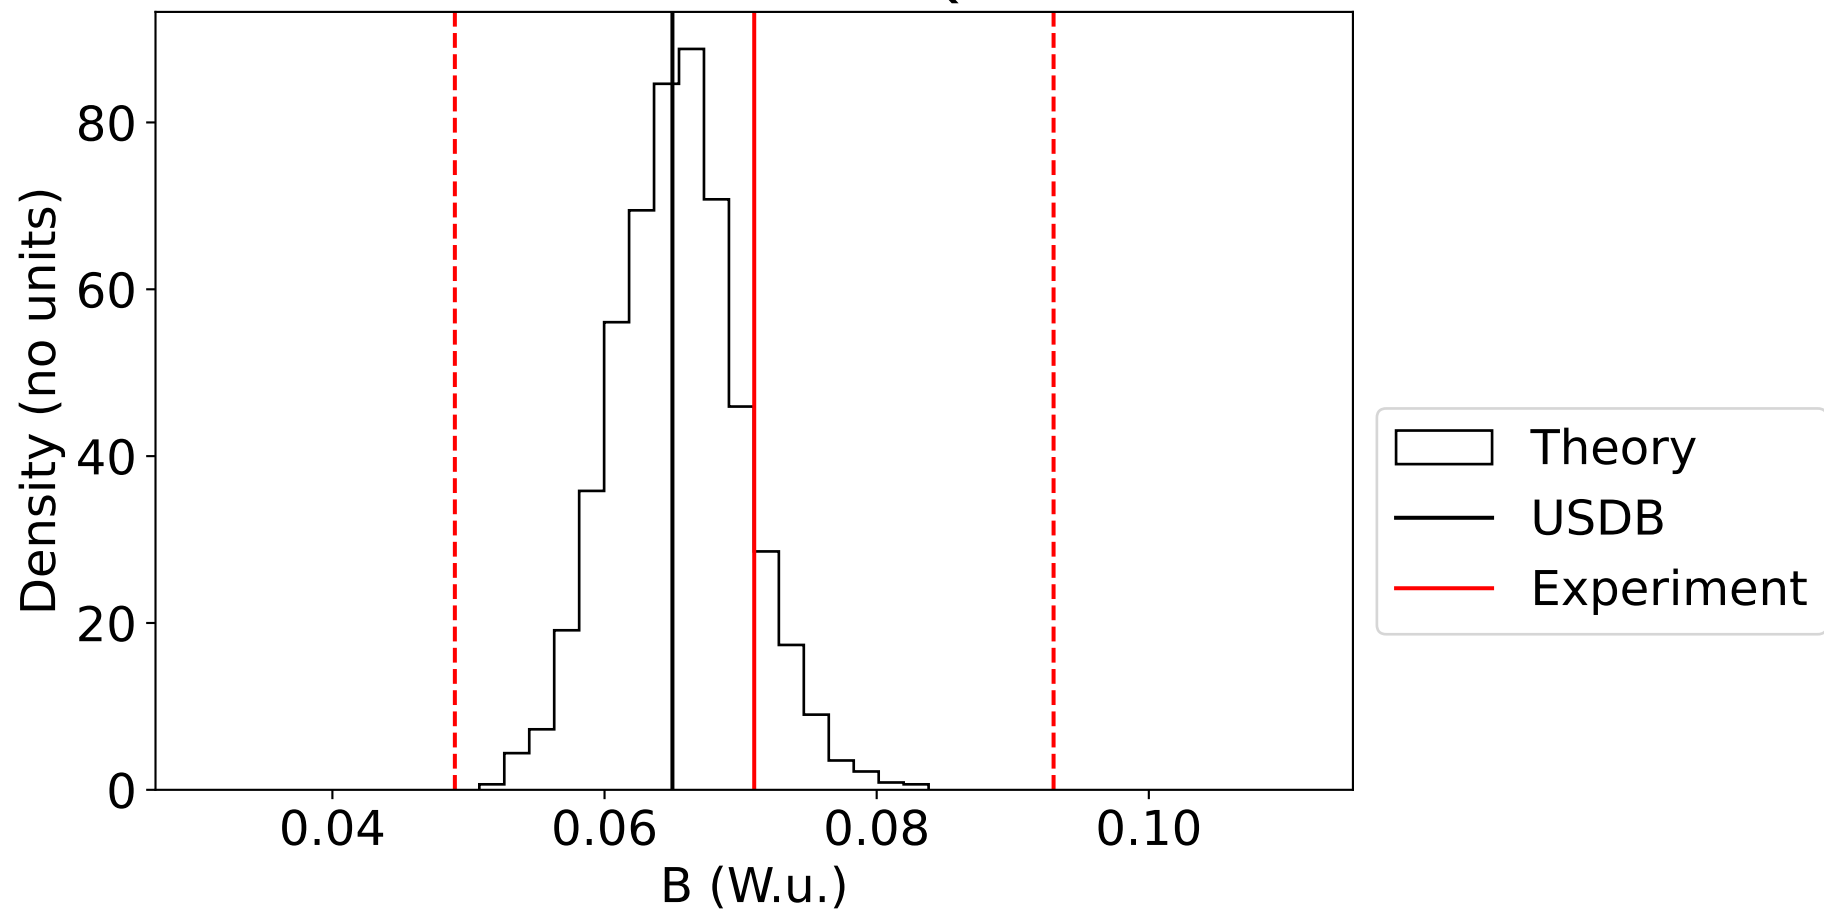

$^{26}\text{Mg} (4_4) \rightarrow (3_1)$   
Included in UQ

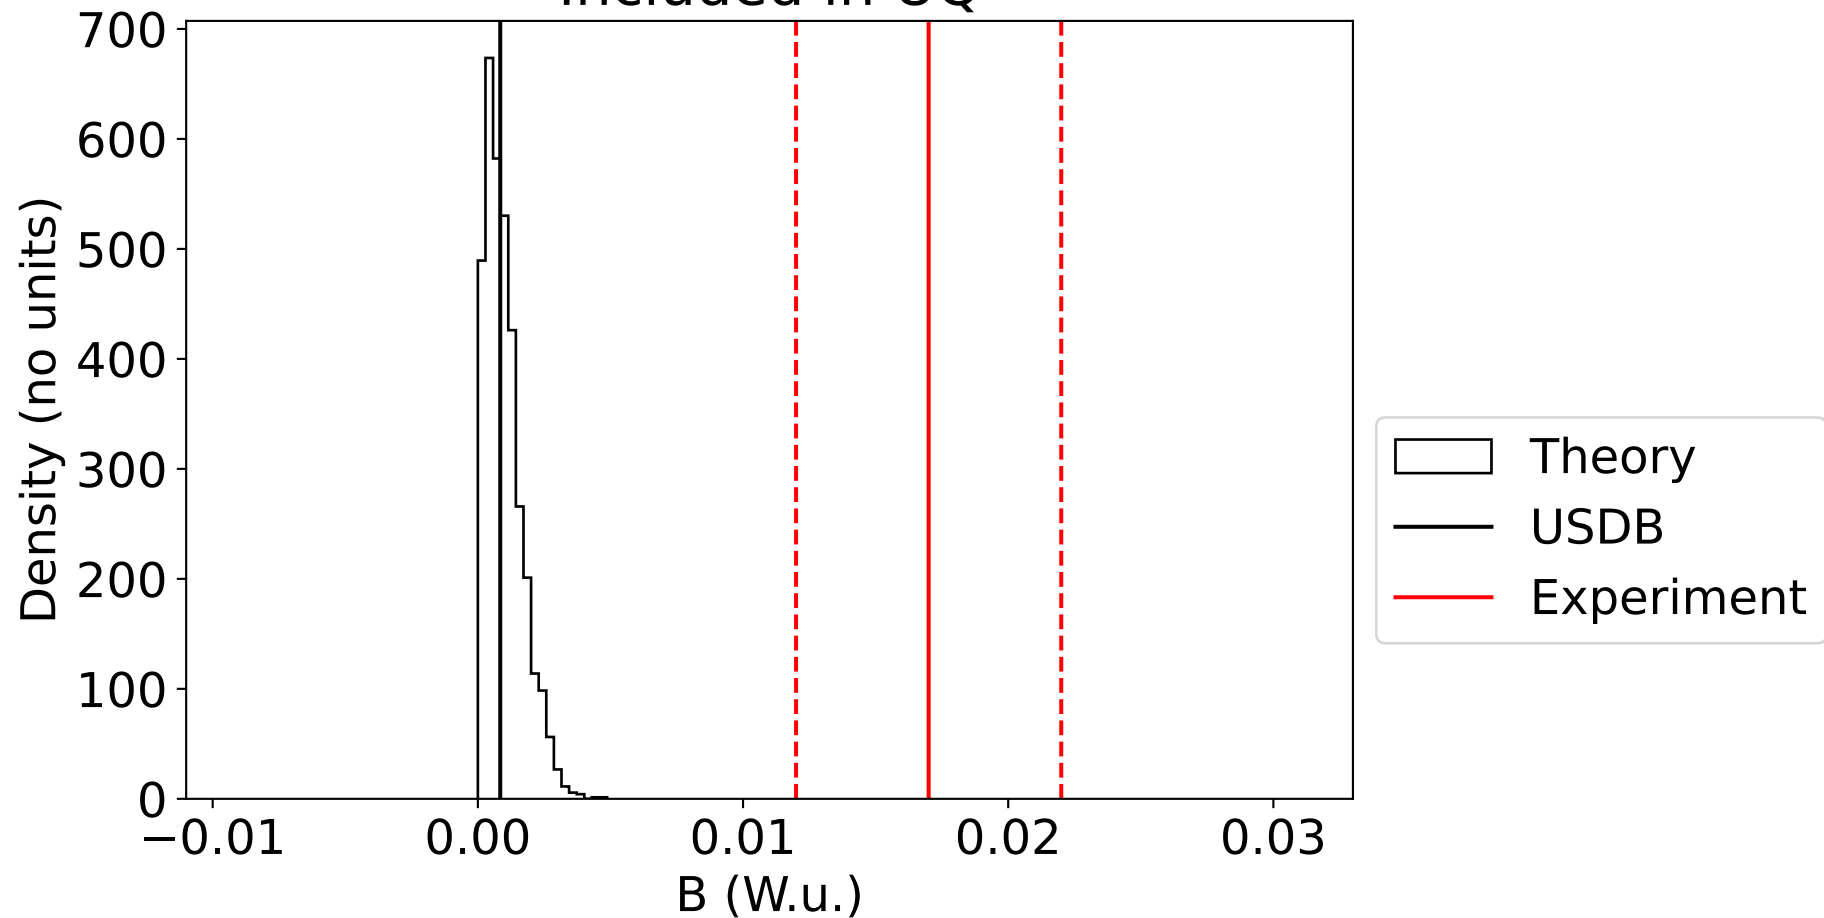

$^{26}\text{Mg} (4_5) \rightarrow (4_3)$   
Included in UQ

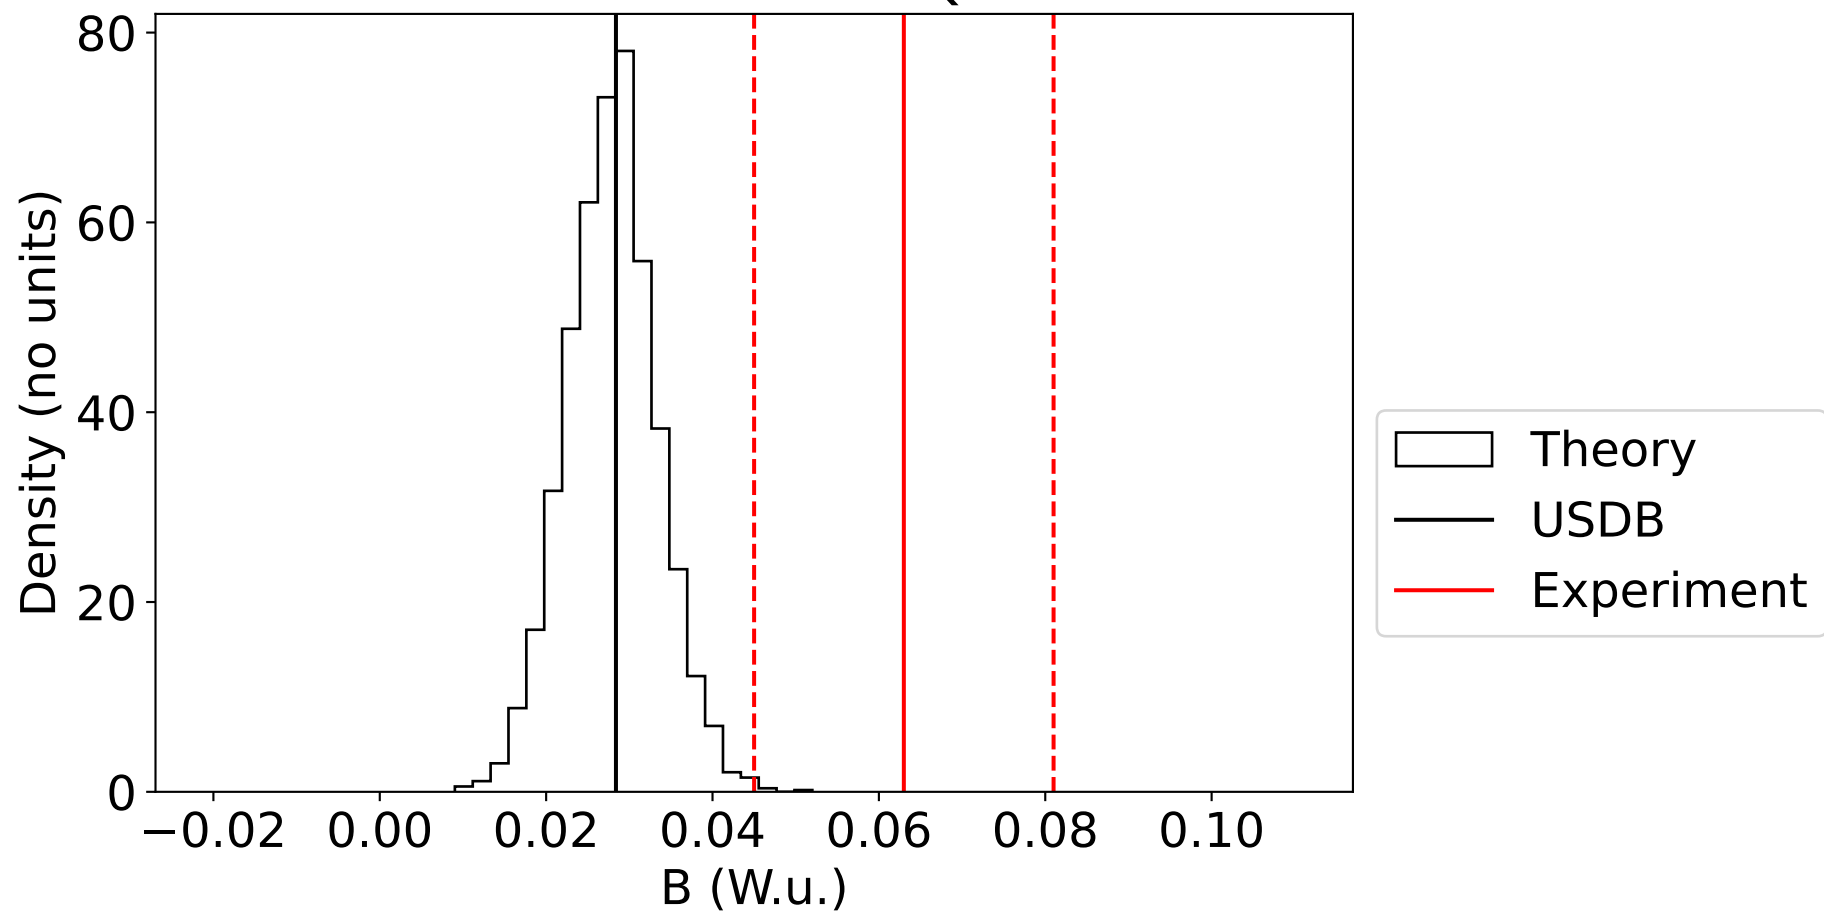

$^{26}\text{Mg} (5_1) \rightarrow (4_1)$   
Included in UQ

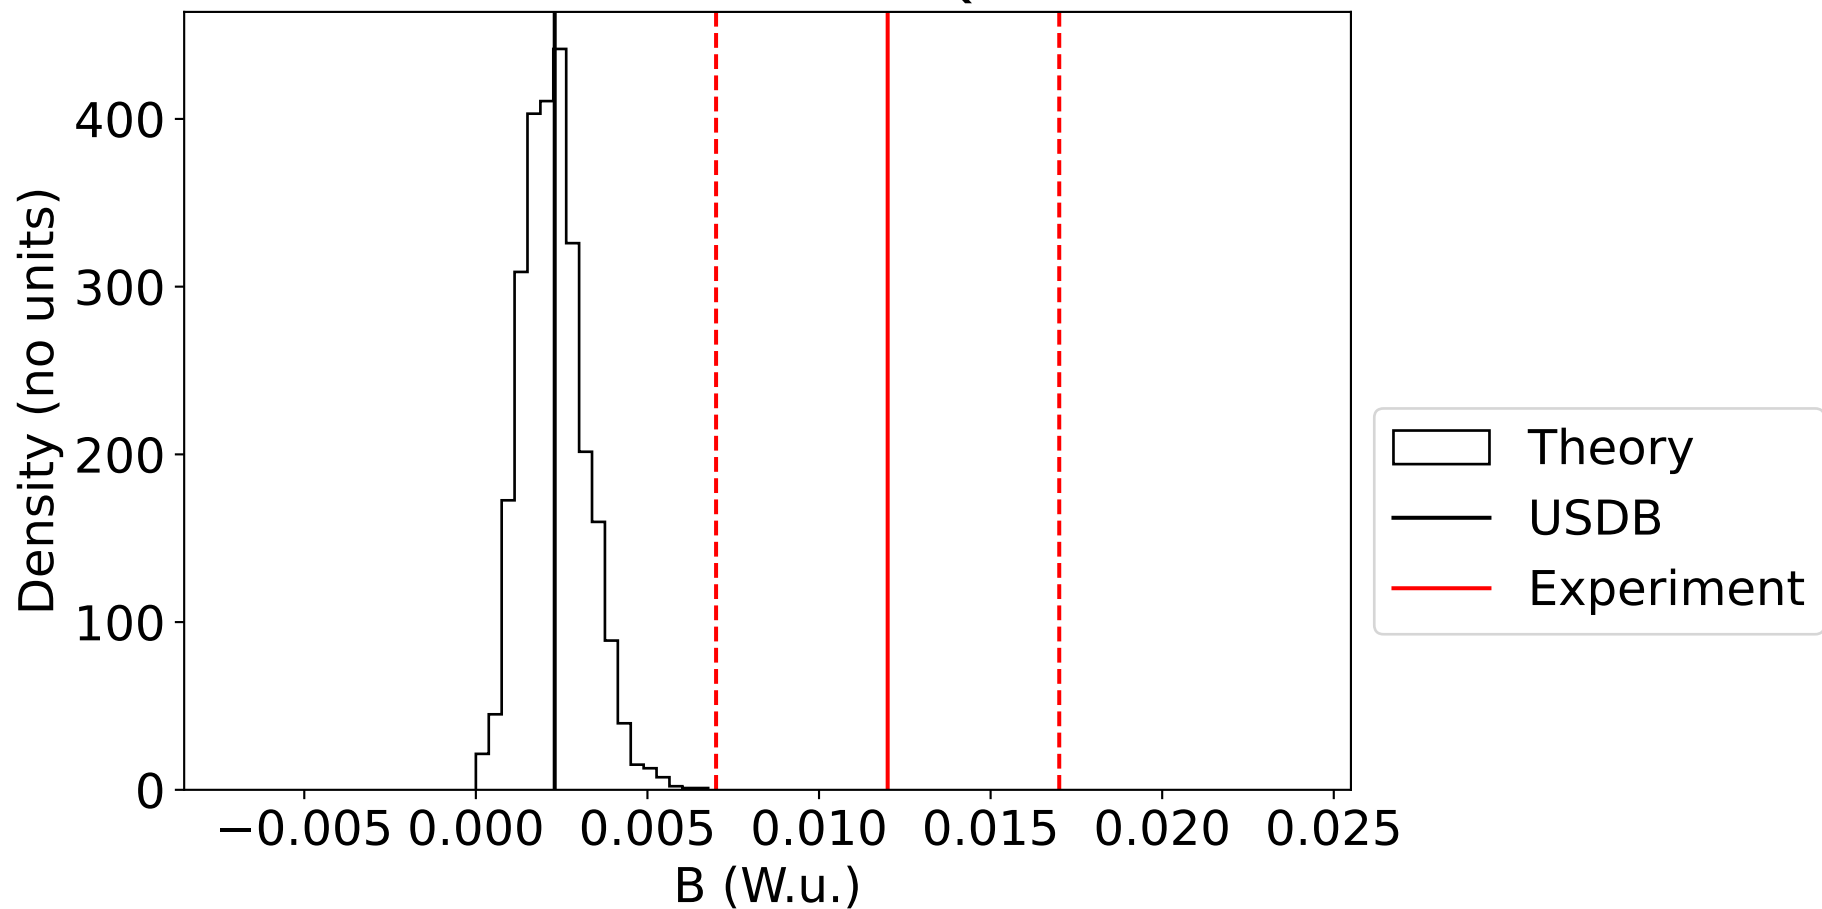

$^{26}\text{Mg} (5_1) \rightarrow (4_3)$   
Included in UQ

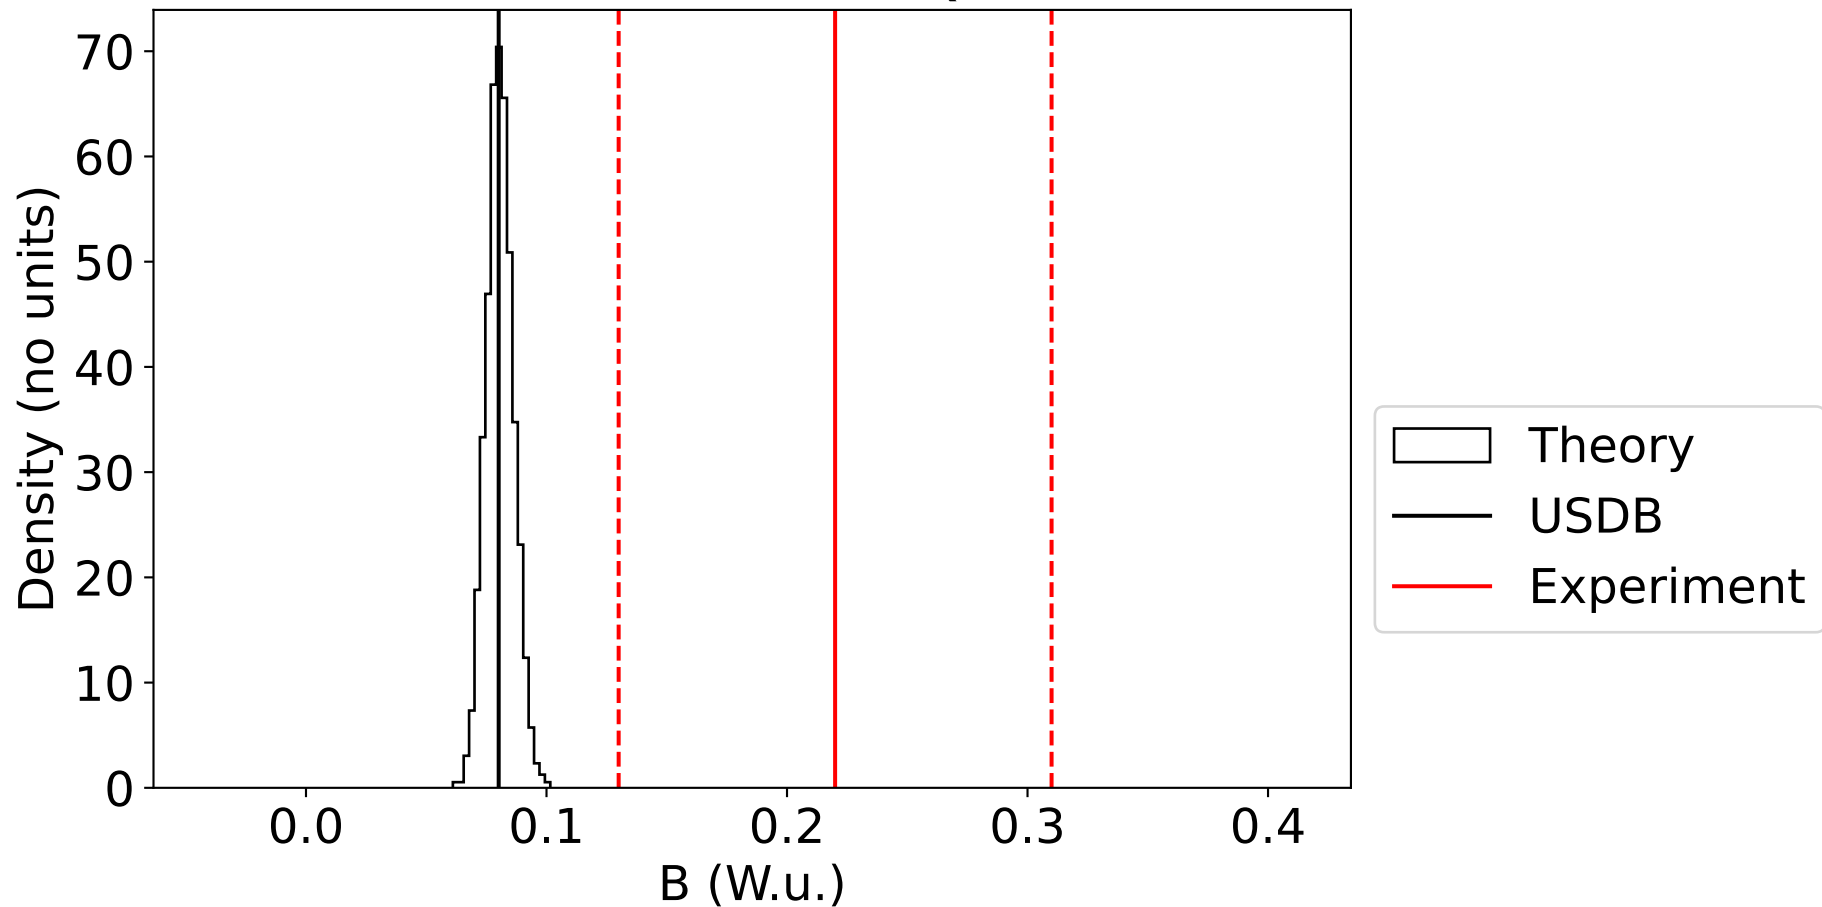



$^{27}\text{Mg} (3/2_1) \rightarrow (1/2_1)$   
Included in UQ

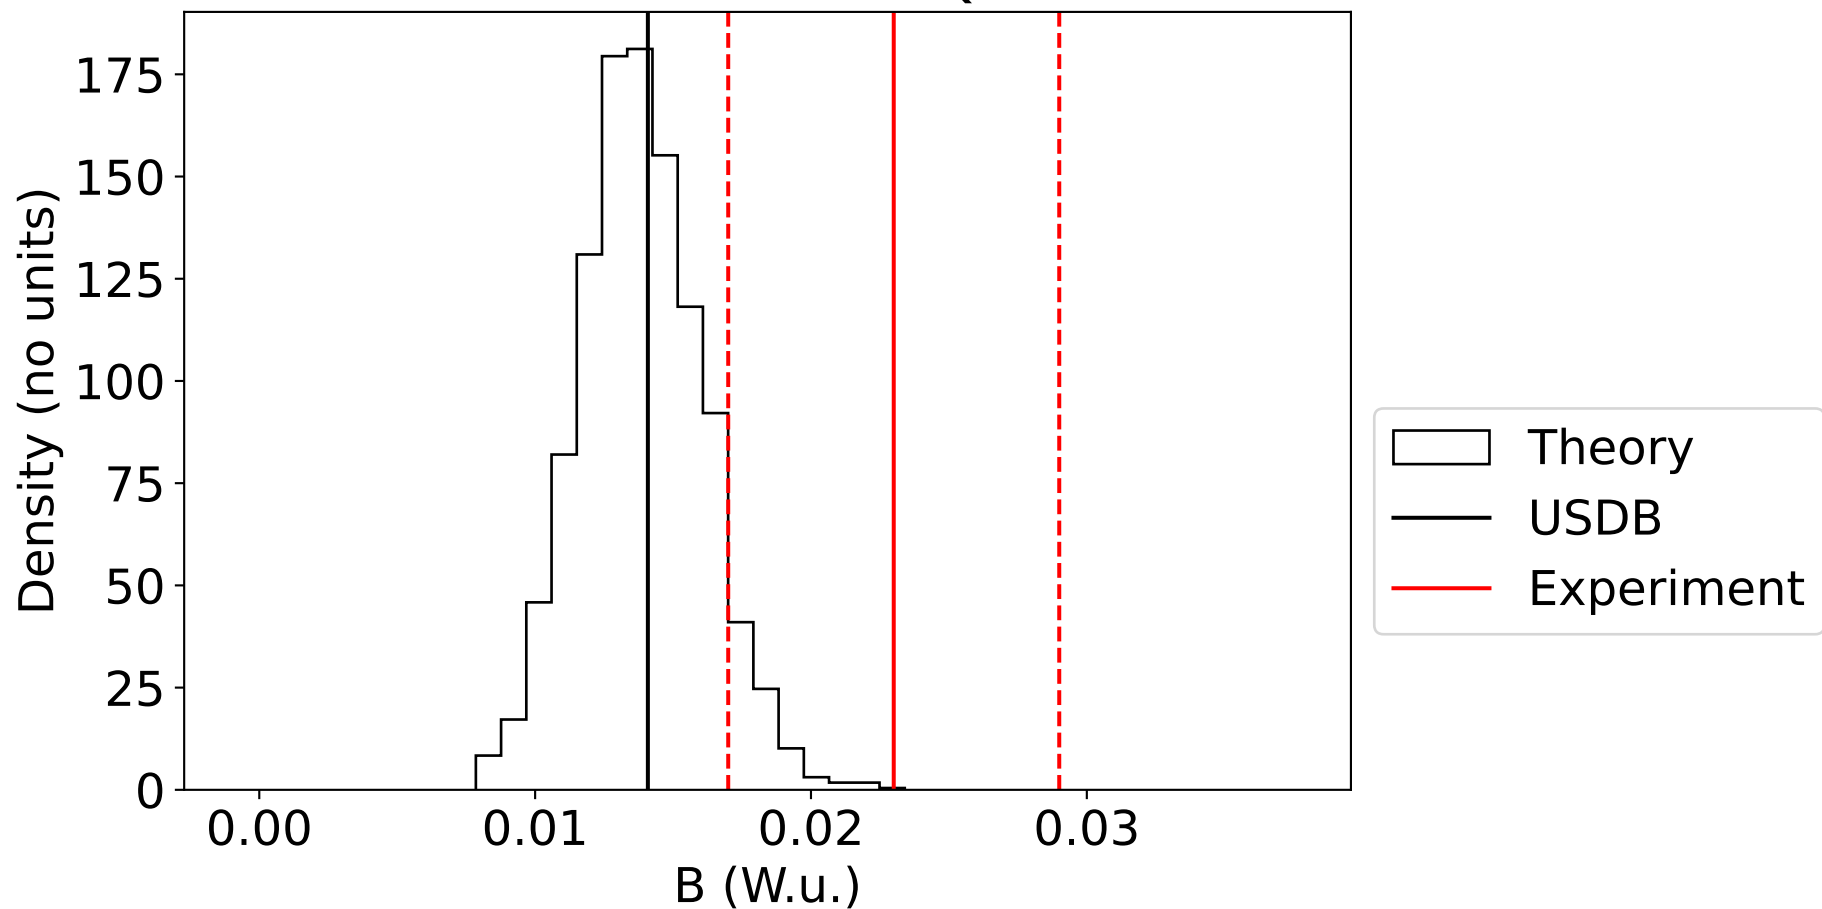

$^{27}\text{Mg } (7/2_1) \rightarrow (5/2_2)$   
Included in UQ

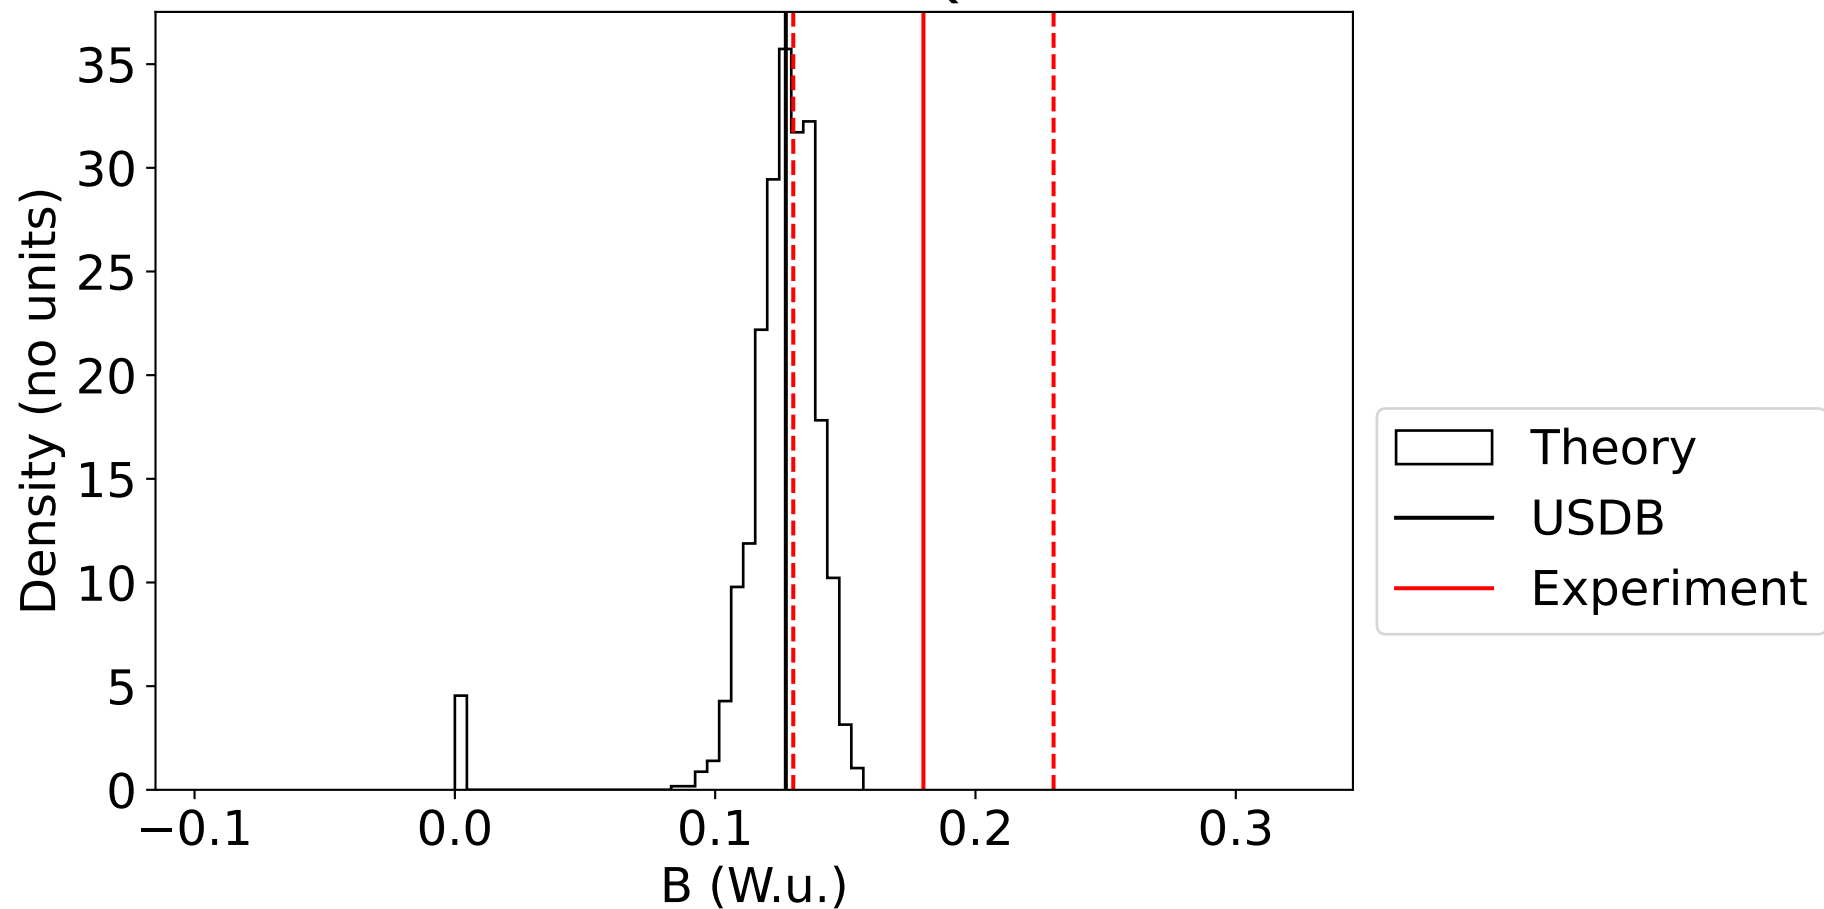

$^{31}\text{Mg} (3/2_1) \rightarrow (1/2_1)$   
Included in UQ

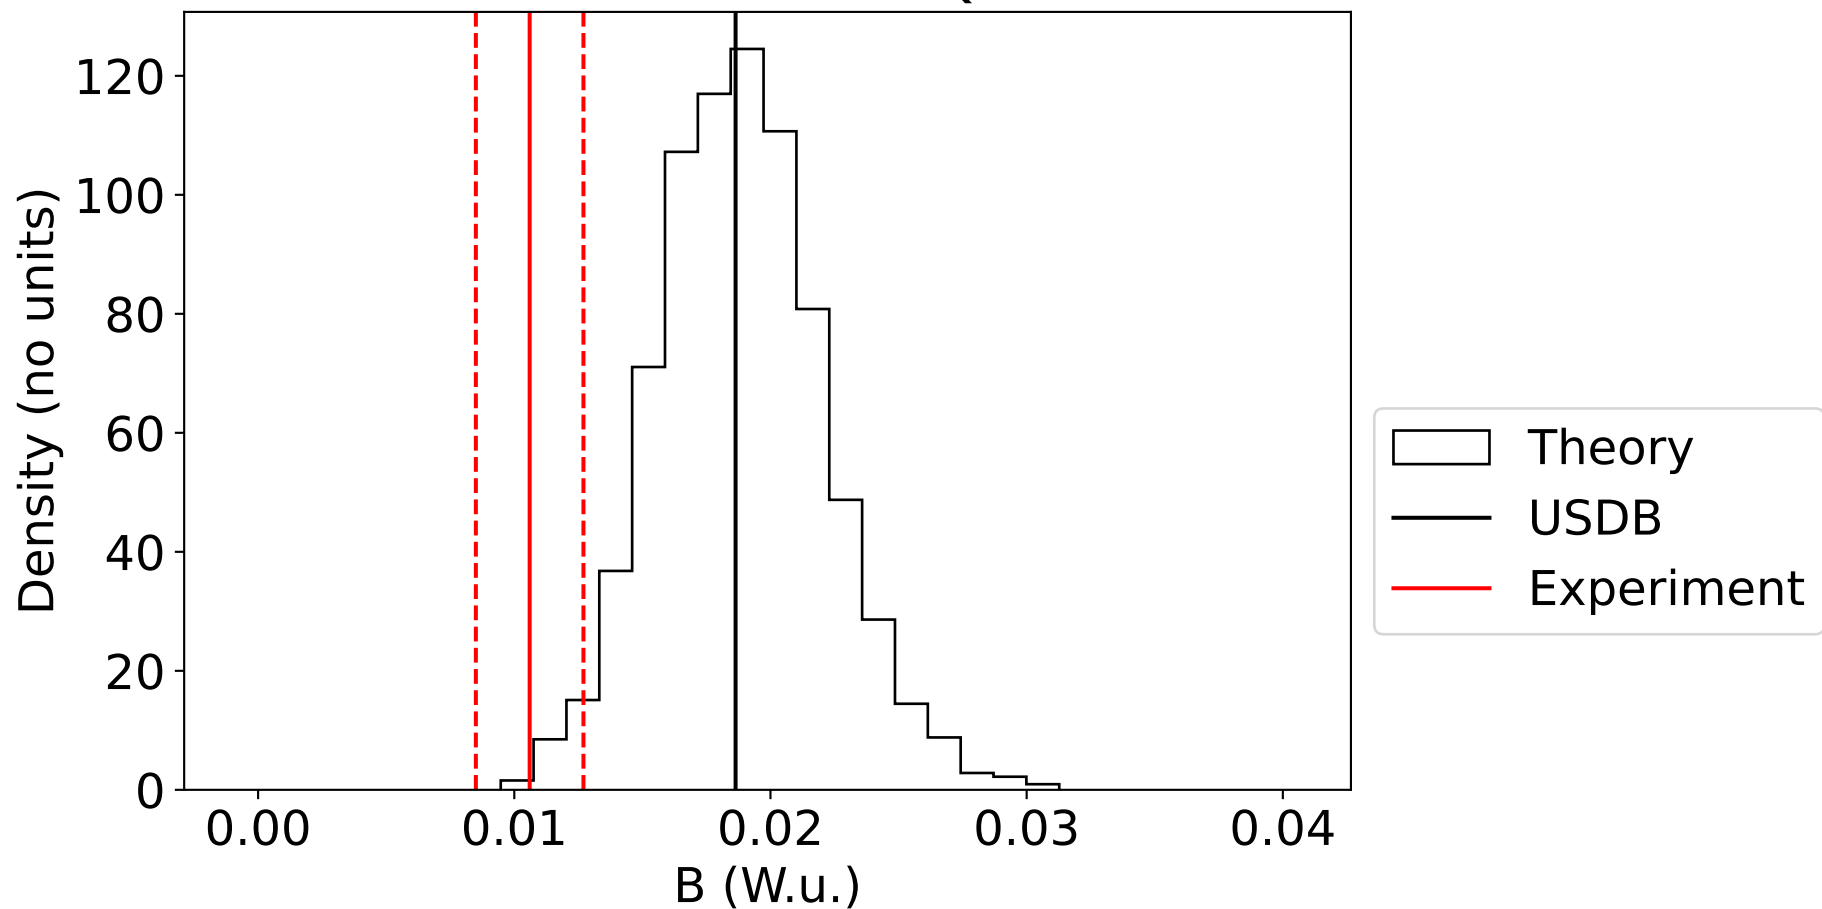

$^{25}\text{Al} (3/2_1) \rightarrow (1/2_1)$   
Included in UQ

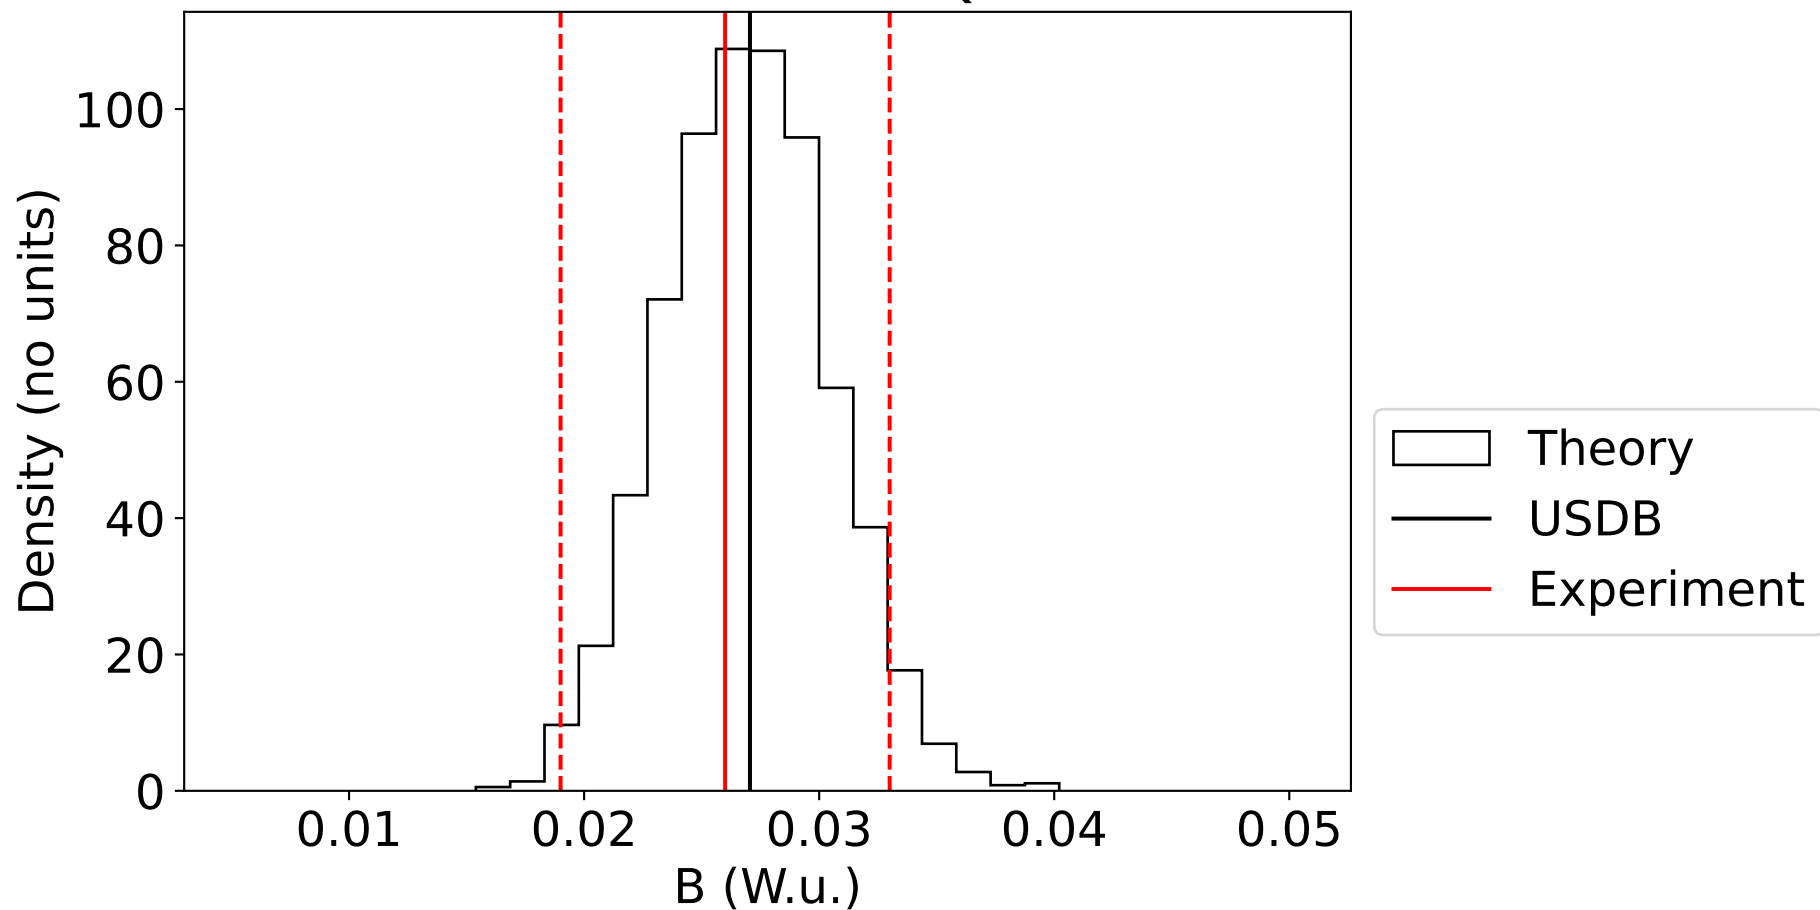

$^{25}\text{Al} (7/2_1) \rightarrow (5/2_1)$   
Included in UQ

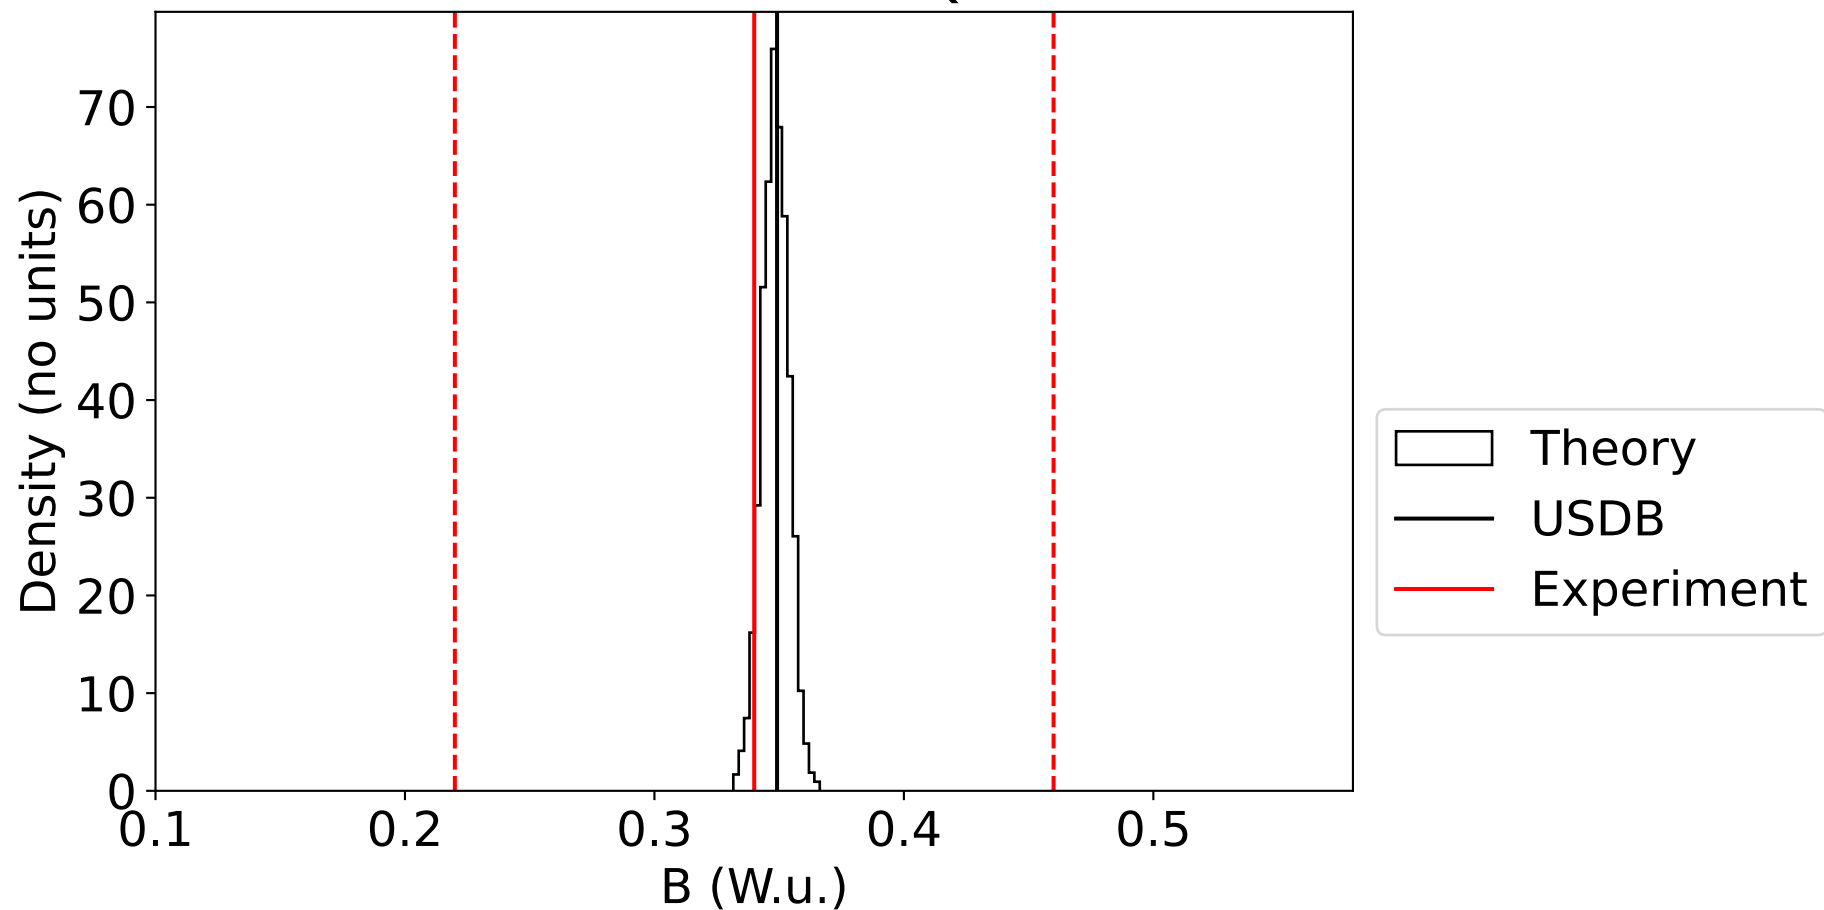

$^{25}\text{Al} (5/2_2) \rightarrow (3/2_1)$   
Included in UQ

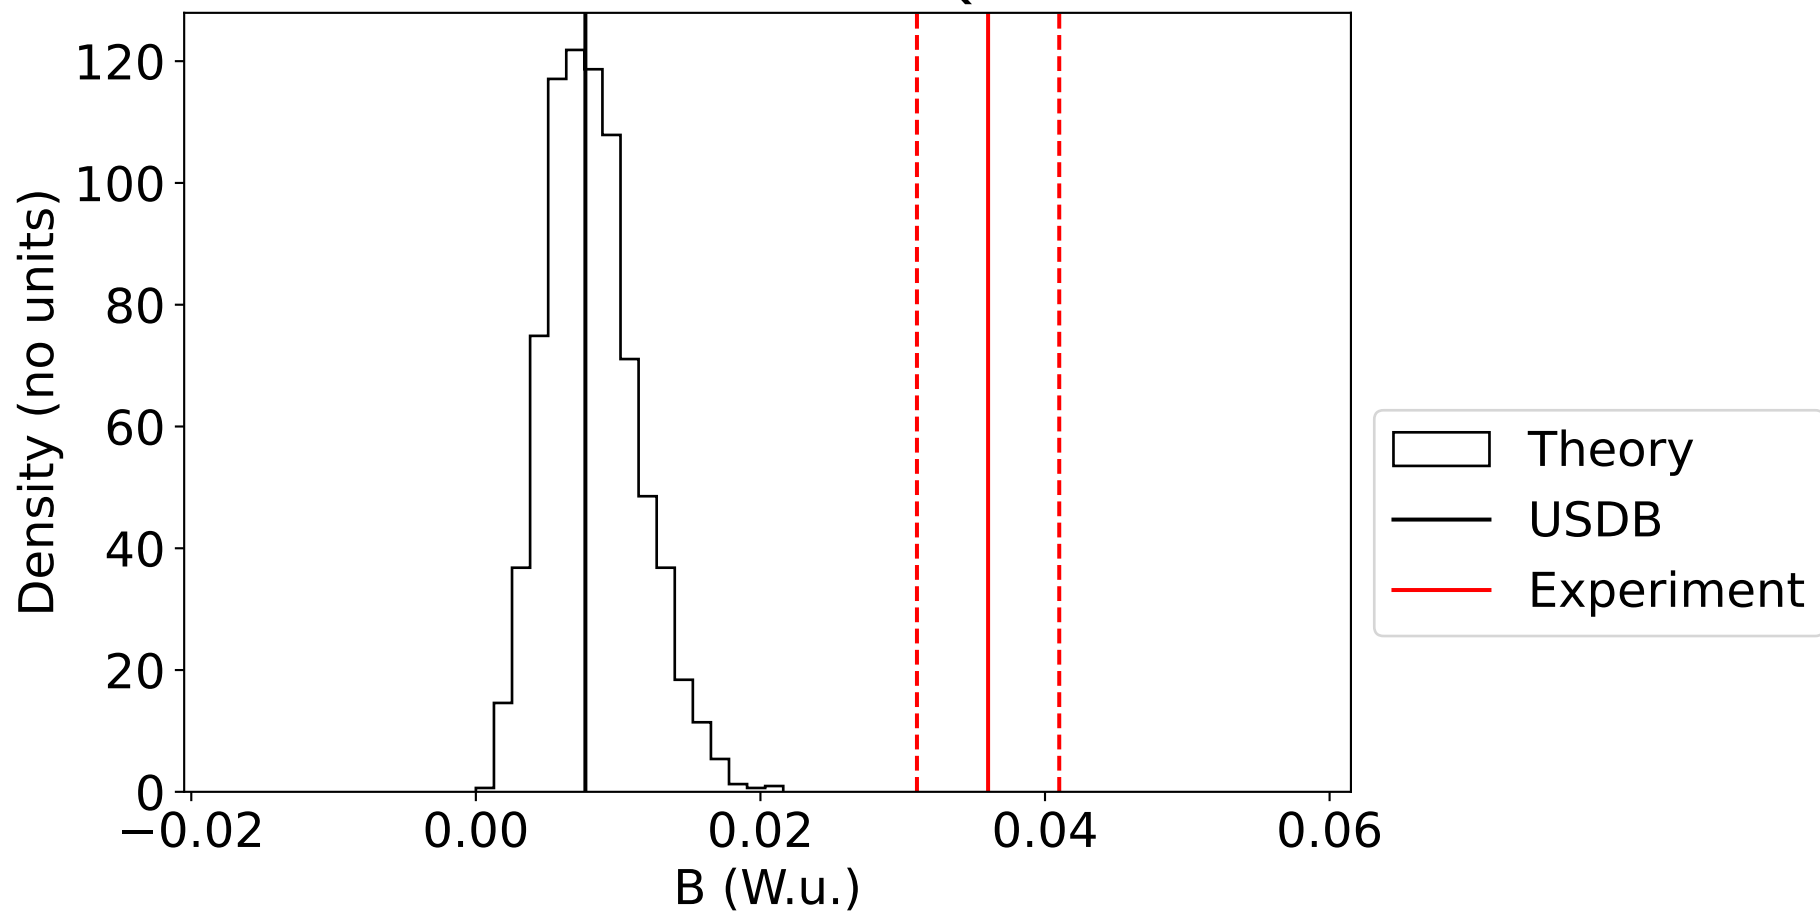

$^{25}\text{Al } (1/2_2) \rightarrow (1/2_1)$   
Included in UQ

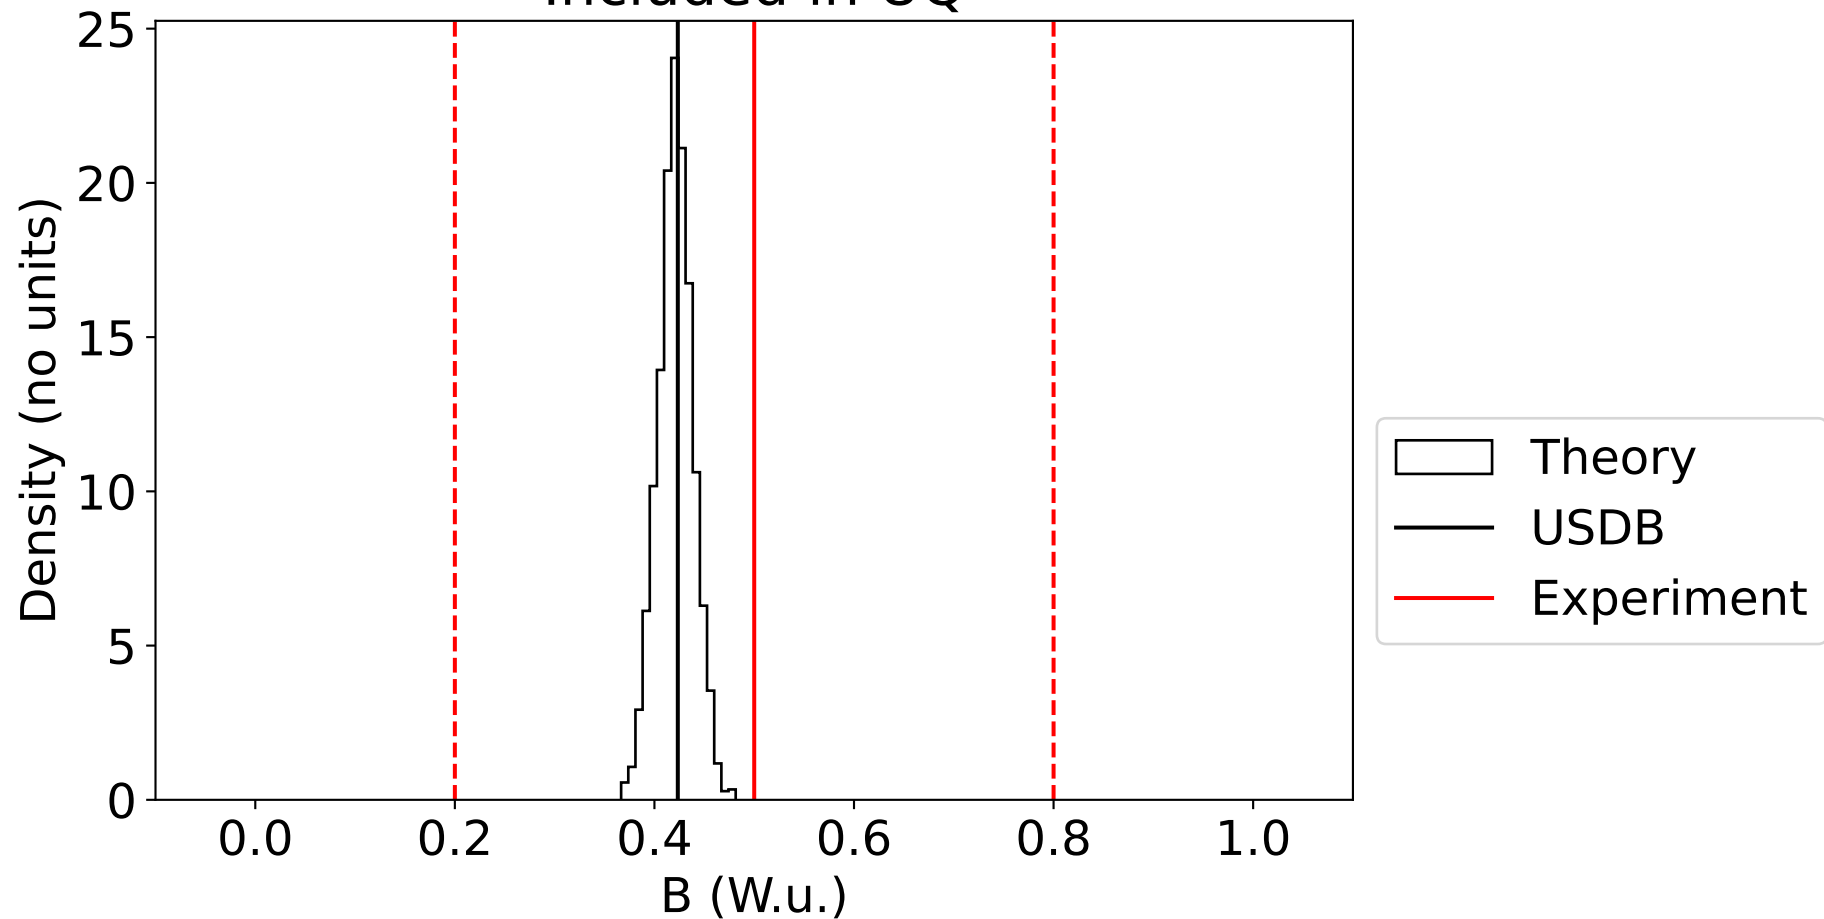

$^{25}\text{Al} (3/2_2) \rightarrow (5/2_1)$   
Included in UQ

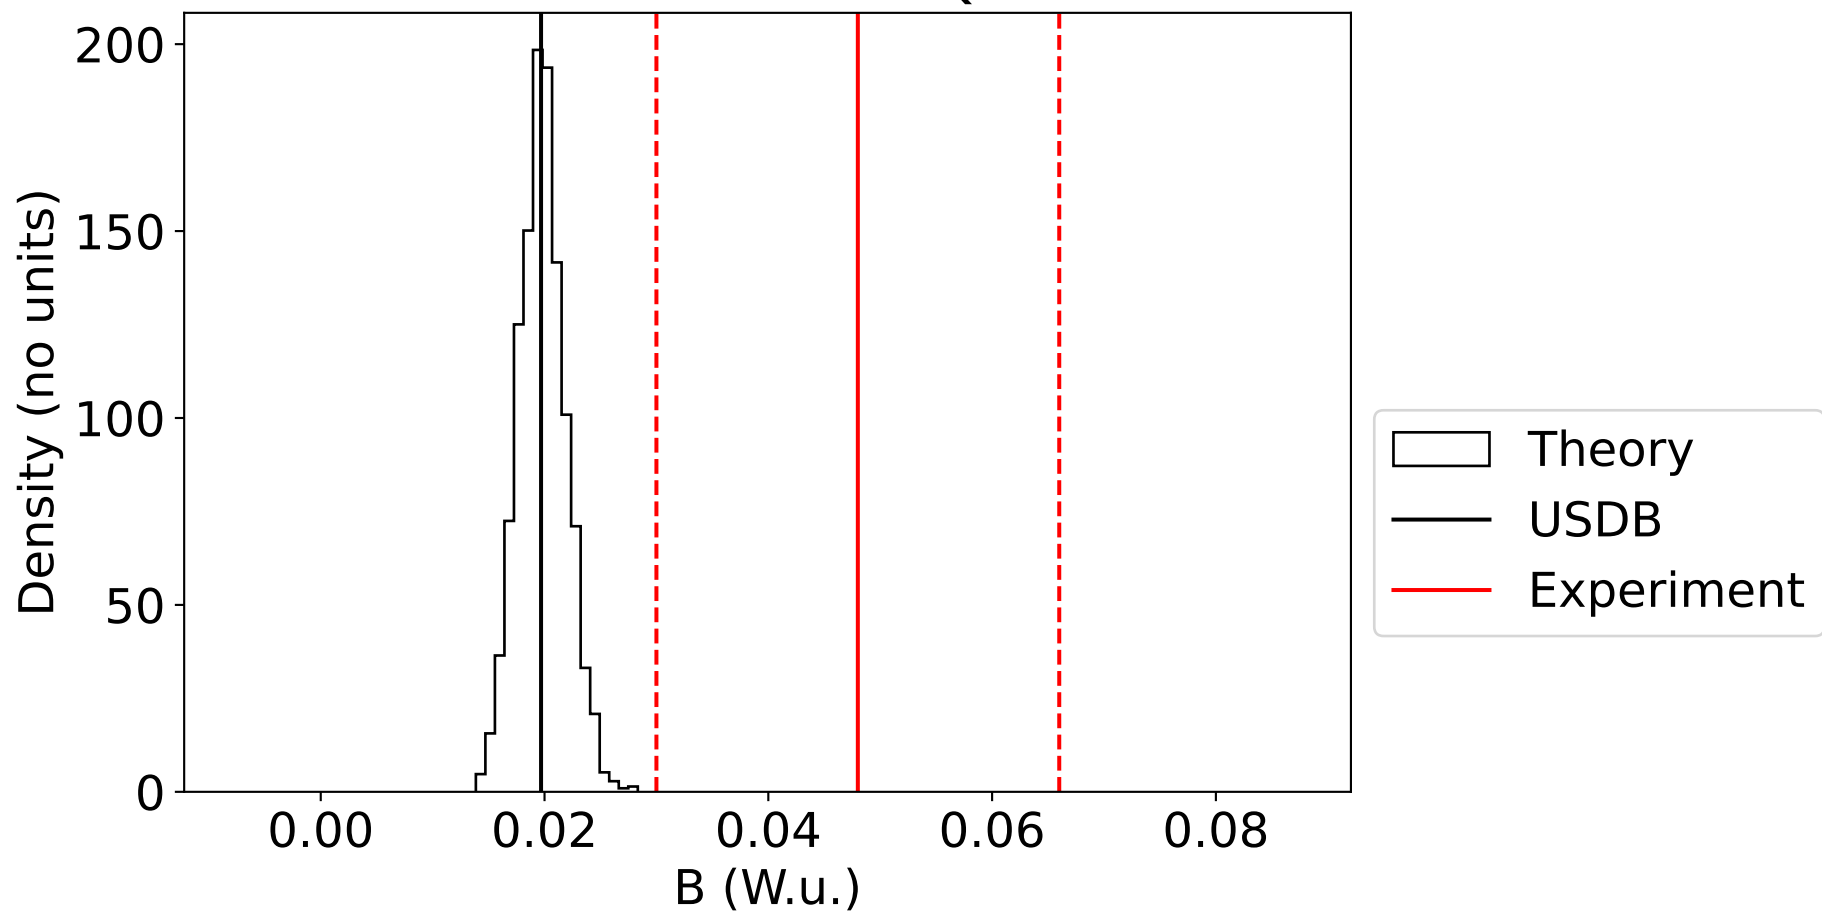



$^{25}\text{Al} (7/2_2) \rightarrow (5/2_2)$   
Included in UQ

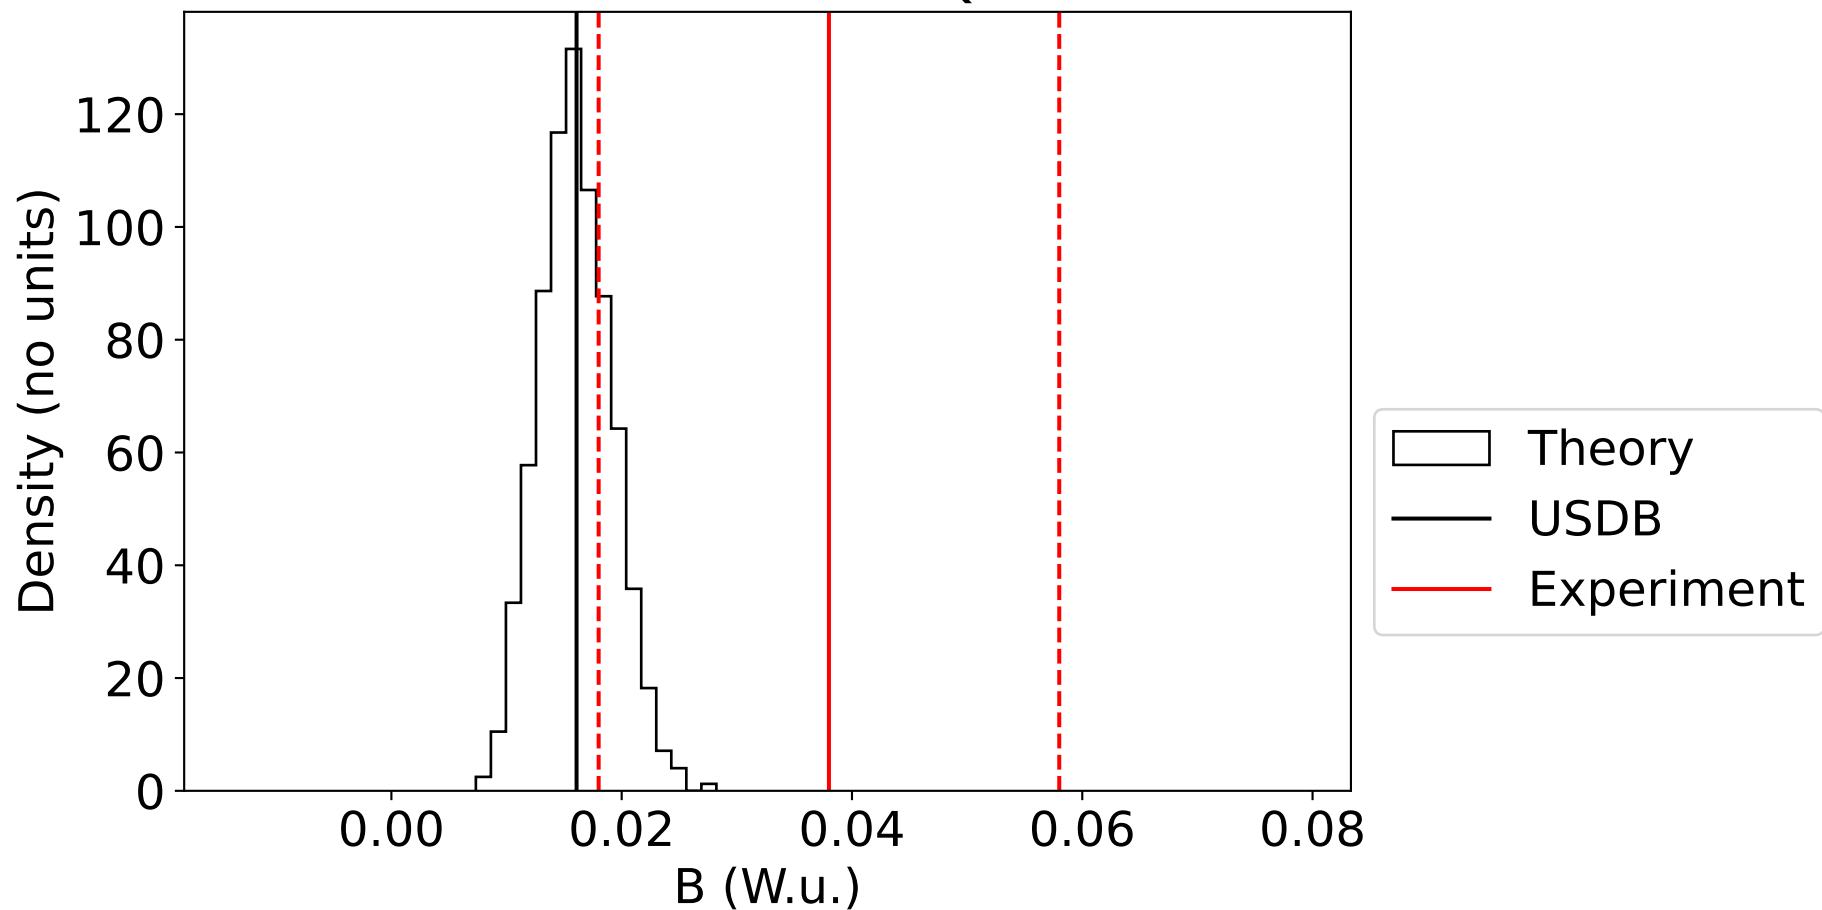

$^{25}\text{Al} (9/2_1) \rightarrow (7/2_1)$   
Included in UQ

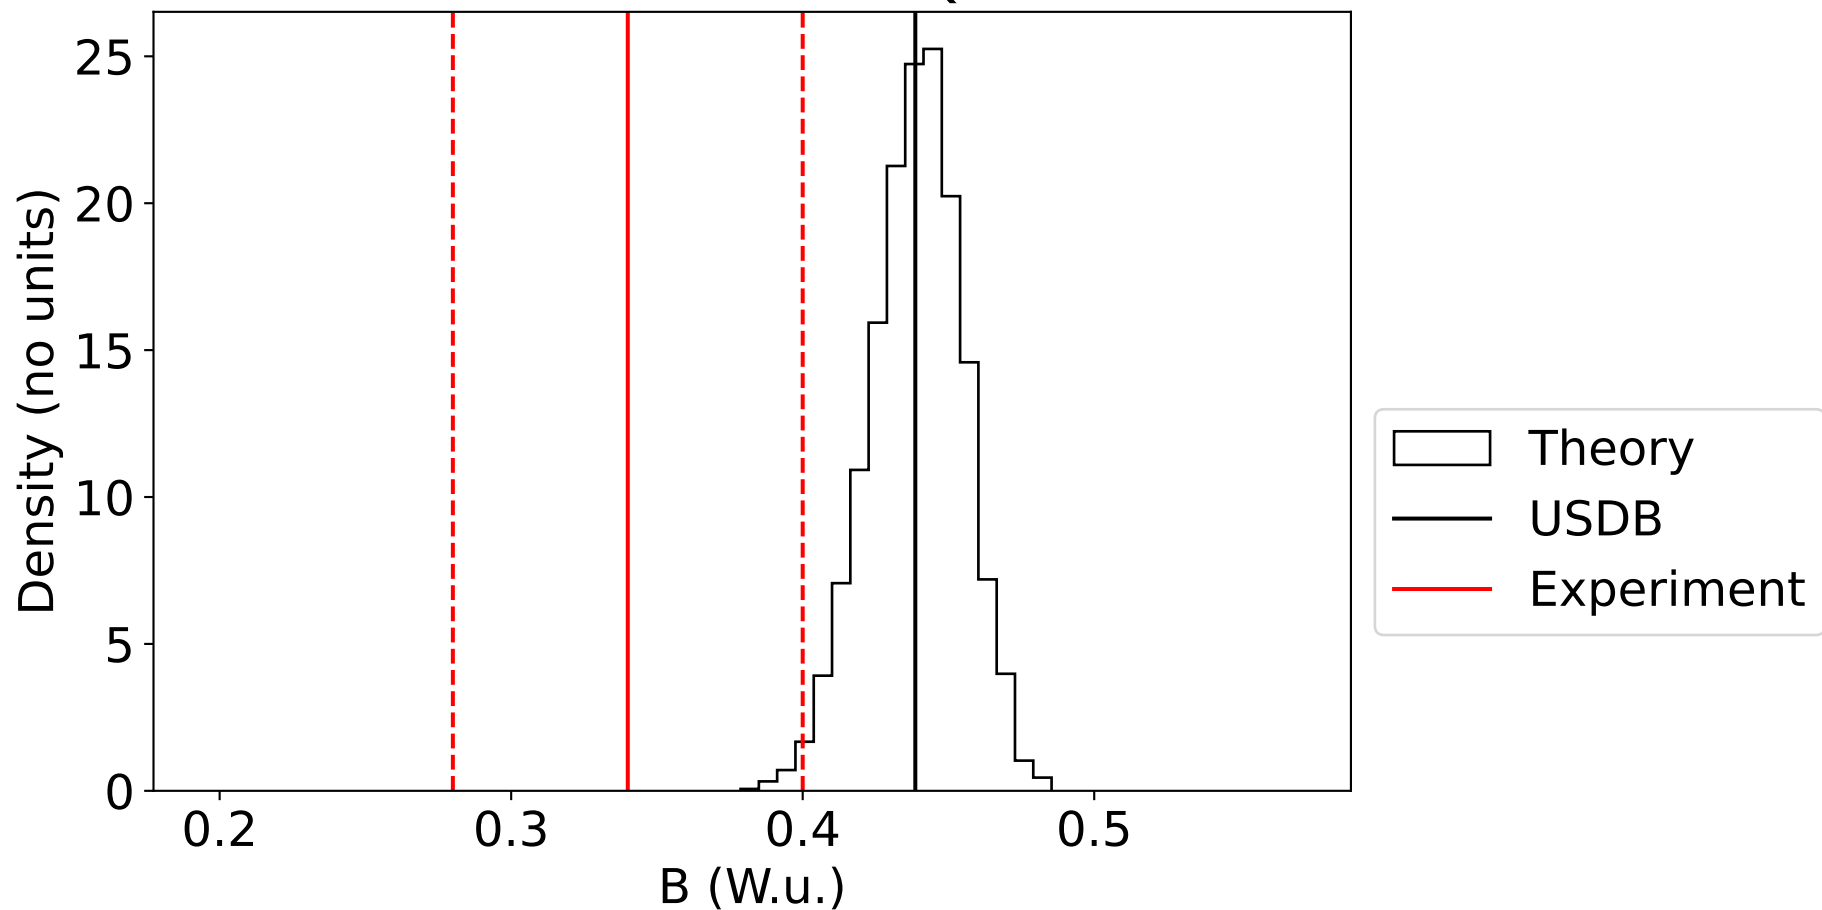

$^{26}\text{Al} (1_1) \rightarrow (0_1)$   
Included in UQ

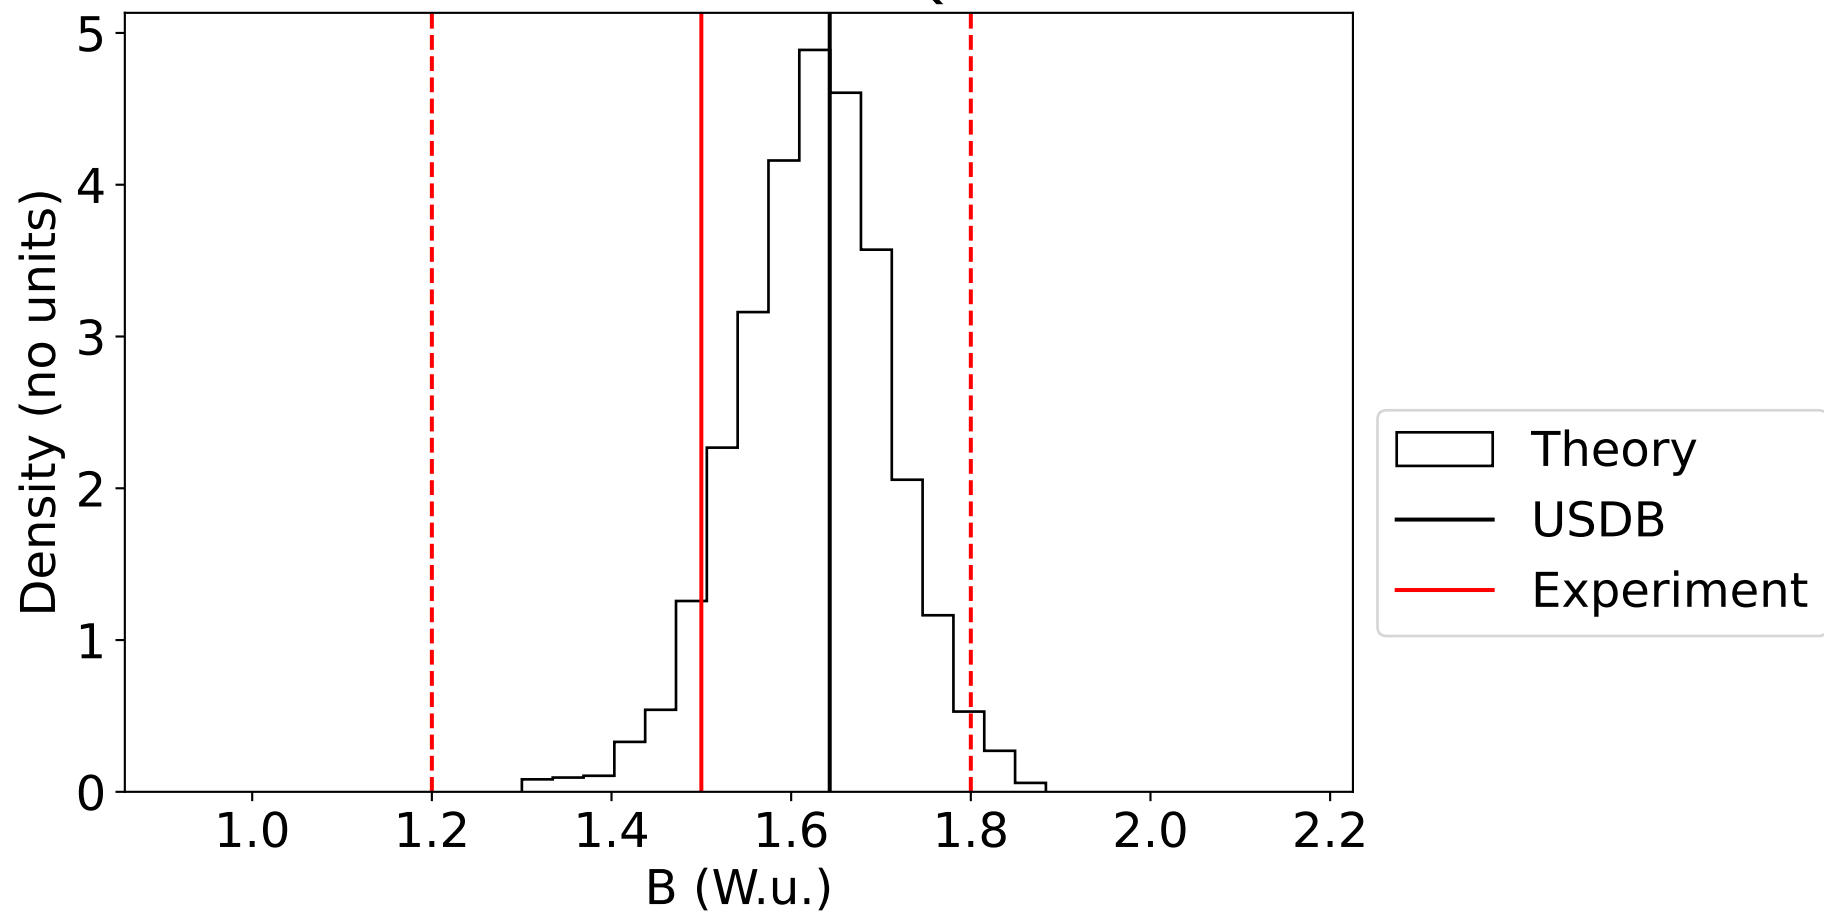

$^{26}\text{Al} (1_2) \rightarrow (0_1)$   
Included in UQ

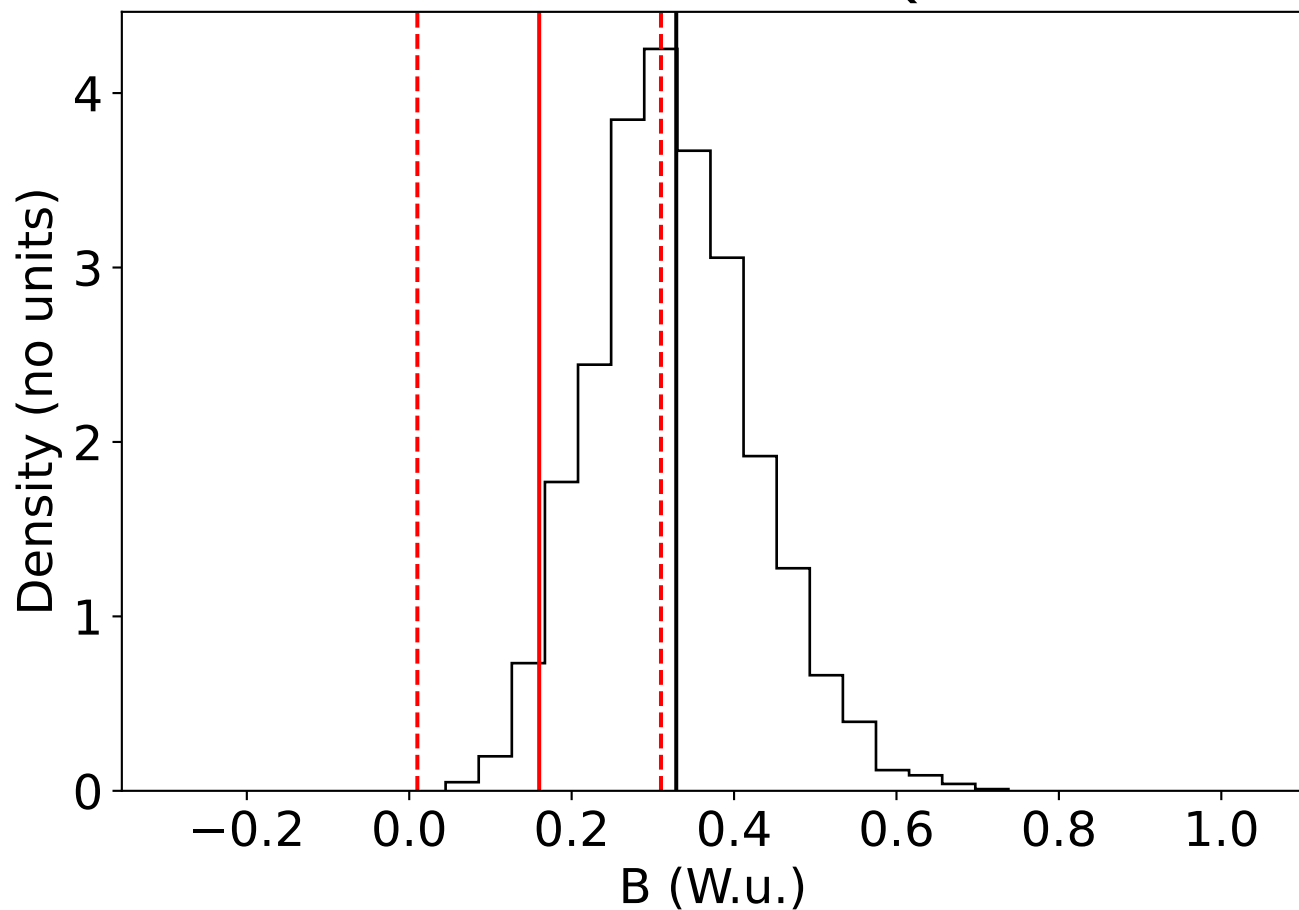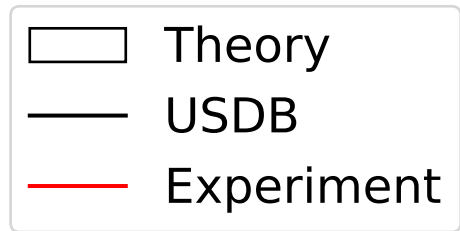

$^{26}\text{Al} (2_2) \rightarrow (1_1)$   
Included in UQ

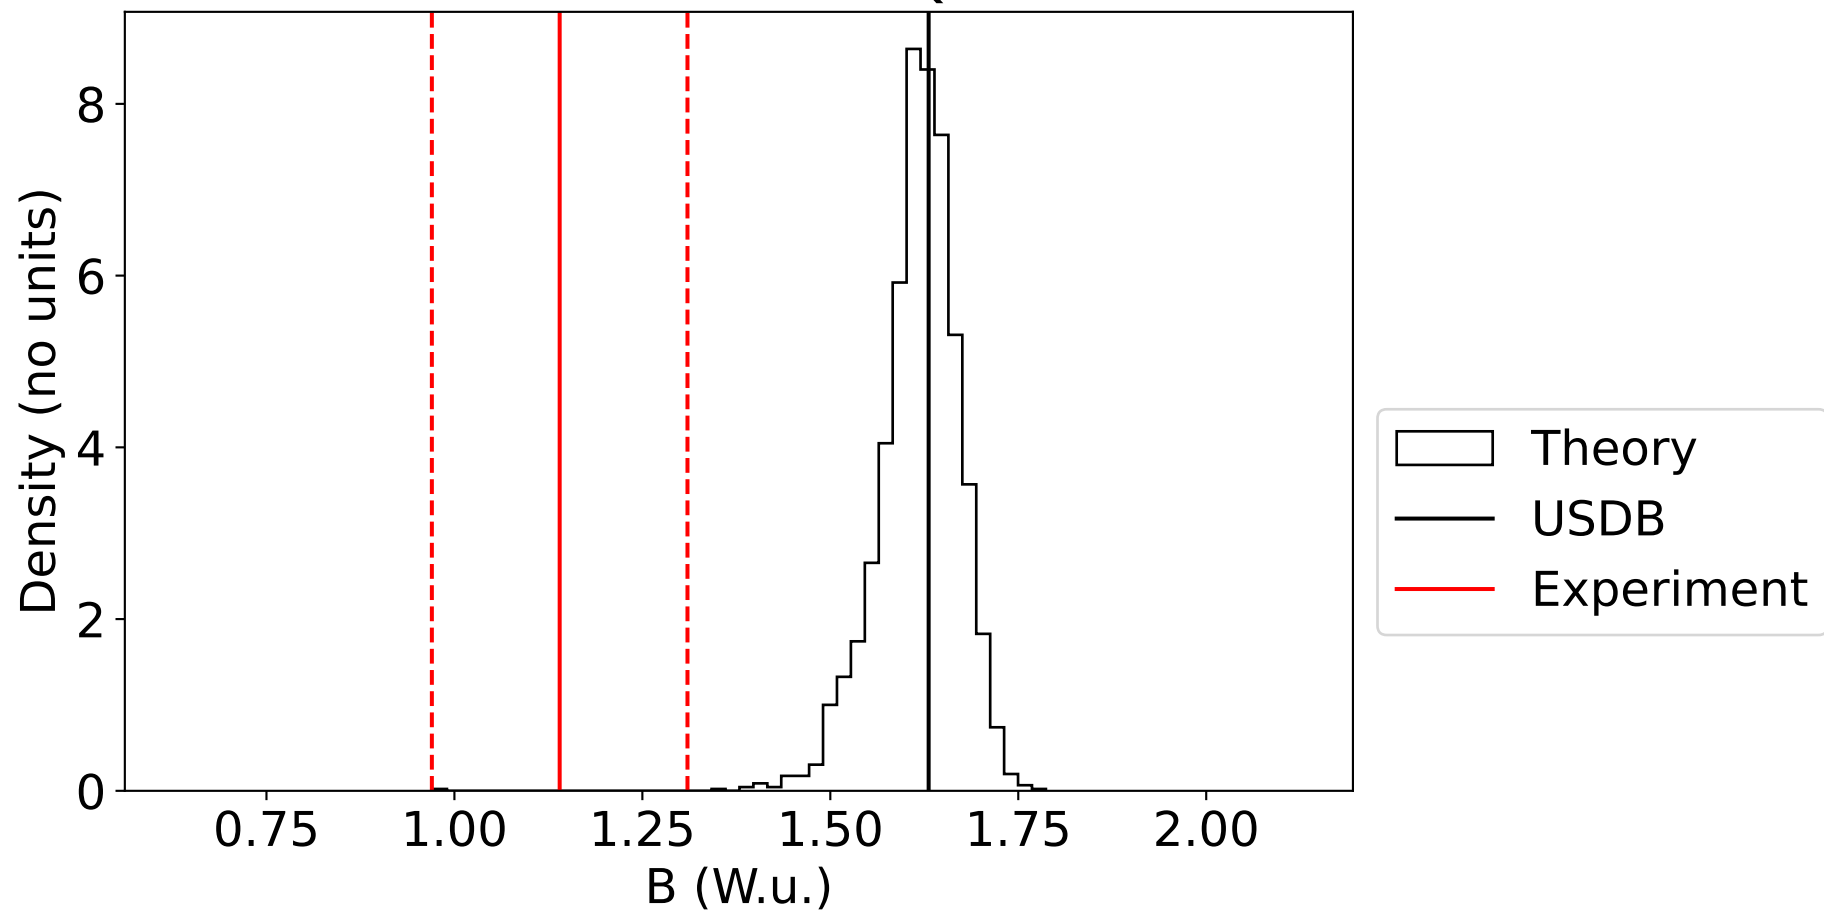

$^{26}\text{Al} (2_2) \rightarrow (2_1)$   
Included in UQ

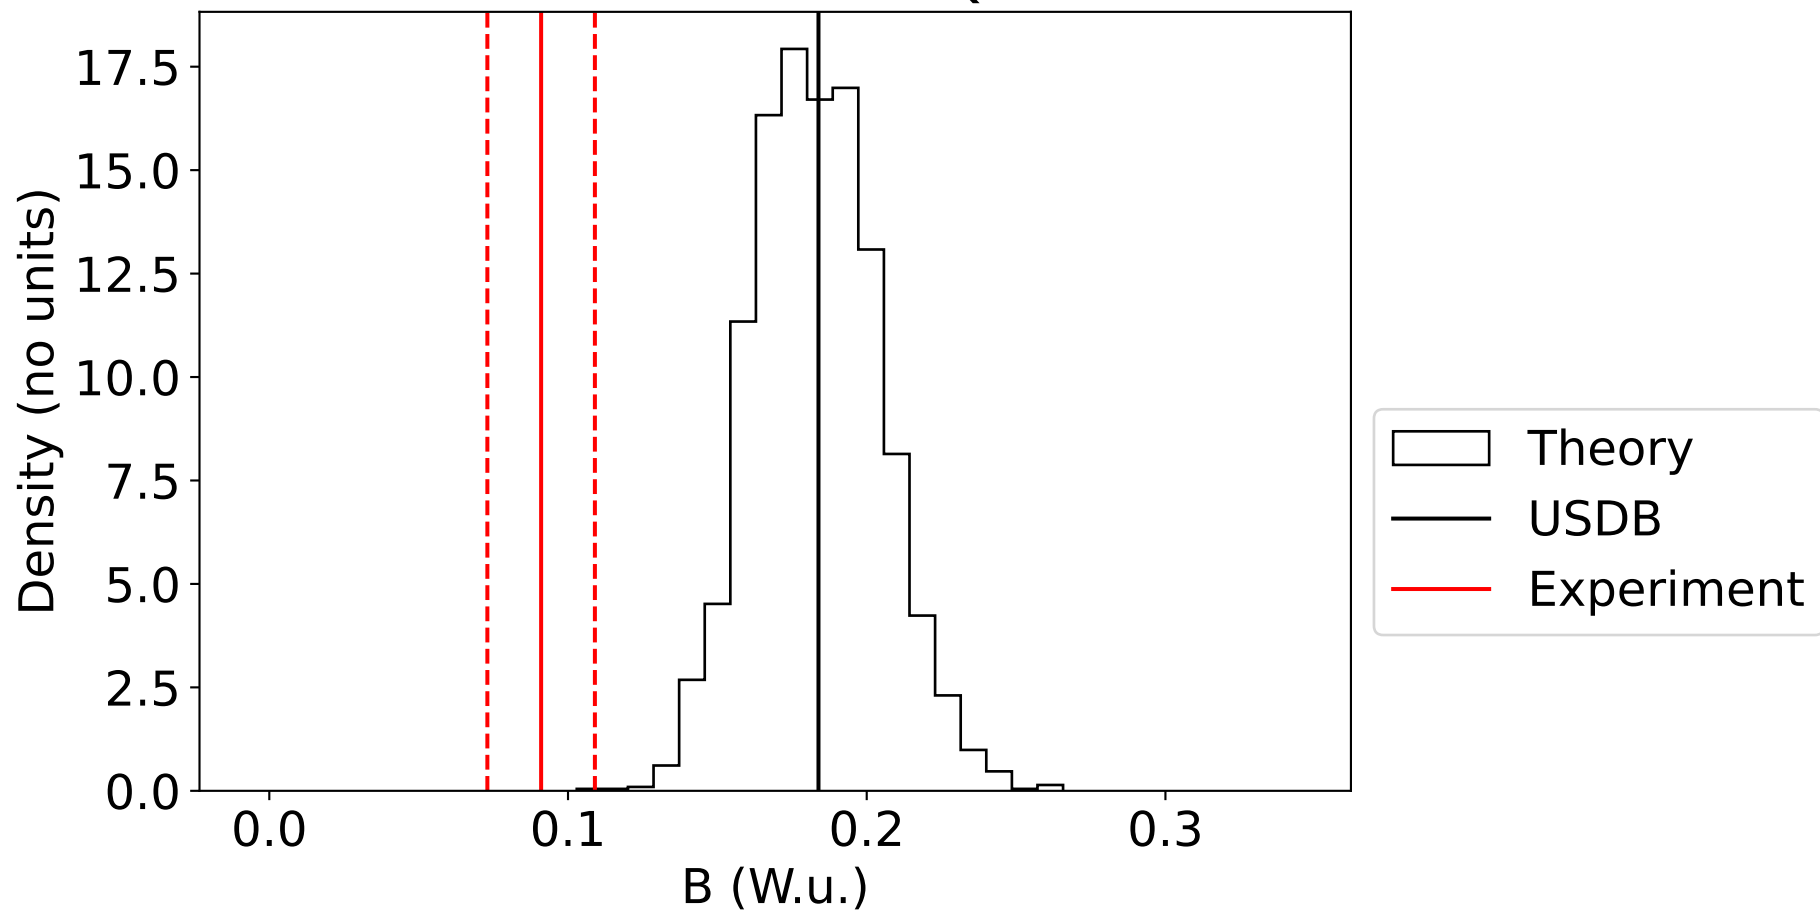

$^{26}\text{Al} (2_2) \rightarrow (1_2)$   
Included in UQ

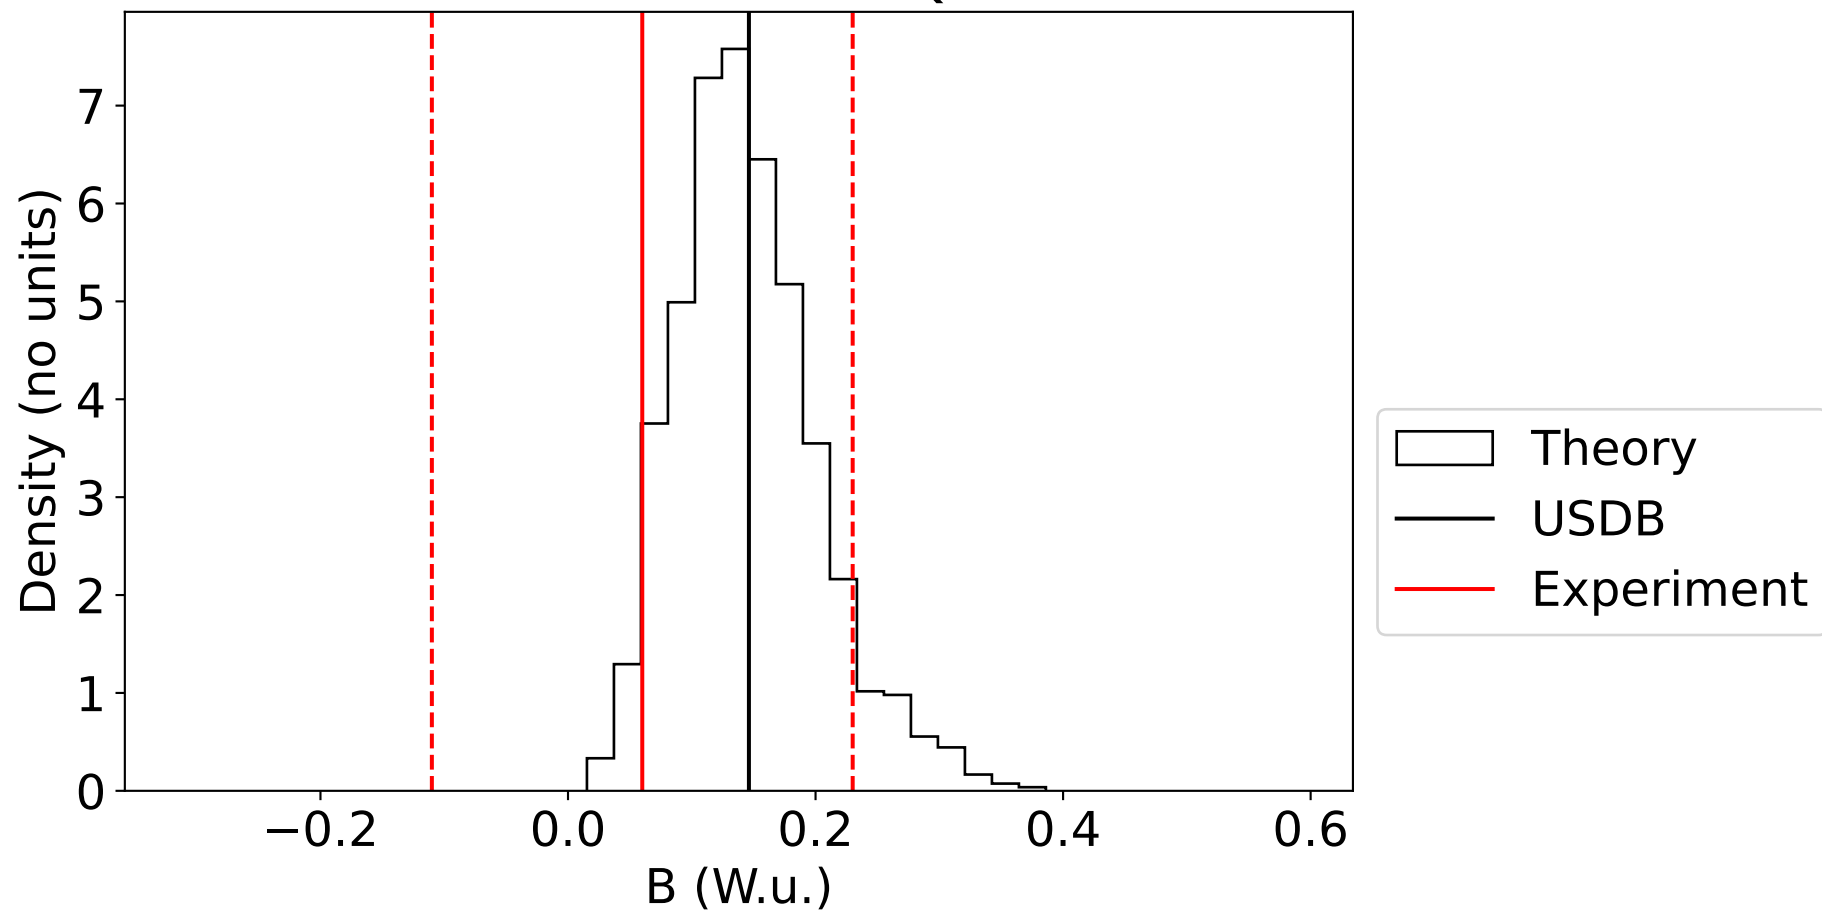

$^{26}\text{Al} (2_2) \rightarrow (3_1)$   
Included in UQ

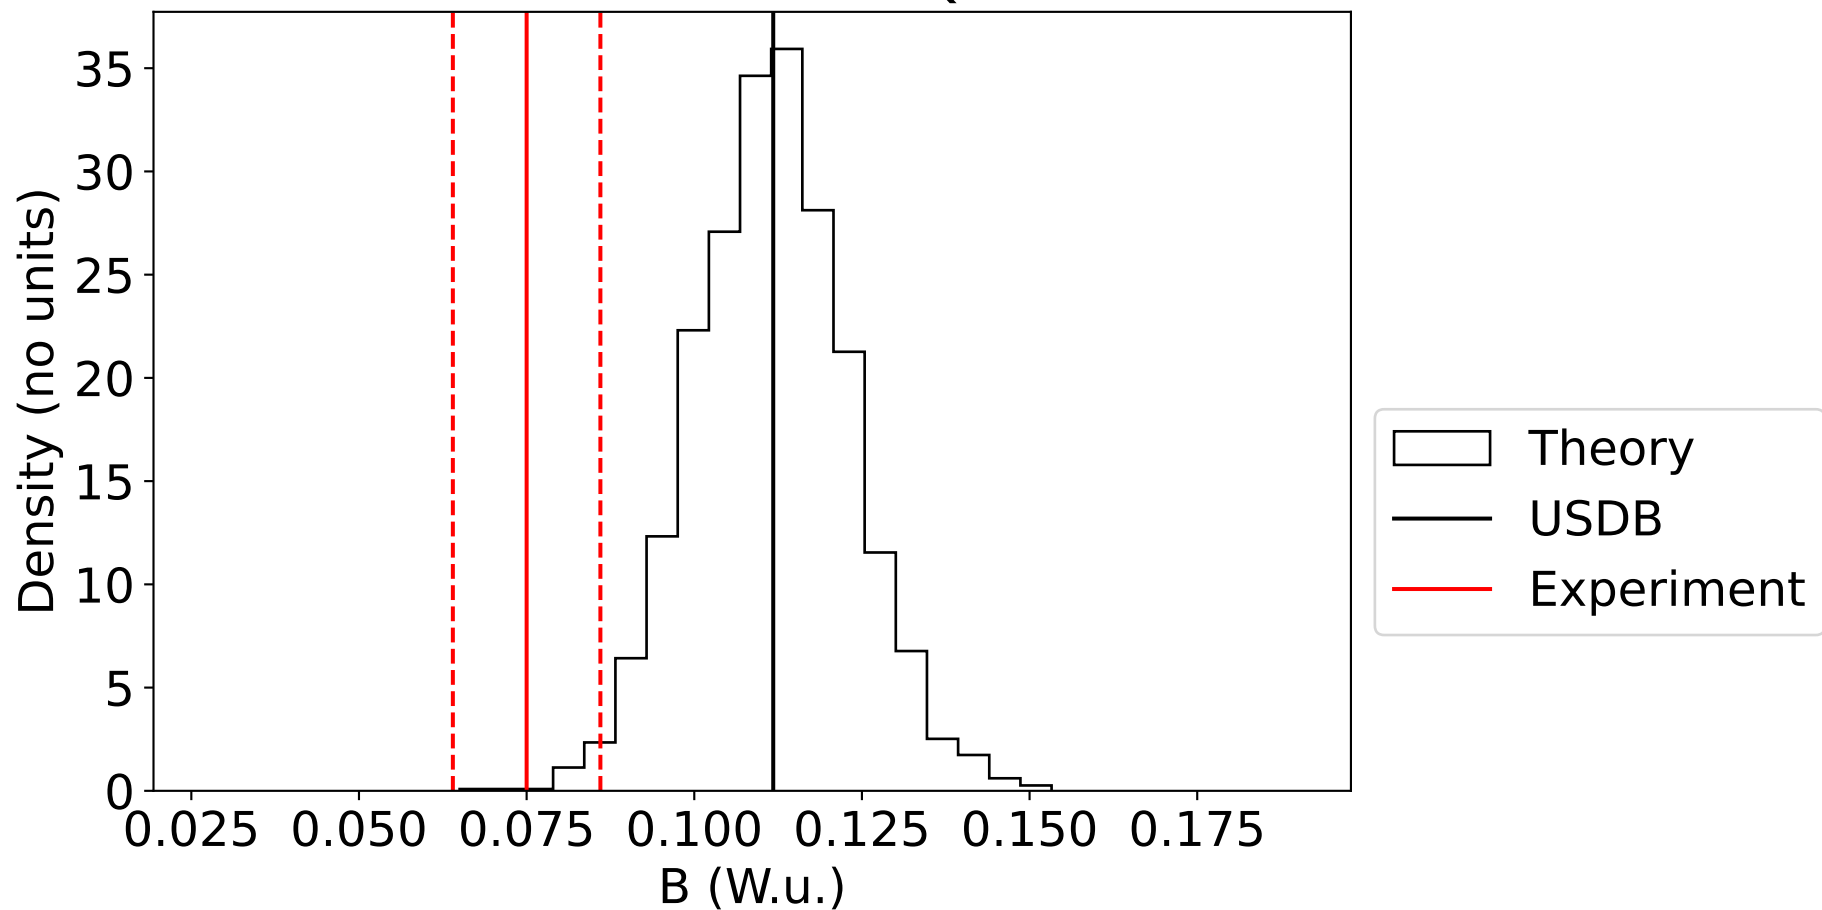



$^{26}\text{Al} (1_4) \rightarrow (0_1)$   
Included in UQ

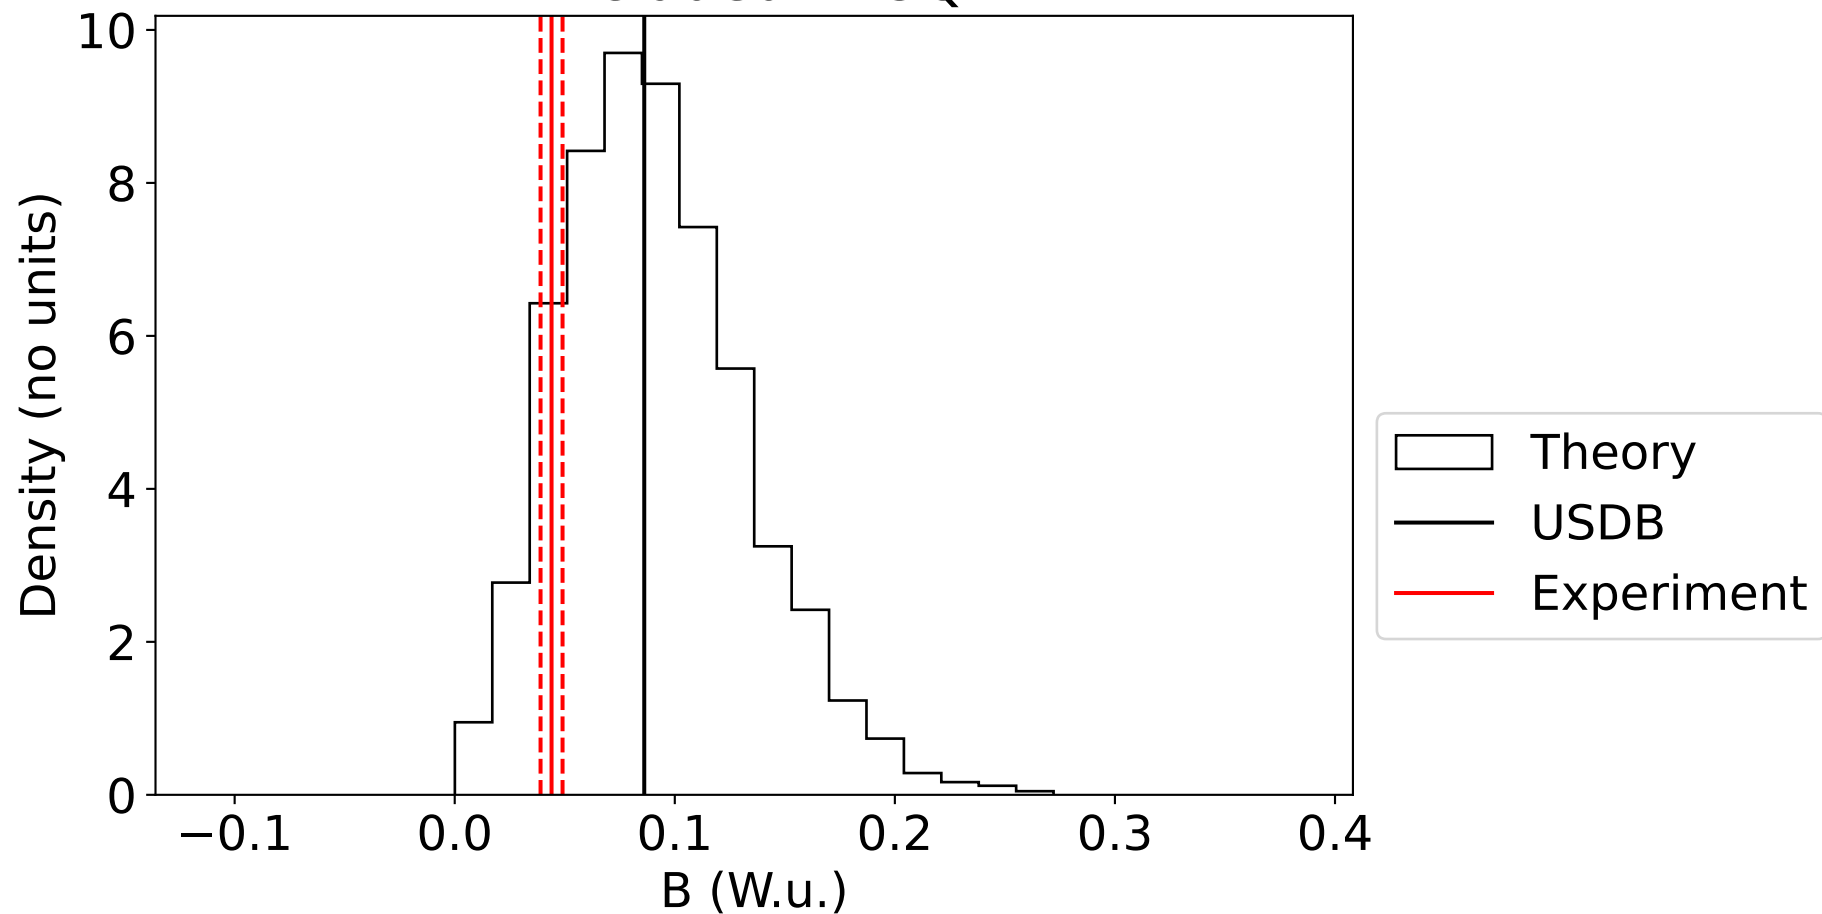

$^{26}\text{Al} (2_5) \rightarrow (2_1)$   
Included in UQ

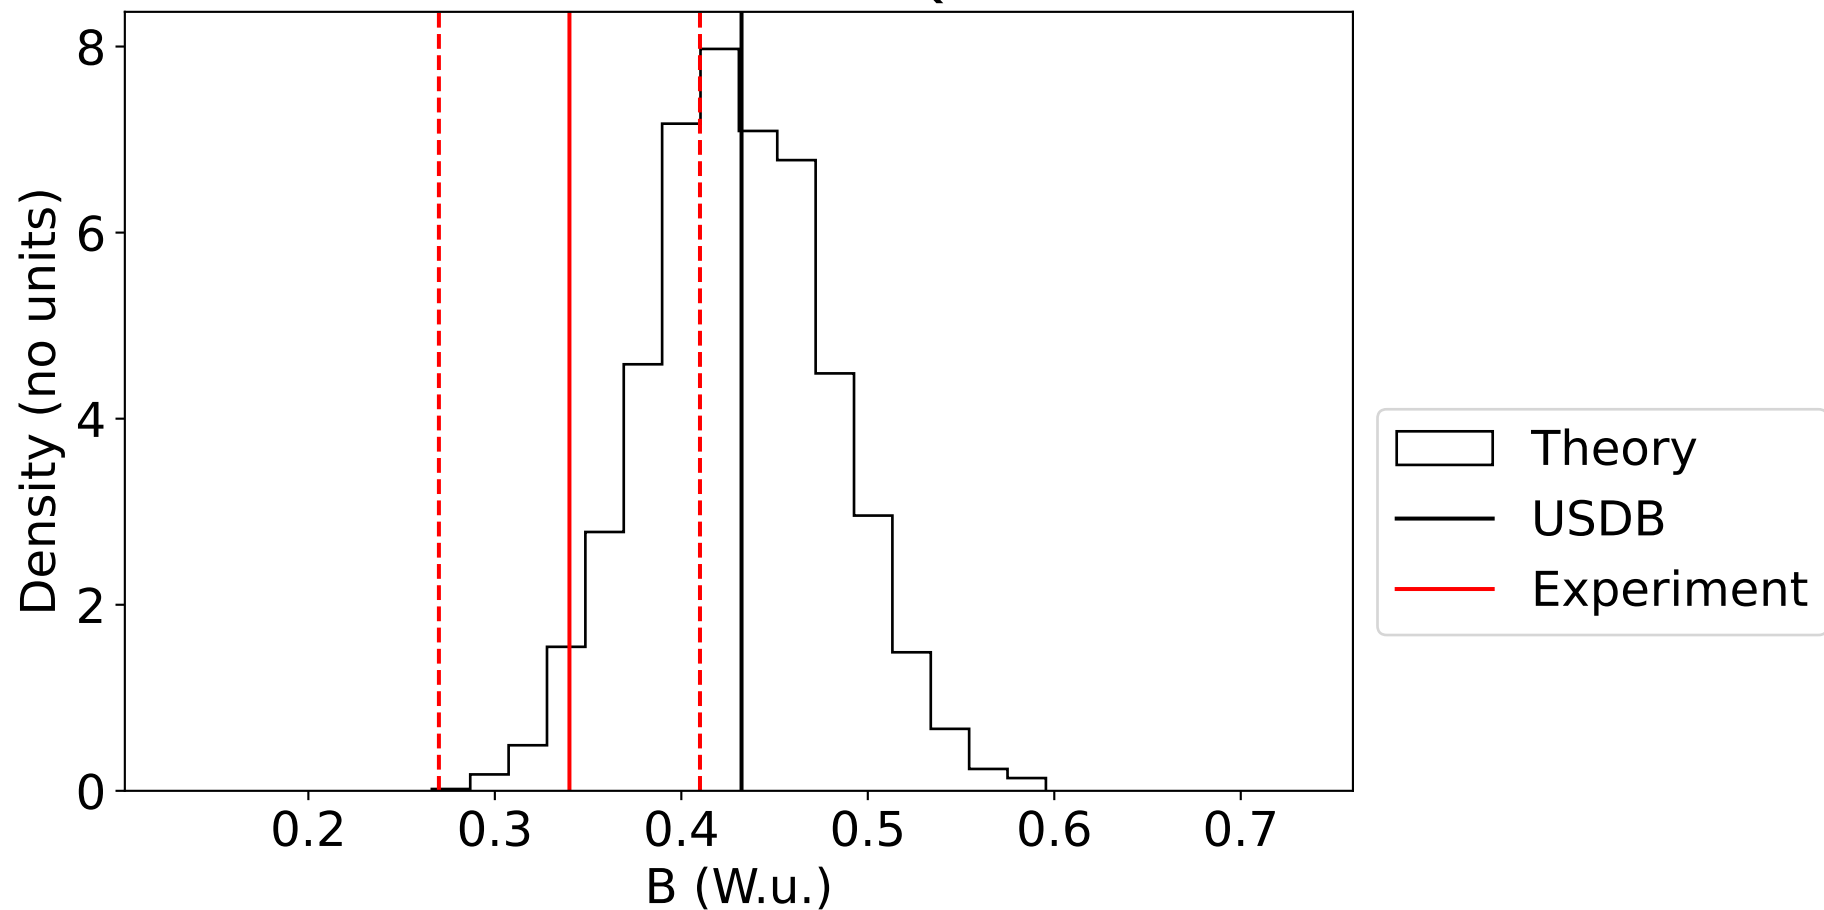

$^{26}\text{Al} (2_5) \rightarrow (3_1)$   
Included in UQ

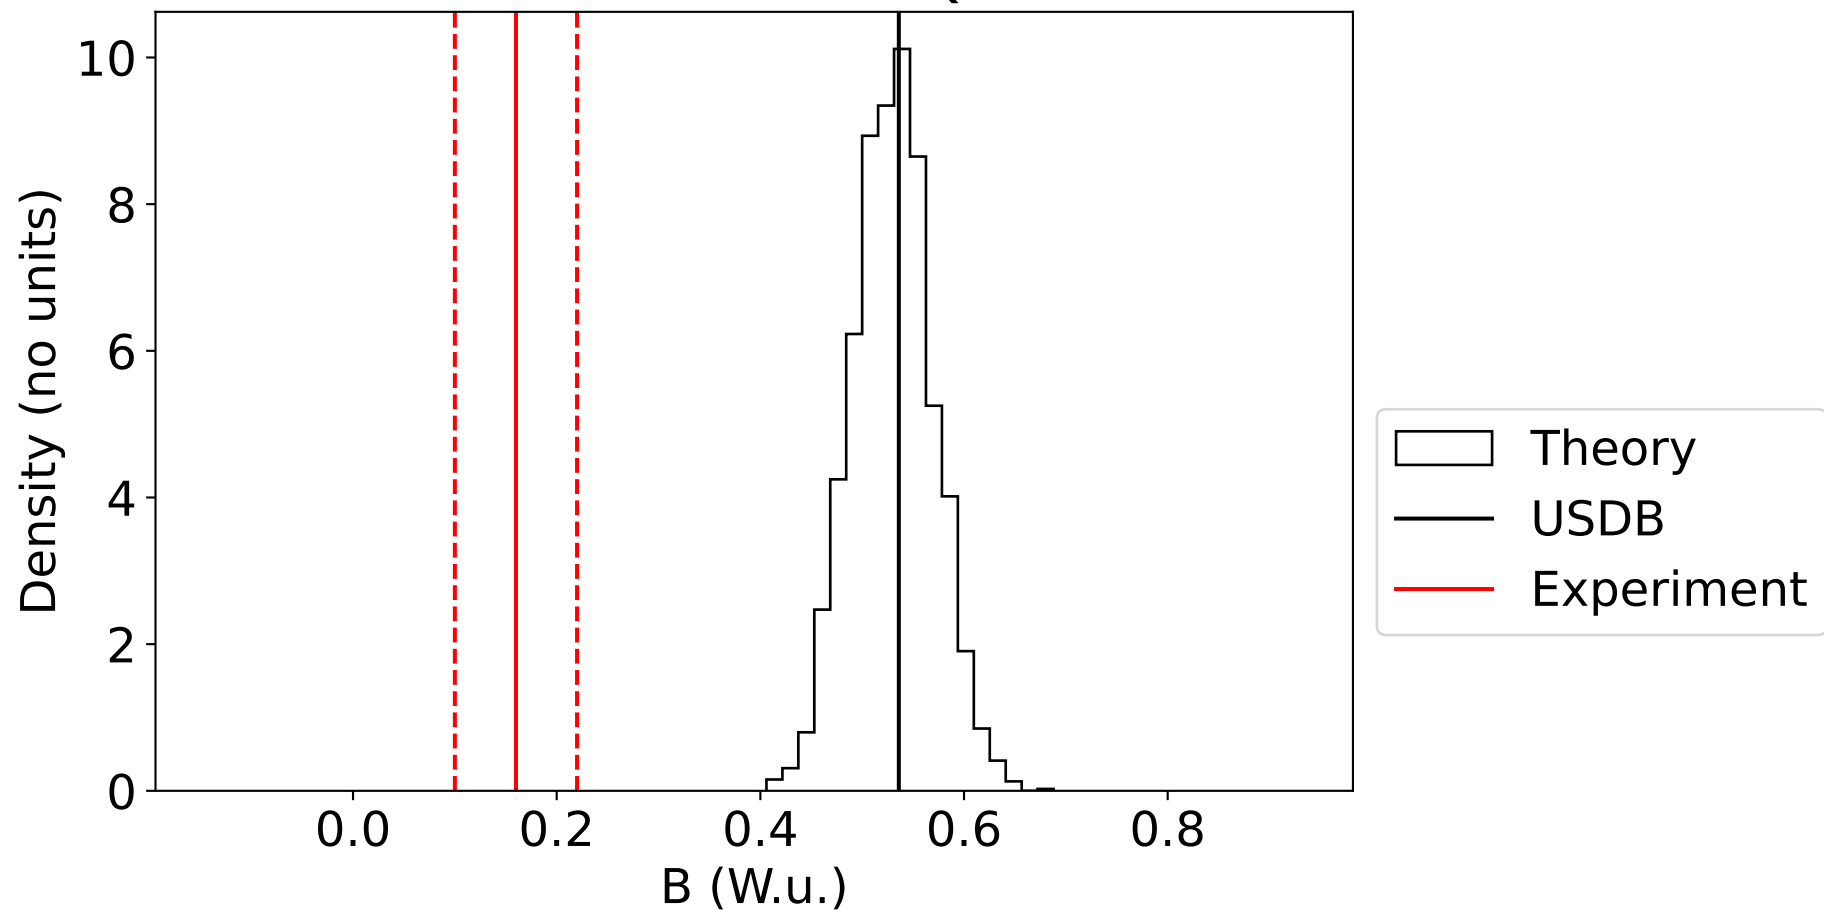

$^{26}\text{Al} (2_5) \rightarrow (3_2)$   
Included in UQ

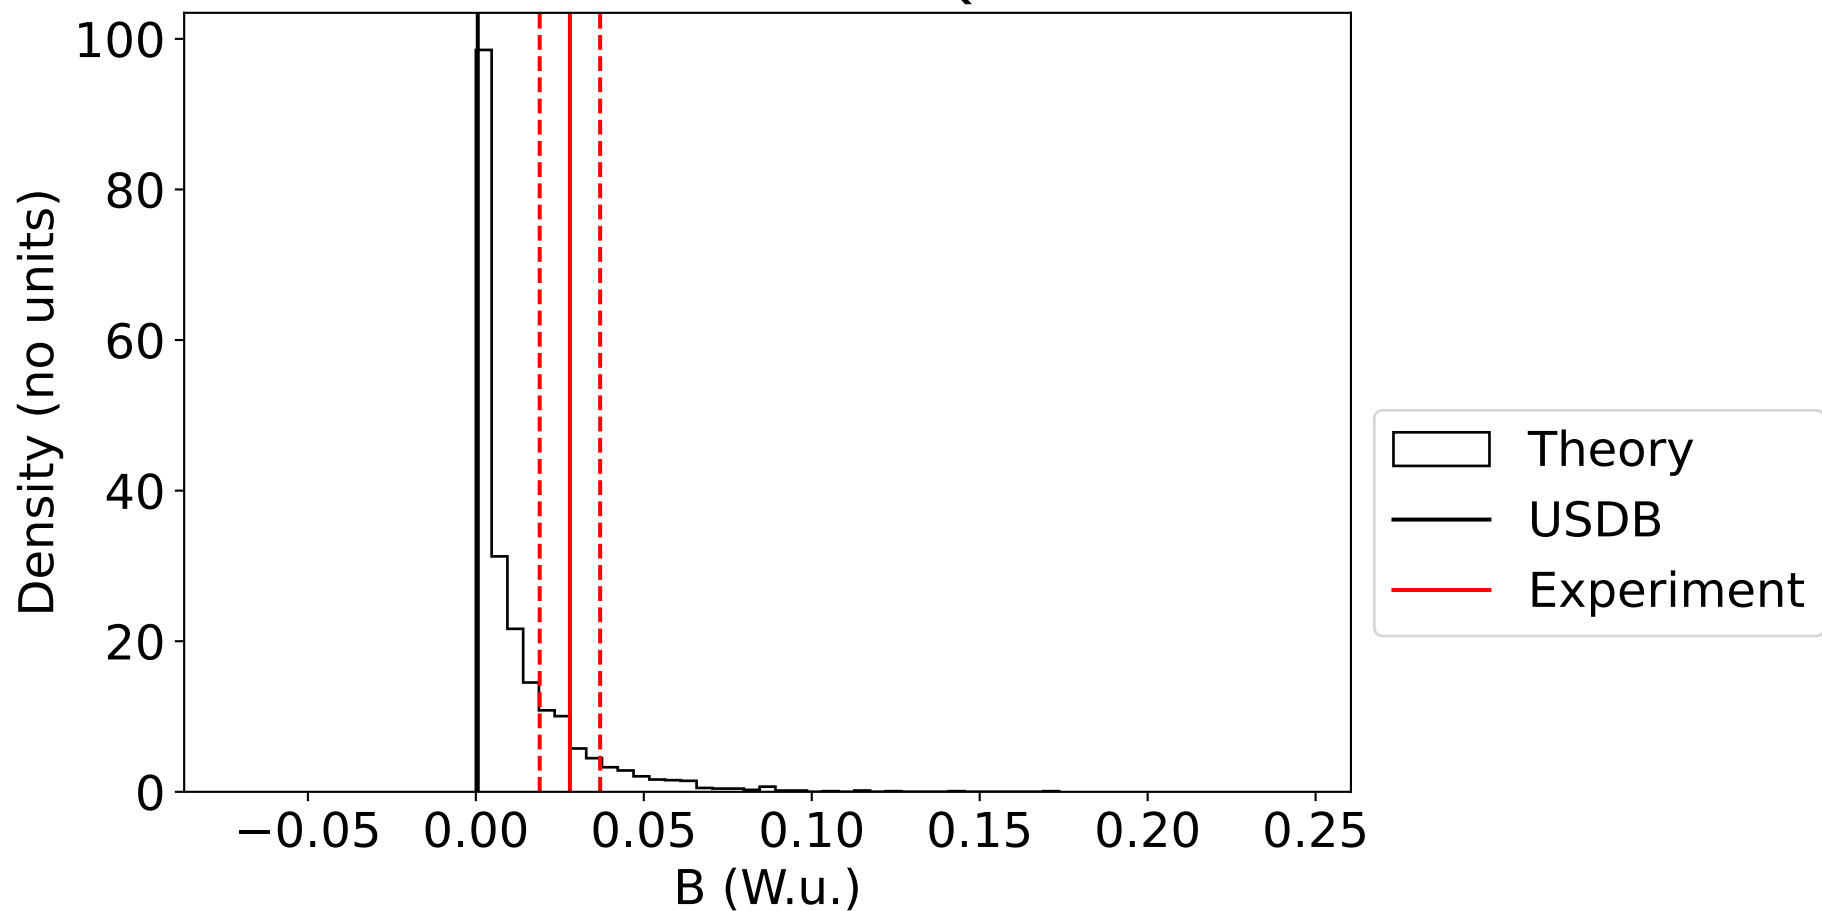

$^{26}\text{Al} (2_5) \rightarrow (1_1)$   
Included in UQ

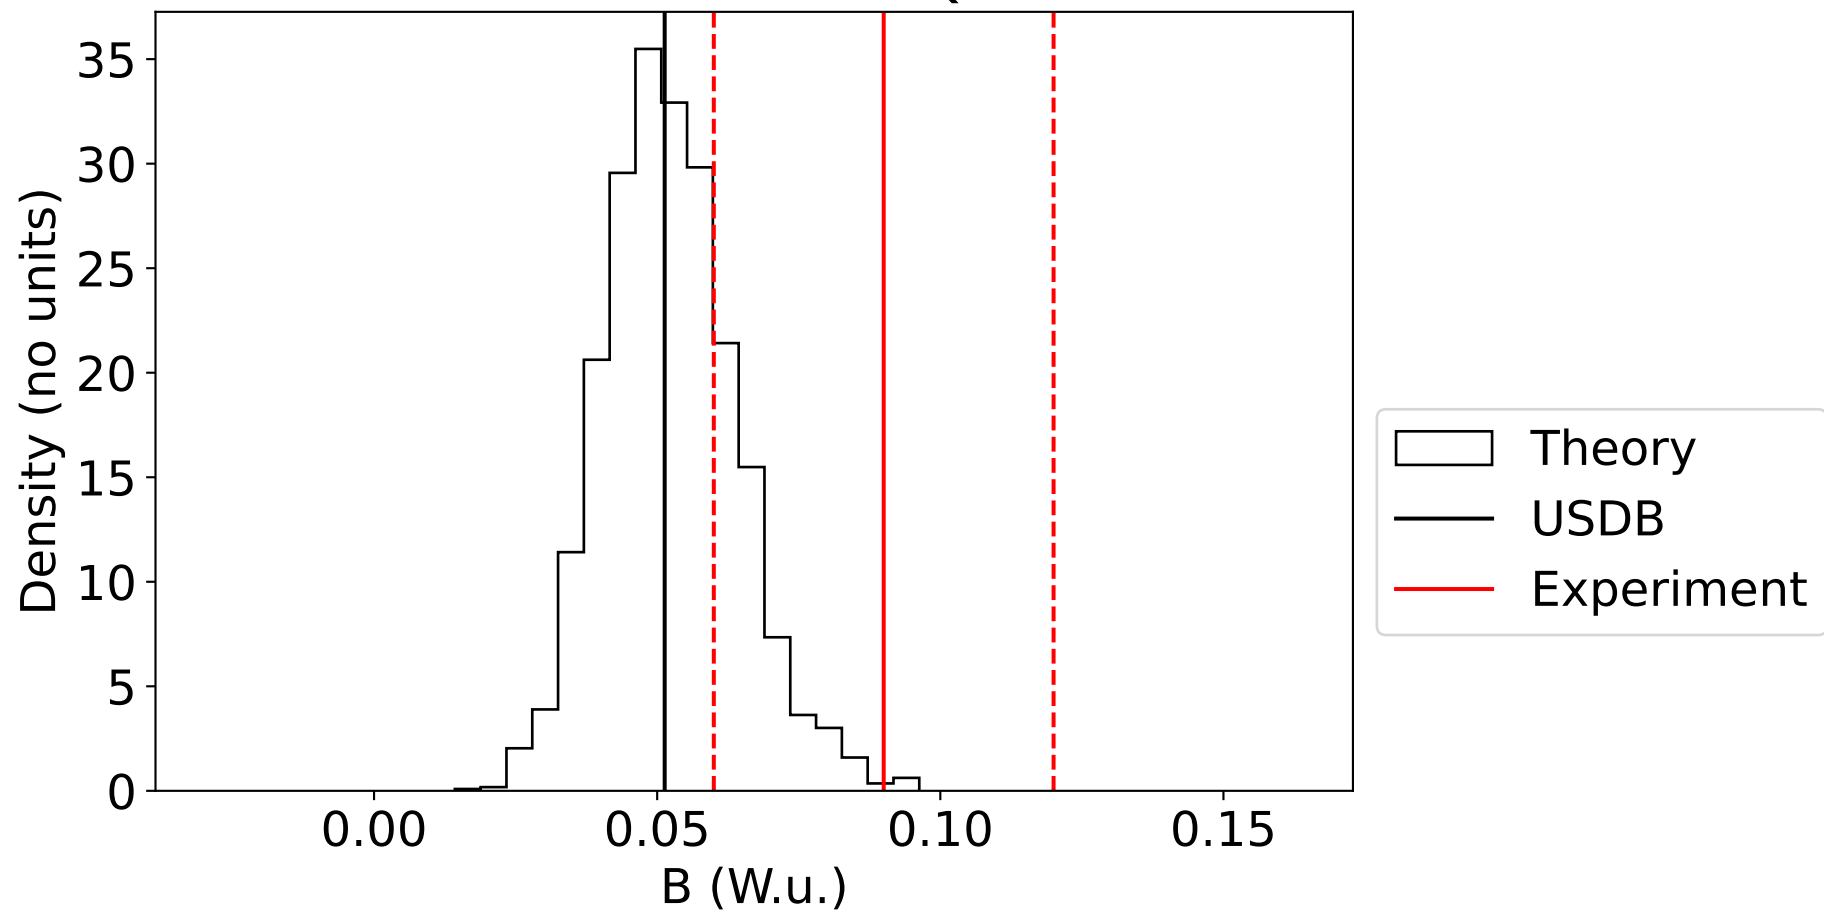

$^{26}\text{Al} (2_5) \rightarrow (3_3)$   
Included in UQ

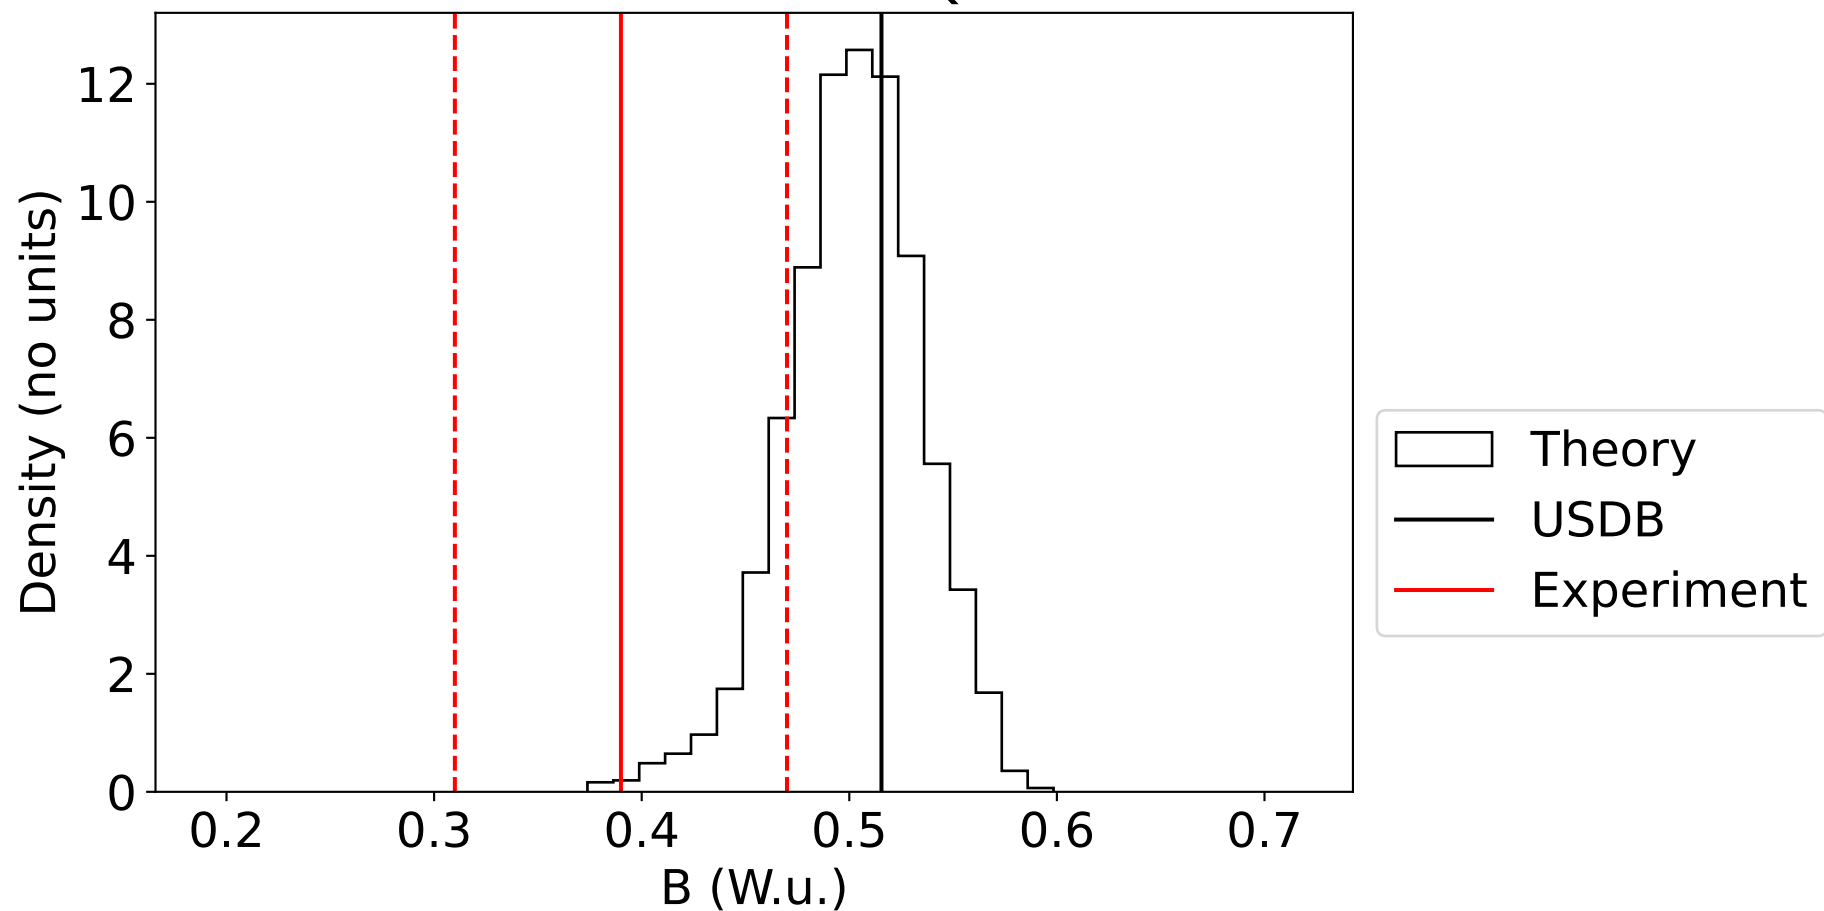

$^{26}\text{Al} (3_6) \rightarrow (2_5)$   
Included in UQ

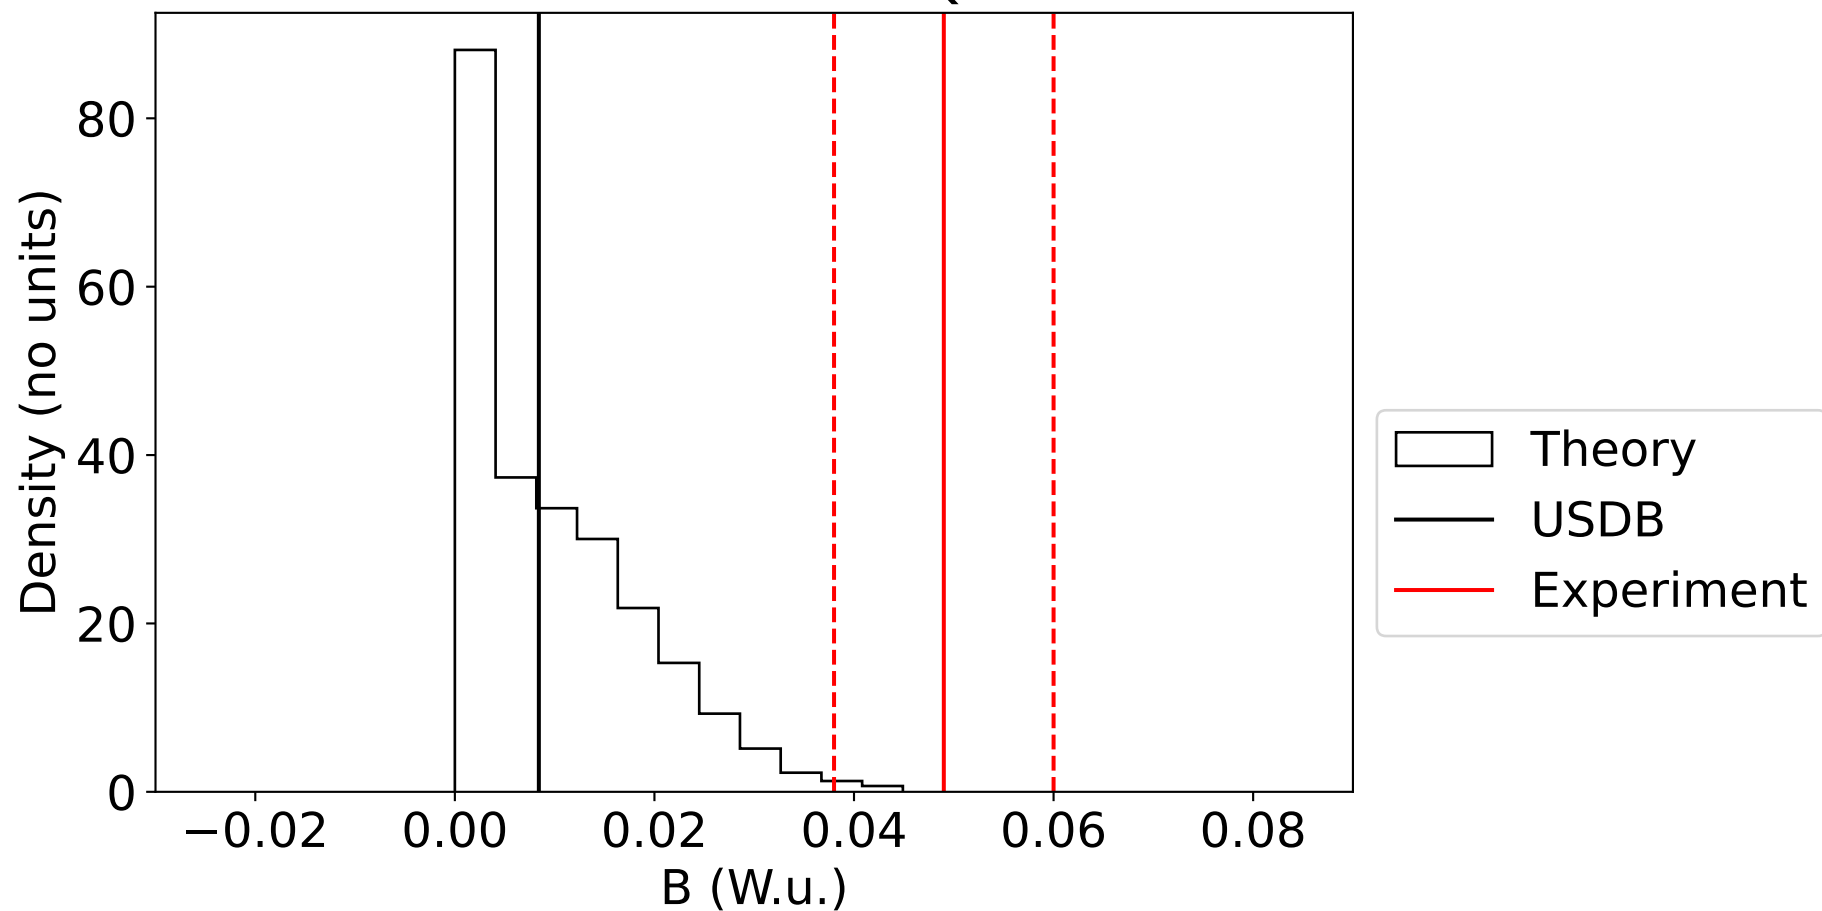

$^{26}\text{Al} (1_5) \rightarrow (0_1)$   
Included in UQ

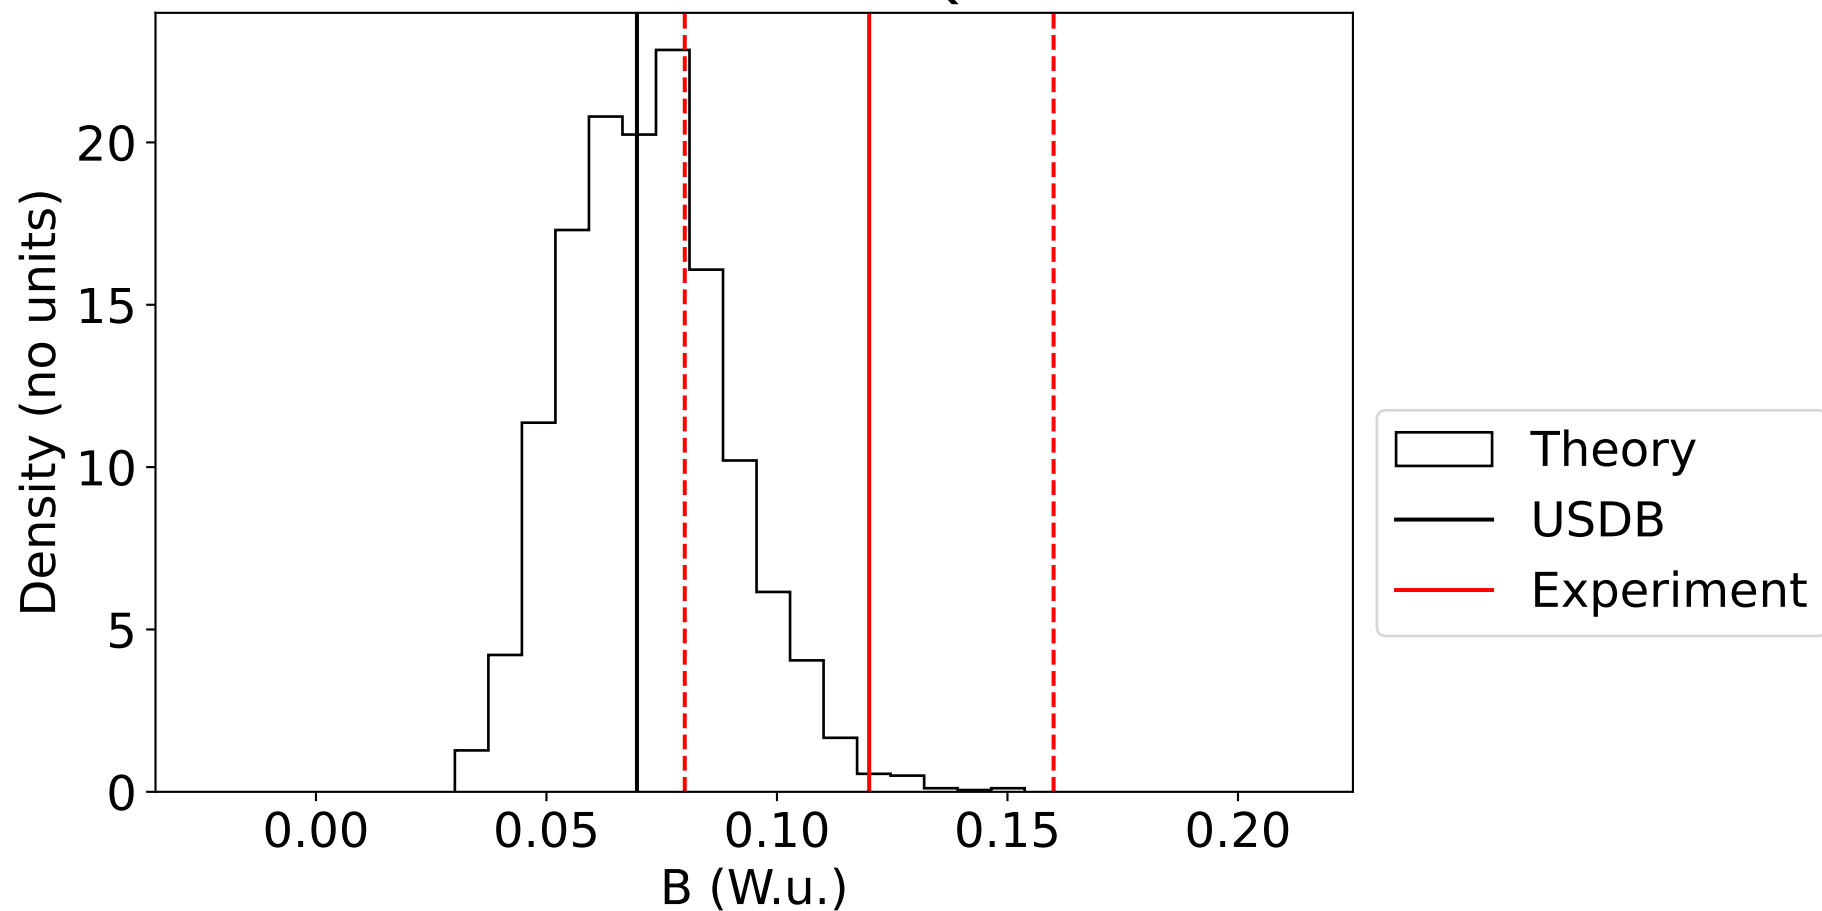



$^{26}\text{Al} (2_6) \rightarrow (2_5)$   
Included in UQ

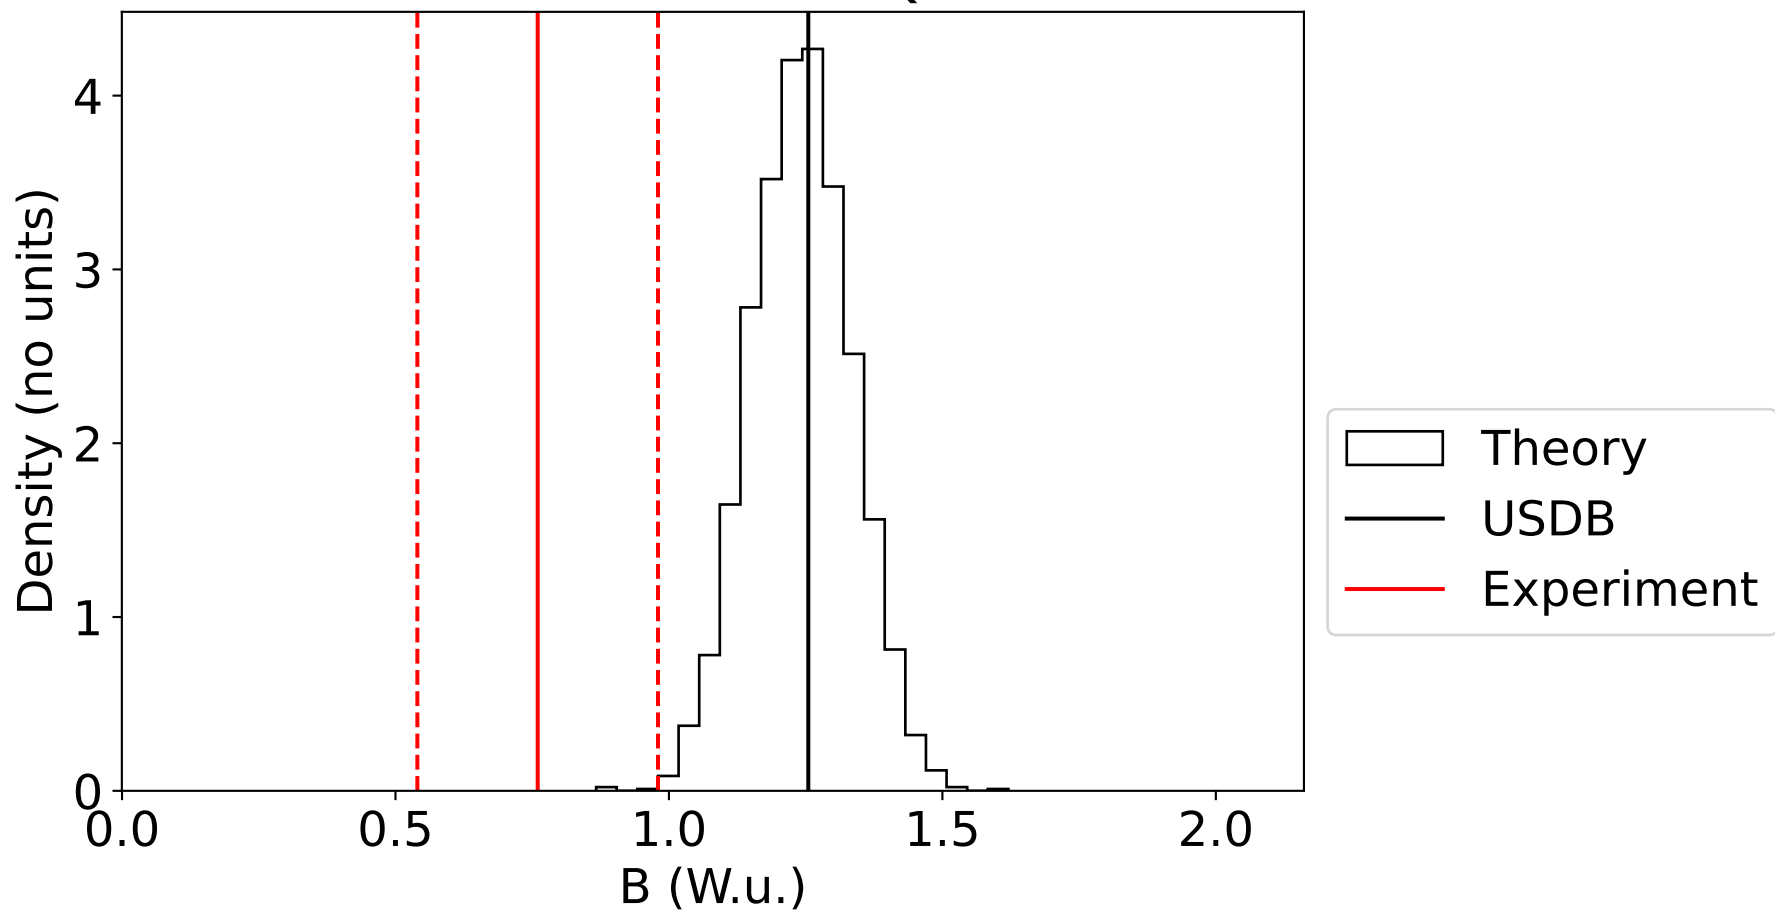

$^{26}\text{Al} (0_2) \rightarrow (1_1)$   
Included in UQ

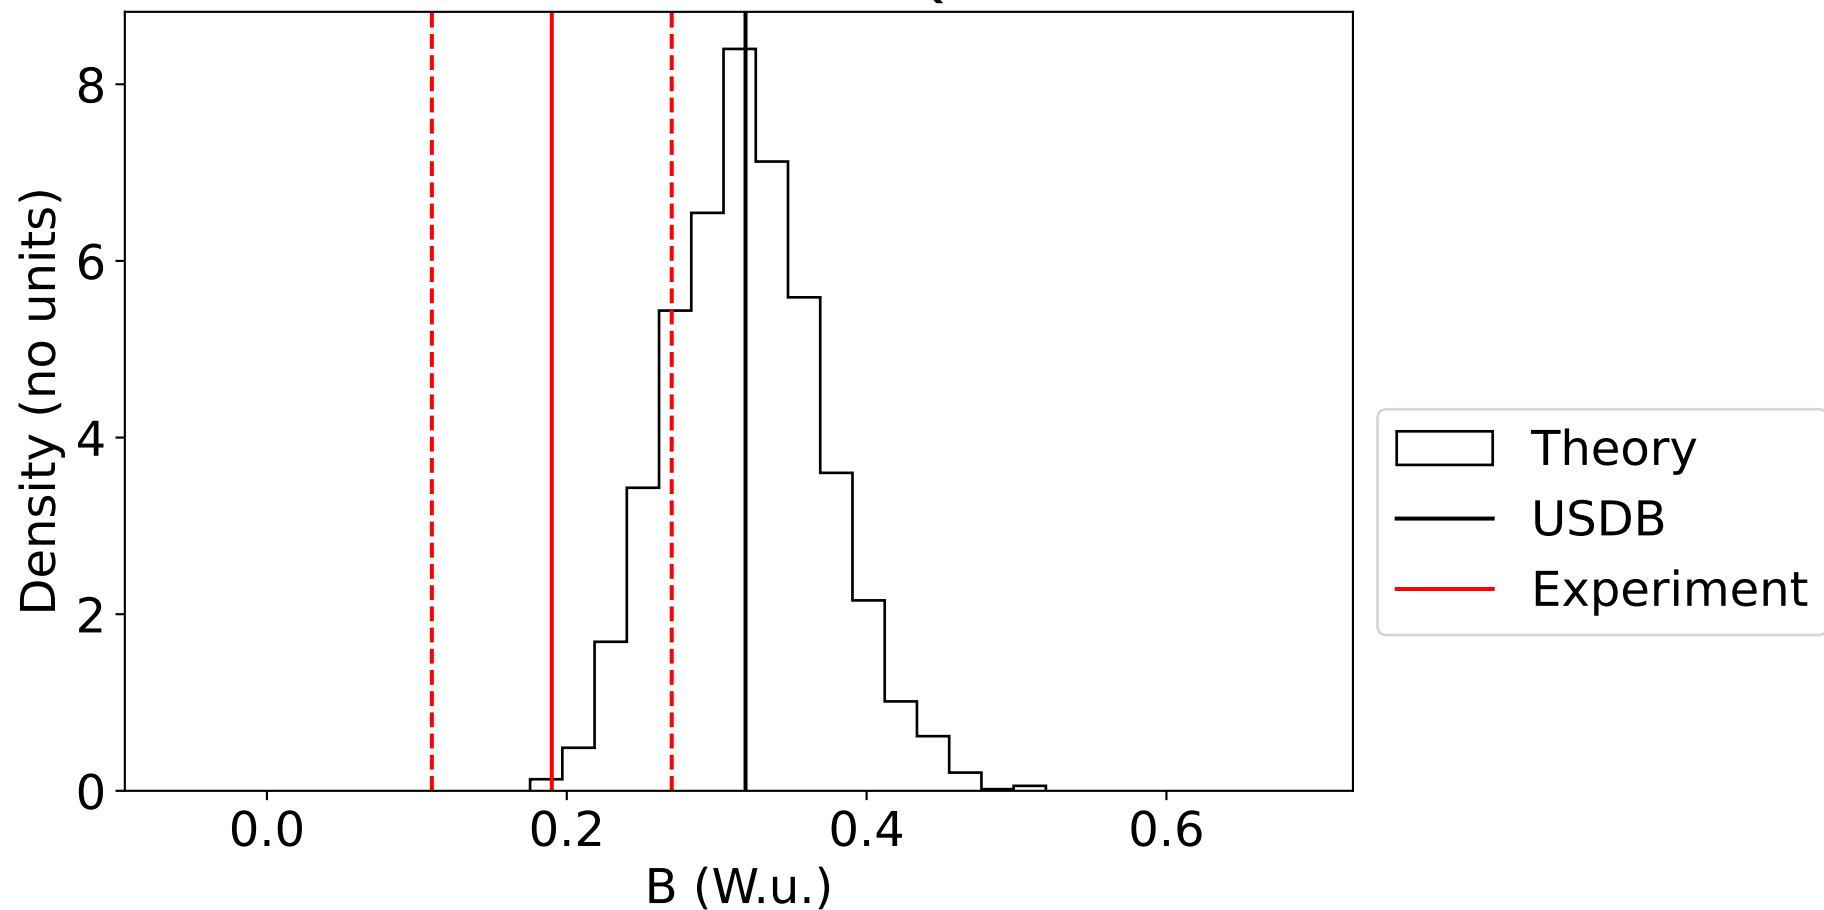

$^{26}\text{Al} (0_2) \rightarrow (1_2)$   
Included in UQ

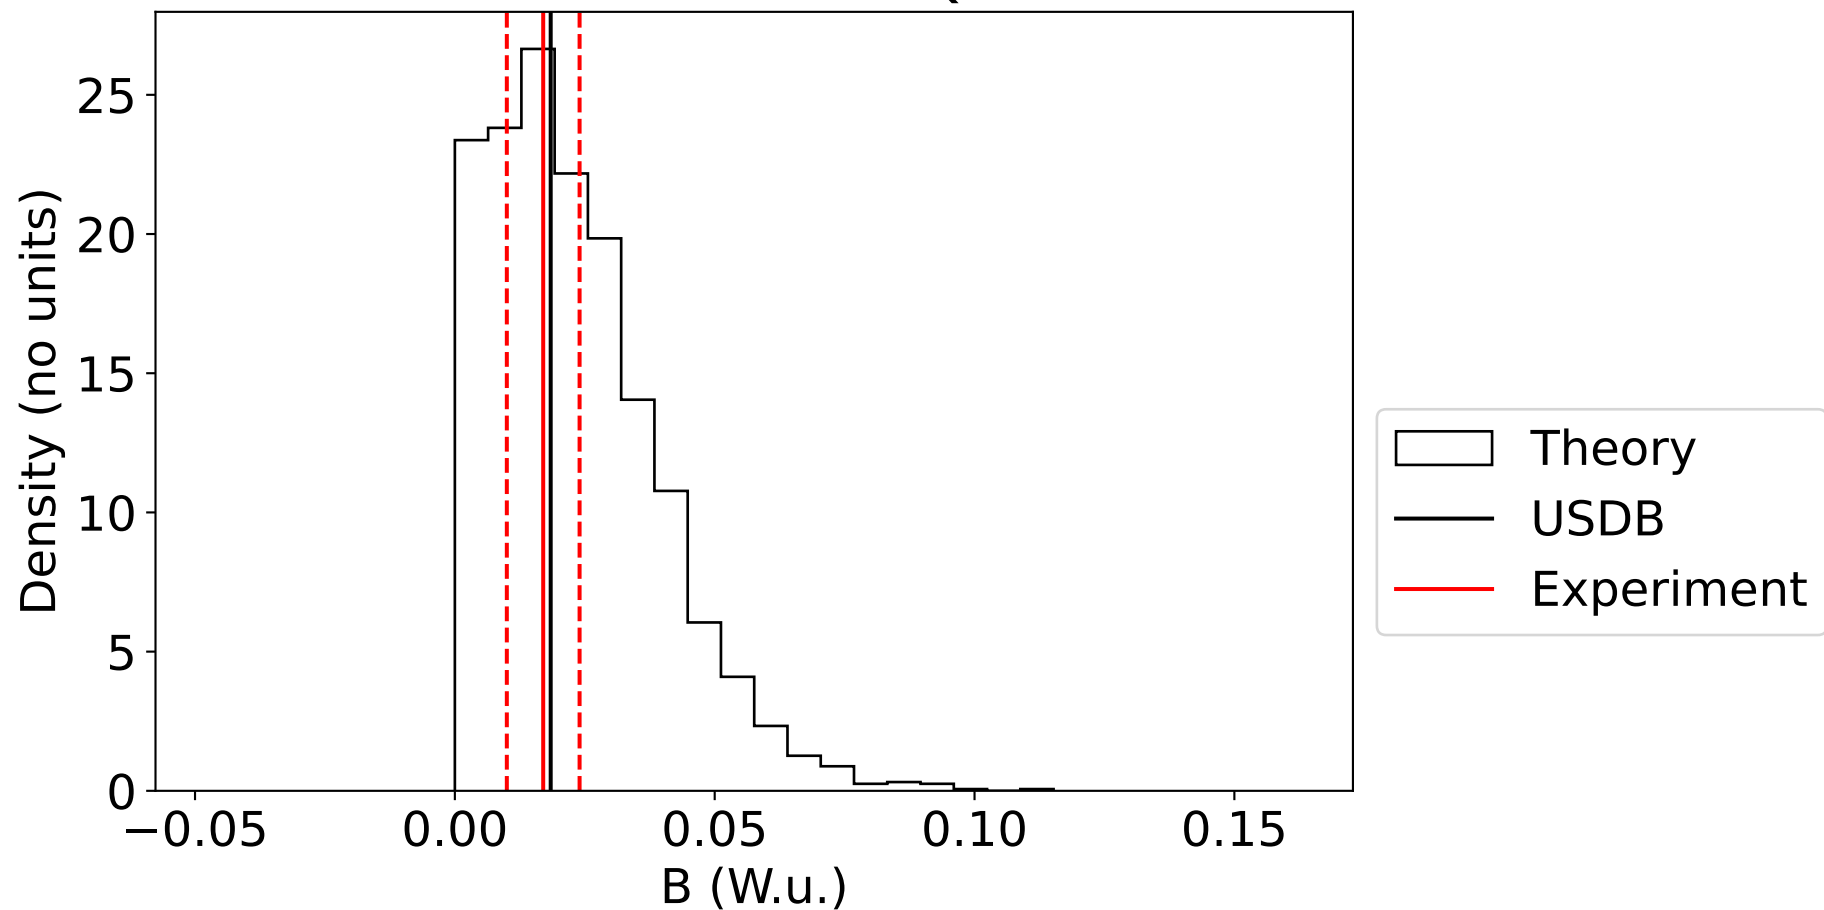

$^{26}\text{Al} (0_2) \rightarrow (1_3)$   
Included in UQ

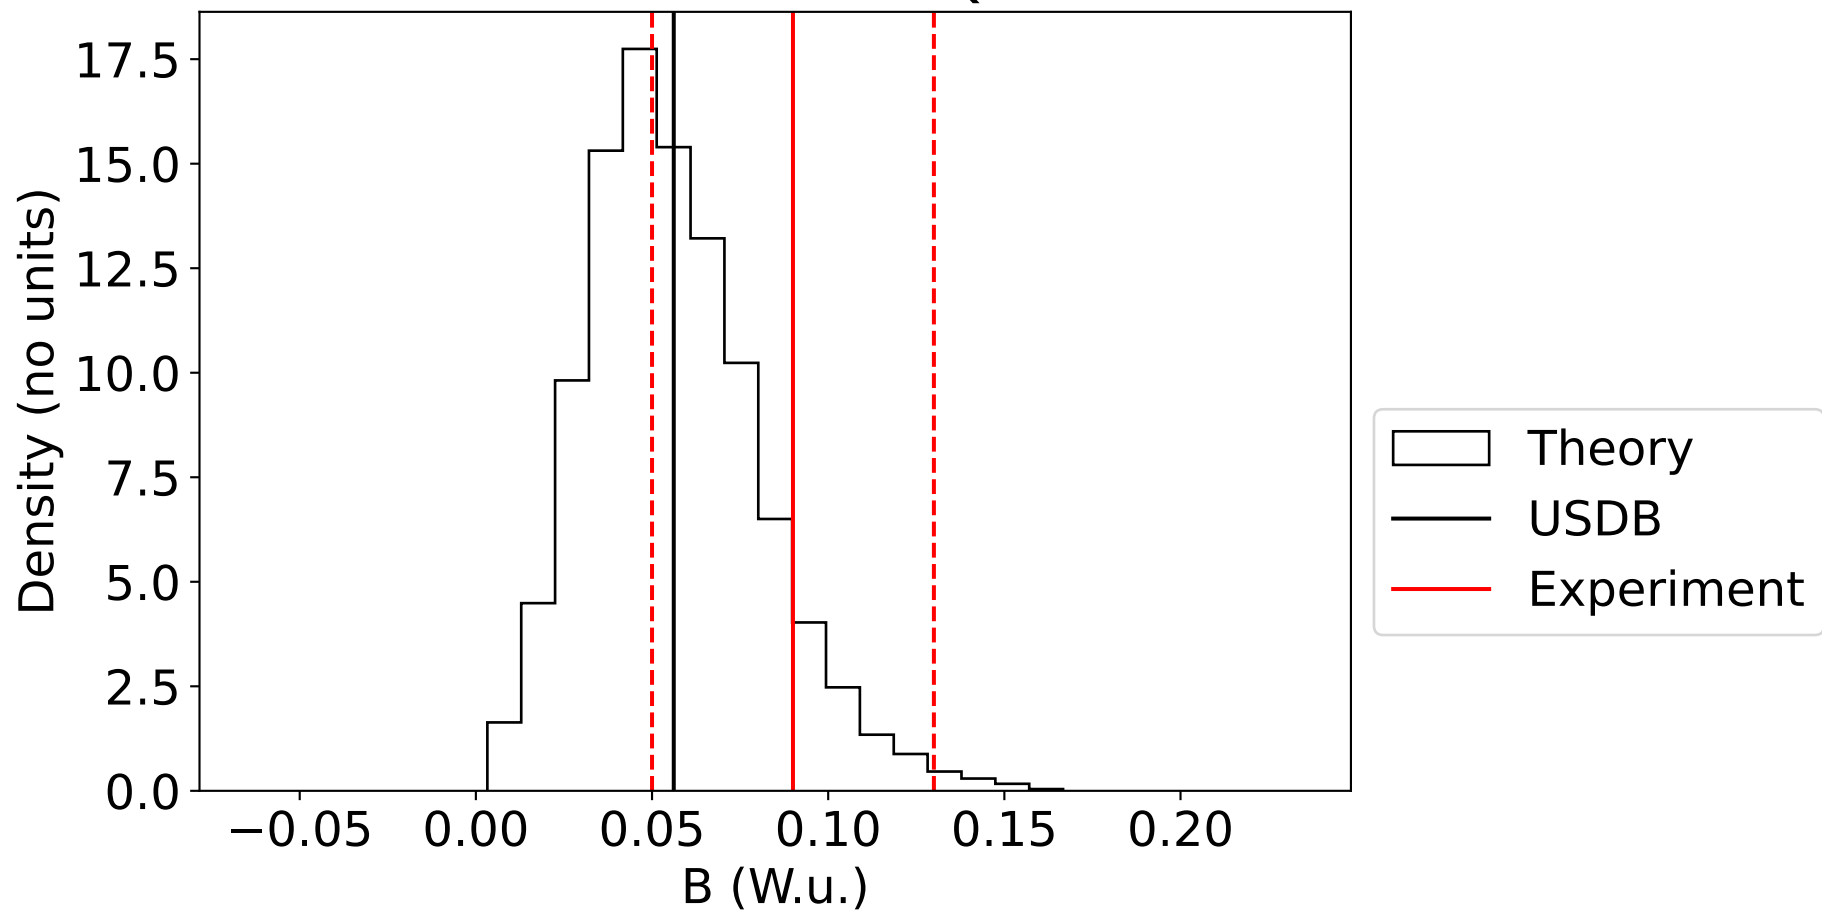

$^{26}\text{Al} (0_2) \rightarrow (1_4)$   
Included in UQ

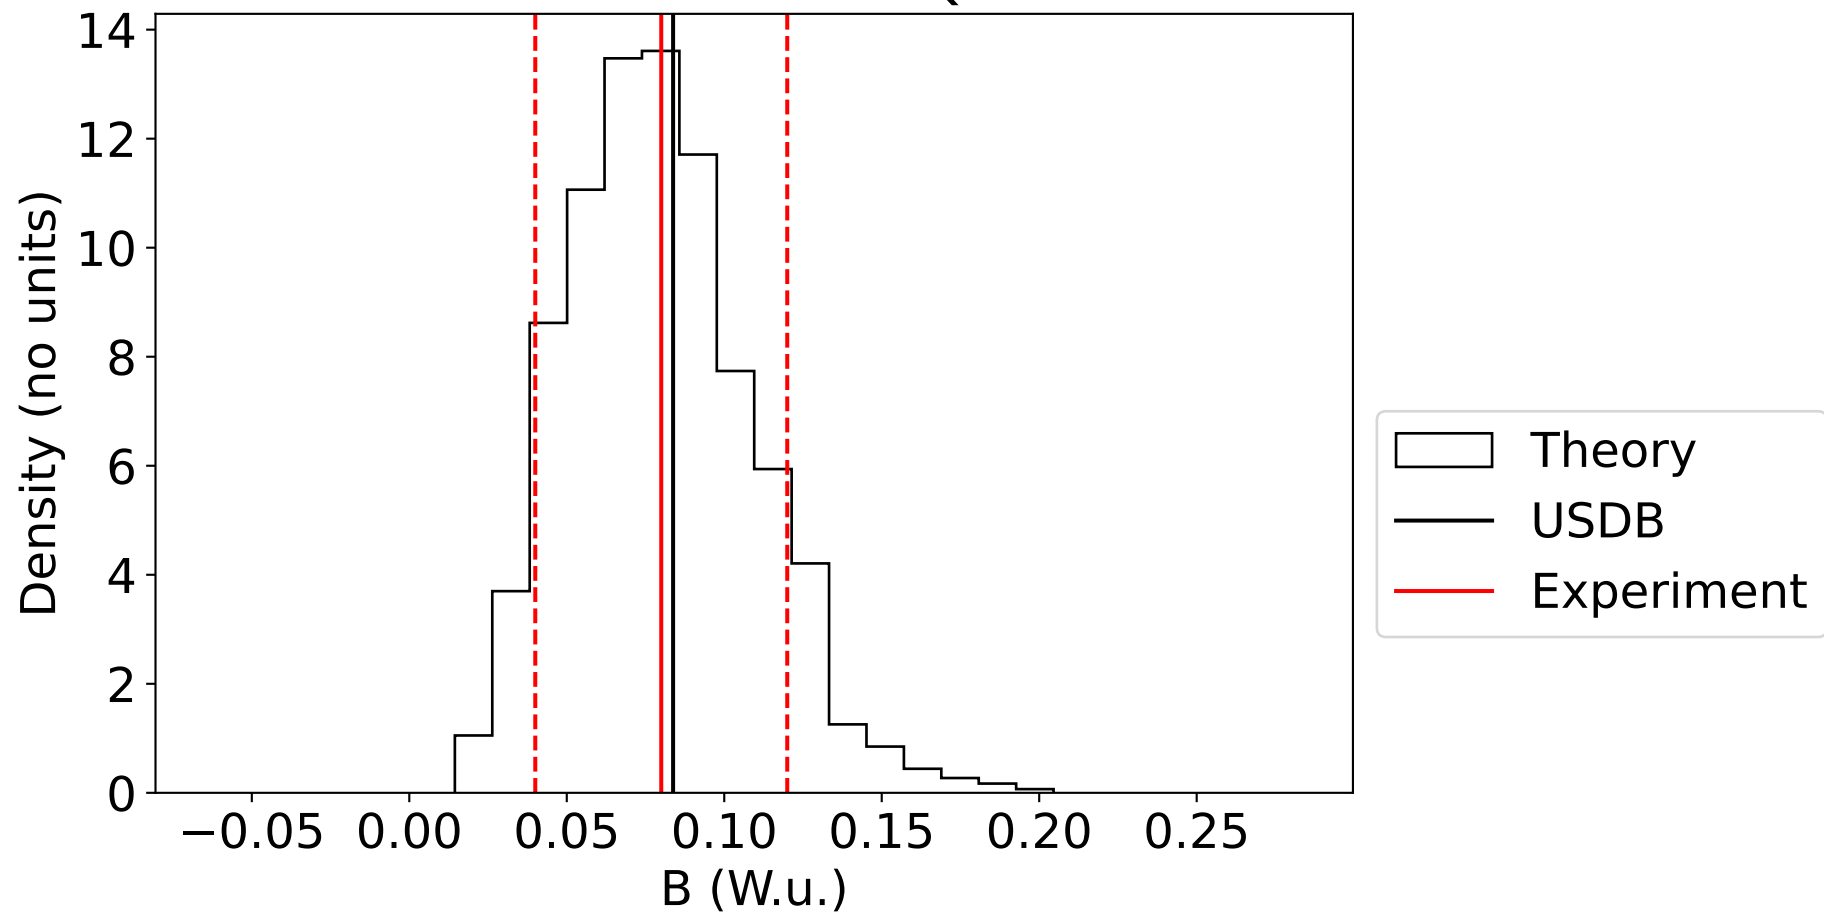

$^{27}\text{Al} (3/2_1) \rightarrow (5/2_1)$   
Included in UQ

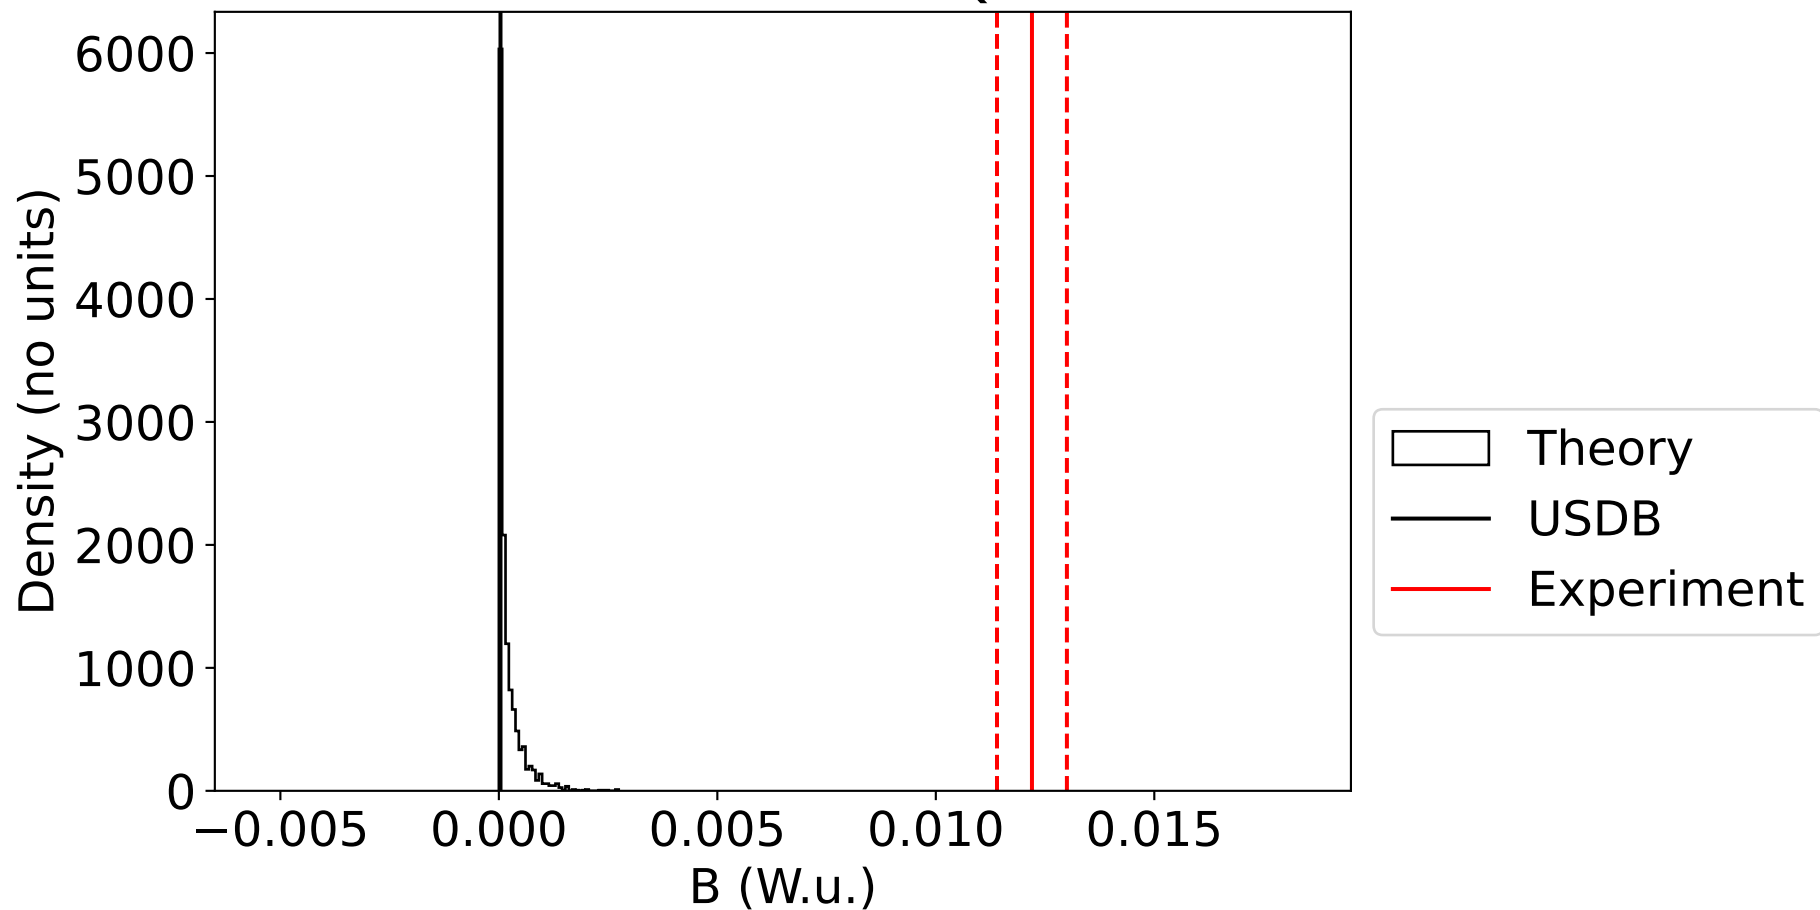

$^{27}\text{Al} (7/2_1) \rightarrow (5/2_1)$   
Included in UQ

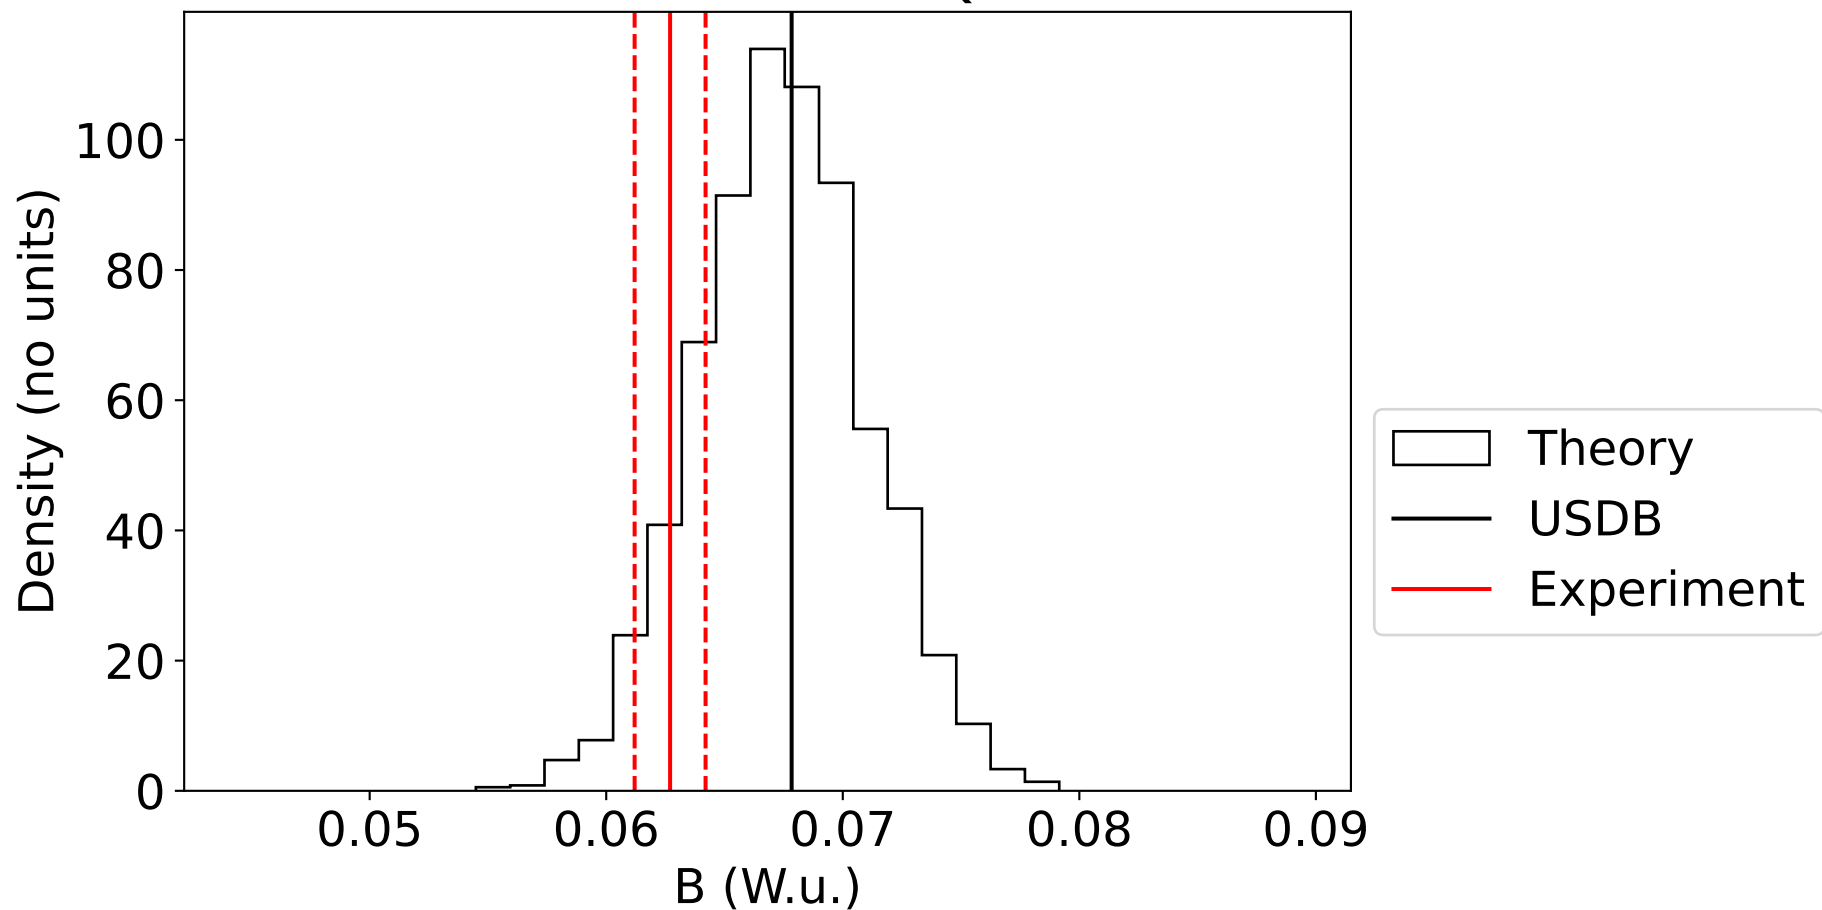

$^{27}\text{Al} (5/2_2) \rightarrow (3/2_1)$   
Included in UQ

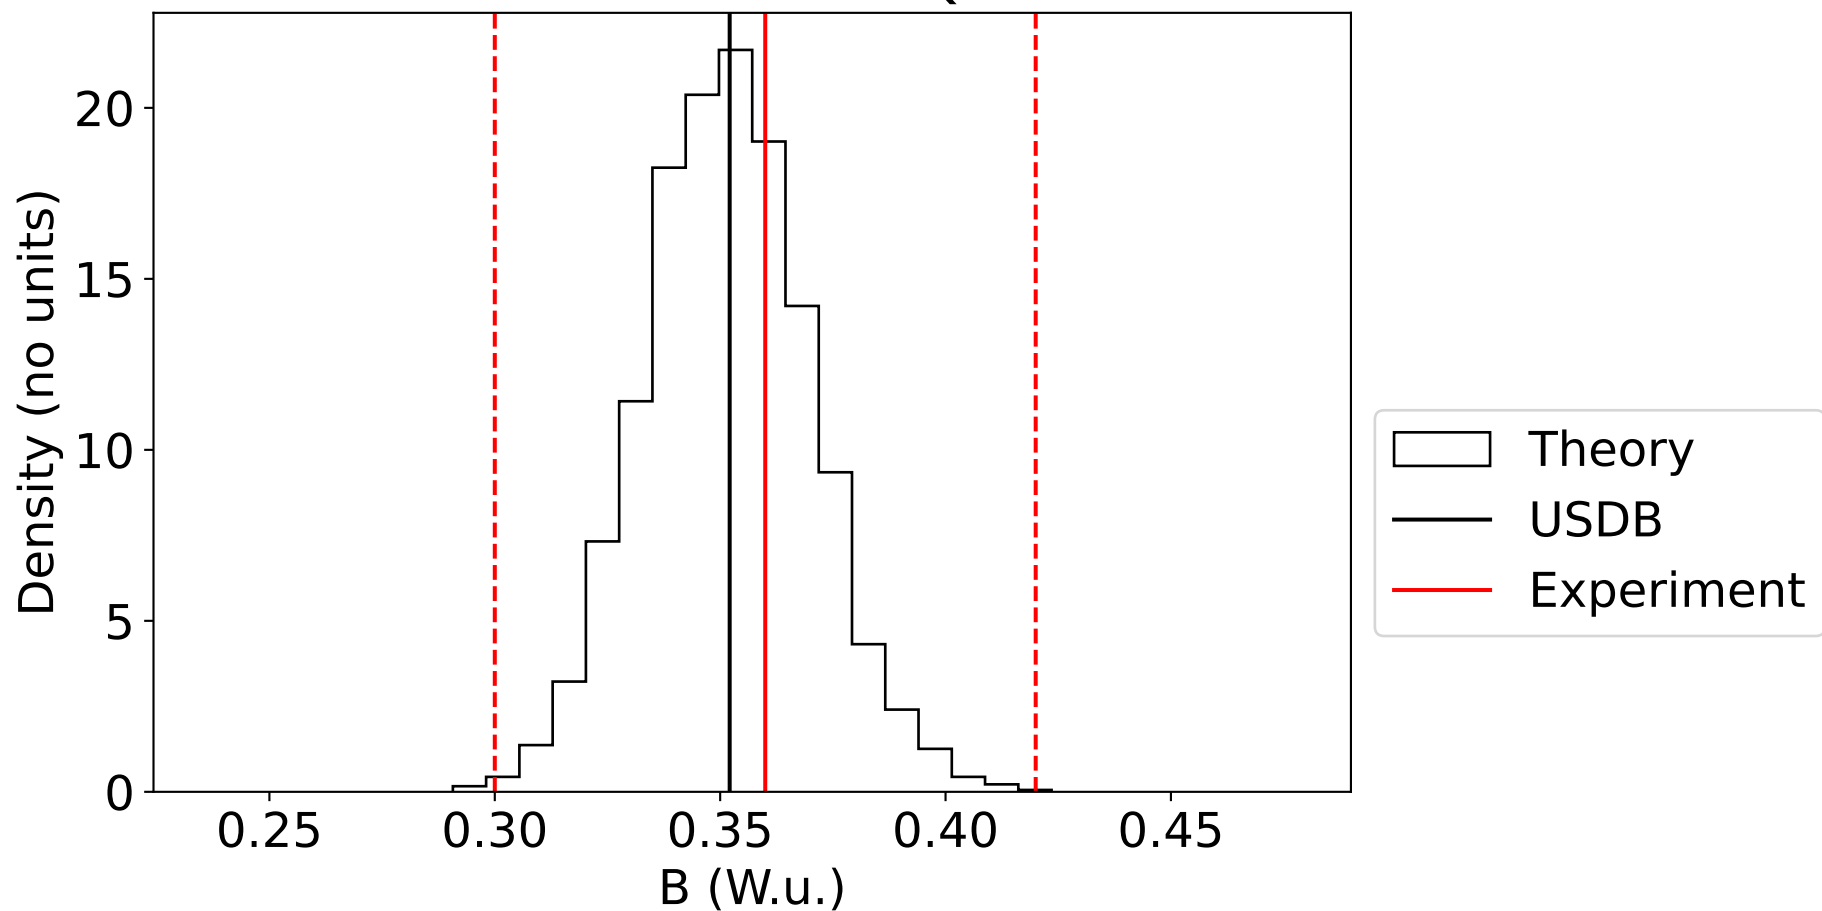



$^{27}\text{Al} (5/2_3) \rightarrow (5/2_1)$   
Included in UQ

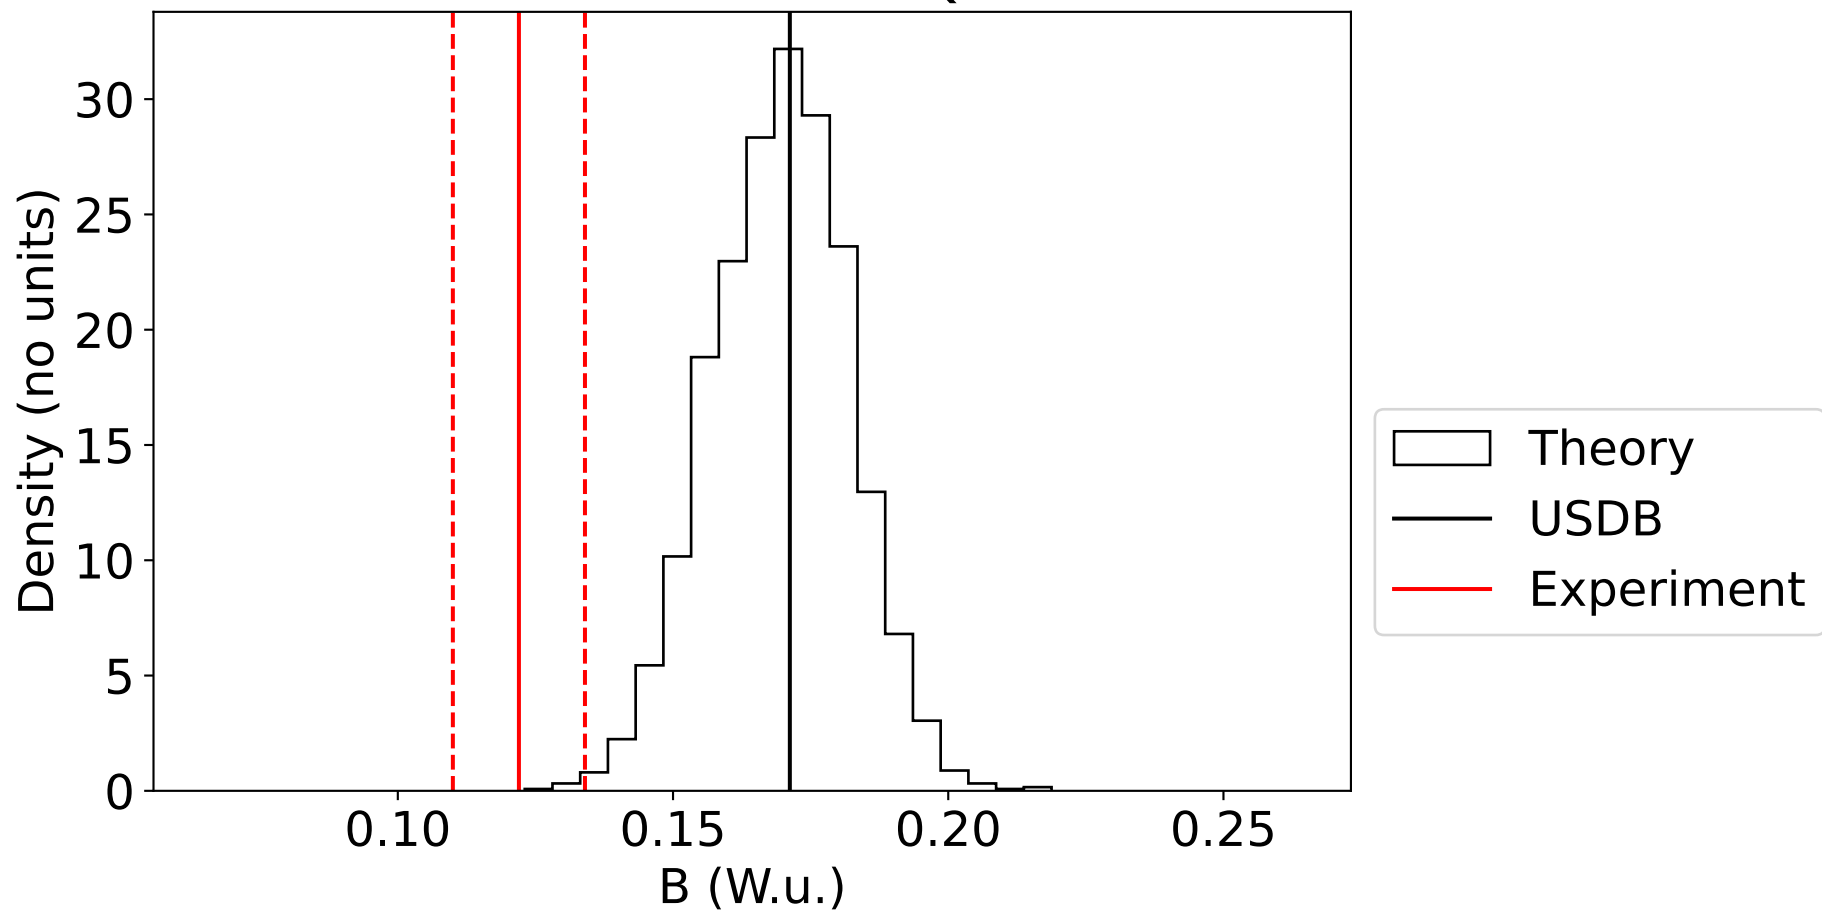

$^{27}\text{Al} (7/2_2) \rightarrow (5/2_1)$   
Included in UQ

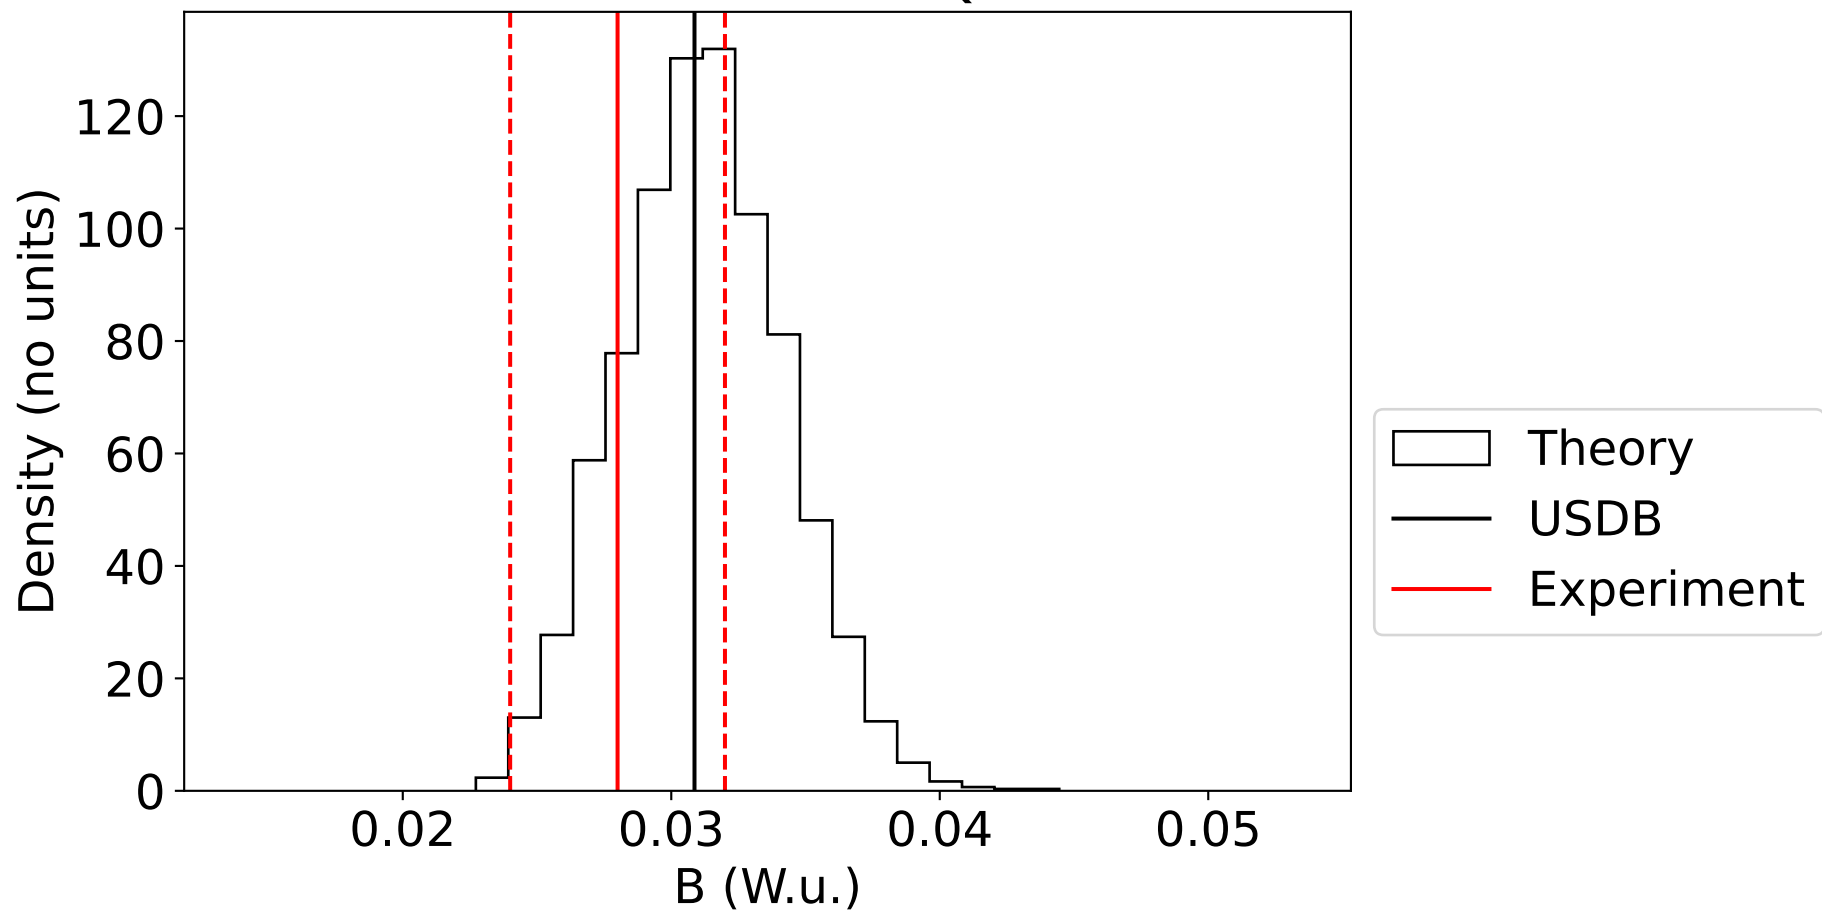

$^{27}\text{Al} (7/2_2) \rightarrow (7/2_1)$   
Included in UQ

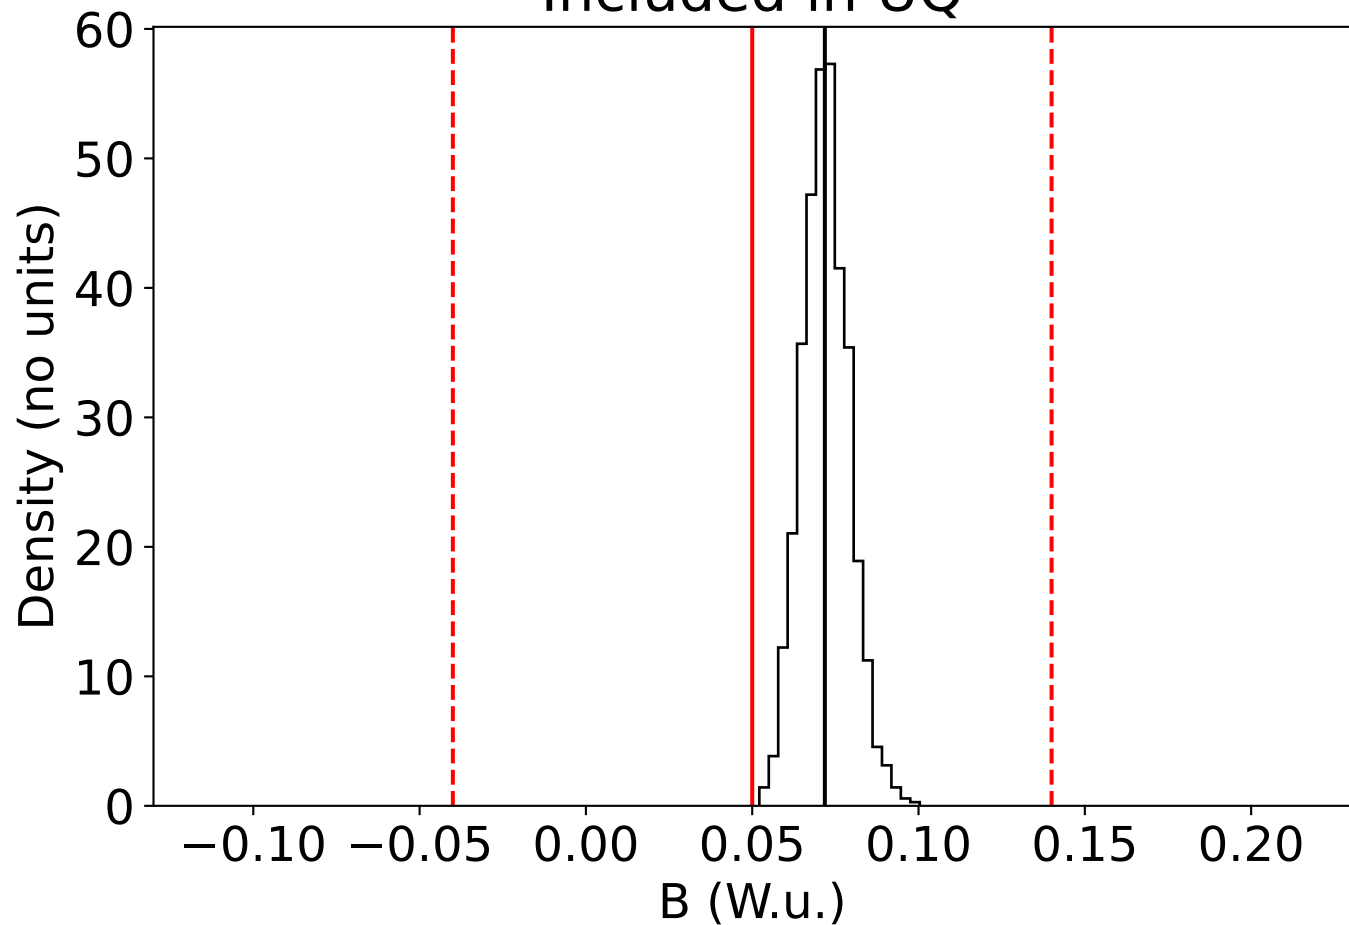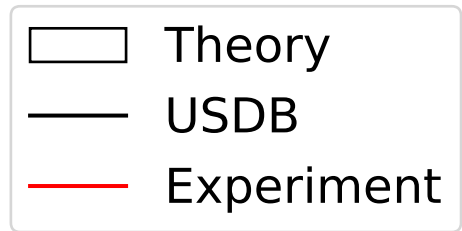

$^{27}\text{Al} (7/2_2) \rightarrow (5/2_2)$   
Included in UQ

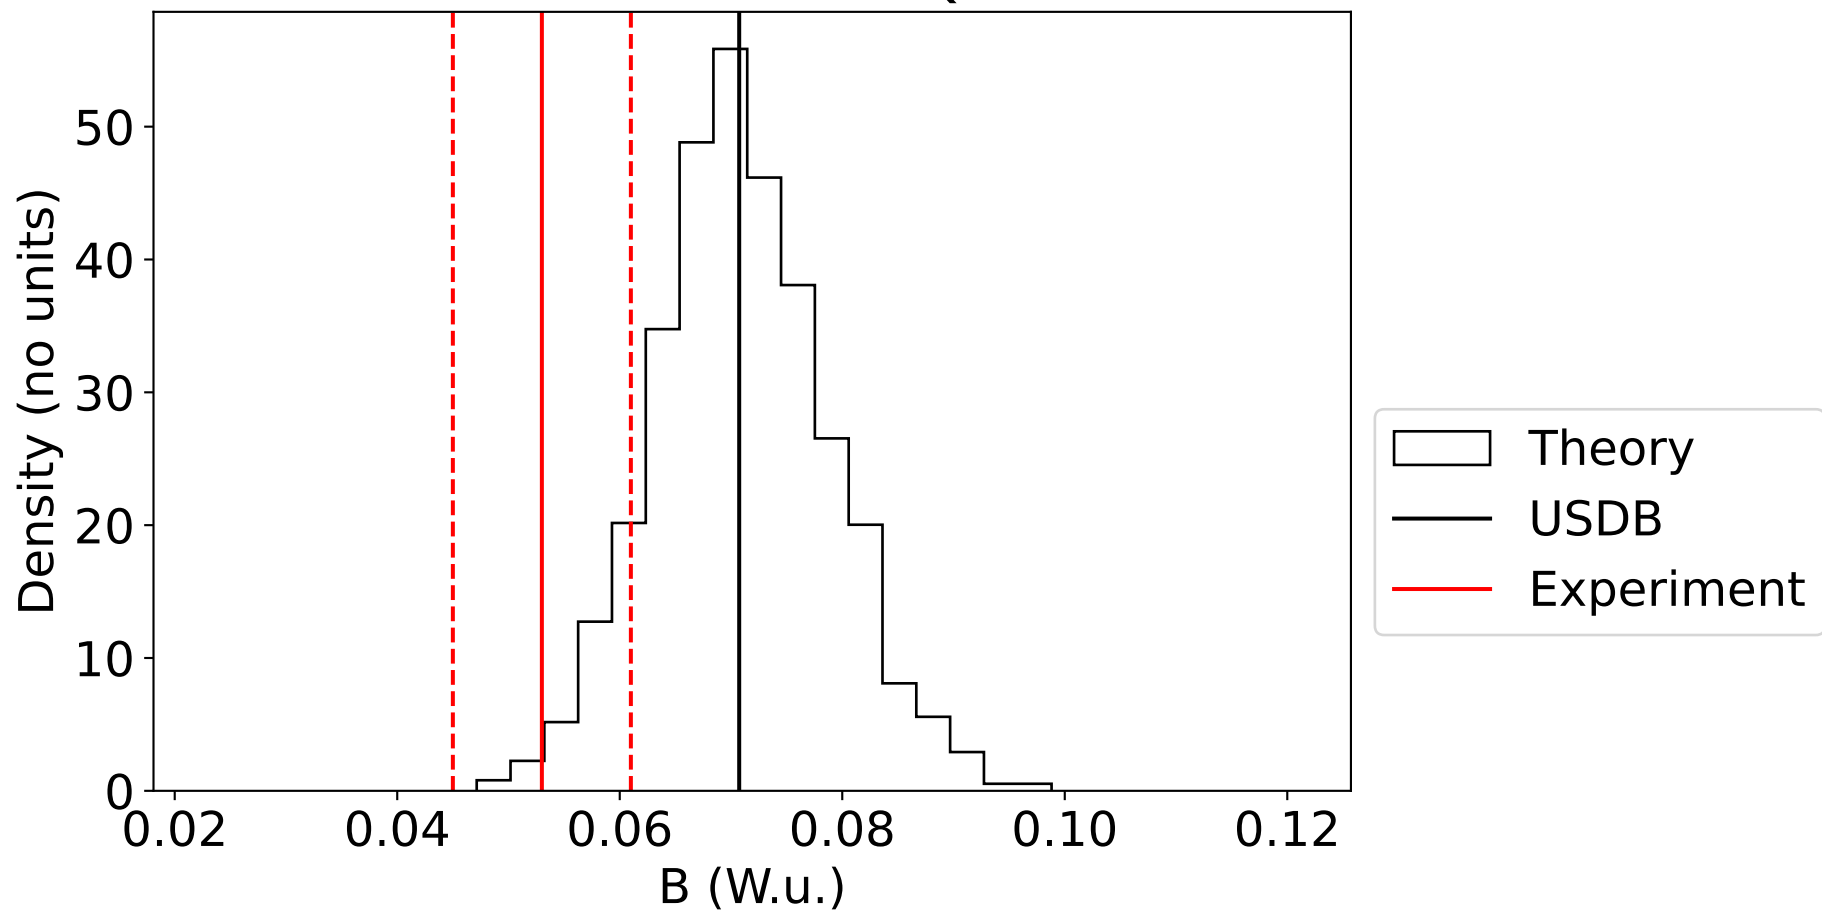

$^{27}\text{Al} (5/2_4) \rightarrow (5/2_1)$   
Included in UQ

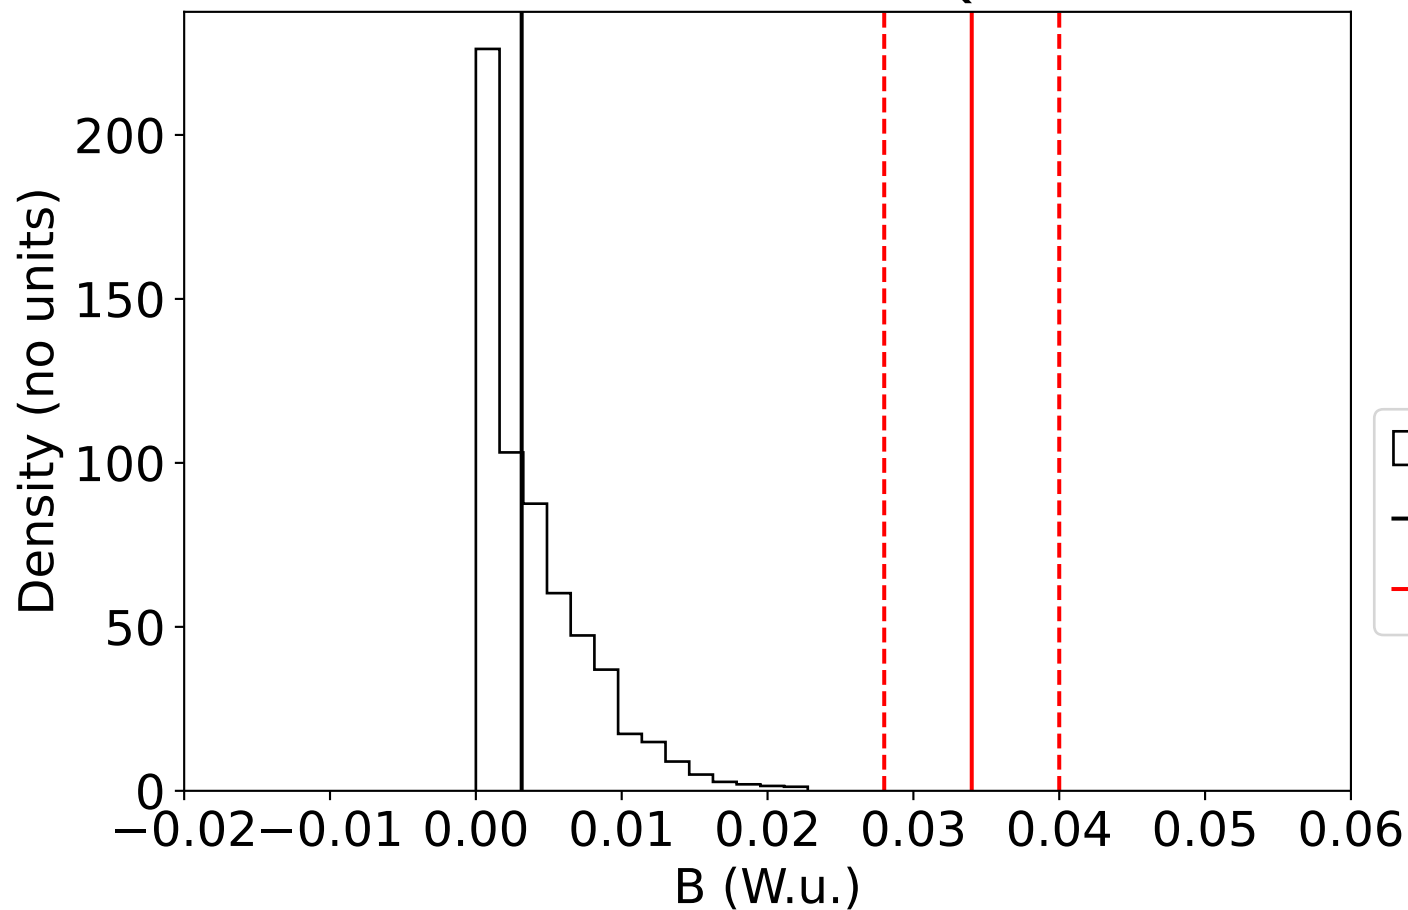

$^{27}\text{Al} (5/2_4) \rightarrow (3/2_1)$   
Included in UQ

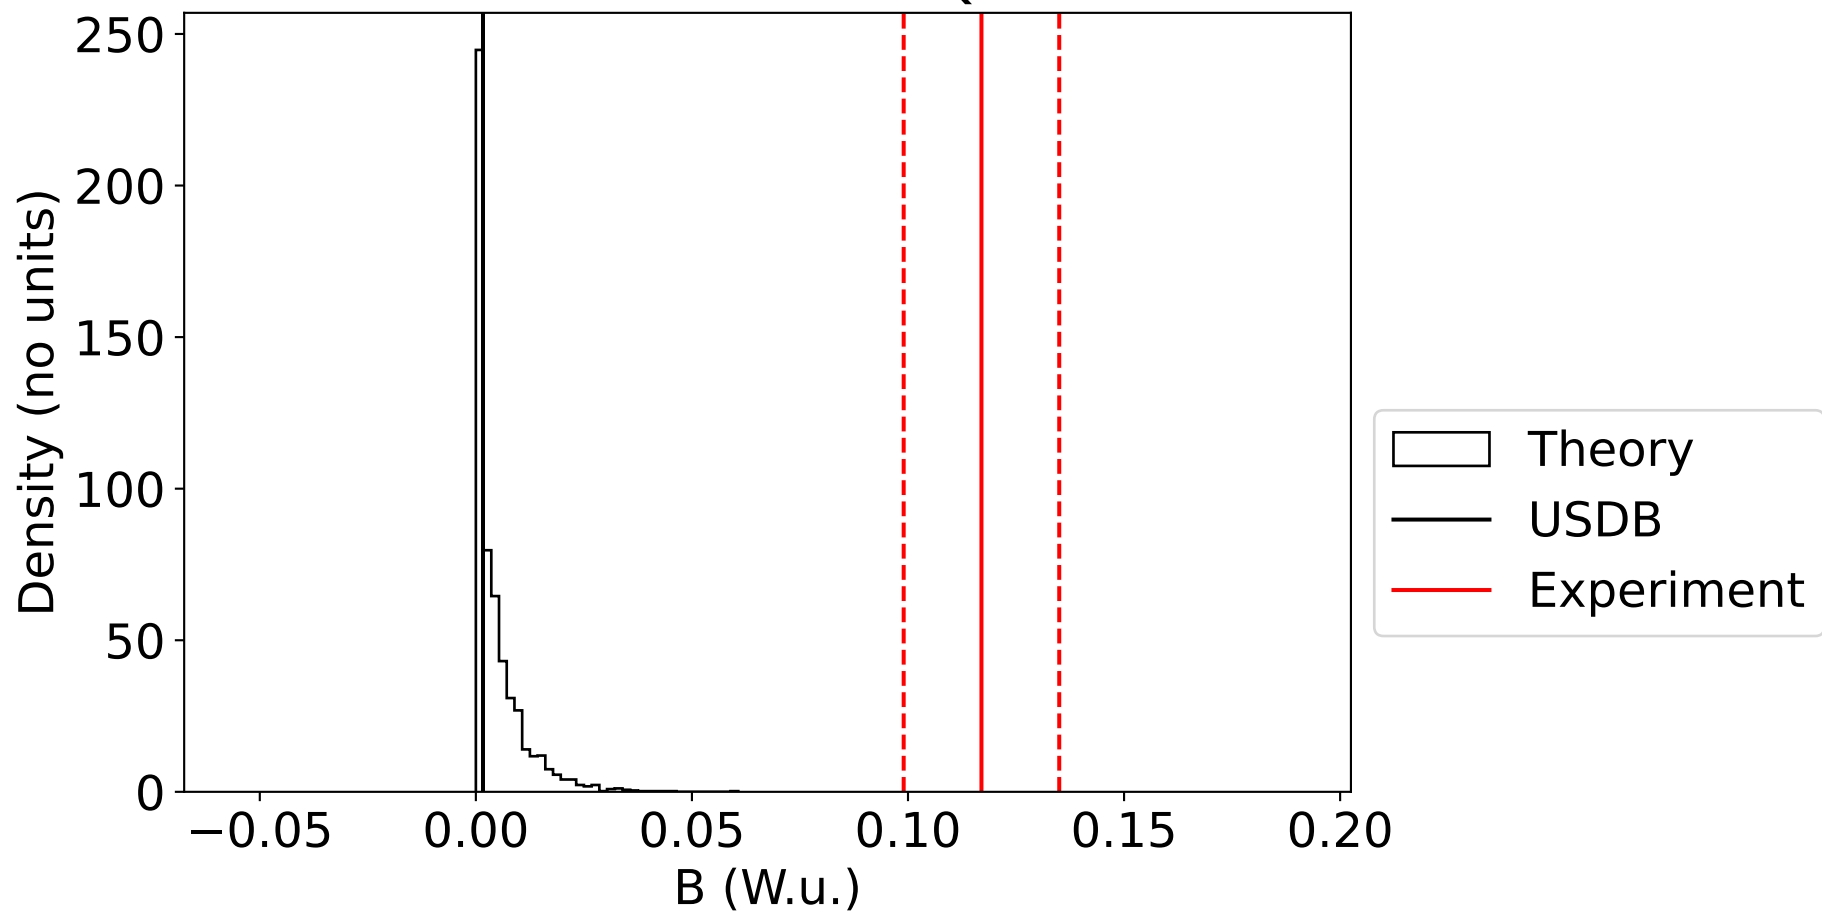

$^{27}\text{Al} (5/2_4) \rightarrow (7/2_1)$   
Included in UQ

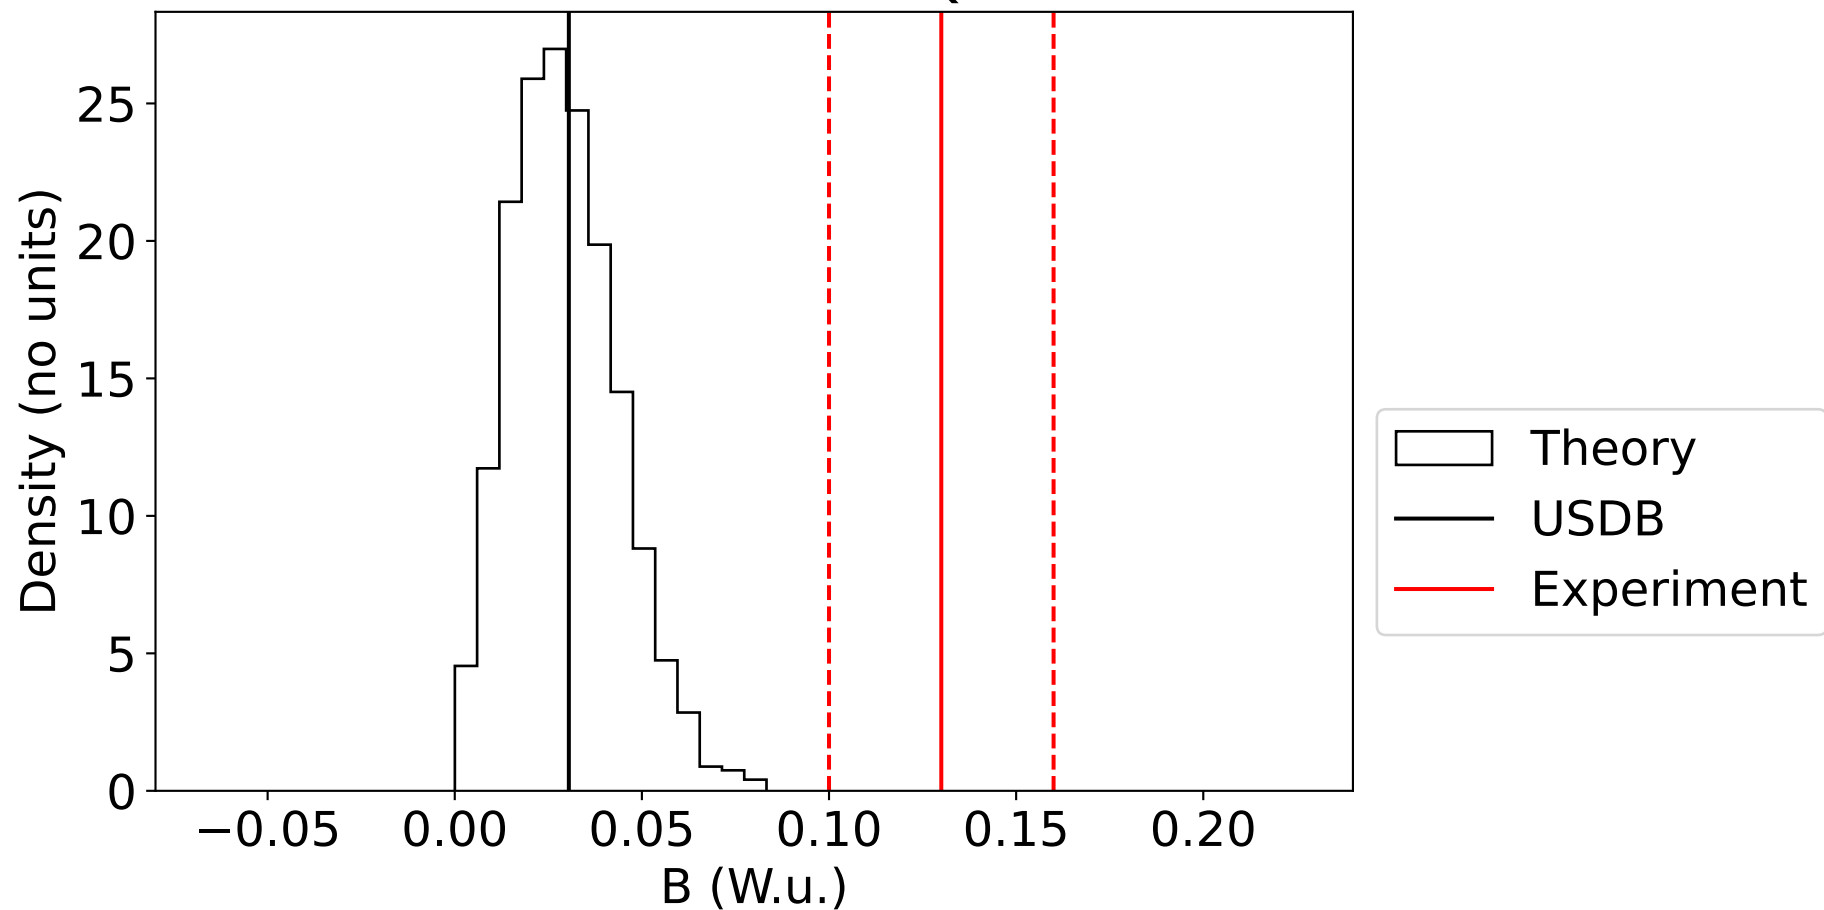

$^{27}\text{Al} (5/2_4) \rightarrow (3/2_2)$   
Included in UQ

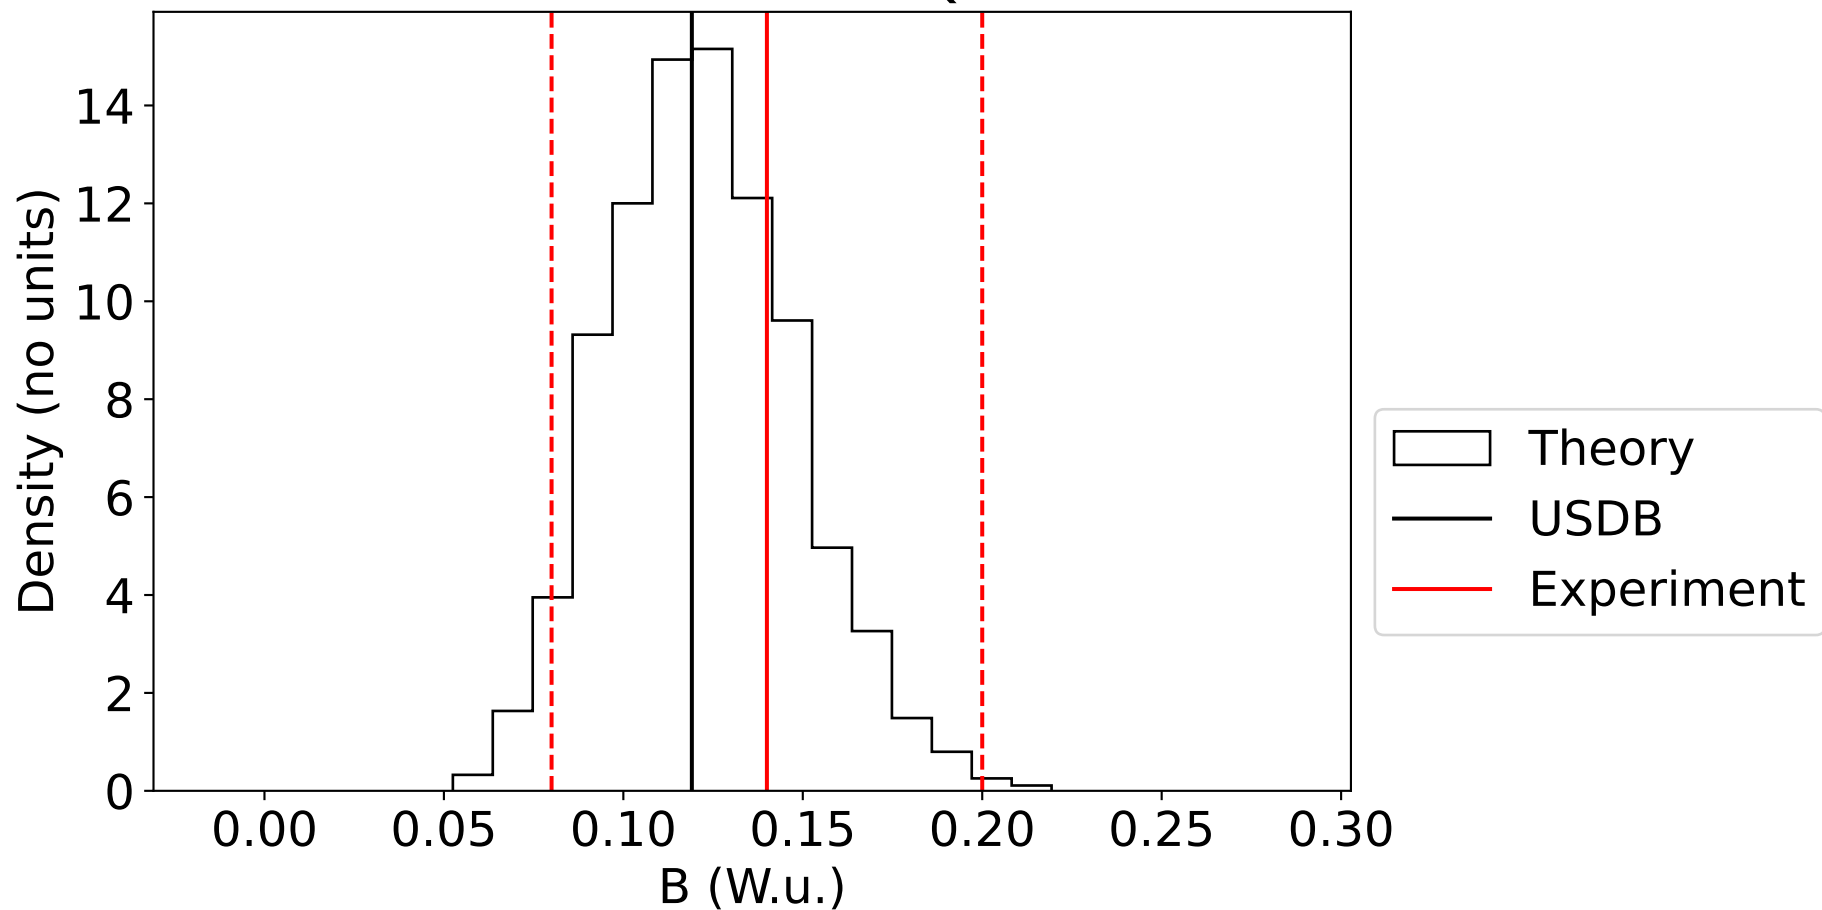



$^{27}\text{Al} (9/2_3) \rightarrow (9/2_1)$   
Included in UQ

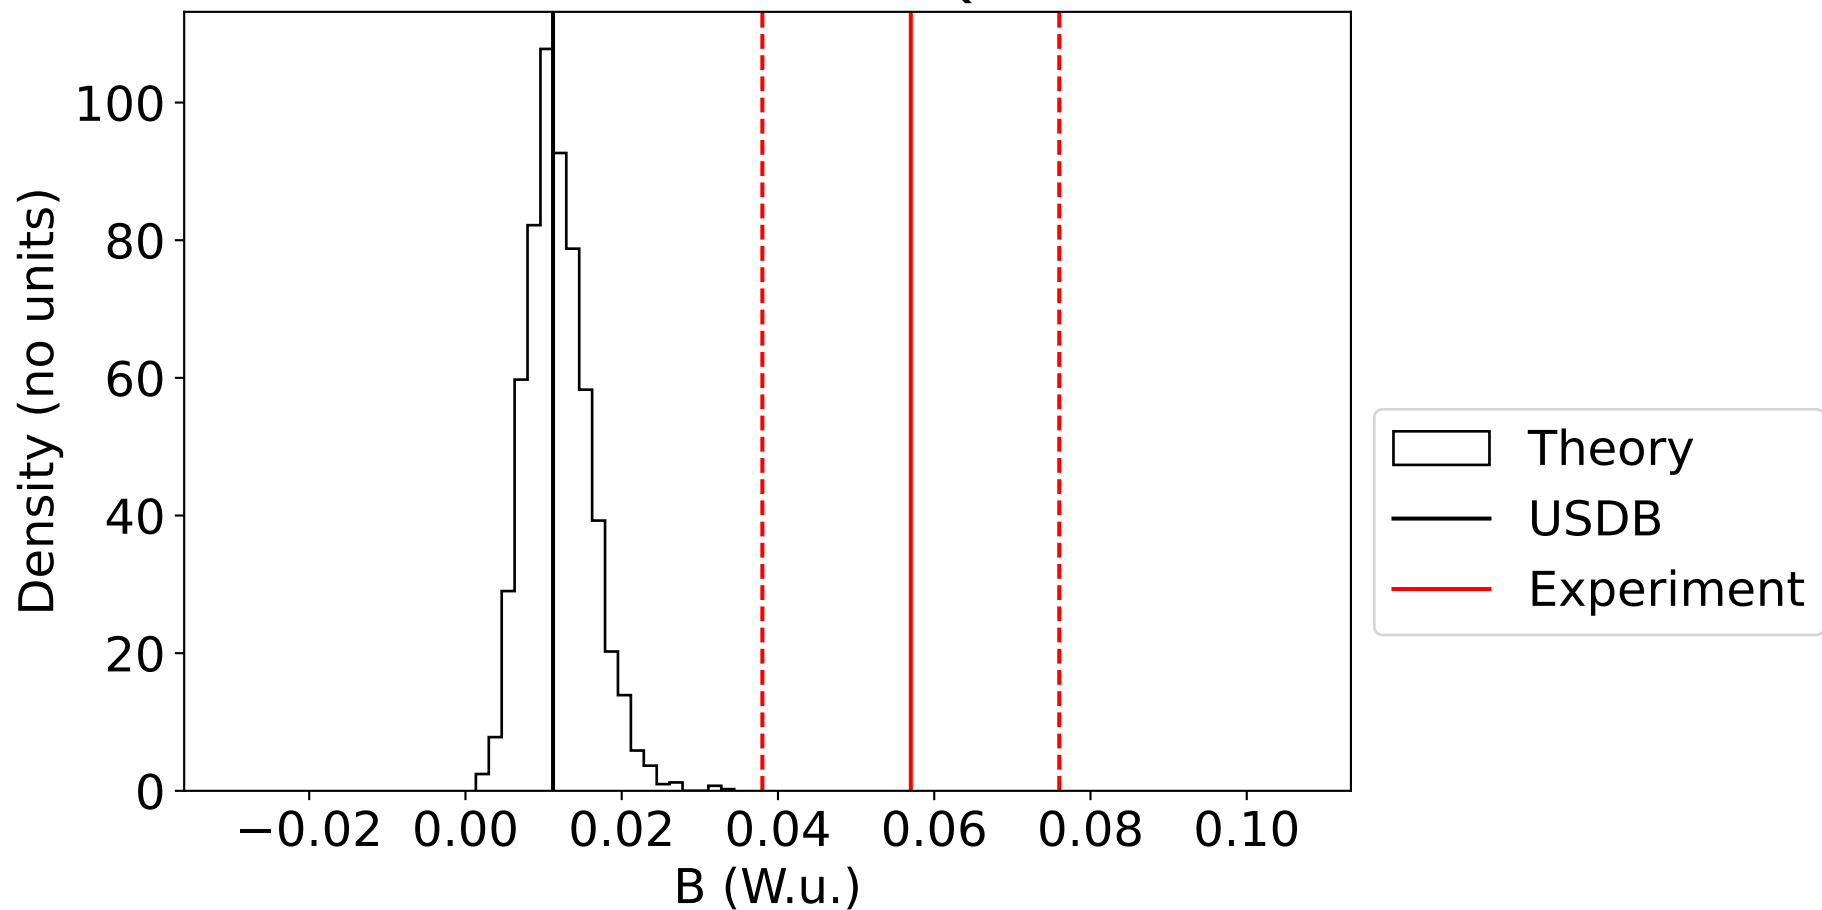

$^{27}\text{Al} (9/2_3) \rightarrow (11/2_1)$   
Included in UQ

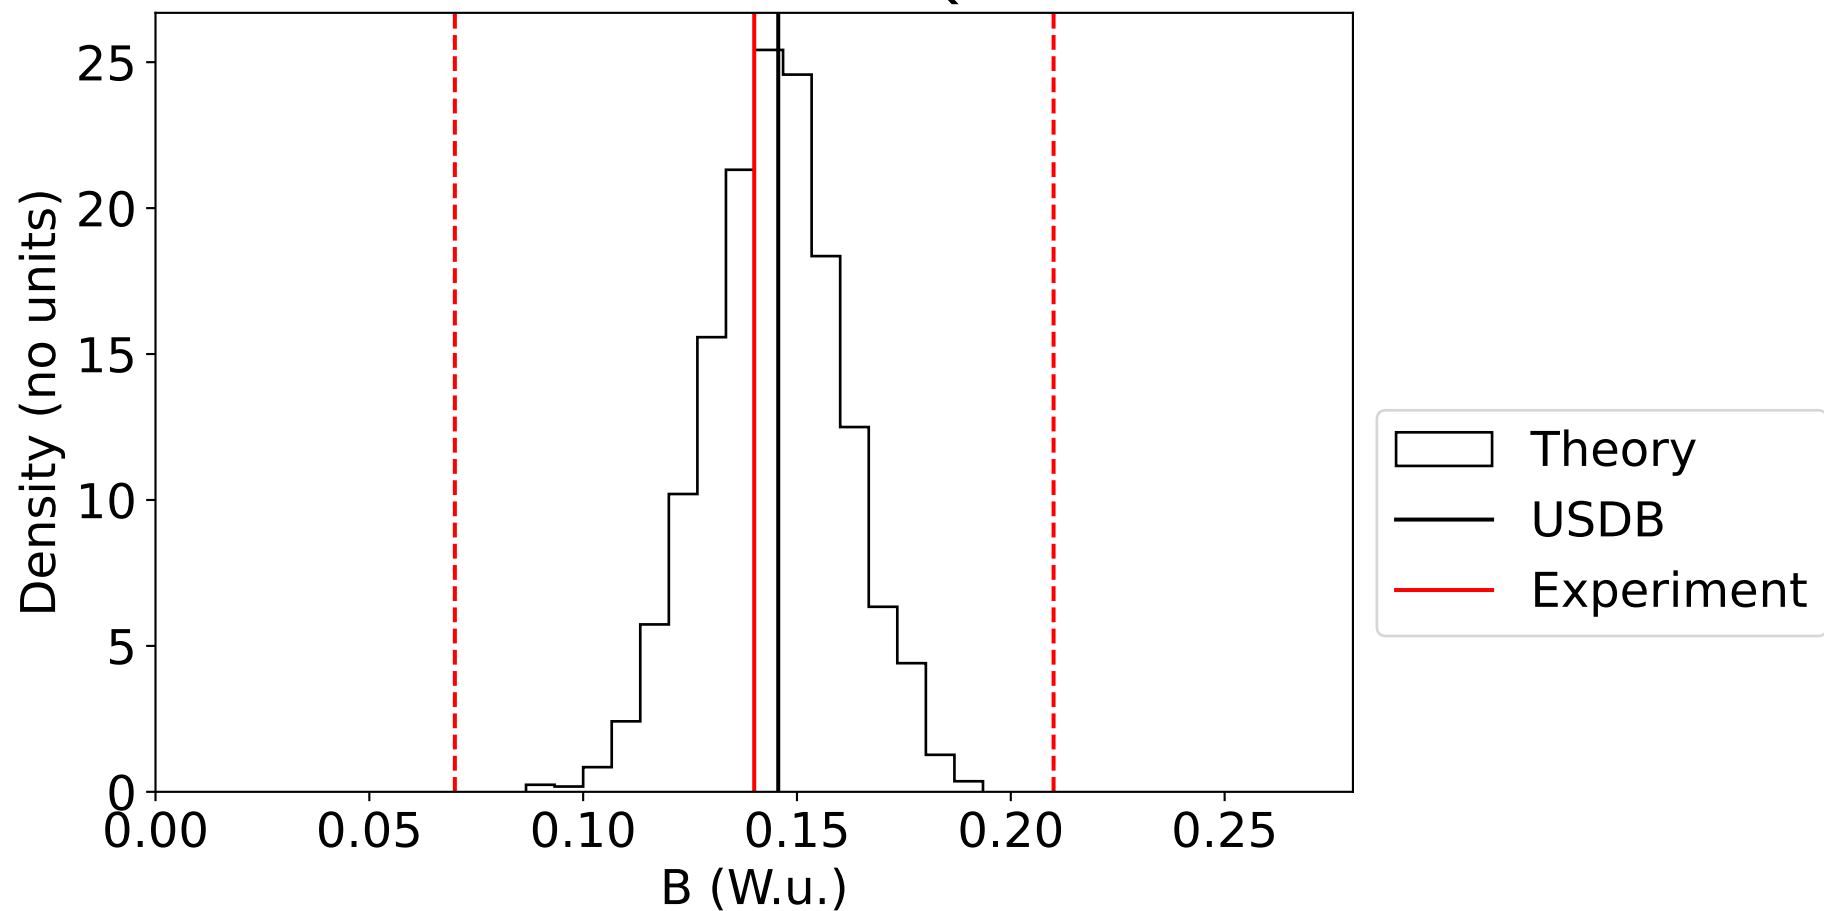

$^{28}\text{Al} (1_1) \rightarrow (2_1)$   
Included in UQ

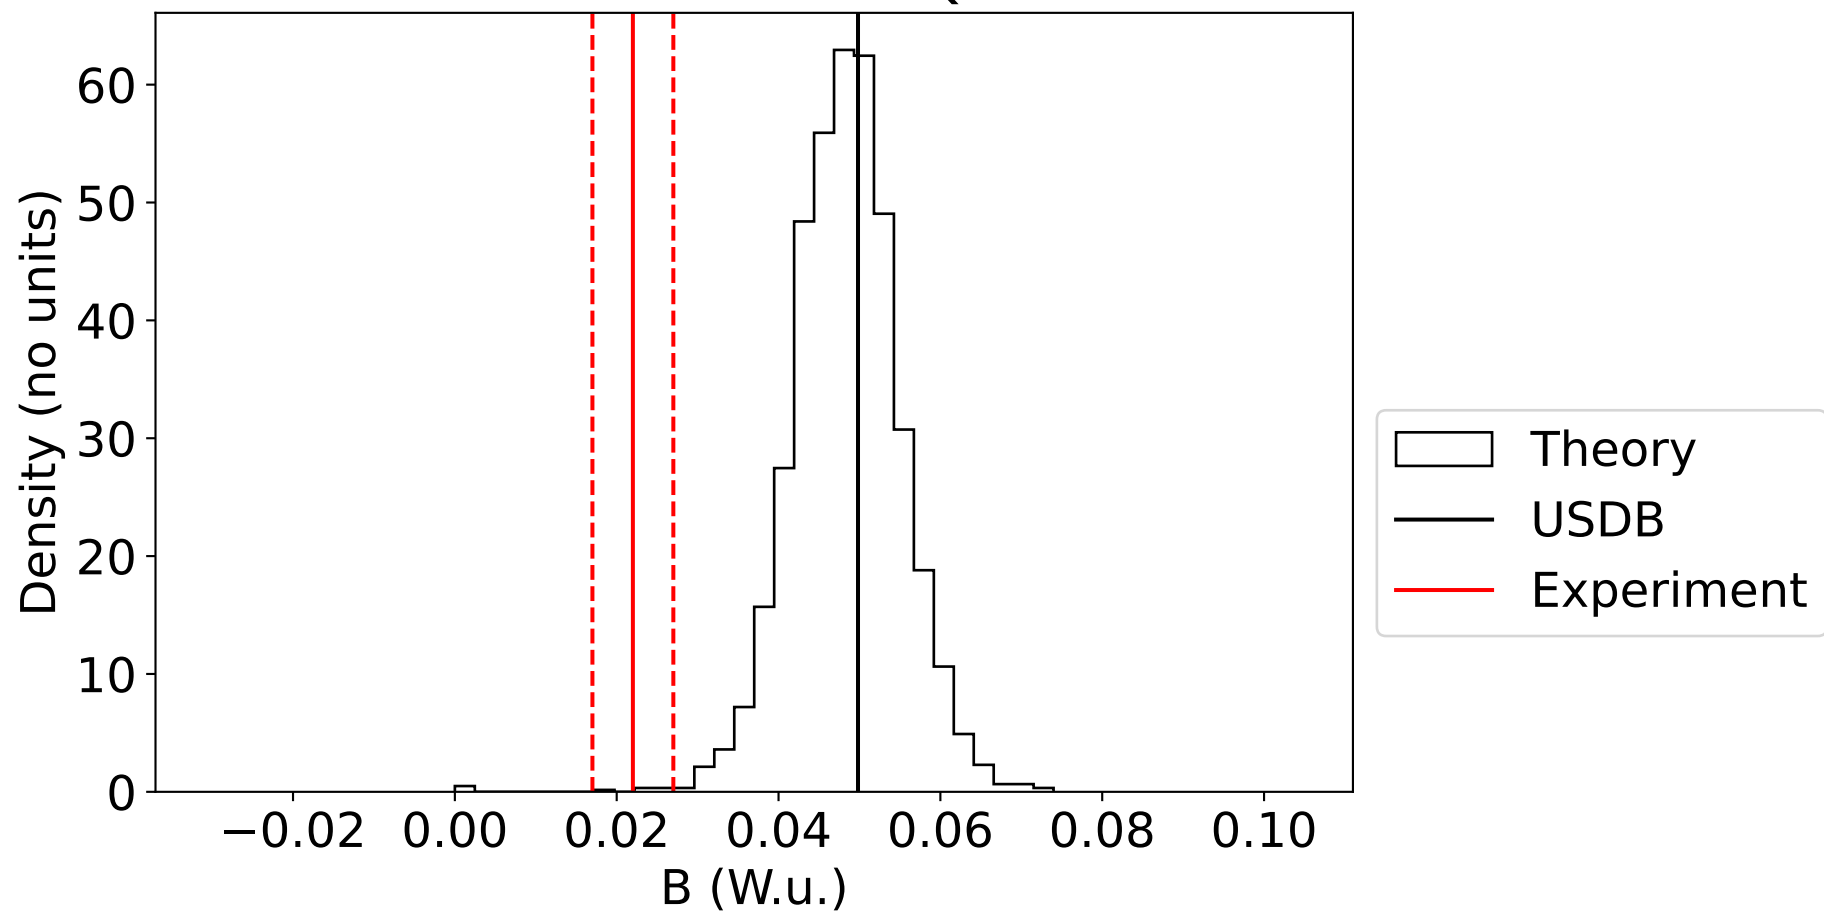

$^{28}\text{Al} (1_1) \rightarrow (0_1)$   
Included in UQ

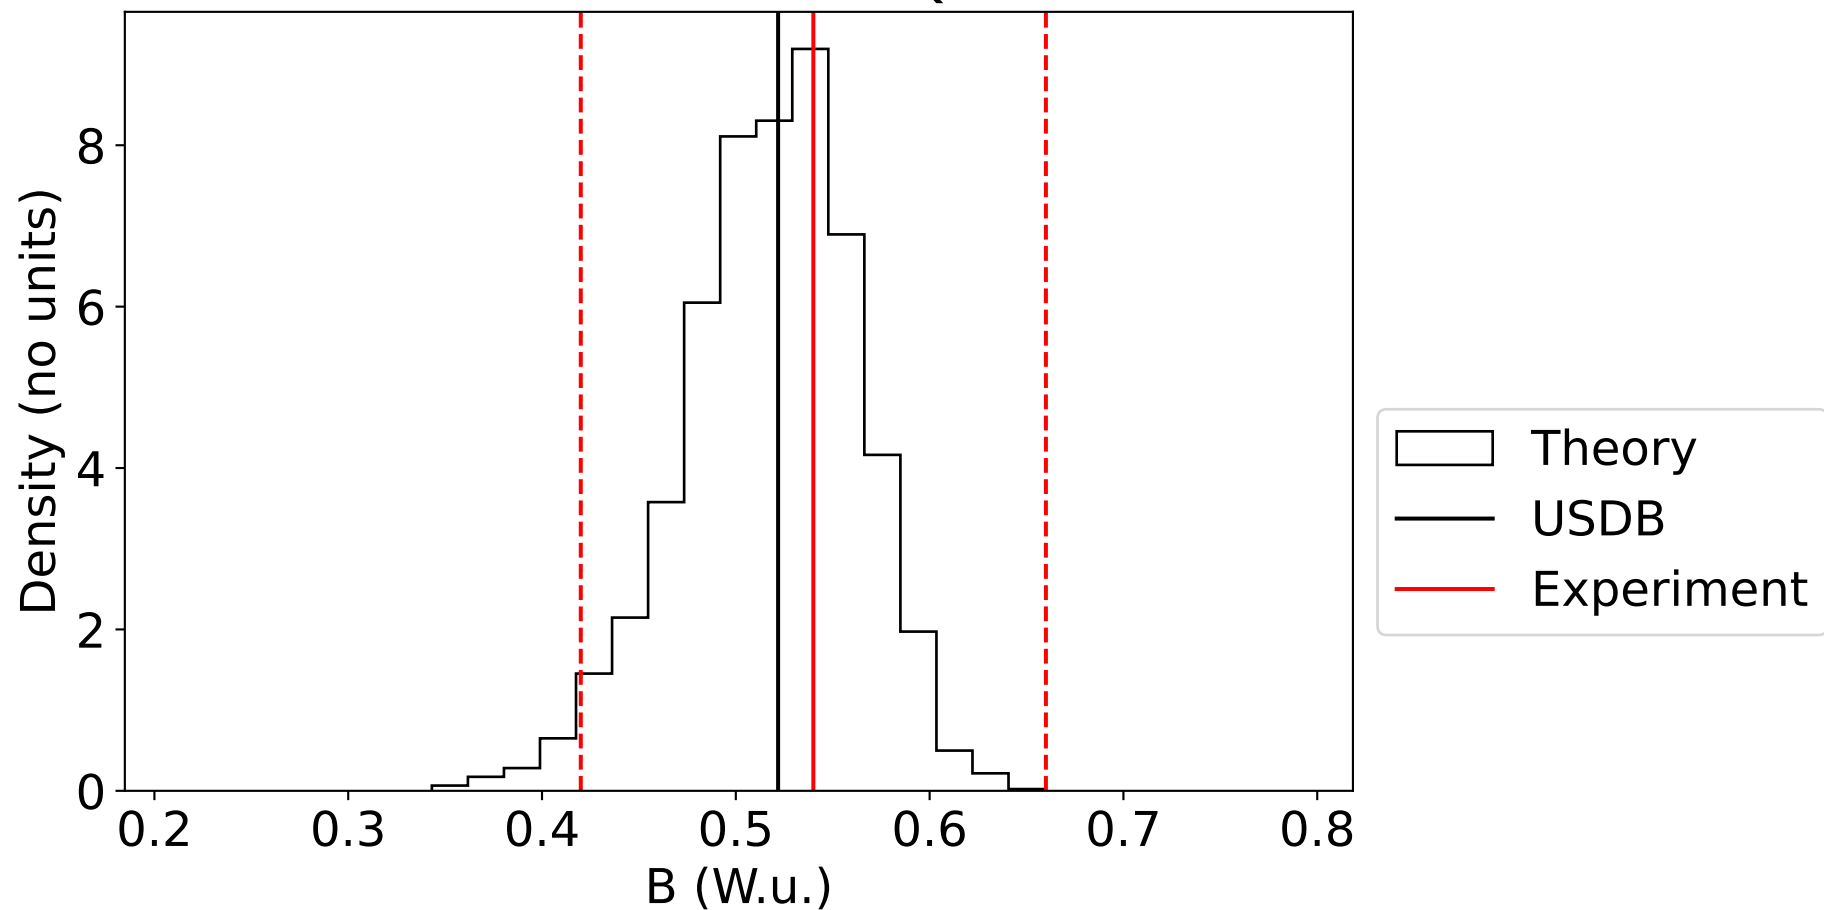

$^{28}\text{Al } (1_2) \rightarrow (0_1)$   
Included in UQ

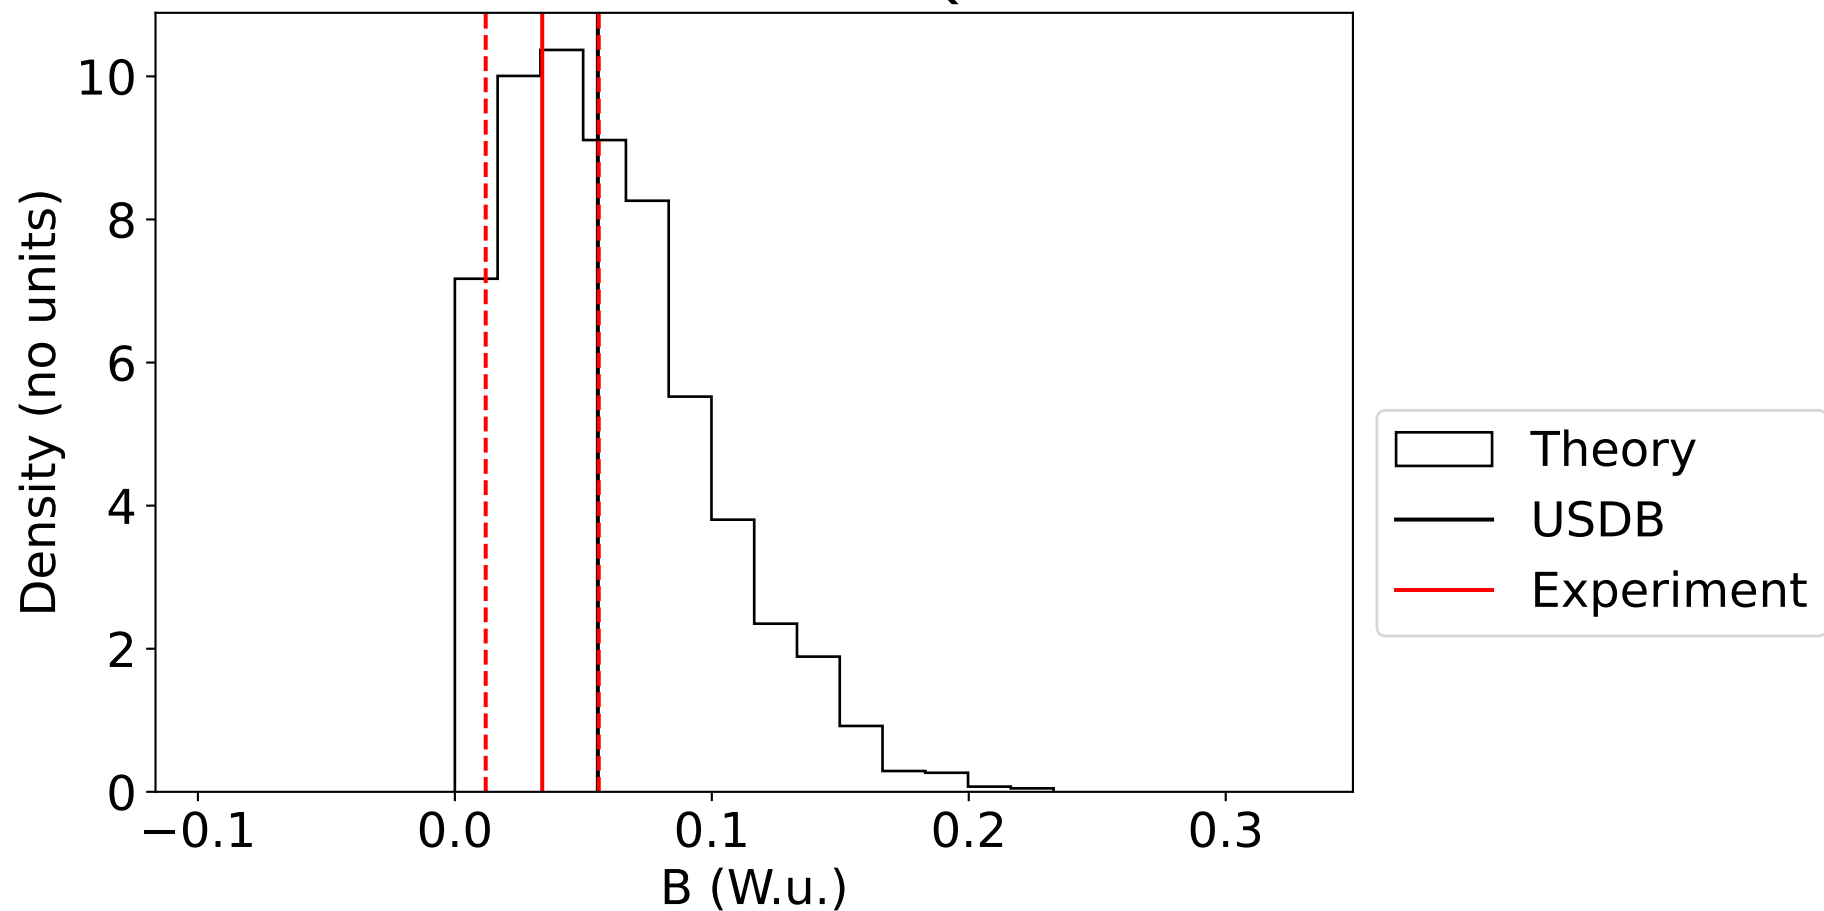

$^{28}\text{Al } (1_2) \rightarrow (2_1)$   
Included in UQ

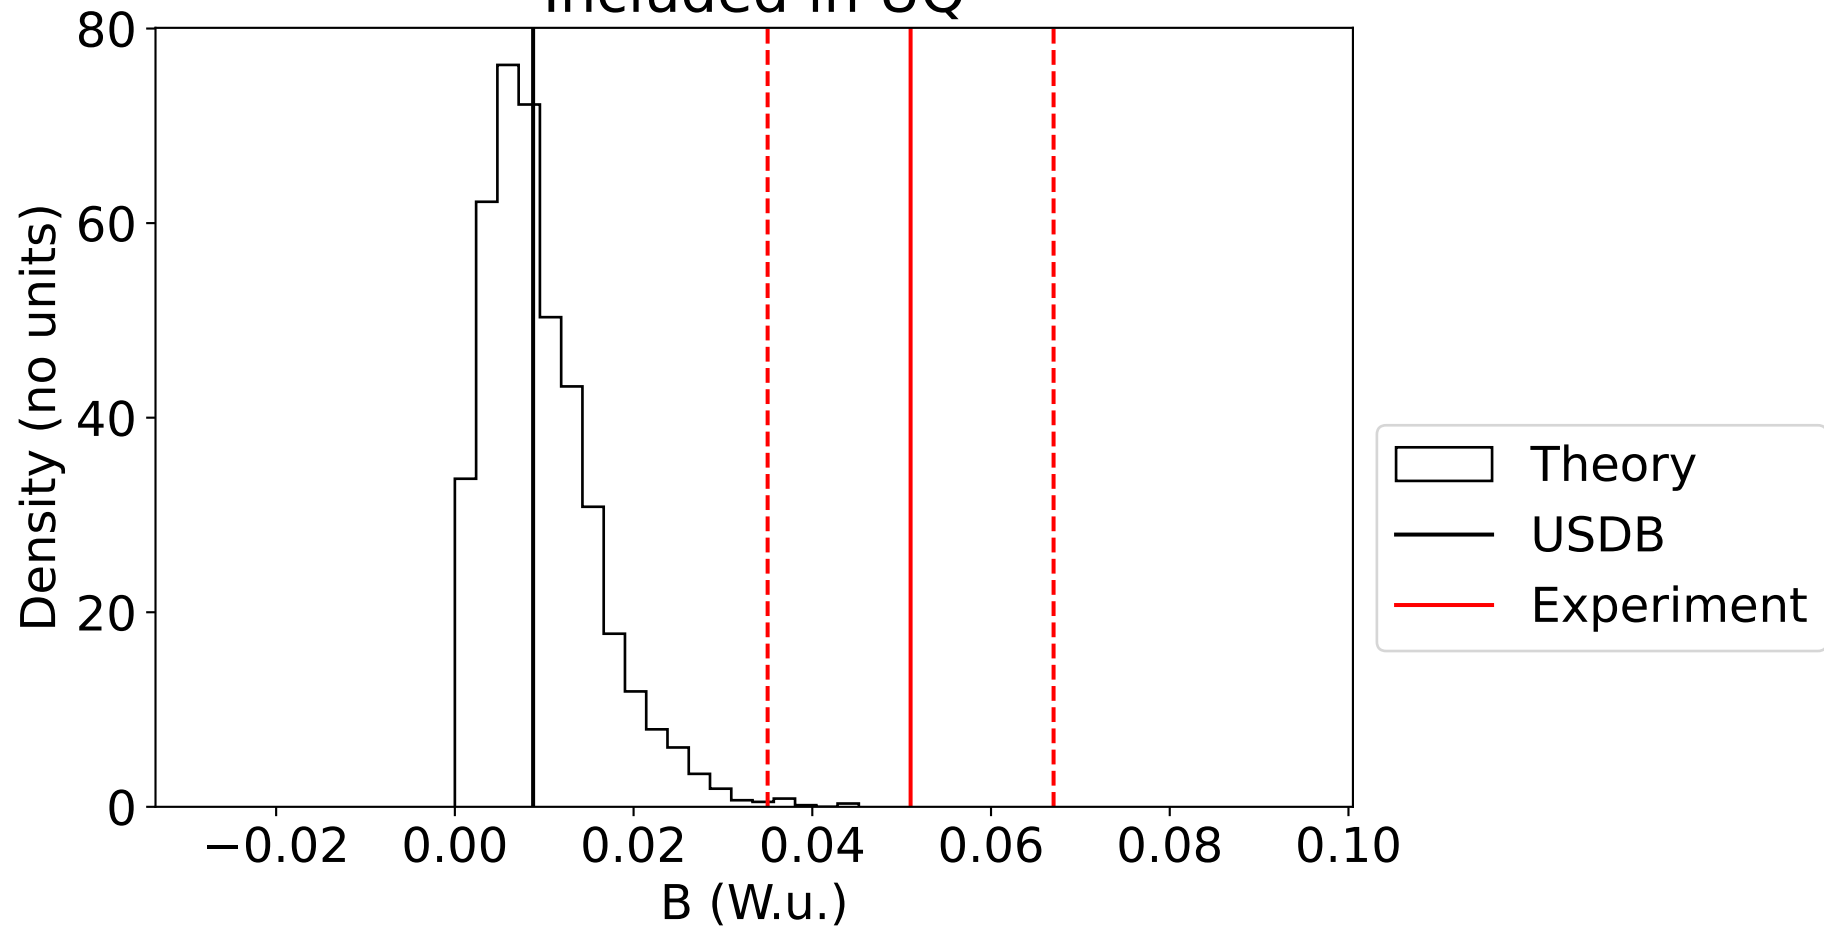

$^{28}\text{Al } (1_3) \rightarrow (0_1)$   
Included in UQ

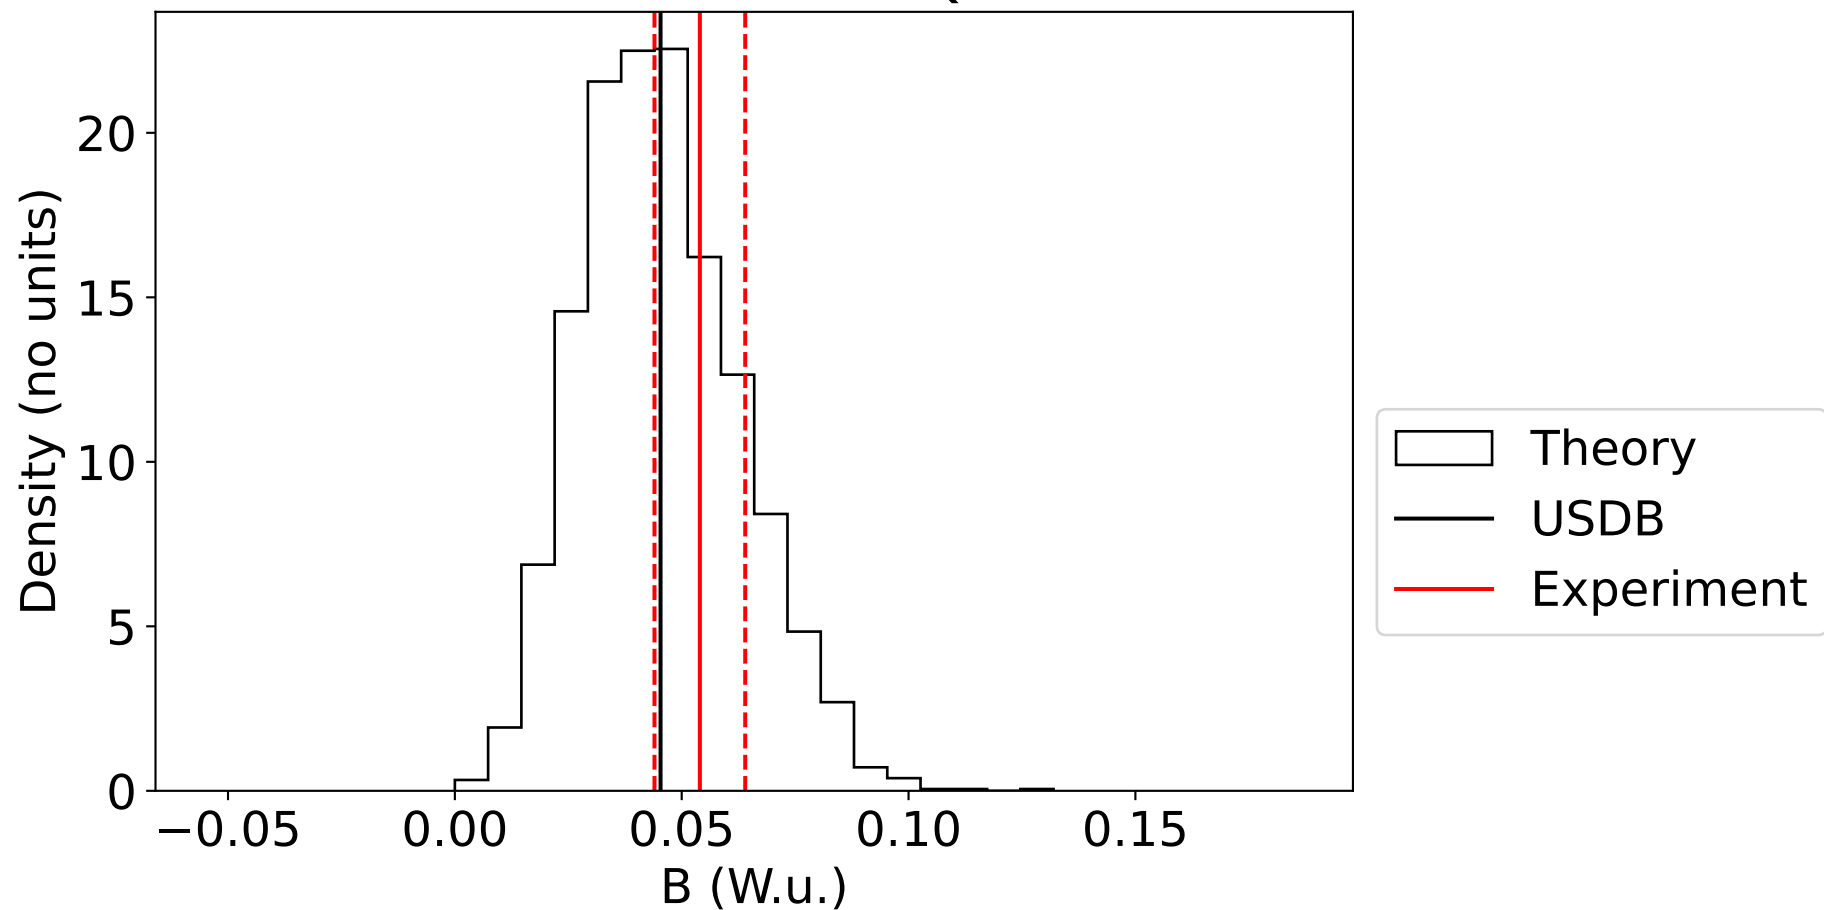

$^{28}\text{Al} (4_1) \rightarrow (3_1)$   
Included in UQ

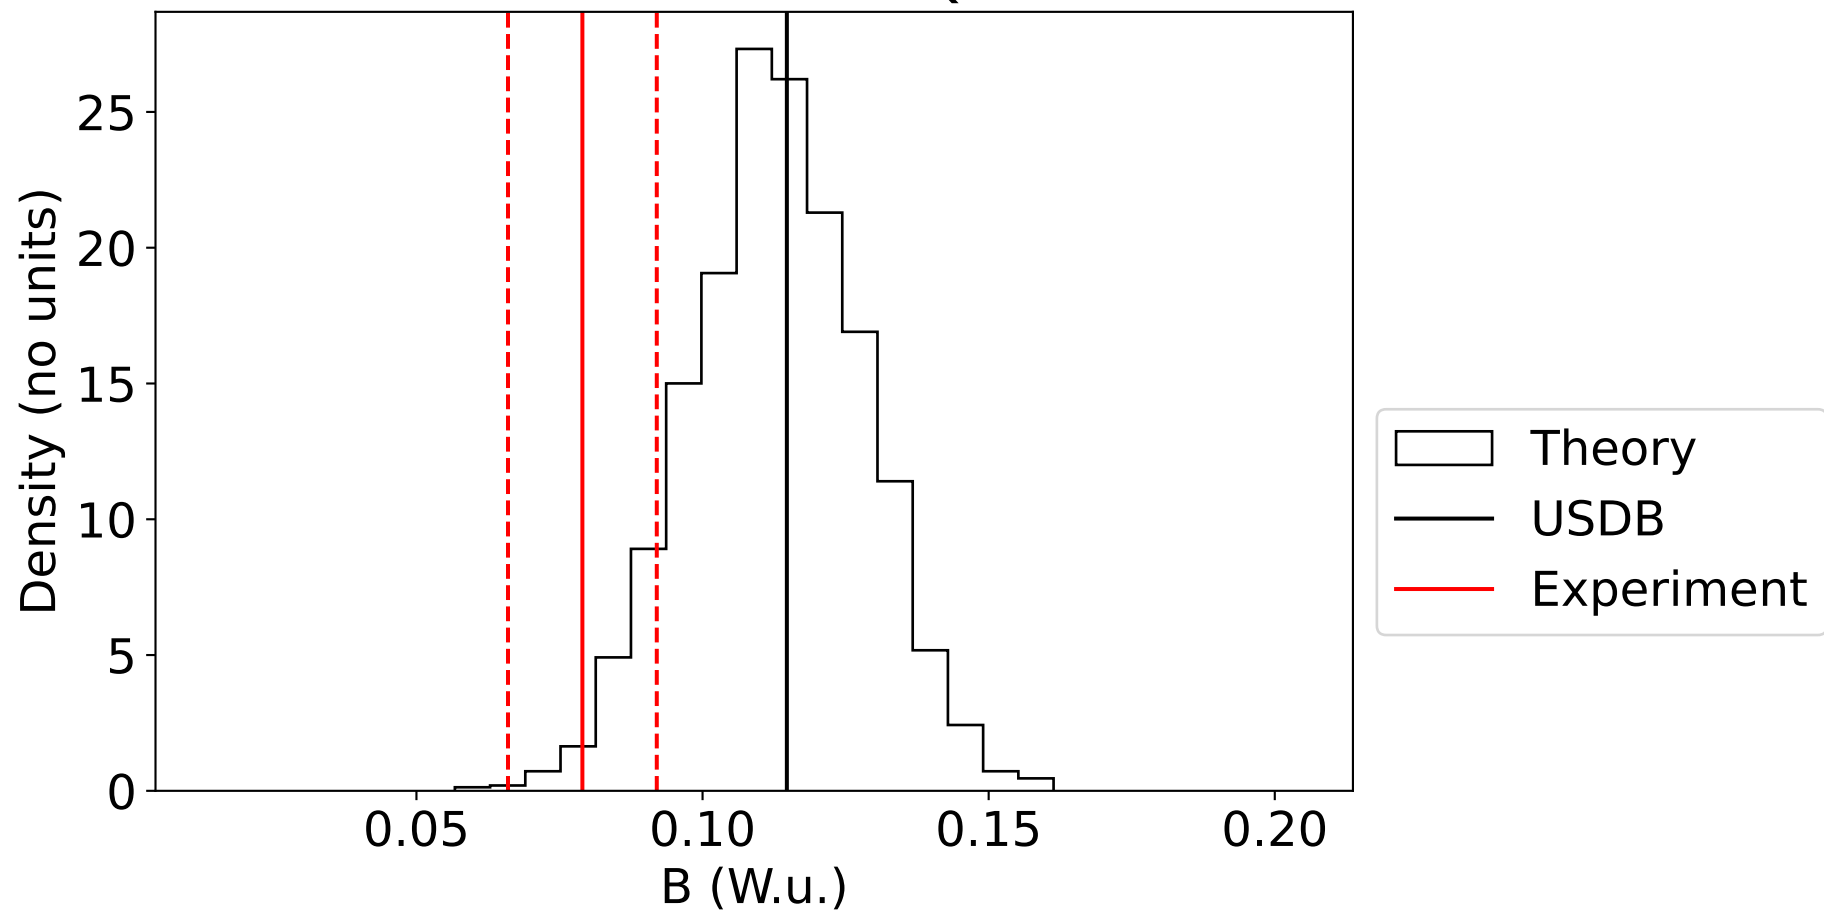



$^{28}\text{Al} (5_1) \rightarrow (4_1)$   
Included in UQ

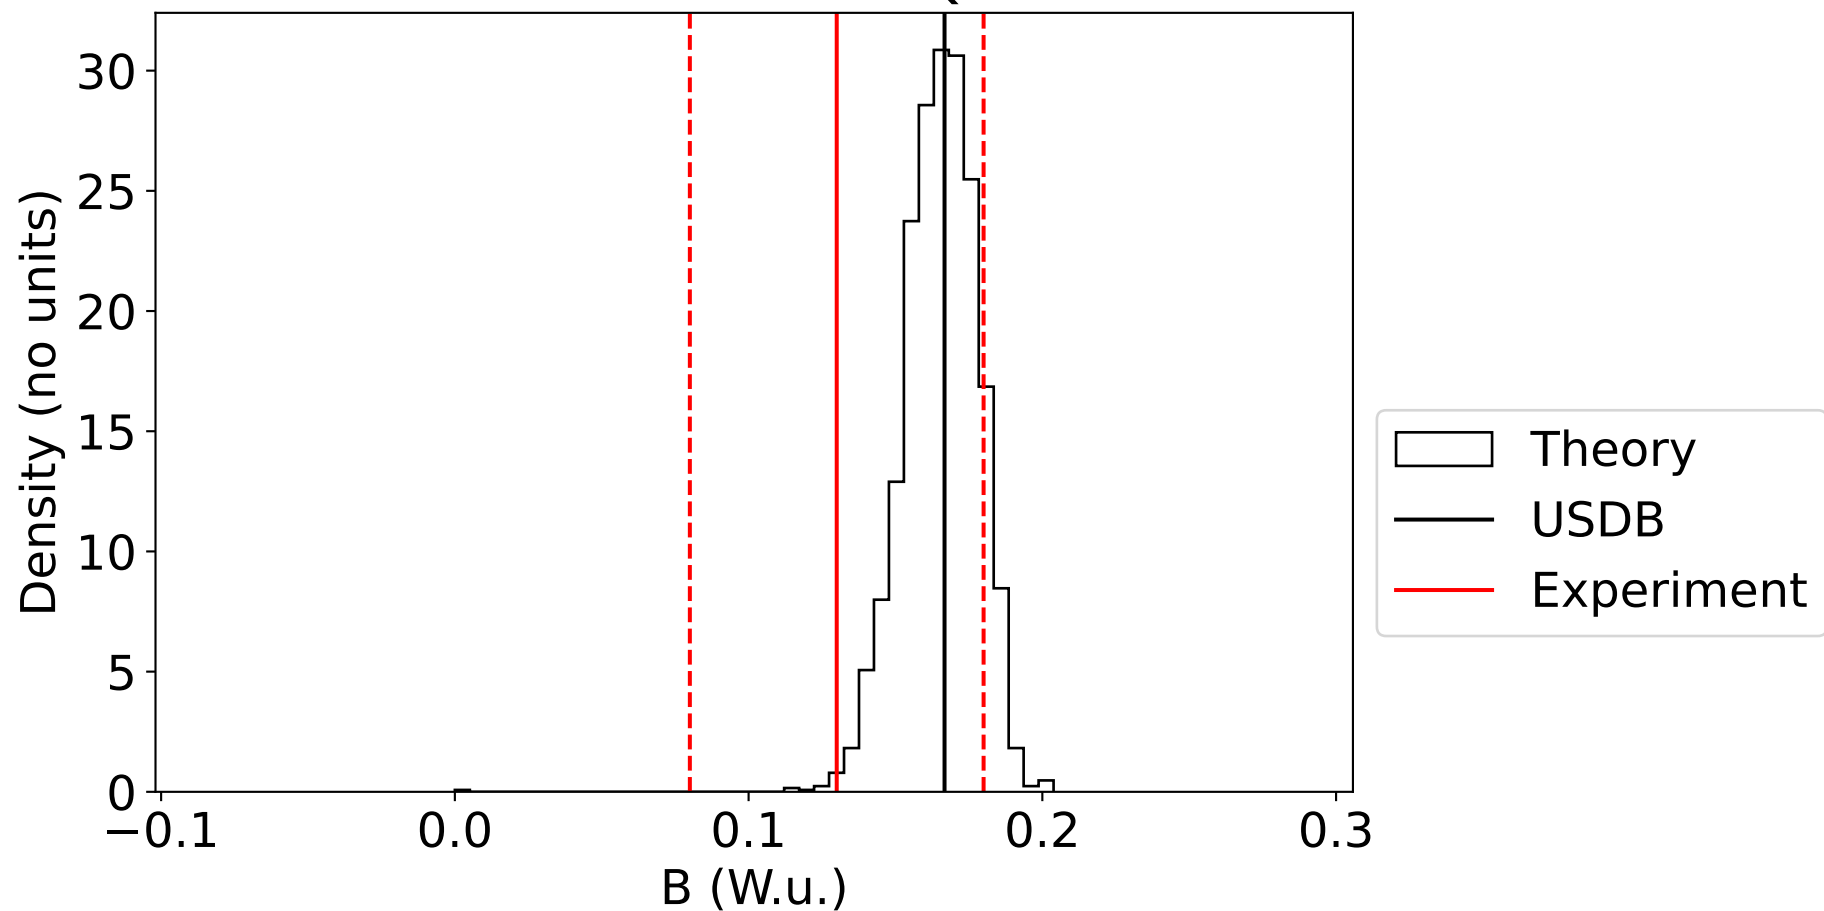

$^{28}\text{Al} (4_2) \rightarrow (3_2)$   
Included in UQ

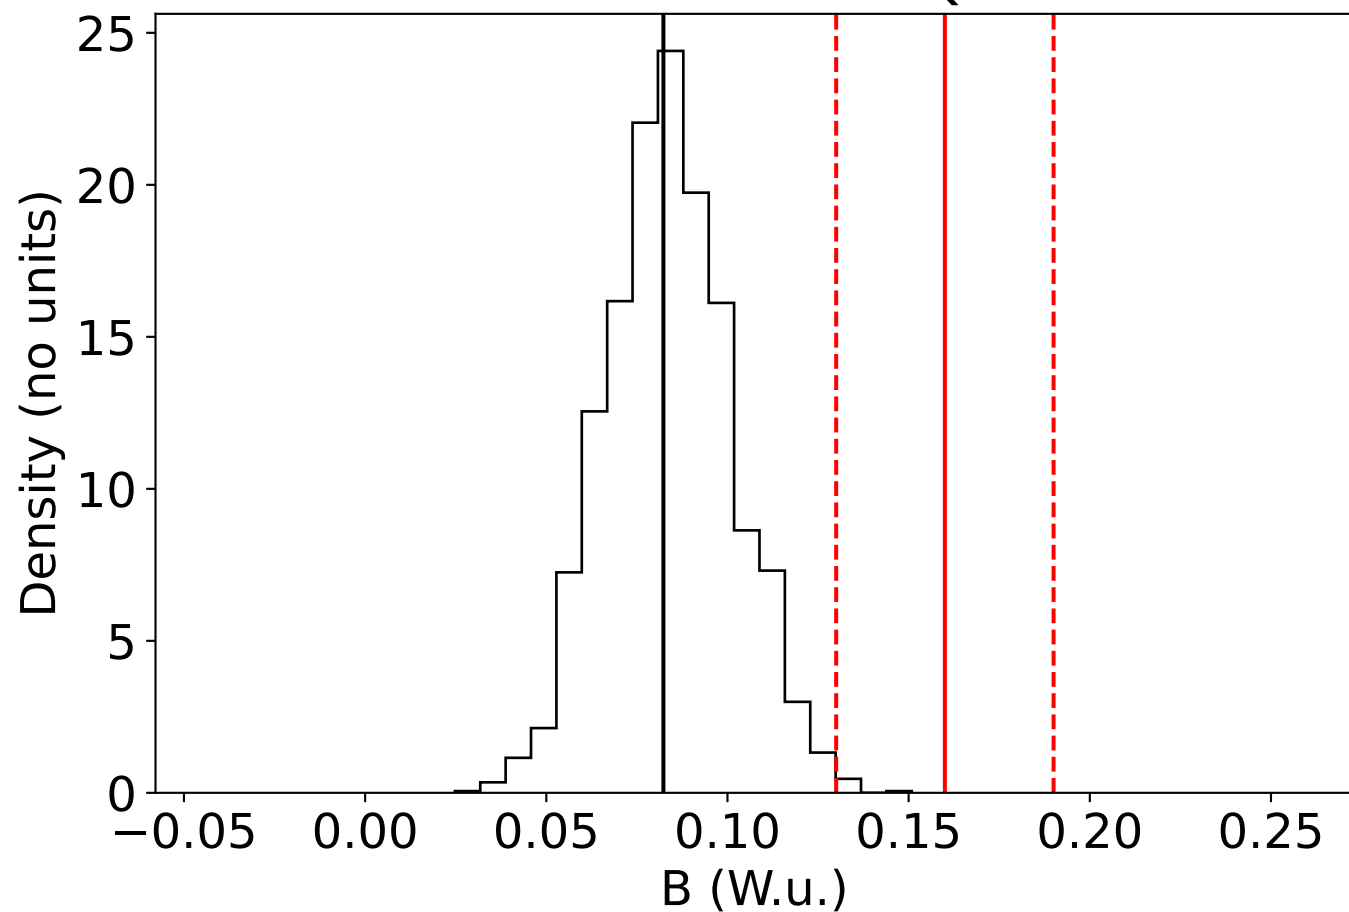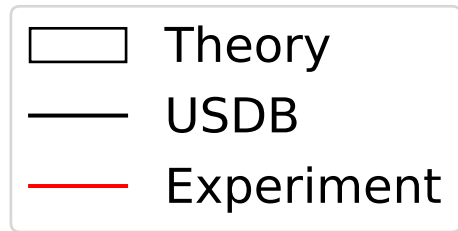

$^{29}\text{Al} (5/2_3) \rightarrow (7/2_1)$   
Included in UQ

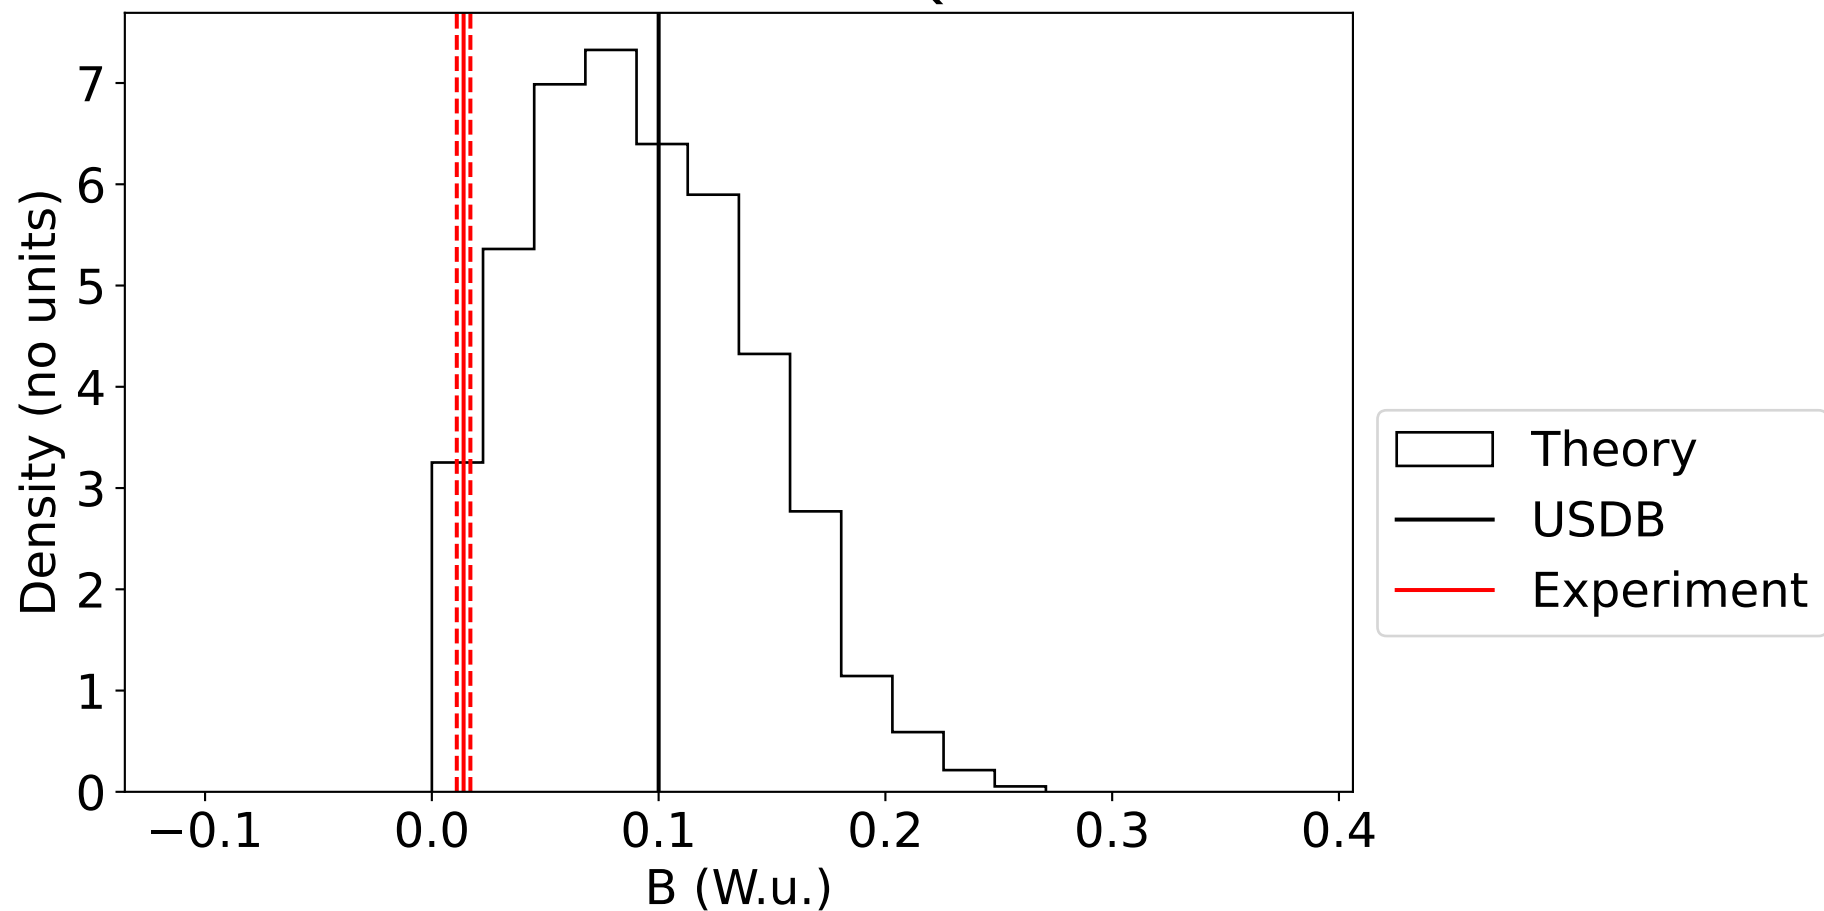

$^{29}\text{Al} (5/2_3) \rightarrow (3/2_1)$   
Included in UQ

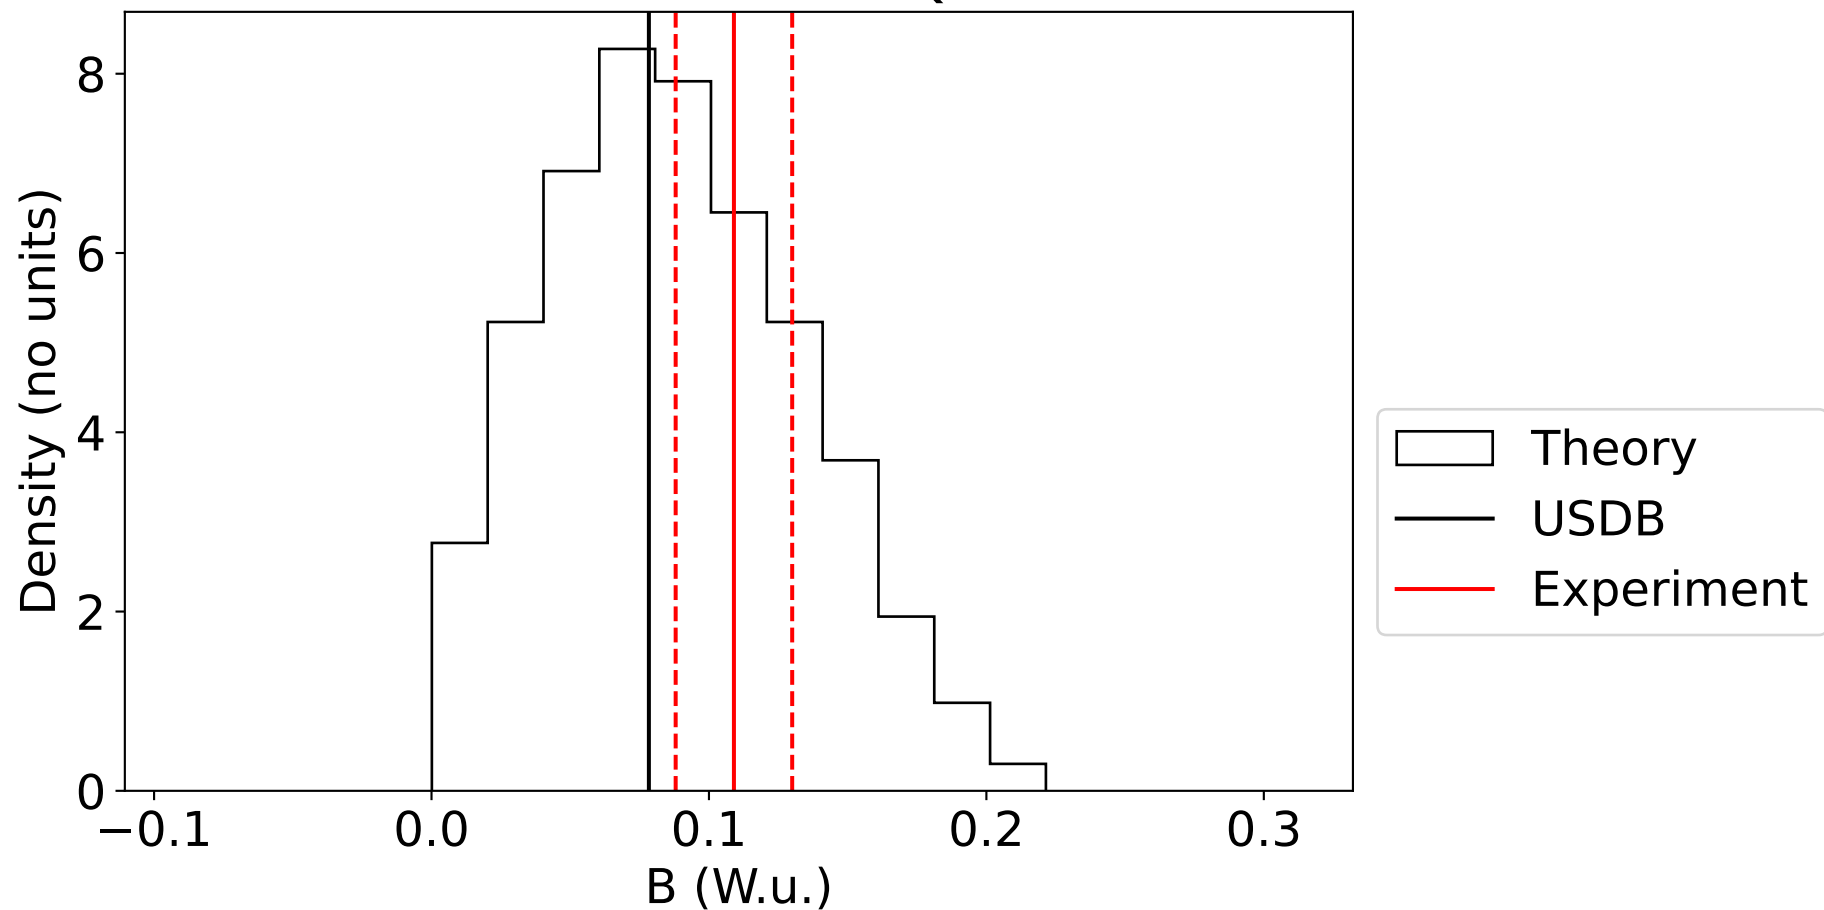

$^{30}\text{Al} (1_1) \rightarrow (2_1)$   
Included in UQ

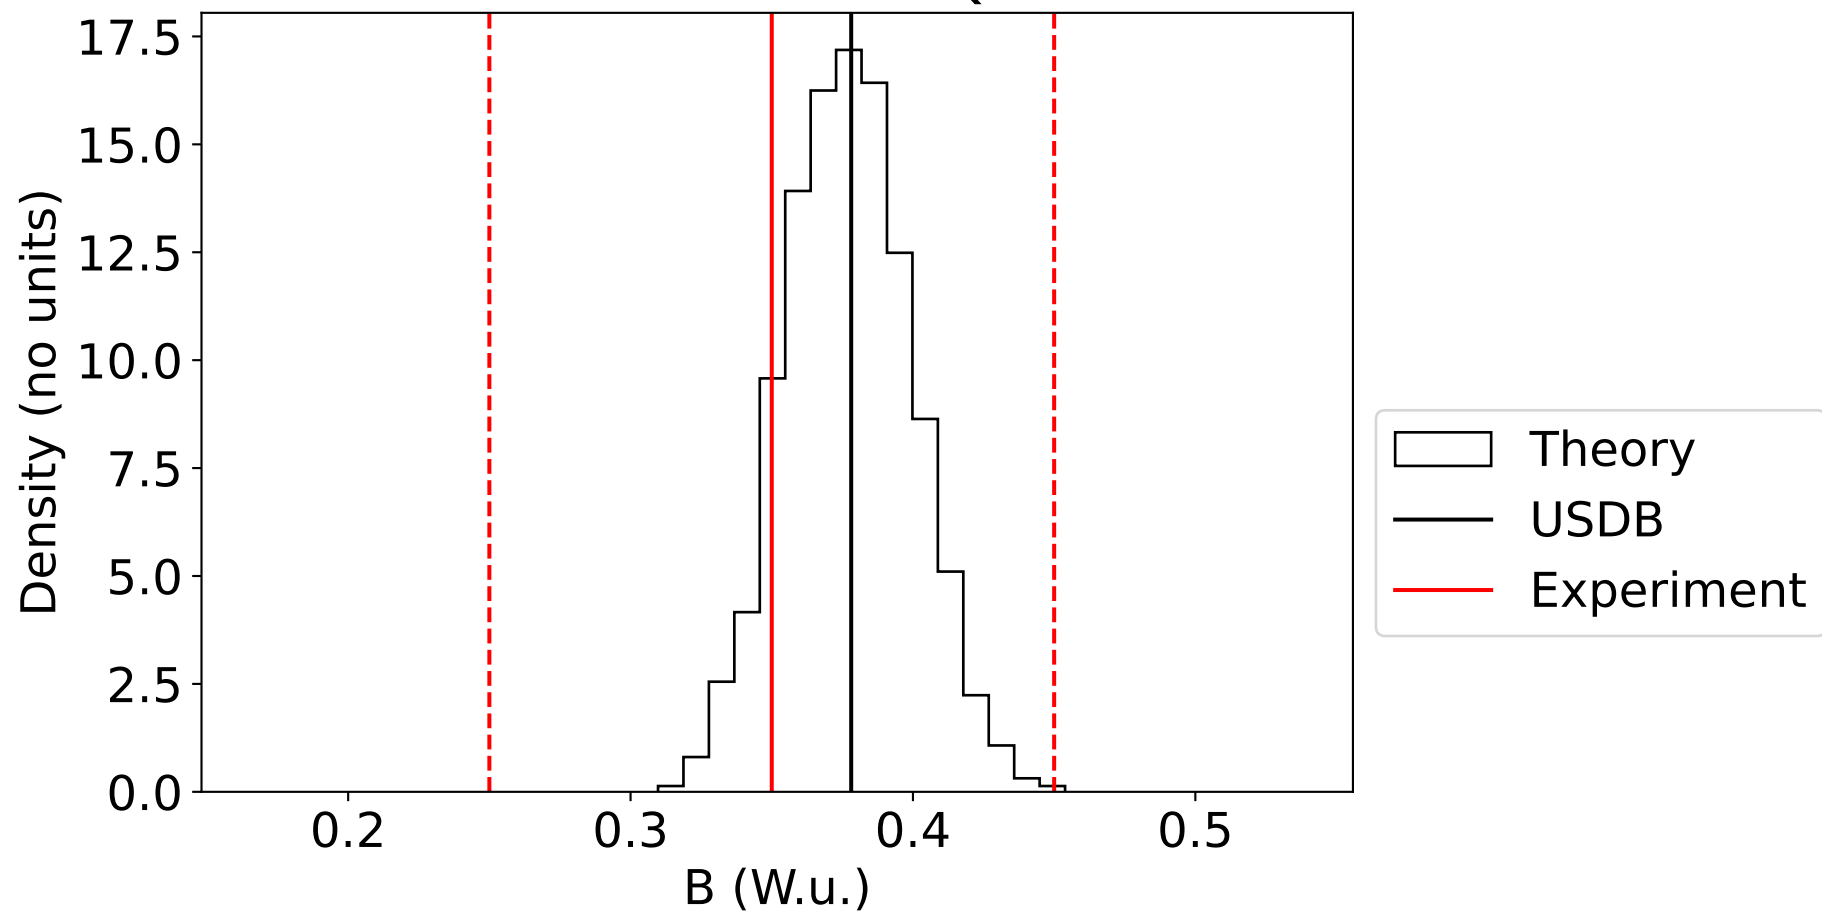

$^{30}\text{Al} (3_2) \rightarrow (2_1)$   
Included in UQ

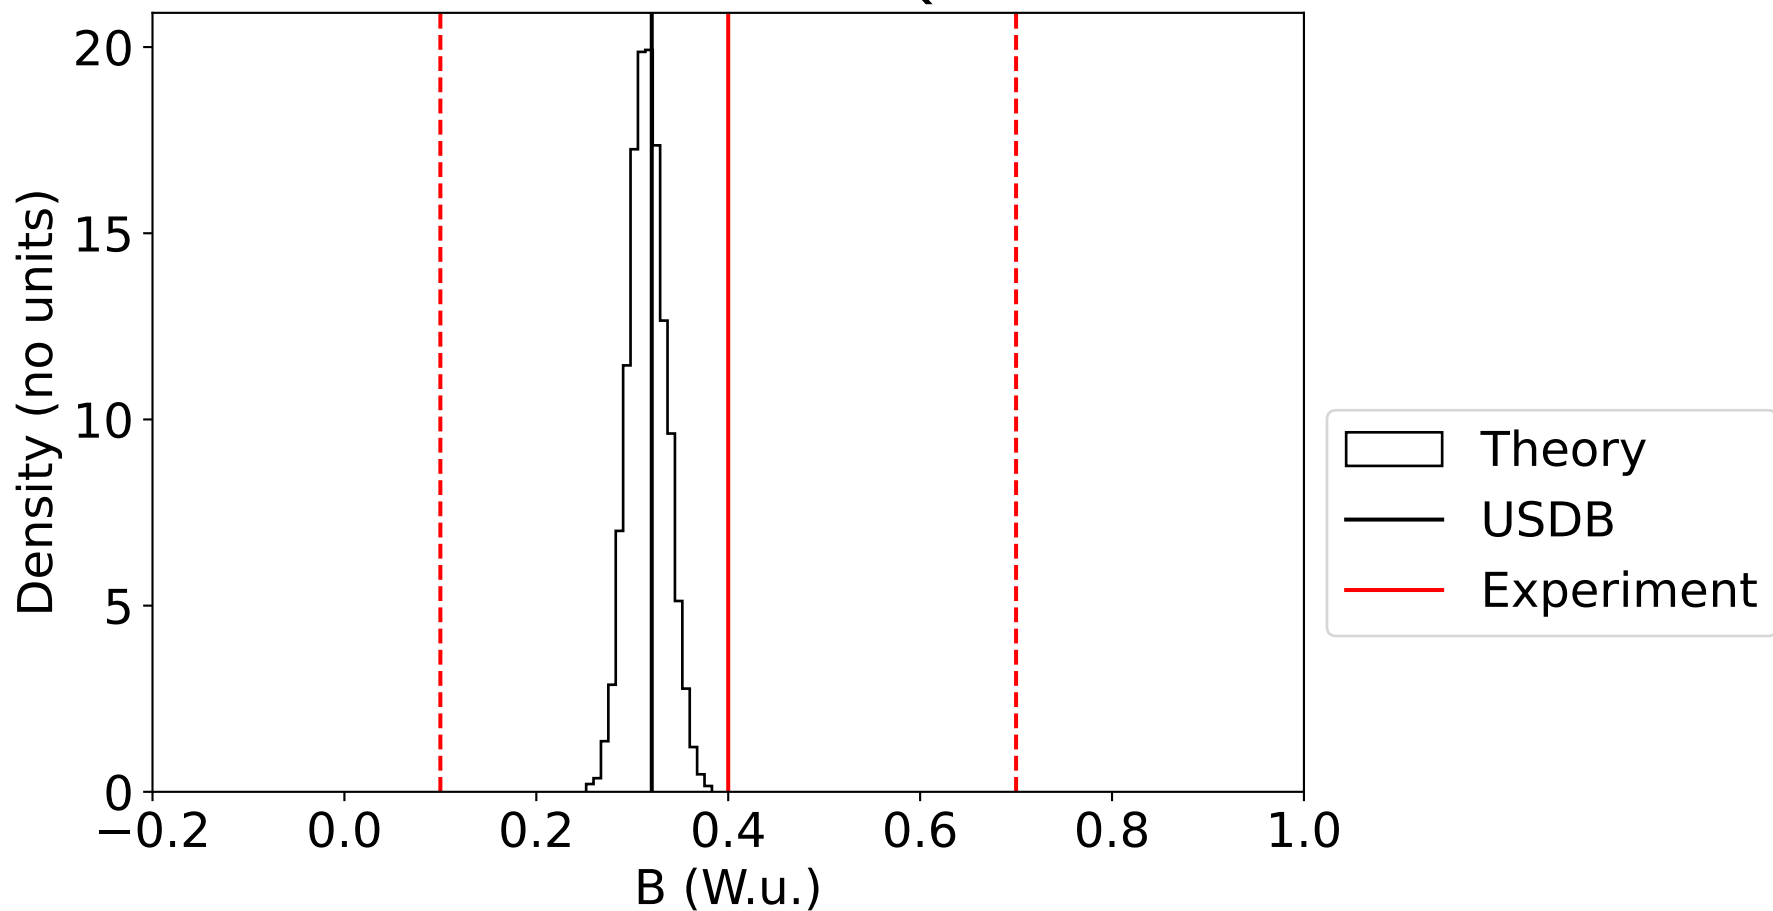

$^{26}\text{Si} (2_2) \rightarrow (2_1)$   
Included in UQ

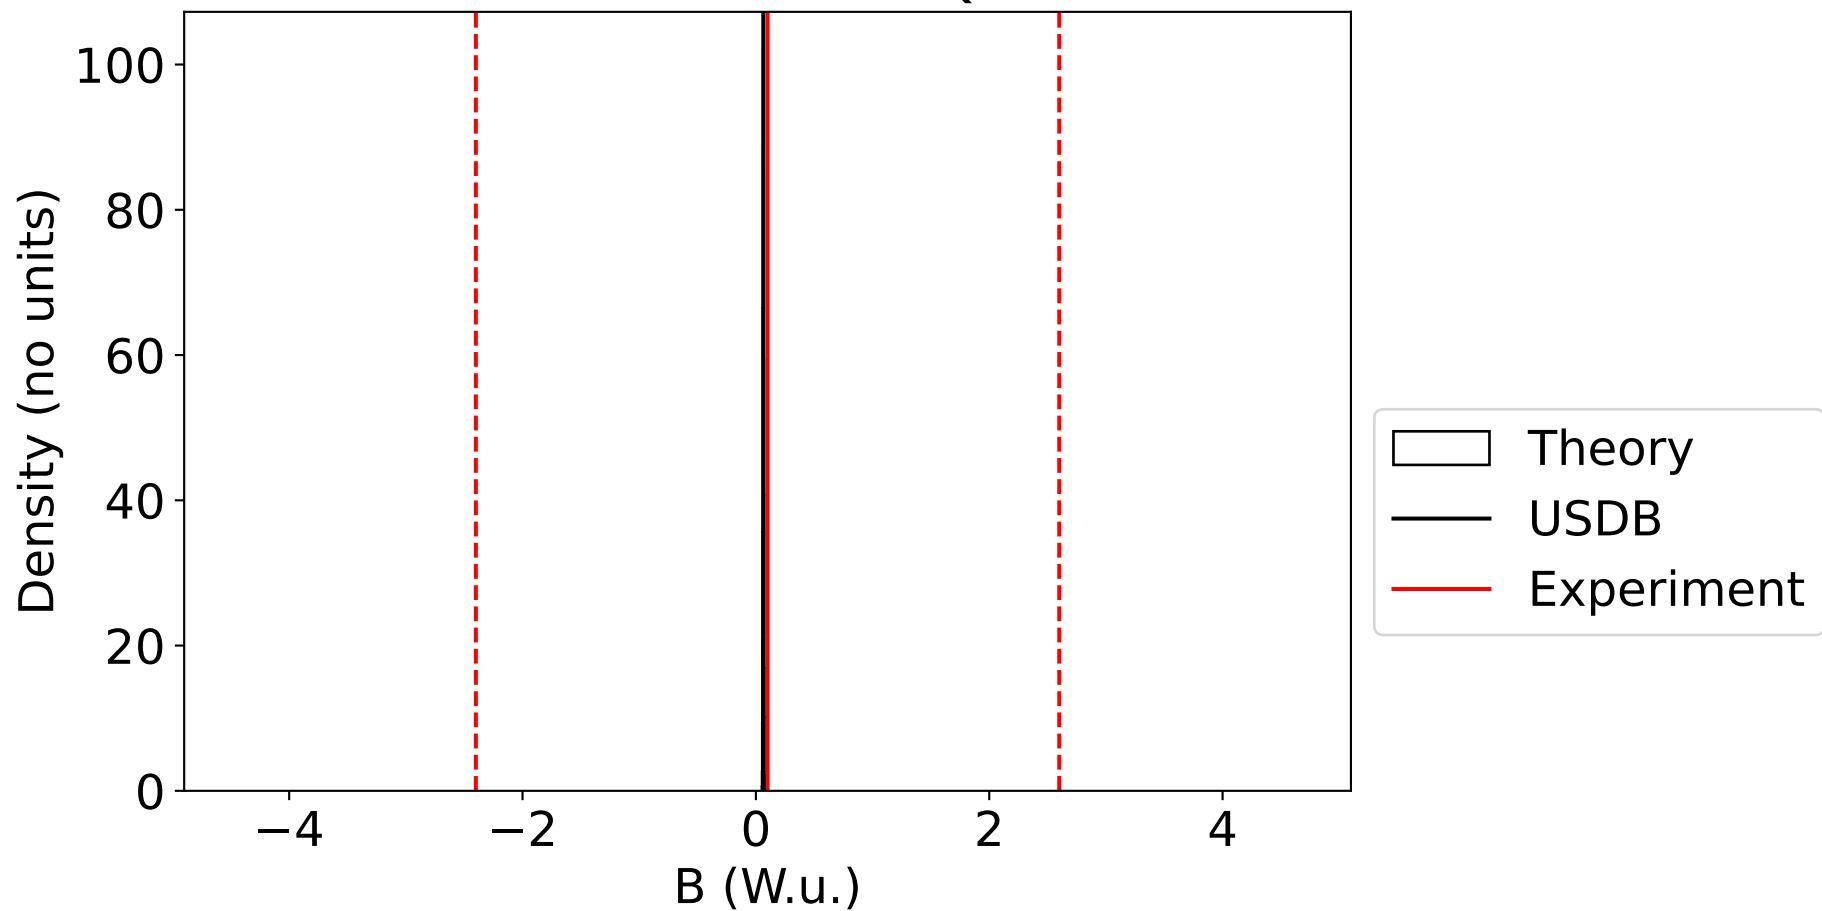

$^{27}\text{Si} (3/2_1) \rightarrow (5/2_1)$   
Included in UQ

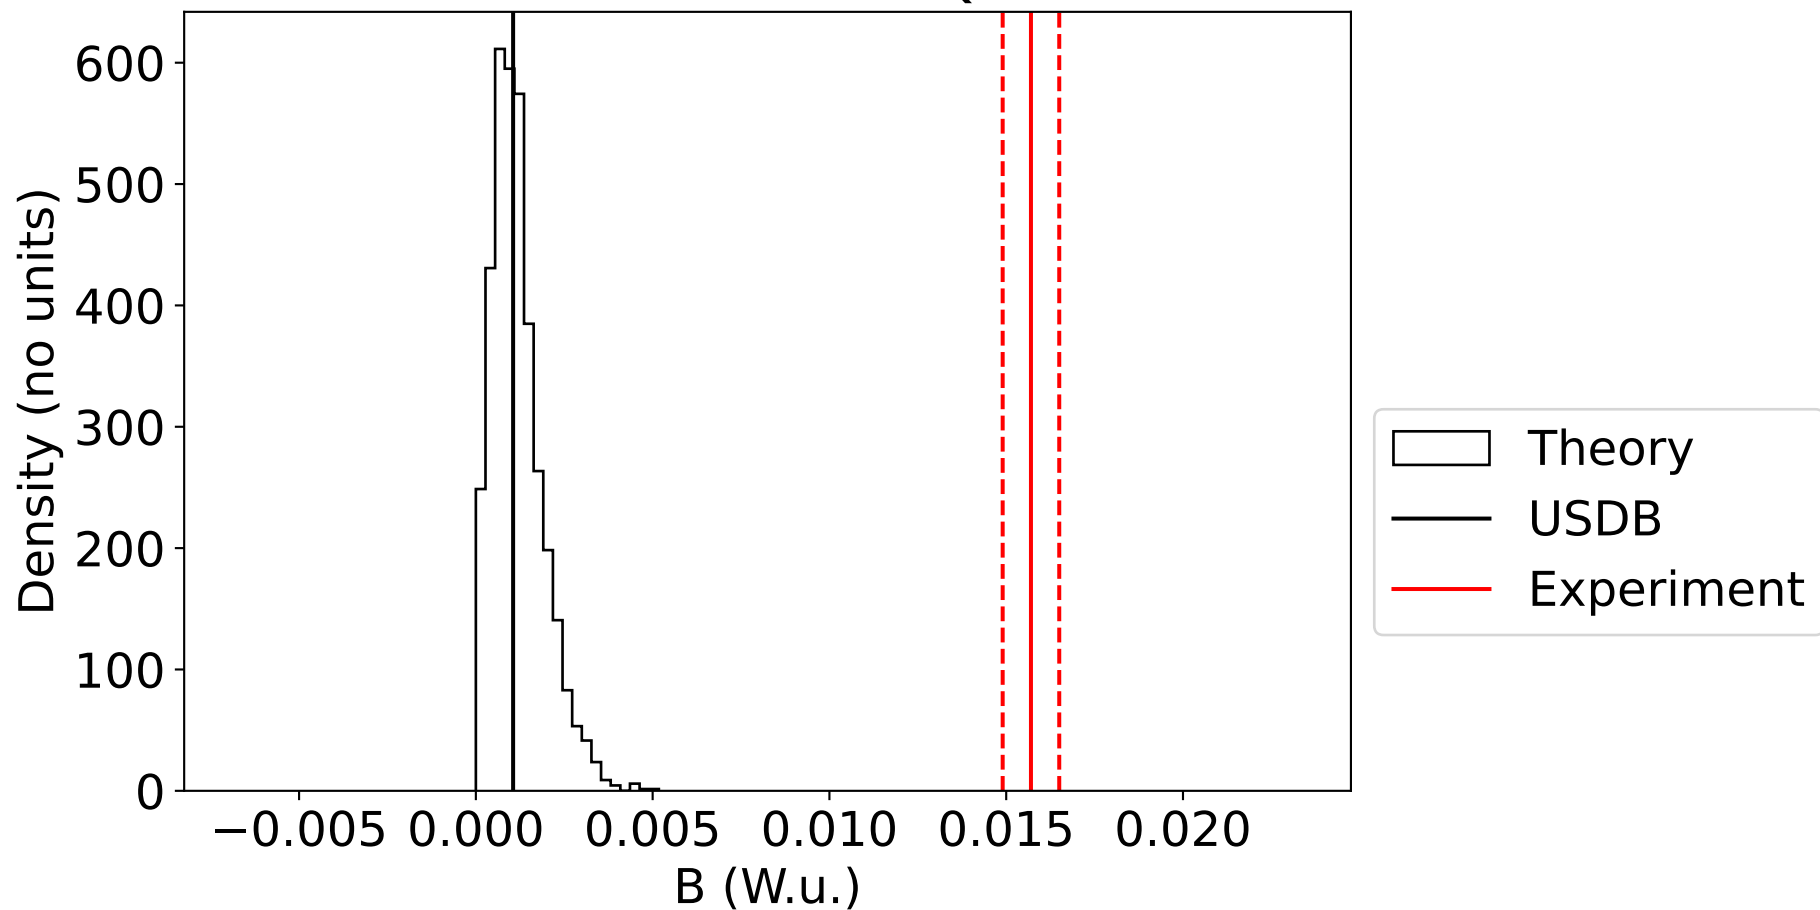



$^{27}\text{Si} (3/2_1) \rightarrow (1/2_1)$   
Included in UQ

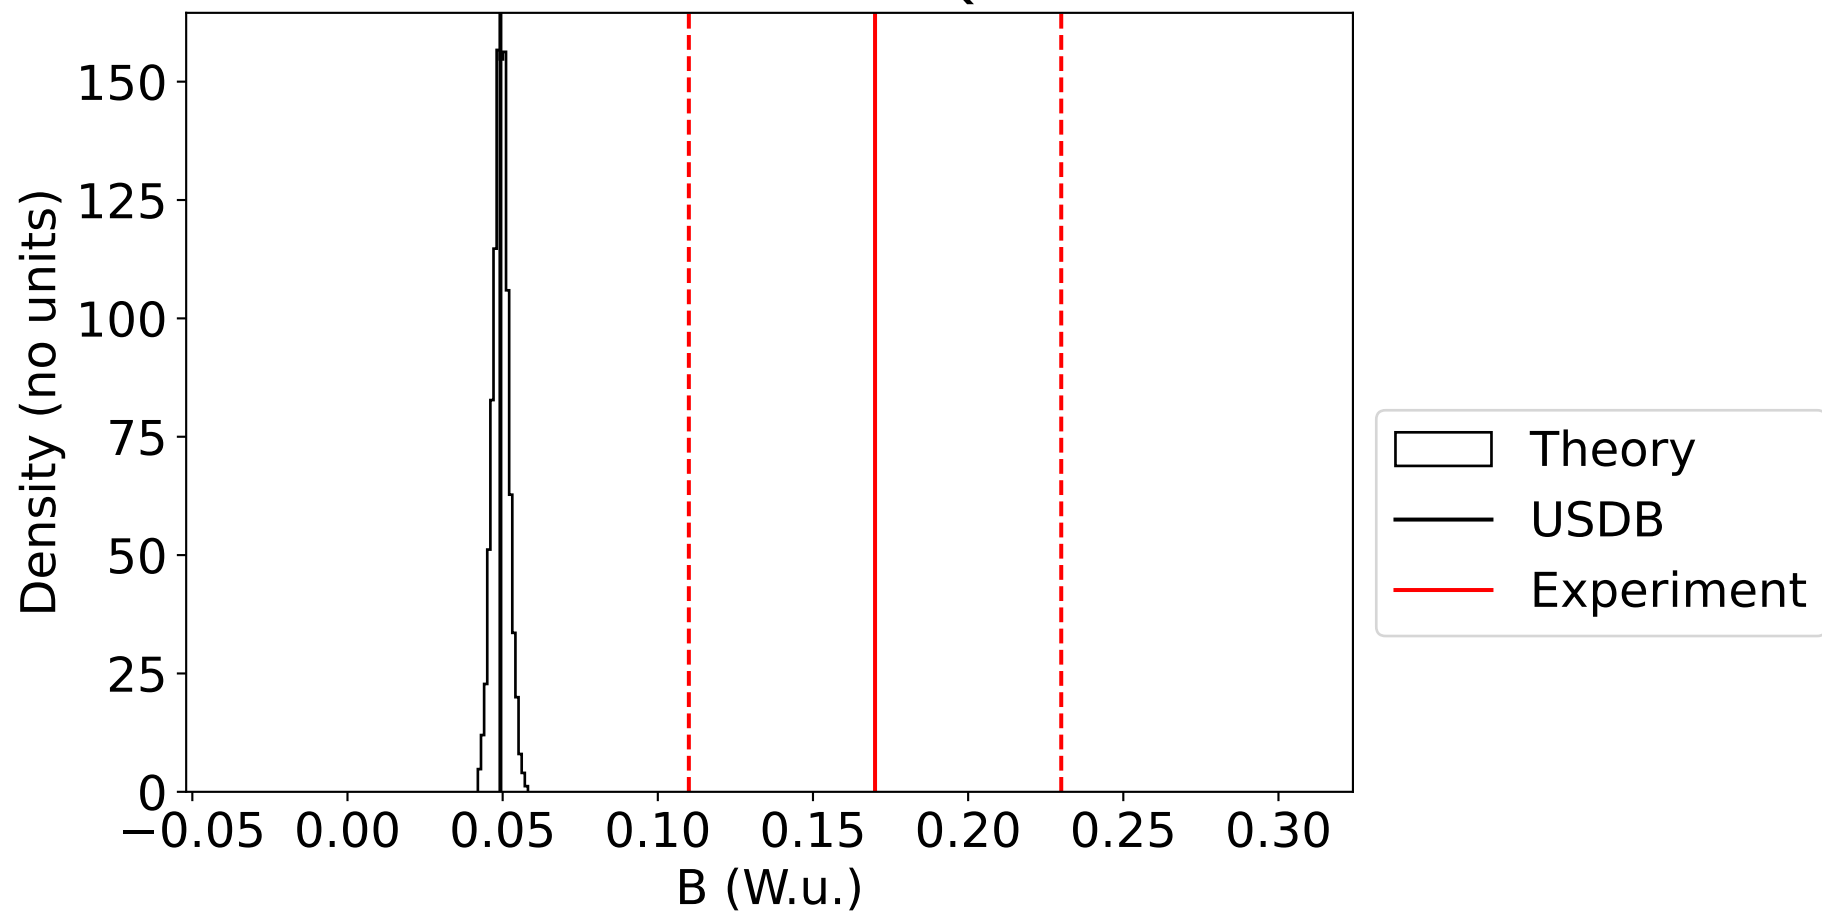

$^{27}\text{Si} (7/2_1) \rightarrow (5/2_1)$   
Included in UQ

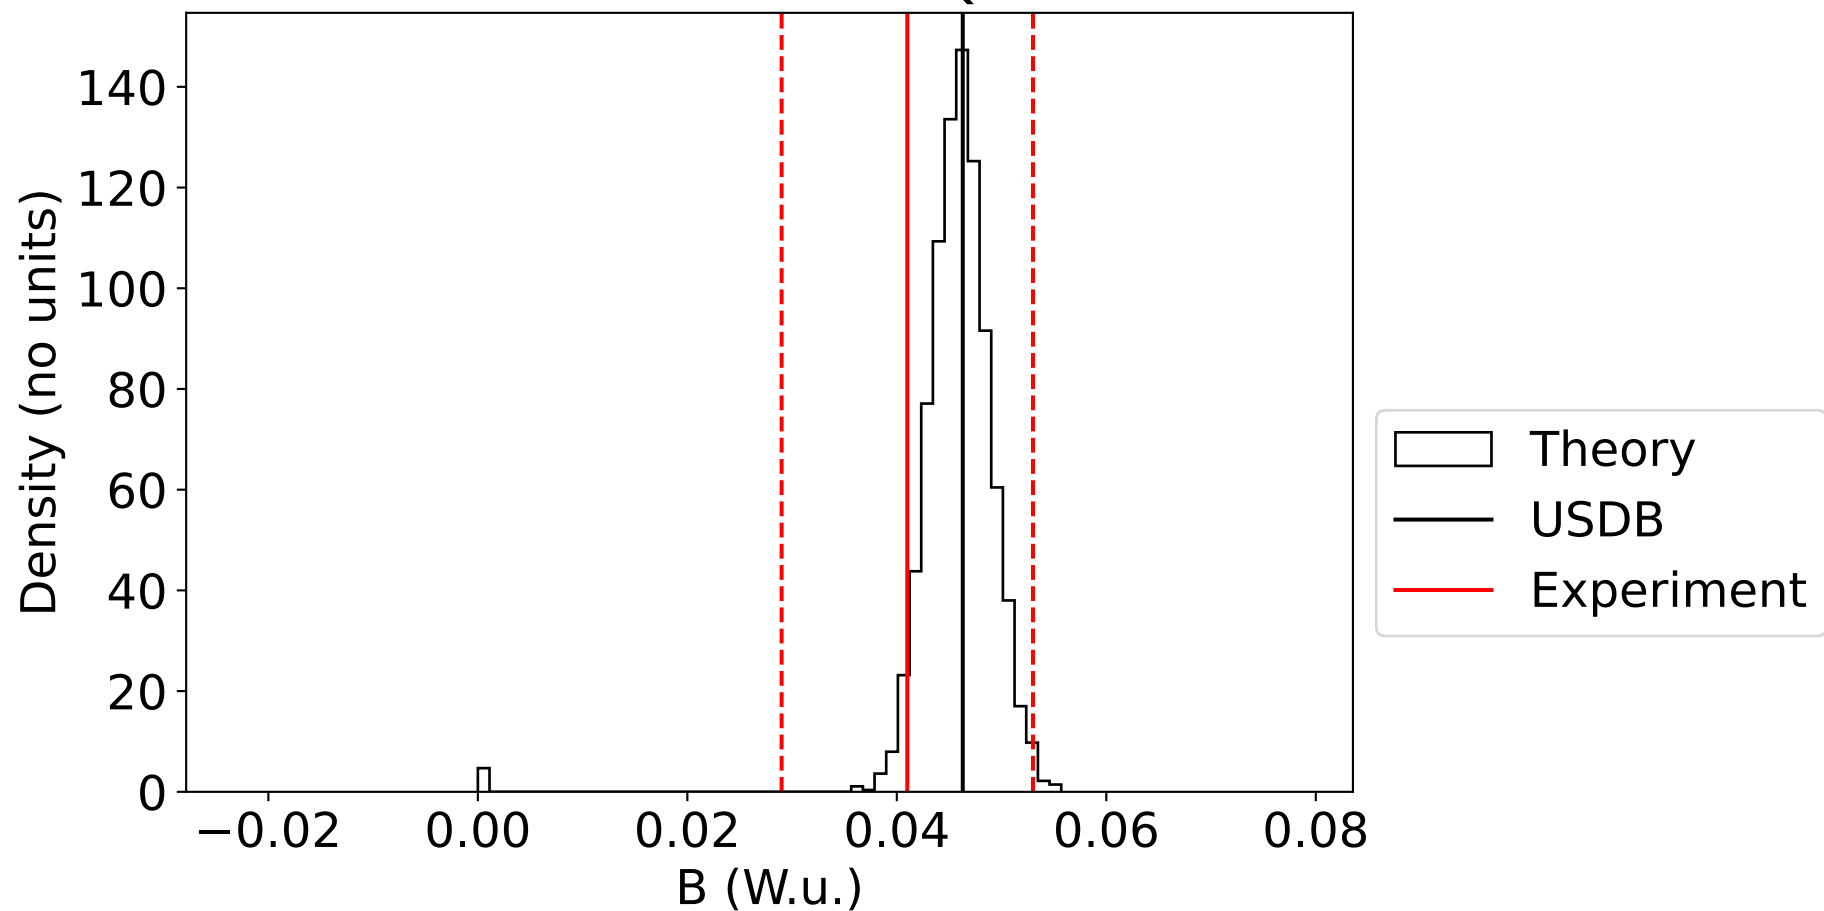

$^{27}\text{Si} (5/2_2) \rightarrow (5/2_1)$   
Included in UQ

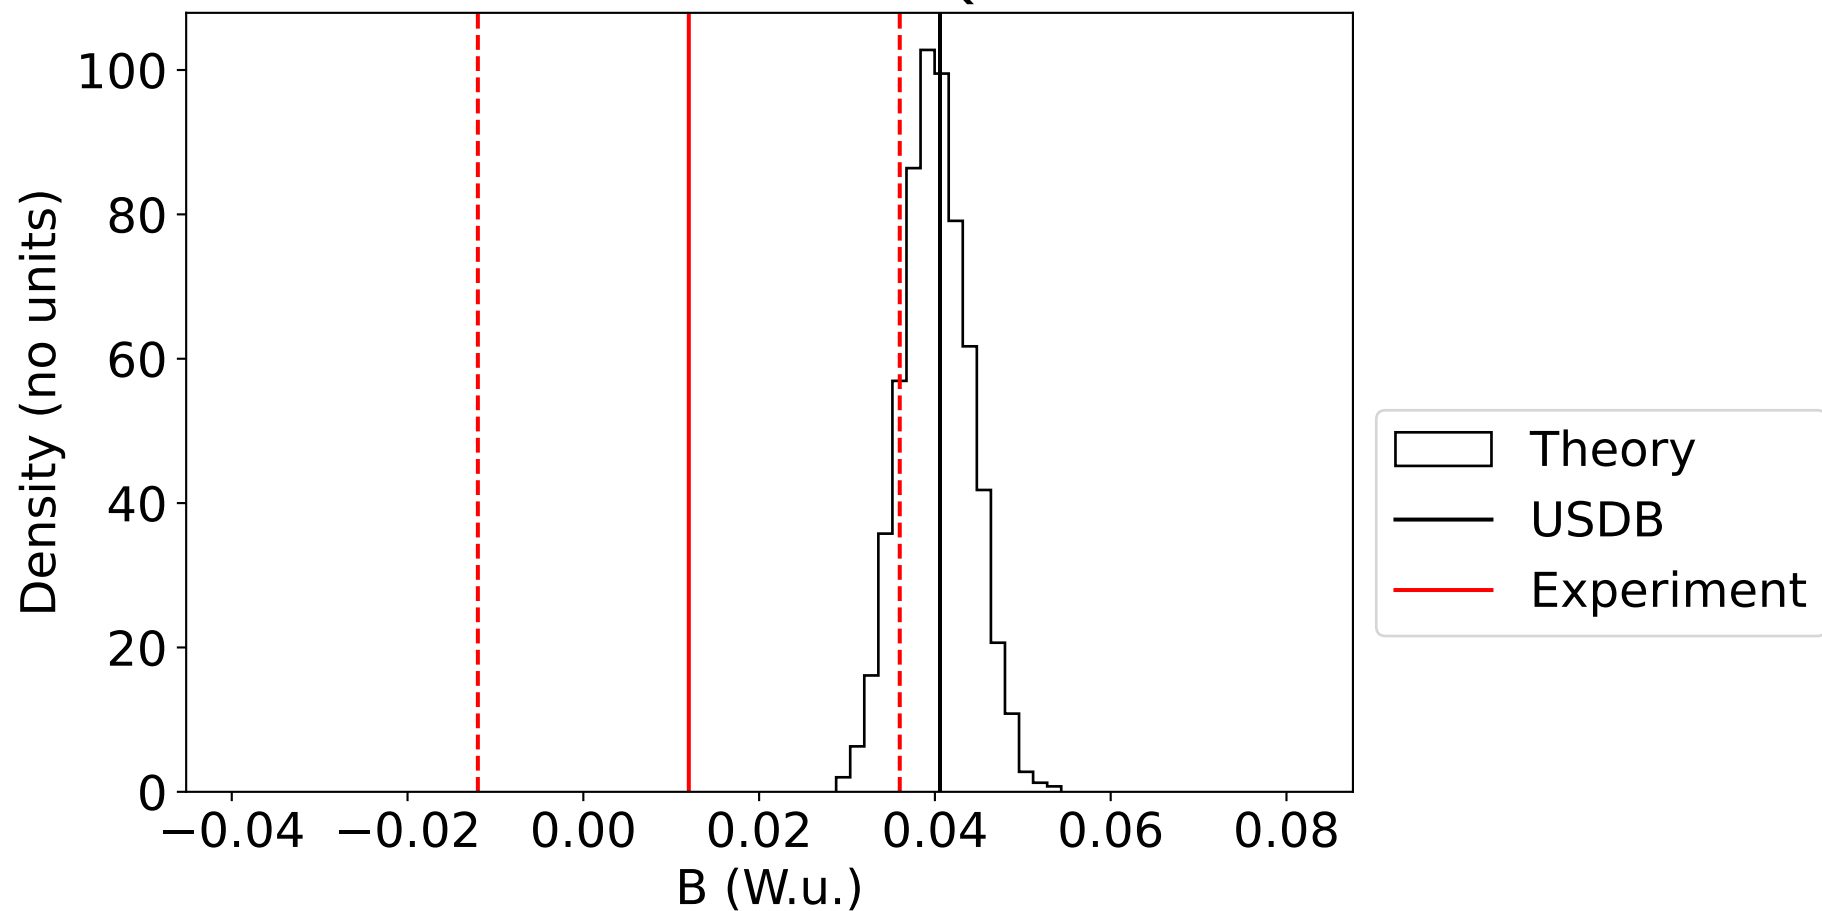

$^{27}\text{Si} (5/2_2) \rightarrow (3/2_1)$   
Included in UQ

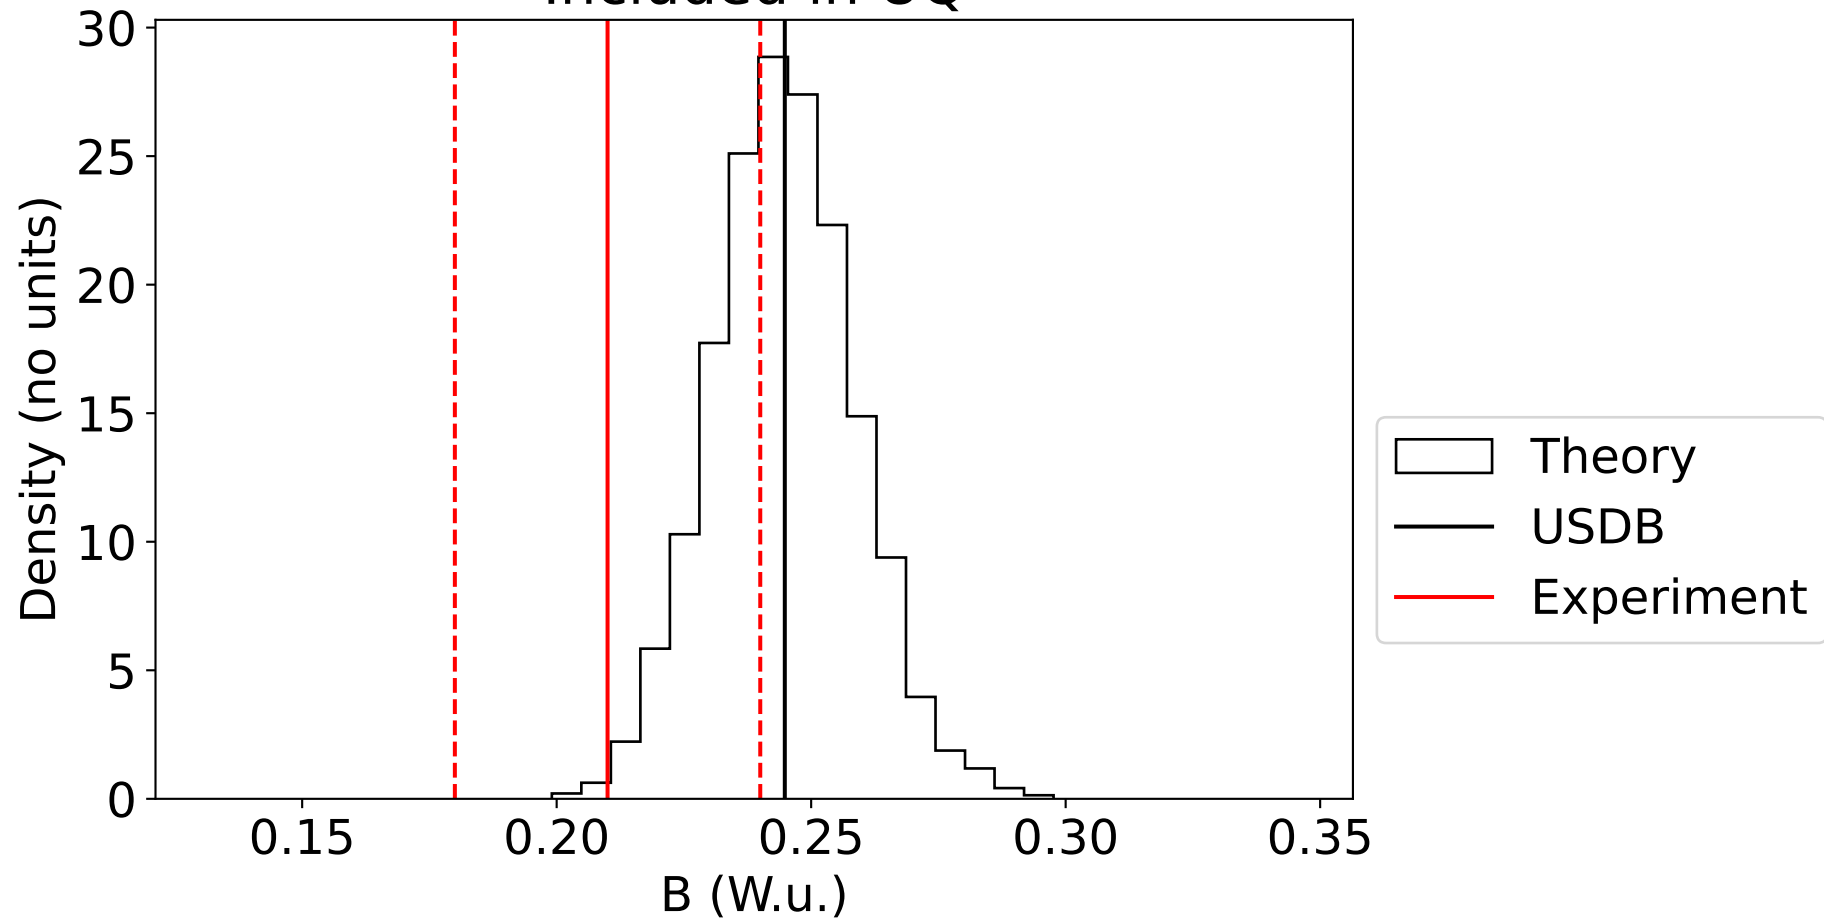

$^{27}\text{Si} (9/2_1) \rightarrow (7/2_1)$   
Included in UQ

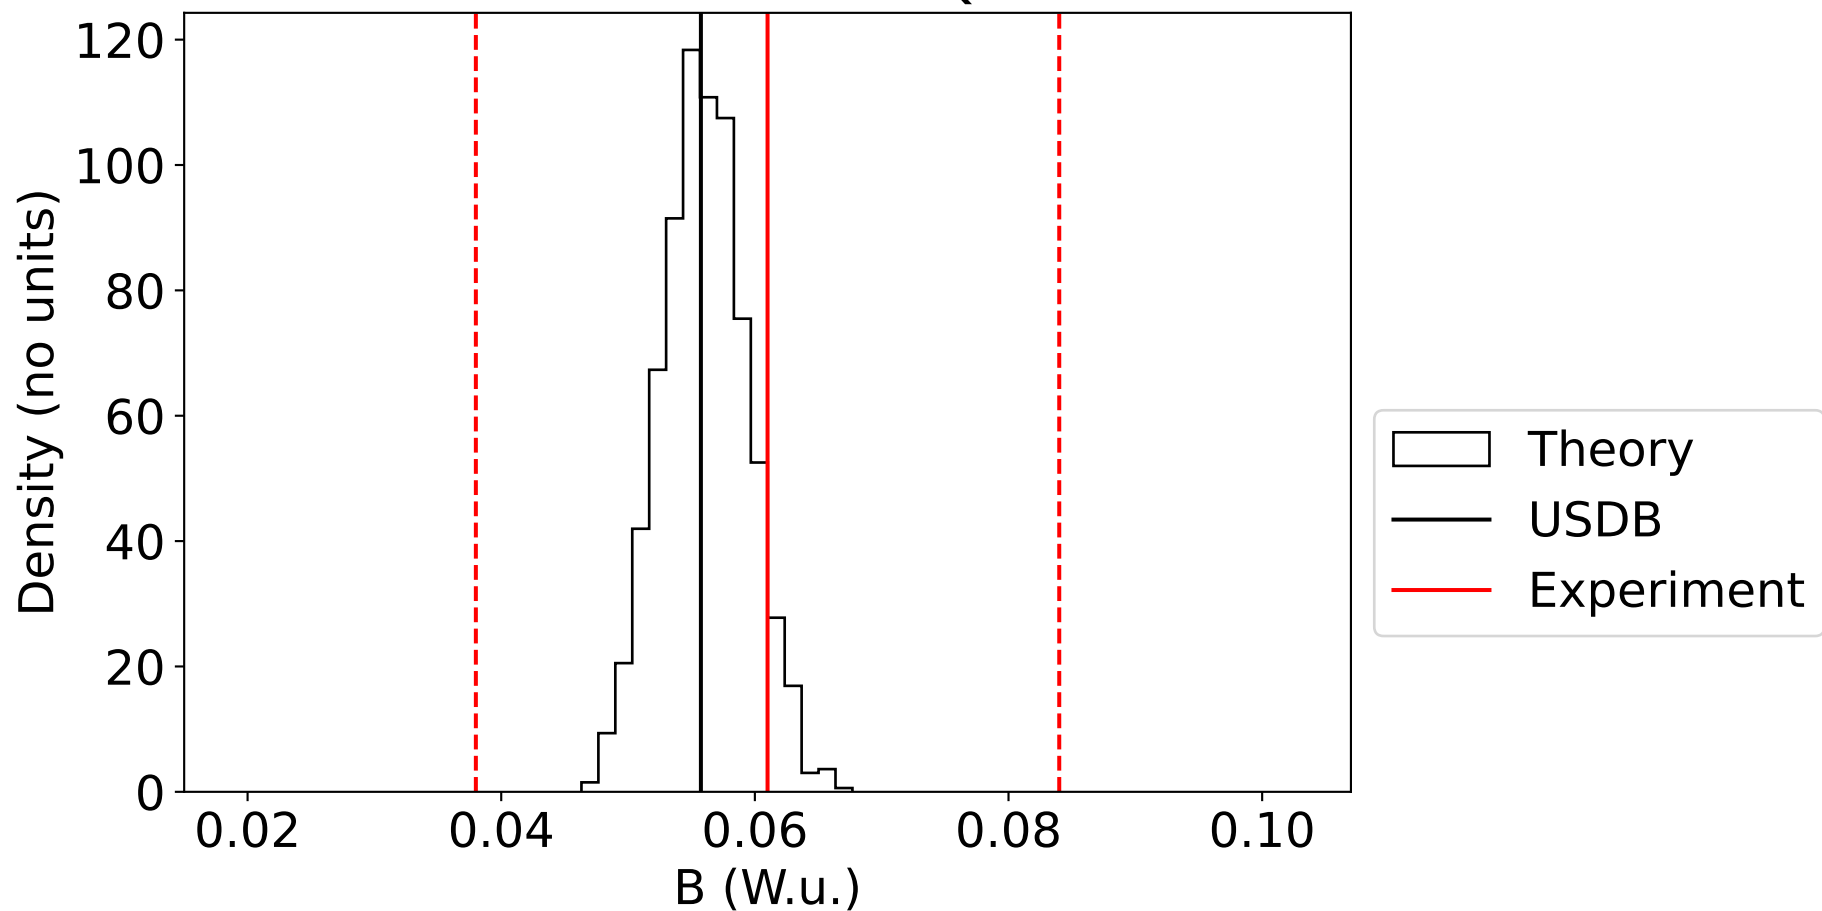

$^{27}\text{Si} (5/2_3) \rightarrow (5/2_1)$   
Included in UQ

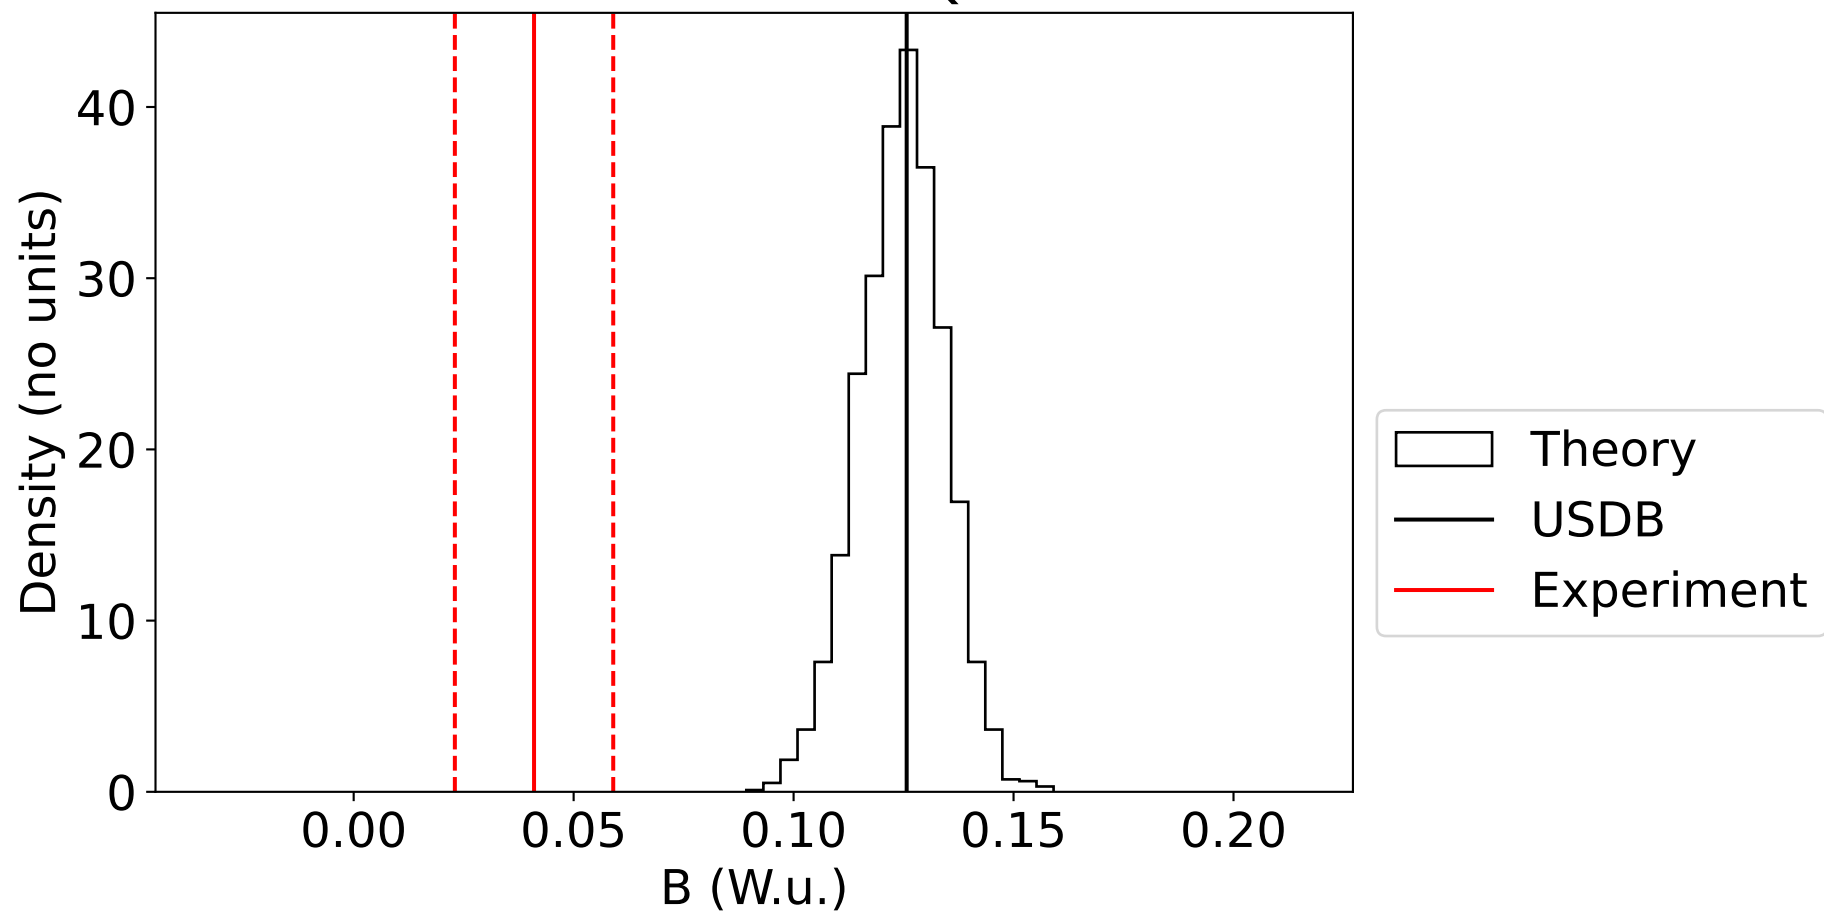

$^{27}\text{Si} (5/2_3) \rightarrow (3/2_1)$   
Included in UQ

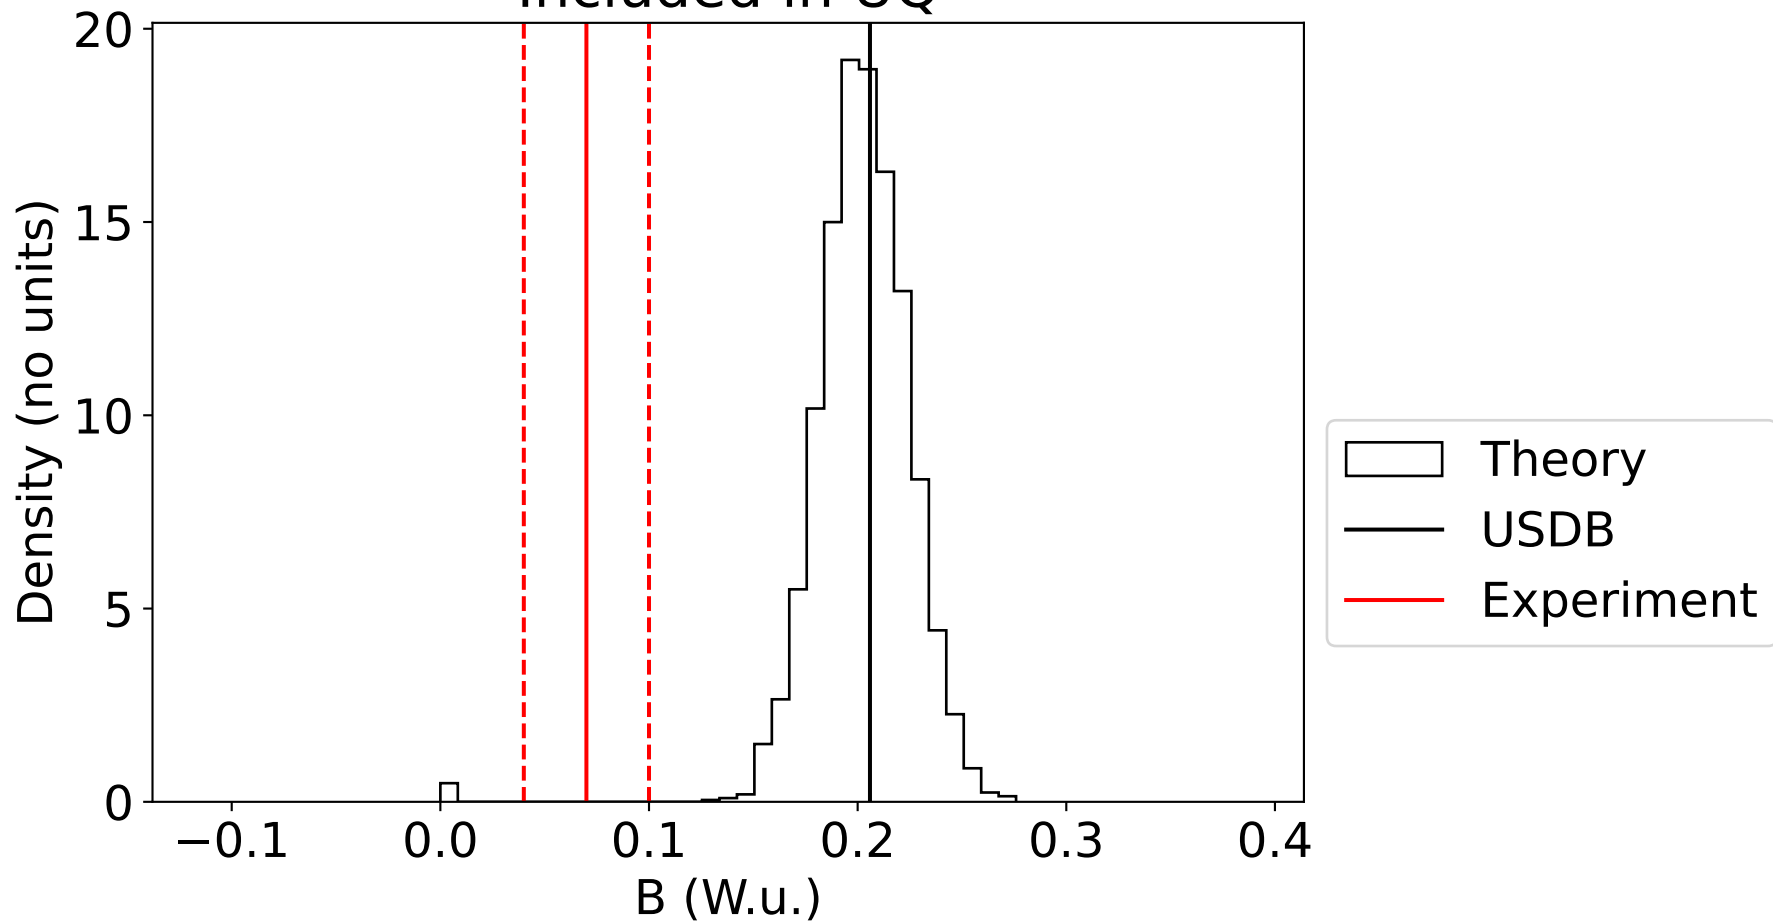

$^{27}\text{Si} (5/2_5) \rightarrow (3/2_1)$   
Included in UQ

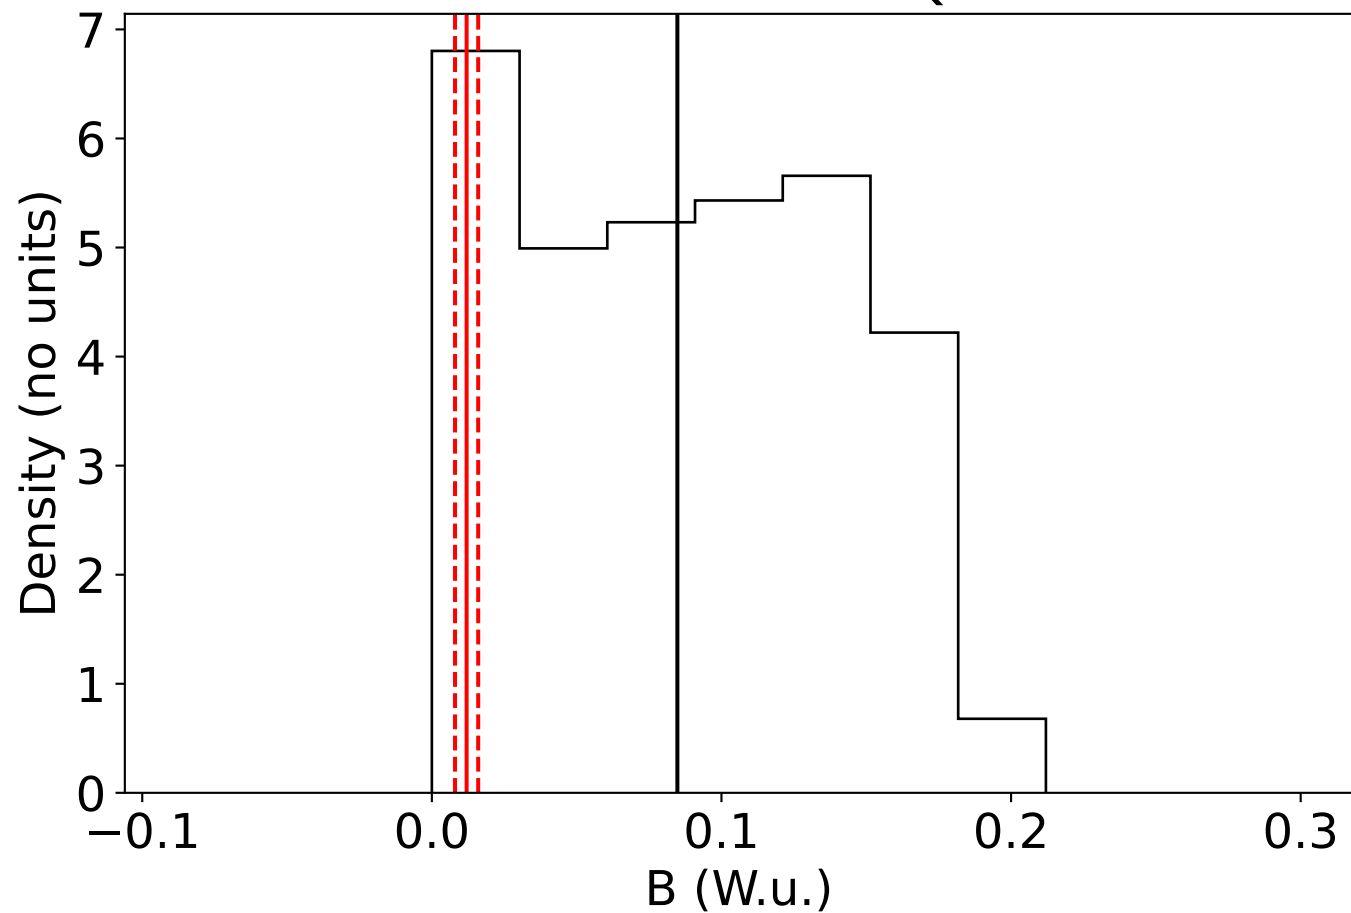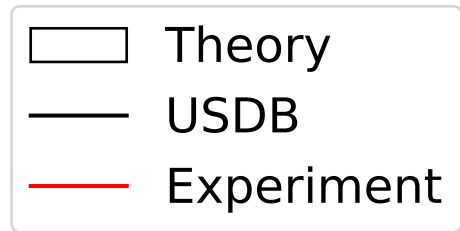



$^{29}\text{Si} (3/2_1) \rightarrow (1/2_1)$   
Included in UQ

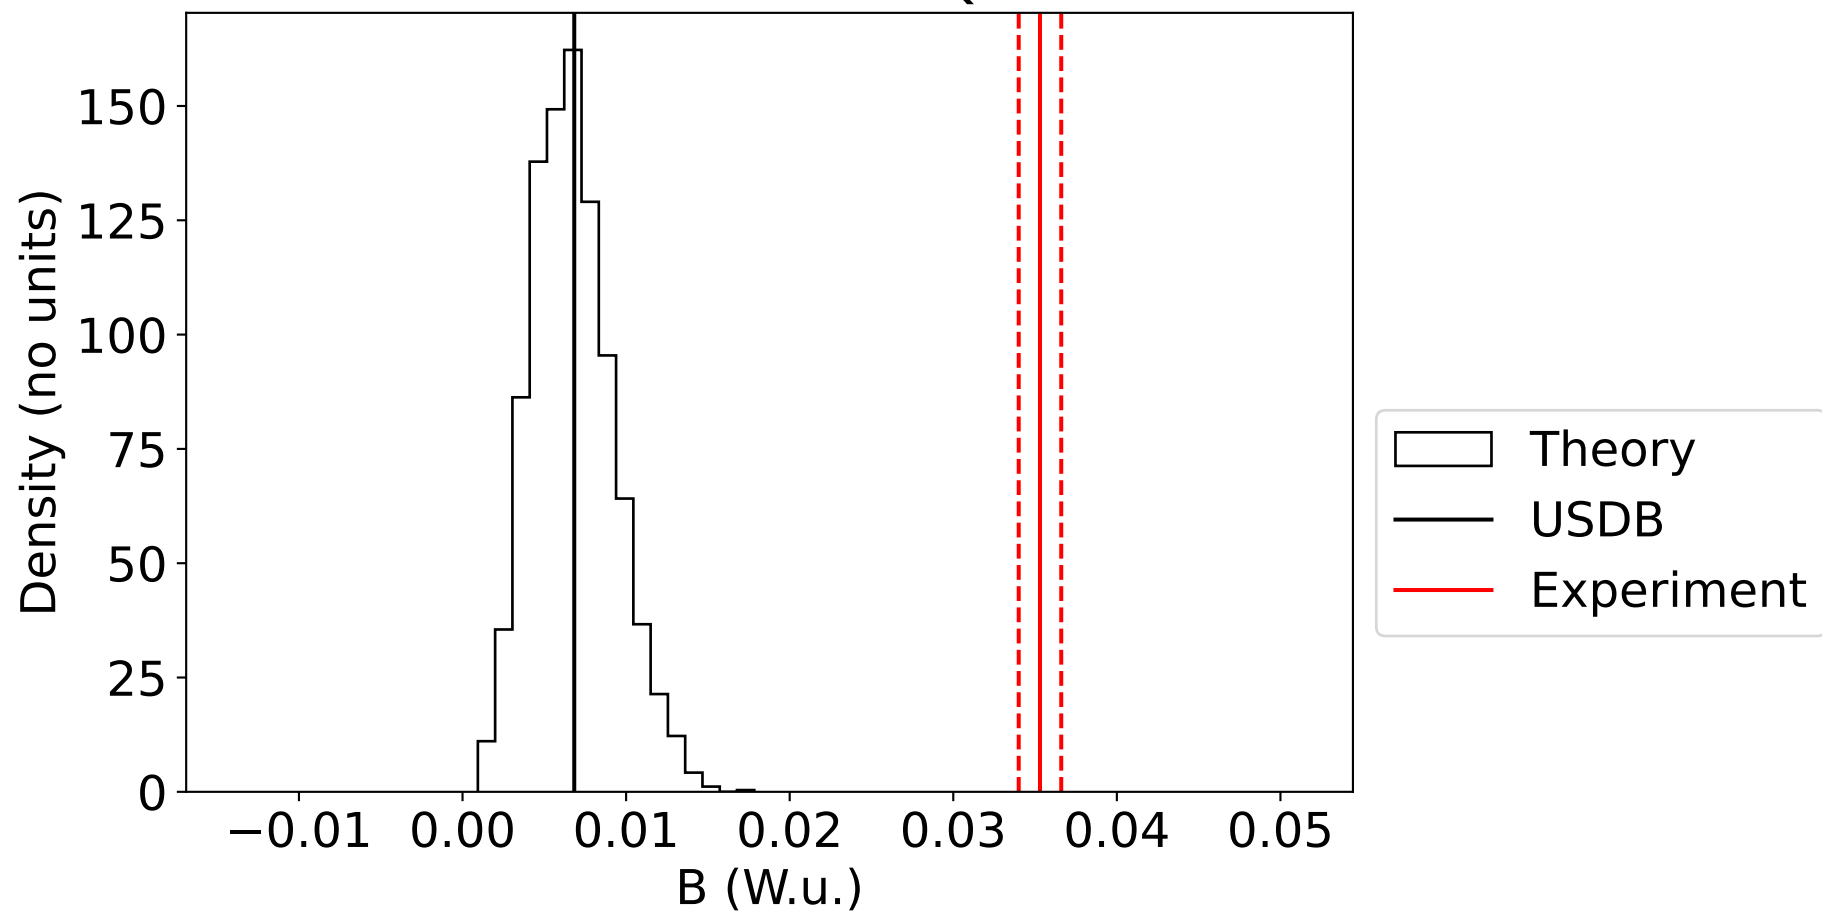

$^{29}\text{Si} (3/2_2) \rightarrow (1/2_1)$   
Included in UQ

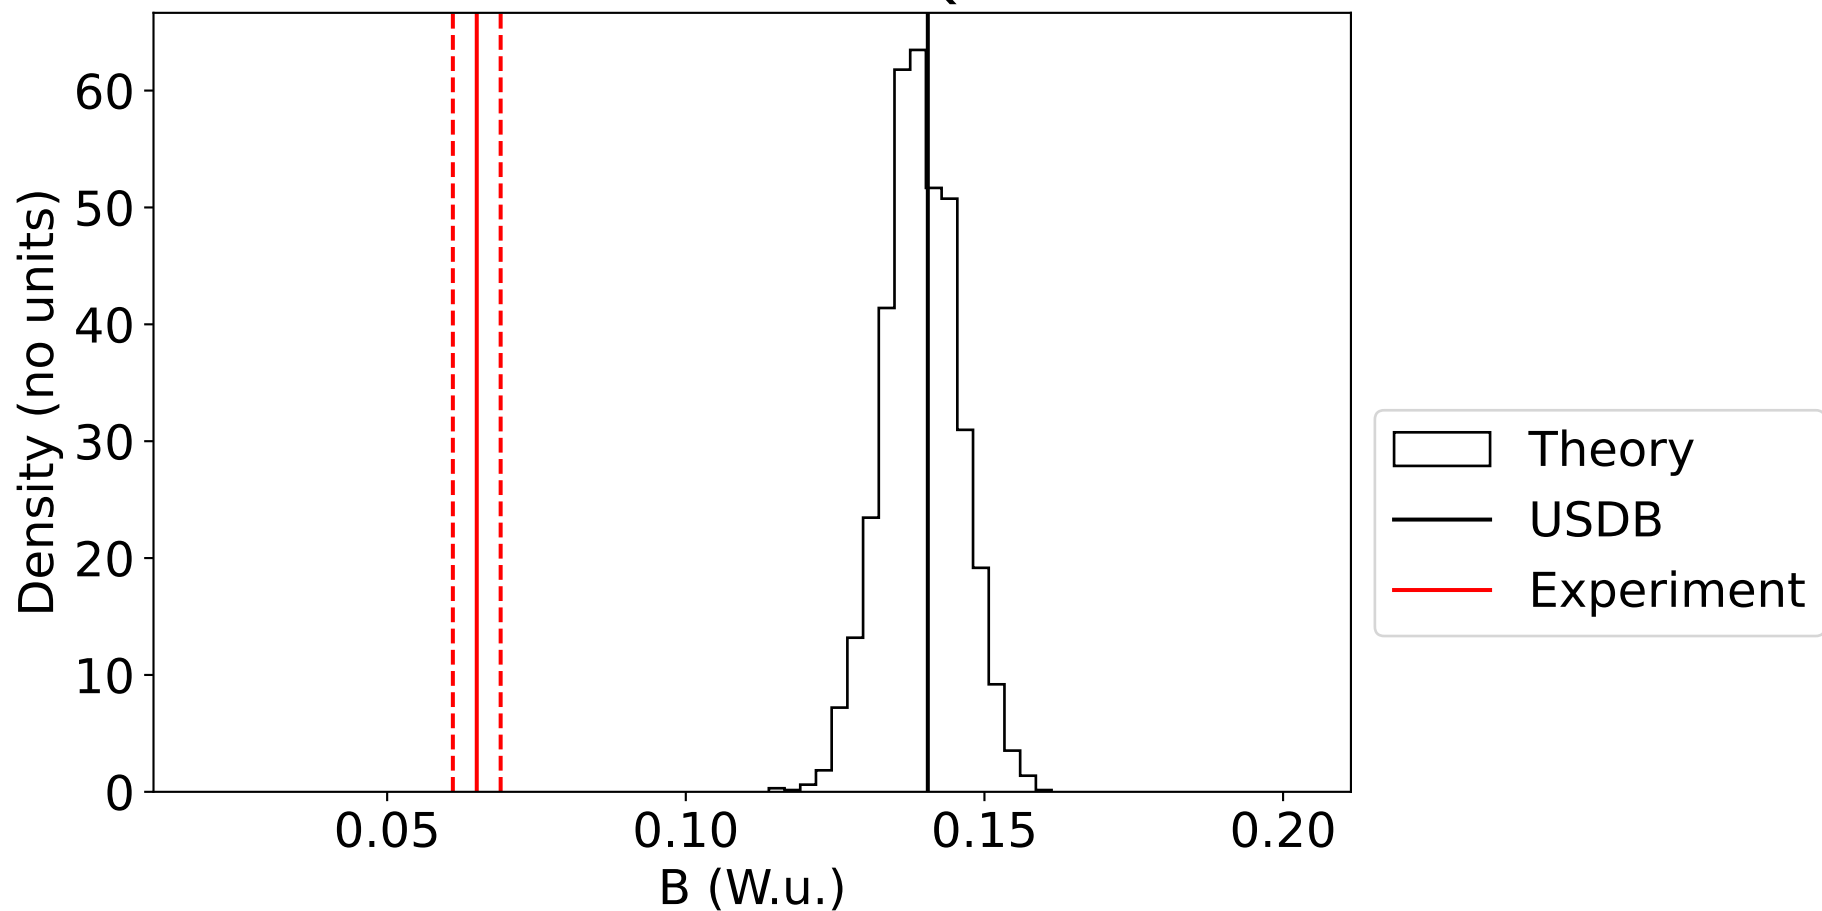

$^{29}\text{Si} (5/2_2) \rightarrow (3/2_1)$   
Included in UQ

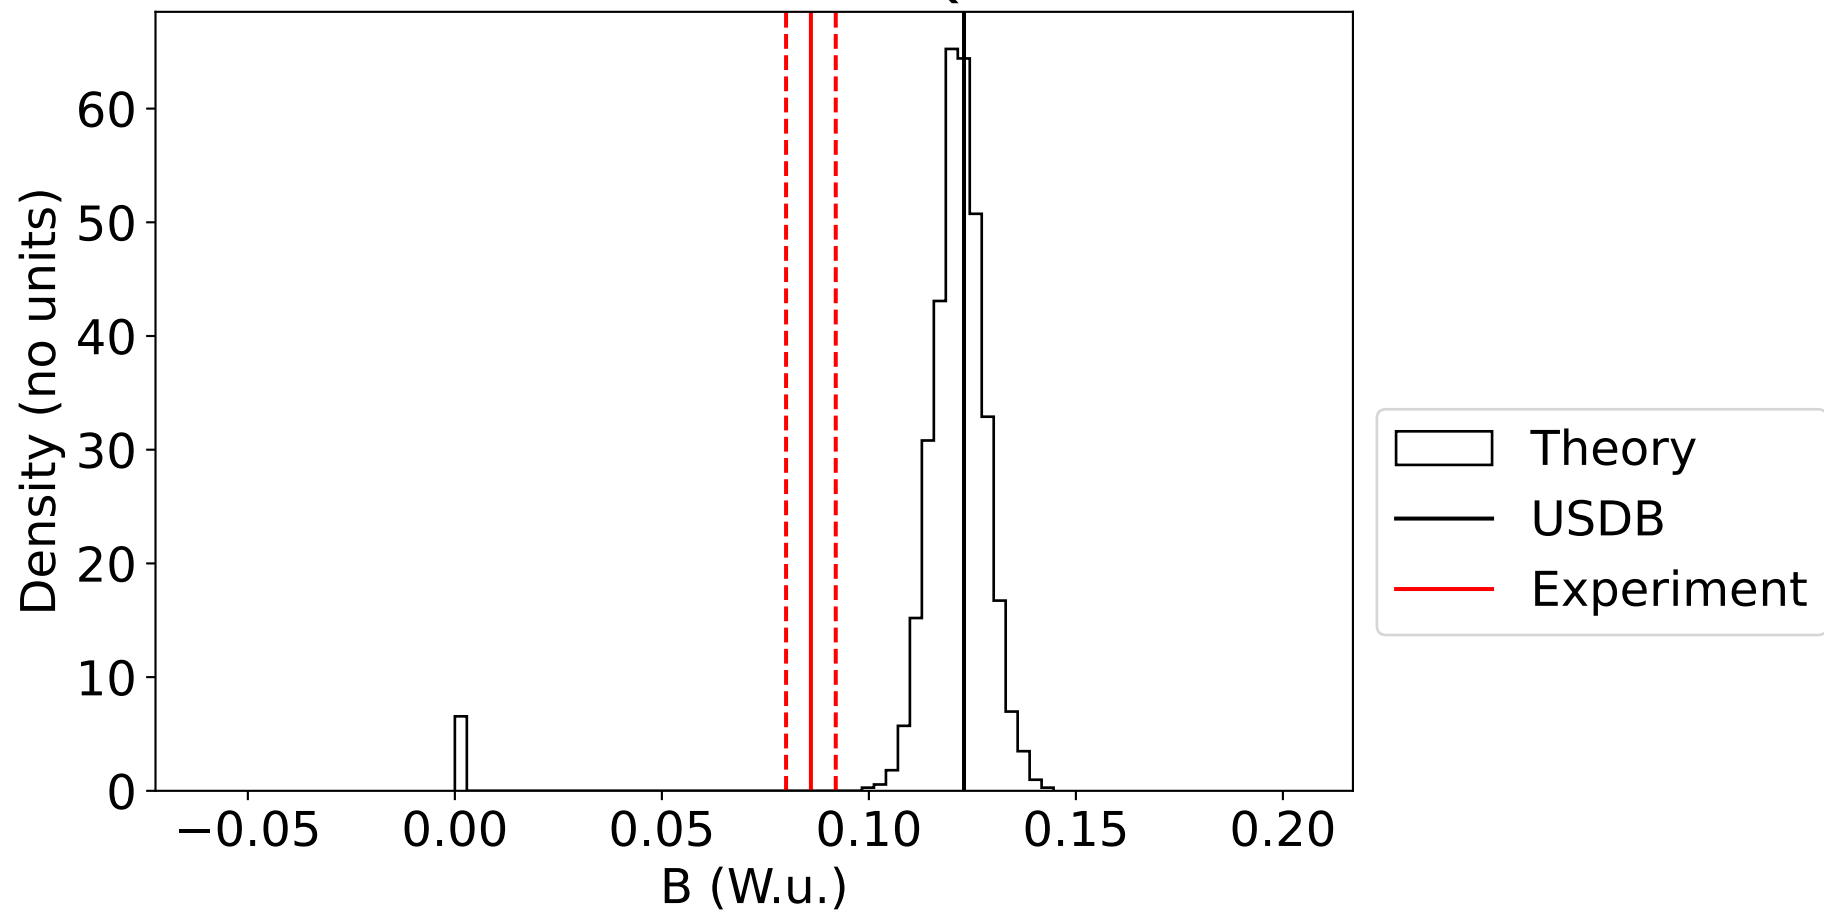

$^{29}\text{Si} (5/2_2) \rightarrow (5/2_1)$   
Included in UQ

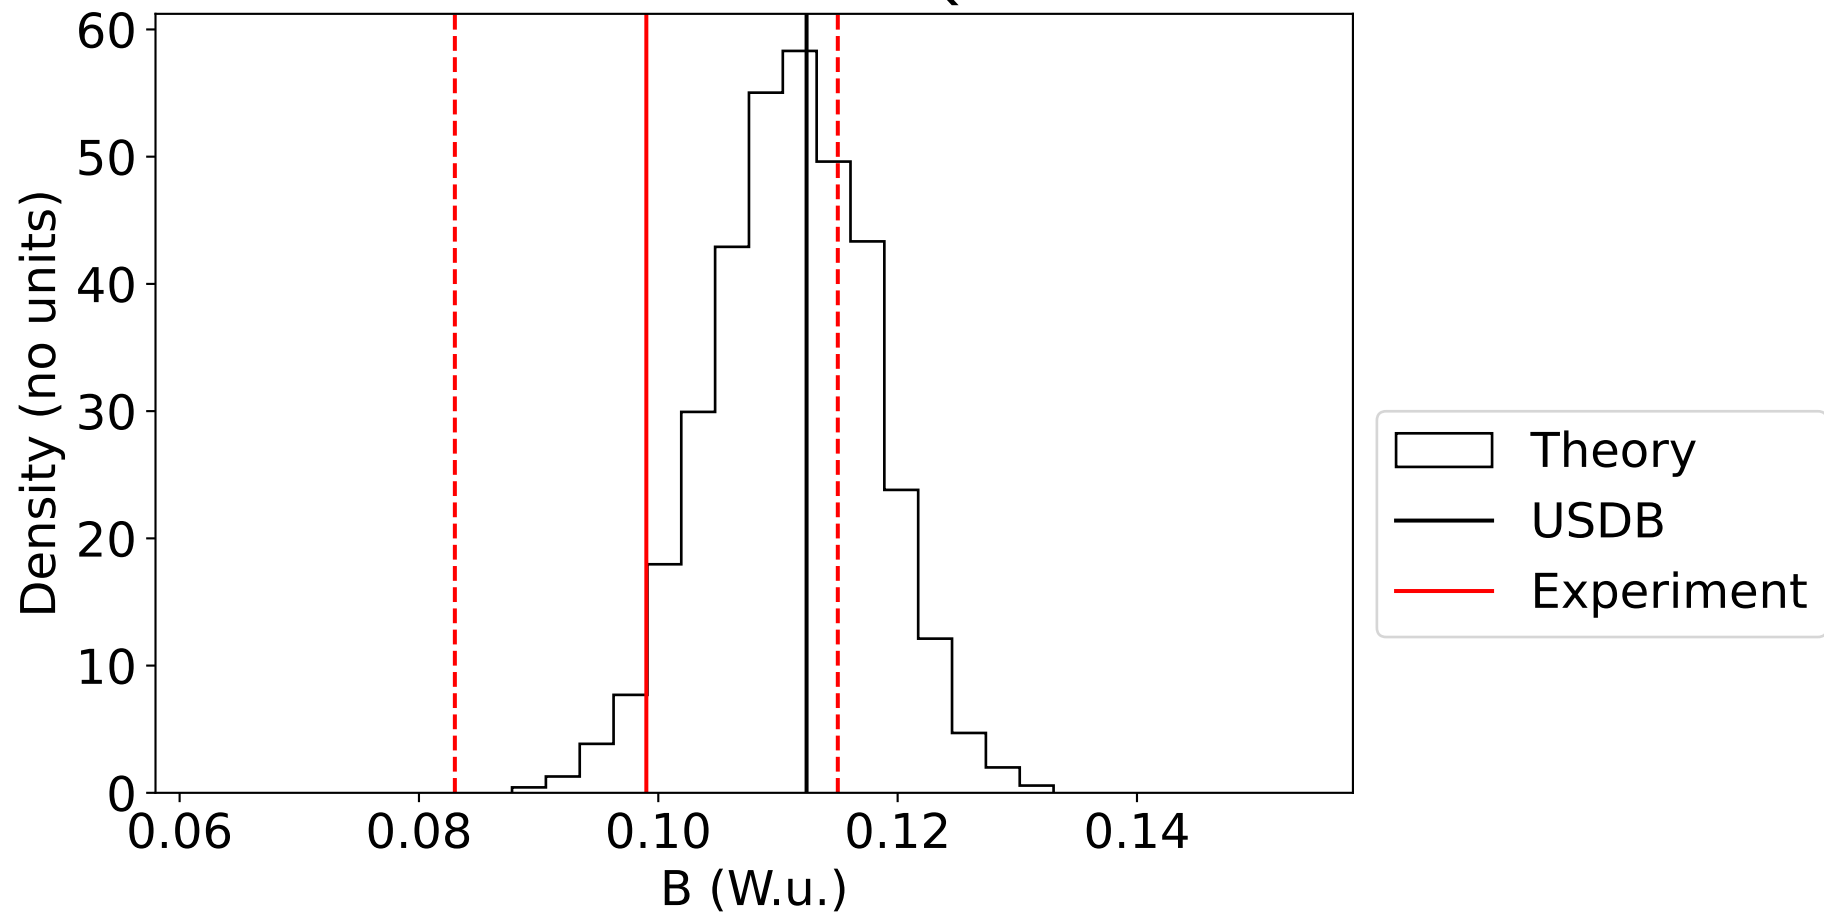

$^{29}\text{Si} (7/2_1) \rightarrow (5/2_1)$   
Included in UQ

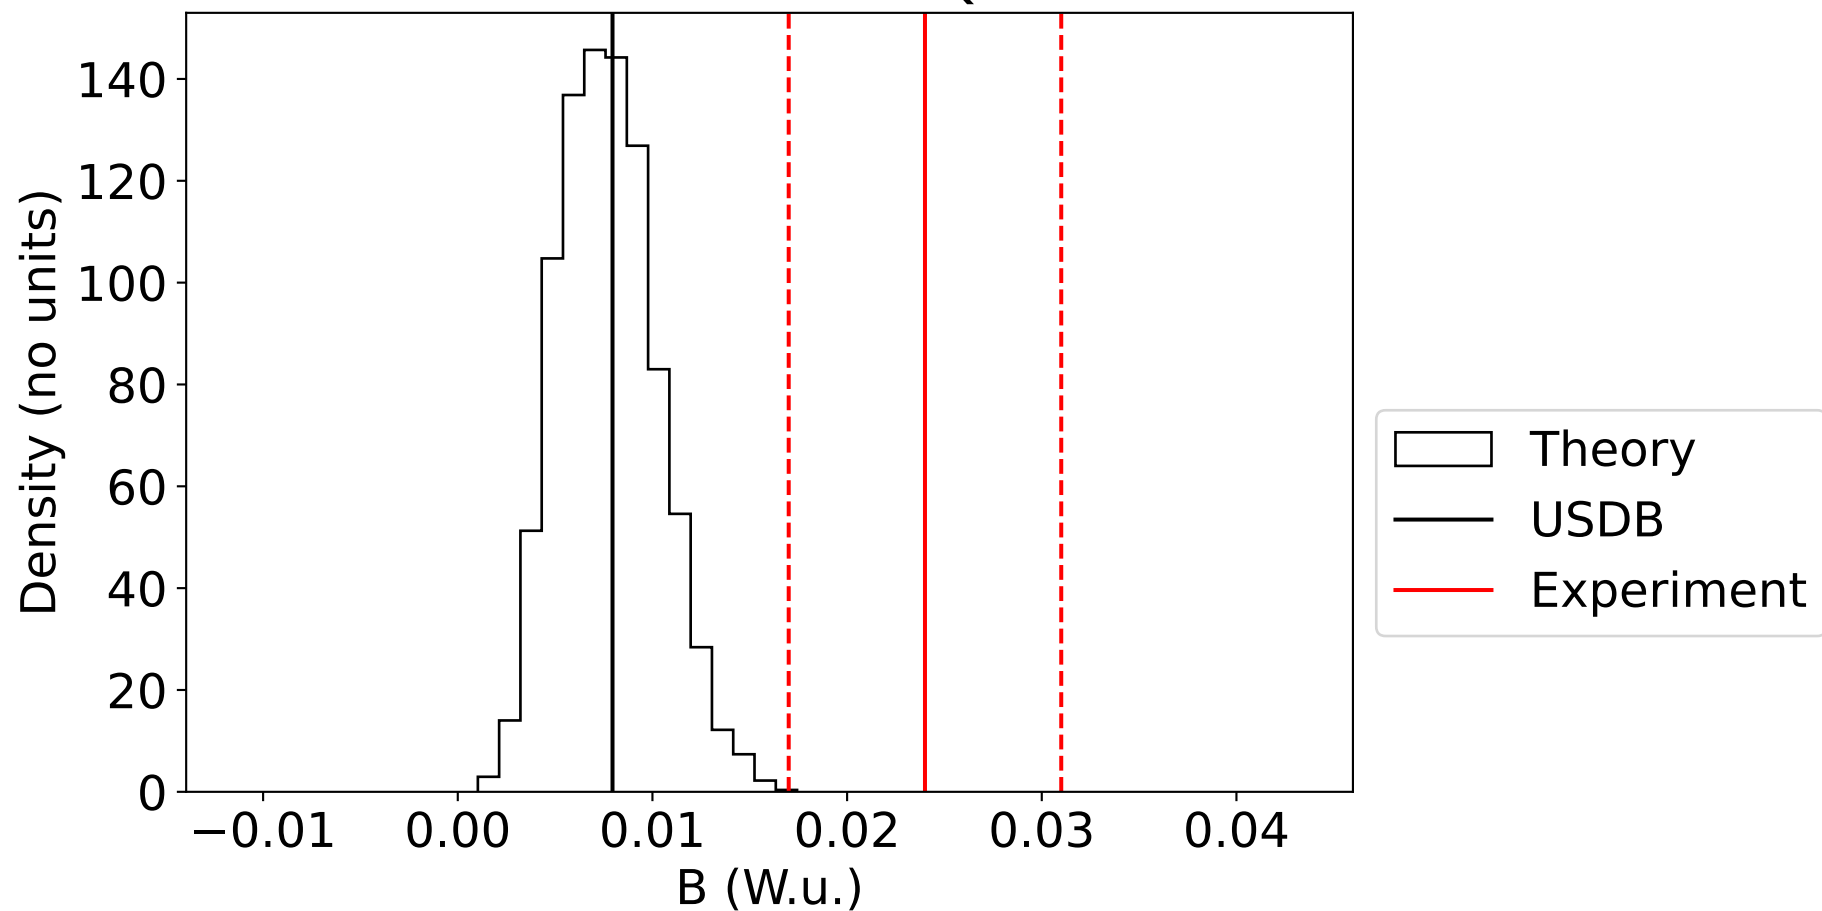

$^{29}\text{Si} (5/2_3) \rightarrow (3/2_1)$   
Included in UQ

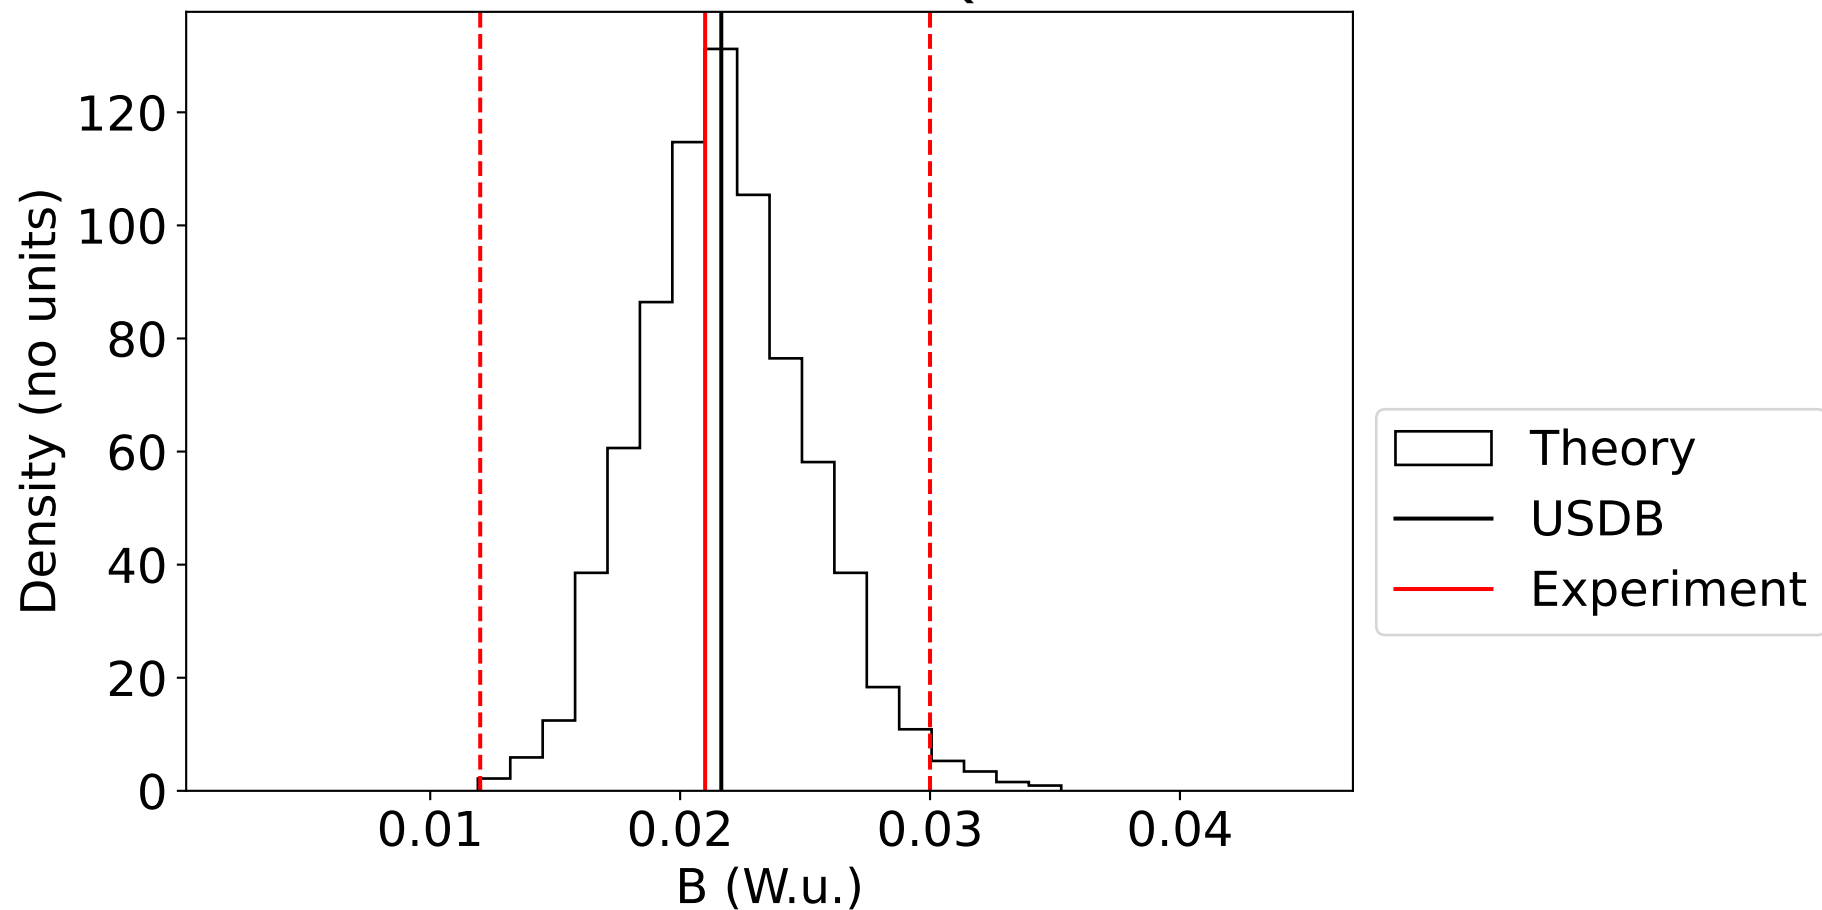

$^{29}\text{Si} (7/2_2) \rightarrow (5/2_1)$   
Included in UQ

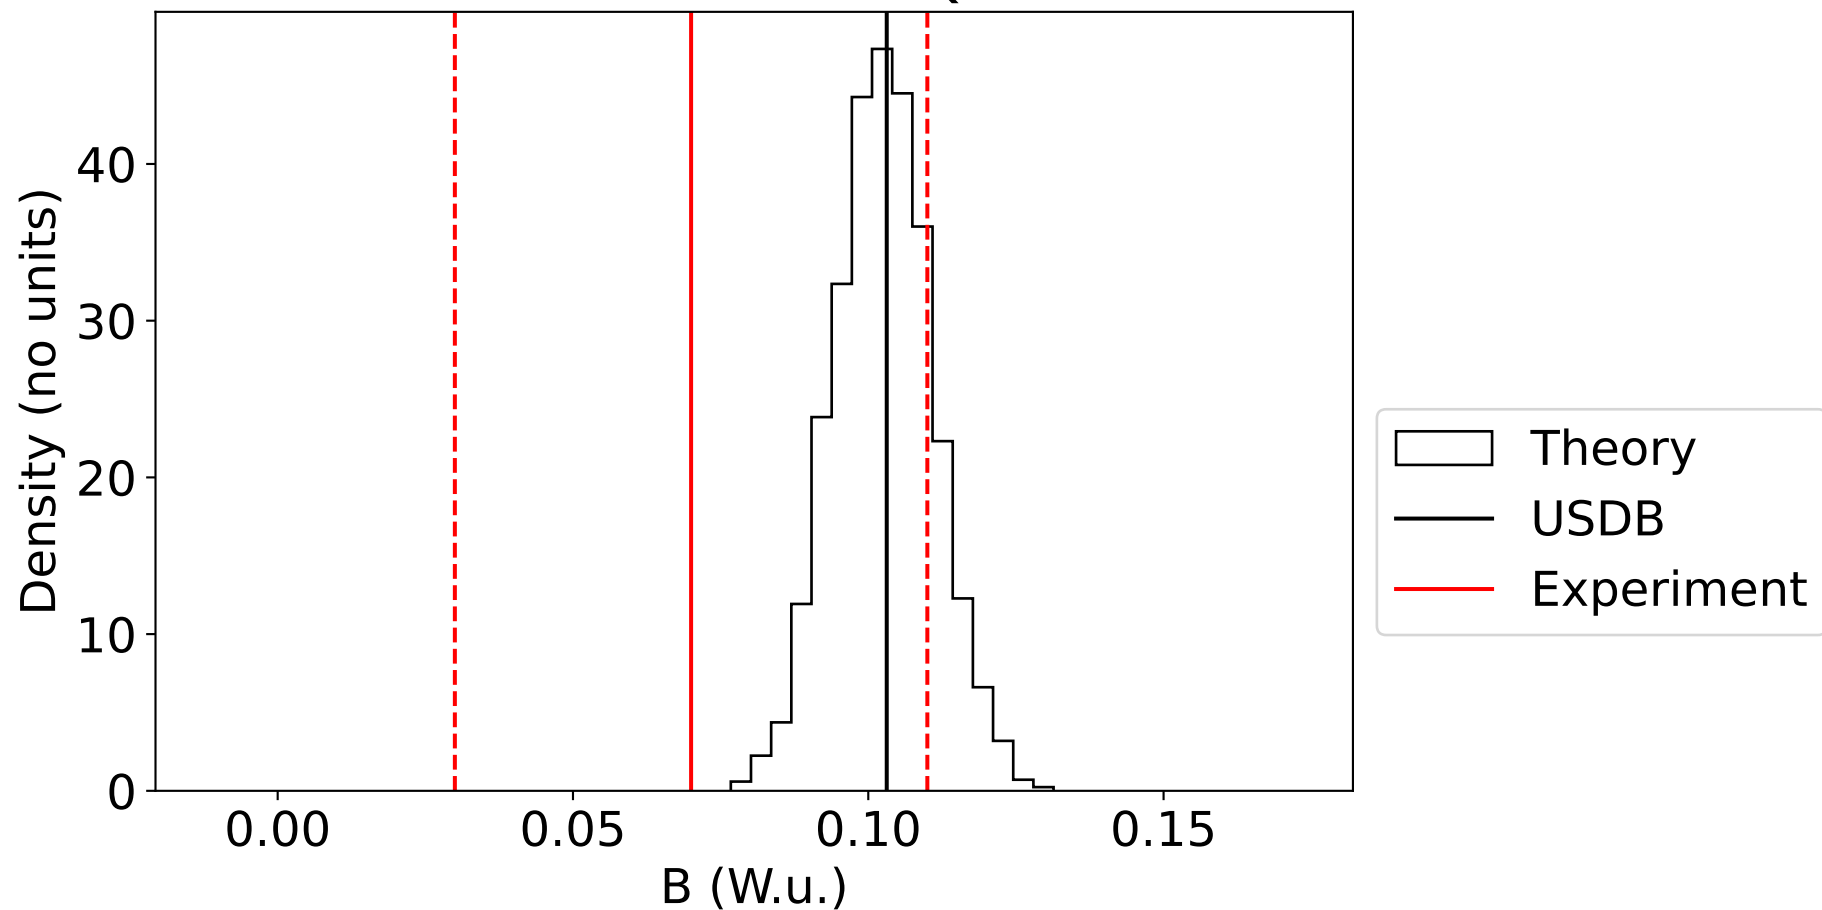

$^{29}\text{Si} (9/2_2) \rightarrow (7/2_1)$   
Included in UQ

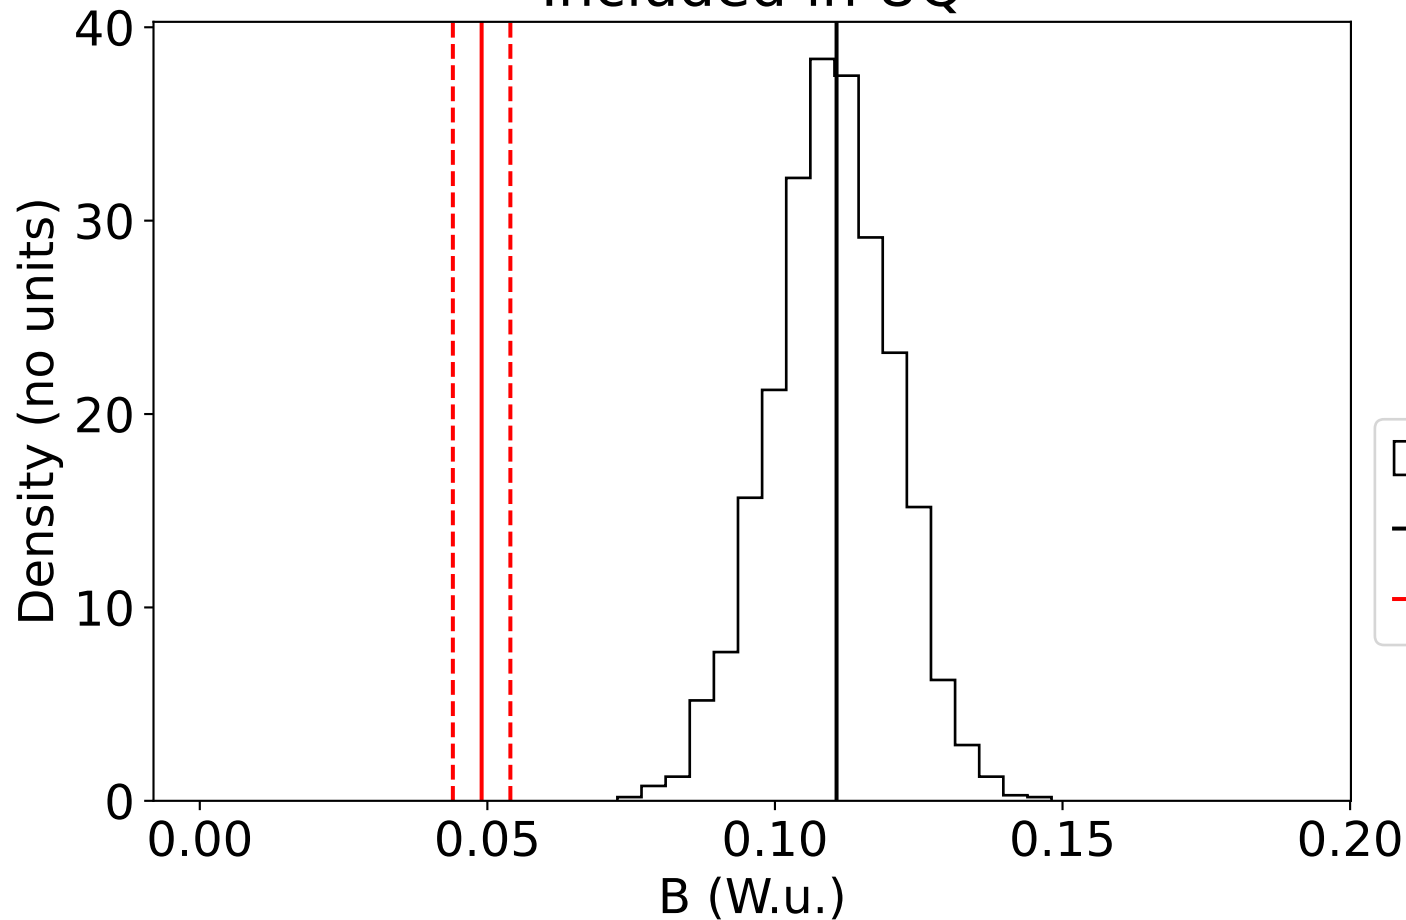



$^{29}\text{Si} (7/2_3) \rightarrow (5/2_2)$   
Included in UQ

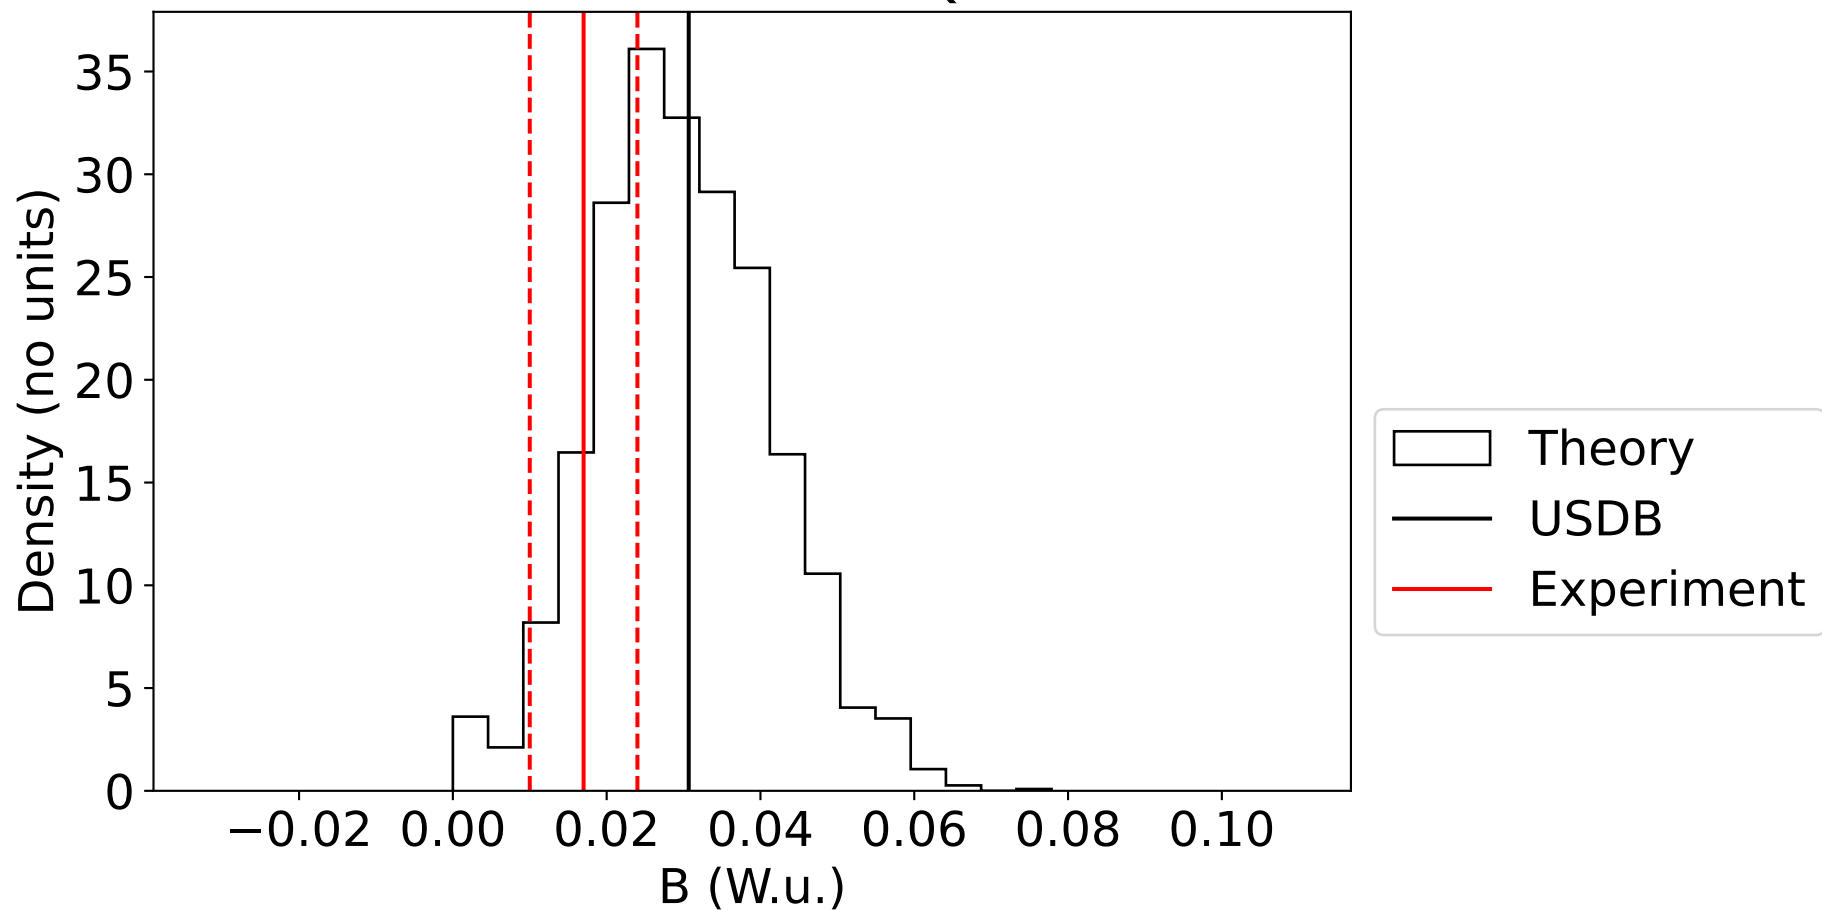

$^{29}\text{Si} (11/2_1) \rightarrow (9/2_2)$   
Included in UQ

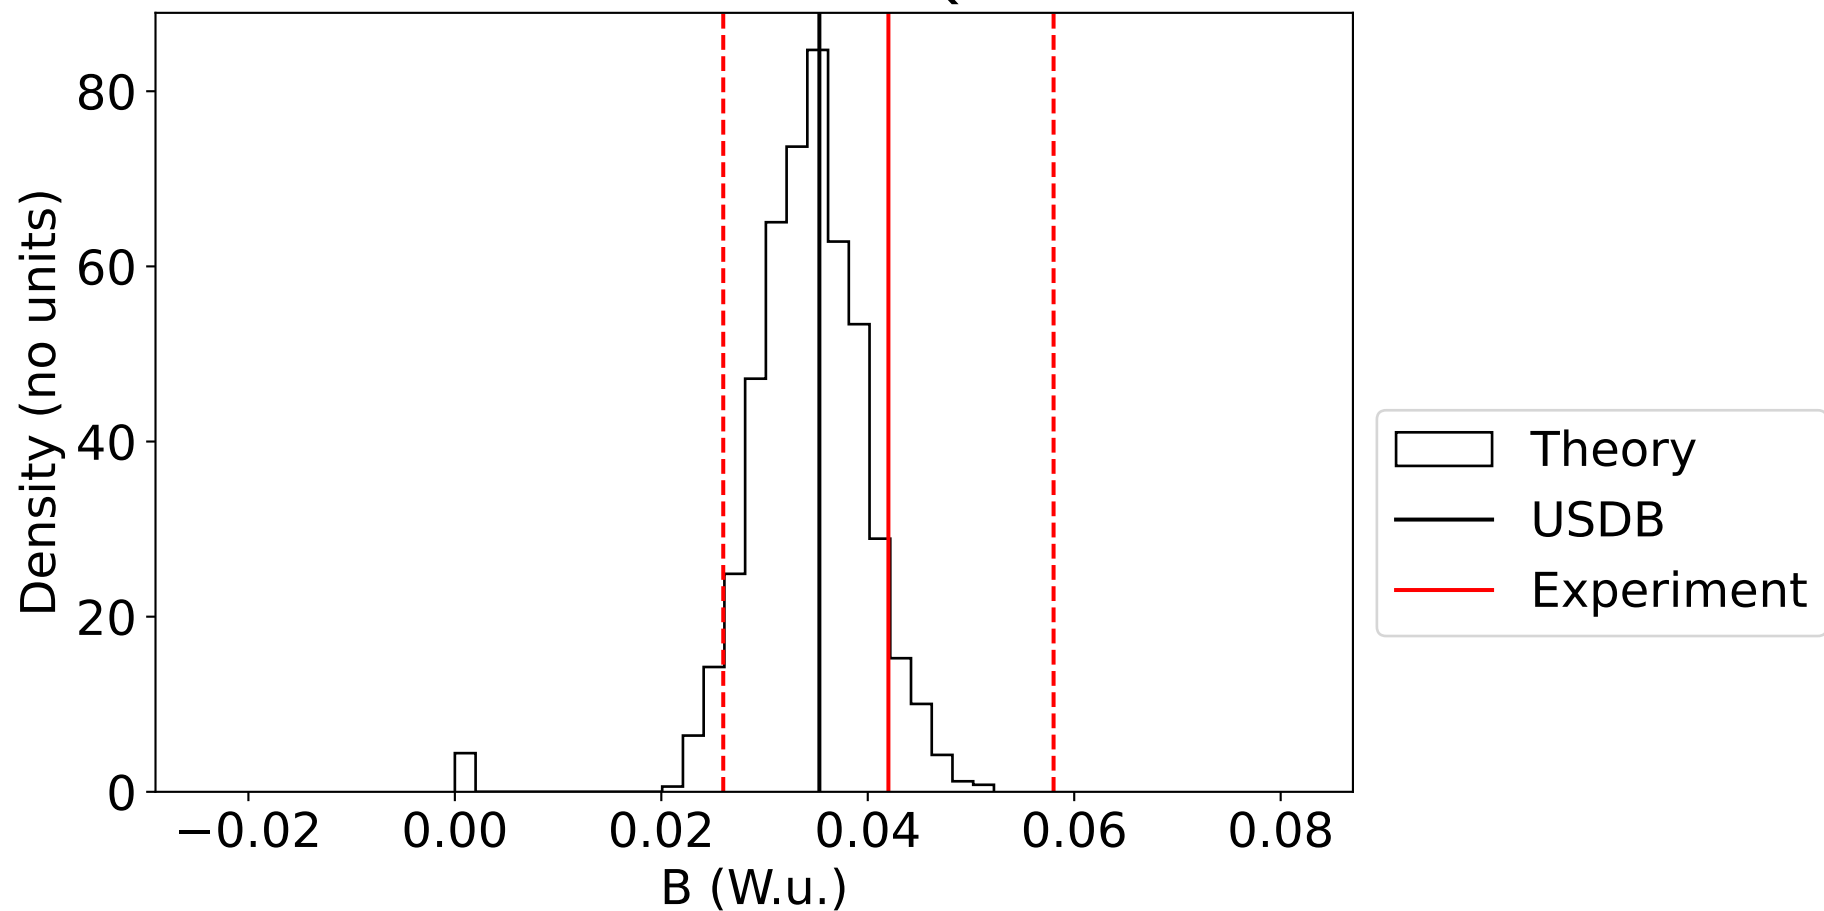

$^{30}\text{Si} (2_2) \rightarrow (2_1)$   
Included in UQ

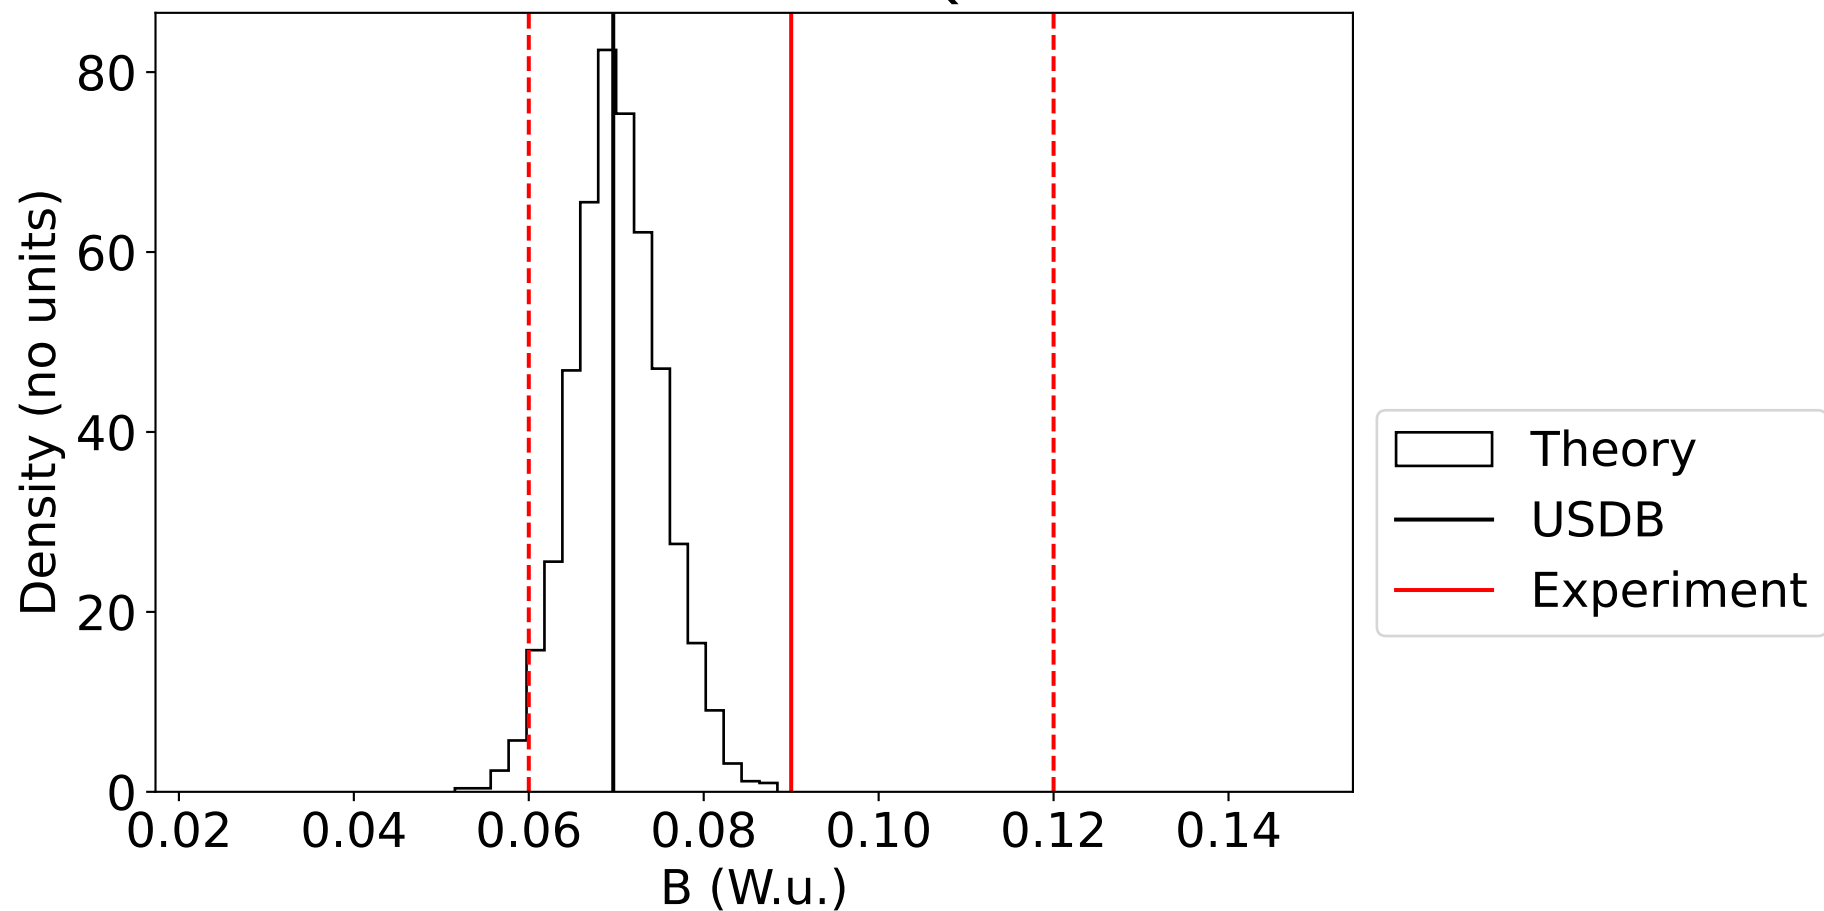

$^{30}\text{Si} (1_1) \rightarrow (2_1)$   
Included in UQ

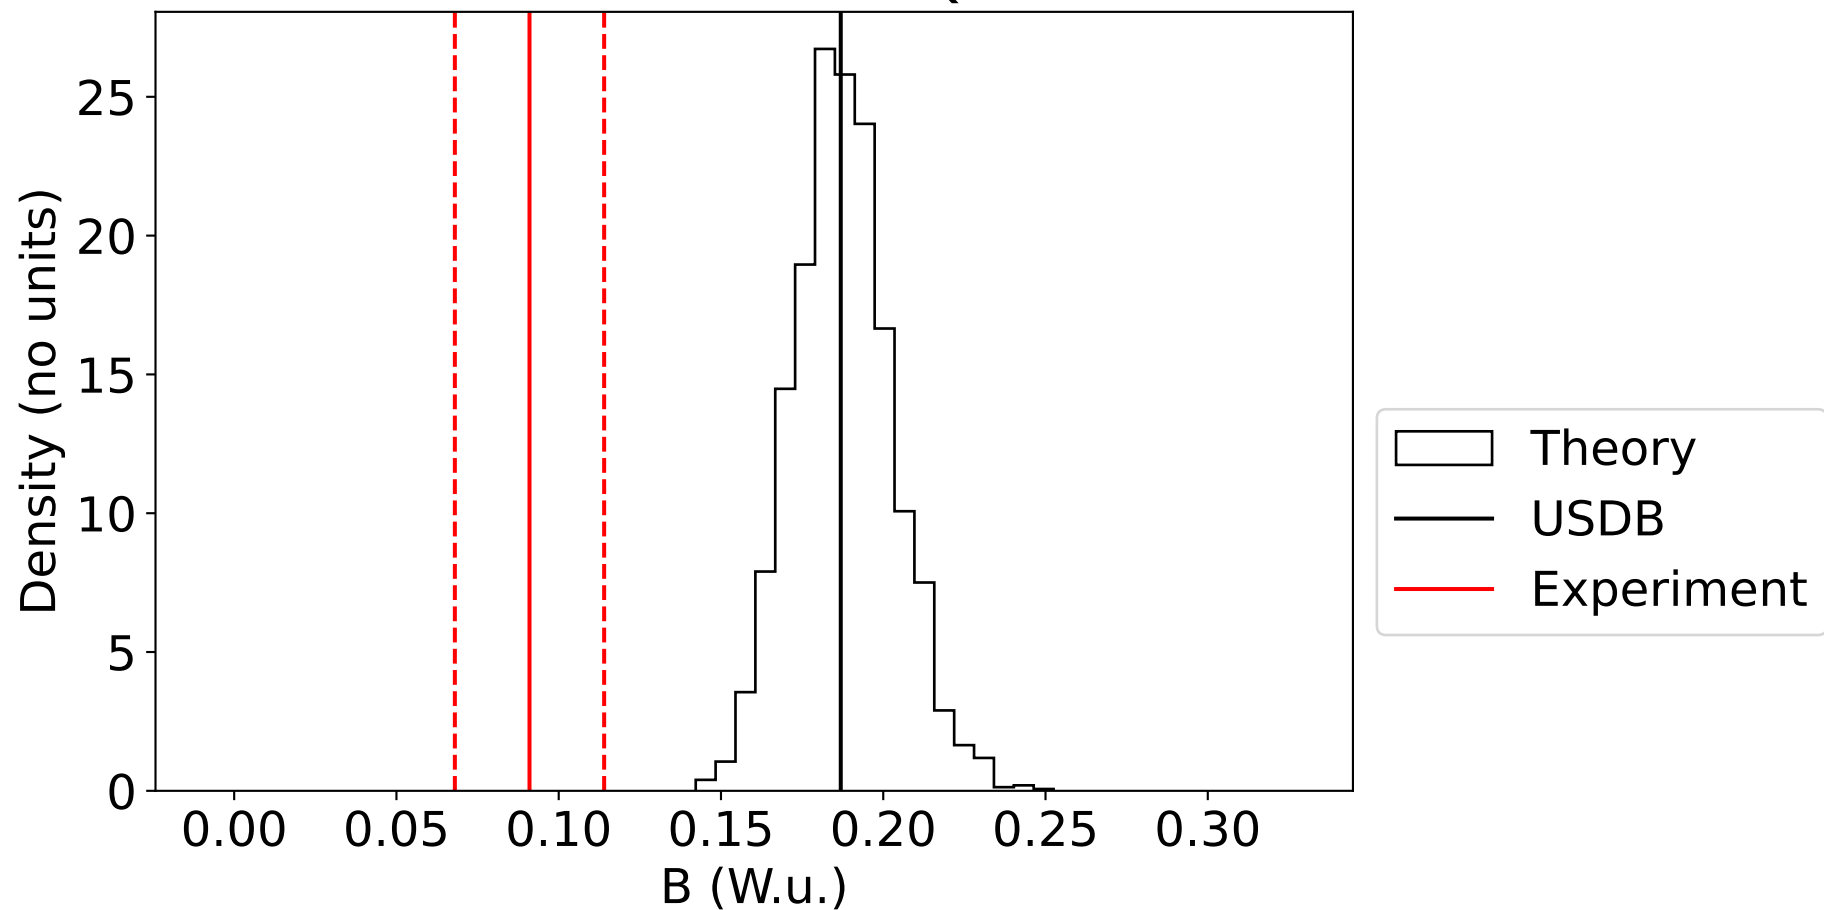

$^{30}\text{Si} (2_3) \rightarrow (2_2)$   
Included in UQ

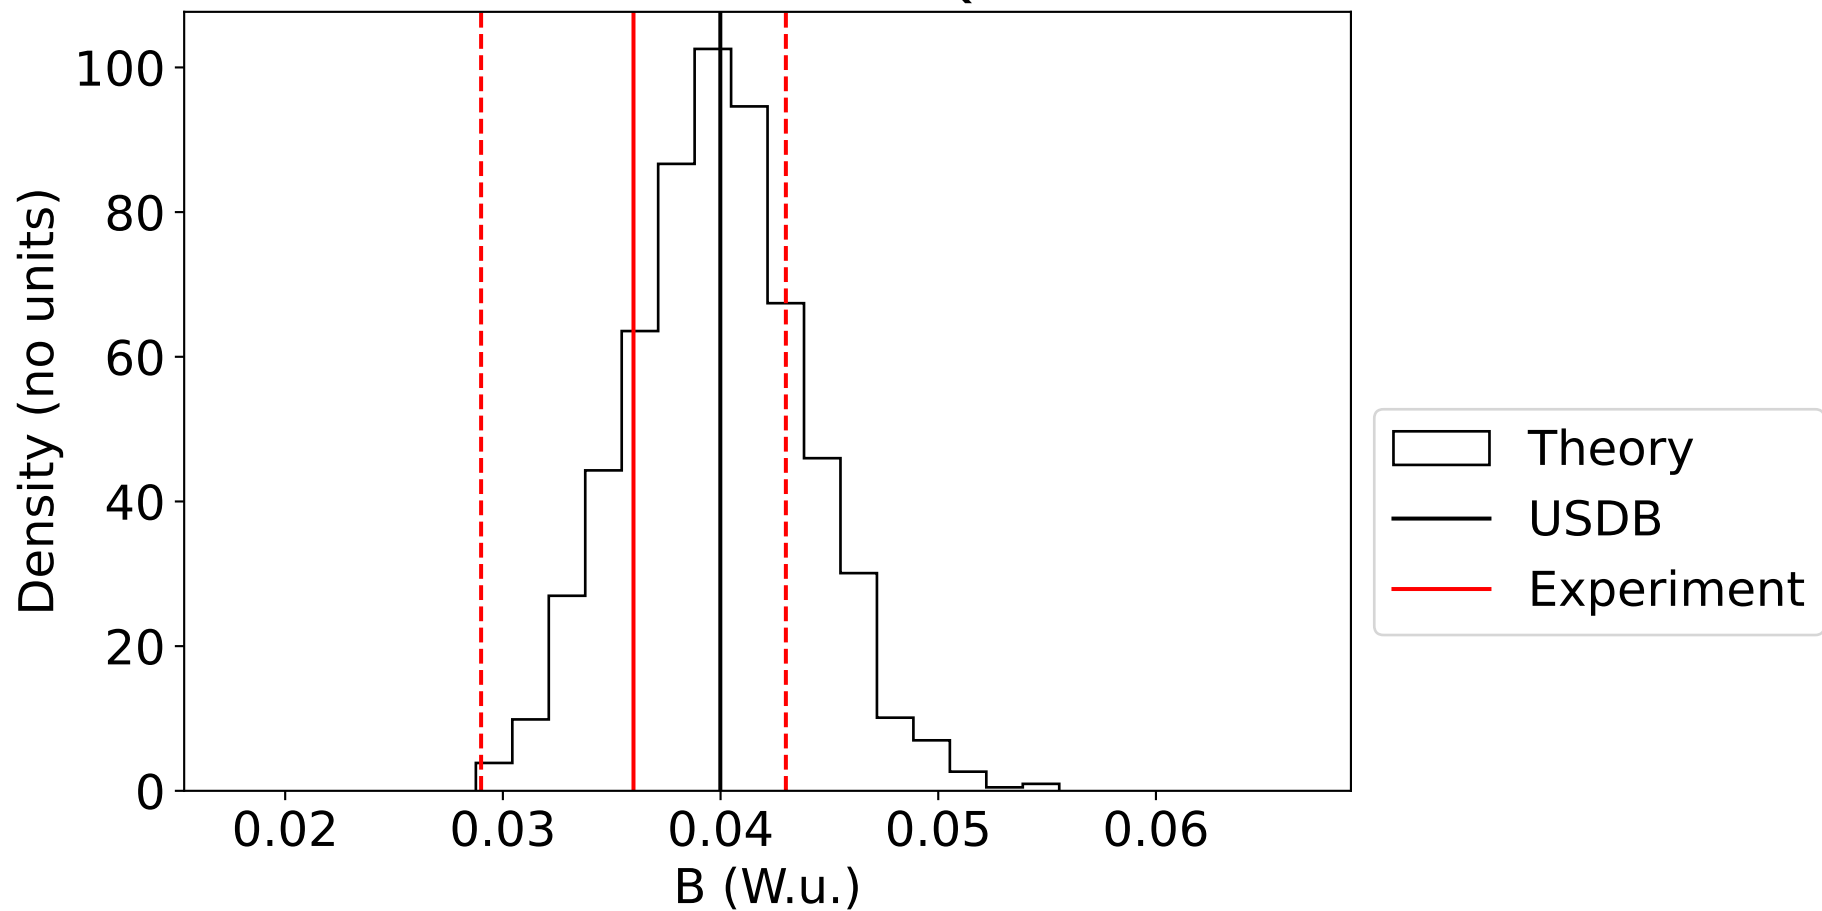

$^{30}\text{Si} (3_2) \rightarrow (2_2)$   
Included in UQ

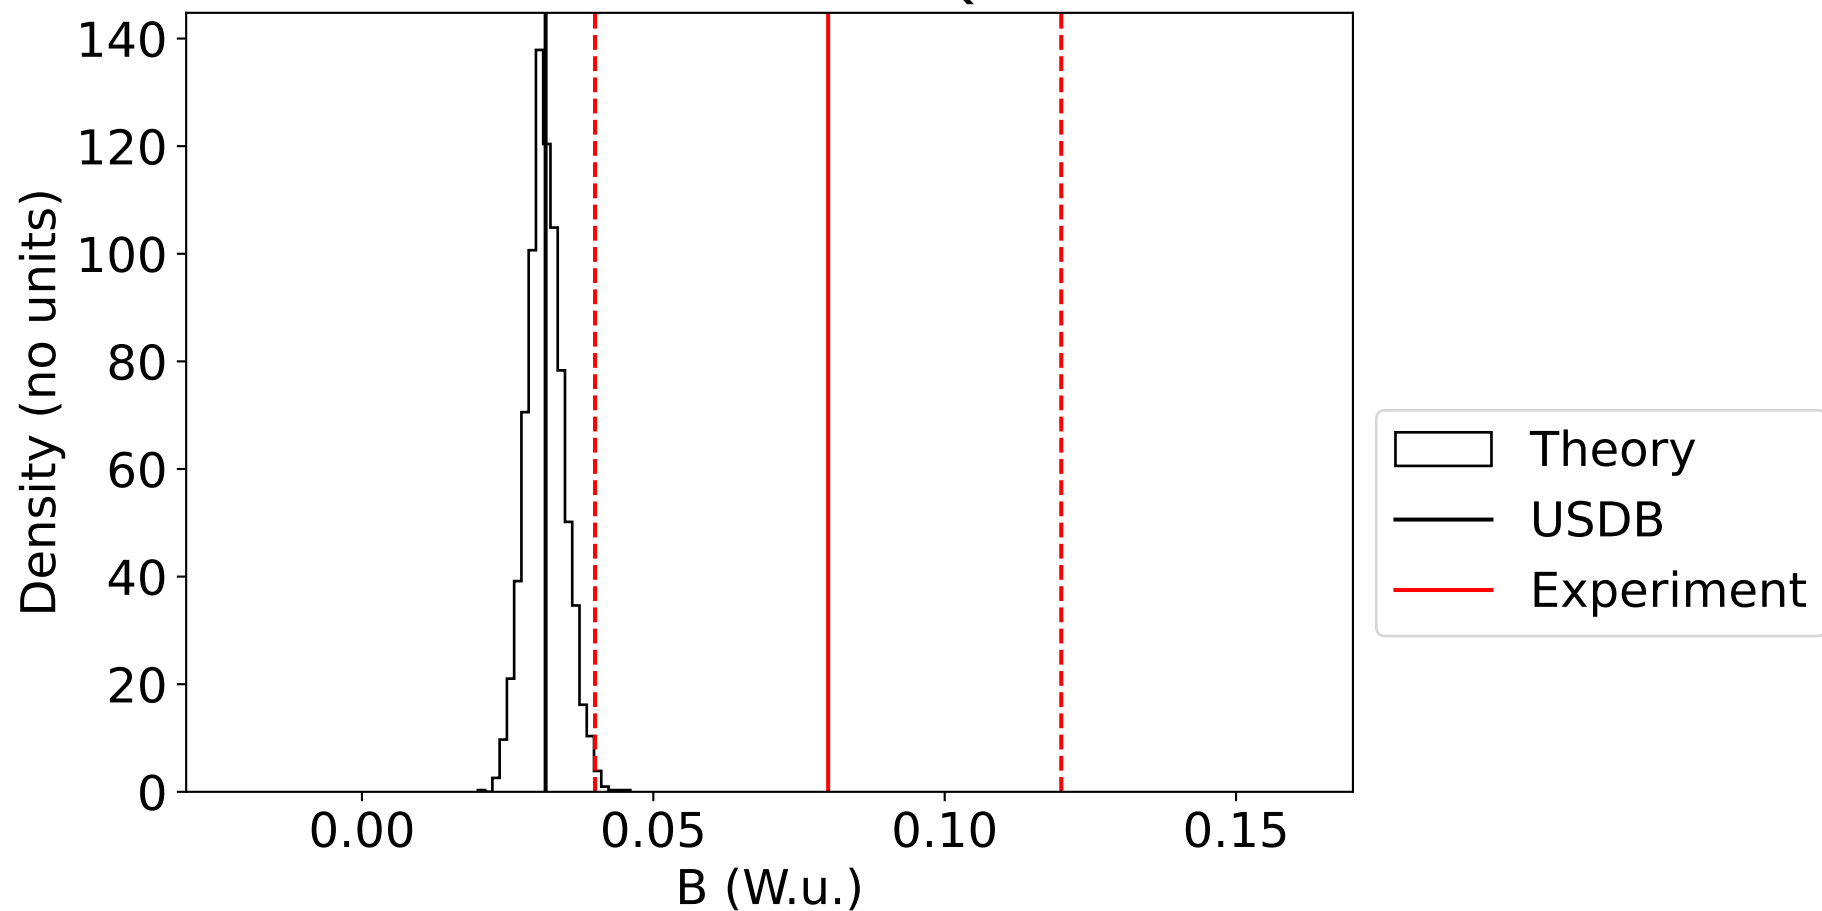

$^{31}\text{Si} (5/2_2) \rightarrow (3/2_1)$   
Included in UQ

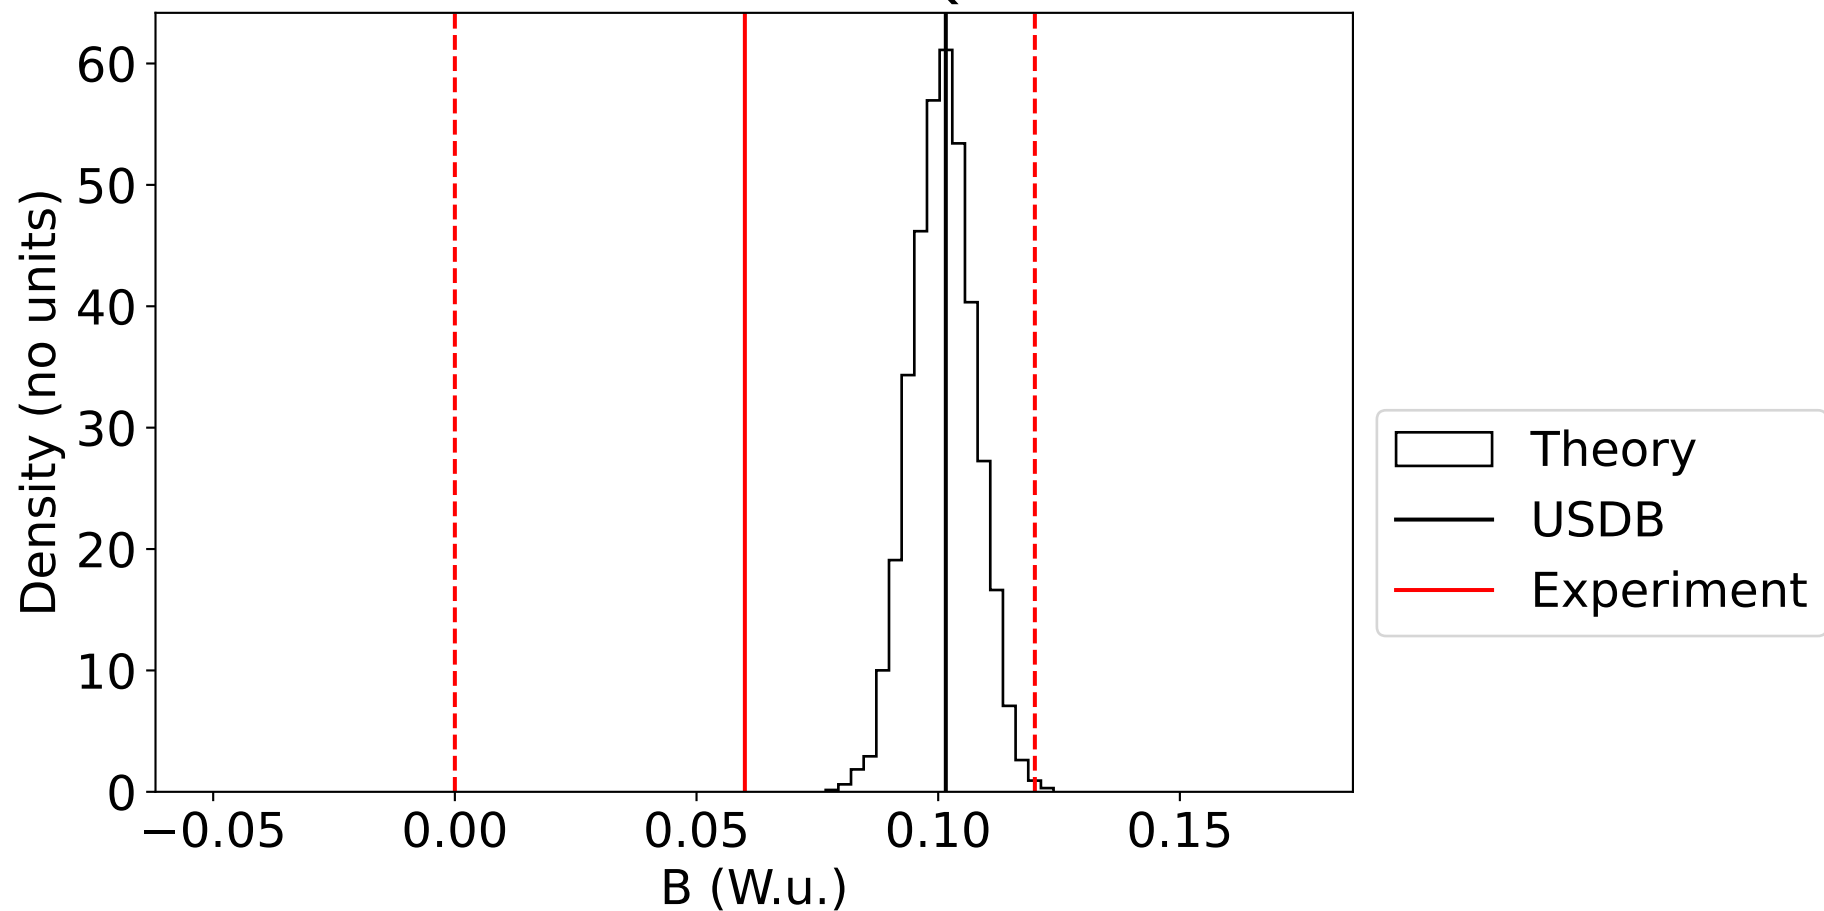

$^{29}\text{P} (3/2_1) \rightarrow (1/2_1)$   
Included in UQ

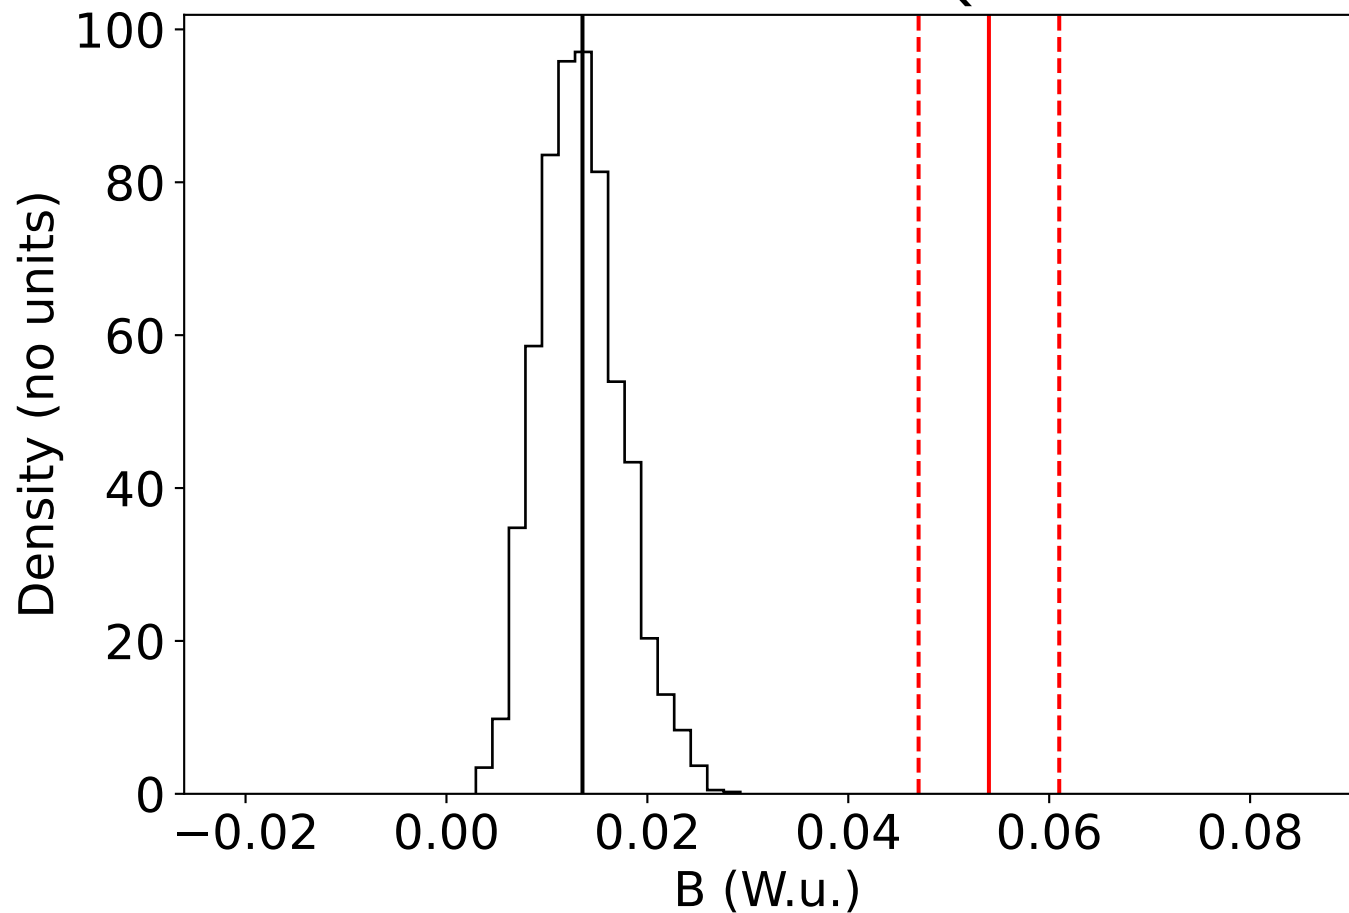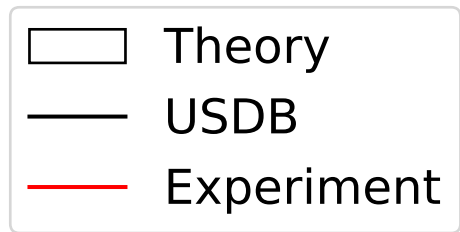



$^{29}\text{P} (5/2_1) \rightarrow (3/2_1)$   
Included in UQ

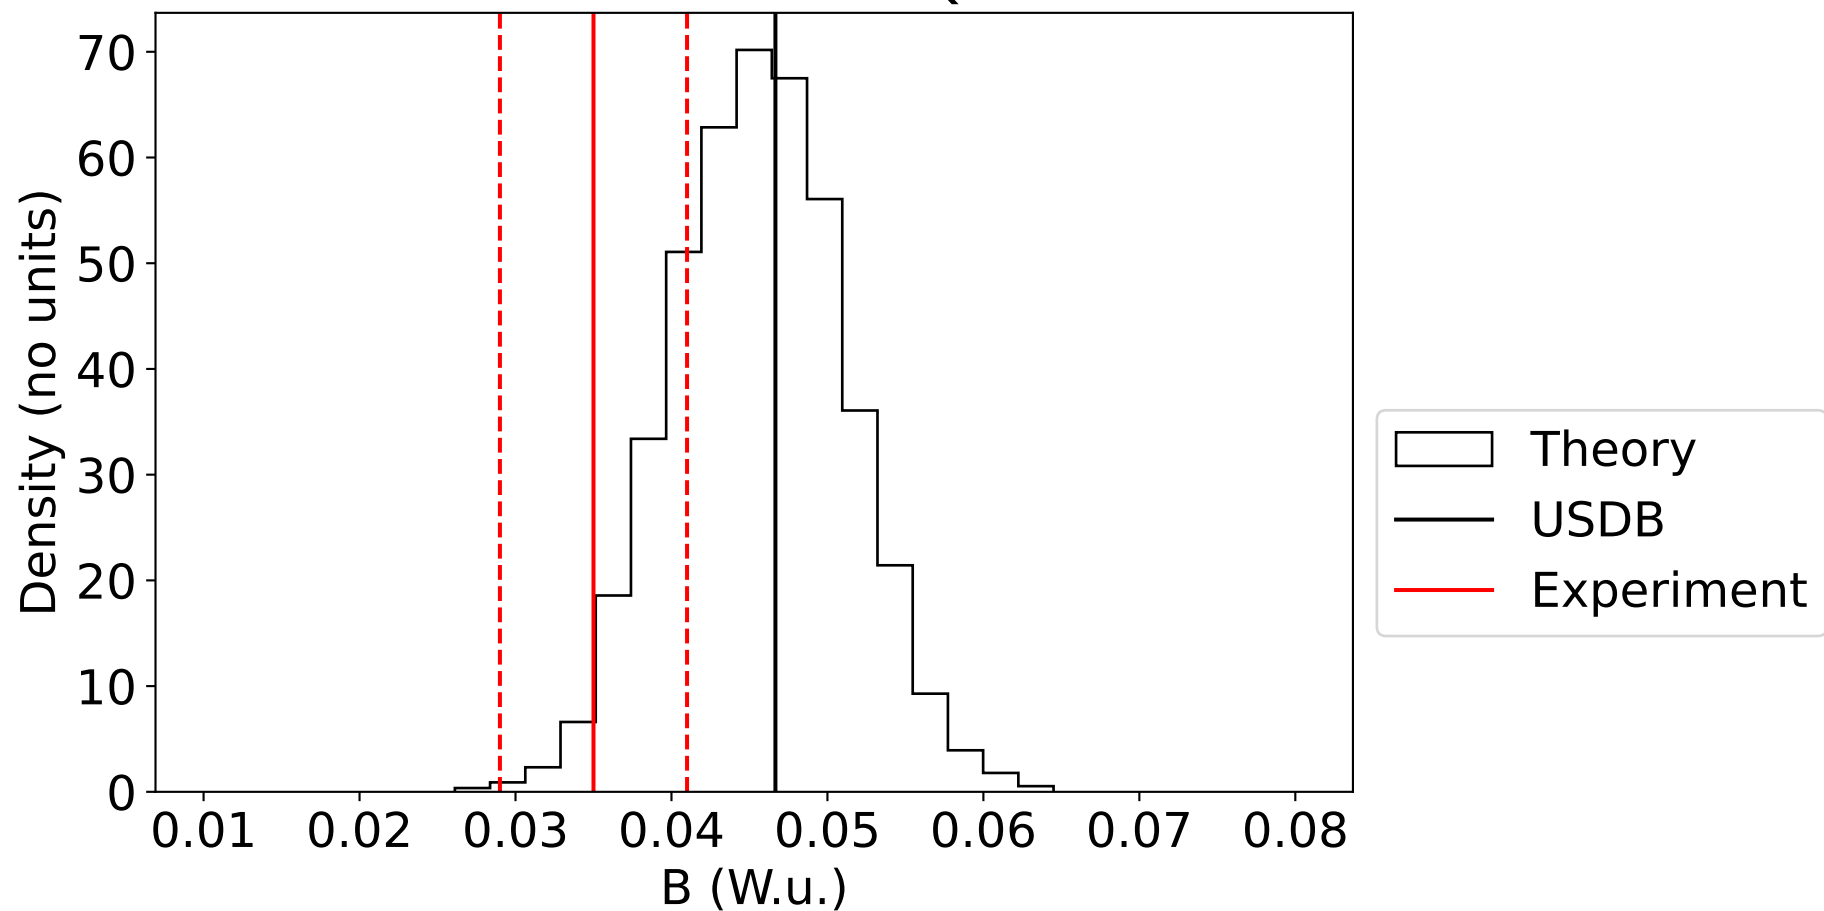

$^{29}\text{P} (3/2_2) \rightarrow (1/2_1)$   
Included in UQ

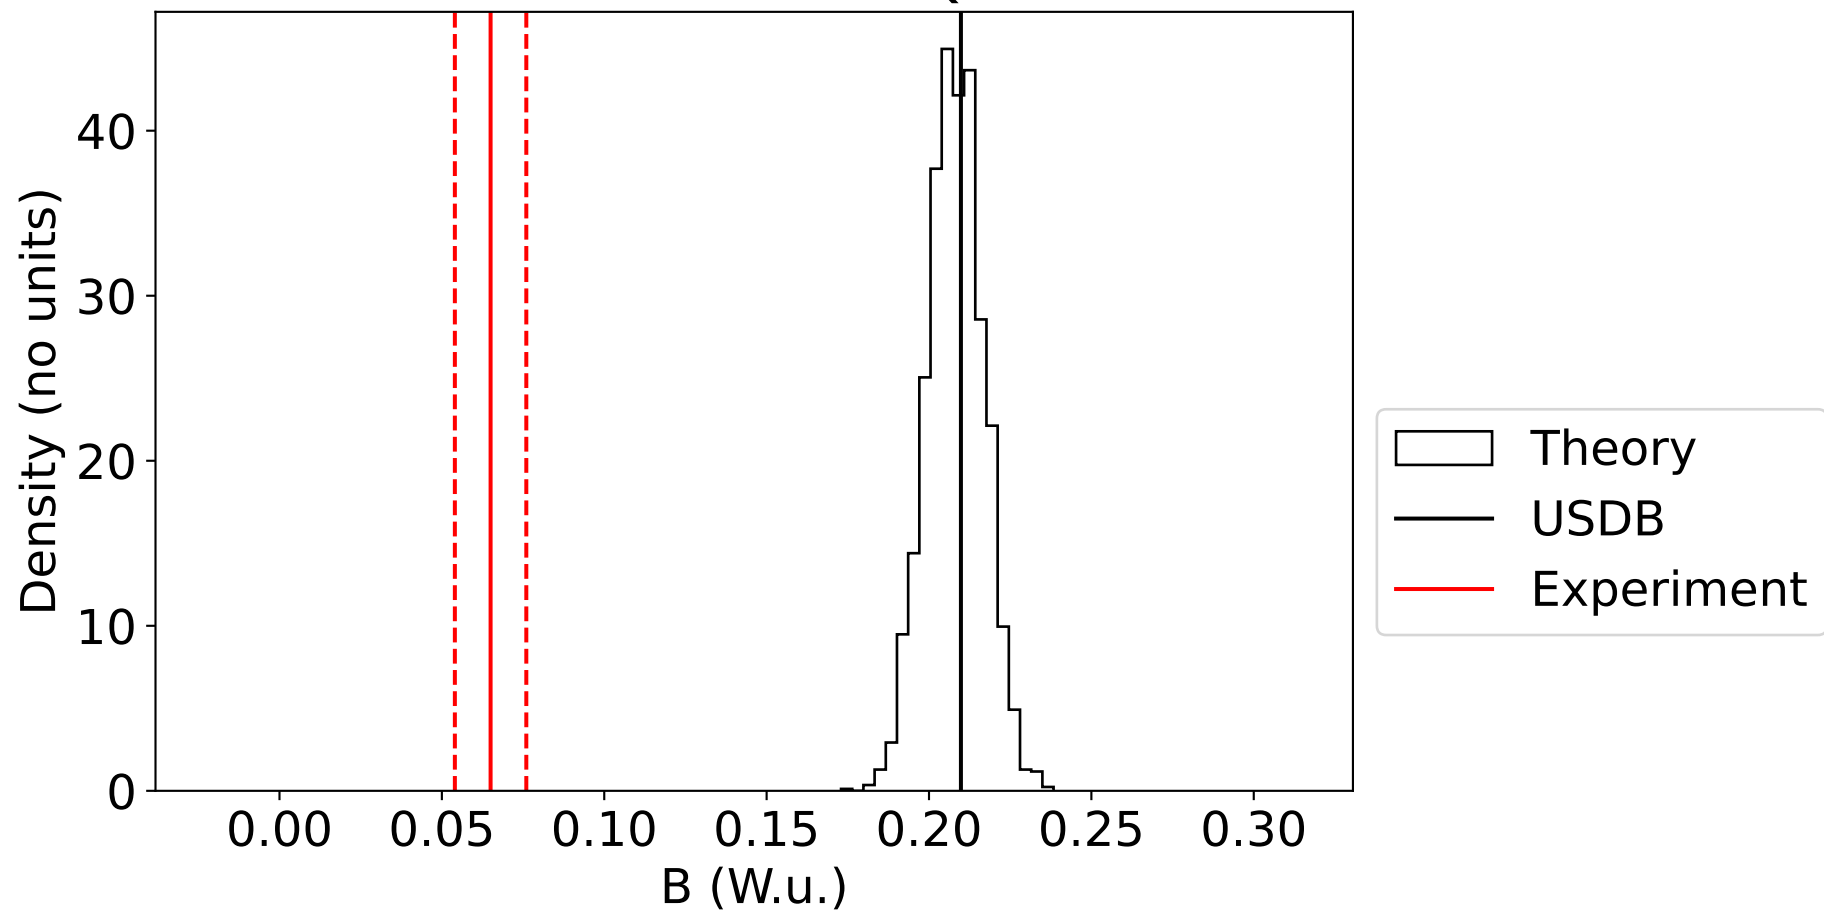

$^{29}\text{P} (3/2_2) \rightarrow (3/2_1)$   
Included in UQ

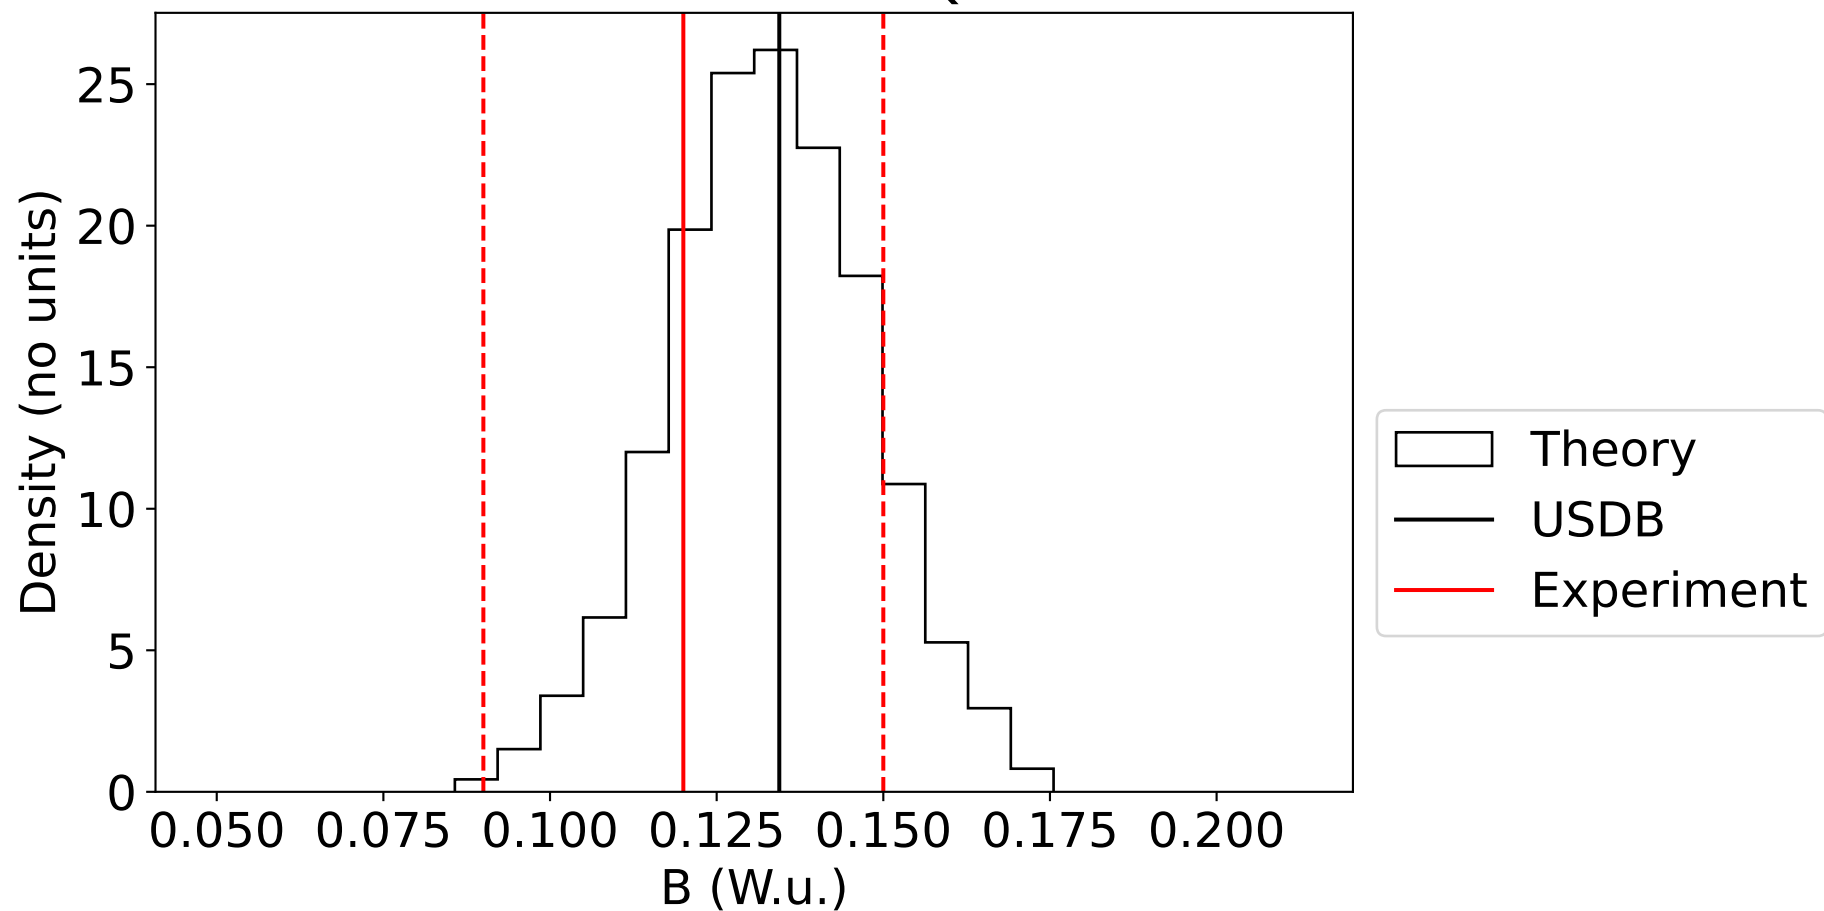

$^{29}\text{P} (5/2_2) \rightarrow (3/2_1)$   
Included in UQ

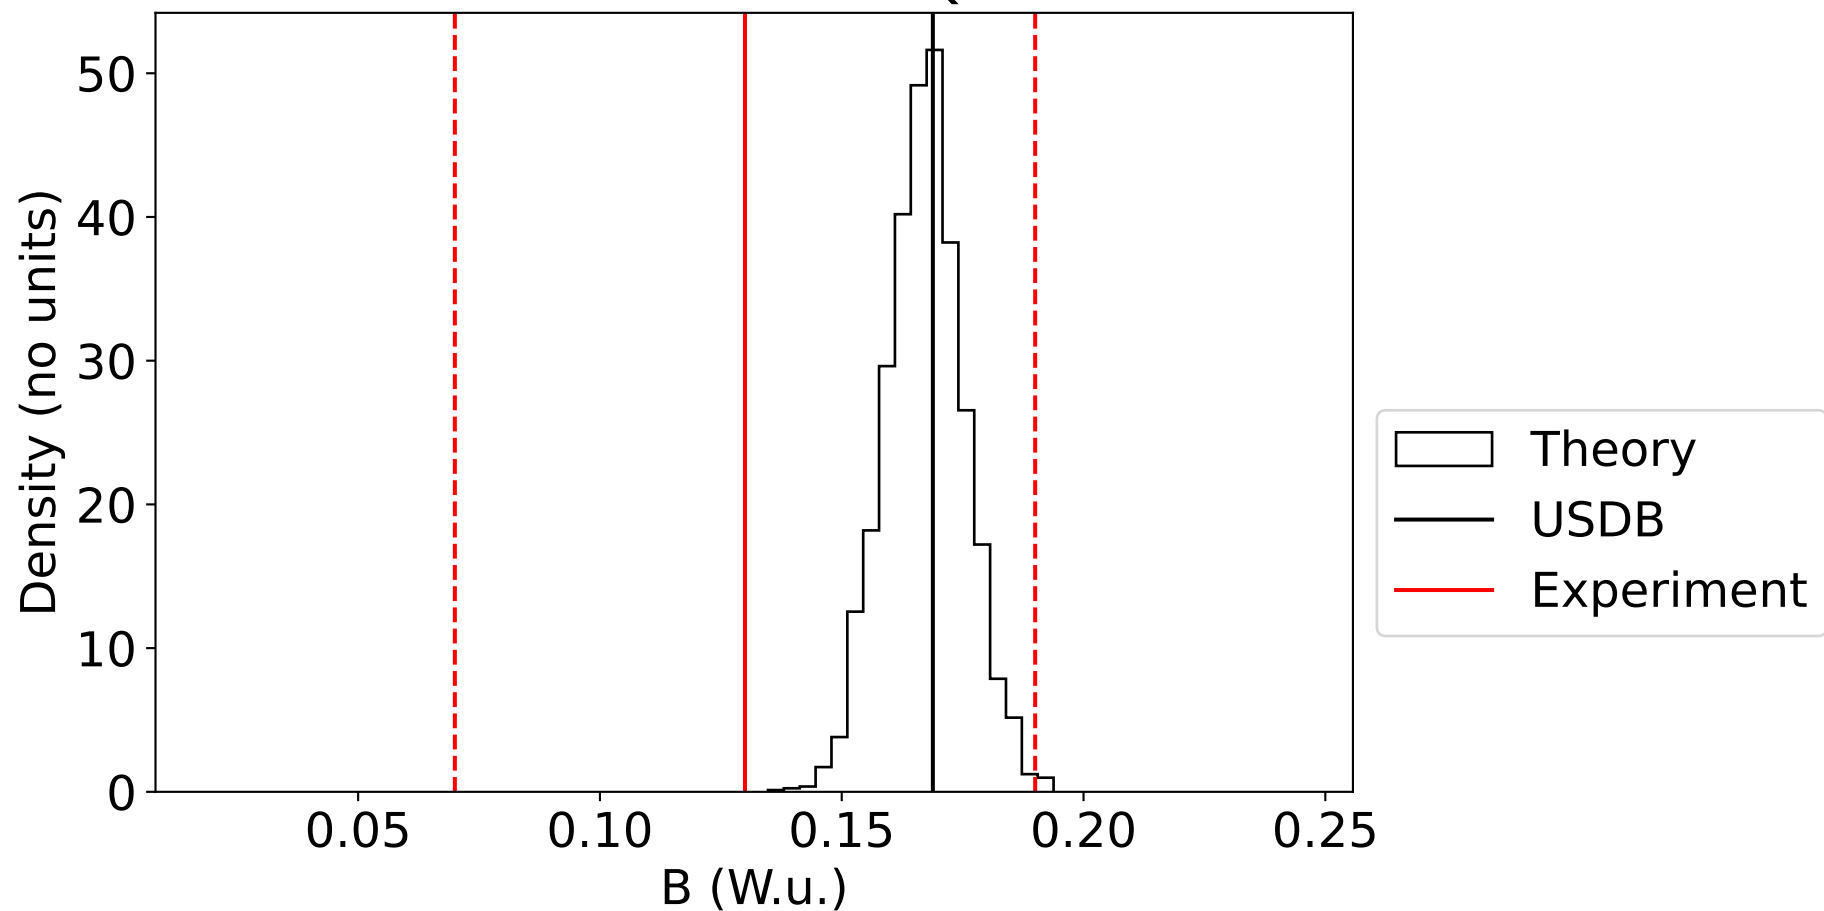

$^{29}\text{P} (7/2_1) \rightarrow (5/2_1)$   
Included in UQ

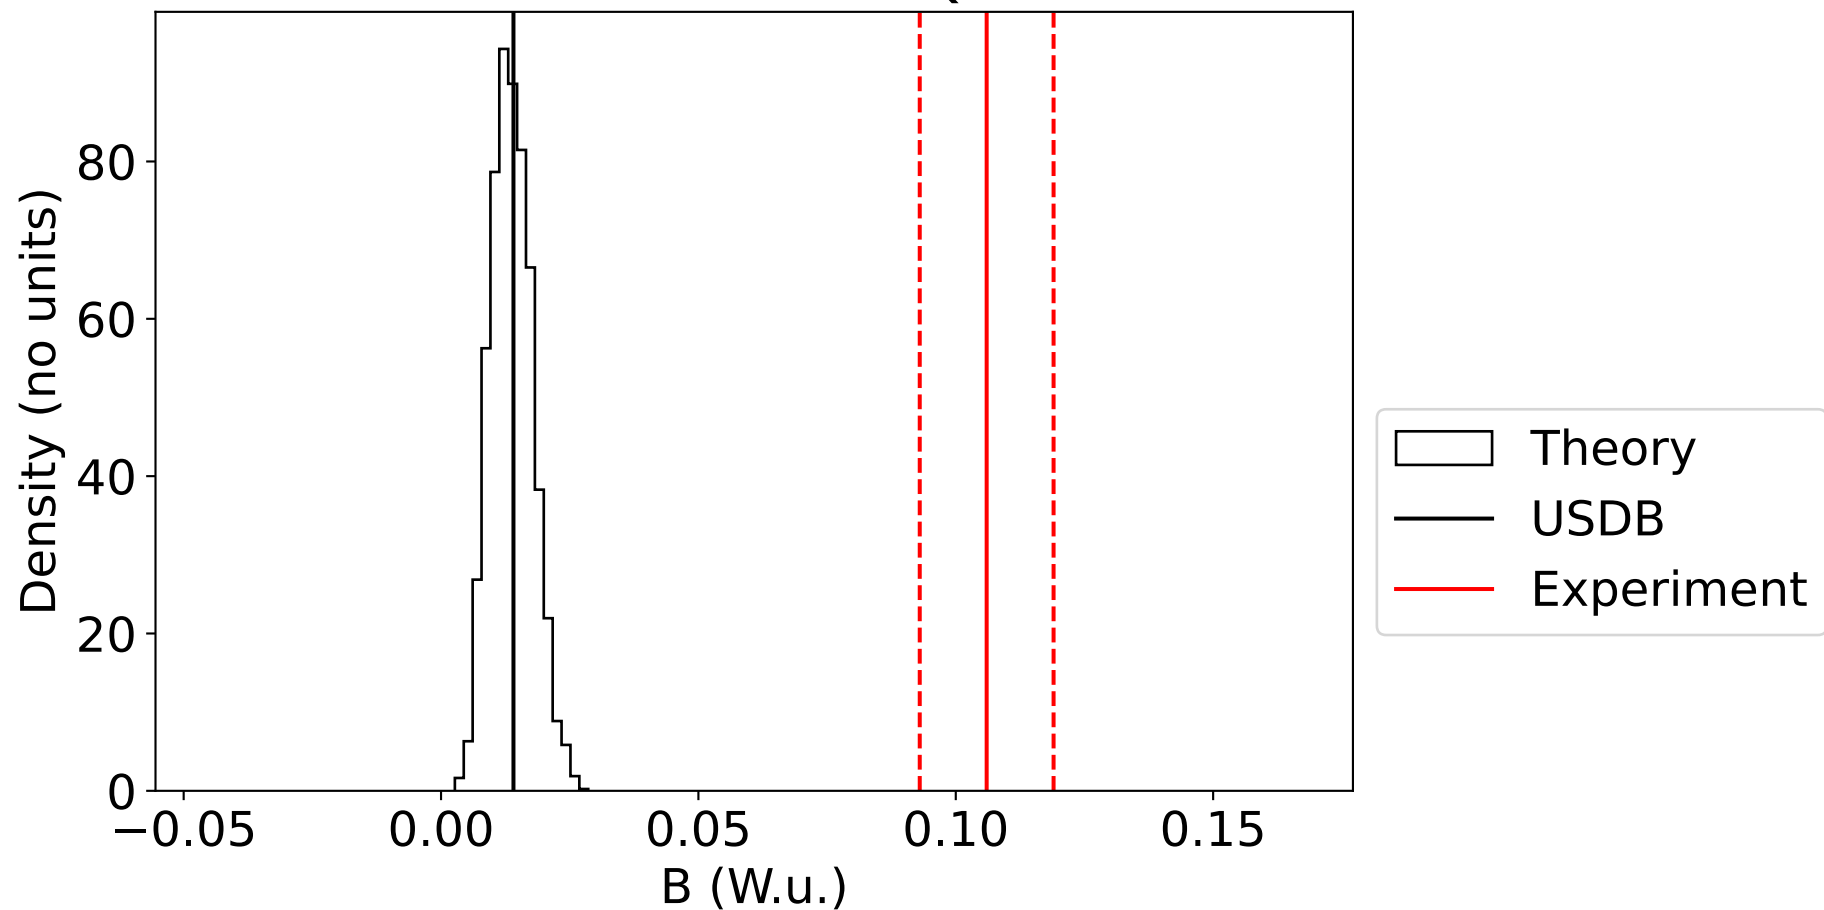

$^{31}\text{P} (3/2_1) \rightarrow (1/2_1)$   
Included in UQ

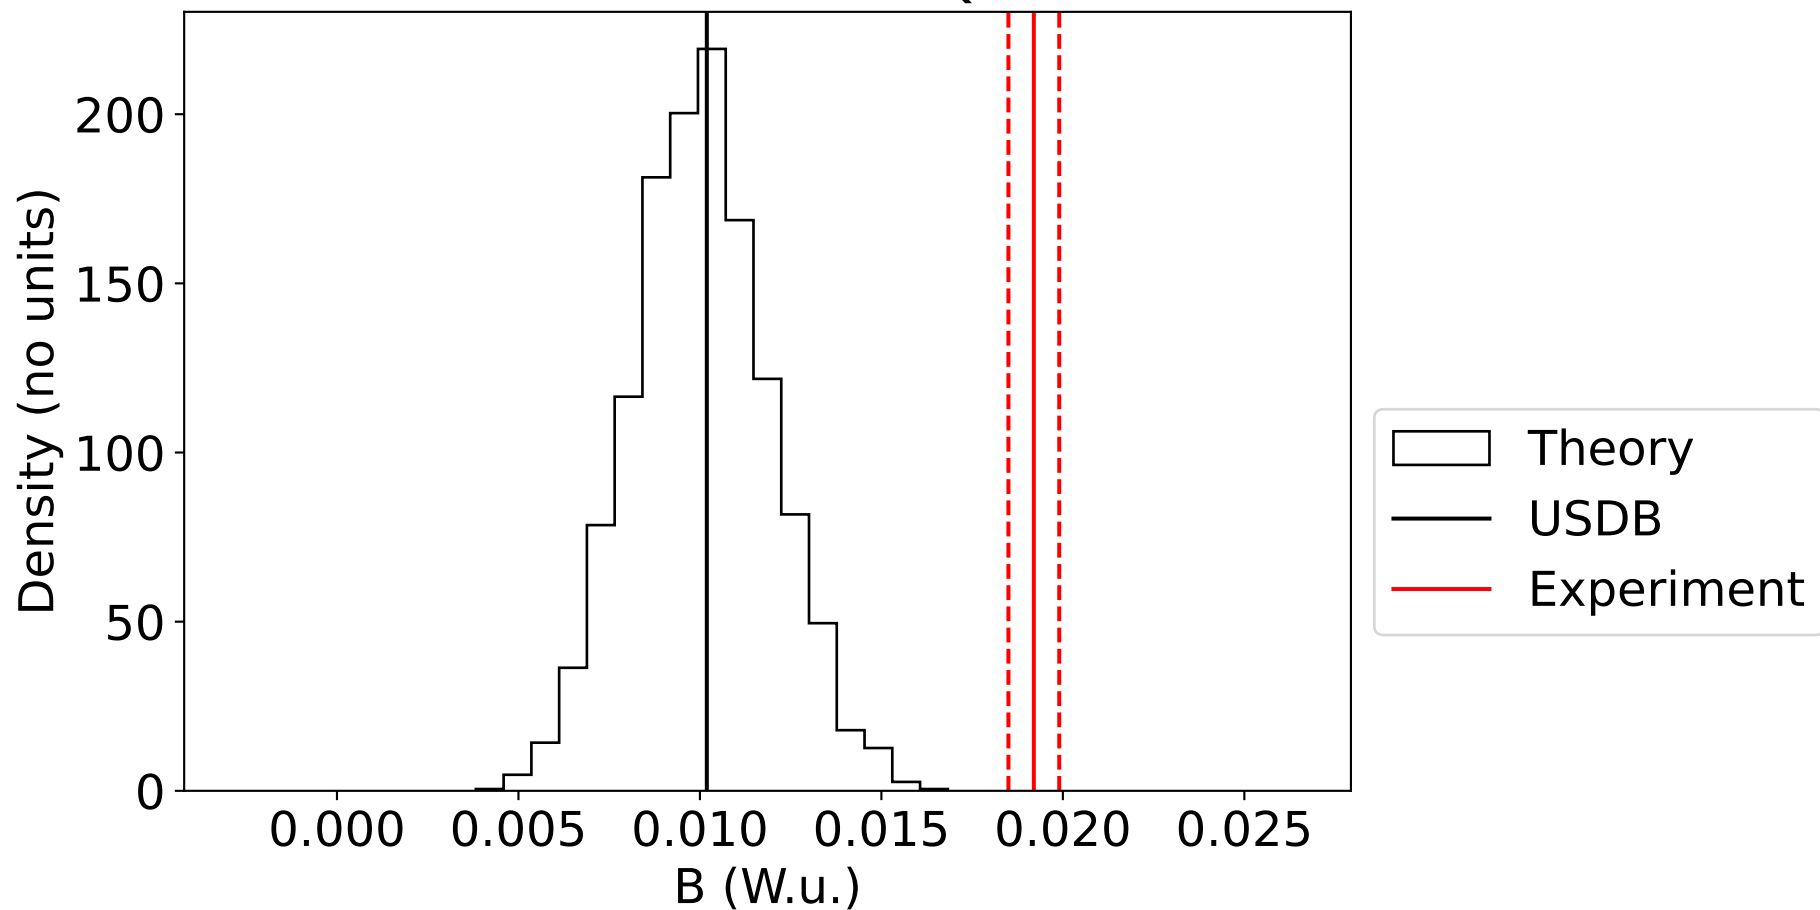

$^{31}\text{P}$  ( $1/2_2 \rightarrow 1/2_1$ )  
Included in UQ

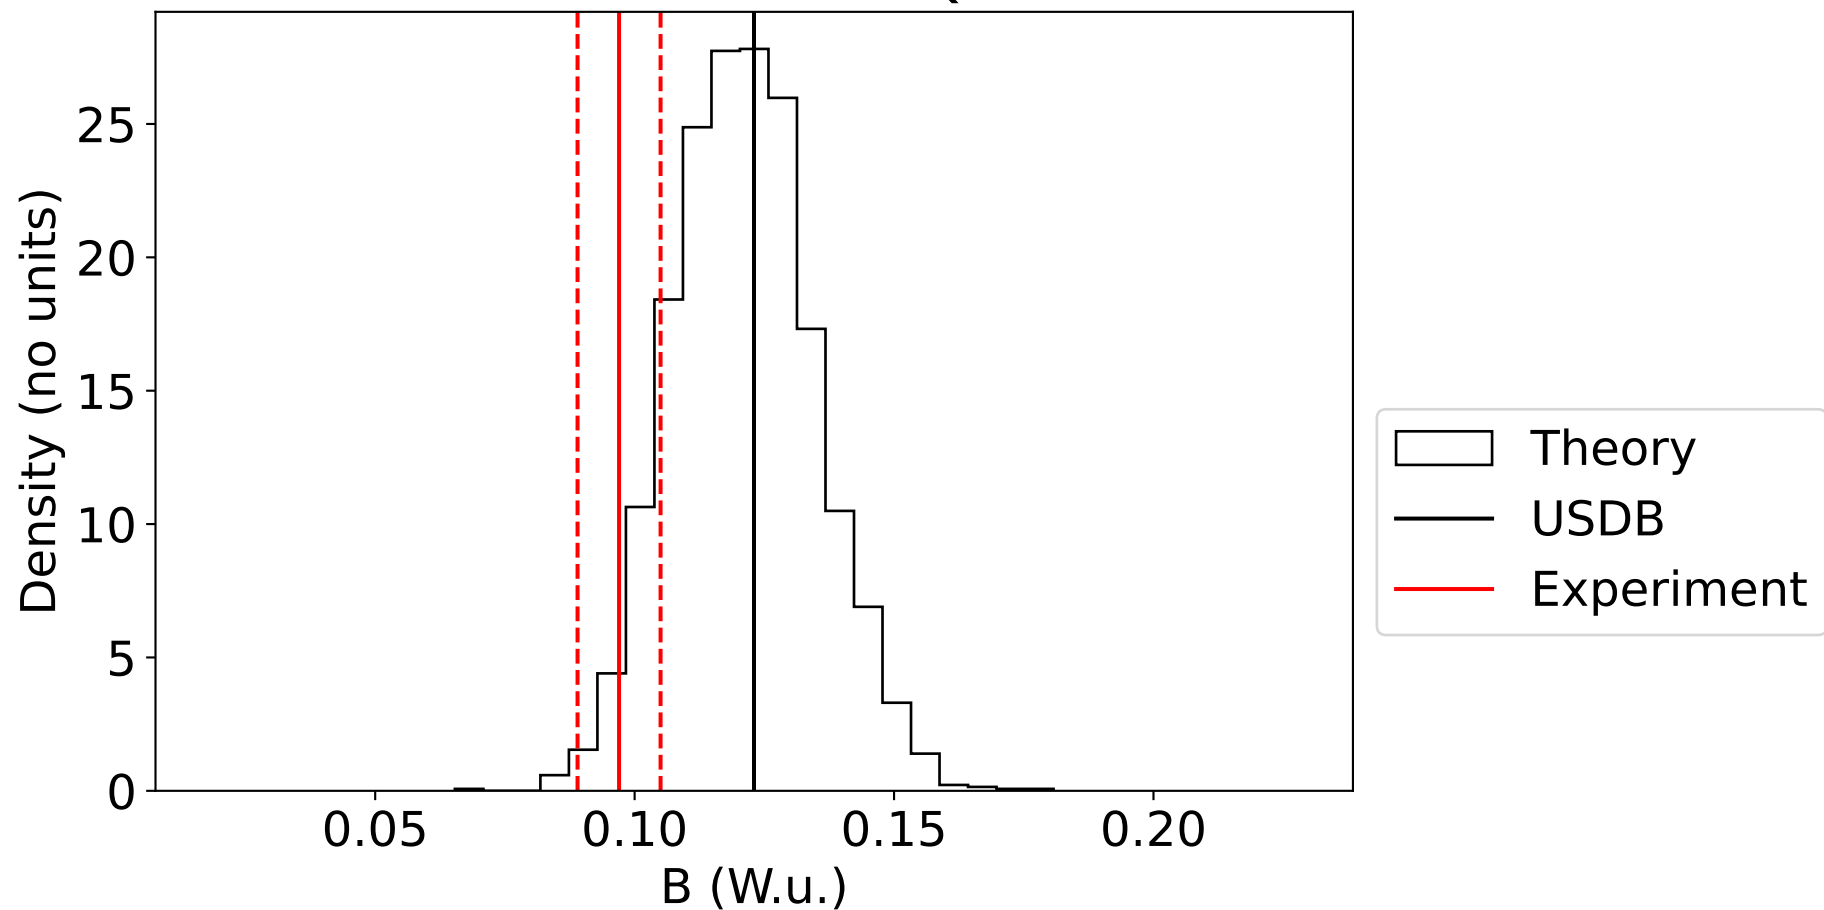

$^{31}\text{P} (5/2_2) \rightarrow (3/2_1)$   
Included in UQ

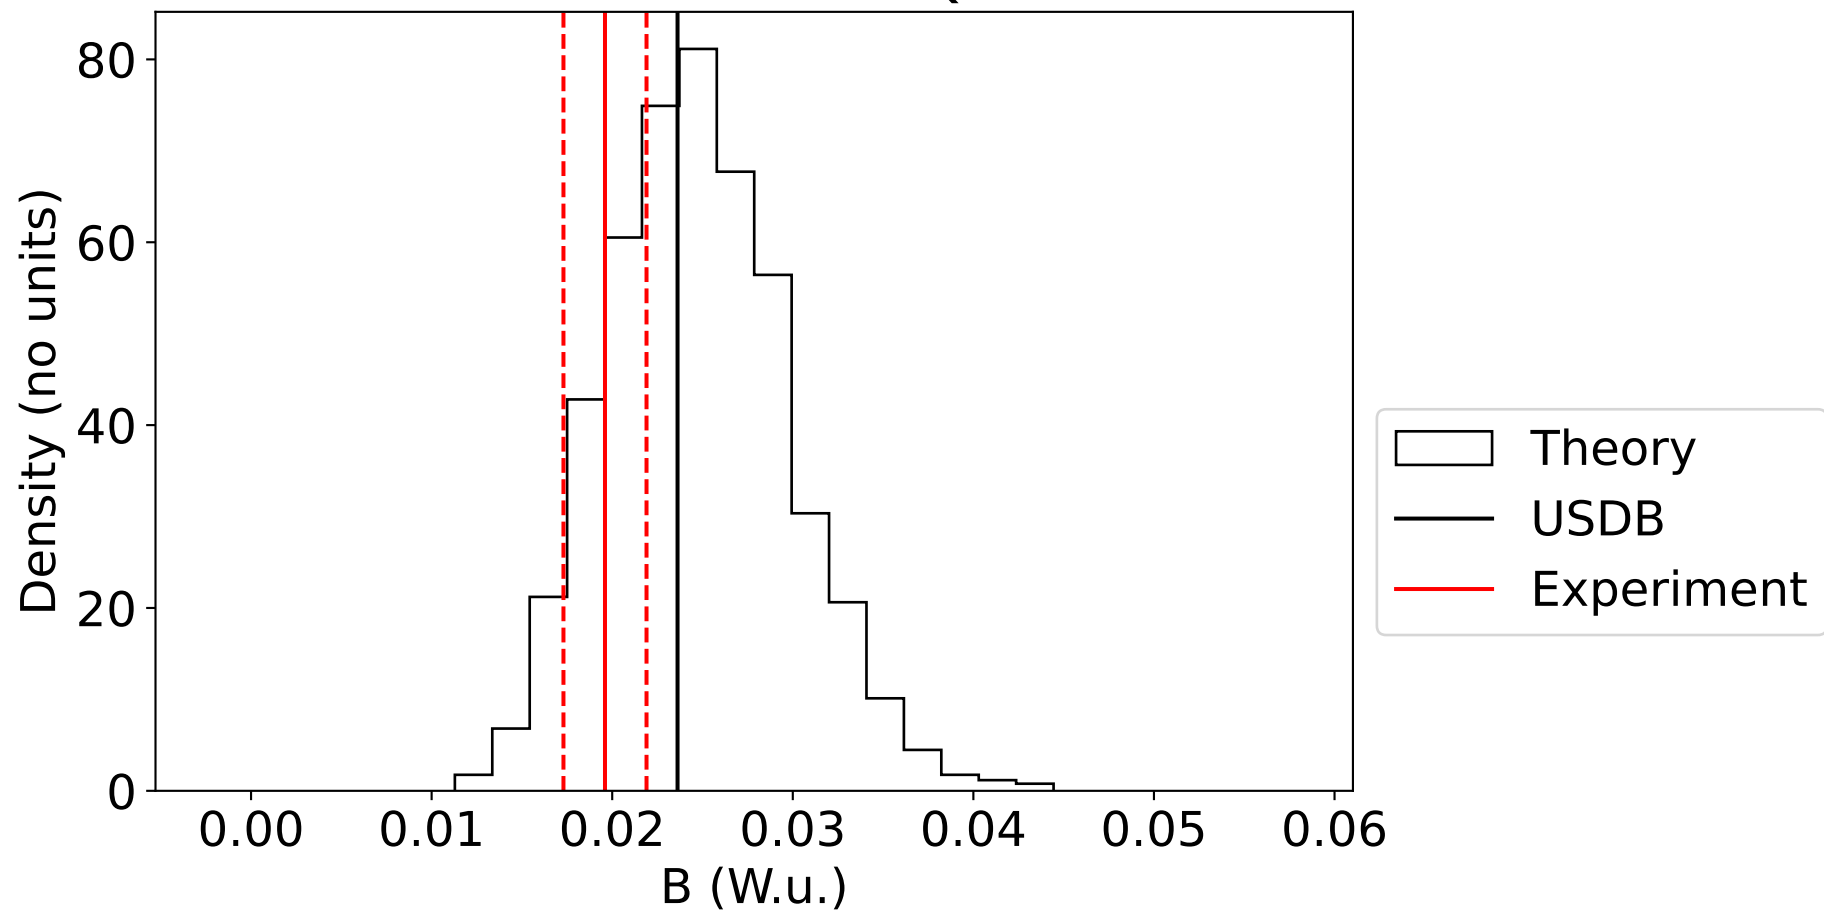



$^{31}\text{P} (5/2_2) \rightarrow (5/2_1)$   
Included in UQ

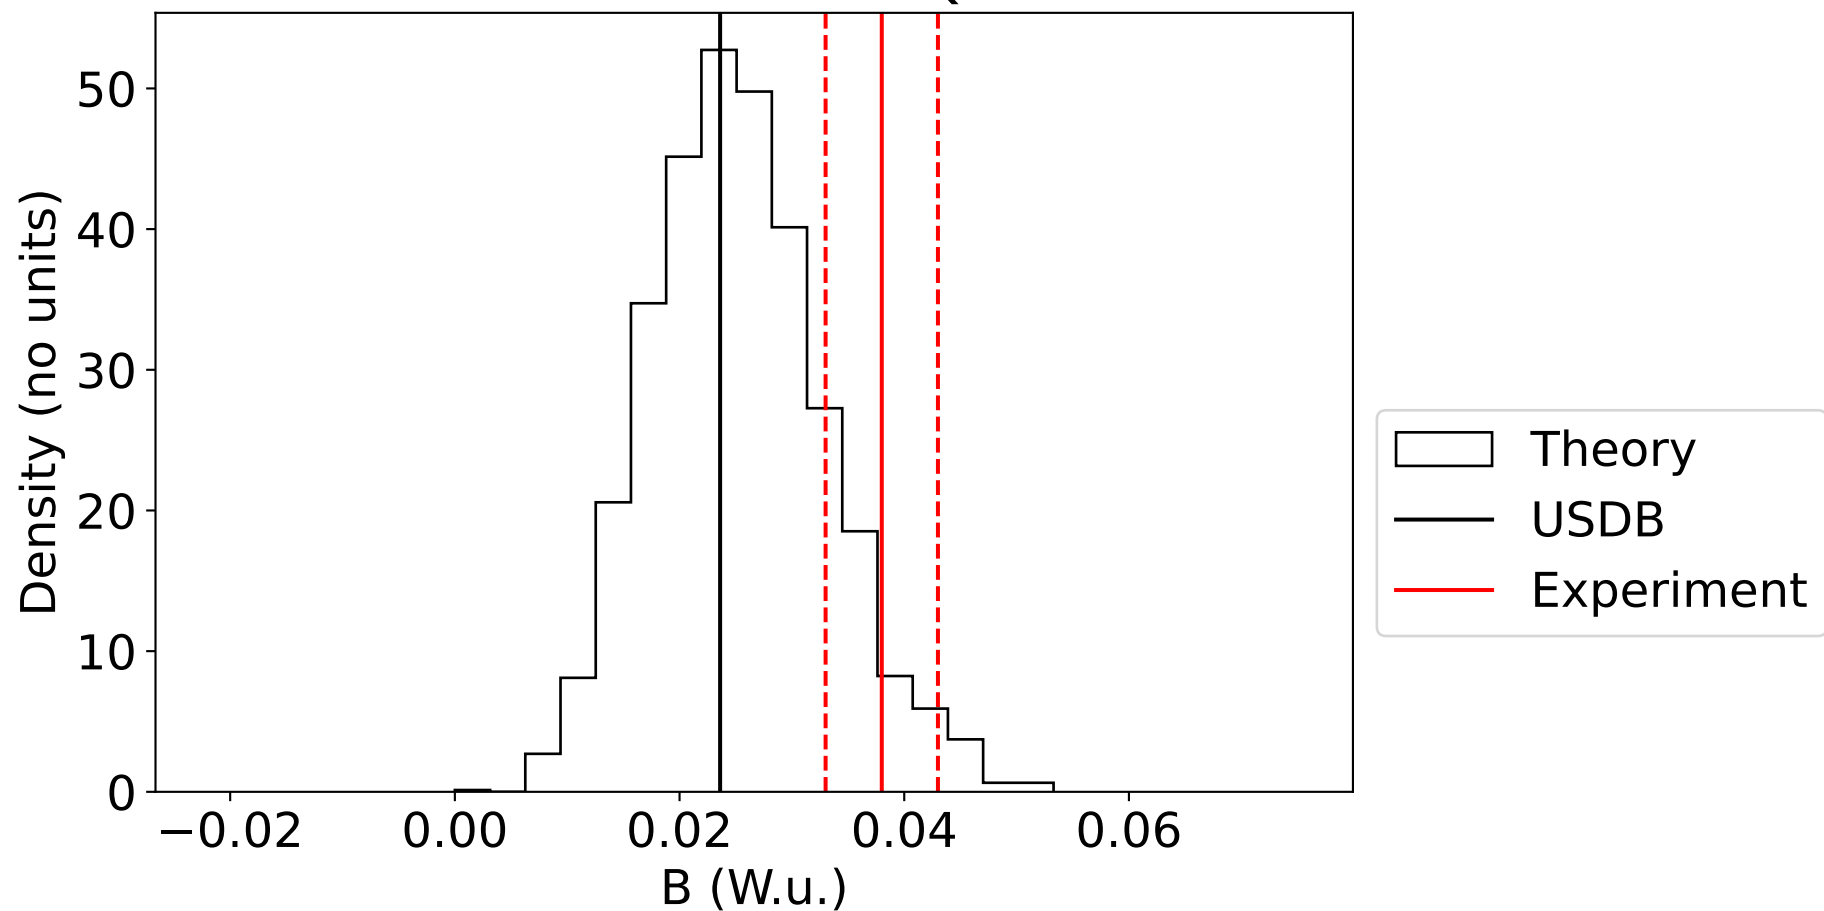

$^{31}\text{P} (3/2_2) \rightarrow (1/2_1)$   
Included in UQ

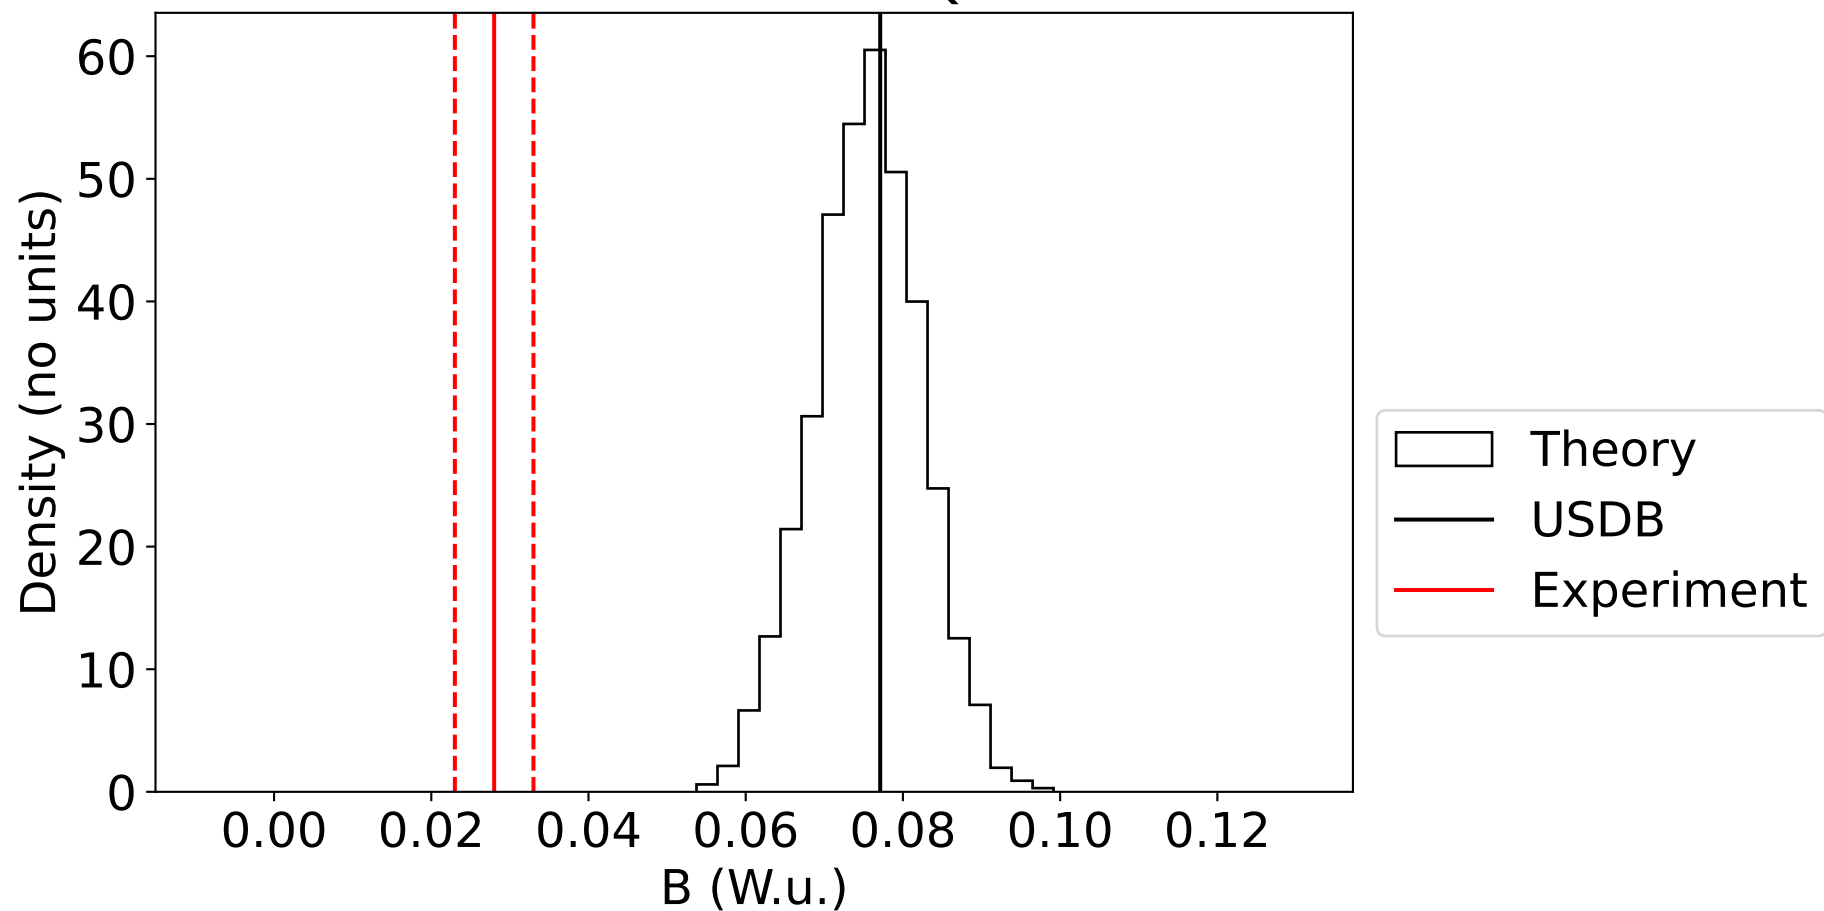

$^{31}\text{P} (5/2_3) \rightarrow (3/2_1)$   
Included in UQ

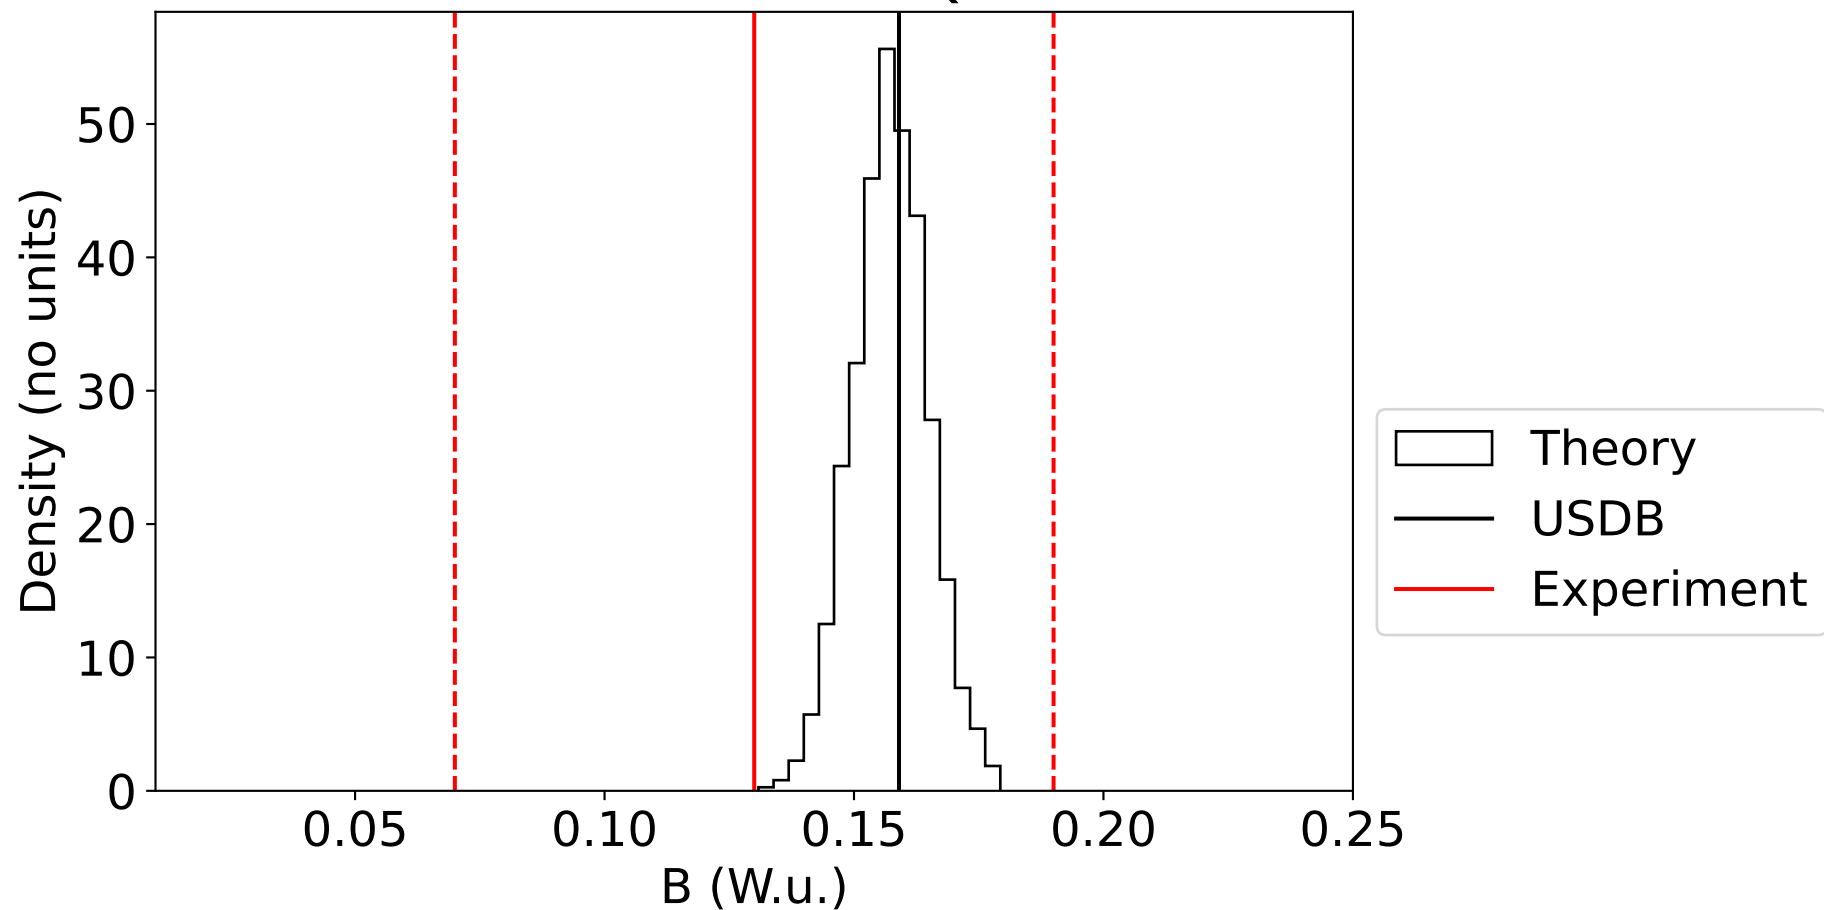

$^{31}\text{P} (3/2_3) \rightarrow (1/2_1)$   
Included in UQ

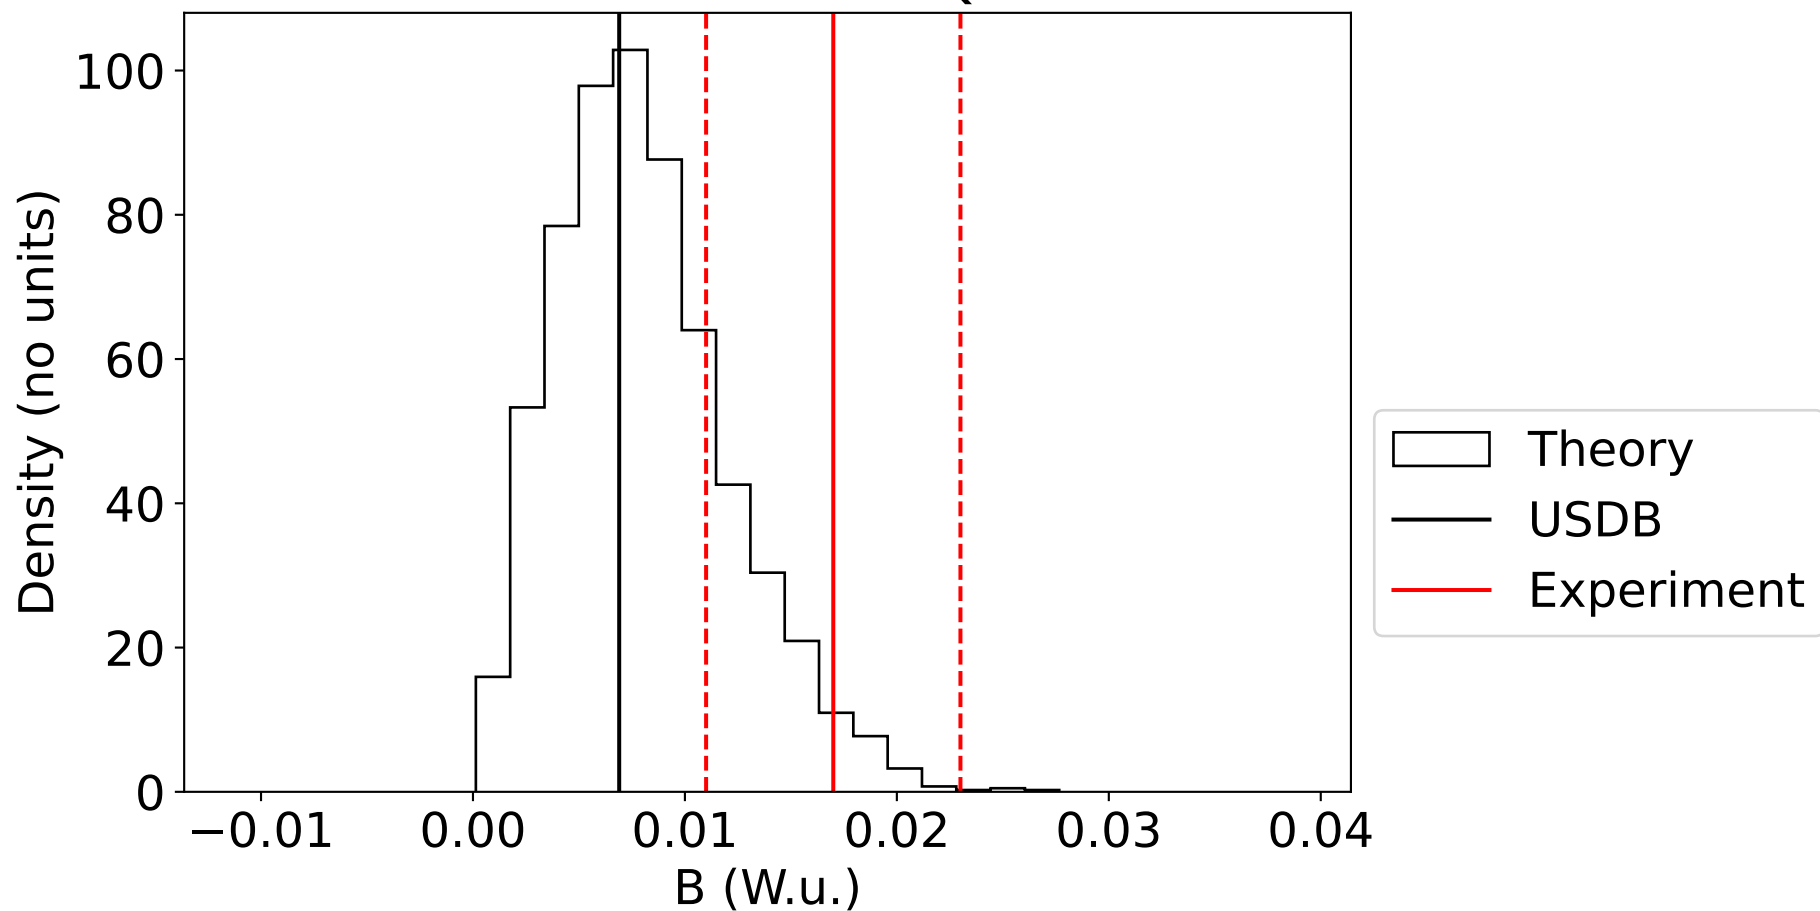

$^{31}\text{P} (3/2_3) \rightarrow (3/2_1)$   
Included in UQ

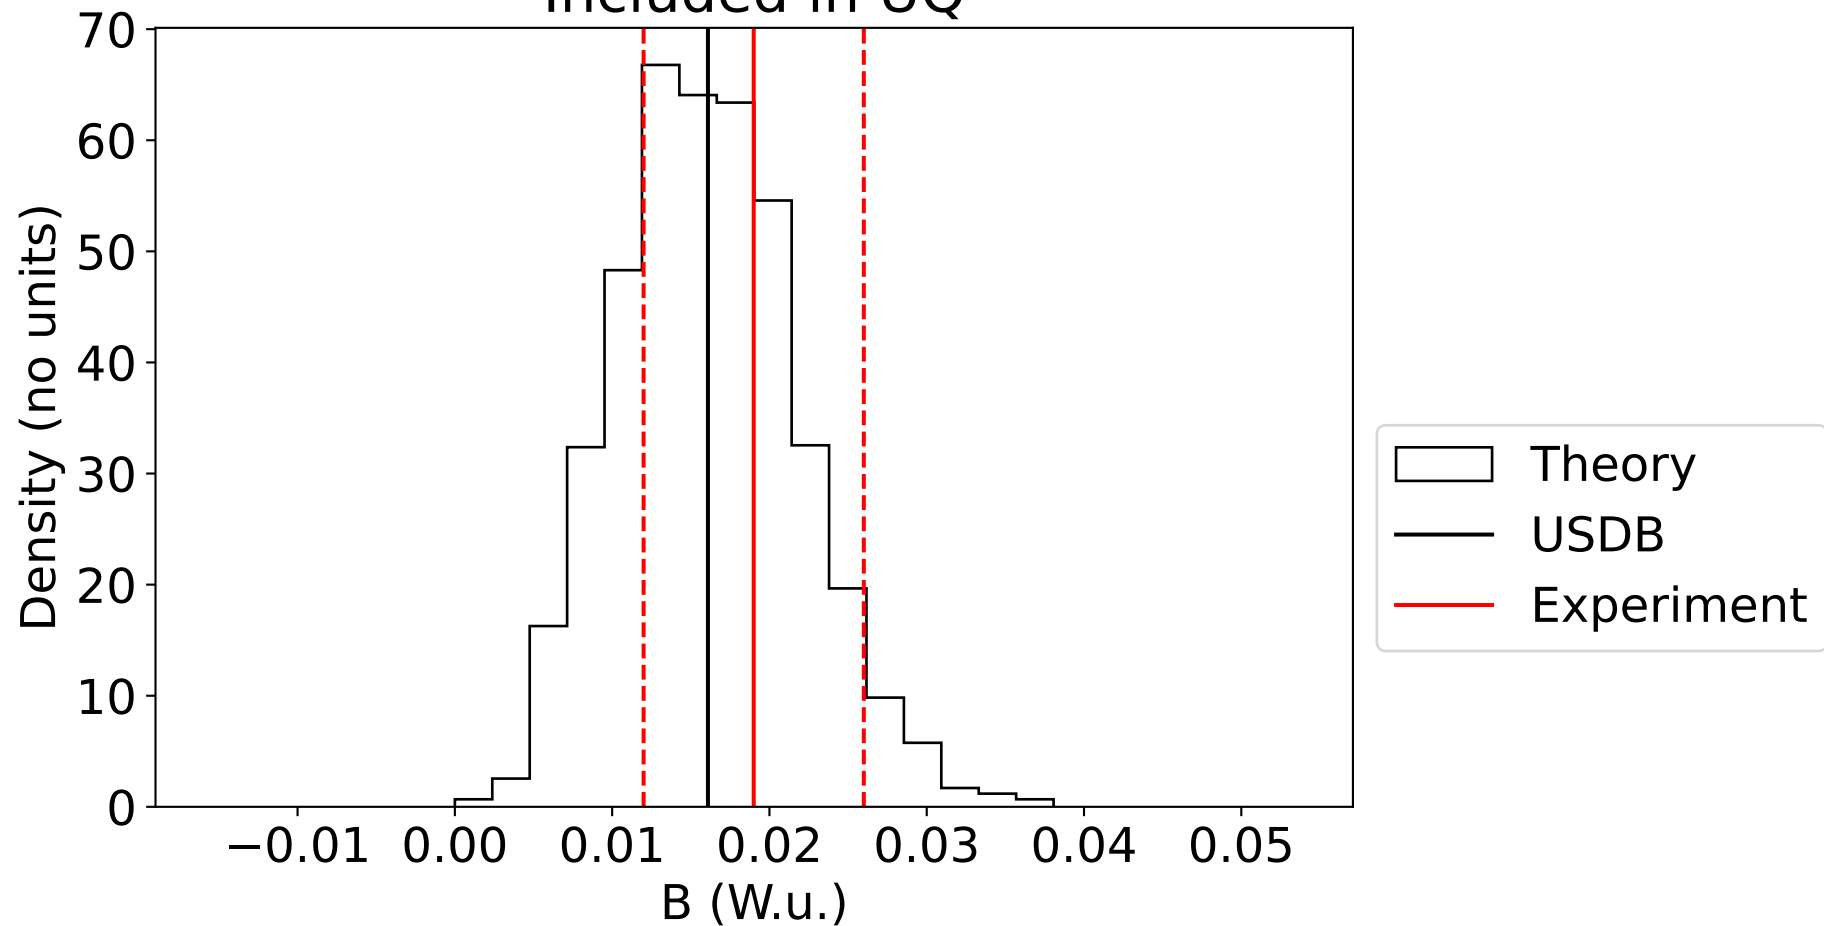

$^{31}\text{P} (3/2_4) \rightarrow (3/2_1)$   
Included in UQ

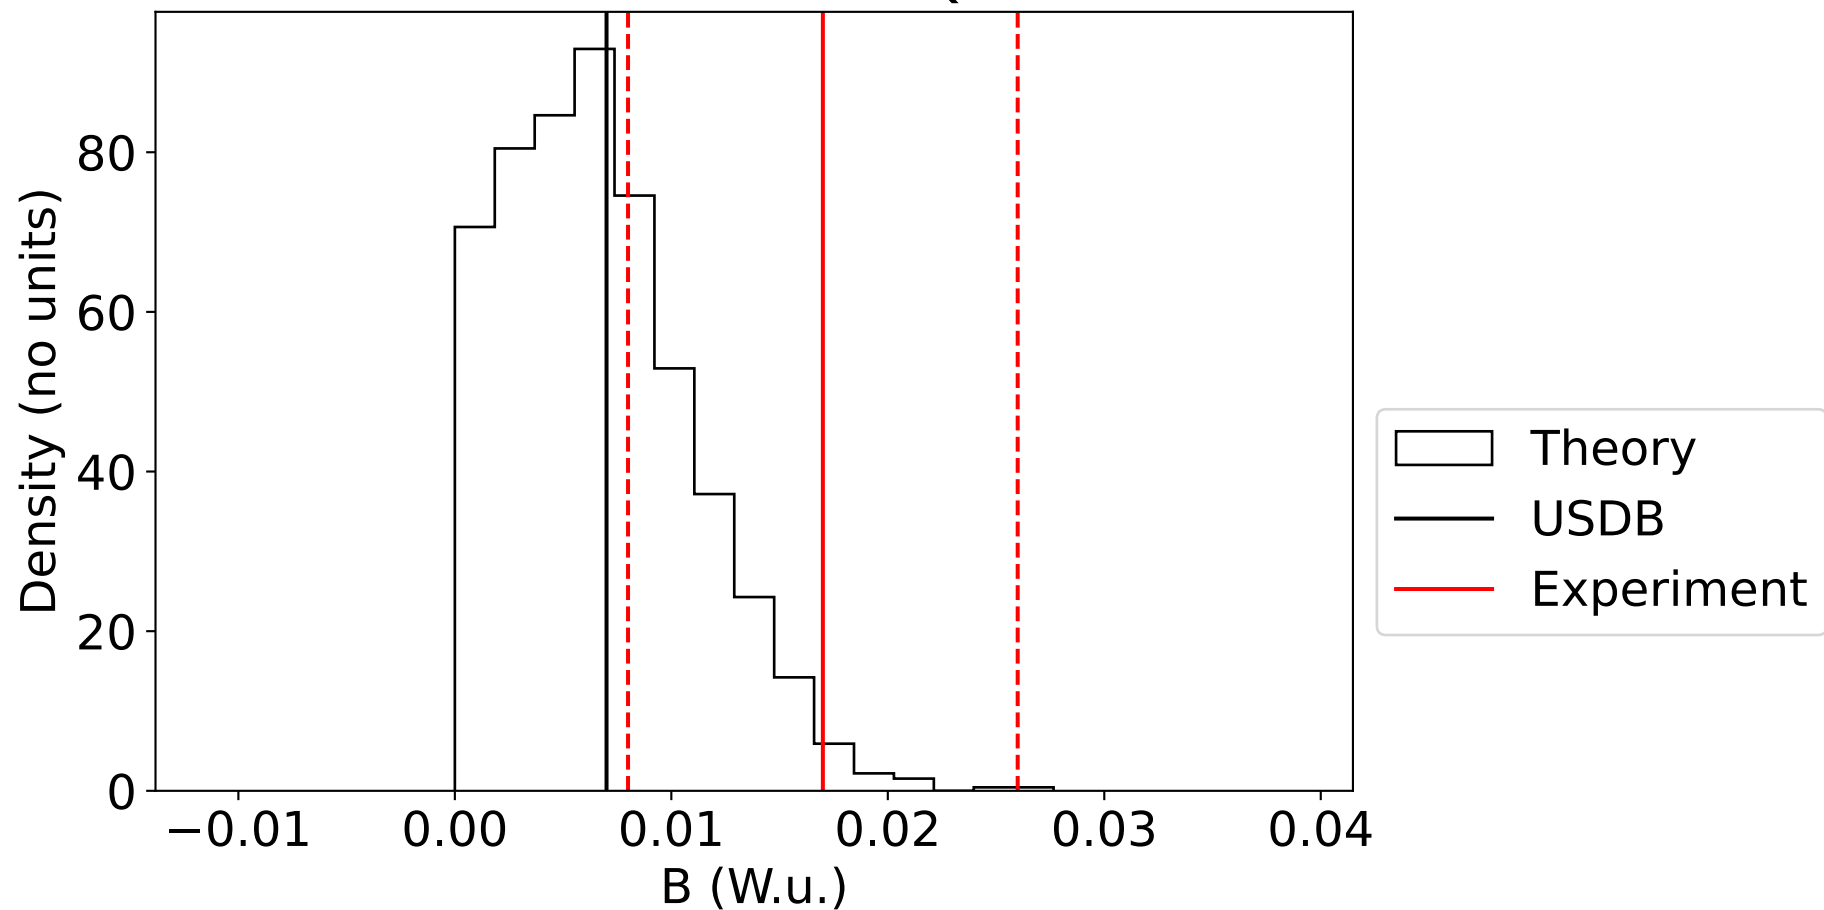

$^{31}\text{P} (7/2_2) \rightarrow (5/2_2)$   
Included in UQ

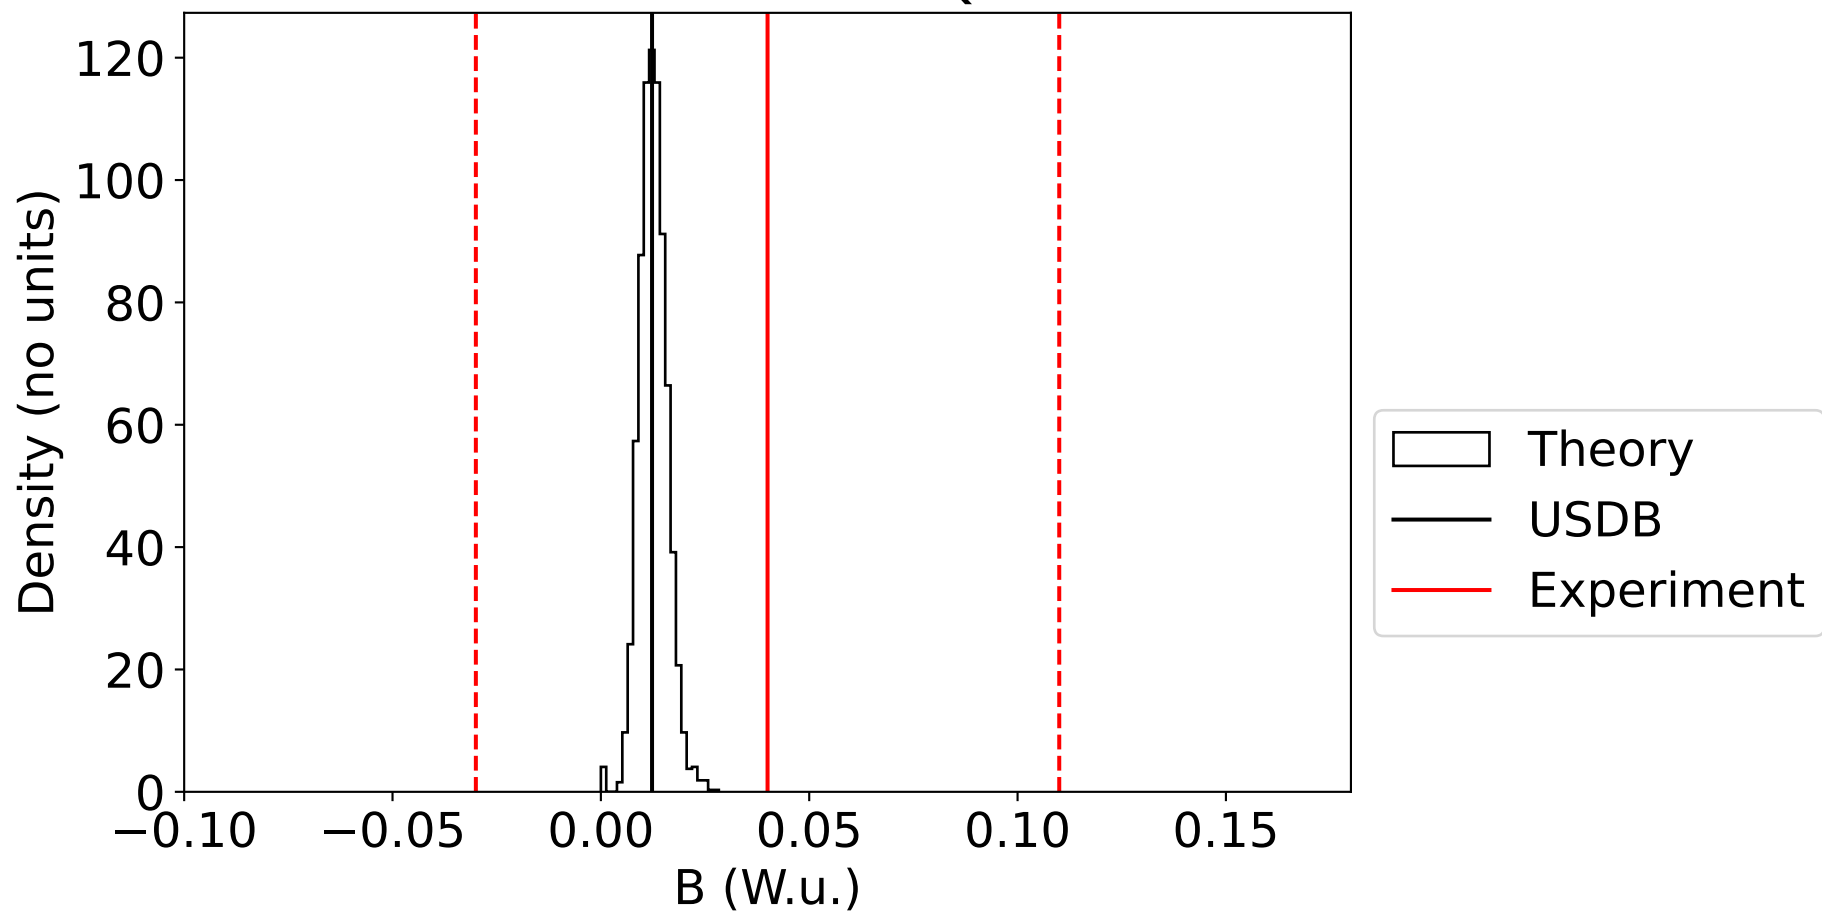

$^{31}\text{P} (7/2_2) \rightarrow (7/2_1)$   
Included in UQ

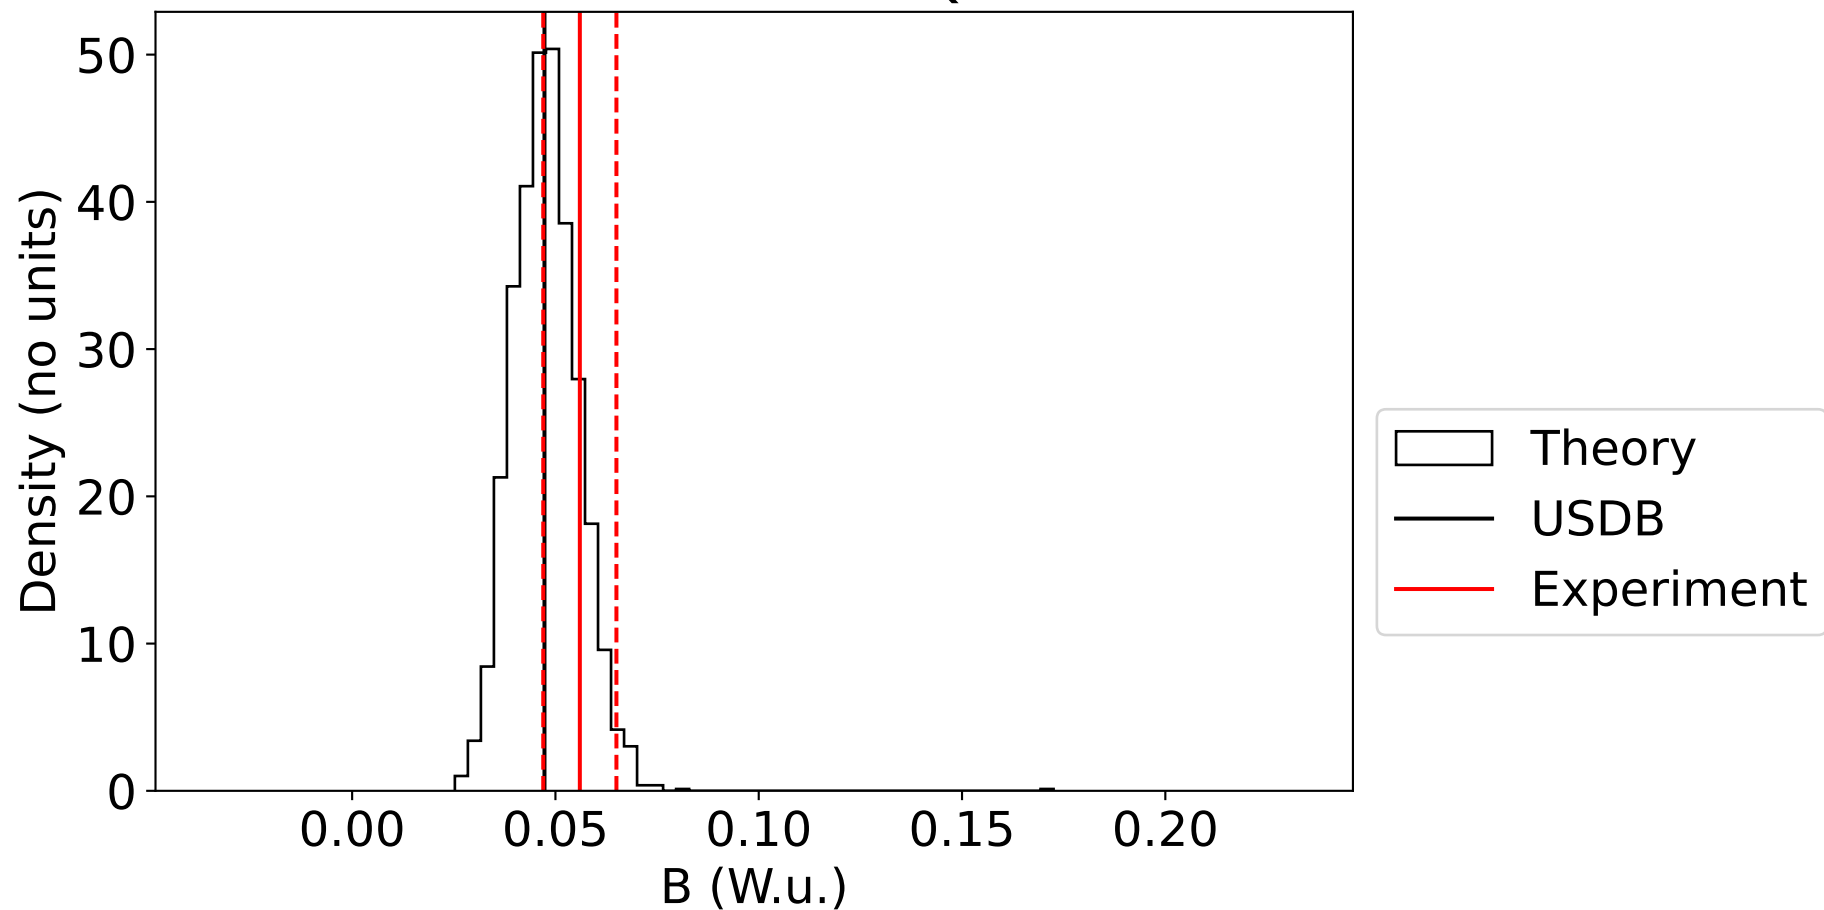



$^{31}\text{P} (5/2_5) \rightarrow (3/2_1)$   
Included in UQ

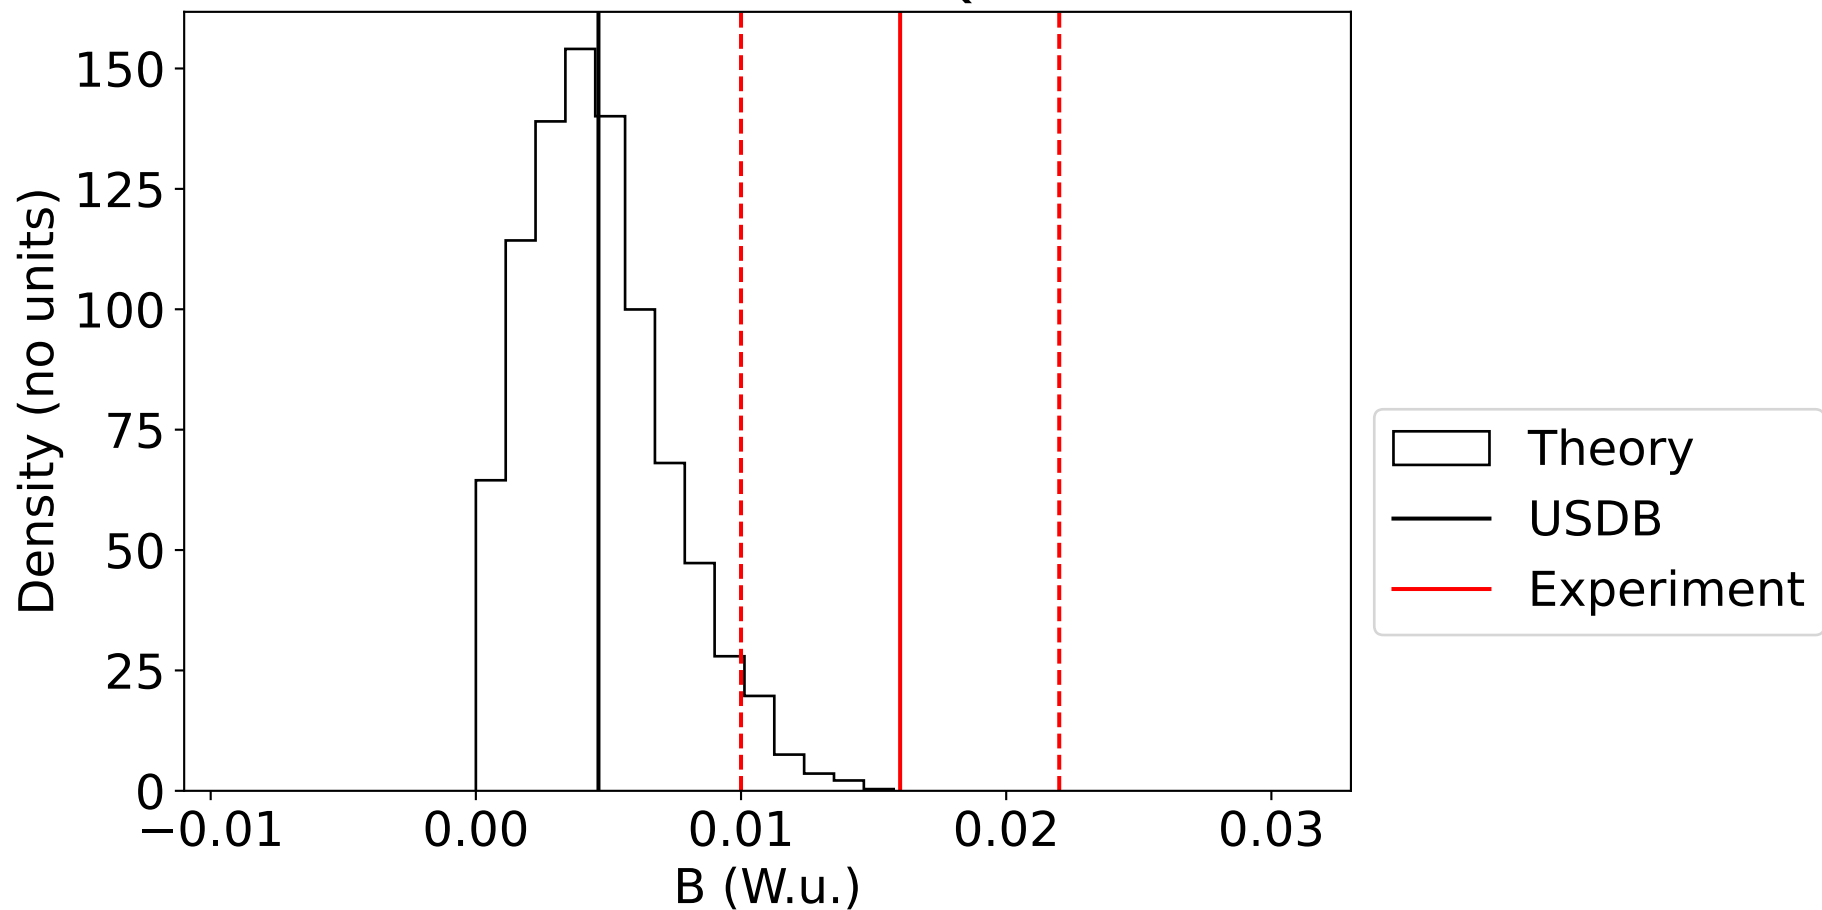

$^{31}\text{P} (5/2_5) \rightarrow (5/2_1)$   
Included in UQ

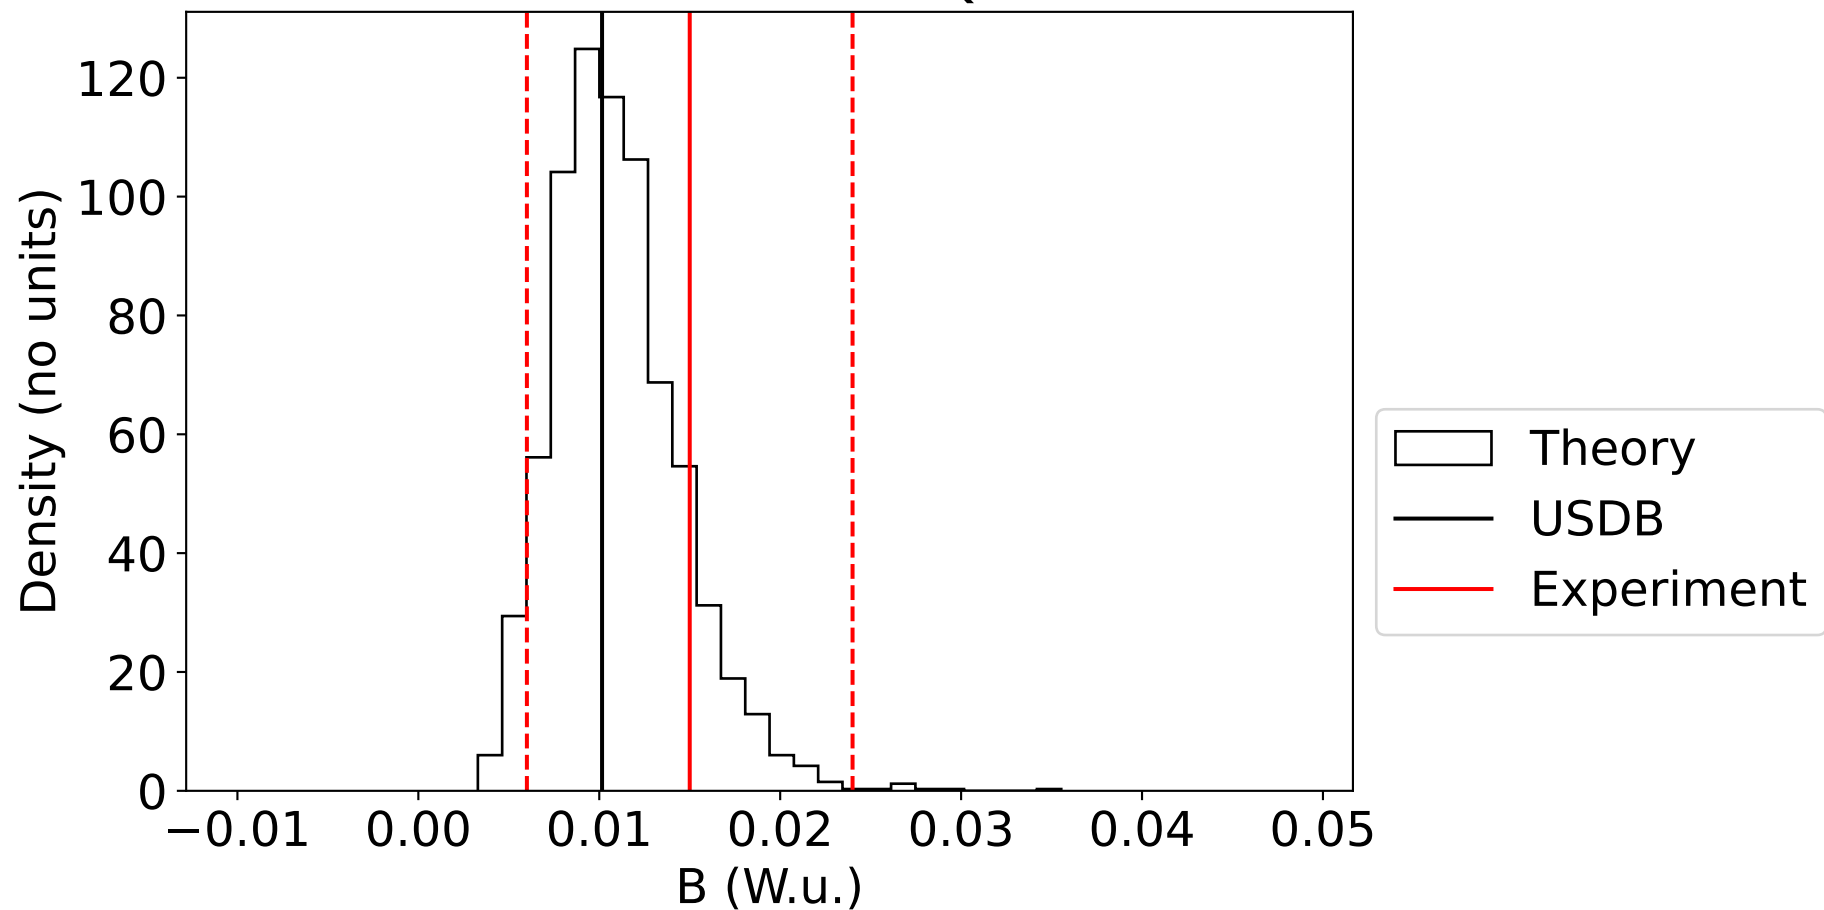

$^{31}\text{P} (9/2_3) \rightarrow (7/2_2)$   
Included in UQ

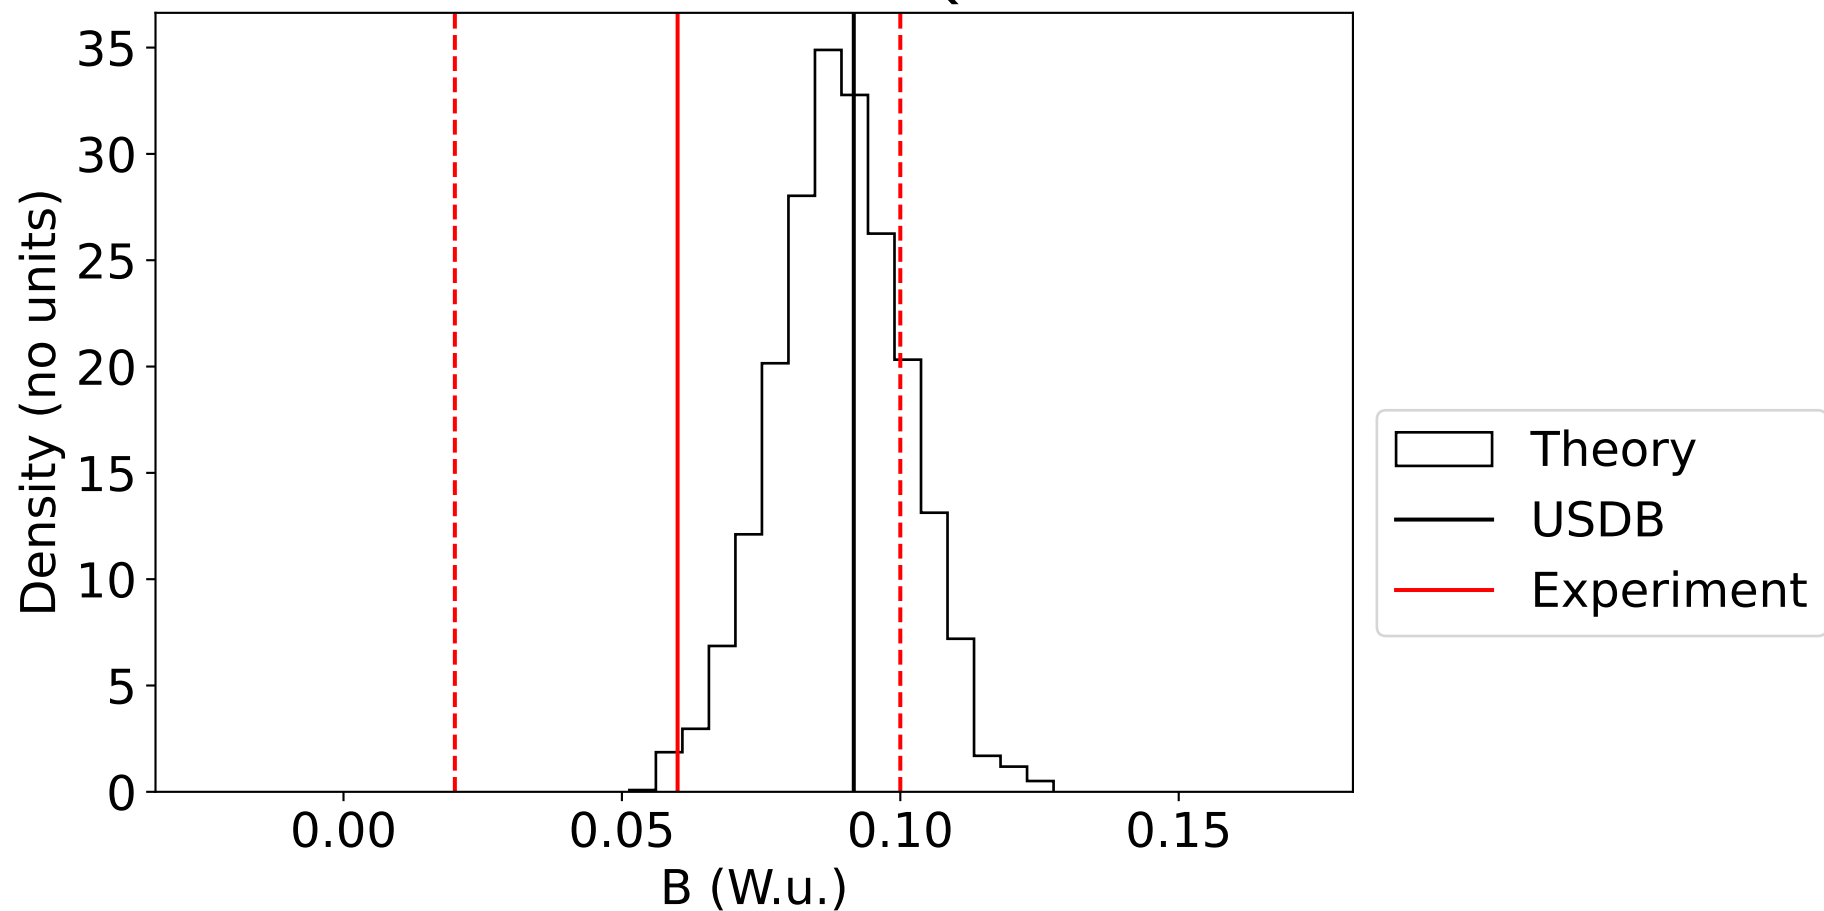

$^{32}\text{P} (2_1) \rightarrow (1_1)$   
Included in UQ

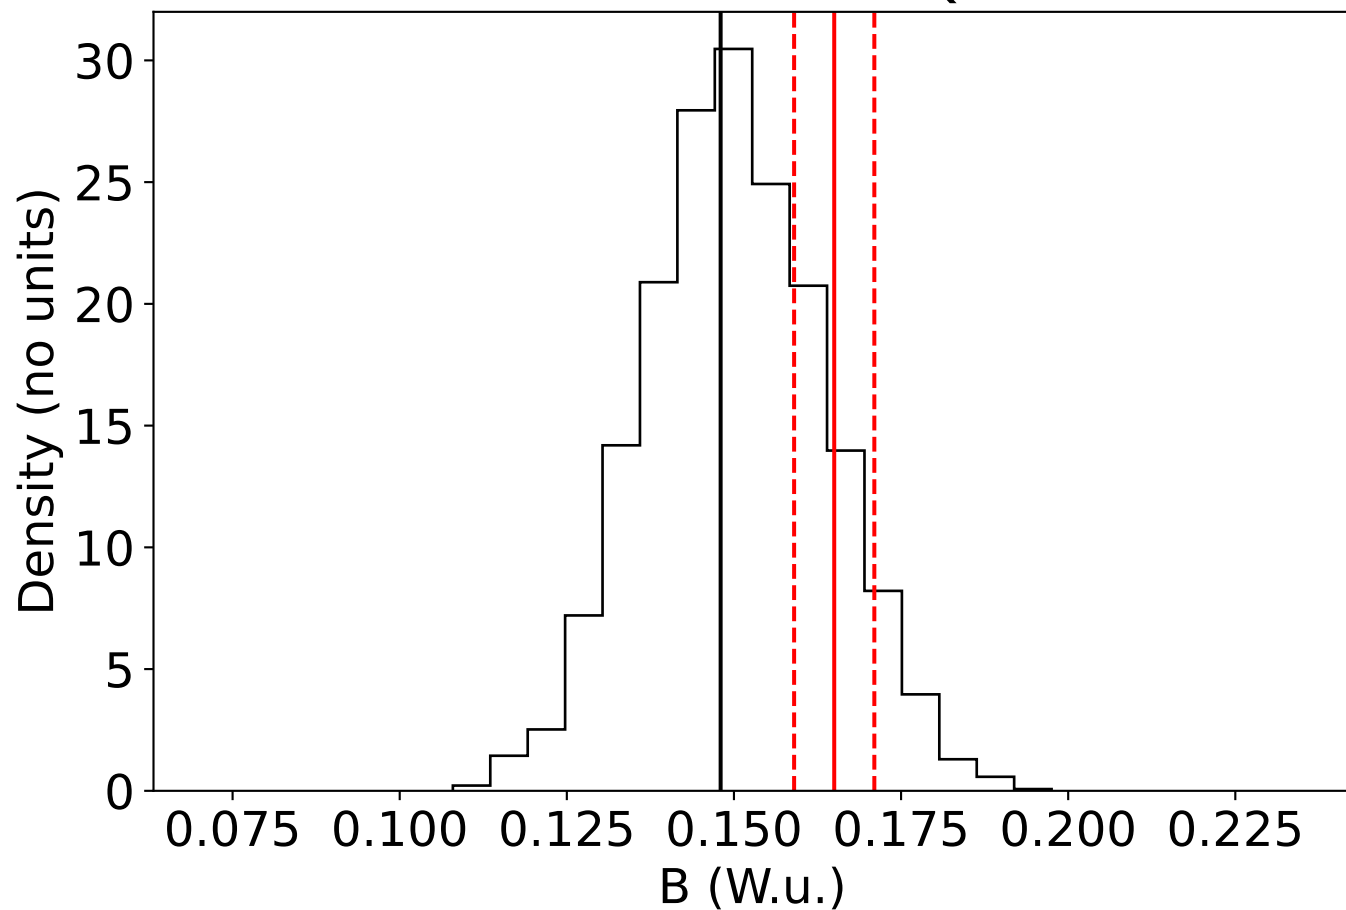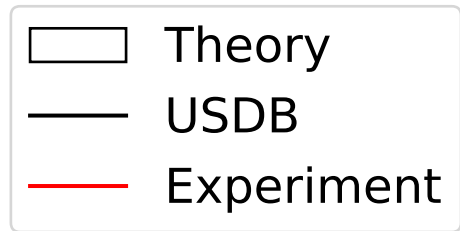

$^{32}\text{P} (0_1) \rightarrow (1_1)$   
Included in UQ

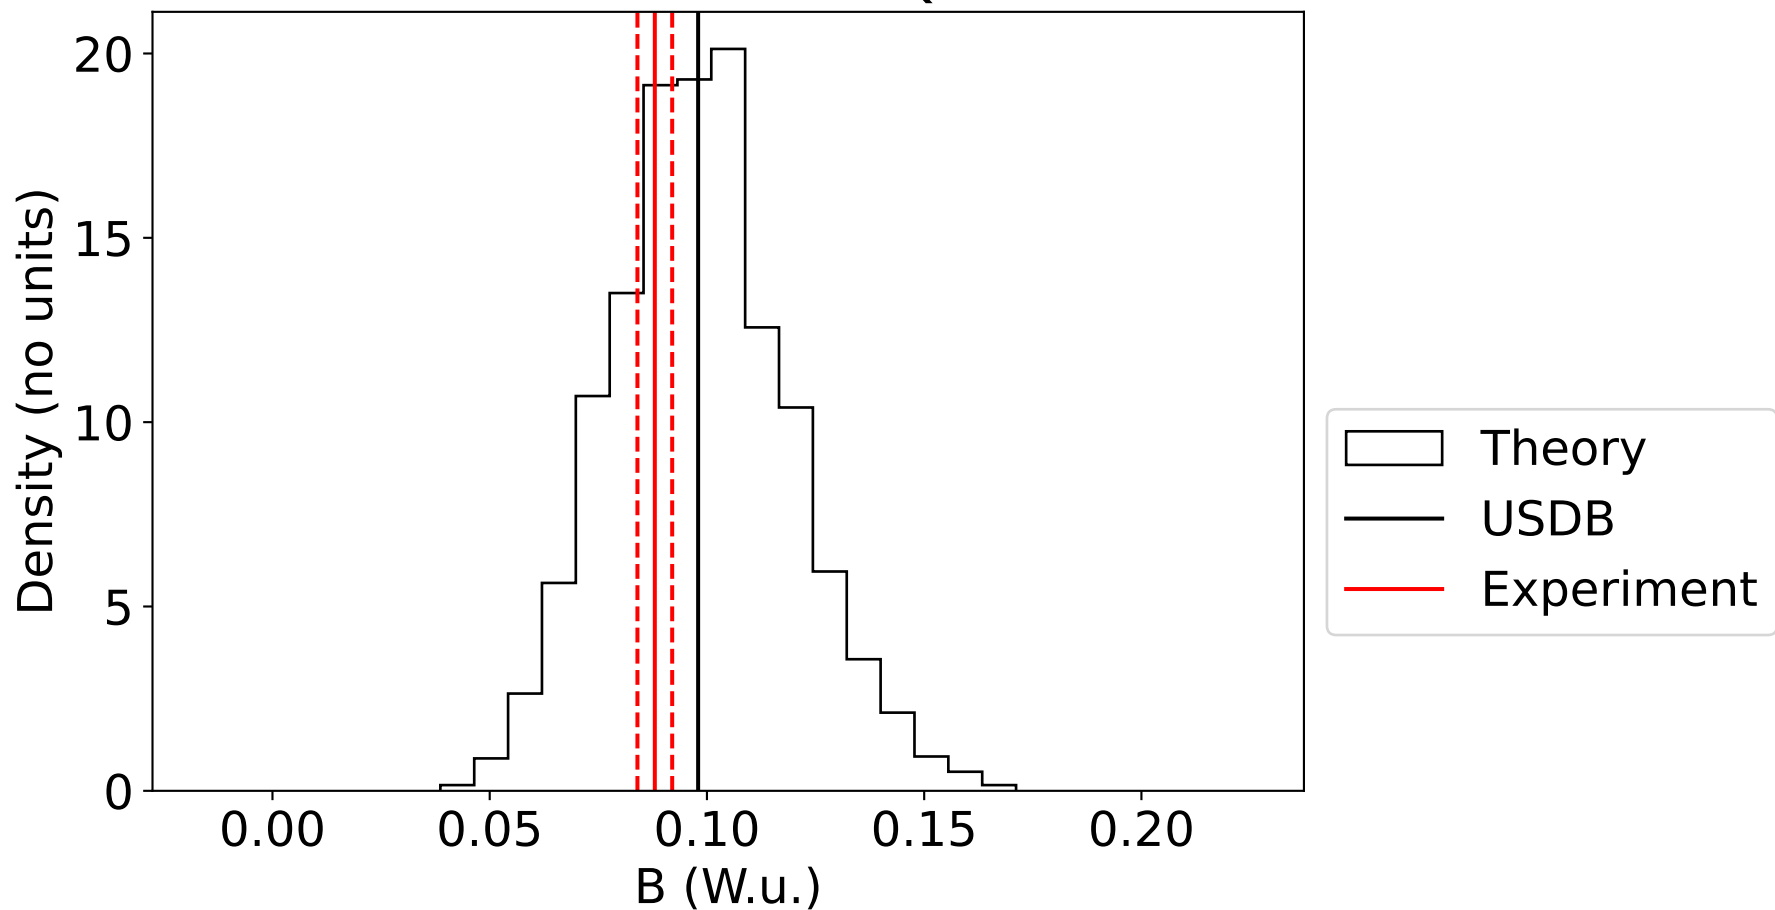

$^{32}\text{P} (1_2) \rightarrow (2_1)$   
Included in UQ

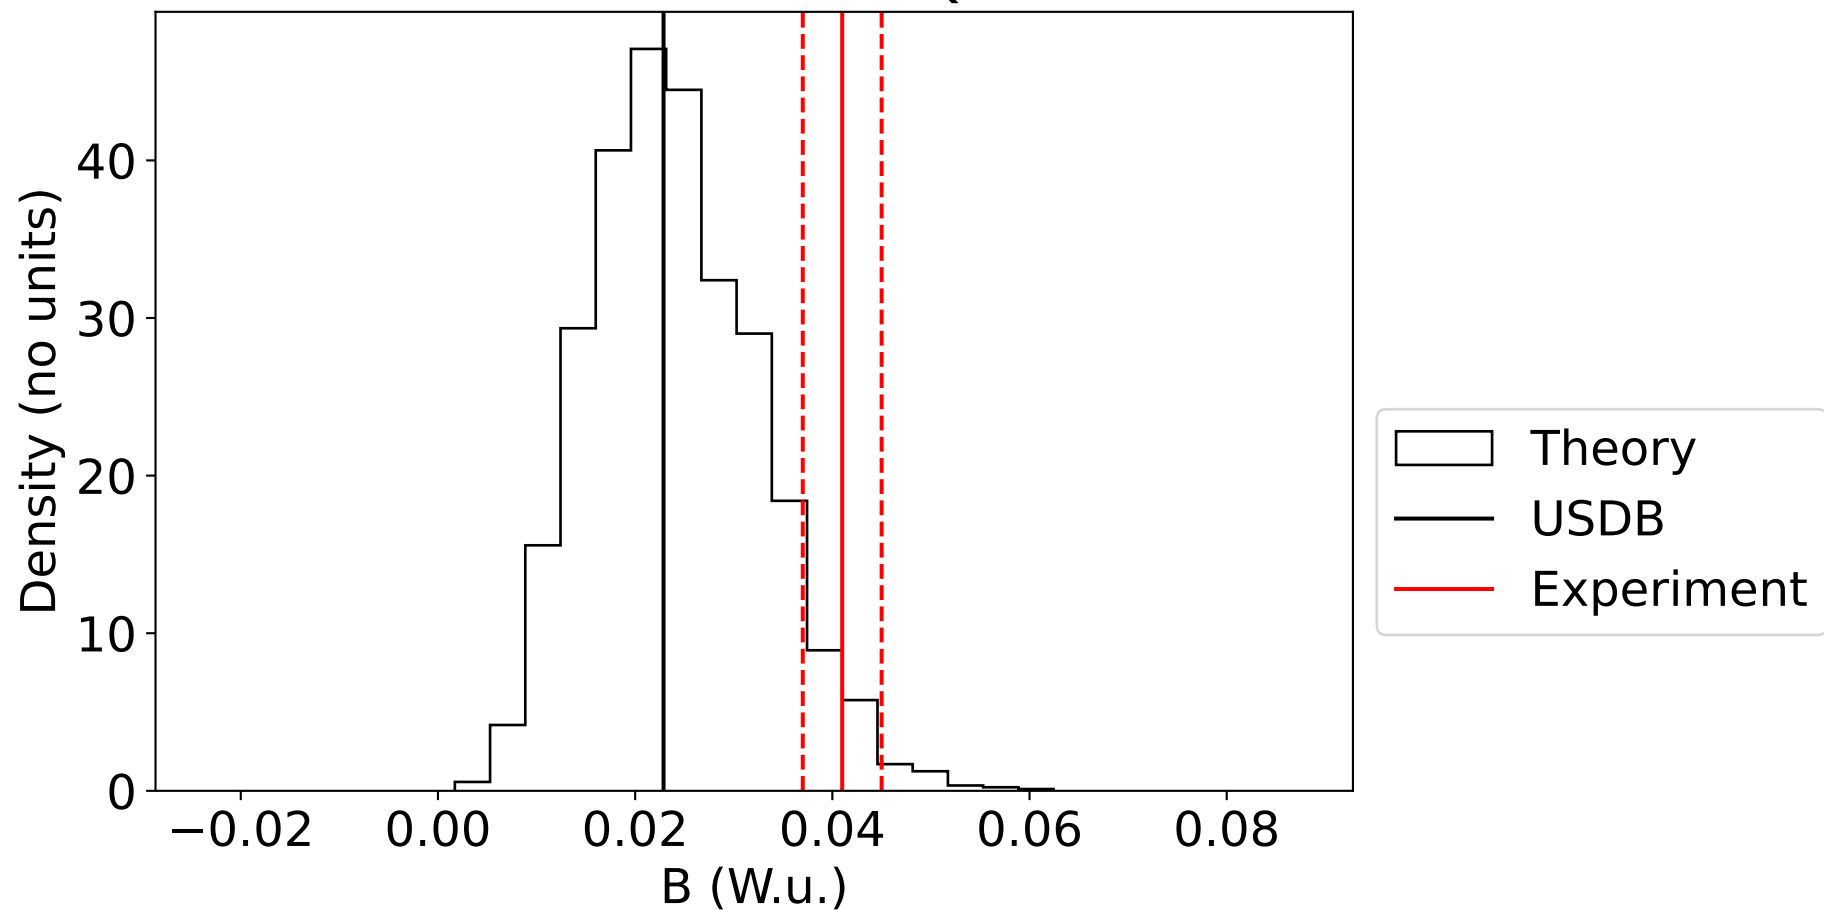

$^{32}\text{P} (1_2) \rightarrow (0_1)$   
Included in UQ

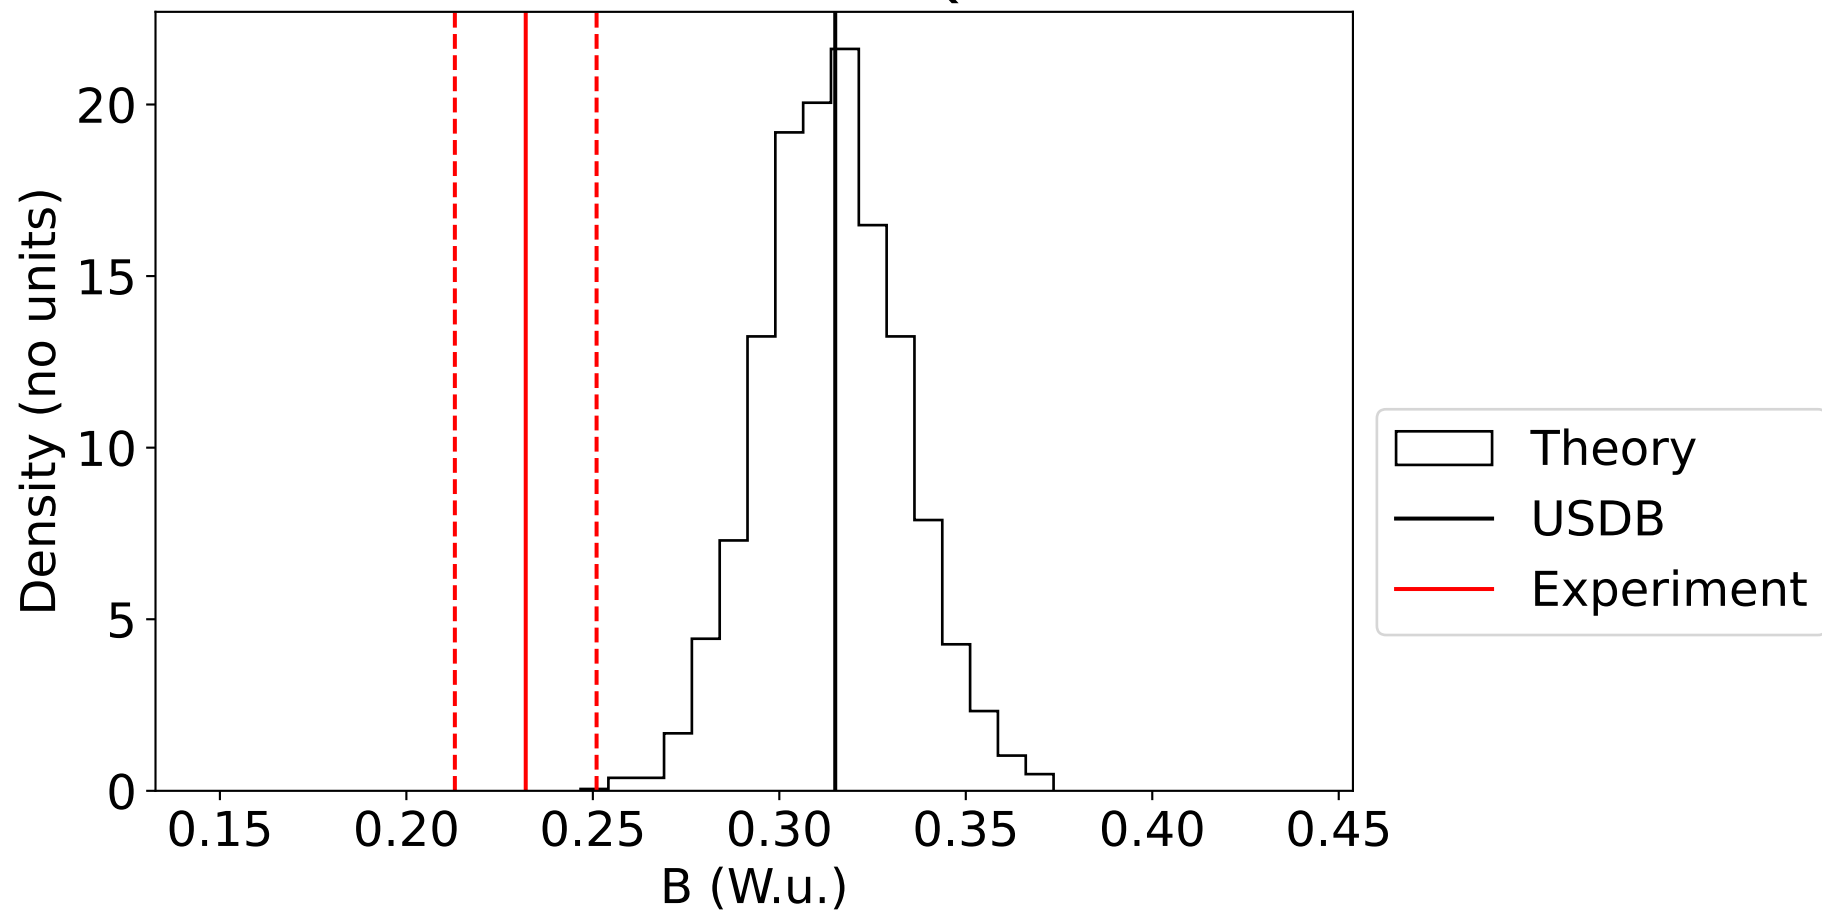

$^{32}\text{P} (3_1) \rightarrow (2_2)$   
Included in UQ

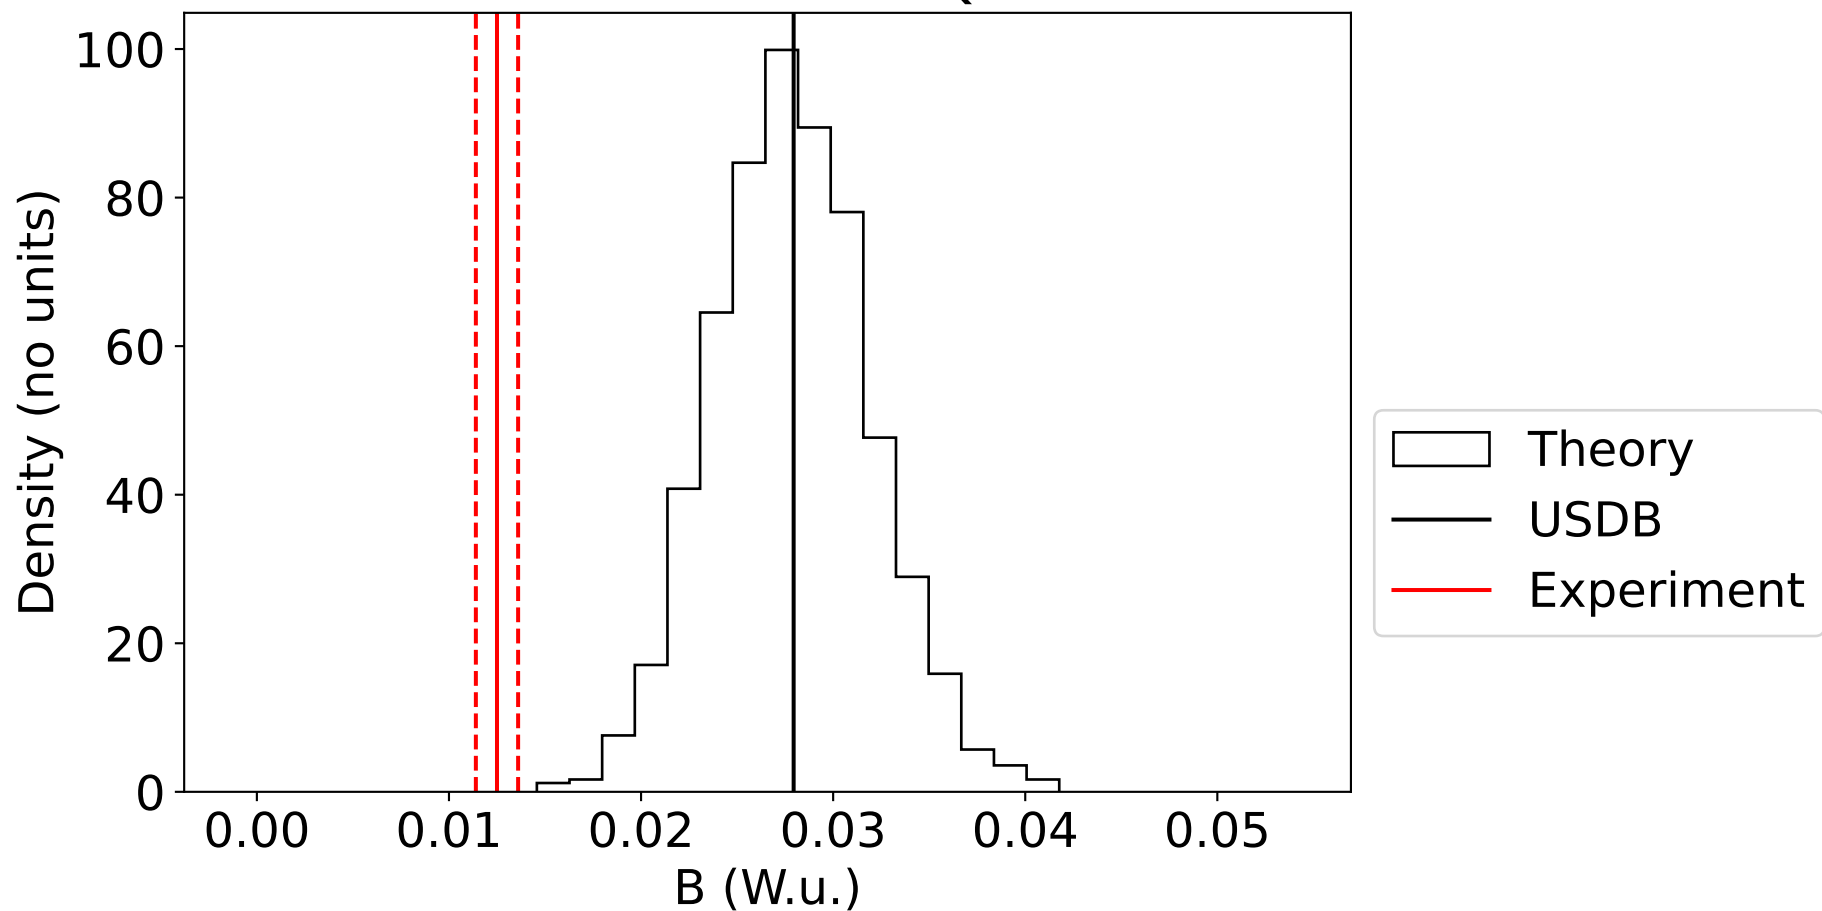



$^{32}\text{P} (3_2) \rightarrow (2_1)$   
Included in UQ

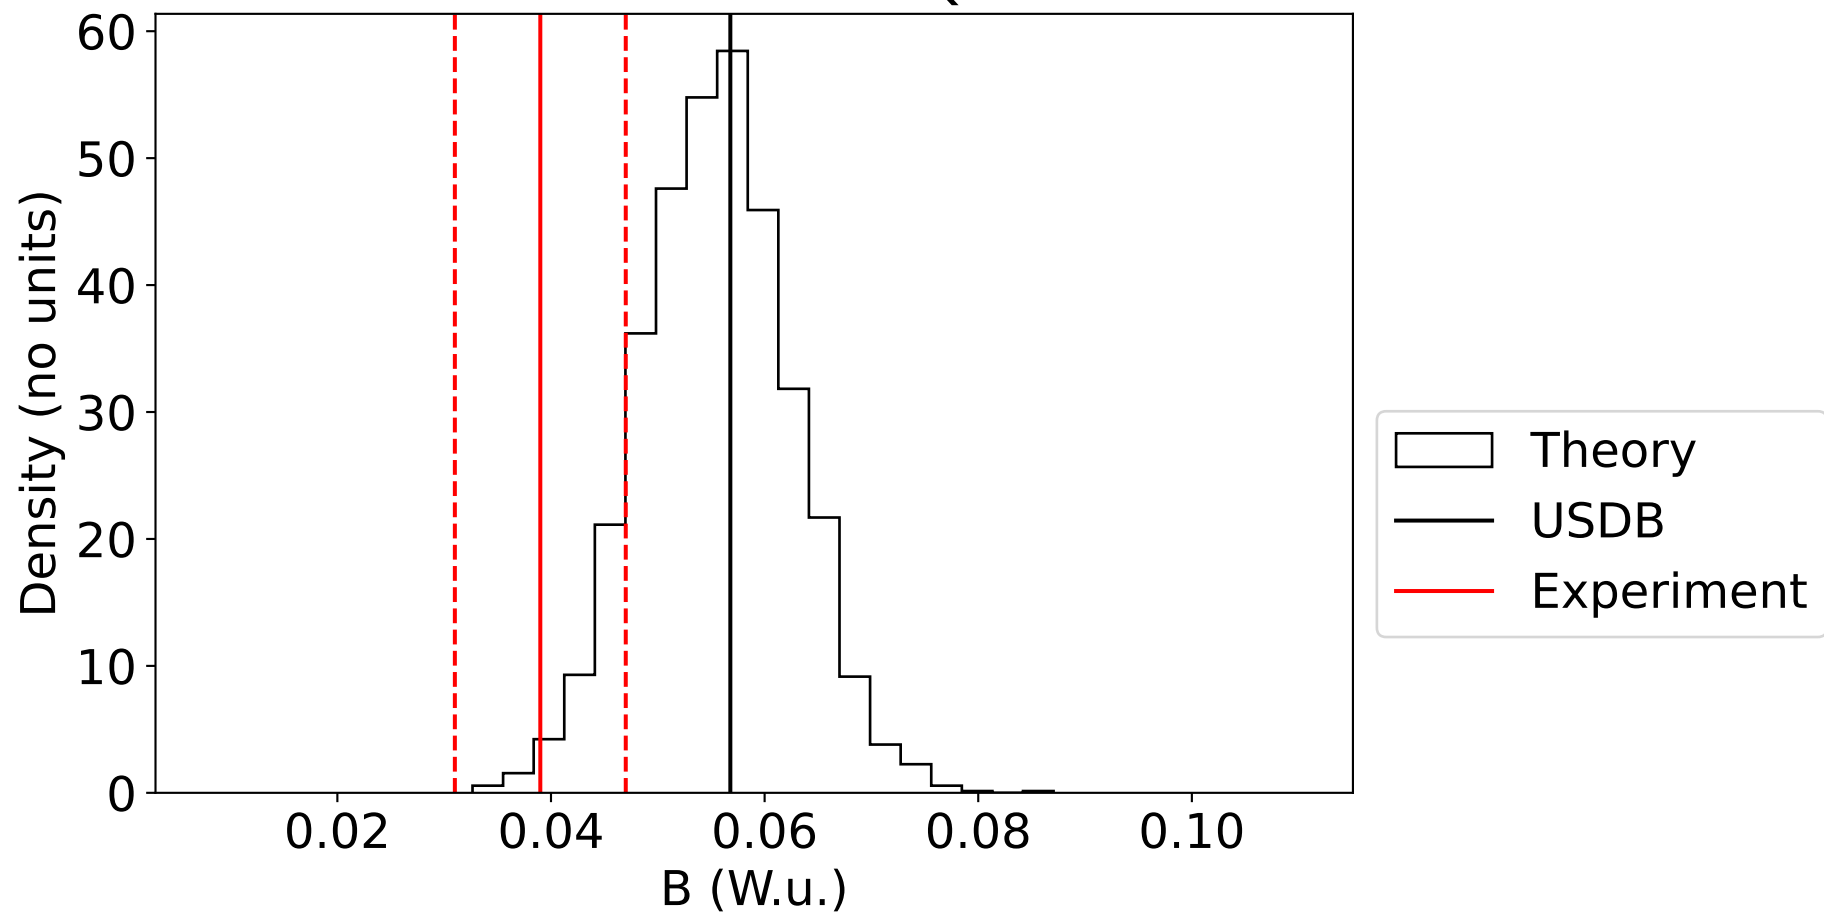

$^{32}\text{P} (2_3) \rightarrow (2_2)$   
Included in UQ

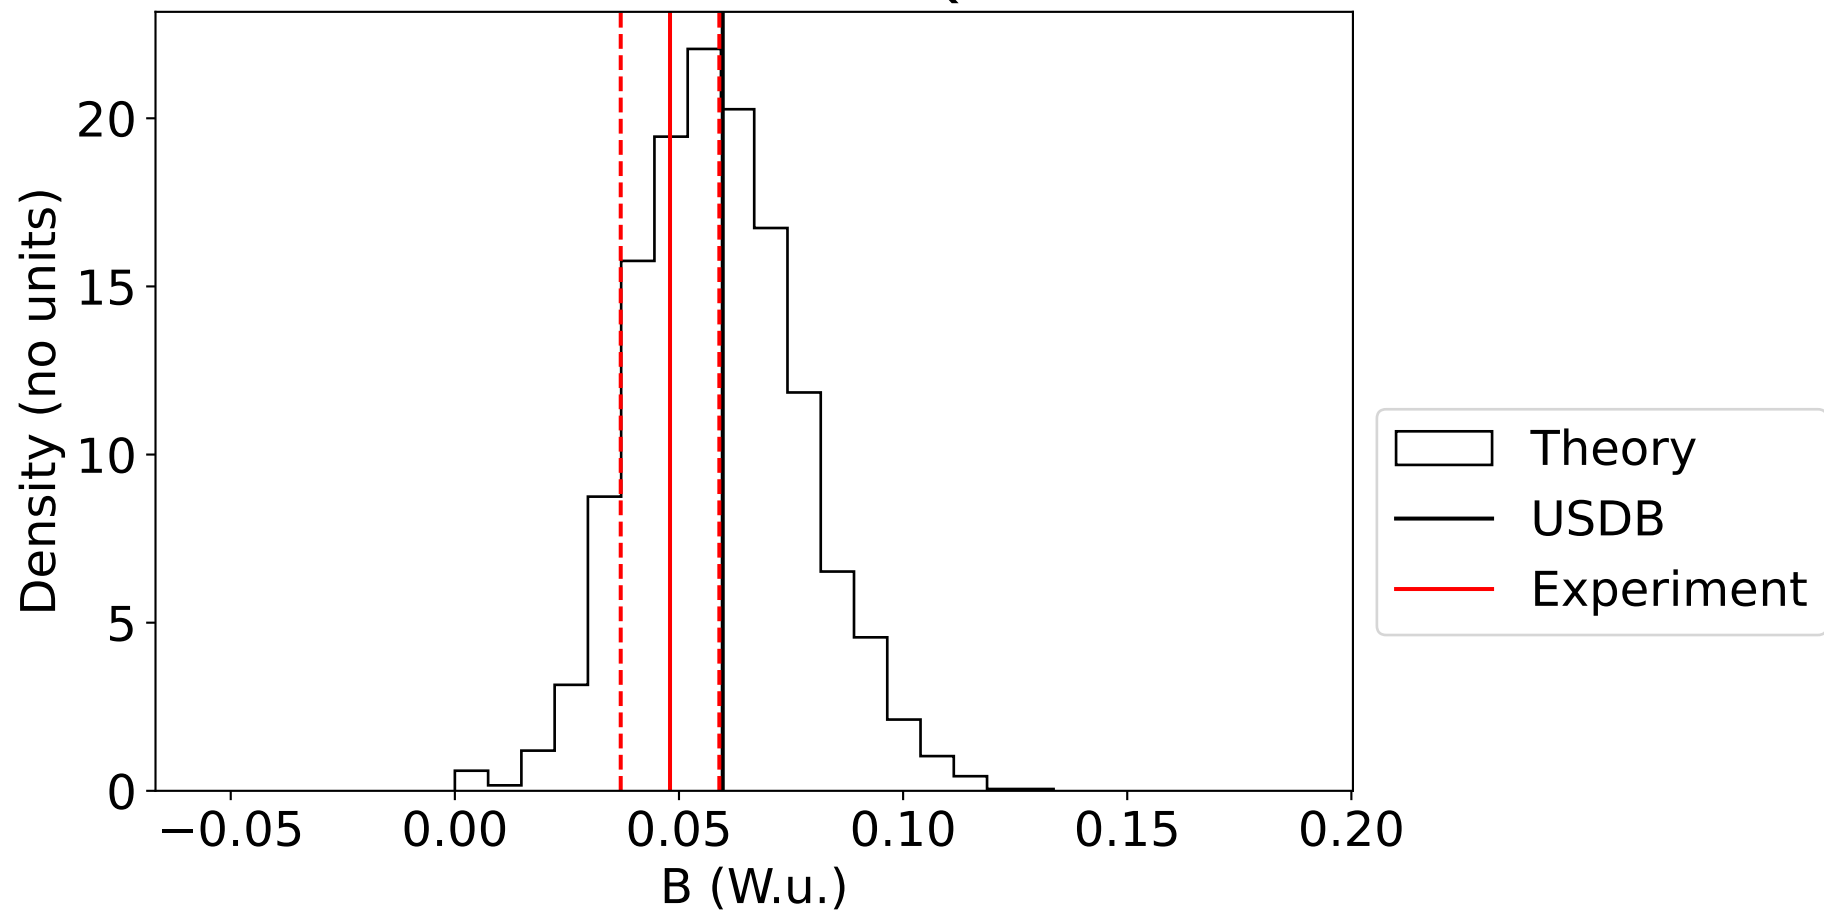

$^{32}\text{P} (2_4) \rightarrow (1_1)$   
Included in UQ

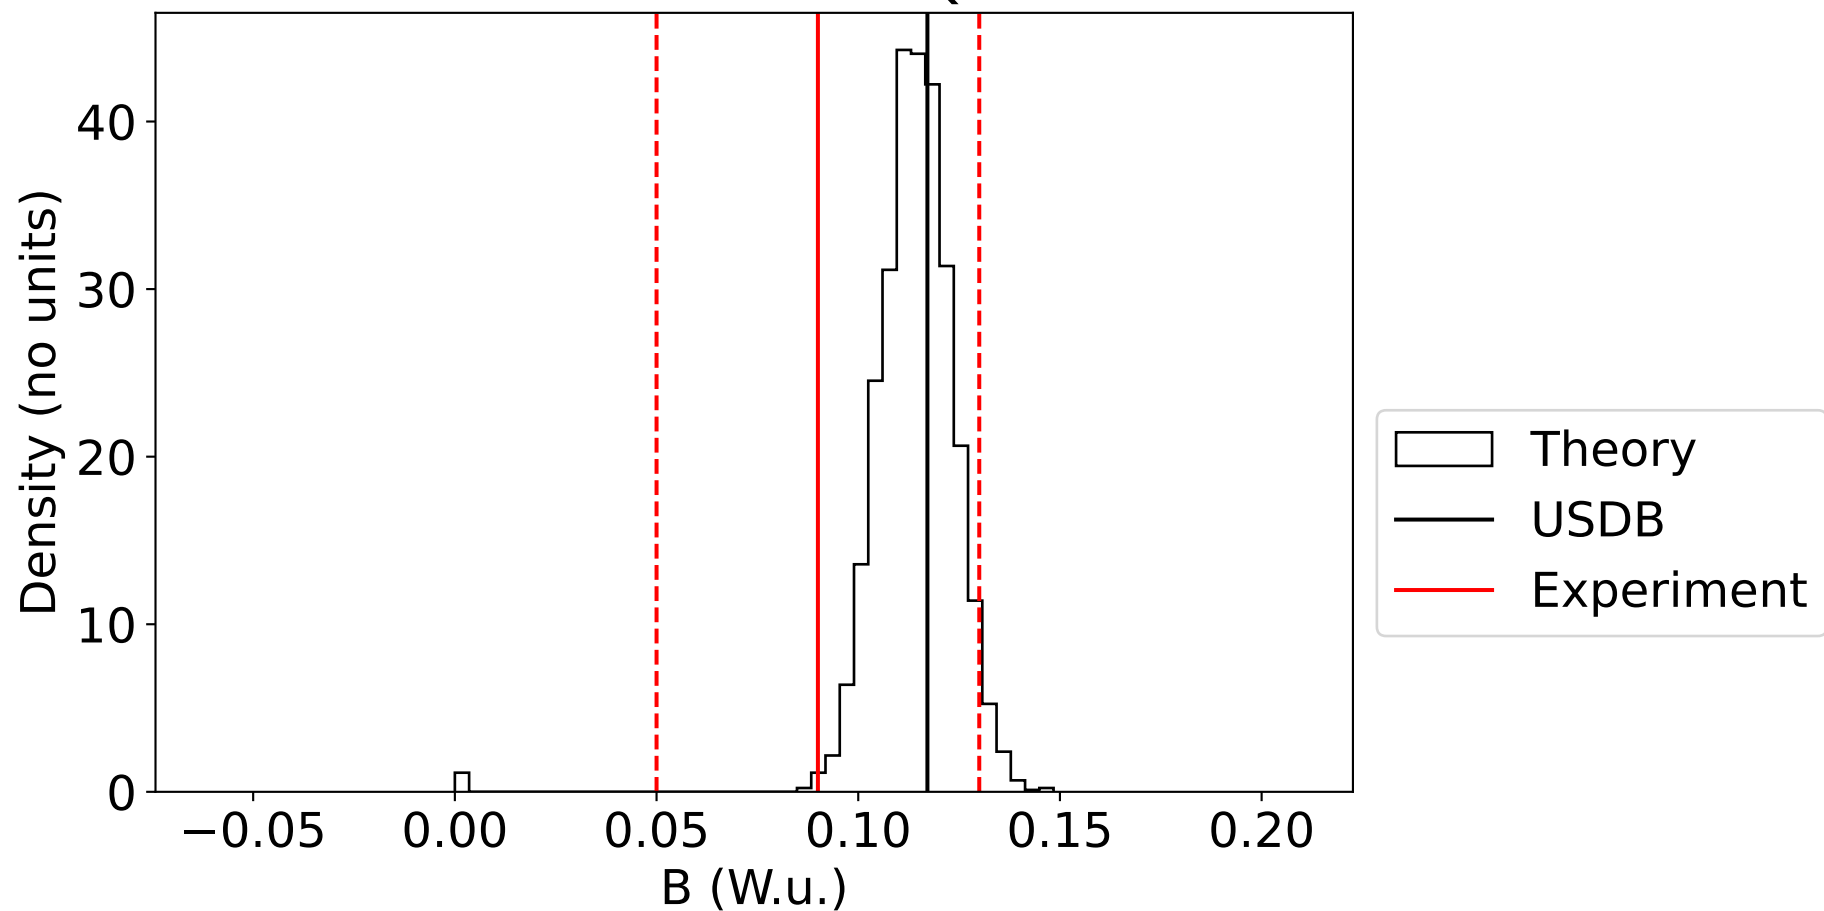

$^{32}\text{P} (2_4) \rightarrow (3_1)$   
Included in UQ

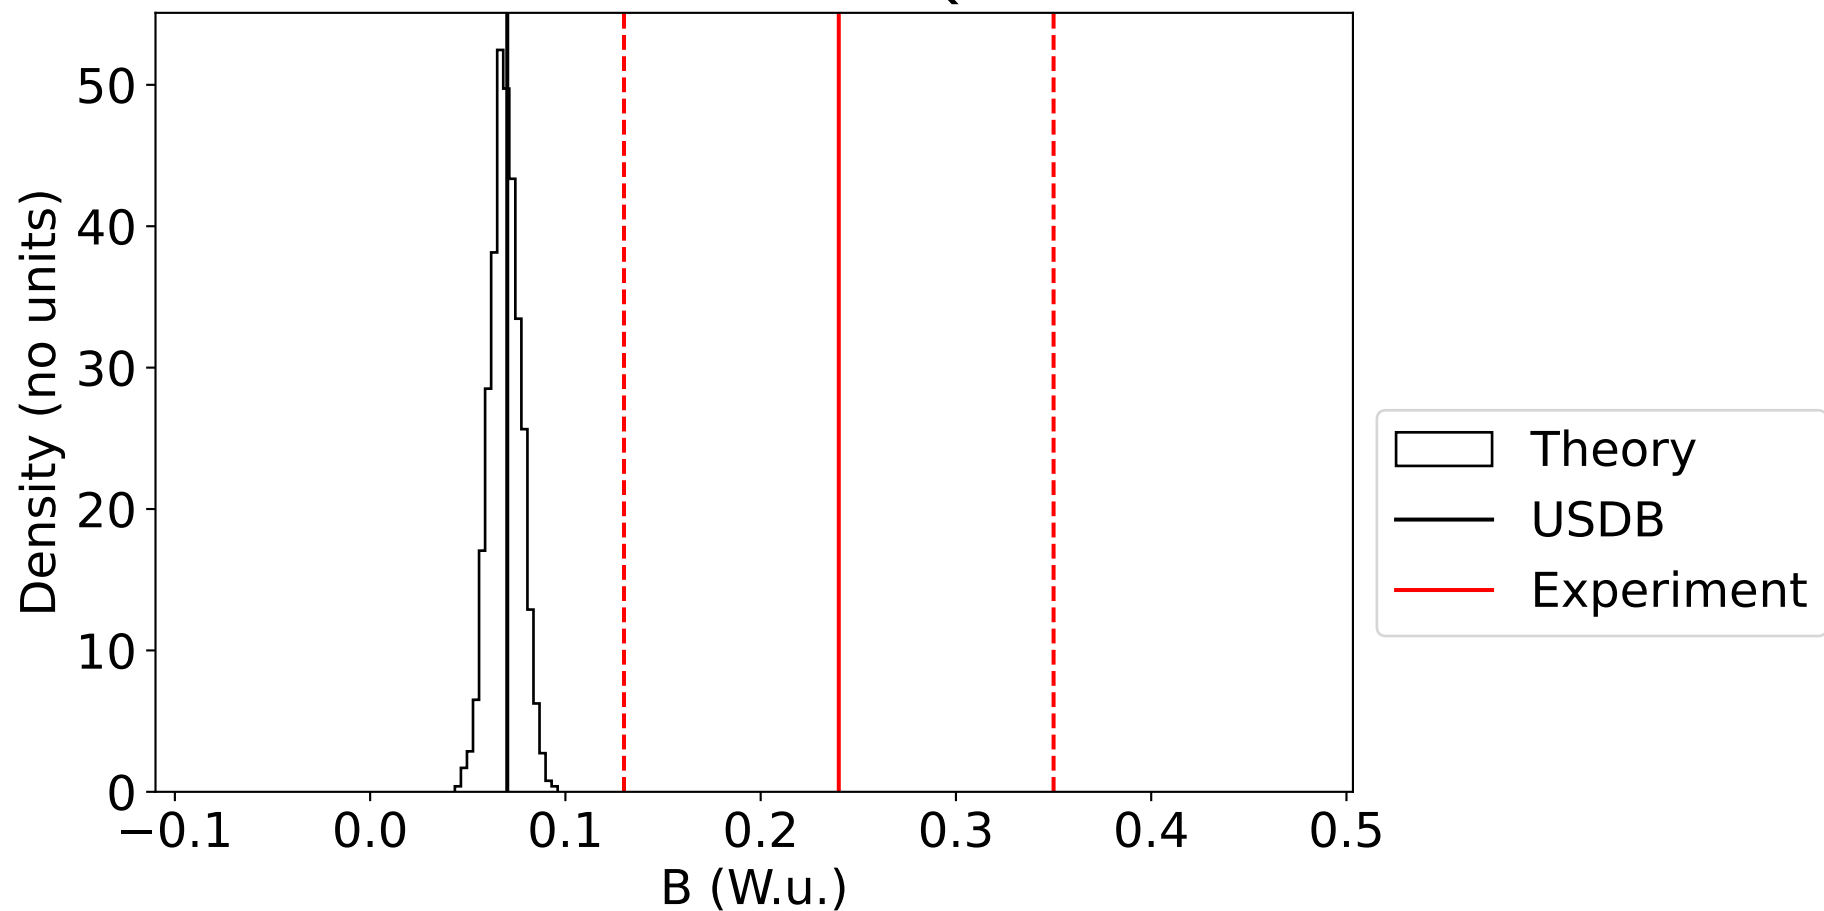

$^{32}\text{P} (1_4) \rightarrow (0_1)$   
Included in UQ

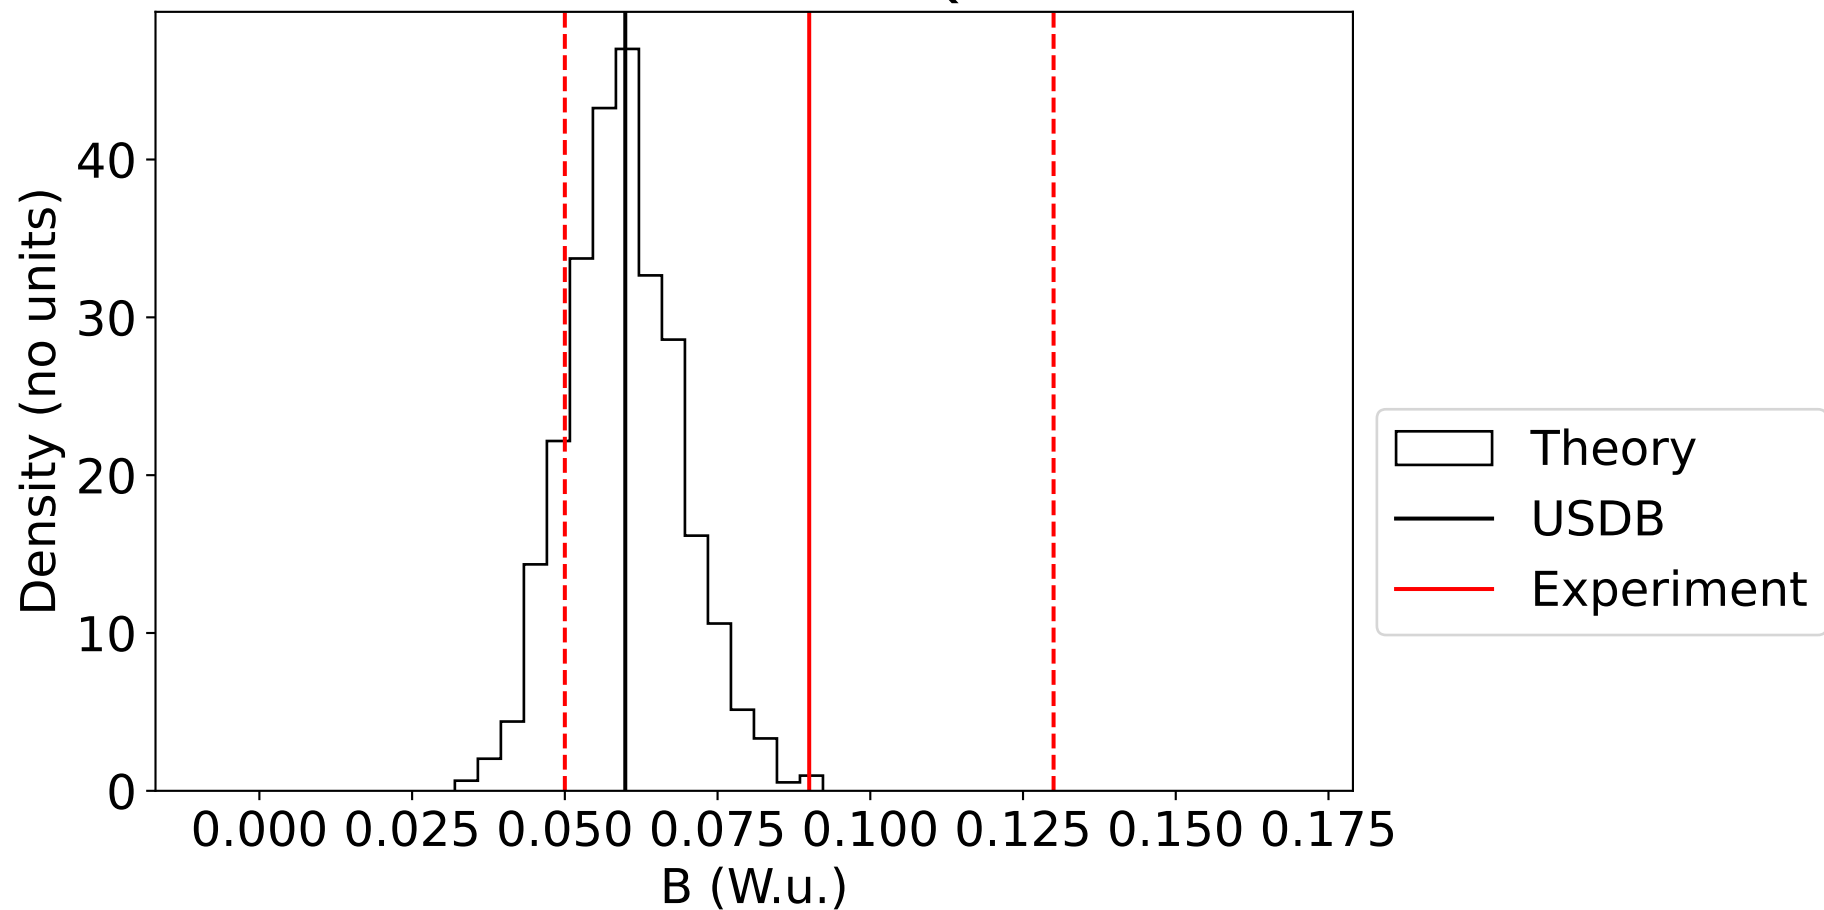

$^{32}\text{P} (4_1) \rightarrow (3_2)$   
Included in UQ

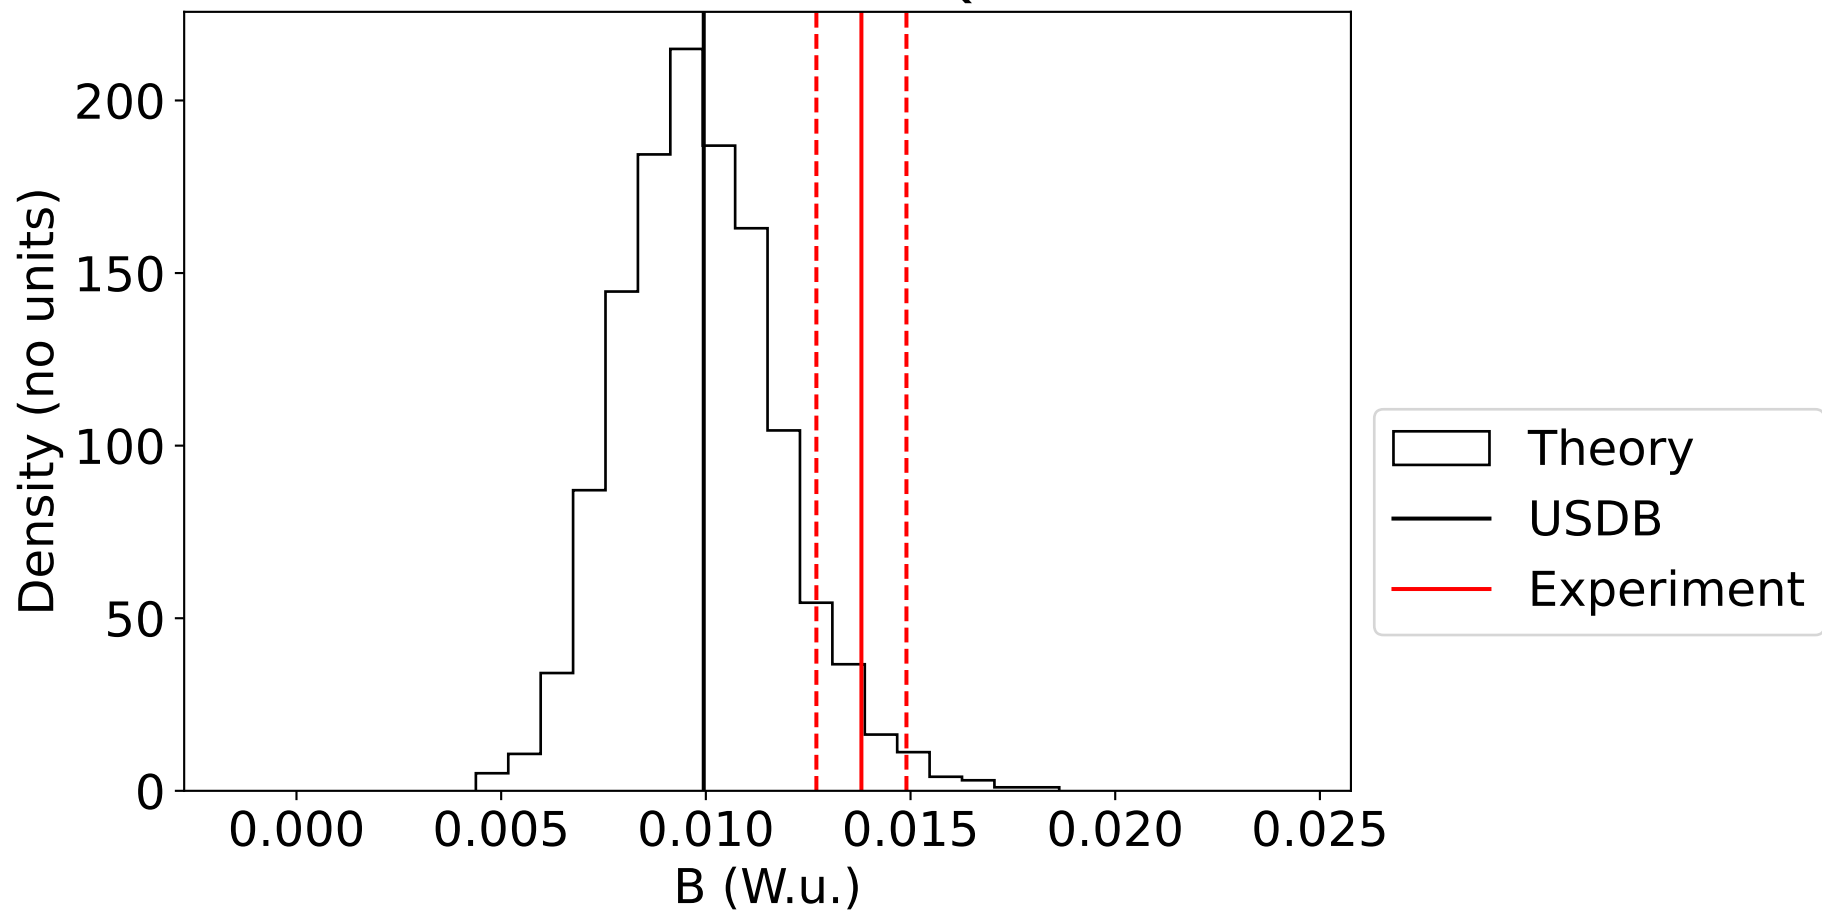

$^{32}\text{P} (5_1) \rightarrow (4_1)$   
Included in UQ

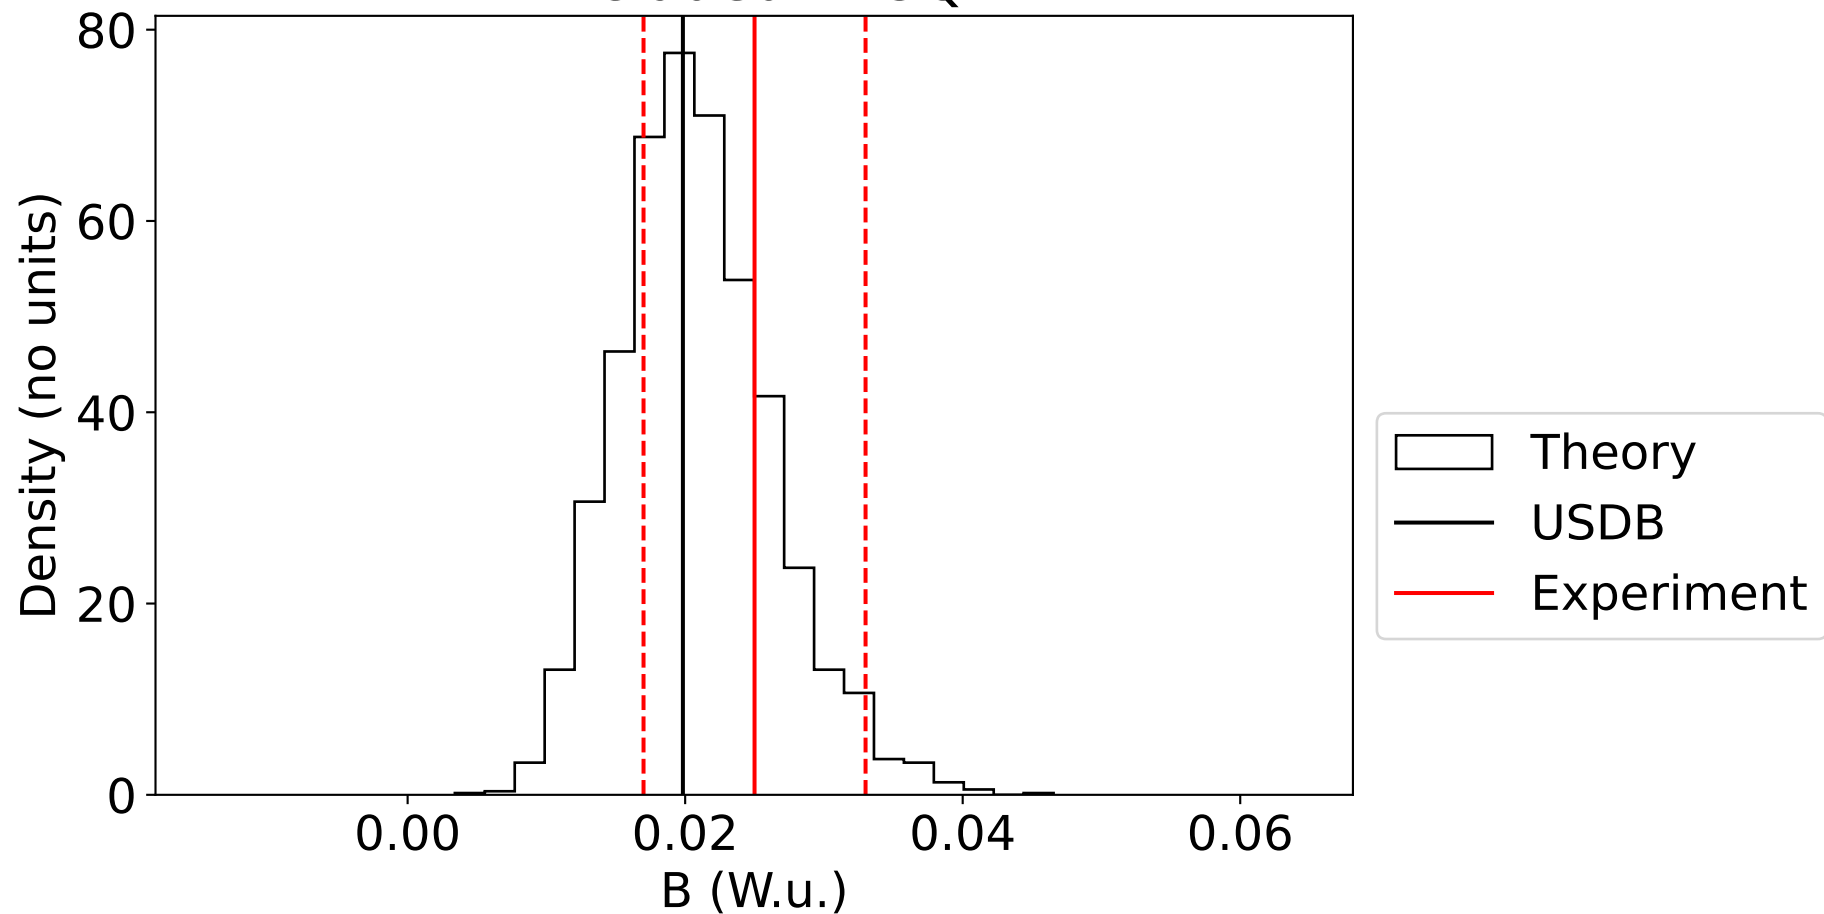

$^{33}\text{P} (3/2_1) \rightarrow (1/2_1)$   
Included in UQ

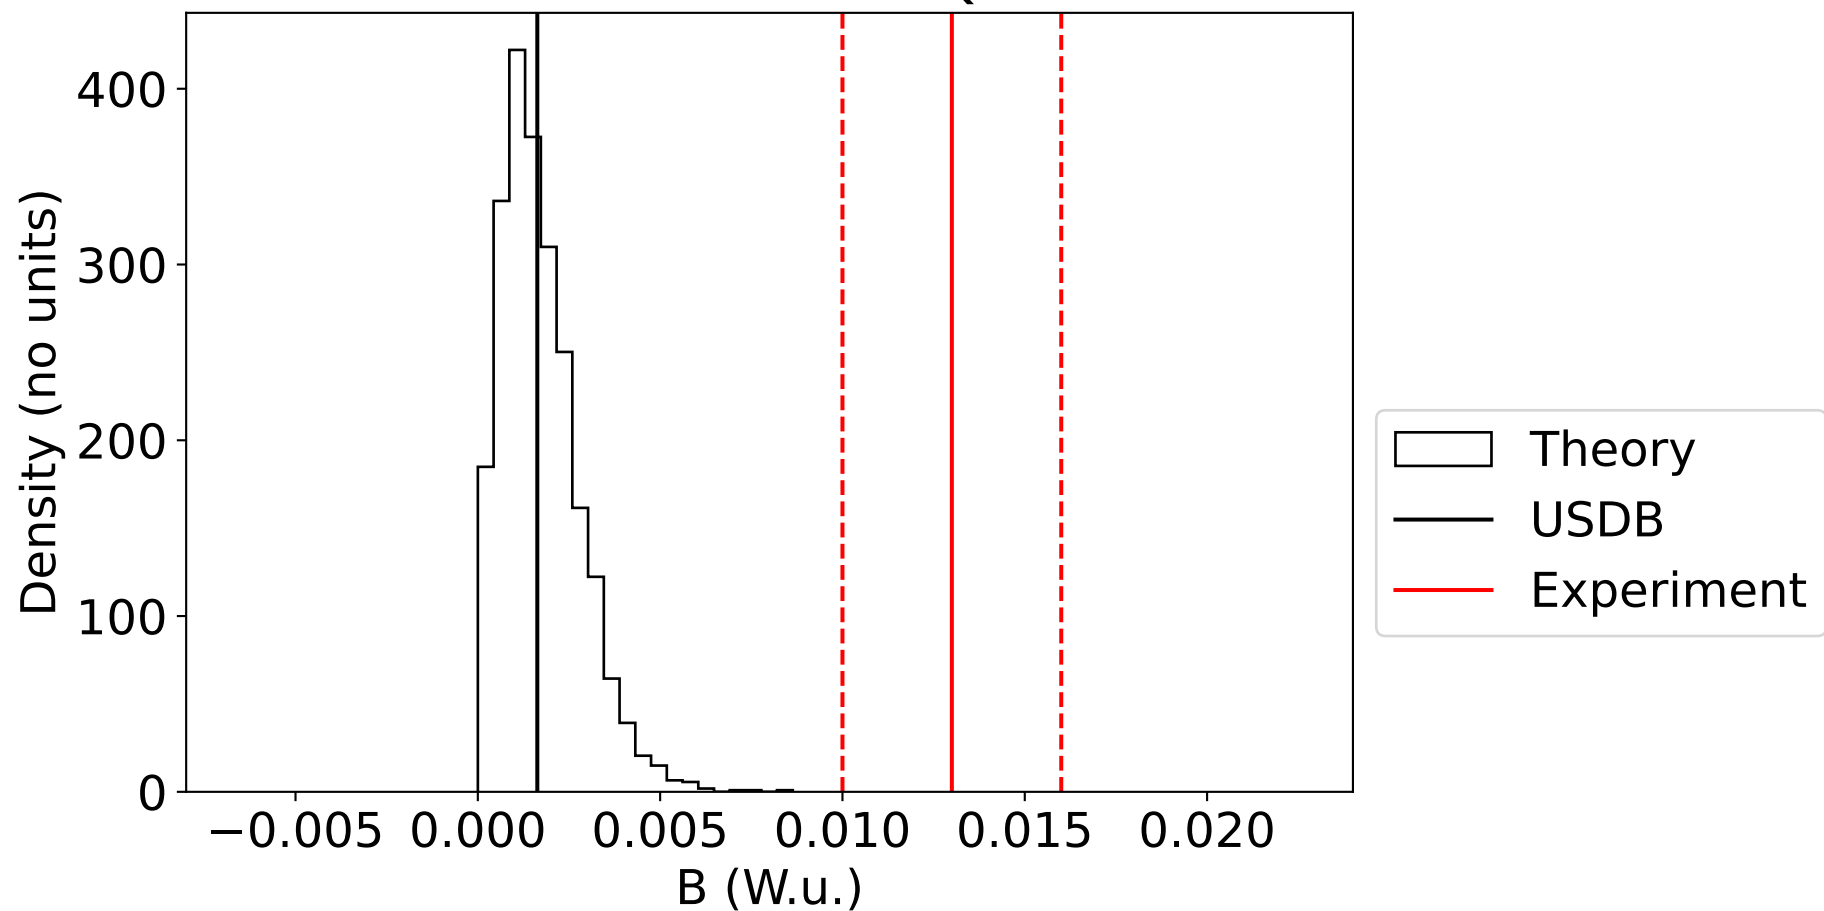



$^{33}\text{P} (3/2_2) \rightarrow (5/2_1)$   
Included in UQ

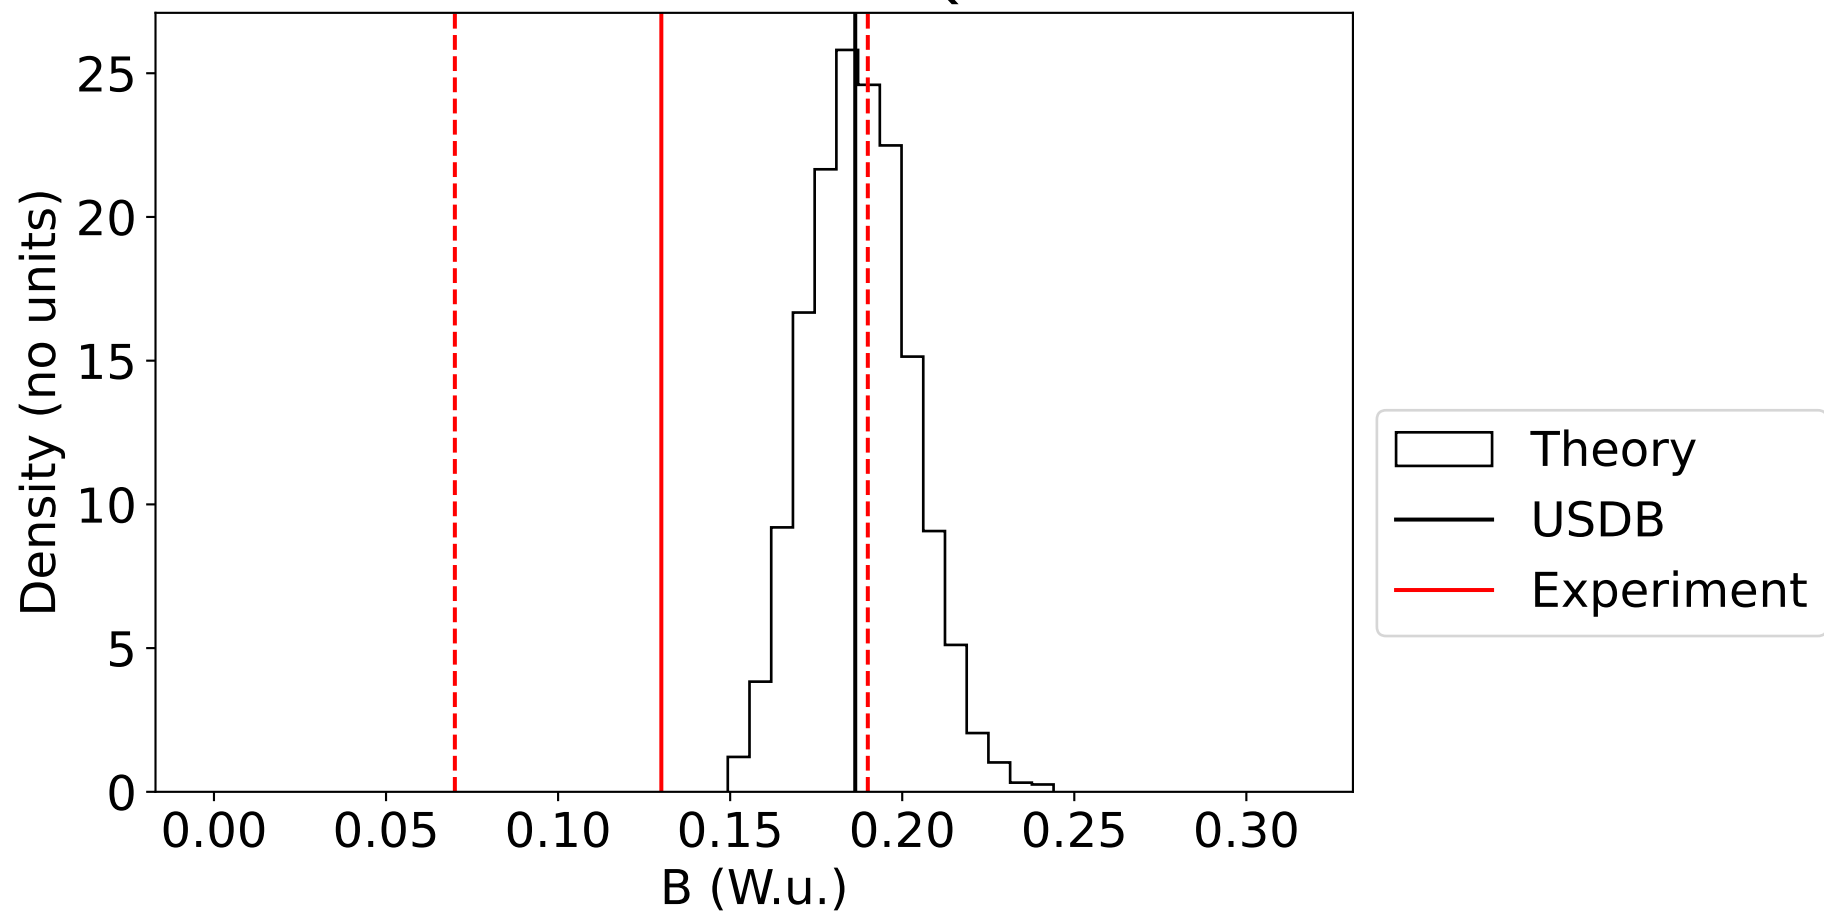

$^{33}\text{P} (3/2_2) \rightarrow (1/2_1)$   
Included in UQ

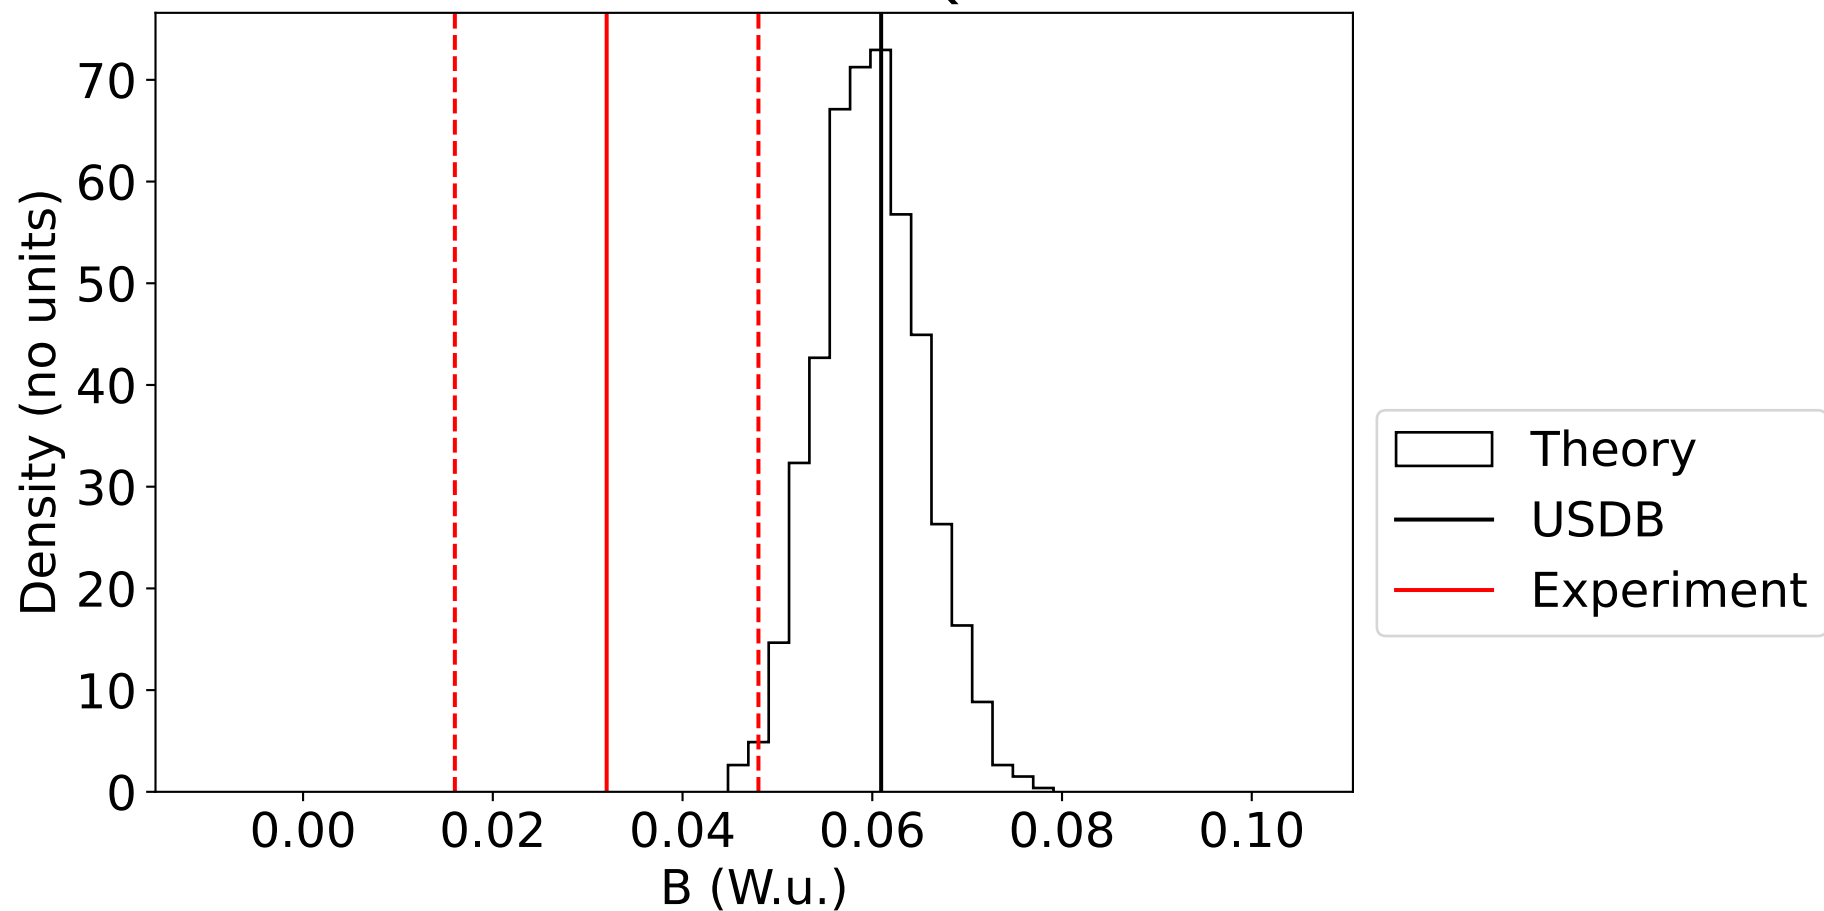

$^{33}\text{P} (3/2_2) \rightarrow (3/2_1)$   
Included in UQ

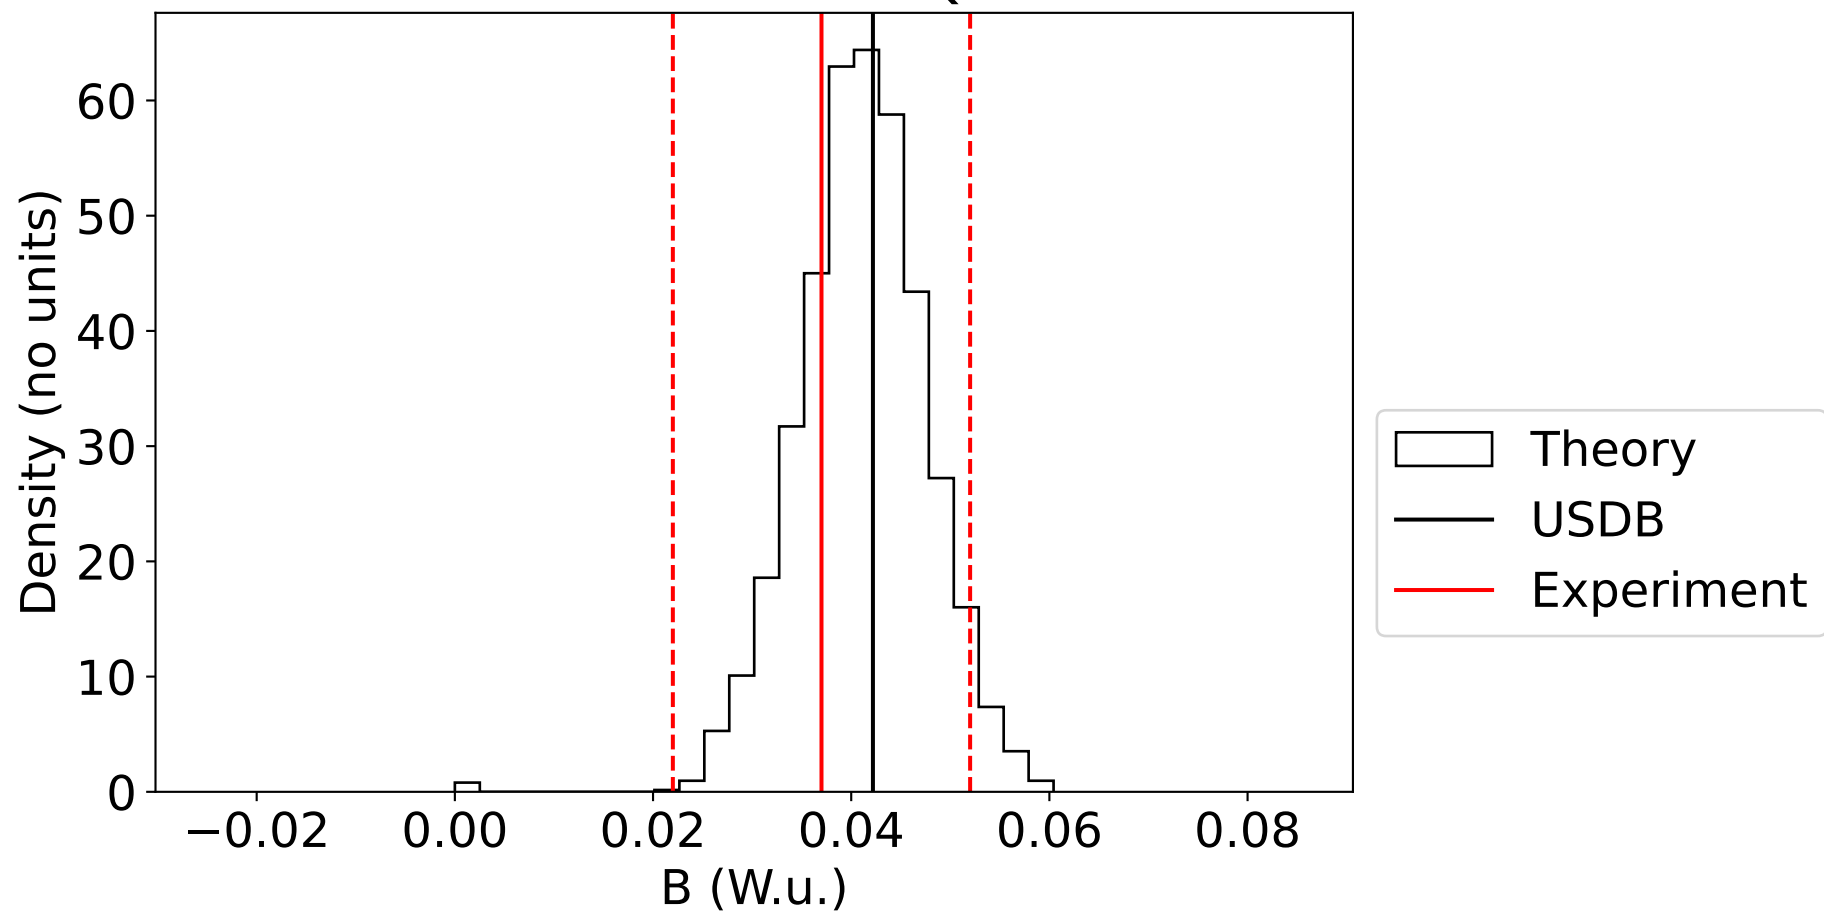

$^{33}\text{P} (5/2_2) \rightarrow (3/2_1)$   
Included in UQ

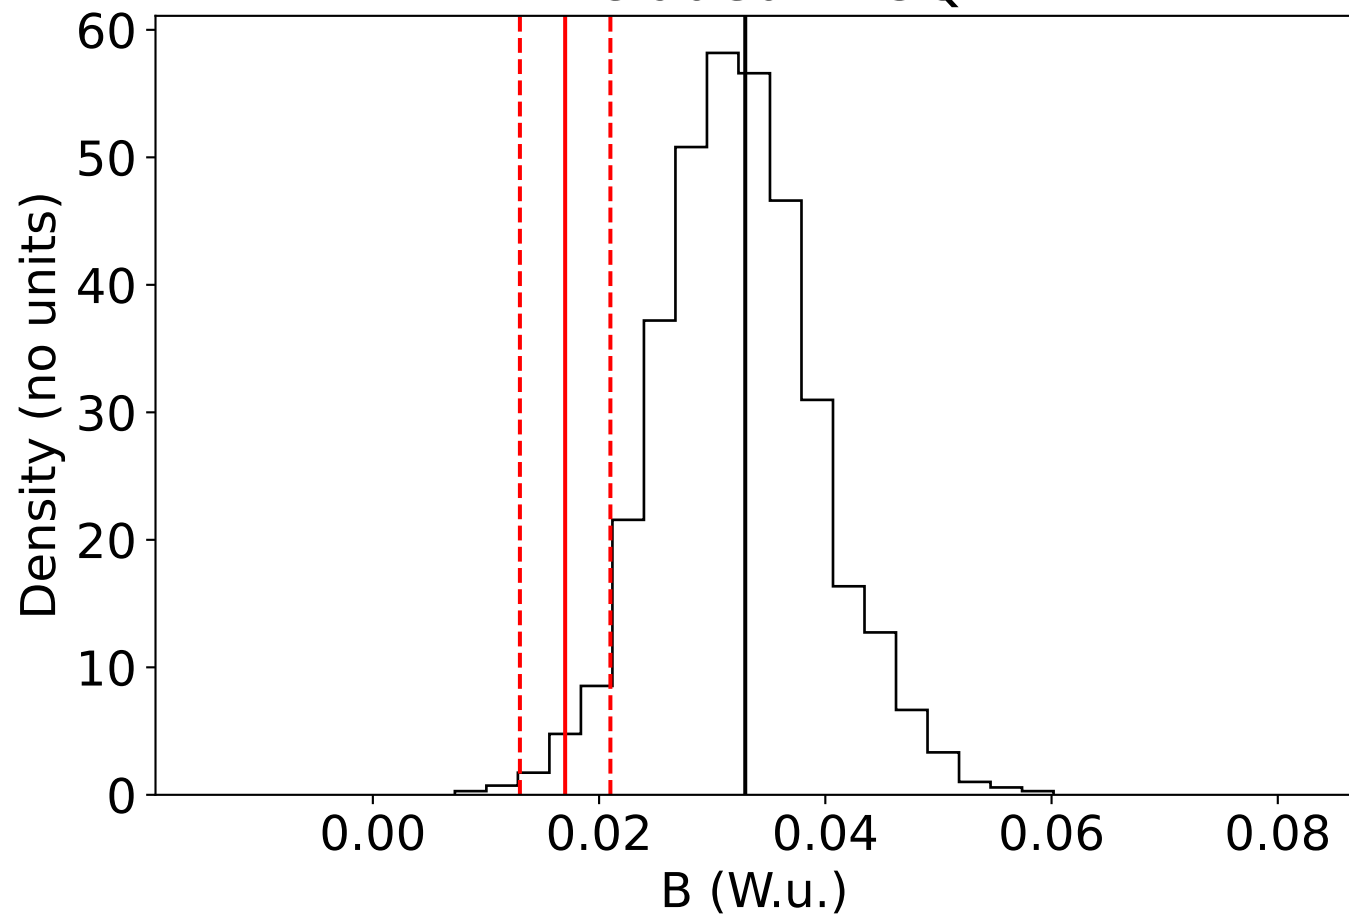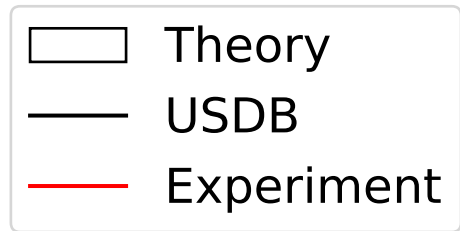

$^{33}\text{P} (5/2_3) \rightarrow (3/2_1)$   
Included in UQ

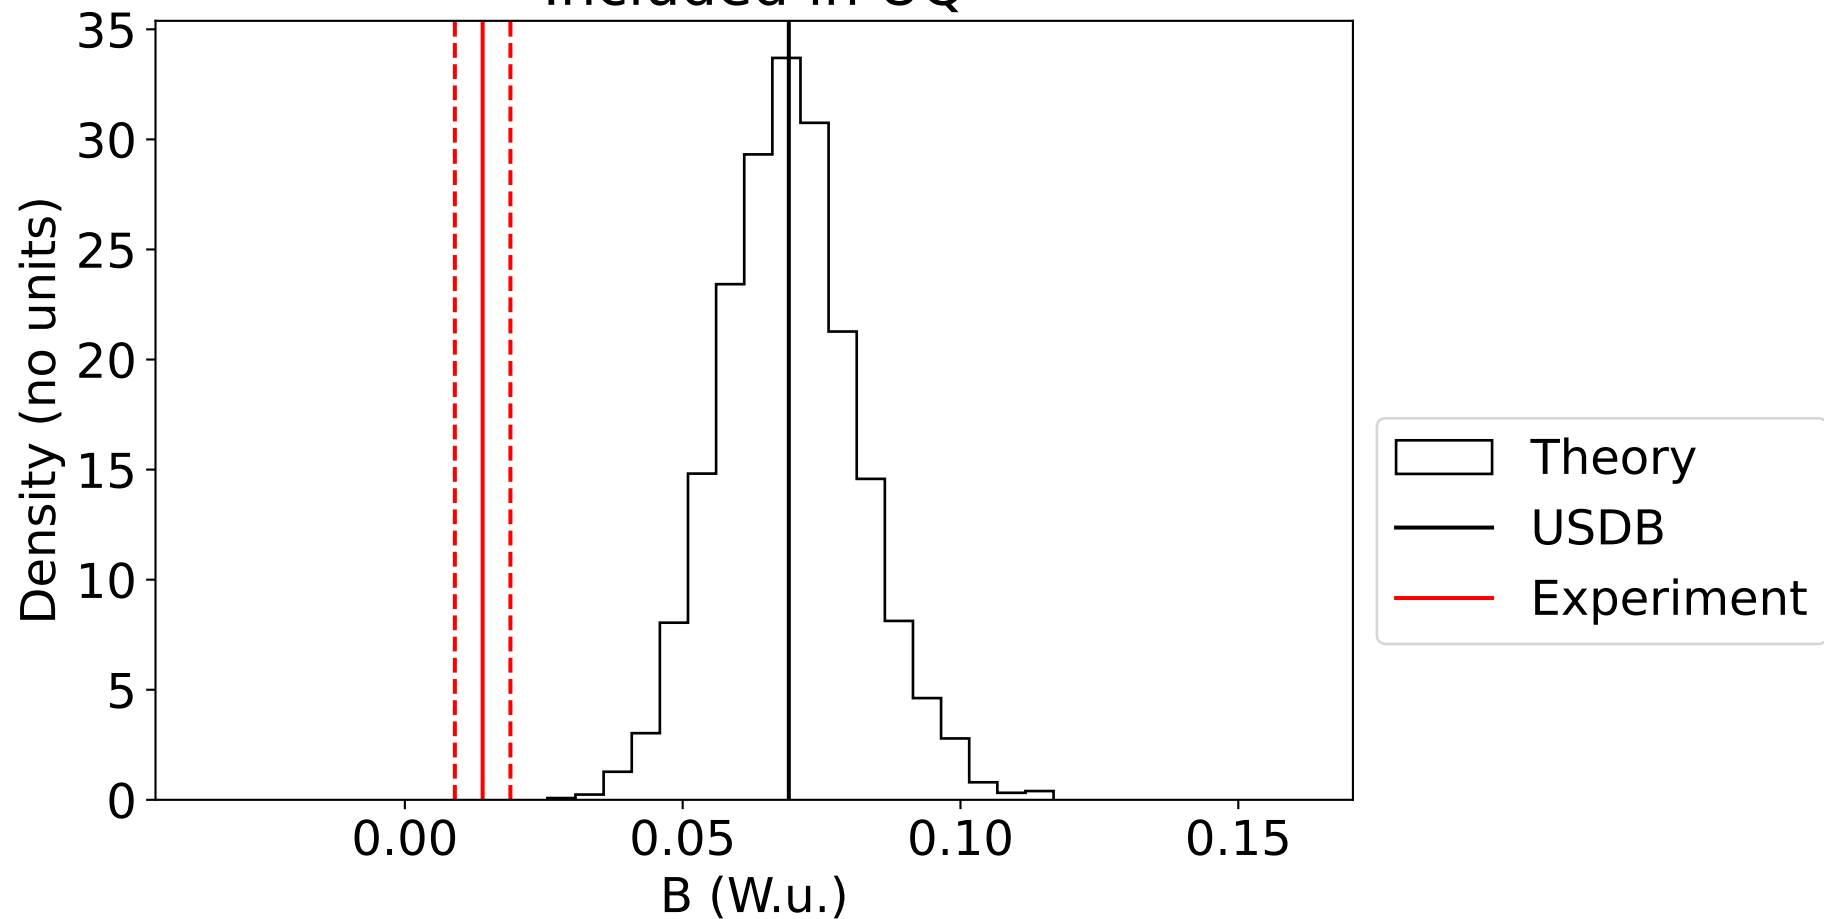

$^{33}\text{P} (5/2_3) \rightarrow (3/2_3)$   
Included in UQ

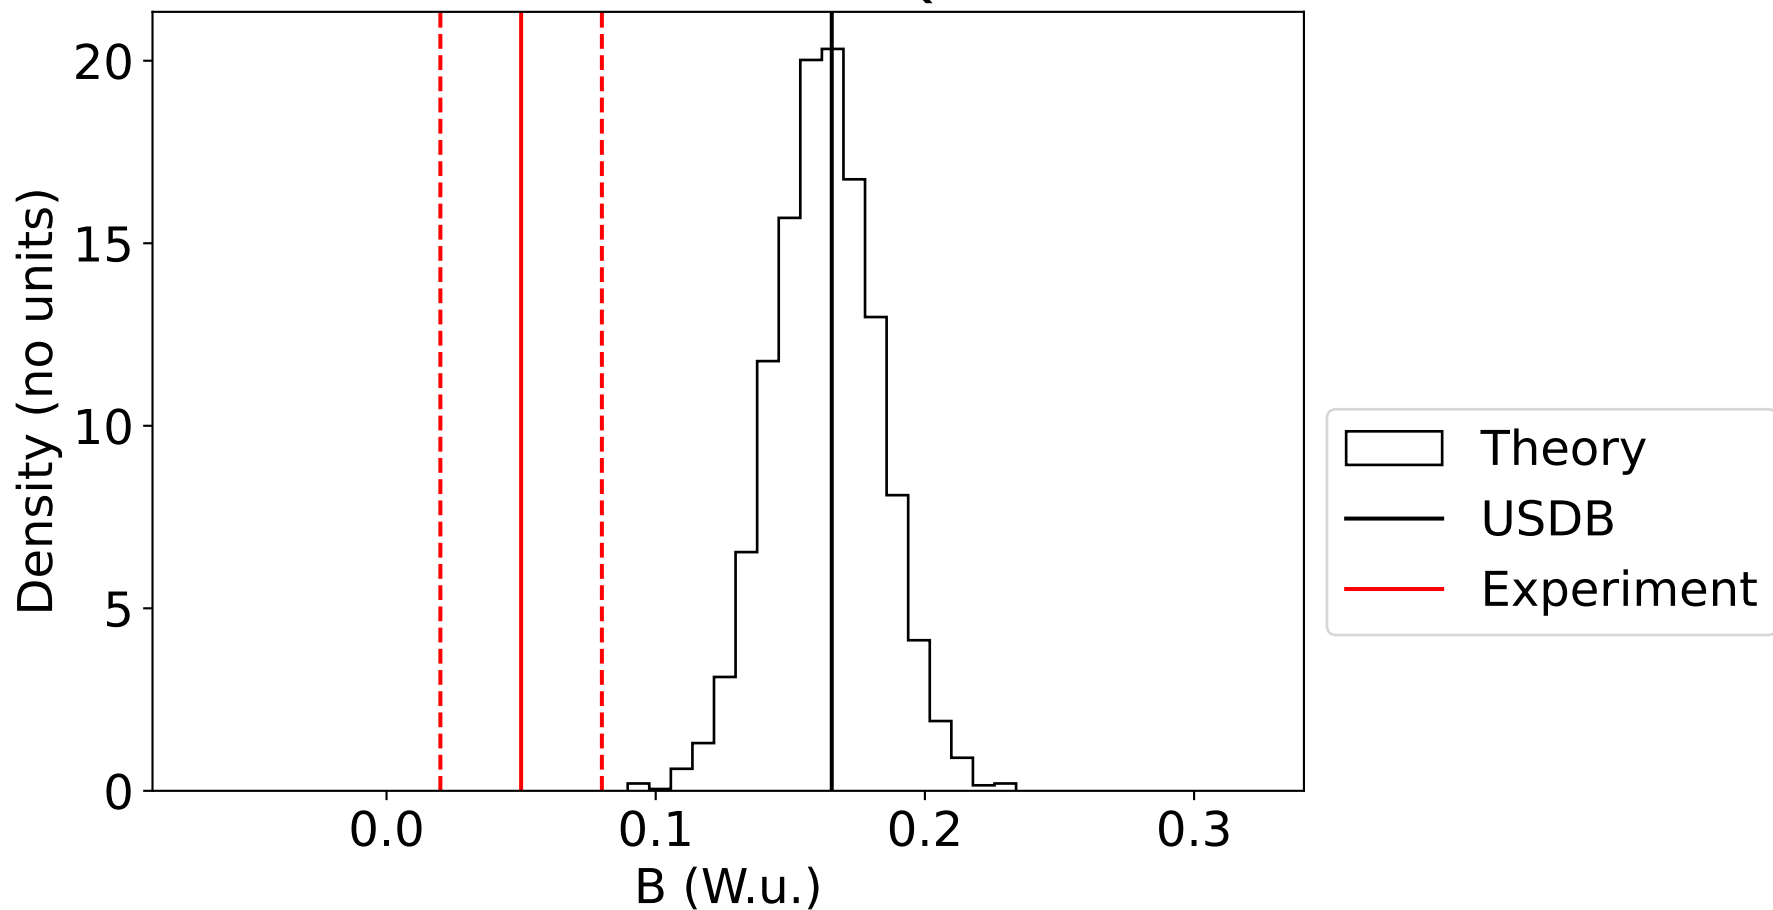

$^{31}\text{S} (3/2_1) \rightarrow (1/2_1)$   
Included in UQ

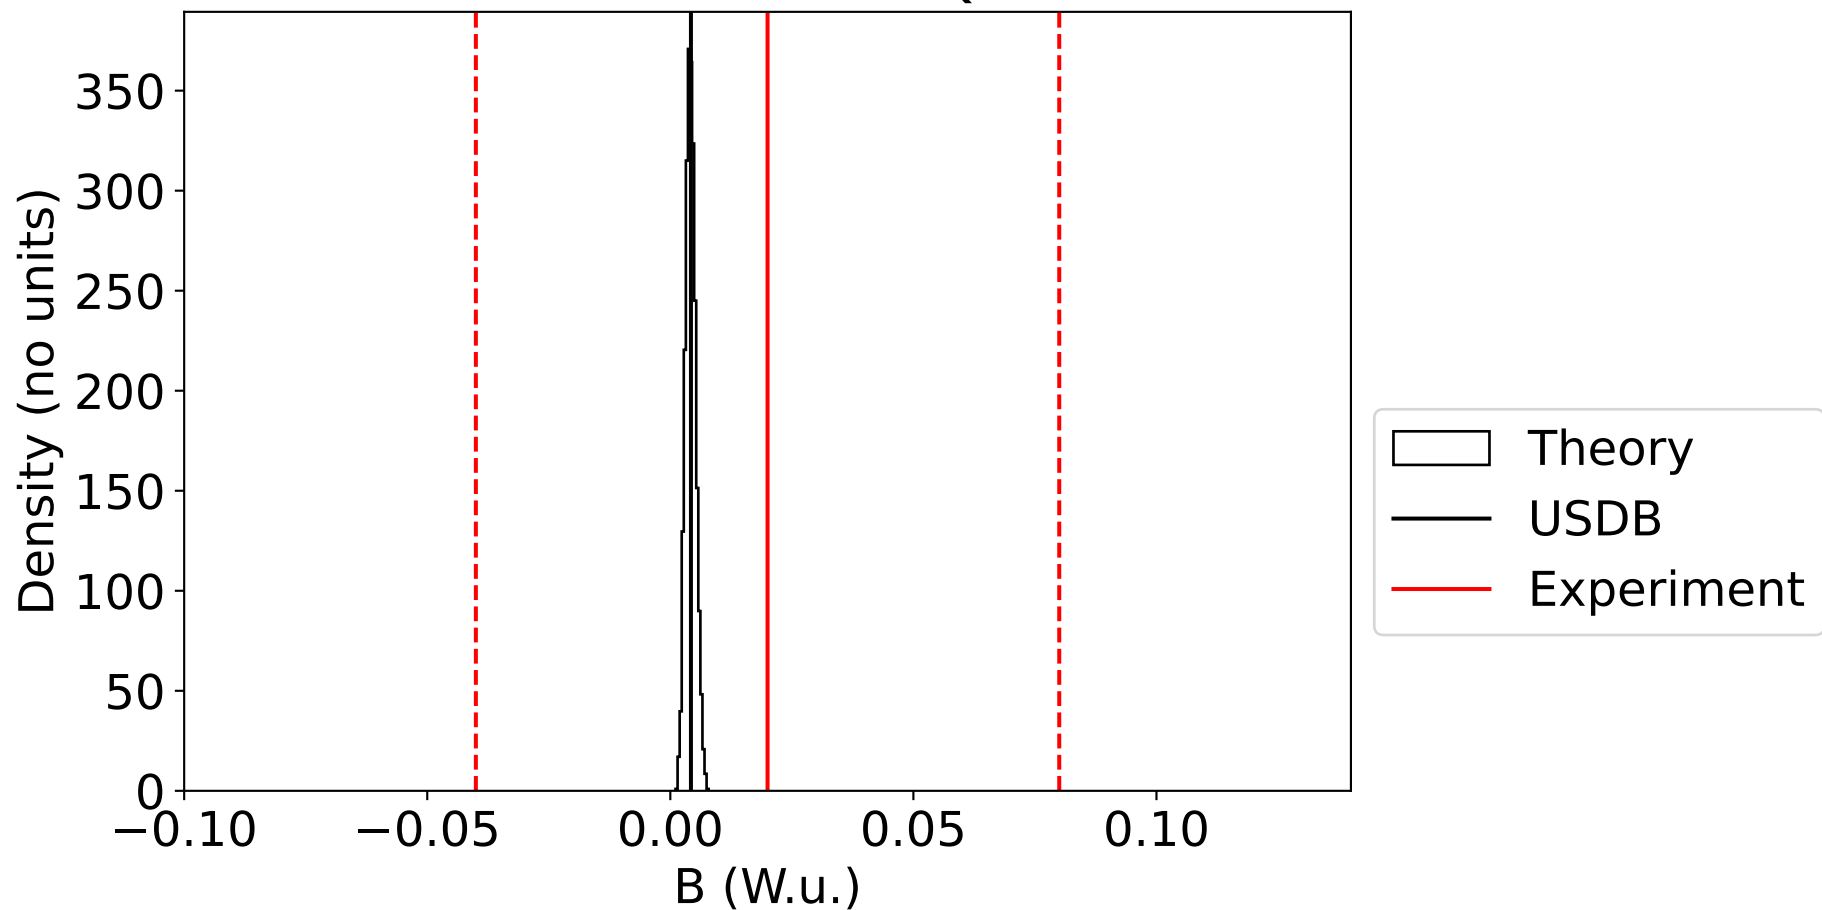

$^{32}\text{S} (2_5) \rightarrow (2_1)$   
Included in UQ

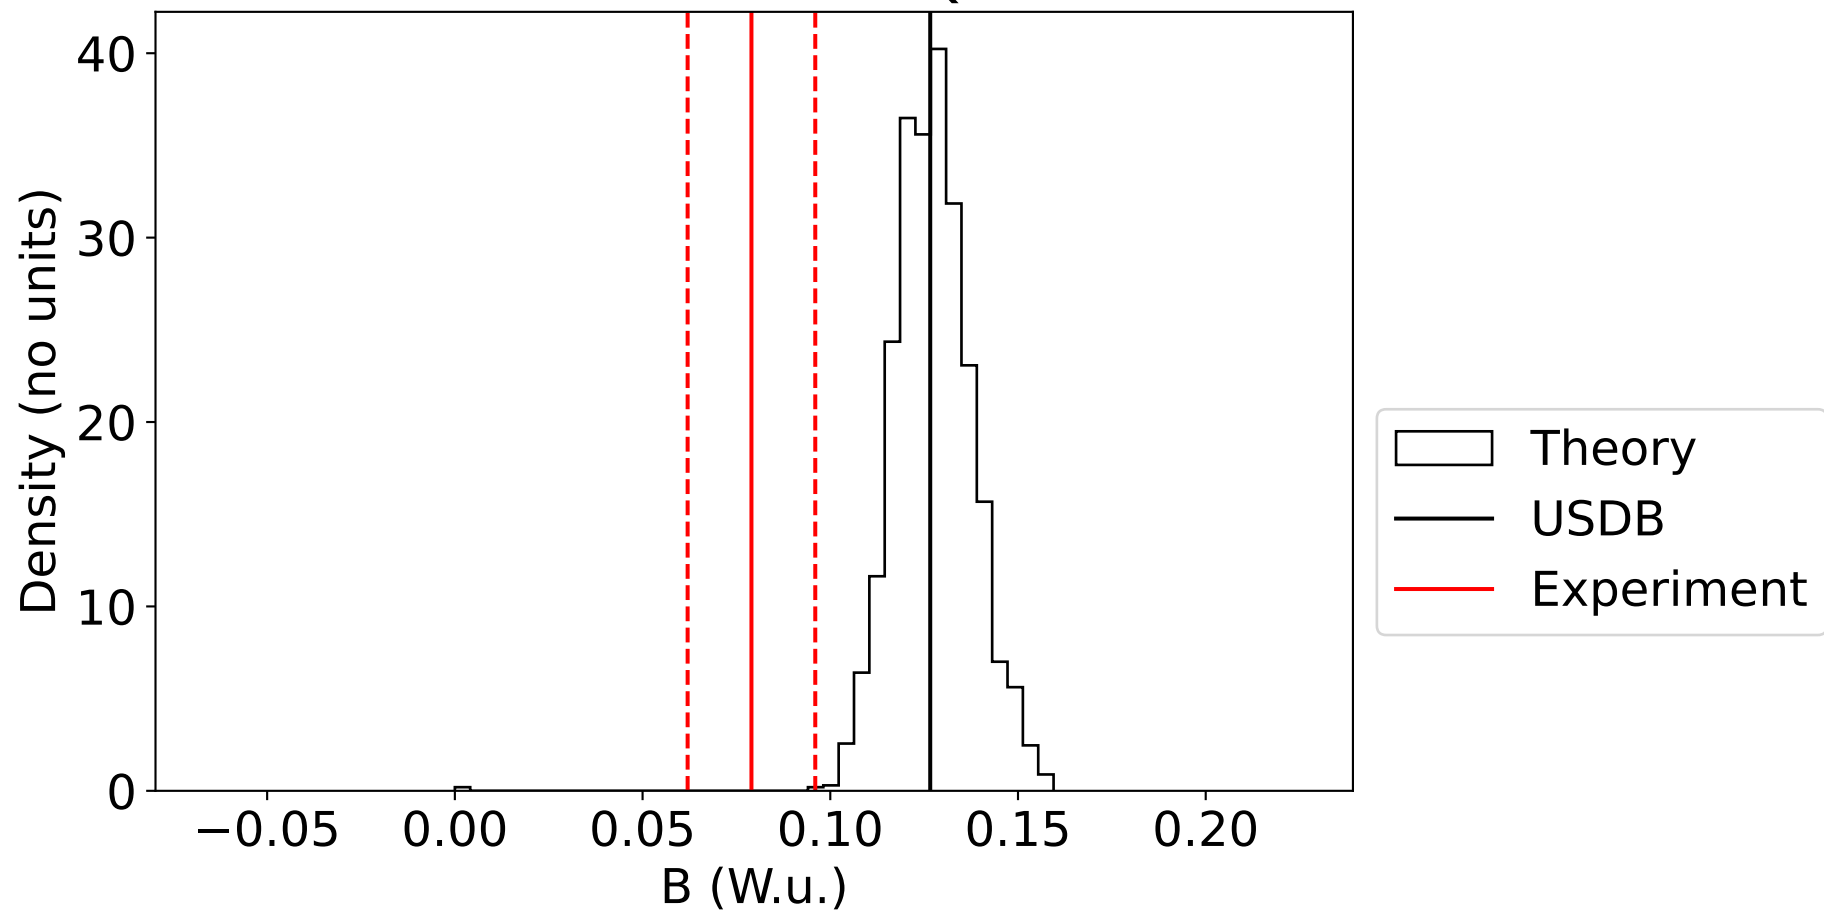



$^{33}\text{S} (1/2_1) \rightarrow (3/2_1)$   
Included in UQ

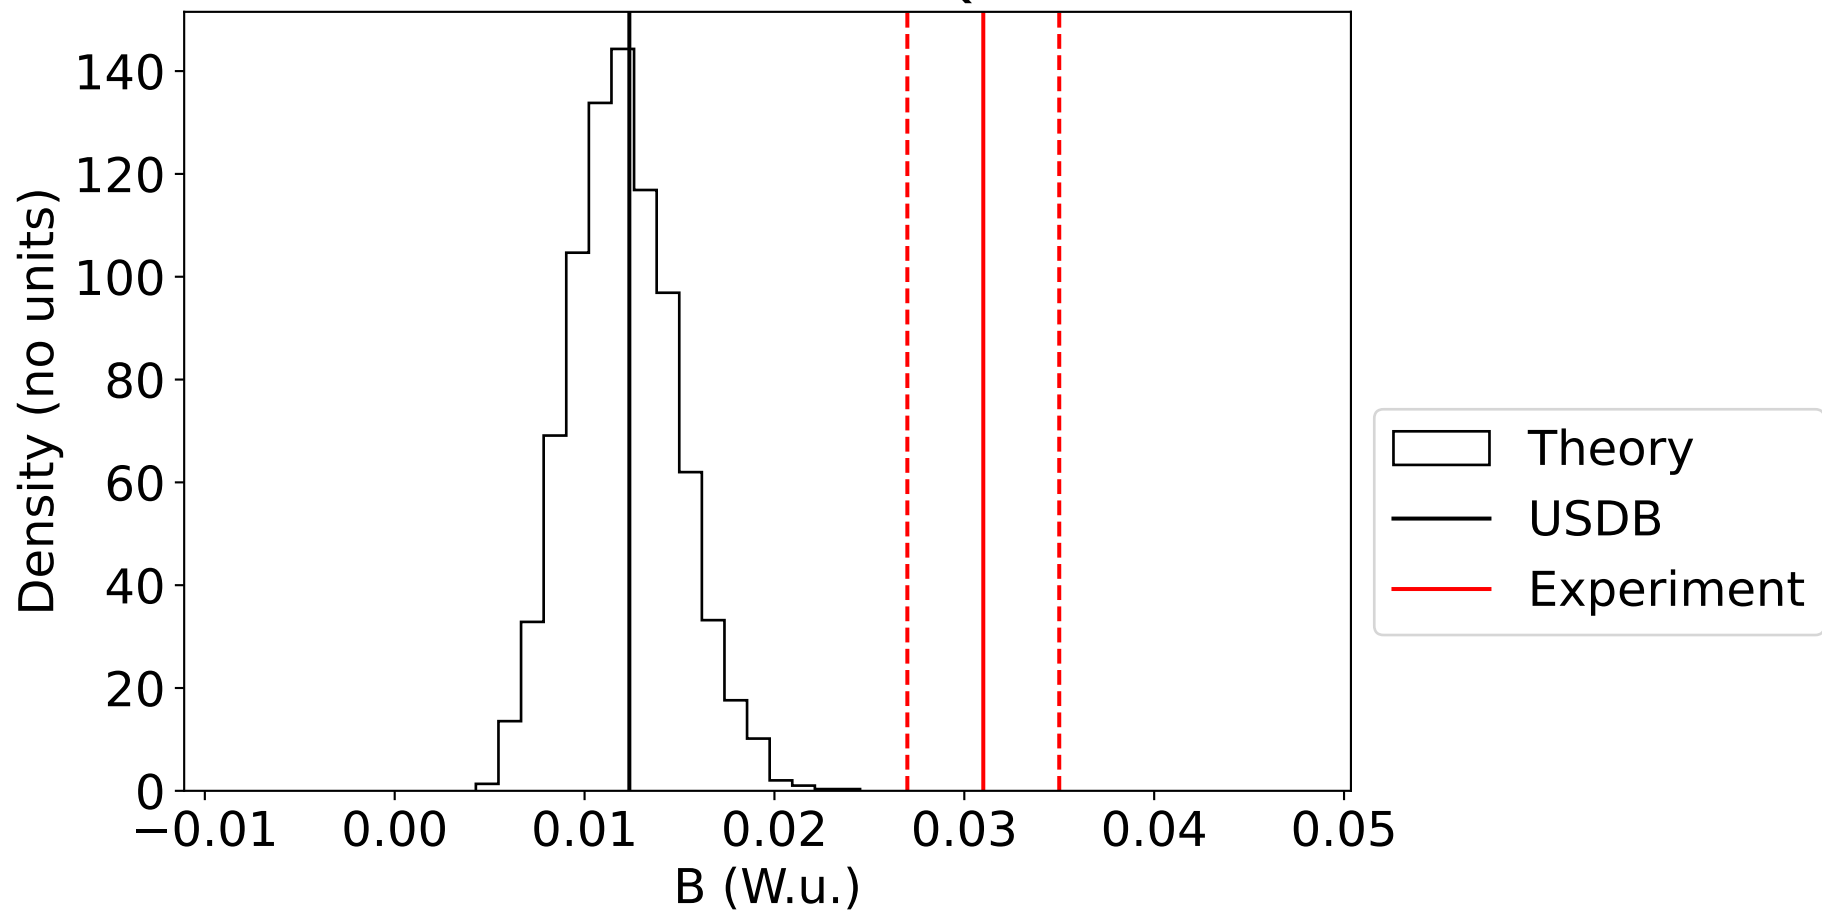

$^{33}\text{S} (5/2_1) \rightarrow (3/2_1)$   
Included in UQ

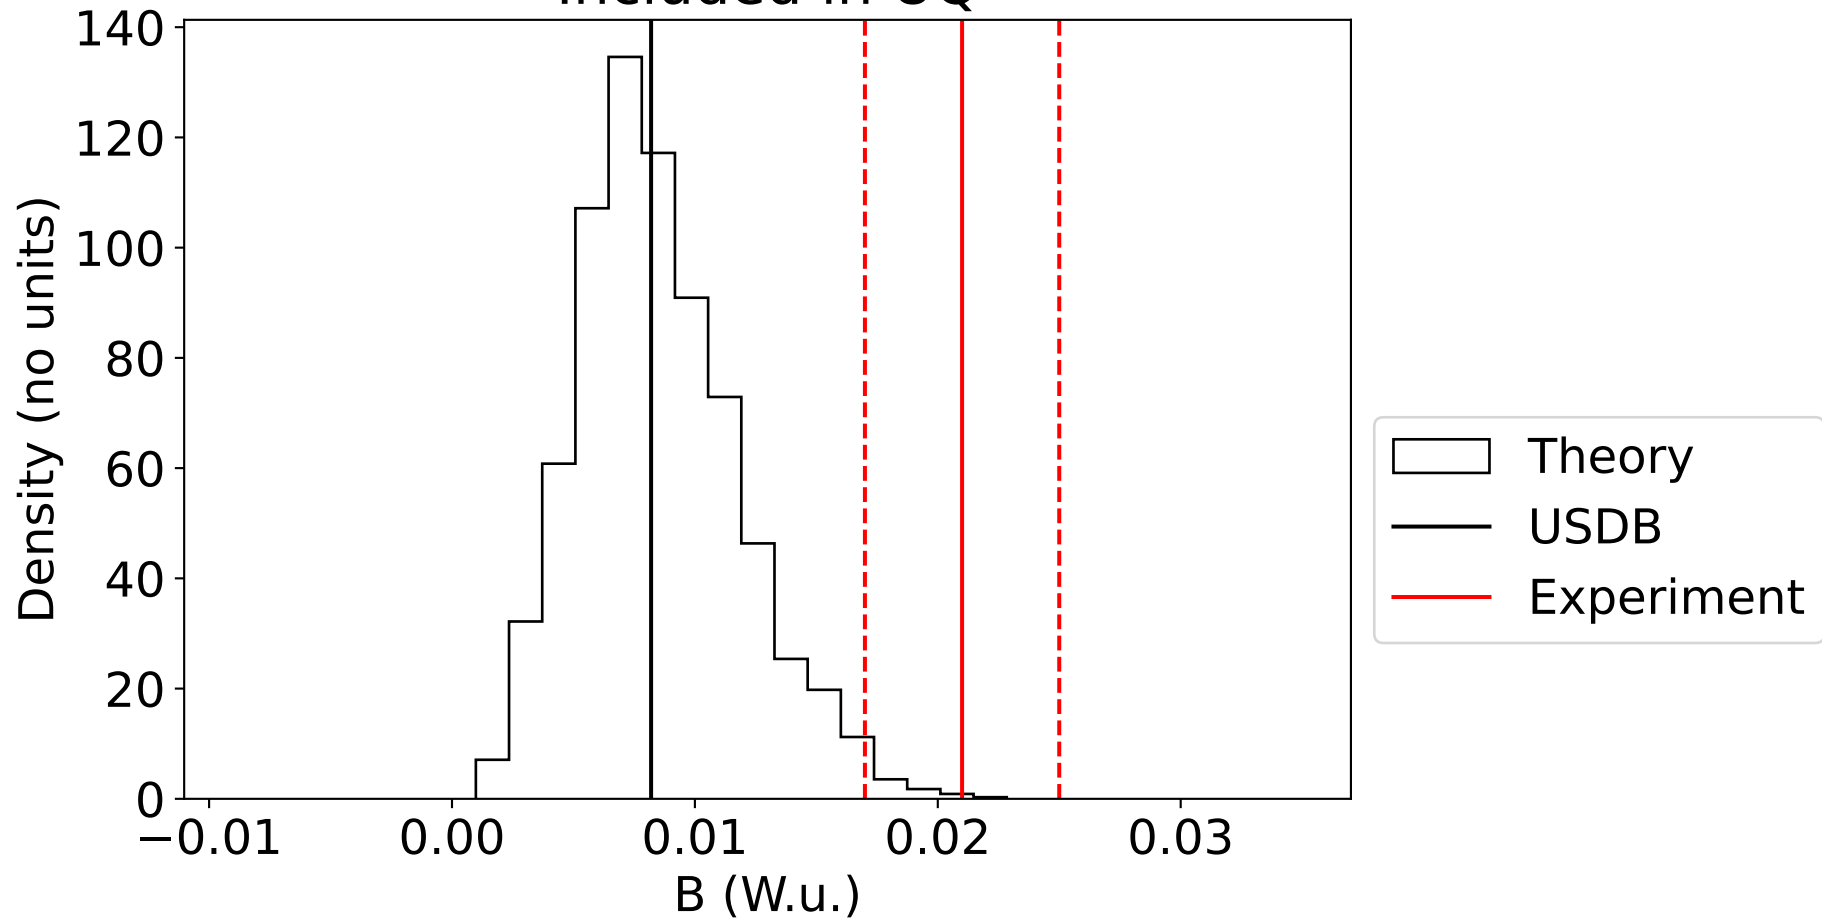

$^{33}\text{S} (3/2_2) \rightarrow (1/2_1)$   
Included in UQ

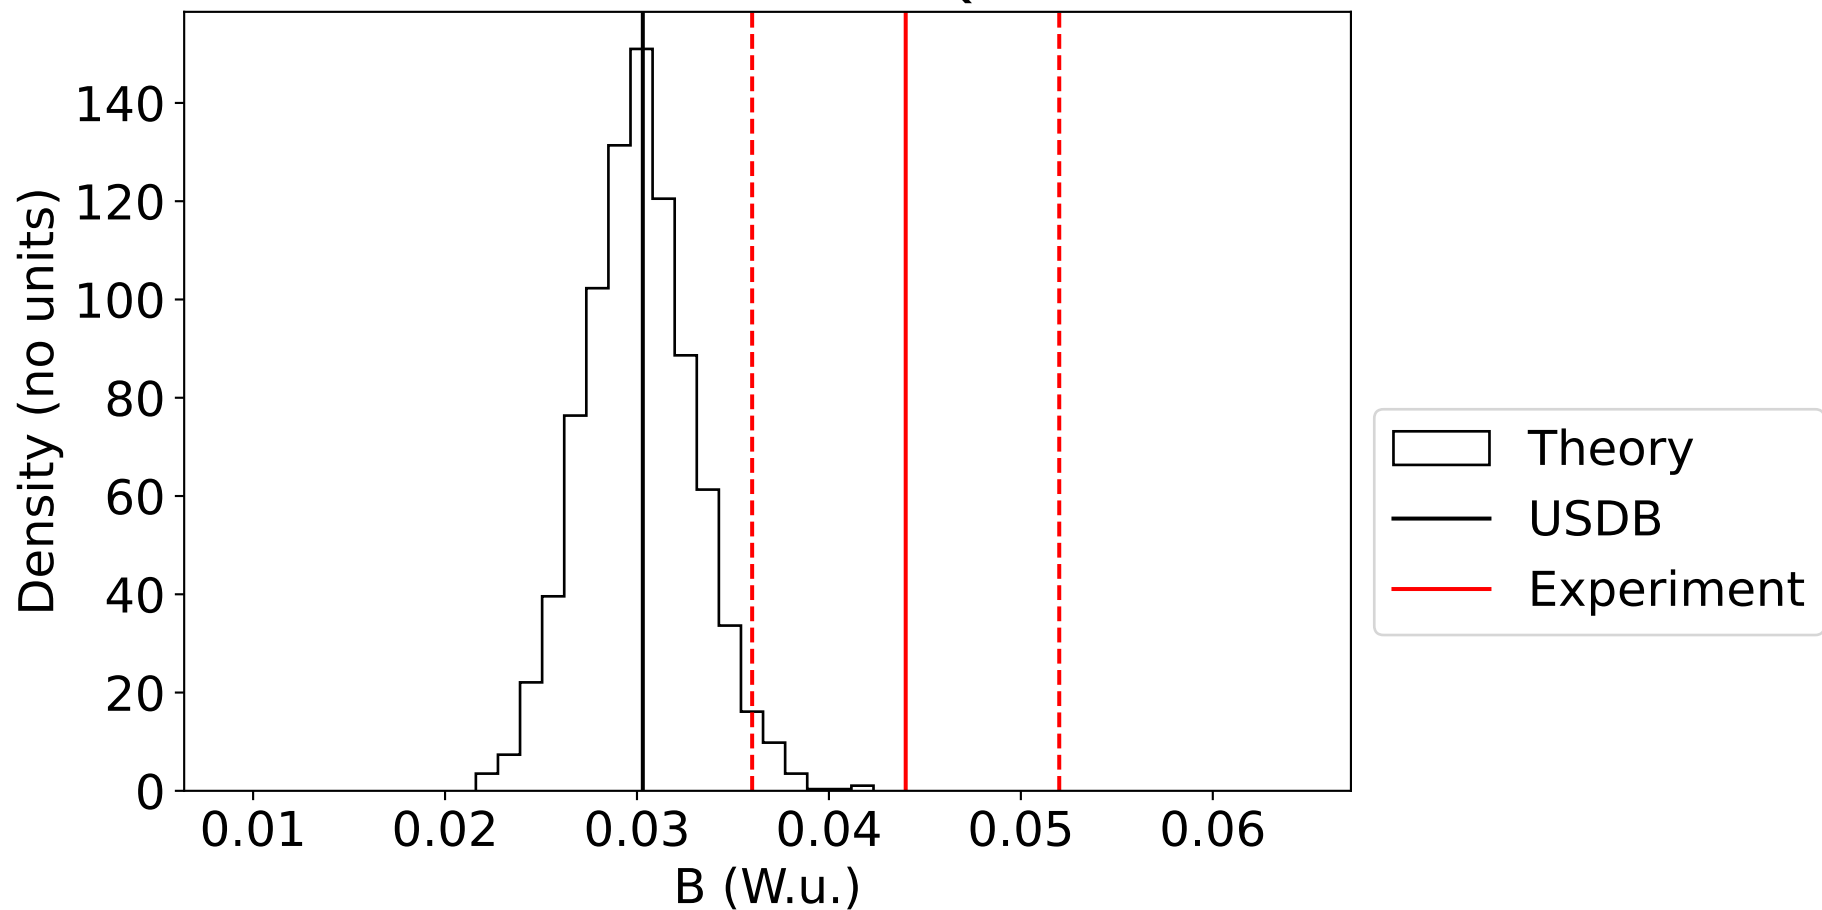

$^{33}\text{S} (3/2_2) \rightarrow (5/2_1)$   
Included in UQ

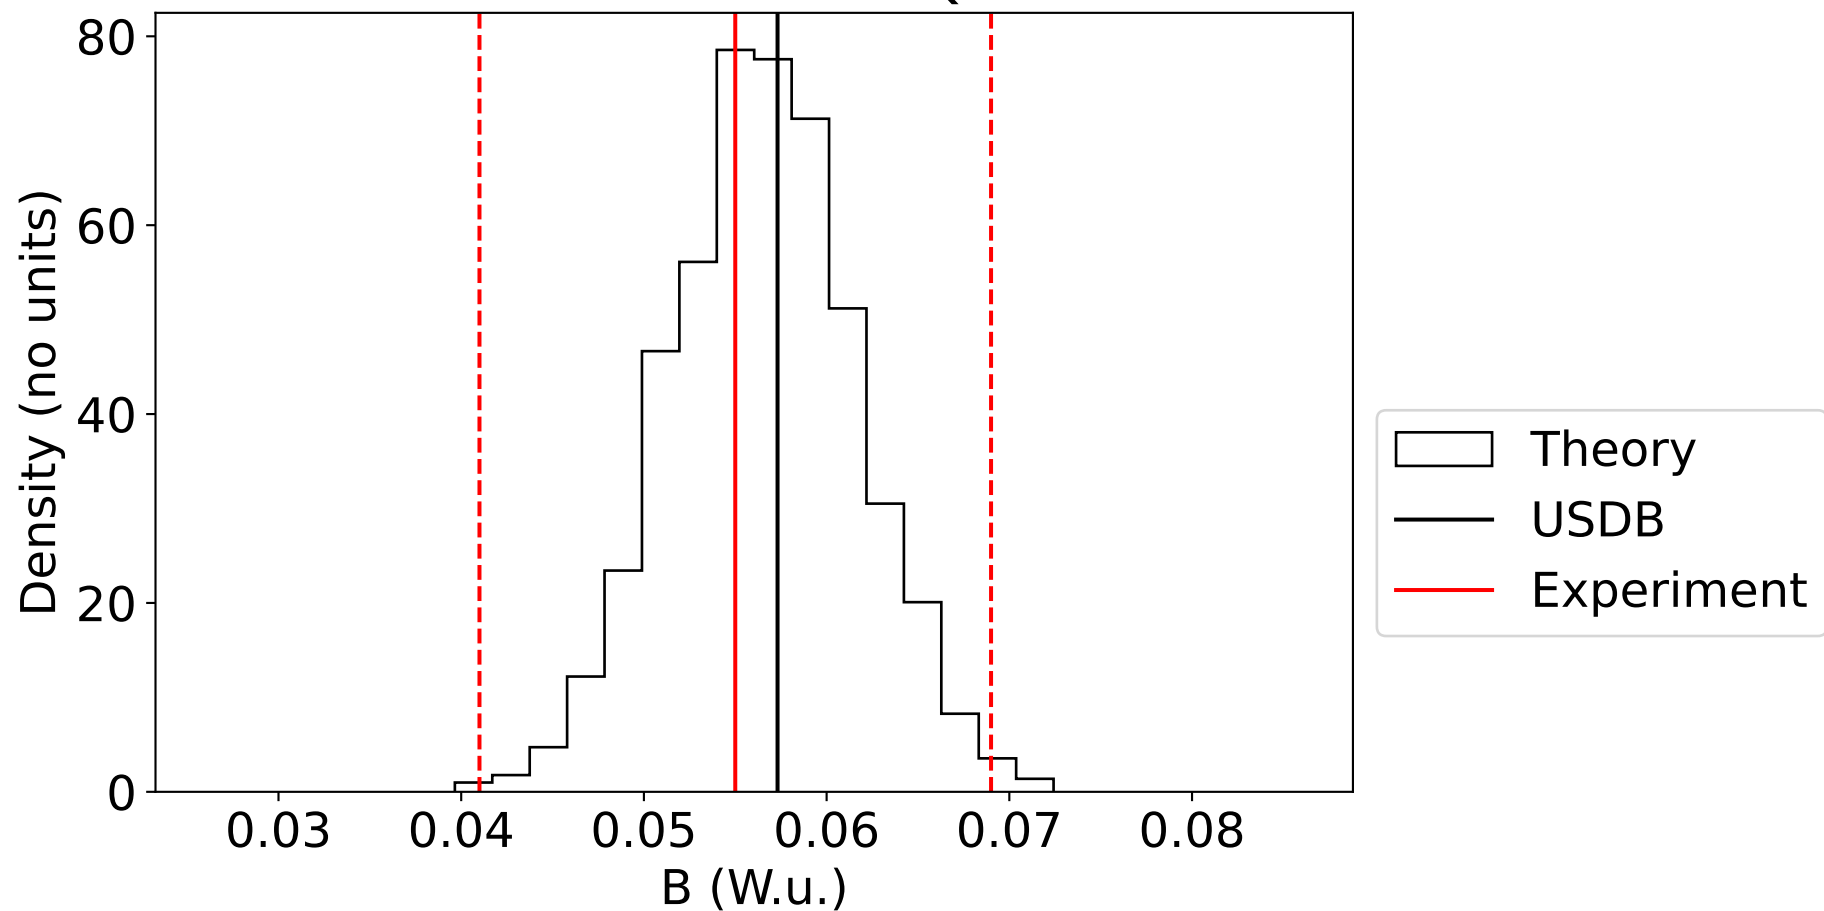

$^{33}\text{S} (5/2_2) \rightarrow (3/2_1)$   
Included in UQ

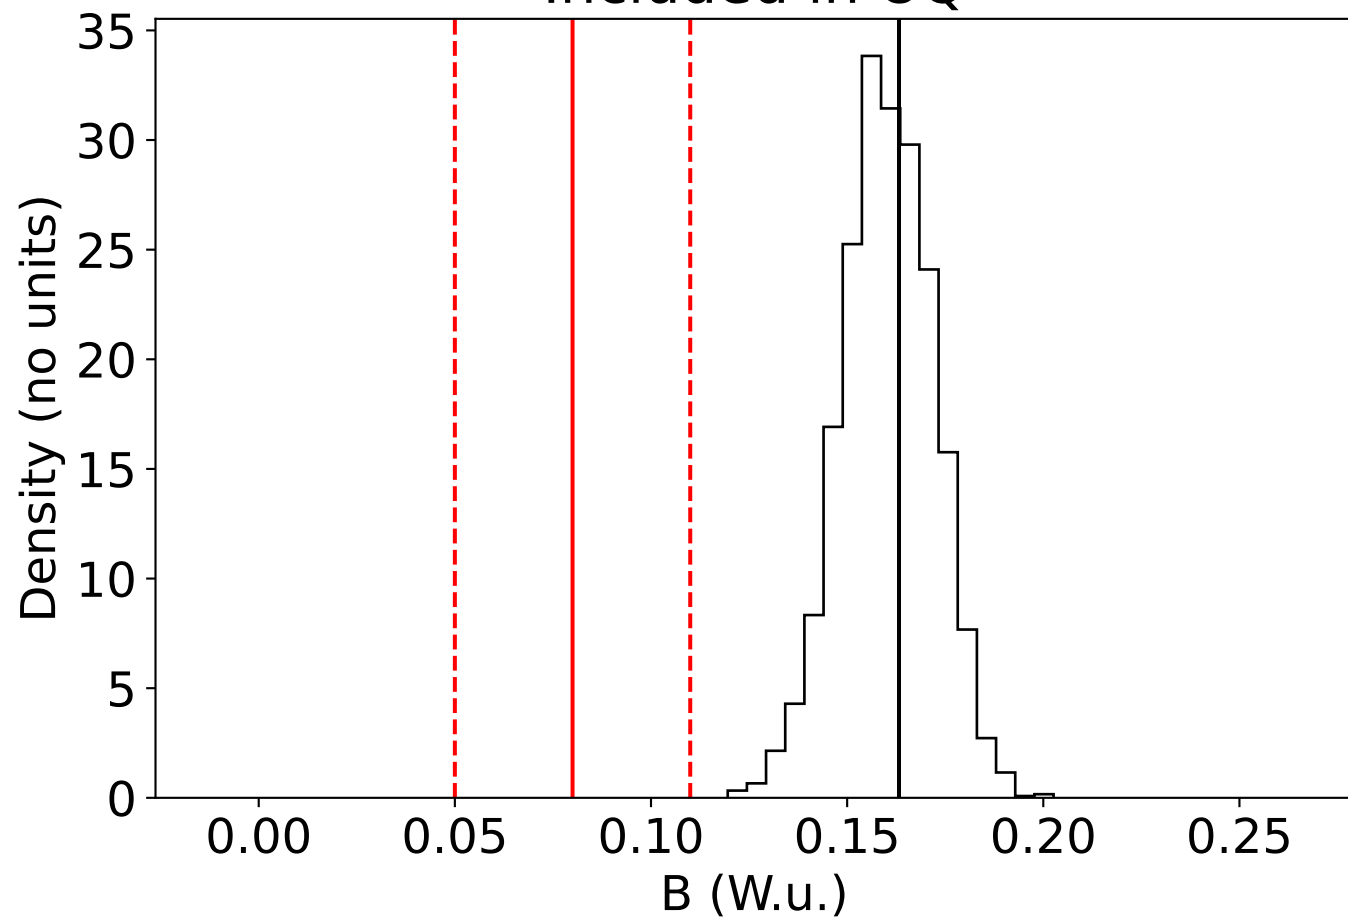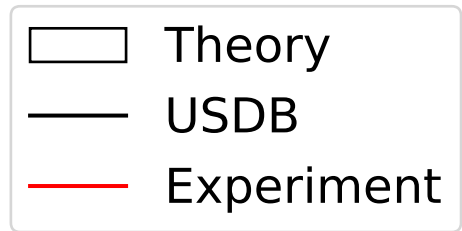

$^{33}\text{S} (5/2_3) \rightarrow (7/2_1)$   
Included in UQ

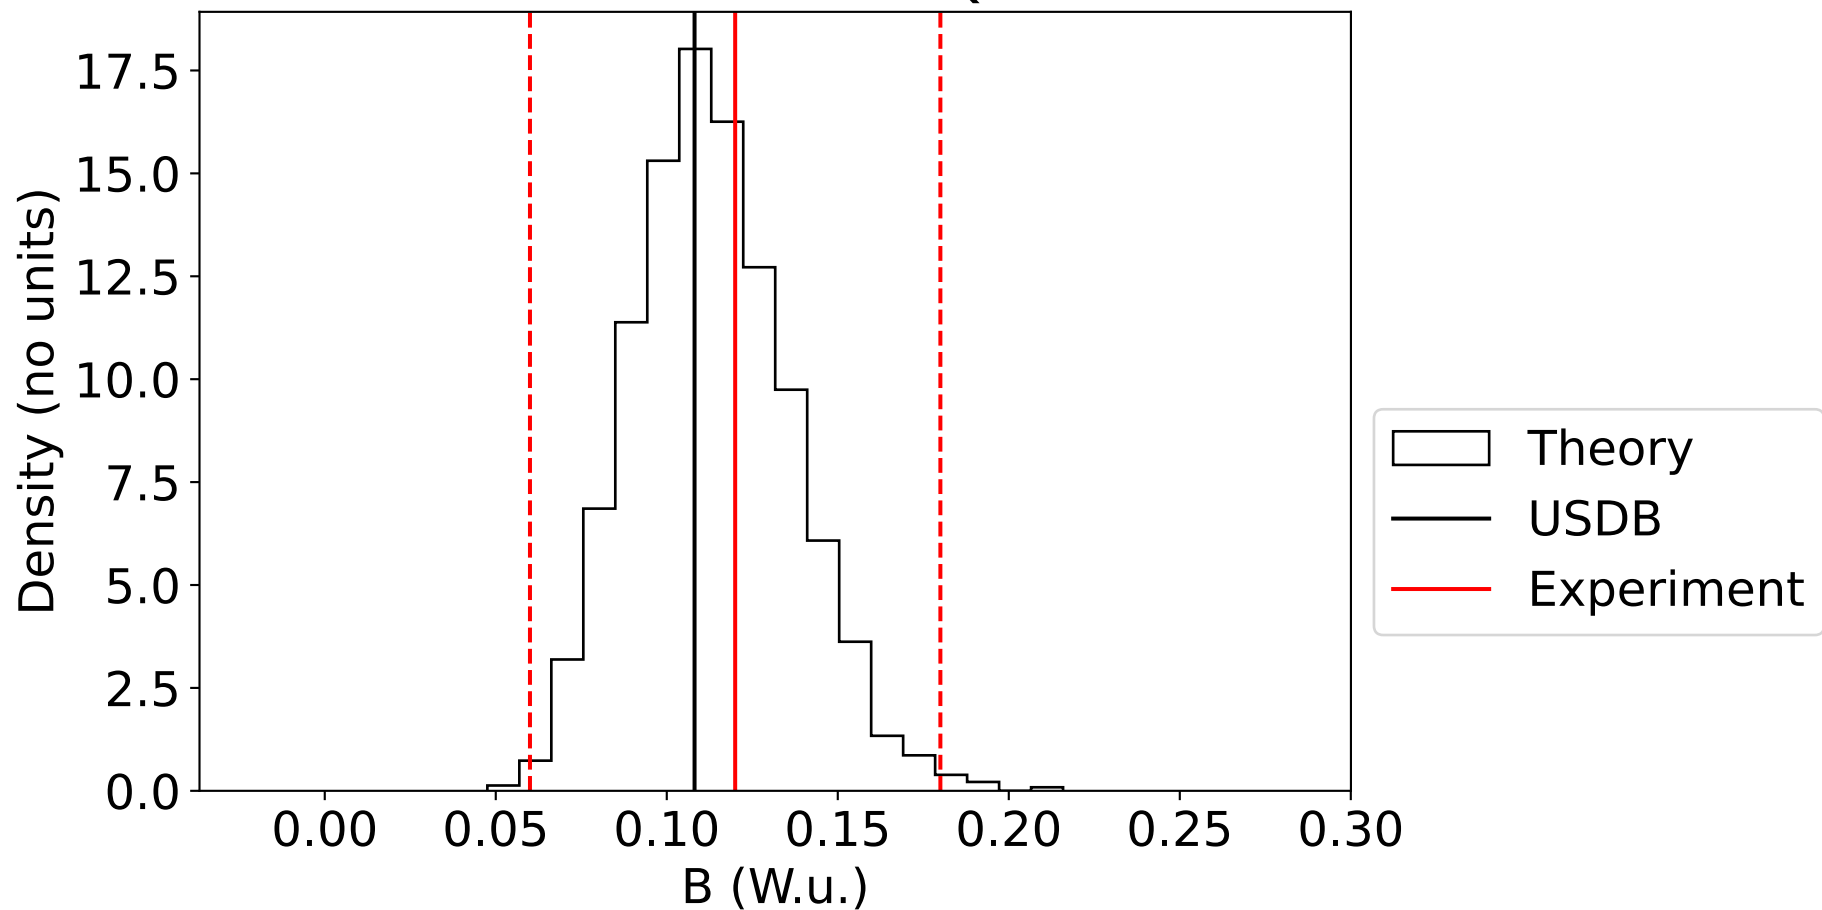

$^{33}\text{S} (7/2_2) \rightarrow (5/2_1)$   
Included in UQ

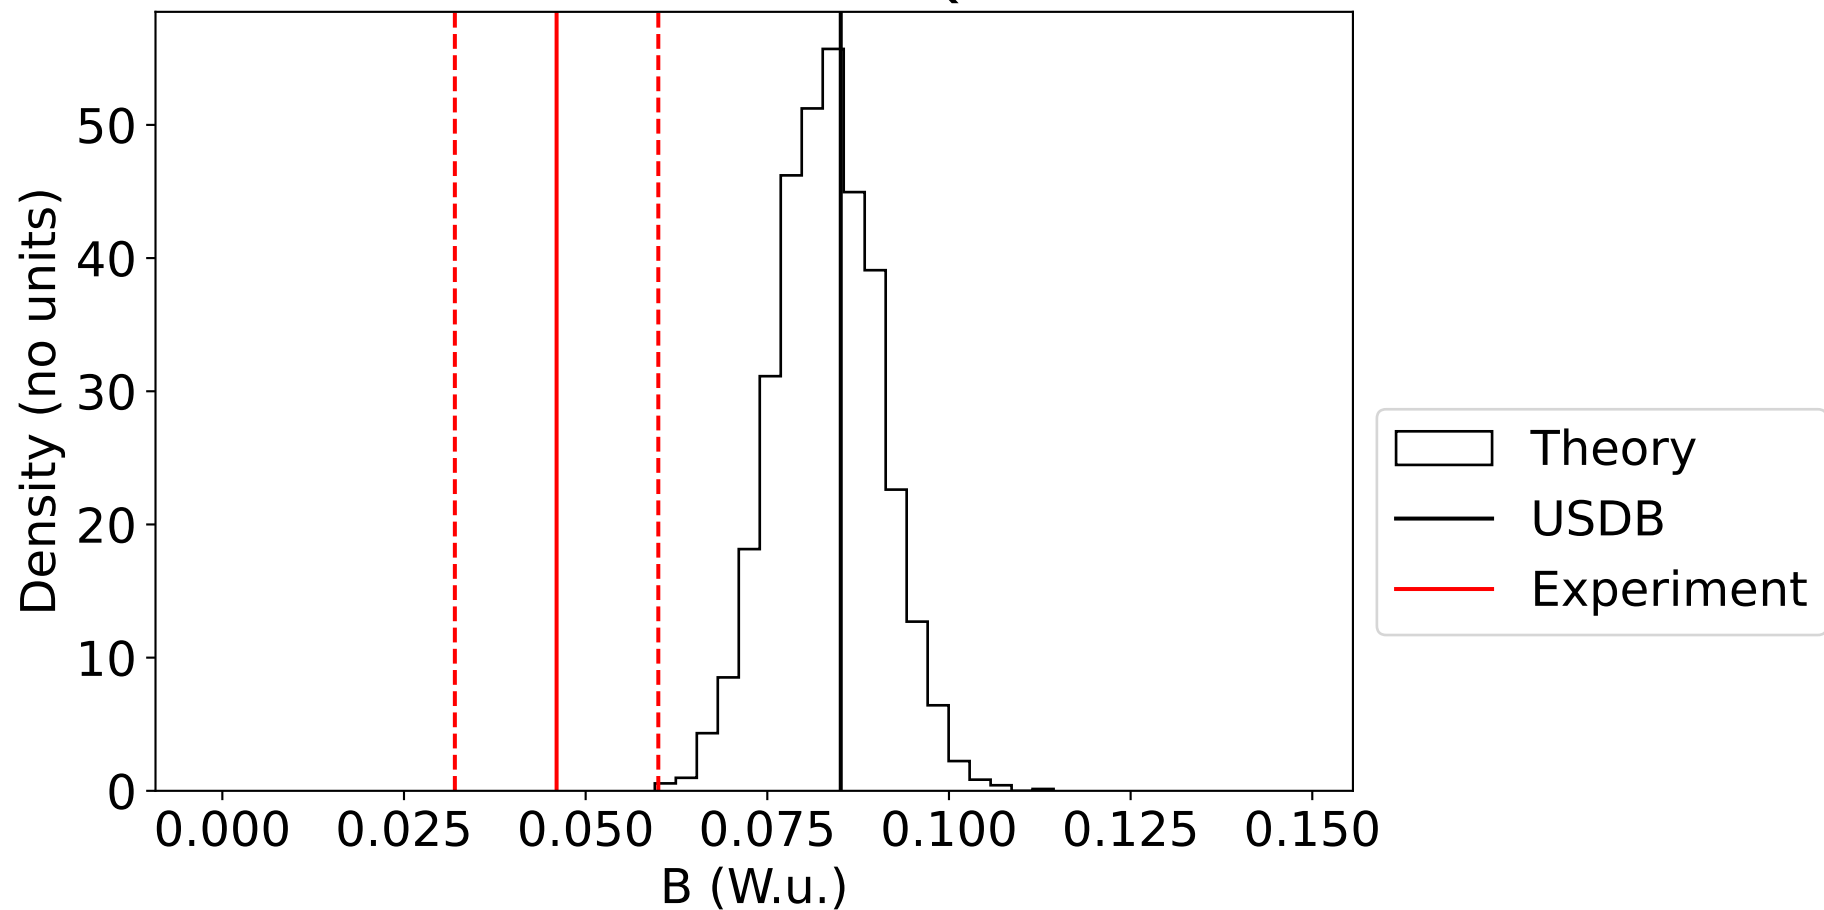

$^{34}\text{S} (2_2) \rightarrow (2_1)$   
Included in UQ

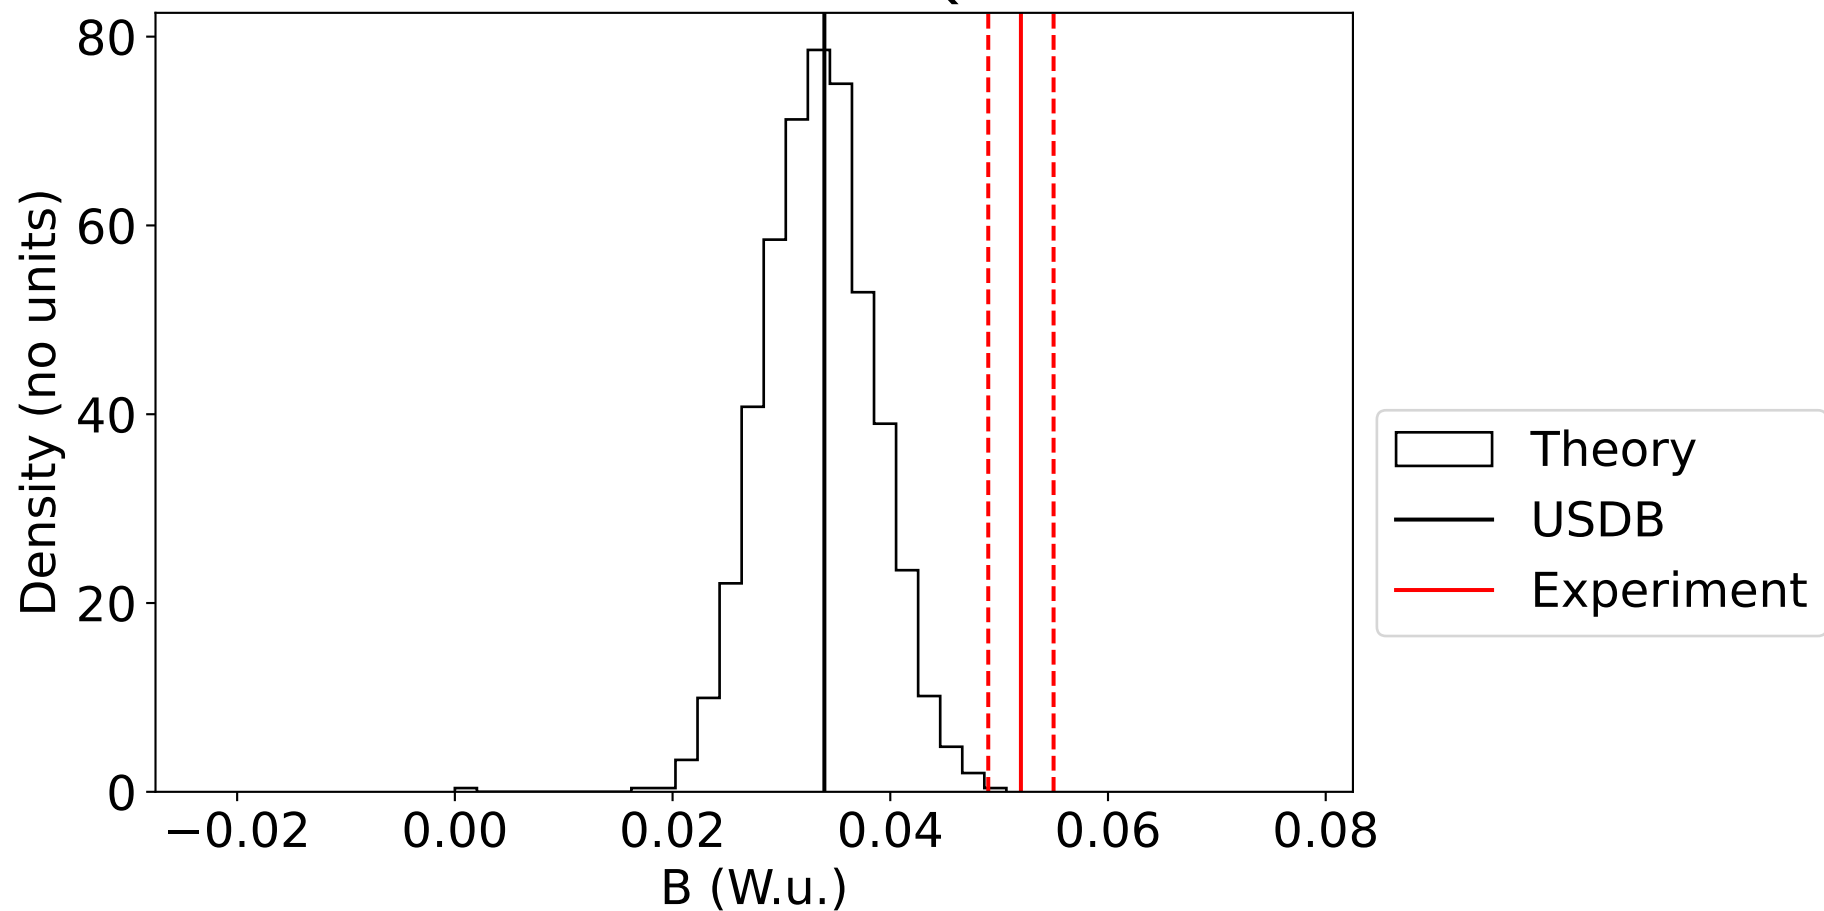



$^{34}\text{S} (2_3) \rightarrow (2_1)$   
Included in UQ

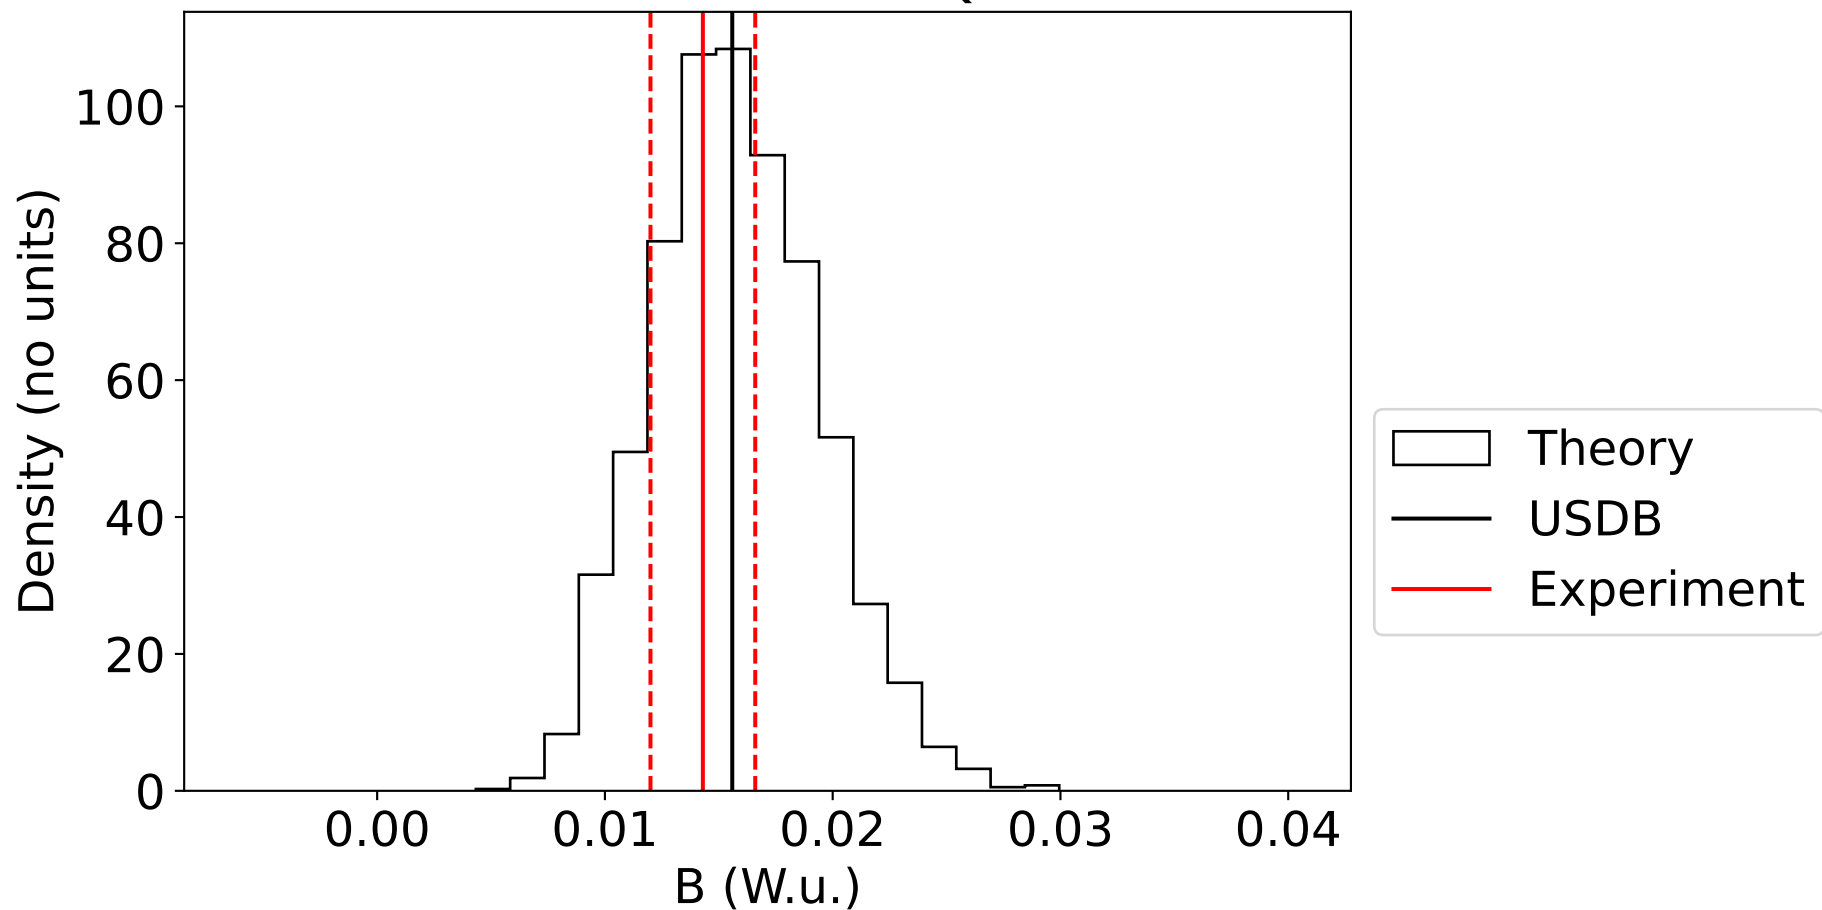

$^{34}\text{S} (3_1) \rightarrow (2_1)$   
Included in UQ

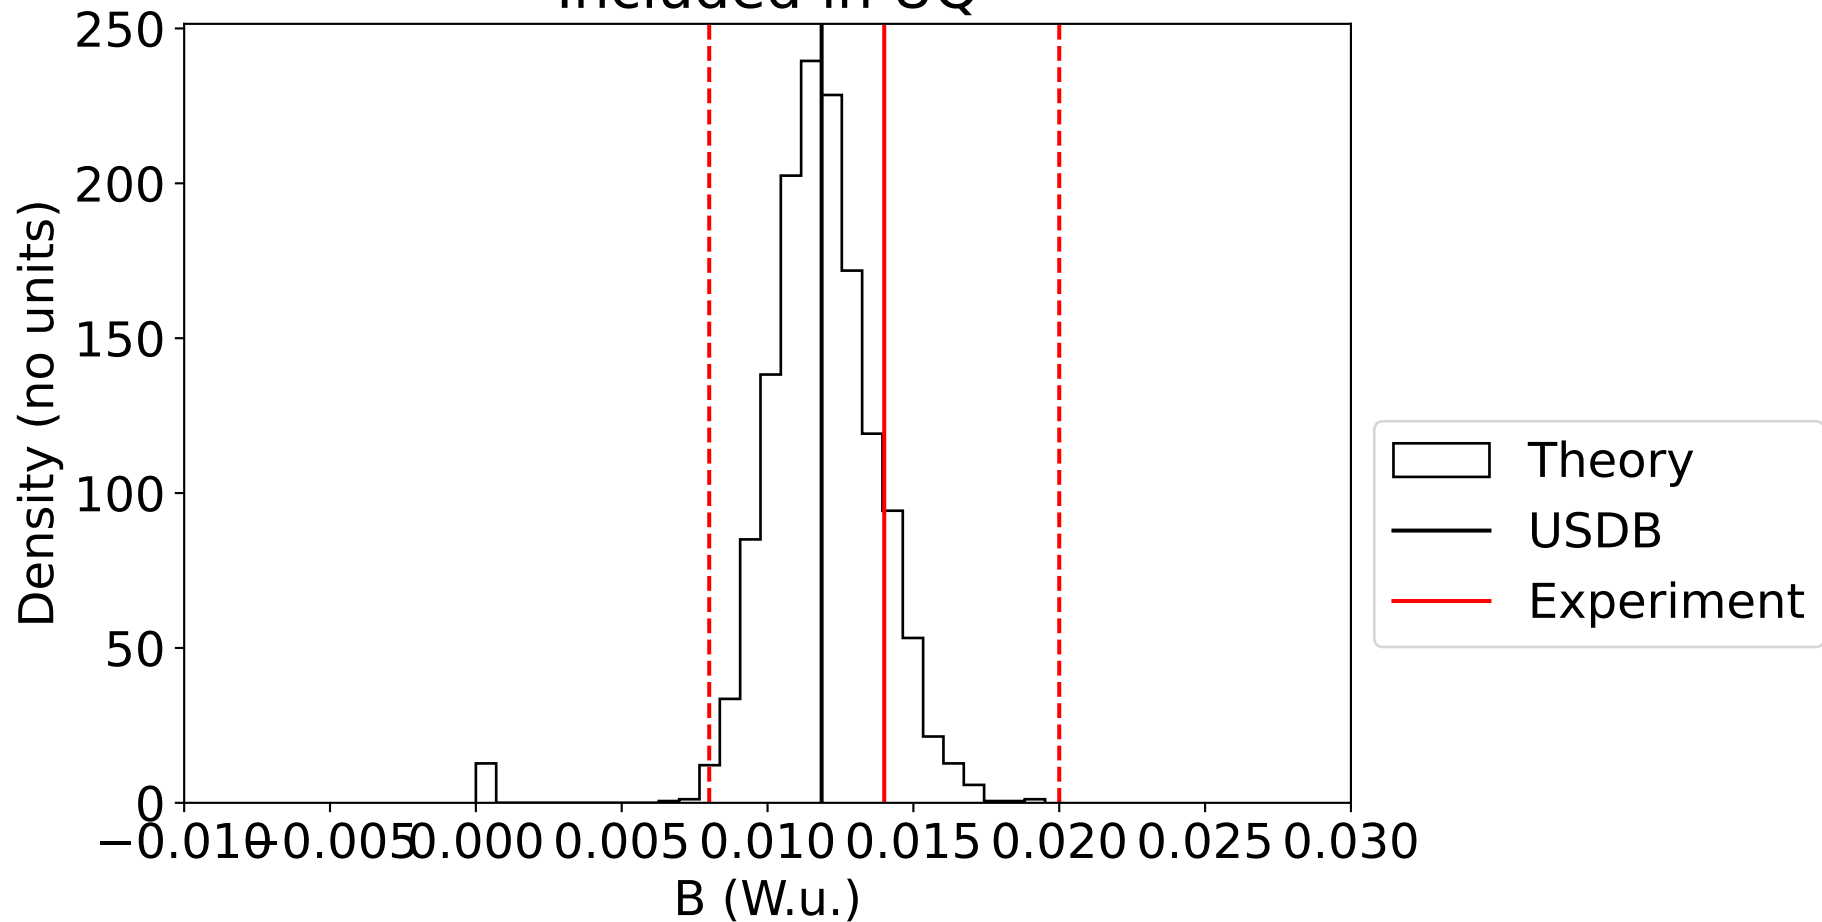

$^{34}\text{S} (3_1) \rightarrow (2_2)$   
Included in UQ

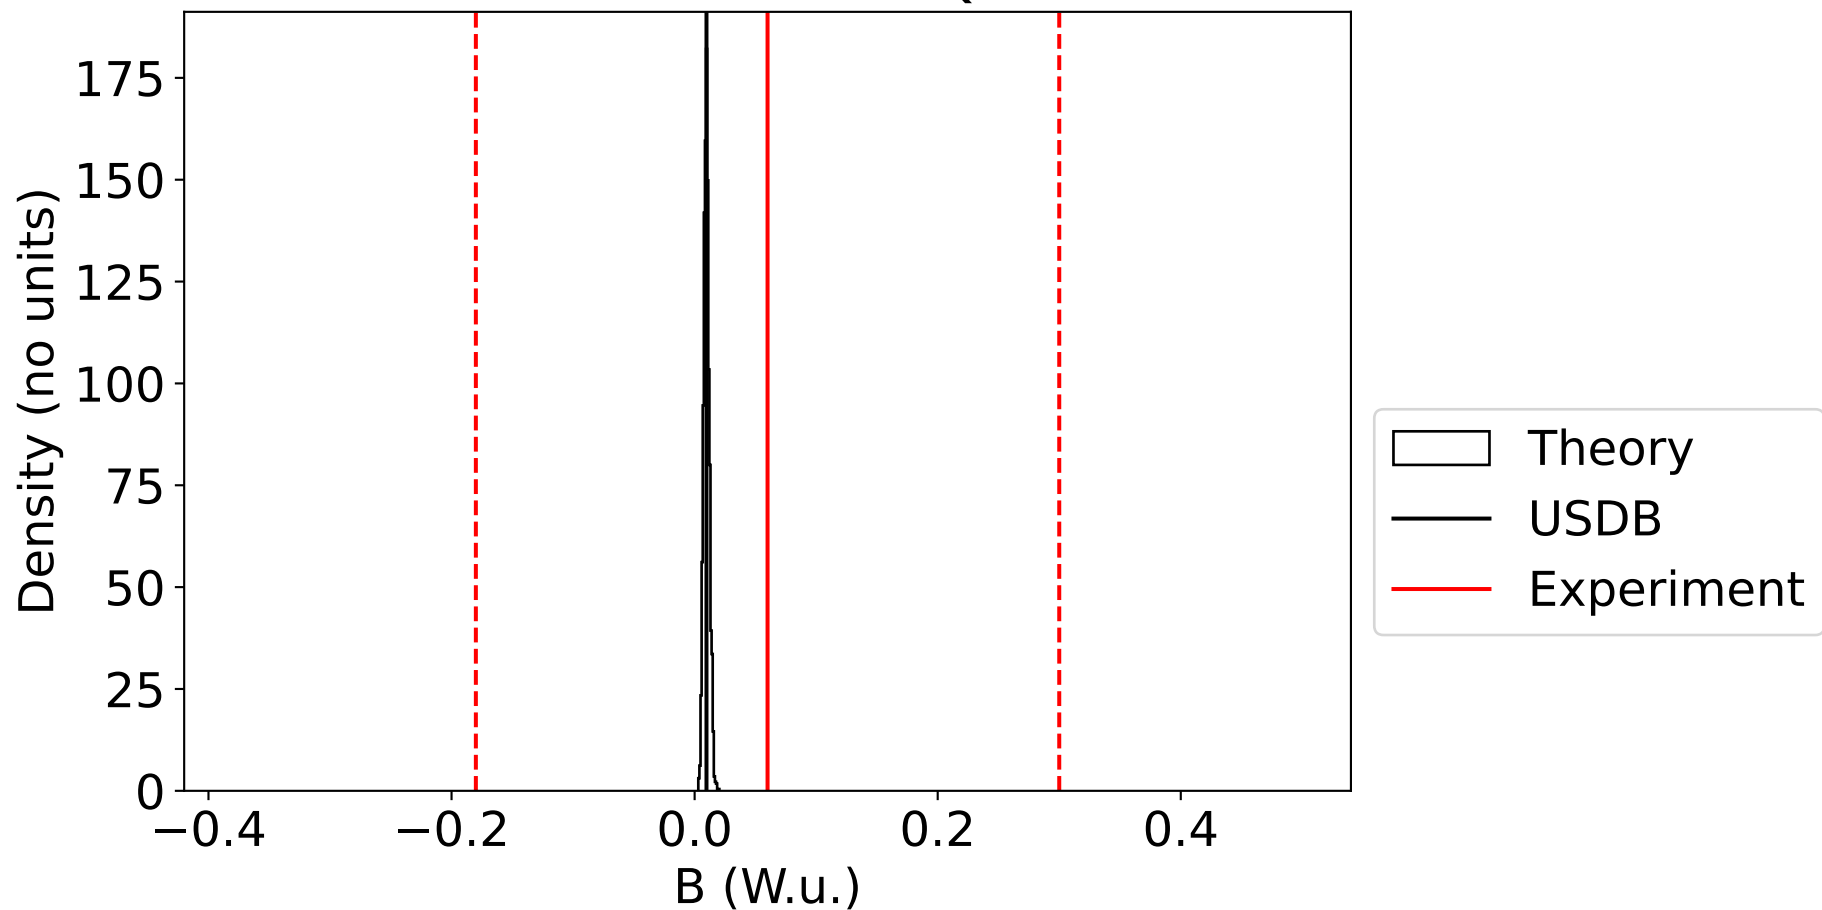

$^{33}\text{Cl} (1/2_1) \rightarrow (3/2_1)$   
Included in UQ

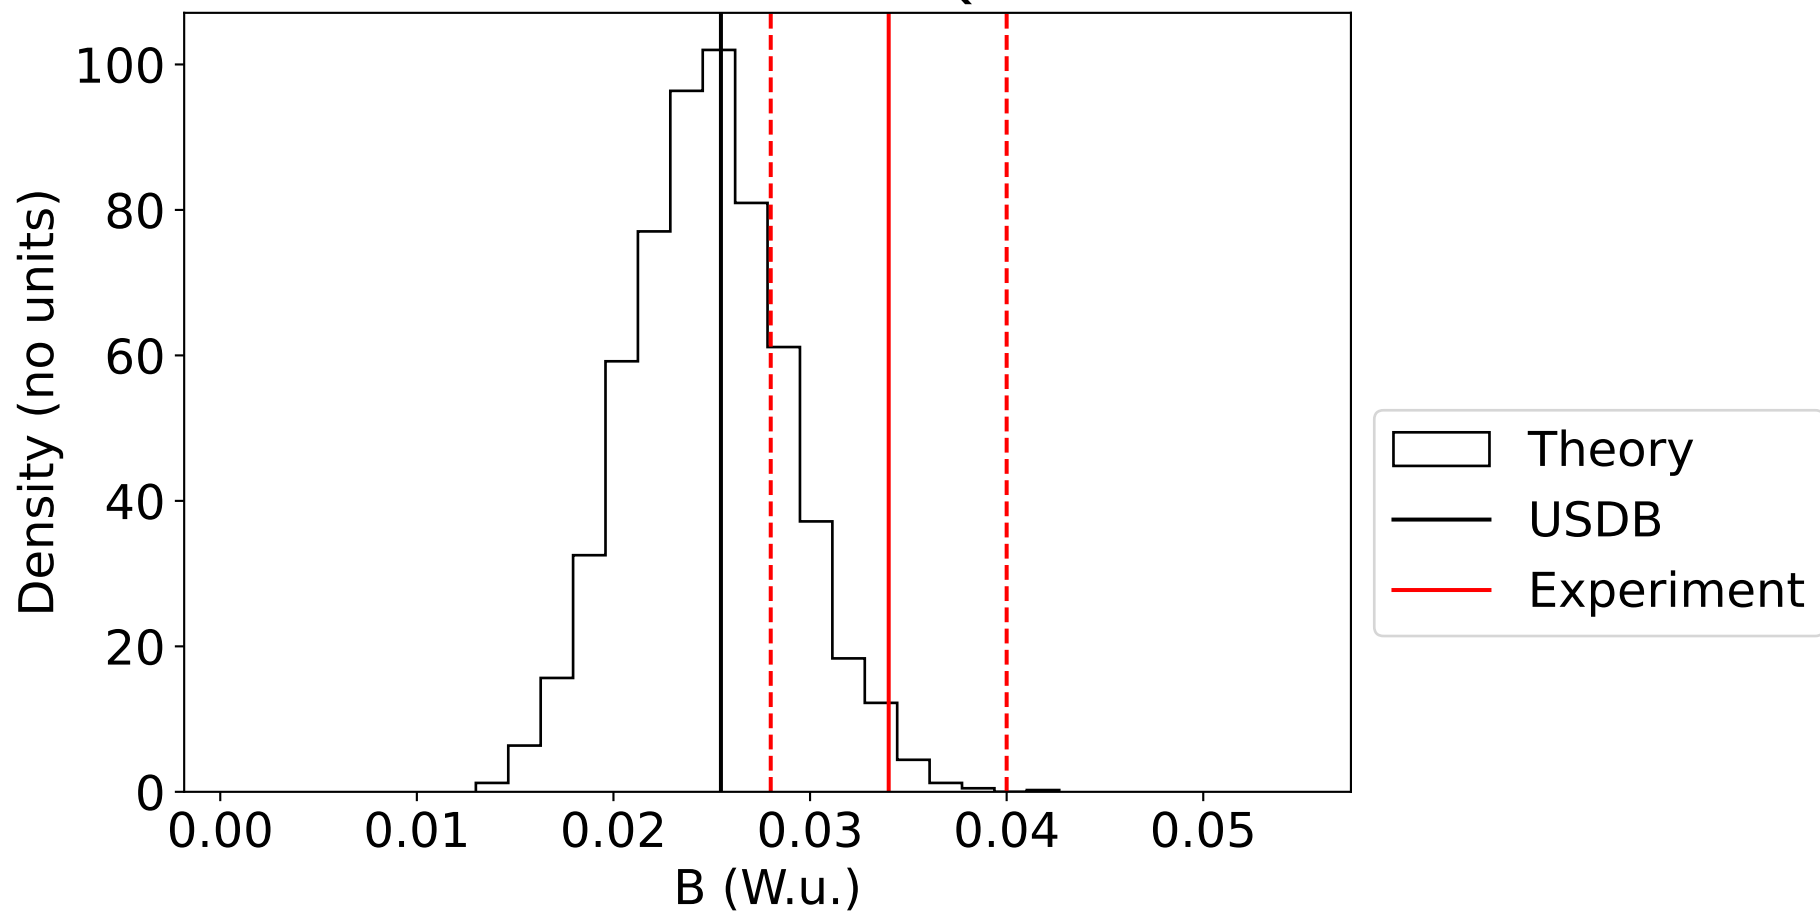

$^{33}\text{Cl} (5/2_1) \rightarrow (3/2_1)$   
Included in UQ

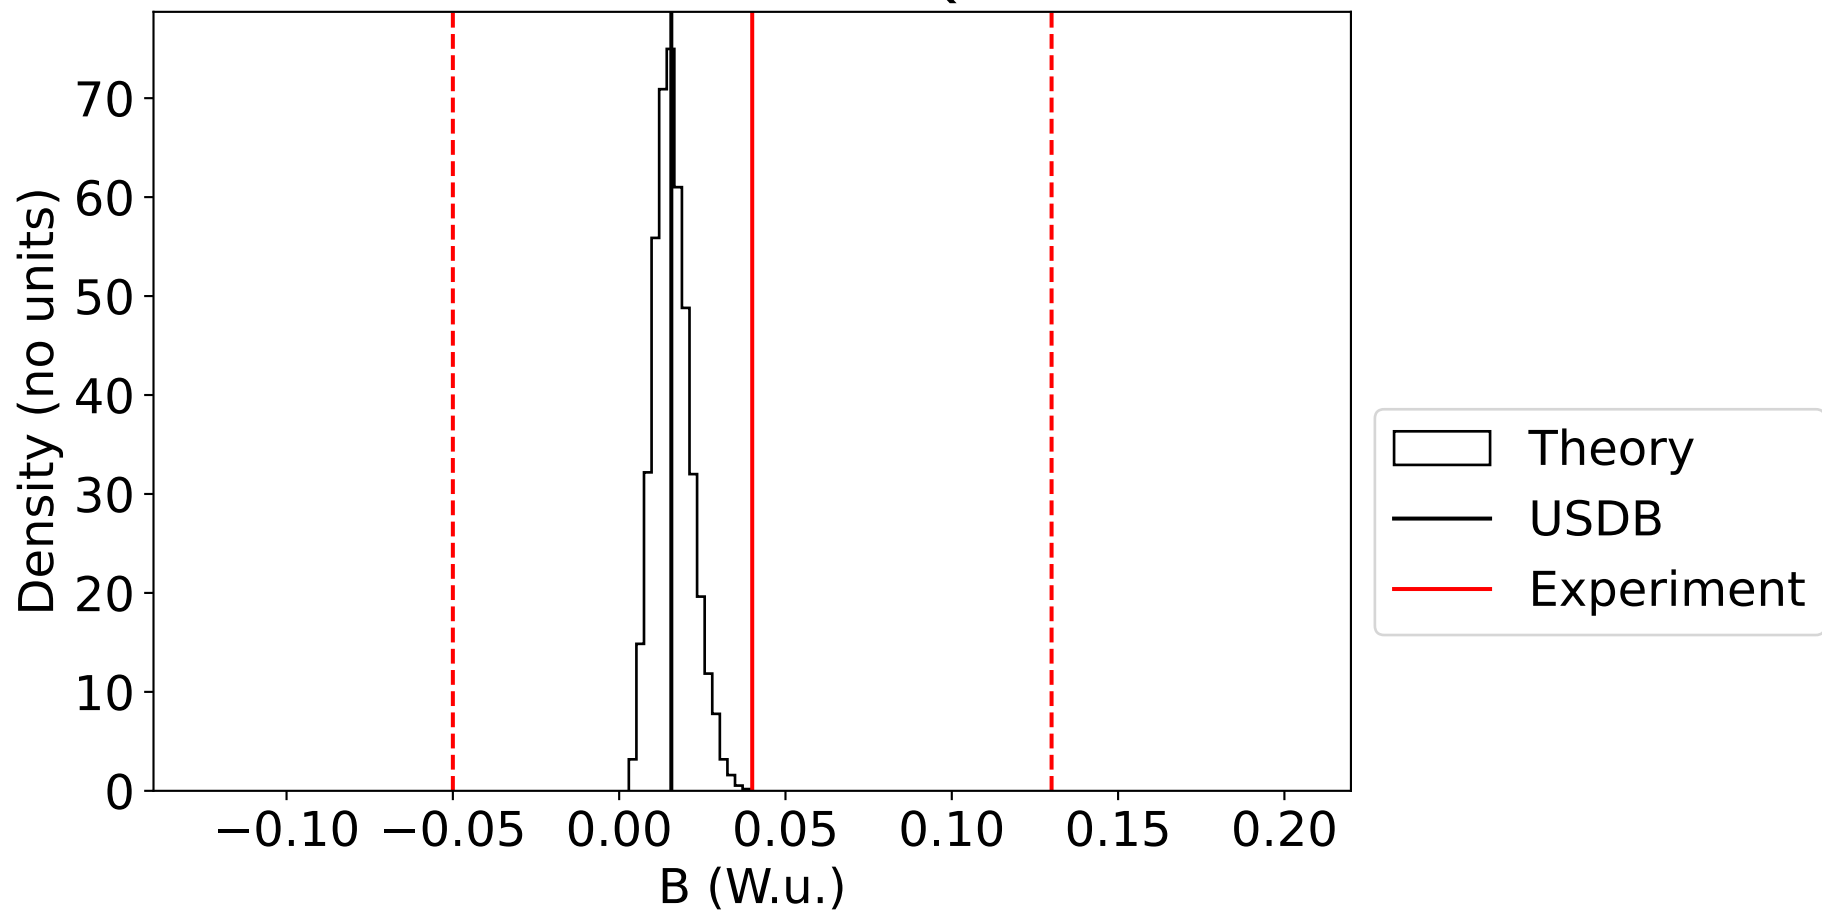

$^{33}\text{Cl} (3/2_2) \rightarrow (1/2_1)$   
Included in UQ

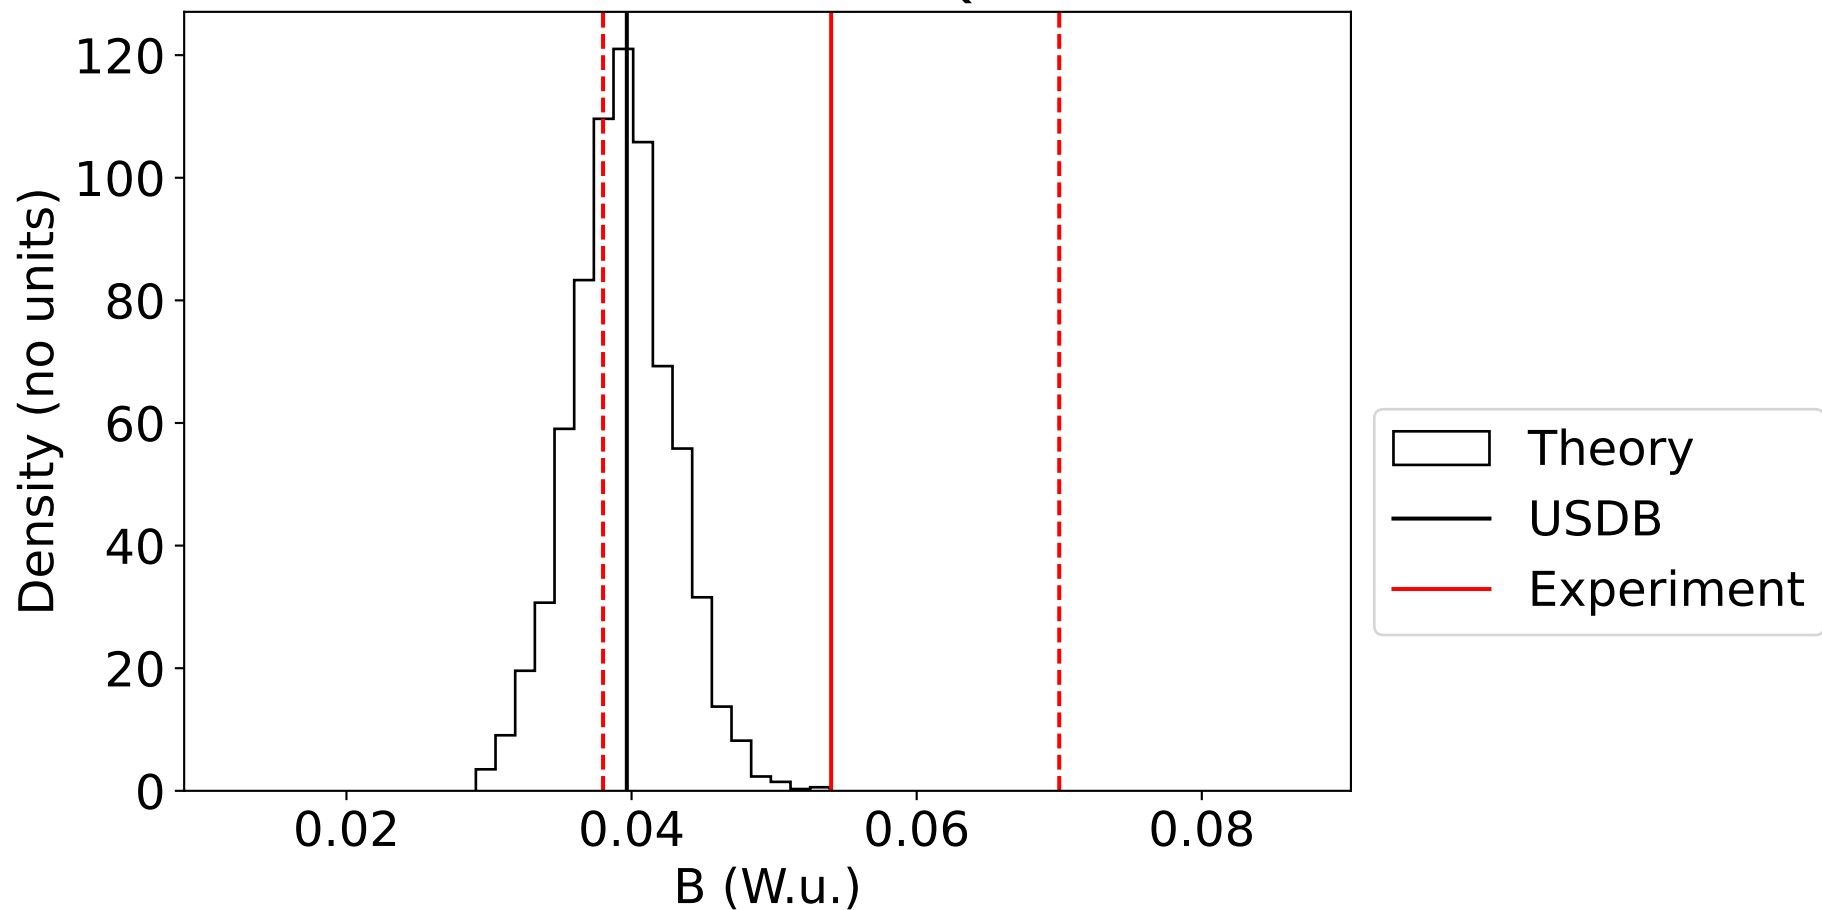

$^{33}\text{Cl} (5/2_2) \rightarrow (3/2_1)$   
Included in UQ

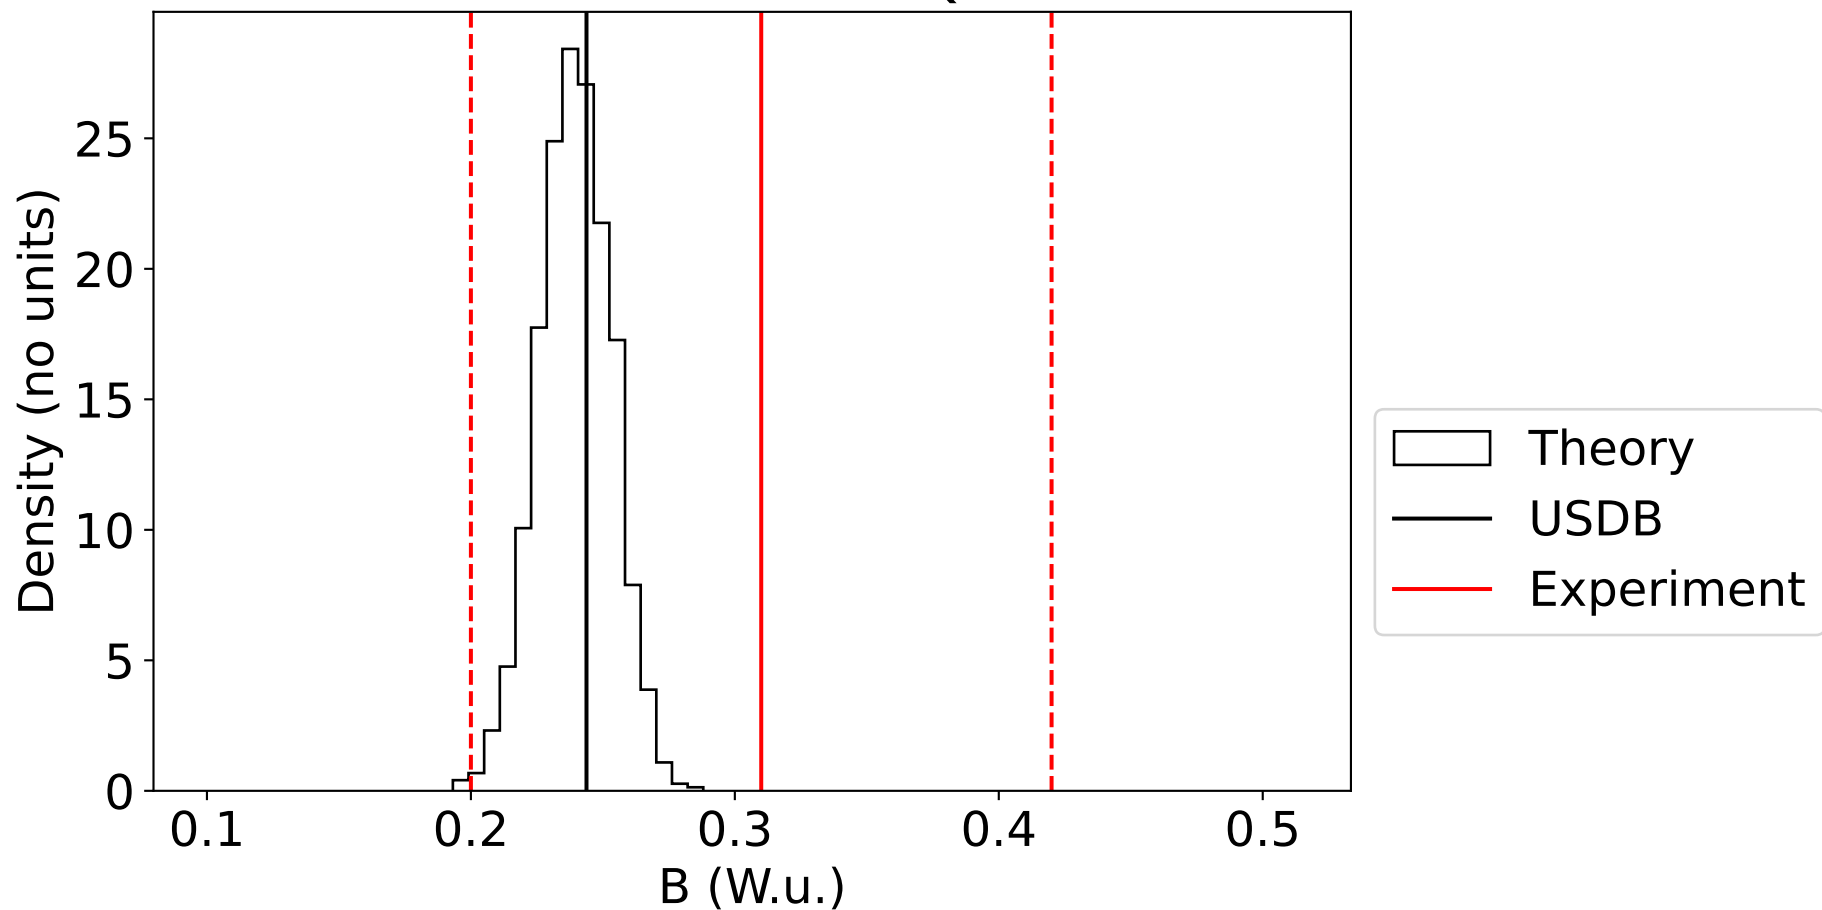

$^{33}\text{Cl} (7/2_1) \rightarrow (5/2_1)$   
Included in UQ

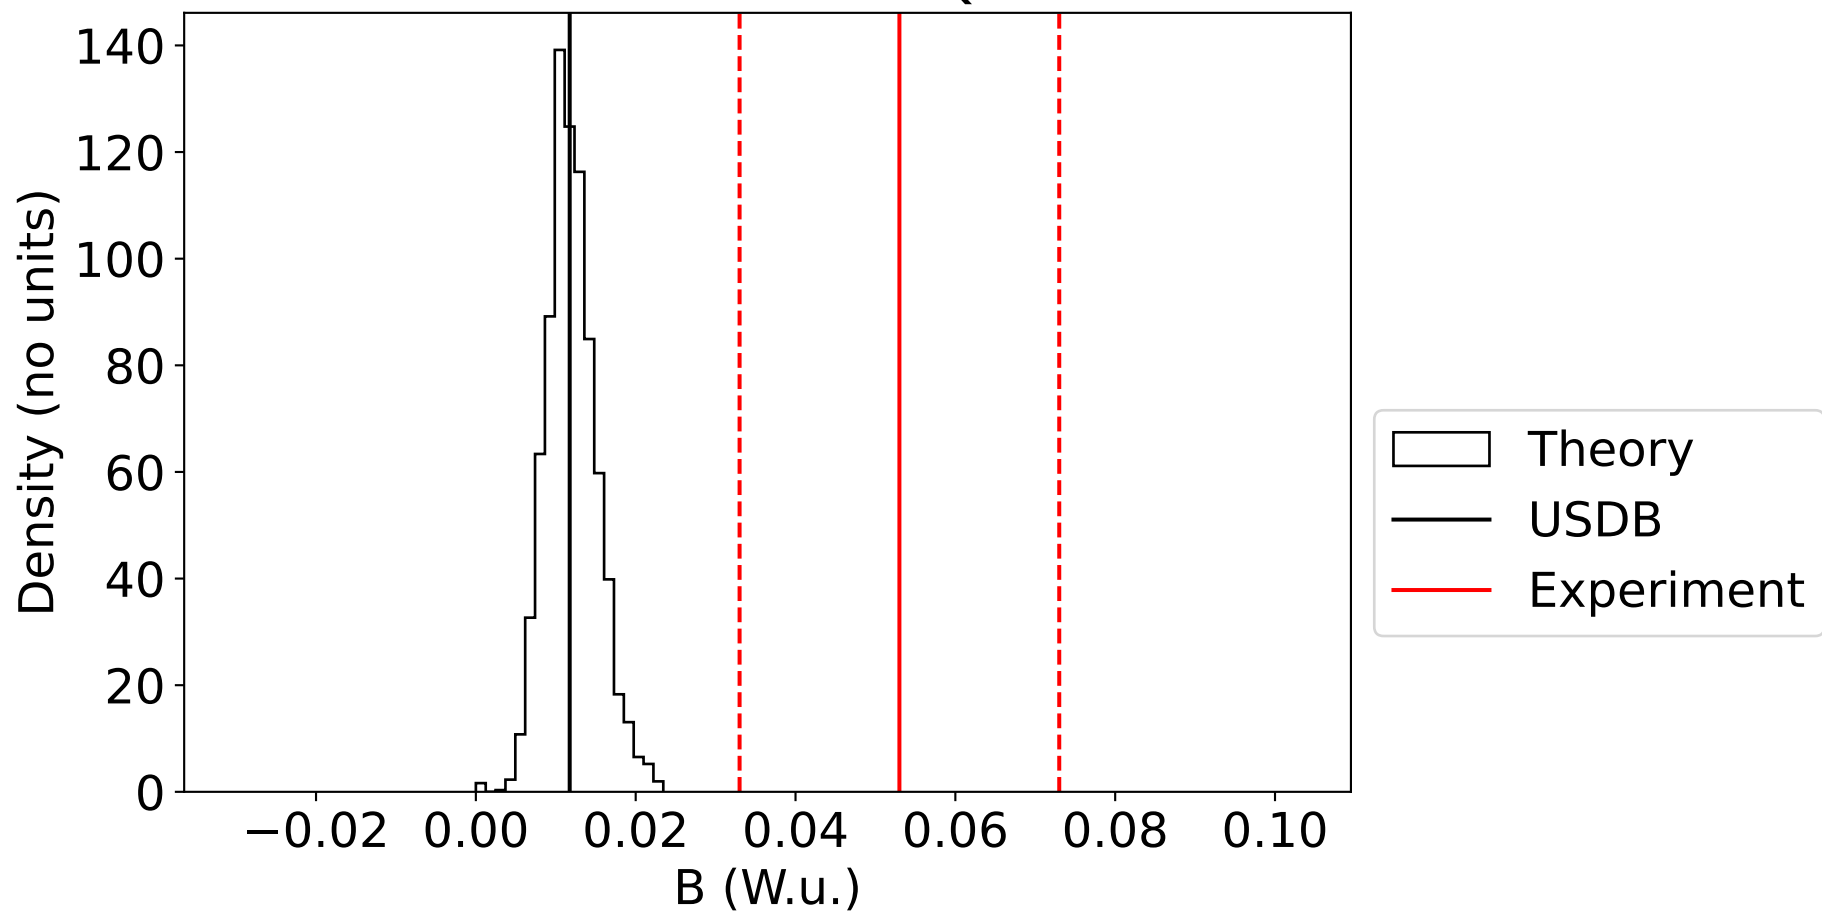



$^{34}\text{Cl} (1_1) \rightarrow (0_1)$   
Included in UQ

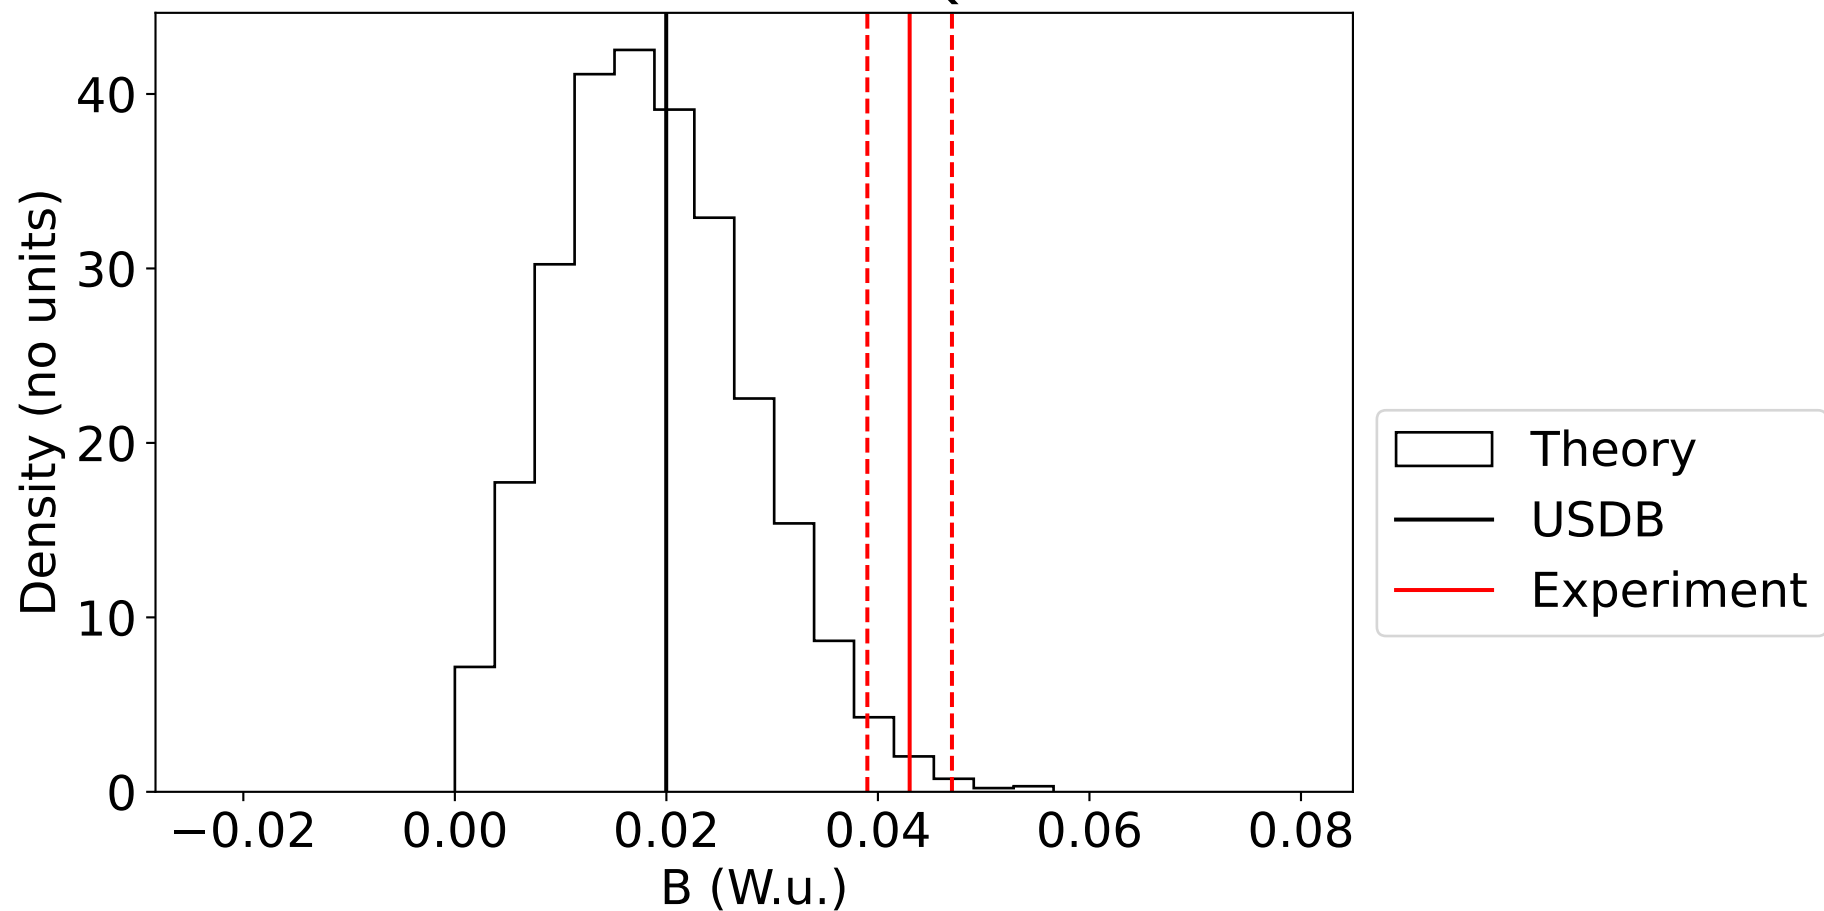

$^{34}\text{Cl} (1_3) \rightarrow (0_1)$   
Included in UQ

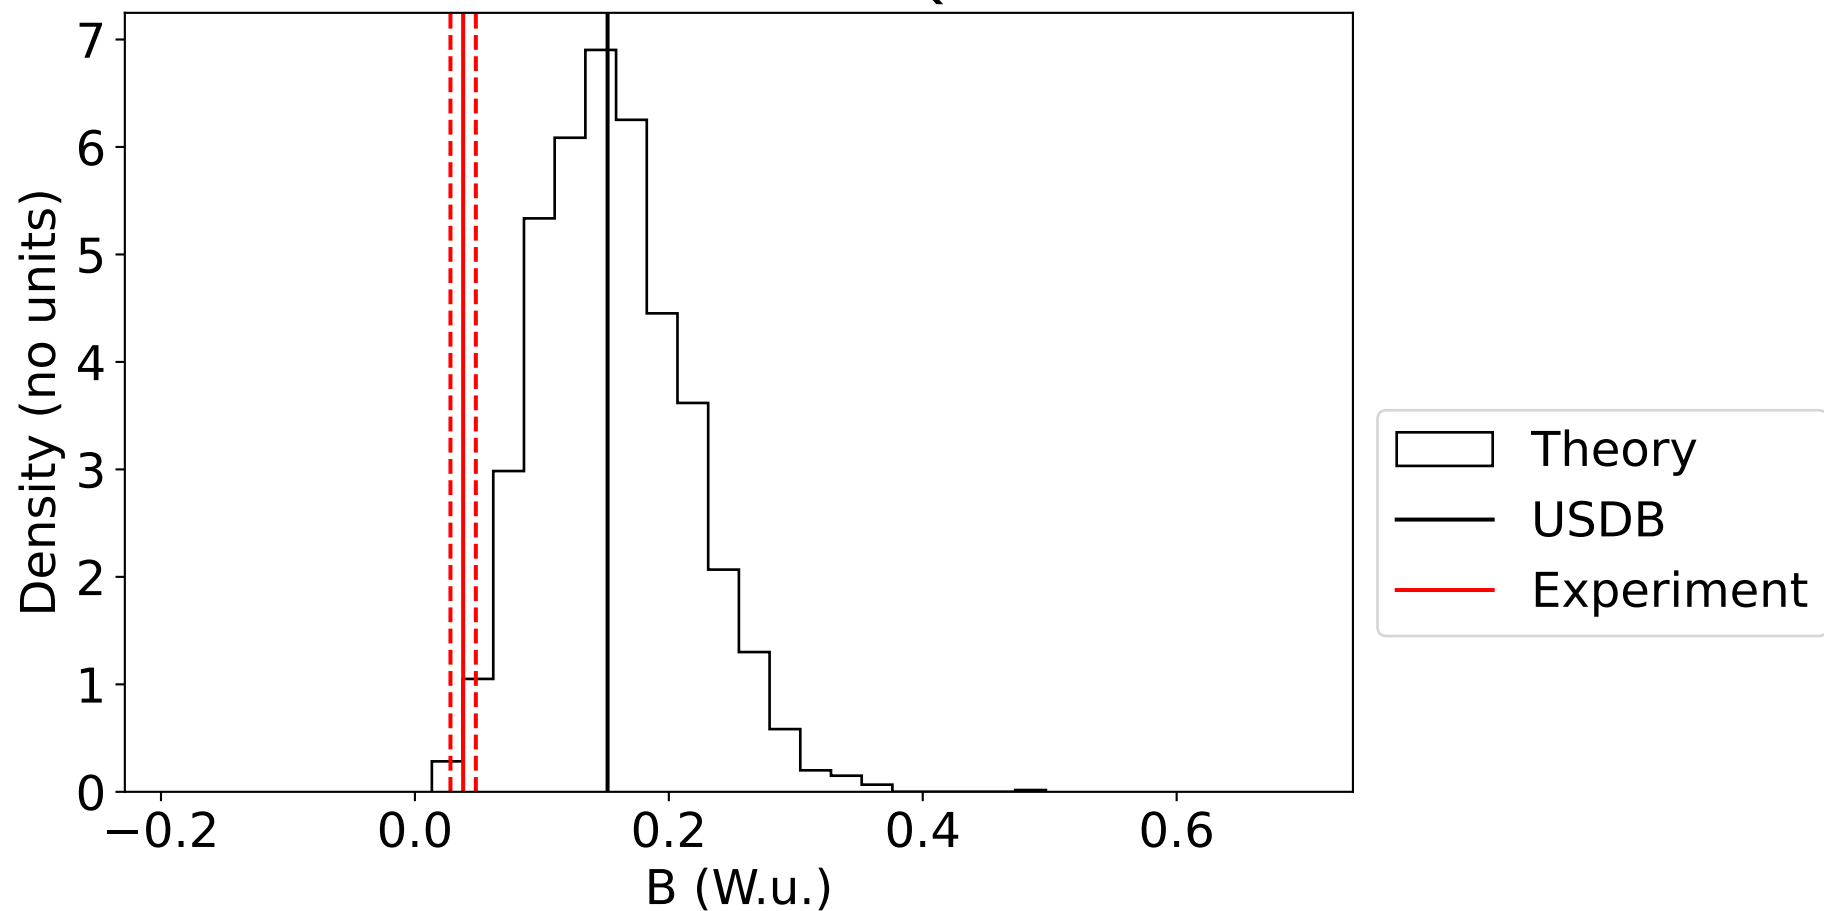

$^{35}\text{Cl} (1/2_1) \rightarrow (3/2_1)$   
Included in UQ

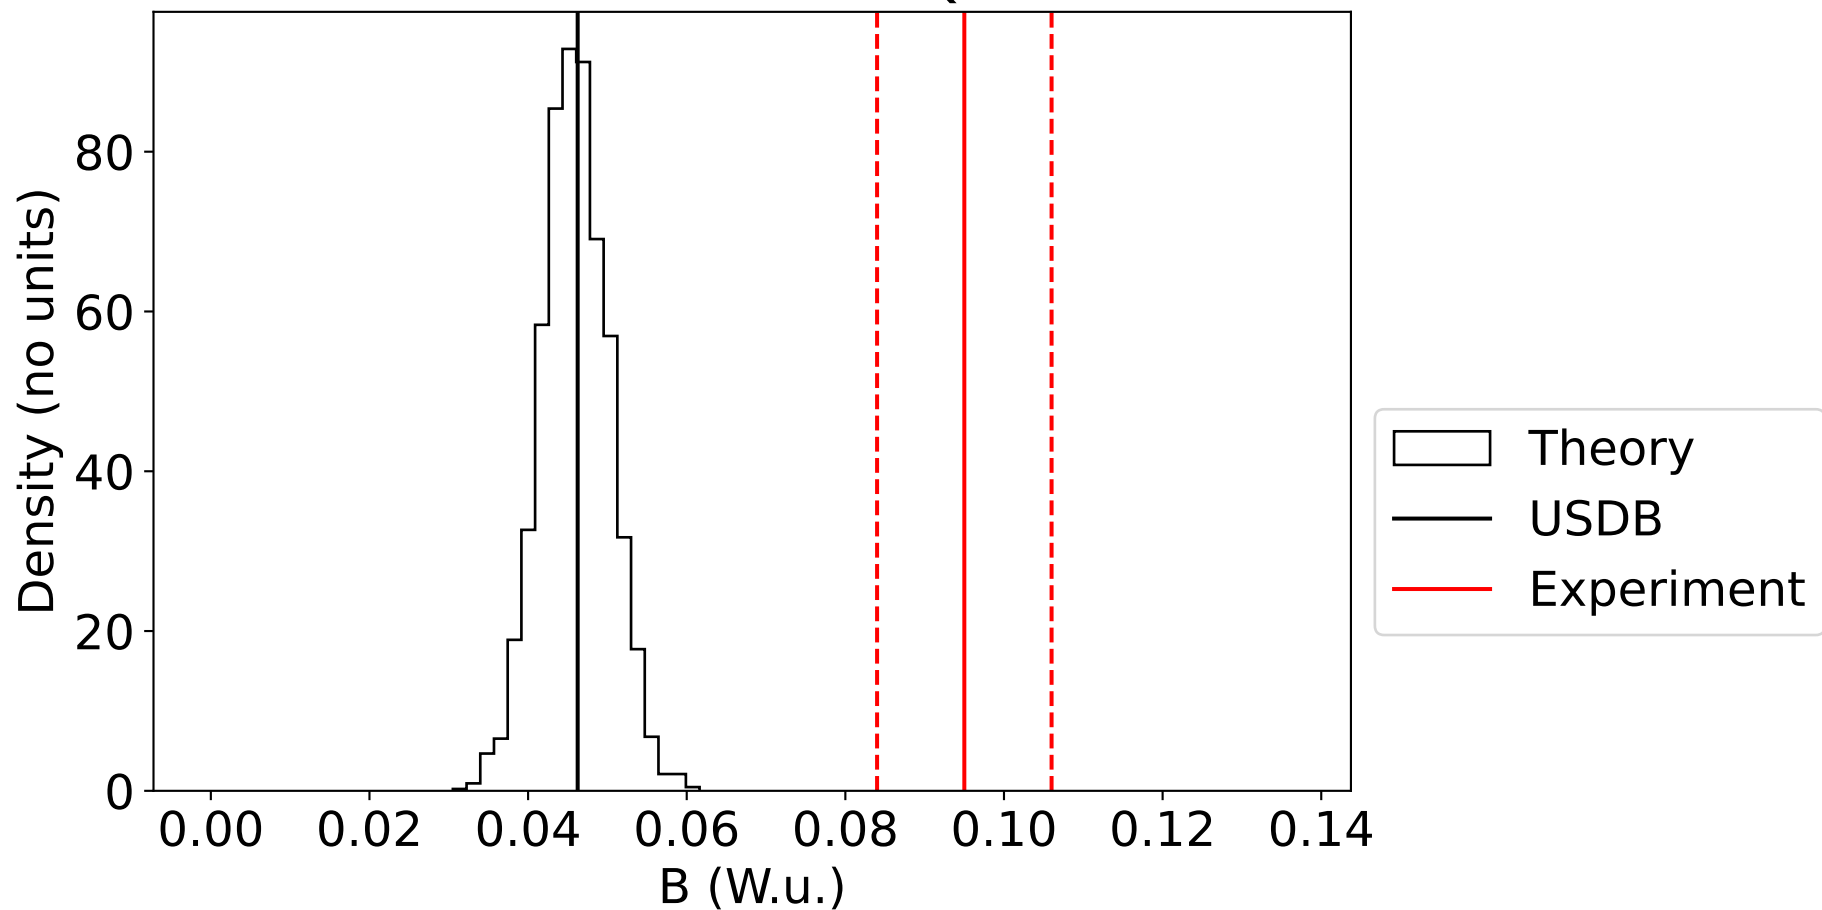

$^{35}\text{Cl} (7/2_1) \rightarrow (5/2_1)$   
Included in UQ

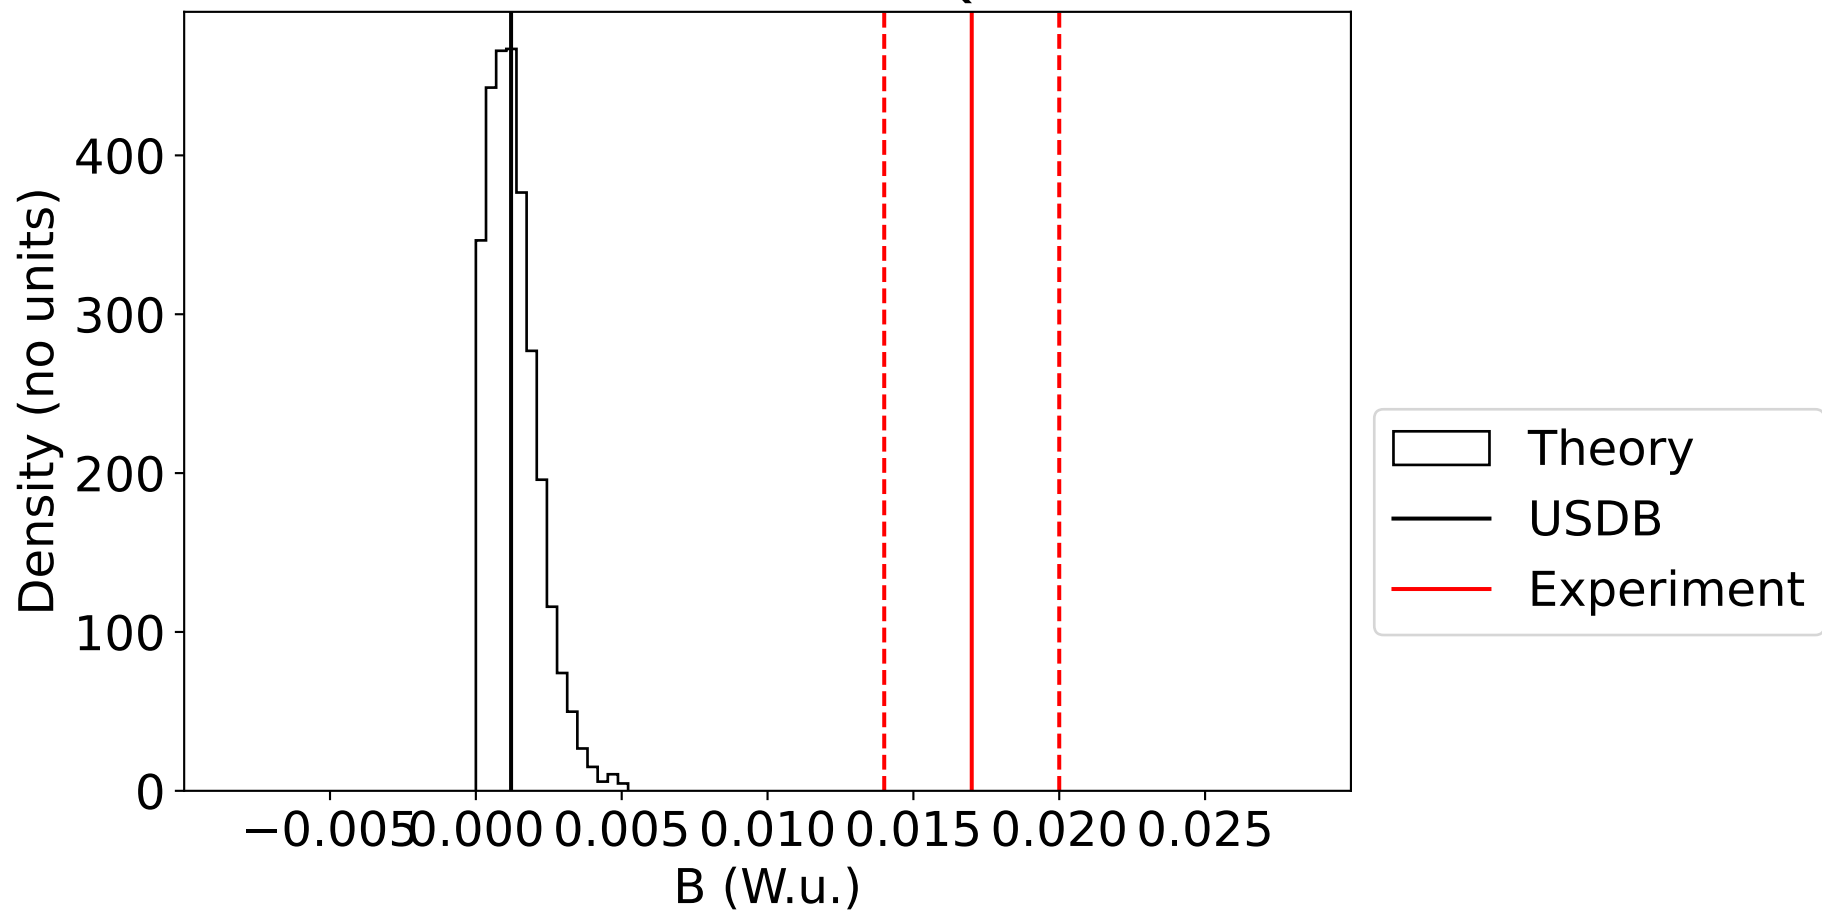

$^{35}\text{Cl} (3/2_2) \rightarrow (5/2_1)$   
Included in UQ

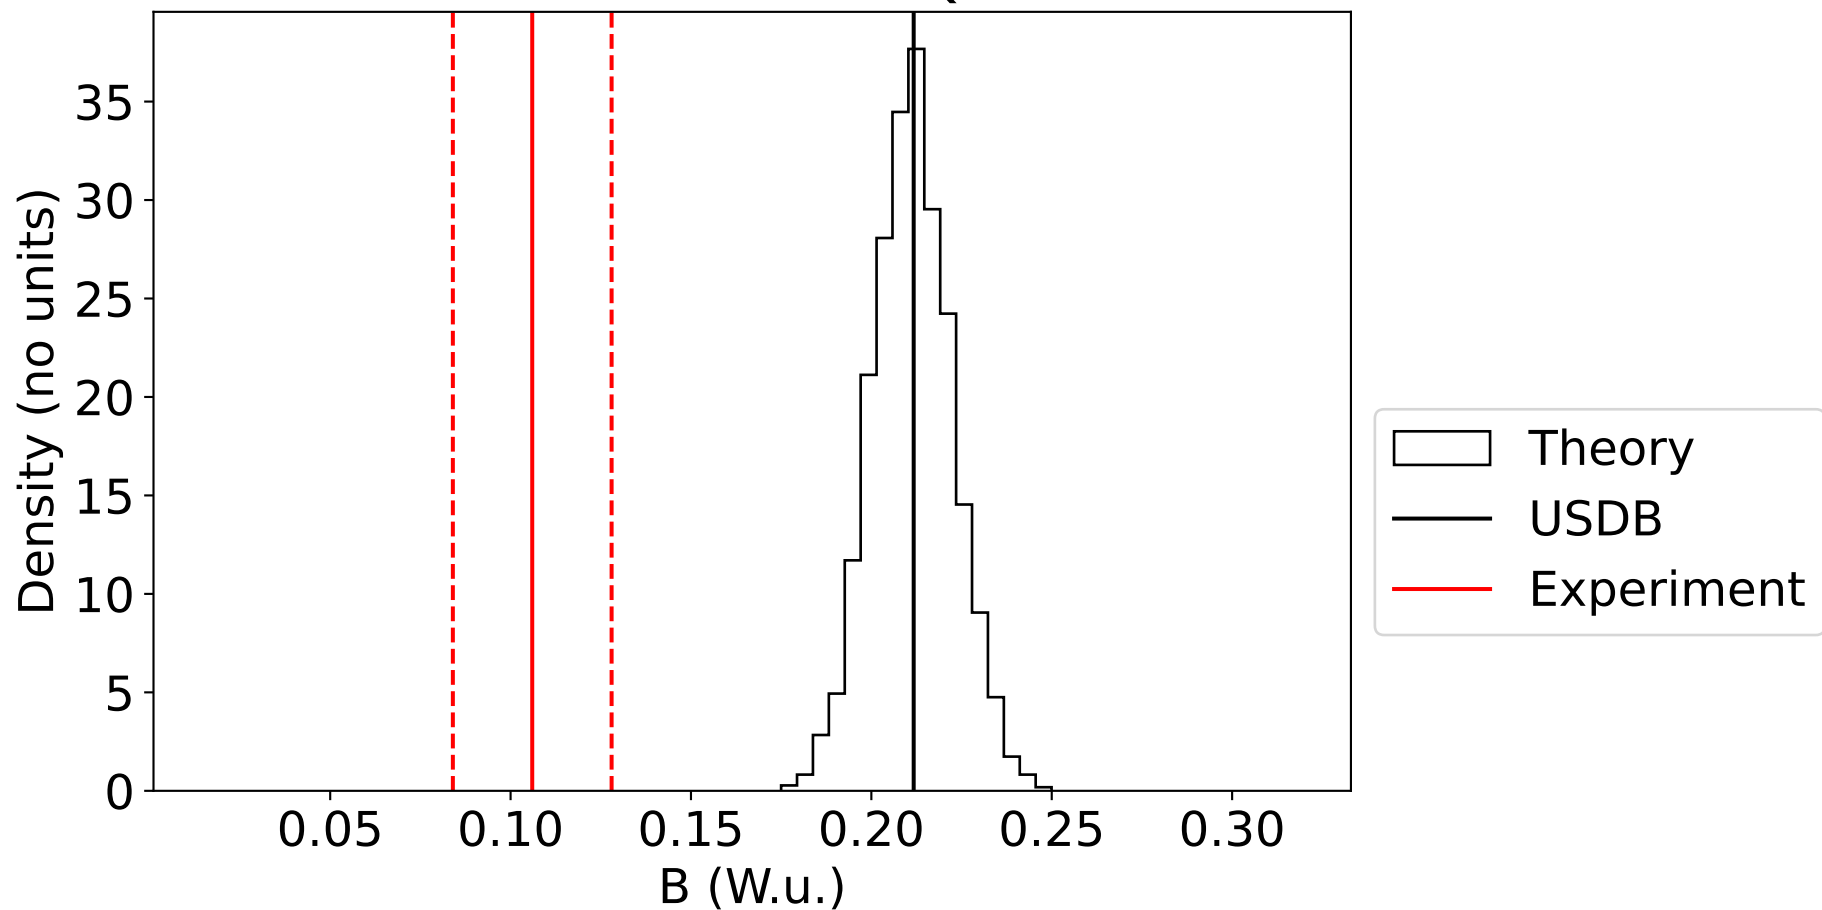

$^{35}\text{Cl } (3/2_2) \rightarrow (3/2_1)$   
Included in UQ

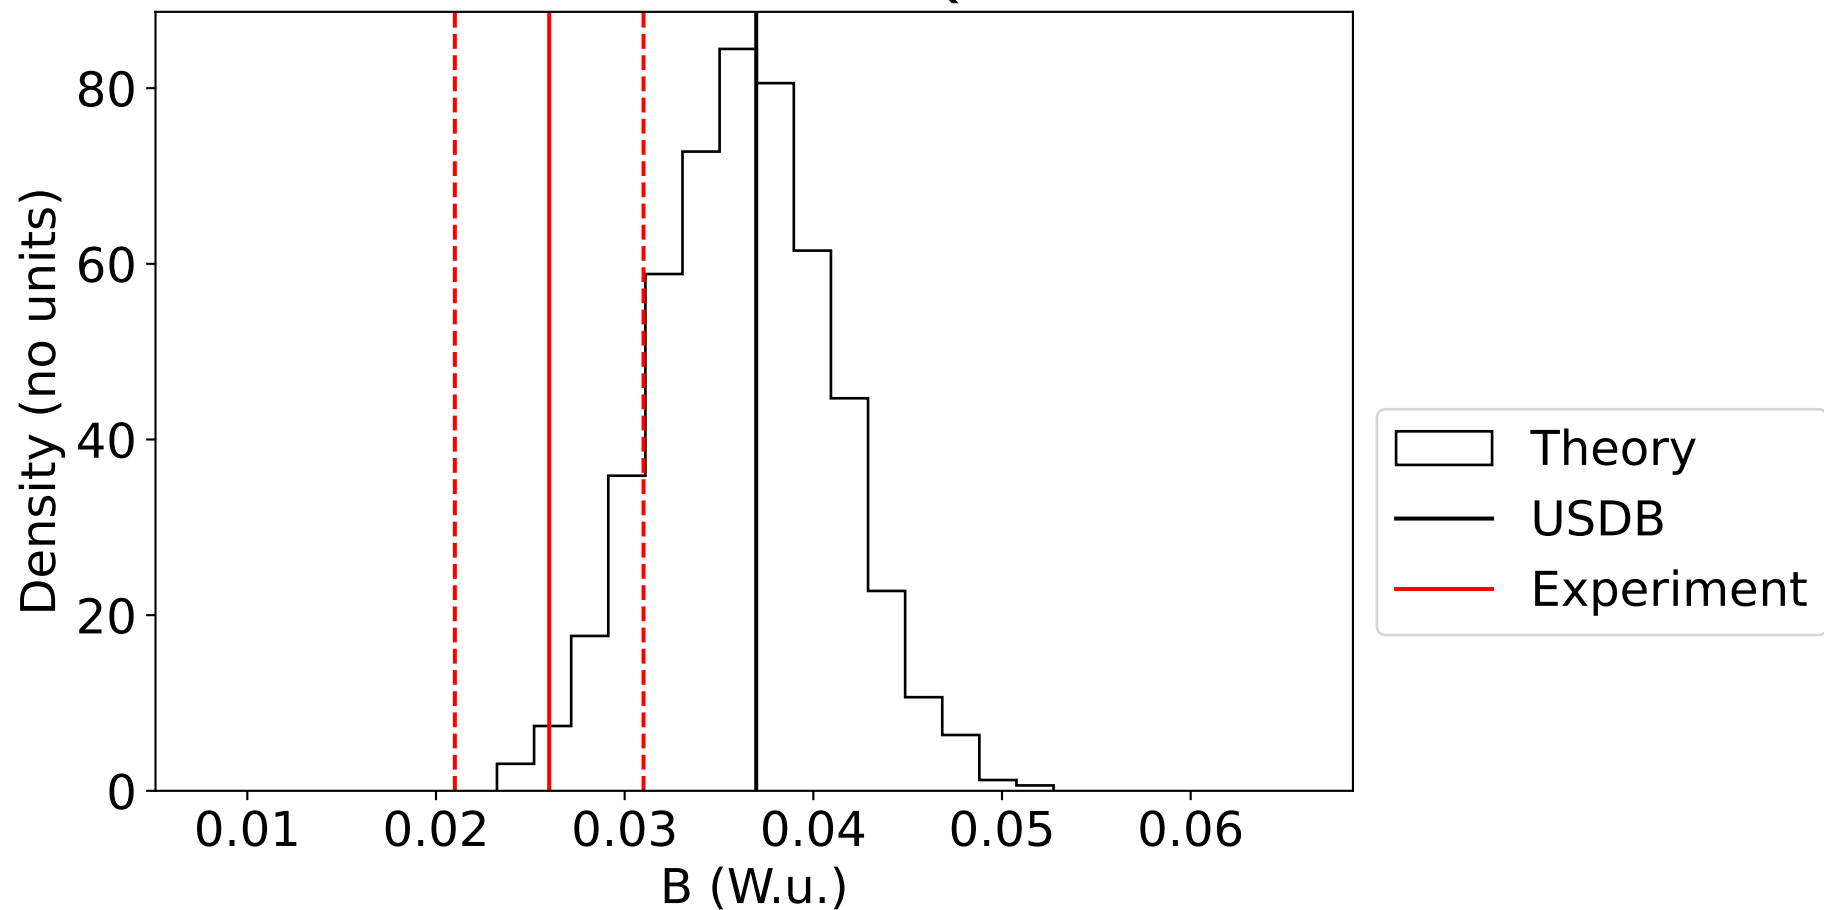

$^{35}\text{Cl} (3/2_2) \rightarrow (1/2_1)$   
Included in UQ

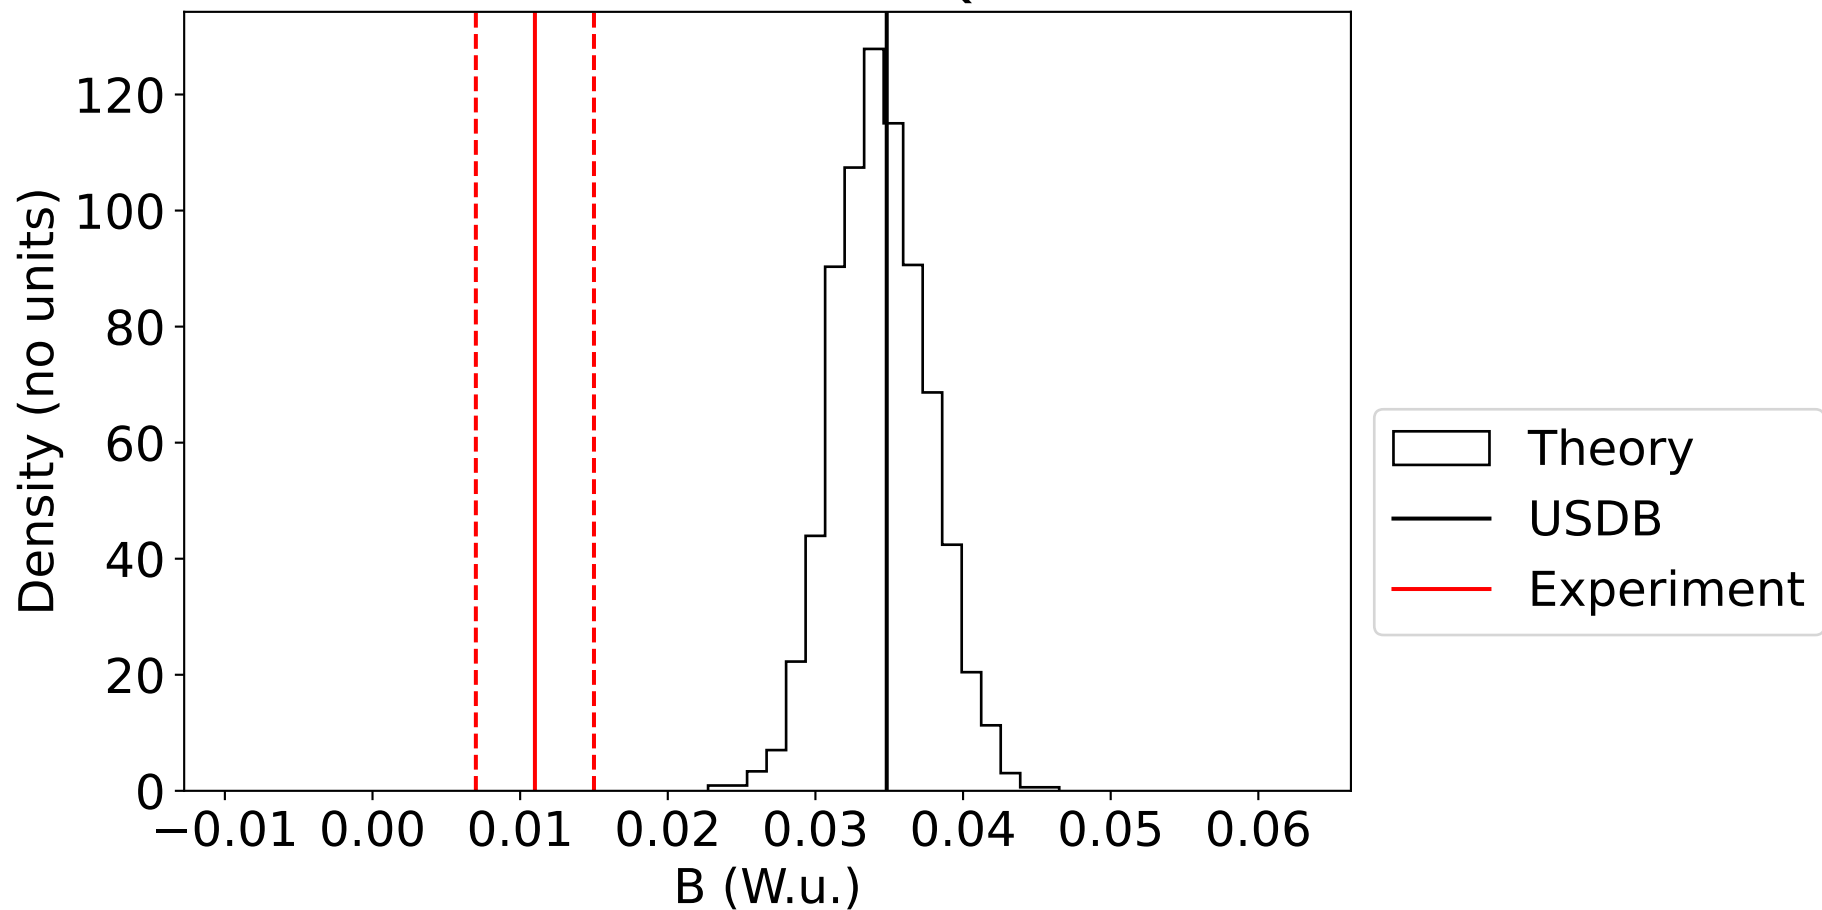

$^{35}\text{Cl} (5/2_2) \rightarrow (3/2_1)$   
Included in UQ

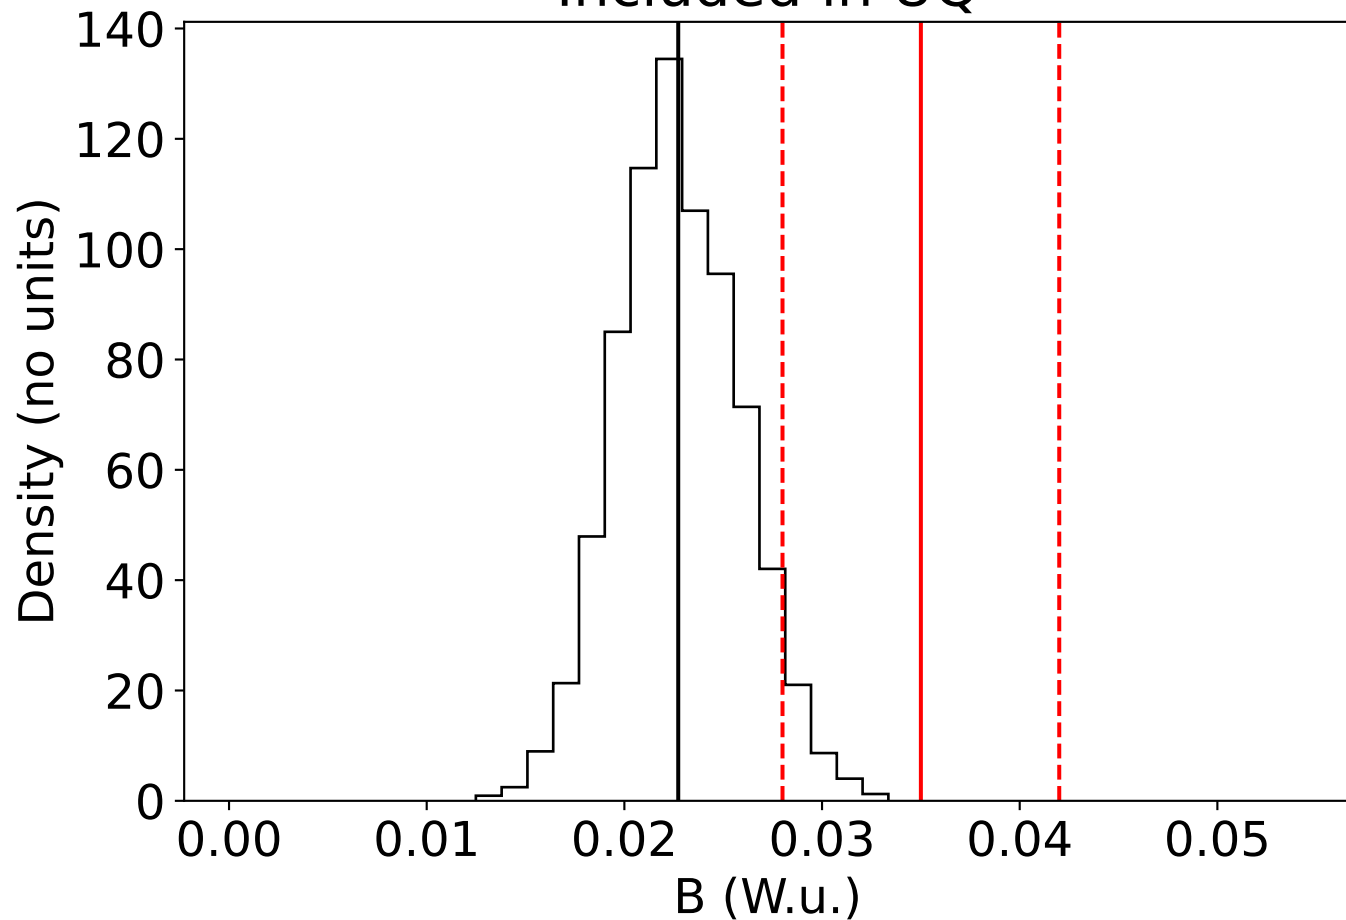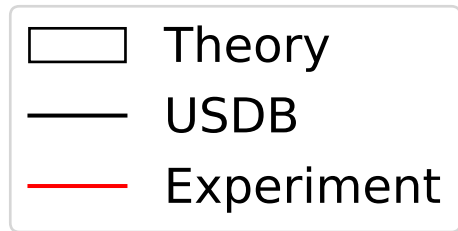



$^{35}\text{Cl} (3/2_3) \rightarrow (3/2_1)$   
Included in UQ

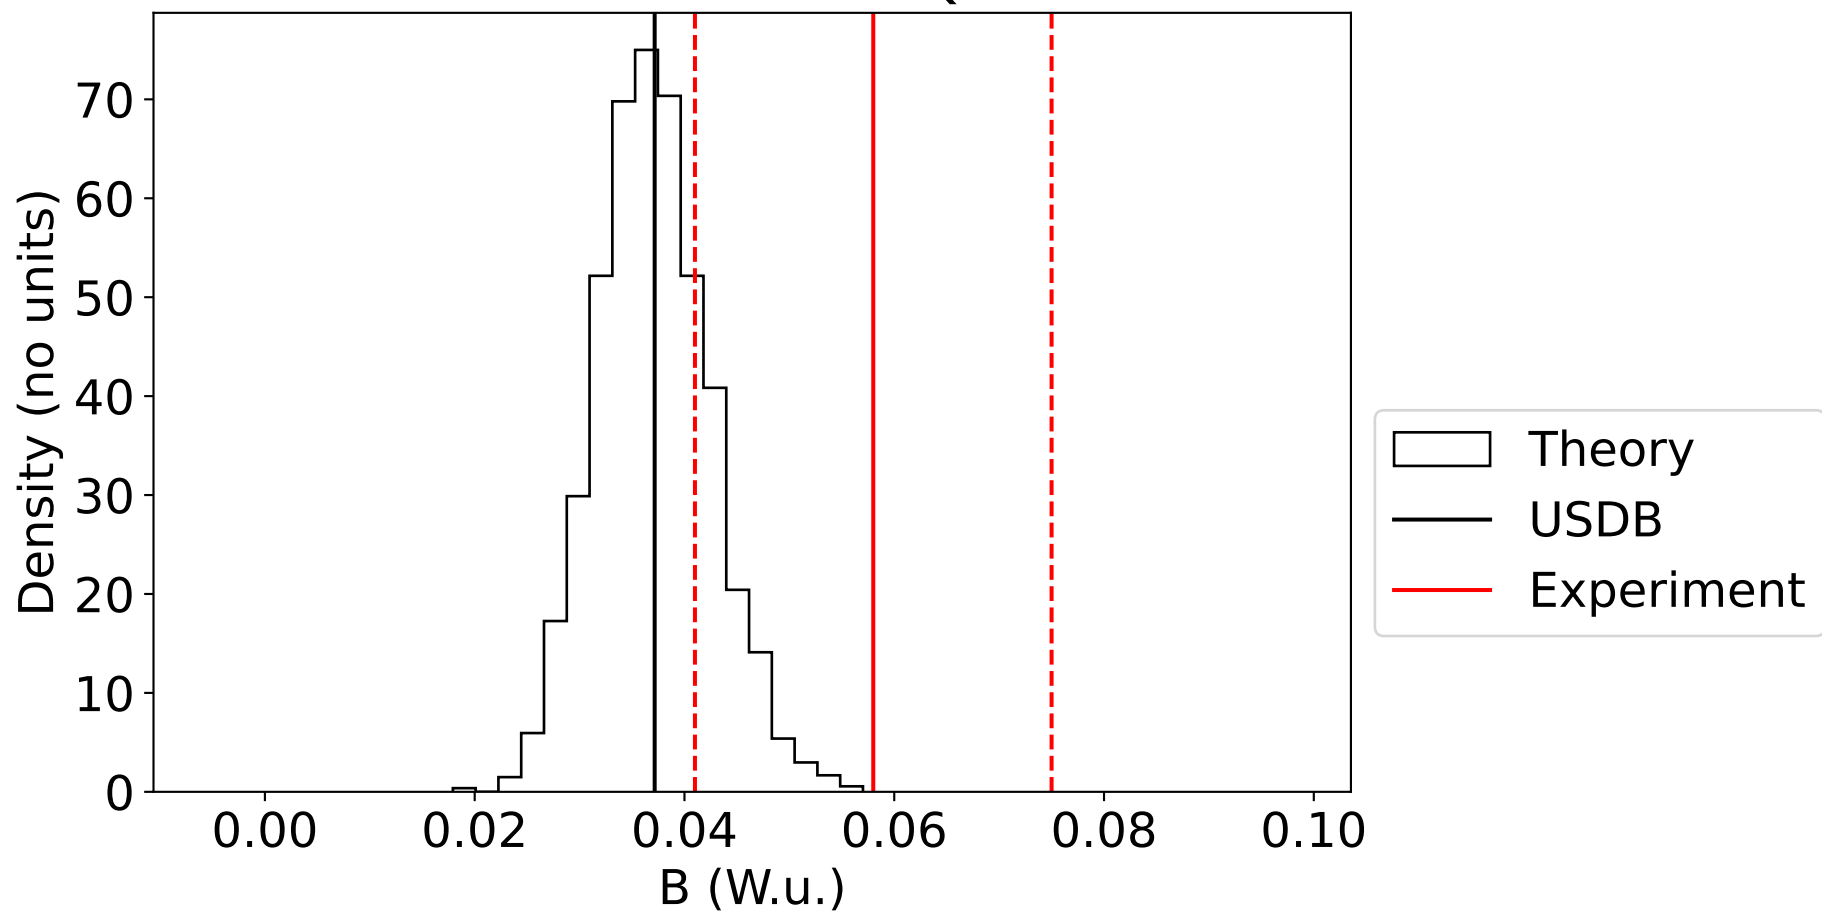

$^{35}\text{Cl} (1/2_2) \rightarrow (1/2_1)$   
Included in UQ

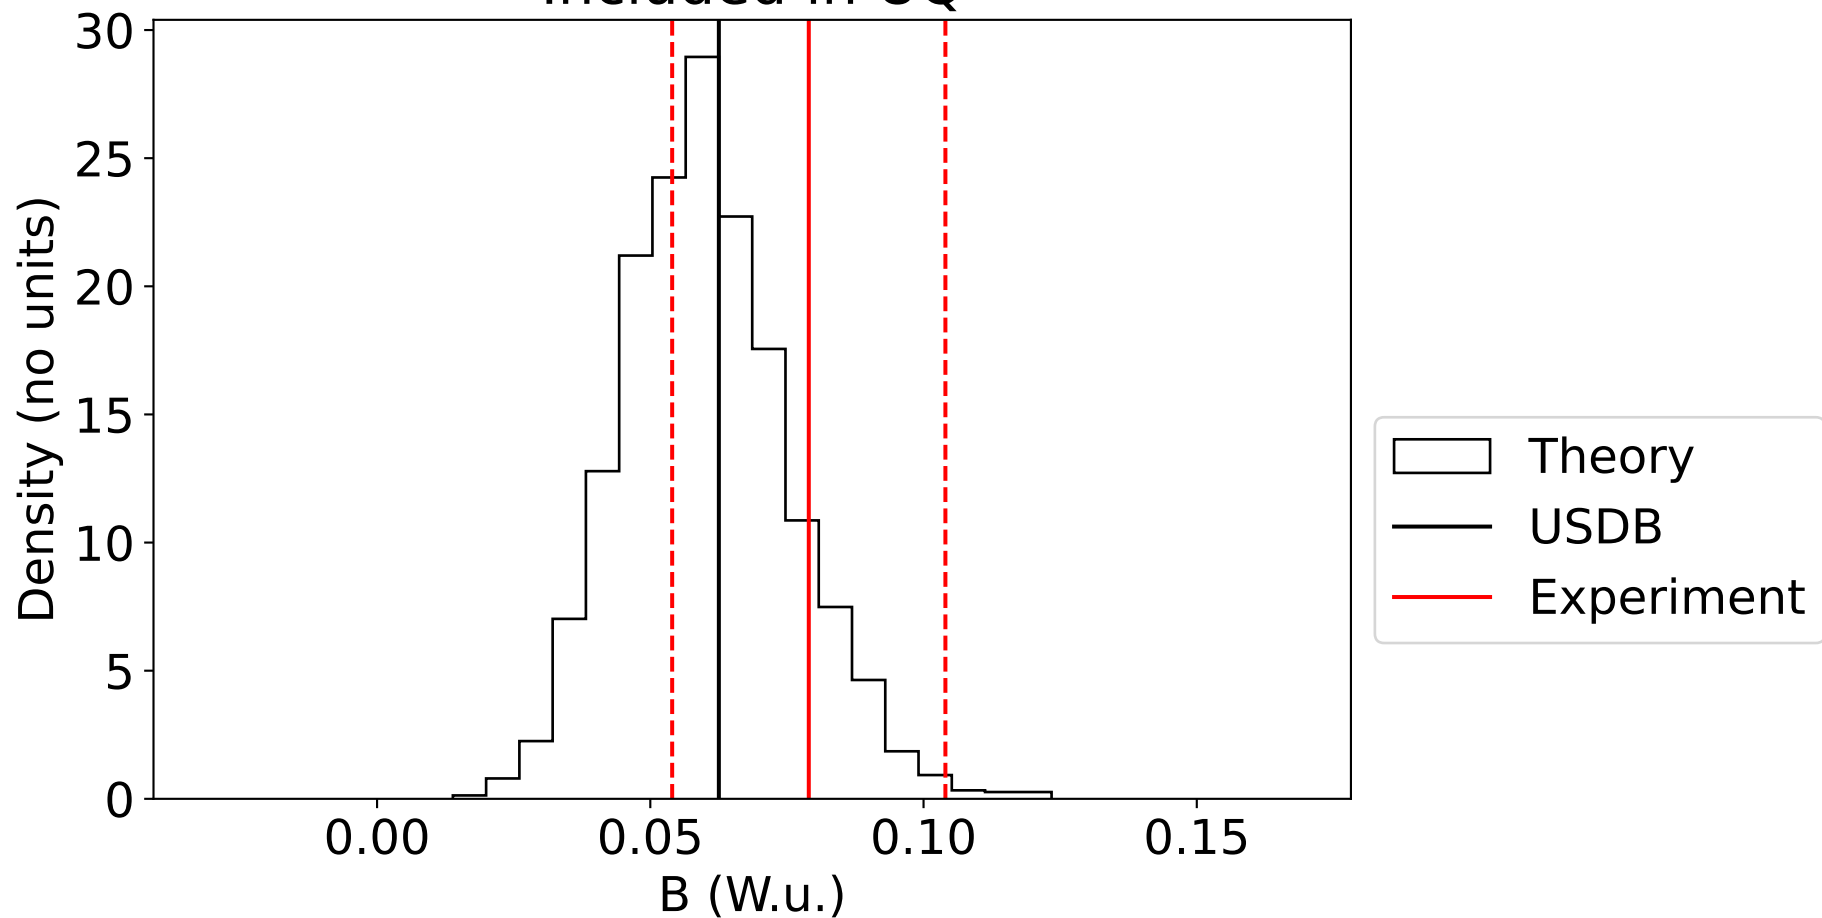

$^{35}\text{Cl} (7/2_2) \rightarrow (5/2_1)$   
Included in UQ

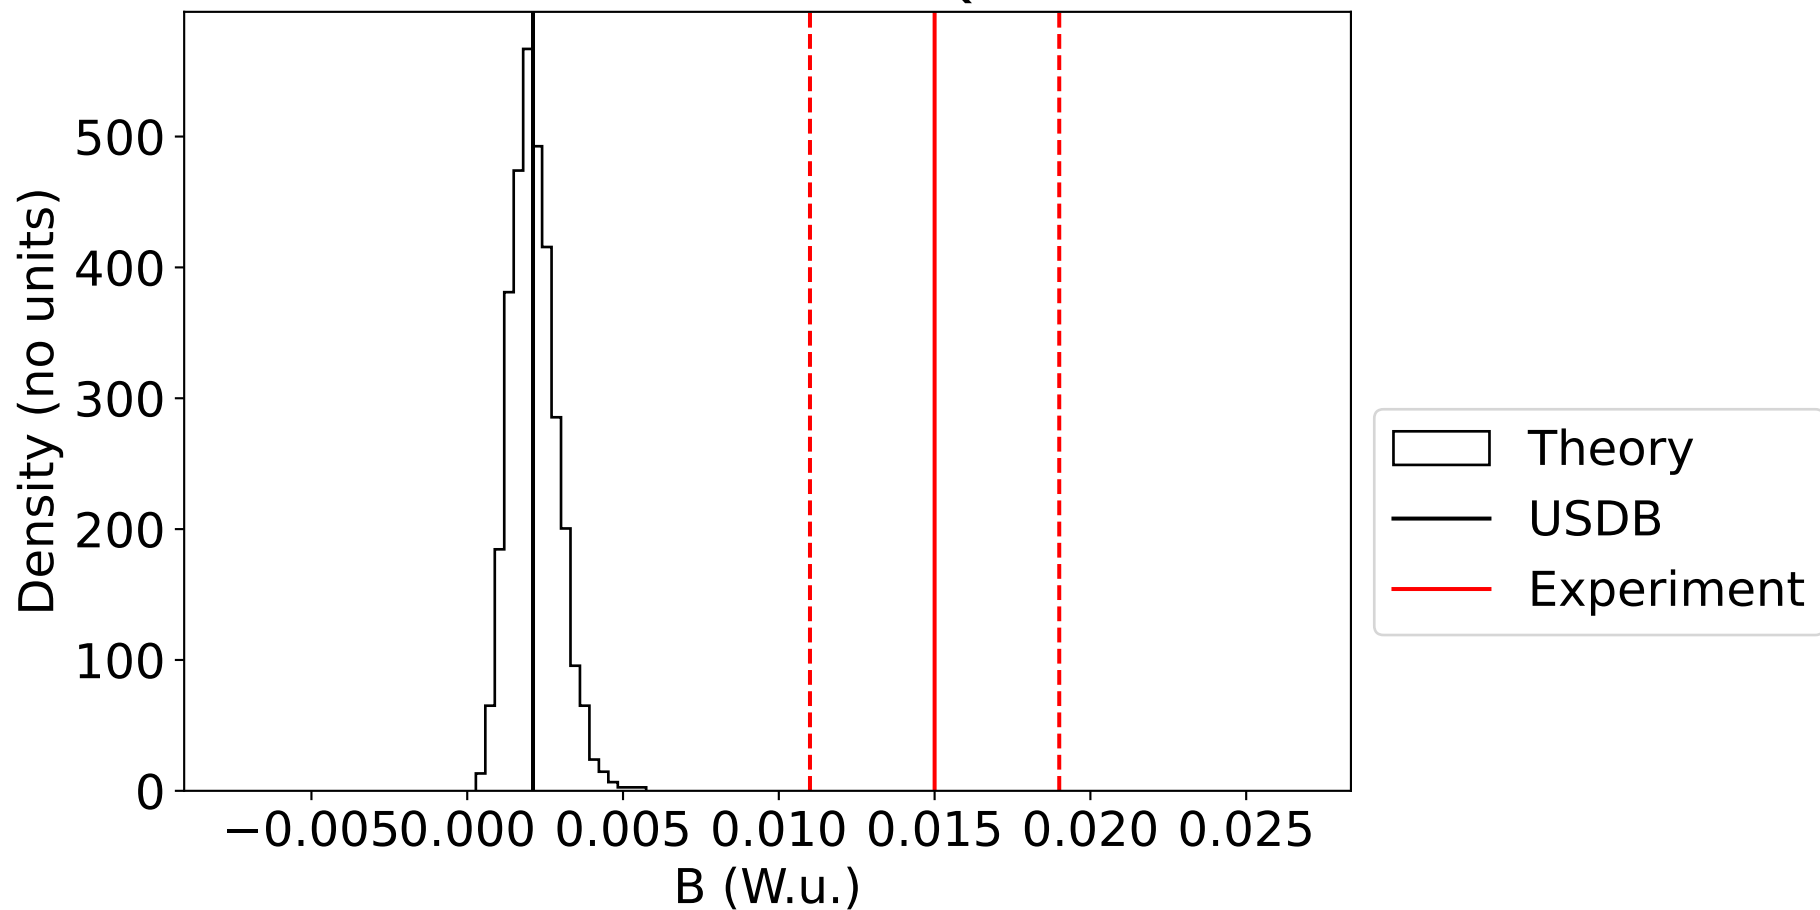

$^{36}\text{Cl} (2_3) \rightarrow (1_1)$   
Included in UQ

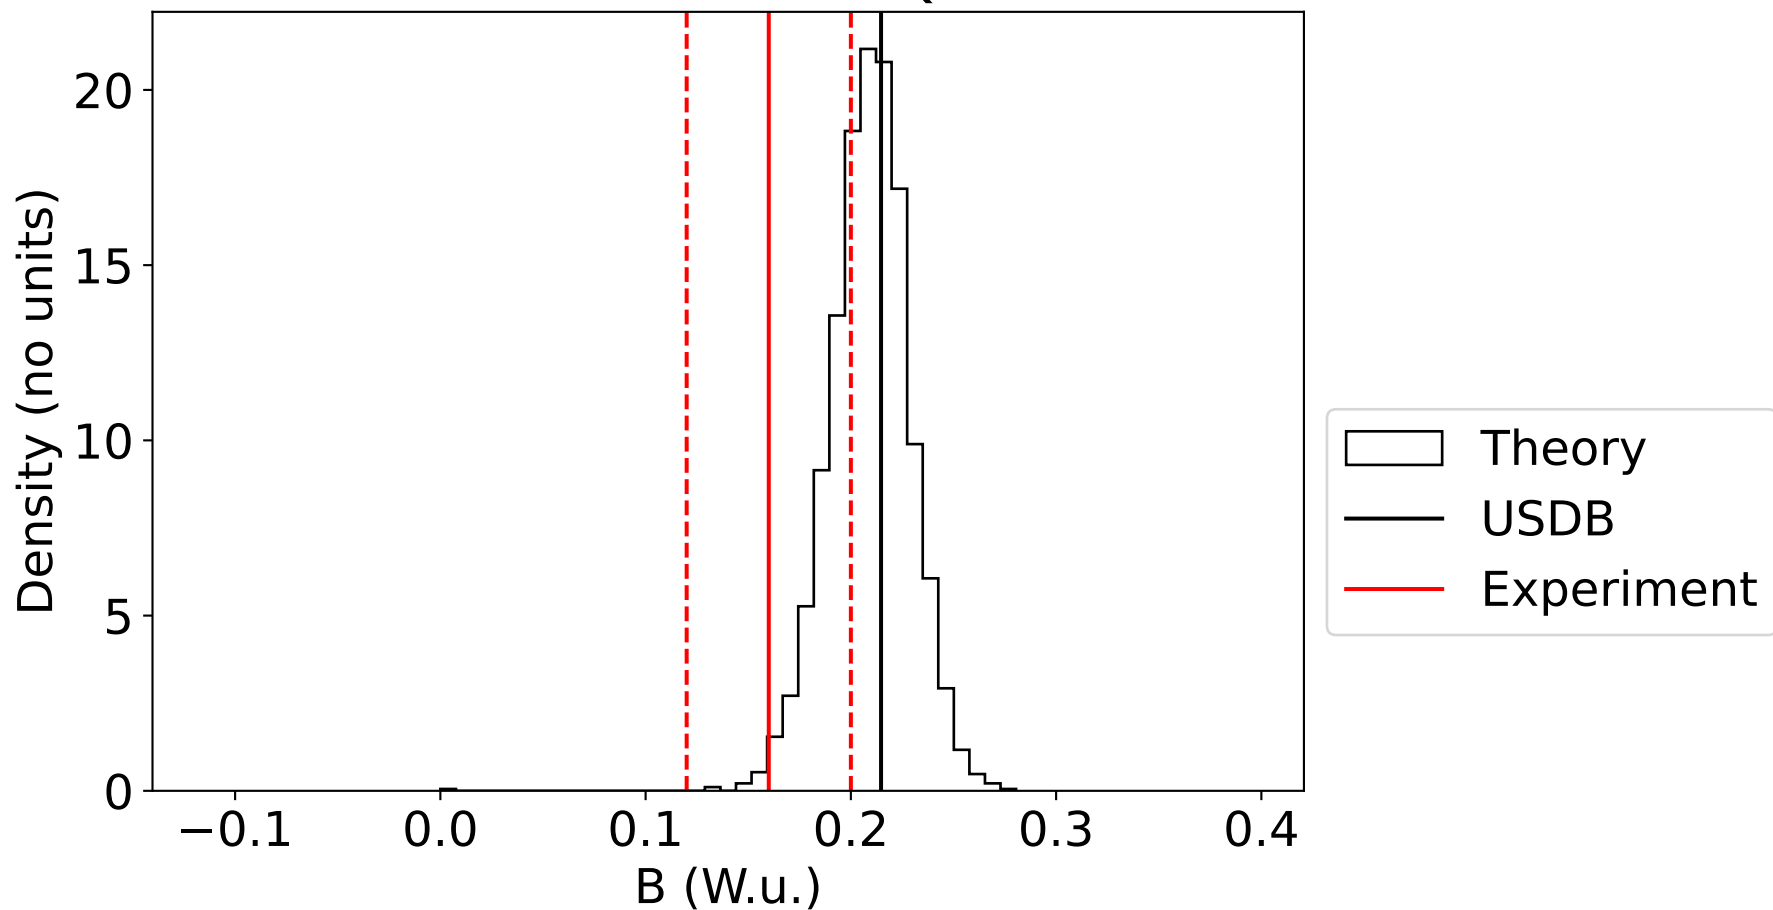

$^{37}\text{Cl} (1/2_1) \rightarrow (3/2_1)$   
Included in UQ

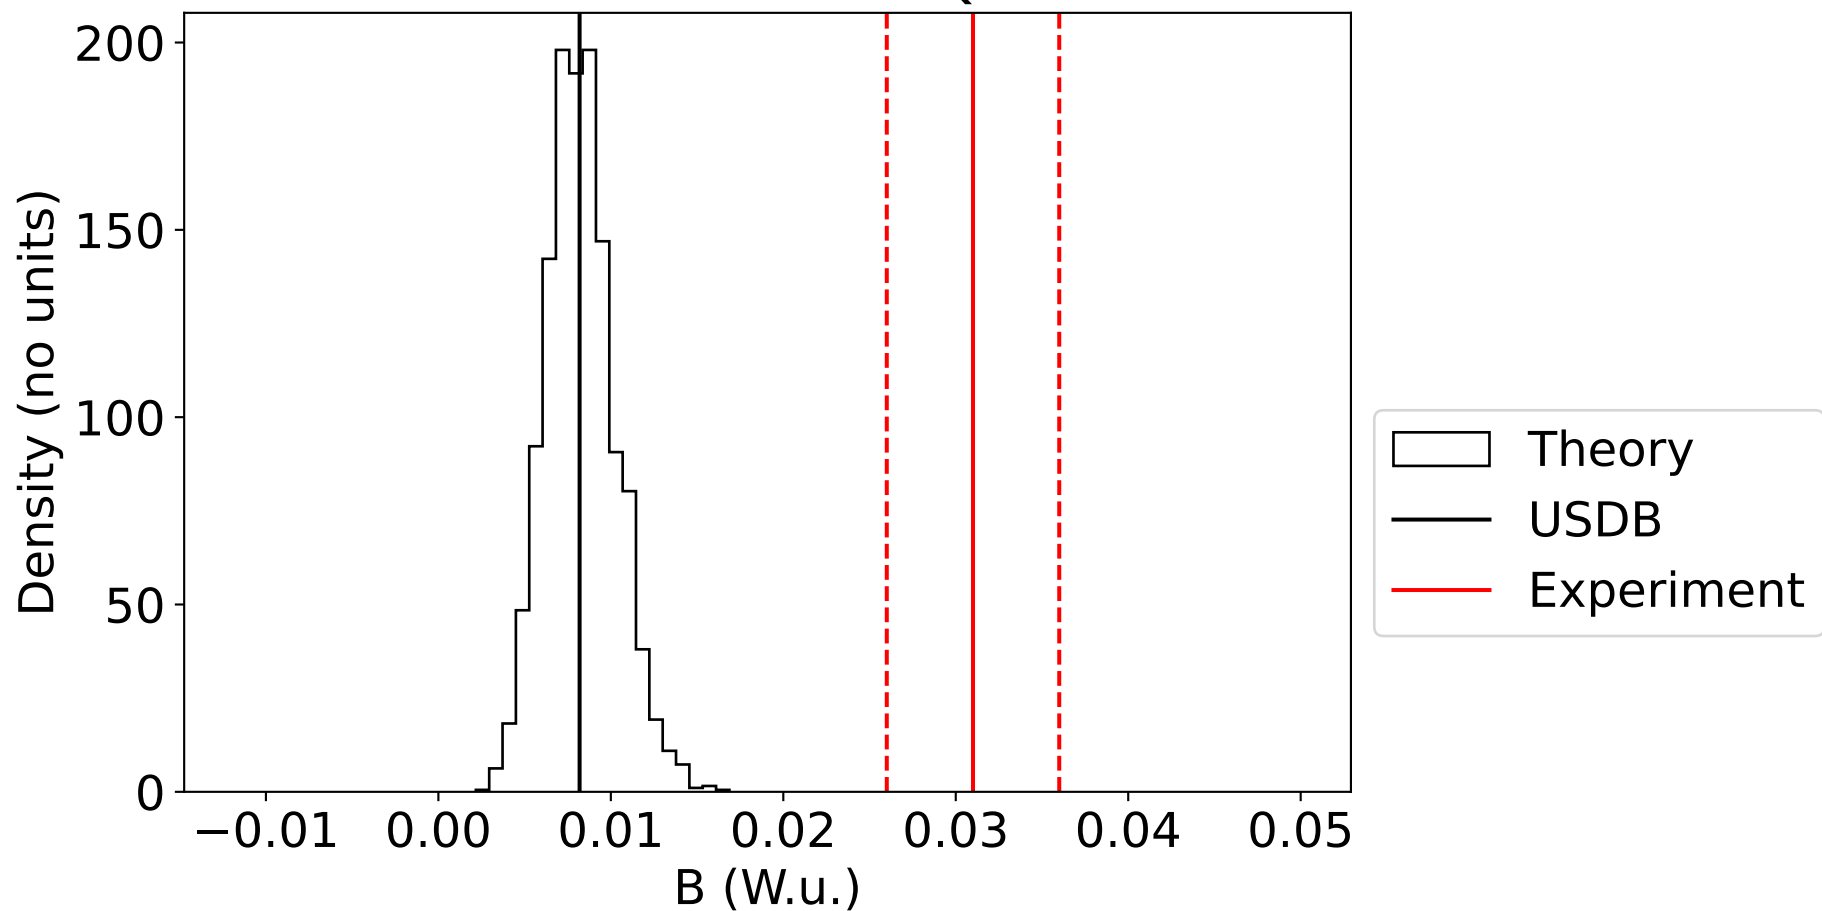

$^{37}\text{Cl} (5/2_1) \rightarrow (3/2_1)$   
Included in UQ

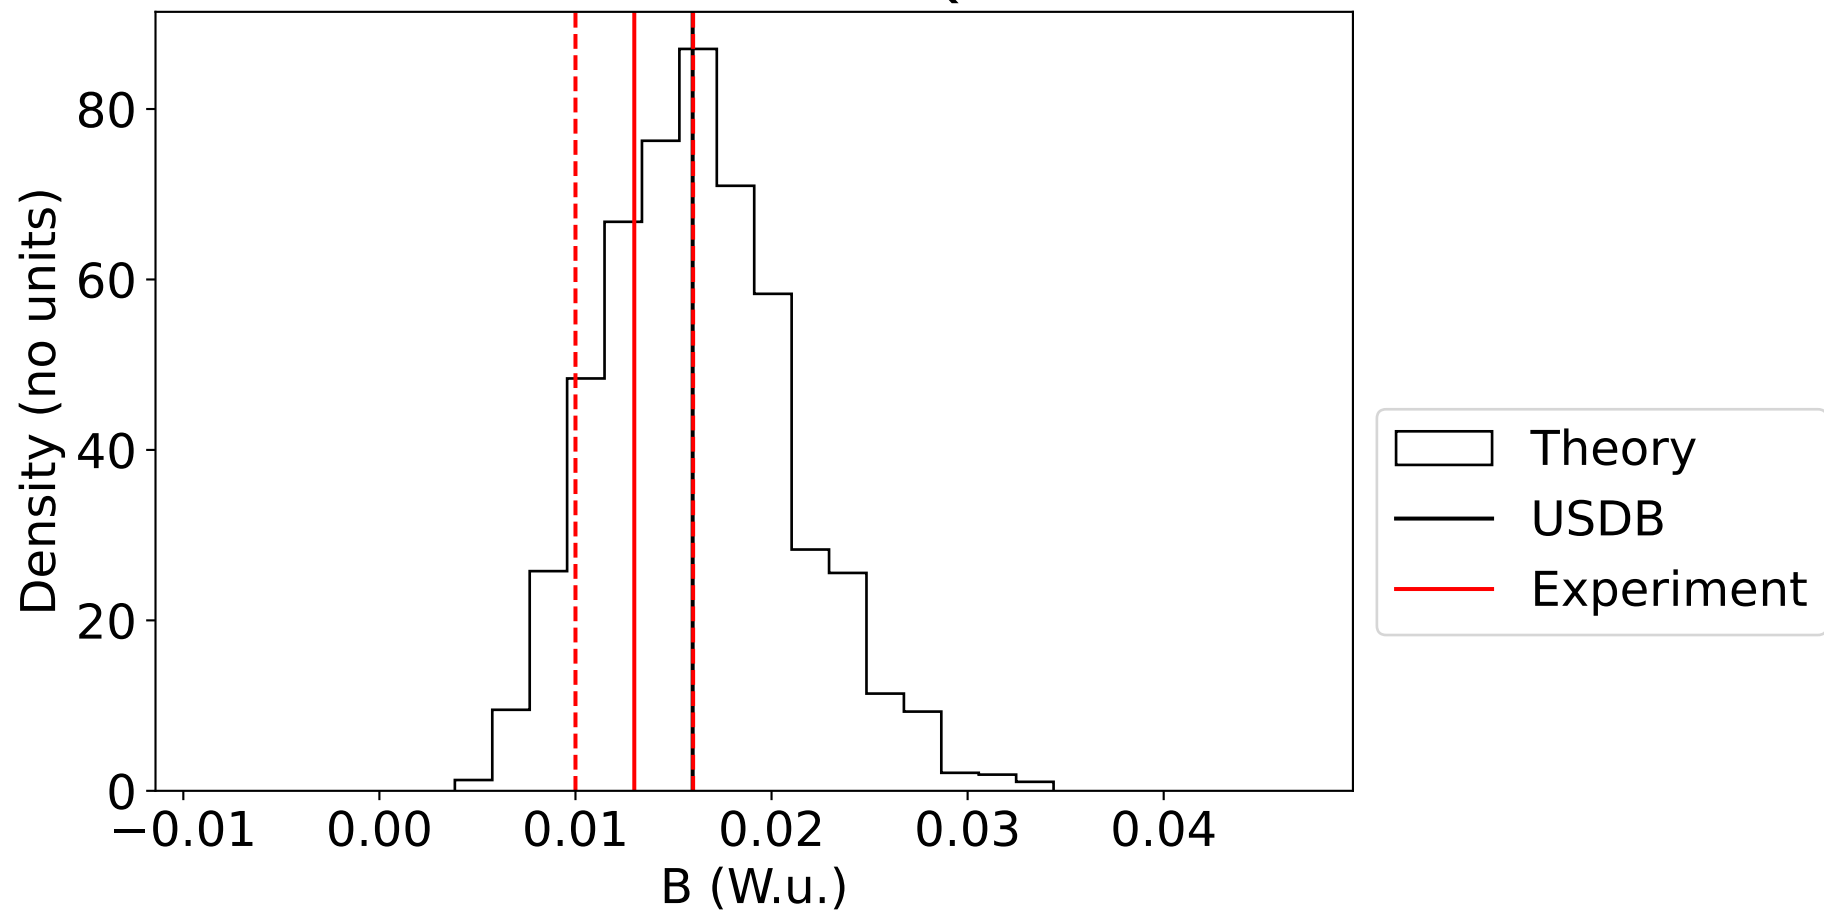

$^{37}\text{Cl} (3/2_4) \rightarrow (5/2_1)$   
Included in UQ

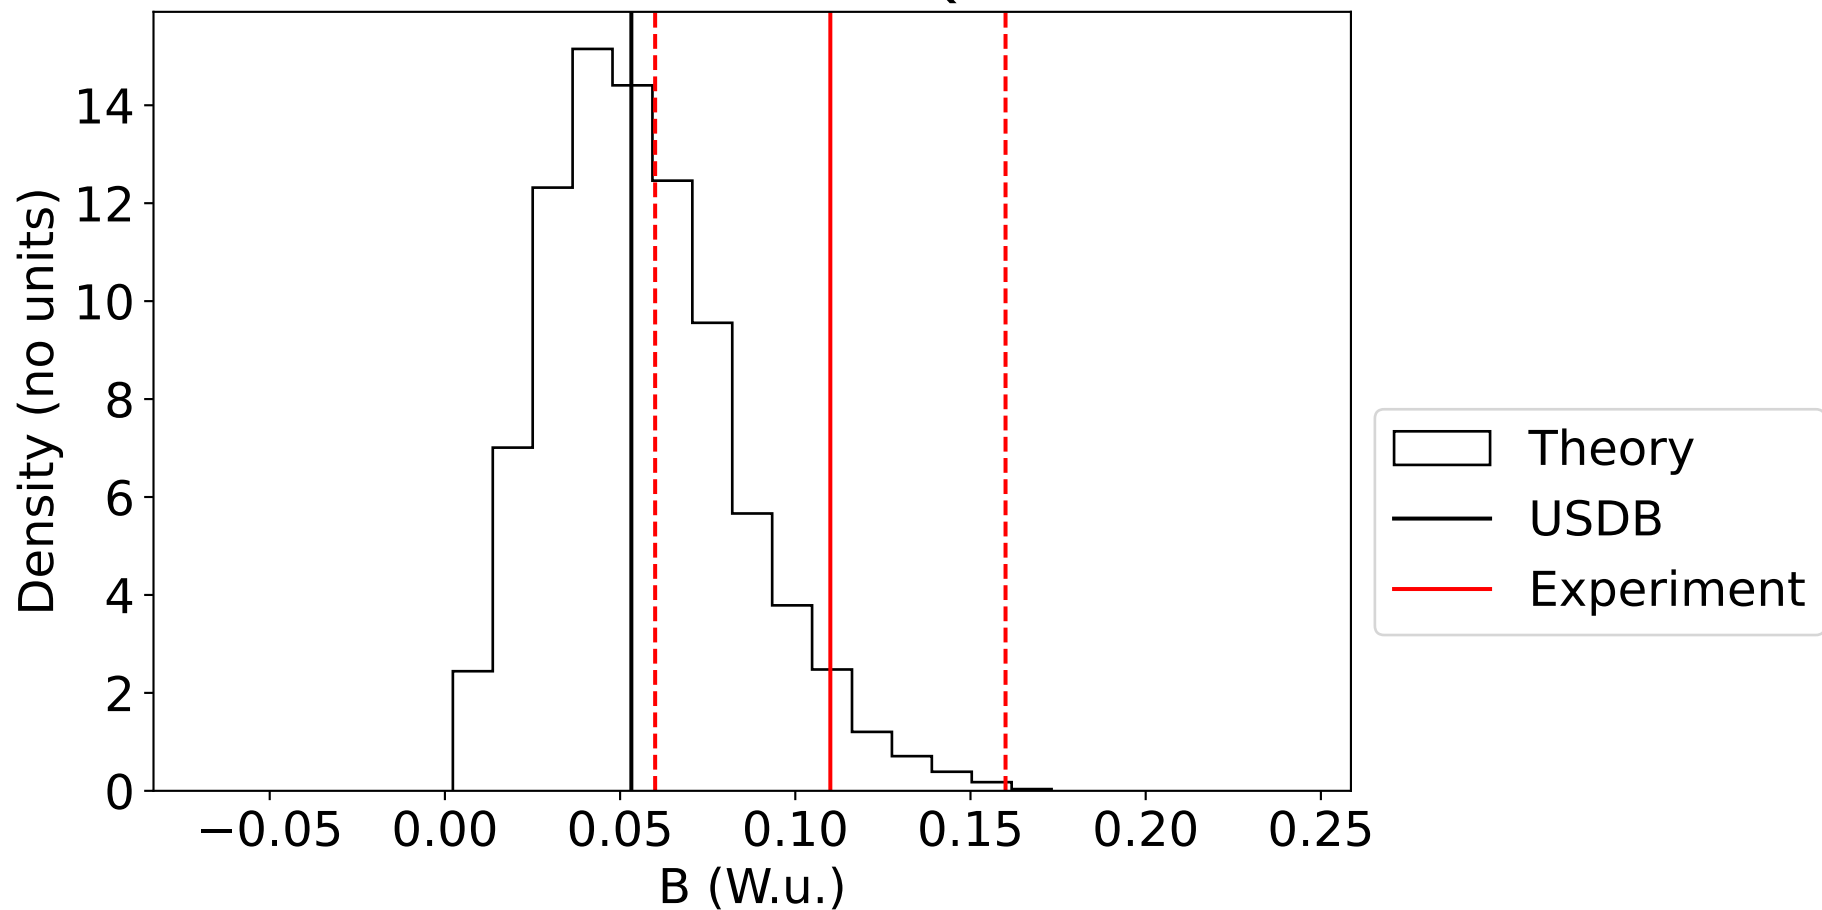

$^{37}\text{Cl } (5/2_4) \rightarrow (3/2_3)$   
Included in UQ

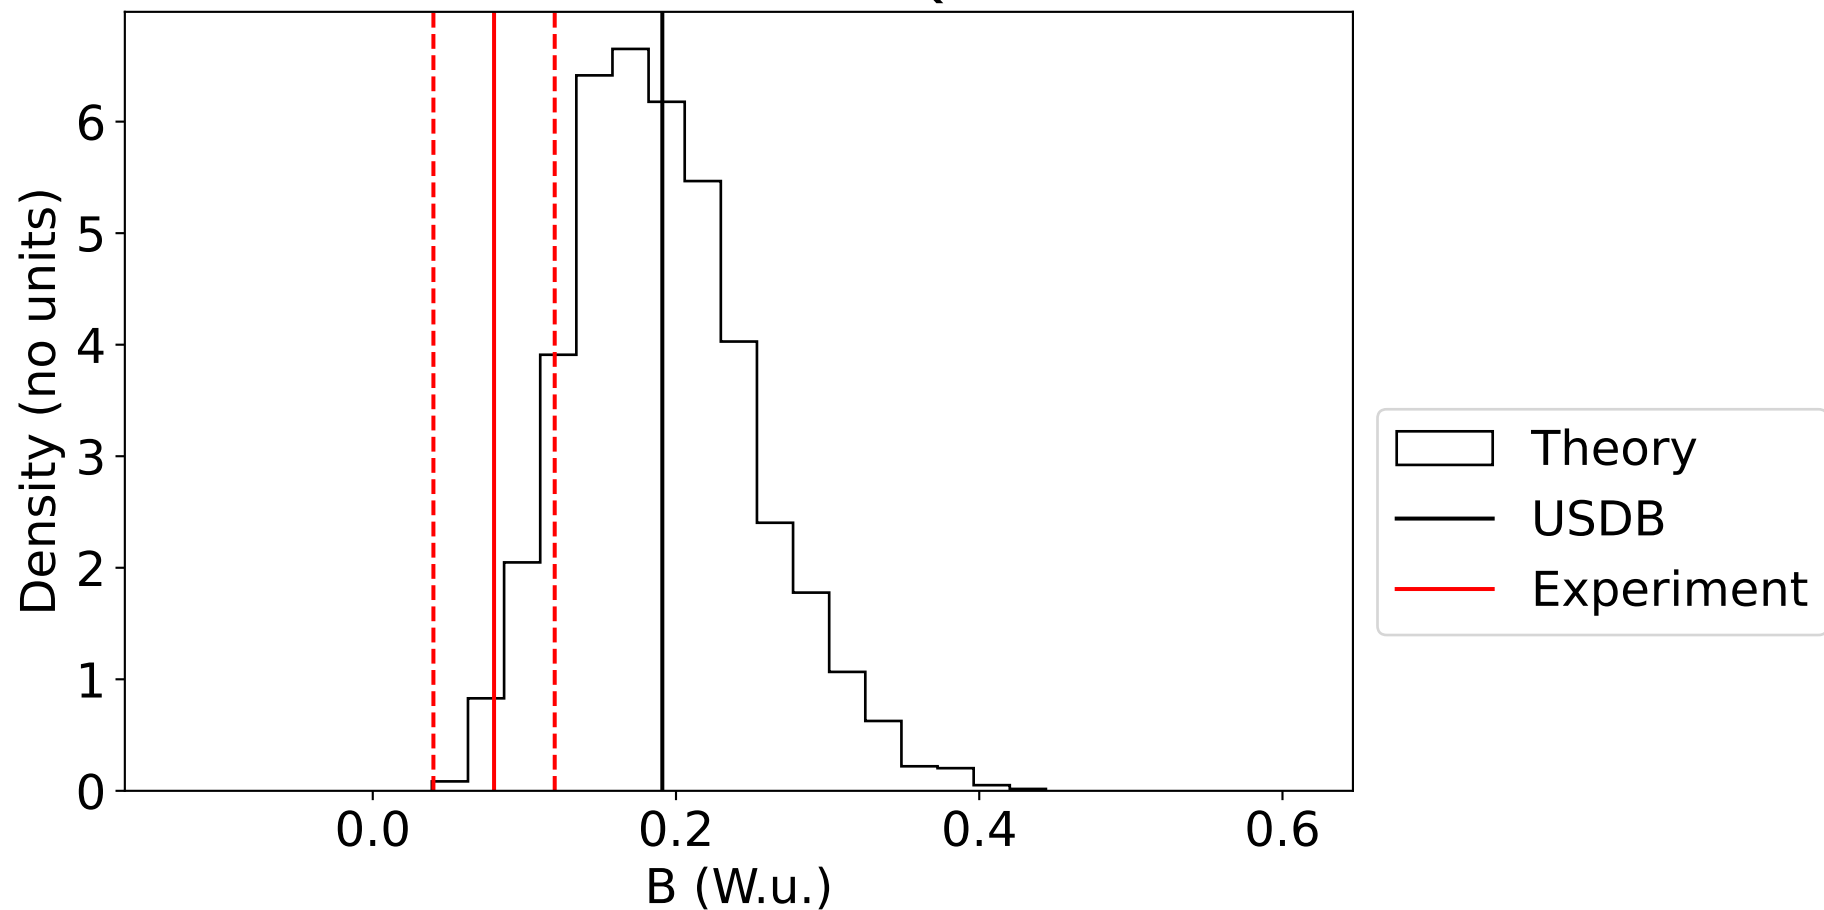



$^{34}\text{Ar} (2_2) \rightarrow (2_1)$   
Included in UQ

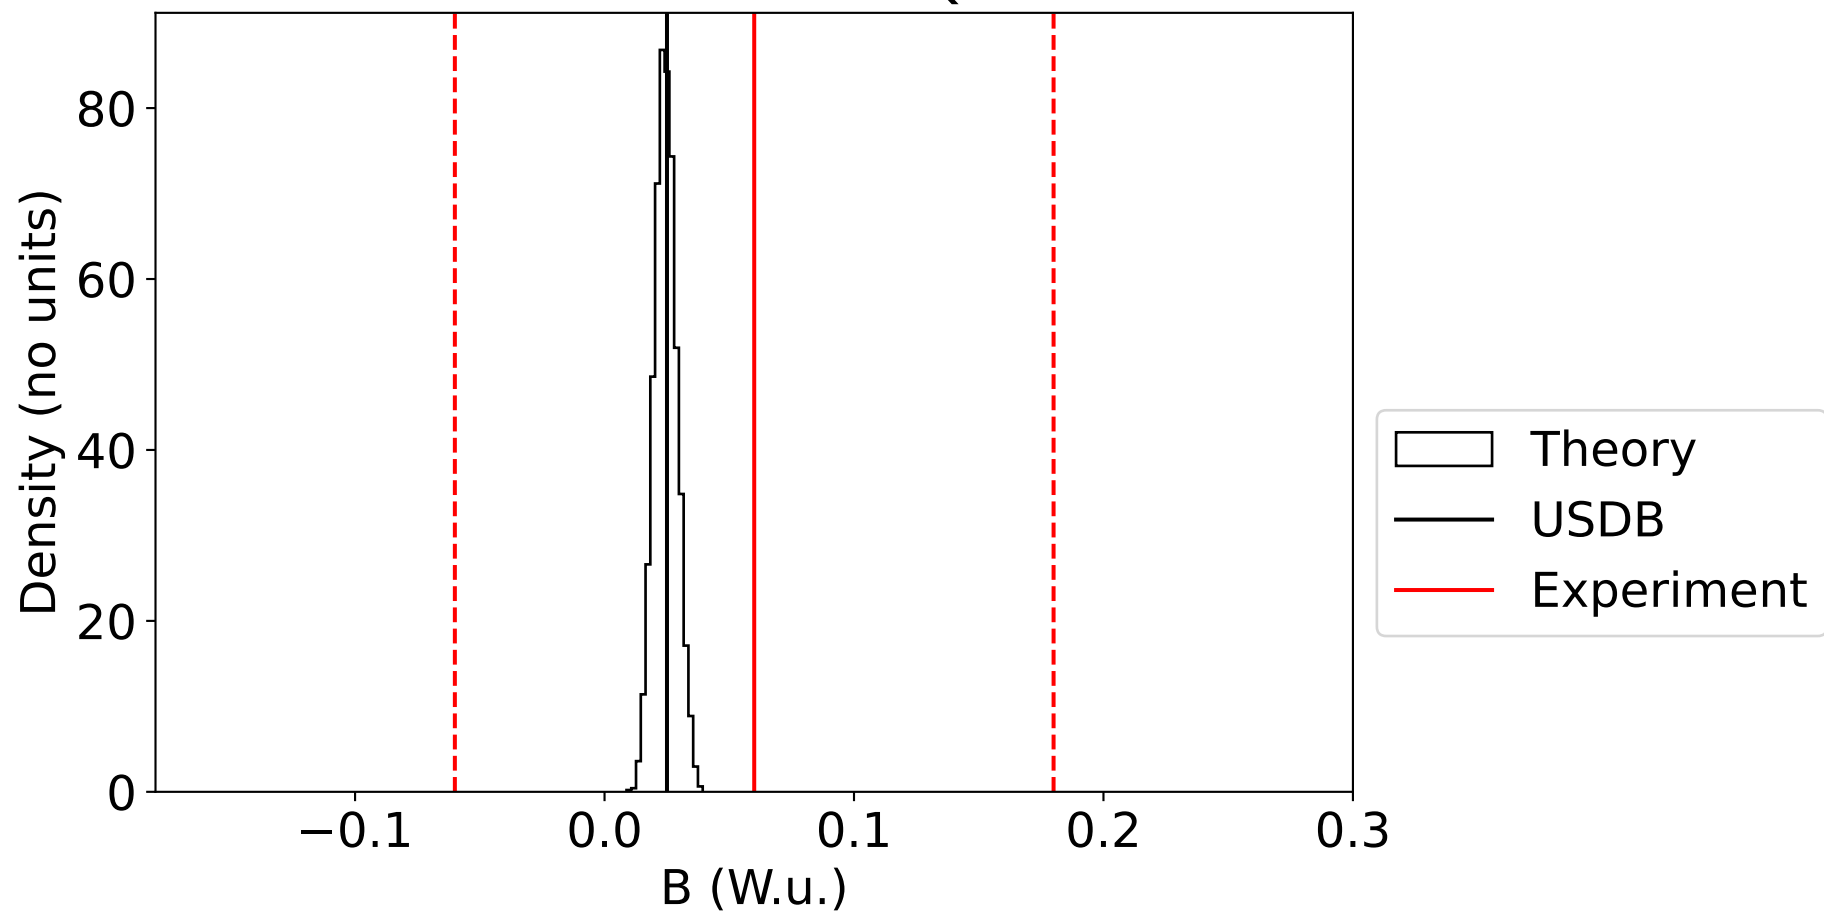

$^{37}\text{Ar} (5/2_1) \rightarrow (3/2_1)$   
Included in UQ

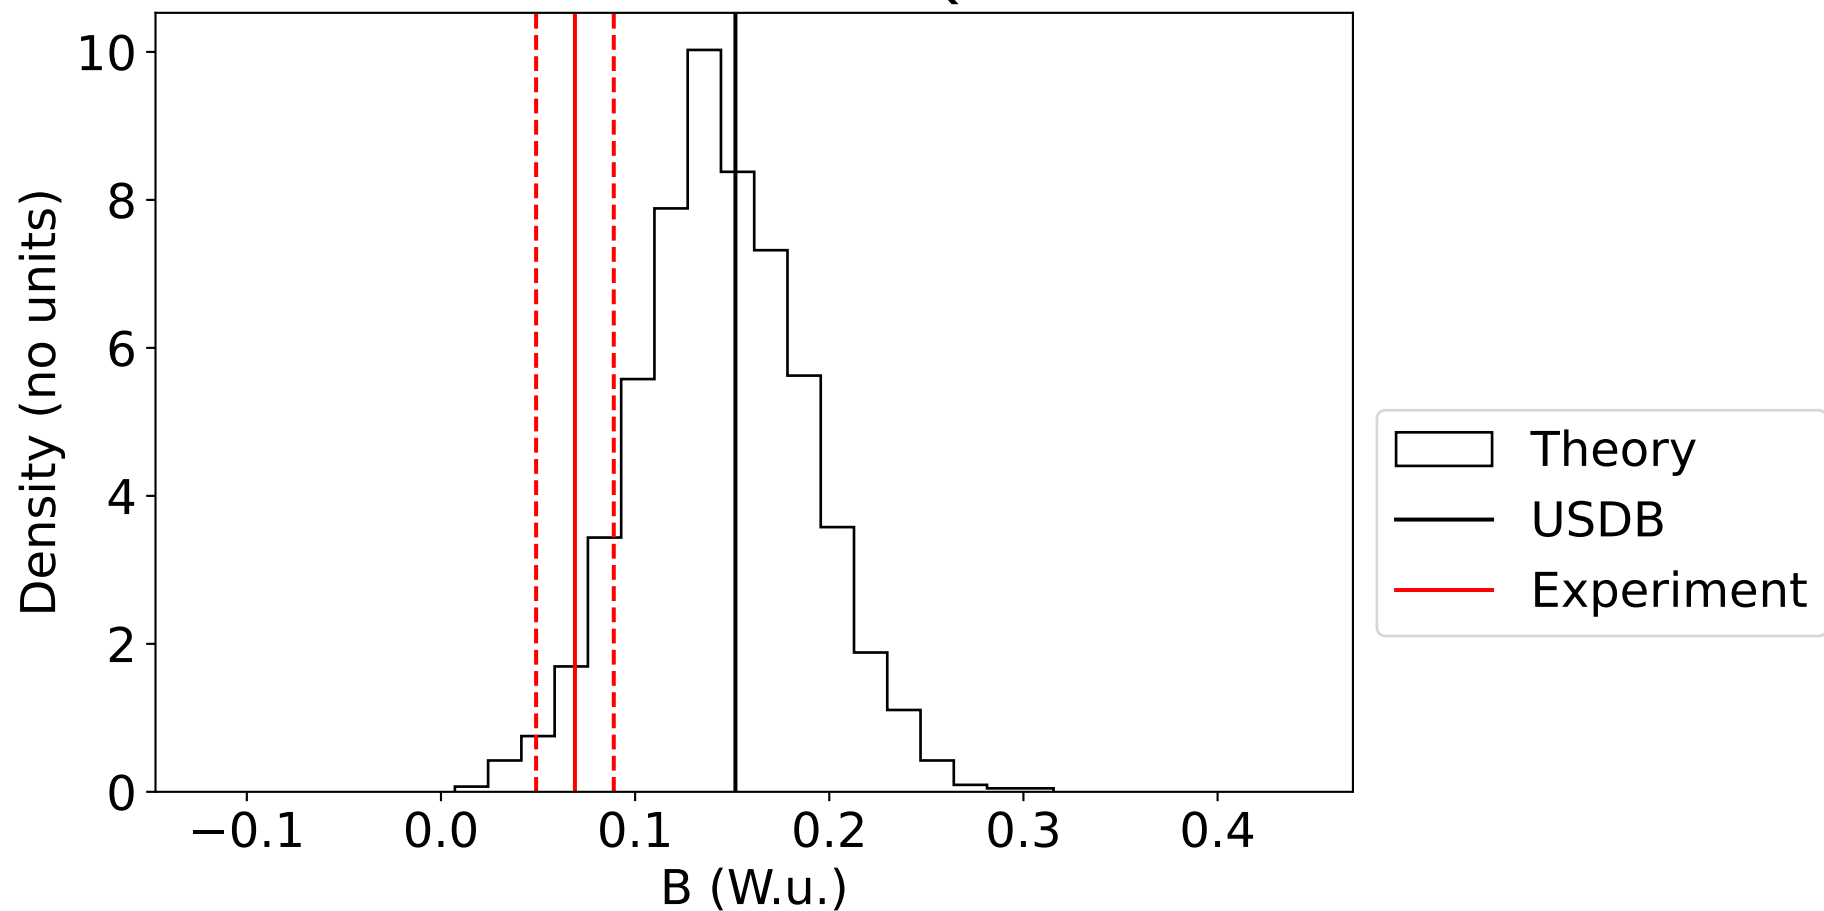

$^{37}\text{Ar} (3/2_2) \rightarrow (3/2_1)$   
Included in UQ

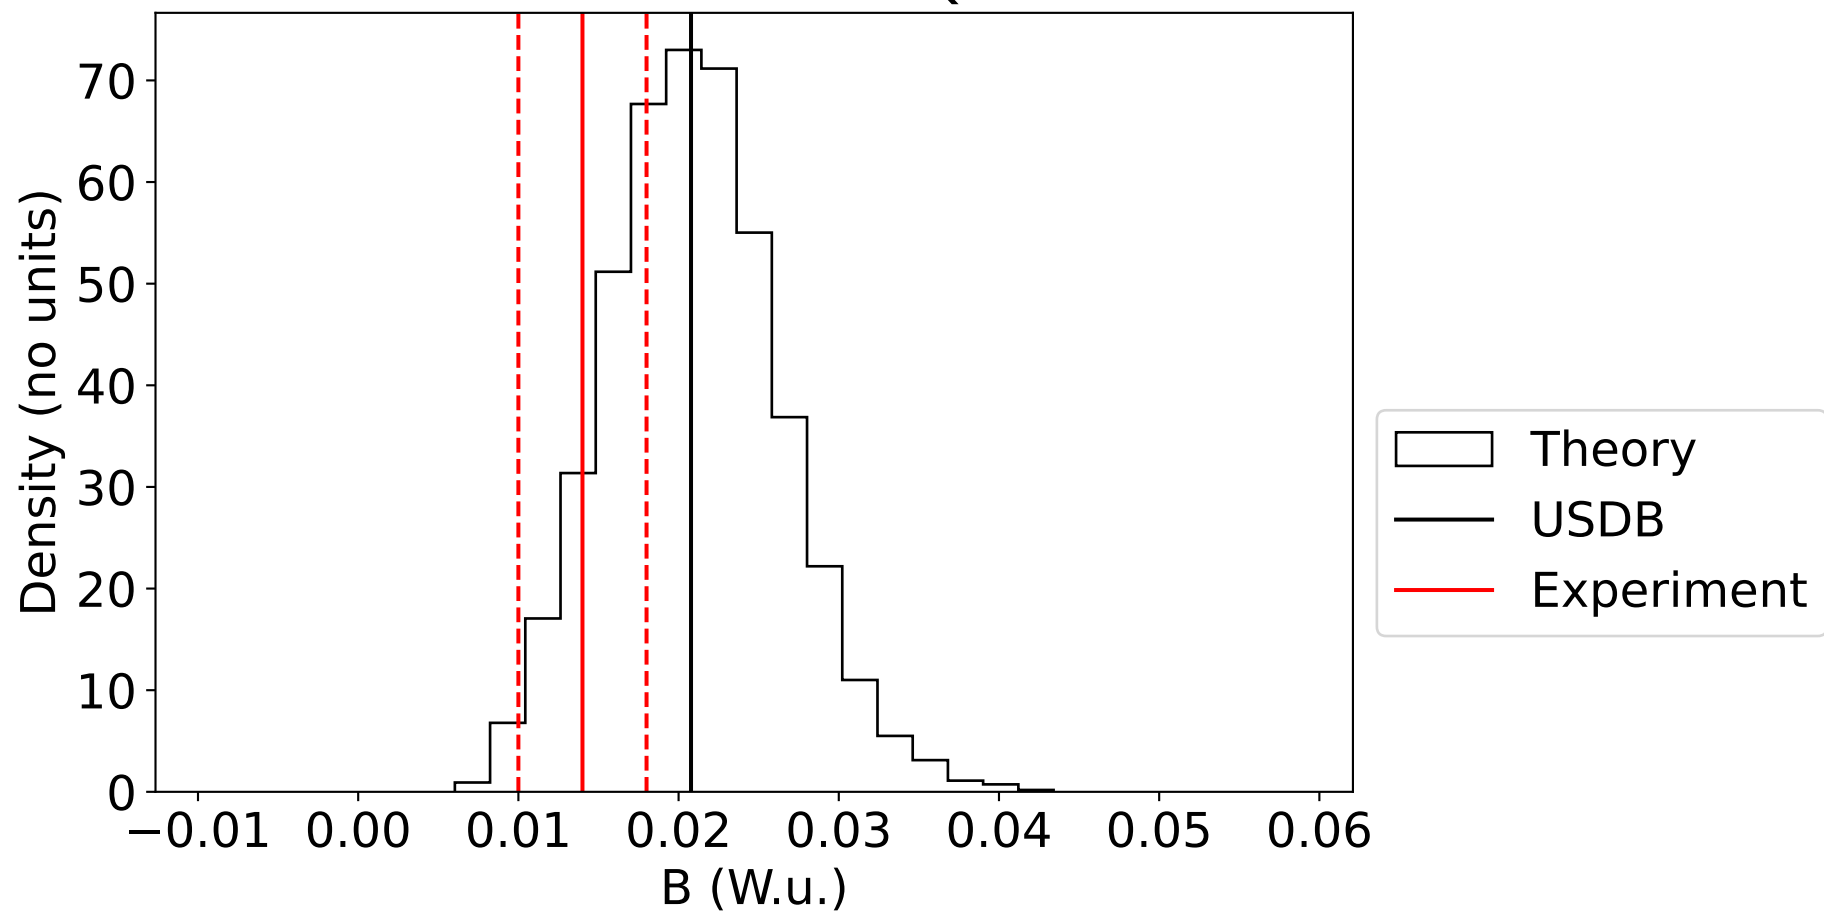

$^{37}\text{Ar} (3/2_3) \rightarrow (3/2_1)$   
Included in UQ

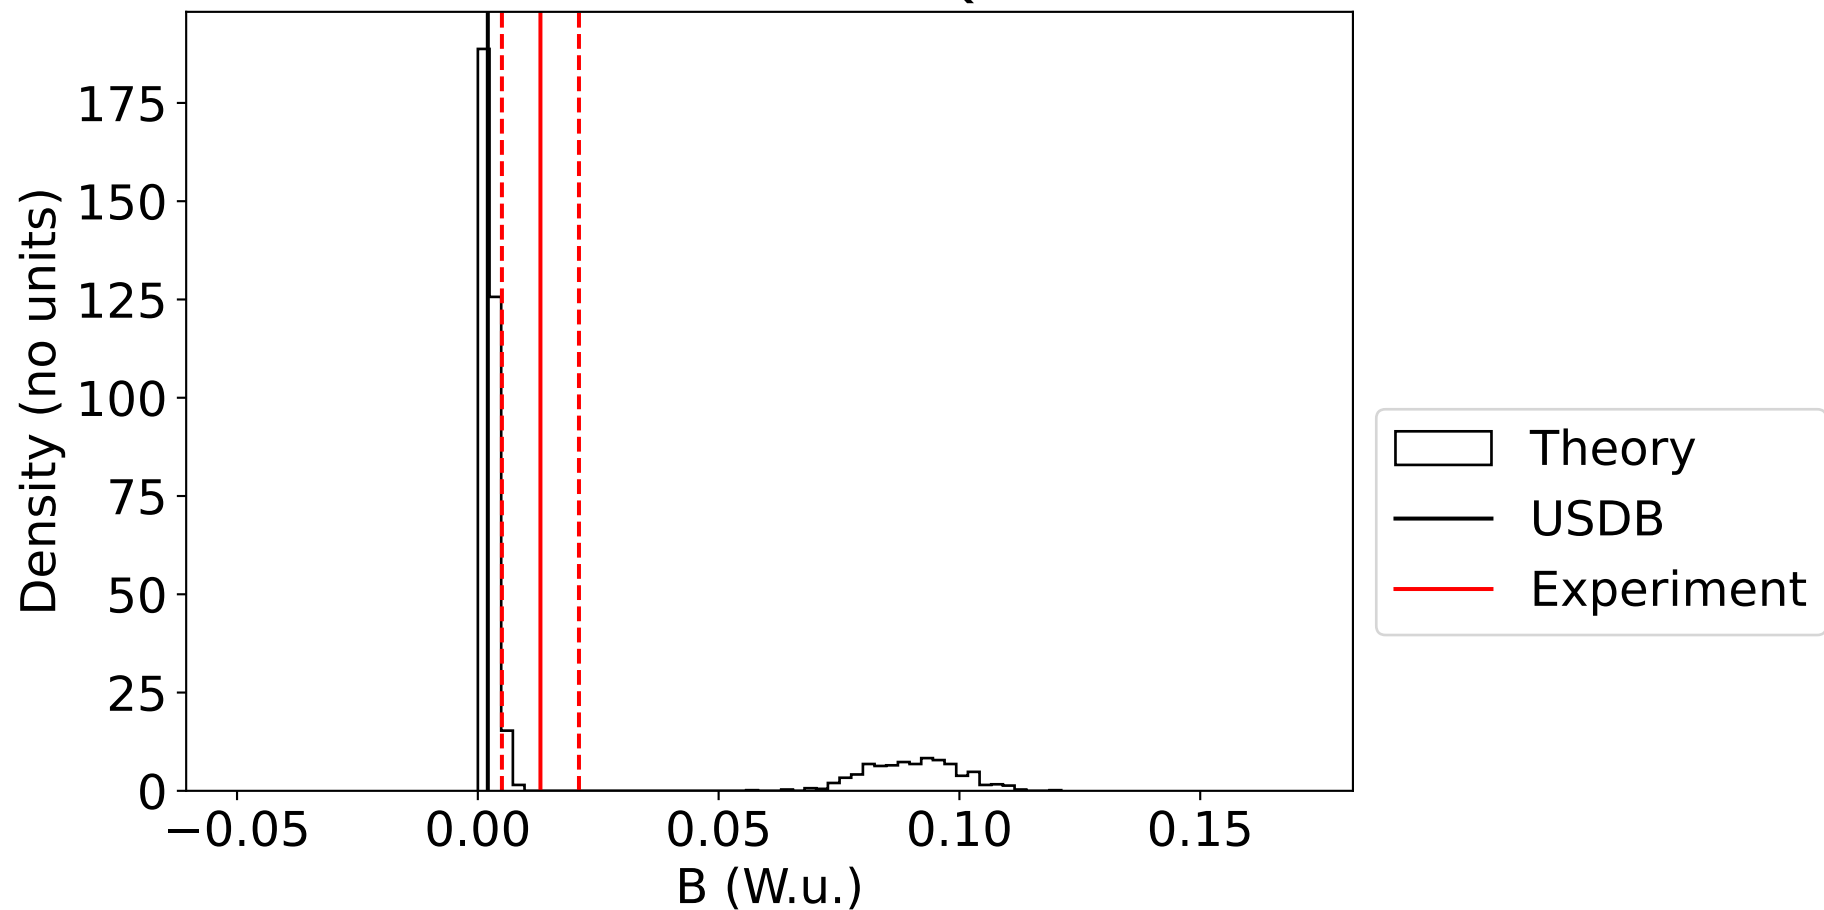

$^{37}\text{Ar} (7/2_2) \rightarrow (5/2_1)$   
Included in UQ

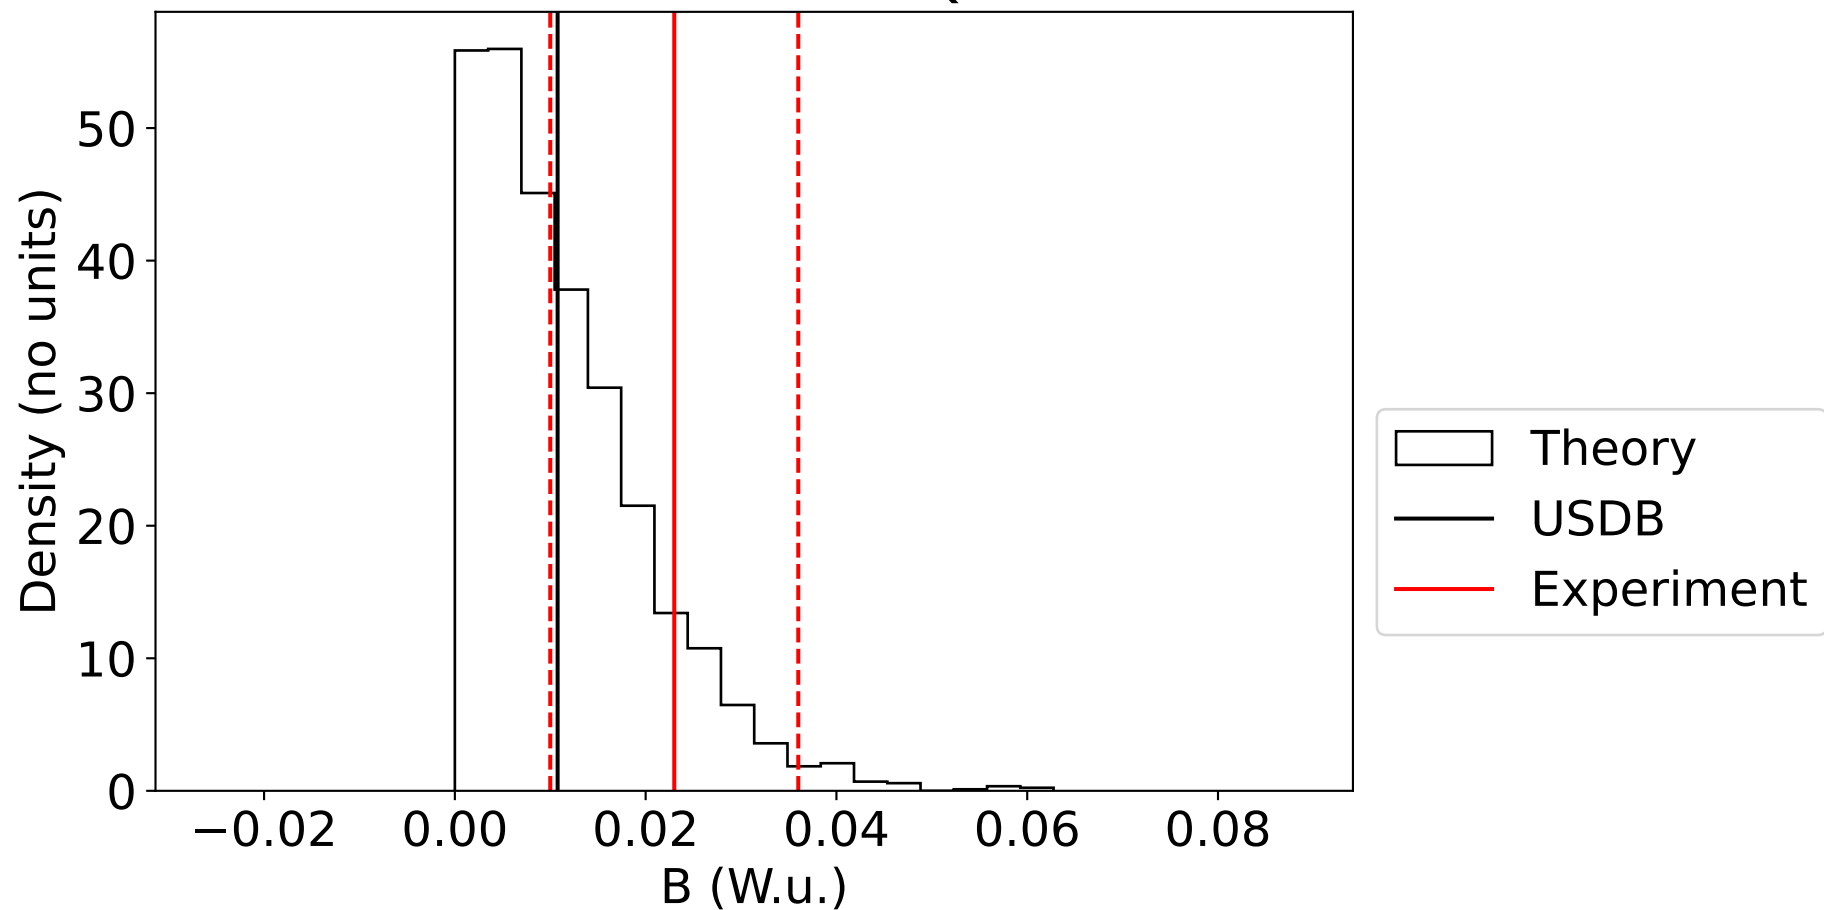

$^{37}\text{K} (5/2_1) \rightarrow (3/2_1)$   
Included in UQ

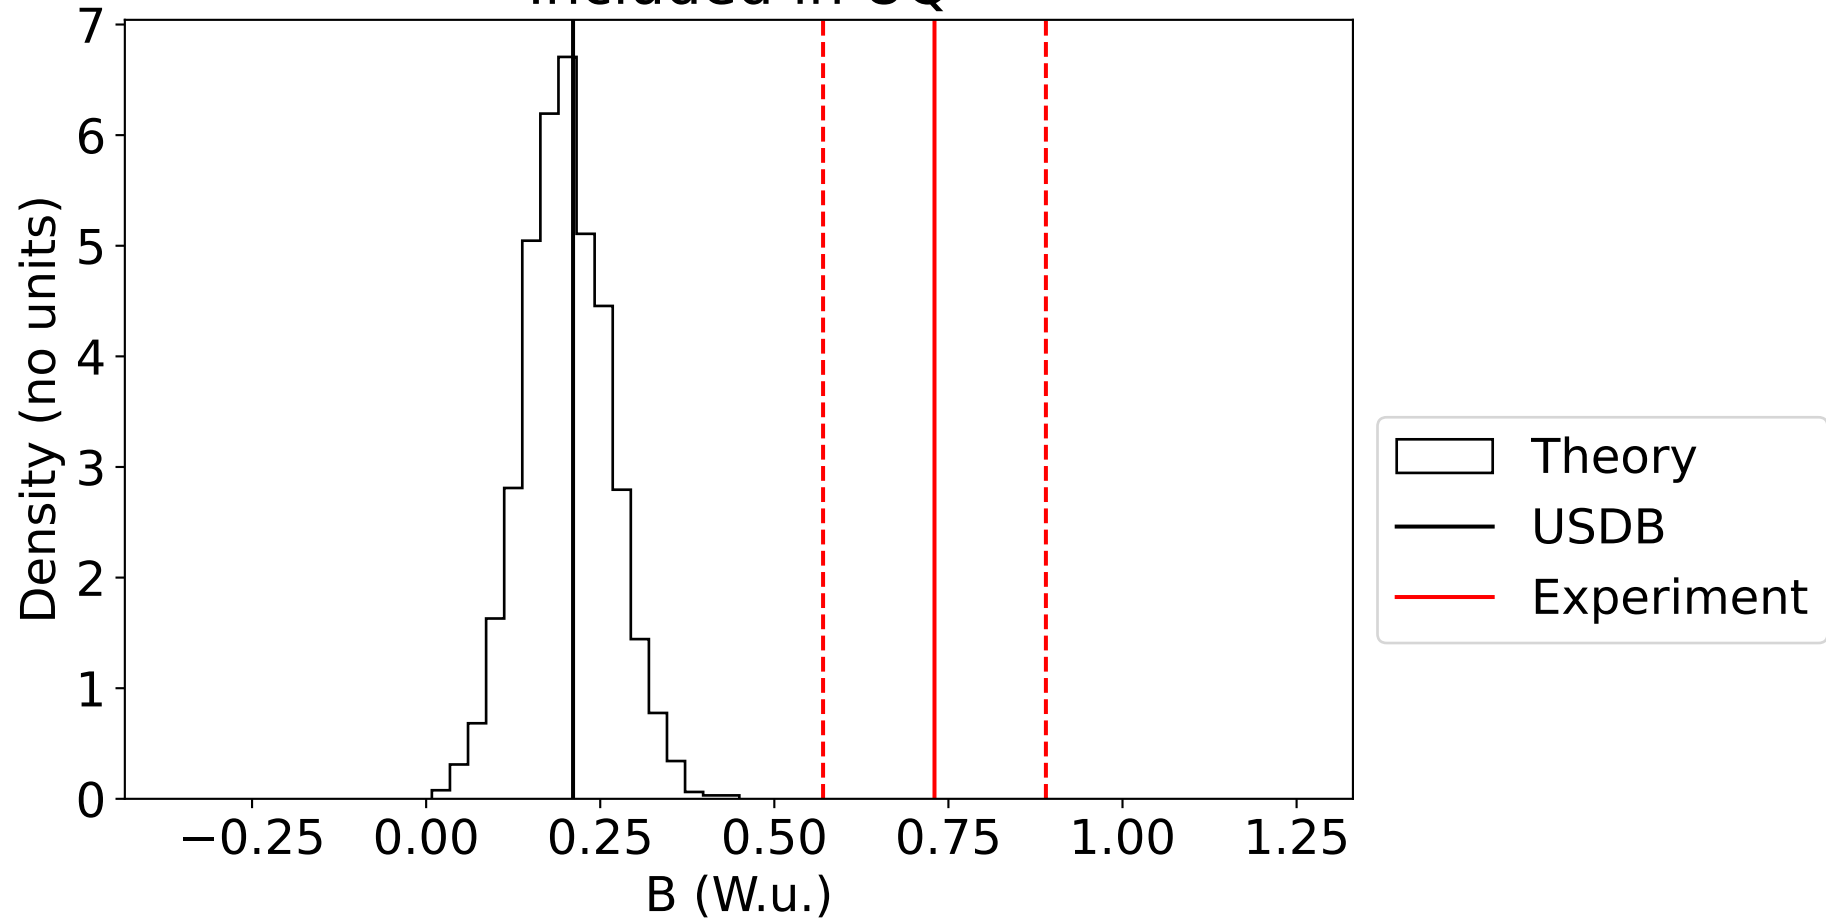

$^{38}\text{K} (1_1) \rightarrow (0_1)$   
Included in UQ

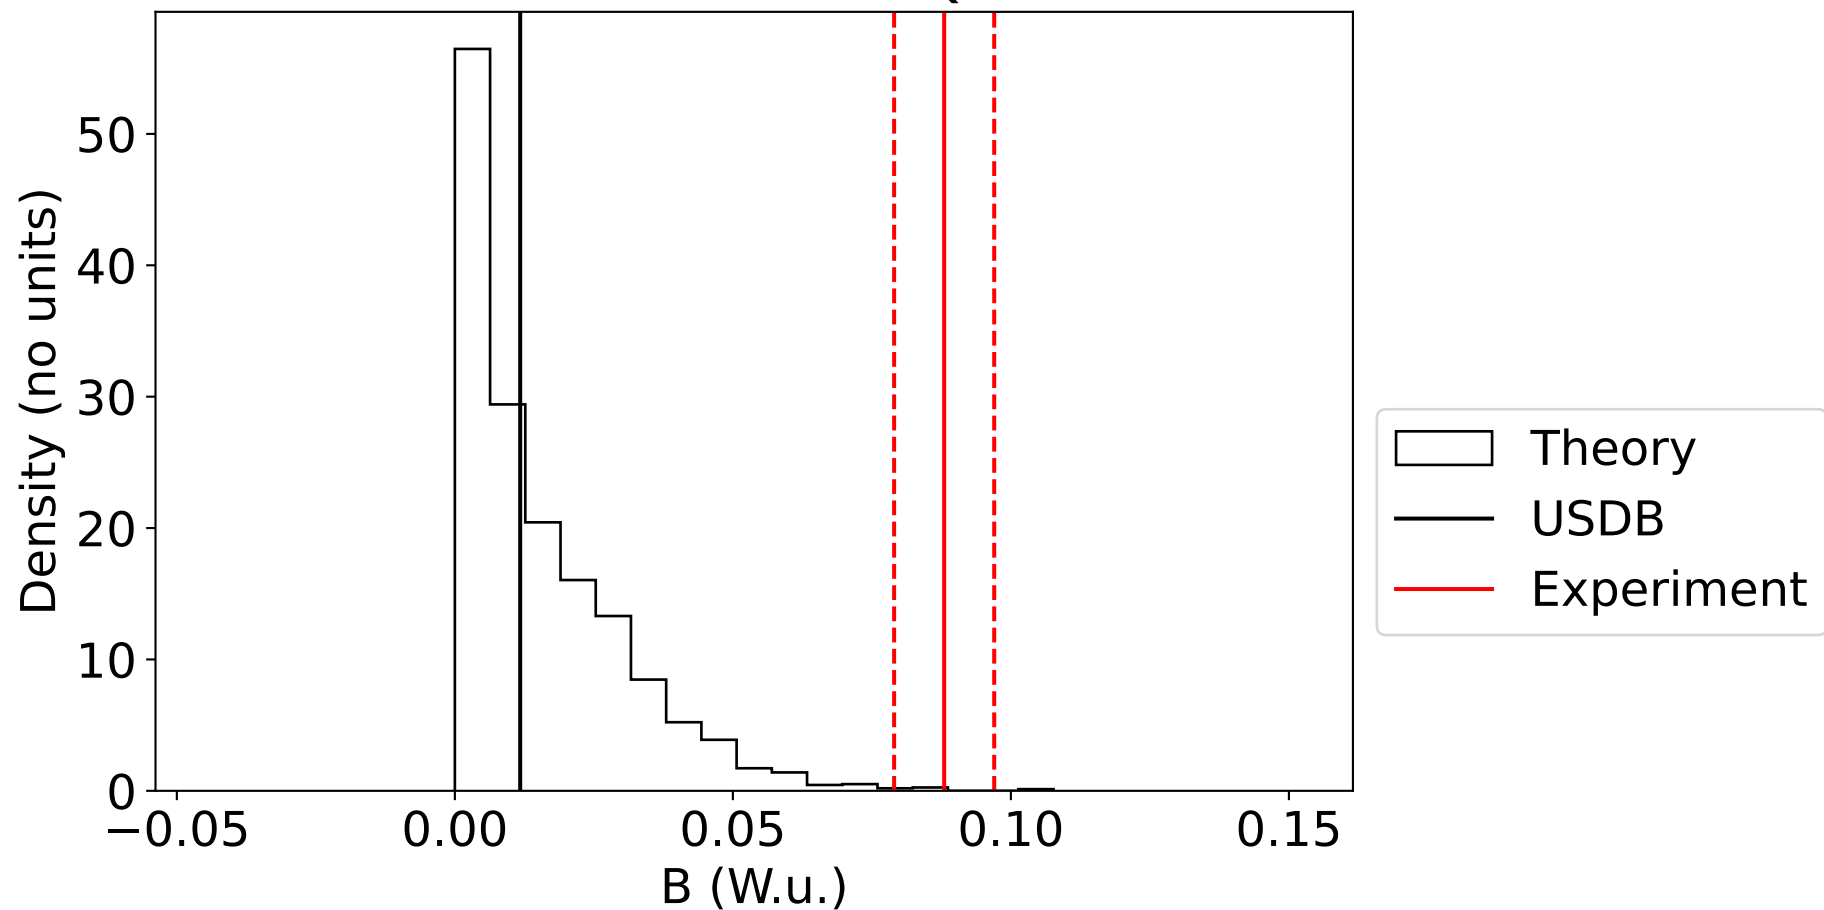

$^{38}\text{K} (1_2) \rightarrow (0_1)$   
Included in UQ

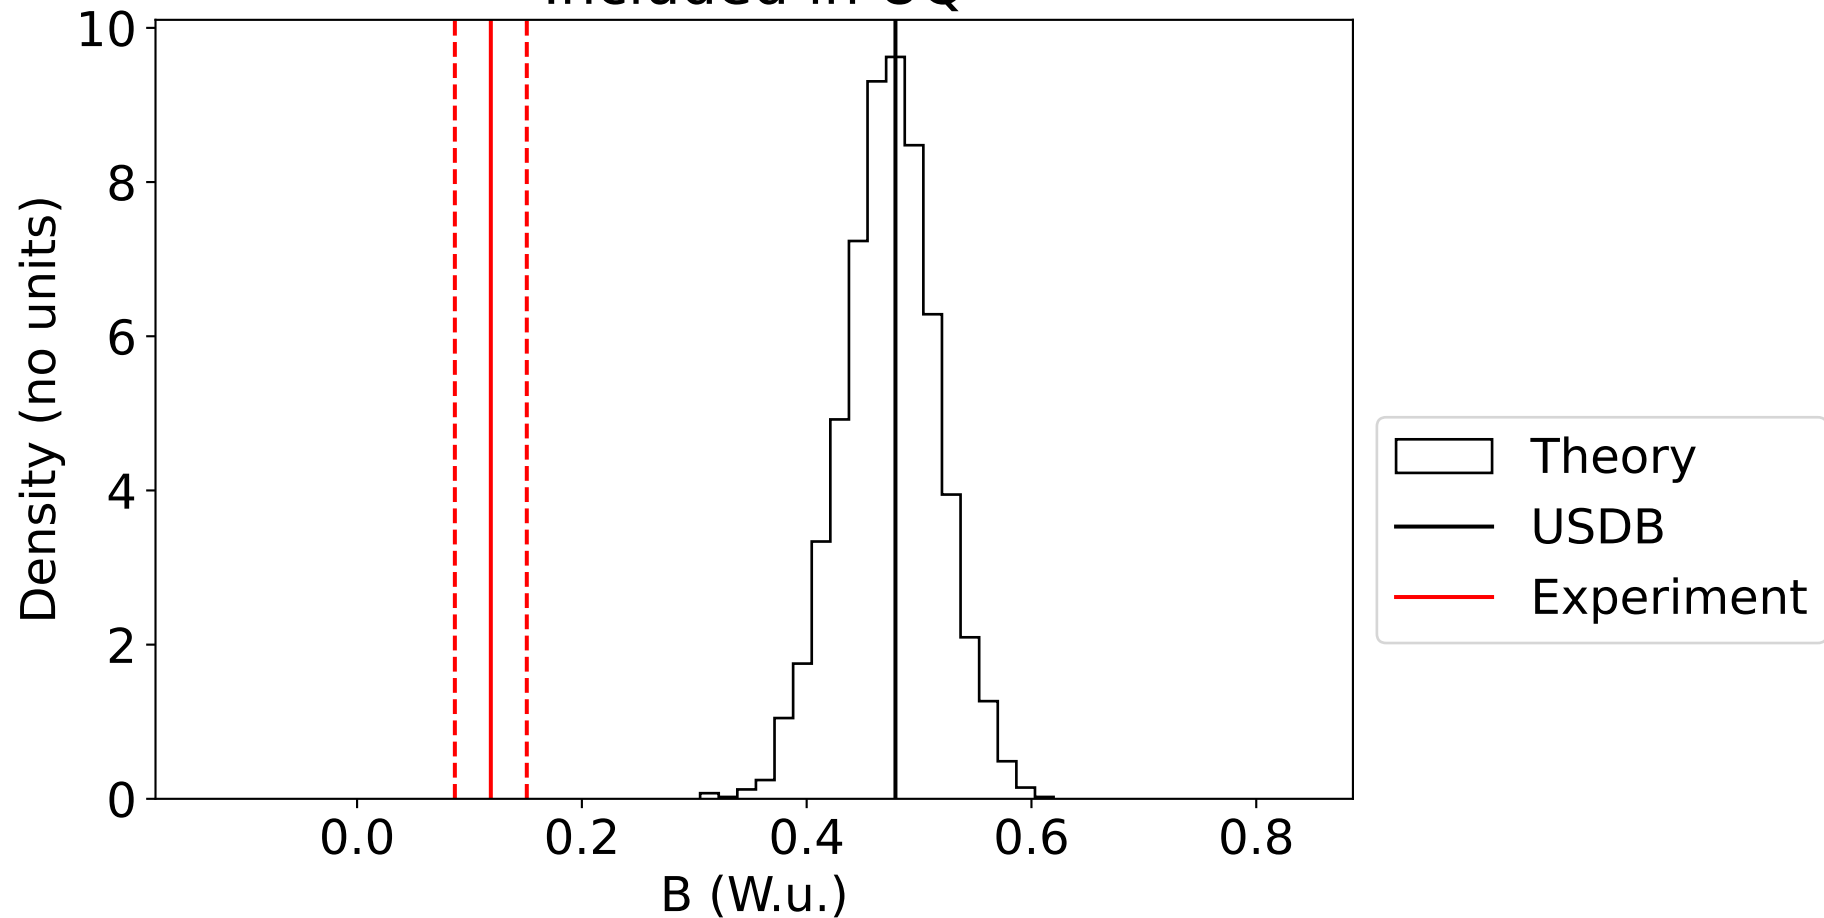



$^{38}\text{K} (2_1) \rightarrow (1_1)$   
Included in UQ

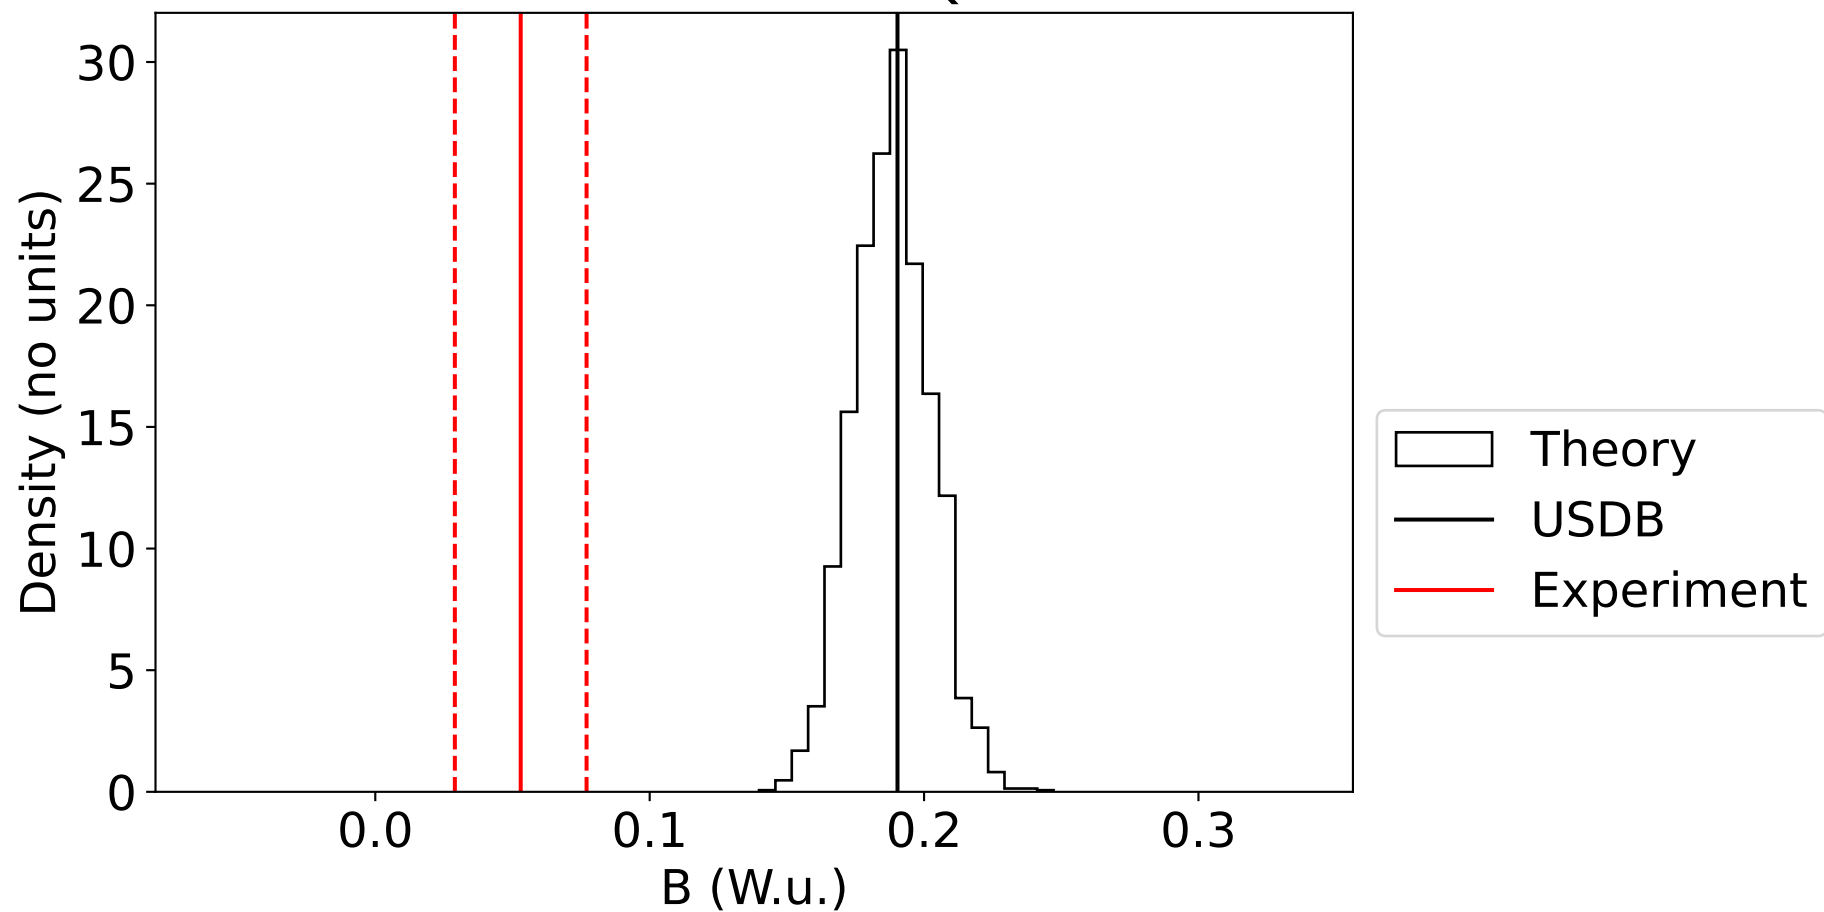

Supplement: Supplementary file 5 [file M1_B_histograms.pdf]
